# Supplementary material for: A 3D foundation model unifying CT interpretation and segmentation
Source: arXiv:2611.06471 source file (2026-11-04)
Supplement: Supplementary file 1 [file table10_grounded_report_generation_text_quality.tex]

\begingroup
\makeatletter
\@ifundefined{color@leftblue}{\definecolor{leftblue}{RGB}{232,242,248}}{}%
\@ifundefined{color@headerblue}{\definecolor{headerblue}{RGB}{218,233,242}}{}%
\makeatother
\setlength{\LTcapwidth}{18.60cm}
\setlength{\LTleft}{\fill}
\setlength{\LTright}{\fill}
\setlength{\LTpre}{0pt}
\setlength{\LTpost}{0pt}
\setlength{\tabcolsep}{0.45pt}
\renewcommand{\arraystretch}{1.00}
\setlength{\extrarowheight}{0pt}
\setlength{\arrayrulewidth}{0.48pt}
\arrayrulecolor{black}
\providecommand{\softcline}[1]{}%
\renewcommand{\softcline}[1]{\arrayrulecolor{black!35}\cline{#1}\arrayrulecolor{black}}
\sloppy
\emergencystretch=2em
\fontsize{5.25pt}{5.85pt}\selectfont
\newcommand{\HoloTaskScore}[4]{%
  \parbox[c][0.64cm][c]{2.32cm}{%
    \centering
    {\fontsize{5.25pt}{5.53pt}\selectfont\strut\mbox{#1}}\\[-0.38ex]%
    {\fontsize{#3}{#4}\selectfont\strut\mbox{#2}}%
  }%
}%
\newcommand{\HoloTaskMetricGroup}[1]{%
  \parbox[c][0.64cm][c]{1.26cm}{%
    \centering\fontsize{4.60pt}{4.90pt}\selectfont\textbf{#1}%
  }%
}%
\newcommand{\HoloTaskMetric}[1]{%
  \parbox[c][0.64cm][c]{1.26cm}{%
    \centering\fontsize{4.60pt}{4.90pt}\selectfont\textbf{#1}%
  }%
}%
\newcommand{\HoloTaskRowSpan}[2]{%
  \parbox[c][0.64cm][c]{#2}{%
    \centering\arraybackslash #1%
  }%
}%
\newcommand{\HoloTaskSpan}[3]{%
  \raisebox{\dimexpr#3-0.11cm\relax}[0pt][0pt]{%
    \parbox[c][0.64cm][c]{#2}{%
      \centering\arraybackslash #1%
    }%
  }%
}%
\newcommand{\HoloTaskSplitHead}[3]{%
  \parbox[c][0.92cm][c]{#3}{%
    \centering\fontsize{6.05pt}{6.30pt}\selectfont\textbf{#1}\\[-0.52ex]%
    \rule{0pt}{0.58ex}\\[-0.52ex]\textbf{#2}%
  }%
}%
\newcommand{\HoloTaskMidHead}[2]{%
  \parbox[c][0.92cm][c]{#2}{%
    \centering\fontsize{6.05pt}{6.30pt}\selectfont\textbf{#1}%
  }%
}%
\newcommand{\HoloTaskModelHead}[2]{%
  \parbox[c][0.92cm][c]{#2}{%
    \centering\fontsize{5.30pt}{5.58pt}\selectfont\textbf{#1}%
  }%
}%
\begin{longtable}{|>{\columncolor{leftblue}\centering\arraybackslash}m{1.35cm}|>{\columncolor{leftblue}\centering\arraybackslash}m{2.30cm}|>{\columncolor{leftblue}\centering\arraybackslash}m{1.30cm}|>{\columncolor{leftblue}\centering\arraybackslash}m{1.30cm}|>{\centering\arraybackslash}m{2.35cm}|>{\centering\arraybackslash}m{2.35cm}|>{\centering\arraybackslash}m{2.35cm}|>{\centering\arraybackslash}m{2.35cm}|>{\centering\arraybackslash}m{2.35cm}|}
\caption[Anatomy-grounded and finding-grounded report generation: text quality]{\textbf{Text-quality performance of HoloCT and competing methods for anatomy-grounded and finding-grounded report generation on RadGenome, ReXGroundingCT and private cohorts.}\newline RadGenome and ReXGroundingCT are internal datasets; Private05 and Private06 are private cohorts. $^{\blacktriangle}$ denotes a fine-tuned baseline. Each score is reported as mean with 95\% confidence interval. NLP metrics include BLEU-4, ROUGE-L, and METEOR; clinical metrics include RaTEScore, LlamaScore, and GREEN.}%
\label{tab:grounded_report_generation_radgenome_text_quality}\\[-0.15ex]
\hline
\rowcolor{headerblue}
\HoloTaskSplitHead{Dataset}{Type}{1.35cm} & \HoloTaskSplitHead{Dataset}{Name}{2.30cm} & \HoloTaskMidHead{Metric Type}{1.30cm} & \HoloTaskMidHead{Metric}{1.30cm} & \HoloTaskModelHead{\mbox{HuluMed-32B}}{2.35cm} & \HoloTaskModelHead{\makecell[c]{HoloCT-4B\\[-0.18ex]w/o grounding}}{2.35cm} & \HoloTaskModelHead{\makecell[c]{HoloCT-4B\\[-0.18ex]w/ grounding}}{2.35cm} & \HoloTaskModelHead{\makecell[c]{HoloCT-8B\\[-0.18ex]w/o grounding}}{2.35cm} & \HoloTaskModelHead{\makecell[c]{HoloCT-8B\\[-0.18ex]w/ grounding}}{2.35cm} \\
\hline
\endfirsthead
\caption*{\textbf{Supplementary Table~\ref{tab:grounded_report_generation_radgenome_text_quality} (continued)\enspace|\enspace Text-quality performance of HoloCT and competing methods for anatomy-grounded and finding-grounded report generation on RadGenome, ReXGroundingCT and private cohorts.}\newline RadGenome and ReXGroundingCT are internal datasets; Private05 and Private06 are private cohorts. $^{\blacktriangle}$ denotes a fine-tuned baseline. Each score is reported as mean with 95\% confidence interval. NLP metrics include BLEU-4, ROUGE-L, and METEOR; clinical metrics include RaTEScore, LlamaScore, and GREEN.}\\[-0.15ex]
\hline
\rowcolor{headerblue}
\HoloTaskSplitHead{Dataset}{Type}{1.35cm} & \HoloTaskSplitHead{Dataset}{Name}{2.30cm} & \HoloTaskMidHead{Metric Type}{1.30cm} & \HoloTaskMidHead{Metric}{1.30cm} & \HoloTaskModelHead{\mbox{HuluMed-32B}}{2.35cm} & \HoloTaskModelHead{\makecell[c]{HoloCT-4B\\[-0.18ex]w/o grounding}}{2.35cm} & \HoloTaskModelHead{\makecell[c]{HoloCT-4B\\[-0.18ex]w/ grounding}}{2.35cm} & \HoloTaskModelHead{\makecell[c]{HoloCT-8B\\[-0.18ex]w/o grounding}}{2.35cm} & \HoloTaskModelHead{\makecell[c]{HoloCT-8B\\[-0.18ex]w/ grounding}}{2.35cm} \\
\hline
\endhead
\endfoot
\endlastfoot
 &  &  & \HoloTaskMetric{\makecell[c]{\mbox{BLEU-4}}} & \HoloTaskScore{0.5543}{(0.5482--0.5604)}{4.55pt}{4.82pt} & \HoloTaskScore{0.6096}{(0.6017--0.6175)}{4.55pt}{4.82pt} & \HoloTaskScore{0.6371}{(0.6292--0.6445)}{4.55pt}{4.82pt} & \HoloTaskScore{0.6261}{(0.6184--0.6340)}{4.55pt}{4.82pt} & \HoloTaskScore{0.6253}{(0.6178--0.6335)}{4.55pt}{4.82pt} \\*
\softcline{4-9}
 &  & \HoloTaskSpan{{\fontsize{4.60pt}{4.90pt}\selectfont \makecell[c]{\textbf{NLP}}}}{1.30cm}{0pt} & \HoloTaskMetric{\makecell[c]{\mbox{ROUGE-L}}} & \HoloTaskScore{0.2832}{(0.2800--0.2867)}{4.55pt}{4.82pt} & \HoloTaskScore{0.4885}{(0.4788--0.4973)}{4.55pt}{4.82pt} & \HoloTaskScore{0.4841}{(0.4742--0.4937)}{4.55pt}{4.82pt} & \HoloTaskScore{0.4830}{(0.4732--0.4918)}{4.55pt}{4.82pt} & \HoloTaskScore{0.4859}{(0.4763--0.4945)}{4.55pt}{4.82pt} \\*
\softcline{4-9}
 &  &  & \HoloTaskMetric{\makecell[c]{\mbox{METEOR}}} & \HoloTaskScore{0.3766}{(0.3710--0.3828)}{4.55pt}{4.82pt} & \HoloTaskScore{0.5249}{(0.5151--0.5340)}{4.55pt}{4.82pt} & \HoloTaskScore{0.5460}{(0.5367--0.5547)}{4.55pt}{4.82pt} & \HoloTaskScore{0.5440}{(0.5349--0.5534)}{4.55pt}{4.82pt} & \HoloTaskScore{0.5460}{(0.5368--0.5552)}{4.55pt}{4.82pt} \\*
\cline{3-9}
 & \HoloTaskSpan{\makecell[c]{RadGenome}}{2.30cm}{0.32cm} &  & \HoloTaskMetric{\makecell[c]{\mbox{RaTEScore}}} & \HoloTaskScore{0.6607}{(0.6573--0.6640)}{4.55pt}{4.82pt} & \HoloTaskScore{0.7465}{(0.7412--0.7514)}{4.55pt}{4.82pt} & \HoloTaskScore{0.7497}{(0.7446--0.7547)}{4.55pt}{4.82pt} & \HoloTaskScore{0.7419}{(0.7370--0.7470)}{4.55pt}{4.82pt} & \HoloTaskScore{0.7482}{(0.7434--0.7533)}{4.55pt}{4.82pt} \\*
\softcline{4-9}
 &  & \HoloTaskSpan{{\fontsize{4.60pt}{4.90pt}\selectfont \makecell[c]{\textbf{Clinical}}}}{1.30cm}{0pt} & \HoloTaskMetric{\makecell[c]{\mbox{Llama}\\[-0.10ex]\mbox{Score}}} & \HoloTaskScore{6.541}{(6.493--6.586)}{4.55pt}{4.82pt} & \HoloTaskScore{6.820}{(6.719--6.911)}{4.55pt}{4.82pt} & \HoloTaskScore{7.230}{(7.149--7.310)}{4.55pt}{4.82pt} & \HoloTaskScore{7.154}{(7.063--7.240)}{4.55pt}{4.82pt} & \HoloTaskScore{7.181}{(7.093--7.271)}{4.55pt}{4.82pt} \\*
\softcline{4-9}
 &  &  & \HoloTaskMetric{\makecell[c]{\mbox{GREEN}}} & \HoloTaskScore{0.3919}{(0.3811--0.4028)}{4.55pt}{4.82pt} & \HoloTaskScore{0.4716}{(0.4580--0.4853)}{4.55pt}{4.82pt} & \HoloTaskScore{0.4595}{(0.4465--0.4727)}{4.55pt}{4.82pt} & \HoloTaskScore{0.4624}{(0.4499--0.4772)}{4.55pt}{4.82pt} & \HoloTaskScore{0.4740}{(0.4606--0.4868)}{4.55pt}{4.82pt} \\
\cline{2-9}
\HoloTaskSpan{\makecell[c]{\textbf{Internal}}}{1.35cm}{0.32cm} &  &  & \HoloTaskMetric{\makecell[c]{\mbox{BLEU-4}}} & \HoloTaskScore{0.1456$^{\blacktriangle}$}{(0.1378--0.1534)}{4.55pt}{4.82pt} & \HoloTaskScore{0.2799}{(0.2591--0.2998)}{4.55pt}{4.82pt} & \HoloTaskScore{0.3288}{(0.3046--0.3528)}{4.55pt}{4.82pt} & \HoloTaskScore{0.3278}{(0.3027--0.3508)}{4.55pt}{4.82pt} & \HoloTaskScore{0.3517}{(0.3257--0.3803)}{4.55pt}{4.82pt} \\*
\softcline{4-9}
 &  & \HoloTaskSpan{{\fontsize{4.60pt}{4.90pt}\selectfont \makecell[c]{\textbf{NLP}}}}{1.30cm}{0pt} & \HoloTaskMetric{\makecell[c]{\mbox{ROUGE-L}}} & \HoloTaskScore{0.3678$^{\blacktriangle}$}{(0.3589--0.3767)}{4.55pt}{4.82pt} & \HoloTaskScore{0.3170}{(0.3002--0.3355)}{4.55pt}{4.82pt} & \HoloTaskScore{0.3313}{(0.3090--0.3542)}{4.55pt}{4.82pt} & \HoloTaskScore{0.3572}{(0.3350--0.3808)}{4.55pt}{4.82pt} & \HoloTaskScore{0.3742}{(0.3481--0.4012)}{4.55pt}{4.82pt} \\*
\softcline{4-9}
 &  &  & \HoloTaskMetric{\makecell[c]{\mbox{METEOR}}} & \HoloTaskScore{0.2567$^{\blacktriangle}$}{(0.2489--0.2645)}{4.55pt}{4.82pt} & \HoloTaskScore{0.2512}{(0.2325--0.2709)}{4.55pt}{4.82pt} & \HoloTaskScore{0.2776}{(0.2543--0.3020)}{4.55pt}{4.82pt} & \HoloTaskScore{0.2975}{(0.2719--0.3209)}{4.55pt}{4.82pt} & \HoloTaskScore{0.3217}{(0.2954--0.3505)}{4.55pt}{4.82pt} \\*
\cline{3-9}
 & \HoloTaskSpan{\makecell[c]{ReXGroundingCT}}{2.30cm}{0.32cm} &  & \HoloTaskMetric{\makecell[c]{\mbox{RaTEScore}}} & \HoloTaskScore{0.5012$^{\blacktriangle}$}{(0.4898--0.5126)}{4.55pt}{4.82pt} & \HoloTaskScore{0.5252}{(0.5109--0.5399)}{4.55pt}{4.82pt} & \HoloTaskScore{0.5236}{(0.5056--0.5414)}{4.55pt}{4.82pt} & \HoloTaskScore{0.5509}{(0.5345--0.5677)}{4.55pt}{4.82pt} & \HoloTaskScore{0.5616}{(0.5444--0.5789)}{4.55pt}{4.82pt} \\*
\softcline{4-9}
 &  & \HoloTaskSpan{{\fontsize{4.60pt}{4.90pt}\selectfont \makecell[c]{\textbf{Clinical}}}}{1.30cm}{0pt} & \HoloTaskMetric{\makecell[c]{\mbox{Llama}\\[-0.10ex]\mbox{Score}}} & \HoloTaskScore{5.654$^{\blacktriangle}$}{(5.412--5.896)}{4.55pt}{4.82pt} & \HoloTaskScore{5.944}{(5.766--6.130)}{4.55pt}{4.82pt} & \HoloTaskScore{6.297}{(6.121--6.476)}{4.55pt}{4.82pt} & \HoloTaskScore{6.179}{(6.007--6.362)}{4.55pt}{4.82pt} & \HoloTaskScore{6.343}{(6.140--6.539)}{4.55pt}{4.82pt} \\*
\softcline{4-9}
 &  &  & \HoloTaskMetric{\makecell[c]{\mbox{GREEN}}} & \HoloTaskScore{0.1987$^{\blacktriangle}$}{(0.1854--0.2120)}{4.55pt}{4.82pt} & \HoloTaskScore{0.1788}{(0.1553--0.2049)}{4.55pt}{4.82pt} & \HoloTaskScore{0.2237}{(0.1969--0.2527)}{4.55pt}{4.82pt} & \HoloTaskScore{0.2173}{(0.1890--0.2465)}{4.55pt}{4.82pt} & \HoloTaskScore{0.2424}{(0.2128--0.2771)}{4.55pt}{4.82pt} \\
\hline
 &  &  & \HoloTaskMetric{\makecell[c]{\mbox{BLEU-4}}} & \HoloTaskScore{0.2759}{(0.2660--0.2847)}{4.55pt}{4.82pt} & \HoloTaskScore{0.4616}{(0.4525--0.4694)}{4.55pt}{4.82pt} & \HoloTaskScore{0.4791}{(0.4692--0.4851)}{4.55pt}{4.82pt} & \HoloTaskScore{0.4596}{(0.4497--0.4687)}{4.55pt}{4.82pt} & \HoloTaskScore{0.4672}{(0.4561--0.4756)}{4.55pt}{4.82pt} \\*
\softcline{4-9}
 &  & \HoloTaskSpan{{\fontsize{4.60pt}{4.90pt}\selectfont \makecell[c]{\textbf{NLP}}}}{1.30cm}{0pt} & \HoloTaskMetric{\makecell[c]{\mbox{ROUGE-L}}} & \HoloTaskScore{0.1309}{(0.1268--0.1350)}{4.55pt}{4.82pt} & \HoloTaskScore{0.2807}{(0.2750--0.2868)}{4.55pt}{4.82pt} & \HoloTaskScore{0.2974}{(0.2916--0.3020)}{4.55pt}{4.82pt} & \HoloTaskScore{0.3182}{(0.3112--0.3251)}{4.55pt}{4.82pt} & \HoloTaskScore{0.3277}{(0.3211--0.3334)}{4.55pt}{4.82pt} \\*
\softcline{4-9}
 &  &  & \HoloTaskMetric{\makecell[c]{\mbox{METEOR}}} & \HoloTaskScore{0.1676}{(0.1634--0.1720)}{4.55pt}{4.82pt} & \HoloTaskScore{0.4046}{(0.3963--0.4129)}{4.55pt}{4.82pt} & \HoloTaskScore{0.4274}{(0.4195--0.4361)}{4.55pt}{4.82pt} & \HoloTaskScore{0.4046}{(0.3952--0.4136)}{4.55pt}{4.82pt} & \HoloTaskScore{0.4117}{(0.4014--0.4210)}{4.55pt}{4.82pt} \\*
\cline{3-9}
 & \HoloTaskSpan{\makecell[c]{Private05(Abdomen\\[-0.10ex]Report)}}{2.30cm}{0.32cm} &  & \HoloTaskMetric{\makecell[c]{\mbox{RaTEScore}}} & \HoloTaskScore{0.4387}{(0.4313--0.4456)}{4.55pt}{4.82pt} & \HoloTaskScore{0.6435}{(0.6396--0.6475)}{4.55pt}{4.82pt} & \HoloTaskScore{0.6606}{(0.6558--0.6653)}{4.55pt}{4.82pt} & \HoloTaskScore{0.6646}{(0.6604--0.6691)}{4.55pt}{4.82pt} & \HoloTaskScore{0.6711}{(0.6671--0.6748)}{4.55pt}{4.82pt} \\*
\softcline{4-9}
 &  & \HoloTaskSpan{{\fontsize{4.60pt}{4.90pt}\selectfont \makecell[c]{\textbf{Clinical}}}}{1.30cm}{0pt} & \HoloTaskMetric{\makecell[c]{\mbox{Llama}\\[-0.10ex]\mbox{Score}}} & \HoloTaskScore{3.078}{(2.991--3.160)}{4.55pt}{4.82pt} & \HoloTaskScore{4.346}{(4.259--4.435)}{4.55pt}{4.82pt} & \HoloTaskScore{4.436}{(4.353--4.523)}{4.55pt}{4.82pt} & \HoloTaskScore{4.377}{(4.283--4.472)}{4.55pt}{4.82pt} & \HoloTaskScore{4.441}{(4.347--4.535)}{4.55pt}{4.82pt} \\*
\softcline{4-9}
 &  &  & \HoloTaskMetric{\makecell[c]{\mbox{GREEN}}} & \HoloTaskScore{0.09411}{(0.08255--0.1071)}{4.20pt}{4.48pt} & \HoloTaskScore{0.2735}{(0.2630--0.2843)}{4.55pt}{4.82pt} & \HoloTaskScore{0.2926}{(0.2802--0.3025)}{4.55pt}{4.82pt} & \HoloTaskScore{0.3256}{(0.3150--0.3357)}{4.55pt}{4.82pt} & \HoloTaskScore{0.3346}{(0.3228--0.3457)}{4.55pt}{4.82pt} \\
\cline{2-9}
\HoloTaskSpan{\makecell[c]{\textbf{Private}\\[-0.10ex]\textbf{(zero-}\\[-0.10ex]\textbf{shot)}}}{1.35cm}{0.32cm} &  &  & \HoloTaskMetric{\makecell[c]{\mbox{BLEU-4}}} & \HoloTaskScore{0.3234}{(0.3128--0.3344)}{4.55pt}{4.82pt} & \HoloTaskScore{0.4178}{(0.4084--0.4264)}{4.55pt}{4.82pt} & \HoloTaskScore{0.4358}{(0.4281--0.4444)}{4.55pt}{4.82pt} & \HoloTaskScore{0.4334}{(0.4243--0.4427)}{4.55pt}{4.82pt} & \HoloTaskScore{0.4412}{(0.4317--0.4500)}{4.55pt}{4.82pt} \\*
\softcline{4-9}
 &  & \HoloTaskSpan{{\fontsize{4.60pt}{4.90pt}\selectfont \makecell[c]{\textbf{NLP}}}}{1.30cm}{0pt} & \HoloTaskMetric{\makecell[c]{\mbox{ROUGE-L}}} & \HoloTaskScore{0.1565}{(0.1524--0.1603)}{4.55pt}{4.82pt} & \HoloTaskScore{0.2146}{(0.2124--0.2171)}{4.55pt}{4.82pt} & \HoloTaskScore{0.2327}{(0.2322--0.2359)}{4.55pt}{4.82pt} & \HoloTaskScore{0.2308}{(0.2281--0.2333)}{4.55pt}{4.82pt} & \HoloTaskScore{0.2424}{(0.2383--0.2462)}{4.55pt}{4.82pt} \\*
\softcline{4-9}
 &  &  & \HoloTaskMetric{\makecell[c]{\mbox{METEOR}}} & \HoloTaskScore{0.1965}{(0.1915--0.2010)}{4.55pt}{4.82pt} & \HoloTaskScore{0.3597}{(0.3525--0.3663)}{4.55pt}{4.82pt} & \HoloTaskScore{0.3859}{(0.3799--0.3920)}{4.55pt}{4.82pt} & \HoloTaskScore{0.3881}{(0.3808--0.3953)}{4.55pt}{4.82pt} & \HoloTaskScore{0.3986}{(0.3905--0.4052)}{4.55pt}{4.82pt} \\*
\cline{3-9}
 & \HoloTaskSpan{\makecell[c]{Private06(Chest\\[-0.10ex]Report)}}{2.30cm}{0.32cm} &  & \HoloTaskMetric{\makecell[c]{\mbox{RaTEScore}}} & \HoloTaskScore{0.5355}{(0.5297--0.5412)}{4.55pt}{4.82pt} & \HoloTaskScore{0.6044}{(0.6010--0.6081)}{4.55pt}{4.82pt} & \HoloTaskScore{0.6241}{(0.6201--0.6289)}{4.55pt}{4.82pt} & \HoloTaskScore{0.6216}{(0.6183--0.6250)}{4.55pt}{4.82pt} & \HoloTaskScore{0.6311}{(0.6296--0.6336)}{4.55pt}{4.82pt} \\*
\softcline{4-9}
 &  & \HoloTaskSpan{{\fontsize{4.60pt}{4.90pt}\selectfont \makecell[c]{\textbf{Clinical}}}}{1.30cm}{0pt} & \HoloTaskMetric{\makecell[c]{\mbox{Llama}\\[-0.10ex]\mbox{Score}}} & \HoloTaskScore{4.019}{(3.833--4.199)}{4.55pt}{4.82pt} & \HoloTaskScore{4.688}{(4.575--4.806)}{4.55pt}{4.82pt} & \HoloTaskScore{4.782}{(4.669--4.904)}{4.55pt}{4.82pt} & \HoloTaskScore{4.556}{(4.438--4.676)}{4.55pt}{4.82pt} & \HoloTaskScore{4.615}{(4.495--4.736)}{4.55pt}{4.82pt} \\*
\softcline{4-9}
 &  &  & \HoloTaskMetric{\makecell[c]{\mbox{GREEN}}} & \HoloTaskScore{0.09659}{(0.07852--0.1163)}{4.20pt}{4.48pt} & \HoloTaskScore{0.08956}{(0.08003--0.09852)}{4.20pt}{4.48pt} & \HoloTaskScore{0.1039}{(0.09320--0.1128)}{4.20pt}{4.48pt} & \HoloTaskScore{0.1149}{(0.1037--0.1265)}{4.55pt}{4.82pt} & \HoloTaskScore{0.1288}{(0.1175--0.1416)}{4.55pt}{4.82pt} \\
\hline
\end{longtable}
\arrayrulecolor{black}
\endgroup
