# Supplementary material for: A 3D foundation model unifying CT interpretation and segmentation
Source: arXiv:2611.06471 source file (2026-11-04)
Supplement: Supplementary file 2 [file table11_grounded_report_generation_radgenome_segmentation.tex]

\begingroup
\makeatletter
\@ifundefined{color@leftblue}{\definecolor{leftblue}{RGB}{232,242,248}}{}%
\@ifundefined{color@headerblue}{\definecolor{headerblue}{RGB}{218,233,242}}{}%
\makeatother
\setlength{\LTcapwidth}{18.60cm}
\setlength{\LTleft}{\fill}
\setlength{\LTright}{\fill}
\setlength{\LTpre}{0pt}
\setlength{\LTpost}{0pt}
\setlength{\tabcolsep}{0.45pt}
\renewcommand{\arraystretch}{1.00}
\setlength{\extrarowheight}{0pt}
\setlength{\arrayrulewidth}{0.48pt}
\arrayrulecolor{black}
\providecommand{\softcline}[1]{}%
\renewcommand{\softcline}[1]{\arrayrulecolor{black!35}\cline{#1}\arrayrulecolor{black}}
\sloppy
\emergencystretch=2em
\fontsize{5.30pt}{5.90pt}\selectfont
\newcommand{\HoloSegScore}[4]{%
  \parbox[c][0.64cm][c]{3.02cm}{%
    \centering
    {\fontsize{5.30pt}{5.58pt}\selectfont\strut\mbox{#1}}\\[-0.38ex]%
    {\fontsize{#3}{#4}\selectfont\strut\mbox{#2}}%
  }%
}%
\newcommand{\HoloSegUnsupported}{%
  \parbox[c][0.64cm][c]{3.02cm}{%
    \centering\fontsize{4.45pt}{4.70pt}\selectfont Not supported%
  }%
}%
\newcommand{\HoloSegMetric}[1]{%
  \parbox[c][0.64cm][c]{0.96cm}{%
    \centering\fontsize{5.45pt}{5.70pt}\selectfont\textbf{#1}%
  }%
}%
\newcommand{\HoloSegSpan}[3]{%
  \raisebox{#3}[0pt][0pt]{%
    \parbox[c]{#2}{\centering\arraybackslash #1}%
  }%
}%
\newcommand{\HoloSegSplitHead}[3]{%
  \parbox[c][0.92cm][c]{#3}{%
    \centering\fontsize{6.10pt}{6.35pt}\selectfont\textbf{#1}\\[-0.52ex]%
    \rule{0pt}{0.58ex}\\[-0.52ex]\textbf{#2}%
  }%
}%
\newcommand{\HoloSegMidHead}[2]{%
  \parbox[c][0.92cm][c]{#2}{%
    \centering\fontsize{5.40pt}{5.70pt}\selectfont\textbf{#1}%
  }%
}%
\begin{longtable}{|>{\columncolor{leftblue}\centering\arraybackslash}m{1.30cm}|>{\columncolor{leftblue}\centering\arraybackslash}m{2.20cm}|>{\columncolor{leftblue}\centering\arraybackslash}m{3.10cm}|>{\columncolor{leftblue}\centering\arraybackslash}m{1.00cm}|>{\centering\arraybackslash}m{1.65cm}|>{\centering\arraybackslash}m{3.05cm}|>{\centering\arraybackslash}m{1.65cm}|>{\centering\arraybackslash}m{3.05cm}|}
\caption[RadGenome segmentation performance for anatomy-grounded report generation]{\textbf{Segmentation performance on RadGenome for anatomy-grounded report generation.}\newline Each score is reported as mean with 95\% confidence interval. Match counts denote matched/reference regions; Dice and HD95 use matched regions. Dice measures volumetric overlap and HD95 denotes the 95th-percentile Hausdorff distance in millimetres.}%
\label{tab:grounded_report_radgenome_segmentation}\\[-0.15ex]
\hline
\rowcolor{headerblue}
\HoloSegSplitHead{Dataset}{Type}{1.30cm} & \HoloSegSplitHead{Dataset}{Name}{2.20cm} & \HoloSegSplitHead{Region}{Name}{3.10cm} & \HoloSegMidHead{Metric}{1.00cm} & \HoloSegMidHead{\makecell[c]{Match\\count-4B}}{1.65cm} & \HoloSegMidHead{HoloCT-4B}{3.05cm} & \HoloSegMidHead{\makecell[c]{Match\\count-8B}}{1.65cm} & \HoloSegMidHead{HoloCT-8B}{3.05cm} \\
\hline
\endfirsthead
\caption*{\textbf{Supplementary Table~\ref{tab:grounded_report_radgenome_segmentation} (continued)\enspace|\enspace Segmentation performance on RadGenome for anatomy-grounded report generation.}\newline Each score is reported as mean with 95\% confidence interval. Match counts denote matched/reference regions; Dice and HD95 use matched regions. Dice measures volumetric overlap and HD95 denotes the 95th-percentile Hausdorff distance in millimetres.}\\[-0.15ex]
\hline
\rowcolor{headerblue}
\HoloSegSplitHead{Dataset}{Type}{1.30cm} & \HoloSegSplitHead{Dataset}{Name}{2.20cm} & \HoloSegSplitHead{Region}{Name}{3.10cm} & \HoloSegMidHead{Metric}{1.00cm} & \HoloSegMidHead{\makecell[c]{Match\\count-4B}}{1.65cm} & \HoloSegMidHead{HoloCT-4B}{3.05cm} & \HoloSegMidHead{\makecell[c]{Match\\count-8B}}{1.65cm} & \HoloSegMidHead{HoloCT-8B}{3.05cm} \\
\hline
\endhead
\endfoot
\endlastfoot
 &  &  & \HoloSegMetric{Dice} &  & \HoloSegScore{0.9053}{(0.9008--0.9094)}{4.55pt}{4.82pt} &  & \HoloSegScore{0.9117}{(0.9075--0.9155)}{4.55pt}{4.82pt} \\*
\softcline{4-4}\softcline{6-6}\softcline{8-8}
 &  & \HoloSegSpan{\makecell[c]{abdomen}}{3.10cm}{0.32cm} & \HoloSegMetric{HD95} & \HoloSegSpan{1518/1518}{1.65cm}{0.32cm} & \HoloSegScore{10.21}{(9.316--11.41)}{4.55pt}{4.82pt} & \HoloSegSpan{1518/1518}{1.65cm}{0.32cm} & \HoloSegScore{10.17}{(9.615--10.74)}{4.55pt}{4.82pt} \\
\cline{3-8}
 &  &  & \HoloSegMetric{Dice} &  & \HoloSegScore{0.9169}{(0.9144--0.9192)}{4.55pt}{4.82pt} &  & \HoloSegScore{0.9192}{(0.9168--0.9211)}{4.55pt}{4.82pt} \\*
\softcline{4-4}\softcline{6-6}\softcline{8-8}
 &  & \HoloSegSpan{\makecell[c]{bone}}{3.10cm}{0.32cm} & \HoloSegMetric{HD95} & \HoloSegSpan{1509/1509}{1.65cm}{0.32cm} & \HoloSegScore{2.091}{(1.572--2.900)}{4.55pt}{4.82pt} & \HoloSegSpan{1509/1509}{1.65cm}{0.32cm} & \HoloSegScore{1.698}{(1.512--1.900)}{4.55pt}{4.82pt} \\
\cline{3-8}
 &  &  & \HoloSegMetric{Dice} &  & \HoloSegScore{0.5384}{(0.4603--0.6109)}{4.55pt}{4.82pt} &  & \HoloSegScore{0.5116}{(0.4367--0.5764)}{4.55pt}{4.82pt} \\*
\softcline{4-4}\softcline{6-6}\softcline{8-8}
 &  & \HoloSegSpan{\makecell[c]{breast}}{3.10cm}{0.32cm} & \HoloSegMetric{HD95} & \HoloSegSpan{58/58}{1.65cm}{0.32cm} & \HoloSegScore{64.27}{(34.52--98.07)}{4.55pt}{4.82pt} & \HoloSegSpan{58/58}{1.65cm}{0.32cm} & \HoloSegScore{63.07}{(31.95--98.62)}{4.55pt}{4.82pt} \\
\cline{3-8}
 &  &  & \HoloSegMetric{Dice} &  & \HoloSegScore{0.8766}{(0.8728--0.8800)}{4.55pt}{4.82pt} &  & \HoloSegScore{0.8758}{(0.8723--0.8789)}{4.55pt}{4.82pt} \\*
\softcline{4-4}\softcline{6-6}\softcline{8-8}
 &  & \HoloSegSpan{\makecell[c]{esophagus}}{3.10cm}{0.32cm} & \HoloSegMetric{HD95} & \HoloSegSpan{1328/1328}{1.65cm}{0.32cm} & \HoloSegScore{2.438}{(1.914--3.392)}{4.55pt}{4.82pt} & \HoloSegSpan{1328/1328}{1.65cm}{0.32cm} & \HoloSegScore{1.962}{(1.843--2.103)}{4.55pt}{4.82pt} \\
\cline{3-8}
 &  &  & \HoloSegMetric{Dice} &  & \HoloSegScore{0.9102}{(0.9050--0.9150)}{4.55pt}{4.82pt} &  & \HoloSegScore{0.9103}{(0.9046--0.9157)}{4.55pt}{4.82pt} \\*
\softcline{4-4}\softcline{6-6}\softcline{8-8}
 &  & \HoloSegSpan{\makecell[c]{heart}}{3.10cm}{0.32cm} & \HoloSegMetric{HD95} & \HoloSegSpan{1433/1433}{1.65cm}{0.32cm} & \HoloSegScore{19.07}{(16.65--21.25)}{4.55pt}{4.82pt} & \HoloSegSpan{1433/1433}{1.65cm}{0.32cm} & \HoloSegScore{19.55}{(17.01--21.97)}{4.55pt}{4.82pt} \\
\cline{3-8}
\HoloSegSpan{\makecell[c]{\textbf{Internal}}}{1.30cm}{0.32cm} & \HoloSegSpan{\makecell[c]{RadGenome}}{2.20cm}{0.32cm} &  & \HoloSegMetric{Dice} &  & \HoloSegScore{0.9717}{(0.9672--0.9760)}{4.55pt}{4.82pt} &  & \HoloSegScore{0.9725}{(0.9680--0.9766)}{4.55pt}{4.82pt} \\*
\softcline{4-4}\softcline{6-6}\softcline{8-8}
 &  & \HoloSegSpan{\makecell[c]{lung}}{3.10cm}{0.32cm} & \HoloSegMetric{HD95} & \HoloSegSpan{1514/1514}{1.65cm}{0.32cm} & \HoloSegScore{4.429}{(3.411--5.795)}{4.55pt}{4.82pt} & \HoloSegSpan{1514/1514}{1.65cm}{0.32cm} & \HoloSegScore{3.606}{(3.067--4.233)}{4.55pt}{4.82pt} \\
\cline{3-8}
 &  &  & \HoloSegMetric{Dice} &  & \HoloSegScore{0.8254}{(0.8209--0.8295)}{4.55pt}{4.82pt} &  & \HoloSegScore{0.8368}{(0.8326--0.8404)}{4.55pt}{4.82pt} \\*
\softcline{4-4}\softcline{6-6}\softcline{8-8}
 &  & \HoloSegSpan{\makecell[c]{mediastinum}}{3.10cm}{0.32cm} & \HoloSegMetric{HD95} & \HoloSegSpan{1523/1523}{1.65cm}{0.32cm} & \HoloSegScore{7.088}{(5.523--8.882)}{4.55pt}{4.82pt} & \HoloSegSpan{1523/1523}{1.65cm}{0.32cm} & \HoloSegScore{6.082}{(4.816--7.520)}{4.55pt}{4.82pt} \\
\cline{3-8}
 &  &  & \HoloSegMetric{Dice} &  & \HoloSegScore{0.9711}{(0.9655--0.9763)}{4.55pt}{4.82pt} &  & \HoloSegScore{0.9721}{(0.9666--0.9769)}{4.55pt}{4.82pt} \\*
\softcline{4-4}\softcline{6-6}\softcline{8-8}
 &  & \HoloSegSpan{\makecell[c]{pleura}}{3.10cm}{0.32cm} & \HoloSegMetric{HD95} & \HoloSegSpan{1172/1172}{1.65cm}{0.32cm} & \HoloSegScore{5.062}{(3.602--6.899)}{4.55pt}{4.82pt} & \HoloSegSpan{1172/1172}{1.65cm}{0.32cm} & \HoloSegScore{4.107}{(3.230--5.071)}{4.55pt}{4.82pt} \\
\cline{3-8}
 &  &  & \HoloSegMetric{Dice} &  & \HoloSegScore{0.7054}{(0.6395--0.7564)}{4.55pt}{4.82pt} &  & \HoloSegScore{0.7182}{(0.6578--0.7691)}{4.55pt}{4.82pt} \\*
\softcline{4-4}\softcline{6-6}\softcline{8-8}
 &  & \HoloSegSpan{\makecell[c]{thyroid}}{3.10cm}{0.32cm} & \HoloSegMetric{HD95} & \HoloSegSpan{51/51}{1.65cm}{0.32cm} & \HoloSegScore{7.121}{(4.199--11.72)}{4.55pt}{4.82pt} & \HoloSegSpan{51/51}{1.65cm}{0.32cm} & \HoloSegScore{4.855}{(3.430--6.600)}{4.55pt}{4.82pt} \\
\cline{3-8}
 &  &  & \HoloSegMetric{Dice} &  & \HoloSegScore{0.9154}{(0.9111--0.9191)}{4.55pt}{4.82pt} &  & \HoloSegScore{0.9175}{(0.9134--0.9210)}{4.55pt}{4.82pt} \\*
\softcline{4-4}\softcline{6-6}\softcline{8-8}
 &  & \HoloSegSpan{\makecell[c]{trachea and\\[-0.10ex]bronchi}}{3.10cm}{0.32cm} & \HoloSegMetric{HD95} & \HoloSegSpan{1417/1417}{1.65cm}{0.32cm} & \HoloSegScore{2.954}{(1.839--4.399)}{4.55pt}{4.82pt} & \HoloSegSpan{1417/1417}{1.65cm}{0.32cm} & \HoloSegScore{3.019}{(1.888--4.331)}{4.55pt}{4.82pt} \\
\hline
\end{longtable}
\arrayrulecolor{black}
\endgroup
