# Supplementary material for: A 3D foundation model unifying CT interpretation and segmentation
Source: arXiv:2611.06471 source file (2026-11-04)
Supplement: Supplementary file 3 [file table12_finding_level_referring_segmentation.tex]

\begingroup
\makeatletter
\@ifundefined{color@leftblue}{\definecolor{leftblue}{RGB}{232,242,248}}{}%
\@ifundefined{color@headerblue}{\definecolor{headerblue}{RGB}{218,233,242}}{}%
\makeatother
\setlength{\LTcapwidth}{18.60cm}
\setlength{\LTleft}{\fill}
\setlength{\LTright}{\fill}
\setlength{\LTpre}{0pt}
\setlength{\LTpost}{0pt}
\setlength{\tabcolsep}{0.45pt}
\renewcommand{\arraystretch}{1.00}
\setlength{\extrarowheight}{0pt}
\setlength{\arrayrulewidth}{0.48pt}
\arrayrulecolor{black}
\fontsize{5.30pt}{5.90pt}\selectfont
\newcommand{\HoloTaskScore}[4]{%
  \parbox[c][0.64cm][c]{3.62cm}{%
    \centering
    {\fontsize{5.30pt}{5.58pt}\selectfont\strut\mbox{#1}}\\[-0.38ex]%
    {\fontsize{#3}{#4}\selectfont\strut\mbox{#2}}%
  }%
}%
\newcommand{\HoloTaskHead}[2]{%
  \parbox[c][0.92cm][c]{#2}{%
    \centering\fontsize{5.80pt}{6.05pt}\selectfont\textbf{#1}%
  }%
}%
\newcommand{\HoloTaskMetric}[1]{%
  \parbox[c][0.64cm][c]{3.26cm}{%
    \centering\fontsize{5.45pt}{5.72pt}\selectfont\textbf{#1}%
  }%
}%
\begin{longtable}{|>{\columncolor{leftblue}\centering\arraybackslash}m{3.30cm}|>{\centering\arraybackslash}m{3.65cm}|>{\centering\arraybackslash}m{3.65cm}|>{\centering\arraybackslash}m{3.65cm}|>{\centering\arraybackslash}m{3.65cm}|}
\caption[Finding-level referring segmentation]{\textbf{Finding-level referring segmentation performance.}\newline Each score is reported as mean with 95\% confidence interval.}%
\label{tab:finding_level_referring_segmentation}\\[-0.15ex]
\hline
\rowcolor{headerblue}
\HoloTaskHead{Metric}{3.30cm} & \HoloTaskHead{\makecell[c]{HoloCT-8B}}{3.65cm} & \HoloTaskHead{\makecell[c]{HoloCT-4B}}{3.65cm} & \HoloTaskHead{\makecell[c]{VoxTell}}{3.65cm} & \HoloTaskHead{\makecell[c]{SAT-Pro}}{3.65cm} \\
\hline
\endfirsthead
\caption*{\textbf{Supplementary Table~\ref{tab:finding_level_referring_segmentation} (continued)\enspace|\enspace Finding-level referring segmentation performance.}\newline Each score is reported as mean with 95\% confidence interval.}\\[-0.15ex]
\hline
\rowcolor{headerblue}
\HoloTaskHead{Metric}{3.30cm} & \HoloTaskHead{\makecell[c]{HoloCT-8B}}{3.65cm} & \HoloTaskHead{\makecell[c]{HoloCT-4B}}{3.65cm} & \HoloTaskHead{\makecell[c]{VoxTell}}{3.65cm} & \HoloTaskHead{\makecell[c]{SAT-Pro}}{3.65cm} \\
\hline
\endhead
\endfoot
\endlastfoot
\HoloTaskMetric{Non-focal Dice} & \HoloTaskScore{0.2517}{(0.2237--0.2767)}{4.55pt}{4.82pt} & \HoloTaskScore{0.1830}{(0.1578--0.2065)}{4.55pt}{4.82pt} & \HoloTaskScore{0.1493}{(0.1292--0.1831)}{4.55pt}{4.82pt} & \HoloTaskScore{0.09780}{(0.08140--0.1241)}{4.20pt}{4.48pt} \\
\hline
\HoloTaskMetric{Focal Dice} & \HoloTaskScore{0.3010}{(0.2864--0.3165)}{4.55pt}{4.82pt} & \HoloTaskScore{0.2414}{(0.2273--0.2554)}{4.55pt}{4.82pt} & \HoloTaskScore{0.2781}{(0.2627--0.2979)}{4.55pt}{4.82pt} & \HoloTaskScore{0.1849}{(0.1781--0.2068)}{4.55pt}{4.82pt} \\
\hline
\HoloTaskMetric{Average Dice} & \HoloTaskScore{0.2908}{(0.2769--0.3038)}{4.55pt}{4.82pt} & \HoloTaskScore{0.2293}{(0.2168--0.2420)}{4.55pt}{4.82pt} & \HoloTaskScore{0.2591}{(0.2404--0.2738)}{4.55pt}{4.82pt} & \HoloTaskScore{0.1681}{(0.1515--0.1846)}{4.55pt}{4.82pt} \\
\hline
\HoloTaskMetric{HIT5\%} & \HoloTaskScore{0.7700}{(0.7457--0.7943)}{4.55pt}{4.82pt} & \HoloTaskScore{0.6936}{(0.6684--0.7205)}{4.55pt}{4.82pt} & \HoloTaskScore{0.6592}{(0.6383--0.6851)}{4.55pt}{4.82pt} & \HoloTaskScore{0.5291}{(0.5013--0.5630)}{4.55pt}{4.82pt} \\
\hline
\HoloTaskMetric{HIT10\%} & \HoloTaskScore{0.7118}{(0.6866--0.7387)}{4.55pt}{4.82pt} & \HoloTaskScore{0.6128}{(0.5868--0.6406)}{4.55pt}{4.82pt} & \HoloTaskScore{0.5991}{(0.5767--0.6251)}{4.55pt}{4.82pt} & \HoloTaskScore{0.4863}{(0.4619--0.5195)}{4.55pt}{4.82pt} \\
\hline
\end{longtable}
\arrayrulecolor{black}
\endgroup
