# Supplementary material for: A 3D foundation model unifying CT interpretation and segmentation
Source: arXiv:2611.06471 source file (2026-11-04)
Supplement: Supplementary file 4 [file table13_grounded_report_generation_rexgrounding_segmentation.tex]

\begingroup
\makeatletter
\@ifundefined{color@leftblue}{\definecolor{leftblue}{RGB}{232,242,248}}{}%
\@ifundefined{color@headerblue}{\definecolor{headerblue}{RGB}{218,233,242}}{}%
\makeatother
\setlength{\LTcapwidth}{18.60cm}
\setlength{\LTleft}{\fill}
\setlength{\LTright}{\fill}
\setlength{\LTpre}{0pt}
\setlength{\LTpost}{0pt}
\setlength{\tabcolsep}{0.45pt}
\renewcommand{\arraystretch}{1.00}
\setlength{\extrarowheight}{0pt}
\setlength{\arrayrulewidth}{0.48pt}
\arrayrulecolor{black}
\fontsize{5.30pt}{5.90pt}\selectfont
\newcommand{\HoloTaskScore}[4]{%
  \parbox[c][0.64cm][c]{4.27cm}{%
    \centering
    {\fontsize{5.30pt}{5.58pt}\selectfont\strut\mbox{#1}}\\[-0.38ex]%
    {\fontsize{#3}{#4}\selectfont\strut\mbox{#2}}%
  }%
}%
\newcommand{\HoloTaskHead}[2]{%
  \parbox[c][0.92cm][c]{#2}{%
    \centering\fontsize{5.80pt}{6.05pt}\selectfont\textbf{#1}%
  }%
}%
\newcommand{\HoloTaskMetric}[1]{%
  \parbox[c][0.64cm][c]{4.26cm}{%
    \centering\fontsize{5.30pt}{5.57pt}\selectfont\textbf{#1}%
  }%
}%
\begin{longtable}{|>{\columncolor{leftblue}\centering\arraybackslash}m{4.30cm}|>{\centering\arraybackslash}m{4.30cm}|>{\centering\arraybackslash}m{4.30cm}|>{\centering\arraybackslash}m{4.30cm}|}
\caption[Finding-grounded report generation]{\textbf{Finding-grounded report generation performance.}\newline Each score is reported as mean with 95\% confidence interval.}%
\label{tab:finding_level_grounded_report_generation}\\[-0.15ex]
\hline
\rowcolor{headerblue}
\HoloTaskHead{Metric}{4.30cm} & \HoloTaskHead{\makecell[c]{HoloCT-8B}}{4.30cm} & \HoloTaskHead{\makecell[c]{HoloCT-4B}}{4.30cm} & \HoloTaskHead{\makecell[c]{HuluMed-32B\\[-0.18ex]+ VoxTell}}{4.30cm} \\
\hline
\endfirsthead
\caption*{\textbf{Supplementary Table~\ref{tab:finding_level_grounded_report_generation} (continued)\enspace|\enspace Finding-grounded report generation performance.}\newline Each score is reported as mean with 95\% confidence interval.}\\[-0.15ex]
\hline
\rowcolor{headerblue}
\HoloTaskHead{Metric}{4.30cm} & \HoloTaskHead{\makecell[c]{HoloCT-8B}}{4.30cm} & \HoloTaskHead{\makecell[c]{HoloCT-4B}}{4.30cm} & \HoloTaskHead{\makecell[c]{HuluMed-32B\\[-0.18ex]+ VoxTell}}{4.30cm} \\
\hline
\endhead
\endfoot
\endlastfoot
\HoloTaskMetric{\makecell[c]{Finding F1}} & \HoloTaskScore{0.2776}{(0.2475--0.3139)}{4.55pt}{4.82pt} & \HoloTaskScore{0.2860}{(0.2579--0.3149)}{4.55pt}{4.82pt} & \HoloTaskScore{0.2386}{(0.2129--0.2777)}{4.55pt}{4.82pt} \\
\hline
\HoloTaskMetric{\makecell[c]{Non-focal\\[-0.12ex]conditional Dice}} & \HoloTaskScore{0.1789}{(0.1233--0.2356)}{4.55pt}{4.82pt} & \HoloTaskScore{0.1020}{(0.05502--0.1574)}{4.20pt}{4.48pt} & \HoloTaskScore{0.1271}{(0.08630--0.1758)}{4.20pt}{4.48pt} \\
\hline
\HoloTaskMetric{\makecell[c]{Focal\\[-0.12ex]conditional Dice}} & \HoloTaskScore{0.2427}{(0.2162--0.2702)}{4.55pt}{4.82pt} & \HoloTaskScore{0.1503}{(0.1284--0.1740)}{4.55pt}{4.82pt} & \HoloTaskScore{0.2073}{(0.1816--0.2307)}{4.55pt}{4.82pt} \\
\hline
\HoloTaskMetric{\makecell[c]{Average\\[-0.12ex]conditional Dice}} & \HoloTaskScore{0.2339}{(0.2093--0.2579)}{4.55pt}{4.82pt} & \HoloTaskScore{0.1432}{(0.1218--0.1637)}{4.55pt}{4.82pt} & \HoloTaskScore{0.1857}{(0.1646--0.2134)}{4.55pt}{4.82pt} \\
\hline
\HoloTaskMetric{\makecell[c]{Conditional\\[-0.12ex]HIT5\%}} & \HoloTaskScore{0.7382}{(0.6864--0.7862)}{4.55pt}{4.82pt} & \HoloTaskScore{0.5131}{(0.4545--0.5715)}{4.55pt}{4.82pt} & \HoloTaskScore{0.7386}{(0.6900--0.7968)}{4.55pt}{4.82pt} \\
\hline
\HoloTaskMetric{\makecell[c]{Conditional\\[-0.12ex]HIT10\%}} & \HoloTaskScore{0.6691}{(0.6127--0.7263)}{4.55pt}{4.82pt} & \HoloTaskScore{0.4444}{(0.3876--0.5017)}{4.55pt}{4.82pt} & \HoloTaskScore{0.5035}{(0.4502--0.5633)}{4.55pt}{4.82pt} \\
\hline
\end{longtable}
\arrayrulecolor{black}
\endgroup
