# Supplementary material for: A 3D foundation model unifying CT interpretation and segmentation
Source: arXiv:2611.06471 source file (2026-11-04)
Supplement: Supplementary file 5 [file table15_S1_S6.tex]

\begingroup
\makeatletter
\@ifundefined{color@leftblue}{\definecolor{leftblue}{RGB}{232,242,248}}{}%
\@ifundefined{color@headerblue}{\definecolor{headerblue}{RGB}{218,233,242}}{}%
\makeatother
\setlength{\LTcapwidth}{18.60cm}
\setlength{\LTleft}{\fill}
\setlength{\LTright}{\fill}
\setlength{\LTpre}{0pt}
\setlength{\LTpost}{0pt}
\setlength{\tabcolsep}{0.45pt}
\renewcommand{\arraystretch}{1.00}
\setlength{\extrarowheight}{0pt}
\setlength{\arrayrulewidth}{0.48pt}
\arrayrulecolor{black}
\providecommand{\softcline}[1]{}%
\renewcommand{\softcline}[1]{\arrayrulecolor{black!35}\cline{#1}\arrayrulecolor{black}}
\sloppy
\emergencystretch=2em
\fontsize{5.20pt}{5.80pt}\selectfont
\newcommand{\AblScoreCI}[5]{%
  \parbox[c][0.64cm][c]{1.97cm}{%
    \centering
    {\fontsize{5.20pt}{5.48pt}\selectfont\strut\mbox{#1#5}}\\[-0.38ex]%
    {\fontsize{#3}{#4}\selectfont\strut\mbox{#2}}%
  }%
}%
\newcommand{\AblScoreSingle}[2]{%
  \parbox[c][0.64cm][c]{1.97cm}{%
    \centering
    {\fontsize{5.20pt}{5.48pt}\selectfont\strut\mbox{#1#2}}%
  }%
}%
\newcommand{\AblMetric}[1]{%
  \parbox[c][0.64cm][c]{1.55cm}{%
    \centering\fontsize{5.05pt}{5.32pt}\selectfont #1%
  }%
}%
\newcommand{\AblOverall}[1]{%
  \parbox[c][0.64cm][c]{\dimexpr2.65cm+1.55cm+2\tabcolsep+\arrayrulewidth\relax}{%
    \centering\fontsize{5.20pt}{5.48pt}\selectfont\textbf{#1}%
  }%
}%
\newcommand{\AblSpan}[3]{%
  \raisebox{\dimexpr#3-0.11cm\relax}[0pt][0pt]{%
    \parbox[c][0.64cm][c]{#2}{\centering\arraybackslash #1}%
  }%
}%
\newcommand{\AblHead}[2]{%
  \parbox[c][0.92cm][c]{#2}{%
    \centering\fontsize{5.90pt}{6.15pt}\selectfont\textbf{#1}%
  }%
}%
\begin{longtable}{|>{\columncolor{leftblue}\centering\arraybackslash}m{2.30cm}|>{\columncolor{leftblue}\centering\arraybackslash}m{2.65cm}|>{\columncolor{leftblue}\centering\arraybackslash}m{1.55cm}|>{\centering\arraybackslash}m{2.00cm}|>{\centering\arraybackslash}m{2.00cm}|>{\centering\arraybackslash}m{2.00cm}|>{\centering\arraybackslash}m{2.00cm}|>{\centering\arraybackslash}m{2.00cm}|>{\centering\arraybackslash}m{2.00cm}|}
\caption[Training-strategy ablations S1--S6 across tasks]{\textbf{Training-strategy ablations S1--S6 across segmentation, grounded lesion screening, grounded visual question answering, and grounded report generation.}\newline For segmentation, Macro Dice denotes the dataset-level macro Dice. For grounded lesion screening, Macro F1 is calculated as the arithmetic mean of label-wise F1 scores within each dataset. For grounded visual question answering, Accu. denotes accuracy. For grounded report generation, BLEU-4, ROUGE-L, METEOR, RaTEScore, LlamaScore, and GREEN are reported. Overall scores retain the supplied task-level summaries and are shown without confidence intervals; the report-generation Overall score is LCS. Dataset scores are reported as mean with 95\% confidence interval when available.}%
\label{tab:ablation_study_detailed_scores}\\[-0.15ex]
\hline
\rowcolor{headerblue}
\AblHead{Task}{2.30cm} & \AblHead{Dataset Name}{2.65cm} & \AblHead{Metric}{1.55cm} & \AblHead{S1}{2.00cm} & \AblHead{S2}{2.00cm} & \AblHead{S3}{2.00cm} & \AblHead{S4}{2.00cm} & \AblHead{S5}{2.00cm} & \AblHead{S6}{2.00cm} \\
\hline
\endfirsthead
\caption*{\textbf{Supplementary Table~\ref{tab:ablation_study_detailed_scores} (continued)\enspace|\enspace Training-strategy ablations S1--S6 across segmentation, grounded lesion screening, grounded visual question answering, and grounded report generation.}\newline For segmentation, Macro Dice denotes the dataset-level macro Dice. For grounded lesion screening, Macro F1 is calculated as the arithmetic mean of label-wise F1 scores within each dataset. For grounded visual question answering, Accu. denotes accuracy. For grounded report generation, BLEU-4, ROUGE-L, METEOR, RaTEScore, LlamaScore, and GREEN are reported. Overall scores retain the supplied task-level summaries and are shown without confidence intervals; the report-generation Overall score is LCS. Dataset scores are reported as mean with 95\% confidence interval when available.}\\[-0.15ex]
\hline
\rowcolor{headerblue}
\AblHead{Task}{2.30cm} & \AblHead{Dataset Name}{2.65cm} & \AblHead{Metric}{1.55cm} & \AblHead{S1}{2.00cm} & \AblHead{S2}{2.00cm} & \AblHead{S3}{2.00cm} & \AblHead{S4}{2.00cm} & \AblHead{S5}{2.00cm} & \AblHead{S6}{2.00cm} \\
\hline
\endhead
\endfoot
\endlastfoot
 & \AblSpan{\makecell[c]{Total-\\[0.05ex]SegmentatorV2}}{2.65cm}{0pt} & \AblMetric{\makecell[c]{\textbf{Macro Dice}}} &  & \AblScoreCI{0.6508}{(0.6384--0.6703)}{4.35pt}{4.62pt}{} & \AblScoreCI{0.6626}{(0.6573--0.6733)}{4.35pt}{4.62pt}{} & \AblScoreCI{0.7467}{(0.7351--0.7584)}{4.35pt}{4.62pt}{} & \AblScoreCI{0.7779}{(0.7604--0.7874)}{4.35pt}{4.62pt}{} & \AblScoreCI{0.7775}{(0.7641--0.7892)}{4.35pt}{4.62pt}{} \\*
\cline{2-3}\cline{5-9}
\AblSpan{\makecell[c]{\textbf{Segmentation}}}{2.30cm}{0pt} & \AblSpan{\makecell[c]{AbdomenAtlas3.0}}{2.65cm}{0pt} & \AblMetric{\makecell[c]{\textbf{Macro Dice}}} & \AblScoreSingle{\fontsize{4.30pt}{4.55pt}\selectfont Not supported}{} & \AblScoreCI{0.5514}{(0.5255--0.5761)}{4.35pt}{4.62pt}{} & \AblScoreCI{0.5631}{(0.5445--0.5827)}{4.35pt}{4.62pt}{} & \AblScoreCI{0.6421}{(0.6275--0.6673)}{4.35pt}{4.62pt}{} & \AblScoreCI{0.6949}{(0.6700--0.7098)}{4.35pt}{4.62pt}{} & \AblScoreCI{0.7015}{(0.6827--0.7160)}{4.35pt}{4.62pt}{} \\*
\cline{2-3}\cline{5-9}
 & \multicolumn{2}{>{\columncolor{leftblue}\centering\arraybackslash}m{\dimexpr2.65cm+1.55cm+2\tabcolsep+\arrayrulewidth\relax}|}{\AblOverall{Overall}} &  & \AblScoreSingle{0.6011}{} & \AblScoreSingle{0.6129}{} & \AblScoreSingle{0.6944}{} & \AblScoreSingle{0.7364}{} & \AblScoreSingle{0.7395}{} \\
\hline
 & \AblSpan{\makecell[c]{AbdomenAtlas3.0}}{2.65cm}{0pt} & \AblMetric{\makecell[c]{\textbf{Macro F1}}} & \AblScoreCI{0.2955}{(0.2557--0.3367)}{4.35pt}{4.62pt}{} & \AblScoreCI{0.3181}{(0.2740--0.3597)}{4.35pt}{4.62pt}{} & \AblScoreCI{0.3720}{(0.3268--0.4169)}{4.35pt}{4.62pt}{} & \AblScoreCI{0.4241}{(0.3753--0.4681)}{4.35pt}{4.62pt}{} & \AblScoreCI{0.4745}{(0.4263--0.5188)}{4.35pt}{4.62pt}{} & \AblScoreCI{0.4852}{(0.4374--0.5296)}{4.35pt}{4.62pt}{} \\
\cline{2-9}
\AblSpan{\makecell[c]{\textbf{Grounded lesion}\\[0.05ex]\textbf{screening}}}{2.30cm}{0pt} & \AblSpan{\makecell[c]{LiMT}}{2.65cm}{0pt} & \AblMetric{\makecell[c]{\textbf{Macro F1}}} & \AblScoreCI{0.2172}{(0.07629--0.3404)}{4.02pt}{4.28pt}{} & \AblScoreCI{0.2320}{(0.07941--0.3628)}{4.02pt}{4.28pt}{} & \AblScoreCI{0.3298}{(0.1483--0.4713)}{4.35pt}{4.62pt}{} & \AblScoreCI{0.4287}{(0.2525--0.5619)}{4.35pt}{4.62pt}{} & \AblScoreCI{0.5060}{(0.3396--0.6299)}{4.35pt}{4.62pt}{} & \AblScoreCI{0.5455}{(0.3521--0.7089)}{4.35pt}{4.62pt}{} \\
\cline{2-9}
 & \multicolumn{2}{>{\columncolor{leftblue}\centering\arraybackslash}m{\dimexpr2.65cm+1.55cm+2\tabcolsep+\arrayrulewidth\relax}|}{\AblOverall{Overall}} & \AblScoreSingle{0.2563}{} & \AblScoreSingle{0.2751}{} & \AblScoreSingle{0.3509}{} & \AblScoreSingle{0.4264}{} & \AblScoreSingle{0.4903}{} & \AblScoreSingle{0.5153}{} \\
\hline
 & \AblSpan{\makecell[c]{AMOS-MM-VQA}}{2.65cm}{0pt} & \AblMetric{\makecell[c]{\textbf{Accu.}}} & \AblScoreCI{0.6958}{(0.6388--0.7529)}{4.35pt}{4.62pt}{} & \AblScoreCI{0.7119}{(0.6550--0.7643)}{4.35pt}{4.62pt}{} & \AblScoreCI{0.7338}{(0.6806--0.7871)}{4.35pt}{4.62pt}{} & \AblScoreCI{0.7496}{(0.6958--0.7985)}{4.35pt}{4.62pt}{} & \AblScoreCI{0.7643}{(0.7148--0.8137)}{4.35pt}{4.62pt}{} & \AblScoreCI{0.7795}{(0.7262--0.8289)}{4.35pt}{4.62pt}{} \\
\cline{2-9}
\AblSpan{\makecell[c]{\textbf{Grounded visual}\\[0.05ex]\textbf{question answering}}}{2.30cm}{0pt} & \AblSpan{\makecell[c]{DeepTumorVQA}}{2.65cm}{0pt} & \AblMetric{\makecell[c]{\textbf{Accu.}}} & \AblScoreCI{0.4553}{(0.4417--0.4688)}{4.35pt}{4.62pt}{} & \AblScoreCI{0.4949}{(0.4811--0.5091)}{4.35pt}{4.62pt}{} & \AblScoreCI{0.5278}{(0.5151--0.5414)}{4.35pt}{4.62pt}{} & \AblScoreCI{0.5549}{(0.5422--0.5694)}{4.35pt}{4.62pt}{} & \AblScoreCI{0.5781}{(0.5647--0.5921)}{4.35pt}{4.62pt}{} & \AblScoreCI{0.5977}{(0.5843--0.6112)}{4.35pt}{4.62pt}{} \\
\cline{2-9}
 & \multicolumn{2}{>{\columncolor{leftblue}\centering\arraybackslash}m{\dimexpr2.65cm+1.55cm+2\tabcolsep+\arrayrulewidth\relax}|}{\AblOverall{Overall}} & \AblScoreSingle{0.5756}{} & \AblScoreSingle{0.6034}{} & \AblScoreSingle{0.6308}{} & \AblScoreSingle{0.6523}{} & \AblScoreSingle{0.6712}{} & \AblScoreSingle{0.6886}{} \\
\hline
 &  & \AblMetric{\makecell[c]{\textbf{BLEU-4}}} & \AblScoreCI{0.4784}{(0.4519--0.4907)}{4.35pt}{4.62pt}{} & \AblScoreCI{0.4482}{(0.4207--0.4650)}{4.35pt}{4.62pt}{} & \AblScoreCI{0.4908}{(0.4702--0.5045)}{4.35pt}{4.62pt}{} & \AblScoreCI{0.5124}{(0.5043--0.5262)}{4.35pt}{4.62pt}{} & \AblScoreCI{0.5474}{(0.5389--0.5534)}{4.35pt}{4.62pt}{} & \AblScoreCI{0.5637}{(0.5534--0.5791)}{4.35pt}{4.62pt}{} \\*
\softcline{3-9}
 &  & \AblMetric{\makecell[c]{\textbf{ROUGE-L}}} & \AblScoreCI{0.3771}{(0.3661--0.3969)}{4.35pt}{4.62pt}{} & \AblScoreCI{0.3562}{(0.3373--0.3715)}{4.35pt}{4.62pt}{} & \AblScoreCI{0.4119}{(0.4015--0.4234)}{4.35pt}{4.62pt}{} & \AblScoreCI{0.4012}{(0.3940--0.4180)}{4.35pt}{4.62pt}{} & \AblScoreCI{0.4269}{(0.4138--0.4341)}{4.35pt}{4.62pt}{} & \AblScoreCI{0.4303}{(0.4244--0.4417)}{4.35pt}{4.62pt}{} \\*
\softcline{3-9}
 &  & \AblMetric{\makecell[c]{\textbf{METEOR}}} & \AblScoreCI{0.4253}{(0.4177--0.4397)}{4.35pt}{4.62pt}{} & \AblScoreCI{0.4084}{(0.3884--0.4208)}{4.35pt}{4.62pt}{} & \AblScoreCI{0.4439}{(0.4332--0.4528)}{4.35pt}{4.62pt}{} & \AblScoreCI{0.4820}{(0.4738--0.4990)}{4.35pt}{4.62pt}{} & \AblScoreCI{0.4732}{(0.4677--0.4813)}{4.35pt}{4.62pt}{} & \AblScoreCI{0.4800}{(0.4792--0.4969)}{4.35pt}{4.62pt}{} \\*
\softcline{3-9}
 & \AblSpan{\makecell[c]{RadGenome}}{2.65cm}{0.32cm} & \AblMetric{\makecell[c]{\textbf{RaTEScore}}} & \AblScoreCI{0.5942}{(0.5867--0.6170)}{4.35pt}{4.62pt}{} & \AblScoreCI{0.5636}{(0.5404--0.5804)}{4.35pt}{4.62pt}{} & \AblScoreCI{0.6119}{(0.6026--0.6279)}{4.35pt}{4.62pt}{} & \AblScoreCI{0.6373}{(0.6242--0.6425)}{4.35pt}{4.62pt}{} & \AblScoreCI{0.6584}{(0.6489--0.6617)}{4.35pt}{4.62pt}{} & \AblScoreCI{0.6737}{(0.6656--0.6882)}{4.35pt}{4.62pt}{} \\*
\softcline{3-9}
 &  & \AblMetric{\textbf{LlamaScore}} & \AblScoreCI{5.886}{(5.763--6.002)}{4.35pt}{4.62pt}{} & \AblScoreCI{5.649}{(5.511--5.776)}{4.35pt}{4.62pt}{} & \AblScoreCI{6.104}{(5.999--6.217)}{4.35pt}{4.62pt}{} & \AblScoreCI{6.253}{(6.159--6.368)}{4.35pt}{4.62pt}{} & \AblScoreCI{6.426}{(6.326--6.511)}{4.35pt}{4.62pt}{} & \AblScoreCI{6.553}{(6.467--6.644)}{4.35pt}{4.62pt}{} \\*
\softcline{3-9}
 &  & \AblMetric{\makecell[c]{\textbf{GREEN}}} & \AblScoreCI{0.3456}{(0.3226--0.3646)}{4.35pt}{4.62pt}{} & \AblScoreCI{0.3267}{(0.3021--0.3458)}{4.35pt}{4.62pt}{} & \AblScoreCI{0.3622}{(0.3524--0.3821)}{4.35pt}{4.62pt}{} & \AblScoreCI{0.3748}{(0.3632--0.3895)}{4.35pt}{4.62pt}{} & \AblScoreCI{0.3930}{(0.3895--0.4027)}{4.35pt}{4.62pt}{} & \AblScoreCI{0.4009}{(0.3910--0.4149)}{4.35pt}{4.62pt}{} \\
\cline{2-9}
\AblSpan{\makecell[c]{\textbf{Grounded report}\\[0.05ex]\textbf{generation}}}{2.30cm}{0pt} &  & \AblMetric{\makecell[c]{\textbf{BLEU-4}}} & \AblScoreCI{0.2422}{(0.2058--0.2823)}{4.35pt}{4.62pt}{} & \AblScoreCI{0.2338}{(0.1952--0.2763)}{4.35pt}{4.62pt}{} & \AblScoreCI{0.2658}{(0.2365--0.3002)}{4.35pt}{4.62pt}{} & \AblScoreCI{0.2706}{(0.2441--0.3005)}{4.35pt}{4.62pt}{} & \AblScoreCI{0.2948}{(0.2606--0.3244)}{4.35pt}{4.62pt}{} & \AblScoreCI{0.3082}{(0.2732--0.3329)}{4.35pt}{4.62pt}{} \\*
\softcline{3-9}
 &  & \AblMetric{\makecell[c]{\textbf{ROUGE-L}}} & \AblScoreCI{0.2743}{(0.2470--0.3089)}{4.35pt}{4.62pt}{} & \AblScoreCI{0.2690}{(0.2205--0.3032)}{4.35pt}{4.62pt}{} & \AblScoreCI{0.2960}{(0.2612--0.3281)}{4.35pt}{4.62pt}{} & \AblScoreCI{0.3071}{(0.2780--0.3340)}{4.35pt}{4.62pt}{} & \AblScoreCI{0.3239}{(0.2975--0.3531)}{4.35pt}{4.62pt}{} & \AblScoreCI{0.3357}{(0.3010--0.3523)}{4.35pt}{4.62pt}{} \\*
\softcline{3-9}
 &  & \AblMetric{\makecell[c]{\textbf{METEOR}}} & \AblScoreCI{0.2473}{(0.2144--0.2776)}{4.35pt}{4.62pt}{} & \AblScoreCI{0.2284}{(0.1954--0.2577)}{4.35pt}{4.62pt}{} & \AblScoreCI{0.2522}{(0.2278--0.2882)}{4.35pt}{4.62pt}{} & \AblScoreCI{0.2771}{(0.2489--0.3057)}{4.35pt}{4.62pt}{} & \AblScoreCI{0.2905}{(0.2775--0.3198)}{4.35pt}{4.62pt}{} & \AblScoreCI{0.2851}{(0.2643--0.3002)}{4.35pt}{4.62pt}{} \\*
\softcline{3-9}
 & \AblSpan{\makecell[c]{ReXGroundingCT}}{2.65cm}{0.32cm} & \AblMetric{\makecell[c]{\textbf{RaTEScore}}} & \AblScoreCI{0.4381}{(0.4012--0.4613)}{4.35pt}{4.62pt}{} & \AblScoreCI{0.4188}{(0.3726--0.4439)}{4.35pt}{4.62pt}{} & \AblScoreCI{0.4546}{(0.4236--0.4896)}{4.35pt}{4.62pt}{} & \AblScoreCI{0.4719}{(0.4490--0.5093)}{4.35pt}{4.62pt}{} & \AblScoreCI{0.4891}{(0.4630--0.5049)}{4.35pt}{4.62pt}{} & \AblScoreCI{0.5070}{(0.4885--0.5242)}{4.35pt}{4.62pt}{} \\*
\softcline{3-9}
 &  & \AblMetric{\textbf{LlamaScore}} & \AblScoreCI{5.312}{(5.010--5.598)}{4.35pt}{4.62pt}{} & \AblScoreCI{5.128}{(4.809--5.438)}{4.35pt}{4.62pt}{} & \AblScoreCI{5.471}{(5.190--5.754)}{4.35pt}{4.62pt}{} & \AblScoreCI{5.657}{(5.381--5.925)}{4.35pt}{4.62pt}{} & \AblScoreCI{5.799}{(5.539--6.043)}{4.35pt}{4.62pt}{} & \AblScoreCI{5.903}{(5.672--6.127)}{4.35pt}{4.62pt}{} \\*
\softcline{3-9}
 &  & \AblMetric{\makecell[c]{\textbf{GREEN}}} & \AblScoreCI{0.1667}{(0.1330--0.1925)}{4.35pt}{4.62pt}{} & \AblScoreCI{0.1538}{(0.1221--0.1834)}{4.35pt}{4.62pt}{} & \AblScoreCI{0.1909}{(0.1778--0.2215)}{4.35pt}{4.62pt}{} & \AblScoreCI{0.1863}{(0.1538--0.2158)}{4.35pt}{4.62pt}{} & \AblScoreCI{0.1913}{(0.1740--0.2202)}{4.35pt}{4.62pt}{} & \AblScoreCI{0.2012}{(0.1898--0.2247)}{4.35pt}{4.62pt}{} \\
\cline{2-9}
 & \multicolumn{2}{>{\columncolor{leftblue}\centering\arraybackslash}m{\dimexpr2.65cm+1.55cm+2\tabcolsep+\arrayrulewidth\relax}|}{\AblOverall{Overall}} & \AblScoreSingle{0.3924}{} & \AblScoreSingle{0.3737}{} & \AblScoreSingle{0.4115}{} & \AblScoreSingle{0.4260}{} & \AblScoreSingle{0.4426}{} & \AblScoreSingle{0.4526}{} \\
\hline
\end{longtable}
\arrayrulecolor{black}
\endgroup
