# Supplementary material for: A 3D foundation model unifying CT interpretation and segmentation
Source: arXiv:2611.06471 source file (2026-11-04)
Supplement: Supplementary file 6 [file table16_mask_remove.tex]

\begingroup
\makeatletter
\@ifundefined{color@leftblue}{\definecolor{leftblue}{RGB}{232,242,248}}{}%
\@ifundefined{color@headerblue}{\definecolor{headerblue}{RGB}{218,233,242}}{}%
\makeatother
\setlength{\LTcapwidth}{18.60cm}
\setlength{\LTleft}{\fill}
\setlength{\LTright}{\fill}
\setlength{\LTpre}{0pt}
\setlength{\LTpost}{0pt}
\setlength{\tabcolsep}{0.45pt}
\renewcommand{\arraystretch}{1.00}
\setlength{\extrarowheight}{0pt}
\setlength{\arrayrulewidth}{0.48pt}
\arrayrulecolor{black}
\providecommand{\softcline}[1]{}%
\renewcommand{\softcline}[1]{\arrayrulecolor{black!35}\cline{#1}\arrayrulecolor{black}}
\sloppy
\emergencystretch=2em
\fontsize{5.20pt}{5.80pt}\selectfont
\newcommand{\AblScoreCI}[5]{%
  \parbox[c][0.64cm][c]{2.62cm}{%
    \centering
    {\fontsize{5.20pt}{5.48pt}\selectfont\strut\mbox{#1#5}}\\[-0.38ex]%
    {\fontsize{#3}{#4}\selectfont\strut\mbox{#2}}%
  }%
}%
\newcommand{\AblScoreSingle}[2]{%
  \parbox[c][0.64cm][c]{2.62cm}{%
    \centering
    {\fontsize{5.20pt}{5.48pt}\selectfont\strut\mbox{#1#2}}%
  }%
}%
\newcommand{\AblMetric}[1]{%
  \parbox[c][0.64cm][c]{1.55cm}{%
    \centering\fontsize{5.05pt}{5.32pt}\selectfont #1%
  }%
}%
\newcommand{\AblOverall}[1]{%
  \parbox[c][0.64cm][c]{\dimexpr2.65cm+1.55cm+2\tabcolsep+\arrayrulewidth\relax}{%
    \centering\fontsize{5.20pt}{5.48pt}\selectfont\textbf{#1}%
  }%
}%
\newcommand{\AblSpan}[3]{%
  \raisebox{\dimexpr#3-0.11cm\relax}[0pt][0pt]{%
    \parbox[c][0.64cm][c]{#2}{%
      \centering\arraybackslash #1%
    }%
  }%
}%
\newcommand{\AblHead}[2]{%
  \parbox[c][0.92cm][c]{#2}{%
    \centering\fontsize{5.55pt}{5.80pt}\selectfont\textbf{#1}%
  }%
}%
\begin{longtable}{|>{\columncolor{leftblue}\centering\arraybackslash}m{2.30cm}|>{\columncolor{leftblue}\centering\arraybackslash}m{2.65cm}|>{\columncolor{leftblue}\centering\arraybackslash}m{1.55cm}|>{\centering\arraybackslash}m{2.65cm}|>{\centering\arraybackslash}m{2.65cm}|>{\centering\arraybackslash}m{2.65cm}|>{\centering\arraybackslash}m{2.65cm}|}
\caption[Masking and grounding-request ablations across tasks]{\textbf{Masking and grounding-request ablations across segmentation, grounded lesion screening, grounded visual question answering, and grounded report generation.}\newline For segmentation, Macro Dice denotes the dataset-level macro Dice. For grounded lesion screening, Macro F1 is calculated as the arithmetic mean of label-wise F1 scores within each dataset. For grounded visual question answering, Accu. denotes accuracy. For grounded report generation, BLEU-4, ROUGE-L, METEOR, RaTEScore, LlamaScore, and GREEN are reported. Overall scores retain the supplied task-level summaries and are shown without confidence intervals; the report-generation Overall score is LCS. Dataset scores are reported as mean with 95\% confidence interval when available.}%
\label{tab:ablation_study_detailed_scores}\\[-0.15ex]
\hline
\rowcolor{headerblue}
\AblHead{Task}{2.30cm} & \AblHead{Dataset Name}{2.65cm} & \AblHead{Metric}{1.55cm} & \AblHead{\makecell[c]{HoloCT-8B\\[-0.16ex]Intact\\[-0.16ex]w/ grounding}}{2.65cm} & \AblHead{\makecell[c]{HoloCT-8B\\[-0.16ex]Intact\\[-0.16ex]w/o grounding}}{2.65cm} & \AblHead{\makecell[c]{HoloCT-8B\\[-0.16ex]Masked\\[-0.16ex]w/ grounding}}{2.65cm} & \AblHead{\makecell[c]{HoloCT-8B\\[-0.16ex]Masked\\[-0.16ex]w/o grounding}}{2.65cm} \\
\hline
\endfirsthead
\caption*{\textbf{Supplementary Table~\ref{tab:ablation_study_detailed_scores} (continued)\enspace|\enspace Masking and grounding-request ablations across segmentation, grounded lesion screening, grounded visual question answering, and grounded report generation.}\newline For segmentation, Macro Dice denotes the dataset-level macro Dice. For grounded lesion screening, Macro F1 is calculated as the arithmetic mean of label-wise F1 scores within each dataset. For grounded visual question answering, Accu. denotes accuracy. For grounded report generation, BLEU-4, ROUGE-L, METEOR, RaTEScore, LlamaScore, and GREEN are reported. Overall scores retain the supplied task-level summaries and are shown without confidence intervals; the report-generation Overall score is LCS. Dataset scores are reported as mean with 95\% confidence interval when available.}\\[-0.15ex]
\hline
\rowcolor{headerblue}
\AblHead{Task}{2.30cm} & \AblHead{Dataset Name}{2.65cm} & \AblHead{Metric}{1.55cm} & \AblHead{\makecell[c]{HoloCT-8B\\[-0.16ex]Intact\\[-0.16ex]w/ grounding}}{2.65cm} & \AblHead{\makecell[c]{HoloCT-8B\\[-0.16ex]Intact\\[-0.16ex]w/o grounding}}{2.65cm} & \AblHead{\makecell[c]{HoloCT-8B\\[-0.16ex]Masked\\[-0.16ex]w/ grounding}}{2.65cm} & \AblHead{\makecell[c]{HoloCT-8B\\[-0.16ex]Masked\\[-0.16ex]w/o grounding}}{2.65cm} \\
\hline
\endhead
\endfoot
\endlastfoot
 & \AblSpan{\makecell[c]{Total-\\[0.05ex]SegmentatorV2}}{2.65cm}{0pt} & \AblMetric{\makecell[c]{\textbf{Macro Dice}}} & \AblScoreCI{0.8776}{(0.8741--0.8806)}{4.35pt}{4.62pt}{} &  & \AblScoreCI{0.8300}{(0.8265--0.8332)}{4.35pt}{4.62pt}{} &  \\*
\cline{2-4}\cline{6-6}
\AblSpan{\makecell[c]{\textbf{Segmentation}}}{2.30cm}{0pt} & \AblSpan{\makecell[c]{AbdomenAtlas3.0}}{2.65cm}{0pt} & \AblMetric{\makecell[c]{\textbf{Macro Dice}}} & \AblScoreCI{0.8018}{(0.7987--0.8046)}{4.35pt}{4.62pt}{} & \AblScoreSingle{\fontsize{4.30pt}{4.55pt}\selectfont Not supported}{} & \AblScoreCI{0.7912}{(0.7880--0.7943)}{4.35pt}{4.62pt}{} & \AblScoreSingle{\fontsize{4.30pt}{4.55pt}\selectfont Not supported}{} \\*
\cline{2-4}\cline{6-6}
 & \multicolumn{2}{>{\columncolor{leftblue}\centering\arraybackslash}m{\dimexpr2.65cm+1.55cm+2\tabcolsep+\arrayrulewidth\relax}|}{\AblOverall{Overall}} & \AblScoreSingle{0.8397}{} &  & \AblScoreSingle{0.8106}{} &  \\
\hline
 & \AblSpan{\makecell[c]{AbdomenAtlas3.0}}{2.65cm}{0pt} & \AblMetric{\makecell[c]{\textbf{Macro F1}}} & \AblScoreSingle{0.6383}{} & \AblScoreSingle{0.6088}{} & \AblScoreCI{0.05895}{(0.03136--0.09357)}{4.02pt}{4.28pt}{} & \AblScoreCI{0.05536}{(0.02878--0.08935)}{4.02pt}{4.28pt}{} \\
\cline{2-7}
\AblSpan{\makecell[c]{\textbf{Grounded lesion}\\[0.05ex]\textbf{screening}}}{2.30cm}{0pt} & \AblSpan{\makecell[c]{LiMT}}{2.65cm}{0pt} & \AblMetric{\makecell[c]{\textbf{Macro F1}}} & \AblScoreCI{0.7175}{(0.4861--0.9308)}{4.35pt}{4.62pt}{} & \AblScoreSingle{0.7175}{} & \AblScoreCI{0.06250}{(0.0000--0.1667)}{4.35pt}{4.62pt}{} & \AblScoreCI{0.05556}{(0.0000--0.1430)}{4.35pt}{4.62pt}{} \\
\cline{2-7}
 & \multicolumn{2}{>{\columncolor{leftblue}\centering\arraybackslash}m{\dimexpr2.65cm+1.55cm+2\tabcolsep+\arrayrulewidth\relax}|}{\AblOverall{Overall}} & \AblScoreSingle{0.6779}{} & \AblScoreSingle{0.6632}{} & \AblScoreSingle{0.06072}{} & \AblScoreSingle{0.05546}{} \\
\hline
 & \AblSpan{\makecell[c]{AMOS-MM-VQA}}{2.65cm}{0pt} & \AblMetric{\makecell[c]{\textbf{Accu.}}} & \AblScoreCI{0.8897}{(0.8479--0.9278)}{4.35pt}{4.62pt}{} & \AblScoreCI{0.8707}{(0.8289--0.9087)}{4.35pt}{4.62pt}{} & \AblScoreCI{0.8707}{(0.8289--0.9087)}{4.35pt}{4.62pt}{} & \AblScoreCI{0.8669}{(0.8251--0.9050)}{4.35pt}{4.62pt}{} \\
\cline{2-7}
\AblSpan{\makecell[c]{\textbf{Grounded visual}\\[0.05ex]\textbf{question answering}}}{2.30cm}{0pt} & \AblSpan{\makecell[c]{DeepTumorVQA}}{2.65cm}{0pt} & \AblMetric{\makecell[c]{\textbf{Accu.}}} & \AblScoreCI{0.6525}{(0.6405--0.6657)}{4.35pt}{4.62pt}{} & \AblScoreCI{0.6467}{(0.6340--0.6593)}{4.35pt}{4.62pt}{} & \AblScoreCI{0.5475}{(0.5344--0.5596)}{4.35pt}{4.62pt}{} & \AblScoreCI{0.5301}{(0.5170--0.5422)}{4.35pt}{4.62pt}{} \\
\cline{2-7}
 & \multicolumn{2}{>{\columncolor{leftblue}\centering\arraybackslash}m{\dimexpr2.65cm+1.55cm+2\tabcolsep+\arrayrulewidth\relax}|}{\AblOverall{Overall}} & \AblScoreSingle{0.7711}{} & \AblScoreSingle{0.7587}{} & \AblScoreSingle{0.7091}{} & \AblScoreSingle{0.6985}{} \\
\hline
 &  & \AblMetric{\makecell[c]{\textbf{BLEU-4}}} & \AblScoreCI{0.6253}{(0.6178--0.6335)}{4.35pt}{4.62pt}{} & \AblScoreCI{0.6261}{(0.6184--0.6340)}{4.35pt}{4.62pt}{} & \AblScoreCI{0.5969}{(0.5888--0.6056)}{4.35pt}{4.62pt}{} & \AblScoreCI{0.5966}{(0.5885--0.6053)}{4.35pt}{4.62pt}{} \\*
\softcline{3-7}
 &  & \AblMetric{\makecell[c]{\textbf{ROUGE-L}}} & \AblScoreCI{0.4859}{(0.4763--0.4945)}{4.35pt}{4.62pt}{} & \AblScoreCI{0.4830}{(0.4732--0.4918)}{4.35pt}{4.62pt}{} & \AblScoreCI{0.4890}{(0.4787--0.4982)}{4.35pt}{4.62pt}{} & \AblScoreCI{0.4887}{(0.4784--0.4979)}{4.35pt}{4.62pt}{} \\*
\softcline{3-7}
 &  & \AblMetric{\makecell[c]{\textbf{METEOR}}} & \AblScoreCI{0.5460}{(0.5368--0.5552)}{4.35pt}{4.62pt}{} & \AblScoreCI{0.5440}{(0.5349--0.5534)}{4.35pt}{4.62pt}{} & \AblScoreCI{0.5215}{(0.5120--0.5315)}{4.35pt}{4.62pt}{} & \AblScoreCI{0.5212}{(0.5117--0.5312)}{4.35pt}{4.62pt}{} \\*
\softcline{3-7}
 & \AblSpan{\makecell[c]{RadGenome}}{2.65cm}{0.32cm} & \AblMetric{\makecell[c]{\textbf{RaTEScore}}} & \AblScoreCI{0.7482}{(0.7434--0.7533)}{4.35pt}{4.62pt}{} & \AblScoreCI{0.7419}{(0.7370--0.7470)}{4.35pt}{4.62pt}{} & \AblScoreCI{0.7510}{(0.7461--0.7560)}{4.35pt}{4.62pt}{} & \AblScoreCI{0.7507}{(0.7458--0.7557)}{4.35pt}{4.62pt}{} \\*
\softcline{3-7}
 &  & \AblMetric{\textbf{LlamaScore}} & \AblScoreCI{7.181}{(7.093--7.271)}{4.35pt}{4.62pt}{} & \AblScoreCI{7.154}{(7.063--7.240)}{4.35pt}{4.62pt}{} & \AblScoreCI{6.583}{(6.484--6.688)}{4.35pt}{4.62pt}{} & \AblScoreCI{6.580}{(6.481--6.685)}{4.35pt}{4.62pt}{} \\*
\softcline{3-7}
 &  & \AblMetric{\makecell[c]{\textbf{GREEN}}} & \AblScoreCI{0.4740}{(0.4606--0.4868)}{4.35pt}{4.62pt}{} & \AblScoreCI{0.4624}{(0.4499--0.4772)}{4.35pt}{4.62pt}{} & \AblScoreCI{0.4746}{(0.4618--0.4880)}{4.35pt}{4.62pt}{} & \AblScoreCI{0.4743}{(0.4615--0.4877)}{4.35pt}{4.62pt}{} \\
\cline{2-7}
\AblSpan{\makecell[c]{\textbf{Grounded report}\\[0.05ex]\textbf{generation}}}{2.30cm}{0pt} &  & \AblMetric{\makecell[c]{\textbf{BLEU-4}}} & \AblScoreCI{0.3517}{(0.3257--0.3803)}{4.35pt}{4.62pt}{} & \AblScoreCI{0.3278}{(0.3027--0.3508)}{4.35pt}{4.62pt}{} & \AblScoreCI{0.2157}{(0.1997--0.2315)}{4.35pt}{4.62pt}{} & \AblScoreCI{0.1943}{(0.1777--0.2119)}{4.35pt}{4.62pt}{} \\*
\softcline{3-7}
 &  & \AblMetric{\makecell[c]{\textbf{ROUGE-L}}} & \AblScoreCI{0.3742}{(0.3481--0.4012)}{4.35pt}{4.62pt}{} & \AblScoreCI{0.3572}{(0.3350--0.3808)}{4.35pt}{4.62pt}{} & \AblScoreCI{0.2413}{(0.2276--0.2555)}{4.35pt}{4.62pt}{} & \AblScoreCI{0.2418}{(0.2280--0.2574)}{4.35pt}{4.62pt}{} \\*
\softcline{3-7}
 &  & \AblMetric{\makecell[c]{\textbf{METEOR}}} & \AblScoreCI{0.3217}{(0.2954--0.3505)}{4.35pt}{4.62pt}{} & \AblScoreCI{0.2975}{(0.2719--0.3209)}{4.35pt}{4.62pt}{} & \AblScoreCI{0.1889}{(0.1737--0.2043)}{4.35pt}{4.62pt}{} & \AblScoreCI{0.1845}{(0.1692--0.1994)}{4.35pt}{4.62pt}{} \\*
\softcline{3-7}
 & \AblSpan{\makecell[c]{ReXGroundingCT}}{2.65cm}{0.32cm} & \AblMetric{\makecell[c]{\textbf{RaTEScore}}} & \AblScoreCI{0.5616}{(0.5444--0.5789)}{4.35pt}{4.62pt}{} & \AblScoreCI{0.5509}{(0.5345--0.5677)}{4.35pt}{4.62pt}{} & \AblScoreCI{0.4530}{(0.4413--0.4659)}{4.35pt}{4.62pt}{} & \AblScoreCI{0.4627}{(0.4503--0.4748)}{4.35pt}{4.62pt}{} \\*
\softcline{3-7}
 &  & \AblMetric{\textbf{LlamaScore}} & \AblScoreCI{6.343}{(6.140--6.539)}{4.35pt}{4.62pt}{} & \AblScoreCI{6.179}{(6.007--6.362)}{4.35pt}{4.62pt}{} & \AblScoreCI{4.853}{(4.703--5.007)}{4.35pt}{4.62pt}{} & \AblScoreCI{4.650}{(4.490--4.812)}{4.35pt}{4.62pt}{} \\*
\softcline{3-7}
 &  & \AblMetric{\makecell[c]{\textbf{GREEN}}} & \AblScoreCI{0.2424}{(0.2128--0.2771)}{4.35pt}{4.62pt}{} & \AblScoreCI{0.2173}{(0.1890--0.2465)}{4.35pt}{4.62pt}{} & \AblScoreCI{0.07198}{(0.05739--0.08845)}{4.02pt}{4.28pt}{} & \AblScoreCI{0.08181}{(0.06572--0.09858)}{4.02pt}{4.28pt}{} \\
\cline{2-7}
 & \multicolumn{2}{>{\columncolor{leftblue}\centering\arraybackslash}m{\dimexpr2.65cm+1.55cm+2\tabcolsep+\arrayrulewidth\relax}|}{\AblOverall{Overall}} & \AblScoreSingle{0.5070}{} & \AblScoreSingle{0.4951}{} & \AblScoreSingle{0.4290}{} & \AblScoreSingle{0.4266}{} \\
\hline
\end{longtable}
\arrayrulecolor{black}
\endgroup
