# Supplementary material for: A 3D foundation model unifying CT interpretation and segmentation
Source: arXiv:2611.06471 source file (2026-11-04)
Supplement: Supplementary file 7 [file table17_subtask2_seg.tex]

\begingroup
\makeatletter
\@ifundefined{color@leftblue}{\definecolor{leftblue}{RGB}{232,242,248}}{}%
\@ifundefined{color@headerblue}{\definecolor{headerblue}{RGB}{218,233,242}}{}%
\makeatother
\setlength{\LTcapwidth}{18.60cm}
\setlength{\LTleft}{\fill}
\setlength{\LTright}{\fill}
\setlength{\LTpre}{0pt}
\setlength{\LTpost}{0pt}
\setlength{\tabcolsep}{0.45pt}
\renewcommand{\arraystretch}{1.00}
\setlength{\extrarowheight}{0pt}
\setlength{\arrayrulewidth}{0.48pt}
\arrayrulecolor{black}
\providecommand{\softcline}[1]{}%
\renewcommand{\softcline}[1]{\arrayrulecolor{black!35}\cline{#1}\arrayrulecolor{black}}
\sloppy
\emergencystretch=2em
\fontsize{5.30pt}{5.90pt}\selectfont
\newcommand{\HoloSegScore}[5]{%
  \parbox[c][0.80cm][c]{2.52cm}{%
    \centering
    {\fontsize{5.30pt}{5.58pt}\selectfont\strut\mbox{#1#5}}\\[-0.38ex]%
    {\fontsize{#3}{#4}\selectfont\strut\mbox{#2}}%
  }%
}%
\newcommand{\HoloSegUnsupported}{%
  \parbox[c][0.80cm][c]{2.52cm}{%
    \centering\fontsize{4.30pt}{4.55pt}\selectfont Not supported%
  }%
}%
\newcommand{\HoloSegSpan}[3]{%
  \raisebox{#3}[0pt][0pt]{%
    \parbox[c][0.80cm][c]{#2}{%
      \centering #1\par%
    }%
  }%
}%
\newcommand{\HoloSegSplitHead}[3]{%
  \parbox[c][0.92cm][c]{#3}{%
    \centering\fontsize{6.10pt}{6.35pt}\selectfont\textbf{#1}\\[-0.52ex]%
    \rule{0pt}{0.58ex}\\[-0.52ex]\textbf{#2}%
  }%
}%
\newcommand{\HoloSegMidHead}[2]{%
  \parbox[c][0.92cm][c]{#2}{%
    \centering\fontsize{5.15pt}{5.45pt}\selectfont\textbf{#1}%
  }%
}%
\begin{longtable}{|>{\columncolor{leftblue}\centering\arraybackslash}m{1.45cm}|>{\columncolor{leftblue}\centering\arraybackslash}m{2.40cm}|>{\columncolor{leftblue}\centering\arraybackslash}m{3.20cm}|>{\centering\arraybackslash}m{2.55cm}|>{\centering\arraybackslash}m{2.55cm}|>{\centering\arraybackslash}m{2.55cm}|>{\centering\arraybackslash}m{2.55cm}|}
\caption[Zero-shot conditional Dice across classification targets]{\textbf{Zero-shot conditional segmentation performance of HoloCT segmentation and grounded variants across classification targets.}\newline Each score is reported as mean with 95\% confidence interval. Cond. Dice denotes conditional Dice. Internal, external-seen and external-unseen objects follow the zero-shot grouping used in the classification--segmentation evaluation.}%
\label{tab:conditional_dice_zeroshot_comparison}\\[-0.15ex]
\hline
\rowcolor{headerblue}
\HoloSegSplitHead{Dataset}{Type}{1.45cm} & \HoloSegSplitHead{Dataset}{Name}{2.40cm} & \HoloSegSplitHead{Label}{Name}{3.20cm} & \HoloSegMidHead{\makecell[c]{HoloCT-4B\\[-0.18ex]Segmentation-only}}{2.55cm} & \HoloSegMidHead{\makecell[c]{HoloCT-4B\\[-0.18ex]w/ grounding}}{2.55cm} & \HoloSegMidHead{\makecell[c]{HoloCT-8B\\[-0.18ex]Segmentation-only}}{2.55cm} & \HoloSegMidHead{\makecell[c]{HoloCT-8B\\[-0.18ex]w/ grounding}}{2.55cm} \\
\hline
\endfirsthead
\caption*{\textbf{Supplementary Table~\ref{tab:conditional_dice_zeroshot_comparison} (continued)\enspace|\enspace Zero-shot conditional segmentation performance of HoloCT segmentation and grounded variants across classification targets.}\newline Each score is reported as mean with 95\% confidence interval. Cond. Dice denotes conditional Dice. Internal, external-seen and external-unseen objects follow the zero-shot grouping used in the classification--segmentation evaluation.}\\[-0.15ex]
\hline
\rowcolor{headerblue}
\HoloSegSplitHead{Dataset}{Type}{1.45cm} & \HoloSegSplitHead{Dataset}{Name}{2.40cm} & \HoloSegSplitHead{Label}{Name}{3.20cm} & \HoloSegMidHead{\makecell[c]{HoloCT-4B\\[-0.18ex]Segmentation-only}}{2.55cm} & \HoloSegMidHead{\makecell[c]{HoloCT-4B\\[-0.18ex]w/ grounding}}{2.55cm} & \HoloSegMidHead{\makecell[c]{HoloCT-8B\\[-0.18ex]Segmentation-only}}{2.55cm} & \HoloSegMidHead{\makecell[c]{HoloCT-8B\\[-0.18ex]w/ grounding}}{2.55cm} \\
\hline
\endhead
\endfoot
\endlastfoot
 &  & \parbox[c][0.80cm][c]{3.20cm}{\centering \makecell[c]{left kidney cyst}\par} & \HoloSegScore{0.9025}{(0.8896--0.9195)}{4.55pt}{4.82pt}{} & \HoloSegScore{0.9016}{(0.8845--0.9240)}{4.55pt}{4.82pt}{} & \HoloSegScore{0.8882}{(0.8882--0.8882)}{4.55pt}{4.82pt}{} & \HoloSegScore{0.8872}{(0.8380--0.9342)}{4.55pt}{4.82pt}{} \\
\cline{3-7}
 & \HoloSegSpan{\makecell[c]{Total-\\[-0.22ex]SegmentatorV2}}{2.40cm}{0.40cm} & \parbox[c][0.80cm][c]{3.20cm}{\centering \makecell[c]{right kidney cyst}\par} & \HoloSegScore{0.8595}{(0.7952--0.9316)}{4.55pt}{4.82pt}{} & \HoloSegScore{0.8536}{(0.7821--0.9343)}{4.55pt}{4.82pt}{} & \HoloSegScore{0.8536}{(0.8536--0.8536)}{4.55pt}{4.82pt}{} & \HoloSegScore{0.8563}{(0.7787--0.9328)}{4.55pt}{4.82pt}{} \\
\cline{2-7}
 & \parbox[c][0.80cm][c]{2.40cm}{\centering \makecell[c]{KiTS23}\par} & \parbox[c][0.80cm][c]{3.20cm}{\centering \makecell[c]{kidney cyst}\par} & \HoloSegScore{0.5913}{(0.5081--0.6765)}{4.55pt}{4.82pt}{} & \HoloSegScore{0.5781}{(0.4930--0.6636)}{4.55pt}{4.82pt}{} & \HoloSegScore{0.7056}{(0.7056--0.7056)}{4.55pt}{4.82pt}{} & \HoloSegScore{0.7046}{(0.6268--0.7816)}{4.55pt}{4.82pt}{} \\
\cline{2-7}
 & \parbox[c][0.80cm][c]{2.40cm}{\centering \makecell[c]{CT-ICH}\par} & \parbox[c][0.80cm][c]{3.20cm}{\centering \makecell[c]{intracranial\\[-0.10ex]hemorrhage}\par} & \HoloSegScore{0.5524}{(0.5155--0.5965)}{4.55pt}{4.82pt}{} & \HoloSegScore{0.5557}{(0.5180--0.6021)}{4.55pt}{4.82pt}{} & \HoloSegScore{0.6682}{(0.4940--0.8423)}{4.55pt}{4.82pt}{} & \HoloSegScore{0.6853}{(0.5247--0.8460)}{4.55pt}{4.82pt}{} \\
\cline{2-7}
 & \parbox[c][0.80cm][c]{2.40cm}{\centering \makecell[c]{PanTS}\par} & \parbox[c][0.80cm][c]{3.20cm}{\centering \makecell[c]{pancreas lesion}\par} & \HoloSegScore{0.4899}{(0.4223--0.5576)}{4.55pt}{4.82pt}{} & \HoloSegScore{0.4920}{(0.4242--0.5574)}{4.55pt}{4.82pt}{} & \HoloSegScore{0.5425}{(0.5425--0.5425)}{4.55pt}{4.82pt}{} & \HoloSegScore{0.5412}{(0.4820--0.6016)}{4.55pt}{4.82pt}{} \\
\cline{2-7}
 &  & \parbox[c][0.80cm][c]{3.20cm}{\centering \makecell[c]{kidney lesion}\par} & \HoloSegScore{0.7349}{(0.6924--0.7738)}{4.55pt}{4.82pt}{} & \HoloSegScore{0.7344}{(0.6924--0.7729)}{4.55pt}{4.82pt}{} & \HoloSegScore{0.8222}{(0.8222--0.8222)}{4.55pt}{4.82pt}{} & \HoloSegScore{0.8221}{(0.7941--0.8475)}{4.55pt}{4.82pt}{} \\
\cline{3-7}
 &  & \parbox[c][0.80cm][c]{3.20cm}{\centering \makecell[c]{liver lesion}\par} & \HoloSegScore{0.7240}{(0.6950--0.7503)}{4.55pt}{4.82pt}{} & \HoloSegScore{0.7248}{(0.6988--0.7506)}{4.55pt}{4.82pt}{} & \HoloSegScore{0.7103}{(0.7103--0.7103)}{4.55pt}{4.82pt}{} & \HoloSegScore{0.7102}{(0.6796--0.7402)}{4.55pt}{4.82pt}{} \\
\cline{3-7}
\HoloSegSpan{\makecell[c]{\textbf{Internal}}}{1.45cm}{0.40cm} & \HoloSegSpan{\makecell[c]{AbdomenAtlas\\[-0.22ex]3.0}}{2.40cm}{0.40cm} & \parbox[c][0.80cm][c]{3.20cm}{\centering \makecell[c]{pancreas lesion}\par} & \HoloSegScore{0.5465}{(0.4900--0.6032)}{4.55pt}{4.82pt}{} & \HoloSegScore{0.5480}{(0.4906--0.6055)}{4.55pt}{4.82pt}{} & \HoloSegScore{0.5722}{(0.5722--0.5722)}{4.55pt}{4.82pt}{} & \HoloSegScore{0.5712}{(0.5176--0.6266)}{4.55pt}{4.82pt}{} \\
\cline{3-7}
 &  & \parbox[c][0.80cm][c]{3.20cm}{\centering \makecell[c]{colon lesion}\par} & \HoloSegScore{0.6692}{(0.5656--0.7475)}{4.55pt}{4.82pt}{} & \HoloSegScore{0.6678}{(0.5685--0.7530)}{4.55pt}{4.82pt}{} & \HoloSegScore{0.7250}{(0.7250--0.7250)}{4.55pt}{4.82pt}{} & \HoloSegScore{0.7231}{(0.6598--0.7816)}{4.55pt}{4.82pt}{} \\
\cline{2-7}
 &  & \parbox[c][0.80cm][c]{3.20cm}{\centering \makecell[c]{liver cyst}\par} & \HoloSegScore{0.6034}{(0.4968--0.7306)}{4.55pt}{4.82pt}{} & \HoloSegScore{0.6003}{(0.4689--0.7237)}{4.55pt}{4.82pt}{} & \HoloSegScore{0.6400}{(0.5092--0.7521)}{4.55pt}{4.82pt}{} & \HoloSegScore{0.6448}{(0.5193--0.7476)}{4.55pt}{4.82pt}{} \\
\cline{3-7}
 &  & \parbox[c][0.80cm][c]{3.20cm}{\centering \makecell[c]{liver hemangioma}\par} & \HoloSegScore{0.8304}{(0.7592--0.8736)}{4.55pt}{4.82pt}{} & \HoloSegScore{0.8313}{(0.7636--0.8765)}{4.55pt}{4.82pt}{} & \HoloSegScore{0.7105}{(0.5285--0.8361)}{4.55pt}{4.82pt}{} & \HoloSegScore{0.7106}{(0.4914--0.8313)}{4.55pt}{4.82pt}{} \\
\cline{3-7}
 & \HoloSegSpan{\makecell[c]{LiMT}}{2.40cm}{0.40cm} & \parbox[c][0.80cm][c]{3.20cm}{\centering \makecell[c]{metastatic liver\\[-0.10ex]cancer}\par} & \HoloSegScore{0.6286}{(0.6286--0.6286)}{4.55pt}{4.82pt}{} & \HoloSegScore{0.6313}{(0.6313--0.6313)}{4.55pt}{4.82pt}{} & \HoloSegScore{0.6601}{(0.6601--0.6601)}{4.55pt}{4.82pt}{} & \HoloSegScore{0.6605}{(0.6605--0.6605)}{4.55pt}{4.82pt}{} \\
\cline{3-7}
 &  & \parbox[c][0.80cm][c]{3.20cm}{\centering \makecell[c]{primary liver\\[-0.10ex]cancer}\par} & \HoloSegScore{0.7394}{(0.6040--0.8634)}{4.55pt}{4.82pt}{} & \HoloSegScore{0.7407}{(0.5913--0.8614)}{4.55pt}{4.82pt}{} & \HoloSegScore{0.6927}{(0.4286--0.8604)}{4.55pt}{4.82pt}{} & \HoloSegScore{0.6904}{(0.4280--0.8608)}{4.55pt}{4.82pt}{} \\
\cline{2-7}
 & \parbox[c][0.80cm][c]{2.40cm}{\centering \makecell[c]{LiMT-oneclass}\par} & \parbox[c][0.80cm][c]{3.20cm}{\centering \makecell[c]{liver lesion}\par} & \HoloSegScore{0.4370}{(0.2359--0.6160)}{4.55pt}{4.82pt}{} & \HoloSegScore{0.6100}{(0.5105--0.7276)}{4.55pt}{4.82pt}{} & \HoloSegScore{0.4110}{(0.2368--0.5851)}{4.55pt}{4.82pt}{} & \HoloSegScore{0.5606}{(0.4261--0.6810)}{4.55pt}{4.82pt}{} \\
\hline
 & \parbox[c][0.80cm][c]{2.40cm}{\centering \makecell[c]{QUBIQ2021}\par} & \parbox[c][0.80cm][c]{3.20cm}{\centering \makecell[c]{pancreas lesion}\par} & \HoloSegScore{0.3470}{(0.3470--0.3470)}{4.55pt}{4.82pt}{} & \HoloSegScore{0.3361}{(0.3361--0.3361)}{4.55pt}{4.82pt}{} & \HoloSegScore{0.3855}{(0.3363--0.4347)}{4.55pt}{4.82pt}{} & \HoloSegScore{0.3867}{(0.3384--0.4350)}{4.55pt}{4.82pt}{} \\
\cline{2-7}
\HoloSegSpan{\makecell[c]{\textbf{External-}\\[-0.22ex]\textbf{seen}\\[-0.22ex]\textbf{(zero-shot)}}}{1.45cm}{0pt} & \parbox[c][0.80cm][c]{2.40cm}{\centering \makecell[c]{TotalSeg-\\[-0.22ex]subtask-\\[-0.22ex]liver-lesion}\par} & \parbox[c][0.80cm][c]{3.20cm}{\centering \makecell[c]{liver lesion}\par} & \HoloSegScore{0.7100}{(0.6807--0.7360)}{4.55pt}{4.82pt}{} & \HoloSegScore{0.7096}{(0.6827--0.7361)}{4.55pt}{4.82pt}{} & \HoloSegScore{0.7441}{(0.7163--0.7702)}{4.55pt}{4.82pt}{} & \HoloSegScore{0.7456}{(0.7185--0.7684)}{4.55pt}{4.82pt}{} \\
\cline{2-7}
 & \parbox[c][0.80cm][c]{2.40cm}{\centering \makecell[c]{MHB-SEG-\\[-0.22ex]oneclass}\par} & \parbox[c][0.80cm][c]{3.20cm}{\centering \makecell[c]{intracranial\\[-0.10ex]hemorrhage}\par} & \HoloSegScore{0.4010}{(0.2727--0.5286)}{4.55pt}{4.82pt}{} & \HoloSegScore{0.4056}{(0.2862--0.5260)}{4.55pt}{4.82pt}{} & \HoloSegScore{0.5052}{(0.5052--0.5052)}{4.55pt}{4.82pt}{} & \HoloSegScore{0.5143}{(0.3883--0.6315)}{4.55pt}{4.82pt}{} \\
\hline
 & \parbox[c][0.80cm][c]{2.40cm}{\centering \makecell[c]{PANORAMA}\par} & \parbox[c][0.80cm][c]{3.20cm}{\centering \makecell[c]{pancreatic ductal\\[-0.10ex]adenocarcinoma}\par} & \HoloSegScore{0.4135}{(0.3522--0.4806)}{4.55pt}{4.82pt}{} & \HoloSegScore{0.4112}{(0.3469--0.4737)}{4.55pt}{4.82pt}{} & \HoloSegScore{0.4515}{(0.3745--0.5222)}{4.55pt}{4.82pt}{} & \HoloSegScore{0.4468}{(0.3702--0.5143)}{4.55pt}{4.82pt}{} \\
\cline{2-7}
\HoloSegSpan{\makecell[c]{\textbf{External-}\\[-0.22ex]\textbf{unseen}\\[-0.22ex]\textbf{(zero-shot)}}}{1.45cm}{0pt} &  & \parbox[c][0.80cm][c]{3.20cm}{\centering \makecell[c]{subdural\\[-0.10ex]hemorrhage}\par} & \HoloSegScore{0.6663}{(0.4673--0.8423)}{4.55pt}{4.82pt}{} & \HoloSegScore{0.6676}{(0.4534--0.8512)}{4.55pt}{4.82pt}{} & \HoloSegScore{0.6755}{(0.6755--0.6755)}{4.55pt}{4.82pt}{} & \HoloSegScore{0.6724}{(0.4538--0.8441)}{4.55pt}{4.82pt}{} \\
\cline{3-7}
 & \HoloSegSpan{\makecell[c]{MHB-SEG-\\[-0.22ex]multiclass}}{2.40cm}{0.40cm} & \parbox[c][0.80cm][c]{3.20cm}{\centering \makecell[c]{subarachnoid\\[-0.10ex]hemorrhage}\par} & \HoloSegScore{0.1746}{(0.002516--0.4351)}{4.20pt}{4.48pt}{} & \HoloSegScore{0.1777}{(0.0000--0.5956)}{4.55pt}{4.82pt}{} & \HoloSegScore{0.4967}{(0.4967--0.4967)}{4.55pt}{4.82pt}{} & \HoloSegScore{0.5016}{(0.2761--0.7039)}{4.55pt}{4.82pt}{} \\
\hline
\end{longtable}
\arrayrulecolor{black}
\endgroup
