# Supplementary material for: A 3D foundation model unifying CT interpretation and segmentation
Source: arXiv:2611.06471 source file (2026-11-04)
Supplement: Supplementary file 8 [file table1_subtask1_part1.tex]

\begingroup
\makeatletter
\@ifundefined{color@leftblue}{\definecolor{leftblue}{RGB}{232,242,248}}{}%
\@ifundefined{color@headerblue}{\definecolor{headerblue}{RGB}{218,233,242}}{}%
\makeatother
\setlength{\LTcapwidth}{18.60cm}
\setlength{\LTleft}{\fill}
\setlength{\LTright}{\fill}
\setlength{\LTpre}{0pt}
\setlength{\LTpost}{0pt}
\setlength{\tabcolsep}{0.45pt}
\renewcommand{\arraystretch}{1.00}
\setlength{\extrarowheight}{0pt}
\setlength{\arrayrulewidth}{0.48pt}
\arrayrulecolor{black}
\providecommand{\softcline}[1]{}%
\renewcommand{\softcline}[1]{\arrayrulecolor{black!35}\cline{#1}\arrayrulecolor{black}}
\sloppy
\emergencystretch=2em
\fontsize{5.30pt}{5.90pt}\selectfont
\newcommand{\HoloSegScore}[5]{%
  \parbox[c][0.64cm][c]{1.68cm}{%
    \centering
    {\fontsize{5.30pt}{5.58pt}\selectfont\strut\adjustbox{max width=\linewidth}{#1#5}}\\[-0.38ex]%
    {\fontsize{#3}{#4}\selectfont\strut\adjustbox{max width=\linewidth}{#2}}%
  }%
}%
\newcommand{\HoloSegUnsupported}{%
  \parbox[c][0.64cm][c]{1.68cm}{%
    \centering\fontsize{4.45pt}{4.70pt}\selectfont Not supported%
  }%
}%
\newcommand{\HoloSegMetric}[1]{%
  \parbox[c][0.64cm][c]{0.84cm}{%
    \centering\fontsize{5.45pt}{5.70pt}\selectfont\adjustbox{max width=\linewidth}{\textbf{#1}}%
  }%
}%
\newcommand{\HoloSegSpan}[3]{%
  \raisebox{#3}[0pt][0pt]{%
    \parbox[c]{#2}{\centering\arraybackslash\adjustbox{max width=#2}{#1}}%
  }%
}%
\newcommand{\HoloSegSplitHead}[3]{%
  \parbox[c][0.92cm][c]{#3}{%
    \centering\fontsize{6.20pt}{6.45pt}\selectfont\textbf{#1}\\[-0.52ex]%
    \rule{0pt}{0.58ex}\\[-0.52ex]\textbf{#2}%
  }%
}%
\newcommand{\HoloSegMidHead}[2]{%
  \parbox[c][0.92cm][c]{#2}{%
    \centering\fontsize{6.20pt}{6.45pt}\selectfont\adjustbox{max width=\linewidth}{\textbf{#1}}%
  }%
}%
\begin{longtable}{|>{\columncolor{leftblue}\centering\arraybackslash}m{1.20cm}|>{\columncolor{leftblue}\centering\arraybackslash}m{1.86cm}|>{\columncolor{leftblue}\centering\arraybackslash}m{2.04cm}|>{\columncolor{leftblue}\centering\arraybackslash}m{0.88cm}|>{\centering\arraybackslash}m{1.70cm}|>{\centering\arraybackslash}m{1.70cm}|>{\centering\arraybackslash}m{1.70cm}|>{\centering\arraybackslash}m{1.70cm}|>{\centering\arraybackslash}m{1.70cm}|>{\centering\arraybackslash}m{1.70cm}|>{\centering\arraybackslash}m{1.70cm}|}
\caption[Detailed Dice and HD95 scores across segmentation benchmarks]{\textbf{Detailed Dice and HD95 scores of HoloCT and competing methods on internal, External-seen (zero-shot), External-unseen (zero-shot), and private zero-shot/fine-tuning segmentation benchmarks.}\newline Each score is reported as mean with 95\% confidence interval. $^{\blacktriangle}$ marks VoxTell results on PANORAMA; because PANORAMA was used to train VoxTell, these results do not constitute external validation for VoxTell. PASTA-Gen-30K-TotalSeg was not included in evaluation. Internal results cover 77 inventory subdatasets and 272 distinct targets.}%
\label{tab:id_ood_segmentation_scores}\\[-0.15ex]
\hline
\rowcolor{headerblue}
\HoloSegSplitHead{Dataset}{Type}{1.20cm} & \HoloSegSplitHead{Dataset}{Name}{1.86cm} & \HoloSegSplitHead{Label}{Name}{2.04cm} & \HoloSegMidHead{Metric}{0.88cm} & \HoloSegMidHead{VISTA3D}{1.70cm} & \HoloSegMidHead{M3D-Phi3-4B}{1.70cm} & \HoloSegMidHead{SAT-Pro}{1.70cm} & \HoloSegMidHead{VoxTell}{1.70cm} & \HoloSegMidHead{nnU-Net}{1.70cm} & \HoloSegMidHead{HoloCT-4B}{1.70cm} & \HoloSegMidHead{HoloCT-8B}{1.70cm} \\
\hline
\endfirsthead
\caption*{\textbf{Supplementary Table~\ref{tab:id_ood_segmentation_scores} (continued)\enspace|\enspace Detailed Dice and HD95 scores of HoloCT and competing methods on internal, External-seen (zero-shot), External-unseen (zero-shot), and private zero-shot/fine-tuning segmentation benchmarks.}\newline Each score is reported as mean with 95\% confidence interval. $^{\blacktriangle}$ marks VoxTell results on PANORAMA; because PANORAMA was used to train VoxTell, these results do not constitute external validation for VoxTell.}\\[-0.15ex]
\hline
\rowcolor{headerblue}
\HoloSegSplitHead{Dataset}{Type}{1.20cm} & \HoloSegSplitHead{Dataset}{Name}{1.86cm} & \HoloSegSplitHead{Label}{Name}{2.04cm} & \HoloSegMidHead{Metric}{0.88cm} & \HoloSegMidHead{VISTA3D}{1.70cm} & \HoloSegMidHead{M3D-Phi3-4B}{1.70cm} & \HoloSegMidHead{SAT-Pro}{1.70cm} & \HoloSegMidHead{VoxTell}{1.70cm} & \HoloSegMidHead{nnU-Net}{1.70cm} & \HoloSegMidHead{HoloCT-4B}{1.70cm} & \HoloSegMidHead{HoloCT-8B}{1.70cm} \\
\hline
\endhead
\endfoot
\endlastfoot
 &  &  & \HoloSegMetric{Dice} & \HoloSegScore{0.9618}{(0.9605--0.9629)}{4.55pt}{4.82pt}{} & \HoloSegScore{0.8959}{(0.8914--0.9002)}{4.55pt}{4.82pt}{} & \HoloSegScore{0.9722}{(0.9706--0.9735)}{4.55pt}{4.82pt}{} & \HoloSegScore{0.9755}{(0.9739--0.9771)}{4.55pt}{4.82pt}{} & \HoloSegScore{0.9684}{(0.9633--0.9752)}{4.55pt}{4.82pt}{} & \HoloSegScore{0.9879}{(0.9858--0.9898)}{4.55pt}{4.82pt}{} & \HoloSegScore{0.9750}{(0.9734--0.9764)}{4.55pt}{4.82pt}{} \\*
\softcline{4-11}
 &  & \HoloSegSpan{\makecell[c]{liver}}{2.04cm}{0.32cm} & \HoloSegMetric{HD95} & \HoloSegScore{5.026}{(4.052--6.588)}{4.55pt}{4.82pt}{} & \HoloSegScore{9.311}{(8.485--10.33)}{4.55pt}{4.82pt}{} & \HoloSegScore{3.224}{(2.941--3.589)}{4.55pt}{4.82pt}{} & \HoloSegScore{3.938}{(3.142--4.817)}{4.55pt}{4.82pt}{} & \HoloSegScore{4.261}{(3.221--4.743)}{4.55pt}{4.82pt}{} & \HoloSegScore{3.237}{(2.633--3.922)}{4.55pt}{4.82pt}{} & \HoloSegScore{3.438}{(2.922--4.085)}{4.55pt}{4.82pt}{} \\
\cline{3-11}
 &  &  & \HoloSegMetric{Dice} & \HoloSegScore{0.9123}{(0.9042--0.9194)}{4.55pt}{4.82pt}{} & \HoloSegScore{0.7248}{(0.6859--0.7648)}{4.55pt}{4.82pt}{} & \HoloSegScore{0.9554}{(0.9529--0.9577)}{4.55pt}{4.82pt}{} & \HoloSegScore{0.9624}{(0.9594--0.9649)}{4.55pt}{4.82pt}{} & \HoloSegScore{0.9419}{(0.9411--0.9504)}{4.55pt}{4.82pt}{} & \HoloSegScore{0.9617}{(0.9557--0.9667)}{4.55pt}{4.82pt}{} & \HoloSegScore{0.9532}{(0.9472--0.9577)}{4.55pt}{4.82pt}{} \\*
\softcline{4-11}
 &  & \HoloSegSpan{\makecell[c]{kidney}}{2.04cm}{0.32cm} & \HoloSegMetric{HD95} & \HoloSegScore{7.731}{(6.851--8.702)}{4.55pt}{4.82pt}{} & \HoloSegScore{9.910}{(8.828--11.08)}{4.55pt}{4.82pt}{} & \HoloSegScore{2.638}{(2.451--2.852)}{4.55pt}{4.82pt}{} & \HoloSegScore{4.799}{(3.227--6.799)}{4.55pt}{4.82pt}{} & \HoloSegScore{4.140}{(1.988--4.163)}{4.55pt}{4.82pt}{} & \HoloSegScore{4.694}{(3.493--6.348)}{4.55pt}{4.82pt}{} & \HoloSegScore{4.093}{(3.555--4.726)}{4.55pt}{4.82pt}{} \\
\cline{3-11}
 & \HoloSegSpan{\makecell[c]{AbdomenCT-\\[-0.10ex]1k}}{1.86cm}{0.32cm} &  & \HoloSegMetric{Dice} & \HoloSegScore{0.9530}{(0.9508--0.9551)}{4.55pt}{4.82pt}{} & \HoloSegScore{0.8423}{(0.8326--0.8521)}{4.55pt}{4.82pt}{} & \HoloSegScore{0.9656}{(0.9628--0.9679)}{4.55pt}{4.82pt}{} & \HoloSegScore{0.9739}{(0.9707--0.9764)}{4.55pt}{4.82pt}{} & \HoloSegScore{0.9420}{(0.9222--0.9443)}{4.55pt}{4.82pt}{} & \HoloSegScore{0.9866}{(0.9847--0.9883)}{4.55pt}{4.82pt}{} & \HoloSegScore{0.9752}{(0.9735--0.9769)}{4.55pt}{4.82pt}{} \\*
\softcline{4-11}
 &  & \HoloSegSpan{\makecell[c]{spleen}}{2.04cm}{0.32cm} & \HoloSegMetric{HD95} & \HoloSegScore{3.394}{(2.847--4.172)}{4.55pt}{4.82pt}{} & \HoloSegScore{7.503}{(6.953--8.156)}{4.55pt}{4.82pt}{} & \HoloSegScore{1.929}{(1.713--2.207)}{4.55pt}{4.82pt}{} & \HoloSegScore{2.158}{(1.496--2.990)}{4.55pt}{4.82pt}{} & \HoloSegScore{2.142}{(1.927--2.842)}{4.55pt}{4.82pt}{} & \HoloSegScore{0.8630}{(0.6660--1.178)}{4.55pt}{4.82pt}{} & \HoloSegScore{1.491}{(1.193--1.865)}{4.55pt}{4.82pt}{} \\
\cline{3-11}
 &  &  & \HoloSegMetric{Dice} & \HoloSegScore{0.8531}{(0.8459--0.8599)}{4.55pt}{4.82pt}{} & \HoloSegScore{0.5979}{(0.5820--0.6136)}{4.55pt}{4.82pt}{} & \HoloSegScore{0.8801}{(0.8741--0.8858)}{4.55pt}{4.82pt}{} & \HoloSegScore{0.8550}{(0.8465--0.8626)}{4.55pt}{4.82pt}{} & \HoloSegScore{0.8506}{(0.8439--0.8523)}{4.55pt}{4.82pt}{} & \HoloSegScore{0.8740}{(0.8647--0.8828)}{4.55pt}{4.82pt}{} & \HoloSegScore{0.8739}{(0.8665--0.8809)}{4.55pt}{4.82pt}{} \\*
\softcline{4-11}
 &  & \HoloSegSpan{\makecell[c]{pancreas}}{2.04cm}{0.32cm} & \HoloSegMetric{HD95} & \HoloSegScore{6.900}{(6.023--7.961)}{4.55pt}{4.82pt}{} & \HoloSegScore{14.99}{(13.36--16.82)}{4.55pt}{4.82pt}{} & \HoloSegScore{3.836}{(3.461--4.314)}{4.55pt}{4.82pt}{} & \HoloSegScore{6.722}{(5.822--7.778)}{4.55pt}{4.82pt}{} & \HoloSegScore{4.011}{(3.562--4.280)}{4.55pt}{4.82pt}{} & \HoloSegScore{4.859}{(4.194--5.717)}{4.55pt}{4.82pt}{} & \HoloSegScore{5.254}{(4.517--6.079)}{4.55pt}{4.82pt}{} \\
\cline{2-11}
 &  &  & \HoloSegMetric{Dice} & \HoloSegScore{0.9222}{(0.9072--0.9330)}{4.55pt}{4.82pt}{} & \HoloSegScore{0.7122}{(0.6707--0.7459)}{4.55pt}{4.82pt}{} & \HoloSegScore{0.9502}{(0.9444--0.9554)}{4.55pt}{4.82pt}{} & \HoloSegScore{0.9364}{(0.9227--0.9481)}{4.55pt}{4.82pt}{} & \HoloSegScore{0.9379}{(0.9189--0.9505)}{4.55pt}{4.82pt}{} & \HoloSegScore{0.9738}{(0.9694--0.9776)}{4.55pt}{4.82pt}{} & \HoloSegScore{0.9552}{(0.9503--0.9599)}{4.55pt}{4.82pt}{} \\*
\softcline{4-11}
 &  & \HoloSegSpan{\makecell[c]{spleen}}{2.04cm}{0.32cm} & \HoloSegMetric{HD95} & \HoloSegScore{7.332}{(4.318--11.60)}{4.55pt}{4.82pt}{} & \HoloSegScore{17.31}{(11.70--26.98)}{4.55pt}{4.82pt}{} & \HoloSegScore{2.788}{(2.120--3.600)}{4.55pt}{4.82pt}{} & \HoloSegScore{6.354}{(3.789--9.422)}{4.55pt}{4.82pt}{} & \HoloSegScore{3.920}{(3.532--5.522)}{4.55pt}{4.82pt}{} & \HoloSegScore{1.966}{(1.287--2.759)}{4.55pt}{4.82pt}{} & \HoloSegScore{2.686}{(2.100--3.345)}{4.55pt}{4.82pt}{} \\
\cline{3-11}
 &  &  & \HoloSegMetric{Dice} & \HoloSegScore{0.9315}{(0.9243--0.9373)}{4.55pt}{4.82pt}{} & \HoloSegScore{0.7018}{(0.6565--0.7413)}{4.55pt}{4.82pt}{} & \HoloSegScore{0.9513}{(0.9443--0.9570)}{4.55pt}{4.82pt}{} & \HoloSegScore{0.9477}{(0.9398--0.9544)}{4.55pt}{4.82pt}{} & \HoloSegScore{0.9448}{(0.9331--0.9538)}{4.55pt}{4.82pt}{} & \HoloSegScore{0.9646}{(0.9571--0.9704)}{4.55pt}{4.82pt}{} & \HoloSegScore{0.9503}{(0.9408--0.9576)}{4.55pt}{4.82pt}{} \\*
\softcline{4-11}
 &  & \HoloSegSpan{\makecell[c]{right kidney}}{2.04cm}{0.32cm} & \HoloSegMetric{HD95} & \HoloSegScore{4.480}{(3.783--5.261)}{4.55pt}{4.82pt}{} & \HoloSegScore{33.48}{(22.22--46.98)}{4.55pt}{4.82pt}{} & \HoloSegScore{2.092}{(1.760--2.489)}{4.55pt}{4.82pt}{} & \HoloSegScore{3.309}{(2.553--4.246)}{4.55pt}{4.82pt}{} & \HoloSegScore{2.684}{(1.978--3.406)}{4.55pt}{4.82pt}{} & \HoloSegScore{2.411}{(1.392--4.028)}{4.55pt}{4.82pt}{} & \HoloSegScore{2.848}{(1.933--4.127)}{4.55pt}{4.82pt}{} \\
\cline{3-11}
 &  &  & \HoloSegMetric{Dice} & \HoloSegScore{0.9183}{(0.8858--0.9378)}{4.55pt}{4.82pt}{} & \HoloSegScore{0.6538}{(0.6020--0.7016)}{4.55pt}{4.82pt}{} & \HoloSegScore{0.9509}{(0.9456--0.9555)}{4.55pt}{4.82pt}{} & \HoloSegScore{0.9461}{(0.9367--0.9545)}{4.55pt}{4.82pt}{} & \HoloSegScore{0.9459}{(0.9272--0.9521)}{4.55pt}{4.82pt}{} & \HoloSegScore{0.9668}{(0.9593--0.9727)}{4.55pt}{4.82pt}{} & \HoloSegScore{0.9491}{(0.9390--0.9570)}{4.55pt}{4.82pt}{} \\*
\softcline{4-11}
 &  & \HoloSegSpan{\makecell[c]{left kidney}}{2.04cm}{0.32cm} & \HoloSegMetric{HD95} & \HoloSegScore{4.827}{(3.448--7.265)}{4.55pt}{4.82pt}{} & \HoloSegScore{49.20}{(35.35--64.36)}{4.55pt}{4.82pt}{} & \HoloSegScore{2.157}{(1.807--2.626)}{4.55pt}{4.82pt}{} & \HoloSegScore{6.699}{(2.685--13.91)}{4.55pt}{4.82pt}{} & \HoloSegScore{4.305}{(3.451--6.695)}{4.55pt}{4.82pt}{} & \HoloSegScore{2.010}{(1.212--3.234)}{4.55pt}{4.82pt}{} & \HoloSegScore{2.502}{(1.753--3.619)}{4.55pt}{4.82pt}{} \\
\cline{3-11}
 &  &  & \HoloSegMetric{Dice} & \HoloSegScore{0.8275}{(0.7967--0.8560)}{4.55pt}{4.82pt}{} & \HoloSegScore{0.2908}{(0.2269--0.3523)}{4.55pt}{4.82pt}{} & \HoloSegScore{0.8700}{(0.8445--0.8903)}{4.55pt}{4.82pt}{} & \HoloSegScore{0.7982}{(0.7492--0.8408)}{4.55pt}{4.82pt}{} & \HoloSegScore{0.8366}{(0.8034--0.8546)}{4.55pt}{4.82pt}{} & \HoloSegScore{0.8668}{(0.8298--0.8975)}{4.55pt}{4.82pt}{} & \HoloSegScore{0.8783}{(0.8585--0.8972)}{4.55pt}{4.82pt}{} \\*
\softcline{4-11}
 &  & \HoloSegSpan{\makecell[c]{gallbladder}}{2.04cm}{0.32cm} & \HoloSegMetric{HD95} & \HoloSegScore{7.525}{(5.984--9.327)}{4.55pt}{4.82pt}{} & \HoloSegScore{35.56}{(22.63--51.06)}{4.55pt}{4.82pt}{} & \HoloSegScore{4.093}{(3.303--5.000)}{4.55pt}{4.82pt}{} & \HoloSegScore{9.833}{(6.999--13.03)}{4.55pt}{4.82pt}{} & \HoloSegScore{9.396}{(7.871--10.45)}{4.55pt}{4.82pt}{} & \HoloSegScore{6.728}{(4.611--9.292)}{4.55pt}{4.82pt}{} & \HoloSegScore{6.026}{(4.265--7.950)}{4.55pt}{4.82pt}{} \\
\cline{3-11}
 &  &  & \HoloSegMetric{Dice} & \HoloSegScore{0.7618}{(0.7342--0.7883)}{4.55pt}{4.82pt}{} & \HoloSegScore{0.3826}{(0.3438--0.4268)}{4.55pt}{4.82pt}{} & \HoloSegScore{0.7955}{(0.7699--0.8184)}{4.55pt}{4.82pt}{} & \HoloSegScore{0.7798}{(0.7529--0.8061)}{4.55pt}{4.82pt}{} & \HoloSegScore{0.7954}{(0.7891--0.8161)}{4.55pt}{4.82pt}{} & \HoloSegScore{0.8307}{(0.8056--0.8544)}{4.55pt}{4.82pt}{} & \HoloSegScore{0.8264}{(0.8052--0.8458)}{4.55pt}{4.82pt}{} \\*
\softcline{4-11}
 &  & \HoloSegSpan{\makecell[c]{esophagus}}{2.04cm}{0.32cm} & \HoloSegMetric{HD95} & \HoloSegScore{51.87}{(30.83--76.71)}{4.55pt}{4.82pt}{} & \HoloSegScore{17.52}{(12.58--25.23)}{4.55pt}{4.82pt}{} & \HoloSegScore{9.354}{(4.839--15.49)}{4.55pt}{4.82pt}{} & \HoloSegScore{11.57}{(6.910--18.50)}{4.55pt}{4.82pt}{} & \HoloSegScore{8.821}{(5.067--13.79)}{4.55pt}{4.82pt}{} & \HoloSegScore{7.676}{(4.118--12.24)}{4.55pt}{4.82pt}{} & \HoloSegScore{8.182}{(3.515--14.63)}{4.55pt}{4.82pt}{} \\
\cline{3-11}
 &  &  & \HoloSegMetric{Dice} & \HoloSegScore{0.9459}{(0.9384--0.9506)}{4.55pt}{4.82pt}{} & \HoloSegScore{0.8206}{(0.7867--0.8429)}{4.55pt}{4.82pt}{} & \HoloSegScore{0.9617}{(0.9530--0.9669)}{4.55pt}{4.82pt}{} & \HoloSegScore{0.9576}{(0.9475--0.9643)}{4.55pt}{4.82pt}{} & \HoloSegScore{0.9712}{(0.9657--0.9871)}{4.55pt}{4.82pt}{} & \HoloSegScore{0.9788}{(0.9712--0.9840)}{4.55pt}{4.82pt}{} & \HoloSegScore{0.9669}{(0.9625--0.9705)}{4.55pt}{4.82pt}{} \\*
\softcline{4-11}
\HoloSegSpan{\makecell[c]{\textbf{Internal}}}{1.20cm}{0.32cm} &  & \HoloSegSpan{\makecell[c]{liver}}{2.04cm}{0.32cm} & \HoloSegMetric{HD95} & \HoloSegScore{5.540}{(4.589--6.882)}{4.55pt}{4.82pt}{} & \HoloSegScore{20.12}{(13.07--31.50)}{4.55pt}{4.82pt}{} & \HoloSegScore{3.703}{(3.050--4.631)}{4.55pt}{4.82pt}{} & \HoloSegScore{6.137}{(4.450--8.366)}{4.55pt}{4.82pt}{} & \HoloSegScore{5.968}{(4.322--8.316)}{4.55pt}{4.82pt}{} & \HoloSegScore{3.529}{(2.405--4.924)}{4.55pt}{4.82pt}{} & \HoloSegScore{3.924}{(3.266--4.796)}{4.55pt}{4.82pt}{} \\
\cline{3-11}
 &  &  & \HoloSegMetric{Dice} & \HoloSegScore{0.8614}{(0.8198--0.8941)}{4.55pt}{4.82pt}{} & \HoloSegScore{0.5750}{(0.5264--0.6213)}{4.55pt}{4.82pt}{} & \HoloSegScore{0.8780}{(0.8339--0.9126)}{4.55pt}{4.82pt}{} & \HoloSegScore{0.8243}{(0.7756--0.8644)}{4.55pt}{4.82pt}{} & \HoloSegScore{0.8563}{(0.8157--0.8781)}{4.55pt}{4.82pt}{} & \HoloSegScore{0.9201}{(0.8814--0.9465)}{4.55pt}{4.82pt}{} & \HoloSegScore{0.9078}{(0.8692--0.9341)}{4.55pt}{4.82pt}{} \\*
\softcline{4-11}
 &  & \HoloSegSpan{\makecell[c]{stomach}}{2.04cm}{0.32cm} & \HoloSegMetric{HD95} & \HoloSegScore{16.85}{(9.919--25.54)}{4.55pt}{4.82pt}{} & \HoloSegScore{26.73}{(19.20--38.88)}{4.55pt}{4.82pt}{} & \HoloSegScore{20.68}{(6.859--38.10)}{4.55pt}{4.82pt}{} & \HoloSegScore{24.30}{(14.77--38.37)}{4.55pt}{4.82pt}{} & \HoloSegScore{12.75}{(8.997--17.21)}{4.55pt}{4.82pt}{} & \HoloSegScore{6.857}{(4.310--10.83)}{4.55pt}{4.82pt}{} & \HoloSegScore{8.632}{(5.319--12.71)}{4.55pt}{4.82pt}{} \\
\cline{3-11}
 &  &  & \HoloSegMetric{Dice} & \HoloSegScore{0.9032}{(0.8941--0.9110)}{4.55pt}{4.82pt}{} & \HoloSegScore{0.7327}{(0.7077--0.7556)}{4.55pt}{4.82pt}{} & \HoloSegScore{0.9113}{(0.9013--0.9200)}{4.55pt}{4.82pt}{} & \HoloSegScore{0.9236}{(0.9130--0.9325)}{4.55pt}{4.82pt}{} & \HoloSegScore{0.9480}{(0.9304--0.9619)}{4.55pt}{4.82pt}{} & \HoloSegScore{0.9397}{(0.9309--0.9473)}{4.55pt}{4.82pt}{} & \HoloSegScore{0.9326}{(0.9262--0.9386)}{4.55pt}{4.82pt}{} \\*
\softcline{4-11}
 & \HoloSegSpan{\makecell[c]{AMOS22}}{1.86cm}{0.32cm} & \HoloSegSpan{\makecell[c]{aorta}}{2.04cm}{0.32cm} & \HoloSegMetric{HD95} & \HoloSegScore{14.86}{(10.17--20.03)}{4.55pt}{4.82pt}{} & \HoloSegScore{15.70}{(11.54--20.62)}{4.55pt}{4.82pt}{} & \HoloSegScore{12.84}{(7.656--18.25)}{4.55pt}{4.82pt}{} & \HoloSegScore{9.546}{(5.394--15.02)}{4.55pt}{4.82pt}{} & \HoloSegScore{9.920}{(6.321--16.52)}{4.55pt}{4.82pt}{} & \HoloSegScore{7.591}{(3.545--12.13)}{4.55pt}{4.82pt}{} & \HoloSegScore{5.250}{(2.893--8.914)}{4.55pt}{4.82pt}{} \\
\cline{3-11}
 &  &  & \HoloSegMetric{Dice} & \HoloSegScore{0.8443}{(0.8249--0.8629)}{4.55pt}{4.82pt}{} & \HoloSegScore{0.6286}{(0.5920--0.6618)}{4.55pt}{4.82pt}{} & \HoloSegScore{0.8834}{(0.8693--0.8960)}{4.55pt}{4.82pt}{} & \HoloSegScore{0.8658}{(0.8460--0.8845)}{4.55pt}{4.82pt}{} & \HoloSegScore{0.8653}{(0.8483--0.8706)}{4.55pt}{4.82pt}{} & \HoloSegScore{0.8642}{(0.8435--0.8822)}{4.55pt}{4.82pt}{} & \HoloSegScore{0.8527}{(0.8344--0.8694)}{4.55pt}{4.82pt}{} \\*
\softcline{4-11}
 &  & \HoloSegSpan{\makecell[c]{inferior\\[-0.10ex]vena cava}}{2.04cm}{0.32cm} & \HoloSegMetric{HD95} & \HoloSegScore{7.634}{(6.560--8.909)}{4.55pt}{4.82pt}{} & \HoloSegScore{17.03}{(12.11--23.34)}{4.55pt}{4.82pt}{} & \HoloSegScore{3.885}{(3.532--4.281)}{4.55pt}{4.82pt}{} & \HoloSegScore{5.266}{(4.016--7.208)}{4.55pt}{4.82pt}{} & \HoloSegScore{5.487}{(4.166--5.964)}{4.55pt}{4.82pt}{} & \HoloSegScore{5.709}{(4.320--7.583)}{4.55pt}{4.82pt}{} & \HoloSegScore{5.681}{(4.517--7.278)}{4.55pt}{4.82pt}{} \\
\cline{3-11}
 &  &  & \HoloSegMetric{Dice} & \HoloSegScore{0.7877}{(0.7437--0.8228)}{4.55pt}{4.82pt}{} & \HoloSegScore{0.4633}{(0.4212--0.5015)}{4.55pt}{4.82pt}{} & \HoloSegScore{0.8238}{(0.7854--0.8522)}{4.55pt}{4.82pt}{} & \HoloSegScore{0.7745}{(0.7334--0.8112)}{4.55pt}{4.82pt}{} & \HoloSegScore{0.8382}{(0.8039--0.8402)}{4.55pt}{4.82pt}{} & \HoloSegScore{0.8441}{(0.8051--0.8740)}{4.55pt}{4.82pt}{} & \HoloSegScore{0.8401}{(0.8038--0.8659)}{4.55pt}{4.82pt}{} \\*
\softcline{4-11}
 &  & \HoloSegSpan{\makecell[c]{pancreas}}{2.04cm}{0.32cm} & \HoloSegMetric{HD95} & \HoloSegScore{10.24}{(7.381--13.91)}{4.55pt}{4.82pt}{} & \HoloSegScore{25.69}{(17.33--37.21)}{4.55pt}{4.82pt}{} & \HoloSegScore{6.421}{(4.395--9.042)}{4.55pt}{4.82pt}{} & \HoloSegScore{11.08}{(8.635--14.28)}{4.55pt}{4.82pt}{} & \HoloSegScore{8.071}{(6.318--12.57)}{4.55pt}{4.82pt}{} & \HoloSegScore{6.185}{(4.188--9.088)}{4.55pt}{4.82pt}{} & \HoloSegScore{6.226}{(4.412--9.015)}{4.55pt}{4.82pt}{} \\
\cline{3-11}
 &  &  & \HoloSegMetric{Dice} & \HoloSegScore{0.6934}{(0.6580--0.7261)}{4.55pt}{4.82pt}{} & \HoloSegScore{0.2357}{(0.2006--0.2721)}{4.55pt}{4.82pt}{} & \HoloSegScore{0.7568}{(0.7310--0.7800)}{4.55pt}{4.82pt}{} & \HoloSegScore{0.7379}{(0.7153--0.7601)}{4.55pt}{4.82pt}{} & \HoloSegScore{0.7019}{(0.6861--0.7187)}{4.55pt}{4.82pt}{} & \HoloSegScore{0.7409}{(0.7170--0.7628)}{4.55pt}{4.82pt}{} & \HoloSegScore{0.7676}{(0.7483--0.7863)}{4.55pt}{4.82pt}{} \\*
\softcline{4-11}
 &  & \HoloSegSpan{\makecell[c]{right\\[-0.10ex]adrenal\\[-0.10ex]gland}}{2.04cm}{0.32cm} & \HoloSegMetric{HD95} & \HoloSegScore{6.486}{(5.530--7.501)}{4.55pt}{4.82pt}{} & \HoloSegScore{24.52}{(14.99--36.95)}{4.55pt}{4.82pt}{} & \HoloSegScore{3.402}{(2.772--4.087)}{4.55pt}{4.82pt}{} & \HoloSegScore{5.089}{(4.334--5.954)}{4.55pt}{4.82pt}{} & \HoloSegScore{10.98}{(9.162--11.19)}{4.55pt}{4.82pt}{} & \HoloSegScore{6.092}{(3.958--8.669)}{4.55pt}{4.82pt}{} & \HoloSegScore{3.687}{(3.114--4.299)}{4.55pt}{4.82pt}{} \\
\cline{3-11}
 &  &  & \HoloSegMetric{Dice} & \HoloSegScore{0.6905}{(0.6468--0.7265)}{4.55pt}{4.82pt}{} & \HoloSegScore{0.2094}{(0.1730--0.2451)}{4.55pt}{4.82pt}{} & \HoloSegScore{0.7517}{(0.7072--0.7855)}{4.55pt}{4.82pt}{} & \HoloSegScore{0.7362}{(0.7014--0.7668)}{4.55pt}{4.82pt}{} & \HoloSegScore{0.7232}{(0.7118--0.7546)}{4.55pt}{4.82pt}{} & \HoloSegScore{0.7547}{(0.7167--0.7883)}{4.55pt}{4.82pt}{} & \HoloSegScore{0.7584}{(0.7283--0.7850)}{4.55pt}{4.82pt}{} \\*
\softcline{4-11}
 &  & \HoloSegSpan{\makecell[c]{left adrenal\\[-0.10ex]gland}}{2.04cm}{0.32cm} & \HoloSegMetric{HD95} & \HoloSegScore{6.943}{(5.746--8.554)}{4.55pt}{4.82pt}{} & \HoloSegScore{35.73}{(20.90--53.08)}{4.55pt}{4.82pt}{} & \HoloSegScore{3.355}{(2.594--4.531)}{4.55pt}{4.82pt}{} & \HoloSegScore{5.550}{(4.400--6.889)}{4.55pt}{4.82pt}{} & \HoloSegScore{7.885}{(3.908--8.232)}{4.55pt}{4.82pt}{} & \HoloSegScore{5.244}{(3.732--7.169)}{4.55pt}{4.82pt}{} & \HoloSegScore{5.928}{(4.374--7.723)}{4.55pt}{4.82pt}{} \\
\cline{3-11}
 &  &  & \HoloSegMetric{Dice} & \HoloSegScore{0.6869}{(0.6441--0.7275)}{4.55pt}{4.82pt}{} & \HoloSegScore{0.3833}{(0.3394--0.4198)}{4.55pt}{4.82pt}{} & \HoloSegScore{0.7734}{(0.7342--0.8041)}{4.55pt}{4.82pt}{} & \HoloSegScore{0.7035}{(0.6654--0.7363)}{4.55pt}{4.82pt}{} & \HoloSegScore{0.7463}{(0.6935--0.7923)}{4.55pt}{4.82pt}{} & \HoloSegScore{0.7662}{(0.7233--0.8004)}{4.55pt}{4.82pt}{} & \HoloSegScore{0.7716}{(0.7304--0.8059)}{4.55pt}{4.82pt}{} \\*
\softcline{4-11}
 &  & \HoloSegSpan{\makecell[c]{duodenum}}{2.04cm}{0.32cm} & \HoloSegMetric{HD95} & \HoloSegScore{15.08}{(12.26--18.52)}{4.55pt}{4.82pt}{} & \HoloSegScore{30.45}{(21.73--40.58)}{4.55pt}{4.82pt}{} & \HoloSegScore{8.060}{(6.321--10.25)}{4.55pt}{4.82pt}{} & \HoloSegScore{14.87}{(12.31--17.59)}{4.55pt}{4.82pt}{} & \HoloSegScore{9.371}{(8.042--12.93)}{4.55pt}{4.82pt}{} & \HoloSegScore{11.49}{(8.873--14.49)}{4.55pt}{4.82pt}{} & \HoloSegScore{9.211}{(7.034--11.92)}{4.55pt}{4.82pt}{} \\
\cline{3-11}
 &  &  & \HoloSegMetric{Dice} & \HoloSegScore{0.8094}{(0.7659--0.8480)}{4.55pt}{4.82pt}{} & \HoloSegScore{0.4055}{(0.3434--0.4703)}{4.55pt}{4.82pt}{} & \HoloSegScore{0.8466}{(0.8078--0.8783)}{4.55pt}{4.82pt}{} & \HoloSegScore{0.8079}{(0.7704--0.8447)}{4.55pt}{4.82pt}{} & \HoloSegScore{0.8088}{(0.7657--0.8553)}{4.55pt}{4.82pt}{} & \HoloSegScore{0.8884}{(0.8499--0.9176)}{4.55pt}{4.82pt}{} & \HoloSegScore{0.8687}{(0.8314--0.8974)}{4.55pt}{4.82pt}{} \\*
\softcline{4-11}
 &  & \HoloSegSpan{\makecell[c]{urinary\\[-0.10ex]bladder}}{2.04cm}{0.32cm} & \HoloSegMetric{HD95} & \HoloSegScore{15.03}{(8.262--25.44)}{4.55pt}{4.82pt}{} & \HoloSegScore{44.00}{(27.84--63.25)}{4.55pt}{4.82pt}{} & \HoloSegScore{7.687}{(5.239--10.73)}{4.55pt}{4.82pt}{} & \HoloSegScore{12.55}{(9.624--16.14)}{4.55pt}{4.82pt}{} & \HoloSegScore{8.819}{(6.488--9.952)}{4.55pt}{4.82pt}{} & \HoloSegScore{6.858}{(4.620--9.520)}{4.55pt}{4.82pt}{} & \HoloSegScore{7.230}{(5.115--9.884)}{4.55pt}{4.82pt}{} \\
\cline{3-11}
 &  &  & \HoloSegMetric{Dice} & \HoloSegScore{0.7680}{(0.7425--0.7899)}{4.55pt}{4.82pt}{} & \HoloSegScore{0.3878}{(0.3283--0.4445)}{4.55pt}{4.82pt}{} & \HoloSegScore{0.0000}{(0.0000--0.0000)}{4.55pt}{4.82pt}{} & \HoloSegScore{0.7808}{(0.7500--0.8070)}{4.55pt}{4.82pt}{} & \HoloSegScore{0.8247}{(0.8109--0.8286)}{4.55pt}{4.82pt}{} & \HoloSegScore{0.8782}{(0.8542--0.8986)}{4.55pt}{4.82pt}{} & \HoloSegScore{0.8260}{(0.7996--0.8527)}{4.55pt}{4.82pt}{} \\*
\softcline{4-11}
 &  & \HoloSegSpan{\makecell[c]{prostate or\\[-0.10ex]uterus}}{2.04cm}{0.32cm} & \HoloSegMetric{HD95} & \HoloSegScore{15.93}{(12.60--18.52)}{4.55pt}{4.82pt}{} & \HoloSegScore{31.77}{(22.81--40.86)}{4.55pt}{4.82pt}{} & \HoloSegScore{239.3}{(175.5--310.9)}{4.55pt}{4.82pt}{} & \HoloSegScore{14.31}{(11.43--17.62)}{4.55pt}{4.82pt}{} & \HoloSegScore{14.32}{(9.235--20.42)}{4.55pt}{4.82pt}{} & \HoloSegScore{9.235}{(5.354--15.61)}{4.55pt}{4.82pt}{} & \HoloSegScore{45.97}{(27.17--67.76)}{4.55pt}{4.82pt}{} \\
\hline
\pagebreak[4]
 &  &  & \HoloSegMetric{Dice} & \HoloSegScore{0.4005}{(0.2856--0.5077)}{4.55pt}{4.82pt}{} & \HoloSegScore{0.02744}{(0.007287--0.05207)}{3.85pt}{4.12pt}{} & \HoloSegScore{0.6740}{(0.5450--0.7863)}{4.55pt}{4.82pt}{} & \HoloSegScore{0.6852}{(0.6052--0.7550)}{4.55pt}{4.82pt}{} & \HoloSegScore{0.4700}{(0.4376--0.5049)}{4.55pt}{4.82pt}{} & \HoloSegScore{0.5877}{(0.4793--0.6891)}{4.55pt}{4.82pt}{} & \HoloSegScore{0.6159}{(0.5046--0.7023)}{4.55pt}{4.82pt}{} \\*
\softcline{4-11}
 & \HoloSegSpan{\makecell[c]{MSD-colon}}{1.86cm}{0.32cm} & \HoloSegSpan{\makecell[c]{colon cancer}}{2.04cm}{0.32cm} & \HoloSegMetric{HD95} & \HoloSegScore{165.8}{(130.6--200.2)}{4.55pt}{4.82pt}{} & \HoloSegScore{159.5}{(132.5--184.9)}{4.55pt}{4.82pt}{} & \HoloSegScore{18.35}{(4.606--38.52)}{4.55pt}{4.82pt}{} & \HoloSegScore{50.57}{(25.94--77.81)}{4.55pt}{4.82pt}{} & \HoloSegScore{50.57}{(35.86--69.49)}{4.55pt}{4.82pt}{} & \HoloSegScore{45.92}{(21.01--80.09)}{4.55pt}{4.82pt}{} & \HoloSegScore{39.64}{(16.25--71.21)}{4.55pt}{4.82pt}{} \\
\cline{2-11}
 &  &  & \HoloSegMetric{Dice} & \HoloSegScore{0.5389}{(0.5072--0.5713)}{4.55pt}{4.82pt}{} & \HoloSegScore{0.2274}{(0.1928--0.2622)}{4.55pt}{4.82pt}{} & \HoloSegScore{0.6835}{(0.6572--0.7063)}{4.55pt}{4.82pt}{} & \HoloSegScore{0.3526}{(0.3163--0.3904)}{4.55pt}{4.82pt}{} & \HoloSegScore{0.5466}{(0.5051--0.5754)}{4.55pt}{4.82pt}{} & \HoloSegScore{0.5575}{(0.5313--0.5861)}{4.55pt}{4.82pt}{} & \HoloSegScore{0.5431}{(0.5141--0.5733)}{4.55pt}{4.82pt}{} \\*
\softcline{4-11}
 &  & \HoloSegSpan{\makecell[c]{hepatic vein}}{2.04cm}{0.32cm} & \HoloSegMetric{HD95} & \HoloSegScore{25.02}{(21.58--28.42)}{4.55pt}{4.82pt}{} & \HoloSegScore{40.57}{(35.26--46.66)}{4.55pt}{4.82pt}{} & \HoloSegScore{11.10}{(9.039--13.33)}{4.55pt}{4.82pt}{} & \HoloSegScore{33.97}{(30.81--37.54)}{4.55pt}{4.82pt}{} & \HoloSegScore{12.67}{(11.13--14.95)}{4.55pt}{4.82pt}{} & \HoloSegScore{23.64}{(20.75--27.14)}{4.55pt}{4.82pt}{} & \HoloSegScore{24.68}{(21.68--28.71)}{4.55pt}{4.82pt}{} \\
\cline{3-11}
 & \HoloSegSpan{\makecell[c]{MSD-\\[-0.10ex]hepatic-\\[-0.10ex]vessel}}{1.86cm}{0.32cm} &  & \HoloSegMetric{Dice} & \HoloSegScore{0.6686}{(0.6051--0.7261)}{4.55pt}{4.82pt}{} & \HoloSegScore{0.4081}{(0.3255--0.4983)}{4.55pt}{4.82pt}{} & \HoloSegScore{0.8317}{(0.7966--0.8588)}{4.55pt}{4.82pt}{} & \HoloSegScore{0.7227}{(0.6660--0.7752)}{4.55pt}{4.82pt}{} & \HoloSegScore{0.6561}{(0.6394--0.7082)}{4.55pt}{4.82pt}{} & \HoloSegScore{0.7244}{(0.6608--0.7792)}{4.55pt}{4.82pt}{} & \HoloSegScore{0.7550}{(0.7148--0.7929)}{4.55pt}{4.82pt}{} \\*
\softcline{4-11}
 &  & \HoloSegSpan{\makecell[c]{liver tumor}}{2.04cm}{0.32cm} & \HoloSegMetric{HD95} & \HoloSegScore{25.97}{(17.43--35.69)}{4.55pt}{4.82pt}{} & \HoloSegScore{52.85}{(39.88--65.89)}{4.55pt}{4.82pt}{} & \HoloSegScore{14.05}{(7.233--23.11)}{4.55pt}{4.82pt}{} & \HoloSegScore{28.49}{(20.02--37.63)}{4.55pt}{4.82pt}{} & \HoloSegScore{46.78}{(37.52--56.03)}{4.55pt}{4.82pt}{} & \HoloSegScore{27.97}{(19.16--38.22)}{4.55pt}{4.82pt}{} & \HoloSegScore{32.13}{(22.91--43.21)}{4.55pt}{4.82pt}{} \\
\cline{2-11}
 &  &  & \HoloSegMetric{Dice} & \HoloSegScore{0.9322}{(0.9153--0.9468)}{4.55pt}{4.82pt}{} & \HoloSegScore{0.8293}{(0.8088--0.8503)}{4.55pt}{4.82pt}{} & \HoloSegScore{0.9413}{(0.9234--0.9556)}{4.55pt}{4.82pt}{} & \HoloSegScore{0.9441}{(0.9274--0.9597)}{4.55pt}{4.82pt}{} & \HoloSegScore{0.9359}{(0.9359--0.9551)}{4.55pt}{4.82pt}{} & \HoloSegScore{0.9614}{(0.9458--0.9751)}{4.55pt}{4.82pt}{} & \HoloSegScore{0.9452}{(0.9282--0.9599)}{4.55pt}{4.82pt}{} \\*
\softcline{4-11}
 &  & \HoloSegSpan{\makecell[c]{liver}}{2.04cm}{0.32cm} & \HoloSegMetric{HD95} & \HoloSegScore{14.75}{(8.405--23.80)}{4.55pt}{4.82pt}{} & \HoloSegScore{15.03}{(13.05--17.05)}{4.55pt}{4.82pt}{} & \HoloSegScore{6.676}{(4.726--8.900)}{4.55pt}{4.82pt}{} & \HoloSegScore{13.53}{(7.388--21.05)}{4.55pt}{4.82pt}{} & \HoloSegScore{8.406}{(7.344--9.245)}{4.55pt}{4.82pt}{} & \HoloSegScore{7.553}{(5.417--10.00)}{4.55pt}{4.82pt}{} & \HoloSegScore{8.063}{(6.008--10.57)}{4.55pt}{4.82pt}{} \\
\cline{3-11}
 & \HoloSegSpan{\makecell[c]{MSD-liver}}{1.86cm}{0.32cm} &  & \HoloSegMetric{Dice} & \HoloSegScore{0.5706}{(0.4435--0.6824)}{4.55pt}{4.82pt}{} & \HoloSegScore{0.1419}{(0.05291--0.2286)}{4.20pt}{4.48pt}{} & \HoloSegScore{0.7759}{(0.7414--0.8088)}{4.55pt}{4.82pt}{} & \HoloSegScore{0.7015}{(0.6234--0.7741)}{4.55pt}{4.82pt}{} & \HoloSegScore{0.6154}{(0.5858--0.6505)}{4.55pt}{4.82pt}{} & \HoloSegScore{0.6953}{(0.6381--0.7538)}{4.55pt}{4.82pt}{} & \HoloSegScore{0.7238}{(0.6599--0.7827)}{4.55pt}{4.82pt}{} \\*
\softcline{4-11}
 &  & \HoloSegSpan{\makecell[c]{liver tumor}}{2.04cm}{0.32cm} & \HoloSegMetric{HD95} & \HoloSegScore{64.06}{(29.87--101.9)}{4.55pt}{4.82pt}{} & \HoloSegScore{104.1}{(78.86--133.4)}{4.55pt}{4.82pt}{} & \HoloSegScore{15.17}{(7.883--23.64)}{4.55pt}{4.82pt}{} & \HoloSegScore{41.16}{(23.29--60.48)}{4.55pt}{4.82pt}{} & \HoloSegScore{26.58}{(20.21--34.43)}{4.55pt}{4.82pt}{} & \HoloSegScore{24.32}{(13.93--37.01)}{4.55pt}{4.82pt}{} & \HoloSegScore{29.35}{(15.05--46.90)}{4.55pt}{4.82pt}{} \\
\cline{2-11}
 &  &  & \HoloSegMetric{Dice} & \HoloSegScore{0.5982}{(0.4332--0.7361)}{4.55pt}{4.82pt}{} & \HoloSegScore{0.2832}{(0.1272--0.4450)}{4.55pt}{4.82pt}{} & \HoloSegScore{0.7533}{(0.6173--0.8433)}{4.55pt}{4.82pt}{} & \HoloSegScore{0.8410}{(0.7961--0.8816)}{4.55pt}{4.82pt}{} & \HoloSegScore{0.5558}{(0.5023--0.6008)}{4.55pt}{4.82pt}{} & \HoloSegScore{0.6743}{(0.5162--0.7923)}{4.55pt}{4.82pt}{} & \HoloSegScore{0.6819}{(0.5300--0.7988)}{4.55pt}{4.82pt}{} \\*
\softcline{4-11}
 & \HoloSegSpan{\makecell[c]{MSD-lung}}{1.86cm}{0.32cm} & \HoloSegSpan{\makecell[c]{lung tumor}}{2.04cm}{0.32cm} & \HoloSegMetric{HD95} & \HoloSegScore{72.63}{(19.53--149.0)}{4.55pt}{4.82pt}{} & \HoloSegScore{87.14}{(44.64--132.1)}{4.55pt}{4.82pt}{} & \HoloSegScore{10.76}{(2.730--25.65)}{4.55pt}{4.82pt}{} & \HoloSegScore{19.73}{(3.047--38.36)}{4.55pt}{4.82pt}{} & \HoloSegScore{52.84}{(35.25--78.39)}{4.55pt}{4.82pt}{} & \HoloSegScore{28.67}{(9.081--55.22)}{4.55pt}{4.82pt}{} & \HoloSegScore{11.80}{(4.696--23.45)}{4.55pt}{4.82pt}{} \\
\cline{2-11}
 &  &  & \HoloSegMetric{Dice} & \HoloSegScore{0.8028}{(0.7900--0.8156)}{4.55pt}{4.82pt}{} & \HoloSegScore{0.6045}{(0.5823--0.6276)}{4.55pt}{4.82pt}{} & \HoloSegScore{0.8444}{(0.8336--0.8545)}{4.55pt}{4.82pt}{} & \HoloSegScore{0.8119}{(0.7984--0.8253)}{4.55pt}{4.82pt}{} & \HoloSegScore{0.8039}{(0.7900--0.8122)}{4.55pt}{4.82pt}{} & \HoloSegScore{0.8232}{(0.8112--0.8364)}{4.55pt}{4.82pt}{} & \HoloSegScore{0.8174}{(0.8050--0.8303)}{4.55pt}{4.82pt}{} \\*
\softcline{4-11}
 &  & \HoloSegSpan{\makecell[c]{pancreas}}{2.04cm}{0.32cm} & \HoloSegMetric{HD95} & \HoloSegScore{7.667}{(6.807--8.631)}{4.55pt}{4.82pt}{} & \HoloSegScore{10.30}{(9.576--11.11)}{4.55pt}{4.82pt}{} & \HoloSegScore{4.161}{(3.842--4.489)}{4.55pt}{4.82pt}{} & \HoloSegScore{6.579}{(5.675--7.642)}{4.55pt}{4.82pt}{} & \HoloSegScore{4.739}{(4.116--5.713)}{4.55pt}{4.82pt}{} & \HoloSegScore{5.890}{(5.108--6.790)}{4.55pt}{4.82pt}{} & \HoloSegScore{7.376}{(5.848--9.335)}{4.55pt}{4.82pt}{} \\
\cline{3-11}
 & \HoloSegSpan{\makecell[c]{MSD-\\[-0.10ex]pancreas}}{1.86cm}{0.32cm} &  & \HoloSegMetric{Dice} & \HoloSegScore{0.3072}{(0.2335--0.3874)}{4.55pt}{4.82pt}{} & \HoloSegScore{0.2065}{(0.1529--0.2669)}{4.55pt}{4.82pt}{} & \HoloSegScore{0.7656}{(0.6933--0.8271)}{4.55pt}{4.82pt}{} & \HoloSegScore{0.6981}{(0.6480--0.7422)}{4.55pt}{4.82pt}{} & \HoloSegScore{0.4819}{(0.4381--0.5140)}{4.55pt}{4.82pt}{} & \HoloSegScore{0.5931}{(0.5269--0.6444)}{4.55pt}{4.82pt}{} & \HoloSegScore{0.6346}{(0.5683--0.6856)}{4.55pt}{4.82pt}{} \\*
\softcline{4-11}
 &  & \HoloSegSpan{\makecell[c]{pancreas\\[-0.10ex]tumor}}{2.04cm}{0.32cm} & \HoloSegMetric{HD95} & \HoloSegScore{67.51}{(45.61--93.08)}{4.55pt}{4.82pt}{} & \HoloSegScore{43.86}{(33.98--54.64)}{4.55pt}{4.82pt}{} & \HoloSegScore{4.453}{(2.965--6.489)}{4.55pt}{4.82pt}{} & \HoloSegScore{16.29}{(9.225--24.80)}{4.55pt}{4.82pt}{} & \HoloSegScore{45.81}{(14.42--78.70)}{4.55pt}{4.82pt}{} & \HoloSegScore{21.10}{(15.39--27.45)}{4.55pt}{4.82pt}{} & \HoloSegScore{25.74}{(18.24--34.65)}{4.55pt}{4.82pt}{} \\
\cline{2-11}
 &  &  & \HoloSegMetric{Dice} & \HoloSegScore{0.9385}{(0.9289--0.9470)}{4.55pt}{4.82pt}{} & \HoloSegScore{0.7589}{(0.7100--0.8104)}{4.55pt}{4.82pt}{} & \HoloSegScore{0.9478}{(0.9286--0.9642)}{4.55pt}{4.82pt}{} & \HoloSegScore{0.9514}{(0.9396--0.9617)}{4.55pt}{4.82pt}{} & \HoloSegScore{0.9441}{(0.9437--0.9482)}{4.55pt}{4.82pt}{} & \HoloSegScore{0.9672}{(0.9594--0.9749)}{4.55pt}{4.82pt}{} & \HoloSegScore{0.9576}{(0.9511--0.9638)}{4.55pt}{4.82pt}{} \\*
\softcline{4-11}
 & \HoloSegSpan{\makecell[c]{MSD-spleen}}{1.86cm}{0.32cm} & \HoloSegSpan{\makecell[c]{spleen}}{2.04cm}{0.32cm} & \HoloSegMetric{HD95} & \HoloSegScore{3.186}{(2.783--3.640)}{4.55pt}{4.82pt}{} & \HoloSegScore{9.828}{(8.470--11.17)}{4.55pt}{4.82pt}{} & \HoloSegScore{2.165}{(1.491--3.151)}{4.55pt}{4.82pt}{} & \HoloSegScore{2.316}{(1.708--3.167)}{4.55pt}{4.82pt}{} & \HoloSegScore{2.605}{(2.512--3.128)}{4.55pt}{4.82pt}{} & \HoloSegScore{1.521}{(1.181--1.947)}{4.55pt}{4.82pt}{} & \HoloSegScore{1.880}{(1.601--2.185)}{4.55pt}{4.82pt}{} \\
\cline{2-11}
 &  &  & \HoloSegMetric{Dice} & \HoloSegScore{0.9456}{(0.9254--0.9580)}{4.55pt}{4.82pt}{} & \HoloSegScore{0.9214}{(0.9067--0.9351)}{4.55pt}{4.82pt}{} & \HoloSegScore{0.9663}{(0.9508--0.9768)}{4.55pt}{4.82pt}{} & \HoloSegScore{0.9710}{(0.9652--0.9769)}{4.55pt}{4.82pt}{} & \HoloSegScore{0.9679}{(0.9565--0.9772)}{4.55pt}{4.82pt}{} & \HoloSegScore{0.9894}{(0.9818--0.9950)}{4.55pt}{4.82pt}{} & \HoloSegScore{0.9799}{(0.9757--0.9840)}{4.55pt}{4.82pt}{} \\*
\softcline{4-11}
\HoloSegSpan{\makecell[c]{\textbf{Internal}}}{1.20cm}{0.32cm} &  & \HoloSegSpan{\makecell[c]{lung}}{2.04cm}{0.32cm} & \HoloSegMetric{HD95} & \HoloSegScore{18.77}{(15.19--22.29)}{4.55pt}{4.82pt}{} & \HoloSegScore{16.16}{(11.22--21.90)}{4.55pt}{4.82pt}{} & \HoloSegScore{13.86}{(7.278--21.13)}{4.55pt}{4.82pt}{} & \HoloSegScore{13.62}{(10.38--17.51)}{4.55pt}{4.82pt}{} & \HoloSegScore{10.04}{(6.125--14.85)}{4.55pt}{4.82pt}{} & \HoloSegScore{6.497}{(2.352--10.64)}{4.55pt}{4.82pt}{} & \HoloSegScore{6.263}{(2.703--9.824)}{4.55pt}{4.82pt}{} \\
\cline{3-11}
 & \HoloSegSpan{\makecell[c]{AeroPath}}{1.86cm}{0.32cm} &  & \HoloSegMetric{Dice} & \HoloSegScore{0.7231}{(0.6776--0.7673)}{4.55pt}{4.82pt}{} & \HoloSegScore{0.6700}{(0.6259--0.7140)}{4.55pt}{4.82pt}{} & \HoloSegScore{0.7718}{(0.7370--0.8038)}{4.55pt}{4.82pt}{} & \HoloSegScore{0.8129}{(0.7474--0.8788)}{4.55pt}{4.82pt}{} & \HoloSegScore{0.8954}{(0.8679--0.9310)}{4.55pt}{4.82pt}{} & \HoloSegScore{0.8403}{(0.7765--0.8994)}{4.55pt}{4.82pt}{} & \HoloSegScore{0.8043}{(0.7434--0.8570)}{4.55pt}{4.82pt}{} \\*
\softcline{4-11}
 &  & \HoloSegSpan{\makecell[c]{trachea}}{2.04cm}{0.32cm} & \HoloSegMetric{HD95} & \HoloSegScore{74.29}{(67.40--83.76)}{4.55pt}{4.82pt}{} & \HoloSegScore{47.20}{(39.14--57.74)}{4.55pt}{4.82pt}{} & \HoloSegScore{40.55}{(30.65--51.73)}{4.55pt}{4.82pt}{} & \HoloSegScore{39.40}{(28.77--50.20)}{4.55pt}{4.82pt}{} & \HoloSegScore{34.57}{(28.66--42.83)}{4.55pt}{4.82pt}{} & \HoloSegScore{34.76}{(21.59--44.43)}{4.55pt}{4.82pt}{} & \HoloSegScore{46.46}{(36.11--55.08)}{4.55pt}{4.82pt}{} \\
\cline{2-11}
 &  &  & \HoloSegMetric{Dice} & \HoloSegScore{0.8468}{(0.8289--0.8636)}{4.55pt}{4.82pt}{} & \HoloSegScore{0.1527}{(0.06277--0.2515)}{4.20pt}{4.48pt}{} & \HoloSegScore{0.8426}{(0.8266--0.8574)}{4.55pt}{4.82pt}{} & \HoloSegScore{0.8881}{(0.8612--0.9114)}{4.55pt}{4.82pt}{} & \HoloSegScore{0.8599}{(0.8486--0.9011)}{4.55pt}{4.82pt}{} & \HoloSegScore{0.8623}{(0.8395--0.8860)}{4.55pt}{4.82pt}{} & \HoloSegScore{0.8821}{(0.8682--0.8963)}{4.55pt}{4.82pt}{} \\*
\softcline{4-11}
 &  & \HoloSegSpan{\makecell[c]{cervical\\[-0.10ex]vertebrae 1\\[-0.10ex](c1)}}{2.04cm}{0.32cm} & \HoloSegMetric{HD95} & \HoloSegScore{3.696}{(2.858--4.615)}{4.55pt}{4.82pt}{} & \HoloSegScore{110.3}{(23.98--250.4)}{4.55pt}{4.82pt}{} & \HoloSegScore{2.131}{(1.732--2.671)}{4.55pt}{4.82pt}{} & \HoloSegScore{3.649}{(2.165--5.280)}{4.55pt}{4.82pt}{} & \HoloSegScore{3.950}{(3.679--5.088)}{4.55pt}{4.82pt}{} & \HoloSegScore{5.063}{(3.034--7.517)}{4.55pt}{4.82pt}{} & \HoloSegScore{1.688}{(1.420--1.991)}{4.55pt}{4.82pt}{} \\
\cline{3-11}
 &  &  & \HoloSegMetric{Dice} & \HoloSegScore{0.8700}{(0.8483--0.8892)}{4.55pt}{4.82pt}{} & \HoloSegScore{0.1498}{(0.04401--0.2614)}{4.20pt}{4.48pt}{} & \HoloSegScore{0.8884}{(0.8800--0.8969)}{4.55pt}{4.82pt}{} & \HoloSegScore{0.9252}{(0.9136--0.9357)}{4.55pt}{4.82pt}{} & \HoloSegScore{0.8569}{(0.8458--0.8619)}{4.55pt}{4.82pt}{} & \HoloSegScore{0.8980}{(0.8713--0.9159)}{4.55pt}{4.82pt}{} & \HoloSegScore{0.9099}{(0.9018--0.9181)}{4.55pt}{4.82pt}{} \\*
\softcline{4-11}
 &  & \HoloSegSpan{\makecell[c]{cervical\\[-0.10ex]vertebrae 2\\[-0.10ex](c2)}}{2.04cm}{0.32cm} & \HoloSegMetric{HD95} & \HoloSegScore{14.72}{(2.685--37.57)}{4.55pt}{4.82pt}{} & \HoloSegScore{106.3}{(23.47--252.4)}{4.55pt}{4.82pt}{} & \HoloSegScore{1.608}{(1.417--1.833)}{4.55pt}{4.82pt}{} & \HoloSegScore{2.541}{(1.503--3.918)}{4.55pt}{4.82pt}{} & \HoloSegScore{7.315}{(5.970--11.67)}{4.55pt}{4.82pt}{} & \HoloSegScore{15.96}{(1.422--43.54)}{4.55pt}{4.82pt}{} & \HoloSegScore{1.679}{(1.381--2.058)}{4.55pt}{4.82pt}{} \\
\cline{3-11}
 &  &  & \HoloSegMetric{Dice} & \HoloSegScore{0.8195}{(0.7598--0.8664)}{4.55pt}{4.82pt}{} & \HoloSegScore{0.08709}{(0.03173--0.1618)}{4.20pt}{4.48pt}{} & \HoloSegScore{0.8315}{(0.8107--0.8506)}{4.55pt}{4.82pt}{} & \HoloSegScore{0.8989}{(0.8668--0.9224)}{4.55pt}{4.82pt}{} & \HoloSegScore{0.8475}{(0.8299--0.8569)}{4.55pt}{4.82pt}{} & \HoloSegScore{0.8274}{(0.7911--0.8584)}{4.55pt}{4.82pt}{} & \HoloSegScore{0.8721}{(0.8527--0.8891)}{4.55pt}{4.82pt}{} \\*
\softcline{4-11}
 &  & \HoloSegSpan{\makecell[c]{cervical\\[-0.10ex]vertebrae 3\\[-0.10ex](c3)}}{2.04cm}{0.32cm} & \HoloSegMetric{HD95} & \HoloSegScore{3.971}{(2.595--5.545)}{4.55pt}{4.82pt}{} & \HoloSegScore{95.47}{(26.83--221.7)}{4.55pt}{4.82pt}{} & \HoloSegScore{23.98}{(2.033--67.53)}{4.55pt}{4.82pt}{} & \HoloSegScore{1.776}{(1.165--2.689)}{4.55pt}{4.82pt}{} & \HoloSegScore{4.077}{(3.052--6.408)}{4.55pt}{4.82pt}{} & \HoloSegScore{4.955}{(3.272--6.939)}{4.55pt}{4.82pt}{} & \HoloSegScore{2.226}{(1.589--3.122)}{4.55pt}{4.82pt}{} \\
\cline{3-11}
 &  &  & \HoloSegMetric{Dice} & \HoloSegScore{0.8446}{(0.8187--0.8647)}{4.55pt}{4.82pt}{} & \HoloSegScore{0.1827}{(0.08219--0.2875)}{4.20pt}{4.48pt}{} & \HoloSegScore{0.8146}{(0.7767--0.8473)}{4.55pt}{4.82pt}{} & \HoloSegScore{0.8905}{(0.8565--0.9168)}{4.55pt}{4.82pt}{} & \HoloSegScore{0.8695}{(0.8447--0.8877)}{4.55pt}{4.82pt}{} & \HoloSegScore{0.5642}{(0.5470--0.5817)}{4.55pt}{4.82pt}{} & \HoloSegScore{0.8648}{(0.8469--0.8806)}{4.55pt}{4.82pt}{} \\*
\softcline{4-11}
 &  & \HoloSegSpan{\makecell[c]{cervical\\[-0.10ex]vertebrae 4\\[-0.10ex](c4)}}{2.04cm}{0.32cm} & \HoloSegMetric{HD95} & \HoloSegScore{21.13}{(2.539--57.23)}{4.55pt}{4.82pt}{} & \HoloSegScore{82.17}{(22.58--189.6)}{4.55pt}{4.82pt}{} & \HoloSegScore{24.92}{(1.997--70.20)}{4.55pt}{4.82pt}{} & \HoloSegScore{2.247}{(1.314--3.485)}{4.55pt}{4.82pt}{} & \HoloSegScore{6.338}{(4.069--8.156)}{4.55pt}{4.82pt}{} & \HoloSegScore{72.95}{(14.13--151.9)}{4.55pt}{4.82pt}{} & \HoloSegScore{2.055}{(1.697--2.413)}{4.55pt}{4.82pt}{} \\
\cline{3-11}
 & \HoloSegSpan{\makecell[c]{VerSe}}{1.86cm}{0.32cm} &  & \HoloSegMetric{Dice} & \HoloSegScore{0.8399}{(0.8209--0.8580)}{4.55pt}{4.82pt}{} & \HoloSegScore{0.1405}{(0.06912--0.2270)}{4.20pt}{4.48pt}{} & \HoloSegScore{0.8192}{(0.7831--0.8459)}{4.55pt}{4.82pt}{} & \HoloSegScore{0.8915}{(0.8656--0.9122)}{4.55pt}{4.82pt}{} & \HoloSegScore{0.8573}{(0.8495--0.8897)}{4.55pt}{4.82pt}{} & \HoloSegScore{0.4128}{(0.3164--0.5123)}{4.55pt}{4.82pt}{} & \HoloSegScore{0.8583}{(0.8414--0.8743)}{4.55pt}{4.82pt}{} \\*
\softcline{4-11}
 &  & \HoloSegSpan{\makecell[c]{cervical\\[-0.10ex]vertebrae 5\\[-0.10ex](c5)}}{2.04cm}{0.32cm} & \HoloSegMetric{HD95} & \HoloSegScore{4.731}{(0.2658--12.78)}{4.55pt}{4.82pt}{} & \HoloSegScore{133.3}{(67.00--217.0)}{4.55pt}{4.82pt}{} & \HoloSegScore{2.358}{(1.907--2.972)}{4.55pt}{4.82pt}{} & \HoloSegScore{2.888}{(1.794--3.988)}{4.55pt}{4.82pt}{} & \HoloSegScore{6.781}{(6.073--10.34)}{4.55pt}{4.82pt}{} & \HoloSegScore{8.910}{(6.957--10.56)}{4.55pt}{4.82pt}{} & \HoloSegScore{2.837}{(1.964--3.955)}{4.55pt}{4.82pt}{} \\
\cline{3-11}
 &  &  & \HoloSegMetric{Dice} & \HoloSegScore{0.8575}{(0.8483--0.8664)}{4.55pt}{4.82pt}{} & \HoloSegScore{0.04104}{(0.009703--0.07959)}{3.85pt}{4.12pt}{} & \HoloSegScore{0.8371}{(0.8228--0.8502)}{4.55pt}{4.82pt}{} & \HoloSegScore{0.8789}{(0.8536--0.9009)}{4.55pt}{4.82pt}{} & \HoloSegScore{0.8186}{(0.8082--0.8266)}{4.55pt}{4.82pt}{} & \HoloSegScore{0.8555}{(0.8374--0.8711)}{4.55pt}{4.82pt}{} & \HoloSegScore{0.8531}{(0.8352--0.8709)}{4.55pt}{4.82pt}{} \\*
\softcline{4-11}
 &  & \HoloSegSpan{\makecell[c]{cervical\\[-0.10ex]vertebrae 6\\[-0.10ex](c6)}}{2.04cm}{0.32cm} & \HoloSegMetric{HD95} & \HoloSegScore{2.686}{(2.464--2.959)}{4.55pt}{4.82pt}{} & \HoloSegScore{161.6}{(101.2--236.2)}{4.55pt}{4.82pt}{} & \HoloSegScore{2.186}{(1.893--2.528)}{4.55pt}{4.82pt}{} & \HoloSegScore{9.161}{(2.019--22.28)}{4.55pt}{4.82pt}{} & \HoloSegScore{3.583}{(3.552--6.216)}{4.55pt}{4.82pt}{} & \HoloSegScore{2.186}{(1.785--2.679)}{4.55pt}{4.82pt}{} & \HoloSegScore{2.743}{(2.193--3.441)}{4.55pt}{4.82pt}{} \\
\cline{3-11}
 &  &  & \HoloSegMetric{Dice} & \HoloSegScore{0.8497}{(0.8136--0.8729)}{4.55pt}{4.82pt}{} & \HoloSegScore{0.006017}{(0.0001674--0.01519)}{3.85pt}{4.12pt}{} & \HoloSegScore{0.8579}{(0.8469--0.8680)}{4.55pt}{4.82pt}{} & \HoloSegScore{0.8817}{(0.8535--0.9036)}{4.55pt}{4.82pt}{} & \HoloSegScore{0.8247}{(0.7978--0.8322)}{4.55pt}{4.82pt}{} & \HoloSegScore{0.8883}{(0.8793--0.8968)}{4.55pt}{4.82pt}{} & \HoloSegScore{0.8869}{(0.8774--0.8955)}{4.55pt}{4.82pt}{} \\*
\softcline{4-11}
 &  & \HoloSegSpan{\makecell[c]{cervical\\[-0.10ex]vertebrae 7\\[-0.10ex](c7)}}{2.04cm}{0.32cm} & \HoloSegMetric{HD95} & \HoloSegScore{3.746}{(2.675--5.184)}{4.55pt}{4.82pt}{} & \HoloSegScore{172.7}{(130.4--227.5)}{4.55pt}{4.82pt}{} & \HoloSegScore{2.357}{(1.930--2.875)}{4.55pt}{4.82pt}{} & \HoloSegScore{4.047}{(2.819--5.444)}{4.55pt}{4.82pt}{} & \HoloSegScore{6.017}{(5.307--9.112)}{4.55pt}{4.82pt}{} & \HoloSegScore{3.415}{(2.624--4.274)}{4.55pt}{4.82pt}{} & \HoloSegScore{2.756}{(2.200--3.424)}{4.55pt}{4.82pt}{} \\
\cline{3-11}
 &  &  & \HoloSegMetric{Dice} & \HoloSegScore{0.8354}{(0.8056--0.8597)}{4.55pt}{4.82pt}{} & \HoloSegScore{0.09463}{(0.05570--0.1328)}{4.20pt}{4.48pt}{} & \HoloSegScore{0.8784}{(0.8690--0.8864)}{4.55pt}{4.82pt}{} & \HoloSegScore{0.9056}{(0.8880--0.9208)}{4.55pt}{4.82pt}{} & \HoloSegScore{0.8035}{(0.7923--0.8118)}{4.55pt}{4.82pt}{} & \HoloSegScore{0.9109}{(0.9038--0.9178)}{4.55pt}{4.82pt}{} & \HoloSegScore{0.9074}{(0.9029--0.9121)}{4.55pt}{4.82pt}{} \\*
\softcline{4-11}
 &  & \HoloSegSpan{\makecell[c]{thoracic\\[-0.10ex]vertebrae 1\\[-0.10ex](t1)}}{2.04cm}{0.32cm} & \HoloSegMetric{HD95} & \HoloSegScore{27.29}{(20.06--35.09)}{4.55pt}{4.82pt}{} & \HoloSegScore{133.1}{(76.78--199.4)}{4.55pt}{4.82pt}{} & \HoloSegScore{2.555}{(1.743--3.650)}{4.55pt}{4.82pt}{} & \HoloSegScore{17.74}{(4.209--43.51)}{4.55pt}{4.82pt}{} & \HoloSegScore{7.411}{(5.121--11.52)}{4.55pt}{4.82pt}{} & \HoloSegScore{1.969}{(1.454--2.593)}{4.55pt}{4.82pt}{} & \HoloSegScore{1.939}{(1.517--2.629)}{4.55pt}{4.82pt}{} \\
\hline
\pagebreak[4]
 &  &  & \HoloSegMetric{Dice} & \HoloSegScore{0.8617}{(0.8251--0.8890)}{4.55pt}{4.82pt}{} & \HoloSegScore{0.1196}{(0.07368--0.1690)}{4.20pt}{4.48pt}{} & \HoloSegScore{0.8786}{(0.8646--0.8893)}{4.55pt}{4.82pt}{} & \HoloSegScore{0.8730}{(0.8373--0.9037)}{4.55pt}{4.82pt}{} & \HoloSegScore{0.8367}{(0.8271--0.8380)}{4.55pt}{4.82pt}{} & \HoloSegScore{0.8744}{(0.8431--0.8949)}{4.55pt}{4.82pt}{} & \HoloSegScore{0.9051}{(0.8861--0.9163)}{4.55pt}{4.82pt}{} \\*
\softcline{4-11}
 &  & \HoloSegSpan{\makecell[c]{thoracic\\[-0.10ex]vertebrae 2\\[-0.10ex](t2)}}{2.04cm}{0.32cm} & \HoloSegMetric{HD95} & \HoloSegScore{14.36}{(3.476--35.35)}{4.55pt}{4.82pt}{} & \HoloSegScore{125.0}{(75.95--178.8)}{4.55pt}{4.82pt}{} & \HoloSegScore{2.919}{(2.010--3.974)}{4.55pt}{4.82pt}{} & \HoloSegScore{17.91}{(5.456--40.78)}{4.55pt}{4.82pt}{} & \HoloSegScore{5.217}{(4.842--6.189)}{4.55pt}{4.82pt}{} & \HoloSegScore{2.887}{(2.116--3.852)}{4.55pt}{4.82pt}{} & \HoloSegScore{1.847}{(1.507--2.347)}{4.55pt}{4.82pt}{} \\
\cline{3-11}
 &  &  & \HoloSegMetric{Dice} & \HoloSegScore{0.8411}{(0.7943--0.8775)}{4.55pt}{4.82pt}{} & \HoloSegScore{0.2320}{(0.1647--0.3043)}{4.55pt}{4.82pt}{} & \HoloSegScore{0.8538}{(0.8158--0.8820)}{4.55pt}{4.82pt}{} & \HoloSegScore{0.8635}{(0.8246--0.8976)}{4.55pt}{4.82pt}{} & \HoloSegScore{0.8417}{(0.8078--0.8764)}{4.55pt}{4.82pt}{} & \HoloSegScore{0.8648}{(0.8212--0.8916)}{4.55pt}{4.82pt}{} & \HoloSegScore{0.8923}{(0.8603--0.9092)}{4.55pt}{4.82pt}{} \\*
\softcline{4-11}
 &  & \HoloSegSpan{\makecell[c]{thoracic\\[-0.10ex]vertebrae 3\\[-0.10ex](t3)}}{2.04cm}{0.32cm} & \HoloSegMetric{HD95} & \HoloSegScore{6.925}{(4.805--9.191)}{4.55pt}{4.82pt}{} & \HoloSegScore{111.4}{(59.10--170.5)}{4.55pt}{4.82pt}{} & \HoloSegScore{3.415}{(2.031--5.133)}{4.55pt}{4.82pt}{} & \HoloSegScore{10.90}{(6.874--15.44)}{4.55pt}{4.82pt}{} & \HoloSegScore{4.667}{(2.294--6.346)}{4.55pt}{4.82pt}{} & \HoloSegScore{8.124}{(6.242--10.22)}{4.55pt}{4.82pt}{} & \HoloSegScore{3.038}{(1.734--5.154)}{4.55pt}{4.82pt}{} \\
\cline{3-11}
 &  &  & \HoloSegMetric{Dice} & \HoloSegScore{0.8465}{(0.8049--0.8768)}{4.55pt}{4.82pt}{} & \HoloSegScore{0.2668}{(0.1859--0.3450)}{4.55pt}{4.82pt}{} & \HoloSegScore{0.8326}{(0.7698--0.8804)}{4.55pt}{4.82pt}{} & \HoloSegScore{0.8842}{(0.8434--0.9140)}{4.55pt}{4.82pt}{} & \HoloSegScore{0.7800}{(0.7352--0.8093)}{4.55pt}{4.82pt}{} & \HoloSegScore{0.7039}{(0.6738--0.7342)}{4.55pt}{4.82pt}{} & \HoloSegScore{0.8960}{(0.8824--0.9067)}{4.55pt}{4.82pt}{} \\*
\softcline{4-11}
 &  & \HoloSegSpan{\makecell[c]{thoracic\\[-0.10ex]vertebrae 4\\[-0.10ex](t4)}}{2.04cm}{0.32cm} & \HoloSegMetric{HD95} & \HoloSegScore{6.357}{(4.233--8.729)}{4.55pt}{4.82pt}{} & \HoloSegScore{105.5}{(53.64--162.7)}{4.55pt}{4.82pt}{} & \HoloSegScore{32.51}{(2.937--77.49)}{4.55pt}{4.82pt}{} & \HoloSegScore{5.874}{(3.226--9.008)}{4.55pt}{4.82pt}{} & \HoloSegScore{9.235}{(6.495--12.27)}{4.55pt}{4.82pt}{} & \HoloSegScore{45.52}{(27.57--66.34)}{4.55pt}{4.82pt}{} & \HoloSegScore{2.612}{(1.867--3.557)}{4.55pt}{4.82pt}{} \\
\cline{3-11}
 &  &  & \HoloSegMetric{Dice} & \HoloSegScore{0.8307}{(0.7784--0.8728)}{4.55pt}{4.82pt}{} & \HoloSegScore{0.2880}{(0.2106--0.3669)}{4.55pt}{4.82pt}{} & \HoloSegScore{0.8052}{(0.7185--0.8741)}{4.55pt}{4.82pt}{} & \HoloSegScore{0.8822}{(0.8378--0.9152)}{4.55pt}{4.82pt}{} & \HoloSegScore{0.7954}{(0.7593--0.8337)}{4.55pt}{4.82pt}{} & \HoloSegScore{0.5814}{(0.4934--0.6747)}{4.55pt}{4.82pt}{} & \HoloSegScore{0.9015}{(0.8888--0.9118)}{4.55pt}{4.82pt}{} \\*
\softcline{4-11}
 &  & \HoloSegSpan{\makecell[c]{thoracic\\[-0.10ex]vertebrae 5\\[-0.10ex](t5)}}{2.04cm}{0.32cm} & \HoloSegMetric{HD95} & \HoloSegScore{18.11}{(4.653--42.24)}{4.55pt}{4.82pt}{} & \HoloSegScore{101.1}{(51.75--157.7)}{4.55pt}{4.82pt}{} & \HoloSegScore{4.197}{(2.398--6.371)}{4.55pt}{4.82pt}{} & \HoloSegScore{5.758}{(3.277--9.028)}{4.55pt}{4.82pt}{} & \HoloSegScore{10.34}{(6.452--12.78)}{4.55pt}{4.82pt}{} & \HoloSegScore{8.838}{(6.613--10.93)}{4.55pt}{4.82pt}{} & \HoloSegScore{2.359}{(1.727--3.342)}{4.55pt}{4.82pt}{} \\
\cline{3-11}
 &  &  & \HoloSegMetric{Dice} & \HoloSegScore{0.8298}{(0.7593--0.8815)}{4.55pt}{4.82pt}{} & \HoloSegScore{0.2813}{(0.2040--0.3603)}{4.55pt}{4.82pt}{} & \HoloSegScore{0.7896}{(0.6966--0.8640)}{4.55pt}{4.82pt}{} & \HoloSegScore{0.8697}{(0.8082--0.9150)}{4.55pt}{4.82pt}{} & \HoloSegScore{0.7830}{(0.7399--0.7974)}{4.55pt}{4.82pt}{} & \HoloSegScore{0.8806}{(0.8577--0.8982)}{4.55pt}{4.82pt}{} & \HoloSegScore{0.8981}{(0.8807--0.9101)}{4.55pt}{4.82pt}{} \\*
\softcline{4-11}
 &  & \HoloSegSpan{\makecell[c]{thoracic\\[-0.10ex]vertebrae 6\\[-0.10ex](t6)}}{2.04cm}{0.32cm} & \HoloSegMetric{HD95} & \HoloSegScore{5.911}{(3.796--8.354)}{4.55pt}{4.82pt}{} & \HoloSegScore{86.21}{(42.69--133.0)}{4.55pt}{4.82pt}{} & \HoloSegScore{4.865}{(2.730--7.392)}{4.55pt}{4.82pt}{} & \HoloSegScore{6.409}{(3.694--9.568)}{4.55pt}{4.82pt}{} & \HoloSegScore{13.37}{(10.51--16.65)}{4.55pt}{4.82pt}{} & \HoloSegScore{3.182}{(2.557--3.824)}{4.55pt}{4.82pt}{} & \HoloSegScore{2.443}{(1.752--3.518)}{4.55pt}{4.82pt}{} \\
\cline{3-11}
 &  &  & \HoloSegMetric{Dice} & \HoloSegScore{0.8324}{(0.7669--0.8829)}{4.55pt}{4.82pt}{} & \HoloSegScore{0.2895}{(0.2084--0.3664)}{4.55pt}{4.82pt}{} & \HoloSegScore{0.7844}{(0.6869--0.8657)}{4.55pt}{4.82pt}{} & \HoloSegScore{0.8768}{(0.8277--0.9148)}{4.55pt}{4.82pt}{} & \HoloSegScore{0.8891}{(0.8690--0.9356)}{4.55pt}{4.82pt}{} & \HoloSegScore{0.9177}{(0.9021--0.9282)}{4.55pt}{4.82pt}{} & \HoloSegScore{0.9133}{(0.9065--0.9197)}{4.55pt}{4.82pt}{} \\*
\softcline{4-11}
 &  & \HoloSegSpan{\makecell[c]{thoracic\\[-0.10ex]vertebrae 7\\[-0.10ex](t7)}}{2.04cm}{0.32cm} & \HoloSegMetric{HD95} & \HoloSegScore{6.512}{(3.999--9.233)}{4.55pt}{4.82pt}{} & \HoloSegScore{72.59}{(40.87--111.0)}{4.55pt}{4.82pt}{} & \HoloSegScore{4.996}{(2.924--7.291)}{4.55pt}{4.82pt}{} & \HoloSegScore{7.826}{(5.149--10.69)}{4.55pt}{4.82pt}{} & \HoloSegScore{4.881}{(3.955--7.530)}{4.55pt}{4.82pt}{} & \HoloSegScore{3.242}{(1.769--5.197)}{4.55pt}{4.82pt}{} & \HoloSegScore{3.176}{(2.397--4.106)}{4.55pt}{4.82pt}{} \\
\cline{3-11}
 &  &  & \HoloSegMetric{Dice} & \HoloSegScore{0.8025}{(0.7210--0.8730)}{4.55pt}{4.82pt}{} & \HoloSegScore{0.2390}{(0.1617--0.3251)}{4.55pt}{4.82pt}{} & \HoloSegScore{0.7822}{(0.6868--0.8687)}{4.55pt}{4.82pt}{} & \HoloSegScore{0.8681}{(0.8150--0.9099)}{4.55pt}{4.82pt}{} & \HoloSegScore{0.8433}{(0.7904--0.8812)}{4.55pt}{4.82pt}{} & \HoloSegScore{0.8936}{(0.8791--0.9056)}{4.55pt}{4.82pt}{} & \HoloSegScore{0.9134}{(0.9054--0.9204)}{4.55pt}{4.82pt}{} \\*
\softcline{4-11}
 &  & \HoloSegSpan{\makecell[c]{thoracic\\[-0.10ex]vertebrae 8\\[-0.10ex](t8)}}{2.04cm}{0.32cm} & \HoloSegMetric{HD95} & \HoloSegScore{16.07}{(5.108--35.83)}{4.55pt}{4.82pt}{} & \HoloSegScore{91.69}{(56.01--128.7)}{4.55pt}{4.82pt}{} & \HoloSegScore{5.960}{(3.441--8.595)}{4.55pt}{4.82pt}{} & \HoloSegScore{9.761}{(6.781--13.07)}{4.55pt}{4.82pt}{} & \HoloSegScore{6.391}{(4.264--7.508)}{4.55pt}{4.82pt}{} & \HoloSegScore{3.453}{(2.756--4.286)}{4.55pt}{4.82pt}{} & \HoloSegScore{5.142}{(3.227--7.179)}{4.55pt}{4.82pt}{} \\
\cline{3-11}
 &  &  & \HoloSegMetric{Dice} & \HoloSegScore{0.8048}{(0.7238--0.8771)}{4.55pt}{4.82pt}{} & \HoloSegScore{0.2446}{(0.1892--0.3000)}{4.55pt}{4.82pt}{} & \HoloSegScore{0.7991}{(0.6966--0.8827)}{4.55pt}{4.82pt}{} & \HoloSegScore{0.8562}{(0.7798--0.9152)}{4.55pt}{4.82pt}{} & \HoloSegScore{0.8221}{(0.7723--0.8704)}{4.55pt}{4.82pt}{} & \HoloSegScore{0.9270}{(0.9169--0.9343)}{4.55pt}{4.82pt}{} & \HoloSegScore{0.9181}{(0.9073--0.9258)}{4.55pt}{4.82pt}{} \\*
\softcline{4-11}
 &  & \HoloSegSpan{\makecell[c]{thoracic\\[-0.10ex]vertebrae 9\\[-0.10ex](t9)}}{2.04cm}{0.32cm} & \HoloSegMetric{HD95} & \HoloSegScore{13.45}{(5.108--27.42)}{4.55pt}{4.82pt}{} & \HoloSegScore{75.94}{(48.41--105.8)}{4.55pt}{4.82pt}{} & \HoloSegScore{5.358}{(3.098--7.733)}{4.55pt}{4.82pt}{} & \HoloSegScore{8.198}{(5.391--11.16)}{4.55pt}{4.82pt}{} & \HoloSegScore{5.165}{(2.669--6.414)}{4.55pt}{4.82pt}{} & \HoloSegScore{5.091}{(2.856--7.617)}{4.55pt}{4.82pt}{} & \HoloSegScore{2.821}{(1.920--4.085)}{4.55pt}{4.82pt}{} \\
\cline{3-11}
 &  &  & \HoloSegMetric{Dice} & \HoloSegScore{0.7927}{(0.7085--0.8617)}{4.55pt}{4.82pt}{} & \HoloSegScore{0.2990}{(0.2427--0.3527)}{4.55pt}{4.82pt}{} & \HoloSegScore{0.8202}{(0.7366--0.8892)}{4.55pt}{4.82pt}{} & \HoloSegScore{0.8601}{(0.7967--0.9110)}{4.55pt}{4.82pt}{} & \HoloSegScore{0.8534}{(0.8095--0.8867)}{4.55pt}{4.82pt}{} & \HoloSegScore{0.8884}{(0.8676--0.9068)}{4.55pt}{4.82pt}{} & \HoloSegScore{0.9189}{(0.9096--0.9270)}{4.55pt}{4.82pt}{} \\*
\softcline{4-11}
 & \HoloSegSpan{\makecell[c]{VerSe}}{1.86cm}{0.32cm} & \HoloSegSpan{\makecell[c]{thoracic\\[-0.10ex]vertebrae 10\\[-0.10ex](t10)}}{2.04cm}{0.32cm} & \HoloSegMetric{HD95} & \HoloSegScore{6.741}{(4.750--9.258)}{4.55pt}{4.82pt}{} & \HoloSegScore{74.76}{(49.98--104.2)}{4.55pt}{4.82pt}{} & \HoloSegScore{4.585}{(2.740--6.643)}{4.55pt}{4.82pt}{} & \HoloSegScore{8.732}{(5.985--11.96)}{4.55pt}{4.82pt}{} & \HoloSegScore{5.913}{(5.138--8.030)}{4.55pt}{4.82pt}{} & \HoloSegScore{9.530}{(7.580--11.57)}{4.55pt}{4.82pt}{} & \HoloSegScore{3.539}{(2.322--4.990)}{4.55pt}{4.82pt}{} \\
\cline{3-11}
 &  &  & \HoloSegMetric{Dice} & \HoloSegScore{0.8162}{(0.7406--0.8785)}{4.55pt}{4.82pt}{} & \HoloSegScore{0.2560}{(0.2064--0.3071)}{4.55pt}{4.82pt}{} & \HoloSegScore{0.8385}{(0.7671--0.8974)}{4.55pt}{4.82pt}{} & \HoloSegScore{0.8796}{(0.8167--0.9236)}{4.55pt}{4.82pt}{} & \HoloSegScore{0.8322}{(0.7896--0.8690)}{4.55pt}{4.82pt}{} & \HoloSegScore{0.8852}{(0.8478--0.9149)}{4.55pt}{4.82pt}{} & \HoloSegScore{0.9148}{(0.8849--0.9342)}{4.55pt}{4.82pt}{} \\*
\softcline{4-11}
\HoloSegSpan{\makecell[c]{\textbf{Internal}}}{1.20cm}{0.32cm} &  & \HoloSegSpan{\makecell[c]{thoracic\\[-0.10ex]vertebrae 11\\[-0.10ex](t11)}}{2.04cm}{0.32cm} & \HoloSegMetric{HD95} & \HoloSegScore{7.269}{(4.836--10.05)}{4.55pt}{4.82pt}{} & \HoloSegScore{62.47}{(47.60--78.31)}{4.55pt}{4.82pt}{} & \HoloSegScore{4.523}{(2.687--6.648)}{4.55pt}{4.82pt}{} & \HoloSegScore{7.459}{(4.451--10.24)}{4.55pt}{4.82pt}{} & \HoloSegScore{7.065}{(2.731--8.076)}{4.55pt}{4.82pt}{} & \HoloSegScore{8.917}{(3.837--16.54)}{4.55pt}{4.82pt}{} & \HoloSegScore{2.724}{(1.803--3.819)}{4.55pt}{4.82pt}{} \\
\cline{3-11}
 &  &  & \HoloSegMetric{Dice} & \HoloSegScore{0.8597}{(0.8056--0.9019)}{4.55pt}{4.82pt}{} & \HoloSegScore{0.09522}{(0.05695--0.1374)}{4.20pt}{4.48pt}{} & \HoloSegScore{0.8930}{(0.8500--0.9194)}{4.55pt}{4.82pt}{} & \HoloSegScore{0.9194}{(0.8883--0.9444)}{4.55pt}{4.82pt}{} & \HoloSegScore{0.7955}{(0.7721--0.8127)}{4.55pt}{4.82pt}{} & \HoloSegScore{0.9113}{(0.8876--0.9289)}{4.55pt}{4.82pt}{} & \HoloSegScore{0.9241}{(0.9009--0.9388)}{4.55pt}{4.82pt}{} \\*
\softcline{4-11}
 &  & \HoloSegSpan{\makecell[c]{thoracic\\[-0.10ex]vertebrae 12\\[-0.10ex](t12)}}{2.04cm}{0.32cm} & \HoloSegMetric{HD95} & \HoloSegScore{7.798}{(5.044--10.99)}{4.55pt}{4.82pt}{} & \HoloSegScore{83.32}{(67.01--102.8)}{4.55pt}{4.82pt}{} & \HoloSegScore{18.10}{(3.406--40.09)}{4.55pt}{4.82pt}{} & \HoloSegScore{4.843}{(2.572--7.825)}{4.55pt}{4.82pt}{} & \HoloSegScore{16.04}{(9.603--23.31)}{4.55pt}{4.82pt}{} & \HoloSegScore{6.373}{(4.590--8.481)}{4.55pt}{4.82pt}{} & \HoloSegScore{2.906}{(1.622--4.798)}{4.55pt}{4.82pt}{} \\
\cline{3-11}
 &  &  & \HoloSegMetric{Dice} & \HoloSegScore{0.8593}{(0.8110--0.8950)}{4.55pt}{4.82pt}{} & \HoloSegScore{0.1364}{(0.09955--0.1758)}{4.20pt}{4.48pt}{} & \HoloSegScore{0.8828}{(0.8461--0.9110)}{4.55pt}{4.82pt}{} & \HoloSegScore{0.9295}{(0.9076--0.9464)}{4.55pt}{4.82pt}{} & \HoloSegScore{0.8725}{(0.8526--0.8905)}{4.55pt}{4.82pt}{} & \HoloSegScore{0.8938}{(0.8587--0.9235)}{4.55pt}{4.82pt}{} & \HoloSegScore{0.9326}{(0.9194--0.9419)}{4.55pt}{4.82pt}{} \\*
\softcline{4-11}
 &  & \HoloSegSpan{\makecell[c]{lumbar\\[-0.10ex]vertebrae 1\\[-0.10ex](l1)}}{2.04cm}{0.32cm} & \HoloSegMetric{HD95} & \HoloSegScore{9.023}{(6.015--12.24)}{4.55pt}{4.82pt}{} & \HoloSegScore{69.96}{(60.72--80.93)}{4.55pt}{4.82pt}{} & \HoloSegScore{17.58}{(4.458--35.97)}{4.55pt}{4.82pt}{} & \HoloSegScore{6.275}{(3.540--9.527)}{4.55pt}{4.82pt}{} & \HoloSegScore{10.35}{(7.565--13.58)}{4.55pt}{4.82pt}{} & \HoloSegScore{13.75}{(6.306--23.10)}{4.55pt}{4.82pt}{} & \HoloSegScore{3.263}{(1.944--4.841)}{4.55pt}{4.82pt}{} \\
\cline{3-11}
 &  &  & \HoloSegMetric{Dice} & \HoloSegScore{0.8143}{(0.7532--0.8681)}{4.55pt}{4.82pt}{} & \HoloSegScore{0.2809}{(0.2307--0.3334)}{4.55pt}{4.82pt}{} & \HoloSegScore{0.8230}{(0.7543--0.8771)}{4.55pt}{4.82pt}{} & \HoloSegScore{0.9197}{(0.8935--0.9402)}{4.55pt}{4.82pt}{} & \HoloSegScore{0.8036}{(0.7748--0.8171)}{4.55pt}{4.82pt}{} & \HoloSegScore{0.8598}{(0.8081--0.8954)}{4.55pt}{4.82pt}{} & \HoloSegScore{0.9318}{(0.9198--0.9400)}{4.55pt}{4.82pt}{} \\*
\softcline{4-11}
 &  & \HoloSegSpan{\makecell[c]{lumbar\\[-0.10ex]vertebrae 2\\[-0.10ex](l2)}}{2.04cm}{0.32cm} & \HoloSegMetric{HD95} & \HoloSegScore{10.11}{(6.875--13.33)}{4.55pt}{4.82pt}{} & \HoloSegScore{51.11}{(42.19--62.19)}{4.55pt}{4.82pt}{} & \HoloSegScore{19.94}{(5.825--39.06)}{4.55pt}{4.82pt}{} & \HoloSegScore{7.195}{(4.066--11.92)}{4.55pt}{4.82pt}{} & \HoloSegScore{10.47}{(10.42--15.27)}{4.55pt}{4.82pt}{} & \HoloSegScore{9.990}{(7.908--12.41)}{4.55pt}{4.82pt}{} & \HoloSegScore{6.684}{(2.035--15.71)}{4.55pt}{4.82pt}{} \\
\cline{3-11}
 &  &  & \HoloSegMetric{Dice} & \HoloSegScore{0.7412}{(0.6574--0.8137)}{4.55pt}{4.82pt}{} & \HoloSegScore{0.3597}{(0.2983--0.4175)}{4.55pt}{4.82pt}{} & \HoloSegScore{0.7539}{(0.6777--0.8299)}{4.55pt}{4.82pt}{} & \HoloSegScore{0.8838}{(0.8380--0.9221)}{4.55pt}{4.82pt}{} & \HoloSegScore{0.8802}{(0.8304--0.9163)}{4.55pt}{4.82pt}{} & \HoloSegScore{0.8818}{(0.8525--0.9064)}{4.55pt}{4.82pt}{} & \HoloSegScore{0.9239}{(0.9132--0.9325)}{4.55pt}{4.82pt}{} \\*
\softcline{4-11}
 &  & \HoloSegSpan{\makecell[c]{lumbar\\[-0.10ex]vertebrae 3\\[-0.10ex](l3)}}{2.04cm}{0.32cm} & \HoloSegMetric{HD95} & \HoloSegScore{12.13}{(8.842--15.98)}{4.55pt}{4.82pt}{} & \HoloSegScore{48.05}{(38.38--58.63)}{4.55pt}{4.82pt}{} & \HoloSegScore{31.31}{(11.51--57.54)}{4.55pt}{4.82pt}{} & \HoloSegScore{10.82}{(6.012--18.49)}{4.55pt}{4.82pt}{} & \HoloSegScore{8.910}{(6.393--11.83)}{4.55pt}{4.82pt}{} & \HoloSegScore{14.70}{(12.06--17.31)}{4.55pt}{4.82pt}{} & \HoloSegScore{5.772}{(4.068--7.568)}{4.55pt}{4.82pt}{} \\
\cline{3-11}
 &  &  & \HoloSegMetric{Dice} & \HoloSegScore{0.6976}{(0.6109--0.7812)}{4.55pt}{4.82pt}{} & \HoloSegScore{0.3387}{(0.2783--0.3921)}{4.55pt}{4.82pt}{} & \HoloSegScore{0.6898}{(0.5936--0.7707)}{4.55pt}{4.82pt}{} & \HoloSegScore{0.8494}{(0.7950--0.8973)}{4.55pt}{4.82pt}{} & \HoloSegScore{0.7697}{(0.7269--0.8140)}{4.55pt}{4.82pt}{} & \HoloSegScore{0.7975}{(0.7503--0.8393)}{4.55pt}{4.82pt}{} & \HoloSegScore{0.9169}{(0.9006--0.9298)}{4.55pt}{4.82pt}{} \\*
\softcline{4-11}
 &  & \HoloSegSpan{\makecell[c]{lumbar\\[-0.10ex]vertebrae 4\\[-0.10ex](l4)}}{2.04cm}{0.32cm} & \HoloSegMetric{HD95} & \HoloSegScore{149.6}{(101.8--196.6)}{4.55pt}{4.82pt}{} & \HoloSegScore{56.24}{(43.52--70.70)}{4.55pt}{4.82pt}{} & \HoloSegScore{40.16}{(15.84--72.41)}{4.55pt}{4.82pt}{} & \HoloSegScore{13.83}{(8.509--21.71)}{4.55pt}{4.82pt}{} & \HoloSegScore{16.19}{(13.79--17.36)}{4.55pt}{4.82pt}{} & \HoloSegScore{47.61}{(24.76--77.16)}{4.55pt}{4.82pt}{} & \HoloSegScore{5.735}{(4.079--7.662)}{4.55pt}{4.82pt}{} \\
\cline{3-11}
 &  &  & \HoloSegMetric{Dice} & \HoloSegScore{0.7304}{(0.6466--0.8073)}{4.55pt}{4.82pt}{} & \HoloSegScore{0.2154}{(0.1603--0.2751)}{4.55pt}{4.82pt}{} & \HoloSegScore{0.6830}{(0.5935--0.7738)}{4.55pt}{4.82pt}{} & \HoloSegScore{0.8191}{(0.7727--0.8596)}{4.55pt}{4.82pt}{} & \HoloSegScore{0.7591}{(0.7004--0.8000)}{4.55pt}{4.82pt}{} & \HoloSegScore{0.8089}{(0.7501--0.8666)}{4.55pt}{4.82pt}{} & \HoloSegScore{0.8581}{(0.8293--0.8843)}{4.55pt}{4.82pt}{} \\*
\softcline{4-11}
 &  & \HoloSegSpan{\makecell[c]{lumbar\\[-0.10ex]vertebrae 5\\[-0.10ex](l5)}}{2.04cm}{0.32cm} & \HoloSegMetric{HD95} & \HoloSegScore{12.68}{(9.305--15.90)}{4.55pt}{4.82pt}{} & \HoloSegScore{67.52}{(51.32--83.28)}{4.55pt}{4.82pt}{} & \HoloSegScore{11.21}{(7.845--14.88)}{4.55pt}{4.82pt}{} & \HoloSegScore{17.06}{(12.02--24.12)}{4.55pt}{4.82pt}{} & \HoloSegScore{15.45}{(11.68--22.11)}{4.55pt}{4.82pt}{} & \HoloSegScore{12.89}{(9.221--17.24)}{4.55pt}{4.82pt}{} & \HoloSegScore{10.16}{(7.465--13.05)}{4.55pt}{4.82pt}{} \\
\cline{3-11}
 &  &  & \HoloSegMetric{Dice} &  & \HoloSegScore{0.02595}{(0.0000--0.06496)}{4.20pt}{4.48pt}{} & \HoloSegScore{0.5369}{(0.4201--0.6494)}{4.55pt}{4.82pt}{} & \HoloSegScore{0.07041}{(0.0000--0.1781)}{4.55pt}{4.82pt}{} & \HoloSegScore{0.4742}{(0.4334--0.5082)}{4.55pt}{4.82pt}{} & \HoloSegScore{0.8005}{(0.7014--0.8828)}{4.55pt}{4.82pt}{} & \HoloSegScore{0.8047}{(0.7585--0.8385)}{4.55pt}{4.82pt}{} \\*
\softcline{4-4}\softcline{6-11}
 &  & \HoloSegSpan{\makecell[c]{lumbar\\[-0.10ex]vertebrae 6\\[-0.10ex](l6)}}{2.04cm}{0.32cm} & \HoloSegMetric{HD95} & \raisebox{0.32cm}[0pt][0pt]{\HoloSegUnsupported} & \HoloSegScore{220.2}{(174.1--264.6)}{4.55pt}{4.82pt}{} & \HoloSegScore{19.36}{(16.67--21.89)}{4.55pt}{4.82pt}{} & \HoloSegScore{19.10}{(18.56--19.63)}{4.55pt}{4.82pt}{} & \HoloSegScore{41.88}{(33.45--49.79)}{4.55pt}{4.82pt}{} & \HoloSegScore{12.47}{(8.074--17.32)}{4.55pt}{4.82pt}{} & \HoloSegScore{21.45}{(18.71--23.77)}{4.55pt}{4.82pt}{} \\
\cline{2-11}
 &  &  & \HoloSegMetric{Dice} & \HoloSegScore{0.9526}{(0.9470--0.9577)}{4.55pt}{4.82pt}{} & \HoloSegScore{0.7209}{(0.6897--0.7494)}{4.55pt}{4.82pt}{} & \HoloSegScore{0.9369}{(0.9172--0.9527)}{4.55pt}{4.82pt}{} & \HoloSegScore{0.9649}{(0.9578--0.9702)}{4.55pt}{4.82pt}{} & \HoloSegScore{0.9643}{(0.9642--0.9772)}{4.55pt}{4.82pt}{} & \HoloSegScore{0.9691}{(0.9593--0.9779)}{4.55pt}{4.82pt}{} & \HoloSegScore{0.9657}{(0.9596--0.9710)}{4.55pt}{4.82pt}{} \\*
\softcline{4-11}
 &  & \HoloSegSpan{\makecell[c]{spleen}}{2.04cm}{0.32cm} & \HoloSegMetric{HD95} & \HoloSegScore{20.33}{(9.383--33.11)}{4.55pt}{4.82pt}{} & \HoloSegScore{23.89}{(17.68--32.07)}{4.55pt}{4.82pt}{} & \HoloSegScore{2.988}{(2.186--3.893)}{4.55pt}{4.82pt}{} & \HoloSegScore{3.014}{(2.161--4.126)}{4.55pt}{4.82pt}{} & \HoloSegScore{4.934}{(4.846--5.274)}{4.55pt}{4.82pt}{} & \HoloSegScore{3.500}{(1.738--6.533)}{4.55pt}{4.82pt}{} & \HoloSegScore{2.501}{(1.941--3.220)}{4.55pt}{4.82pt}{} \\
\cline{3-11}
 & \HoloSegSpan{\makecell[c]{Total-\\[-0.10ex]SegmentatorV2}}{1.86cm}{0.32cm} &  & \HoloSegMetric{Dice} & \HoloSegScore{0.9187}{(0.8958--0.9370)}{4.55pt}{4.82pt}{} & \HoloSegScore{0.6254}{(0.5895--0.6588)}{4.55pt}{4.82pt}{} & \HoloSegScore{0.9088}{(0.8860--0.9300)}{4.55pt}{4.82pt}{} & \HoloSegScore{0.9356}{(0.9117--0.9554)}{4.55pt}{4.82pt}{} & \HoloSegScore{0.9430}{(0.9226--0.9668)}{4.55pt}{4.82pt}{} & \HoloSegScore{0.9352}{(0.9098--0.9581)}{4.55pt}{4.82pt}{} & \HoloSegScore{0.9201}{(0.8963--0.9414)}{4.55pt}{4.82pt}{} \\*
\softcline{4-11}
 &  & \HoloSegSpan{\makecell[c]{right kidney}}{2.04cm}{0.32cm} & \HoloSegMetric{HD95} & \HoloSegScore{11.13}{(5.069--19.07)}{4.55pt}{4.82pt}{} & \HoloSegScore{48.52}{(39.08--58.62)}{4.55pt}{4.82pt}{} & \HoloSegScore{2.366}{(1.977--2.774)}{4.55pt}{4.82pt}{} & \HoloSegScore{2.583}{(1.982--3.318)}{4.55pt}{4.82pt}{} & \HoloSegScore{3.493}{(2.839--3.970)}{4.55pt}{4.82pt}{} & \HoloSegScore{5.282}{(2.173--10.27)}{4.55pt}{4.82pt}{} & \HoloSegScore{3.957}{(3.089--4.900)}{4.55pt}{4.82pt}{} \\
\hline
\pagebreak[4]
 &  &  & \HoloSegMetric{Dice} & \HoloSegScore{0.9063}{(0.8749--0.9335)}{4.55pt}{4.82pt}{} & \HoloSegScore{0.6382}{(0.6000--0.6727)}{4.55pt}{4.82pt}{} & \HoloSegScore{0.9168}{(0.8909--0.9368)}{4.55pt}{4.82pt}{} & \HoloSegScore{0.9185}{(0.8847--0.9474)}{4.55pt}{4.82pt}{} & \HoloSegScore{0.9211}{(0.8985--0.9327)}{4.55pt}{4.82pt}{} & \HoloSegScore{0.9281}{(0.8957--0.9549)}{4.55pt}{4.82pt}{} & \HoloSegScore{0.9324}{(0.9090--0.9525)}{4.55pt}{4.82pt}{} \\*
\softcline{4-11}
 &  & \HoloSegSpan{\makecell[c]{left kidney}}{2.04cm}{0.32cm} & \HoloSegMetric{HD95} & \HoloSegScore{4.359}{(3.384--5.442)}{4.55pt}{4.82pt}{} & \HoloSegScore{46.40}{(36.99--56.72)}{4.55pt}{4.82pt}{} & \HoloSegScore{2.442}{(1.836--3.414)}{4.55pt}{4.82pt}{} & \HoloSegScore{3.221}{(2.020--4.724)}{4.55pt}{4.82pt}{} & \HoloSegScore{2.859}{(0.4540--3.014)}{4.55pt}{4.82pt}{} & \HoloSegScore{9.600}{(4.172--16.28)}{4.55pt}{4.82pt}{} & \HoloSegScore{2.998}{(2.228--3.827)}{4.55pt}{4.82pt}{} \\
\cline{3-11}
 &  &  & \HoloSegMetric{Dice} & \HoloSegScore{0.8171}{(0.7730--0.8575)}{4.55pt}{4.82pt}{} & \HoloSegScore{0.3347}{(0.2908--0.3806)}{4.55pt}{4.82pt}{} & \HoloSegScore{0.8209}{(0.7848--0.8560)}{4.55pt}{4.82pt}{} & \HoloSegScore{0.8042}{(0.7566--0.8477)}{4.55pt}{4.82pt}{} & \HoloSegScore{0.8406}{(0.7956--0.8817)}{4.55pt}{4.82pt}{} & \HoloSegScore{0.8113}{(0.7616--0.8539)}{4.55pt}{4.82pt}{} & \HoloSegScore{0.8131}{(0.7653--0.8530)}{4.55pt}{4.82pt}{} \\*
\softcline{4-11}
 &  & \HoloSegSpan{\makecell[c]{gallbladder}}{2.04cm}{0.32cm} & \HoloSegMetric{HD95} & \HoloSegScore{8.566}{(5.904--12.67)}{4.55pt}{4.82pt}{} & \HoloSegScore{40.53}{(30.70--51.73)}{4.55pt}{4.82pt}{} & \HoloSegScore{7.975}{(3.897--15.76)}{4.55pt}{4.82pt}{} & \HoloSegScore{5.802}{(4.418--7.529)}{4.55pt}{4.82pt}{} & \HoloSegScore{6.723}{(3.888--9.440)}{4.55pt}{4.82pt}{} & \HoloSegScore{9.292}{(5.804--14.58)}{4.55pt}{4.82pt}{} & \HoloSegScore{6.153}{(4.756--7.936)}{4.55pt}{4.82pt}{} \\
\cline{3-11}
 &  &  & \HoloSegMetric{Dice} & \HoloSegScore{0.9503}{(0.9341--0.9626)}{4.55pt}{4.82pt}{} & \HoloSegScore{0.8167}{(0.7877--0.8394)}{4.55pt}{4.82pt}{} & \HoloSegScore{0.9535}{(0.9370--0.9655)}{4.55pt}{4.82pt}{} & \HoloSegScore{0.9568}{(0.9371--0.9711)}{4.55pt}{4.82pt}{} & \HoloSegScore{0.9618}{(0.9235--0.9632)}{4.55pt}{4.82pt}{} & \HoloSegScore{0.9619}{(0.9428--0.9791)}{4.55pt}{4.82pt}{} & \HoloSegScore{0.9539}{(0.9367--0.9689)}{4.55pt}{4.82pt}{} \\*
\softcline{4-11}
 &  & \HoloSegSpan{\makecell[c]{liver}}{2.04cm}{0.32cm} & \HoloSegMetric{HD95} & \HoloSegScore{14.37}{(5.884--24.77)}{4.55pt}{4.82pt}{} & \HoloSegScore{16.94}{(13.96--20.39)}{4.55pt}{4.82pt}{} & \HoloSegScore{3.326}{(2.698--4.383)}{4.55pt}{4.82pt}{} & \HoloSegScore{3.539}{(3.164--3.971)}{4.55pt}{4.82pt}{} & \HoloSegScore{4.306}{(1.958--6.752)}{4.55pt}{4.82pt}{} & \HoloSegScore{5.986}{(3.033--10.58)}{4.55pt}{4.82pt}{} & \HoloSegScore{4.018}{(3.101--5.252)}{4.55pt}{4.82pt}{} \\
\cline{3-11}
 &  &  & \HoloSegMetric{Dice} & \HoloSegScore{0.9173}{(0.8972--0.9345)}{4.55pt}{4.82pt}{} & \HoloSegScore{0.6204}{(0.5871--0.6514)}{4.55pt}{4.82pt}{} & \HoloSegScore{0.8805}{(0.8565--0.9029)}{4.55pt}{4.82pt}{} & \HoloSegScore{0.9190}{(0.8977--0.9363)}{4.55pt}{4.82pt}{} & \HoloSegScore{0.9372}{(0.9287--0.9646)}{4.55pt}{4.82pt}{} & \HoloSegScore{0.9319}{(0.9110--0.9490)}{4.55pt}{4.82pt}{} & \HoloSegScore{0.9262}{(0.9091--0.9402)}{4.55pt}{4.82pt}{} \\*
\softcline{4-11}
 &  & \HoloSegSpan{\makecell[c]{stomach}}{2.04cm}{0.32cm} & \HoloSegMetric{HD95} & \HoloSegScore{9.378}{(6.074--13.42)}{4.55pt}{4.82pt}{} & \HoloSegScore{26.21}{(21.18--31.87)}{4.55pt}{4.82pt}{} & \HoloSegScore{41.35}{(23.07--61.45)}{4.55pt}{4.82pt}{} & \HoloSegScore{6.047}{(5.005--7.271)}{4.55pt}{4.82pt}{} & \HoloSegScore{3.029}{(2.718--3.568)}{4.55pt}{4.82pt}{} & \HoloSegScore{6.361}{(4.796--8.532)}{4.55pt}{4.82pt}{} & \HoloSegScore{13.70}{(7.073--21.46)}{4.55pt}{4.82pt}{} \\
\cline{3-11}
 &  &  & \HoloSegMetric{Dice} & \HoloSegScore{0.8460}{(0.8216--0.8675)}{4.55pt}{4.82pt}{} & \HoloSegScore{0.4827}{(0.4510--0.5130)}{4.55pt}{4.82pt}{} & \HoloSegScore{0.8412}{(0.8171--0.8615)}{4.55pt}{4.82pt}{} & \HoloSegScore{0.8395}{(0.8136--0.8637)}{4.55pt}{4.82pt}{} & \HoloSegScore{0.8608}{(0.8304--0.9013)}{4.55pt}{4.82pt}{} & \HoloSegScore{0.8535}{(0.8277--0.8770)}{4.55pt}{4.82pt}{} & \HoloSegScore{0.8587}{(0.8378--0.8784)}{4.55pt}{4.82pt}{} \\*
\softcline{4-11}
 &  & \HoloSegSpan{\makecell[c]{pancreas}}{2.04cm}{0.32cm} & \HoloSegMetric{HD95} & \HoloSegScore{6.937}{(5.505--8.669)}{4.55pt}{4.82pt}{} & \HoloSegScore{23.37}{(18.65--28.76)}{4.55pt}{4.82pt}{} & \HoloSegScore{3.959}{(3.327--4.752)}{4.55pt}{4.82pt}{} & \HoloSegScore{5.938}{(5.006--7.076)}{4.55pt}{4.82pt}{} & \HoloSegScore{4.553}{(1.444--4.613)}{4.55pt}{4.82pt}{} & \HoloSegScore{4.918}{(3.757--6.341)}{4.55pt}{4.82pt}{} & \HoloSegScore{5.570}{(4.056--7.724)}{4.55pt}{4.82pt}{} \\
\cline{3-11}
 &  &  & \HoloSegMetric{Dice} & \HoloSegScore{0.8503}{(0.8290--0.8691)}{4.55pt}{4.82pt}{} & \HoloSegScore{0.2793}{(0.2579--0.3021)}{4.55pt}{4.82pt}{} & \HoloSegScore{0.7947}{(0.7745--0.8105)}{4.55pt}{4.82pt}{} & \HoloSegScore{0.8186}{(0.7957--0.8375)}{4.55pt}{4.82pt}{} & \HoloSegScore{0.8747}{(0.8594--0.8877)}{4.55pt}{4.82pt}{} & \HoloSegScore{0.8089}{(0.7876--0.8288)}{4.55pt}{4.82pt}{} & \HoloSegScore{0.8231}{(0.7982--0.8424)}{4.55pt}{4.82pt}{} \\*
\softcline{4-11}
 &  & \HoloSegSpan{\makecell[c]{right\\[-0.10ex]adrenal\\[-0.10ex]gland}}{2.04cm}{0.32cm} & \HoloSegMetric{HD95} & \HoloSegScore{3.409}{(2.992--3.980)}{4.55pt}{4.82pt}{} & \HoloSegScore{22.64}{(16.34--29.55)}{4.55pt}{4.82pt}{} & \HoloSegScore{2.093}{(1.863--2.382)}{4.55pt}{4.82pt}{} & \HoloSegScore{3.114}{(2.583--3.729)}{4.55pt}{4.82pt}{} & \HoloSegScore{4.608}{(3.277--5.360)}{4.55pt}{4.82pt}{} & \HoloSegScore{10.92}{(3.328--20.61)}{4.55pt}{4.82pt}{} & \HoloSegScore{3.443}{(2.537--4.523)}{4.55pt}{4.82pt}{} \\
\cline{3-11}
 &  &  & \HoloSegMetric{Dice} & \HoloSegScore{0.8603}{(0.8397--0.8788)}{4.55pt}{4.82pt}{} & \HoloSegScore{0.2709}{(0.2462--0.2930)}{4.55pt}{4.82pt}{} & \HoloSegScore{0.8054}{(0.7869--0.8221)}{4.55pt}{4.82pt}{} & \HoloSegScore{0.8278}{(0.8064--0.8468)}{4.55pt}{4.82pt}{} & \HoloSegScore{0.8650}{(0.8467--0.8918)}{4.55pt}{4.82pt}{} & \HoloSegScore{0.8345}{(0.8134--0.8537)}{4.55pt}{4.82pt}{} & \HoloSegScore{0.8290}{(0.8077--0.8482)}{4.55pt}{4.82pt}{} \\*
\softcline{4-11}
 &  & \HoloSegSpan{\makecell[c]{left adrenal\\[-0.10ex]gland}}{2.04cm}{0.32cm} & \HoloSegMetric{HD95} & \HoloSegScore{3.493}{(3.067--4.006)}{4.55pt}{4.82pt}{} & \HoloSegScore{30.63}{(22.70--39.61)}{4.55pt}{4.82pt}{} & \HoloSegScore{2.186}{(1.901--2.598)}{4.55pt}{4.82pt}{} & \HoloSegScore{3.010}{(2.612--3.441)}{4.55pt}{4.82pt}{} & \HoloSegScore{2.184}{(1.826--2.352)}{4.55pt}{4.82pt}{} & \HoloSegScore{6.072}{(2.203--13.64)}{4.55pt}{4.82pt}{} & \HoloSegScore{5.112}{(3.465--7.134)}{4.55pt}{4.82pt}{} \\
\cline{3-11}
 &  &  & \HoloSegMetric{Dice} & \HoloSegScore{0.9396}{(0.9293--0.9498)}{4.55pt}{4.82pt}{} & \HoloSegScore{0.6772}{(0.6416--0.7147)}{4.55pt}{4.82pt}{} & \HoloSegScore{0.9204}{(0.9070--0.9322)}{4.55pt}{4.82pt}{} & \HoloSegScore{0.9306}{(0.9180--0.9431)}{4.55pt}{4.82pt}{} & \HoloSegScore{0.9387}{(0.9315--0.9586)}{4.55pt}{4.82pt}{} & \HoloSegScore{0.9163}{(0.9023--0.9291)}{4.55pt}{4.82pt}{} & \HoloSegScore{0.9148}{(0.9013--0.9267)}{4.55pt}{4.82pt}{} \\*
\softcline{4-11}
 &  & \HoloSegSpan{\makecell[c]{left lung\\[-0.10ex]upper lobe}}{2.04cm}{0.32cm} & \HoloSegMetric{HD95} & \HoloSegScore{8.872}{(6.606--11.73)}{4.55pt}{4.82pt}{} & \HoloSegScore{27.11}{(22.96--31.53)}{4.55pt}{4.82pt}{} & \HoloSegScore{7.215}{(5.484--9.370)}{4.55pt}{4.82pt}{} & \HoloSegScore{9.149}{(7.246--11.80)}{4.55pt}{4.82pt}{} & \HoloSegScore{10.49}{(7.197--12.85)}{4.55pt}{4.82pt}{} & \HoloSegScore{24.51}{(21.43--27.73)}{4.55pt}{4.82pt}{} & \HoloSegScore{9.551}{(7.918--11.59)}{4.55pt}{4.82pt}{} \\
\cline{3-11}
 &  &  & \HoloSegMetric{Dice} & \HoloSegScore{0.9261}{(0.9074--0.9428)}{4.55pt}{4.82pt}{} & \HoloSegScore{0.7189}{(0.6870--0.7484)}{4.55pt}{4.82pt}{} & \HoloSegScore{0.9102}{(0.8907--0.9276)}{4.55pt}{4.82pt}{} & \HoloSegScore{0.9160}{(0.8952--0.9340)}{4.55pt}{4.82pt}{} & \HoloSegScore{0.9504}{(0.9302--0.9557)}{4.55pt}{4.82pt}{} & \HoloSegScore{0.8837}{(0.8594--0.9063)}{4.55pt}{4.82pt}{} & \HoloSegScore{0.9028}{(0.8817--0.9223)}{4.55pt}{4.82pt}{} \\*
\softcline{4-11}
 &  & \HoloSegSpan{\makecell[c]{left lung\\[-0.10ex]lower lobe}}{2.04cm}{0.32cm} & \HoloSegMetric{HD95} & \HoloSegScore{6.129}{(5.054--7.231)}{4.55pt}{4.82pt}{} & \HoloSegScore{30.15}{(25.44--35.55)}{4.55pt}{4.82pt}{} & \HoloSegScore{5.131}{(4.369--5.995)}{4.55pt}{4.82pt}{} & \HoloSegScore{7.252}{(6.103--8.605)}{4.55pt}{4.82pt}{} & \HoloSegScore{3.846}{(2.143--5.269)}{4.55pt}{4.82pt}{} & \HoloSegScore{24.01}{(20.34--28.03)}{4.55pt}{4.82pt}{} & \HoloSegScore{14.07}{(9.883--19.30)}{4.55pt}{4.82pt}{} \\
\cline{3-11}
 &  &  & \HoloSegMetric{Dice} & \HoloSegScore{0.8703}{(0.8337--0.8997)}{4.55pt}{4.82pt}{} & \HoloSegScore{0.6295}{(0.5833--0.6744)}{4.55pt}{4.82pt}{} & \HoloSegScore{0.8485}{(0.8095--0.8832)}{4.55pt}{4.82pt}{} & \HoloSegScore{0.8492}{(0.8088--0.8903)}{4.55pt}{4.82pt}{} & \HoloSegScore{0.9158}{(0.8830--0.9362)}{4.55pt}{4.82pt}{} & \HoloSegScore{0.8290}{(0.7874--0.8709)}{4.55pt}{4.82pt}{} & \HoloSegScore{0.8297}{(0.7884--0.8703)}{4.55pt}{4.82pt}{} \\*
\softcline{4-11}
\HoloSegSpan{\makecell[c]{\textbf{Internal}}}{1.20cm}{0.32cm} & \HoloSegSpan{\makecell[c]{Total-\\[-0.10ex]SegmentatorV2}}{1.86cm}{0.32cm} & \HoloSegSpan{\makecell[c]{right lung\\[-0.10ex]upper lobe}}{2.04cm}{0.32cm} & \HoloSegMetric{HD95} & \HoloSegScore{14.71}{(9.192--21.21)}{4.55pt}{4.82pt}{} & \HoloSegScore{38.67}{(32.10--46.07)}{4.55pt}{4.82pt}{} & \HoloSegScore{6.893}{(5.135--9.001)}{4.55pt}{4.82pt}{} & \HoloSegScore{8.079}{(6.242--10.52)}{4.55pt}{4.82pt}{} & \HoloSegScore{4.145}{(2.326--5.878)}{4.55pt}{4.82pt}{} & \HoloSegScore{20.26}{(15.20--26.26)}{4.55pt}{4.82pt}{} & \HoloSegScore{21.97}{(15.86--28.74)}{4.55pt}{4.82pt}{} \\
\cline{3-11}
 &  &  & \HoloSegMetric{Dice} & \HoloSegScore{0.9037}{(0.8802--0.9232)}{4.55pt}{4.82pt}{} & \HoloSegScore{0.5085}{(0.4650--0.5499)}{4.55pt}{4.82pt}{} & \HoloSegScore{0.8648}{(0.8353--0.8906)}{4.55pt}{4.82pt}{} & \HoloSegScore{0.8839}{(0.8581--0.9049)}{4.55pt}{4.82pt}{} & \HoloSegScore{0.9423}{(0.9115--0.9709)}{4.55pt}{4.82pt}{} & \HoloSegScore{0.8320}{(0.8025--0.8578)}{4.55pt}{4.82pt}{} & \HoloSegScore{0.8364}{(0.8075--0.8610)}{4.55pt}{4.82pt}{} \\*
\softcline{4-11}
 &  & \HoloSegSpan{\makecell[c]{right lung\\[-0.10ex]middle lobe}}{2.04cm}{0.32cm} & \HoloSegMetric{HD95} & \HoloSegScore{16.06}{(7.463--30.13)}{4.55pt}{4.82pt}{} & \HoloSegScore{33.14}{(27.46--39.37)}{4.55pt}{4.82pt}{} & \HoloSegScore{7.163}{(5.844--8.795)}{4.55pt}{4.82pt}{} & \HoloSegScore{8.752}{(7.440--10.46)}{4.55pt}{4.82pt}{} & \HoloSegScore{4.376}{(2.266--6.330)}{4.55pt}{4.82pt}{} & \HoloSegScore{14.59}{(12.22--17.51)}{4.55pt}{4.82pt}{} & \HoloSegScore{13.97}{(11.33--17.55)}{4.55pt}{4.82pt}{} \\
\cline{3-11}
 &  &  & \HoloSegMetric{Dice} & \HoloSegScore{0.9293}{(0.9097--0.9464)}{4.55pt}{4.82pt}{} & \HoloSegScore{0.7127}{(0.6785--0.7443)}{4.55pt}{4.82pt}{} & \HoloSegScore{0.9050}{(0.8811--0.9257)}{4.55pt}{4.82pt}{} & \HoloSegScore{0.9164}{(0.8908--0.9367)}{4.55pt}{4.82pt}{} & \HoloSegScore{0.9547}{(0.9353--0.9744)}{4.55pt}{4.82pt}{} & \HoloSegScore{0.8932}{(0.8684--0.9141)}{4.55pt}{4.82pt}{} & \HoloSegScore{0.8932}{(0.8694--0.9136)}{4.55pt}{4.82pt}{} \\*
\softcline{4-11}
 &  & \HoloSegSpan{\makecell[c]{right lung\\[-0.10ex]lower lobe}}{2.04cm}{0.32cm} & \HoloSegMetric{HD95} & \HoloSegScore{13.94}{(5.646--28.32)}{4.55pt}{4.82pt}{} & \HoloSegScore{28.31}{(23.68--33.07)}{4.55pt}{4.82pt}{} & \HoloSegScore{5.976}{(5.049--6.978)}{4.55pt}{4.82pt}{} & \HoloSegScore{6.604}{(5.380--7.986)}{4.55pt}{4.82pt}{} & \HoloSegScore{6.800}{(4.668--9.140)}{4.55pt}{4.82pt}{} & \HoloSegScore{25.04}{(22.59--27.54)}{4.55pt}{4.82pt}{} & \HoloSegScore{13.96}{(11.86--16.27)}{4.55pt}{4.82pt}{} \\
\cline{3-11}
 &  &  & \HoloSegMetric{Dice} & \HoloSegScore{0.8906}{(0.8756--0.9022)}{4.55pt}{4.82pt}{} & \HoloSegScore{0.5364}{(0.5143--0.5556)}{4.55pt}{4.82pt}{} & \HoloSegScore{0.8684}{(0.8543--0.8791)}{4.55pt}{4.82pt}{} & \HoloSegScore{0.8650}{(0.8532--0.8754)}{4.55pt}{4.82pt}{} & \HoloSegScore{0.9172}{(0.8927--0.9256)}{4.55pt}{4.82pt}{} & \HoloSegScore{0.8738}{(0.8605--0.8852)}{4.55pt}{4.82pt}{} & \HoloSegScore{0.8730}{(0.8592--0.8840)}{4.55pt}{4.82pt}{} \\*
\softcline{4-11}
 &  & \HoloSegSpan{\makecell[c]{esophagus}}{2.04cm}{0.32cm} & \HoloSegMetric{HD95} & \HoloSegScore{15.36}{(8.887--23.35)}{4.55pt}{4.82pt}{} & \HoloSegScore{10.89}{(9.337--12.77)}{4.55pt}{4.82pt}{} & \HoloSegScore{2.292}{(2.090--2.540)}{4.55pt}{4.82pt}{} & \HoloSegScore{2.707}{(2.405--3.060)}{4.55pt}{4.82pt}{} & \HoloSegScore{3.253}{(1.603--4.305)}{4.55pt}{4.82pt}{} & \HoloSegScore{3.327}{(2.442--4.686)}{4.55pt}{4.82pt}{} & \HoloSegScore{2.635}{(2.373--2.939)}{4.55pt}{4.82pt}{} \\
\cline{3-11}
 &  &  & \HoloSegMetric{Dice} & \HoloSegScore{0.9275}{(0.9200--0.9342)}{4.55pt}{4.82pt}{} & \HoloSegScore{0.6449}{(0.6188--0.6711)}{4.55pt}{4.82pt}{} & \HoloSegScore{0.9048}{(0.8938--0.9138)}{4.55pt}{4.82pt}{} & \HoloSegScore{0.9395}{(0.9305--0.9466)}{4.55pt}{4.82pt}{} & \HoloSegScore{0.9434}{(0.9333--0.9472)}{4.55pt}{4.82pt}{} & \HoloSegScore{0.9135}{(0.9017--0.9233)}{4.55pt}{4.82pt}{} & \HoloSegScore{0.9096}{(0.8999--0.9178)}{4.55pt}{4.82pt}{} \\*
\softcline{4-11}
 &  & \HoloSegSpan{\makecell[c]{trachea}}{2.04cm}{0.32cm} & \HoloSegMetric{HD95} & \HoloSegScore{4.196}{(3.270--5.272)}{4.55pt}{4.82pt}{} & \HoloSegScore{12.07}{(10.52--13.95)}{4.55pt}{4.82pt}{} & \HoloSegScore{4.798}{(3.238--6.581)}{4.55pt}{4.82pt}{} & \HoloSegScore{4.647}{(2.915--6.988)}{4.55pt}{4.82pt}{} & \HoloSegScore{4.848}{(4.054--5.435)}{4.55pt}{4.82pt}{} & \HoloSegScore{10.22}{(7.917--12.51)}{4.55pt}{4.82pt}{} & \HoloSegScore{7.672}{(5.998--9.512)}{4.55pt}{4.82pt}{} \\
\cline{3-11}
 &  &  & \HoloSegMetric{Dice} & \HoloSegScore{0.8486}{(0.8265--0.8667)}{4.55pt}{4.82pt}{} & \HoloSegScore{0.0000}{(0.0000--0.0000)}{4.55pt}{4.82pt}{} & \HoloSegScore{0.8315}{(0.8152--0.8465)}{4.55pt}{4.82pt}{} & \HoloSegScore{0.8524}{(0.8328--0.8679)}{4.55pt}{4.82pt}{} & \HoloSegScore{0.8817}{(0.8497--0.8948)}{4.55pt}{4.82pt}{} & \HoloSegScore{0.8555}{(0.8338--0.8730)}{4.55pt}{4.82pt}{} & \HoloSegScore{0.8436}{(0.8243--0.8606)}{4.55pt}{4.82pt}{} \\*
\softcline{4-11}
 &  & \HoloSegSpan{\makecell[c]{thyroid\\[-0.10ex]gland}}{2.04cm}{0.32cm} & \HoloSegMetric{HD95} & \HoloSegScore{4.314}{(3.850--4.876)}{4.55pt}{4.82pt}{} & \HoloSegScore{215.6}{(201.2--229.6)}{4.55pt}{4.82pt}{} & \HoloSegScore{3.028}{(2.506--3.784)}{4.55pt}{4.82pt}{} & \HoloSegScore{2.916}{(2.584--3.240)}{4.55pt}{4.82pt}{} & \HoloSegScore{4.421}{(4.421--5.321)}{4.55pt}{4.82pt}{} & \HoloSegScore{2.647}{(2.246--3.131)}{4.55pt}{4.82pt}{} & \HoloSegScore{5.460}{(3.077--9.717)}{4.55pt}{4.82pt}{} \\
\cline{3-11}
 &  &  & \HoloSegMetric{Dice} & \HoloSegScore{0.8176}{(0.7922--0.8417)}{4.55pt}{4.82pt}{} & \HoloSegScore{0.5136}{(0.4828--0.5463)}{4.55pt}{4.82pt}{} & \HoloSegScore{0.8294}{(0.8061--0.8501)}{4.55pt}{4.82pt}{} & \HoloSegScore{0.8030}{(0.7739--0.8320)}{4.55pt}{4.82pt}{} & \HoloSegScore{0.8649}{(0.8367--0.9015)}{4.55pt}{4.82pt}{} & \HoloSegScore{0.8168}{(0.7859--0.8412)}{4.55pt}{4.82pt}{} & \HoloSegScore{0.8181}{(0.7891--0.8416)}{4.55pt}{4.82pt}{} \\*
\softcline{4-11}
 &  & \HoloSegSpan{\makecell[c]{small bowel}}{2.04cm}{0.32cm} & \HoloSegMetric{HD95} & \HoloSegScore{16.68}{(11.24--22.78)}{4.55pt}{4.82pt}{} & \HoloSegScore{29.45}{(23.56--37.83)}{4.55pt}{4.82pt}{} & \HoloSegScore{8.517}{(7.119--10.11)}{4.55pt}{4.82pt}{} & \HoloSegScore{12.66}{(10.47--15.48)}{4.55pt}{4.82pt}{} & \HoloSegScore{7.870}{(6.470--9.740)}{4.55pt}{4.82pt}{} & \HoloSegScore{20.48}{(13.54--28.48)}{4.55pt}{4.82pt}{} & \HoloSegScore{15.99}{(9.938--23.66)}{4.55pt}{4.82pt}{} \\
\cline{3-11}
 &  &  & \HoloSegMetric{Dice} & \HoloSegScore{0.8087}{(0.7854--0.8304)}{4.55pt}{4.82pt}{} & \HoloSegScore{0.4202}{(0.3898--0.4499)}{4.55pt}{4.82pt}{} & \HoloSegScore{0.8003}{(0.7762--0.8211)}{4.55pt}{4.82pt}{} & \HoloSegScore{0.7696}{(0.7389--0.7964)}{4.55pt}{4.82pt}{} & \HoloSegScore{0.8076}{(0.7998--0.8081)}{4.55pt}{4.82pt}{} & \HoloSegScore{0.7698}{(0.7439--0.7939)}{4.55pt}{4.82pt}{} & \HoloSegScore{0.7797}{(0.7559--0.8027)}{4.55pt}{4.82pt}{} \\*
\softcline{4-11}
 &  & \HoloSegSpan{\makecell[c]{duodenum}}{2.04cm}{0.32cm} & \HoloSegMetric{HD95} & \HoloSegScore{9.475}{(7.470--12.11)}{4.55pt}{4.82pt}{} & \HoloSegScore{30.06}{(24.28--36.83)}{4.55pt}{4.82pt}{} & \HoloSegScore{9.347}{(5.518--14.95)}{4.55pt}{4.82pt}{} & \HoloSegScore{10.93}{(8.443--13.77)}{4.55pt}{4.82pt}{} & \HoloSegScore{10.27}{(7.463--14.29)}{4.55pt}{4.82pt}{} & \HoloSegScore{10.17}{(8.252--12.75)}{4.55pt}{4.82pt}{} & \HoloSegScore{9.418}{(7.678--11.86)}{4.55pt}{4.82pt}{} \\
\cline{3-11}
 &  &  & \HoloSegMetric{Dice} & \HoloSegScore{0.8827}{(0.8696--0.8932)}{4.55pt}{4.82pt}{} & \HoloSegScore{0.5392}{(0.5115--0.5653)}{4.55pt}{4.82pt}{} & \HoloSegScore{0.8624}{(0.8510--0.8726)}{4.55pt}{4.82pt}{} & \HoloSegScore{0.8482}{(0.8359--0.8597)}{4.55pt}{4.82pt}{} & \HoloSegScore{0.8770}{(0.8727--0.9047)}{4.55pt}{4.82pt}{} & \HoloSegScore{0.8386}{(0.8211--0.8544)}{4.55pt}{4.82pt}{} & \HoloSegScore{0.8562}{(0.8447--0.8665)}{4.55pt}{4.82pt}{} \\*
\softcline{4-11}
 &  & \HoloSegSpan{\makecell[c]{colon}}{2.04cm}{0.32cm} & \HoloSegMetric{HD95} & \HoloSegScore{15.74}{(11.10--22.29)}{4.55pt}{4.82pt}{} & \HoloSegScore{33.11}{(27.21--40.25)}{4.55pt}{4.82pt}{} & \HoloSegScore{14.61}{(7.962--26.42)}{4.55pt}{4.82pt}{} & \HoloSegScore{18.67}{(14.87--24.06)}{4.55pt}{4.82pt}{} & \HoloSegScore{14.30}{(9.280--21.50)}{4.55pt}{4.82pt}{} & \HoloSegScore{28.44}{(19.64--38.74)}{4.55pt}{4.82pt}{} & \HoloSegScore{23.79}{(15.37--35.11)}{4.55pt}{4.82pt}{} \\
\cline{3-11}
 &  &  & \HoloSegMetric{Dice} & \HoloSegScore{0.8851}{(0.8568--0.9071)}{4.55pt}{4.82pt}{} & \HoloSegScore{0.5290}{(0.4812--0.5779)}{4.55pt}{4.82pt}{} & \HoloSegScore{0.8839}{(0.8590--0.9061)}{4.55pt}{4.82pt}{} & \HoloSegScore{0.8838}{(0.8506--0.9070)}{4.55pt}{4.82pt}{} & \HoloSegScore{0.9019}{(0.8731--0.9371)}{4.55pt}{4.82pt}{} & \HoloSegScore{0.8739}{(0.8437--0.8974)}{4.55pt}{4.82pt}{} & \HoloSegScore{0.8900}{(0.8621--0.9104)}{4.55pt}{4.82pt}{} \\*
\softcline{4-11}
 &  & \HoloSegSpan{\makecell[c]{urinary\\[-0.10ex]bladder}}{2.04cm}{0.32cm} & \HoloSegMetric{HD95} & \HoloSegScore{49.39}{(28.46--74.91)}{4.55pt}{4.82pt}{} & \HoloSegScore{35.81}{(26.00--46.56)}{4.55pt}{4.82pt}{} & \HoloSegScore{8.932}{(4.121--17.69)}{4.55pt}{4.82pt}{} & \HoloSegScore{6.262}{(5.064--7.712)}{4.55pt}{4.82pt}{} & \HoloSegScore{7.030}{(5.279--9.140)}{4.55pt}{4.82pt}{} & \HoloSegScore{9.550}{(6.288--13.43)}{4.55pt}{4.82pt}{} & \HoloSegScore{7.924}{(5.331--11.28)}{4.55pt}{4.82pt}{} \\
\hline
\pagebreak[4]
 &  &  & \HoloSegMetric{Dice} & \HoloSegScore{0.7170}{(0.6548--0.7757)}{4.55pt}{4.82pt}{} & \HoloSegScore{0.1789}{(0.1333--0.2293)}{4.55pt}{4.82pt}{} & \HoloSegScore{0.7621}{(0.6851--0.8319)}{4.55pt}{4.82pt}{} & \HoloSegScore{0.7330}{(0.6600--0.7933)}{4.55pt}{4.82pt}{} & \HoloSegScore{0.7486}{(0.6963--0.8186)}{4.55pt}{4.82pt}{} & \HoloSegScore{0.7427}{(0.6752--0.8011)}{4.55pt}{4.82pt}{} & \HoloSegScore{0.7255}{(0.6623--0.7831)}{4.55pt}{4.82pt}{} \\*
\softcline{4-11}
 &  & \HoloSegSpan{\makecell[c]{prostate}}{2.04cm}{0.32cm} & \HoloSegMetric{HD95} & \HoloSegScore{22.65}{(18.30--27.44)}{4.55pt}{4.82pt}{} & \HoloSegScore{50.83}{(41.34--60.90)}{4.55pt}{4.82pt}{} & \HoloSegScore{5.539}{(3.876--7.526)}{4.55pt}{4.82pt}{} & \HoloSegScore{5.944}{(4.733--7.368)}{4.55pt}{4.82pt}{} & \HoloSegScore{8.427}{(7.057--9.650)}{4.55pt}{4.82pt}{} & \HoloSegScore{20.06}{(9.117--34.89)}{4.55pt}{4.82pt}{} & \HoloSegScore{71.86}{(46.64--100.8)}{4.55pt}{4.82pt}{} \\
\cline{3-11}
 &  &  & \HoloSegMetric{Dice} & \HoloSegScore{0.6743}{(0.4239--0.8632)}{4.55pt}{4.82pt}{} & \HoloSegScore{0.1251}{(0.01252--0.2704)}{4.20pt}{4.48pt}{} & \HoloSegScore{0.8678}{(0.8259--0.8992)}{4.55pt}{4.82pt}{} & \HoloSegScore{0.0000}{(0.0000--0.0000)}{4.55pt}{4.82pt}{} & \HoloSegScore{0.8544}{(0.8083--0.8807)}{4.55pt}{4.82pt}{} & \HoloSegScore{0.9079}{(0.8712--0.9380)}{4.55pt}{4.82pt}{} & \HoloSegScore{0.8763}{(0.8345--0.9168)}{4.55pt}{4.82pt}{} \\*
\softcline{4-11}
 &  & \HoloSegSpan{\makecell[c]{left kidney\\[-0.10ex]cyst}}{2.04cm}{0.32cm} & \HoloSegMetric{HD95} & \HoloSegScore{56.57}{(5.137--152.9)}{4.55pt}{4.82pt}{} & \HoloSegScore{71.05}{(47.56--90.74)}{4.55pt}{4.82pt}{} & \HoloSegScore{68.36}{(18.89--122.3)}{4.55pt}{4.82pt}{} & \HoloSegScore{--}{(--\,--)}{4.55pt}{4.82pt}{} & \HoloSegScore{5.811}{(3.895--7.440)}{4.55pt}{4.82pt}{} & \HoloSegScore{41.05}{(2.765--96.98)}{4.55pt}{4.82pt}{} & \HoloSegScore{21.44}{(4.177--52.10)}{4.55pt}{4.82pt}{} \\
\cline{3-11}
 &  &  & \HoloSegMetric{Dice} & \HoloSegScore{0.5917}{(0.3232--0.7966)}{4.55pt}{4.82pt}{} & \HoloSegScore{0.1737}{(0.0000--0.3921)}{4.55pt}{4.82pt}{} & \HoloSegScore{0.8106}{(0.7687--0.8515)}{4.55pt}{4.82pt}{} & \HoloSegScore{0.0000}{(0.0000--0.0000)}{4.55pt}{4.82pt}{} & \HoloSegScore{0.8449}{(0.8440--0.8484)}{4.55pt}{4.82pt}{} & \HoloSegScore{0.7168}{(0.4366--0.8904)}{4.55pt}{4.82pt}{} & \HoloSegScore{0.7062}{(0.4024--0.8871)}{4.55pt}{4.82pt}{} \\*
\softcline{4-11}
 &  & \HoloSegSpan{\makecell[c]{right kidney\\[-0.10ex]cyst}}{2.04cm}{0.32cm} & \HoloSegMetric{HD95} & \HoloSegScore{48.20}{(7.517--126.9)}{4.55pt}{4.82pt}{} & \HoloSegScore{58.37}{(27.66--94.05)}{4.55pt}{4.82pt}{} & \HoloSegScore{4.709}{(3.132--6.527)}{4.55pt}{4.82pt}{} & \HoloSegScore{--}{(--\,--)}{4.55pt}{4.82pt}{} & \HoloSegScore{4.541}{(2.121--6.424)}{4.55pt}{4.82pt}{} & \HoloSegScore{11.97}{(5.290--21.72)}{4.55pt}{4.82pt}{} & \HoloSegScore{4.819}{(3.371--6.919)}{4.55pt}{4.82pt}{} \\
\cline{3-11}
 &  &  & \HoloSegMetric{Dice} & \HoloSegScore{0.8684}{(0.8401--0.8901)}{4.55pt}{4.82pt}{} & \HoloSegScore{0.5202}{(0.4930--0.5450)}{4.55pt}{4.82pt}{} & \HoloSegScore{0.8049}{(0.7858--0.8192)}{4.55pt}{4.82pt}{} & \HoloSegScore{0.8985}{(0.8787--0.9133)}{4.55pt}{4.82pt}{} & \HoloSegScore{0.9345}{(0.9324--0.9516)}{4.55pt}{4.82pt}{} & \HoloSegScore{0.8756}{(0.8451--0.8992)}{4.55pt}{4.82pt}{} & \HoloSegScore{0.8927}{(0.8710--0.9084)}{4.55pt}{4.82pt}{} \\*
\softcline{4-11}
 &  & \HoloSegSpan{\makecell[c]{sacrum}}{2.04cm}{0.32cm} & \HoloSegMetric{HD95} & \HoloSegScore{21.91}{(17.93--25.66)}{4.55pt}{4.82pt}{} & \HoloSegScore{16.04}{(13.25--19.39)}{4.55pt}{4.82pt}{} & \HoloSegScore{18.88}{(7.670--37.37)}{4.55pt}{4.82pt}{} & \HoloSegScore{6.703}{(5.313--8.410)}{4.55pt}{4.82pt}{} & \HoloSegScore{3.533}{(1.258--6.300)}{4.55pt}{4.82pt}{} & \HoloSegScore{81.49}{(51.69--110.1)}{4.55pt}{4.82pt}{} & \HoloSegScore{14.30}{(5.737--30.27)}{4.55pt}{4.82pt}{} \\
\cline{3-11}
 &  &  & \HoloSegMetric{Dice} & \HoloSegScore{0.8861}{(0.8585--0.9092)}{4.55pt}{4.82pt}{} & \HoloSegScore{0.01010}{(0.002950--0.01869)}{3.85pt}{4.12pt}{} & \HoloSegScore{0.8742}{(0.8446--0.8974)}{4.55pt}{4.82pt}{} & \HoloSegScore{0.8548}{(0.8279--0.8756)}{4.55pt}{4.82pt}{} & \HoloSegScore{0.9076}{(0.8774--0.9197)}{4.55pt}{4.82pt}{} & \HoloSegScore{0.8280}{(0.7950--0.8552)}{4.55pt}{4.82pt}{} & \HoloSegScore{0.8540}{(0.8221--0.8806)}{4.55pt}{4.82pt}{} \\*
\softcline{4-11}
 &  & \HoloSegSpan{\makecell[c]{sacral\\[-0.10ex]vertebrae 1\\[-0.10ex](s1)}}{2.04cm}{0.32cm} & \HoloSegMetric{HD95} & \HoloSegScore{66.00}{(38.72--98.64)}{4.55pt}{4.82pt}{} & \HoloSegScore{61.98}{(56.12--70.77)}{4.55pt}{4.82pt}{} & \HoloSegScore{9.882}{(2.528--21.13)}{4.55pt}{4.82pt}{} & \HoloSegScore{6.009}{(5.073--7.164)}{4.55pt}{4.82pt}{} & \HoloSegScore{6.168}{(4.305--7.560)}{4.55pt}{4.82pt}{} & \HoloSegScore{72.40}{(46.20--99.45)}{4.55pt}{4.82pt}{} & \HoloSegScore{9.667}{(4.957--18.44)}{4.55pt}{4.82pt}{} \\
\cline{3-11}
 &  &  & \HoloSegMetric{Dice} & \HoloSegScore{0.9017}{(0.8668--0.9304)}{4.55pt}{4.82pt}{} & \HoloSegScore{0.1649}{(0.1275--0.2005)}{4.55pt}{4.82pt}{} & \HoloSegScore{0.8837}{(0.8516--0.9100)}{4.55pt}{4.82pt}{} & \HoloSegScore{0.9142}{(0.8821--0.9408)}{4.55pt}{4.82pt}{} & \HoloSegScore{0.9341}{(0.9132--0.9660)}{4.55pt}{4.82pt}{} & \HoloSegScore{0.9096}{(0.8788--0.9348)}{4.55pt}{4.82pt}{} & \HoloSegScore{0.9097}{(0.8795--0.9332)}{4.55pt}{4.82pt}{} \\*
\softcline{4-11}
 &  & \HoloSegSpan{\makecell[c]{lumbar\\[-0.10ex]vertebrae 5\\[-0.10ex](l5)}}{2.04cm}{0.32cm} & \HoloSegMetric{HD95} & \HoloSegScore{16.81}{(4.933--35.50)}{4.55pt}{4.82pt}{} & \HoloSegScore{37.64}{(34.33--40.83)}{4.55pt}{4.82pt}{} & \HoloSegScore{22.79}{(9.069--40.23)}{4.55pt}{4.82pt}{} & \HoloSegScore{4.696}{(3.315--6.248)}{4.55pt}{4.82pt}{} & \HoloSegScore{2.850}{(1.119--4.014)}{4.55pt}{4.82pt}{} & \HoloSegScore{12.93}{(6.979--20.51)}{4.55pt}{4.82pt}{} & \HoloSegScore{4.655}{(3.465--6.098)}{4.55pt}{4.82pt}{} \\
\cline{3-11}
 &  &  & \HoloSegMetric{Dice} & \HoloSegScore{0.8570}{(0.8161--0.8918)}{4.55pt}{4.82pt}{} & \HoloSegScore{0.3136}{(0.2731--0.3571)}{4.55pt}{4.82pt}{} & \HoloSegScore{0.8746}{(0.8410--0.9032)}{4.55pt}{4.82pt}{} & \HoloSegScore{0.9053}{(0.8665--0.9380)}{4.55pt}{4.82pt}{} & \HoloSegScore{0.9328}{(0.8959--0.9800)}{4.55pt}{4.82pt}{} & \HoloSegScore{0.8487}{(0.8129--0.8802)}{4.55pt}{4.82pt}{} & \HoloSegScore{0.9011}{(0.8684--0.9292)}{4.55pt}{4.82pt}{} \\*
\softcline{4-11}
 &  & \HoloSegSpan{\makecell[c]{lumbar\\[-0.10ex]vertebrae 4\\[-0.10ex](l4)}}{2.04cm}{0.32cm} & \HoloSegMetric{HD95} & \HoloSegScore{19.39}{(16.04--22.81)}{4.55pt}{4.82pt}{} & \HoloSegScore{31.03}{(25.41--38.56)}{4.55pt}{4.82pt}{} & \HoloSegScore{38.13}{(21.16--60.28)}{4.55pt}{4.82pt}{} & \HoloSegScore{4.183}{(2.950--5.630)}{4.55pt}{4.82pt}{} & \HoloSegScore{2.594}{(1.176--3.897)}{4.55pt}{4.82pt}{} & \HoloSegScore{47.39}{(29.38--68.16)}{4.55pt}{4.82pt}{} & \HoloSegScore{4.785}{(3.288--6.810)}{4.55pt}{4.82pt}{} \\
\cline{3-11}
 &  &  & \HoloSegMetric{Dice} & \HoloSegScore{0.9124}{(0.8848--0.9353)}{4.55pt}{4.82pt}{} & \HoloSegScore{0.3852}{(0.3450--0.4255)}{4.55pt}{4.82pt}{} & \HoloSegScore{0.8955}{(0.8711--0.9147)}{4.55pt}{4.82pt}{} & \HoloSegScore{0.9193}{(0.8898--0.9447)}{4.55pt}{4.82pt}{} & \HoloSegScore{0.9297}{(0.9173--0.9570)}{4.55pt}{4.82pt}{} & \HoloSegScore{0.8855}{(0.8522--0.9149)}{4.55pt}{4.82pt}{} & \HoloSegScore{0.9058}{(0.8766--0.9291)}{4.55pt}{4.82pt}{} \\*
\softcline{4-11}
 &  & \HoloSegSpan{\makecell[c]{lumbar\\[-0.10ex]vertebrae 3\\[-0.10ex](l3)}}{2.04cm}{0.32cm} & \HoloSegMetric{HD95} & \HoloSegScore{18.08}{(6.349--35.85)}{4.55pt}{4.82pt}{} & \HoloSegScore{29.26}{(21.89--38.65)}{4.55pt}{4.82pt}{} & \HoloSegScore{15.55}{(4.717--28.72)}{4.55pt}{4.82pt}{} & \HoloSegScore{2.899}{(2.219--3.803)}{4.55pt}{4.82pt}{} & \HoloSegScore{3.219}{(3.007--4.017)}{4.55pt}{4.82pt}{} & \HoloSegScore{20.86}{(13.03--29.76)}{4.55pt}{4.82pt}{} & \HoloSegScore{7.629}{(5.062--11.33)}{4.55pt}{4.82pt}{} \\
\cline{3-11}
 &  &  & \HoloSegMetric{Dice} & \HoloSegScore{0.9256}{(0.9056--0.9425)}{4.55pt}{4.82pt}{} & \HoloSegScore{0.4017}{(0.3715--0.4352)}{4.55pt}{4.82pt}{} & \HoloSegScore{0.9122}{(0.9027--0.9202)}{4.55pt}{4.82pt}{} & \HoloSegScore{0.9427}{(0.9280--0.9548)}{4.55pt}{4.82pt}{} & \HoloSegScore{0.9297}{(0.9106--0.9554)}{4.55pt}{4.82pt}{} & \HoloSegScore{0.8699}{(0.8455--0.8892)}{4.55pt}{4.82pt}{} & \HoloSegScore{0.9362}{(0.9247--0.9461)}{4.55pt}{4.82pt}{} \\*
\softcline{4-11}
 &  & \HoloSegSpan{\makecell[c]{lumbar\\[-0.10ex]vertebrae 2\\[-0.10ex](l2)}}{2.04cm}{0.32cm} & \HoloSegMetric{HD95} & \HoloSegScore{21.63}{(6.402--40.86)}{4.55pt}{4.82pt}{} & \HoloSegScore{24.65}{(20.70--30.59)}{4.55pt}{4.82pt}{} & \HoloSegScore{2.082}{(1.758--2.438)}{4.55pt}{4.82pt}{} & \HoloSegScore{3.447}{(2.552--4.633)}{4.55pt}{4.82pt}{} & \HoloSegScore{2.215}{(2.186--2.587)}{4.55pt}{4.82pt}{} & \HoloSegScore{10.84}{(9.580--12.35)}{4.55pt}{4.82pt}{} & \HoloSegScore{4.079}{(3.026--5.240)}{4.55pt}{4.82pt}{} \\
\cline{3-11}
 &  &  & \HoloSegMetric{Dice} & \HoloSegScore{0.9127}{(0.8865--0.9376)}{4.55pt}{4.82pt}{} & \HoloSegScore{0.1864}{(0.1552--0.2161)}{4.55pt}{4.82pt}{} & \HoloSegScore{0.9061}{(0.8932--0.9174)}{4.55pt}{4.82pt}{} & \HoloSegScore{0.9255}{(0.8993--0.9476)}{4.55pt}{4.82pt}{} & \HoloSegScore{0.9124}{(0.8950--0.9340)}{4.55pt}{4.82pt}{} & \HoloSegScore{0.8953}{(0.8667--0.9190)}{4.55pt}{4.82pt}{} & \HoloSegScore{0.9258}{(0.9025--0.9437)}{4.55pt}{4.82pt}{} \\*
\softcline{4-11}
\HoloSegSpan{\makecell[c]{\textbf{Internal}}}{1.20cm}{0.32cm} & \HoloSegSpan{\makecell[c]{Total-\\[-0.10ex]SegmentatorV2}}{1.86cm}{0.32cm} & \HoloSegSpan{\makecell[c]{lumbar\\[-0.10ex]vertebrae 1\\[-0.10ex](l1)}}{2.04cm}{0.32cm} & \HoloSegMetric{HD95} & \HoloSegScore{4.818}{(3.769--5.910)}{4.55pt}{4.82pt}{} & \HoloSegScore{36.97}{(32.43--42.33)}{4.55pt}{4.82pt}{} & \HoloSegScore{4.661}{(1.858--9.745)}{4.55pt}{4.82pt}{} & \HoloSegScore{3.171}{(2.309--4.191)}{4.55pt}{4.82pt}{} & \HoloSegScore{5.824}{(5.493--6.007)}{4.55pt}{4.82pt}{} & \HoloSegScore{27.06}{(19.02--35.31)}{4.55pt}{4.82pt}{} & \HoloSegScore{7.480}{(3.440--12.65)}{4.55pt}{4.82pt}{} \\
\cline{3-11}
 &  &  & \HoloSegMetric{Dice} & \HoloSegScore{0.8918}{(0.8593--0.9201)}{4.55pt}{4.82pt}{} & \HoloSegScore{0.08564}{(0.06386--0.1105)}{4.20pt}{4.48pt}{} & \HoloSegScore{0.8934}{(0.8703--0.9131)}{4.55pt}{4.82pt}{} & \HoloSegScore{0.9166}{(0.8863--0.9420)}{4.55pt}{4.82pt}{} & \HoloSegScore{0.9108}{(0.8860--0.9306)}{4.55pt}{4.82pt}{} & \HoloSegScore{0.8933}{(0.8686--0.9132)}{4.55pt}{4.82pt}{} & \HoloSegScore{0.9137}{(0.8860--0.9373)}{4.55pt}{4.82pt}{} \\*
\softcline{4-11}
 &  & \HoloSegSpan{\makecell[c]{thoracic\\[-0.10ex]vertebrae 12\\[-0.10ex](t12)}}{2.04cm}{0.32cm} & \HoloSegMetric{HD95} & \HoloSegScore{25.77}{(15.53--36.85)}{4.55pt}{4.82pt}{} & \HoloSegScore{43.82}{(39.77--48.06)}{4.55pt}{4.82pt}{} & \HoloSegScore{12.88}{(4.505--22.98)}{4.55pt}{4.82pt}{} & \HoloSegScore{3.429}{(2.501--4.478)}{4.55pt}{4.82pt}{} & \HoloSegScore{4.629}{(4.603--5.073)}{4.55pt}{4.82pt}{} & \HoloSegScore{9.650}{(7.169--13.39)}{4.55pt}{4.82pt}{} & \HoloSegScore{4.522}{(2.597--8.145)}{4.55pt}{4.82pt}{} \\
\cline{3-11}
 &  &  & \HoloSegMetric{Dice} & \HoloSegScore{0.8896}{(0.8597--0.9177)}{4.55pt}{4.82pt}{} & \HoloSegScore{0.2960}{(0.2605--0.3308)}{4.55pt}{4.82pt}{} & \HoloSegScore{0.8991}{(0.8829--0.9131)}{4.55pt}{4.82pt}{} & \HoloSegScore{0.9238}{(0.8997--0.9428)}{4.55pt}{4.82pt}{} & \HoloSegScore{0.9209}{(0.8847--0.9390)}{4.55pt}{4.82pt}{} & \HoloSegScore{0.8907}{(0.8626--0.9155)}{4.55pt}{4.82pt}{} & \HoloSegScore{0.9241}{(0.9069--0.9379)}{4.55pt}{4.82pt}{} \\*
\softcline{4-11}
 &  & \HoloSegSpan{\makecell[c]{thoracic\\[-0.10ex]vertebrae 11\\[-0.10ex](t11)}}{2.04cm}{0.32cm} & \HoloSegMetric{HD95} & \HoloSegScore{7.373}{(4.878--11.64)}{4.55pt}{4.82pt}{} & \HoloSegScore{30.35}{(27.38--33.61)}{4.55pt}{4.82pt}{} & \HoloSegScore{2.360}{(1.932--2.817)}{4.55pt}{4.82pt}{} & \HoloSegScore{3.148}{(2.421--3.933)}{4.55pt}{4.82pt}{} & \HoloSegScore{2.379}{(2.253--3.302)}{4.55pt}{4.82pt}{} & \HoloSegScore{6.331}{(4.517--8.720)}{4.55pt}{4.82pt}{} & \HoloSegScore{3.653}{(2.798--4.582)}{4.55pt}{4.82pt}{} \\
\cline{3-11}
 &  &  & \HoloSegMetric{Dice} & \HoloSegScore{0.8898}{(0.8607--0.9162)}{4.55pt}{4.82pt}{} & \HoloSegScore{0.4046}{(0.3680--0.4375)}{4.55pt}{4.82pt}{} & \HoloSegScore{0.8905}{(0.8733--0.9060)}{4.55pt}{4.82pt}{} & \HoloSegScore{0.9229}{(0.8996--0.9436)}{4.55pt}{4.82pt}{} & \HoloSegScore{0.9166}{(0.9039--0.9211)}{4.55pt}{4.82pt}{} & \HoloSegScore{0.8634}{(0.8392--0.8842)}{4.55pt}{4.82pt}{} & \HoloSegScore{0.9055}{(0.8864--0.9231)}{4.55pt}{4.82pt}{} \\*
\softcline{4-11}
 &  & \HoloSegSpan{\makecell[c]{thoracic\\[-0.10ex]vertebrae 10\\[-0.10ex](t10)}}{2.04cm}{0.32cm} & \HoloSegMetric{HD95} & \HoloSegScore{5.460}{(4.485--6.663)}{4.55pt}{4.82pt}{} & \HoloSegScore{27.43}{(23.45--32.07)}{4.55pt}{4.82pt}{} & \HoloSegScore{2.313}{(1.892--2.786)}{4.55pt}{4.82pt}{} & \HoloSegScore{3.120}{(2.467--3.891)}{4.55pt}{4.82pt}{} & \HoloSegScore{4.172}{(2.796--5.120)}{4.55pt}{4.82pt}{} & \HoloSegScore{12.74}{(10.99--15.04)}{4.55pt}{4.82pt}{} & \HoloSegScore{6.774}{(5.110--9.103)}{4.55pt}{4.82pt}{} \\
\cline{3-11}
 &  &  & \HoloSegMetric{Dice} & \HoloSegScore{0.8856}{(0.8545--0.9132)}{4.55pt}{4.82pt}{} & \HoloSegScore{0.2593}{(0.2284--0.2892)}{4.55pt}{4.82pt}{} & \HoloSegScore{0.8765}{(0.8577--0.8924)}{4.55pt}{4.82pt}{} & \HoloSegScore{0.9189}{(0.8917--0.9418)}{4.55pt}{4.82pt}{} & \HoloSegScore{0.9160}{(0.8920--0.9329)}{4.55pt}{4.82pt}{} & \HoloSegScore{0.9055}{(0.8889--0.9205)}{4.55pt}{4.82pt}{} & \HoloSegScore{0.9080}{(0.8882--0.9247)}{4.55pt}{4.82pt}{} \\*
\softcline{4-11}
 &  & \HoloSegSpan{\makecell[c]{thoracic\\[-0.10ex]vertebrae 9\\[-0.10ex](t9)}}{2.04cm}{0.32cm} & \HoloSegMetric{HD95} & \HoloSegScore{10.23}{(6.109--15.69)}{4.55pt}{4.82pt}{} & \HoloSegScore{35.17}{(31.02--40.14)}{4.55pt}{4.82pt}{} & \HoloSegScore{2.817}{(2.192--3.485)}{4.55pt}{4.82pt}{} & \HoloSegScore{3.198}{(2.520--3.980)}{4.55pt}{4.82pt}{} & \HoloSegScore{1.981}{(0.5620--2.236)}{4.55pt}{4.82pt}{} & \HoloSegScore{7.350}{(5.874--8.921)}{4.55pt}{4.82pt}{} & \HoloSegScore{5.678}{(4.354--7.152)}{4.55pt}{4.82pt}{} \\
\cline{3-11}
 &  &  & \HoloSegMetric{Dice} & \HoloSegScore{0.8687}{(0.8325--0.8987)}{4.55pt}{4.82pt}{} & \HoloSegScore{0.3180}{(0.2843--0.3527)}{4.55pt}{4.82pt}{} & \HoloSegScore{0.8504}{(0.8240--0.8755)}{4.55pt}{4.82pt}{} & \HoloSegScore{0.8924}{(0.8591--0.9164)}{4.55pt}{4.82pt}{} & \HoloSegScore{0.8977}{(0.8968--0.9432)}{4.55pt}{4.82pt}{} & \HoloSegScore{0.7506}{(0.7005--0.7984)}{4.55pt}{4.82pt}{} & \HoloSegScore{0.8797}{(0.8514--0.9043)}{4.55pt}{4.82pt}{} \\*
\softcline{4-11}
 &  & \HoloSegSpan{\makecell[c]{thoracic\\[-0.10ex]vertebrae 8\\[-0.10ex](t8)}}{2.04cm}{0.32cm} & \HoloSegMetric{HD95} & \HoloSegScore{21.68}{(10.36--36.99)}{4.55pt}{4.82pt}{} & \HoloSegScore{50.74}{(43.02--59.24)}{4.55pt}{4.82pt}{} & \HoloSegScore{2.885}{(2.344--3.546)}{4.55pt}{4.82pt}{} & \HoloSegScore{3.870}{(2.941--5.028)}{4.55pt}{4.82pt}{} & \HoloSegScore{4.166}{(3.285--7.583)}{4.55pt}{4.82pt}{} & \HoloSegScore{8.120}{(6.468--9.970)}{4.55pt}{4.82pt}{} & \HoloSegScore{7.874}{(6.643--9.155)}{4.55pt}{4.82pt}{} \\
\cline{3-11}
 &  &  & \HoloSegMetric{Dice} & \HoloSegScore{0.8440}{(0.8099--0.8763)}{4.55pt}{4.82pt}{} & \HoloSegScore{0.3718}{(0.3310--0.4113)}{4.55pt}{4.82pt}{} & \HoloSegScore{0.8215}{(0.7876--0.8510)}{4.55pt}{4.82pt}{} & \HoloSegScore{0.8420}{(0.8014--0.8815)}{4.55pt}{4.82pt}{} & \HoloSegScore{0.8908}{(0.8665--0.9242)}{4.55pt}{4.82pt}{} & \HoloSegScore{0.7980}{(0.7522--0.8395)}{4.55pt}{4.82pt}{} & \HoloSegScore{0.8427}{(0.8069--0.8773)}{4.55pt}{4.82pt}{} \\*
\softcline{4-11}
 &  & \HoloSegSpan{\makecell[c]{thoracic\\[-0.10ex]vertebrae 7\\[-0.10ex](t7)}}{2.04cm}{0.32cm} & \HoloSegMetric{HD95} & \HoloSegScore{6.841}{(5.543--8.243)}{4.55pt}{4.82pt}{} & \HoloSegScore{32.16}{(25.79--38.78)}{4.55pt}{4.82pt}{} & \HoloSegScore{3.890}{(2.761--5.129)}{4.55pt}{4.82pt}{} & \HoloSegScore{4.317}{(3.329--5.525)}{4.55pt}{4.82pt}{} & \HoloSegScore{3.552}{(2.035--4.949)}{4.55pt}{4.82pt}{} & \HoloSegScore{7.998}{(5.360--12.06)}{4.55pt}{4.82pt}{} & \HoloSegScore{6.014}{(4.862--7.371)}{4.55pt}{4.82pt}{} \\
\cline{3-11}
 &  &  & \HoloSegMetric{Dice} & \HoloSegScore{0.8751}{(0.8448--0.9051)}{4.55pt}{4.82pt}{} & \HoloSegScore{0.4224}{(0.3891--0.4551)}{4.55pt}{4.82pt}{} & \HoloSegScore{0.8438}{(0.8175--0.8671)}{4.55pt}{4.82pt}{} & \HoloSegScore{0.8852}{(0.8528--0.9120)}{4.55pt}{4.82pt}{} & \HoloSegScore{0.8975}{(0.8837--0.9103)}{4.55pt}{4.82pt}{} & \HoloSegScore{0.8336}{(0.8011--0.8642)}{4.55pt}{4.82pt}{} & \HoloSegScore{0.8729}{(0.8497--0.8950)}{4.55pt}{4.82pt}{} \\*
\softcline{4-11}
 &  & \HoloSegSpan{\makecell[c]{thoracic\\[-0.10ex]vertebrae 6\\[-0.10ex](t6)}}{2.04cm}{0.32cm} & \HoloSegMetric{HD95} & \HoloSegScore{5.367}{(4.561--6.349)}{4.55pt}{4.82pt}{} & \HoloSegScore{24.56}{(19.69--30.17)}{4.55pt}{4.82pt}{} & \HoloSegScore{2.766}{(2.272--3.333)}{4.55pt}{4.82pt}{} & \HoloSegScore{3.621}{(2.884--4.401)}{4.55pt}{4.82pt}{} & \HoloSegScore{4.317}{(3.995--6.186)}{4.55pt}{4.82pt}{} & \HoloSegScore{5.229}{(4.116--6.511)}{4.55pt}{4.82pt}{} & \HoloSegScore{5.078}{(3.880--6.405)}{4.55pt}{4.82pt}{} \\
\cline{3-11}
 &  &  & \HoloSegMetric{Dice} & \HoloSegScore{0.8807}{(0.8499--0.9068)}{4.55pt}{4.82pt}{} & \HoloSegScore{0.3973}{(0.3634--0.4311)}{4.55pt}{4.82pt}{} & \HoloSegScore{0.8428}{(0.8143--0.8679)}{4.55pt}{4.82pt}{} & \HoloSegScore{0.8918}{(0.8601--0.9160)}{4.55pt}{4.82pt}{} & \HoloSegScore{0.9272}{(0.9060--0.9322)}{4.55pt}{4.82pt}{} & \HoloSegScore{0.6285}{(0.5780--0.6729)}{4.55pt}{4.82pt}{} & \HoloSegScore{0.8840}{(0.8570--0.9074)}{4.55pt}{4.82pt}{} \\*
\softcline{4-11}
 &  & \HoloSegSpan{\makecell[c]{thoracic\\[-0.10ex]vertebrae 5\\[-0.10ex](t5)}}{2.04cm}{0.32cm} & \HoloSegMetric{HD95} & \HoloSegScore{8.177}{(4.774--14.26)}{4.55pt}{4.82pt}{} & \HoloSegScore{17.35}{(14.89--20.57)}{4.55pt}{4.82pt}{} & \HoloSegScore{3.457}{(2.599--4.545)}{4.55pt}{4.82pt}{} & \HoloSegScore{3.439}{(2.758--4.177)}{4.55pt}{4.82pt}{} & \HoloSegScore{3.864}{(2.921--4.332)}{4.55pt}{4.82pt}{} & \HoloSegScore{7.866}{(6.884--8.860)}{4.55pt}{4.82pt}{} & \HoloSegScore{3.877}{(3.256--4.624)}{4.55pt}{4.82pt}{} \\
\cline{3-11}
 &  &  & \HoloSegMetric{Dice} & \HoloSegScore{0.8743}{(0.8390--0.9037)}{4.55pt}{4.82pt}{} & \HoloSegScore{0.4247}{(0.3952--0.4539)}{4.55pt}{4.82pt}{} & \HoloSegScore{0.8604}{(0.8357--0.8802)}{4.55pt}{4.82pt}{} & \HoloSegScore{0.8982}{(0.8674--0.9240)}{4.55pt}{4.82pt}{} & \HoloSegScore{0.9135}{(0.9006--0.9155)}{4.55pt}{4.82pt}{} & \HoloSegScore{0.7150}{(0.6919--0.7370)}{4.55pt}{4.82pt}{} & \HoloSegScore{0.8950}{(0.8719--0.9129)}{4.55pt}{4.82pt}{} \\*
\softcline{4-11}
 &  & \HoloSegSpan{\makecell[c]{thoracic\\[-0.10ex]vertebrae 4\\[-0.10ex](t4)}}{2.04cm}{0.32cm} & \HoloSegMetric{HD95} & \HoloSegScore{5.581}{(4.578--6.719)}{4.55pt}{4.82pt}{} & \HoloSegScore{13.78}{(12.81--14.81)}{4.55pt}{4.82pt}{} & \HoloSegScore{3.297}{(2.412--4.467)}{4.55pt}{4.82pt}{} & \HoloSegScore{3.305}{(2.629--4.180)}{4.55pt}{4.82pt}{} & \HoloSegScore{5.004}{(2.390--6.671)}{4.55pt}{4.82pt}{} & \HoloSegScore{54.52}{(45.94--62.56)}{4.55pt}{4.82pt}{} & \HoloSegScore{3.726}{(2.987--4.528)}{4.55pt}{4.82pt}{} \\
\hline
\pagebreak[4]
 &  &  & \HoloSegMetric{Dice} & \HoloSegScore{0.8828}{(0.8501--0.9143)}{4.55pt}{4.82pt}{} & \HoloSegScore{0.3902}{(0.3644--0.4184)}{4.55pt}{4.82pt}{} & \HoloSegScore{0.8526}{(0.8257--0.8763)}{4.55pt}{4.82pt}{} & \HoloSegScore{0.8973}{(0.8662--0.9248)}{4.55pt}{4.82pt}{} & \HoloSegScore{0.9278}{(0.9145--0.9617)}{4.55pt}{4.82pt}{} & \HoloSegScore{0.8738}{(0.8498--0.8951)}{4.55pt}{4.82pt}{} & \HoloSegScore{0.9045}{(0.8824--0.9235)}{4.55pt}{4.82pt}{} \\*
\softcline{4-11}
 &  & \HoloSegSpan{\makecell[c]{thoracic\\[-0.10ex]vertebrae 3\\[-0.10ex](t3)}}{2.04cm}{0.32cm} & \HoloSegMetric{HD95} & \HoloSegScore{5.508}{(4.435--6.844)}{4.55pt}{4.82pt}{} & \HoloSegScore{15.51}{(14.16--16.95)}{4.55pt}{4.82pt}{} & \HoloSegScore{2.545}{(2.071--3.086)}{4.55pt}{4.82pt}{} & \HoloSegScore{3.007}{(2.394--3.694)}{4.55pt}{4.82pt}{} & \HoloSegScore{4.991}{(4.373--5.252)}{4.55pt}{4.82pt}{} & \HoloSegScore{12.78}{(9.550--16.84)}{4.55pt}{4.82pt}{} & \HoloSegScore{4.168}{(2.888--6.235)}{4.55pt}{4.82pt}{} \\
\cline{3-11}
 &  &  & \HoloSegMetric{Dice} & \HoloSegScore{0.9087}{(0.8797--0.9315)}{4.55pt}{4.82pt}{} & \HoloSegScore{0.2012}{(0.1733--0.2302)}{4.55pt}{4.82pt}{} & \HoloSegScore{0.8694}{(0.8520--0.8861)}{4.55pt}{4.82pt}{} & \HoloSegScore{0.9052}{(0.8746--0.9334)}{4.55pt}{4.82pt}{} & \HoloSegScore{0.9176}{(0.8927--0.9360)}{4.55pt}{4.82pt}{} & \HoloSegScore{0.8744}{(0.8482--0.8955)}{4.55pt}{4.82pt}{} & \HoloSegScore{0.9215}{(0.9089--0.9328)}{4.55pt}{4.82pt}{} \\*
\softcline{4-11}
 &  & \HoloSegSpan{\makecell[c]{thoracic\\[-0.10ex]vertebrae 2\\[-0.10ex](t2)}}{2.04cm}{0.32cm} & \HoloSegMetric{HD95} & \HoloSegScore{21.08}{(10.39--34.75)}{4.55pt}{4.82pt}{} & \HoloSegScore{22.01}{(20.01--24.56)}{4.55pt}{4.82pt}{} & \HoloSegScore{2.232}{(1.848--2.735)}{4.55pt}{4.82pt}{} & \HoloSegScore{2.415}{(1.912--3.033)}{4.55pt}{4.82pt}{} & \HoloSegScore{4.266}{(3.180--4.435)}{4.55pt}{4.82pt}{} & \HoloSegScore{3.338}{(2.635--4.215)}{4.55pt}{4.82pt}{} & \HoloSegScore{2.547}{(2.091--3.055)}{4.55pt}{4.82pt}{} \\
\cline{3-11}
 &  &  & \HoloSegMetric{Dice} & \HoloSegScore{0.9060}{(0.8852--0.9249)}{4.55pt}{4.82pt}{} & \HoloSegScore{0.2260}{(0.1997--0.2535)}{4.55pt}{4.82pt}{} & \HoloSegScore{0.8711}{(0.8513--0.8863)}{4.55pt}{4.82pt}{} & \HoloSegScore{0.9254}{(0.9047--0.9429)}{4.55pt}{4.82pt}{} & \HoloSegScore{0.9455}{(0.9337--0.9542)}{4.55pt}{4.82pt}{} & \HoloSegScore{0.9170}{(0.8970--0.9312)}{4.55pt}{4.82pt}{} & \HoloSegScore{0.9236}{(0.9125--0.9323)}{4.55pt}{4.82pt}{} \\*
\softcline{4-11}
 &  & \HoloSegSpan{\makecell[c]{thoracic\\[-0.10ex]vertebrae 1\\[-0.10ex](t1)}}{2.04cm}{0.32cm} & \HoloSegMetric{HD95} & \HoloSegScore{16.02}{(12.53--19.54)}{4.55pt}{4.82pt}{} & \HoloSegScore{23.63}{(20.72--26.82)}{4.55pt}{4.82pt}{} & \HoloSegScore{2.144}{(1.834--2.498)}{4.55pt}{4.82pt}{} & \HoloSegScore{2.099}{(1.688--2.624)}{4.55pt}{4.82pt}{} & \HoloSegScore{2.185}{(0.8640--3.492)}{4.55pt}{4.82pt}{} & \HoloSegScore{2.365}{(1.823--2.946)}{4.55pt}{4.82pt}{} & \HoloSegScore{2.277}{(1.918--2.734)}{4.55pt}{4.82pt}{} \\
\cline{3-11}
 &  &  & \HoloSegMetric{Dice} & \HoloSegScore{0.9039}{(0.8795--0.9226)}{4.55pt}{4.82pt}{} & \HoloSegScore{0.0000}{(0.0000--0.0000)}{4.55pt}{4.82pt}{} & \HoloSegScore{0.8404}{(0.8195--0.8581)}{4.55pt}{4.82pt}{} & \HoloSegScore{0.8948}{(0.8690--0.9177)}{4.55pt}{4.82pt}{} & \HoloSegScore{0.9466}{(0.9396--0.9834)}{4.55pt}{4.82pt}{} & \HoloSegScore{0.8722}{(0.8451--0.8938)}{4.55pt}{4.82pt}{} & \HoloSegScore{0.8963}{(0.8731--0.9152)}{4.55pt}{4.82pt}{} \\*
\softcline{4-11}
 &  & \HoloSegSpan{\makecell[c]{cervical\\[-0.10ex]vertebrae 7\\[-0.10ex](c7)}}{2.04cm}{0.32cm} & \HoloSegMetric{HD95} & \HoloSegScore{3.346}{(2.878--4.001)}{4.55pt}{4.82pt}{} & \HoloSegScore{157.6}{(150.9--164.3)}{4.55pt}{4.82pt}{} & \HoloSegScore{2.354}{(2.023--2.835)}{4.55pt}{4.82pt}{} & \HoloSegScore{2.514}{(2.051--3.143)}{4.55pt}{4.82pt}{} & \HoloSegScore{1.624}{(1.548--2.010)}{4.55pt}{4.82pt}{} & \HoloSegScore{7.425}{(4.791--11.81)}{4.55pt}{4.82pt}{} & \HoloSegScore{3.837}{(2.644--5.489)}{4.55pt}{4.82pt}{} \\
\cline{3-11}
 &  &  & \HoloSegMetric{Dice} & \HoloSegScore{0.8796}{(0.8526--0.9021)}{4.55pt}{4.82pt}{} & \HoloSegScore{0.02665}{(0.01215--0.04564)}{4.20pt}{4.48pt}{} & \HoloSegScore{0.7637}{(0.7338--0.7907)}{4.55pt}{4.82pt}{} & \HoloSegScore{0.8124}{(0.7675--0.8553)}{4.55pt}{4.82pt}{} & \HoloSegScore{0.8432}{(0.8130--0.8816)}{4.55pt}{4.82pt}{} & \HoloSegScore{0.8168}{(0.7832--0.8490)}{4.55pt}{4.82pt}{} & \HoloSegScore{0.8336}{(0.8007--0.8626)}{4.55pt}{4.82pt}{} \\*
\softcline{4-11}
 &  & \HoloSegSpan{\makecell[c]{cervical\\[-0.10ex]vertebrae 6\\[-0.10ex](c6)}}{2.04cm}{0.32cm} & \HoloSegMetric{HD95} & \HoloSegScore{4.042}{(3.208--5.004)}{4.55pt}{4.82pt}{} & \HoloSegScore{127.2}{(117.9--136.5)}{4.55pt}{4.82pt}{} & \HoloSegScore{2.839}{(2.313--3.630)}{4.55pt}{4.82pt}{} & \HoloSegScore{3.529}{(2.633--4.577)}{4.55pt}{4.82pt}{} & \HoloSegScore{2.708}{(1.588--3.102)}{4.55pt}{4.82pt}{} & \HoloSegScore{4.358}{(3.343--5.515)}{4.55pt}{4.82pt}{} & \HoloSegScore{6.453}{(2.940--12.69)}{4.55pt}{4.82pt}{} \\
\cline{3-11}
 &  &  & \HoloSegMetric{Dice} & \HoloSegScore{0.8064}{(0.7467--0.8568)}{4.55pt}{4.82pt}{} & \HoloSegScore{0.05967}{(0.03120--0.09090)}{4.20pt}{4.48pt}{} & \HoloSegScore{0.7435}{(0.6931--0.7904)}{4.55pt}{4.82pt}{} & \HoloSegScore{0.7841}{(0.7166--0.8456)}{4.55pt}{4.82pt}{} & \HoloSegScore{0.8496}{(0.8151--0.8707)}{4.55pt}{4.82pt}{} & \HoloSegScore{0.4599}{(0.4001--0.5181)}{4.55pt}{4.82pt}{} & \HoloSegScore{0.8142}{(0.7626--0.8564)}{4.55pt}{4.82pt}{} \\*
\softcline{4-11}
 &  & \HoloSegSpan{\makecell[c]{cervical\\[-0.10ex]vertebrae 5\\[-0.10ex](c5)}}{2.04cm}{0.32cm} & \HoloSegMetric{HD95} & \HoloSegScore{10.01}{(5.684--14.33)}{4.55pt}{4.82pt}{} & \HoloSegScore{62.68}{(53.37--73.14)}{4.55pt}{4.82pt}{} & \HoloSegScore{2.986}{(2.227--4.416)}{4.55pt}{4.82pt}{} & \HoloSegScore{2.218}{(1.861--2.694)}{4.55pt}{4.82pt}{} & \HoloSegScore{2.542}{(2.376--5.631)}{4.55pt}{4.82pt}{} & \HoloSegScore{7.871}{(6.975--8.897)}{4.55pt}{4.82pt}{} & \HoloSegScore{3.146}{(2.752--3.592)}{4.55pt}{4.82pt}{} \\
\cline{3-11}
 &  &  & \HoloSegMetric{Dice} & \HoloSegScore{0.8866}{(0.8432--0.9170)}{4.55pt}{4.82pt}{} & \HoloSegScore{0.1273}{(0.08531--0.1720)}{4.20pt}{4.48pt}{} & \HoloSegScore{0.8180}{(0.7798--0.8468)}{4.55pt}{4.82pt}{} & \HoloSegScore{0.8967}{(0.8609--0.9223)}{4.55pt}{4.82pt}{} & \HoloSegScore{0.8613}{(0.8346--0.8795)}{4.55pt}{4.82pt}{} & \HoloSegScore{0.5396}{(0.5073--0.5679)}{4.55pt}{4.82pt}{} & \HoloSegScore{0.8642}{(0.8224--0.8976)}{4.55pt}{4.82pt}{} \\*
\softcline{4-11}
 &  & \HoloSegSpan{\makecell[c]{cervical\\[-0.10ex]vertebrae 4\\[-0.10ex](c4)}}{2.04cm}{0.32cm} & \HoloSegMetric{HD95} & \HoloSegScore{29.37}{(11.62--50.15)}{4.55pt}{4.82pt}{} & \HoloSegScore{32.37}{(25.87--38.83)}{4.55pt}{4.82pt}{} & \HoloSegScore{2.454}{(1.992--3.170)}{4.55pt}{4.82pt}{} & \HoloSegScore{2.031}{(1.746--2.387)}{4.55pt}{4.82pt}{} & \HoloSegScore{3.803}{(3.439--4.239)}{4.55pt}{4.82pt}{} & \HoloSegScore{100.8}{(65.56--135.8)}{4.55pt}{4.82pt}{} & \HoloSegScore{2.597}{(2.128--3.162)}{4.55pt}{4.82pt}{} \\
\cline{3-11}
 &  &  & \HoloSegMetric{Dice} & \HoloSegScore{0.8976}{(0.8618--0.9244)}{4.55pt}{4.82pt}{} & \HoloSegScore{0.03431}{(0.006584--0.06950)}{3.85pt}{4.12pt}{} & \HoloSegScore{0.8405}{(0.8039--0.8717)}{4.55pt}{4.82pt}{} & \HoloSegScore{0.8997}{(0.8584--0.9320)}{4.55pt}{4.82pt}{} & \HoloSegScore{0.9371}{(0.9119--0.9532)}{4.55pt}{4.82pt}{} & \HoloSegScore{0.8354}{(0.7884--0.8739)}{4.55pt}{4.82pt}{} & \HoloSegScore{0.8857}{(0.8387--0.9174)}{4.55pt}{4.82pt}{} \\*
\softcline{4-11}
 &  & \HoloSegSpan{\makecell[c]{cervical\\[-0.10ex]vertebrae 3\\[-0.10ex](c3)}}{2.04cm}{0.32cm} & \HoloSegMetric{HD95} & \HoloSegScore{30.29}{(14.23--50.38)}{4.55pt}{4.82pt}{} & \HoloSegScore{39.94}{(34.26--46.31)}{4.55pt}{4.82pt}{} & \HoloSegScore{2.037}{(1.725--2.486)}{4.55pt}{4.82pt}{} & \HoloSegScore{2.086}{(1.691--2.566)}{4.55pt}{4.82pt}{} & \HoloSegScore{2.637}{(1.891--3.906)}{4.55pt}{4.82pt}{} & \HoloSegScore{5.589}{(4.380--6.847)}{4.55pt}{4.82pt}{} & \HoloSegScore{2.472}{(1.937--3.130)}{4.55pt}{4.82pt}{} \\
\cline{3-11}
 &  &  & \HoloSegMetric{Dice} & \HoloSegScore{0.8974}{(0.8608--0.9261)}{4.55pt}{4.82pt}{} & \HoloSegScore{0.1426}{(0.09709--0.1910)}{4.20pt}{4.48pt}{} & \HoloSegScore{0.8550}{(0.8095--0.8919)}{4.55pt}{4.82pt}{} & \HoloSegScore{0.9273}{(0.8929--0.9494)}{4.55pt}{4.82pt}{} & \HoloSegScore{0.9541}{(0.9127--0.9792)}{4.55pt}{4.82pt}{} & \HoloSegScore{0.8960}{(0.8662--0.9232)}{4.55pt}{4.82pt}{} & \HoloSegScore{0.8664}{(0.8097--0.9139)}{4.55pt}{4.82pt}{} \\*
\softcline{4-11}
 &  & \HoloSegSpan{\makecell[c]{cervical\\[-0.10ex]vertebrae 2\\[-0.10ex](c2)}}{2.04cm}{0.32cm} & \HoloSegMetric{HD95} & \HoloSegScore{21.44}{(9.527--34.46)}{4.55pt}{4.82pt}{} & \HoloSegScore{31.33}{(26.71--36.68)}{4.55pt}{4.82pt}{} & \HoloSegScore{3.363}{(1.595--6.245)}{4.55pt}{4.82pt}{} & \HoloSegScore{2.130}{(1.450--3.031)}{4.55pt}{4.82pt}{} & \HoloSegScore{2.673}{(2.020--3.843)}{4.55pt}{4.82pt}{} & \HoloSegScore{8.551}{(1.966--20.96)}{4.55pt}{4.82pt}{} & \HoloSegScore{7.246}{(2.489--15.69)}{4.55pt}{4.82pt}{} \\
\cline{3-11}
 &  &  & \HoloSegMetric{Dice} & \HoloSegScore{0.8614}{(0.8092--0.9022)}{4.55pt}{4.82pt}{} & \HoloSegScore{0.3072}{(0.2601--0.3544)}{4.55pt}{4.82pt}{} & \HoloSegScore{0.8145}{(0.7621--0.8546)}{4.55pt}{4.82pt}{} & \HoloSegScore{0.8862}{(0.8314--0.9281)}{4.55pt}{4.82pt}{} & \HoloSegScore{0.8572}{(0.8238--0.8943)}{4.55pt}{4.82pt}{} & \HoloSegScore{0.8463}{(0.7849--0.8922)}{4.55pt}{4.82pt}{} & \HoloSegScore{0.8567}{(0.7904--0.9044)}{4.55pt}{4.82pt}{} \\*
\softcline{4-11}
\HoloSegSpan{\makecell[c]{\textbf{Internal}}}{1.20cm}{0.32cm} & \HoloSegSpan{\makecell[c]{Total-\\[-0.10ex]SegmentatorV2}}{1.86cm}{0.32cm} & \HoloSegSpan{\makecell[c]{cervical\\[-0.10ex]vertebrae 1\\[-0.10ex](c1)}}{2.04cm}{0.32cm} & \HoloSegMetric{HD95} & \HoloSegScore{31.12}{(9.915--60.06)}{4.55pt}{4.82pt}{} & \HoloSegScore{17.58}{(15.33--20.10)}{4.55pt}{4.82pt}{} & \HoloSegScore{10.48}{(1.730--35.74)}{4.55pt}{4.82pt}{} & \HoloSegScore{2.253}{(1.624--3.201)}{4.55pt}{4.82pt}{} & \HoloSegScore{13.67}{(10.65--17.13)}{4.55pt}{4.82pt}{} & \HoloSegScore{25.31}{(6.757--51.48)}{4.55pt}{4.82pt}{} & \HoloSegScore{19.17}{(2.219--45.49)}{4.55pt}{4.82pt}{} \\
\cline{3-11}
 &  &  & \HoloSegMetric{Dice} & \HoloSegScore{0.8963}{(0.8728--0.9159)}{4.55pt}{4.82pt}{} & \HoloSegScore{0.2719}{(0.2516--0.2916)}{4.55pt}{4.82pt}{} & \HoloSegScore{0.9016}{(0.8783--0.9208)}{4.55pt}{4.82pt}{} & \HoloSegScore{0.9077}{(0.8828--0.9275)}{4.55pt}{4.82pt}{} & \HoloSegScore{0.9264}{(0.9098--0.9455)}{4.55pt}{4.82pt}{} & \HoloSegScore{0.9102}{(0.8874--0.9302)}{4.55pt}{4.82pt}{} & \HoloSegScore{0.9050}{(0.8837--0.9234)}{4.55pt}{4.82pt}{} \\*
\softcline{4-11}
 &  & \HoloSegSpan{\makecell[c]{heart}}{2.04cm}{0.32cm} & \HoloSegMetric{HD95} & \HoloSegScore{11.39}{(9.217--13.59)}{4.55pt}{4.82pt}{} & \HoloSegScore{47.98}{(46.01--50.00)}{4.55pt}{4.82pt}{} & \HoloSegScore{11.42}{(6.743--17.69)}{4.55pt}{4.82pt}{} & \HoloSegScore{4.550}{(4.021--5.232)}{4.55pt}{4.82pt}{} & \HoloSegScore{5.745}{(2.767--8.090)}{4.55pt}{4.82pt}{} & \HoloSegScore{18.79}{(13.47--24.64)}{4.55pt}{4.82pt}{} & \HoloSegScore{7.490}{(5.150--10.40)}{4.55pt}{4.82pt}{} \\
\cline{3-11}
 &  &  & \HoloSegMetric{Dice} & \HoloSegScore{0.9419}{(0.9305--0.9503)}{4.55pt}{4.82pt}{} & \HoloSegScore{0.7028}{(0.6822--0.7205)}{4.55pt}{4.82pt}{} & \HoloSegScore{0.9174}{(0.9002--0.9314)}{4.55pt}{4.82pt}{} & \HoloSegScore{0.9545}{(0.9439--0.9625)}{4.55pt}{4.82pt}{} & \HoloSegScore{0.9568}{(0.9365--0.9609)}{4.55pt}{4.82pt}{} & \HoloSegScore{0.9493}{(0.9356--0.9592)}{4.55pt}{4.82pt}{} & \HoloSegScore{0.9416}{(0.9297--0.9512)}{4.55pt}{4.82pt}{} \\*
\softcline{4-11}
 &  & \HoloSegSpan{\makecell[c]{aorta}}{2.04cm}{0.32cm} & \HoloSegMetric{HD95} & \HoloSegScore{3.260}{(2.936--3.634)}{4.55pt}{4.82pt}{} & \HoloSegScore{15.45}{(13.37--17.74)}{4.55pt}{4.82pt}{} & \HoloSegScore{3.837}{(2.688--5.495)}{4.55pt}{4.82pt}{} & \HoloSegScore{2.637}{(2.056--3.434)}{4.55pt}{4.82pt}{} & \HoloSegScore{2.124}{(1.590--2.890)}{4.55pt}{4.82pt}{} & \HoloSegScore{7.521}{(4.748--11.48)}{4.55pt}{4.82pt}{} & \HoloSegScore{5.631}{(3.773--7.862)}{4.55pt}{4.82pt}{} \\
\cline{3-11}
 &  &  & \HoloSegMetric{Dice} & \HoloSegScore{0.6835}{(0.6445--0.7245)}{4.55pt}{4.82pt}{} & \HoloSegScore{0.005716}{(0.003492--0.008508)}{3.85pt}{4.12pt}{} & \HoloSegScore{0.7795}{(0.7512--0.8041)}{4.55pt}{4.82pt}{} & \HoloSegScore{0.8276}{(0.8016--0.8528)}{4.55pt}{4.82pt}{} & \HoloSegScore{0.8223}{(0.8119--0.8508)}{4.55pt}{4.82pt}{} & \HoloSegScore{0.7772}{(0.7523--0.8019)}{4.55pt}{4.82pt}{} & \HoloSegScore{0.8154}{(0.7889--0.8413)}{4.55pt}{4.82pt}{} \\*
\softcline{4-11}
 &  & \HoloSegSpan{\makecell[c]{pulmonary\\[-0.10ex]vein}}{2.04cm}{0.32cm} & \HoloSegMetric{HD95} & \HoloSegScore{184.9}{(158.9--212.2)}{4.55pt}{4.82pt}{} & \HoloSegScore{92.10}{(86.63--97.59)}{4.55pt}{4.82pt}{} & \HoloSegScore{5.382}{(3.814--7.358)}{4.55pt}{4.82pt}{} & \HoloSegScore{7.469}{(5.164--10.02)}{4.55pt}{4.82pt}{} & \HoloSegScore{7.522}{(5.663--10.25)}{4.55pt}{4.82pt}{} & \HoloSegScore{12.45}{(9.479--16.18)}{4.55pt}{4.82pt}{} & \HoloSegScore{9.880}{(7.530--12.52)}{4.55pt}{4.82pt}{} \\
\cline{3-11}
 &  &  & \HoloSegMetric{Dice} & \HoloSegScore{0.8840}{(0.8683--0.8968)}{4.55pt}{4.82pt}{} & \HoloSegScore{0.009225}{(0.005542--0.01349)}{3.85pt}{4.12pt}{} & \HoloSegScore{0.8568}{(0.8371--0.8710)}{4.55pt}{4.82pt}{} & \HoloSegScore{0.8804}{(0.8621--0.8951)}{4.55pt}{4.82pt}{} & \HoloSegScore{0.8962}{(0.8920--0.9368)}{4.55pt}{4.82pt}{} & \HoloSegScore{0.8691}{(0.8505--0.8856)}{4.55pt}{4.82pt}{} & \HoloSegScore{0.8799}{(0.8642--0.8922)}{4.55pt}{4.82pt}{} \\*
\softcline{4-11}
 &  & \HoloSegSpan{\makecell[c]{brachiocephalic\\[-0.10ex]trunk}}{2.04cm}{0.32cm} & \HoloSegMetric{HD95} & \HoloSegScore{7.689}{(5.078--10.47)}{4.55pt}{4.82pt}{} & \HoloSegScore{100.7}{(89.96--111.8)}{4.55pt}{4.82pt}{} & \HoloSegScore{5.574}{(2.210--12.10)}{4.55pt}{4.82pt}{} & \HoloSegScore{2.774}{(2.475--3.131)}{4.55pt}{4.82pt}{} & \HoloSegScore{4.090}{(3.936--4.683)}{4.55pt}{4.82pt}{} & \HoloSegScore{4.711}{(3.962--5.534)}{4.55pt}{4.82pt}{} & \HoloSegScore{5.749}{(3.170--9.979)}{4.55pt}{4.82pt}{} \\
\cline{3-11}
 &  &  & \HoloSegMetric{Dice} & \HoloSegScore{0.8463}{(0.8267--0.8642)}{4.55pt}{4.82pt}{} & \HoloSegScore{0.001032}{(0.0001986--0.002105)}{3.52pt}{3.80pt}{} & \HoloSegScore{0.8133}{(0.8015--0.8236)}{4.55pt}{4.82pt}{} & \HoloSegScore{0.8584}{(0.8382--0.8758)}{4.55pt}{4.82pt}{} & \HoloSegScore{0.8671}{(0.8641--0.8727)}{4.55pt}{4.82pt}{} & \HoloSegScore{0.8341}{(0.8173--0.8494)}{4.55pt}{4.82pt}{} & \HoloSegScore{0.8490}{(0.8288--0.8649)}{4.55pt}{4.82pt}{} \\*
\softcline{4-11}
 &  & \HoloSegSpan{\makecell[c]{right\\[-0.10ex]subclavian\\[-0.10ex]artery}}{2.04cm}{0.32cm} & \HoloSegMetric{HD95} & \HoloSegScore{27.34}{(13.44--43.13)}{4.55pt}{4.82pt}{} & \HoloSegScore{124.2}{(107.8--142.7)}{4.55pt}{4.82pt}{} & \HoloSegScore{4.528}{(2.314--8.721)}{4.55pt}{4.82pt}{} & \HoloSegScore{3.350}{(2.779--3.954)}{4.55pt}{4.82pt}{} & \HoloSegScore{2.759}{(2.653--4.715)}{4.55pt}{4.82pt}{} & \HoloSegScore{15.49}{(8.998--23.59)}{4.55pt}{4.82pt}{} & \HoloSegScore{4.987}{(3.956--6.116)}{4.55pt}{4.82pt}{} \\
\cline{3-11}
 &  &  & \HoloSegMetric{Dice} & \HoloSegScore{0.8565}{(0.8404--0.8713)}{4.55pt}{4.82pt}{} & \HoloSegScore{0.006123}{(0.001615--0.01262)}{3.85pt}{4.12pt}{} & \HoloSegScore{0.8346}{(0.8205--0.8450)}{4.55pt}{4.82pt}{} & \HoloSegScore{0.8804}{(0.8714--0.8894)}{4.55pt}{4.82pt}{} & \HoloSegScore{0.9045}{(0.9003--0.9086)}{4.55pt}{4.82pt}{} & \HoloSegScore{0.8439}{(0.8274--0.8580)}{4.55pt}{4.82pt}{} & \HoloSegScore{0.8596}{(0.8460--0.8708)}{4.55pt}{4.82pt}{} \\*
\softcline{4-11}
 &  & \HoloSegSpan{\makecell[c]{left\\[-0.10ex]subclavian\\[-0.10ex]artery}}{2.04cm}{0.32cm} & \HoloSegMetric{HD95} & \HoloSegScore{7.682}{(4.926--10.51)}{4.55pt}{4.82pt}{} & \HoloSegScore{184.4}{(156.7--214.9)}{4.55pt}{4.82pt}{} & \HoloSegScore{5.744}{(2.008--13.03)}{4.55pt}{4.82pt}{} & \HoloSegScore{3.372}{(2.567--4.613)}{4.55pt}{4.82pt}{} & \HoloSegScore{2.702}{(1.734--3.505)}{4.55pt}{4.82pt}{} & \HoloSegScore{7.552}{(5.809--9.590)}{4.55pt}{4.82pt}{} & \HoloSegScore{6.327}{(4.657--8.604)}{4.55pt}{4.82pt}{} \\
\cline{3-11}
 &  &  & \HoloSegMetric{Dice} & \HoloSegScore{0.7975}{(0.7736--0.8169)}{4.55pt}{4.82pt}{} & \HoloSegScore{0.00003876}{(0.000003283--0.00008297)}{3.25pt}{3.52pt}{} & \HoloSegScore{0.7922}{(0.7726--0.8086)}{4.55pt}{4.82pt}{} & \HoloSegScore{0.8043}{(0.7829--0.8243)}{4.55pt}{4.82pt}{} & \HoloSegScore{0.8547}{(0.8529--0.8583)}{4.55pt}{4.82pt}{} & \HoloSegScore{0.7855}{(0.7645--0.8061)}{4.55pt}{4.82pt}{} & \HoloSegScore{0.8163}{(0.7944--0.8354)}{4.55pt}{4.82pt}{} \\*
\softcline{4-11}
 &  & \HoloSegSpan{\makecell[c]{right common\\[-0.10ex]carotid\\[-0.10ex]artery}}{2.04cm}{0.32cm} & \HoloSegMetric{HD95} & \HoloSegScore{9.831}{(5.803--16.79)}{4.55pt}{4.82pt}{} & \HoloSegScore{80.31}{(71.79--89.57)}{4.55pt}{4.82pt}{} & \HoloSegScore{7.681}{(2.705--15.10)}{4.55pt}{4.82pt}{} & \HoloSegScore{4.833}{(3.959--5.788)}{4.55pt}{4.82pt}{} & \HoloSegScore{5.897}{(5.399--6.303)}{4.55pt}{4.82pt}{} & \HoloSegScore{6.763}{(5.014--8.964)}{4.55pt}{4.82pt}{} & \HoloSegScore{7.510}{(4.134--12.35)}{4.55pt}{4.82pt}{} \\
\cline{3-11}
 &  &  & \HoloSegMetric{Dice} & \HoloSegScore{0.8541}{(0.8351--0.8704)}{4.55pt}{4.82pt}{} & \HoloSegScore{0.005155}{(0.001001--0.01390)}{3.85pt}{4.12pt}{} & \HoloSegScore{0.8416}{(0.8305--0.8516)}{4.55pt}{4.82pt}{} & \HoloSegScore{0.8766}{(0.8651--0.8872)}{4.55pt}{4.82pt}{} & \HoloSegScore{0.8845}{(0.8623--0.9053)}{4.55pt}{4.82pt}{} & \HoloSegScore{0.8274}{(0.8073--0.8464)}{4.55pt}{4.82pt}{} & \HoloSegScore{0.8772}{(0.8626--0.8893)}{4.55pt}{4.82pt}{} \\*
\softcline{4-11}
 &  & \HoloSegSpan{\makecell[c]{left common\\[-0.10ex]carotid\\[-0.10ex]artery}}{2.04cm}{0.32cm} & \HoloSegMetric{HD95} & \HoloSegScore{9.919}{(4.973--17.52)}{4.55pt}{4.82pt}{} & \HoloSegScore{117.0}{(99.84--135.3)}{4.55pt}{4.82pt}{} & \HoloSegScore{10.96}{(4.452--20.61)}{4.55pt}{4.82pt}{} & \HoloSegScore{4.133}{(3.317--5.111)}{4.55pt}{4.82pt}{} & \HoloSegScore{2.727}{(1.785--5.124)}{4.55pt}{4.82pt}{} & \HoloSegScore{5.346}{(4.410--6.486)}{4.55pt}{4.82pt}{} & \HoloSegScore{15.74}{(8.905--24.13)}{4.55pt}{4.82pt}{} \\
\cline{3-11}
 &  &  & \HoloSegMetric{Dice} & \HoloSegScore{0.7650}{(0.7340--0.7944)}{4.55pt}{4.82pt}{} & \HoloSegScore{0.0006165}{(0.00006731--0.001503)}{3.52pt}{3.80pt}{} & \HoloSegScore{0.8547}{(0.8412--0.8669)}{4.55pt}{4.82pt}{} & \HoloSegScore{0.9008}{(0.8881--0.9133)}{4.55pt}{4.82pt}{} & \HoloSegScore{0.9228}{(0.9197--0.9366)}{4.55pt}{4.82pt}{} & \HoloSegScore{0.8808}{(0.8657--0.8940)}{4.55pt}{4.82pt}{} & \HoloSegScore{0.8895}{(0.8792--0.8990)}{4.55pt}{4.82pt}{} \\*
\softcline{4-11}
 &  & \HoloSegSpan{\makecell[c]{left\\[-0.10ex]brachiocephalic\\[-0.10ex]vein}}{2.04cm}{0.32cm} & \HoloSegMetric{HD95} & \HoloSegScore{17.51}{(13.70--21.07)}{4.55pt}{4.82pt}{} & \HoloSegScore{235.3}{(210.1--262.4)}{4.55pt}{4.82pt}{} & \HoloSegScore{55.44}{(35.78--78.44)}{4.55pt}{4.82pt}{} & \HoloSegScore{3.417}{(2.359--4.876)}{4.55pt}{4.82pt}{} & \HoloSegScore{3.332}{(2.850--5.045)}{4.55pt}{4.82pt}{} & \HoloSegScore{6.915}{(4.538--10.00)}{4.55pt}{4.82pt}{} & \HoloSegScore{3.607}{(2.719--4.759)}{4.55pt}{4.82pt}{} \\
\hline
\pagebreak[4]
 &  &  & \HoloSegMetric{Dice} & \HoloSegScore{0.8706}{(0.8563--0.8833)}{4.55pt}{4.82pt}{} & \HoloSegScore{0.0006354}{(0.0001379--0.001390)}{3.52pt}{3.80pt}{} & \HoloSegScore{0.8471}{(0.8282--0.8625)}{4.55pt}{4.82pt}{} & \HoloSegScore{0.8801}{(0.8644--0.8939)}{4.55pt}{4.82pt}{} & \HoloSegScore{0.9121}{(0.9001--0.9124)}{4.55pt}{4.82pt}{} & \HoloSegScore{0.8474}{(0.8337--0.8598)}{4.55pt}{4.82pt}{} & \HoloSegScore{0.8731}{(0.8559--0.8864)}{4.55pt}{4.82pt}{} \\*
\softcline{4-11}
 &  & \HoloSegSpan{\makecell[c]{right\\[-0.10ex]brachiocephalic\\[-0.10ex]vein}}{2.04cm}{0.32cm} & \HoloSegMetric{HD95} & \HoloSegScore{4.469}{(4.038--5.055)}{4.55pt}{4.82pt}{} & \HoloSegScore{249.5}{(223.9--273.4)}{4.55pt}{4.82pt}{} & \HoloSegScore{24.30}{(10.85--39.31)}{4.55pt}{4.82pt}{} & \HoloSegScore{3.384}{(2.868--3.991)}{4.55pt}{4.82pt}{} & \HoloSegScore{2.358}{(0.8580--2.753)}{4.55pt}{4.82pt}{} & \HoloSegScore{7.001}{(5.154--10.28)}{4.55pt}{4.82pt}{} & \HoloSegScore{2.816}{(2.554--3.086)}{4.55pt}{4.82pt}{} \\
\cline{3-11}
 &  &  & \HoloSegMetric{Dice} & \HoloSegScore{0.8819}{(0.8655--0.8949)}{4.55pt}{4.82pt}{} & \HoloSegScore{0.0004524}{(0.0000--0.001224)}{4.20pt}{4.48pt}{} & \HoloSegScore{0.0000}{(0.0000--0.0000)}{4.55pt}{4.82pt}{} & \HoloSegScore{0.8727}{(0.8551--0.8862)}{4.55pt}{4.82pt}{} & \HoloSegScore{0.8961}{(0.8908--0.9130)}{4.55pt}{4.82pt}{} & \HoloSegScore{0.6563}{(0.6257--0.6856)}{4.55pt}{4.82pt}{} & \HoloSegScore{0.8670}{(0.8481--0.8815)}{4.55pt}{4.82pt}{} \\*
\softcline{4-11}
 &  & \HoloSegSpan{\makecell[c]{left atrial\\[-0.10ex]appendage of\\[-0.10ex]heart}}{2.04cm}{0.32cm} & \HoloSegMetric{HD95} & \HoloSegScore{12.50}{(3.378--24.59)}{4.55pt}{4.82pt}{} & \HoloSegScore{132.2}{(127.0--138.0)}{4.55pt}{4.82pt}{} & \HoloSegScore{70.90}{(60.28--88.34)}{4.55pt}{4.82pt}{} & \HoloSegScore{3.321}{(2.753--3.931)}{4.55pt}{4.82pt}{} & \HoloSegScore{5.325}{(4.323--6.645)}{4.55pt}{4.82pt}{} & \HoloSegScore{4.926}{(4.458--5.432)}{4.55pt}{4.82pt}{} & \HoloSegScore{4.276}{(2.911--6.042)}{4.55pt}{4.82pt}{} \\
\cline{3-11}
 &  &  & \HoloSegMetric{Dice} & \HoloSegScore{0.7630}{(0.7270--0.7963)}{4.55pt}{4.82pt}{} & \HoloSegScore{0.003658}{(0.0002010--0.009604)}{3.52pt}{3.80pt}{} & \HoloSegScore{0.8840}{(0.8653--0.9011)}{4.55pt}{4.82pt}{} & \HoloSegScore{0.9106}{(0.8907--0.9266)}{4.55pt}{4.82pt}{} & \HoloSegScore{0.8991}{(0.8660--0.9052)}{4.55pt}{4.82pt}{} & \HoloSegScore{0.8756}{(0.8498--0.8982)}{4.55pt}{4.82pt}{} & \HoloSegScore{0.8936}{(0.8686--0.9135)}{4.55pt}{4.82pt}{} \\*
\softcline{4-11}
 &  & \HoloSegSpan{\makecell[c]{superior\\[-0.10ex]vena cava}}{2.04cm}{0.32cm} & \HoloSegMetric{HD95} & \HoloSegScore{16.64}{(13.48--19.77)}{4.55pt}{4.82pt}{} & \HoloSegScore{157.4}{(145.7--168.4)}{4.55pt}{4.82pt}{} & \HoloSegScore{2.683}{(2.345--3.086)}{4.55pt}{4.82pt}{} & \HoloSegScore{2.572}{(2.290--2.895)}{4.55pt}{4.82pt}{} & \HoloSegScore{2.357}{(1.579--2.645)}{4.55pt}{4.82pt}{} & \HoloSegScore{15.28}{(8.722--22.51)}{4.55pt}{4.82pt}{} & \HoloSegScore{3.817}{(3.119--4.787)}{4.55pt}{4.82pt}{} \\
\cline{3-11}
 &  &  & \HoloSegMetric{Dice} & \HoloSegScore{0.8880}{(0.8680--0.9047)}{4.55pt}{4.82pt}{} & \HoloSegScore{0.6637}{(0.6357--0.6885)}{4.55pt}{4.82pt}{} & \HoloSegScore{0.8990}{(0.8833--0.9119)}{4.55pt}{4.82pt}{} & \HoloSegScore{0.8898}{(0.8734--0.9044)}{4.55pt}{4.82pt}{} & \HoloSegScore{0.9020}{(0.8838--0.9140)}{4.55pt}{4.82pt}{} & \HoloSegScore{0.8815}{(0.8610--0.8997)}{4.55pt}{4.82pt}{} & \HoloSegScore{0.8801}{(0.8604--0.8962)}{4.55pt}{4.82pt}{} \\*
\softcline{4-11}
 &  & \HoloSegSpan{\makecell[c]{inferior\\[-0.10ex]vena cava}}{2.04cm}{0.32cm} & \HoloSegMetric{HD95} & \HoloSegScore{5.022}{(4.071--6.449)}{4.55pt}{4.82pt}{} & \HoloSegScore{13.28}{(10.29--16.62)}{4.55pt}{4.82pt}{} & \HoloSegScore{3.041}{(2.316--4.353)}{4.55pt}{4.82pt}{} & \HoloSegScore{4.272}{(3.324--5.655)}{4.55pt}{4.82pt}{} & \HoloSegScore{6.089}{(6.046--7.927)}{4.55pt}{4.82pt}{} & \HoloSegScore{4.037}{(3.195--5.289)}{4.55pt}{4.82pt}{} & \HoloSegScore{4.486}{(3.565--5.601)}{4.55pt}{4.82pt}{} \\
\cline{3-11}
 &  &  & \HoloSegMetric{Dice} & \HoloSegScore{0.7943}{(0.7659--0.8194)}{4.55pt}{4.82pt}{} & \HoloSegScore{0.2655}{(0.2417--0.2893)}{4.55pt}{4.82pt}{} & \HoloSegScore{0.7647}{(0.7397--0.7887)}{4.55pt}{4.82pt}{} & \HoloSegScore{0.7627}{(0.7299--0.7944)}{4.55pt}{4.82pt}{} & \HoloSegScore{0.8338}{(0.8072--0.8653)}{4.55pt}{4.82pt}{} & \HoloSegScore{0.7656}{(0.7339--0.7914)}{4.55pt}{4.82pt}{} & \HoloSegScore{0.7848}{(0.7563--0.8096)}{4.55pt}{4.82pt}{} \\*
\softcline{4-11}
 &  & \HoloSegSpan{\makecell[c]{portal vein\\[-0.10ex]and splenic\\[-0.10ex]vein}}{2.04cm}{0.32cm} & \HoloSegMetric{HD95} & \HoloSegScore{6.945}{(5.706--8.486)}{4.55pt}{4.82pt}{} & \HoloSegScore{49.46}{(42.83--56.27)}{4.55pt}{4.82pt}{} & \HoloSegScore{6.035}{(4.658--7.789)}{4.55pt}{4.82pt}{} & \HoloSegScore{12.45}{(9.619--16.02)}{4.55pt}{4.82pt}{} & \HoloSegScore{7.266}{(5.731--8.780)}{4.55pt}{4.82pt}{} & \HoloSegScore{10.69}{(8.402--13.39)}{4.55pt}{4.82pt}{} & \HoloSegScore{10.08}{(7.806--12.56)}{4.55pt}{4.82pt}{} \\
\cline{3-11}
 &  &  & \HoloSegMetric{Dice} & \HoloSegScore{0.8423}{(0.8139--0.8653)}{4.55pt}{4.82pt}{} & \HoloSegScore{0.3313}{(0.3052--0.3564)}{4.55pt}{4.82pt}{} & \HoloSegScore{0.8622}{(0.8468--0.8750)}{4.55pt}{4.82pt}{} & \HoloSegScore{0.8571}{(0.8289--0.8810)}{4.55pt}{4.82pt}{} & \HoloSegScore{0.9008}{(0.8732--0.9347)}{4.55pt}{4.82pt}{} & \HoloSegScore{0.8223}{(0.7893--0.8519)}{4.55pt}{4.82pt}{} & \HoloSegScore{0.8144}{(0.7901--0.8378)}{4.55pt}{4.82pt}{} \\*
\softcline{4-11}
 &  & \HoloSegSpan{\makecell[c]{left iliac\\[-0.10ex]artery}}{2.04cm}{0.32cm} & \HoloSegMetric{HD95} & \HoloSegScore{16.41}{(13.29--19.78)}{4.55pt}{4.82pt}{} & \HoloSegScore{21.44}{(17.78--25.63)}{4.55pt}{4.82pt}{} & \HoloSegScore{14.62}{(4.953--27.57)}{4.55pt}{4.82pt}{} & \HoloSegScore{4.410}{(3.606--5.226)}{4.55pt}{4.82pt}{} & \HoloSegScore{3.824}{(3.158--6.674)}{4.55pt}{4.82pt}{} & \HoloSegScore{13.91}{(7.857--23.77)}{4.55pt}{4.82pt}{} & \HoloSegScore{14.70}{(8.518--24.77)}{4.55pt}{4.82pt}{} \\
\cline{3-11}
 &  &  & \HoloSegMetric{Dice} & \HoloSegScore{0.7870}{(0.7563--0.8160)}{4.55pt}{4.82pt}{} & \HoloSegScore{0.2815}{(0.2574--0.3048)}{4.55pt}{4.82pt}{} & \HoloSegScore{0.8552}{(0.8329--0.8730)}{4.55pt}{4.82pt}{} & \HoloSegScore{0.8501}{(0.8190--0.8780)}{4.55pt}{4.82pt}{} & \HoloSegScore{0.8751}{(0.8543--0.9004)}{4.55pt}{4.82pt}{} & \HoloSegScore{0.8199}{(0.7835--0.8498)}{4.55pt}{4.82pt}{} & \HoloSegScore{0.8423}{(0.8150--0.8653)}{4.55pt}{4.82pt}{} \\*
\softcline{4-11}
 &  & \HoloSegSpan{\makecell[c]{right iliac\\[-0.10ex]artery}}{2.04cm}{0.32cm} & \HoloSegMetric{HD95} & \HoloSegScore{16.21}{(13.50--18.78)}{4.55pt}{4.82pt}{} & \HoloSegScore{24.30}{(19.53--29.54)}{4.55pt}{4.82pt}{} & \HoloSegScore{10.71}{(2.049--21.96)}{4.55pt}{4.82pt}{} & \HoloSegScore{4.328}{(3.434--5.371)}{4.55pt}{4.82pt}{} & \HoloSegScore{4.889}{(3.042--6.145)}{4.55pt}{4.82pt}{} & \HoloSegScore{92.35}{(65.90--119.9)}{4.55pt}{4.82pt}{} & \HoloSegScore{9.788}{(5.352--17.40)}{4.55pt}{4.82pt}{} \\
\cline{3-11}
 &  &  & \HoloSegMetric{Dice} & \HoloSegScore{0.9044}{(0.8911--0.9147)}{4.55pt}{4.82pt}{} & \HoloSegScore{0.3923}{(0.3626--0.4205)}{4.55pt}{4.82pt}{} & \HoloSegScore{0.8900}{(0.8780--0.9007)}{4.55pt}{4.82pt}{} & \HoloSegScore{0.8797}{(0.8626--0.8936)}{4.55pt}{4.82pt}{} & \HoloSegScore{0.8978}{(0.8885--0.8999)}{4.55pt}{4.82pt}{} & \HoloSegScore{0.8654}{(0.8441--0.8838)}{4.55pt}{4.82pt}{} & \HoloSegScore{0.8718}{(0.8549--0.8861)}{4.55pt}{4.82pt}{} \\*
\softcline{4-11}
 &  & \HoloSegSpan{\makecell[c]{left iliac\\[-0.10ex]vena}}{2.04cm}{0.32cm} & \HoloSegMetric{HD95} & \HoloSegScore{6.022}{(3.119--10.76)}{4.55pt}{4.82pt}{} & \HoloSegScore{20.81}{(15.99--26.34)}{4.55pt}{4.82pt}{} & \HoloSegScore{5.233}{(1.843--14.72)}{4.55pt}{4.82pt}{} & \HoloSegScore{3.042}{(2.561--3.581)}{4.55pt}{4.82pt}{} & \HoloSegScore{5.074}{(2.677--6.051)}{4.55pt}{4.82pt}{} & \HoloSegScore{8.522}{(4.534--14.67)}{4.55pt}{4.82pt}{} & \HoloSegScore{5.861}{(4.443--7.790)}{4.55pt}{4.82pt}{} \\
\cline{3-11}
 &  &  & \HoloSegMetric{Dice} & \HoloSegScore{0.8540}{(0.8248--0.8771)}{4.55pt}{4.82pt}{} & \HoloSegScore{0.3742}{(0.3470--0.4012)}{4.55pt}{4.82pt}{} & \HoloSegScore{0.8722}{(0.8468--0.8903)}{4.55pt}{4.82pt}{} & \HoloSegScore{0.8559}{(0.8277--0.8794)}{4.55pt}{4.82pt}{} & \HoloSegScore{0.8879}{(0.8623--0.9021)}{4.55pt}{4.82pt}{} & \HoloSegScore{0.8401}{(0.8154--0.8633)}{4.55pt}{4.82pt}{} & \HoloSegScore{0.8534}{(0.8273--0.8767)}{4.55pt}{4.82pt}{} \\*
\softcline{4-11}
 &  & \HoloSegSpan{\makecell[c]{right iliac\\[-0.10ex]vena}}{2.04cm}{0.32cm} & \HoloSegMetric{HD95} & \HoloSegScore{13.84}{(11.08--16.52)}{4.55pt}{4.82pt}{} & \HoloSegScore{20.55}{(15.75--25.87)}{4.55pt}{4.82pt}{} & \HoloSegScore{4.935}{(1.894--10.84)}{4.55pt}{4.82pt}{} & \HoloSegScore{3.430}{(2.801--4.160)}{4.55pt}{4.82pt}{} & \HoloSegScore{4.193}{(4.108--5.165)}{4.55pt}{4.82pt}{} & \HoloSegScore{12.27}{(5.145--22.25)}{4.55pt}{4.82pt}{} & \HoloSegScore{6.681}{(3.100--12.96)}{4.55pt}{4.82pt}{} \\
\cline{3-11}
 &  &  & \HoloSegMetric{Dice} & \HoloSegScore{0.6027}{(0.5586--0.6420)}{4.55pt}{4.82pt}{} & \HoloSegScore{0.5589}{(0.5103--0.6047)}{4.55pt}{4.82pt}{} & \HoloSegScore{0.8388}{(0.7951--0.8799)}{4.55pt}{4.82pt}{} & \HoloSegScore{0.8814}{(0.8346--0.9191)}{4.55pt}{4.82pt}{} & \HoloSegScore{0.8689}{(0.8474--0.9057)}{4.55pt}{4.82pt}{} & \HoloSegScore{0.8742}{(0.8285--0.9150)}{4.55pt}{4.82pt}{} & \HoloSegScore{0.8732}{(0.8325--0.9121)}{4.55pt}{4.82pt}{} \\*
\softcline{4-11}
\HoloSegSpan{\makecell[c]{\textbf{Internal}}}{1.20cm}{0.32cm} & \HoloSegSpan{\makecell[c]{Total-\\[-0.10ex]SegmentatorV2}}{1.86cm}{0.32cm} & \HoloSegSpan{\makecell[c]{left humerus}}{2.04cm}{0.32cm} & \HoloSegMetric{HD95} & \HoloSegScore{41.64}{(38.16--45.04)}{4.55pt}{4.82pt}{} & \HoloSegScore{22.75}{(13.73--36.17)}{4.55pt}{4.82pt}{} & \HoloSegScore{28.85}{(12.68--48.41)}{4.55pt}{4.82pt}{} & \HoloSegScore{4.345}{(2.535--6.367)}{4.55pt}{4.82pt}{} & \HoloSegScore{6.993}{(0.8770--15.50)}{4.55pt}{4.82pt}{} & \HoloSegScore{15.93}{(8.006--26.61)}{4.55pt}{4.82pt}{} & \HoloSegScore{8.073}{(4.804--12.98)}{4.55pt}{4.82pt}{} \\
\cline{3-11}
 &  &  & \HoloSegMetric{Dice} & \HoloSegScore{0.7016}{(0.6587--0.7386)}{4.55pt}{4.82pt}{} & \HoloSegScore{0.5677}{(0.5231--0.6125)}{4.55pt}{4.82pt}{} & \HoloSegScore{0.8251}{(0.7762--0.8714)}{4.55pt}{4.82pt}{} & \HoloSegScore{0.8600}{(0.8048--0.9025)}{4.55pt}{4.82pt}{} & \HoloSegScore{0.7946}{(0.7540--0.8351)}{4.55pt}{4.82pt}{} & \HoloSegScore{0.8412}{(0.7851--0.8896)}{4.55pt}{4.82pt}{} & \HoloSegScore{0.8689}{(0.8204--0.9107)}{4.55pt}{4.82pt}{} \\*
\softcline{4-11}
 &  & \HoloSegSpan{\makecell[c]{right\\[-0.10ex]humerus}}{2.04cm}{0.32cm} & \HoloSegMetric{HD95} & \HoloSegScore{39.23}{(35.87--42.35)}{4.55pt}{4.82pt}{} & \HoloSegScore{31.57}{(18.21--48.06)}{4.55pt}{4.82pt}{} & \HoloSegScore{20.11}{(8.357--34.00)}{4.55pt}{4.82pt}{} & \HoloSegScore{4.522}{(2.543--7.316)}{4.55pt}{4.82pt}{} & \HoloSegScore{8.303}{(6.117--11.68)}{4.55pt}{4.82pt}{} & \HoloSegScore{11.20}{(5.826--18.78)}{4.55pt}{4.82pt}{} & \HoloSegScore{9.540}{(3.507--18.80)}{4.55pt}{4.82pt}{} \\
\cline{3-11}
 &  &  & \HoloSegMetric{Dice} & \HoloSegScore{0.8984}{(0.8807--0.9145)}{4.55pt}{4.82pt}{} & \HoloSegScore{0.5227}{(0.4888--0.5551)}{4.55pt}{4.82pt}{} & \HoloSegScore{0.8517}{(0.8253--0.8775)}{4.55pt}{4.82pt}{} & \HoloSegScore{0.9040}{(0.8809--0.9215)}{4.55pt}{4.82pt}{} & \HoloSegScore{0.9487}{(0.9370--0.9570)}{4.55pt}{4.82pt}{} & \HoloSegScore{0.8935}{(0.8728--0.9087)}{4.55pt}{4.82pt}{} & \HoloSegScore{0.9026}{(0.8845--0.9177)}{4.55pt}{4.82pt}{} \\*
\softcline{4-11}
 &  & \HoloSegSpan{\makecell[c]{left scapula}}{2.04cm}{0.32cm} & \HoloSegMetric{HD95} & \HoloSegScore{6.170}{(3.730--10.09)}{4.55pt}{4.82pt}{} & \HoloSegScore{13.97}{(9.929--19.31)}{4.55pt}{4.82pt}{} & \HoloSegScore{3.502}{(2.517--4.733)}{4.55pt}{4.82pt}{} & \HoloSegScore{2.907}{(2.340--3.557)}{4.55pt}{4.82pt}{} & \HoloSegScore{2.349}{(0.1230--2.893)}{4.55pt}{4.82pt}{} & \HoloSegScore{14.67}{(9.478--20.56)}{4.55pt}{4.82pt}{} & \HoloSegScore{4.723}{(2.739--7.878)}{4.55pt}{4.82pt}{} \\
\cline{3-11}
 &  &  & \HoloSegMetric{Dice} & \HoloSegScore{0.9021}{(0.8832--0.9178)}{4.55pt}{4.82pt}{} & \HoloSegScore{0.5181}{(0.4783--0.5500)}{4.55pt}{4.82pt}{} & \HoloSegScore{0.8801}{(0.8610--0.8964)}{4.55pt}{4.82pt}{} & \HoloSegScore{0.9166}{(0.8956--0.9335)}{4.55pt}{4.82pt}{} & \HoloSegScore{0.9236}{(0.9032--0.9502)}{4.55pt}{4.82pt}{} & \HoloSegScore{0.8886}{(0.8702--0.9029)}{4.55pt}{4.82pt}{} & \HoloSegScore{0.9078}{(0.8896--0.9225)}{4.55pt}{4.82pt}{} \\*
\softcline{4-11}
 &  & \HoloSegSpan{\makecell[c]{right\\[-0.10ex]scapula}}{2.04cm}{0.32cm} & \HoloSegMetric{HD95} & \HoloSegScore{41.58}{(27.13--59.38)}{4.55pt}{4.82pt}{} & \HoloSegScore{13.31}{(9.605--18.11)}{4.55pt}{4.82pt}{} & \HoloSegScore{4.617}{(1.675--10.29)}{4.55pt}{4.82pt}{} & \HoloSegScore{1.977}{(1.686--2.343)}{4.55pt}{4.82pt}{} & \HoloSegScore{2.770}{(1.884--2.863)}{4.55pt}{4.82pt}{} & \HoloSegScore{14.41}{(7.021--23.38)}{4.55pt}{4.82pt}{} & \HoloSegScore{3.660}{(2.110--6.434)}{4.55pt}{4.82pt}{} \\
\cline{3-11}
 &  &  & \HoloSegMetric{Dice} & \HoloSegScore{0.9383}{(0.9209--0.9495)}{4.55pt}{4.82pt}{} & \HoloSegScore{0.4012}{(0.3696--0.4298)}{4.55pt}{4.82pt}{} & \HoloSegScore{0.8882}{(0.8644--0.9049)}{4.55pt}{4.82pt}{} & \HoloSegScore{0.9542}{(0.9382--0.9641)}{4.55pt}{4.82pt}{} & \HoloSegScore{0.9192}{(0.9020--0.9370)}{4.55pt}{4.82pt}{} & \HoloSegScore{0.9416}{(0.9204--0.9572)}{4.55pt}{4.82pt}{} & \HoloSegScore{0.9261}{(0.9022--0.9444)}{4.55pt}{4.82pt}{} \\*
\softcline{4-11}
 &  & \HoloSegSpan{\makecell[c]{left\\[-0.10ex]clavicle}}{2.04cm}{0.32cm} & \HoloSegMetric{HD95} & \HoloSegScore{17.51}{(6.668--29.83)}{4.55pt}{4.82pt}{} & \HoloSegScore{22.58}{(18.69--26.77)}{4.55pt}{4.82pt}{} & \HoloSegScore{13.07}{(1.642--32.76)}{4.55pt}{4.82pt}{} & \HoloSegScore{1.458}{(1.079--2.044)}{4.55pt}{4.82pt}{} & \HoloSegScore{4.132}{(3.566--5.770)}{4.55pt}{4.82pt}{} & \HoloSegScore{17.21}{(9.680--26.64)}{4.55pt}{4.82pt}{} & \HoloSegScore{6.038}{(1.824--14.08)}{4.55pt}{4.82pt}{} \\
\cline{3-11}
 &  &  & \HoloSegMetric{Dice} & \HoloSegScore{0.9331}{(0.9208--0.9414)}{4.55pt}{4.82pt}{} & \HoloSegScore{0.4364}{(0.4067--0.4652)}{4.55pt}{4.82pt}{} & \HoloSegScore{0.8982}{(0.8881--0.9062)}{4.55pt}{4.82pt}{} & \HoloSegScore{0.9453}{(0.9343--0.9523)}{4.55pt}{4.82pt}{} & \HoloSegScore{0.9375}{(0.9280--0.9483)}{4.55pt}{4.82pt}{} & \HoloSegScore{0.9389}{(0.9242--0.9507)}{4.55pt}{4.82pt}{} & \HoloSegScore{0.9380}{(0.9283--0.9467)}{4.55pt}{4.82pt}{} \\*
\softcline{4-11}
 &  & \HoloSegSpan{\makecell[c]{right\\[-0.10ex]clavicle}}{2.04cm}{0.32cm} & \HoloSegMetric{HD95} & \HoloSegScore{14.36}{(5.300--26.21)}{4.55pt}{4.82pt}{} & \HoloSegScore{19.94}{(16.45--23.97)}{4.55pt}{4.82pt}{} & \HoloSegScore{3.982}{(1.628--8.570)}{4.55pt}{4.82pt}{} & \HoloSegScore{1.763}{(1.561--1.973)}{4.55pt}{4.82pt}{} & \HoloSegScore{1.427}{(1.165--1.629)}{4.55pt}{4.82pt}{} & \HoloSegScore{7.426}{(4.416--10.97)}{4.55pt}{4.82pt}{} & \HoloSegScore{4.557}{(1.789--11.38)}{4.55pt}{4.82pt}{} \\
\cline{3-11}
 &  &  & \HoloSegMetric{Dice} & \HoloSegScore{0.9102}{(0.8832--0.9325)}{4.55pt}{4.82pt}{} & \HoloSegScore{0.7449}{(0.7084--0.7773)}{4.55pt}{4.82pt}{} & \HoloSegScore{0.8957}{(0.8667--0.9217)}{4.55pt}{4.82pt}{} & \HoloSegScore{0.9555}{(0.9286--0.9759)}{4.55pt}{4.82pt}{} & \HoloSegScore{0.8843}{(0.8565--0.8903)}{4.55pt}{4.82pt}{} & \HoloSegScore{0.9449}{(0.9143--0.9703)}{4.55pt}{4.82pt}{} & \HoloSegScore{0.9135}{(0.8852--0.9369)}{4.55pt}{4.82pt}{} \\*
\softcline{4-11}
 &  & \HoloSegSpan{\makecell[c]{left femur}}{2.04cm}{0.32cm} & \HoloSegMetric{HD95} & \HoloSegScore{35.43}{(32.96--37.94)}{4.55pt}{4.82pt}{} & \HoloSegScore{18.40}{(11.77--25.75)}{4.55pt}{4.82pt}{} & \HoloSegScore{130.4}{(88.51--172.3)}{4.55pt}{4.82pt}{} & \HoloSegScore{2.851}{(1.682--4.909)}{4.55pt}{4.82pt}{} & \HoloSegScore{8.004}{(6.995--12.05)}{4.55pt}{4.82pt}{} & \HoloSegScore{81.21}{(50.79--113.2)}{4.55pt}{4.82pt}{} & \HoloSegScore{63.62}{(46.15--81.86)}{4.55pt}{4.82pt}{} \\
\cline{3-11}
 &  &  & \HoloSegMetric{Dice} & \HoloSegScore{0.8858}{(0.8552--0.9107)}{4.55pt}{4.82pt}{} & \HoloSegScore{0.7436}{(0.7111--0.7725)}{4.55pt}{4.82pt}{} & \HoloSegScore{0.8888}{(0.8647--0.9108)}{4.55pt}{4.82pt}{} & \HoloSegScore{0.9682}{(0.9468--0.9805)}{4.55pt}{4.82pt}{} & \HoloSegScore{0.9130}{(0.8828--0.9245)}{4.55pt}{4.82pt}{} & \HoloSegScore{0.9588}{(0.9296--0.9799)}{4.55pt}{4.82pt}{} & \HoloSegScore{0.9619}{(0.9435--0.9749)}{4.55pt}{4.82pt}{} \\*
\softcline{4-11}
 &  & \HoloSegSpan{\makecell[c]{right femur}}{2.04cm}{0.32cm} & \HoloSegMetric{HD95} & \HoloSegScore{28.76}{(23.82--33.30)}{4.55pt}{4.82pt}{} & \HoloSegScore{14.20}{(9.334--20.12)}{4.55pt}{4.82pt}{} & \HoloSegScore{196.9}{(153.4--246.0)}{4.55pt}{4.82pt}{} & \HoloSegScore{1.799}{(1.556--2.099)}{4.55pt}{4.82pt}{} & \HoloSegScore{11.84}{(8.827--14.44)}{4.55pt}{4.82pt}{} & \HoloSegScore{16.20}{(5.888--28.11)}{4.55pt}{4.82pt}{} & \HoloSegScore{18.97}{(5.073--38.01)}{4.55pt}{4.82pt}{} \\
\cline{3-11}
 &  &  & \HoloSegMetric{Dice} & \HoloSegScore{0.9262}{(0.9024--0.9429)}{4.55pt}{4.82pt}{} & \HoloSegScore{0.6507}{(0.6274--0.6730)}{4.55pt}{4.82pt}{} & \HoloSegScore{0.9214}{(0.8999--0.9380)}{4.55pt}{4.82pt}{} & \HoloSegScore{0.9452}{(0.9218--0.9633)}{4.55pt}{4.82pt}{} & \HoloSegScore{0.9334}{(0.9091--0.9504)}{4.55pt}{4.82pt}{} & \HoloSegScore{0.9342}{(0.9106--0.9537)}{4.55pt}{4.82pt}{} & \HoloSegScore{0.9360}{(0.9160--0.9516)}{4.55pt}{4.82pt}{} \\*
\softcline{4-11}
 &  & \HoloSegSpan{\makecell[c]{left hip}}{2.04cm}{0.32cm} & \HoloSegMetric{HD95} & \HoloSegScore{51.92}{(30.18--75.20)}{4.55pt}{4.82pt}{} & \HoloSegScore{16.50}{(11.02--24.38)}{4.55pt}{4.82pt}{} & \HoloSegScore{10.02}{(2.128--22.07)}{4.55pt}{4.82pt}{} & \HoloSegScore{1.965}{(1.605--2.524)}{4.55pt}{4.82pt}{} & \HoloSegScore{11.61}{(6.224--19.56)}{4.55pt}{4.82pt}{} & \HoloSegScore{72.35}{(53.77--92.73)}{4.55pt}{4.82pt}{} & \HoloSegScore{47.67}{(26.47--74.19)}{4.55pt}{4.82pt}{} \\
\cline{3-11}
 &  &  & \HoloSegMetric{Dice} & \HoloSegScore{0.8979}{(0.8703--0.9213)}{4.55pt}{4.82pt}{} & \HoloSegScore{0.6754}{(0.6398--0.7051)}{4.55pt}{4.82pt}{} & \HoloSegScore{0.9275}{(0.9031--0.9429)}{4.55pt}{4.82pt}{} & \HoloSegScore{0.9379}{(0.9092--0.9592)}{4.55pt}{4.82pt}{} & \HoloSegScore{0.9321}{(0.9250--0.9340)}{4.55pt}{4.82pt}{} & \HoloSegScore{0.9391}{(0.9093--0.9601)}{4.55pt}{4.82pt}{} & \HoloSegScore{0.9357}{(0.9098--0.9539)}{4.55pt}{4.82pt}{} \\*
\softcline{4-11}
 &  & \HoloSegSpan{\makecell[c]{right hip}}{2.04cm}{0.32cm} & \HoloSegMetric{HD95} & \HoloSegScore{21.60}{(17.71--25.35)}{4.55pt}{4.82pt}{} & \HoloSegScore{27.27}{(18.98--36.90)}{4.55pt}{4.82pt}{} & \HoloSegScore{18.17}{(3.874--36.68)}{4.55pt}{4.82pt}{} & \HoloSegScore{2.703}{(1.553--4.792)}{4.55pt}{4.82pt}{} & \HoloSegScore{3.953}{(2.551--7.664)}{4.55pt}{4.82pt}{} & \HoloSegScore{32.57}{(18.58--49.50)}{4.55pt}{4.82pt}{} & \HoloSegScore{19.05}{(6.468--35.19)}{4.55pt}{4.82pt}{} \\
\hline
\pagebreak[4]
 &  &  & \HoloSegMetric{Dice} & \HoloSegScore{0.9205}{(0.9157--0.9251)}{4.55pt}{4.82pt}{} & \HoloSegScore{0.006804}{(0.004890--0.009071)}{3.85pt}{4.12pt}{} & \HoloSegScore{0.9068}{(0.8980--0.9141)}{4.55pt}{4.82pt}{} & \HoloSegScore{0.9227}{(0.9185--0.9273)}{4.55pt}{4.82pt}{} & \HoloSegScore{0.9546}{(0.9332--0.9662)}{4.55pt}{4.82pt}{} & \HoloSegScore{0.8497}{(0.8382--0.8596)}{4.55pt}{4.82pt}{} & \HoloSegScore{0.8993}{(0.8923--0.9054)}{4.55pt}{4.82pt}{} \\*
\softcline{4-11}
 &  & \HoloSegSpan{\makecell[c]{spinal cord}}{2.04cm}{0.32cm} & \HoloSegMetric{HD95} & \HoloSegScore{2.844}{(2.669--3.084)}{4.55pt}{4.82pt}{} & \HoloSegScore{177.7}{(164.2--191.5)}{4.55pt}{4.82pt}{} & \HoloSegScore{1.968}{(1.724--2.333)}{4.55pt}{4.82pt}{} & \HoloSegScore{1.871}{(1.676--2.127)}{4.55pt}{4.82pt}{} & \HoloSegScore{1.512}{(0.7330--3.169)}{4.55pt}{4.82pt}{} & \HoloSegScore{20.34}{(17.52--23.65)}{4.55pt}{4.82pt}{} & \HoloSegScore{9.701}{(6.697--13.13)}{4.55pt}{4.82pt}{} \\
\cline{3-11}
 &  &  & \HoloSegMetric{Dice} & \HoloSegScore{0.9257}{(0.9098--0.9380)}{4.55pt}{4.82pt}{} & \HoloSegScore{0.8166}{(0.7887--0.8406)}{4.55pt}{4.82pt}{} & \HoloSegScore{0.9333}{(0.9137--0.9473)}{4.55pt}{4.82pt}{} & \HoloSegScore{0.9311}{(0.9089--0.9459)}{4.55pt}{4.82pt}{} & \HoloSegScore{0.9294}{(0.9177--0.9299)}{4.55pt}{4.82pt}{} & \HoloSegScore{0.9156}{(0.8936--0.9311)}{4.55pt}{4.82pt}{} & \HoloSegScore{0.9115}{(0.8873--0.9267)}{4.55pt}{4.82pt}{} \\*
\softcline{4-11}
 &  & \HoloSegSpan{\makecell[c]{left gluteus\\[-0.10ex]maximus}}{2.04cm}{0.32cm} & \HoloSegMetric{HD95} & \HoloSegScore{20.14}{(10.19--33.14)}{4.55pt}{4.82pt}{} & \HoloSegScore{9.173}{(7.843--11.06)}{4.55pt}{4.82pt}{} & \HoloSegScore{2.818}{(2.440--3.330)}{4.55pt}{4.82pt}{} & \HoloSegScore{2.912}{(2.497--3.501)}{4.55pt}{4.82pt}{} & \HoloSegScore{5.131}{(4.930--5.903)}{4.55pt}{4.82pt}{} & \HoloSegScore{38.15}{(26.51--50.48)}{4.55pt}{4.82pt}{} & \HoloSegScore{9.690}{(5.374--16.50)}{4.55pt}{4.82pt}{} \\
\cline{3-11}
 &  &  & \HoloSegMetric{Dice} & \HoloSegScore{0.9228}{(0.9024--0.9402)}{4.55pt}{4.82pt}{} & \HoloSegScore{0.8226}{(0.7897--0.8521)}{4.55pt}{4.82pt}{} & \HoloSegScore{0.9362}{(0.9138--0.9514)}{4.55pt}{4.82pt}{} & \HoloSegScore{0.9298}{(0.9026--0.9487)}{4.55pt}{4.82pt}{} & \HoloSegScore{0.9342}{(0.9125--0.9551)}{4.55pt}{4.82pt}{} & \HoloSegScore{0.9086}{(0.8757--0.9349)}{4.55pt}{4.82pt}{} & \HoloSegScore{0.9109}{(0.8839--0.9310)}{4.55pt}{4.82pt}{} \\*
\softcline{4-11}
 &  & \HoloSegSpan{\makecell[c]{right\\[-0.10ex]gluteus\\[-0.10ex]maximus}}{2.04cm}{0.32cm} & \HoloSegMetric{HD95} & \HoloSegScore{14.24}{(5.442--26.36)}{4.55pt}{4.82pt}{} & \HoloSegScore{18.64}{(12.36--26.47)}{4.55pt}{4.82pt}{} & \HoloSegScore{2.533}{(2.309--2.778)}{4.55pt}{4.82pt}{} & \HoloSegScore{2.880}{(2.403--3.414)}{4.55pt}{4.82pt}{} & \HoloSegScore{4.192}{(3.764--4.595)}{4.55pt}{4.82pt}{} & \HoloSegScore{21.42}{(10.14--35.20)}{4.55pt}{4.82pt}{} & \HoloSegScore{14.72}{(4.741--27.10)}{4.55pt}{4.82pt}{} \\
\cline{3-11}
 &  &  & \HoloSegMetric{Dice} & \HoloSegScore{0.8969}{(0.8680--0.9200)}{4.55pt}{4.82pt}{} & \HoloSegScore{0.7628}{(0.7316--0.7923)}{4.55pt}{4.82pt}{} & \HoloSegScore{0.9103}{(0.8801--0.9349)}{4.55pt}{4.82pt}{} & \HoloSegScore{0.9107}{(0.8908--0.9252)}{4.55pt}{4.82pt}{} & \HoloSegScore{0.9254}{(0.9083--0.9423)}{4.55pt}{4.82pt}{} & \HoloSegScore{0.8849}{(0.8579--0.9062)}{4.55pt}{4.82pt}{} & \HoloSegScore{0.8882}{(0.8674--0.9058)}{4.55pt}{4.82pt}{} \\*
\softcline{4-11}
 &  & \HoloSegSpan{\makecell[c]{left gluteus\\[-0.10ex]medius}}{2.04cm}{0.32cm} & \HoloSegMetric{HD95} & \HoloSegScore{12.47}{(8.787--16.15)}{4.55pt}{4.82pt}{} & \HoloSegScore{14.11}{(9.604--20.55)}{4.55pt}{4.82pt}{} & \HoloSegScore{5.868}{(2.604--12.26)}{4.55pt}{4.82pt}{} & \HoloSegScore{3.330}{(3.107--3.589)}{4.55pt}{4.82pt}{} & \HoloSegScore{4.332}{(4.130--4.998)}{4.55pt}{4.82pt}{} & \HoloSegScore{24.61}{(12.40--37.91)}{4.55pt}{4.82pt}{} & \HoloSegScore{5.669}{(4.153--8.288)}{4.55pt}{4.82pt}{} \\
\cline{3-11}
 &  &  & \HoloSegMetric{Dice} & \HoloSegScore{0.9143}{(0.8978--0.9264)}{4.55pt}{4.82pt}{} & \HoloSegScore{0.7600}{(0.7308--0.7863)}{4.55pt}{4.82pt}{} & \HoloSegScore{0.9283}{(0.9199--0.9354)}{4.55pt}{4.82pt}{} & \HoloSegScore{0.9319}{(0.9273--0.9361)}{4.55pt}{4.82pt}{} & \HoloSegScore{0.9319}{(0.9294--0.9321)}{4.55pt}{4.82pt}{} & \HoloSegScore{0.8945}{(0.8849--0.9034)}{4.55pt}{4.82pt}{} & \HoloSegScore{0.9091}{(0.9005--0.9164)}{4.55pt}{4.82pt}{} \\*
\softcline{4-11}
 &  & \HoloSegSpan{\makecell[c]{right\\[-0.10ex]gluteus\\[-0.10ex]medius}}{2.04cm}{0.32cm} & \HoloSegMetric{HD95} & \HoloSegScore{14.36}{(11.22--17.50)}{4.55pt}{4.82pt}{} & \HoloSegScore{21.26}{(12.83--31.76)}{4.55pt}{4.82pt}{} & \HoloSegScore{2.901}{(2.712--3.117)}{4.55pt}{4.82pt}{} & \HoloSegScore{2.841}{(2.650--3.038)}{4.55pt}{4.82pt}{} & \HoloSegScore{3.180}{(2.137--5.510)}{4.55pt}{4.82pt}{} & \HoloSegScore{15.43}{(7.517--26.23)}{4.55pt}{4.82pt}{} & \HoloSegScore{4.710}{(4.122--5.440)}{4.55pt}{4.82pt}{} \\
\cline{3-11}
 &  &  & \HoloSegMetric{Dice} & \HoloSegScore{0.9008}{(0.8952--0.9063)}{4.55pt}{4.82pt}{} & \HoloSegScore{0.6467}{(0.6185--0.6717)}{4.55pt}{4.82pt}{} & \HoloSegScore{0.8921}{(0.8858--0.8970)}{4.55pt}{4.82pt}{} & \HoloSegScore{0.8866}{(0.8810--0.8920)}{4.55pt}{4.82pt}{} & \HoloSegScore{0.9210}{(0.9085--0.9248)}{4.55pt}{4.82pt}{} & \HoloSegScore{0.8485}{(0.8382--0.8573)}{4.55pt}{4.82pt}{} & \HoloSegScore{0.8564}{(0.8475--0.8640)}{4.55pt}{4.82pt}{} \\*
\softcline{4-11}
 &  & \HoloSegSpan{\makecell[c]{left gluteus\\[-0.10ex]minimus}}{2.04cm}{0.32cm} & \HoloSegMetric{HD95} & \HoloSegScore{3.373}{(3.201--3.572)}{4.55pt}{4.82pt}{} & \HoloSegScore{13.96}{(9.674--19.44)}{4.55pt}{4.82pt}{} & \HoloSegScore{10.69}{(2.500--23.25)}{4.55pt}{4.82pt}{} & \HoloSegScore{2.820}{(2.668--2.975)}{4.55pt}{4.82pt}{} & \HoloSegScore{3.672}{(3.352--5.210)}{4.55pt}{4.82pt}{} & \HoloSegScore{39.87}{(26.87--54.60)}{4.55pt}{4.82pt}{} & \HoloSegScore{4.259}{(3.493--5.612)}{4.55pt}{4.82pt}{} \\
\cline{3-11}
 &  &  & \HoloSegMetric{Dice} & \HoloSegScore{0.9010}{(0.8822--0.9121)}{4.55pt}{4.82pt}{} & \HoloSegScore{0.6194}{(0.5844--0.6526)}{4.55pt}{4.82pt}{} & \HoloSegScore{0.8974}{(0.8916--0.9024)}{4.55pt}{4.82pt}{} & \HoloSegScore{0.8914}{(0.8719--0.9031)}{4.55pt}{4.82pt}{} & \HoloSegScore{0.9232}{(0.9212--0.9372)}{4.55pt}{4.82pt}{} & \HoloSegScore{0.8609}{(0.8401--0.8729)}{4.55pt}{4.82pt}{} & \HoloSegScore{0.8330}{(0.8174--0.8438)}{4.55pt}{4.82pt}{} \\*
\softcline{4-11}
 &  & \HoloSegSpan{\makecell[c]{right\\[-0.10ex]gluteus\\[-0.10ex]minimus}}{2.04cm}{0.32cm} & \HoloSegMetric{HD95} & \HoloSegScore{7.164}{(3.046--15.30)}{4.55pt}{4.82pt}{} & \HoloSegScore{38.25}{(25.95--51.36)}{4.55pt}{4.82pt}{} & \HoloSegScore{6.921}{(2.462--15.69)}{4.55pt}{4.82pt}{} & \HoloSegScore{2.634}{(2.489--2.791)}{4.55pt}{4.82pt}{} & \HoloSegScore{1.858}{(0.9770--2.397)}{4.55pt}{4.82pt}{} & \HoloSegScore{3.489}{(3.213--3.801)}{4.55pt}{4.82pt}{} & \HoloSegScore{6.009}{(5.197--7.023)}{4.55pt}{4.82pt}{} \\
\cline{3-11}
 &  &  & \HoloSegMetric{Dice} & \HoloSegScore{0.9373}{(0.9334--0.9408)}{4.55pt}{4.82pt}{} & \HoloSegScore{0.8024}{(0.7848--0.8198)}{4.55pt}{4.82pt}{} & \HoloSegScore{0.9396}{(0.9335--0.9446)}{4.55pt}{4.82pt}{} & \HoloSegScore{0.9360}{(0.9306--0.9406)}{4.55pt}{4.82pt}{} & \HoloSegScore{0.9315}{(0.9228--0.9466)}{4.55pt}{4.82pt}{} & \HoloSegScore{0.8968}{(0.8848--0.9060)}{4.55pt}{4.82pt}{} & \HoloSegScore{0.8969}{(0.8846--0.9063)}{4.55pt}{4.82pt}{} \\*
\softcline{4-11}
 &  & \HoloSegSpan{\makecell[c]{left\\[-0.10ex]autochthon}}{2.04cm}{0.32cm} & \HoloSegMetric{HD95} & \HoloSegScore{5.171}{(2.978--8.747)}{4.55pt}{4.82pt}{} & \HoloSegScore{7.971}{(6.790--9.273)}{4.55pt}{4.82pt}{} & \HoloSegScore{2.058}{(1.955--2.169)}{4.55pt}{4.82pt}{} & \HoloSegScore{2.276}{(2.101--2.454)}{4.55pt}{4.82pt}{} & \HoloSegScore{2.411}{(2.184--3.361)}{4.55pt}{4.82pt}{} & \HoloSegScore{15.93}{(12.16--20.91)}{4.55pt}{4.82pt}{} & \HoloSegScore{6.414}{(5.158--7.894)}{4.55pt}{4.82pt}{} \\
\cline{3-11}
 &  &  & \HoloSegMetric{Dice} & \HoloSegScore{0.9282}{(0.9144--0.9388)}{4.55pt}{4.82pt}{} & \HoloSegScore{0.7973}{(0.7756--0.8141)}{4.55pt}{4.82pt}{} & \HoloSegScore{0.9398}{(0.9343--0.9439)}{4.55pt}{4.82pt}{} & \HoloSegScore{0.9292}{(0.9161--0.9403)}{4.55pt}{4.82pt}{} & \HoloSegScore{0.9306}{(0.9144--0.9479)}{4.55pt}{4.82pt}{} & \HoloSegScore{0.8907}{(0.8748--0.9036)}{4.55pt}{4.82pt}{} & \HoloSegScore{0.8983}{(0.8851--0.9090)}{4.55pt}{4.82pt}{} \\*
\softcline{4-11}
 &  & \HoloSegSpan{\makecell[c]{right\\[-0.10ex]autochthon}}{2.04cm}{0.32cm} & \HoloSegMetric{HD95} & \HoloSegScore{4.925}{(2.909--9.425)}{4.55pt}{4.82pt}{} & \HoloSegScore{8.120}{(6.875--9.651)}{4.55pt}{4.82pt}{} & \HoloSegScore{3.593}{(1.929--8.351)}{4.55pt}{4.82pt}{} & \HoloSegScore{3.694}{(1.984--6.994)}{4.55pt}{4.82pt}{} & \HoloSegScore{3.254}{(1.651--4.451)}{4.55pt}{4.82pt}{} & \HoloSegScore{11.59}{(8.356--15.48)}{4.55pt}{4.82pt}{} & \HoloSegScore{5.766}{(4.321--7.699)}{4.55pt}{4.82pt}{} \\
\cline{3-11}
 &  &  & \HoloSegMetric{Dice} & \HoloSegScore{0.9085}{(0.8957--0.9189)}{4.55pt}{4.82pt}{} & \HoloSegScore{0.6271}{(0.5945--0.6586)}{4.55pt}{4.82pt}{} & \HoloSegScore{0.8980}{(0.8816--0.9111)}{4.55pt}{4.82pt}{} & \HoloSegScore{0.8868}{(0.8632--0.9058)}{4.55pt}{4.82pt}{} & \HoloSegScore{0.9057}{(0.8706--0.9118)}{4.55pt}{4.82pt}{} & \HoloSegScore{0.8558}{(0.8307--0.8781)}{4.55pt}{4.82pt}{} & \HoloSegScore{0.8527}{(0.8308--0.8715)}{4.55pt}{4.82pt}{} \\*
\softcline{4-11}
\HoloSegSpan{\makecell[c]{\textbf{Internal}}}{1.20cm}{0.32cm} & \HoloSegSpan{\makecell[c]{Total-\\[-0.10ex]SegmentatorV2}}{1.86cm}{0.32cm} & \HoloSegSpan{\makecell[c]{left\\[-0.10ex]iliopsoas}}{2.04cm}{0.32cm} & \HoloSegMetric{HD95} & \HoloSegScore{3.469}{(2.965--4.352)}{4.55pt}{4.82pt}{} & \HoloSegScore{19.77}{(12.85--27.97)}{4.55pt}{4.82pt}{} & \HoloSegScore{8.272}{(2.358--16.70)}{4.55pt}{4.82pt}{} & \HoloSegScore{2.982}{(2.632--3.381)}{4.55pt}{4.82pt}{} & \HoloSegScore{3.120}{(2.380--4.301)}{4.55pt}{4.82pt}{} & \HoloSegScore{20.99}{(11.58--32.82)}{4.55pt}{4.82pt}{} & \HoloSegScore{14.61}{(8.849--22.11)}{4.55pt}{4.82pt}{} \\
\cline{3-11}
 &  &  & \HoloSegMetric{Dice} & \HoloSegScore{0.8941}{(0.8700--0.9144)}{4.55pt}{4.82pt}{} & \HoloSegScore{0.5868}{(0.5478--0.6225)}{4.55pt}{4.82pt}{} & \HoloSegScore{0.8949}{(0.8730--0.9131)}{4.55pt}{4.82pt}{} & \HoloSegScore{0.8857}{(0.8605--0.9080)}{4.55pt}{4.82pt}{} & \HoloSegScore{0.9129}{(0.8888--0.9251)}{4.55pt}{4.82pt}{} & \HoloSegScore{0.8535}{(0.8258--0.8776)}{4.55pt}{4.82pt}{} & \HoloSegScore{0.8087}{(0.7801--0.8369)}{4.55pt}{4.82pt}{} \\*
\softcline{4-11}
 &  & \HoloSegSpan{\makecell[c]{right\\[-0.10ex]iliopsoas}}{2.04cm}{0.32cm} & \HoloSegMetric{HD95} & \HoloSegScore{8.183}{(3.407--14.97)}{4.55pt}{4.82pt}{} & \HoloSegScore{27.33}{(20.73--35.77)}{4.55pt}{4.82pt}{} & \HoloSegScore{2.195}{(2.015--2.425)}{4.55pt}{4.82pt}{} & \HoloSegScore{2.655}{(2.258--3.123)}{4.55pt}{4.82pt}{} & \HoloSegScore{2.695}{(1.898--5.079)}{4.55pt}{4.82pt}{} & \HoloSegScore{23.61}{(12.68--35.91)}{4.55pt}{4.82pt}{} & \HoloSegScore{26.64}{(18.84--36.68)}{4.55pt}{4.82pt}{} \\
\cline{3-11}
 &  &  & \HoloSegMetric{Dice} & \HoloSegScore{0.8690}{(0.8197--0.9134)}{4.55pt}{4.82pt}{} & \HoloSegScore{0.6046}{(0.5225--0.6758)}{4.55pt}{4.82pt}{} & \HoloSegScore{0.8650}{(0.8167--0.9080)}{4.55pt}{4.82pt}{} & \HoloSegScore{0.8801}{(0.8309--0.9220)}{4.55pt}{4.82pt}{} & \HoloSegScore{0.9276}{(0.8727--0.9907)}{4.55pt}{4.82pt}{} & \HoloSegScore{0.8661}{(0.8064--0.9100)}{4.55pt}{4.82pt}{} & \HoloSegScore{0.8717}{(0.8146--0.9135)}{4.55pt}{4.82pt}{} \\*
\softcline{4-11}
 &  & \HoloSegSpan{\makecell[c]{brain}}{2.04cm}{0.32cm} & \HoloSegMetric{HD95} & \HoloSegScore{21.11}{(9.915--36.00)}{4.55pt}{4.82pt}{} & \HoloSegScore{25.43}{(18.29--33.98)}{4.55pt}{4.82pt}{} & \HoloSegScore{6.622}{(4.652--8.810)}{4.55pt}{4.82pt}{} & \HoloSegScore{6.631}{(4.526--9.174)}{4.55pt}{4.82pt}{} & \HoloSegScore{4.507}{(0.7870--4.952)}{4.55pt}{4.82pt}{} & \HoloSegScore{53.79}{(22.81--90.11)}{4.55pt}{4.82pt}{} & \HoloSegScore{21.21}{(7.750--38.59)}{4.55pt}{4.82pt}{} \\
\cline{3-11}
 &  &  & \HoloSegMetric{Dice} & \HoloSegScore{0.7819}{(0.7223--0.8331)}{4.55pt}{4.82pt}{} & \HoloSegScore{0.03119}{(0.02192--0.04115)}{4.20pt}{4.48pt}{} & \HoloSegScore{0.7638}{(0.7146--0.8107)}{4.55pt}{4.82pt}{} & \HoloSegScore{0.8195}{(0.7595--0.8714)}{4.55pt}{4.82pt}{} & \HoloSegScore{0.8529}{(0.8518--0.8633)}{4.55pt}{4.82pt}{} & \HoloSegScore{0.7912}{(0.7434--0.8342)}{4.55pt}{4.82pt}{} & \HoloSegScore{0.7950}{(0.7474--0.8400)}{4.55pt}{4.82pt}{} \\*
\softcline{4-11}
 &  & \HoloSegSpan{\makecell[c]{skull}}{2.04cm}{0.32cm} & \HoloSegMetric{HD95} & \HoloSegScore{11.86}{(7.900--16.58)}{4.55pt}{4.82pt}{} & \HoloSegScore{108.1}{(98.57--117.5)}{4.55pt}{4.82pt}{} & \HoloSegScore{17.09}{(9.511--26.47)}{4.55pt}{4.82pt}{} & \HoloSegScore{4.548}{(2.492--7.213)}{4.55pt}{4.82pt}{} & \HoloSegScore{3.128}{(2.535--6.792)}{4.55pt}{4.82pt}{} & \HoloSegScore{110.9}{(87.08--138.1)}{4.55pt}{4.82pt}{} & \HoloSegScore{29.89}{(14.60--47.55)}{4.55pt}{4.82pt}{} \\
\cline{3-11}
 &  &  & \HoloSegMetric{Dice} & \HoloSegScore{0.8913}{(0.8653--0.9134)}{4.55pt}{4.82pt}{} & \HoloSegScore{0.1689}{(0.1502--0.1886)}{4.55pt}{4.82pt}{} & \HoloSegScore{0.8313}{(0.8111--0.8483)}{4.55pt}{4.82pt}{} & \HoloSegScore{0.9115}{(0.8879--0.9315)}{4.55pt}{4.82pt}{} & \HoloSegScore{0.9421}{(0.9249--0.9555)}{4.55pt}{4.82pt}{} & \HoloSegScore{0.6920}{(0.6632--0.7219)}{4.55pt}{4.82pt}{} & \HoloSegScore{0.8930}{(0.8667--0.9159)}{4.55pt}{4.82pt}{} \\*
\softcline{4-11}
 &  & \HoloSegSpan{\makecell[c]{right rib 4}}{2.04cm}{0.32cm} & \HoloSegMetric{HD95} & \HoloSegScore{6.637}{(4.586--9.178)}{4.55pt}{4.82pt}{} & \HoloSegScore{25.33}{(21.58--30.08)}{4.55pt}{4.82pt}{} & \HoloSegScore{4.806}{(1.918--8.383)}{4.55pt}{4.82pt}{} & \HoloSegScore{3.937}{(1.990--6.433)}{4.55pt}{4.82pt}{} & \HoloSegScore{3.302}{(1.159--5.125)}{4.55pt}{4.82pt}{} & \HoloSegScore{30.69}{(25.93--36.04)}{4.55pt}{4.82pt}{} & \HoloSegScore{7.006}{(4.311--10.66)}{4.55pt}{4.82pt}{} \\
\cline{3-11}
 &  &  & \HoloSegMetric{Dice} & \HoloSegScore{0.8835}{(0.8591--0.9044)}{4.55pt}{4.82pt}{} & \HoloSegScore{0.1436}{(0.1269--0.1606)}{4.55pt}{4.82pt}{} & \HoloSegScore{0.7976}{(0.7738--0.8181)}{4.55pt}{4.82pt}{} & \HoloSegScore{0.8925}{(0.8673--0.9156)}{4.55pt}{4.82pt}{} & \HoloSegScore{0.9367}{(0.9070--0.9693)}{4.55pt}{4.82pt}{} & \HoloSegScore{0.6803}{(0.6455--0.7143)}{4.55pt}{4.82pt}{} & \HoloSegScore{0.8570}{(0.8253--0.8863)}{4.55pt}{4.82pt}{} \\*
\softcline{4-11}
 &  & \HoloSegSpan{\makecell[c]{right rib 3}}{2.04cm}{0.32cm} & \HoloSegMetric{HD95} & \HoloSegScore{5.956}{(3.771--9.639)}{4.55pt}{4.82pt}{} & \HoloSegScore{44.79}{(36.87--53.18)}{4.55pt}{4.82pt}{} & \HoloSegScore{5.181}{(1.840--9.844)}{4.55pt}{4.82pt}{} & \HoloSegScore{4.139}{(1.816--8.162)}{4.55pt}{4.82pt}{} & \HoloSegScore{4.206}{(2.094--7.801)}{4.55pt}{4.82pt}{} & \HoloSegScore{24.38}{(21.67--27.69)}{4.55pt}{4.82pt}{} & \HoloSegScore{8.339}{(4.995--13.14)}{4.55pt}{4.82pt}{} \\
\cline{3-11}
 &  &  & \HoloSegMetric{Dice} & \HoloSegScore{0.8908}{(0.8698--0.9057)}{4.55pt}{4.82pt}{} & \HoloSegScore{0.2101}{(0.1908--0.2310)}{4.55pt}{4.82pt}{} & \HoloSegScore{0.8014}{(0.7857--0.8138)}{4.55pt}{4.82pt}{} & \HoloSegScore{0.8952}{(0.8787--0.9084)}{4.55pt}{4.82pt}{} & \HoloSegScore{0.9385}{(0.9325--0.9580)}{4.55pt}{4.82pt}{} & \HoloSegScore{0.8704}{(0.8458--0.8897)}{4.55pt}{4.82pt}{} & \HoloSegScore{0.8823}{(0.8619--0.8970)}{4.55pt}{4.82pt}{} \\*
\softcline{4-11}
 &  & \HoloSegSpan{\makecell[c]{left rib 1}}{2.04cm}{0.32cm} & \HoloSegMetric{HD95} & \HoloSegScore{3.265}{(2.990--3.608)}{4.55pt}{4.82pt}{} & \HoloSegScore{15.57}{(13.27--18.28)}{4.55pt}{4.82pt}{} & \HoloSegScore{28.19}{(16.67--40.82)}{4.55pt}{4.82pt}{} & \HoloSegScore{2.188}{(1.968--2.436)}{4.55pt}{4.82pt}{} & \HoloSegScore{1.898}{(1.879--3.600)}{4.55pt}{4.82pt}{} & \HoloSegScore{17.24}{(13.25--21.64)}{4.55pt}{4.82pt}{} & \HoloSegScore{4.183}{(3.320--5.162)}{4.55pt}{4.82pt}{} \\
\cline{3-11}
 &  &  & \HoloSegMetric{Dice} & \HoloSegScore{0.9181}{(0.9005--0.9318)}{4.55pt}{4.82pt}{} & \HoloSegScore{0.2124}{(0.1921--0.2321)}{4.55pt}{4.82pt}{} & \HoloSegScore{0.8225}{(0.8084--0.8334)}{4.55pt}{4.82pt}{} & \HoloSegScore{0.9293}{(0.9216--0.9365)}{4.55pt}{4.82pt}{} & \HoloSegScore{0.9298}{(0.9223--0.9500)}{4.55pt}{4.82pt}{} & \HoloSegScore{0.8617}{(0.8429--0.8791)}{4.55pt}{4.82pt}{} & \HoloSegScore{0.9159}{(0.9044--0.9250)}{4.55pt}{4.82pt}{} \\*
\softcline{4-11}
 &  & \HoloSegSpan{\makecell[c]{left rib 2}}{2.04cm}{0.32cm} & \HoloSegMetric{HD95} & \HoloSegScore{6.685}{(3.045--13.05)}{4.55pt}{4.82pt}{} & \HoloSegScore{19.01}{(16.43--22.00)}{4.55pt}{4.82pt}{} & \HoloSegScore{10.73}{(4.346--19.27)}{4.55pt}{4.82pt}{} & \HoloSegScore{1.957}{(1.250--3.167)}{4.55pt}{4.82pt}{} & \HoloSegScore{3.350}{(2.858--7.031)}{4.55pt}{4.82pt}{} & \HoloSegScore{12.80}{(10.12--15.75)}{4.55pt}{4.82pt}{} & \HoloSegScore{3.791}{(2.429--5.585)}{4.55pt}{4.82pt}{} \\
\cline{3-11}
 &  &  & \HoloSegMetric{Dice} & \HoloSegScore{0.8141}{(0.7853--0.8422)}{4.55pt}{4.82pt}{} & \HoloSegScore{0.2142}{(0.1932--0.2369)}{4.55pt}{4.82pt}{} & \HoloSegScore{0.8114}{(0.7879--0.8303)}{4.55pt}{4.82pt}{} & \HoloSegScore{0.9103}{(0.8906--0.9258)}{4.55pt}{4.82pt}{} & \HoloSegScore{0.9308}{(0.9294--0.9401)}{4.55pt}{4.82pt}{} & \HoloSegScore{0.7546}{(0.7313--0.7765)}{4.55pt}{4.82pt}{} & \HoloSegScore{0.8707}{(0.8492--0.8889)}{4.55pt}{4.82pt}{} \\*
\softcline{4-11}
 &  & \HoloSegSpan{\makecell[c]{left rib 3}}{2.04cm}{0.32cm} & \HoloSegMetric{HD95} & \HoloSegScore{16.17}{(13.26--19.21)}{4.55pt}{4.82pt}{} & \HoloSegScore{24.00}{(20.82--27.40)}{4.55pt}{4.82pt}{} & \HoloSegScore{4.588}{(2.412--7.920)}{4.55pt}{4.82pt}{} & \HoloSegScore{2.752}{(1.890--3.717)}{4.55pt}{4.82pt}{} & \HoloSegScore{2.421}{(0.4370--5.045)}{4.55pt}{4.82pt}{} & \HoloSegScore{23.74}{(19.70--30.03)}{4.55pt}{4.82pt}{} & \HoloSegScore{8.192}{(6.684--9.722)}{4.55pt}{4.82pt}{} \\
\cline{3-11}
 &  &  & \HoloSegMetric{Dice} & \HoloSegScore{0.8865}{(0.8585--0.9123)}{4.55pt}{4.82pt}{} & \HoloSegScore{0.2364}{(0.2125--0.2600)}{4.55pt}{4.82pt}{} & \HoloSegScore{0.8231}{(0.7978--0.8447)}{4.55pt}{4.82pt}{} & \HoloSegScore{0.9038}{(0.8797--0.9259)}{4.55pt}{4.82pt}{} & \HoloSegScore{0.9358}{(0.9241--0.9606)}{4.55pt}{4.82pt}{} & \HoloSegScore{0.6584}{(0.6371--0.6801)}{4.55pt}{4.82pt}{} & \HoloSegScore{0.8737}{(0.8481--0.8946)}{4.55pt}{4.82pt}{} \\*
\softcline{4-11}
 &  & \HoloSegSpan{\makecell[c]{left rib 4}}{2.04cm}{0.32cm} & \HoloSegMetric{HD95} & \HoloSegScore{6.645}{(5.191--8.341)}{4.55pt}{4.82pt}{} & \HoloSegScore{20.84}{(18.71--23.16)}{4.55pt}{4.82pt}{} & \HoloSegScore{3.987}{(2.313--6.419)}{4.55pt}{4.82pt}{} & \HoloSegScore{3.217}{(2.096--4.544)}{4.55pt}{4.82pt}{} & \HoloSegScore{2.632}{(2.459--4.368)}{4.55pt}{4.82pt}{} & \HoloSegScore{98.73}{(88.94--108.7)}{4.55pt}{4.82pt}{} & \HoloSegScore{9.200}{(7.387--11.14)}{4.55pt}{4.82pt}{} \\
\hline
\pagebreak[4]
 &  &  & \HoloSegMetric{Dice} & \HoloSegScore{0.8706}{(0.8446--0.8963)}{4.55pt}{4.82pt}{} & \HoloSegScore{0.2265}{(0.2018--0.2540)}{4.55pt}{4.82pt}{} & \HoloSegScore{0.8263}{(0.8057--0.8435)}{4.55pt}{4.82pt}{} & \HoloSegScore{0.8809}{(0.8512--0.9064)}{4.55pt}{4.82pt}{} & \HoloSegScore{0.8972}{(0.8888--0.9005)}{4.55pt}{4.82pt}{} & \HoloSegScore{0.7741}{(0.7433--0.8011)}{4.55pt}{4.82pt}{} & \HoloSegScore{0.8428}{(0.8149--0.8671)}{4.55pt}{4.82pt}{} \\*
\softcline{4-11}
 &  & \HoloSegSpan{\makecell[c]{left rib 5}}{2.04cm}{0.32cm} & \HoloSegMetric{HD95} & \HoloSegScore{8.756}{(5.338--14.31)}{4.55pt}{4.82pt}{} & \HoloSegScore{23.95}{(20.78--28.11)}{4.55pt}{4.82pt}{} & \HoloSegScore{3.809}{(2.862--4.988)}{4.55pt}{4.82pt}{} & \HoloSegScore{4.101}{(3.036--5.231)}{4.55pt}{4.82pt}{} & \HoloSegScore{3.217}{(2.803--3.879)}{4.55pt}{4.82pt}{} & \HoloSegScore{27.78}{(21.23--34.42)}{4.55pt}{4.82pt}{} & \HoloSegScore{5.496}{(4.135--7.114)}{4.55pt}{4.82pt}{} \\
\cline{3-11}
 &  &  & \HoloSegMetric{Dice} & \HoloSegScore{0.8563}{(0.8259--0.8840)}{4.55pt}{4.82pt}{} & \HoloSegScore{0.2535}{(0.2286--0.2784)}{4.55pt}{4.82pt}{} & \HoloSegScore{0.8229}{(0.7970--0.8469)}{4.55pt}{4.82pt}{} & \HoloSegScore{0.8760}{(0.8468--0.9037)}{4.55pt}{4.82pt}{} & \HoloSegScore{0.9078}{(0.8978--0.9184)}{4.55pt}{4.82pt}{} & \HoloSegScore{0.8310}{(0.8048--0.8534)}{4.55pt}{4.82pt}{} & \HoloSegScore{0.8479}{(0.8215--0.8707)}{4.55pt}{4.82pt}{} \\*
\softcline{4-11}
 &  & \HoloSegSpan{\makecell[c]{left rib 6}}{2.04cm}{0.32cm} & \HoloSegMetric{HD95} & \HoloSegScore{7.988}{(6.143--10.16)}{4.55pt}{4.82pt}{} & \HoloSegScore{27.76}{(23.23--33.31)}{4.55pt}{4.82pt}{} & \HoloSegScore{3.372}{(2.565--4.285)}{4.55pt}{4.82pt}{} & \HoloSegScore{6.129}{(4.683--7.602)}{4.55pt}{4.82pt}{} & \HoloSegScore{5.056}{(3.764--6.348)}{4.55pt}{4.82pt}{} & \HoloSegScore{19.13}{(15.61--23.42)}{4.55pt}{4.82pt}{} & \HoloSegScore{5.920}{(4.451--7.858)}{4.55pt}{4.82pt}{} \\
\cline{3-11}
 &  &  & \HoloSegMetric{Dice} & \HoloSegScore{0.8694}{(0.8444--0.8922)}{4.55pt}{4.82pt}{} & \HoloSegScore{0.2819}{(0.2563--0.3076)}{4.55pt}{4.82pt}{} & \HoloSegScore{0.8508}{(0.8301--0.8697)}{4.55pt}{4.82pt}{} & \HoloSegScore{0.8815}{(0.8536--0.9051)}{4.55pt}{4.82pt}{} & \HoloSegScore{0.9022}{(0.8880--0.9182)}{4.55pt}{4.82pt}{} & \HoloSegScore{0.8940}{(0.8721--0.9120)}{4.55pt}{4.82pt}{} & \HoloSegScore{0.9007}{(0.8839--0.9162)}{4.55pt}{4.82pt}{} \\*
\softcline{4-11}
 &  & \HoloSegSpan{\makecell[c]{left rib 7}}{2.04cm}{0.32cm} & \HoloSegMetric{HD95} & \HoloSegScore{7.803}{(6.262--9.687)}{4.55pt}{4.82pt}{} & \HoloSegScore{25.70}{(22.00--30.04)}{4.55pt}{4.82pt}{} & \HoloSegScore{3.525}{(2.513--4.760)}{4.55pt}{4.82pt}{} & \HoloSegScore{9.493}{(7.060--12.47)}{4.55pt}{4.82pt}{} & \HoloSegScore{3.938}{(3.223--5.417)}{4.55pt}{4.82pt}{} & \HoloSegScore{14.05}{(10.80--17.82)}{4.55pt}{4.82pt}{} & \HoloSegScore{6.631}{(5.240--8.094)}{4.55pt}{4.82pt}{} \\
\cline{3-11}
 &  &  & \HoloSegMetric{Dice} & \HoloSegScore{0.8788}{(0.8541--0.8997)}{4.55pt}{4.82pt}{} & \HoloSegScore{0.2856}{(0.2587--0.3101)}{4.55pt}{4.82pt}{} & \HoloSegScore{0.8478}{(0.8257--0.8677)}{4.55pt}{4.82pt}{} & \HoloSegScore{0.9067}{(0.8885--0.9217)}{4.55pt}{4.82pt}{} & \HoloSegScore{0.8924}{(0.8813--0.8938)}{4.55pt}{4.82pt}{} & \HoloSegScore{0.9058}{(0.8875--0.9206)}{4.55pt}{4.82pt}{} & \HoloSegScore{0.9185}{(0.9073--0.9281)}{4.55pt}{4.82pt}{} \\*
\softcline{4-11}
 &  & \HoloSegSpan{\makecell[c]{left rib 8}}{2.04cm}{0.32cm} & \HoloSegMetric{HD95} & \HoloSegScore{8.642}{(7.200--10.25)}{4.55pt}{4.82pt}{} & \HoloSegScore{26.20}{(22.18--30.69)}{4.55pt}{4.82pt}{} & \HoloSegScore{3.597}{(2.523--4.865)}{4.55pt}{4.82pt}{} & \HoloSegScore{5.646}{(4.354--7.131)}{4.55pt}{4.82pt}{} & \HoloSegScore{4.863}{(3.854--7.132)}{4.55pt}{4.82pt}{} & \HoloSegScore{6.351}{(4.401--8.733)}{4.55pt}{4.82pt}{} & \HoloSegScore{4.440}{(3.344--5.662)}{4.55pt}{4.82pt}{} \\
\cline{3-11}
 &  &  & \HoloSegMetric{Dice} & \HoloSegScore{0.8856}{(0.8587--0.9082)}{4.55pt}{4.82pt}{} & \HoloSegScore{0.2709}{(0.2454--0.2952)}{4.55pt}{4.82pt}{} & \HoloSegScore{0.8499}{(0.8282--0.8693)}{4.55pt}{4.82pt}{} & \HoloSegScore{0.9003}{(0.8781--0.9175)}{4.55pt}{4.82pt}{} & \HoloSegScore{0.9002}{(0.8980--0.9268)}{4.55pt}{4.82pt}{} & \HoloSegScore{0.8958}{(0.8809--0.9092)}{4.55pt}{4.82pt}{} & \HoloSegScore{0.9144}{(0.9010--0.9259)}{4.55pt}{4.82pt}{} \\*
\softcline{4-11}
 &  & \HoloSegSpan{\makecell[c]{left rib 9}}{2.04cm}{0.32cm} & \HoloSegMetric{HD95} & \HoloSegScore{8.355}{(6.245--11.35)}{4.55pt}{4.82pt}{} & \HoloSegScore{29.41}{(25.05--34.26)}{4.55pt}{4.82pt}{} & \HoloSegScore{4.865}{(2.512--7.967)}{4.55pt}{4.82pt}{} & \HoloSegScore{7.087}{(5.142--9.239)}{4.55pt}{4.82pt}{} & \HoloSegScore{6.396}{(4.774--7.760)}{4.55pt}{4.82pt}{} & \HoloSegScore{19.45}{(15.80--23.61)}{4.55pt}{4.82pt}{} & \HoloSegScore{5.921}{(4.490--7.351)}{4.55pt}{4.82pt}{} \\
\cline{3-11}
 &  &  & \HoloSegMetric{Dice} & \HoloSegScore{0.8808}{(0.8525--0.9068)}{4.55pt}{4.82pt}{} & \HoloSegScore{0.2551}{(0.2333--0.2782)}{4.55pt}{4.82pt}{} & \HoloSegScore{0.8556}{(0.8344--0.8733)}{4.55pt}{4.82pt}{} & \HoloSegScore{0.8972}{(0.8738--0.9166)}{4.55pt}{4.82pt}{} & \HoloSegScore{0.8817}{(0.8543--0.8967)}{4.55pt}{4.82pt}{} & \HoloSegScore{0.8394}{(0.8201--0.8570)}{4.55pt}{4.82pt}{} & \HoloSegScore{0.9108}{(0.8927--0.9252)}{4.55pt}{4.82pt}{} \\*
\softcline{4-11}
 &  & \HoloSegSpan{\makecell[c]{left rib 10}}{2.04cm}{0.32cm} & \HoloSegMetric{HD95} & \HoloSegScore{9.876}{(7.504--12.70)}{4.55pt}{4.82pt}{} & \HoloSegScore{28.24}{(23.49--33.47)}{4.55pt}{4.82pt}{} & \HoloSegScore{5.692}{(3.192--9.352)}{4.55pt}{4.82pt}{} & \HoloSegScore{8.802}{(6.136--11.90)}{4.55pt}{4.82pt}{} & \HoloSegScore{5.867}{(4.339--8.097)}{4.55pt}{4.82pt}{} & \HoloSegScore{65.85}{(56.31--75.93)}{4.55pt}{4.82pt}{} & \HoloSegScore{6.729}{(5.206--8.463)}{4.55pt}{4.82pt}{} \\
\cline{3-11}
 &  &  & \HoloSegMetric{Dice} & \HoloSegScore{0.8929}{(0.8684--0.9136)}{4.55pt}{4.82pt}{} & \HoloSegScore{0.2634}{(0.2408--0.2875)}{4.55pt}{4.82pt}{} & \HoloSegScore{0.8506}{(0.8314--0.8646)}{4.55pt}{4.82pt}{} & \HoloSegScore{0.8932}{(0.8743--0.9109)}{4.55pt}{4.82pt}{} & \HoloSegScore{0.8913}{(0.8783--0.9122)}{4.55pt}{4.82pt}{} & \HoloSegScore{0.7983}{(0.7696--0.8266)}{4.55pt}{4.82pt}{} & \HoloSegScore{0.9088}{(0.8916--0.9234)}{4.55pt}{4.82pt}{} \\*
\softcline{4-11}
 &  & \HoloSegSpan{\makecell[c]{left rib 11}}{2.04cm}{0.32cm} & \HoloSegMetric{HD95} & \HoloSegScore{6.830}{(5.198--8.740)}{4.55pt}{4.82pt}{} & \HoloSegScore{23.54}{(19.68--28.03)}{4.55pt}{4.82pt}{} & \HoloSegScore{5.530}{(2.463--9.357)}{4.55pt}{4.82pt}{} & \HoloSegScore{7.459}{(5.193--10.13)}{4.55pt}{4.82pt}{} & \HoloSegScore{6.223}{(6.171--9.228)}{4.55pt}{4.82pt}{} & \HoloSegScore{42.07}{(30.45--53.84)}{4.55pt}{4.82pt}{} & \HoloSegScore{3.975}{(2.589--5.561)}{4.55pt}{4.82pt}{} \\
\cline{3-11}
 &  &  & \HoloSegMetric{Dice} & \HoloSegScore{0.8759}{(0.8504--0.9002)}{4.55pt}{4.82pt}{} & \HoloSegScore{0.1967}{(0.1723--0.2189)}{4.55pt}{4.82pt}{} & \HoloSegScore{0.8102}{(0.7896--0.8295)}{4.55pt}{4.82pt}{} & \HoloSegScore{0.8667}{(0.8357--0.8941)}{4.55pt}{4.82pt}{} & \HoloSegScore{0.8716}{(0.8613--0.9009)}{4.55pt}{4.82pt}{} & \HoloSegScore{0.8500}{(0.8219--0.8762)}{4.55pt}{4.82pt}{} & \HoloSegScore{0.8107}{(0.7752--0.8419)}{4.55pt}{4.82pt}{} \\*
\softcline{4-11}
 &  & \HoloSegSpan{\makecell[c]{left rib 12}}{2.04cm}{0.32cm} & \HoloSegMetric{HD95} & \HoloSegScore{6.053}{(4.099--8.407)}{4.55pt}{4.82pt}{} & \HoloSegScore{25.06}{(20.72--30.51)}{4.55pt}{4.82pt}{} & \HoloSegScore{11.34}{(4.729--18.86)}{4.55pt}{4.82pt}{} & \HoloSegScore{5.280}{(3.598--7.335)}{4.55pt}{4.82pt}{} & \HoloSegScore{5.887}{(5.525--7.483)}{4.55pt}{4.82pt}{} & \HoloSegScore{36.85}{(26.15--49.40)}{4.55pt}{4.82pt}{} & \HoloSegScore{19.24}{(15.55--23.64)}{4.55pt}{4.82pt}{} \\
\cline{3-11}
 &  &  & \HoloSegMetric{Dice} & \HoloSegScore{0.8911}{(0.8722--0.9053)}{4.55pt}{4.82pt}{} & \HoloSegScore{0.1657}{(0.1491--0.1840)}{4.55pt}{4.82pt}{} & \HoloSegScore{0.7913}{(0.7763--0.8048)}{4.55pt}{4.82pt}{} & \HoloSegScore{0.8978}{(0.8791--0.9131)}{4.55pt}{4.82pt}{} & \HoloSegScore{0.9371}{(0.9249--0.9709)}{4.55pt}{4.82pt}{} & \HoloSegScore{0.8616}{(0.8407--0.8820)}{4.55pt}{4.82pt}{} & \HoloSegScore{0.8923}{(0.8717--0.9091)}{4.55pt}{4.82pt}{} \\*
\softcline{4-11}
 &  & \HoloSegSpan{\makecell[c]{right rib 1}}{2.04cm}{0.32cm} & \HoloSegMetric{HD95} & \HoloSegScore{8.505}{(3.562--14.80)}{4.55pt}{4.82pt}{} & \HoloSegScore{17.12}{(14.64--20.05)}{4.55pt}{4.82pt}{} & \HoloSegScore{37.74}{(24.34--52.42)}{4.55pt}{4.82pt}{} & \HoloSegScore{2.134}{(1.801--2.550)}{4.55pt}{4.82pt}{} & \HoloSegScore{1.354}{(0.6460--1.928)}{4.55pt}{4.82pt}{} & \HoloSegScore{14.90}{(10.62--20.60)}{4.55pt}{4.82pt}{} & \HoloSegScore{2.772}{(2.156--3.606)}{4.55pt}{4.82pt}{} \\
\cline{3-11}
 &  &  & \HoloSegMetric{Dice} & \HoloSegScore{0.9096}{(0.8945--0.9226)}{4.55pt}{4.82pt}{} & \HoloSegScore{0.1562}{(0.1382--0.1729)}{4.55pt}{4.82pt}{} & \HoloSegScore{0.8074}{(0.7942--0.8175)}{4.55pt}{4.82pt}{} & \HoloSegScore{0.9211}{(0.9035--0.9329)}{4.55pt}{4.82pt}{} & \HoloSegScore{0.9481}{(0.9339--0.9739)}{4.55pt}{4.82pt}{} & \HoloSegScore{0.8497}{(0.8326--0.8644)}{4.55pt}{4.82pt}{} & \HoloSegScore{0.9091}{(0.8937--0.9198)}{4.55pt}{4.82pt}{} \\*
\softcline{4-11}
\HoloSegSpan{\makecell[c]{\textbf{Internal}}}{1.20cm}{0.32cm} & \HoloSegSpan{\makecell[c]{Total-\\[-0.10ex]SegmentatorV2}}{1.86cm}{0.32cm} & \HoloSegSpan{\makecell[c]{right rib 2}}{2.04cm}{0.32cm} & \HoloSegMetric{HD95} & \HoloSegScore{4.638}{(2.820--8.246)}{4.55pt}{4.82pt}{} & \HoloSegScore{22.92}{(19.21--27.13)}{4.55pt}{4.82pt}{} & \HoloSegScore{8.587}{(2.858--15.99)}{4.55pt}{4.82pt}{} & \HoloSegScore{1.503}{(1.180--1.894)}{4.55pt}{4.82pt}{} & \HoloSegScore{2.849}{(1.371--4.467)}{4.55pt}{4.82pt}{} & \HoloSegScore{13.63}{(11.79--15.43)}{4.55pt}{4.82pt}{} & \HoloSegScore{2.731}{(1.848--3.880)}{4.55pt}{4.82pt}{} \\
\cline{3-11}
 &  &  & \HoloSegMetric{Dice} & \HoloSegScore{0.8574}{(0.8298--0.8844)}{4.55pt}{4.82pt}{} & \HoloSegScore{0.1779}{(0.1555--0.2003)}{4.55pt}{4.82pt}{} & \HoloSegScore{0.8060}{(0.7789--0.8292)}{4.55pt}{4.82pt}{} & \HoloSegScore{0.8570}{(0.8176--0.8899)}{4.55pt}{4.82pt}{} & \HoloSegScore{0.8977}{(0.8693--0.9254)}{4.55pt}{4.82pt}{} & \HoloSegScore{0.6700}{(0.6333--0.7094)}{4.55pt}{4.82pt}{} & \HoloSegScore{0.8730}{(0.8460--0.8968)}{4.55pt}{4.82pt}{} \\*
\softcline{4-11}
 &  & \HoloSegSpan{\makecell[c]{right rib 5}}{2.04cm}{0.32cm} & \HoloSegMetric{HD95} & \HoloSegScore{15.20}{(6.169--30.30)}{4.55pt}{4.82pt}{} & \HoloSegScore{34.49}{(27.02--43.97)}{4.55pt}{4.82pt}{} & \HoloSegScore{4.887}{(2.613--7.675)}{4.55pt}{4.82pt}{} & \HoloSegScore{4.538}{(2.728--7.287)}{4.55pt}{4.82pt}{} & \HoloSegScore{3.433}{(0.5940--6.004)}{4.55pt}{4.82pt}{} & \HoloSegScore{23.23}{(18.45--28.03)}{4.55pt}{4.82pt}{} & \HoloSegScore{5.944}{(3.648--9.037)}{4.55pt}{4.82pt}{} \\
\cline{3-11}
 &  &  & \HoloSegMetric{Dice} & \HoloSegScore{0.8702}{(0.8458--0.8962)}{4.55pt}{4.82pt}{} & \HoloSegScore{0.1726}{(0.1506--0.1964)}{4.55pt}{4.82pt}{} & \HoloSegScore{0.8388}{(0.8212--0.8562)}{4.55pt}{4.82pt}{} & \HoloSegScore{0.8718}{(0.8437--0.8963)}{4.55pt}{4.82pt}{} & \HoloSegScore{0.9311}{(0.9155--0.9567)}{4.55pt}{4.82pt}{} & \HoloSegScore{0.8506}{(0.8282--0.8712)}{4.55pt}{4.82pt}{} & \HoloSegScore{0.8952}{(0.8780--0.9110)}{4.55pt}{4.82pt}{} \\*
\softcline{4-11}
 &  & \HoloSegSpan{\makecell[c]{right rib 6}}{2.04cm}{0.32cm} & \HoloSegMetric{HD95} & \HoloSegScore{8.293}{(6.751--9.878)}{4.55pt}{4.82pt}{} & \HoloSegScore{90.16}{(77.60--104.4)}{4.55pt}{4.82pt}{} & \HoloSegScore{4.387}{(2.543--7.452)}{4.55pt}{4.82pt}{} & \HoloSegScore{9.197}{(6.653--12.36)}{4.55pt}{4.82pt}{} & \HoloSegScore{3.547}{(0.9560--4.877)}{4.55pt}{4.82pt}{} & \HoloSegScore{20.38}{(16.14--25.67)}{4.55pt}{4.82pt}{} & \HoloSegScore{6.314}{(3.702--9.700)}{4.55pt}{4.82pt}{} \\
\cline{3-11}
 &  &  & \HoloSegMetric{Dice} & \HoloSegScore{0.8722}{(0.8426--0.8973)}{4.55pt}{4.82pt}{} & \HoloSegScore{0.2241}{(0.2027--0.2462)}{4.55pt}{4.82pt}{} & \HoloSegScore{0.8655}{(0.8522--0.8774)}{4.55pt}{4.82pt}{} & \HoloSegScore{0.8974}{(0.8730--0.9178)}{4.55pt}{4.82pt}{} & \HoloSegScore{0.9167}{(0.9144--0.9329)}{4.55pt}{4.82pt}{} & \HoloSegScore{0.8640}{(0.8492--0.8771)}{4.55pt}{4.82pt}{} & \HoloSegScore{0.8888}{(0.8689--0.9053)}{4.55pt}{4.82pt}{} \\*
\softcline{4-11}
 &  & \HoloSegSpan{\makecell[c]{right rib 7}}{2.04cm}{0.32cm} & \HoloSegMetric{HD95} & \HoloSegScore{9.559}{(7.457--12.17)}{4.55pt}{4.82pt}{} & \HoloSegScore{27.94}{(23.17--33.30)}{4.55pt}{4.82pt}{} & \HoloSegScore{4.112}{(2.582--6.362)}{4.55pt}{4.82pt}{} & \HoloSegScore{8.399}{(6.165--11.03)}{4.55pt}{4.82pt}{} & \HoloSegScore{5.448}{(3.359--9.480)}{4.55pt}{4.82pt}{} & \HoloSegScore{28.45}{(22.88--34.32)}{4.55pt}{4.82pt}{} & \HoloSegScore{11.47}{(8.975--14.11)}{4.55pt}{4.82pt}{} \\
\cline{3-11}
 &  &  & \HoloSegMetric{Dice} & \HoloSegScore{0.8730}{(0.8447--0.8977)}{4.55pt}{4.82pt}{} & \HoloSegScore{0.2378}{(0.2166--0.2611)}{4.55pt}{4.82pt}{} & \HoloSegScore{0.8625}{(0.8506--0.8737)}{4.55pt}{4.82pt}{} & \HoloSegScore{0.8954}{(0.8736--0.9146)}{4.55pt}{4.82pt}{} & \HoloSegScore{0.9272}{(0.9141--0.9514)}{4.55pt}{4.82pt}{} & \HoloSegScore{0.8898}{(0.8733--0.9045)}{4.55pt}{4.82pt}{} & \HoloSegScore{0.8928}{(0.8809--0.9040)}{4.55pt}{4.82pt}{} \\*
\softcline{4-11}
 &  & \HoloSegSpan{\makecell[c]{right rib 8}}{2.04cm}{0.32cm} & \HoloSegMetric{HD95} & \HoloSegScore{13.62}{(8.421--20.43)}{4.55pt}{4.82pt}{} & \HoloSegScore{30.25}{(25.81--35.25)}{4.55pt}{4.82pt}{} & \HoloSegScore{4.998}{(2.936--7.500)}{4.55pt}{4.82pt}{} & \HoloSegScore{7.458}{(5.281--10.23)}{4.55pt}{4.82pt}{} & \HoloSegScore{3.385}{(1.281--7.351)}{4.55pt}{4.82pt}{} & \HoloSegScore{14.56}{(11.40--18.28)}{4.55pt}{4.82pt}{} & \HoloSegScore{11.75}{(9.435--14.33)}{4.55pt}{4.82pt}{} \\
\cline{3-11}
 &  &  & \HoloSegMetric{Dice} & \HoloSegScore{0.8720}{(0.8423--0.8980)}{4.55pt}{4.82pt}{} & \HoloSegScore{0.2691}{(0.2478--0.2895)}{4.55pt}{4.82pt}{} & \HoloSegScore{0.8676}{(0.8524--0.8798)}{4.55pt}{4.82pt}{} & \HoloSegScore{0.8960}{(0.8739--0.9147)}{4.55pt}{4.82pt}{} & \HoloSegScore{0.9232}{(0.9033--0.9426)}{4.55pt}{4.82pt}{} & \HoloSegScore{0.8439}{(0.8258--0.8615)}{4.55pt}{4.82pt}{} & \HoloSegScore{0.8973}{(0.8816--0.9106)}{4.55pt}{4.82pt}{} \\*
\softcline{4-11}
 &  & \HoloSegSpan{\makecell[c]{right rib 9}}{2.04cm}{0.32cm} & \HoloSegMetric{HD95} & \HoloSegScore{14.30}{(8.937--22.34)}{4.55pt}{4.82pt}{} & \HoloSegScore{30.94}{(25.91--36.90)}{4.55pt}{4.82pt}{} & \HoloSegScore{4.152}{(2.465--6.432)}{4.55pt}{4.82pt}{} & \HoloSegScore{7.299}{(5.443--9.486)}{4.55pt}{4.82pt}{} & \HoloSegScore{6.475}{(5.652--8.120)}{4.55pt}{4.82pt}{} & \HoloSegScore{28.28}{(25.38--31.41)}{4.55pt}{4.82pt}{} & \HoloSegScore{12.66}{(10.64--14.81)}{4.55pt}{4.82pt}{} \\
\cline{3-11}
 &  &  & \HoloSegMetric{Dice} & \HoloSegScore{0.8871}{(0.8618--0.9082)}{4.55pt}{4.82pt}{} & \HoloSegScore{0.2549}{(0.2331--0.2780)}{4.55pt}{4.82pt}{} & \HoloSegScore{0.8711}{(0.8603--0.8795)}{4.55pt}{4.82pt}{} & \HoloSegScore{0.8966}{(0.8724--0.9169)}{4.55pt}{4.82pt}{} & \HoloSegScore{0.9227}{(0.8744--0.9341)}{4.55pt}{4.82pt}{} & \HoloSegScore{0.7202}{(0.6911--0.7481)}{4.55pt}{4.82pt}{} & \HoloSegScore{0.8156}{(0.7885--0.8426)}{4.55pt}{4.82pt}{} \\*
\softcline{4-11}
 &  & \HoloSegSpan{\makecell[c]{right rib 10}}{2.04cm}{0.32cm} & \HoloSegMetric{HD95} & \HoloSegScore{35.12}{(21.54--51.64)}{4.55pt}{4.82pt}{} & \HoloSegScore{45.95}{(38.02--54.56)}{4.55pt}{4.82pt}{} & \HoloSegScore{4.713}{(2.780--7.575)}{4.55pt}{4.82pt}{} & \HoloSegScore{7.605}{(5.511--9.682)}{4.55pt}{4.82pt}{} & \HoloSegScore{3.581}{(2.937--5.813)}{4.55pt}{4.82pt}{} & \HoloSegScore{26.76}{(24.82--28.74)}{4.55pt}{4.82pt}{} & \HoloSegScore{8.484}{(6.642--10.41)}{4.55pt}{4.82pt}{} \\
\cline{3-11}
 &  &  & \HoloSegMetric{Dice} & \HoloSegScore{0.8790}{(0.8484--0.9040)}{4.55pt}{4.82pt}{} & \HoloSegScore{0.2291}{(0.2077--0.2503)}{4.55pt}{4.82pt}{} & \HoloSegScore{0.8407}{(0.8199--0.8575)}{4.55pt}{4.82pt}{} & \HoloSegScore{0.8715}{(0.8437--0.8955)}{4.55pt}{4.82pt}{} & \HoloSegScore{0.9183}{(0.8982--0.9308)}{4.55pt}{4.82pt}{} & \HoloSegScore{0.6799}{(0.6369--0.7193)}{4.55pt}{4.82pt}{} & \HoloSegScore{0.8891}{(0.8629--0.9140)}{4.55pt}{4.82pt}{} \\*
\softcline{4-11}
 &  & \HoloSegSpan{\makecell[c]{right rib 11}}{2.04cm}{0.32cm} & \HoloSegMetric{HD95} & \HoloSegScore{7.688}{(5.780--9.855)}{4.55pt}{4.82pt}{} & \HoloSegScore{37.96}{(31.48--45.05)}{4.55pt}{4.82pt}{} & \HoloSegScore{4.217}{(2.271--7.623)}{4.55pt}{4.82pt}{} & \HoloSegScore{8.350}{(5.853--10.99)}{4.55pt}{4.82pt}{} & \HoloSegScore{4.356}{(0.4170--4.400)}{4.55pt}{4.82pt}{} & \HoloSegScore{20.94}{(15.93--26.59)}{4.55pt}{4.82pt}{} & \HoloSegScore{3.456}{(2.386--4.726)}{4.55pt}{4.82pt}{} \\
\cline{3-11}
 &  &  & \HoloSegMetric{Dice} & \HoloSegScore{0.8701}{(0.8410--0.8953)}{4.55pt}{4.82pt}{} & \HoloSegScore{0.1270}{(0.1112--0.1431)}{4.55pt}{4.82pt}{} & \HoloSegScore{0.8076}{(0.7877--0.8256)}{4.55pt}{4.82pt}{} & \HoloSegScore{0.8615}{(0.8307--0.8897)}{4.55pt}{4.82pt}{} & \HoloSegScore{0.9088}{(0.9010--0.9399)}{4.55pt}{4.82pt}{} & \HoloSegScore{0.8521}{(0.8229--0.8787)}{4.55pt}{4.82pt}{} & \HoloSegScore{0.8854}{(0.8604--0.9065)}{4.55pt}{4.82pt}{} \\*
\softcline{4-11}
 &  & \HoloSegSpan{\makecell[c]{right rib 12}}{2.04cm}{0.32cm} & \HoloSegMetric{HD95} & \HoloSegScore{9.898}{(5.946--14.86)}{4.55pt}{4.82pt}{} & \HoloSegScore{35.99}{(29.24--43.45)}{4.55pt}{4.82pt}{} & \HoloSegScore{9.969}{(3.906--17.81)}{4.55pt}{4.82pt}{} & \HoloSegScore{6.963}{(4.587--9.889)}{4.55pt}{4.82pt}{} & \HoloSegScore{4.602}{(1.213--4.969)}{4.55pt}{4.82pt}{} & \HoloSegScore{31.12}{(20.25--42.57)}{4.55pt}{4.82pt}{} & \HoloSegScore{8.049}{(4.722--12.49)}{4.55pt}{4.82pt}{} \\
\cline{3-11}
 &  &  & \HoloSegMetric{Dice} & \HoloSegScore{0.8878}{(0.8672--0.9058)}{4.55pt}{4.82pt}{} & \HoloSegScore{0.0002803}{(0.0001041--0.0005131)}{3.52pt}{3.80pt}{} & \HoloSegScore{0.8530}{(0.8261--0.8791)}{4.55pt}{4.82pt}{} & \HoloSegScore{0.8923}{(0.8686--0.9131)}{4.55pt}{4.82pt}{} & \HoloSegScore{0.9031}{(0.8827--0.9161)}{4.55pt}{4.82pt}{} & \HoloSegScore{0.8842}{(0.8608--0.9049)}{4.55pt}{4.82pt}{} & \HoloSegScore{0.8658}{(0.8366--0.8924)}{4.55pt}{4.82pt}{} \\*
\softcline{4-11}
 &  & \HoloSegSpan{\makecell[c]{sternum}}{2.04cm}{0.32cm} & \HoloSegMetric{HD95} & \HoloSegScore{4.628}{(3.461--6.173)}{4.55pt}{4.82pt}{} & \HoloSegScore{146.8}{(141.4--152.3)}{4.55pt}{4.82pt}{} & \HoloSegScore{13.71}{(3.583--29.32)}{4.55pt}{4.82pt}{} & \HoloSegScore{3.837}{(2.679--5.293)}{4.55pt}{4.82pt}{} & \HoloSegScore{3.394}{(1.041--3.407)}{4.55pt}{4.82pt}{} & \HoloSegScore{7.751}{(5.016--11.23)}{4.55pt}{4.82pt}{} & \HoloSegScore{3.400}{(2.433--4.728)}{4.55pt}{4.82pt}{} \\
\hline
\pagebreak[4]
 &  &  & \HoloSegMetric{Dice} & \HoloSegScore{0.8416}{(0.8217--0.8590)}{4.55pt}{4.82pt}{} & \HoloSegScore{0.003181}{(0.002157--0.004239)}{3.85pt}{4.12pt}{} & \HoloSegScore{0.7986}{(0.7800--0.8155)}{4.55pt}{4.82pt}{} & \HoloSegScore{0.8186}{(0.7952--0.8384)}{4.55pt}{4.82pt}{} & \HoloSegScore{0.8630}{(0.8490--0.8843)}{4.55pt}{4.82pt}{} & \HoloSegScore{0.8144}{(0.7938--0.8327)}{4.55pt}{4.82pt}{} & \HoloSegScore{0.8223}{(0.8033--0.8392)}{4.55pt}{4.82pt}{} \\*
\softcline{4-11}
 & \HoloSegSpan{\makecell[c]{Total-\\[-0.10ex]SegmentatorV2}}{1.86cm}{0.32cm} & \HoloSegSpan{\makecell[c]{costal\\[-0.10ex]cartilage}}{2.04cm}{0.32cm} & \HoloSegMetric{HD95} & \HoloSegScore{8.004}{(5.274--11.20)}{4.55pt}{4.82pt}{} & \HoloSegScore{192.4}{(182.4--203.0)}{4.55pt}{4.82pt}{} & \HoloSegScore{8.492}{(4.494--13.81)}{4.55pt}{4.82pt}{} & \HoloSegScore{5.949}{(4.279--7.978)}{4.55pt}{4.82pt}{} & \HoloSegScore{5.372}{(4.728--7.700)}{4.55pt}{4.82pt}{} & \HoloSegScore{9.422}{(6.533--12.97)}{4.55pt}{4.82pt}{} & \HoloSegScore{7.822}{(5.481--10.77)}{4.55pt}{4.82pt}{} \\
\cline{2-11}
 &  &  & \HoloSegMetric{Dice} & \HoloSegScore{0.8410}{(0.8269--0.8530)}{4.55pt}{4.82pt}{} & \HoloSegScore{0.5967}{(0.5461--0.6355)}{4.55pt}{4.82pt}{} & \HoloSegScore{0.8636}{(0.8472--0.8779)}{4.55pt}{4.82pt}{} & \HoloSegScore{0.8581}{(0.8440--0.8712)}{4.55pt}{4.82pt}{} & \HoloSegScore{0.8562}{(0.8432--0.8676)}{4.55pt}{4.82pt}{} & \HoloSegScore{0.8634}{(0.8495--0.8780)}{4.55pt}{4.82pt}{} & \HoloSegScore{0.8527}{(0.8391--0.8670)}{4.55pt}{4.82pt}{} \\*
\softcline{4-11}
 & \HoloSegSpan{\makecell[c]{Pancreas-\\[-0.10ex]CT}}{1.86cm}{0.32cm} & \HoloSegSpan{\makecell[c]{pancreas}}{2.04cm}{0.32cm} & \HoloSegMetric{HD95} & \HoloSegScore{5.249}{(4.469--6.225)}{4.55pt}{4.82pt}{} & \HoloSegScore{13.80}{(9.282--18.85)}{4.55pt}{4.82pt}{} & \HoloSegScore{3.188}{(2.522--3.985)}{4.55pt}{4.82pt}{} & \HoloSegScore{3.607}{(3.139--4.142)}{4.55pt}{4.82pt}{} & \HoloSegScore{4.044}{(3.235--4.075)}{4.55pt}{4.82pt}{} & \HoloSegScore{3.884}{(3.102--4.999)}{4.55pt}{4.82pt}{} & \HoloSegScore{5.350}{(3.750--7.595)}{4.55pt}{4.82pt}{} \\
\cline{2-11}
 &  &  & \HoloSegMetric{Dice} & \HoloSegScore{0.9315}{(0.9071--0.9473)}{4.55pt}{4.82pt}{} & \HoloSegScore{0.8031}{(0.7775--0.8267)}{4.55pt}{4.82pt}{} & \HoloSegScore{0.9585}{(0.9520--0.9649)}{4.55pt}{4.82pt}{} & \HoloSegScore{0.9606}{(0.9524--0.9671)}{4.55pt}{4.82pt}{} & \HoloSegScore{0.9583}{(0.9580--0.9684)}{4.55pt}{4.82pt}{} & \HoloSegScore{0.9759}{(0.9659--0.9845)}{4.55pt}{4.82pt}{} & \HoloSegScore{0.9639}{(0.9560--0.9699)}{4.55pt}{4.82pt}{} \\*
\softcline{4-11}
 &  & \HoloSegSpan{\makecell[c]{spleen}}{2.04cm}{0.32cm} & \HoloSegMetric{HD95} & \HoloSegScore{7.124}{(3.387--14.20)}{4.55pt}{4.82pt}{} & \HoloSegScore{9.811}{(8.487--11.21)}{4.55pt}{4.82pt}{} & \HoloSegScore{2.017}{(1.722--2.333)}{4.55pt}{4.82pt}{} & \HoloSegScore{1.946}{(1.565--2.388)}{4.55pt}{4.82pt}{} & \HoloSegScore{4.213}{(2.787--4.812)}{4.55pt}{4.82pt}{} & \HoloSegScore{1.293}{(0.8280--1.713)}{4.55pt}{4.82pt}{} & \HoloSegScore{1.631}{(1.411--1.928)}{4.55pt}{4.82pt}{} \\
\cline{3-11}
 &  &  & \HoloSegMetric{Dice} & \HoloSegScore{0.9297}{(0.9219--0.9373)}{4.55pt}{4.82pt}{} & \HoloSegScore{0.7291}{(0.6499--0.7857)}{4.55pt}{4.82pt}{} & \HoloSegScore{0.9452}{(0.9387--0.9508)}{4.55pt}{4.82pt}{} & \HoloSegScore{0.9449}{(0.9354--0.9520)}{4.55pt}{4.82pt}{} & \HoloSegScore{0.9497}{(0.9411--0.9599)}{4.55pt}{4.82pt}{} & \HoloSegScore{0.9637}{(0.9547--0.9705)}{4.55pt}{4.82pt}{} & \HoloSegScore{0.9507}{(0.9432--0.9577)}{4.55pt}{4.82pt}{} \\*
\softcline{4-11}
 &  & \HoloSegSpan{\makecell[c]{right kidney}}{2.04cm}{0.32cm} & \HoloSegMetric{HD95} & \HoloSegScore{4.527}{(3.363--5.800)}{4.55pt}{4.82pt}{} & \HoloSegScore{71.81}{(34.37--107.3)}{4.55pt}{4.82pt}{} & \HoloSegScore{2.642}{(2.103--3.166)}{4.55pt}{4.82pt}{} & \HoloSegScore{3.219}{(2.187--4.361)}{4.55pt}{4.82pt}{} & \HoloSegScore{3.211}{(2.502--4.534)}{4.55pt}{4.82pt}{} & \HoloSegScore{1.713}{(0.9450--2.737)}{4.55pt}{4.82pt}{} & \HoloSegScore{2.413}{(1.278--3.771)}{4.55pt}{4.82pt}{} \\
\cline{3-11}
 &  &  & \HoloSegMetric{Dice} & \HoloSegScore{0.9284}{(0.9181--0.9385)}{4.55pt}{4.82pt}{} & \HoloSegScore{0.6127}{(0.5298--0.7008)}{4.55pt}{4.82pt}{} & \HoloSegScore{0.9504}{(0.9422--0.9572)}{4.55pt}{4.82pt}{} & \HoloSegScore{0.9501}{(0.9422--0.9571)}{4.55pt}{4.82pt}{} & \HoloSegScore{0.9332}{(0.9205--0.9423)}{4.55pt}{4.82pt}{} & \HoloSegScore{0.9665}{(0.9610--0.9710)}{4.55pt}{4.82pt}{} & \HoloSegScore{0.9571}{(0.9523--0.9603)}{4.55pt}{4.82pt}{} \\*
\softcline{4-11}
 &  & \HoloSegSpan{\makecell[c]{left kidney}}{2.04cm}{0.32cm} & \HoloSegMetric{HD95} & \HoloSegScore{6.735}{(3.023--13.04)}{4.55pt}{4.82pt}{} & \HoloSegScore{98.78}{(62.57--123.9)}{4.55pt}{4.82pt}{} & \HoloSegScore{2.351}{(1.732--3.079)}{4.55pt}{4.82pt}{} & \HoloSegScore{2.348}{(1.598--3.025)}{4.55pt}{4.82pt}{} & \HoloSegScore{4.079}{(3.068--6.058)}{4.55pt}{4.82pt}{} & \HoloSegScore{1.917}{(0.8350--3.132)}{4.55pt}{4.82pt}{} & \HoloSegScore{1.473}{(1.137--1.805)}{4.55pt}{4.82pt}{} \\
\cline{3-11}
 &  &  & \HoloSegMetric{Dice} & \HoloSegScore{0.7718}{(0.5755--0.8902)}{4.55pt}{4.82pt}{} & \HoloSegScore{0.3024}{(0.07825--0.5348)}{4.20pt}{4.48pt}{} & \HoloSegScore{0.7902}{(0.5760--0.9149)}{4.55pt}{4.82pt}{} & \HoloSegScore{0.7085}{(0.4070--0.8995)}{4.55pt}{4.82pt}{} & \HoloSegScore{0.7731}{(0.5719--0.8910)}{4.55pt}{4.82pt}{} & \HoloSegScore{0.8988}{(0.8471--0.9360)}{4.55pt}{4.82pt}{} & \HoloSegScore{0.8997}{(0.8698--0.9260)}{4.55pt}{4.82pt}{} \\*
\softcline{4-11}
 &  & \HoloSegSpan{\makecell[c]{gallbladder}}{2.04cm}{0.32cm} & \HoloSegMetric{HD95} & \HoloSegScore{7.718}{(4.473--12.89)}{4.55pt}{4.82pt}{} & \HoloSegScore{40.39}{(8.823--97.51)}{4.55pt}{4.82pt}{} & \HoloSegScore{6.483}{(2.324--13.75)}{4.55pt}{4.82pt}{} & \HoloSegScore{15.92}{(3.669--37.58)}{4.55pt}{4.82pt}{} & \HoloSegScore{6.960}{(3.066--10.81)}{4.55pt}{4.82pt}{} & \HoloSegScore{2.349}{(1.477--3.439)}{4.55pt}{4.82pt}{} & \HoloSegScore{2.723}{(2.148--3.383)}{4.55pt}{4.82pt}{} \\
\cline{3-11}
 &  &  & \HoloSegMetric{Dice} & \HoloSegScore{0.7672}{(0.7559--0.7809)}{4.55pt}{4.82pt}{} & \HoloSegScore{0.5313}{(0.4868--0.5817)}{4.55pt}{4.82pt}{} & \HoloSegScore{0.7962}{(0.7832--0.8113)}{4.55pt}{4.82pt}{} & \HoloSegScore{0.7978}{(0.7624--0.8324)}{4.55pt}{4.82pt}{} & \HoloSegScore{0.7400}{(0.7303--0.7621)}{4.55pt}{4.82pt}{} & \HoloSegScore{0.8763}{(0.8518--0.8983)}{4.55pt}{4.82pt}{} & \HoloSegScore{0.8692}{(0.8459--0.8954)}{4.55pt}{4.82pt}{} \\*
\softcline{4-11}
 &  & \HoloSegSpan{\makecell[c]{esophagus}}{2.04cm}{0.32cm} & \HoloSegMetric{HD95} & \HoloSegScore{11.82}{(4.270--19.88)}{4.55pt}{4.82pt}{} & \HoloSegScore{9.610}{(6.890--13.98)}{4.55pt}{4.82pt}{} & \HoloSegScore{4.437}{(3.731--5.036)}{4.55pt}{4.82pt}{} & \HoloSegScore{6.018}{(4.259--7.901)}{4.55pt}{4.82pt}{} & \HoloSegScore{6.910}{(5.091--7.447)}{4.55pt}{4.82pt}{} & \HoloSegScore{2.400}{(1.625--3.453)}{4.55pt}{4.82pt}{} & \HoloSegScore{2.360}{(1.858--2.807)}{4.55pt}{4.82pt}{} \\
\cline{3-11}
 &  &  & \HoloSegMetric{Dice} & \HoloSegScore{0.9546}{(0.9498--0.9580)}{4.55pt}{4.82pt}{} & \HoloSegScore{0.8678}{(0.8544--0.8802)}{4.55pt}{4.82pt}{} & \HoloSegScore{0.9668}{(0.9626--0.9702)}{4.55pt}{4.82pt}{} & \HoloSegScore{0.9660}{(0.9619--0.9702)}{4.55pt}{4.82pt}{} & \HoloSegScore{0.9659}{(0.9588--0.9824)}{4.55pt}{4.82pt}{} & \HoloSegScore{0.9840}{(0.9802--0.9872)}{4.55pt}{4.82pt}{} & \HoloSegScore{0.9706}{(0.9673--0.9735)}{4.55pt}{4.82pt}{} \\*
\softcline{4-11}
 &  & \HoloSegSpan{\makecell[c]{liver}}{2.04cm}{0.32cm} & \HoloSegMetric{HD95} & \HoloSegScore{6.730}{(4.729--8.876)}{4.55pt}{4.82pt}{} & \HoloSegScore{11.57}{(9.813--13.75)}{4.55pt}{4.82pt}{} & \HoloSegScore{4.011}{(3.247--4.874)}{4.55pt}{4.82pt}{} & \HoloSegScore{6.011}{(4.380--7.866)}{4.55pt}{4.82pt}{} & \HoloSegScore{2.920}{(1.042--4.767)}{4.55pt}{4.82pt}{} & \HoloSegScore{3.102}{(2.596--3.783)}{4.55pt}{4.82pt}{} & \HoloSegScore{4.049}{(3.330--4.855)}{4.55pt}{4.82pt}{} \\
\cline{3-11}
 &  &  & \HoloSegMetric{Dice} & \HoloSegScore{0.9315}{(0.9221--0.9393)}{4.55pt}{4.82pt}{} & \HoloSegScore{0.7742}{(0.7543--0.7968)}{4.55pt}{4.82pt}{} & \HoloSegScore{0.8463}{(0.6740--0.9399)}{4.55pt}{4.82pt}{} & \HoloSegScore{0.9254}{(0.9097--0.9408)}{4.55pt}{4.82pt}{} & \HoloSegScore{0.7927}{(0.7891--0.8026)}{4.55pt}{4.82pt}{} & \HoloSegScore{0.9628}{(0.9540--0.9707)}{4.55pt}{4.82pt}{} & \HoloSegScore{0.9519}{(0.9452--0.9575)}{4.55pt}{4.82pt}{} \\*
\softcline{4-11}
 & \HoloSegSpan{\makecell[c]{BTCV-\\[-0.10ex]Abdomen}}{1.86cm}{0.32cm} & \HoloSegSpan{\makecell[c]{stomach}}{2.04cm}{0.32cm} & \HoloSegMetric{HD95} & \HoloSegScore{5.419}{(4.527--6.430)}{4.55pt}{4.82pt}{} & \HoloSegScore{12.64}{(11.39--13.98)}{4.55pt}{4.82pt}{} & \HoloSegScore{57.95}{(3.510--165.7)}{4.55pt}{4.82pt}{} & \HoloSegScore{10.37}{(4.882--18.47)}{4.55pt}{4.82pt}{} & \HoloSegScore{19.33}{(18.84--20.42)}{4.55pt}{4.82pt}{} & \HoloSegScore{3.372}{(2.631--4.108)}{4.55pt}{4.82pt}{} & \HoloSegScore{3.596}{(3.034--4.174)}{4.55pt}{4.82pt}{} \\
\cline{3-11}
 &  &  & \HoloSegMetric{Dice} & \HoloSegScore{0.9169}{(0.9070--0.9271)}{4.55pt}{4.82pt}{} & \HoloSegScore{0.8156}{(0.7929--0.8403)}{4.55pt}{4.82pt}{} & \HoloSegScore{0.9140}{(0.8851--0.9324)}{4.55pt}{4.82pt}{} & \HoloSegScore{0.9380}{(0.9284--0.9462)}{4.55pt}{4.82pt}{} & \HoloSegScore{0.9059}{(0.8968--0.9173)}{4.55pt}{4.82pt}{} & \HoloSegScore{0.9535}{(0.9454--0.9611)}{4.55pt}{4.82pt}{} & \HoloSegScore{0.9388}{(0.9290--0.9479)}{4.55pt}{4.82pt}{} \\*
\softcline{4-11}
\HoloSegSpan{\makecell[c]{\textbf{Internal}}}{1.20cm}{0.32cm} &  & \HoloSegSpan{\makecell[c]{aorta}}{2.04cm}{0.32cm} & \HoloSegMetric{HD95} & \HoloSegScore{3.071}{(2.315--4.295)}{4.55pt}{4.82pt}{} & \HoloSegScore{5.147}{(3.658--6.742)}{4.55pt}{4.82pt}{} & \HoloSegScore{27.74}{(2.038--77.35)}{4.55pt}{4.82pt}{} & \HoloSegScore{1.283}{(1.058--1.498)}{4.55pt}{4.82pt}{} & \HoloSegScore{2.035}{(1.724--2.555)}{4.55pt}{4.82pt}{} & \HoloSegScore{0.6480}{(0.3822--0.9160)}{4.55pt}{4.82pt}{} & \HoloSegScore{1.260}{(1.054--1.467)}{4.55pt}{4.82pt}{} \\
\cline{3-11}
 &  &  & \HoloSegMetric{Dice} & \HoloSegScore{0.8267}{(0.7541--0.8840)}{4.55pt}{4.82pt}{} & \HoloSegScore{0.6952}{(0.5514--0.8062)}{4.55pt}{4.82pt}{} & \HoloSegScore{0.8684}{(0.8223--0.9094)}{4.55pt}{4.82pt}{} & \HoloSegScore{0.8603}{(0.8056--0.9042)}{4.55pt}{4.82pt}{} & \HoloSegScore{0.8256}{(0.7690--0.8642)}{4.55pt}{4.82pt}{} & \HoloSegScore{0.8901}{(0.8497--0.9274)}{4.55pt}{4.82pt}{} & \HoloSegScore{0.8889}{(0.8571--0.9194)}{4.55pt}{4.82pt}{} \\*
\softcline{4-11}
 &  & \HoloSegSpan{\makecell[c]{inferior\\[-0.10ex]vena cava}}{2.04cm}{0.32cm} & \HoloSegMetric{HD95} & \HoloSegScore{19.67}{(13.42--26.18)}{4.55pt}{4.82pt}{} & \HoloSegScore{8.720}{(6.027--11.70)}{4.55pt}{4.82pt}{} & \HoloSegScore{5.979}{(4.415--7.855)}{4.55pt}{4.82pt}{} & \HoloSegScore{6.302}{(3.749--9.362)}{4.55pt}{4.82pt}{} & \HoloSegScore{8.475}{(6.942--11.29)}{4.55pt}{4.82pt}{} & \HoloSegScore{3.400}{(1.922--5.087)}{4.55pt}{4.82pt}{} & \HoloSegScore{3.463}{(2.339--4.579)}{4.55pt}{4.82pt}{} \\
\cline{3-11}
 &  &  & \HoloSegMetric{Dice} & \HoloSegScore{0.7689}{(0.7208--0.8116)}{4.55pt}{4.82pt}{} & \HoloSegScore{0.2380}{(0.1280--0.3294)}{4.55pt}{4.82pt}{} & \HoloSegScore{0.7772}{(0.7416--0.8112)}{4.55pt}{4.82pt}{} & \HoloSegScore{0.6829}{(0.5884--0.7675)}{4.55pt}{4.82pt}{} & \HoloSegScore{0.7480}{(0.6960--0.7807)}{4.55pt}{4.82pt}{} & \HoloSegScore{0.8339}{(0.7968--0.8755)}{4.55pt}{4.82pt}{} & \HoloSegScore{0.8326}{(0.8027--0.8676)}{4.55pt}{4.82pt}{} \\*
\softcline{4-11}
 &  & \HoloSegSpan{\makecell[c]{portal vein\\[-0.10ex]and splenic\\[-0.10ex]vein}}{2.04cm}{0.32cm} & \HoloSegMetric{HD95} & \HoloSegScore{7.122}{(5.254--9.389)}{4.55pt}{4.82pt}{} & \HoloSegScore{38.39}{(29.44--48.19)}{4.55pt}{4.82pt}{} & \HoloSegScore{6.256}{(3.726--8.802)}{4.55pt}{4.82pt}{} & \HoloSegScore{22.56}{(9.725--38.85)}{4.55pt}{4.82pt}{} & \HoloSegScore{7.913}{(7.224--11.53)}{4.55pt}{4.82pt}{} & \HoloSegScore{3.857}{(2.361--5.606)}{4.55pt}{4.82pt}{} & \HoloSegScore{4.635}{(3.280--5.897)}{4.55pt}{4.82pt}{} \\
\cline{3-11}
 &  &  & \HoloSegMetric{Dice} & \HoloSegScore{0.8263}{(0.7991--0.8492)}{4.55pt}{4.82pt}{} & \HoloSegScore{0.5561}{(0.5151--0.6010)}{4.55pt}{4.82pt}{} & \HoloSegScore{0.8494}{(0.8376--0.8614)}{4.55pt}{4.82pt}{} & \HoloSegScore{0.8130}{(0.7640--0.8485)}{4.55pt}{4.82pt}{} & \HoloSegScore{0.8250}{(0.8138--0.8376)}{4.55pt}{4.82pt}{} & \HoloSegScore{0.8769}{(0.8571--0.8955)}{4.55pt}{4.82pt}{} & \HoloSegScore{0.8510}{(0.8042--0.8822)}{4.55pt}{4.82pt}{} \\*
\softcline{4-11}
 &  & \HoloSegSpan{\makecell[c]{pancreas}}{2.04cm}{0.32cm} & \HoloSegMetric{HD95} & \HoloSegScore{11.28}{(5.723--20.17)}{4.55pt}{4.82pt}{} & \HoloSegScore{15.73}{(11.51--20.70)}{4.55pt}{4.82pt}{} & \HoloSegScore{4.466}{(3.874--4.936)}{4.55pt}{4.82pt}{} & \HoloSegScore{12.58}{(5.076--26.22)}{4.55pt}{4.82pt}{} & \HoloSegScore{7.612}{(5.376--8.179)}{4.55pt}{4.82pt}{} & \HoloSegScore{4.532}{(3.258--6.250)}{4.55pt}{4.82pt}{} & \HoloSegScore{10.13}{(3.966--20.56)}{4.55pt}{4.82pt}{} \\
\cline{3-11}
 &  &  & \HoloSegMetric{Dice} & \HoloSegScore{0.6703}{(0.6271--0.7159)}{4.55pt}{4.82pt}{} & \HoloSegScore{0.3156}{(0.2546--0.3767)}{4.55pt}{4.82pt}{} & \HoloSegScore{0.7467}{(0.7155--0.7742)}{4.55pt}{4.82pt}{} & \HoloSegScore{0.7151}{(0.6759--0.7547)}{4.55pt}{4.82pt}{} & \HoloSegScore{0.6616}{(0.6341--0.6851)}{4.55pt}{4.82pt}{} & \HoloSegScore{0.7598}{(0.7131--0.7967)}{4.55pt}{4.82pt}{} & \HoloSegScore{0.8074}{(0.7904--0.8255)}{4.55pt}{4.82pt}{} \\*
\softcline{4-11}
 &  & \HoloSegSpan{\makecell[c]{right\\[-0.10ex]adrenal\\[-0.10ex]gland}}{2.04cm}{0.32cm} & \HoloSegMetric{HD95} & \HoloSegScore{6.527}{(4.039--9.228)}{4.55pt}{4.82pt}{} & \HoloSegScore{9.723}{(8.302--11.07)}{4.55pt}{4.82pt}{} & \HoloSegScore{3.454}{(2.371--4.575)}{4.55pt}{4.82pt}{} & \HoloSegScore{4.591}{(2.190--7.142)}{4.55pt}{4.82pt}{} & \HoloSegScore{7.318}{(6.779--7.522)}{4.55pt}{4.82pt}{} & \HoloSegScore{2.873}{(1.694--4.241)}{4.55pt}{4.82pt}{} & \HoloSegScore{1.658}{(1.408--1.990)}{4.55pt}{4.82pt}{} \\
\cline{3-11}
 &  &  & \HoloSegMetric{Dice} & \HoloSegScore{0.6417}{(0.4345--0.7760)}{4.55pt}{4.82pt}{} & \HoloSegScore{0.2156}{(0.1050--0.3244)}{4.55pt}{4.82pt}{} & \HoloSegScore{0.7827}{(0.7472--0.8307)}{4.55pt}{4.82pt}{} & \HoloSegScore{0.7394}{(0.6197--0.8212)}{4.55pt}{4.82pt}{} & \HoloSegScore{0.6395}{(0.6029--0.6872)}{4.55pt}{4.82pt}{} & \HoloSegScore{0.8098}{(0.7530--0.8548)}{4.55pt}{4.82pt}{} & \HoloSegScore{0.8223}{(0.7911--0.8547)}{4.55pt}{4.82pt}{} \\*
\softcline{4-11}
 &  & \HoloSegSpan{\makecell[c]{left adrenal\\[-0.10ex]gland}}{2.04cm}{0.32cm} & \HoloSegMetric{HD95} & \HoloSegScore{9.681}{(4.296--18.81)}{4.55pt}{4.82pt}{} & \HoloSegScore{24.01}{(13.07--35.09)}{4.55pt}{4.82pt}{} & \HoloSegScore{2.824}{(1.892--3.705)}{4.55pt}{4.82pt}{} & \HoloSegScore{5.621}{(3.435--8.278)}{4.55pt}{4.82pt}{} & \HoloSegScore{5.767}{(5.287--7.035)}{4.55pt}{4.82pt}{} & \HoloSegScore{2.207}{(1.494--3.192)}{4.55pt}{4.82pt}{} & \HoloSegScore{2.139}{(1.422--3.334)}{4.55pt}{4.82pt}{} \\
\cline{2-11}
 &  &  & \HoloSegMetric{Dice} & \HoloSegScore{0.4910}{(0.2551--0.7404)}{4.55pt}{4.82pt}{} & \HoloSegScore{0.3014}{(0.04782--0.5618)}{4.20pt}{4.48pt}{} & \HoloSegScore{0.8934}{(0.8665--0.9238)}{4.55pt}{4.82pt}{} & \HoloSegScore{0.8993}{(0.8710--0.9267)}{4.55pt}{4.82pt}{} & \HoloSegScore{0.7559}{(0.7346--0.7719)}{4.55pt}{4.82pt}{} & \HoloSegScore{0.9071}{(0.8774--0.9405)}{4.55pt}{4.82pt}{} & \HoloSegScore{0.9188}{(0.9023--0.9388)}{4.55pt}{4.82pt}{} \\*
\softcline{4-11}
 &  & \HoloSegSpan{\makecell[c]{urinary\\[-0.10ex]bladder}}{2.04cm}{0.32cm} & \HoloSegMetric{HD95} & \HoloSegScore{65.95}{(20.37--145.2)}{4.55pt}{4.82pt}{} & \HoloSegScore{35.84}{(21.71--49.89)}{4.55pt}{4.82pt}{} & \HoloSegScore{3.643}{(3.061--4.319)}{4.55pt}{4.82pt}{} & \HoloSegScore{3.986}{(2.724--5.684)}{4.55pt}{4.82pt}{} & \HoloSegScore{10.62}{(10.37--11.87)}{4.55pt}{4.82pt}{} & \HoloSegScore{3.142}{(2.322--4.409)}{4.55pt}{4.82pt}{} & \HoloSegScore{2.718}{(2.587--2.849)}{4.55pt}{4.82pt}{} \\
\cline{3-11}
 &  &  & \HoloSegMetric{Dice} & \HoloSegScore{0.4706}{(0.2592--0.7134)}{4.55pt}{4.82pt}{} & \HoloSegScore{0.2136}{(0.1118--0.3222)}{4.55pt}{4.82pt}{} & \HoloSegScore{0.7954}{(0.7460--0.8506)}{4.55pt}{4.82pt}{} & \HoloSegScore{0.7969}{(0.7352--0.8602)}{4.55pt}{4.82pt}{} & \HoloSegScore{0.6703}{(0.6268--0.7298)}{4.55pt}{4.82pt}{} & \HoloSegScore{0.8277}{(0.7752--0.8808)}{4.55pt}{4.82pt}{} & \HoloSegScore{0.8200}{(0.7715--0.8681)}{4.55pt}{4.82pt}{} \\*
\softcline{4-11}
 &  & \HoloSegSpan{\makecell[c]{uterus}}{2.04cm}{0.32cm} & \HoloSegMetric{HD95} & \HoloSegScore{74.66}{(47.90--112.2)}{4.55pt}{4.82pt}{} & \HoloSegScore{55.42}{(40.94--71.19)}{4.55pt}{4.82pt}{} & \HoloSegScore{12.81}{(8.631--17.50)}{4.55pt}{4.82pt}{} & \HoloSegScore{17.65}{(10.34--25.28)}{4.55pt}{4.82pt}{} & \HoloSegScore{33.27}{(30.47--38.61)}{4.55pt}{4.82pt}{} & \HoloSegScore{10.19}{(6.806--13.59)}{4.55pt}{4.82pt}{} & \HoloSegScore{36.03}{(8.990--88.31)}{4.55pt}{4.82pt}{} \\
\cline{3-11}
 & \HoloSegSpan{\makecell[c]{BTCV-\\[-0.10ex]Cervix}}{1.86cm}{0.32cm} &  & \HoloSegMetric{Dice} &  & \HoloSegScore{0.1099}{(0.01854--0.2124)}{4.20pt}{4.48pt}{} & \HoloSegScore{0.8379}{(0.7930--0.8780)}{4.55pt}{4.82pt}{} & \HoloSegScore{0.8662}{(0.8459--0.8866)}{4.55pt}{4.82pt}{} & \HoloSegScore{0.6899}{(0.6678--0.7188)}{4.55pt}{4.82pt}{} & \HoloSegScore{0.8373}{(0.7783--0.8886)}{4.55pt}{4.82pt}{} & \HoloSegScore{0.8731}{(0.8512--0.8933)}{4.55pt}{4.82pt}{} \\*
\softcline{4-4}\softcline{6-11}
 &  & \HoloSegSpan{\makecell[c]{rectum}}{2.04cm}{0.32cm} & \HoloSegMetric{HD95} & \raisebox{0.32cm}[0pt][0pt]{\HoloSegUnsupported} & \HoloSegScore{52.36}{(30.36--78.00)}{4.55pt}{4.82pt}{} & \HoloSegScore{6.321}{(3.955--8.383)}{4.55pt}{4.82pt}{} & \HoloSegScore{5.734}{(3.871--8.025)}{4.55pt}{4.82pt}{} & \HoloSegScore{12.87}{(11.00--15.52)}{4.55pt}{4.82pt}{} & \HoloSegScore{7.075}{(4.262--10.16)}{4.55pt}{4.82pt}{} & \HoloSegScore{19.81}{(4.399--40.14)}{4.55pt}{4.82pt}{} \\
\cline{3-11}
 &  &  & \HoloSegMetric{Dice} & \HoloSegScore{0.3293}{(0.2089--0.4368)}{4.55pt}{4.82pt}{} & \HoloSegScore{0.2758}{(0.1549--0.4249)}{4.55pt}{4.82pt}{} & \HoloSegScore{0.6778}{(0.5450--0.7653)}{4.55pt}{4.82pt}{} & \HoloSegScore{0.6588}{(0.4877--0.7776)}{4.55pt}{4.82pt}{} & \HoloSegScore{0.5251}{(0.3808--0.6363)}{4.55pt}{4.82pt}{} & \HoloSegScore{0.7680}{(0.7192--0.8169)}{4.55pt}{4.82pt}{} & \HoloSegScore{0.7677}{(0.7057--0.8204)}{4.55pt}{4.82pt}{} \\*
\softcline{4-11}
 &  & \HoloSegSpan{\makecell[c]{small bowel}}{2.04cm}{0.32cm} & \HoloSegMetric{HD95} & \HoloSegScore{107.7}{(63.57--141.8)}{4.55pt}{4.82pt}{} & \HoloSegScore{105.9}{(76.76--131.2)}{4.55pt}{4.82pt}{} & \HoloSegScore{51.13}{(11.93--90.43)}{4.55pt}{4.82pt}{} & \HoloSegScore{48.38}{(19.75--84.00)}{4.55pt}{4.82pt}{} & \HoloSegScore{64.56}{(35.58--90.66)}{4.55pt}{4.82pt}{} & \HoloSegScore{50.38}{(21.50--92.12)}{4.55pt}{4.82pt}{} & \HoloSegScore{43.32}{(13.22--85.87)}{4.55pt}{4.82pt}{} \\
\hline
\pagebreak[4]
 &  &  & \HoloSegMetric{Dice} & \HoloSegScore{0.9313}{(0.9264--0.9357)}{4.55pt}{4.82pt}{} & \HoloSegScore{0.8676}{(0.8338--0.8890)}{4.55pt}{4.82pt}{} & \HoloSegScore{0.9420}{(0.9372--0.9461)}{4.55pt}{4.82pt}{} & \HoloSegScore{0.9446}{(0.9392--0.9492)}{4.55pt}{4.82pt}{} & \HoloSegScore{0.9404}{(0.9274--0.9482)}{4.55pt}{4.82pt}{} & \HoloSegScore{0.9610}{(0.9576--0.9641)}{4.55pt}{4.82pt}{} & \HoloSegScore{0.9456}{(0.9417--0.9494)}{4.55pt}{4.82pt}{} \\*
\softcline{4-11}
 &  & \HoloSegSpan{\makecell[c]{liver}}{2.04cm}{0.32cm} & \HoloSegMetric{HD95} & \HoloSegScore{22.62}{(21.40--23.81)}{4.55pt}{4.82pt}{} & \HoloSegScore{18.60}{(15.97--22.75)}{4.55pt}{4.82pt}{} & \HoloSegScore{17.51}{(16.18--18.88)}{4.55pt}{4.82pt}{} & \HoloSegScore{24.41}{(22.85--26.37)}{4.55pt}{4.82pt}{} & \HoloSegScore{19.89}{(18.75--21.21)}{4.55pt}{4.82pt}{} & \HoloSegScore{19.45}{(18.53--20.36)}{4.55pt}{4.82pt}{} & \HoloSegScore{22.11}{(21.19--22.96)}{4.55pt}{4.82pt}{} \\
\cline{3-11}
 &  &  & \HoloSegMetric{Dice} & \HoloSegScore{0.4671}{(0.4135--0.5113)}{4.55pt}{4.82pt}{} & \HoloSegScore{0.1001}{(0.07545--0.1270)}{4.20pt}{4.48pt}{} & \HoloSegScore{0.4195}{(0.3761--0.4622)}{4.55pt}{4.82pt}{} & \HoloSegScore{0.1494}{(0.1155--0.1865)}{4.55pt}{4.82pt}{} & \HoloSegScore{0.4918}{(0.4586--0.5188)}{4.55pt}{4.82pt}{} & \HoloSegScore{0.5073}{(0.4607--0.5503)}{4.55pt}{4.82pt}{} & \HoloSegScore{0.5260}{(0.4789--0.5717)}{4.55pt}{4.82pt}{} \\*
\softcline{4-11}
 &  & \HoloSegSpan{\makecell[c]{hepatic vein}}{2.04cm}{0.32cm} & \HoloSegMetric{HD95} & \HoloSegScore{28.01}{(22.75--34.02)}{4.55pt}{4.82pt}{} & \HoloSegScore{81.33}{(71.86--90.28)}{4.55pt}{4.82pt}{} & \HoloSegScore{27.13}{(22.28--32.62)}{4.55pt}{4.82pt}{} & \HoloSegScore{39.03}{(34.93--44.54)}{4.55pt}{4.82pt}{} & \HoloSegScore{29.65}{(24.57--34.89)}{4.55pt}{4.82pt}{} & \HoloSegScore{24.53}{(19.76--30.99)}{4.55pt}{4.82pt}{} & \HoloSegScore{25.74}{(20.46--33.09)}{4.55pt}{4.82pt}{} \\
\cline{3-11}
 & \HoloSegSpan{\makecell[c]{CRLM-CT}}{1.86cm}{0.32cm} &  & \HoloSegMetric{Dice} & \HoloSegScore{0.4619}{(0.4322--0.4938)}{4.55pt}{4.82pt}{} & \HoloSegScore{0.08952}{(0.06067--0.1220)}{4.20pt}{4.48pt}{} & \HoloSegScore{0.2715}{(0.2321--0.3132)}{4.55pt}{4.82pt}{} & \HoloSegScore{0.4883}{(0.4627--0.5129)}{4.55pt}{4.82pt}{} & \HoloSegScore{0.5301}{(0.5113--0.6482)}{4.55pt}{4.82pt}{} & \HoloSegScore{0.5934}{(0.5635--0.6204)}{4.55pt}{4.82pt}{} & \HoloSegScore{0.6508}{(0.6231--0.6729)}{4.55pt}{4.82pt}{} \\*
\softcline{4-11}
 &  & \HoloSegSpan{\makecell[c]{portal vein}}{2.04cm}{0.32cm} & \HoloSegMetric{HD95} & \HoloSegScore{97.68}{(88.51--106.2)}{4.55pt}{4.82pt}{} & \HoloSegScore{91.06}{(81.59--101.1)}{4.55pt}{4.82pt}{} & \HoloSegScore{91.46}{(83.49--99.73)}{4.55pt}{4.82pt}{} & \HoloSegScore{80.52}{(70.32--92.03)}{4.55pt}{4.82pt}{} & \HoloSegScore{37.60}{(31.88--43.50)}{4.55pt}{4.82pt}{} & \HoloSegScore{29.80}{(24.15--37.04)}{4.55pt}{4.82pt}{} & \HoloSegScore{27.82}{(22.93--34.63)}{4.55pt}{4.82pt}{} \\
\cline{3-11}
 &  &  & \HoloSegMetric{Dice} & \HoloSegScore{0.6206}{(0.5362--0.7031)}{4.55pt}{4.82pt}{} & \HoloSegScore{0.08934}{(0.02796--0.1611)}{4.20pt}{4.48pt}{} & \HoloSegScore{0.6307}{(0.5362--0.7203)}{4.55pt}{4.82pt}{} & \HoloSegScore{0.6161}{(0.5261--0.6978)}{4.55pt}{4.82pt}{} & \HoloSegScore{0.6270}{(0.5519--0.6862)}{4.55pt}{4.82pt}{} & \HoloSegScore{0.6875}{(0.6099--0.7583)}{4.55pt}{4.82pt}{} & \HoloSegScore{0.6898}{(0.6202--0.7546)}{4.55pt}{4.82pt}{} \\*
\softcline{4-11}
 &  & \HoloSegSpan{\makecell[c]{liver tumor}}{2.04cm}{0.32cm} & \HoloSegMetric{HD95} & \HoloSegScore{43.58}{(25.26--64.56)}{4.55pt}{4.82pt}{} & \HoloSegScore{125.8}{(106.2--145.6)}{4.55pt}{4.82pt}{} & \HoloSegScore{21.65}{(10.65--37.00)}{4.55pt}{4.82pt}{} & \HoloSegScore{47.54}{(27.73--66.35)}{4.55pt}{4.82pt}{} & \HoloSegScore{44.21}{(29.58--60.99)}{4.55pt}{4.82pt}{} & \HoloSegScore{36.05}{(20.86--53.45)}{4.55pt}{4.82pt}{} & \HoloSegScore{40.84}{(25.58--59.00)}{4.55pt}{4.82pt}{} \\
\cline{2-11}
 &  &  & \HoloSegMetric{Dice} &  & \HoloSegScore{0.1697}{(0.1209--0.2185)}{4.55pt}{4.82pt}{} & \HoloSegScore{0.7552}{(0.7069--0.8011)}{4.55pt}{4.82pt}{} & \HoloSegScore{0.7870}{(0.7644--0.8138)}{4.55pt}{4.82pt}{} & \HoloSegScore{0.7673}{(0.7451--0.7896)}{4.55pt}{4.82pt}{} & \HoloSegScore{0.7096}{(0.6631--0.7530)}{4.55pt}{4.82pt}{} & \HoloSegScore{0.8218}{(0.8003--0.8413)}{4.55pt}{4.82pt}{} \\*
\softcline{4-4}\softcline{6-11}
 &  & \HoloSegSpan{\makecell[c]{left carotid\\[-0.10ex]artery}}{2.04cm}{0.32cm} & \HoloSegMetric{HD95} & \raisebox{0.32cm}[0pt][0pt]{\HoloSegUnsupported} & \HoloSegScore{39.53}{(29.49--50.55)}{4.55pt}{4.82pt}{} & \HoloSegScore{10.53}{(7.754--13.12)}{4.55pt}{4.82pt}{} & \HoloSegScore{16.72}{(14.91--18.28)}{4.55pt}{4.82pt}{} & \HoloSegScore{8.325}{(6.872--10.38)}{4.55pt}{4.82pt}{} & \HoloSegScore{24.98}{(19.95--32.43)}{4.55pt}{4.82pt}{} & \HoloSegScore{2.388}{(2.024--2.776)}{4.55pt}{4.82pt}{} \\
\cline{3-11}
 &  &  & \HoloSegMetric{Dice} &  & \HoloSegScore{0.1760}{(0.1327--0.2183)}{4.55pt}{4.82pt}{} & \HoloSegScore{0.7716}{(0.7350--0.8001)}{4.55pt}{4.82pt}{} & \HoloSegScore{0.7911}{(0.7706--0.8132)}{4.55pt}{4.82pt}{} & \HoloSegScore{0.7755}{(0.7648--0.7967)}{4.55pt}{4.82pt}{} & \HoloSegScore{0.7586}{(0.7298--0.7877)}{4.55pt}{4.82pt}{} & \HoloSegScore{0.8086}{(0.7848--0.8331)}{4.55pt}{4.82pt}{} \\*
\softcline{4-4}\softcline{6-11}
 &  & \HoloSegSpan{\makecell[c]{right\\[-0.10ex]carotid\\[-0.10ex]artery}}{2.04cm}{0.32cm} & \HoloSegMetric{HD95} & \raisebox{0.32cm}[0pt][0pt]{\HoloSegUnsupported} & \HoloSegScore{30.61}{(22.03--40.08)}{4.55pt}{4.82pt}{} & \HoloSegScore{10.58}{(7.730--13.05)}{4.55pt}{4.82pt}{} & \HoloSegScore{18.13}{(14.31--20.94)}{4.55pt}{4.82pt}{} & \HoloSegScore{18.51}{(14.47--20.59)}{4.55pt}{4.82pt}{} & \HoloSegScore{20.54}{(18.21--22.72)}{4.55pt}{4.82pt}{} & \HoloSegScore{2.260}{(1.738--2.782)}{4.55pt}{4.82pt}{} \\
\cline{3-11}
 &  &  & \HoloSegMetric{Dice} &  & \HoloSegScore{0.05639}{(0.01929--0.09761)}{4.20pt}{4.48pt}{} & \HoloSegScore{0.4791}{(0.3834--0.5704)}{4.55pt}{4.82pt}{} & \HoloSegScore{0.5628}{(0.4592--0.6517)}{4.55pt}{4.82pt}{} & \HoloSegScore{0.5436}{(0.5042--0.5970)}{4.55pt}{4.82pt}{} & \HoloSegScore{0.5992}{(0.5287--0.6584)}{4.55pt}{4.82pt}{} & \HoloSegScore{0.6959}{(0.6442--0.7502)}{4.55pt}{4.82pt}{} \\*
\softcline{4-4}\softcline{6-11}
 &  & \HoloSegSpan{\makecell[c]{arytenoid}}{2.04cm}{0.32cm} & \HoloSegMetric{HD95} & \raisebox{0.32cm}[0pt][0pt]{\HoloSegUnsupported} & \HoloSegScore{27.05}{(14.16--47.72)}{4.55pt}{4.82pt}{} & \HoloSegScore{3.164}{(2.621--3.684)}{4.55pt}{4.82pt}{} & \HoloSegScore{3.120}{(2.399--3.818)}{4.55pt}{4.82pt}{} & \HoloSegScore{4.733}{(3.546--5.792)}{4.55pt}{4.82pt}{} & \HoloSegScore{2.783}{(1.981--3.840)}{4.55pt}{4.82pt}{} & \HoloSegScore{1.907}{(1.551--2.327)}{4.55pt}{4.82pt}{} \\
\cline{3-11}
 &  &  & \HoloSegMetric{Dice} &  & \HoloSegScore{0.5040}{(0.3718--0.5916)}{4.55pt}{4.82pt}{} & \HoloSegScore{0.9211}{(0.9131--0.9291)}{4.55pt}{4.82pt}{} & \HoloSegScore{0.9417}{(0.9316--0.9490)}{4.55pt}{4.82pt}{} & \HoloSegScore{0.9103}{(0.8955--0.9325)}{4.55pt}{4.82pt}{} & \HoloSegScore{0.9151}{(0.8989--0.9266)}{4.55pt}{4.82pt}{} & \HoloSegScore{0.9301}{(0.9198--0.9394)}{4.55pt}{4.82pt}{} \\*
\softcline{4-4}\softcline{6-11}
 &  & \HoloSegSpan{\makecell[c]{mandible}}{2.04cm}{0.32cm} & \HoloSegMetric{HD95} & \raisebox{0.32cm}[0pt][0pt]{\HoloSegUnsupported} & \HoloSegScore{16.24}{(11.12--23.02)}{4.55pt}{4.82pt}{} & \HoloSegScore{1.941}{(1.560--2.319)}{4.55pt}{4.82pt}{} & \HoloSegScore{1.922}{(1.265--2.697)}{4.55pt}{4.82pt}{} & \HoloSegScore{2.064}{(1.627--2.810)}{4.55pt}{4.82pt}{} & \HoloSegScore{10.29}{(2.369--24.04)}{4.55pt}{4.82pt}{} & \HoloSegScore{2.258}{(1.481--3.092)}{4.55pt}{4.82pt}{} \\
\cline{3-11}
 &  &  & \HoloSegMetric{Dice} &  & \HoloSegScore{0.4967}{(0.3413--0.6424)}{4.55pt}{4.82pt}{} & \HoloSegScore{0.8125}{(0.7847--0.8372)}{4.55pt}{4.82pt}{} & \HoloSegScore{0.7820}{(0.7405--0.8194)}{4.55pt}{4.82pt}{} & \HoloSegScore{0.8165}{(0.7805--0.8423)}{4.55pt}{4.82pt}{} & \HoloSegScore{0.8302}{(0.8000--0.8568)}{4.55pt}{4.82pt}{} & \HoloSegScore{0.8748}{(0.8686--0.8815)}{4.55pt}{4.82pt}{} \\*
\softcline{4-4}\softcline{6-11}
 &  & \HoloSegSpan{\makecell[c]{brainstem}}{2.04cm}{0.32cm} & \HoloSegMetric{HD95} & \raisebox{0.32cm}[0pt][0pt]{\HoloSegUnsupported} & \HoloSegScore{18.47}{(9.270--33.67)}{4.55pt}{4.82pt}{} & \HoloSegScore{5.125}{(4.031--6.435)}{4.55pt}{4.82pt}{} & \HoloSegScore{5.988}{(4.268--8.059)}{4.55pt}{4.82pt}{} & \HoloSegScore{6.864}{(4.840--8.766)}{4.55pt}{4.82pt}{} & \HoloSegScore{5.417}{(3.677--7.378)}{4.55pt}{4.82pt}{} & \HoloSegScore{2.955}{(2.732--3.174)}{4.55pt}{4.82pt}{} \\
\cline{3-11}
 &  &  & \HoloSegMetric{Dice} &  & \HoloSegScore{0.1970}{(0.1306--0.2690)}{4.55pt}{4.82pt}{} & \HoloSegScore{0.5573}{(0.4876--0.6167)}{4.55pt}{4.82pt}{} & \HoloSegScore{0.5857}{(0.5310--0.6456)}{4.55pt}{4.82pt}{} & \HoloSegScore{0.5487}{(0.4798--0.6160)}{4.55pt}{4.82pt}{} & \HoloSegScore{0.6096}{(0.5583--0.6639)}{4.55pt}{4.82pt}{} & \HoloSegScore{0.7467}{(0.7120--0.7802)}{4.55pt}{4.82pt}{} \\*
\softcline{4-4}\softcline{6-11}
\HoloSegSpan{\makecell[c]{\textbf{Internal}}}{1.20cm}{0.32cm} &  & \HoloSegSpan{\makecell[c]{buccal\\[-0.10ex]mucosa}}{2.04cm}{0.32cm} & \HoloSegMetric{HD95} & \raisebox{0.32cm}[0pt][0pt]{\HoloSegUnsupported} & \HoloSegScore{29.35}{(23.83--34.14)}{4.55pt}{4.82pt}{} & \HoloSegScore{6.513}{(4.708--8.963)}{4.55pt}{4.82pt}{} & \HoloSegScore{7.630}{(5.645--9.779)}{4.55pt}{4.82pt}{} & \HoloSegScore{7.171}{(3.824--9.181)}{4.55pt}{4.82pt}{} & \HoloSegScore{15.21}{(8.625--23.82)}{4.55pt}{4.82pt}{} & \HoloSegScore{3.292}{(3.060--3.532)}{4.55pt}{4.82pt}{} \\
\cline{3-11}
 &  &  & \HoloSegMetric{Dice} &  & \HoloSegScore{0.7066}{(0.6718--0.7398)}{4.55pt}{4.82pt}{} & \HoloSegScore{0.8645}{(0.8359--0.8912)}{4.55pt}{4.82pt}{} & \HoloSegScore{0.8551}{(0.8209--0.8851)}{4.55pt}{4.82pt}{} & \HoloSegScore{0.8623}{(0.8411--0.8972)}{4.55pt}{4.82pt}{} & \HoloSegScore{0.8803}{(0.8613--0.8983)}{4.55pt}{4.82pt}{} & \HoloSegScore{0.9070}{(0.8963--0.9184)}{4.55pt}{4.82pt}{} \\*
\softcline{4-4}\softcline{6-11}
 &  & \HoloSegSpan{\makecell[c]{oral cavity}}{2.04cm}{0.32cm} & \HoloSegMetric{HD95} & \raisebox{0.32cm}[0pt][0pt]{\HoloSegUnsupported} & \HoloSegScore{15.12}{(12.74--17.77)}{4.55pt}{4.82pt}{} & \HoloSegScore{6.065}{(4.433--8.073)}{4.55pt}{4.82pt}{} & \HoloSegScore{8.052}{(5.516--11.24)}{4.55pt}{4.82pt}{} & \HoloSegScore{8.020}{(5.730--8.381)}{4.55pt}{4.82pt}{} & \HoloSegScore{6.795}{(4.542--9.966)}{4.55pt}{4.82pt}{} & \HoloSegScore{3.933}{(3.256--4.701)}{4.55pt}{4.82pt}{} \\
\cline{3-11}
 &  &  & \HoloSegMetric{Dice} &  & \HoloSegScore{0.0000}{(0.0000--0.0000)}{4.55pt}{4.82pt}{} & \HoloSegScore{0.5713}{(0.5075--0.6408)}{4.55pt}{4.82pt}{} & \HoloSegScore{0.6478}{(0.5868--0.6997)}{4.55pt}{4.82pt}{} & \HoloSegScore{0.6312}{(0.6255--0.6346)}{4.55pt}{4.82pt}{} & \HoloSegScore{0.7068}{(0.6320--0.7802)}{4.55pt}{4.82pt}{} & \HoloSegScore{0.7716}{(0.7225--0.8257)}{4.55pt}{4.82pt}{} \\*
\softcline{4-4}\softcline{6-11}
 & \HoloSegSpan{\makecell[c]{HaN-Seg}}{1.86cm}{0.32cm} & \HoloSegSpan{\makecell[c]{left cochlea}}{2.04cm}{0.32cm} & \HoloSegMetric{HD95} & \raisebox{0.32cm}[0pt][0pt]{\HoloSegUnsupported} & \HoloSegScore{97.34}{(84.64--110.9)}{4.55pt}{4.82pt}{} & \HoloSegScore{2.340}{(1.946--2.661)}{4.55pt}{4.82pt}{} & \HoloSegScore{1.790}{(1.413--2.195)}{4.55pt}{4.82pt}{} & \HoloSegScore{3.194}{(2.161--4.702)}{4.55pt}{4.82pt}{} & \HoloSegScore{1.699}{(1.221--2.276)}{4.55pt}{4.82pt}{} & \HoloSegScore{1.118}{(0.6804--1.804)}{4.55pt}{4.82pt}{} \\
\cline{3-11}
 &  &  & \HoloSegMetric{Dice} &  & \HoloSegScore{0.0000}{(0.0000--0.0000)}{4.55pt}{4.82pt}{} & \HoloSegScore{0.5778}{(0.5211--0.6316)}{4.55pt}{4.82pt}{} & \HoloSegScore{0.6486}{(0.5666--0.7316)}{4.55pt}{4.82pt}{} & \HoloSegScore{0.5686}{(0.5362--0.5887)}{4.55pt}{4.82pt}{} & \HoloSegScore{0.7442}{(0.6725--0.8068)}{4.55pt}{4.82pt}{} & \HoloSegScore{0.8038}{(0.7798--0.8296)}{4.55pt}{4.82pt}{} \\*
\softcline{4-4}\softcline{6-11}
 &  & \HoloSegSpan{\makecell[c]{right\\[-0.10ex]cochlea}}{2.04cm}{0.32cm} & \HoloSegMetric{HD95} & \raisebox{0.32cm}[0pt][0pt]{\HoloSegUnsupported} & \HoloSegScore{113.5}{(77.09--132.8)}{4.55pt}{4.82pt}{} & \HoloSegScore{2.228}{(1.847--2.625)}{4.55pt}{4.82pt}{} & \HoloSegScore{1.834}{(1.275--2.553)}{4.55pt}{4.82pt}{} & \HoloSegScore{2.754}{(1.922--4.005)}{4.55pt}{4.82pt}{} & \HoloSegScore{1.674}{(1.120--2.191)}{4.55pt}{4.82pt}{} & \HoloSegScore{0.7156}{(0.6286--0.8110)}{4.55pt}{4.82pt}{} \\
\cline{3-11}
 &  &  & \HoloSegMetric{Dice} &  & \HoloSegScore{0.1526}{(0.07340--0.2367)}{4.20pt}{4.48pt}{} & \HoloSegScore{0.6526}{(0.5859--0.7043)}{4.55pt}{4.82pt}{} & \HoloSegScore{0.7162}{(0.6705--0.7547)}{4.55pt}{4.82pt}{} & \HoloSegScore{0.6663}{(0.6209--0.7063)}{4.55pt}{4.82pt}{} & \HoloSegScore{0.6955}{(0.6648--0.7228)}{4.55pt}{4.82pt}{} & \HoloSegScore{0.8182}{(0.7852--0.8444)}{4.55pt}{4.82pt}{} \\*
\softcline{4-4}\softcline{6-11}
 &  & \HoloSegSpan{\makecell[c]{cricopharyngeal\\[-0.10ex]inlet}}{2.04cm}{0.32cm} & \HoloSegMetric{HD95} & \raisebox{0.32cm}[0pt][0pt]{\HoloSegUnsupported} & \HoloSegScore{37.56}{(17.49--68.89)}{4.55pt}{4.82pt}{} & \HoloSegScore{5.173}{(3.589--7.383)}{4.55pt}{4.82pt}{} & \HoloSegScore{3.899}{(3.033--4.890)}{4.55pt}{4.82pt}{} & \HoloSegScore{3.930}{(2.925--6.293)}{4.55pt}{4.82pt}{} & \HoloSegScore{4.057}{(3.294--4.904)}{4.55pt}{4.82pt}{} & \HoloSegScore{2.076}{(1.652--2.494)}{4.55pt}{4.82pt}{} \\
\cline{3-11}
 &  &  & \HoloSegMetric{Dice} &  & \HoloSegScore{0.1777}{(0.1276--0.2359)}{4.55pt}{4.82pt}{} & \HoloSegScore{0.6533}{(0.6049--0.6996)}{4.55pt}{4.82pt}{} & \HoloSegScore{0.7388}{(0.6985--0.7785)}{4.55pt}{4.82pt}{} & \HoloSegScore{0.6974}{(0.6544--0.7539)}{4.55pt}{4.82pt}{} & \HoloSegScore{0.7995}{(0.7632--0.8255)}{4.55pt}{4.82pt}{} & \HoloSegScore{0.8681}{(0.8443--0.8944)}{4.55pt}{4.82pt}{} \\*
\softcline{4-4}\softcline{6-11}
 &  & \HoloSegSpan{\makecell[c]{cervical\\[-0.10ex]esophagus}}{2.04cm}{0.32cm} & \HoloSegMetric{HD95} & \raisebox{0.32cm}[0pt][0pt]{\HoloSegUnsupported} & \HoloSegScore{29.99}{(20.76--41.77)}{4.55pt}{4.82pt}{} & \HoloSegScore{5.342}{(4.466--6.139)}{4.55pt}{4.82pt}{} & \HoloSegScore{4.286}{(3.228--5.330)}{4.55pt}{4.82pt}{} & \HoloSegScore{5.864}{(5.453--6.539)}{4.55pt}{4.82pt}{} & \HoloSegScore{3.427}{(2.625--4.402)}{4.55pt}{4.82pt}{} & \HoloSegScore{1.788}{(1.370--2.225)}{4.55pt}{4.82pt}{} \\
\cline{3-11}
 &  &  & \HoloSegMetric{Dice} &  & \HoloSegScore{0.1063}{(0.04647--0.1806)}{4.20pt}{4.48pt}{} & \HoloSegScore{0.6971}{(0.6575--0.7395)}{4.55pt}{4.82pt}{} & \HoloSegScore{0.7514}{(0.7086--0.7933)}{4.55pt}{4.82pt}{} & \HoloSegScore{0.7210}{(0.6818--0.7753)}{4.55pt}{4.82pt}{} & \HoloSegScore{0.8339}{(0.7848--0.8702)}{4.55pt}{4.82pt}{} & \HoloSegScore{0.8428}{(0.8164--0.8718)}{4.55pt}{4.82pt}{} \\*
\softcline{4-4}\softcline{6-11}
 &  & \HoloSegSpan{\makecell[c]{left\\[-0.10ex]anterior\\[-0.10ex]eyeball}}{2.04cm}{0.32cm} & \HoloSegMetric{HD95} & \raisebox{0.32cm}[0pt][0pt]{\HoloSegUnsupported} & \HoloSegScore{14.18}{(11.82--16.64)}{4.55pt}{4.82pt}{} & \HoloSegScore{3.139}{(2.262--4.130)}{4.55pt}{4.82pt}{} & \HoloSegScore{2.595}{(2.196--2.957)}{4.55pt}{4.82pt}{} & \HoloSegScore{3.810}{(2.860--4.034)}{4.55pt}{4.82pt}{} & \HoloSegScore{1.778}{(1.307--2.280)}{4.55pt}{4.82pt}{} & \HoloSegScore{1.676}{(1.298--2.050)}{4.55pt}{4.82pt}{} \\
\cline{3-11}
 &  &  & \HoloSegMetric{Dice} &  & \HoloSegScore{0.06729}{(0.03001--0.1004)}{4.20pt}{4.48pt}{} & \HoloSegScore{0.7071}{(0.6539--0.7580)}{4.55pt}{4.82pt}{} & \HoloSegScore{0.7682}{(0.7241--0.8094)}{4.55pt}{4.82pt}{} & \HoloSegScore{0.7667}{(0.7475--0.8131)}{4.55pt}{4.82pt}{} & \HoloSegScore{0.8136}{(0.7846--0.8426)}{4.55pt}{4.82pt}{} & \HoloSegScore{0.8290}{(0.7996--0.8574)}{4.55pt}{4.82pt}{} \\*
\softcline{4-4}\softcline{6-11}
 &  & \HoloSegSpan{\makecell[c]{right\\[-0.10ex]anterior\\[-0.10ex]eyeball}}{2.04cm}{0.32cm} & \HoloSegMetric{HD95} & \raisebox{0.32cm}[0pt][0pt]{\HoloSegUnsupported} & \HoloSegScore{16.92}{(14.73--19.39)}{4.55pt}{4.82pt}{} & \HoloSegScore{3.234}{(2.476--4.190)}{4.55pt}{4.82pt}{} & \HoloSegScore{2.652}{(1.869--3.653)}{4.55pt}{4.82pt}{} & \HoloSegScore{4.737}{(3.634--5.184)}{4.55pt}{4.82pt}{} & \HoloSegScore{1.758}{(1.413--2.183)}{4.55pt}{4.82pt}{} & \HoloSegScore{1.477}{(1.135--1.852)}{4.55pt}{4.82pt}{} \\
\cline{3-11}
 &  &  & \HoloSegMetric{Dice} &  & \HoloSegScore{0.4885}{(0.4366--0.5566)}{4.55pt}{4.82pt}{} & \HoloSegScore{0.9040}{(0.8928--0.9137)}{4.55pt}{4.82pt}{} & \HoloSegScore{0.8988}{(0.8911--0.9075)}{4.55pt}{4.82pt}{} & \HoloSegScore{0.8944}{(0.8923--0.9042)}{4.55pt}{4.82pt}{} & \HoloSegScore{0.9202}{(0.9026--0.9330)}{4.55pt}{4.82pt}{} & \HoloSegScore{0.9316}{(0.9211--0.9398)}{4.55pt}{4.82pt}{} \\*
\softcline{4-4}\softcline{6-11}
 &  & \HoloSegSpan{\makecell[c]{left\\[-0.10ex]posterior\\[-0.10ex]eyeball}}{2.04cm}{0.32cm} & \HoloSegMetric{HD95} & \raisebox{0.32cm}[0pt][0pt]{\HoloSegUnsupported} & \HoloSegScore{10.82}{(8.974--12.58)}{4.55pt}{4.82pt}{} & \HoloSegScore{1.994}{(1.693--2.323)}{4.55pt}{4.82pt}{} & \HoloSegScore{2.321}{(2.036--2.599)}{4.55pt}{4.82pt}{} & \HoloSegScore{4.022}{(3.169--4.122)}{4.55pt}{4.82pt}{} & \HoloSegScore{1.569}{(1.257--2.009)}{4.55pt}{4.82pt}{} & \HoloSegScore{1.283}{(1.100--1.476)}{4.55pt}{4.82pt}{} \\
\cline{3-11}
 &  &  & \HoloSegMetric{Dice} &  & \HoloSegScore{0.5039}{(0.4184--0.5784)}{4.55pt}{4.82pt}{} & \HoloSegScore{0.9062}{(0.9005--0.9134)}{4.55pt}{4.82pt}{} & \HoloSegScore{0.8955}{(0.8823--0.9103)}{4.55pt}{4.82pt}{} & \HoloSegScore{0.8852}{(0.8702--0.8969)}{4.55pt}{4.82pt}{} & \HoloSegScore{0.9122}{(0.9033--0.9218)}{4.55pt}{4.82pt}{} & \HoloSegScore{0.9293}{(0.9211--0.9362)}{4.55pt}{4.82pt}{} \\*
\softcline{4-4}\softcline{6-11}
 &  & \HoloSegSpan{\makecell[c]{right\\[-0.10ex]posterior\\[-0.10ex]eyeball}}{2.04cm}{0.32cm} & \HoloSegMetric{HD95} & \raisebox{0.32cm}[0pt][0pt]{\HoloSegUnsupported} & \HoloSegScore{10.71}{(8.487--12.79)}{4.55pt}{4.82pt}{} & \HoloSegScore{1.885}{(1.657--2.034)}{4.55pt}{4.82pt}{} & \HoloSegScore{2.078}{(1.798--2.421)}{4.55pt}{4.82pt}{} & \HoloSegScore{3.890}{(3.140--4.349)}{4.55pt}{4.82pt}{} & \HoloSegScore{1.810}{(1.505--2.204)}{4.55pt}{4.82pt}{} & \HoloSegScore{1.445}{(1.151--1.774)}{4.55pt}{4.82pt}{} \\
\hline
\pagebreak[4]
 &  &  & \HoloSegMetric{Dice} &  & \HoloSegScore{0.2007}{(0.09178--0.3300)}{4.20pt}{4.48pt}{} & \HoloSegScore{0.5300}{(0.3870--0.6326)}{4.55pt}{4.82pt}{} & \HoloSegScore{0.0000}{(0.0000--0.0000)}{4.55pt}{4.82pt}{} & \HoloSegScore{0.5280}{(0.5161--0.5298)}{4.55pt}{4.82pt}{} & \HoloSegScore{0.3817}{(0.2499--0.4961)}{4.55pt}{4.82pt}{} & \HoloSegScore{0.7802}{(0.7454--0.8059)}{4.55pt}{4.82pt}{} \\*
\softcline{4-4}\softcline{6-11}
 &  & \HoloSegSpan{\makecell[c]{left\\[-0.10ex]lacrimal\\[-0.10ex]gland}}{2.04cm}{0.32cm} & \HoloSegMetric{HD95} & \raisebox{0.32cm}[0pt][0pt]{\HoloSegUnsupported} & \HoloSegScore{33.46}{(10.02--61.37)}{4.55pt}{4.82pt}{} & \HoloSegScore{4.404}{(2.728--6.754)}{4.55pt}{4.82pt}{} & \HoloSegScore{--}{(--\,--)}{4.55pt}{4.82pt}{} & \HoloSegScore{5.584}{(4.995--6.750)}{4.55pt}{4.82pt}{} & \HoloSegScore{4.392}{(3.381--5.333)}{4.55pt}{4.82pt}{} & \HoloSegScore{1.807}{(1.238--2.494)}{4.55pt}{4.82pt}{} \\
\cline{3-11}
 &  &  & \HoloSegMetric{Dice} &  & \HoloSegScore{0.1025}{(0.05153--0.1520)}{4.20pt}{4.48pt}{} & \HoloSegScore{0.4334}{(0.3186--0.5382)}{4.55pt}{4.82pt}{} & \HoloSegScore{0.0000}{(0.0000--0.0000)}{4.55pt}{4.82pt}{} & \HoloSegScore{0.5158}{(0.4654--0.5681)}{4.55pt}{4.82pt}{} & \HoloSegScore{0.6667}{(0.5507--0.7585)}{4.55pt}{4.82pt}{} & \HoloSegScore{0.6795}{(0.5950--0.7390)}{4.55pt}{4.82pt}{} \\*
\softcline{4-4}\softcline{6-11}
 &  & \HoloSegSpan{\makecell[c]{right\\[-0.10ex]lacrimal\\[-0.10ex]gland}}{2.04cm}{0.32cm} & \HoloSegMetric{HD95} & \raisebox{0.32cm}[0pt][0pt]{\HoloSegUnsupported} & \HoloSegScore{17.85}{(13.86--22.33)}{4.55pt}{4.82pt}{} & \HoloSegScore{4.933}{(3.582--6.427)}{4.55pt}{4.82pt}{} & \HoloSegScore{--}{(--\,--)}{4.55pt}{4.82pt}{} & \HoloSegScore{5.791}{(4.841--6.983)}{4.55pt}{4.82pt}{} & \HoloSegScore{2.914}{(1.744--4.816)}{4.55pt}{4.82pt}{} & \HoloSegScore{2.028}{(1.464--2.718)}{4.55pt}{4.82pt}{} \\
\cline{3-11}
 &  &  & \HoloSegMetric{Dice} &  & \HoloSegScore{0.4114}{(0.3025--0.5113)}{4.55pt}{4.82pt}{} & \HoloSegScore{0.8340}{(0.8048--0.8642)}{4.55pt}{4.82pt}{} & \HoloSegScore{0.8565}{(0.8417--0.8716)}{4.55pt}{4.82pt}{} & \HoloSegScore{0.8553}{(0.8245--0.8789)}{4.55pt}{4.82pt}{} & \HoloSegScore{0.8450}{(0.8148--0.8702)}{4.55pt}{4.82pt}{} & \HoloSegScore{0.8882}{(0.8660--0.9034)}{4.55pt}{4.82pt}{} \\*
\softcline{4-4}\softcline{6-11}
 &  & \HoloSegSpan{\makecell[c]{left\\[-0.10ex]submandibular\\[-0.10ex]gland}}{2.04cm}{0.32cm} & \HoloSegMetric{HD95} & \raisebox{0.32cm}[0pt][0pt]{\HoloSegUnsupported} & \HoloSegScore{33.71}{(16.03--55.84)}{4.55pt}{4.82pt}{} & \HoloSegScore{3.894}{(2.635--5.343)}{4.55pt}{4.82pt}{} & \HoloSegScore{3.691}{(2.548--5.214)}{4.55pt}{4.82pt}{} & \HoloSegScore{3.988}{(3.395--4.017)}{4.55pt}{4.82pt}{} & \HoloSegScore{2.820}{(2.174--3.506)}{4.55pt}{4.82pt}{} & \HoloSegScore{2.038}{(1.522--2.569)}{4.55pt}{4.82pt}{} \\
\cline{3-11}
 &  &  & \HoloSegMetric{Dice} &  & \HoloSegScore{0.3547}{(0.2342--0.4755)}{4.55pt}{4.82pt}{} & \HoloSegScore{0.7913}{(0.7188--0.8501)}{4.55pt}{4.82pt}{} & \HoloSegScore{0.8498}{(0.8309--0.8698)}{4.55pt}{4.82pt}{} & \HoloSegScore{0.8398}{(0.8274--0.8845)}{4.55pt}{4.82pt}{} & \HoloSegScore{0.8528}{(0.8178--0.8851)}{4.55pt}{4.82pt}{} & \HoloSegScore{0.8566}{(0.8311--0.8770)}{4.55pt}{4.82pt}{} \\*
\softcline{4-4}\softcline{6-11}
 &  & \HoloSegSpan{\makecell[c]{right\\[-0.10ex]submandibular\\[-0.10ex]gland}}{2.04cm}{0.32cm} & \HoloSegMetric{HD95} & \raisebox{0.32cm}[0pt][0pt]{\HoloSegUnsupported} & \HoloSegScore{30.94}{(15.38--45.70)}{4.55pt}{4.82pt}{} & \HoloSegScore{4.851}{(2.932--7.223)}{4.55pt}{4.82pt}{} & \HoloSegScore{3.178}{(2.511--4.018)}{4.55pt}{4.82pt}{} & \HoloSegScore{5.004}{(4.535--7.257)}{4.55pt}{4.82pt}{} & \HoloSegScore{2.883}{(2.133--3.719)}{4.55pt}{4.82pt}{} & \HoloSegScore{2.432}{(2.006--2.900)}{4.55pt}{4.82pt}{} \\
\cline{3-11}
 &  &  & \HoloSegMetric{Dice} & \HoloSegScore{0.8137}{(0.7950--0.8325)}{4.55pt}{4.82pt}{} & \HoloSegScore{0.0000}{(0.0000--0.0000)}{4.55pt}{4.82pt}{} & \HoloSegScore{0.8479}{(0.8367--0.8613)}{4.55pt}{4.82pt}{} & \HoloSegScore{0.8677}{(0.8532--0.8816)}{4.55pt}{4.82pt}{} & \HoloSegScore{0.8253}{(0.7967--0.8263)}{4.55pt}{4.82pt}{} & \HoloSegScore{0.8703}{(0.8588--0.8852)}{4.55pt}{4.82pt}{} & \HoloSegScore{0.8716}{(0.8543--0.8910)}{4.55pt}{4.82pt}{} \\*
\softcline{4-11}
 &  & \HoloSegSpan{\makecell[c]{thyroid}}{2.04cm}{0.32cm} & \HoloSegMetric{HD95} & \HoloSegScore{3.905}{(3.128--4.753)}{4.55pt}{4.82pt}{} & \HoloSegScore{110.7}{(99.82--118.6)}{4.55pt}{4.82pt}{} & \HoloSegScore{2.293}{(1.992--2.771)}{4.55pt}{4.82pt}{} & \HoloSegScore{2.147}{(1.619--2.775)}{4.55pt}{4.82pt}{} & \HoloSegScore{3.296}{(3.193--3.456)}{4.55pt}{4.82pt}{} & \HoloSegScore{1.992}{(1.641--2.400)}{4.55pt}{4.82pt}{} & \HoloSegScore{2.021}{(1.617--2.428)}{4.55pt}{4.82pt}{} \\
\cline{3-11}
 &  &  & \HoloSegMetric{Dice} &  & \HoloSegScore{0.1268}{(0.05605--0.1989)}{4.20pt}{4.48pt}{} & \HoloSegScore{0.6792}{(0.6251--0.7346)}{4.55pt}{4.82pt}{} & \HoloSegScore{0.7068}{(0.6351--0.7692)}{4.55pt}{4.82pt}{} & \HoloSegScore{0.6764}{(0.6255--0.7295)}{4.55pt}{4.82pt}{} & \HoloSegScore{0.7462}{(0.6932--0.7965)}{4.55pt}{4.82pt}{} & \HoloSegScore{0.7859}{(0.7703--0.8006)}{4.55pt}{4.82pt}{} \\*
\softcline{4-4}\softcline{6-11}
 &  & \HoloSegSpan{\makecell[c]{larynx\\[-0.10ex]glottis}}{2.04cm}{0.32cm} & \HoloSegMetric{HD95} & \raisebox{0.32cm}[0pt][0pt]{\HoloSegUnsupported} & \HoloSegScore{15.92}{(13.03--19.25)}{4.55pt}{4.82pt}{} & \HoloSegScore{3.798}{(2.746--4.798)}{4.55pt}{4.82pt}{} & \HoloSegScore{3.852}{(2.524--5.109)}{4.55pt}{4.82pt}{} & \HoloSegScore{5.479}{(4.040--5.657)}{4.55pt}{4.82pt}{} & \HoloSegScore{2.570}{(2.246--2.901)}{4.55pt}{4.82pt}{} & \HoloSegScore{2.663}{(2.252--3.113)}{4.55pt}{4.82pt}{} \\
\cline{3-11}
 &  &  & \HoloSegMetric{Dice} &  & \HoloSegScore{0.3091}{(0.2042--0.4112)}{4.55pt}{4.82pt}{} & \HoloSegScore{0.7602}{(0.7392--0.7794)}{4.55pt}{4.82pt}{} & \HoloSegScore{0.7934}{(0.7563--0.8271)}{4.55pt}{4.82pt}{} & \HoloSegScore{0.7573}{(0.7337--0.7868)}{4.55pt}{4.82pt}{} & \HoloSegScore{0.8200}{(0.8075--0.8336)}{4.55pt}{4.82pt}{} & \HoloSegScore{0.8336}{(0.8135--0.8513)}{4.55pt}{4.82pt}{} \\*
\softcline{4-4}\softcline{6-11}
 &  & \HoloSegSpan{\makecell[c]{larynx\\[-0.10ex]supraglottis}}{2.04cm}{0.32cm} & \HoloSegMetric{HD95} & \raisebox{0.32cm}[0pt][0pt]{\HoloSegUnsupported} & \HoloSegScore{34.45}{(18.97--52.07)}{4.55pt}{4.82pt}{} & \HoloSegScore{3.880}{(3.358--4.530)}{4.55pt}{4.82pt}{} & \HoloSegScore{3.872}{(2.877--5.020)}{4.55pt}{4.82pt}{} & \HoloSegScore{6.034}{(4.601--6.892)}{4.55pt}{4.82pt}{} & \HoloSegScore{3.452}{(2.883--4.099)}{4.55pt}{4.82pt}{} & \HoloSegScore{2.756}{(2.490--2.988)}{4.55pt}{4.82pt}{} \\
\cline{3-11}
 &  &  & \HoloSegMetric{Dice} &  & \HoloSegScore{0.4118}{(0.3514--0.4768)}{4.55pt}{4.82pt}{} & \HoloSegScore{0.6170}{(0.5683--0.6715)}{4.55pt}{4.82pt}{} & \HoloSegScore{0.6486}{(0.5858--0.7207)}{4.55pt}{4.82pt}{} & \HoloSegScore{0.6411}{(0.5798--0.6915)}{4.55pt}{4.82pt}{} & \HoloSegScore{0.7135}{(0.6789--0.7486)}{4.55pt}{4.82pt}{} & \HoloSegScore{0.7840}{(0.7431--0.8269)}{4.55pt}{4.82pt}{} \\*
\softcline{4-4}\softcline{6-11}
 & \HoloSegSpan{\makecell[c]{HaN-Seg}}{1.86cm}{0.32cm} & \HoloSegSpan{\makecell[c]{lips}}{2.04cm}{0.32cm} & \HoloSegMetric{HD95} & \raisebox{0.32cm}[0pt][0pt]{\HoloSegUnsupported} & \HoloSegScore{12.61}{(10.76--14.29)}{4.55pt}{4.82pt}{} & \HoloSegScore{6.915}{(5.774--8.462)}{4.55pt}{4.82pt}{} & \HoloSegScore{8.342}{(5.769--10.95)}{4.55pt}{4.82pt}{} & \HoloSegScore{6.332}{(5.583--8.446)}{4.55pt}{4.82pt}{} & \HoloSegScore{4.667}{(4.034--5.315)}{4.55pt}{4.82pt}{} & \HoloSegScore{3.112}{(2.742--3.458)}{4.55pt}{4.82pt}{} \\
\cline{3-11}
 &  &  & \HoloSegMetric{Dice} &  & \HoloSegScore{0.0000}{(0.0000--0.0000)}{4.55pt}{4.82pt}{} & \HoloSegScore{0.4159}{(0.3603--0.4634)}{4.55pt}{4.82pt}{} & \HoloSegScore{0.5223}{(0.4716--0.5662)}{4.55pt}{4.82pt}{} & \HoloSegScore{0.3865}{(0.3505--0.4273)}{4.55pt}{4.82pt}{} & \HoloSegScore{0.5704}{(0.5148--0.6292)}{4.55pt}{4.82pt}{} & \HoloSegScore{0.6780}{(0.6170--0.7286)}{4.55pt}{4.82pt}{} \\*
\softcline{4-4}\softcline{6-11}
 &  & \HoloSegSpan{\makecell[c]{optic chiasm}}{2.04cm}{0.32cm} & \HoloSegMetric{HD95} & \raisebox{0.32cm}[0pt][0pt]{\HoloSegUnsupported} & \HoloSegScore{156.7}{(142.2--168.2)}{4.55pt}{4.82pt}{} & \HoloSegScore{3.677}{(3.080--4.360)}{4.55pt}{4.82pt}{} & \HoloSegScore{3.721}{(2.971--4.548)}{4.55pt}{4.82pt}{} & \HoloSegScore{4.678}{(3.971--6.244)}{4.55pt}{4.82pt}{} & \HoloSegScore{3.097}{(2.618--3.556)}{4.55pt}{4.82pt}{} & \HoloSegScore{2.658}{(2.216--3.122)}{4.55pt}{4.82pt}{} \\
\cline{3-11}
 &  &  & \HoloSegMetric{Dice} &  & \HoloSegScore{0.0001222}{(0.0000--0.0003666)}{3.85pt}{4.12pt}{} & \HoloSegScore{0.5747}{(0.4451--0.6662)}{4.55pt}{4.82pt}{} & \HoloSegScore{0.6153}{(0.5424--0.6899)}{4.55pt}{4.82pt}{} & \HoloSegScore{0.5652}{(0.5223--0.6177)}{4.55pt}{4.82pt}{} & \HoloSegScore{0.7131}{(0.6553--0.7583)}{4.55pt}{4.82pt}{} & \HoloSegScore{0.7903}{(0.7339--0.8368)}{4.55pt}{4.82pt}{} \\*
\softcline{4-4}\softcline{6-11}
\HoloSegSpan{\makecell[c]{\textbf{Internal}}}{1.20cm}{0.32cm} &  & \HoloSegSpan{\makecell[c]{left optic\\[-0.10ex]nerve}}{2.04cm}{0.32cm} & \HoloSegMetric{HD95} & \raisebox{0.32cm}[0pt][0pt]{\HoloSegUnsupported} & \HoloSegScore{123.9}{(95.42--140.3)}{4.55pt}{4.82pt}{} & \HoloSegScore{3.003}{(2.443--3.588)}{4.55pt}{4.82pt}{} & \HoloSegScore{5.691}{(3.519--8.045)}{4.55pt}{4.82pt}{} & \HoloSegScore{4.792}{(3.726--7.302)}{4.55pt}{4.82pt}{} & \HoloSegScore{12.02}{(2.525--23.16)}{4.55pt}{4.82pt}{} & \HoloSegScore{1.936}{(1.434--2.435)}{4.55pt}{4.82pt}{} \\
\cline{3-11}
 &  &  & \HoloSegMetric{Dice} &  & \HoloSegScore{0.004694}{(0.0000--0.01408)}{4.20pt}{4.48pt}{} & \HoloSegScore{0.6576}{(0.6025--0.7092)}{4.55pt}{4.82pt}{} & \HoloSegScore{0.6609}{(0.6082--0.6971)}{4.55pt}{4.82pt}{} & \HoloSegScore{0.6433}{(0.5937--0.6743)}{4.55pt}{4.82pt}{} & \HoloSegScore{0.7405}{(0.7170--0.7655)}{4.55pt}{4.82pt}{} & \HoloSegScore{0.7218}{(0.6509--0.7756)}{4.55pt}{4.82pt}{} \\*
\softcline{4-4}\softcline{6-11}
 &  & \HoloSegSpan{\makecell[c]{right optic\\[-0.10ex]nerve}}{2.04cm}{0.32cm} & \HoloSegMetric{HD95} & \raisebox{0.32cm}[0pt][0pt]{\HoloSegUnsupported} & \HoloSegScore{77.57}{(41.38--117.6)}{4.55pt}{4.82pt}{} & \HoloSegScore{3.037}{(2.404--3.991)}{4.55pt}{4.82pt}{} & \HoloSegScore{4.108}{(2.687--5.596)}{4.55pt}{4.82pt}{} & \HoloSegScore{4.330}{(2.523--5.427)}{4.55pt}{4.82pt}{} & \HoloSegScore{3.571}{(2.653--4.564)}{4.55pt}{4.82pt}{} & \HoloSegScore{2.478}{(1.812--3.136)}{4.55pt}{4.82pt}{} \\
\cline{3-11}
 &  &  & \HoloSegMetric{Dice} &  & \HoloSegScore{0.5415}{(0.4404--0.6314)}{4.55pt}{4.82pt}{} & \HoloSegScore{0.8186}{(0.7915--0.8418)}{4.55pt}{4.82pt}{} & \HoloSegScore{0.8267}{(0.7975--0.8537)}{4.55pt}{4.82pt}{} & \HoloSegScore{0.8070}{(0.7661--0.8416)}{4.55pt}{4.82pt}{} & \HoloSegScore{0.8446}{(0.8274--0.8582)}{4.55pt}{4.82pt}{} & \HoloSegScore{0.8567}{(0.8365--0.8737)}{4.55pt}{4.82pt}{} \\*
\softcline{4-4}\softcline{6-11}
 &  & \HoloSegSpan{\makecell[c]{left parotid\\[-0.10ex]gland}}{2.04cm}{0.32cm} & \HoloSegMetric{HD95} & \raisebox{0.32cm}[0pt][0pt]{\HoloSegUnsupported} & \HoloSegScore{24.11}{(10.43--44.59)}{4.55pt}{4.82pt}{} & \HoloSegScore{6.398}{(4.891--8.804)}{4.55pt}{4.82pt}{} & \HoloSegScore{7.011}{(5.452--9.054)}{4.55pt}{4.82pt}{} & \HoloSegScore{8.537}{(6.659--10.82)}{4.55pt}{4.82pt}{} & \HoloSegScore{5.482}{(3.694--7.709)}{4.55pt}{4.82pt}{} & \HoloSegScore{5.381}{(3.799--7.526)}{4.55pt}{4.82pt}{} \\
\cline{3-11}
 &  &  & \HoloSegMetric{Dice} &  & \HoloSegScore{0.5631}{(0.4671--0.6505)}{4.55pt}{4.82pt}{} & \HoloSegScore{0.7916}{(0.7402--0.8383)}{4.55pt}{4.82pt}{} & \HoloSegScore{0.7985}{(0.7503--0.8393)}{4.55pt}{4.82pt}{} & \HoloSegScore{0.7861}{(0.7333--0.8297)}{4.55pt}{4.82pt}{} & \HoloSegScore{0.8312}{(0.8099--0.8499)}{4.55pt}{4.82pt}{} & \HoloSegScore{0.8581}{(0.8388--0.8763)}{4.55pt}{4.82pt}{} \\*
\softcline{4-4}\softcline{6-11}
 &  & \HoloSegSpan{\makecell[c]{right\\[-0.10ex]parotid\\[-0.10ex]gland}}{2.04cm}{0.32cm} & \HoloSegMetric{HD95} & \raisebox{0.32cm}[0pt][0pt]{\HoloSegUnsupported} & \HoloSegScore{21.11}{(8.910--44.17)}{4.55pt}{4.82pt}{} & \HoloSegScore{5.459}{(4.519--6.602)}{4.55pt}{4.82pt}{} & \HoloSegScore{6.442}{(5.288--7.806)}{4.55pt}{4.82pt}{} & \HoloSegScore{9.373}{(8.275--11.24)}{4.55pt}{4.82pt}{} & \HoloSegScore{4.875}{(3.784--6.161)}{4.55pt}{4.82pt}{} & \HoloSegScore{3.221}{(2.911--3.542)}{4.55pt}{4.82pt}{} \\
\cline{3-11}
 &  &  & \HoloSegMetric{Dice} &  & \HoloSegScore{0.0000}{(0.0000--0.0000)}{4.55pt}{4.82pt}{} & \HoloSegScore{0.6126}{(0.5044--0.7052)}{4.55pt}{4.82pt}{} & \HoloSegScore{0.7403}{(0.6793--0.8064)}{4.55pt}{4.82pt}{} & \HoloSegScore{0.6551}{(0.5798--0.7039)}{4.55pt}{4.82pt}{} & \HoloSegScore{0.7674}{(0.6220--0.8487)}{4.55pt}{4.82pt}{} & \HoloSegScore{0.7953}{(0.7589--0.8254)}{4.55pt}{4.82pt}{} \\*
\softcline{4-4}\softcline{6-11}
 &  & \HoloSegSpan{\makecell[c]{pituitary\\[-0.10ex]gland}}{2.04cm}{0.32cm} & \HoloSegMetric{HD95} & \raisebox{0.32cm}[0pt][0pt]{\HoloSegUnsupported} & \HoloSegScore{147.0}{(138.8--154.7)}{4.55pt}{4.82pt}{} & \HoloSegScore{2.815}{(2.138--3.414)}{4.55pt}{4.82pt}{} & \HoloSegScore{1.965}{(1.469--2.500)}{4.55pt}{4.82pt}{} & \HoloSegScore{4.164}{(2.061--4.501)}{4.55pt}{4.82pt}{} & \HoloSegScore{1.393}{(1.007--1.889)}{4.55pt}{4.82pt}{} & \HoloSegScore{1.462}{(1.234--1.686)}{4.55pt}{4.82pt}{} \\
\cline{3-11}
 &  &  & \HoloSegMetric{Dice} & \HoloSegScore{0.3798}{(0.3482--0.4187)}{4.55pt}{4.82pt}{} & \HoloSegScore{0.3246}{(0.2266--0.4031)}{4.55pt}{4.82pt}{} & \HoloSegScore{0.7291}{(0.6480--0.7843)}{4.55pt}{4.82pt}{} & \HoloSegScore{0.4867}{(0.4522--0.5249)}{4.55pt}{4.82pt}{} & \HoloSegScore{0.7224}{(0.6868--0.7596)}{4.55pt}{4.82pt}{} & \HoloSegScore{0.8082}{(0.7866--0.8327)}{4.55pt}{4.82pt}{} & \HoloSegScore{0.7892}{(0.7642--0.8125)}{4.55pt}{4.82pt}{} \\*
\softcline{4-11}
 &  & \HoloSegSpan{\makecell[c]{spinal cord}}{2.04cm}{0.32cm} & \HoloSegMetric{HD95} & \HoloSegScore{80.45}{(74.34--87.15)}{4.55pt}{4.82pt}{} & \HoloSegScore{47.27}{(32.51--63.18)}{4.55pt}{4.82pt}{} & \HoloSegScore{10.21}{(2.433--25.42)}{4.55pt}{4.82pt}{} & \HoloSegScore{78.12}{(71.77--84.23)}{4.55pt}{4.82pt}{} & \HoloSegScore{12.13}{(7.890--17.83)}{4.55pt}{4.82pt}{} & \HoloSegScore{2.127}{(1.824--2.453)}{4.55pt}{4.82pt}{} & \HoloSegScore{8.460}{(2.442--20.12)}{4.55pt}{4.82pt}{} \\
\cline{2-11}
 &  &  & \HoloSegMetric{Dice} & \HoloSegScore{0.8548}{(0.8311--0.8749)}{4.55pt}{4.82pt}{} & \HoloSegScore{0.7126}{(0.6868--0.7349)}{4.55pt}{4.82pt}{} & \HoloSegScore{0.8560}{(0.8271--0.8850)}{4.55pt}{4.82pt}{} & \HoloSegScore{0.8589}{(0.8298--0.8867)}{4.55pt}{4.82pt}{} & \HoloSegScore{0.9031}{(0.8762--0.9199)}{4.55pt}{4.82pt}{} & \HoloSegScore{0.9231}{(0.9032--0.9374)}{4.55pt}{4.82pt}{} & \HoloSegScore{0.9196}{(0.8977--0.9352)}{4.55pt}{4.82pt}{} \\*
\softcline{4-11}
 &  & \HoloSegSpan{\makecell[c]{kidney}}{2.04cm}{0.32cm} & \HoloSegMetric{HD95} & \HoloSegScore{14.67}{(10.48--19.51)}{4.55pt}{4.82pt}{} & \HoloSegScore{18.87}{(14.81--24.01)}{4.55pt}{4.82pt}{} & \HoloSegScore{9.862}{(6.794--13.77)}{4.55pt}{4.82pt}{} & \HoloSegScore{11.49}{(7.874--15.84)}{4.55pt}{4.82pt}{} & \HoloSegScore{13.89}{(10.11--17.81)}{4.55pt}{4.82pt}{} & \HoloSegScore{11.01}{(7.595--15.52)}{4.55pt}{4.82pt}{} & \HoloSegScore{9.792}{(6.622--13.92)}{4.55pt}{4.82pt}{} \\
\cline{3-11}
 &  &  & \HoloSegMetric{Dice} &  & \HoloSegScore{0.2293}{(0.1747--0.2853)}{4.55pt}{4.82pt}{} & \HoloSegScore{0.6648}{(0.6083--0.7217)}{4.55pt}{4.82pt}{} & \HoloSegScore{0.8045}{(0.7578--0.8429)}{4.55pt}{4.82pt}{} & \HoloSegScore{0.7980}{(0.7797--0.8258)}{4.55pt}{4.82pt}{} & \HoloSegScore{0.7273}{(0.6728--0.7784)}{4.55pt}{4.82pt}{} & \HoloSegScore{0.7423}{(0.6918--0.7921)}{4.55pt}{4.82pt}{} \\*
\softcline{4-4}\softcline{6-11}
 & \HoloSegSpan{\makecell[c]{KiTS23}}{1.86cm}{0.32cm} & \HoloSegSpan{\makecell[c]{kidney tumor}}{2.04cm}{0.32cm} & \HoloSegMetric{HD95} & \raisebox{0.32cm}[0pt][0pt]{\HoloSegUnsupported} & \HoloSegScore{102.9}{(88.85--116.2)}{4.55pt}{4.82pt}{} & \HoloSegScore{21.43}{(13.85--30.37)}{4.55pt}{4.82pt}{} & \HoloSegScore{24.21}{(15.95--33.43)}{4.55pt}{4.82pt}{} & \HoloSegScore{21.88}{(14.33--30.05)}{4.55pt}{4.82pt}{} & \HoloSegScore{39.78}{(28.49--52.17)}{4.55pt}{4.82pt}{} & \HoloSegScore{30.95}{(21.79--41.64)}{4.55pt}{4.82pt}{} \\
\cline{3-11}
 &  &  & \HoloSegMetric{Dice} & \HoloSegScore{0.2168}{(0.1476--0.2892)}{4.55pt}{4.82pt}{} & \HoloSegScore{0.04249}{(0.01424--0.07457)}{4.20pt}{4.48pt}{} & \HoloSegScore{0.4887}{(0.4021--0.5744)}{4.55pt}{4.82pt}{} & \HoloSegScore{0.0000}{(0.0000--0.0000)}{4.55pt}{4.82pt}{} & \HoloSegScore{0.5587}{(0.5342--0.6164)}{4.55pt}{4.82pt}{} & \HoloSegScore{0.5008}{(0.4198--0.5839)}{4.55pt}{4.82pt}{} & \HoloSegScore{0.6101}{(0.5298--0.6828)}{4.55pt}{4.82pt}{} \\*
\softcline{4-11}
 &  & \HoloSegSpan{\makecell[c]{kidney cyst}}{2.04cm}{0.32cm} & \HoloSegMetric{HD95} & \HoloSegScore{100.9}{(84.82--118.7)}{4.55pt}{4.82pt}{} & \HoloSegScore{111.2}{(93.01--129.0)}{4.55pt}{4.82pt}{} & \HoloSegScore{46.93}{(32.80--60.68)}{4.55pt}{4.82pt}{} & \HoloSegScore{--}{(--\,--)}{4.55pt}{4.82pt}{} & \HoloSegScore{46.42}{(32.77--60.41)}{4.55pt}{4.82pt}{} & \HoloSegScore{52.41}{(38.00--66.49)}{4.55pt}{4.82pt}{} & \HoloSegScore{58.91}{(45.17--75.34)}{4.55pt}{4.82pt}{} \\
\cline{2-11}
 &  &  & \HoloSegMetric{Dice} &  & \HoloSegScore{0.6385}{(0.6065--0.6700)}{4.55pt}{4.82pt}{} & \HoloSegScore{0.6772}{(0.6098--0.7348)}{4.55pt}{4.82pt}{} & \HoloSegScore{0.8394}{(0.8168--0.8607)}{4.55pt}{4.82pt}{} & \HoloSegScore{0.7543}{(0.7246--0.7997)}{4.55pt}{4.82pt}{} & \HoloSegScore{0.7422}{(0.6977--0.7823)}{4.55pt}{4.82pt}{} & \HoloSegScore{0.7976}{(0.7622--0.8286)}{4.55pt}{4.82pt}{} \\*
\softcline{4-4}\softcline{6-11}
 & \HoloSegSpan{\makecell[c]{KiPA22}}{1.86cm}{0.32cm} & \HoloSegSpan{\makecell[c]{renal vein}}{2.04cm}{0.32cm} & \HoloSegMetric{HD95} & \raisebox{0.32cm}[0pt][0pt]{\HoloSegUnsupported} & \HoloSegScore{6.152}{(5.076--7.427)}{4.55pt}{4.82pt}{} & \HoloSegScore{6.641}{(4.734--9.093)}{4.55pt}{4.82pt}{} & \HoloSegScore{3.773}{(2.805--4.862)}{4.55pt}{4.82pt}{} & \HoloSegScore{4.370}{(1.470--7.038)}{4.55pt}{4.82pt}{} & \HoloSegScore{8.281}{(6.031--11.29)}{4.55pt}{4.82pt}{} & \HoloSegScore{5.026}{(3.795--6.334)}{4.55pt}{4.82pt}{} \\
\hline
\pagebreak[4]
 &  &  & \HoloSegMetric{Dice} & \HoloSegScore{0.8311}{(0.6946--0.9087)}{4.55pt}{4.82pt}{} & \HoloSegScore{0.9259}{(0.9194--0.9311)}{4.55pt}{4.82pt}{} & \HoloSegScore{0.8802}{(0.8415--0.9135)}{4.55pt}{4.82pt}{} & \HoloSegScore{0.8849}{(0.8324--0.9271)}{4.55pt}{4.82pt}{} & \HoloSegScore{0.9133}{(0.9106--0.9198)}{4.55pt}{4.82pt}{} & \HoloSegScore{0.9377}{(0.9277--0.9463)}{4.55pt}{4.82pt}{} & \HoloSegScore{0.9475}{(0.9429--0.9517)}{4.55pt}{4.82pt}{} \\*
\softcline{4-11}
 &  & \HoloSegSpan{\makecell[c]{kidney}}{2.04cm}{0.32cm} & \HoloSegMetric{HD95} & \HoloSegScore{10.85}{(6.635--16.81)}{4.55pt}{4.82pt}{} & \HoloSegScore{3.969}{(3.537--4.473)}{4.55pt}{4.82pt}{} & \HoloSegScore{11.22}{(6.606--17.01)}{4.55pt}{4.82pt}{} & \HoloSegScore{13.44}{(8.381--20.07)}{4.55pt}{4.82pt}{} & \HoloSegScore{4.564}{(2.791--5.287)}{4.55pt}{4.82pt}{} & \HoloSegScore{5.803}{(4.671--7.620)}{4.55pt}{4.82pt}{} & \HoloSegScore{3.989}{(3.538--4.513)}{4.55pt}{4.82pt}{} \\
\cline{3-11}
 &  &  & \HoloSegMetric{Dice} &  & \HoloSegScore{0.4047}{(0.3813--0.4295)}{4.55pt}{4.82pt}{} & \HoloSegScore{0.6205}{(0.5985--0.6397)}{4.55pt}{4.82pt}{} & \HoloSegScore{0.8634}{(0.8353--0.8878)}{4.55pt}{4.82pt}{} & \HoloSegScore{0.8552}{(0.8412--0.8781)}{4.55pt}{4.82pt}{} & \HoloSegScore{0.6887}{(0.6540--0.7210)}{4.55pt}{4.82pt}{} & \HoloSegScore{0.6579}{(0.6157--0.6935)}{4.55pt}{4.82pt}{} \\*
\softcline{4-4}\softcline{6-11}
 & \HoloSegSpan{\makecell[c]{KiPA22}}{1.86cm}{0.32cm} & \HoloSegSpan{\makecell[c]{renal artery}}{2.04cm}{0.32cm} & \HoloSegMetric{HD95} & \raisebox{0.32cm}[0pt][0pt]{\HoloSegUnsupported} & \HoloSegScore{16.05}{(13.97--17.82)}{4.55pt}{4.82pt}{} & \HoloSegScore{10.48}{(3.746--23.20)}{4.55pt}{4.82pt}{} & \HoloSegScore{2.765}{(2.252--3.333)}{4.55pt}{4.82pt}{} & \HoloSegScore{14.08}{(13.66--15.20)}{4.55pt}{4.82pt}{} & \HoloSegScore{12.18}{(9.391--16.66)}{4.55pt}{4.82pt}{} & \HoloSegScore{14.27}{(12.63--16.09)}{4.55pt}{4.82pt}{} \\
\cline{3-11}
 &  &  & \HoloSegMetric{Dice} &  & \HoloSegScore{0.8362}{(0.8121--0.8623)}{4.55pt}{4.82pt}{} & \HoloSegScore{0.5844}{(0.3893--0.7493)}{4.55pt}{4.82pt}{} & \HoloSegScore{0.9332}{(0.9230--0.9436)}{4.55pt}{4.82pt}{} & \HoloSegScore{0.8347}{(0.8127--0.8627)}{4.55pt}{4.82pt}{} & \HoloSegScore{0.8031}{(0.6565--0.9043)}{4.55pt}{4.82pt}{} & \HoloSegScore{0.8585}{(0.8113--0.8995)}{4.55pt}{4.82pt}{} \\*
\softcline{4-4}\softcline{6-11}
 &  & \HoloSegSpan{\makecell[c]{kidney tumor}}{2.04cm}{0.32cm} & \HoloSegMetric{HD95} & \raisebox{0.32cm}[0pt][0pt]{\HoloSegUnsupported} & \HoloSegScore{4.719}{(3.396--6.790)}{4.55pt}{4.82pt}{} & \HoloSegScore{7.071}{(4.251--10.02)}{4.55pt}{4.82pt}{} & \HoloSegScore{1.877}{(1.458--2.322)}{4.55pt}{4.82pt}{} & \HoloSegScore{4.924}{(4.365--5.946)}{4.55pt}{4.82pt}{} & \HoloSegScore{12.79}{(3.201--26.65)}{4.55pt}{4.82pt}{} & \HoloSegScore{3.950}{(2.630--5.652)}{4.55pt}{4.82pt}{} \\
\cline{2-11}
 &  &  & \HoloSegMetric{Dice} & \HoloSegScore{0.8941}{(0.8801--0.9133)}{4.55pt}{4.82pt}{} & \HoloSegScore{0.6998}{(0.2360--0.9467)}{4.55pt}{4.82pt}{} & \HoloSegScore{0.8343}{(0.8050--0.8637)}{4.55pt}{4.82pt}{} & \HoloSegScore{0.9393}{(0.9117--0.9596)}{4.55pt}{4.82pt}{} & \HoloSegScore{0.9431}{(0.9416--0.9511)}{4.55pt}{4.82pt}{} & \HoloSegScore{0.9687}{(0.9632--0.9747)}{4.55pt}{4.82pt}{} & \HoloSegScore{0.9705}{(0.9647--0.9763)}{4.55pt}{4.82pt}{} \\*
\softcline{4-11}
 & \HoloSegSpan{\makecell[c]{CHAOS}}{1.86cm}{0.32cm} & \HoloSegSpan{\makecell[c]{liver}}{2.04cm}{0.32cm} & \HoloSegMetric{HD95} & \HoloSegScore{25.69}{(20.36--31.01)}{4.55pt}{4.82pt}{} & \HoloSegScore{42.36}{(7.634--109.9)}{4.55pt}{4.82pt}{} & \HoloSegScore{34.21}{(27.13--46.20)}{4.55pt}{4.82pt}{} & \HoloSegScore{24.71}{(11.78--43.68)}{4.55pt}{4.82pt}{} & \HoloSegScore{7.890}{(4.861--8.858)}{4.55pt}{4.82pt}{} & \HoloSegScore{5.325}{(4.077--6.754)}{4.55pt}{4.82pt}{} & \HoloSegScore{4.235}{(3.273--5.420)}{4.55pt}{4.82pt}{} \\
\cline{2-11}
 &  &  & \HoloSegMetric{Dice} & \HoloSegScore{0.9641}{(0.9615--0.9668)}{4.55pt}{4.82pt}{} & \HoloSegScore{0.9058}{(0.8919--0.9155)}{4.55pt}{4.82pt}{} & \HoloSegScore{0.9767}{(0.9745--0.9788)}{4.55pt}{4.82pt}{} & \HoloSegScore{0.9804}{(0.9760--0.9843)}{4.55pt}{4.82pt}{} & \HoloSegScore{0.9405}{(0.9313--0.9570)}{4.55pt}{4.82pt}{} & \HoloSegScore{0.9933}{(0.9897--0.9964)}{4.55pt}{4.82pt}{} & \HoloSegScore{0.9800}{(0.9761--0.9837)}{4.55pt}{4.82pt}{} \\*
\softcline{4-11}
 &  & \HoloSegSpan{\makecell[c]{liver}}{2.04cm}{0.32cm} & \HoloSegMetric{HD95} & \HoloSegScore{3.763}{(3.414--4.343)}{4.55pt}{4.82pt}{} & \HoloSegScore{7.101}{(6.296--8.215)}{4.55pt}{4.82pt}{} & \HoloSegScore{2.737}{(2.500--3.210)}{4.55pt}{4.82pt}{} & \HoloSegScore{2.174}{(1.535--3.056)}{4.55pt}{4.82pt}{} & \HoloSegScore{3.819}{(2.350--3.892)}{4.55pt}{4.82pt}{} & \HoloSegScore{1.681}{(1.344--2.058)}{4.55pt}{4.82pt}{} & \HoloSegScore{1.978}{(1.633--2.366)}{4.55pt}{4.82pt}{} \\
\cline{3-11}
 &  &  & \HoloSegMetric{Dice} & \HoloSegScore{0.8977}{(0.8219--0.9402)}{4.55pt}{4.82pt}{} & \HoloSegScore{0.7498}{(0.5355--0.8737)}{4.55pt}{4.82pt}{} & \HoloSegScore{0.9682}{(0.9642--0.9720)}{4.55pt}{4.82pt}{} & \HoloSegScore{0.9718}{(0.9669--0.9767)}{4.55pt}{4.82pt}{} & \HoloSegScore{0.9332}{(0.9270--0.9352)}{4.55pt}{4.82pt}{} & \HoloSegScore{0.9826}{(0.9777--0.9873)}{4.55pt}{4.82pt}{} & \HoloSegScore{0.9786}{(0.9736--0.9828)}{4.55pt}{4.82pt}{} \\*
\softcline{4-11}
 &  & \HoloSegSpan{\makecell[c]{right kidney}}{2.04cm}{0.32cm} & \HoloSegMetric{HD95} & \HoloSegScore{11.48}{(7.652--15.56)}{4.55pt}{4.82pt}{} & \HoloSegScore{34.20}{(7.088--67.31)}{4.55pt}{4.82pt}{} & \HoloSegScore{3.524}{(2.288--5.153)}{4.55pt}{4.82pt}{} & \HoloSegScore{5.591}{(3.348--7.891)}{4.55pt}{4.82pt}{} & \HoloSegScore{5.163}{(4.174--7.799)}{4.55pt}{4.82pt}{} & \HoloSegScore{6.805}{(3.274--10.63)}{4.55pt}{4.82pt}{} & \HoloSegScore{2.718}{(1.608--4.440)}{4.55pt}{4.82pt}{} \\
\cline{3-11}
 &  &  & \HoloSegMetric{Dice} & \HoloSegScore{0.9586}{(0.9533--0.9629)}{4.55pt}{4.82pt}{} & \HoloSegScore{0.8574}{(0.8214--0.8872)}{4.55pt}{4.82pt}{} & \HoloSegScore{0.9716}{(0.9688--0.9747)}{4.55pt}{4.82pt}{} & \HoloSegScore{0.9842}{(0.9789--0.9884)}{4.55pt}{4.82pt}{} & \HoloSegScore{0.9608}{(0.9526--0.9680)}{4.55pt}{4.82pt}{} & \HoloSegScore{0.9957}{(0.9920--0.9993)}{4.55pt}{4.82pt}{} & \HoloSegScore{0.9829}{(0.9783--0.9868)}{4.55pt}{4.82pt}{} \\*
\softcline{4-11}
 &  & \HoloSegSpan{\makecell[c]{spleen}}{2.04cm}{0.32cm} & \HoloSegMetric{HD95} & \HoloSegScore{2.681}{(2.355--3.028)}{4.55pt}{4.82pt}{} & \HoloSegScore{5.692}{(5.103--6.631)}{4.55pt}{4.82pt}{} & \HoloSegScore{1.897}{(1.557--2.229)}{4.55pt}{4.82pt}{} & \HoloSegScore{0.7127}{(0.4451--0.9165)}{4.55pt}{4.82pt}{} & \HoloSegScore{2.821}{(1.739--4.213)}{4.55pt}{4.82pt}{} & \HoloSegScore{0.3951}{(0.3166--0.4873)}{4.55pt}{4.82pt}{} & \HoloSegScore{0.8911}{(0.8289--0.9557)}{4.55pt}{4.82pt}{} \\
\cline{3-11}
 &  &  & \HoloSegMetric{Dice} & \HoloSegScore{0.8610}{(0.8419--0.8789)}{4.55pt}{4.82pt}{} & \HoloSegScore{0.6625}{(0.6255--0.7008)}{4.55pt}{4.82pt}{} & \HoloSegScore{0.8756}{(0.8417--0.8999)}{4.55pt}{4.82pt}{} & \HoloSegScore{0.8849}{(0.8738--0.8976)}{4.55pt}{4.82pt}{} & \HoloSegScore{0.8796}{(0.8791--0.8865)}{4.55pt}{4.82pt}{} & \HoloSegScore{0.9067}{(0.8948--0.9199)}{4.55pt}{4.82pt}{} & \HoloSegScore{0.8954}{(0.8828--0.9078)}{4.55pt}{4.82pt}{} \\*
\softcline{4-11}
 &  & \HoloSegSpan{\makecell[c]{pancreas}}{2.04cm}{0.32cm} & \HoloSegMetric{HD95} & \HoloSegScore{6.081}{(4.531--8.499)}{4.55pt}{4.82pt}{} & \HoloSegScore{9.191}{(7.637--10.66)}{4.55pt}{4.82pt}{} & \HoloSegScore{4.809}{(3.029--7.594)}{4.55pt}{4.82pt}{} & \HoloSegScore{4.420}{(3.218--5.906)}{4.55pt}{4.82pt}{} & \HoloSegScore{5.145}{(3.820--5.795)}{4.55pt}{4.82pt}{} & \HoloSegScore{2.876}{(2.330--3.532)}{4.55pt}{4.82pt}{} & \HoloSegScore{3.282}{(2.854--3.748)}{4.55pt}{4.82pt}{} \\
\cline{3-11}
 &  &  & \HoloSegMetric{Dice} & \HoloSegScore{0.9089}{(0.8716--0.9357)}{4.55pt}{4.82pt}{} & \HoloSegScore{0.8390}{(0.8211--0.8558)}{4.55pt}{4.82pt}{} & \HoloSegScore{0.9467}{(0.9385--0.9538)}{4.55pt}{4.82pt}{} & \HoloSegScore{0.9490}{(0.9297--0.9647)}{4.55pt}{4.82pt}{} & \HoloSegScore{0.9345}{(0.9193--0.9471)}{4.55pt}{4.82pt}{} & \HoloSegScore{0.9740}{(0.9669--0.9800)}{4.55pt}{4.82pt}{} & \HoloSegScore{0.9580}{(0.9523--0.9633)}{4.55pt}{4.82pt}{} \\*
\softcline{4-11}
 &  & \HoloSegSpan{\makecell[c]{aorta}}{2.04cm}{0.32cm} & \HoloSegMetric{HD95} & \HoloSegScore{19.71}{(2.426--44.01)}{4.55pt}{4.82pt}{} & \HoloSegScore{4.260}{(3.779--4.775)}{4.55pt}{4.82pt}{} & \HoloSegScore{7.923}{(2.052--18.81)}{4.55pt}{4.82pt}{} & \HoloSegScore{17.30}{(0.9245--40.96)}{4.55pt}{4.82pt}{} & \HoloSegScore{2.735}{(1.477--3.997)}{4.55pt}{4.82pt}{} & \HoloSegScore{1.568}{(0.3805--3.808)}{4.55pt}{4.82pt}{} & \HoloSegScore{2.132}{(1.001--3.986)}{4.55pt}{4.82pt}{} \\
\cline{3-11}
 &  &  & \HoloSegMetric{Dice} & \HoloSegScore{0.8892}{(0.8712--0.9048)}{4.55pt}{4.82pt}{} & \HoloSegScore{0.7685}{(0.7402--0.7943)}{4.55pt}{4.82pt}{} & \HoloSegScore{0.9176}{(0.8962--0.9350)}{4.55pt}{4.82pt}{} & \HoloSegScore{0.9202}{(0.9051--0.9342)}{4.55pt}{4.82pt}{} & \HoloSegScore{0.9197}{(0.9076--0.9372)}{4.55pt}{4.82pt}{} & \HoloSegScore{0.9201}{(0.9060--0.9320)}{4.55pt}{4.82pt}{} & \HoloSegScore{0.9323}{(0.9197--0.9444)}{4.55pt}{4.82pt}{} \\*
\softcline{4-11}
\HoloSegSpan{\makecell[c]{\textbf{Internal}}}{1.20cm}{0.32cm} &  & \HoloSegSpan{\makecell[c]{inferior\\[-0.10ex]vena cava}}{2.04cm}{0.32cm} & \HoloSegMetric{HD95} & \HoloSegScore{10.37}{(7.105--13.70)}{4.55pt}{4.82pt}{} & \HoloSegScore{11.01}{(7.534--15.36)}{4.55pt}{4.82pt}{} & \HoloSegScore{4.232}{(2.713--6.623)}{4.55pt}{4.82pt}{} & \HoloSegScore{5.181}{(3.222--7.485)}{4.55pt}{4.82pt}{} & \HoloSegScore{4.828}{(3.311--6.897)}{4.55pt}{4.82pt}{} & \HoloSegScore{4.898}{(2.498--9.024)}{4.55pt}{4.82pt}{} & \HoloSegScore{3.027}{(2.193--3.995)}{4.55pt}{4.82pt}{} \\
\cline{3-11}
 &  &  & \HoloSegMetric{Dice} & \HoloSegScore{0.7829}{(0.7191--0.8333)}{4.55pt}{4.82pt}{} & \HoloSegScore{0.3339}{(0.2752--0.3872)}{4.55pt}{4.82pt}{} & \HoloSegScore{0.8380}{(0.8111--0.8601)}{4.55pt}{4.82pt}{} & \HoloSegScore{0.8405}{(0.7783--0.8900)}{4.55pt}{4.82pt}{} & \HoloSegScore{0.8165}{(0.7935--0.8579)}{4.55pt}{4.82pt}{} & \HoloSegScore{0.8623}{(0.8305--0.8900)}{4.55pt}{4.82pt}{} & \HoloSegScore{0.8651}{(0.8312--0.8934)}{4.55pt}{4.82pt}{} \\*
\softcline{4-11}
 & \HoloSegSpan{\makecell[c]{Flare22}}{1.86cm}{0.32cm} & \HoloSegSpan{\makecell[c]{right\\[-0.10ex]adrenal\\[-0.10ex]gland}}{2.04cm}{0.32cm} & \HoloSegMetric{HD95} & \HoloSegScore{4.653}{(3.217--6.362)}{4.55pt}{4.82pt}{} & \HoloSegScore{9.848}{(8.252--11.48)}{4.55pt}{4.82pt}{} & \HoloSegScore{1.873}{(1.497--2.245)}{4.55pt}{4.82pt}{} & \HoloSegScore{2.657}{(1.046--4.546)}{4.55pt}{4.82pt}{} & \HoloSegScore{5.358}{(5.015--6.450)}{4.55pt}{4.82pt}{} & \HoloSegScore{1.375}{(0.8850--1.825)}{4.55pt}{4.82pt}{} & \HoloSegScore{1.439}{(0.8488--2.343)}{4.55pt}{4.82pt}{} \\
\cline{3-11}
 &  &  & \HoloSegMetric{Dice} & \HoloSegScore{0.8070}{(0.7741--0.8386)}{4.55pt}{4.82pt}{} & \HoloSegScore{0.3795}{(0.3159--0.4437)}{4.55pt}{4.82pt}{} & \HoloSegScore{0.8379}{(0.8198--0.8530)}{4.55pt}{4.82pt}{} & \HoloSegScore{0.8697}{(0.8427--0.8933)}{4.55pt}{4.82pt}{} & \HoloSegScore{0.8312}{(0.8061--0.8391)}{4.55pt}{4.82pt}{} & \HoloSegScore{0.8899}{(0.8614--0.9124)}{4.55pt}{4.82pt}{} & \HoloSegScore{0.8824}{(0.8639--0.8997)}{4.55pt}{4.82pt}{} \\*
\softcline{4-11}
 &  & \HoloSegSpan{\makecell[c]{left adrenal\\[-0.10ex]gland}}{2.04cm}{0.32cm} & \HoloSegMetric{HD95} & \HoloSegScore{3.593}{(2.985--4.223)}{4.55pt}{4.82pt}{} & \HoloSegScore{10.93}{(8.756--13.26)}{4.55pt}{4.82pt}{} & \HoloSegScore{1.986}{(1.741--2.268)}{4.55pt}{4.82pt}{} & \HoloSegScore{1.737}{(1.210--2.288)}{4.55pt}{4.82pt}{} & \HoloSegScore{3.195}{(2.459--4.858)}{4.55pt}{4.82pt}{} & \HoloSegScore{0.8690}{(0.4833--1.403)}{4.55pt}{4.82pt}{} & \HoloSegScore{1.061}{(0.9029--1.249)}{4.55pt}{4.82pt}{} \\
\cline{3-11}
 &  &  & \HoloSegMetric{Dice} & \HoloSegScore{0.8971}{(0.8781--0.9158)}{4.55pt}{4.82pt}{} & \HoloSegScore{0.5550}{(0.3989--0.6810)}{4.55pt}{4.82pt}{} & \HoloSegScore{0.9145}{(0.9001--0.9289)}{4.55pt}{4.82pt}{} & \HoloSegScore{0.9075}{(0.8820--0.9307)}{4.55pt}{4.82pt}{} & \HoloSegScore{0.8999}{(0.8932--0.9212)}{4.55pt}{4.82pt}{} & \HoloSegScore{0.9241}{(0.8906--0.9546)}{4.55pt}{4.82pt}{} & \HoloSegScore{0.9264}{(0.9067--0.9453)}{4.55pt}{4.82pt}{} \\*
\softcline{4-11}
 &  & \HoloSegSpan{\makecell[c]{gallbladder}}{2.04cm}{0.32cm} & \HoloSegMetric{HD95} & \HoloSegScore{4.139}{(3.308--5.492)}{4.55pt}{4.82pt}{} & \HoloSegScore{40.35}{(14.06--81.01)}{4.55pt}{4.82pt}{} & \HoloSegScore{2.462}{(2.147--2.803)}{4.55pt}{4.82pt}{} & \HoloSegScore{3.951}{(2.295--6.022)}{4.55pt}{4.82pt}{} & \HoloSegScore{3.575}{(3.009--4.955)}{4.55pt}{4.82pt}{} & \HoloSegScore{3.003}{(1.487--4.684)}{4.55pt}{4.82pt}{} & \HoloSegScore{1.999}{(1.489--2.491)}{4.55pt}{4.82pt}{} \\
\cline{3-11}
 &  &  & \HoloSegMetric{Dice} & \HoloSegScore{0.8154}{(0.7851--0.8493)}{4.55pt}{4.82pt}{} & \HoloSegScore{0.6599}{(0.6163--0.7015)}{4.55pt}{4.82pt}{} & \HoloSegScore{0.8747}{(0.8584--0.8922)}{4.55pt}{4.82pt}{} & \HoloSegScore{0.8750}{(0.8587--0.8918)}{4.55pt}{4.82pt}{} & \HoloSegScore{0.8678}{(0.8554--0.8823)}{4.55pt}{4.82pt}{} & \HoloSegScore{0.9101}{(0.8975--0.9245)}{4.55pt}{4.82pt}{} & \HoloSegScore{0.8956}{(0.8779--0.9112)}{4.55pt}{4.82pt}{} \\*
\softcline{4-11}
 &  & \HoloSegSpan{\makecell[c]{esophagus}}{2.04cm}{0.32cm} & \HoloSegMetric{HD95} & \HoloSegScore{8.587}{(6.280--11.48)}{4.55pt}{4.82pt}{} & \HoloSegScore{7.227}{(5.508--9.251)}{4.55pt}{4.82pt}{} & \HoloSegScore{3.604}{(2.553--5.137)}{4.55pt}{4.82pt}{} & \HoloSegScore{4.395}{(2.854--6.410)}{4.55pt}{4.82pt}{} & \HoloSegScore{4.042}{(2.782--6.122)}{4.55pt}{4.82pt}{} & \HoloSegScore{1.980}{(1.608--2.418)}{4.55pt}{4.82pt}{} & \HoloSegScore{2.908}{(2.324--3.628)}{4.55pt}{4.82pt}{} \\
\cline{3-11}
 &  &  & \HoloSegMetric{Dice} & \HoloSegScore{0.9319}{(0.9201--0.9423)}{4.55pt}{4.82pt}{} & \HoloSegScore{0.7885}{(0.7380--0.8325)}{4.55pt}{4.82pt}{} & \HoloSegScore{0.9468}{(0.9360--0.9547)}{4.55pt}{4.82pt}{} & \HoloSegScore{0.9426}{(0.9222--0.9582)}{4.55pt}{4.82pt}{} & \HoloSegScore{0.9448}{(0.9330--0.9638)}{4.55pt}{4.82pt}{} & \HoloSegScore{0.9745}{(0.9695--0.9792)}{4.55pt}{4.82pt}{} & \HoloSegScore{0.9594}{(0.9536--0.9644)}{4.55pt}{4.82pt}{} \\*
\softcline{4-11}
 &  & \HoloSegSpan{\makecell[c]{stomach}}{2.04cm}{0.32cm} & \HoloSegMetric{HD95} & \HoloSegScore{5.138}{(3.852--6.645)}{4.55pt}{4.82pt}{} & \HoloSegScore{8.958}{(7.334--10.78)}{4.55pt}{4.82pt}{} & \HoloSegScore{2.772}{(2.500--3.272)}{4.55pt}{4.82pt}{} & \HoloSegScore{11.32}{(3.590--21.90)}{4.55pt}{4.82pt}{} & \HoloSegScore{4.460}{(2.930--5.059)}{4.55pt}{4.82pt}{} & \HoloSegScore{2.056}{(1.538--2.725)}{4.55pt}{4.82pt}{} & \HoloSegScore{2.498}{(2.037--3.089)}{4.55pt}{4.82pt}{} \\
\cline{3-11}
 &  &  & \HoloSegMetric{Dice} & \HoloSegScore{0.7722}{(0.7503--0.7922)}{4.55pt}{4.82pt}{} & \HoloSegScore{0.5796}{(0.5136--0.6356)}{4.55pt}{4.82pt}{} & \HoloSegScore{0.8608}{(0.8458--0.8768)}{4.55pt}{4.82pt}{} & \HoloSegScore{0.8318}{(0.7925--0.8659)}{4.55pt}{4.82pt}{} & \HoloSegScore{0.8152}{(0.7988--0.8438)}{4.55pt}{4.82pt}{} & \HoloSegScore{0.8767}{(0.8590--0.8904)}{4.55pt}{4.82pt}{} & \HoloSegScore{0.8798}{(0.8554--0.8996)}{4.55pt}{4.82pt}{} \\*
\softcline{4-11}
 &  & \HoloSegSpan{\makecell[c]{duodenum}}{2.04cm}{0.32cm} & \HoloSegMetric{HD95} & \HoloSegScore{18.59}{(14.21--23.43)}{4.55pt}{4.82pt}{} & \HoloSegScore{15.03}{(11.08--19.01)}{4.55pt}{4.82pt}{} & \HoloSegScore{5.419}{(3.973--7.062)}{4.55pt}{4.82pt}{} & \HoloSegScore{10.13}{(6.702--14.07)}{4.55pt}{4.82pt}{} & \HoloSegScore{8.918}{(8.783--10.30)}{4.55pt}{4.82pt}{} & \HoloSegScore{8.105}{(5.321--11.00)}{4.55pt}{4.82pt}{} & \HoloSegScore{7.327}{(3.877--11.48)}{4.55pt}{4.82pt}{} \\
\cline{3-11}
 &  &  & \HoloSegMetric{Dice} & \HoloSegScore{0.9306}{(0.9220--0.9389)}{4.55pt}{4.82pt}{} & \HoloSegScore{0.7600}{(0.5819--0.8691)}{4.55pt}{4.82pt}{} & \HoloSegScore{0.9643}{(0.9601--0.9690)}{4.55pt}{4.82pt}{} & \HoloSegScore{0.9686}{(0.9636--0.9733)}{4.55pt}{4.82pt}{} & \HoloSegScore{0.9599}{(0.9522--0.9658)}{4.55pt}{4.82pt}{} & \HoloSegScore{0.9848}{(0.9791--0.9899)}{4.55pt}{4.82pt}{} & \HoloSegScore{0.9724}{(0.9680--0.9762)}{4.55pt}{4.82pt}{} \\*
\softcline{4-11}
 &  & \HoloSegSpan{\makecell[c]{left kidney}}{2.04cm}{0.32cm} & \HoloSegMetric{HD95} & \HoloSegScore{7.479}{(5.235--10.17)}{4.55pt}{4.82pt}{} & \HoloSegScore{44.69}{(7.154--83.34)}{4.55pt}{4.82pt}{} & \HoloSegScore{3.351}{(2.272--5.016)}{4.55pt}{4.82pt}{} & \HoloSegScore{3.732}{(2.504--5.516)}{4.55pt}{4.82pt}{} & \HoloSegScore{6.401}{(4.397--6.936)}{4.55pt}{4.82pt}{} & \HoloSegScore{2.885}{(1.222--5.654)}{4.55pt}{4.82pt}{} & \HoloSegScore{3.526}{(1.912--6.077)}{4.55pt}{4.82pt}{} \\
\cline{2-11}
 &  &  & \HoloSegMetric{Dice} & \HoloSegScore{0.9691}{(0.9646--0.9726)}{4.55pt}{4.82pt}{} & \HoloSegScore{0.6001}{(0.5393--0.6586)}{4.55pt}{4.82pt}{} & \HoloSegScore{0.6568}{(0.5946--0.7160)}{4.55pt}{4.82pt}{} & \HoloSegScore{0.6922}{(0.6358--0.7502)}{4.55pt}{4.82pt}{} & \HoloSegScore{0.9611}{(0.9511--0.9768)}{4.55pt}{4.82pt}{} & \HoloSegScore{0.9704}{(0.9666--0.9735)}{4.55pt}{4.82pt}{} & \HoloSegScore{0.9691}{(0.9653--0.9725)}{4.55pt}{4.82pt}{} \\*
\softcline{4-11}
 &  & \HoloSegSpan{\makecell[c]{liver}}{2.04cm}{0.32cm} & \HoloSegMetric{HD95} & \HoloSegScore{5.875}{(4.074--8.386)}{4.55pt}{4.82pt}{} & \HoloSegScore{10.30}{(9.352--11.49)}{4.55pt}{4.82pt}{} & \HoloSegScore{4.424}{(3.477--5.855)}{4.55pt}{4.82pt}{} & \HoloSegScore{43.43}{(35.94--51.26)}{4.55pt}{4.82pt}{} & \HoloSegScore{7.335}{(6.506--8.890)}{4.55pt}{4.82pt}{} & \HoloSegScore{4.920}{(4.004--5.988)}{4.55pt}{4.82pt}{} & \HoloSegScore{5.082}{(3.973--6.568)}{4.55pt}{4.82pt}{} \\
\cline{3-11}
 & \HoloSegSpan{\makecell[c]{Flare23}}{1.86cm}{0.32cm} &  & \HoloSegMetric{Dice} & \HoloSegScore{0.9007}{(0.8823--0.9168)}{4.55pt}{4.82pt}{} & \HoloSegScore{0.4992}{(0.4439--0.5478)}{4.55pt}{4.82pt}{} & \HoloSegScore{0.6187}{(0.5595--0.6822)}{4.55pt}{4.82pt}{} & \HoloSegScore{0.6264}{(0.5668--0.6880)}{4.55pt}{4.82pt}{} & \HoloSegScore{0.9141}{(0.8885--0.9270)}{4.55pt}{4.82pt}{} & \HoloSegScore{0.9247}{(0.9112--0.9369)}{4.55pt}{4.82pt}{} & \HoloSegScore{0.9402}{(0.9291--0.9496)}{4.55pt}{4.82pt}{} \\*
\softcline{4-11}
 &  & \HoloSegSpan{\makecell[c]{right kidney}}{2.04cm}{0.32cm} & \HoloSegMetric{HD95} & \HoloSegScore{7.150}{(5.863--9.209)}{4.55pt}{4.82pt}{} & \HoloSegScore{72.96}{(62.02--83.64)}{4.55pt}{4.82pt}{} & \HoloSegScore{4.794}{(4.075--5.582)}{4.55pt}{4.82pt}{} & \HoloSegScore{37.92}{(30.98--45.05)}{4.55pt}{4.82pt}{} & \HoloSegScore{6.318}{(5.618--8.355)}{4.55pt}{4.82pt}{} & \HoloSegScore{5.826}{(4.816--7.288)}{4.55pt}{4.82pt}{} & \HoloSegScore{5.035}{(4.036--6.458)}{4.55pt}{4.82pt}{} \\
\hline
\pagebreak[4]
 &  &  & \HoloSegMetric{Dice} & \HoloSegScore{0.9660}{(0.9632--0.9682)}{4.55pt}{4.82pt}{} & \HoloSegScore{0.5599}{(0.5020--0.6130)}{4.55pt}{4.82pt}{} & \HoloSegScore{0.6536}{(0.5897--0.7226)}{4.55pt}{4.82pt}{} & \HoloSegScore{0.6585}{(0.5920--0.7232)}{4.55pt}{4.82pt}{} & \HoloSegScore{0.9358}{(0.9349--0.9430)}{4.55pt}{4.82pt}{} & \HoloSegScore{0.9697}{(0.9632--0.9742)}{4.55pt}{4.82pt}{} & \HoloSegScore{0.9710}{(0.9644--0.9754)}{4.55pt}{4.82pt}{} \\*
\softcline{4-11}
 &  & \HoloSegSpan{\makecell[c]{spleen}}{2.04cm}{0.32cm} & \HoloSegMetric{HD95} & \HoloSegScore{1.884}{(1.690--2.127)}{4.55pt}{4.82pt}{} & \HoloSegScore{8.940}{(7.697--10.48)}{4.55pt}{4.82pt}{} & \HoloSegScore{2.126}{(1.719--2.682)}{4.55pt}{4.82pt}{} & \HoloSegScore{64.13}{(51.45--77.15)}{4.55pt}{4.82pt}{} & \HoloSegScore{3.541}{(2.754--5.397)}{4.55pt}{4.82pt}{} & \HoloSegScore{1.758}{(1.289--2.371)}{4.55pt}{4.82pt}{} & \HoloSegScore{1.960}{(1.378--2.712)}{4.55pt}{4.82pt}{} \\
\cline{3-11}
 &  &  & \HoloSegMetric{Dice} & \HoloSegScore{0.8412}{(0.8253--0.8541)}{4.55pt}{4.82pt}{} & \HoloSegScore{0.3905}{(0.3491--0.4333)}{4.55pt}{4.82pt}{} & \HoloSegScore{0.5791}{(0.5182--0.6365)}{4.55pt}{4.82pt}{} & \HoloSegScore{0.5590}{(0.5066--0.6136)}{4.55pt}{4.82pt}{} & \HoloSegScore{0.7998}{(0.7802--0.8217)}{4.55pt}{4.82pt}{} & \HoloSegScore{0.8350}{(0.8148--0.8536)}{4.55pt}{4.82pt}{} & \HoloSegScore{0.8413}{(0.8233--0.8581)}{4.55pt}{4.82pt}{} \\*
\softcline{4-11}
 &  & \HoloSegSpan{\makecell[c]{pancreas}}{2.04cm}{0.32cm} & \HoloSegMetric{HD95} & \HoloSegScore{7.216}{(5.620--8.998)}{4.55pt}{4.82pt}{} & \HoloSegScore{14.97}{(13.02--17.07)}{4.55pt}{4.82pt}{} & \HoloSegScore{5.589}{(4.236--7.698)}{4.55pt}{4.82pt}{} & \HoloSegScore{48.91}{(40.23--58.21)}{4.55pt}{4.82pt}{} & \HoloSegScore{9.322}{(6.771--13.14)}{4.55pt}{4.82pt}{} & \HoloSegScore{6.854}{(5.338--9.014)}{4.55pt}{4.82pt}{} & \HoloSegScore{7.735}{(5.902--9.948)}{4.55pt}{4.82pt}{} \\
\cline{3-11}
 & \HoloSegSpan{\makecell[c]{Flare23}}{1.86cm}{0.32cm} &  & \HoloSegMetric{Dice} & \HoloSegScore{0.9177}{(0.9064--0.9263)}{4.55pt}{4.82pt}{} & \HoloSegScore{0.5120}{(0.4585--0.5625)}{4.55pt}{4.82pt}{} & \HoloSegScore{0.6223}{(0.5664--0.6812)}{4.55pt}{4.82pt}{} & \HoloSegScore{0.6337}{(0.5720--0.7006)}{4.55pt}{4.82pt}{} & \HoloSegScore{0.9320}{(0.9183--0.9415)}{4.55pt}{4.82pt}{} & \HoloSegScore{0.9397}{(0.9300--0.9481)}{4.55pt}{4.82pt}{} & \HoloSegScore{0.9429}{(0.9377--0.9481)}{4.55pt}{4.82pt}{} \\*
\softcline{4-11}
 &  & \HoloSegSpan{\makecell[c]{left kidney}}{2.04cm}{0.32cm} & \HoloSegMetric{HD95} & \HoloSegScore{6.414}{(5.542--7.527)}{4.55pt}{4.82pt}{} & \HoloSegScore{69.17}{(58.26--80.57)}{4.55pt}{4.82pt}{} & \HoloSegScore{6.087}{(4.263--8.764)}{4.55pt}{4.82pt}{} & \HoloSegScore{59.48}{(47.84--70.57)}{4.55pt}{4.82pt}{} & \HoloSegScore{5.511}{(5.217--5.902)}{4.55pt}{4.82pt}{} & \HoloSegScore{4.932}{(3.995--6.139)}{4.55pt}{4.82pt}{} & \HoloSegScore{4.902}{(4.095--5.903)}{4.55pt}{4.82pt}{} \\
\cline{3-11}
 &  &  & \HoloSegMetric{Dice} &  & \HoloSegScore{0.2622}{(0.2207--0.3041)}{4.55pt}{4.82pt}{} & \HoloSegScore{0.003614}{(0.0000--0.009096)}{4.20pt}{4.48pt}{} & \HoloSegScore{0.6045}{(0.5621--0.6437)}{4.55pt}{4.82pt}{} & \HoloSegScore{0.5997}{(0.5651--0.6359)}{4.55pt}{4.82pt}{} & \HoloSegScore{0.5915}{(0.5384--0.6407)}{4.55pt}{4.82pt}{} & \HoloSegScore{0.6312}{(0.5844--0.6753)}{4.55pt}{4.82pt}{} \\*
\softcline{4-4}\softcline{6-11}
 &  & \HoloSegSpan{\makecell[c]{tumor}}{2.04cm}{0.32cm} & \HoloSegMetric{HD95} & \raisebox{0.32cm}[0pt][0pt]{\HoloSegUnsupported} & \HoloSegScore{89.03}{(79.72--98.30)}{4.55pt}{4.82pt}{} & \HoloSegScore{182.6}{(164.4--204.9)}{4.55pt}{4.82pt}{} & \HoloSegScore{83.64}{(72.94--95.86)}{4.55pt}{4.82pt}{} & \HoloSegScore{42.56}{(31.95--50.35)}{4.55pt}{4.82pt}{} & \HoloSegScore{48.99}{(37.26--61.30)}{4.55pt}{4.82pt}{} & \HoloSegScore{48.20}{(38.37--59.08)}{4.55pt}{4.82pt}{} \\
\cline{2-11}
 &  &  & \HoloSegMetric{Dice} & \HoloSegScore{0.9316}{(0.9010--0.9556)}{4.55pt}{4.82pt}{} & \HoloSegScore{0.7965}{(0.6988--0.8623)}{4.55pt}{4.82pt}{} & \HoloSegScore{0.9641}{(0.9589--0.9690)}{4.55pt}{4.82pt}{} & \HoloSegScore{0.9605}{(0.9485--0.9701)}{4.55pt}{4.82pt}{} & \HoloSegScore{0.9581}{(0.9395--0.9640)}{4.55pt}{4.82pt}{} & \HoloSegScore{0.9749}{(0.9666--0.9825)}{4.55pt}{4.82pt}{} & \HoloSegScore{0.9672}{(0.9620--0.9721)}{4.55pt}{4.82pt}{} \\*
\softcline{4-11}
 &  & \HoloSegSpan{\makecell[c]{liver}}{2.04cm}{0.32cm} & \HoloSegMetric{HD95} & \HoloSegScore{27.59}{(9.466--50.69)}{4.55pt}{4.82pt}{} & \HoloSegScore{30.93}{(12.89--56.54)}{4.55pt}{4.82pt}{} & \HoloSegScore{3.290}{(2.778--3.865)}{4.55pt}{4.82pt}{} & \HoloSegScore{23.18}{(8.058--45.09)}{4.55pt}{4.82pt}{} & \HoloSegScore{9.563}{(6.468--14.16)}{4.55pt}{4.82pt}{} & \HoloSegScore{6.221}{(3.516--9.520)}{4.55pt}{4.82pt}{} & \HoloSegScore{4.011}{(2.988--5.222)}{4.55pt}{4.82pt}{} \\
\cline{3-11}
 &  &  & \HoloSegMetric{Dice} & \HoloSegScore{0.8502}{(0.7703--0.9115)}{4.55pt}{4.82pt}{} & \HoloSegScore{0.4785}{(0.3376--0.6073)}{4.55pt}{4.82pt}{} & \HoloSegScore{0.9024}{(0.8682--0.9321)}{4.55pt}{4.82pt}{} & \HoloSegScore{0.8595}{(0.7708--0.9223)}{4.55pt}{4.82pt}{} & \HoloSegScore{0.8609}{(0.8363--0.8913)}{4.55pt}{4.82pt}{} & \HoloSegScore{0.8749}{(0.7966--0.9352)}{4.55pt}{4.82pt}{} & \HoloSegScore{0.8841}{(0.8386--0.9257)}{4.55pt}{4.82pt}{} \\*
\softcline{4-11}
 &  & \HoloSegSpan{\makecell[c]{urinary\\[-0.10ex]bladder}}{2.04cm}{0.32cm} & \HoloSegMetric{HD95} & \HoloSegScore{6.424}{(0.8233--14.46)}{4.55pt}{4.82pt}{} & \HoloSegScore{82.24}{(23.46--148.7)}{4.55pt}{4.82pt}{} & \HoloSegScore{4.880}{(3.572--6.444)}{4.55pt}{4.82pt}{} & \HoloSegScore{13.63}{(6.651--21.27)}{4.55pt}{4.82pt}{} & \HoloSegScore{8.232}{(7.286--10.79)}{4.55pt}{4.82pt}{} & \HoloSegScore{43.63}{(7.129--91.16)}{4.55pt}{4.82pt}{} & \HoloSegScore{9.856}{(5.227--17.64)}{4.55pt}{4.82pt}{} \\
\cline{3-11}
 &  &  & \HoloSegMetric{Dice} & \HoloSegScore{0.9133}{(0.8774--0.9397)}{4.55pt}{4.82pt}{} & \HoloSegScore{0.7051}{(0.5866--0.8075)}{4.55pt}{4.82pt}{} & \HoloSegScore{0.9522}{(0.9335--0.9644)}{4.55pt}{4.82pt}{} & \HoloSegScore{0.9545}{(0.9289--0.9691)}{4.55pt}{4.82pt}{} & \HoloSegScore{0.9456}{(0.9212--0.9644)}{4.55pt}{4.82pt}{} & \HoloSegScore{0.9773}{(0.9537--0.9906)}{4.55pt}{4.82pt}{} & \HoloSegScore{0.9643}{(0.9394--0.9788)}{4.55pt}{4.82pt}{} \\*
\softcline{4-11}
 & \HoloSegSpan{\makecell[c]{CT-ORG}}{1.86cm}{0.32cm} & \HoloSegSpan{\makecell[c]{lung}}{2.04cm}{0.32cm} & \HoloSegMetric{HD95} & \HoloSegScore{31.53}{(13.14--56.49)}{4.55pt}{4.82pt}{} & \HoloSegScore{41.02}{(19.10--65.02)}{4.55pt}{4.82pt}{} & \HoloSegScore{16.85}{(9.673--28.95)}{4.55pt}{4.82pt}{} & \HoloSegScore{25.57}{(9.520--48.71)}{4.55pt}{4.82pt}{} & \HoloSegScore{17.32}{(9.853--29.56)}{4.55pt}{4.82pt}{} & \HoloSegScore{22.12}{(6.698--43.45)}{4.55pt}{4.82pt}{} & \HoloSegScore{20.29}{(8.203--36.06)}{4.55pt}{4.82pt}{} \\
\cline{3-11}
 &  &  & \HoloSegMetric{Dice} & \HoloSegScore{0.9106}{(0.8971--0.9236)}{4.55pt}{4.82pt}{} & \HoloSegScore{0.6838}{(0.5773--0.7704)}{4.55pt}{4.82pt}{} & \HoloSegScore{0.9318}{(0.9226--0.9415)}{4.55pt}{4.82pt}{} & \HoloSegScore{0.9203}{(0.9038--0.9369)}{4.55pt}{4.82pt}{} & \HoloSegScore{0.9035}{(0.8704--0.9303)}{4.55pt}{4.82pt}{} & \HoloSegScore{0.9344}{(0.9179--0.9487)}{4.55pt}{4.82pt}{} & \HoloSegScore{0.9265}{(0.9118--0.9392)}{4.55pt}{4.82pt}{} \\*
\softcline{4-11}
 &  & \HoloSegSpan{\makecell[c]{kidney}}{2.04cm}{0.32cm} & \HoloSegMetric{HD95} & \HoloSegScore{8.231}{(6.746--9.961)}{4.55pt}{4.82pt}{} & \HoloSegScore{35.71}{(12.53--65.52)}{4.55pt}{4.82pt}{} & \HoloSegScore{4.578}{(3.622--5.602)}{4.55pt}{4.82pt}{} & \HoloSegScore{6.229}{(5.015--7.709)}{4.55pt}{4.82pt}{} & \HoloSegScore{5.628}{(5.247--6.297)}{4.55pt}{4.82pt}{} & \HoloSegScore{5.371}{(4.331--6.530)}{4.55pt}{4.82pt}{} & \HoloSegScore{6.195}{(5.112--7.321)}{4.55pt}{4.82pt}{} \\
\cline{3-11}
 &  &  & \HoloSegMetric{Dice} &  & \HoloSegScore{0.6677}{(0.5772--0.7437)}{4.55pt}{4.82pt}{} & \HoloSegScore{0.7172}{(0.5945--0.8202)}{4.55pt}{4.82pt}{} & \HoloSegScore{0.8050}{(0.7554--0.8400)}{4.55pt}{4.82pt}{} & \HoloSegScore{0.7921}{(0.7578--0.8000)}{4.55pt}{4.82pt}{} & \HoloSegScore{0.8355}{(0.7877--0.8683)}{4.55pt}{4.82pt}{} & \HoloSegScore{0.8362}{(0.7889--0.8682)}{4.55pt}{4.82pt}{} \\*
\softcline{4-4}\softcline{6-11}
 &  & \HoloSegSpan{\makecell[c]{bone}}{2.04cm}{0.32cm} & \HoloSegMetric{HD95} & \raisebox{0.32cm}[0pt][0pt]{\HoloSegUnsupported} & \HoloSegScore{51.95}{(32.43--75.51)}{4.55pt}{4.82pt}{} & \HoloSegScore{59.52}{(34.62--87.62)}{4.55pt}{4.82pt}{} & \HoloSegScore{47.32}{(33.95--63.23)}{4.55pt}{4.82pt}{} & \HoloSegScore{49.05}{(35.84--64.77)}{4.55pt}{4.82pt}{} & \HoloSegScore{50.54}{(34.01--66.62)}{4.55pt}{4.82pt}{} & \HoloSegScore{45.97}{(30.15--62.23)}{4.55pt}{4.82pt}{} \\
\cline{2-11}
 &  &  & \HoloSegMetric{Dice} & \HoloSegScore{0.1598}{(0.1188--0.2042)}{4.55pt}{4.82pt}{} & \HoloSegScore{0.01719}{(0.004692--0.03352)}{3.85pt}{4.12pt}{} & \HoloSegScore{0.3663}{(0.3045--0.4234)}{4.55pt}{4.82pt}{} & \HoloSegScore{0.5179}{(0.4611--0.5771)}{4.55pt}{4.82pt}{} & \HoloSegScore{0.5425}{(0.5271--0.5876)}{4.55pt}{4.82pt}{} & \HoloSegScore{0.6134}{(0.5650--0.6601)}{4.55pt}{4.82pt}{} & \HoloSegScore{0.6614}{(0.6189--0.7052)}{4.55pt}{4.82pt}{} \\*
\softcline{4-11}
\HoloSegSpan{\makecell[c]{\textbf{Internal}}}{1.20cm}{0.32cm} & \HoloSegSpan{\makecell[c]{LIDC-IDRI}}{1.86cm}{0.32cm} & \HoloSegSpan{\makecell[c]{pulmonary\\[-0.10ex]nodule}}{2.04cm}{0.32cm} & \HoloSegMetric{HD95} & \HoloSegScore{184.2}{(175.7--193.1)}{4.55pt}{4.82pt}{} & \HoloSegScore{168.1}{(158.5--178.5)}{4.55pt}{4.82pt}{} & \HoloSegScore{98.44}{(84.44--113.4)}{4.55pt}{4.82pt}{} & \HoloSegScore{93.66}{(79.00--108.9)}{4.55pt}{4.82pt}{} & \HoloSegScore{44.70}{(27.31--52.22)}{4.55pt}{4.82pt}{} & \HoloSegScore{73.98}{(60.32--88.28)}{4.55pt}{4.82pt}{} & \HoloSegScore{52.53}{(40.93--64.77)}{4.55pt}{4.82pt}{} \\
\cline{2-11}
 &  &  & \HoloSegMetric{Dice} & \HoloSegScore{0.9721}{(0.9689--0.9761)}{4.55pt}{4.82pt}{} & \HoloSegScore{0.9190}{(0.8940--0.9389)}{4.55pt}{4.82pt}{} & \HoloSegScore{0.9726}{(0.9682--0.9755)}{4.55pt}{4.82pt}{} & \HoloSegScore{0.9750}{(0.9730--0.9766)}{4.55pt}{4.82pt}{} & \HoloSegScore{0.9693}{(0.9470--0.9726)}{4.55pt}{4.82pt}{} & \HoloSegScore{0.9747}{(0.9714--0.9775)}{4.55pt}{4.82pt}{} & \HoloSegScore{0.9750}{(0.9715--0.9777)}{4.55pt}{4.82pt}{} \\*
\softcline{4-11}
 & \HoloSegSpan{\makecell[c]{SLIVER07}}{1.86cm}{0.32cm} & \HoloSegSpan{\makecell[c]{liver}}{2.04cm}{0.32cm} & \HoloSegMetric{HD95} & \HoloSegScore{4.239}{(2.740--6.107)}{4.55pt}{4.82pt}{} & \HoloSegScore{8.254}{(5.282--13.34)}{4.55pt}{4.82pt}{} & \HoloSegScore{3.323}{(2.427--4.366)}{4.55pt}{4.82pt}{} & \HoloSegScore{4.555}{(2.713--6.397)}{4.55pt}{4.82pt}{} & \HoloSegScore{3.822}{(2.051--4.774)}{4.55pt}{4.82pt}{} & \HoloSegScore{4.581}{(3.647--5.514)}{4.55pt}{4.82pt}{} & \HoloSegScore{4.650}{(2.500--7.717)}{4.55pt}{4.82pt}{} \\
\cline{2-11}
 &  &  & \HoloSegMetric{Dice} & \HoloSegScore{0.9715}{(0.9601--0.9775)}{4.55pt}{4.82pt}{} & \HoloSegScore{0.8927}{(0.8689--0.9134)}{4.55pt}{4.82pt}{} & \HoloSegScore{0.9771}{(0.9656--0.9831)}{4.55pt}{4.82pt}{} & \HoloSegScore{0.9618}{(0.9472--0.9699)}{4.55pt}{4.82pt}{} & \HoloSegScore{0.9599}{(0.9526--0.9627)}{4.55pt}{4.82pt}{} & \HoloSegScore{0.9761}{(0.9647--0.9821)}{4.55pt}{4.82pt}{} & \HoloSegScore{0.9776}{(0.9662--0.9836)}{4.55pt}{4.82pt}{} \\*
\softcline{4-11}
 &  & \HoloSegSpan{\makecell[c]{left lung}}{2.04cm}{0.32cm} & \HoloSegMetric{HD95} & \HoloSegScore{9.887}{(8.527--11.54)}{4.55pt}{4.82pt}{} & \HoloSegScore{12.94}{(9.781--17.60)}{4.55pt}{4.82pt}{} & \HoloSegScore{3.116}{(1.802--5.193)}{4.55pt}{4.82pt}{} & \HoloSegScore{16.13}{(13.92--18.31)}{4.55pt}{4.82pt}{} & \HoloSegScore{3.371}{(2.861--4.843)}{4.55pt}{4.82pt}{} & \HoloSegScore{3.297}{(2.306--5.138)}{4.55pt}{4.82pt}{} & \HoloSegScore{3.502}{(2.526--5.543)}{4.55pt}{4.82pt}{} \\
\cline{3-11}
 &  &  & \HoloSegMetric{Dice} & \HoloSegScore{0.9697}{(0.9585--0.9760)}{4.55pt}{4.82pt}{} & \HoloSegScore{0.8924}{(0.8692--0.9112)}{4.55pt}{4.82pt}{} & \HoloSegScore{0.9786}{(0.9671--0.9844)}{4.55pt}{4.82pt}{} & \HoloSegScore{0.9695}{(0.9568--0.9768)}{4.55pt}{4.82pt}{} & \HoloSegScore{0.9709}{(0.9574--0.9718)}{4.55pt}{4.82pt}{} & \HoloSegScore{0.9767}{(0.9654--0.9828)}{4.55pt}{4.82pt}{} & \HoloSegScore{0.9790}{(0.9676--0.9850)}{4.55pt}{4.82pt}{} \\*
\softcline{4-11}
 & \HoloSegSpan{\makecell[c]{LUNA16}}{1.86cm}{0.32cm} & \HoloSegSpan{\makecell[c]{right lung}}{2.04cm}{0.32cm} & \HoloSegMetric{HD95} & \HoloSegScore{19.75}{(18.52--21.43)}{4.55pt}{4.82pt}{} & \HoloSegScore{20.69}{(16.25--25.75)}{4.55pt}{4.82pt}{} & \HoloSegScore{2.747}{(1.796--4.356)}{4.55pt}{4.82pt}{} & \HoloSegScore{16.06}{(13.85--18.56)}{4.55pt}{4.82pt}{} & \HoloSegScore{7.386}{(7.111--7.888)}{4.55pt}{4.82pt}{} & \HoloSegScore{10.49}{(8.829--12.43)}{4.55pt}{4.82pt}{} & \HoloSegScore{4.958}{(3.684--6.637)}{4.55pt}{4.82pt}{} \\
\cline{3-11}
 &  &  & \HoloSegMetric{Dice} & \HoloSegScore{0.8383}{(0.8327--0.8432)}{4.55pt}{4.82pt}{} & \HoloSegScore{0.6779}{(0.6590--0.6912)}{4.55pt}{4.82pt}{} & \HoloSegScore{0.8947}{(0.8905--0.8984)}{4.55pt}{4.82pt}{} & \HoloSegScore{0.8827}{(0.8781--0.8871)}{4.55pt}{4.82pt}{} & \HoloSegScore{0.8760}{(0.8616--0.8781)}{4.55pt}{4.82pt}{} & \HoloSegScore{0.8917}{(0.8872--0.8957)}{4.55pt}{4.82pt}{} & \HoloSegScore{0.8867}{(0.8819--0.8908)}{4.55pt}{4.82pt}{} \\*
\softcline{4-11}
 &  & \HoloSegSpan{\makecell[c]{trachea}}{2.04cm}{0.32cm} & \HoloSegMetric{HD95} & \HoloSegScore{26.20}{(24.61--27.70)}{4.55pt}{4.82pt}{} & \HoloSegScore{14.83}{(12.97--17.35)}{4.55pt}{4.82pt}{} & \HoloSegScore{4.225}{(3.455--5.332)}{4.55pt}{4.82pt}{} & \HoloSegScore{16.52}{(15.19--18.00)}{4.55pt}{4.82pt}{} & \HoloSegScore{4.549}{(1.616--6.051)}{4.55pt}{4.82pt}{} & \HoloSegScore{7.353}{(6.351--8.514)}{4.55pt}{4.82pt}{} & \HoloSegScore{7.772}{(6.780--8.957)}{4.55pt}{4.82pt}{} \\
\cline{2-11}
 &  &  & \HoloSegMetric{Dice} & \HoloSegScore{0.4581}{(0.0000--0.9162)}{4.55pt}{4.82pt}{} & \HoloSegScore{0.9024}{(0.8516--0.9364)}{4.55pt}{4.82pt}{} & \HoloSegScore{0.8499}{(0.7594--0.9349)}{4.55pt}{4.82pt}{} & \HoloSegScore{0.8199}{(0.7280--0.9348)}{4.55pt}{4.82pt}{} & \HoloSegScore{0.9601}{(0.9232--0.9764)}{4.55pt}{4.82pt}{} & \HoloSegScore{0.9515}{(0.9115--0.9763)}{4.55pt}{4.82pt}{} & \HoloSegScore{0.9643}{(0.9404--0.9802)}{4.55pt}{4.82pt}{} \\*
\softcline{4-11}
 &  & \HoloSegSpan{\makecell[c]{left lung}}{2.04cm}{0.32cm} & \HoloSegMetric{HD95} & \HoloSegScore{13.09}{(11.64--14.54)}{4.55pt}{4.82pt}{} & \HoloSegScore{10.91}{(8.718--12.87)}{4.55pt}{4.82pt}{} & \HoloSegScore{17.46}{(7.221--27.70)}{4.55pt}{4.82pt}{} & \HoloSegScore{49.84}{(13.84--85.84)}{4.55pt}{4.82pt}{} & \HoloSegScore{6.010}{(3.455--9.142)}{4.55pt}{4.82pt}{} & \HoloSegScore{7.263}{(4.123--10.54)}{4.55pt}{4.82pt}{} & \HoloSegScore{5.421}{(3.152--8.301)}{4.55pt}{4.82pt}{} \\
\cline{3-11}
 &  &  & \HoloSegMetric{Dice} & \HoloSegScore{0.4656}{(0.0000--0.9312)}{4.55pt}{4.82pt}{} & \HoloSegScore{0.8864}{(0.8363--0.9365)}{4.55pt}{4.82pt}{} & \HoloSegScore{0.8934}{(0.8336--0.9552)}{4.55pt}{4.82pt}{} & \HoloSegScore{0.7656}{(0.5692--0.9375)}{4.55pt}{4.82pt}{} & \HoloSegScore{0.9322}{(0.8986--0.9406)}{4.55pt}{4.82pt}{} & \HoloSegScore{0.9588}{(0.9403--0.9773)}{4.55pt}{4.82pt}{} & \HoloSegScore{0.9614}{(0.9409--0.9812)}{4.55pt}{4.82pt}{} \\*
\softcline{4-11}
 & \HoloSegSpan{\makecell[c]{COVID-19}}{1.86cm}{0.32cm} & \HoloSegSpan{\makecell[c]{right lung}}{2.04cm}{0.32cm} & \HoloSegMetric{HD95} & \HoloSegScore{197.8}{(13.38--382.2)}{4.55pt}{4.82pt}{} & \HoloSegScore{16.60}{(7.227--29.82)}{4.55pt}{4.82pt}{} & \HoloSegScore{45.13}{(3.688--86.57)}{4.55pt}{4.82pt}{} & \HoloSegScore{54.55}{(12.80--96.30)}{4.55pt}{4.82pt}{} & \HoloSegScore{5.748}{(4.957--6.569)}{4.55pt}{4.82pt}{} & \HoloSegScore{7.403}{(3.519--13.74)}{4.55pt}{4.82pt}{} & \HoloSegScore{5.415}{(2.494--8.288)}{4.55pt}{4.82pt}{} \\
\cline{3-11}
 &  &  & \HoloSegMetric{Dice} &  & \HoloSegScore{0.2189}{(0.02432--0.4707)}{4.20pt}{4.48pt}{} & \HoloSegScore{0.4256}{(0.2012--0.6500)}{4.55pt}{4.82pt}{} & \HoloSegScore{0.6341}{(0.4630--0.8052)}{4.55pt}{4.82pt}{} & \HoloSegScore{0.7247}{(0.6373--0.7767)}{4.55pt}{4.82pt}{} & \HoloSegScore{0.5948}{(0.4876--0.6919)}{4.55pt}{4.82pt}{} & \HoloSegScore{0.7218}{(0.6176--0.7959)}{4.55pt}{4.82pt}{} \\*
\softcline{4-4}\softcline{6-11}
 &  & \HoloSegSpan{\makecell[c]{covid-19\\[-0.10ex]infection}}{2.04cm}{0.32cm} & \HoloSegMetric{HD95} & \raisebox{0.32cm}[0pt][0pt]{\HoloSegUnsupported} & \HoloSegScore{103.3}{(39.29--167.4)}{4.55pt}{4.82pt}{} & \HoloSegScore{82.85}{(25.23--164.6)}{4.55pt}{4.82pt}{} & \HoloSegScore{97.60}{(38.15--157.1)}{4.55pt}{4.82pt}{} & \HoloSegScore{18.73}{(15.90--24.00)}{4.55pt}{4.82pt}{} & \HoloSegScore{22.19}{(14.24--30.14)}{4.55pt}{4.82pt}{} & \HoloSegScore{18.95}{(9.096--29.27)}{4.55pt}{4.82pt}{} \\
\cline{2-11}
 &  &  & \HoloSegMetric{Dice} & \HoloSegScore{0.9256}{(0.9225--0.9283)}{4.55pt}{4.82pt}{} & \HoloSegScore{0.5029}{(0.3841--0.6059)}{4.55pt}{4.82pt}{} & \HoloSegScore{0.9384}{(0.9360--0.9405)}{4.55pt}{4.82pt}{} & \HoloSegScore{0.9586}{(0.9472--0.9655)}{4.55pt}{4.82pt}{} & \HoloSegScore{0.9360}{(0.9310--0.9441)}{4.55pt}{4.82pt}{} & \HoloSegScore{0.9370}{(0.9271--0.9460)}{4.55pt}{4.82pt}{} & \HoloSegScore{0.9511}{(0.9465--0.9548)}{4.55pt}{4.82pt}{} \\*
\softcline{4-11}
 &  & \HoloSegSpan{\makecell[c]{sacrum}}{2.04cm}{0.32cm} & \HoloSegMetric{HD95} & \HoloSegScore{2.561}{(2.381--2.770)}{4.55pt}{4.82pt}{} & \HoloSegScore{49.60}{(27.72--74.25)}{4.55pt}{4.82pt}{} & \HoloSegScore{1.298}{(1.227--1.376)}{4.55pt}{4.82pt}{} & \HoloSegScore{1.395}{(1.069--1.837)}{4.55pt}{4.82pt}{} & \HoloSegScore{3.424}{(2.945--3.439)}{4.55pt}{4.82pt}{} & \HoloSegScore{2.729}{(2.028--3.490)}{4.55pt}{4.82pt}{} & \HoloSegScore{1.565}{(1.215--2.023)}{4.55pt}{4.82pt}{} \\
\cline{3-11}
 & \HoloSegSpan{\makecell[c]{CTPelvic1K-\\[-0.10ex]CLINIC}}{1.86cm}{0.32cm} &  & \HoloSegMetric{Dice} & \HoloSegScore{0.9402}{(0.9369--0.9428)}{4.55pt}{4.82pt}{} & \HoloSegScore{0.5004}{(0.3707--0.6192)}{4.55pt}{4.82pt}{} & \HoloSegScore{0.9565}{(0.9543--0.9586)}{4.55pt}{4.82pt}{} & \HoloSegScore{0.9782}{(0.9745--0.9816)}{4.55pt}{4.82pt}{} & \HoloSegScore{0.9418}{(0.9363--0.9463)}{4.55pt}{4.82pt}{} & \HoloSegScore{0.9747}{(0.9700--0.9791)}{4.55pt}{4.82pt}{} & \HoloSegScore{0.9701}{(0.9663--0.9735)}{4.55pt}{4.82pt}{} \\*
\softcline{4-11}
 &  & \HoloSegSpan{\makecell[c]{left hip}}{2.04cm}{0.32cm} & \HoloSegMetric{HD95} & \HoloSegScore{2.218}{(2.118--2.336)}{4.55pt}{4.82pt}{} & \HoloSegScore{73.94}{(46.72--104.6)}{4.55pt}{4.82pt}{} & \HoloSegScore{1.060}{(0.9921--1.140)}{4.55pt}{4.82pt}{} & \HoloSegScore{2.297}{(0.8213--5.165)}{4.55pt}{4.82pt}{} & \HoloSegScore{2.155}{(1.959--3.059)}{4.55pt}{4.82pt}{} & \HoloSegScore{19.88}{(9.540--31.90)}{4.55pt}{4.82pt}{} & \HoloSegScore{1.465}{(0.9573--2.127)}{4.55pt}{4.82pt}{} \\
\hline
\pagebreak[4]
 &  &  & \HoloSegMetric{Dice} & \HoloSegScore{0.9375}{(0.9311--0.9418)}{4.55pt}{4.82pt}{} & \HoloSegScore{0.5015}{(0.3707--0.6242)}{4.55pt}{4.82pt}{} & \HoloSegScore{0.9542}{(0.9487--0.9578)}{4.55pt}{4.82pt}{} & \HoloSegScore{0.9736}{(0.9660--0.9798)}{4.55pt}{4.82pt}{} & \HoloSegScore{0.9351}{(0.9342--0.9385)}{4.55pt}{4.82pt}{} & \HoloSegScore{0.9768}{(0.9687--0.9829)}{4.55pt}{4.82pt}{} & \HoloSegScore{0.9659}{(0.9576--0.9722)}{4.55pt}{4.82pt}{} \\*
\softcline{4-11}
 &  & \HoloSegSpan{\makecell[c]{right hip}}{2.04cm}{0.32cm} & \HoloSegMetric{HD95} & \HoloSegScore{2.378}{(2.152--2.743)}{4.55pt}{4.82pt}{} & \HoloSegScore{83.44}{(59.90--107.8)}{4.55pt}{4.82pt}{} & \HoloSegScore{1.249}{(1.118--1.468)}{4.55pt}{4.82pt}{} & \HoloSegScore{2.782}{(0.8894--6.253)}{4.55pt}{4.82pt}{} & \HoloSegScore{1.810}{(1.422--3.800)}{4.55pt}{4.82pt}{} & \HoloSegScore{1.184}{(0.5340--1.983)}{4.55pt}{4.82pt}{} & \HoloSegScore{1.642}{(0.9241--2.449)}{4.55pt}{4.82pt}{} \\
\cline{3-11}
 & \HoloSegSpan{\makecell[c]{CTPelvic1K-\\[-0.10ex]CLINIC}}{1.86cm}{0.32cm} &  & \HoloSegMetric{Dice} & \HoloSegScore{0.9270}{(0.9242--0.9297)}{4.55pt}{4.82pt}{} & \HoloSegScore{0.4387}{(0.3573--0.5134)}{4.55pt}{4.82pt}{} & \HoloSegScore{0.9345}{(0.9307--0.9379)}{4.55pt}{4.82pt}{} & \HoloSegScore{0.9567}{(0.9370--0.9698)}{4.55pt}{4.82pt}{} & \HoloSegScore{0.9307}{(0.9277--0.9321)}{4.55pt}{4.82pt}{} & \HoloSegScore{0.9685}{(0.9650--0.9715)}{4.55pt}{4.82pt}{} & \HoloSegScore{0.9586}{(0.9557--0.9612)}{4.55pt}{4.82pt}{} \\*
\softcline{4-11}
 &  & \HoloSegSpan{\makecell[c]{lumbar\\[-0.10ex]vertebrae}}{2.04cm}{0.32cm} & \HoloSegMetric{HD95} & \HoloSegScore{2.241}{(2.172--2.317)}{4.55pt}{4.82pt}{} & \HoloSegScore{60.96}{(32.64--91.73)}{4.55pt}{4.82pt}{} & \HoloSegScore{1.238}{(1.172--1.317)}{4.55pt}{4.82pt}{} & \HoloSegScore{3.053}{(0.8704--6.514)}{4.55pt}{4.82pt}{} & \HoloSegScore{2.100}{(1.898--3.499)}{4.55pt}{4.82pt}{} & \HoloSegScore{7.106}{(1.050--17.57)}{4.55pt}{4.82pt}{} & \HoloSegScore{1.762}{(1.110--2.606)}{4.55pt}{4.82pt}{} \\
\cline{2-11}
 &  &  & \HoloSegMetric{Dice} & \HoloSegScore{0.9167}{(0.9071--0.9252)}{4.55pt}{4.82pt}{} & \HoloSegScore{0.4816}{(0.4426--0.5208)}{4.55pt}{4.82pt}{} & \HoloSegScore{0.9264}{(0.9148--0.9337)}{4.55pt}{4.82pt}{} & \HoloSegScore{0.9728}{(0.9703--0.9750)}{4.55pt}{4.82pt}{} & \HoloSegScore{0.9534}{(0.9396--0.9638)}{4.55pt}{4.82pt}{} & \HoloSegScore{0.9229}{(0.9171--0.9282)}{4.55pt}{4.82pt}{} & \HoloSegScore{0.9499}{(0.9469--0.9527)}{4.55pt}{4.82pt}{} \\*
\softcline{4-11}
 &  & \HoloSegSpan{\makecell[c]{sacrum}}{2.04cm}{0.32cm} & \HoloSegMetric{HD95} & \HoloSegScore{4.375}{(2.930--6.452)}{4.55pt}{4.82pt}{} & \HoloSegScore{37.55}{(29.66--45.36)}{4.55pt}{4.82pt}{} & \HoloSegScore{1.956}{(1.552--2.511)}{4.55pt}{4.82pt}{} & \HoloSegScore{1.888}{(1.196--2.904)}{4.55pt}{4.82pt}{} & \HoloSegScore{4.080}{(1.425--5.627)}{4.55pt}{4.82pt}{} & \HoloSegScore{3.865}{(3.332--4.458)}{4.55pt}{4.82pt}{} & \HoloSegScore{1.860}{(1.567--2.237)}{4.55pt}{4.82pt}{} \\
\cline{3-11}
 &  &  & \HoloSegMetric{Dice} & \HoloSegScore{0.9365}{(0.9156--0.9505)}{4.55pt}{4.82pt}{} & \HoloSegScore{0.6547}{(0.6241--0.6819)}{4.55pt}{4.82pt}{} & \HoloSegScore{0.9259}{(0.9062--0.9403)}{4.55pt}{4.82pt}{} & \HoloSegScore{0.9778}{(0.9706--0.9827)}{4.55pt}{4.82pt}{} & \HoloSegScore{0.9437}{(0.9305--0.9530)}{4.55pt}{4.82pt}{} & \HoloSegScore{0.9672}{(0.9646--0.9692)}{4.55pt}{4.82pt}{} & \HoloSegScore{0.9672}{(0.9647--0.9691)}{4.55pt}{4.82pt}{} \\*
\softcline{4-11}
 &  & \HoloSegSpan{\makecell[c]{left hip}}{2.04cm}{0.32cm} & \HoloSegMetric{HD95} & \HoloSegScore{4.987}{(1.691--9.549)}{4.55pt}{4.82pt}{} & \HoloSegScore{22.32}{(17.58--27.97)}{4.55pt}{4.82pt}{} & \HoloSegScore{4.406}{(1.686--8.144)}{4.55pt}{4.82pt}{} & \HoloSegScore{6.495}{(2.837--11.00)}{4.55pt}{4.82pt}{} & \HoloSegScore{4.124}{(3.563--5.920)}{4.55pt}{4.82pt}{} & \HoloSegScore{14.65}{(7.572--23.26)}{4.55pt}{4.82pt}{} & \HoloSegScore{2.178}{(0.8370--4.386)}{4.55pt}{4.82pt}{} \\
\cline{3-11}
 & \HoloSegSpan{\makecell[c]{CTPelvic1K-\\[-0.10ex]COLONOG}}{1.86cm}{0.32cm} &  & \HoloSegMetric{Dice} & \HoloSegScore{0.9354}{(0.9149--0.9493)}{4.55pt}{4.82pt}{} & \HoloSegScore{0.5441}{(0.5089--0.5786)}{4.55pt}{4.82pt}{} & \HoloSegScore{0.9204}{(0.8994--0.9344)}{4.55pt}{4.82pt}{} & \HoloSegScore{0.9786}{(0.9711--0.9838)}{4.55pt}{4.82pt}{} & \HoloSegScore{0.9640}{(0.9524--0.9735)}{4.55pt}{4.82pt}{} & \HoloSegScore{0.9699}{(0.9678--0.9716)}{4.55pt}{4.82pt}{} & \HoloSegScore{0.9688}{(0.9666--0.9706)}{4.55pt}{4.82pt}{} \\*
\softcline{4-11}
 &  & \HoloSegSpan{\makecell[c]{right hip}}{2.04cm}{0.32cm} & \HoloSegMetric{HD95} & \HoloSegScore{6.173}{(1.356--11.96)}{4.55pt}{4.82pt}{} & \HoloSegScore{78.93}{(66.81--90.86)}{4.55pt}{4.82pt}{} & \HoloSegScore{4.478}{(1.846--8.194)}{4.55pt}{4.82pt}{} & \HoloSegScore{4.655}{(1.458--8.643)}{4.55pt}{4.82pt}{} & \HoloSegScore{2.250}{(2.000--2.495)}{4.55pt}{4.82pt}{} & \HoloSegScore{1.284}{(0.8303--2.107)}{4.55pt}{4.82pt}{} & \HoloSegScore{1.165}{(0.7772--1.921)}{4.55pt}{4.82pt}{} \\
\cline{3-11}
 &  &  & \HoloSegMetric{Dice} & \HoloSegScore{0.6543}{(0.6368--0.6713)}{4.55pt}{4.82pt}{} & \HoloSegScore{0.4506}{(0.4263--0.4763)}{4.55pt}{4.82pt}{} & \HoloSegScore{0.6484}{(0.6305--0.6656)}{4.55pt}{4.82pt}{} & \HoloSegScore{0.6807}{(0.6622--0.6982)}{4.55pt}{4.82pt}{} & \HoloSegScore{0.8248}{(0.8189--0.8414)}{4.55pt}{4.82pt}{} & \HoloSegScore{0.8492}{(0.8376--0.8605)}{4.55pt}{4.82pt}{} & \HoloSegScore{0.8789}{(0.8676--0.8895)}{4.55pt}{4.82pt}{} \\*
\softcline{4-11}
 &  & \HoloSegSpan{\makecell[c]{lumbar\\[-0.10ex]vertebrae}}{2.04cm}{0.32cm} & \HoloSegMetric{HD95} & \HoloSegScore{71.52}{(67.80--75.50)}{4.55pt}{4.82pt}{} & \HoloSegScore{42.72}{(37.14--48.64)}{4.55pt}{4.82pt}{} & \HoloSegScore{71.27}{(65.67--76.88)}{4.55pt}{4.82pt}{} & \HoloSegScore{70.55}{(66.77--74.30)}{4.55pt}{4.82pt}{} & \HoloSegScore{13.84}{(11.67--15.80)}{4.55pt}{4.82pt}{} & \HoloSegScore{16.23}{(12.62--21.00)}{4.55pt}{4.82pt}{} & \HoloSegScore{18.69}{(14.14--24.03)}{4.55pt}{4.82pt}{} \\
\cline{2-11}
 &  &  & \HoloSegMetric{Dice} & \HoloSegScore{0.8322}{(0.8197--0.8435)}{4.55pt}{4.82pt}{} & \HoloSegScore{0.04111}{(0.007349--0.08688)}{3.85pt}{4.12pt}{} & \HoloSegScore{0.9261}{(0.9093--0.9373)}{4.55pt}{4.82pt}{} & \HoloSegScore{0.9551}{(0.9395--0.9679)}{4.55pt}{4.82pt}{} & \HoloSegScore{0.9488}{(0.9252--0.9754)}{4.55pt}{4.82pt}{} & \HoloSegScore{0.8771}{(0.8501--0.9027)}{4.55pt}{4.82pt}{} & \HoloSegScore{0.8931}{(0.8613--0.9218)}{4.55pt}{4.82pt}{} \\*
\softcline{4-11}
 &  & \HoloSegSpan{\makecell[c]{sacrum}}{2.04cm}{0.32cm} & \HoloSegMetric{HD95} & \HoloSegScore{13.02}{(4.269--25.44)}{4.55pt}{4.82pt}{} & \HoloSegScore{176.3}{(119.1--262.9)}{4.55pt}{4.82pt}{} & \HoloSegScore{2.667}{(1.646--4.170)}{4.55pt}{4.82pt}{} & \HoloSegScore{3.031}{(1.005--5.375)}{4.55pt}{4.82pt}{} & \HoloSegScore{3.463}{(2.920--4.026)}{4.55pt}{4.82pt}{} & \HoloSegScore{7.240}{(4.790--9.987)}{4.55pt}{4.82pt}{} & \HoloSegScore{4.972}{(2.990--7.384)}{4.55pt}{4.82pt}{} \\
\cline{3-11}
 &  &  & \HoloSegMetric{Dice} & \HoloSegScore{0.9415}{(0.9245--0.9548)}{4.55pt}{4.82pt}{} & \HoloSegScore{0.3451}{(0.2494--0.4227)}{4.55pt}{4.82pt}{} & \HoloSegScore{0.9348}{(0.9176--0.9481)}{4.55pt}{4.82pt}{} & \HoloSegScore{0.9645}{(0.9469--0.9784)}{4.55pt}{4.82pt}{} & \HoloSegScore{0.9096}{(0.9017--0.9297)}{4.55pt}{4.82pt}{} & \HoloSegScore{0.9521}{(0.9344--0.9673)}{4.55pt}{4.82pt}{} & \HoloSegScore{0.9492}{(0.9334--0.9635)}{4.55pt}{4.82pt}{} \\*
\softcline{4-11}
 &  & \HoloSegSpan{\makecell[c]{left hip}}{2.04cm}{0.32cm} & \HoloSegMetric{HD95} & \HoloSegScore{5.851}{(2.026--10.81)}{4.55pt}{4.82pt}{} & \HoloSegScore{127.2}{(86.23--164.7)}{4.55pt}{4.82pt}{} & \HoloSegScore{4.291}{(1.971--7.867)}{4.55pt}{4.82pt}{} & \HoloSegScore{5.406}{(1.581--10.87)}{4.55pt}{4.82pt}{} & \HoloSegScore{6.387}{(3.327--9.970)}{4.55pt}{4.82pt}{} & \HoloSegScore{8.481}{(3.362--15.01)}{4.55pt}{4.82pt}{} & \HoloSegScore{5.727}{(1.729--10.87)}{4.55pt}{4.82pt}{} \\
\cline{3-11}
 & \HoloSegSpan{\makecell[c]{CTPelvic1K-\\[-0.10ex]KiTS}}{1.86cm}{0.32cm} &  & \HoloSegMetric{Dice} & \HoloSegScore{0.9263}{(0.9063--0.9437)}{4.55pt}{4.82pt}{} & \HoloSegScore{0.2479}{(0.1970--0.3053)}{4.55pt}{4.82pt}{} & \HoloSegScore{0.9275}{(0.9084--0.9413)}{4.55pt}{4.82pt}{} & \HoloSegScore{0.9640}{(0.9433--0.9791)}{4.55pt}{4.82pt}{} & \HoloSegScore{0.9218}{(0.9012--0.9313)}{4.55pt}{4.82pt}{} & \HoloSegScore{0.9518}{(0.9336--0.9672)}{4.55pt}{4.82pt}{} & \HoloSegScore{0.9463}{(0.9281--0.9623)}{4.55pt}{4.82pt}{} \\*
\softcline{4-11}
 &  & \HoloSegSpan{\makecell[c]{right hip}}{2.04cm}{0.32cm} & \HoloSegMetric{HD95} & \HoloSegScore{12.11}{(0.8379--23.78)}{4.55pt}{4.82pt}{} & \HoloSegScore{163.3}{(149.9--176.0)}{4.55pt}{4.82pt}{} & \HoloSegScore{4.959}{(2.083--9.008)}{4.55pt}{4.82pt}{} & \HoloSegScore{5.240}{(0.8015--11.77)}{4.55pt}{4.82pt}{} & \HoloSegScore{5.478}{(3.100--9.060)}{4.55pt}{4.82pt}{} & \HoloSegScore{6.196}{(1.211--11.92)}{4.55pt}{4.82pt}{} & \HoloSegScore{5.491}{(1.114--11.13)}{4.55pt}{4.82pt}{} \\
\cline{3-11}
 &  &  & \HoloSegMetric{Dice} & \HoloSegScore{0.4156}{(0.2920--0.5208)}{4.55pt}{4.82pt}{} & \HoloSegScore{0.2165}{(0.1326--0.2947)}{4.55pt}{4.82pt}{} & \HoloSegScore{0.4105}{(0.2856--0.5123)}{4.55pt}{4.82pt}{} & \HoloSegScore{0.4302}{(0.3150--0.5321)}{4.55pt}{4.82pt}{} & \HoloSegScore{0.6397}{(0.5184--0.7467)}{4.55pt}{4.82pt}{} & \HoloSegScore{0.7022}{(0.5160--0.8399)}{4.55pt}{4.82pt}{} & \HoloSegScore{0.7034}{(0.5083--0.8530)}{4.55pt}{4.82pt}{} \\*
\softcline{4-11}
\HoloSegSpan{\makecell[c]{\textbf{Internal}}}{1.20cm}{0.32cm} &  & \HoloSegSpan{\makecell[c]{lumbar\\[-0.10ex]vertebrae}}{2.04cm}{0.32cm} & \HoloSegMetric{HD95} & \HoloSegScore{177.6}{(105.0--275.3)}{4.55pt}{4.82pt}{} & \HoloSegScore{120.2}{(98.67--143.7)}{4.55pt}{4.82pt}{} & \HoloSegScore{115.1}{(94.13--138.2)}{4.55pt}{4.82pt}{} & \HoloSegScore{116.8}{(93.39--140.4)}{4.55pt}{4.82pt}{} & \HoloSegScore{31.97}{(18.81--45.16)}{4.55pt}{4.82pt}{} & \HoloSegScore{79.73}{(18.67--183.5)}{4.55pt}{4.82pt}{} & \HoloSegScore{85.11}{(29.82--157.5)}{4.55pt}{4.82pt}{} \\
\cline{2-11}
 &  &  & \HoloSegMetric{Dice} & \HoloSegScore{0.8123}{(0.8038--0.8204)}{4.55pt}{4.82pt}{} & \HoloSegScore{0.5830}{(0.5012--0.6306)}{4.55pt}{4.82pt}{} & \HoloSegScore{0.9299}{(0.9219--0.9369)}{4.55pt}{4.82pt}{} & \HoloSegScore{0.9133}{(0.8967--0.9271)}{4.55pt}{4.82pt}{} & \HoloSegScore{0.8991}{(0.8981--0.9109)}{4.55pt}{4.82pt}{} & \HoloSegScore{0.8963}{(0.8753--0.9153)}{4.55pt}{4.82pt}{} & \HoloSegScore{0.9262}{(0.9121--0.9385)}{4.55pt}{4.82pt}{} \\*
\softcline{4-11}
 &  & \HoloSegSpan{\makecell[c]{sacrum}}{2.04cm}{0.32cm} & \HoloSegMetric{HD95} & \HoloSegScore{9.761}{(3.524--18.13)}{4.55pt}{4.82pt}{} & \HoloSegScore{11.09}{(9.948--12.43)}{4.55pt}{4.82pt}{} & \HoloSegScore{1.977}{(1.676--2.319)}{4.55pt}{4.82pt}{} & \HoloSegScore{5.347}{(3.558--7.420)}{4.55pt}{4.82pt}{} & \HoloSegScore{5.670}{(5.397--6.162)}{4.55pt}{4.82pt}{} & \HoloSegScore{5.000}{(3.683--6.763)}{4.55pt}{4.82pt}{} & \HoloSegScore{2.742}{(1.923--3.721)}{4.55pt}{4.82pt}{} \\
\cline{3-11}
 &  &  & \HoloSegMetric{Dice} & \HoloSegScore{0.9388}{(0.9344--0.9432)}{4.55pt}{4.82pt}{} & \HoloSegScore{0.6900}{(0.6739--0.7079)}{4.55pt}{4.82pt}{} & \HoloSegScore{0.9467}{(0.9428--0.9501)}{4.55pt}{4.82pt}{} & \HoloSegScore{0.9606}{(0.9553--0.9660)}{4.55pt}{4.82pt}{} & \HoloSegScore{0.9365}{(0.9284--0.9376)}{4.55pt}{4.82pt}{} & \HoloSegScore{0.9559}{(0.9505--0.9609)}{4.55pt}{4.82pt}{} & \HoloSegScore{0.9564}{(0.9506--0.9621)}{4.55pt}{4.82pt}{} \\*
\softcline{4-11}
 &  & \HoloSegSpan{\makecell[c]{left hip}}{2.04cm}{0.32cm} & \HoloSegMetric{HD95} & \HoloSegScore{2.780}{(2.444--3.165)}{4.55pt}{4.82pt}{} & \HoloSegScore{10.23}{(9.631--10.86)}{4.55pt}{4.82pt}{} & \HoloSegScore{1.866}{(1.673--2.045)}{4.55pt}{4.82pt}{} & \HoloSegScore{1.927}{(1.295--2.754)}{4.55pt}{4.82pt}{} & \HoloSegScore{2.556}{(1.848--3.487)}{4.55pt}{4.82pt}{} & \HoloSegScore{12.07}{(3.318--24.79)}{4.55pt}{4.82pt}{} & \HoloSegScore{13.23}{(1.152--36.98)}{4.55pt}{4.82pt}{} \\
\cline{3-11}
 & \HoloSegSpan{\makecell[c]{CTPelvic1K-\\[-0.10ex]MSD-colon}}{1.86cm}{0.32cm} &  & \HoloSegMetric{Dice} & \HoloSegScore{0.9351}{(0.9288--0.9406)}{4.55pt}{4.82pt}{} & \HoloSegScore{0.5504}{(0.4703--0.6315)}{4.55pt}{4.82pt}{} & \HoloSegScore{0.9451}{(0.9408--0.9485)}{4.55pt}{4.82pt}{} & \HoloSegScore{0.9614}{(0.9566--0.9656)}{4.55pt}{4.82pt}{} & \HoloSegScore{0.9607}{(0.9408--0.9680)}{4.55pt}{4.82pt}{} & \HoloSegScore{0.9582}{(0.9514--0.9640)}{4.55pt}{4.82pt}{} & \HoloSegScore{0.9574}{(0.9511--0.9629)}{4.55pt}{4.82pt}{} \\*
\softcline{4-11}
 &  & \HoloSegSpan{\makecell[c]{right hip}}{2.04cm}{0.32cm} & \HoloSegMetric{HD95} & \HoloSegScore{7.501}{(1.880--13.97)}{4.55pt}{4.82pt}{} & \HoloSegScore{89.88}{(55.56--125.0)}{4.55pt}{4.82pt}{} & \HoloSegScore{2.533}{(2.149--2.945)}{4.55pt}{4.82pt}{} & \HoloSegScore{1.470}{(1.105--1.875)}{4.55pt}{4.82pt}{} & \HoloSegScore{1.996}{(1.885--2.415)}{4.55pt}{4.82pt}{} & \HoloSegScore{1.483}{(1.065--1.979)}{4.55pt}{4.82pt}{} & \HoloSegScore{1.307}{(0.9499--1.722)}{4.55pt}{4.82pt}{} \\
\cline{3-11}
 &  &  & \HoloSegMetric{Dice} & \HoloSegScore{0.6423}{(0.6073--0.6792)}{4.55pt}{4.82pt}{} & \HoloSegScore{0.4567}{(0.4032--0.5113)}{4.55pt}{4.82pt}{} & \HoloSegScore{0.6598}{(0.6252--0.6975)}{4.55pt}{4.82pt}{} & \HoloSegScore{0.6547}{(0.6184--0.6935)}{4.55pt}{4.82pt}{} & \HoloSegScore{0.8135}{(0.7884--0.8406)}{4.55pt}{4.82pt}{} & \HoloSegScore{0.8361}{(0.8059--0.8649)}{4.55pt}{4.82pt}{} & \HoloSegScore{0.8621}{(0.8409--0.8818)}{4.55pt}{4.82pt}{} \\*
\softcline{4-11}
 &  & \HoloSegSpan{\makecell[c]{lumbar\\[-0.10ex]vertebrae}}{2.04cm}{0.32cm} & \HoloSegMetric{HD95} & \HoloSegScore{131.2}{(87.25--182.2)}{4.55pt}{4.82pt}{} & \HoloSegScore{36.53}{(30.39--41.88)}{4.55pt}{4.82pt}{} & \HoloSegScore{74.85}{(60.45--92.93)}{4.55pt}{4.82pt}{} & \HoloSegScore{74.60}{(65.73--83.01)}{4.55pt}{4.82pt}{} & \HoloSegScore{28.42}{(22.75--32.50)}{4.55pt}{4.82pt}{} & \HoloSegScore{40.53}{(12.76--82.62)}{4.55pt}{4.82pt}{} & \HoloSegScore{60.81}{(22.05--107.9)}{4.55pt}{4.82pt}{} \\
\cline{2-11}
 &  &  & \HoloSegMetric{Dice} & \HoloSegScore{0.4370}{(0.2470--0.6753)}{4.55pt}{4.82pt}{} & \HoloSegScore{0.5539}{(0.4622--0.6372)}{4.55pt}{4.82pt}{} & \HoloSegScore{0.3867}{(0.2177--0.6611)}{4.55pt}{4.82pt}{} & \HoloSegScore{0.9445}{(0.9389--0.9503)}{4.55pt}{4.82pt}{} & \HoloSegScore{0.8933}{(0.8853--0.9094)}{4.55pt}{4.82pt}{} & \HoloSegScore{0.9034}{(0.8796--0.9255)}{4.55pt}{4.82pt}{} & \HoloSegScore{0.9362}{(0.9263--0.9461)}{4.55pt}{4.82pt}{} \\*
\softcline{4-11}
 &  & \HoloSegSpan{\makecell[c]{sacrum}}{2.04cm}{0.32cm} & \HoloSegMetric{HD95} & \HoloSegScore{46.58}{(28.10--61.85)}{4.55pt}{4.82pt}{} & \HoloSegScore{25.90}{(9.754--55.15)}{4.55pt}{4.82pt}{} & \HoloSegScore{23.82}{(12.55--32.32)}{4.55pt}{4.82pt}{} & \HoloSegScore{1.963}{(1.300--2.666)}{4.55pt}{4.82pt}{} & \HoloSegScore{5.003}{(4.326--5.702)}{4.55pt}{4.82pt}{} & \HoloSegScore{3.747}{(2.353--5.142)}{4.55pt}{4.82pt}{} & \HoloSegScore{2.013}{(1.477--2.464)}{4.55pt}{4.82pt}{} \\
\cline{3-11}
 &  &  & \HoloSegMetric{Dice} & \HoloSegScore{0.2018}{(0.007974--0.5748)}{4.20pt}{4.48pt}{} & \HoloSegScore{0.6768}{(0.6454--0.7075)}{4.55pt}{4.82pt}{} & \HoloSegScore{0.1916}{(0.0000--0.5744)}{4.55pt}{4.82pt}{} & \HoloSegScore{0.6785}{(0.5911--0.8250)}{4.55pt}{4.82pt}{} & \HoloSegScore{0.9227}{(0.9009--0.9369)}{4.55pt}{4.82pt}{} & \HoloSegScore{0.9613}{(0.9570--0.9656)}{4.55pt}{4.82pt}{} & \HoloSegScore{0.9634}{(0.9588--0.9662)}{4.55pt}{4.82pt}{} \\*
\softcline{4-11}
 &  & \HoloSegSpan{\makecell[c]{left hip}}{2.04cm}{0.32cm} & \HoloSegMetric{HD95} & \HoloSegScore{138.7}{(70.13--174.7)}{4.55pt}{4.82pt}{} & \HoloSegScore{36.93}{(8.907--91.85)}{4.55pt}{4.82pt}{} & \HoloSegScore{136.8}{(68.21--175.2)}{4.55pt}{4.82pt}{} & \HoloSegScore{128.8}{(64.06--163.9)}{4.55pt}{4.82pt}{} & \HoloSegScore{8.413}{(5.008--13.63)}{4.55pt}{4.82pt}{} & \HoloSegScore{1.299}{(0.9766--1.782)}{4.55pt}{4.82pt}{} & \HoloSegScore{0.9766}{(0.9766--0.9766)}{4.55pt}{4.82pt}{} \\
\cline{3-11}
 & \HoloSegSpan{\makecell[c]{CTPelvic1K-\\[-0.10ex]BTCV-\\[-0.10ex]Cervix}}{1.86cm}{0.32cm} &  & \HoloSegMetric{Dice} & \HoloSegScore{0.1917}{(0.0005502--0.5721)}{3.85pt}{4.12pt}{} & \HoloSegScore{0.6283}{(0.4701--0.7265)}{4.55pt}{4.82pt}{} & \HoloSegScore{0.1913}{(0.0000--0.5738)}{4.55pt}{4.82pt}{} & \HoloSegScore{0.6867}{(0.5979--0.8326)}{4.55pt}{4.82pt}{} & \HoloSegScore{0.9437}{(0.9250--0.9499)}{4.55pt}{4.82pt}{} & \HoloSegScore{0.9627}{(0.9591--0.9664)}{4.55pt}{4.82pt}{} & \HoloSegScore{0.9651}{(0.9600--0.9687)}{4.55pt}{4.82pt}{} \\*
\softcline{4-11}
 &  & \HoloSegSpan{\makecell[c]{right hip}}{2.04cm}{0.32cm} & \HoloSegMetric{HD95} & \HoloSegScore{140.2}{(71.21--178.5)}{4.55pt}{4.82pt}{} & \HoloSegScore{39.70}{(8.653--95.46)}{4.55pt}{4.82pt}{} & \HoloSegScore{139.1}{(68.41--177.6)}{4.55pt}{4.82pt}{} & \HoloSegScore{131.3}{(65.72--167.0)}{4.55pt}{4.82pt}{} & \HoloSegScore{2.374}{(1.948--2.895)}{4.55pt}{4.82pt}{} & \HoloSegScore{0.9766}{(0.9766--0.9766)}{4.55pt}{4.82pt}{} & \HoloSegScore{0.9766}{(0.9766--0.9766)}{4.55pt}{4.82pt}{} \\
\cline{3-11}
 &  &  & \HoloSegMetric{Dice} & \HoloSegScore{0.5000}{(0.4508--0.5457)}{4.55pt}{4.82pt}{} & \HoloSegScore{0.3137}{(0.1782--0.4369)}{4.55pt}{4.82pt}{} & \HoloSegScore{0.2146}{(0.1487--0.3195)}{4.55pt}{4.82pt}{} & \HoloSegScore{0.4517}{(0.4214--0.4925)}{4.55pt}{4.82pt}{} & \HoloSegScore{0.8175}{(0.7714--0.8341)}{4.55pt}{4.82pt}{} & \HoloSegScore{0.8160}{(0.7863--0.8453)}{4.55pt}{4.82pt}{} & \HoloSegScore{0.8381}{(0.8097--0.8721)}{4.55pt}{4.82pt}{} \\*
\softcline{4-11}
 &  & \HoloSegSpan{\makecell[c]{lumbar\\[-0.10ex]vertebrae}}{2.04cm}{0.32cm} & \HoloSegMetric{HD95} & \HoloSegScore{96.09}{(81.57--111.2)}{4.55pt}{4.82pt}{} & \HoloSegScore{44.58}{(23.63--77.29)}{4.55pt}{4.82pt}{} & \HoloSegScore{119.6}{(96.00--145.8)}{4.55pt}{4.82pt}{} & \HoloSegScore{116.7}{(96.66--138.3)}{4.55pt}{4.82pt}{} & \HoloSegScore{12.94}{(8.876--17.44)}{4.55pt}{4.82pt}{} & \HoloSegScore{20.64}{(13.15--28.54)}{4.55pt}{4.82pt}{} & \HoloSegScore{9.199}{(4.623--14.39)}{4.55pt}{4.82pt}{} \\
\cline{2-11}
 &  &  & \HoloSegMetric{Dice} & \HoloSegScore{0.8126}{(0.8035--0.8223)}{4.55pt}{4.82pt}{} & \HoloSegScore{0.6179}{(0.5610--0.6676)}{4.55pt}{4.82pt}{} & \HoloSegScore{0.9303}{(0.9201--0.9427)}{4.55pt}{4.82pt}{} & \HoloSegScore{0.9303}{(0.9190--0.9433)}{4.55pt}{4.82pt}{} & \HoloSegScore{0.9166}{(0.8984--0.9402)}{4.55pt}{4.82pt}{} & \HoloSegScore{0.8944}{(0.8712--0.9156)}{4.55pt}{4.82pt}{} & \HoloSegScore{0.9267}{(0.9187--0.9366)}{4.55pt}{4.82pt}{} \\*
\softcline{4-11}
 & \HoloSegSpan{\makecell[c]{CTPelvic1K-\\[-0.10ex]BTCV-\\[-0.10ex]Abdomen}}{1.86cm}{0.32cm} & \HoloSegSpan{\makecell[c]{sacrum}}{2.04cm}{0.32cm} & \HoloSegMetric{HD95} & \HoloSegScore{13.71}{(11.86--15.51)}{4.55pt}{4.82pt}{} & \HoloSegScore{10.82}{(8.072--15.71)}{4.55pt}{4.82pt}{} & \HoloSegScore{1.838}{(1.330--2.281)}{4.55pt}{4.82pt}{} & \HoloSegScore{2.132}{(1.593--2.638)}{4.55pt}{4.82pt}{} & \HoloSegScore{1.724}{(1.570--2.418)}{4.55pt}{4.82pt}{} & \HoloSegScore{3.757}{(2.663--4.834)}{4.55pt}{4.82pt}{} & \HoloSegScore{2.600}{(1.822--3.518)}{4.55pt}{4.82pt}{} \\
\hline
\pagebreak[4]
 &  &  & \HoloSegMetric{Dice} & \HoloSegScore{0.9434}{(0.9406--0.9465)}{4.55pt}{4.82pt}{} & \HoloSegScore{0.5621}{(0.4270--0.6891)}{4.55pt}{4.82pt}{} & \HoloSegScore{0.9445}{(0.9398--0.9490)}{4.55pt}{4.82pt}{} & \HoloSegScore{0.9635}{(0.9615--0.9660)}{4.55pt}{4.82pt}{} & \HoloSegScore{0.9444}{(0.9325--0.9526)}{4.55pt}{4.82pt}{} & \HoloSegScore{0.9633}{(0.9593--0.9673)}{4.55pt}{4.82pt}{} & \HoloSegScore{0.9618}{(0.9585--0.9656)}{4.55pt}{4.82pt}{} \\*
\softcline{4-11}
 &  & \HoloSegSpan{\makecell[c]{right hip}}{2.04cm}{0.32cm} & \HoloSegMetric{HD95} & \HoloSegScore{2.030}{(1.566--2.608)}{4.55pt}{4.82pt}{} & \HoloSegScore{77.01}{(24.33--133.3)}{4.55pt}{4.82pt}{} & \HoloSegScore{2.506}{(2.152--2.860)}{4.55pt}{4.82pt}{} & \HoloSegScore{1.178}{(0.8530--1.578)}{4.55pt}{4.82pt}{} & \HoloSegScore{3.053}{(2.728--3.892)}{4.55pt}{4.82pt}{} & \HoloSegScore{0.9573}{(0.7570--1.196)}{4.55pt}{4.82pt}{} & \HoloSegScore{0.7812}{(0.6963--0.8934)}{4.55pt}{4.82pt}{} \\
\cline{3-11}
 &  &  & \HoloSegMetric{Dice} & \HoloSegScore{0.9433}{(0.9392--0.9480)}{4.55pt}{4.82pt}{} & \HoloSegScore{0.7105}{(0.6835--0.7331)}{4.55pt}{4.82pt}{} & \HoloSegScore{0.9494}{(0.9428--0.9556)}{4.55pt}{4.82pt}{} & \HoloSegScore{0.9665}{(0.9615--0.9721)}{4.55pt}{4.82pt}{} & \HoloSegScore{0.9628}{(0.9467--0.9664)}{4.55pt}{4.82pt}{} & \HoloSegScore{0.9609}{(0.9564--0.9639)}{4.55pt}{4.82pt}{} & \HoloSegScore{0.9628}{(0.9588--0.9665)}{4.55pt}{4.82pt}{} \\*
\softcline{4-11}
 & \HoloSegSpan{\makecell[c]{CTPelvic1K-\\[-0.10ex]BTCV-\\[-0.10ex]Abdomen}}{1.86cm}{0.32cm} & \HoloSegSpan{\makecell[c]{left hip}}{2.04cm}{0.32cm} & \HoloSegMetric{HD95} & \HoloSegScore{1.837}{(1.398--2.340)}{4.55pt}{4.82pt}{} & \HoloSegScore{25.20}{(7.329--59.87)}{4.55pt}{4.82pt}{} & \HoloSegScore{1.860}{(1.376--2.374)}{4.55pt}{4.82pt}{} & \HoloSegScore{1.174}{(0.7265--1.740)}{4.55pt}{4.82pt}{} & \HoloSegScore{1.977}{(1.678--3.409)}{4.55pt}{4.82pt}{} & \HoloSegScore{13.83}{(1.662--35.05)}{4.55pt}{4.82pt}{} & \HoloSegScore{0.8535}{(0.6921--1.119)}{4.55pt}{4.82pt}{} \\
\cline{3-11}
 &  &  & \HoloSegMetric{Dice} & \HoloSegScore{0.6483}{(0.5893--0.6862)}{4.55pt}{4.82pt}{} & \HoloSegScore{0.5031}{(0.3993--0.5843)}{4.55pt}{4.82pt}{} & \HoloSegScore{0.6577}{(0.5978--0.6961)}{4.55pt}{4.82pt}{} & \HoloSegScore{0.6505}{(0.5820--0.6922)}{4.55pt}{4.82pt}{} & \HoloSegScore{0.8457}{(0.8338--0.8692)}{4.55pt}{4.82pt}{} & \HoloSegScore{0.8485}{(0.8155--0.8791)}{4.55pt}{4.82pt}{} & \HoloSegScore{0.8646}{(0.8387--0.8850)}{4.55pt}{4.82pt}{} \\*
\softcline{4-11}
 &  & \HoloSegSpan{\makecell[c]{lumbar\\[-0.10ex]vertebrae}}{2.04cm}{0.32cm} & \HoloSegMetric{HD95} & \HoloSegScore{74.49}{(65.26--87.57)}{4.55pt}{4.82pt}{} & \HoloSegScore{26.58}{(20.62--32.10)}{4.55pt}{4.82pt}{} & \HoloSegScore{67.51}{(57.34--81.17)}{4.55pt}{4.82pt}{} & \HoloSegScore{72.12}{(63.41--85.30)}{4.55pt}{4.82pt}{} & \HoloSegScore{9.361}{(6.437--11.02)}{4.55pt}{4.82pt}{} & \HoloSegScore{12.14}{(4.684--19.73)}{4.55pt}{4.82pt}{} & \HoloSegScore{13.15}{(7.635--19.32)}{4.55pt}{4.82pt}{} \\
\cline{2-11}
 &  &  & \HoloSegMetric{Dice} &  & \HoloSegScore{0.05244}{(0.03391--0.07375)}{4.20pt}{4.48pt}{} & \HoloSegScore{0.8621}{(0.8449--0.8742)}{4.55pt}{4.82pt}{} & \HoloSegScore{0.5513}{(0.5232--0.5778)}{4.55pt}{4.82pt}{} & \HoloSegScore{0.7882}{(0.7738--0.8122)}{4.55pt}{4.82pt}{} & \HoloSegScore{0.8315}{(0.8183--0.8451)}{4.55pt}{4.82pt}{} & \HoloSegScore{0.8458}{(0.8356--0.8550)}{4.55pt}{4.82pt}{} \\*
\softcline{4-4}\softcline{6-11}
 &  & \HoloSegSpan{\makecell[c]{caudate lobe}}{2.04cm}{0.32cm} & \HoloSegMetric{HD95} & \raisebox{0.32cm}[0pt][0pt]{\HoloSegUnsupported} & \HoloSegScore{66.12}{(52.78--79.67)}{4.55pt}{4.82pt}{} & \HoloSegScore{4.882}{(4.492--5.397)}{4.55pt}{4.82pt}{} & \HoloSegScore{25.19}{(23.76--26.63)}{4.55pt}{4.82pt}{} & \HoloSegScore{11.07}{(9.365--12.63)}{4.55pt}{4.82pt}{} & \HoloSegScore{6.885}{(5.930--7.957)}{4.55pt}{4.82pt}{} & \HoloSegScore{5.606}{(5.166--6.105)}{4.55pt}{4.82pt}{} \\
\cline{3-11}
 &  &  & \HoloSegMetric{Dice} &  & \HoloSegScore{0.0000}{(0.0000--0.0000)}{4.55pt}{4.82pt}{} & \HoloSegScore{0.8844}{(0.8526--0.9082)}{4.55pt}{4.82pt}{} & \HoloSegScore{0.8186}{(0.7894--0.8446)}{4.55pt}{4.82pt}{} & \HoloSegScore{0.8431}{(0.8172--0.8786)}{4.55pt}{4.82pt}{} & \HoloSegScore{0.8855}{(0.8612--0.9054)}{4.55pt}{4.82pt}{} & \HoloSegScore{0.9081}{(0.8965--0.9182)}{4.55pt}{4.82pt}{} \\*
\softcline{4-4}\softcline{6-11}
 &  & \HoloSegSpan{\makecell[c]{left lateral\\[-0.10ex]superior\\[-0.10ex]segment of\\[-0.10ex]liver}}{2.04cm}{0.32cm} & \HoloSegMetric{HD95} & \raisebox{0.32cm}[0pt][0pt]{\HoloSegUnsupported} & \HoloSegScore{130.8}{(119.4--140.7)}{4.55pt}{4.82pt}{} & \HoloSegScore{6.506}{(5.203--8.467)}{4.55pt}{4.82pt}{} & \HoloSegScore{13.35}{(10.41--16.79)}{4.55pt}{4.82pt}{} & \HoloSegScore{11.34}{(11.15--12.84)}{4.55pt}{4.82pt}{} & \HoloSegScore{8.853}{(6.911--11.06)}{4.55pt}{4.82pt}{} & \HoloSegScore{6.609}{(5.605--7.926)}{4.55pt}{4.82pt}{} \\
\cline{3-11}
 &  &  & \HoloSegMetric{Dice} &  & \HoloSegScore{0.0000}{(0.0000--0.0000)}{4.55pt}{4.82pt}{} & \HoloSegScore{0.8633}{(0.8306--0.8897)}{4.55pt}{4.82pt}{} & \HoloSegScore{0.7637}{(0.7110--0.8091)}{4.55pt}{4.82pt}{} & \HoloSegScore{0.8613}{(0.8499--0.8662)}{4.55pt}{4.82pt}{} & \HoloSegScore{0.8689}{(0.8181--0.9059)}{4.55pt}{4.82pt}{} & \HoloSegScore{0.8752}{(0.8227--0.9103)}{4.55pt}{4.82pt}{} \\*
\softcline{4-4}\softcline{6-11}
 &  & \HoloSegSpan{\makecell[c]{left lateral\\[-0.10ex]inferior\\[-0.10ex]segment of\\[-0.10ex]liver}}{2.04cm}{0.32cm} & \HoloSegMetric{HD95} & \raisebox{0.32cm}[0pt][0pt]{\HoloSegUnsupported} & \HoloSegScore{160.1}{(147.1--172.3)}{4.55pt}{4.82pt}{} & \HoloSegScore{7.674}{(5.527--10.47)}{4.55pt}{4.82pt}{} & \HoloSegScore{16.61}{(12.18--22.01)}{4.55pt}{4.82pt}{} & \HoloSegScore{11.69}{(6.601--16.43)}{4.55pt}{4.82pt}{} & \HoloSegScore{8.620}{(5.486--12.78)}{4.55pt}{4.82pt}{} & \HoloSegScore{8.003}{(4.927--12.22)}{4.55pt}{4.82pt}{} \\
\cline{3-11}
 &  &  & \HoloSegMetric{Dice} &  & \HoloSegScore{0.0000}{(0.0000--0.0000)}{4.55pt}{4.82pt}{} & \HoloSegScore{0.8793}{(0.8449--0.9006)}{4.55pt}{4.82pt}{} & \HoloSegScore{0.7888}{(0.7694--0.8056)}{4.55pt}{4.82pt}{} & \HoloSegScore{0.8166}{(0.7923--0.8276)}{4.55pt}{4.82pt}{} & \HoloSegScore{0.8623}{(0.8479--0.8755)}{4.55pt}{4.82pt}{} & \HoloSegScore{0.8699}{(0.8588--0.8812)}{4.55pt}{4.82pt}{} \\*
\softcline{4-4}\softcline{6-11}
 &  & \HoloSegSpan{\makecell[c]{left medial\\[-0.10ex]segment of\\[-0.10ex]liver}}{2.04cm}{0.32cm} & \HoloSegMetric{HD95} & \raisebox{0.32cm}[0pt][0pt]{\HoloSegUnsupported} & \HoloSegScore{158.9}{(149.3--169.0)}{4.55pt}{4.82pt}{} & \HoloSegScore{5.829}{(4.613--8.033)}{4.55pt}{4.82pt}{} & \HoloSegScore{18.53}{(14.25--23.90)}{4.55pt}{4.82pt}{} & \HoloSegScore{10.69}{(9.193--13.24)}{4.55pt}{4.82pt}{} & \HoloSegScore{9.761}{(7.534--12.38)}{4.55pt}{4.82pt}{} & \HoloSegScore{6.615}{(5.937--7.351)}{4.55pt}{4.82pt}{} \\
\cline{3-11}
 & \HoloSegSpan{\makecell[c]{Couinaud-\\[-0.10ex]Liver\\[-0.10ex](MSD-\\[-0.10ex]hepaticvessel)}}{1.86cm}{0.32cm} &  & \HoloSegMetric{Dice} &  & \HoloSegScore{0.008415}{(0.0006640--0.02088)}{3.85pt}{4.12pt}{} & \HoloSegScore{0.8437}{(0.7886--0.8820)}{4.55pt}{4.82pt}{} & \HoloSegScore{0.7630}{(0.7210--0.7992)}{4.55pt}{4.82pt}{} & \HoloSegScore{0.7886}{(0.7575--0.8248)}{4.55pt}{4.82pt}{} & \HoloSegScore{0.8365}{(0.8013--0.8647)}{4.55pt}{4.82pt}{} & \HoloSegScore{0.8519}{(0.8172--0.8793)}{4.55pt}{4.82pt}{} \\*
\softcline{4-4}\softcline{6-11}
 &  & \HoloSegSpan{\makecell[c]{right\\[-0.10ex]anterior\\[-0.10ex]inferior\\[-0.10ex]segment of\\[-0.10ex]liver}}{2.04cm}{0.32cm} & \HoloSegMetric{HD95} & \raisebox{0.32cm}[0pt][0pt]{\HoloSegUnsupported} & \HoloSegScore{76.84}{(70.87--83.20)}{4.55pt}{4.82pt}{} & \HoloSegScore{8.190}{(6.597--10.21)}{4.55pt}{4.82pt}{} & \HoloSegScore{18.42}{(15.94--20.89)}{4.55pt}{4.82pt}{} & \HoloSegScore{16.44}{(13.75--18.89)}{4.55pt}{4.82pt}{} & \HoloSegScore{14.78}{(10.61--19.93)}{4.55pt}{4.82pt}{} & \HoloSegScore{11.00}{(9.245--13.00)}{4.55pt}{4.82pt}{} \\
\cline{3-11}
 &  &  & \HoloSegMetric{Dice} &  & \HoloSegScore{0.04553}{(0.009687--0.1063)}{4.20pt}{4.48pt}{} & \HoloSegScore{0.8694}{(0.8427--0.8931)}{4.55pt}{4.82pt}{} & \HoloSegScore{0.7636}{(0.7207--0.8006)}{4.55pt}{4.82pt}{} & \HoloSegScore{0.8639}{(0.8374--0.8948)}{4.55pt}{4.82pt}{} & \HoloSegScore{0.8424}{(0.7983--0.8801)}{4.55pt}{4.82pt}{} & \HoloSegScore{0.8725}{(0.8466--0.8944)}{4.55pt}{4.82pt}{} \\*
\softcline{4-4}\softcline{6-11}
 &  & \HoloSegSpan{\makecell[c]{right\\[-0.10ex]posterior\\[-0.10ex]inferior\\[-0.10ex]segment of\\[-0.10ex]liver}}{2.04cm}{0.32cm} & \HoloSegMetric{HD95} & \raisebox{0.32cm}[0pt][0pt]{\HoloSegUnsupported} & \HoloSegScore{70.60}{(60.32--82.29)}{4.55pt}{4.82pt}{} & \HoloSegScore{8.832}{(6.639--11.83)}{4.55pt}{4.82pt}{} & \HoloSegScore{20.14}{(16.09--24.23)}{4.55pt}{4.82pt}{} & \HoloSegScore{12.44}{(10.95--15.26)}{4.55pt}{4.82pt}{} & \HoloSegScore{13.63}{(10.23--18.03)}{4.55pt}{4.82pt}{} & \HoloSegScore{20.26}{(9.812--33.12)}{4.55pt}{4.82pt}{} \\
\cline{3-11}
 &  &  & \HoloSegMetric{Dice} &  & \HoloSegScore{0.006829}{(0.002929--0.01113)}{3.85pt}{4.12pt}{} & \HoloSegScore{0.9041}{(0.8844--0.9180)}{4.55pt}{4.82pt}{} & \HoloSegScore{0.8505}{(0.8293--0.8686)}{4.55pt}{4.82pt}{} & \HoloSegScore{0.8922}{(0.8832--0.9034)}{4.55pt}{4.82pt}{} & \HoloSegScore{0.8911}{(0.8715--0.9072)}{4.55pt}{4.82pt}{} & \HoloSegScore{0.9040}{(0.8872--0.9177)}{4.55pt}{4.82pt}{} \\*
\softcline{4-4}\softcline{6-11}
\HoloSegSpan{\makecell[c]{\textbf{Internal}}}{1.20cm}{0.32cm} &  & \HoloSegSpan{\makecell[c]{right\\[-0.10ex]posterior\\[-0.10ex]superior\\[-0.10ex]segment of\\[-0.10ex]liver}}{2.04cm}{0.32cm} & \HoloSegMetric{HD95} & \raisebox{0.32cm}[0pt][0pt]{\HoloSegUnsupported} & \HoloSegScore{89.51}{(81.71--98.33)}{4.55pt}{4.82pt}{} & \HoloSegScore{10.77}{(6.270--18.13)}{4.55pt}{4.82pt}{} & \HoloSegScore{17.83}{(14.81--21.00)}{4.55pt}{4.82pt}{} & \HoloSegScore{10.90}{(8.603--13.88)}{4.55pt}{4.82pt}{} & \HoloSegScore{13.42}{(8.863--20.29)}{4.55pt}{4.82pt}{} & \HoloSegScore{8.250}{(6.491--10.23)}{4.55pt}{4.82pt}{} \\
\cline{3-11}
 &  &  & \HoloSegMetric{Dice} &  & \HoloSegScore{0.004849}{(0.0009141--0.01040)}{3.85pt}{4.12pt}{} & \HoloSegScore{0.8746}{(0.8429--0.8976)}{4.55pt}{4.82pt}{} & \HoloSegScore{0.8204}{(0.8017--0.8392)}{4.55pt}{4.82pt}{} & \HoloSegScore{0.8556}{(0.8379--0.8692)}{4.55pt}{4.82pt}{} & \HoloSegScore{0.8687}{(0.8398--0.8931)}{4.55pt}{4.82pt}{} & \HoloSegScore{0.8845}{(0.8617--0.9026)}{4.55pt}{4.82pt}{} \\*
\softcline{4-4}\softcline{6-11}
 &  & \HoloSegSpan{\makecell[c]{right\\[-0.10ex]anterior\\[-0.10ex]superior\\[-0.10ex]segment of\\[-0.10ex]liver}}{2.04cm}{0.32cm} & \HoloSegMetric{HD95} & \raisebox{0.32cm}[0pt][0pt]{\HoloSegUnsupported} & \HoloSegScore{103.7}{(95.49--111.1)}{4.55pt}{4.82pt}{} & \HoloSegScore{10.57}{(8.080--13.17)}{4.55pt}{4.82pt}{} & \HoloSegScore{19.97}{(16.64--23.79)}{4.55pt}{4.82pt}{} & \HoloSegScore{15.29}{(13.74--18.74)}{4.55pt}{4.82pt}{} & \HoloSegScore{11.37}{(8.349--14.73)}{4.55pt}{4.82pt}{} & \HoloSegScore{9.916}{(7.405--13.54)}{4.55pt}{4.82pt}{} \\
\cline{2-11}
 &  &  & \HoloSegMetric{Dice} &  & \HoloSegScore{0.009012}{(0.007278--0.01067)}{3.85pt}{4.12pt}{} & \HoloSegScore{0.9442}{(0.9393--0.9479)}{4.55pt}{4.82pt}{} & \HoloSegScore{0.6639}{(0.6493--0.6773)}{4.55pt}{4.82pt}{} & \HoloSegScore{0.8536}{(0.8337--0.8682)}{4.55pt}{4.82pt}{} & \HoloSegScore{0.8676}{(0.8601--0.8745)}{4.55pt}{4.82pt}{} & \HoloSegScore{0.8651}{(0.8570--0.8718)}{4.55pt}{4.82pt}{} \\*
\softcline{4-4}\softcline{6-11}
 &  & \HoloSegSpan{\makecell[c]{muscle}}{2.04cm}{0.32cm} & \HoloSegMetric{HD95} & \raisebox{0.32cm}[0pt][0pt]{\HoloSegUnsupported} & \HoloSegScore{466.8}{(446.4--488.7)}{4.55pt}{4.82pt}{} & \HoloSegScore{2.627}{(2.507--2.831)}{4.55pt}{4.82pt}{} & \HoloSegScore{25.29}{(24.41--26.18)}{4.55pt}{4.82pt}{} & \HoloSegScore{15.16}{(14.71--17.95)}{4.55pt}{4.82pt}{} & \HoloSegScore{17.72}{(16.62--19.07)}{4.55pt}{4.82pt}{} & \HoloSegScore{13.29}{(12.13--14.67)}{4.55pt}{4.82pt}{} \\
\cline{3-11}
 &  &  & \HoloSegMetric{Dice} &  & \HoloSegScore{0.000003231}{(0.0000001422--0.000008618)}{3.25pt}{3.52pt}{} & \HoloSegScore{0.9530}{(0.9472--0.9581)}{4.55pt}{4.82pt}{} & \HoloSegScore{0.9329}{(0.9251--0.9398)}{4.55pt}{4.82pt}{} & \HoloSegScore{0.9176}{(0.9172--0.9253)}{4.55pt}{4.82pt}{} & \HoloSegScore{0.8737}{(0.8616--0.8870)}{4.55pt}{4.82pt}{} & \HoloSegScore{0.9019}{(0.8913--0.9126)}{4.55pt}{4.82pt}{} \\*
\softcline{4-4}\softcline{6-11}
 &  & \HoloSegSpan{\makecell[c]{fat}}{2.04cm}{0.32cm} & \HoloSegMetric{HD95} & \raisebox{0.32cm}[0pt][0pt]{\HoloSegUnsupported} & \HoloSegScore{424.1}{(411.2--435.9)}{4.55pt}{4.82pt}{} & \HoloSegScore{2.352}{(2.065--2.770)}{4.55pt}{4.82pt}{} & \HoloSegScore{6.006}{(4.827--7.329)}{4.55pt}{4.82pt}{} & \HoloSegScore{3.452}{(2.171--4.842)}{4.55pt}{4.82pt}{} & \HoloSegScore{33.98}{(30.35--37.47)}{4.55pt}{4.82pt}{} & \HoloSegScore{12.01}{(10.72--13.58)}{4.55pt}{4.82pt}{} \\
\cline{3-11}
 &  &  & \HoloSegMetric{Dice} &  & \HoloSegScore{0.1121}{(0.1023--0.1223)}{4.55pt}{4.82pt}{} & \HoloSegScore{0.9130}{(0.9000--0.9252)}{4.55pt}{4.82pt}{} & \HoloSegScore{0.9089}{(0.8924--0.9226)}{4.55pt}{4.82pt}{} & \HoloSegScore{0.9082}{(0.9062--0.9346)}{4.55pt}{4.82pt}{} & \HoloSegScore{0.8677}{(0.8498--0.8839)}{4.55pt}{4.82pt}{} & \HoloSegScore{0.8838}{(0.8647--0.9009)}{4.55pt}{4.82pt}{} \\*
\softcline{4-4}\softcline{6-11}
 &  & \HoloSegSpan{\makecell[c]{abdominal\\[-0.10ex]tissue}}{2.04cm}{0.32cm} & \HoloSegMetric{HD95} & \raisebox{0.32cm}[0pt][0pt]{\HoloSegUnsupported} & \HoloSegScore{93.79}{(87.51--100.8)}{4.55pt}{4.82pt}{} & \HoloSegScore{2.463}{(2.414--2.501)}{4.55pt}{4.82pt}{} & \HoloSegScore{4.481}{(3.528--5.696)}{4.55pt}{4.82pt}{} & \HoloSegScore{2.562}{(2.358--2.799)}{4.55pt}{4.82pt}{} & \HoloSegScore{61.29}{(52.29--70.11)}{4.55pt}{4.82pt}{} & \HoloSegScore{7.783}{(5.778--10.78)}{4.55pt}{4.82pt}{} \\
\cline{3-11}
 &  &  & \HoloSegMetric{Dice} &  & \HoloSegScore{0.01913}{(0.01386--0.02495)}{4.20pt}{4.48pt}{} & \HoloSegScore{0.8406}{(0.8240--0.8550)}{4.55pt}{4.82pt}{} & \HoloSegScore{0.8088}{(0.7902--0.8271)}{4.55pt}{4.82pt}{} & \HoloSegScore{0.8281}{(0.8243--0.8390)}{4.55pt}{4.82pt}{} & \HoloSegScore{0.7647}{(0.7364--0.7870)}{4.55pt}{4.82pt}{} & \HoloSegScore{0.7541}{(0.7291--0.7754)}{4.55pt}{4.82pt}{} \\*
\softcline{4-4}\softcline{6-11}
 &  & \HoloSegSpan{\makecell[c]{mediastinal\\[-0.10ex]tissue}}{2.04cm}{0.32cm} & \HoloSegMetric{HD95} & \raisebox{0.32cm}[0pt][0pt]{\HoloSegUnsupported} & \HoloSegScore{115.5}{(104.8--125.9)}{4.55pt}{4.82pt}{} & \HoloSegScore{2.454}{(2.398--2.507)}{4.55pt}{4.82pt}{} & \HoloSegScore{4.358}{(3.688--5.157)}{4.55pt}{4.82pt}{} & \HoloSegScore{4.664}{(4.238--5.142)}{4.55pt}{4.82pt}{} & \HoloSegScore{10.64}{(8.659--13.02)}{4.55pt}{4.82pt}{} & \HoloSegScore{9.545}{(8.093--11.34)}{4.55pt}{4.82pt}{} \\
\cline{3-11}
 & \HoloSegSpan{\makecell[c]{DAP-Atlas\\[-0.10ex](AutoPETIII)}}{1.86cm}{0.32cm} &  & \HoloSegMetric{Dice} & \HoloSegScore{0.8334}{(0.8064--0.8561)}{4.55pt}{4.82pt}{} & \HoloSegScore{0.3318}{(0.3007--0.3631)}{4.55pt}{4.82pt}{} & \HoloSegScore{0.8882}{(0.8724--0.9004)}{4.55pt}{4.82pt}{} & \HoloSegScore{0.8666}{(0.8387--0.8902)}{4.55pt}{4.82pt}{} & \HoloSegScore{0.8867}{(0.8833--0.9150)}{4.55pt}{4.82pt}{} & \HoloSegScore{0.8658}{(0.8520--0.8792)}{4.55pt}{4.82pt}{} & \HoloSegScore{0.8718}{(0.8541--0.8845)}{4.55pt}{4.82pt}{} \\*
\softcline{4-11}
 &  & \HoloSegSpan{\makecell[c]{esophagus}}{2.04cm}{0.32cm} & \HoloSegMetric{HD95} & \HoloSegScore{7.785}{(4.249--13.11)}{4.55pt}{4.82pt}{} & \HoloSegScore{20.51}{(17.41--25.60)}{4.55pt}{4.82pt}{} & \HoloSegScore{4.763}{(2.058--9.639)}{4.55pt}{4.82pt}{} & \HoloSegScore{5.840}{(2.535--10.72)}{4.55pt}{4.82pt}{} & \HoloSegScore{8.665}{(5.849--13.99)}{4.55pt}{4.82pt}{} & \HoloSegScore{5.533}{(2.574--10.46)}{4.55pt}{4.82pt}{} & \HoloSegScore{7.644}{(2.317--14.78)}{4.55pt}{4.82pt}{} \\
\cline{3-11}
 &  &  & \HoloSegMetric{Dice} & \HoloSegScore{0.9558}{(0.9508--0.9599)}{4.55pt}{4.82pt}{} & \HoloSegScore{0.5807}{(0.5450--0.6148)}{4.55pt}{4.82pt}{} & \HoloSegScore{0.1405}{(0.1128--0.1707)}{4.55pt}{4.82pt}{} & \HoloSegScore{0.9612}{(0.9568--0.9652)}{4.55pt}{4.82pt}{} & \HoloSegScore{0.9418}{(0.9209--0.9448)}{4.55pt}{4.82pt}{} & \HoloSegScore{0.9587}{(0.9542--0.9628)}{4.55pt}{4.82pt}{} & \HoloSegScore{0.9592}{(0.9552--0.9626)}{4.55pt}{4.82pt}{} \\*
\softcline{4-11}
 &  & \HoloSegSpan{\makecell[c]{stomach}}{2.04cm}{0.32cm} & \HoloSegMetric{HD95} & \HoloSegScore{3.451}{(2.725--4.602)}{4.55pt}{4.82pt}{} & \HoloSegScore{23.37}{(21.81--24.92)}{4.55pt}{4.82pt}{} & \HoloSegScore{442.4}{(431.1--453.4)}{4.55pt}{4.82pt}{} & \HoloSegScore{12.69}{(2.489--32.64)}{4.55pt}{4.82pt}{} & \HoloSegScore{5.174}{(3.756--5.865)}{4.55pt}{4.82pt}{} & \HoloSegScore{3.178}{(2.596--4.019)}{4.55pt}{4.82pt}{} & \HoloSegScore{3.019}{(2.577--3.584)}{4.55pt}{4.82pt}{} \\
\cline{3-11}
 &  &  & \HoloSegMetric{Dice} & \HoloSegScore{0.8767}{(0.8629--0.8892)}{4.55pt}{4.82pt}{} & \HoloSegScore{0.5020}{(0.4746--0.5284)}{4.55pt}{4.82pt}{} & \HoloSegScore{0.9317}{(0.9264--0.9364)}{4.55pt}{4.82pt}{} & \HoloSegScore{0.9037}{(0.8927--0.9143)}{4.55pt}{4.82pt}{} & \HoloSegScore{0.8993}{(0.8836--0.9117)}{4.55pt}{4.82pt}{} & \HoloSegScore{0.9012}{(0.8903--0.9112)}{4.55pt}{4.82pt}{} & \HoloSegScore{0.8912}{(0.8794--0.9030)}{4.55pt}{4.82pt}{} \\*
\softcline{4-11}
 &  & \HoloSegSpan{\makecell[c]{small bowel}}{2.04cm}{0.32cm} & \HoloSegMetric{HD95} & \HoloSegScore{8.799}{(6.805--11.01)}{4.55pt}{4.82pt}{} & \HoloSegScore{31.53}{(26.31--39.00)}{4.55pt}{4.82pt}{} & \HoloSegScore{3.068}{(2.762--3.406)}{4.55pt}{4.82pt}{} & \HoloSegScore{13.91}{(8.500--24.46)}{4.55pt}{4.82pt}{} & \HoloSegScore{6.194}{(4.839--7.272)}{4.55pt}{4.82pt}{} & \HoloSegScore{7.498}{(6.103--9.162)}{4.55pt}{4.82pt}{} & \HoloSegScore{34.70}{(14.57--64.18)}{4.55pt}{4.82pt}{} \\
\cline{3-11}
 &  &  & \HoloSegMetric{Dice} & \HoloSegScore{0.8508}{(0.8252--0.8758)}{4.55pt}{4.82pt}{} & \HoloSegScore{0.3621}{(0.3387--0.3880)}{4.55pt}{4.82pt}{} & \HoloSegScore{0.8825}{(0.8629--0.9013)}{4.55pt}{4.82pt}{} & \HoloSegScore{0.8378}{(0.8016--0.8694)}{4.55pt}{4.82pt}{} & \HoloSegScore{0.8638}{(0.8492--0.8826)}{4.55pt}{4.82pt}{} & \HoloSegScore{0.8685}{(0.8398--0.8929)}{4.55pt}{4.82pt}{} & \HoloSegScore{0.8737}{(0.8511--0.8936)}{4.55pt}{4.82pt}{} \\*
\softcline{4-11}
 &  & \HoloSegSpan{\makecell[c]{duodenum}}{2.04cm}{0.32cm} & \HoloSegMetric{HD95} & \HoloSegScore{7.366}{(5.589--9.131)}{4.55pt}{4.82pt}{} & \HoloSegScore{28.14}{(25.37--31.42)}{4.55pt}{4.82pt}{} & \HoloSegScore{3.741}{(3.022--4.630)}{4.55pt}{4.82pt}{} & \HoloSegScore{13.48}{(6.915--24.70)}{4.55pt}{4.82pt}{} & \HoloSegScore{4.752}{(3.560--4.821)}{4.55pt}{4.82pt}{} & \HoloSegScore{5.309}{(3.678--7.542)}{4.55pt}{4.82pt}{} & \HoloSegScore{5.392}{(3.692--7.559)}{4.55pt}{4.82pt}{} \\
\hline
\pagebreak[4]
 &  &  & \HoloSegMetric{Dice} & \HoloSegScore{0.8806}{(0.8703--0.8906)}{4.55pt}{4.82pt}{} & \HoloSegScore{0.4457}{(0.4170--0.4758)}{4.55pt}{4.82pt}{} & \HoloSegScore{0.9305}{(0.9241--0.9361)}{4.55pt}{4.82pt}{} & \HoloSegScore{0.8980}{(0.8870--0.9091)}{4.55pt}{4.82pt}{} & \HoloSegScore{0.8988}{(0.8910--0.9105)}{4.55pt}{4.82pt}{} & \HoloSegScore{0.8595}{(0.8480--0.8700)}{4.55pt}{4.82pt}{} & \HoloSegScore{0.8968}{(0.8865--0.9068)}{4.55pt}{4.82pt}{} \\*
\softcline{4-11}
 &  & \HoloSegSpan{\makecell[c]{colon}}{2.04cm}{0.32cm} & \HoloSegMetric{HD95} & \HoloSegScore{14.56}{(10.51--19.00)}{4.55pt}{4.82pt}{} & \HoloSegScore{35.16}{(31.71--39.08)}{4.55pt}{4.82pt}{} & \HoloSegScore{3.751}{(3.077--4.553)}{4.55pt}{4.82pt}{} & \HoloSegScore{12.62}{(10.43--14.88)}{4.55pt}{4.82pt}{} & \HoloSegScore{5.098}{(3.280--5.356)}{4.55pt}{4.82pt}{} & \HoloSegScore{25.80}{(12.54--44.31)}{4.55pt}{4.82pt}{} & \HoloSegScore{11.13}{(9.050--13.28)}{4.55pt}{4.82pt}{} \\
\cline{3-11}
 &  &  & \HoloSegMetric{Dice} & \HoloSegScore{0.7116}{(0.6030--0.8096)}{4.55pt}{4.82pt}{} & \HoloSegScore{0.2240}{(0.1644--0.2843)}{4.55pt}{4.82pt}{} & \HoloSegScore{0.7513}{(0.6483--0.8458)}{4.55pt}{4.82pt}{} & \HoloSegScore{0.7276}{(0.6180--0.8221)}{4.55pt}{4.82pt}{} & \HoloSegScore{0.7216}{(0.6354--0.7908)}{4.55pt}{4.82pt}{} & \HoloSegScore{0.7644}{(0.6627--0.8548)}{4.55pt}{4.82pt}{} & \HoloSegScore{0.7963}{(0.6946--0.8794)}{4.55pt}{4.82pt}{} \\*
\softcline{4-11}
 &  & \HoloSegSpan{\makecell[c]{gallbladder}}{2.04cm}{0.32cm} & \HoloSegMetric{HD95} & \HoloSegScore{52.06}{(19.69--91.94)}{4.55pt}{4.82pt}{} & \HoloSegScore{45.72}{(30.71--62.92)}{4.55pt}{4.82pt}{} & \HoloSegScore{19.45}{(7.457--33.90)}{4.55pt}{4.82pt}{} & \HoloSegScore{20.94}{(8.252--37.47)}{4.55pt}{4.82pt}{} & \HoloSegScore{19.13}{(6.383--35.00)}{4.55pt}{4.82pt}{} & \HoloSegScore{18.53}{(5.304--34.10)}{4.55pt}{4.82pt}{} & \HoloSegScore{47.14}{(15.98--84.82)}{4.55pt}{4.82pt}{} \\
\cline{3-11}
 &  &  & \HoloSegMetric{Dice} & \HoloSegScore{0.9533}{(0.9497--0.9564)}{4.55pt}{4.82pt}{} & \HoloSegScore{0.7686}{(0.7593--0.7778)}{4.55pt}{4.82pt}{} & \HoloSegScore{0.9743}{(0.9731--0.9755)}{4.55pt}{4.82pt}{} & \HoloSegScore{0.9731}{(0.9720--0.9741)}{4.55pt}{4.82pt}{} & \HoloSegScore{0.9499}{(0.9453--0.9786)}{4.55pt}{4.82pt}{} & \HoloSegScore{0.9754}{(0.9742--0.9766)}{4.55pt}{4.82pt}{} & \HoloSegScore{0.9766}{(0.9753--0.9778)}{4.55pt}{4.82pt}{} \\*
\softcline{4-11}
 &  & \HoloSegSpan{\makecell[c]{liver}}{2.04cm}{0.32cm} & \HoloSegMetric{HD95} & \HoloSegScore{36.18}{(33.48--38.45)}{4.55pt}{4.82pt}{} & \HoloSegScore{22.49}{(21.61--23.34)}{4.55pt}{4.82pt}{} & \HoloSegScore{2.630}{(2.521--2.772)}{4.55pt}{4.82pt}{} & \HoloSegScore{2.685}{(2.534--2.883)}{4.55pt}{4.82pt}{} & \HoloSegScore{3.681}{(3.553--3.994)}{4.55pt}{4.82pt}{} & \HoloSegScore{2.784}{(2.530--3.078)}{4.55pt}{4.82pt}{} & \HoloSegScore{2.841}{(2.570--3.172)}{4.55pt}{4.82pt}{} \\
\cline{3-11}
 &  &  & \HoloSegMetric{Dice} & \HoloSegScore{0.8783}{(0.8414--0.9024)}{4.55pt}{4.82pt}{} & \HoloSegScore{0.3736}{(0.3276--0.4214)}{4.55pt}{4.82pt}{} & \HoloSegScore{0.9049}{(0.8885--0.9168)}{4.55pt}{4.82pt}{} & \HoloSegScore{0.9076}{(0.8739--0.9272)}{4.55pt}{4.82pt}{} & \HoloSegScore{0.8815}{(0.8702--0.9068)}{4.55pt}{4.82pt}{} & \HoloSegScore{0.9042}{(0.8762--0.9230)}{4.55pt}{4.82pt}{} & \HoloSegScore{0.9094}{(0.8857--0.9252)}{4.55pt}{4.82pt}{} \\*
\softcline{4-11}
 &  & \HoloSegSpan{\makecell[c]{pancreas}}{2.04cm}{0.32cm} & \HoloSegMetric{HD95} & \HoloSegScore{18.26}{(3.672--40.21)}{4.55pt}{4.82pt}{} & \HoloSegScore{27.17}{(22.38--33.01)}{4.55pt}{4.82pt}{} & \HoloSegScore{3.297}{(2.511--4.762)}{4.55pt}{4.82pt}{} & \HoloSegScore{4.415}{(2.587--7.261)}{4.55pt}{4.82pt}{} & \HoloSegScore{3.244}{(1.737--5.426)}{4.55pt}{4.82pt}{} & \HoloSegScore{3.941}{(2.447--6.417)}{4.55pt}{4.82pt}{} & \HoloSegScore{3.664}{(2.413--5.915)}{4.55pt}{4.82pt}{} \\
\cline{3-11}
 &  &  & \HoloSegMetric{Dice} & \HoloSegScore{0.8996}{(0.8241--0.9482)}{4.55pt}{4.82pt}{} & \HoloSegScore{0.6216}{(0.5649--0.6664)}{4.55pt}{4.82pt}{} & \HoloSegScore{0.9170}{(0.8417--0.9669)}{4.55pt}{4.82pt}{} & \HoloSegScore{0.9106}{(0.8286--0.9666)}{4.55pt}{4.82pt}{} & \HoloSegScore{0.9017}{(0.8391--0.9522)}{4.55pt}{4.82pt}{} & \HoloSegScore{0.9235}{(0.8437--0.9764)}{4.55pt}{4.82pt}{} & \HoloSegScore{0.9206}{(0.8390--0.9753)}{4.55pt}{4.82pt}{} \\*
\softcline{4-11}
 &  & \HoloSegSpan{\makecell[c]{left kidney}}{2.04cm}{0.32cm} & \HoloSegMetric{HD95} & \HoloSegScore{14.40}{(4.297--31.94)}{4.55pt}{4.82pt}{} & \HoloSegScore{64.59}{(47.99--81.97)}{4.55pt}{4.82pt}{} & \HoloSegScore{2.729}{(1.932--3.832)}{4.55pt}{4.82pt}{} & \HoloSegScore{3.872}{(3.090--4.937)}{4.55pt}{4.82pt}{} & \HoloSegScore{3.554}{(2.913--3.976)}{4.55pt}{4.82pt}{} & \HoloSegScore{2.856}{(1.718--4.516)}{4.55pt}{4.82pt}{} & \HoloSegScore{2.579}{(1.991--3.551)}{4.55pt}{4.82pt}{} \\
\cline{3-11}
 &  &  & \HoloSegMetric{Dice} & \HoloSegScore{0.9523}{(0.9486--0.9554)}{4.55pt}{4.82pt}{} & \HoloSegScore{0.6754}{(0.6641--0.6864)}{4.55pt}{4.82pt}{} & \HoloSegScore{0.9600}{(0.9578--0.9619)}{4.55pt}{4.82pt}{} & \HoloSegScore{0.9621}{(0.9591--0.9651)}{4.55pt}{4.82pt}{} & \HoloSegScore{0.9518}{(0.9410--0.9584)}{4.55pt}{4.82pt}{} & \HoloSegScore{0.9742}{(0.9694--0.9778)}{4.55pt}{4.82pt}{} & \HoloSegScore{0.9744}{(0.9713--0.9767)}{4.55pt}{4.82pt}{} \\*
\softcline{4-11}
 &  & \HoloSegSpan{\makecell[c]{right kidney}}{2.04cm}{0.32cm} & \HoloSegMetric{HD95} & \HoloSegScore{4.462}{(4.022--4.982)}{4.55pt}{4.82pt}{} & \HoloSegScore{19.74}{(16.64--25.03)}{4.55pt}{4.82pt}{} & \HoloSegScore{2.233}{(2.109--2.385)}{4.55pt}{4.82pt}{} & \HoloSegScore{3.537}{(3.000--4.014)}{4.55pt}{4.82pt}{} & \HoloSegScore{3.614}{(2.605--4.989)}{4.55pt}{4.82pt}{} & \HoloSegScore{1.817}{(1.454--2.278)}{4.55pt}{4.82pt}{} & \HoloSegScore{2.057}{(1.675--2.531)}{4.55pt}{4.82pt}{} \\
\cline{3-11}
 &  &  & \HoloSegMetric{Dice} & \HoloSegScore{0.8749}{(0.8455--0.8997)}{4.55pt}{4.82pt}{} & \HoloSegScore{0.2285}{(0.1778--0.2836)}{4.55pt}{4.82pt}{} & \HoloSegScore{0.9122}{(0.8972--0.9259)}{4.55pt}{4.82pt}{} & \HoloSegScore{0.8725}{(0.8457--0.8974)}{4.55pt}{4.82pt}{} & \HoloSegScore{0.9087}{(0.8810--0.9135)}{4.55pt}{4.82pt}{} & \HoloSegScore{0.9169}{(0.9014--0.9313)}{4.55pt}{4.82pt}{} & \HoloSegScore{0.9252}{(0.9103--0.9382)}{4.55pt}{4.82pt}{} \\*
\softcline{4-11}
 &  & \HoloSegSpan{\makecell[c]{urinary\\[-0.10ex]bladder}}{2.04cm}{0.32cm} & \HoloSegMetric{HD95} & \HoloSegScore{9.717}{(4.621--15.97)}{4.55pt}{4.82pt}{} & \HoloSegScore{39.48}{(34.13--45.19)}{4.55pt}{4.82pt}{} & \HoloSegScore{77.13}{(25.85--136.6)}{4.55pt}{4.82pt}{} & \HoloSegScore{5.728}{(4.047--7.749)}{4.55pt}{4.82pt}{} & \HoloSegScore{8.880}{(7.783--9.757)}{4.55pt}{4.82pt}{} & \HoloSegScore{15.00}{(4.148--30.97)}{4.55pt}{4.82pt}{} & \HoloSegScore{4.147}{(3.354--5.022)}{4.55pt}{4.82pt}{} \\
\cline{3-11}
 &  &  & \HoloSegMetric{Dice} &  & \HoloSegScore{0.0000}{(0.0000--0.0000)}{4.55pt}{4.82pt}{} & \HoloSegScore{0.4151}{(0.2881--0.5385)}{4.55pt}{4.82pt}{} & \HoloSegScore{0.0000}{(0.0000--0.0000)}{4.55pt}{4.82pt}{} & \HoloSegScore{0.08021}{(0.07733--0.09382)}{4.20pt}{4.48pt}{} & \HoloSegScore{0.08758}{(0.04011--0.1419)}{4.20pt}{4.48pt}{} & \HoloSegScore{0.2624}{(0.1761--0.3503)}{4.55pt}{4.82pt}{} \\*
\softcline{4-4}\softcline{6-11}
 &  & \HoloSegSpan{\makecell[c]{gonad}}{2.04cm}{0.32cm} & \HoloSegMetric{HD95} & \raisebox{0.32cm}[0pt][0pt]{\HoloSegUnsupported} & \HoloSegScore{662.0}{(546.4--766.3)}{4.55pt}{4.82pt}{} & \HoloSegScore{60.44}{(14.06--137.5)}{4.55pt}{4.82pt}{} & \HoloSegScore{126.7}{(116.4--136.6)}{4.55pt}{4.82pt}{} & \HoloSegScore{62.12}{(51.61--72.65)}{4.55pt}{4.82pt}{} & \HoloSegScore{270.4}{(158.5--392.1)}{4.55pt}{4.82pt}{} & \HoloSegScore{99.54}{(24.87--200.8)}{4.55pt}{4.82pt}{} \\
\cline{3-11}
 &  &  & \HoloSegMetric{Dice} & \HoloSegScore{0.5521}{(0.5009--0.6028)}{4.55pt}{4.82pt}{} & \HoloSegScore{0.05424}{(0.02490--0.09018)}{4.20pt}{4.48pt}{} & \HoloSegScore{0.8669}{(0.8369--0.8920)}{4.55pt}{4.82pt}{} & \HoloSegScore{0.6782}{(0.6143--0.7346)}{4.55pt}{4.82pt}{} & \HoloSegScore{0.8266}{(0.7815--0.8470)}{4.55pt}{4.82pt}{} & \HoloSegScore{0.8233}{(0.8008--0.8445)}{4.55pt}{4.82pt}{} & \HoloSegScore{0.7919}{(0.7585--0.8231)}{4.55pt}{4.82pt}{} \\*
\softcline{4-11}
 &  & \HoloSegSpan{\makecell[c]{prostate}}{2.04cm}{0.32cm} & \HoloSegMetric{HD95} & \HoloSegScore{38.65}{(35.88--40.70)}{4.55pt}{4.82pt}{} & \HoloSegScore{107.4}{(50.62--187.2)}{4.55pt}{4.82pt}{} & \HoloSegScore{3.131}{(2.783--3.517)}{4.55pt}{4.82pt}{} & \HoloSegScore{8.583}{(6.780--10.48)}{4.55pt}{4.82pt}{} & \HoloSegScore{4.435}{(3.701--5.808)}{4.55pt}{4.82pt}{} & \HoloSegScore{4.100}{(3.547--4.693)}{4.55pt}{4.82pt}{} & \HoloSegScore{8.998}{(4.130--17.98)}{4.55pt}{4.82pt}{} \\
\cline{3-11}
 &  &  & \HoloSegMetric{Dice} &  & \HoloSegScore{0.03835}{(0.0006883--0.09554)}{3.85pt}{4.12pt}{} & \HoloSegScore{0.5232}{(0.2860--0.7446)}{4.55pt}{4.82pt}{} & \HoloSegScore{0.3348}{(0.1187--0.5857)}{4.55pt}{4.82pt}{} & \HoloSegScore{0.4204}{(0.2071--0.6275)}{4.55pt}{4.82pt}{} & \HoloSegScore{0.4032}{(0.1875--0.6289)}{4.55pt}{4.82pt}{} & \HoloSegScore{0.4939}{(0.2622--0.6914)}{4.55pt}{4.82pt}{} \\*
\softcline{4-4}\softcline{6-11}
\HoloSegSpan{\makecell[c]{\textbf{Internal}}}{1.20cm}{0.32cm} & \HoloSegSpan{\makecell[c]{DAP-Atlas\\[-0.10ex](AutoPETIII)}}{1.86cm}{0.32cm} & \HoloSegSpan{\makecell[c]{uterocervix}}{2.04cm}{0.32cm} & \HoloSegMetric{HD95} & \raisebox{0.32cm}[0pt][0pt]{\HoloSegUnsupported} & \HoloSegScore{87.91}{(60.61--116.0)}{4.55pt}{4.82pt}{} & \HoloSegScore{13.31}{(5.590--23.16)}{4.55pt}{4.82pt}{} & \HoloSegScore{28.83}{(13.92--45.34)}{4.55pt}{4.82pt}{} & \HoloSegScore{13.64}{(7.953--19.65)}{4.55pt}{4.82pt}{} & \HoloSegScore{10.13}{(5.014--15.69)}{4.55pt}{4.82pt}{} & \HoloSegScore{30.20}{(9.509--62.70)}{4.55pt}{4.82pt}{} \\
\cline{3-11}
 &  &  & \HoloSegMetric{Dice} &  & \HoloSegScore{0.03145}{(0.01007--0.05463)}{4.20pt}{4.48pt}{} & \HoloSegScore{0.7764}{(0.7290--0.8254)}{4.55pt}{4.82pt}{} & \HoloSegScore{0.5552}{(0.3767--0.6999)}{4.55pt}{4.82pt}{} & \HoloSegScore{0.6871}{(0.6111--0.7341)}{4.55pt}{4.82pt}{} & \HoloSegScore{0.6952}{(0.6120--0.7699)}{4.55pt}{4.82pt}{} & \HoloSegScore{0.6916}{(0.6188--0.7614)}{4.55pt}{4.82pt}{} \\*
\softcline{4-4}\softcline{6-11}
 &  & \HoloSegSpan{\makecell[c]{uterus}}{2.04cm}{0.32cm} & \HoloSegMetric{HD95} & \raisebox{0.32cm}[0pt][0pt]{\HoloSegUnsupported} & \HoloSegScore{83.43}{(63.24--103.3)}{4.55pt}{4.82pt}{} & \HoloSegScore{6.711}{(4.551--9.036)}{4.55pt}{4.82pt}{} & \HoloSegScore{19.73}{(13.89--27.05)}{4.55pt}{4.82pt}{} & \HoloSegScore{17.16}{(11.97--23.77)}{4.55pt}{4.82pt}{} & \HoloSegScore{70.74}{(8.865--185.0)}{4.55pt}{4.82pt}{} & \HoloSegScore{160.7}{(64.95--273.2)}{4.55pt}{4.82pt}{} \\
\cline{3-11}
 &  &  & \HoloSegMetric{Dice} &  & \HoloSegScore{0.000007628}{(0.0000--0.00002248)}{3.85pt}{4.12pt}{} & \HoloSegScore{0.6123}{(0.4964--0.7146)}{4.55pt}{4.82pt}{} & \HoloSegScore{0.3997}{(0.2744--0.5219)}{4.55pt}{4.82pt}{} & \HoloSegScore{0.4434}{(0.3568--0.5258)}{4.55pt}{4.82pt}{} & \HoloSegScore{0.5491}{(0.4311--0.6567)}{4.55pt}{4.82pt}{} & \HoloSegScore{0.5137}{(0.3931--0.6339)}{4.55pt}{4.82pt}{} \\*
\softcline{4-4}\softcline{6-11}
 &  & \HoloSegSpan{\makecell[c]{left breast}}{2.04cm}{0.32cm} & \HoloSegMetric{HD95} & \raisebox{0.32cm}[0pt][0pt]{\HoloSegUnsupported} & \HoloSegScore{234.2}{(184.0--291.2)}{4.55pt}{4.82pt}{} & \HoloSegScore{74.99}{(23.99--142.6)}{4.55pt}{4.82pt}{} & \HoloSegScore{238.1}{(168.4--308.6)}{4.55pt}{4.82pt}{} & \HoloSegScore{76.49}{(24.82--134.2)}{4.55pt}{4.82pt}{} & \HoloSegScore{84.46}{(27.78--151.1)}{4.55pt}{4.82pt}{} & \HoloSegScore{95.46}{(28.55--166.3)}{4.55pt}{4.82pt}{} \\
\cline{3-11}
 &  &  & \HoloSegMetric{Dice} &  & \HoloSegScore{0.00001726}{(0.0000--0.00005052)}{3.85pt}{4.12pt}{} & \HoloSegScore{0.5869}{(0.4758--0.6875)}{4.55pt}{4.82pt}{} & \HoloSegScore{0.4356}{(0.3264--0.5410)}{4.55pt}{4.82pt}{} & \HoloSegScore{0.5751}{(0.5716--0.5755)}{4.55pt}{4.82pt}{} & \HoloSegScore{0.5866}{(0.4781--0.6790)}{4.55pt}{4.82pt}{} & \HoloSegScore{0.5813}{(0.4722--0.6745)}{4.55pt}{4.82pt}{} \\*
\softcline{4-4}\softcline{6-11}
 &  & \HoloSegSpan{\makecell[c]{right breast}}{2.04cm}{0.32cm} & \HoloSegMetric{HD95} & \raisebox{0.32cm}[0pt][0pt]{\HoloSegUnsupported} & \HoloSegScore{225.7}{(184.4--279.7)}{4.55pt}{4.82pt}{} & \HoloSegScore{63.03}{(15.06--123.3)}{4.55pt}{4.82pt}{} & \HoloSegScore{133.3}{(77.95--197.3)}{4.55pt}{4.82pt}{} & \HoloSegScore{73.43}{(28.16--129.5)}{4.55pt}{4.82pt}{} & \HoloSegScore{91.85}{(34.08--150.2)}{4.55pt}{4.82pt}{} & \HoloSegScore{82.47}{(31.89--137.1)}{4.55pt}{4.82pt}{} \\
\cline{3-11}
 &  &  & \HoloSegMetric{Dice} &  & \HoloSegScore{0.003224}{(0.001240--0.005448)}{3.85pt}{4.12pt}{} & \HoloSegScore{0.9183}{(0.9096--0.9257)}{4.55pt}{4.82pt}{} & \HoloSegScore{0.9117}{(0.9025--0.9211)}{4.55pt}{4.82pt}{} & \HoloSegScore{0.9088}{(0.8975--0.9179)}{4.55pt}{4.82pt}{} & \HoloSegScore{0.8165}{(0.8012--0.8312)}{4.55pt}{4.82pt}{} & \HoloSegScore{0.8859}{(0.8767--0.8949)}{4.55pt}{4.82pt}{} \\*
\softcline{4-4}\softcline{6-11}
 &  & \HoloSegSpan{\makecell[c]{spinal canal}}{2.04cm}{0.32cm} & \HoloSegMetric{HD95} & \raisebox{0.32cm}[0pt][0pt]{\HoloSegUnsupported} & \HoloSegScore{239.9}{(200.4--284.4)}{4.55pt}{4.82pt}{} & \HoloSegScore{4.027}{(2.050--6.332)}{4.55pt}{4.82pt}{} & \HoloSegScore{19.81}{(12.45--28.53)}{4.55pt}{4.82pt}{} & \HoloSegScore{4.881}{(2.757--6.233)}{4.55pt}{4.82pt}{} & \HoloSegScore{83.49}{(74.82--92.87)}{4.55pt}{4.82pt}{} & \HoloSegScore{34.16}{(24.18--44.81)}{4.55pt}{4.82pt}{} \\
\cline{3-11}
 &  &  & \HoloSegMetric{Dice} & \HoloSegScore{0.9400}{(0.9283--0.9506)}{4.55pt}{4.82pt}{} & \HoloSegScore{0.6182}{(0.5582--0.6695)}{4.55pt}{4.82pt}{} & \HoloSegScore{0.9676}{(0.9623--0.9722)}{4.55pt}{4.82pt}{} & \HoloSegScore{0.9737}{(0.9706--0.9765)}{4.55pt}{4.82pt}{} & \HoloSegScore{0.9694}{(0.9648--0.9705)}{4.55pt}{4.82pt}{} & \HoloSegScore{0.9609}{(0.9556--0.9662)}{4.55pt}{4.82pt}{} & \HoloSegScore{0.9643}{(0.9575--0.9700)}{4.55pt}{4.82pt}{} \\*
\softcline{4-11}
 &  & \HoloSegSpan{\makecell[c]{brain}}{2.04cm}{0.32cm} & \HoloSegMetric{HD95} & \HoloSegScore{16.89}{(6.629--32.19)}{4.55pt}{4.82pt}{} & \HoloSegScore{31.85}{(28.54--35.59)}{4.55pt}{4.82pt}{} & \HoloSegScore{3.190}{(2.786--3.623)}{4.55pt}{4.82pt}{} & \HoloSegScore{2.507}{(2.309--2.747)}{4.55pt}{4.82pt}{} & \HoloSegScore{3.713}{(3.205--4.631)}{4.55pt}{4.82pt}{} & \HoloSegScore{196.0}{(115.2--279.2)}{4.55pt}{4.82pt}{} & \HoloSegScore{12.58}{(3.227--39.19)}{4.55pt}{4.82pt}{} \\
\cline{3-11}
 &  &  & \HoloSegMetric{Dice} & \HoloSegScore{0.9499}{(0.9339--0.9613)}{4.55pt}{4.82pt}{} & \HoloSegScore{0.6603}{(0.6223--0.6907)}{4.55pt}{4.82pt}{} & \HoloSegScore{0.9418}{(0.9306--0.9510)}{4.55pt}{4.82pt}{} & \HoloSegScore{0.9718}{(0.9640--0.9773)}{4.55pt}{4.82pt}{} & \HoloSegScore{0.9442}{(0.9223--0.9583)}{4.55pt}{4.82pt}{} & \HoloSegScore{0.9692}{(0.9600--0.9751)}{4.55pt}{4.82pt}{} & \HoloSegScore{0.9691}{(0.9579--0.9772)}{4.55pt}{4.82pt}{} \\*
\softcline{4-11}
 &  & \HoloSegSpan{\makecell[c]{spleen}}{2.04cm}{0.32cm} & \HoloSegMetric{HD95} & \HoloSegScore{21.75}{(16.10--27.39)}{4.55pt}{4.82pt}{} & \HoloSegScore{21.85}{(18.92--26.96)}{4.55pt}{4.82pt}{} & \HoloSegScore{256.0}{(195.7--307.9)}{4.55pt}{4.82pt}{} & \HoloSegScore{1.332}{(0.9155--2.103)}{4.55pt}{4.82pt}{} & \HoloSegScore{4.887}{(4.337--6.546)}{4.55pt}{4.82pt}{} & \HoloSegScore{2.408}{(1.113--4.338)}{4.55pt}{4.82pt}{} & \HoloSegScore{1.910}{(1.040--3.494)}{4.55pt}{4.82pt}{} \\
\cline{3-11}
 &  &  & \HoloSegMetric{Dice} & \HoloSegScore{0.8327}{(0.8116--0.8518)}{4.55pt}{4.82pt}{} & \HoloSegScore{0.1565}{(0.1167--0.1958)}{4.55pt}{4.82pt}{} & \HoloSegScore{0.8206}{(0.7986--0.8381)}{4.55pt}{4.82pt}{} & \HoloSegScore{0.8887}{(0.8674--0.9071)}{4.55pt}{4.82pt}{} & \HoloSegScore{0.8685}{(0.8336--0.8875)}{4.55pt}{4.82pt}{} & \HoloSegScore{0.8702}{(0.8517--0.8859)}{4.55pt}{4.82pt}{} & \HoloSegScore{0.8766}{(0.8611--0.8905)}{4.55pt}{4.82pt}{} \\*
\softcline{4-11}
 &  & \HoloSegSpan{\makecell[c]{left adrenal\\[-0.10ex]gland}}{2.04cm}{0.32cm} & \HoloSegMetric{HD95} & \HoloSegScore{3.606}{(2.626--4.746)}{4.55pt}{4.82pt}{} & \HoloSegScore{24.79}{(21.18--29.10)}{4.55pt}{4.82pt}{} & \HoloSegScore{25.73}{(2.279--60.62)}{4.55pt}{4.82pt}{} & \HoloSegScore{2.669}{(1.674--3.914)}{4.55pt}{4.82pt}{} & \HoloSegScore{3.688}{(3.646--4.524)}{4.55pt}{4.82pt}{} & \HoloSegScore{2.196}{(1.684--2.849)}{4.55pt}{4.82pt}{} & \HoloSegScore{1.970}{(1.358--2.897)}{4.55pt}{4.82pt}{} \\
\cline{3-11}
 &  &  & \HoloSegMetric{Dice} & \HoloSegScore{0.7753}{(0.7159--0.8191)}{4.55pt}{4.82pt}{} & \HoloSegScore{0.1912}{(0.1523--0.2289)}{4.55pt}{4.82pt}{} & \HoloSegScore{0.7763}{(0.7201--0.8211)}{4.55pt}{4.82pt}{} & \HoloSegScore{0.8503}{(0.8003--0.8921)}{4.55pt}{4.82pt}{} & \HoloSegScore{0.8419}{(0.8086--0.8763)}{4.55pt}{4.82pt}{} & \HoloSegScore{0.8194}{(0.7646--0.8626)}{4.55pt}{4.82pt}{} & \HoloSegScore{0.8461}{(0.7950--0.8816)}{4.55pt}{4.82pt}{} \\*
\softcline{4-11}
 &  & \HoloSegSpan{\makecell[c]{right\\[-0.10ex]adrenal\\[-0.10ex]gland}}{2.04cm}{0.32cm} & \HoloSegMetric{HD95} & \HoloSegScore{9.532}{(2.948--22.14)}{4.55pt}{4.82pt}{} & \HoloSegScore{20.92}{(18.48--23.75)}{4.55pt}{4.82pt}{} & \HoloSegScore{2.998}{(2.077--4.106)}{4.55pt}{4.82pt}{} & \HoloSegScore{2.036}{(1.403--2.885)}{4.55pt}{4.82pt}{} & \HoloSegScore{6.361}{(6.070--7.654)}{4.55pt}{4.82pt}{} & \HoloSegScore{4.137}{(2.287--6.342)}{4.55pt}{4.82pt}{} & \HoloSegScore{6.709}{(2.144--12.68)}{4.55pt}{4.82pt}{} \\
\cline{3-11}
 &  &  & \HoloSegMetric{Dice} &  & \HoloSegScore{0.0000}{(0.0000--0.0000)}{4.55pt}{4.82pt}{} & \HoloSegScore{0.6797}{(0.5567--0.7816)}{4.55pt}{4.82pt}{} & \HoloSegScore{0.6112}{(0.5027--0.7127)}{4.55pt}{4.82pt}{} & \HoloSegScore{0.6586}{(0.5705--0.7366)}{4.55pt}{4.82pt}{} & \HoloSegScore{0.6879}{(0.5831--0.7820)}{4.55pt}{4.82pt}{} & \HoloSegScore{0.7009}{(0.5917--0.7938)}{4.55pt}{4.82pt}{} \\*
\softcline{4-4}\softcline{6-11}
 &  & \HoloSegSpan{\makecell[c]{left thyroid}}{2.04cm}{0.32cm} & \HoloSegMetric{HD95} & \raisebox{0.32cm}[0pt][0pt]{\HoloSegUnsupported} & \HoloSegScore{292.4}{(267.2--317.5)}{4.55pt}{4.82pt}{} & \HoloSegScore{76.53}{(18.33--155.6)}{4.55pt}{4.82pt}{} & \HoloSegScore{15.09}{(6.298--27.55)}{4.55pt}{4.82pt}{} & \HoloSegScore{13.83}{(5.222--24.32)}{4.55pt}{4.82pt}{} & \HoloSegScore{12.40}{(3.720--24.98)}{4.55pt}{4.82pt}{} & \HoloSegScore{12.10}{(3.305--25.10)}{4.55pt}{4.82pt}{} \\
\hline
\pagebreak[4]
 &  &  & \HoloSegMetric{Dice} &  & \HoloSegScore{0.0000}{(0.0000--0.0000)}{4.55pt}{4.82pt}{} & \HoloSegScore{0.7590}{(0.6559--0.8451)}{4.55pt}{4.82pt}{} & \HoloSegScore{0.7041}{(0.6002--0.7992)}{4.55pt}{4.82pt}{} & \HoloSegScore{0.7506}{(0.7306--0.7707)}{4.55pt}{4.82pt}{} & \HoloSegScore{0.7456}{(0.6431--0.8304)}{4.55pt}{4.82pt}{} & \HoloSegScore{0.7217}{(0.6104--0.8212)}{4.55pt}{4.82pt}{} \\*
\softcline{4-4}\softcline{6-11}
 &  & \HoloSegSpan{\makecell[c]{right\\[-0.10ex]thyroid}}{2.04cm}{0.32cm} & \HoloSegMetric{HD95} & \raisebox{0.32cm}[0pt][0pt]{\HoloSegUnsupported} & \HoloSegScore{281.9}{(271.3--294.9)}{4.55pt}{4.82pt}{} & \HoloSegScore{17.40}{(6.194--31.19)}{4.55pt}{4.82pt}{} & \HoloSegScore{11.56}{(4.541--21.11)}{4.55pt}{4.82pt}{} & \HoloSegScore{11.57}{(5.551--20.82)}{4.55pt}{4.82pt}{} & \HoloSegScore{7.794}{(3.159--15.42)}{4.55pt}{4.82pt}{} & \HoloSegScore{10.30}{(2.984--20.29)}{4.55pt}{4.82pt}{} \\
\cline{3-11}
 &  &  & \HoloSegMetric{Dice} &  & \HoloSegScore{0.0000}{(0.0000--0.0000)}{4.55pt}{4.82pt}{} & \HoloSegScore{0.4088}{(0.2787--0.5439)}{4.55pt}{4.82pt}{} & \HoloSegScore{0.0000}{(0.0000--0.0000)}{4.55pt}{4.82pt}{} & \HoloSegScore{0.4017}{(0.3930--0.4019)}{4.55pt}{4.82pt}{} & \HoloSegScore{0.3794}{(0.2324--0.5277)}{4.55pt}{4.82pt}{} & \HoloSegScore{0.3311}{(0.1994--0.4529)}{4.55pt}{4.82pt}{} \\*
\softcline{4-4}\softcline{6-11}
 &  & \HoloSegSpan{\makecell[c]{thymus}}{2.04cm}{0.32cm} & \HoloSegMetric{HD95} & \raisebox{0.32cm}[0pt][0pt]{\HoloSegUnsupported} & \HoloSegScore{180.3}{(163.7--194.6)}{4.55pt}{4.82pt}{} & \HoloSegScore{79.16}{(4.618--191.4)}{4.55pt}{4.82pt}{} & \HoloSegScore{--}{(--\,--)}{4.55pt}{4.82pt}{} & \HoloSegScore{14.74}{(8.039--25.18)}{4.55pt}{4.82pt}{} & \HoloSegScore{10.80}{(3.860--21.04)}{4.55pt}{4.82pt}{} & \HoloSegScore{23.49}{(15.73--31.70)}{4.55pt}{4.82pt}{} \\
\cline{3-11}
 &  &  & \HoloSegMetric{Dice} & \HoloSegScore{0.9250}{(0.9198--0.9295)}{4.55pt}{4.82pt}{} & \HoloSegScore{0.7879}{(0.7744--0.8016)}{4.55pt}{4.82pt}{} & \HoloSegScore{0.9609}{(0.9585--0.9630)}{4.55pt}{4.82pt}{} & \HoloSegScore{0.9508}{(0.9471--0.9540)}{4.55pt}{4.82pt}{} & \HoloSegScore{0.9466}{(0.9355--0.9490)}{4.55pt}{4.82pt}{} & \HoloSegScore{0.9371}{(0.9325--0.9412)}{4.55pt}{4.82pt}{} & \HoloSegScore{0.9459}{(0.9427--0.9490)}{4.55pt}{4.82pt}{} \\*
\softcline{4-11}
 &  & \HoloSegSpan{\makecell[c]{left gluteus\\[-0.10ex]maximus}}{2.04cm}{0.32cm} & \HoloSegMetric{HD95} & \HoloSegScore{52.42}{(19.13--94.62)}{4.55pt}{4.82pt}{} & \HoloSegScore{15.73}{(13.63--18.54)}{4.55pt}{4.82pt}{} & \HoloSegScore{2.321}{(2.137--2.524)}{4.55pt}{4.82pt}{} & \HoloSegScore{3.109}{(2.695--3.639)}{4.55pt}{4.82pt}{} & \HoloSegScore{2.885}{(2.551--3.353)}{4.55pt}{4.82pt}{} & \HoloSegScore{28.83}{(16.33--43.83)}{4.55pt}{4.82pt}{} & \HoloSegScore{3.266}{(2.992--3.539)}{4.55pt}{4.82pt}{} \\
\cline{3-11}
 &  &  & \HoloSegMetric{Dice} & \HoloSegScore{0.9264}{(0.9200--0.9324)}{4.55pt}{4.82pt}{} & \HoloSegScore{0.7849}{(0.7730--0.7969)}{4.55pt}{4.82pt}{} & \HoloSegScore{0.9625}{(0.9583--0.9659)}{4.55pt}{4.82pt}{} & \HoloSegScore{0.9420}{(0.9370--0.9471)}{4.55pt}{4.82pt}{} & \HoloSegScore{0.9555}{(0.9533--0.9578)}{4.55pt}{4.82pt}{} & \HoloSegScore{0.9376}{(0.9318--0.9423)}{4.55pt}{4.82pt}{} & \HoloSegScore{0.9485}{(0.9425--0.9533)}{4.55pt}{4.82pt}{} \\*
\softcline{4-11}
 &  & \HoloSegSpan{\makecell[c]{right\\[-0.10ex]gluteus\\[-0.10ex]maximus}}{2.04cm}{0.32cm} & \HoloSegMetric{HD95} & \HoloSegScore{38.56}{(11.48--72.16)}{4.55pt}{4.82pt}{} & \HoloSegScore{17.48}{(14.84--21.63)}{4.55pt}{4.82pt}{} & \HoloSegScore{2.969}{(2.368--3.863)}{4.55pt}{4.82pt}{} & \HoloSegScore{3.866}{(3.265--4.639)}{4.55pt}{4.82pt}{} & \HoloSegScore{3.120}{(2.475--3.998)}{4.55pt}{4.82pt}{} & \HoloSegScore{5.334}{(4.277--6.863)}{4.55pt}{4.82pt}{} & \HoloSegScore{3.443}{(2.771--4.511)}{4.55pt}{4.82pt}{} \\
\cline{3-11}
 &  &  & \HoloSegMetric{Dice} & \HoloSegScore{0.8486}{(0.8331--0.8635)}{4.55pt}{4.82pt}{} & \HoloSegScore{0.7093}{(0.6893--0.7272)}{4.55pt}{4.82pt}{} & \HoloSegScore{0.9603}{(0.9584--0.9620)}{4.55pt}{4.82pt}{} & \HoloSegScore{0.9423}{(0.9393--0.9450)}{4.55pt}{4.82pt}{} & \HoloSegScore{0.9588}{(0.9562--0.9734)}{4.55pt}{4.82pt}{} & \HoloSegScore{0.9059}{(0.9029--0.9089)}{4.55pt}{4.82pt}{} & \HoloSegScore{0.9358}{(0.9329--0.9386)}{4.55pt}{4.82pt}{} \\*
\softcline{4-11}
 &  & \HoloSegSpan{\makecell[c]{left gluteus\\[-0.10ex]medius}}{2.04cm}{0.32cm} & \HoloSegMetric{HD95} & \HoloSegScore{63.75}{(62.57--64.81)}{4.55pt}{4.82pt}{} & \HoloSegScore{22.34}{(17.00--29.16)}{4.55pt}{4.82pt}{} & \HoloSegScore{19.92}{(2.062--55.53)}{4.55pt}{4.82pt}{} & \HoloSegScore{2.761}{(2.573--2.964)}{4.55pt}{4.82pt}{} & \HoloSegScore{6.383}{(6.137--6.401)}{4.55pt}{4.82pt}{} & \HoloSegScore{4.688}{(4.360--5.045)}{4.55pt}{4.82pt}{} & \HoloSegScore{3.162}{(2.953--3.388)}{4.55pt}{4.82pt}{} \\
\cline{3-11}
 &  &  & \HoloSegMetric{Dice} & \HoloSegScore{0.9104}{(0.9068--0.9141)}{4.55pt}{4.82pt}{} & \HoloSegScore{0.7320}{(0.7197--0.7438)}{4.55pt}{4.82pt}{} & \HoloSegScore{0.9612}{(0.9593--0.9631)}{4.55pt}{4.82pt}{} & \HoloSegScore{0.9379}{(0.9351--0.9406)}{4.55pt}{4.82pt}{} & \HoloSegScore{0.9368}{(0.9342--0.9491)}{4.55pt}{4.82pt}{} & \HoloSegScore{0.9171}{(0.9139--0.9206)}{4.55pt}{4.82pt}{} & \HoloSegScore{0.9345}{(0.9303--0.9382)}{4.55pt}{4.82pt}{} \\*
\softcline{4-11}
 &  & \HoloSegSpan{\makecell[c]{right\\[-0.10ex]gluteus\\[-0.10ex]medius}}{2.04cm}{0.32cm} & \HoloSegMetric{HD95} & \HoloSegScore{29.17}{(23.93--34.43)}{4.55pt}{4.82pt}{} & \HoloSegScore{14.71}{(13.63--16.25)}{4.55pt}{4.82pt}{} & \HoloSegScore{1.985}{(1.869--2.118)}{4.55pt}{4.82pt}{} & \HoloSegScore{3.244}{(3.005--3.515)}{4.55pt}{4.82pt}{} & \HoloSegScore{3.275}{(1.918--5.110)}{4.55pt}{4.82pt}{} & \HoloSegScore{4.203}{(3.943--4.504)}{4.55pt}{4.82pt}{} & \HoloSegScore{3.197}{(2.923--3.515)}{4.55pt}{4.82pt}{} \\
\cline{3-11}
 &  &  & \HoloSegMetric{Dice} & \HoloSegScore{0.8492}{(0.8425--0.8564)}{4.55pt}{4.82pt}{} & \HoloSegScore{0.4525}{(0.3697--0.5208)}{4.55pt}{4.82pt}{} & \HoloSegScore{0.8883}{(0.8786--0.8983)}{4.55pt}{4.82pt}{} & \HoloSegScore{0.9076}{(0.9023--0.9125)}{4.55pt}{4.82pt}{} & \HoloSegScore{0.8840}{(0.8699--0.8871)}{4.55pt}{4.82pt}{} & \HoloSegScore{0.8862}{(0.8771--0.8948)}{4.55pt}{4.82pt}{} & \HoloSegScore{0.8969}{(0.8905--0.9031)}{4.55pt}{4.82pt}{} \\*
\softcline{4-11}
 &  & \HoloSegSpan{\makecell[c]{left gluteus\\[-0.10ex]minimus}}{2.04cm}{0.32cm} & \HoloSegMetric{HD95} & \HoloSegScore{27.89}{(5.032--61.98)}{4.55pt}{4.82pt}{} & \HoloSegScore{50.43}{(28.62--75.72)}{4.55pt}{4.82pt}{} & \HoloSegScore{455.1}{(399.0--496.5)}{4.55pt}{4.82pt}{} & \HoloSegScore{2.900}{(2.587--3.284)}{4.55pt}{4.82pt}{} & \HoloSegScore{4.596}{(3.597--6.038)}{4.55pt}{4.82pt}{} & \HoloSegScore{3.707}{(3.355--4.079)}{4.55pt}{4.82pt}{} & \HoloSegScore{2.777}{(2.581--2.975)}{4.55pt}{4.82pt}{} \\
\cline{3-11}
 &  &  & \HoloSegMetric{Dice} & \HoloSegScore{0.8741}{(0.8671--0.8807)}{4.55pt}{4.82pt}{} & \HoloSegScore{0.4653}{(0.3990--0.5292)}{4.55pt}{4.82pt}{} & \HoloSegScore{0.8674}{(0.8573--0.8787)}{4.55pt}{4.82pt}{} & \HoloSegScore{0.9070}{(0.8997--0.9141)}{4.55pt}{4.82pt}{} & \HoloSegScore{0.8920}{(0.8786--0.9092)}{4.55pt}{4.82pt}{} & \HoloSegScore{0.8850}{(0.8765--0.8930)}{4.55pt}{4.82pt}{} & \HoloSegScore{0.8626}{(0.8516--0.8731)}{4.55pt}{4.82pt}{} \\*
\softcline{4-11}
 &  & \HoloSegSpan{\makecell[c]{right\\[-0.10ex]gluteus\\[-0.10ex]minimus}}{2.04cm}{0.32cm} & \HoloSegMetric{HD95} & \HoloSegScore{5.227}{(4.863--5.620)}{4.55pt}{4.82pt}{} & \HoloSegScore{44.08}{(24.80--68.70)}{4.55pt}{4.82pt}{} & \HoloSegScore{482.4}{(439.9--516.5)}{4.55pt}{4.82pt}{} & \HoloSegScore{2.466}{(2.285--2.645)}{4.55pt}{4.82pt}{} & \HoloSegScore{4.538}{(3.697--5.966)}{4.55pt}{4.82pt}{} & \HoloSegScore{3.244}{(2.914--3.667)}{4.55pt}{4.82pt}{} & \HoloSegScore{4.257}{(3.828--4.724)}{4.55pt}{4.82pt}{} \\
\cline{3-11}
 &  &  & \HoloSegMetric{Dice} & \HoloSegScore{0.9377}{(0.9340--0.9411)}{4.55pt}{4.82pt}{} & \HoloSegScore{0.5615}{(0.5022--0.6153)}{4.55pt}{4.82pt}{} & \HoloSegScore{0.9429}{(0.9383--0.9471)}{4.55pt}{4.82pt}{} & \HoloSegScore{0.9575}{(0.9538--0.9607)}{4.55pt}{4.82pt}{} & \HoloSegScore{0.9404}{(0.9368--0.9452)}{4.55pt}{4.82pt}{} & \HoloSegScore{0.9434}{(0.9393--0.9471)}{4.55pt}{4.82pt}{} & \HoloSegScore{0.9319}{(0.9282--0.9356)}{4.55pt}{4.82pt}{} \\*
\softcline{4-11}
 &  & \HoloSegSpan{\makecell[c]{left\\[-0.10ex]iliopsoas}}{2.04cm}{0.32cm} & \HoloSegMetric{HD95} & \HoloSegScore{3.045}{(2.478--4.041)}{4.55pt}{4.82pt}{} & \HoloSegScore{31.13}{(22.53--40.47)}{4.55pt}{4.82pt}{} & \HoloSegScore{2.107}{(1.977--2.267)}{4.55pt}{4.82pt}{} & \HoloSegScore{1.792}{(1.559--2.140)}{4.55pt}{4.82pt}{} & \HoloSegScore{4.784}{(4.415--7.069)}{4.55pt}{4.82pt}{} & \HoloSegScore{4.925}{(2.706--8.040)}{4.55pt}{4.82pt}{} & \HoloSegScore{9.488}{(5.217--16.23)}{4.55pt}{4.82pt}{} \\
\cline{3-11}
 &  &  & \HoloSegMetric{Dice} & \HoloSegScore{0.9400}{(0.9362--0.9437)}{4.55pt}{4.82pt}{} & \HoloSegScore{0.5845}{(0.5356--0.6259)}{4.55pt}{4.82pt}{} & \HoloSegScore{0.9518}{(0.9489--0.9546)}{4.55pt}{4.82pt}{} & \HoloSegScore{0.9599}{(0.9571--0.9625)}{4.55pt}{4.82pt}{} & \HoloSegScore{0.9393}{(0.9377--0.9401)}{4.55pt}{4.82pt}{} & \HoloSegScore{0.9395}{(0.9354--0.9433)}{4.55pt}{4.82pt}{} & \HoloSegScore{0.9065}{(0.9003--0.9124)}{4.55pt}{4.82pt}{} \\*
\softcline{4-11}
\HoloSegSpan{\makecell[c]{\textbf{Internal}}}{1.20cm}{0.32cm} & \HoloSegSpan{\makecell[c]{DAP-Atlas\\[-0.10ex](AutoPETIII)}}{1.86cm}{0.32cm} & \HoloSegSpan{\makecell[c]{right\\[-0.10ex]iliopsoas}}{2.04cm}{0.32cm} & \HoloSegMetric{HD95} & \HoloSegScore{2.362}{(2.227--2.490)}{4.55pt}{4.82pt}{} & \HoloSegScore{24.42}{(17.04--33.16)}{4.55pt}{4.82pt}{} & \HoloSegScore{1.790}{(1.745--1.831)}{4.55pt}{4.82pt}{} & \HoloSegScore{1.440}{(1.309--1.579)}{4.55pt}{4.82pt}{} & \HoloSegScore{2.165}{(1.401--2.407)}{4.55pt}{4.82pt}{} & \HoloSegScore{9.407}{(3.621--18.70)}{4.55pt}{4.82pt}{} & \HoloSegScore{35.96}{(31.24--40.83)}{4.55pt}{4.82pt}{} \\
\cline{3-11}
 &  &  & \HoloSegMetric{Dice} & \HoloSegScore{0.9462}{(0.9416--0.9501)}{4.55pt}{4.82pt}{} & \HoloSegScore{0.7395}{(0.7269--0.7505)}{4.55pt}{4.82pt}{} & \HoloSegScore{0.9627}{(0.9603--0.9649)}{4.55pt}{4.82pt}{} & \HoloSegScore{0.9506}{(0.9464--0.9544)}{4.55pt}{4.82pt}{} & \HoloSegScore{0.9620}{(0.9573--0.9683)}{4.55pt}{4.82pt}{} & \HoloSegScore{0.9162}{(0.9107--0.9212)}{4.55pt}{4.82pt}{} & \HoloSegScore{0.9249}{(0.9190--0.9301)}{4.55pt}{4.82pt}{} \\*
\softcline{4-11}
 &  & \HoloSegSpan{\makecell[c]{left\\[-0.10ex]autochthon}}{2.04cm}{0.32cm} & \HoloSegMetric{HD95} & \HoloSegScore{2.527}{(2.229--2.947)}{4.55pt}{4.82pt}{} & \HoloSegScore{14.38}{(11.99--18.19)}{4.55pt}{4.82pt}{} & \HoloSegScore{1.737}{(1.630--1.849)}{4.55pt}{4.82pt}{} & \HoloSegScore{2.013}{(1.755--2.380)}{4.55pt}{4.82pt}{} & \HoloSegScore{2.891}{(2.638--3.574)}{4.55pt}{4.82pt}{} & \HoloSegScore{22.35}{(15.80--29.65)}{4.55pt}{4.82pt}{} & \HoloSegScore{4.286}{(3.172--5.876)}{4.55pt}{4.82pt}{} \\
\cline{3-11}
 &  &  & \HoloSegMetric{Dice} & \HoloSegScore{0.9399}{(0.9356--0.9434)}{4.55pt}{4.82pt}{} & \HoloSegScore{0.7396}{(0.7244--0.7529)}{4.55pt}{4.82pt}{} & \HoloSegScore{0.9613}{(0.9587--0.9636)}{4.55pt}{4.82pt}{} & \HoloSegScore{0.9453}{(0.9405--0.9497)}{4.55pt}{4.82pt}{} & \HoloSegScore{0.9585}{(0.9420--0.9596)}{4.55pt}{4.82pt}{} & \HoloSegScore{0.9118}{(0.9049--0.9170)}{4.55pt}{4.82pt}{} & \HoloSegScore{0.9266}{(0.9213--0.9309)}{4.55pt}{4.82pt}{} \\*
\softcline{4-11}
 &  & \HoloSegSpan{\makecell[c]{right\\[-0.10ex]autochthon}}{2.04cm}{0.32cm} & \HoloSegMetric{HD95} & \HoloSegScore{2.554}{(2.358--2.817)}{4.55pt}{4.82pt}{} & \HoloSegScore{15.77}{(12.52--20.05)}{4.55pt}{4.82pt}{} & \HoloSegScore{1.677}{(1.579--1.784)}{4.55pt}{4.82pt}{} & \HoloSegScore{2.220}{(1.958--2.541)}{4.55pt}{4.82pt}{} & \HoloSegScore{4.044}{(2.946--5.117)}{4.55pt}{4.82pt}{} & \HoloSegScore{9.458}{(4.806--15.76)}{4.55pt}{4.82pt}{} & \HoloSegScore{3.207}{(2.936--3.571)}{4.55pt}{4.82pt}{} \\
\cline{3-11}
 &  &  & \HoloSegMetric{Dice} &  & \HoloSegScore{0.0006846}{(0.0004049--0.001021)}{3.52pt}{3.80pt}{} & \HoloSegScore{0.7606}{(0.7547--0.7663)}{4.55pt}{4.82pt}{} & \HoloSegScore{0.7798}{(0.7721--0.7865)}{4.55pt}{4.82pt}{} & \HoloSegScore{0.7761}{(0.7620--0.7883)}{4.55pt}{4.82pt}{} & \HoloSegScore{0.7347}{(0.7286--0.7399)}{4.55pt}{4.82pt}{} & \HoloSegScore{0.7466}{(0.7411--0.7516)}{4.55pt}{4.82pt}{} \\*
\softcline{4-4}\softcline{6-11}
 &  & \HoloSegSpan{\makecell[c]{skin}}{2.04cm}{0.32cm} & \HoloSegMetric{HD95} & \raisebox{0.32cm}[0pt][0pt]{\HoloSegUnsupported} & \HoloSegScore{115.9}{(106.4--128.3)}{4.55pt}{4.82pt}{} & \HoloSegScore{1.336}{(1.211--1.478)}{4.55pt}{4.82pt}{} & \HoloSegScore{21.35}{(13.20--30.45)}{4.55pt}{4.82pt}{} & \HoloSegScore{2.245}{(1.912--3.152)}{4.55pt}{4.82pt}{} & \HoloSegScore{3.549}{(3.092--4.016)}{4.55pt}{4.82pt}{} & \HoloSegScore{2.566}{(2.264--2.850)}{4.55pt}{4.82pt}{} \\
\cline{3-11}
 &  &  & \HoloSegMetric{Dice} & \HoloSegScore{0.8652}{(0.8582--0.8711)}{4.55pt}{4.82pt}{} & \HoloSegScore{0.1337}{(0.1009--0.1672)}{4.55pt}{4.82pt}{} & \HoloSegScore{0.8663}{(0.8552--0.8754)}{4.55pt}{4.82pt}{} & \HoloSegScore{0.9089}{(0.9027--0.9146)}{4.55pt}{4.82pt}{} & \HoloSegScore{0.8360}{(0.8262--0.8381)}{4.55pt}{4.82pt}{} & \HoloSegScore{0.8881}{(0.8796--0.8959)}{4.55pt}{4.82pt}{} & \HoloSegScore{0.9033}{(0.8968--0.9088)}{4.55pt}{4.82pt}{} \\*
\softcline{4-11}
 &  & \HoloSegSpan{\makecell[c]{cervical\\[-0.10ex]vertebrae 1\\[-0.10ex](c1)}}{2.04cm}{0.32cm} & \HoloSegMetric{HD95} & \HoloSegScore{55.47}{(24.99--93.20)}{4.55pt}{4.82pt}{} & \HoloSegScore{39.34}{(34.85--43.70)}{4.55pt}{4.82pt}{} & \HoloSegScore{42.37}{(11.94--82.21)}{4.55pt}{4.82pt}{} & \HoloSegScore{1.997}{(1.762--2.193)}{4.55pt}{4.82pt}{} & \HoloSegScore{1.974}{(1.704--2.682)}{4.55pt}{4.82pt}{} & \HoloSegScore{2.466}{(2.194--2.760)}{4.55pt}{4.82pt}{} & \HoloSegScore{1.947}{(1.716--2.168)}{4.55pt}{4.82pt}{} \\
\cline{3-11}
 &  &  & \HoloSegMetric{Dice} & \HoloSegScore{0.8886}{(0.8814--0.8950)}{4.55pt}{4.82pt}{} & \HoloSegScore{0.09402}{(0.05907--0.1298)}{4.20pt}{4.48pt}{} & \HoloSegScore{0.6908}{(0.6411--0.7415)}{4.55pt}{4.82pt}{} & \HoloSegScore{0.9217}{(0.9170--0.9263)}{4.55pt}{4.82pt}{} & \HoloSegScore{0.8593}{(0.8378--0.8639)}{4.55pt}{4.82pt}{} & \HoloSegScore{0.9057}{(0.8969--0.9124)}{4.55pt}{4.82pt}{} & \HoloSegScore{0.9203}{(0.9153--0.9251)}{4.55pt}{4.82pt}{} \\*
\softcline{4-11}
 &  & \HoloSegSpan{\makecell[c]{cervical\\[-0.10ex]vertebrae 2\\[-0.10ex](c2)}}{2.04cm}{0.32cm} & \HoloSegMetric{HD95} & \HoloSegScore{10.44}{(5.533--16.24)}{4.55pt}{4.82pt}{} & \HoloSegScore{45.17}{(41.15--49.21)}{4.55pt}{4.82pt}{} & \HoloSegScore{354.5}{(309.0--395.3)}{4.55pt}{4.82pt}{} & \HoloSegScore{1.863}{(1.610--2.144)}{4.55pt}{4.82pt}{} & \HoloSegScore{2.482}{(2.225--2.846)}{4.55pt}{4.82pt}{} & \HoloSegScore{2.180}{(1.952--2.411)}{4.55pt}{4.82pt}{} & \HoloSegScore{1.741}{(1.509--1.954)}{4.55pt}{4.82pt}{} \\
\cline{3-11}
 &  &  & \HoloSegMetric{Dice} & \HoloSegScore{0.8555}{(0.8437--0.8667)}{4.55pt}{4.82pt}{} & \HoloSegScore{0.03676}{(0.01260--0.06253)}{4.20pt}{4.48pt}{} & \HoloSegScore{0.3834}{(0.3495--0.4221)}{4.55pt}{4.82pt}{} & \HoloSegScore{0.9014}{(0.8935--0.9089)}{4.55pt}{4.82pt}{} & \HoloSegScore{0.8853}{(0.8699--0.8951)}{4.55pt}{4.82pt}{} & \HoloSegScore{0.8936}{(0.8822--0.9035)}{4.55pt}{4.82pt}{} & \HoloSegScore{0.9052}{(0.8993--0.9102)}{4.55pt}{4.82pt}{} \\*
\softcline{4-11}
 &  & \HoloSegSpan{\makecell[c]{cervical\\[-0.10ex]vertebrae 3\\[-0.10ex](c3)}}{2.04cm}{0.32cm} & \HoloSegMetric{HD95} & \HoloSegScore{8.191}{(4.535--12.42)}{4.55pt}{4.82pt}{} & \HoloSegScore{56.13}{(51.42--61.33)}{4.55pt}{4.82pt}{} & \HoloSegScore{408.3}{(399.3--416.2)}{4.55pt}{4.82pt}{} & \HoloSegScore{2.122}{(1.841--2.421)}{4.55pt}{4.82pt}{} & \HoloSegScore{2.825}{(2.054--3.317)}{4.55pt}{4.82pt}{} & \HoloSegScore{2.199}{(1.973--2.429)}{4.55pt}{4.82pt}{} & \HoloSegScore{1.757}{(1.543--1.964)}{4.55pt}{4.82pt}{} \\
\cline{3-11}
 &  &  & \HoloSegMetric{Dice} & \HoloSegScore{0.8670}{(0.8575--0.8757)}{4.55pt}{4.82pt}{} & \HoloSegScore{0.03874}{(0.01351--0.06714)}{4.20pt}{4.48pt}{} & \HoloSegScore{0.2733}{(0.2628--0.2857)}{4.55pt}{4.82pt}{} & \HoloSegScore{0.9068}{(0.8978--0.9146)}{4.55pt}{4.82pt}{} & \HoloSegScore{0.9009}{(0.8711--0.9301)}{4.55pt}{4.82pt}{} & \HoloSegScore{0.6374}{(0.6239--0.6518)}{4.55pt}{4.82pt}{} & \HoloSegScore{0.8865}{(0.8750--0.8978)}{4.55pt}{4.82pt}{} \\*
\softcline{4-11}
 &  & \HoloSegSpan{\makecell[c]{cervical\\[-0.10ex]vertebrae 4\\[-0.10ex](c4)}}{2.04cm}{0.32cm} & \HoloSegMetric{HD95} & \HoloSegScore{41.55}{(16.23--76.42)}{4.55pt}{4.82pt}{} & \HoloSegScore{63.03}{(55.77--70.54)}{4.55pt}{4.82pt}{} & \HoloSegScore{424.1}{(414.5--432.7)}{4.55pt}{4.82pt}{} & \HoloSegScore{1.751}{(1.541--1.989)}{4.55pt}{4.82pt}{} & \HoloSegScore{3.487}{(3.479--5.099)}{4.55pt}{4.82pt}{} & \HoloSegScore{119.2}{(70.16--175.0)}{4.55pt}{4.82pt}{} & \HoloSegScore{2.296}{(2.026--2.575)}{4.55pt}{4.82pt}{} \\
\cline{3-11}
 &  &  & \HoloSegMetric{Dice} & \HoloSegScore{0.8166}{(0.7853--0.8404)}{4.55pt}{4.82pt}{} & \HoloSegScore{0.000009553}{(0.0000--0.00002866)}{3.85pt}{4.12pt}{} & \HoloSegScore{0.3229}{(0.3043--0.3452)}{4.55pt}{4.82pt}{} & \HoloSegScore{0.8904}{(0.8787--0.8998)}{4.55pt}{4.82pt}{} & \HoloSegScore{0.7931}{(0.7865--0.8011)}{4.55pt}{4.82pt}{} & \HoloSegScore{0.7119}{(0.6687--0.7530)}{4.55pt}{4.82pt}{} & \HoloSegScore{0.8590}{(0.8457--0.8714)}{4.55pt}{4.82pt}{} \\*
\softcline{4-11}
 &  & \HoloSegSpan{\makecell[c]{cervical\\[-0.10ex]vertebrae 5\\[-0.10ex](c5)}}{2.04cm}{0.32cm} & \HoloSegMetric{HD95} & \HoloSegScore{26.35}{(18.56--35.17)}{4.55pt}{4.82pt}{} & \HoloSegScore{128.2}{(121.5--134.9)}{4.55pt}{4.82pt}{} & \HoloSegScore{437.8}{(428.7--445.7)}{4.55pt}{4.82pt}{} & \HoloSegScore{2.017}{(1.817--2.223)}{4.55pt}{4.82pt}{} & \HoloSegScore{3.457}{(2.050--5.522)}{4.55pt}{4.82pt}{} & \HoloSegScore{4.911}{(4.282--5.621)}{4.55pt}{4.82pt}{} & \HoloSegScore{3.161}{(2.769--3.581)}{4.55pt}{4.82pt}{} \\
\cline{3-11}
 &  &  & \HoloSegMetric{Dice} & \HoloSegScore{0.8553}{(0.8437--0.8658)}{4.55pt}{4.82pt}{} & \HoloSegScore{0.0000}{(0.0000--0.0000)}{4.55pt}{4.82pt}{} & \HoloSegScore{0.8489}{(0.8259--0.8667)}{4.55pt}{4.82pt}{} & \HoloSegScore{0.8944}{(0.8830--0.9036)}{4.55pt}{4.82pt}{} & \HoloSegScore{0.8704}{(0.8570--0.8958)}{4.55pt}{4.82pt}{} & \HoloSegScore{0.8681}{(0.8582--0.8774)}{4.55pt}{4.82pt}{} & \HoloSegScore{0.8788}{(0.8705--0.8872)}{4.55pt}{4.82pt}{} \\*
\softcline{4-11}
 &  & \HoloSegSpan{\makecell[c]{cervical\\[-0.10ex]vertebrae 6\\[-0.10ex](c6)}}{2.04cm}{0.32cm} & \HoloSegMetric{HD95} & \HoloSegScore{21.56}{(2.727--46.19)}{4.55pt}{4.82pt}{} & \HoloSegScore{160.6}{(152.7--169.1)}{4.55pt}{4.82pt}{} & \HoloSegScore{58.84}{(14.32--107.1)}{4.55pt}{4.82pt}{} & \HoloSegScore{2.034}{(1.813--2.301)}{4.55pt}{4.82pt}{} & \HoloSegScore{3.319}{(2.285--3.629)}{4.55pt}{4.82pt}{} & \HoloSegScore{2.556}{(2.359--2.787)}{4.55pt}{4.82pt}{} & \HoloSegScore{2.285}{(2.068--2.512)}{4.55pt}{4.82pt}{} \\
\hline
\pagebreak[4]
 &  &  & \HoloSegMetric{Dice} & \HoloSegScore{0.8850}{(0.8728--0.8946)}{4.55pt}{4.82pt}{} & \HoloSegScore{0.0000}{(0.0000--0.0000)}{4.55pt}{4.82pt}{} & \HoloSegScore{0.6335}{(0.5790--0.6878)}{4.55pt}{4.82pt}{} & \HoloSegScore{0.9074}{(0.8985--0.9160)}{4.55pt}{4.82pt}{} & \HoloSegScore{0.9063}{(0.8871--0.9205)}{4.55pt}{4.82pt}{} & \HoloSegScore{0.8681}{(0.8566--0.8789)}{4.55pt}{4.82pt}{} & \HoloSegScore{0.8875}{(0.8792--0.8952)}{4.55pt}{4.82pt}{} \\*
\softcline{4-11}
 &  & \HoloSegSpan{\makecell[c]{cervical\\[-0.10ex]vertebrae 7\\[-0.10ex](c7)}}{2.04cm}{0.32cm} & \HoloSegMetric{HD95} & \HoloSegScore{2.509}{(2.295--2.816)}{4.55pt}{4.82pt}{} & \HoloSegScore{173.9}{(164.8--183.4)}{4.55pt}{4.82pt}{} & \HoloSegScore{397.9}{(353.3--436.3)}{4.55pt}{4.82pt}{} & \HoloSegScore{1.871}{(1.647--2.100)}{4.55pt}{4.82pt}{} & \HoloSegScore{3.805}{(2.607--4.658)}{4.55pt}{4.82pt}{} & \HoloSegScore{4.378}{(3.598--5.280)}{4.55pt}{4.82pt}{} & \HoloSegScore{2.540}{(2.418--2.667)}{4.55pt}{4.82pt}{} \\
\cline{3-11}
 &  &  & \HoloSegMetric{Dice} & \HoloSegScore{0.8697}{(0.8471--0.8867)}{4.55pt}{4.82pt}{} & \HoloSegScore{0.04665}{(0.02127--0.07478)}{4.20pt}{4.48pt}{} & \HoloSegScore{0.8186}{(0.7643--0.8576)}{4.55pt}{4.82pt}{} & \HoloSegScore{0.9201}{(0.9087--0.9301)}{4.55pt}{4.82pt}{} & \HoloSegScore{0.9180}{(0.9045--0.9223)}{4.55pt}{4.82pt}{} & \HoloSegScore{0.9076}{(0.8936--0.9195)}{4.55pt}{4.82pt}{} & \HoloSegScore{0.9096}{(0.9026--0.9165)}{4.55pt}{4.82pt}{} \\*
\softcline{4-11}
 &  & \HoloSegSpan{\makecell[c]{thoracic\\[-0.10ex]vertebrae 1\\[-0.10ex](t1)}}{2.04cm}{0.32cm} & \HoloSegMetric{HD95} & \HoloSegScore{32.50}{(24.64--39.14)}{4.55pt}{4.82pt}{} & \HoloSegScore{46.20}{(41.81--50.65)}{4.55pt}{4.82pt}{} & \HoloSegScore{111.4}{(52.15--180.7)}{4.55pt}{4.82pt}{} & \HoloSegScore{1.922}{(1.560--2.375)}{4.55pt}{4.82pt}{} & \HoloSegScore{2.937}{(1.751--3.865)}{4.55pt}{4.82pt}{} & \HoloSegScore{2.336}{(1.849--2.981)}{4.55pt}{4.82pt}{} & \HoloSegScore{2.263}{(1.934--2.721)}{4.55pt}{4.82pt}{} \\
\cline{3-11}
 &  &  & \HoloSegMetric{Dice} & \HoloSegScore{0.8815}{(0.8438--0.9054)}{4.55pt}{4.82pt}{} & \HoloSegScore{0.1498}{(0.1061--0.2014)}{4.55pt}{4.82pt}{} & \HoloSegScore{0.8767}{(0.8560--0.8925)}{4.55pt}{4.82pt}{} & \HoloSegScore{0.9108}{(0.8853--0.9279)}{4.55pt}{4.82pt}{} & \HoloSegScore{0.8865}{(0.8661--0.8962)}{4.55pt}{4.82pt}{} & \HoloSegScore{0.8261}{(0.7971--0.8504)}{4.55pt}{4.82pt}{} & \HoloSegScore{0.9135}{(0.9019--0.9234)}{4.55pt}{4.82pt}{} \\*
\softcline{4-11}
 &  & \HoloSegSpan{\makecell[c]{thoracic\\[-0.10ex]vertebrae 2\\[-0.10ex](t2)}}{2.04cm}{0.32cm} & \HoloSegMetric{HD95} & \HoloSegScore{36.55}{(4.912--72.80)}{4.55pt}{4.82pt}{} & \HoloSegScore{33.72}{(29.27--38.18)}{4.55pt}{4.82pt}{} & \HoloSegScore{2.870}{(2.526--3.331)}{4.55pt}{4.82pt}{} & \HoloSegScore{3.464}{(2.185--5.117)}{4.55pt}{4.82pt}{} & \HoloSegScore{3.609}{(2.909--4.689)}{4.55pt}{4.82pt}{} & \HoloSegScore{5.902}{(4.428--7.690)}{4.55pt}{4.82pt}{} & \HoloSegScore{2.252}{(1.600--3.183)}{4.55pt}{4.82pt}{} \\
\cline{3-11}
 &  &  & \HoloSegMetric{Dice} & \HoloSegScore{0.8630}{(0.8031--0.9019)}{4.55pt}{4.82pt}{} & \HoloSegScore{0.2691}{(0.2137--0.3261)}{4.55pt}{4.82pt}{} & \HoloSegScore{0.8712}{(0.8444--0.8912)}{4.55pt}{4.82pt}{} & \HoloSegScore{0.8887}{(0.8461--0.9220)}{4.55pt}{4.82pt}{} & \HoloSegScore{0.8723}{(0.8524--0.8765)}{4.55pt}{4.82pt}{} & \HoloSegScore{0.8593}{(0.8389--0.8777)}{4.55pt}{4.82pt}{} & \HoloSegScore{0.9043}{(0.8818--0.9199)}{4.55pt}{4.82pt}{} \\*
\softcline{4-11}
 &  & \HoloSegSpan{\makecell[c]{thoracic\\[-0.10ex]vertebrae 3\\[-0.10ex](t3)}}{2.04cm}{0.32cm} & \HoloSegMetric{HD95} & \HoloSegScore{3.716}{(2.388--5.554)}{4.55pt}{4.82pt}{} & \HoloSegScore{24.15}{(20.58--28.46)}{4.55pt}{4.82pt}{} & \HoloSegScore{3.214}{(2.467--4.246)}{4.55pt}{4.82pt}{} & \HoloSegScore{3.885}{(2.489--5.784)}{4.55pt}{4.82pt}{} & \HoloSegScore{3.495}{(2.876--5.008)}{4.55pt}{4.82pt}{} & \HoloSegScore{8.934}{(5.834--13.76)}{4.55pt}{4.82pt}{} & \HoloSegScore{2.556}{(1.734--3.748)}{4.55pt}{4.82pt}{} \\
\cline{3-11}
 &  &  & \HoloSegMetric{Dice} & \HoloSegScore{0.8282}{(0.7574--0.8892)}{4.55pt}{4.82pt}{} & \HoloSegScore{0.2990}{(0.2578--0.3399)}{4.55pt}{4.82pt}{} & \HoloSegScore{0.8445}{(0.8110--0.8719)}{4.55pt}{4.82pt}{} & \HoloSegScore{0.8711}{(0.8129--0.9137)}{4.55pt}{4.82pt}{} & \HoloSegScore{0.8383}{(0.8183--0.8484)}{4.55pt}{4.82pt}{} & \HoloSegScore{0.6945}{(0.6582--0.7287)}{4.55pt}{4.82pt}{} & \HoloSegScore{0.8896}{(0.8621--0.9107)}{4.55pt}{4.82pt}{} \\*
\softcline{4-11}
 &  & \HoloSegSpan{\makecell[c]{thoracic\\[-0.10ex]vertebrae 4\\[-0.10ex](t4)}}{2.04cm}{0.32cm} & \HoloSegMetric{HD95} & \HoloSegScore{4.875}{(3.039--7.248)}{4.55pt}{4.82pt}{} & \HoloSegScore{22.35}{(20.21--24.49)}{4.55pt}{4.82pt}{} & \HoloSegScore{71.35}{(18.82--136.4)}{4.55pt}{4.82pt}{} & \HoloSegScore{3.742}{(2.196--5.729)}{4.55pt}{4.82pt}{} & \HoloSegScore{4.342}{(3.084--7.294)}{4.55pt}{4.82pt}{} & \HoloSegScore{85.24}{(70.53--98.28)}{4.55pt}{4.82pt}{} & \HoloSegScore{2.702}{(1.905--3.778)}{4.55pt}{4.82pt}{} \\
\cline{3-11}
 &  &  & \HoloSegMetric{Dice} & \HoloSegScore{0.8483}{(0.8056--0.8858)}{4.55pt}{4.82pt}{} & \HoloSegScore{0.3722}{(0.3318--0.4075)}{4.55pt}{4.82pt}{} & \HoloSegScore{0.8729}{(0.8561--0.8877)}{4.55pt}{4.82pt}{} & \HoloSegScore{0.8806}{(0.8353--0.9140)}{4.55pt}{4.82pt}{} & \HoloSegScore{0.8797}{(0.8727--0.8956)}{4.55pt}{4.82pt}{} & \HoloSegScore{0.5884}{(0.5166--0.6625)}{4.55pt}{4.82pt}{} & \HoloSegScore{0.8967}{(0.8814--0.9103)}{4.55pt}{4.82pt}{} \\*
\softcline{4-11}
 &  & \HoloSegSpan{\makecell[c]{thoracic\\[-0.10ex]vertebrae 5\\[-0.10ex](t5)}}{2.04cm}{0.32cm} & \HoloSegMetric{HD95} & \HoloSegScore{5.424}{(3.849--7.185)}{4.55pt}{4.82pt}{} & \HoloSegScore{20.76}{(18.59--23.27)}{4.55pt}{4.82pt}{} & \HoloSegScore{3.337}{(2.706--4.252)}{4.55pt}{4.82pt}{} & \HoloSegScore{3.930}{(2.611--5.468)}{4.55pt}{4.82pt}{} & \HoloSegScore{3.557}{(1.653--4.966)}{4.55pt}{4.82pt}{} & \HoloSegScore{10.68}{(8.760--12.75)}{4.55pt}{4.82pt}{} & \HoloSegScore{3.020}{(2.225--3.944)}{4.55pt}{4.82pt}{} \\
\cline{3-11}
 &  &  & \HoloSegMetric{Dice} & \HoloSegScore{0.8619}{(0.8218--0.8941)}{4.55pt}{4.82pt}{} & \HoloSegScore{0.4088}{(0.3583--0.4548)}{4.55pt}{4.82pt}{} & \HoloSegScore{0.8698}{(0.8562--0.8818)}{4.55pt}{4.82pt}{} & \HoloSegScore{0.8860}{(0.8479--0.9154)}{4.55pt}{4.82pt}{} & \HoloSegScore{0.8656}{(0.8624--0.8824)}{4.55pt}{4.82pt}{} & \HoloSegScore{0.8245}{(0.7874--0.8564)}{4.55pt}{4.82pt}{} & \HoloSegScore{0.8851}{(0.8678--0.9001)}{4.55pt}{4.82pt}{} \\*
\softcline{4-11}
 &  & \HoloSegSpan{\makecell[c]{thoracic\\[-0.10ex]vertebrae 6\\[-0.10ex](t6)}}{2.04cm}{0.32cm} & \HoloSegMetric{HD95} & \HoloSegScore{4.294}{(3.120--5.873)}{4.55pt}{4.82pt}{} & \HoloSegScore{22.86}{(16.81--32.56)}{4.55pt}{4.82pt}{} & \HoloSegScore{2.925}{(2.652--3.215)}{4.55pt}{4.82pt}{} & \HoloSegScore{3.775}{(2.638--5.161)}{4.55pt}{4.82pt}{} & \HoloSegScore{5.833}{(5.390--7.790)}{4.55pt}{4.82pt}{} & \HoloSegScore{5.538}{(4.277--6.869)}{4.55pt}{4.82pt}{} & \HoloSegScore{3.511}{(2.723--4.377)}{4.55pt}{4.82pt}{} \\
\cline{3-11}
 &  &  & \HoloSegMetric{Dice} & \HoloSegScore{0.8672}{(0.8285--0.8972)}{4.55pt}{4.82pt}{} & \HoloSegScore{0.2734}{(0.2048--0.3403)}{4.55pt}{4.82pt}{} & \HoloSegScore{0.8790}{(0.8646--0.8917)}{4.55pt}{4.82pt}{} & \HoloSegScore{0.8951}{(0.8560--0.9242)}{4.55pt}{4.82pt}{} & \HoloSegScore{0.8653}{(0.8617--0.8718)}{4.55pt}{4.82pt}{} & \HoloSegScore{0.8986}{(0.8818--0.9125)}{4.55pt}{4.82pt}{} & \HoloSegScore{0.9004}{(0.8816--0.9146)}{4.55pt}{4.82pt}{} \\*
\softcline{4-11}
 &  & \HoloSegSpan{\makecell[c]{thoracic\\[-0.10ex]vertebrae 7\\[-0.10ex](t7)}}{2.04cm}{0.32cm} & \HoloSegMetric{HD95} & \HoloSegScore{4.591}{(3.186--6.308)}{4.55pt}{4.82pt}{} & \HoloSegScore{43.84}{(32.07--58.44)}{4.55pt}{4.82pt}{} & \HoloSegScore{3.198}{(2.663--3.871)}{4.55pt}{4.82pt}{} & \HoloSegScore{3.704}{(2.619--4.901)}{4.55pt}{4.82pt}{} & \HoloSegScore{4.950}{(3.863--5.624)}{4.55pt}{4.82pt}{} & \HoloSegScore{3.632}{(2.696--4.826)}{4.55pt}{4.82pt}{} & \HoloSegScore{3.338}{(2.439--4.458)}{4.55pt}{4.82pt}{} \\
\cline{3-11}
 &  &  & \HoloSegMetric{Dice} & \HoloSegScore{0.8723}{(0.8526--0.8910)}{4.55pt}{4.82pt}{} & \HoloSegScore{0.2173}{(0.1549--0.2820)}{4.55pt}{4.82pt}{} & \HoloSegScore{0.8763}{(0.8493--0.8953)}{4.55pt}{4.82pt}{} & \HoloSegScore{0.9106}{(0.8826--0.9332)}{4.55pt}{4.82pt}{} & \HoloSegScore{0.8846}{(0.8506--0.9006)}{4.55pt}{4.82pt}{} & \HoloSegScore{0.8770}{(0.8532--0.8967)}{4.55pt}{4.82pt}{} & \HoloSegScore{0.9005}{(0.8840--0.9143)}{4.55pt}{4.82pt}{} \\*
\softcline{4-11}
 &  & \HoloSegSpan{\makecell[c]{thoracic\\[-0.10ex]vertebrae 8\\[-0.10ex](t8)}}{2.04cm}{0.32cm} & \HoloSegMetric{HD95} & \HoloSegScore{25.00}{(19.53--30.23)}{4.55pt}{4.82pt}{} & \HoloSegScore{63.35}{(46.77--81.52)}{4.55pt}{4.82pt}{} & \HoloSegScore{2.911}{(2.533--3.417)}{4.55pt}{4.82pt}{} & \HoloSegScore{3.142}{(2.204--4.367)}{4.55pt}{4.82pt}{} & \HoloSegScore{4.126}{(3.255--6.915)}{4.55pt}{4.82pt}{} & \HoloSegScore{4.716}{(3.737--5.830)}{4.55pt}{4.82pt}{} & \HoloSegScore{3.723}{(2.742--4.859)}{4.55pt}{4.82pt}{} \\
\cline{3-11}
 &  &  & \HoloSegMetric{Dice} & \HoloSegScore{0.9013}{(0.8854--0.9144)}{4.55pt}{4.82pt}{} & \HoloSegScore{0.3543}{(0.2906--0.4167)}{4.55pt}{4.82pt}{} & \HoloSegScore{0.8779}{(0.8463--0.9005)}{4.55pt}{4.82pt}{} & \HoloSegScore{0.9187}{(0.8913--0.9396)}{4.55pt}{4.82pt}{} & \HoloSegScore{0.9042}{(0.8845--0.9374)}{4.55pt}{4.82pt}{} & \HoloSegScore{0.9050}{(0.8864--0.9195)}{4.55pt}{4.82pt}{} & \HoloSegScore{0.9147}{(0.8993--0.9271)}{4.55pt}{4.82pt}{} \\*
\softcline{4-11}
\HoloSegSpan{\makecell[c]{\textbf{Internal}}}{1.20cm}{0.32cm} & \HoloSegSpan{\makecell[c]{DAP-Atlas\\[-0.10ex](AutoPETIII)}}{1.86cm}{0.32cm} & \HoloSegSpan{\makecell[c]{thoracic\\[-0.10ex]vertebrae 9\\[-0.10ex](t9)}}{2.04cm}{0.32cm} & \HoloSegMetric{HD95} & \HoloSegScore{52.22}{(23.84--85.27)}{4.55pt}{4.82pt}{} & \HoloSegScore{28.54}{(22.08--36.96)}{4.55pt}{4.82pt}{} & \HoloSegScore{3.529}{(2.626--4.682)}{4.55pt}{4.82pt}{} & \HoloSegScore{2.805}{(2.015--3.754)}{4.55pt}{4.82pt}{} & \HoloSegScore{3.816}{(3.062--4.779)}{4.55pt}{4.82pt}{} & \HoloSegScore{3.615}{(2.798--4.661)}{4.55pt}{4.82pt}{} & \HoloSegScore{2.749}{(2.173--3.475)}{4.55pt}{4.82pt}{} \\
\cline{3-11}
 &  &  & \HoloSegMetric{Dice} & \HoloSegScore{0.9029}{(0.8829--0.9210)}{4.55pt}{4.82pt}{} & \HoloSegScore{0.2824}{(0.2272--0.3424)}{4.55pt}{4.82pt}{} & \HoloSegScore{0.8786}{(0.8472--0.9001)}{4.55pt}{4.82pt}{} & \HoloSegScore{0.9211}{(0.8952--0.9402)}{4.55pt}{4.82pt}{} & \HoloSegScore{0.8920}{(0.8890--0.9238)}{4.55pt}{4.82pt}{} & \HoloSegScore{0.9058}{(0.8916--0.9188)}{4.55pt}{4.82pt}{} & \HoloSegScore{0.9177}{(0.9078--0.9273)}{4.55pt}{4.82pt}{} \\*
\softcline{4-11}
 &  & \HoloSegSpan{\makecell[c]{thoracic\\[-0.10ex]vertebrae 10\\[-0.10ex](t10)}}{2.04cm}{0.32cm} & \HoloSegMetric{HD95} & \HoloSegScore{4.485}{(2.869--6.493)}{4.55pt}{4.82pt}{} & \HoloSegScore{31.01}{(25.11--38.28)}{4.55pt}{4.82pt}{} & \HoloSegScore{3.460}{(2.583--4.614)}{4.55pt}{4.82pt}{} & \HoloSegScore{3.215}{(2.197--4.486)}{4.55pt}{4.82pt}{} & \HoloSegScore{4.769}{(3.730--6.316)}{4.55pt}{4.82pt}{} & \HoloSegScore{4.726}{(3.619--5.963)}{4.55pt}{4.82pt}{} & \HoloSegScore{3.015}{(2.333--3.755)}{4.55pt}{4.82pt}{} \\
\cline{3-11}
 &  &  & \HoloSegMetric{Dice} & \HoloSegScore{0.8898}{(0.8243--0.9339)}{4.55pt}{4.82pt}{} & \HoloSegScore{0.2793}{(0.2252--0.3450)}{4.55pt}{4.82pt}{} & \HoloSegScore{0.8774}{(0.8379--0.9091)}{4.55pt}{4.82pt}{} & \HoloSegScore{0.9202}{(0.8799--0.9473)}{4.55pt}{4.82pt}{} & \HoloSegScore{0.8932}{(0.8771--0.9089)}{4.55pt}{4.82pt}{} & \HoloSegScore{0.9232}{(0.8944--0.9404)}{4.55pt}{4.82pt}{} & \HoloSegScore{0.9273}{(0.9125--0.9394)}{4.55pt}{4.82pt}{} \\*
\softcline{4-11}
 &  & \HoloSegSpan{\makecell[c]{thoracic\\[-0.10ex]vertebrae 11\\[-0.10ex](t11)}}{2.04cm}{0.32cm} & \HoloSegMetric{HD95} & \HoloSegScore{8.889}{(2.415--19.73)}{4.55pt}{4.82pt}{} & \HoloSegScore{37.60}{(30.27--45.60)}{4.55pt}{4.82pt}{} & \HoloSegScore{4.209}{(2.464--6.993)}{4.55pt}{4.82pt}{} & \HoloSegScore{3.864}{(1.942--6.546)}{4.55pt}{4.82pt}{} & \HoloSegScore{4.005}{(2.536--7.482)}{4.55pt}{4.82pt}{} & \HoloSegScore{3.276}{(1.866--5.597)}{4.55pt}{4.82pt}{} & \HoloSegScore{2.549}{(1.798--3.459)}{4.55pt}{4.82pt}{} \\
\cline{3-11}
 &  &  & \HoloSegMetric{Dice} & \HoloSegScore{0.8943}{(0.8417--0.9304)}{4.55pt}{4.82pt}{} & \HoloSegScore{0.02524}{(0.003933--0.05160)}{3.85pt}{4.12pt}{} & \HoloSegScore{0.8199}{(0.7724--0.8504)}{4.55pt}{4.82pt}{} & \HoloSegScore{0.9251}{(0.8859--0.9511)}{4.55pt}{4.82pt}{} & \HoloSegScore{0.9249}{(0.9100--0.9262)}{4.55pt}{4.82pt}{} & \HoloSegScore{0.9093}{(0.8853--0.9284)}{4.55pt}{4.82pt}{} & \HoloSegScore{0.9315}{(0.9151--0.9439)}{4.55pt}{4.82pt}{} \\*
\softcline{4-11}
 &  & \HoloSegSpan{\makecell[c]{thoracic\\[-0.10ex]vertebrae 12\\[-0.10ex](t12)}}{2.04cm}{0.32cm} & \HoloSegMetric{HD95} & \HoloSegScore{11.14}{(6.518--15.85)}{4.55pt}{4.82pt}{} & \HoloSegScore{78.20}{(66.52--90.16)}{4.55pt}{4.82pt}{} & \HoloSegScore{358.5}{(350.2--366.3)}{4.55pt}{4.82pt}{} & \HoloSegScore{2.972}{(1.611--4.916)}{4.55pt}{4.82pt}{} & \HoloSegScore{4.693}{(4.353--8.157)}{4.55pt}{4.82pt}{} & \HoloSegScore{4.560}{(3.385--5.985)}{4.55pt}{4.82pt}{} & \HoloSegScore{2.822}{(1.720--4.311)}{4.55pt}{4.82pt}{} \\
\cline{3-11}
 &  &  & \HoloSegMetric{Dice} & \HoloSegScore{0.9096}{(0.8711--0.9357)}{4.55pt}{4.82pt}{} & \HoloSegScore{0.2764}{(0.2254--0.3282)}{4.55pt}{4.82pt}{} & \HoloSegScore{0.8643}{(0.8414--0.8841)}{4.55pt}{4.82pt}{} & \HoloSegScore{0.9377}{(0.9101--0.9575)}{4.55pt}{4.82pt}{} & \HoloSegScore{0.9061}{(0.8791--0.9172)}{4.55pt}{4.82pt}{} & \HoloSegScore{0.9220}{(0.9085--0.9336)}{4.55pt}{4.82pt}{} & \HoloSegScore{0.9364}{(0.9225--0.9467)}{4.55pt}{4.82pt}{} \\*
\softcline{4-11}
 &  & \HoloSegSpan{\makecell[c]{lumbar\\[-0.10ex]vertebrae 1\\[-0.10ex](l1)}}{2.04cm}{0.32cm} & \HoloSegMetric{HD95} & \HoloSegScore{4.364}{(2.086--7.420)}{4.55pt}{4.82pt}{} & \HoloSegScore{36.08}{(31.66--41.02)}{4.55pt}{4.82pt}{} & \HoloSegScore{279.7}{(225.2--326.7)}{4.55pt}{4.82pt}{} & \HoloSegScore{3.727}{(1.710--6.899)}{4.55pt}{4.82pt}{} & \HoloSegScore{4.285}{(3.695--6.641)}{4.55pt}{4.82pt}{} & \HoloSegScore{4.597}{(2.795--7.668)}{4.55pt}{4.82pt}{} & \HoloSegScore{3.210}{(1.609--5.340)}{4.55pt}{4.82pt}{} \\
\cline{3-11}
 &  &  & \HoloSegMetric{Dice} & \HoloSegScore{0.9119}{(0.8814--0.9325)}{4.55pt}{4.82pt}{} & \HoloSegScore{0.4744}{(0.4355--0.5082)}{4.55pt}{4.82pt}{} & \HoloSegScore{0.8980}{(0.8834--0.9108)}{4.55pt}{4.82pt}{} & \HoloSegScore{0.9436}{(0.9261--0.9570)}{4.55pt}{4.82pt}{} & \HoloSegScore{0.9262}{(0.9059--0.9592)}{4.55pt}{4.82pt}{} & \HoloSegScore{0.8923}{(0.8659--0.9107)}{4.55pt}{4.82pt}{} & \HoloSegScore{0.9329}{(0.9218--0.9422)}{4.55pt}{4.82pt}{} \\*
\softcline{4-11}
 &  & \HoloSegSpan{\makecell[c]{lumbar\\[-0.10ex]vertebrae 2\\[-0.10ex](l2)}}{2.04cm}{0.32cm} & \HoloSegMetric{HD95} & \HoloSegScore{4.261}{(2.290--6.578)}{4.55pt}{4.82pt}{} & \HoloSegScore{20.42}{(18.47--22.58)}{4.55pt}{4.82pt}{} & \HoloSegScore{62.43}{(22.21--113.7)}{4.55pt}{4.82pt}{} & \HoloSegScore{2.826}{(1.542--4.758)}{4.55pt}{4.82pt}{} & \HoloSegScore{2.961}{(1.873--4.046)}{4.55pt}{4.82pt}{} & \HoloSegScore{5.972}{(4.503--7.804)}{4.55pt}{4.82pt}{} & \HoloSegScore{3.944}{(2.264--6.202)}{4.55pt}{4.82pt}{} \\
\cline{3-11}
 &  &  & \HoloSegMetric{Dice} & \HoloSegScore{0.9096}{(0.8826--0.9307)}{4.55pt}{4.82pt}{} & \HoloSegScore{0.2596}{(0.2123--0.3080)}{4.55pt}{4.82pt}{} & \HoloSegScore{0.9056}{(0.8923--0.9161)}{4.55pt}{4.82pt}{} & \HoloSegScore{0.9377}{(0.9163--0.9543)}{4.55pt}{4.82pt}{} & \HoloSegScore{0.9356}{(0.9278--0.9451)}{4.55pt}{4.82pt}{} & \HoloSegScore{0.9271}{(0.9167--0.9362)}{4.55pt}{4.82pt}{} & \HoloSegScore{0.9314}{(0.9201--0.9409)}{4.55pt}{4.82pt}{} \\*
\softcline{4-11}
 &  & \HoloSegSpan{\makecell[c]{lumbar\\[-0.10ex]vertebrae 3\\[-0.10ex](l3)}}{2.04cm}{0.32cm} & \HoloSegMetric{HD95} & \HoloSegScore{4.911}{(0.4736--10.32)}{4.55pt}{4.82pt}{} & \HoloSegScore{34.62}{(30.98--37.97)}{4.55pt}{4.82pt}{} & \HoloSegScore{3.170}{(2.417--4.462)}{4.55pt}{4.82pt}{} & \HoloSegScore{3.520}{(1.935--5.893)}{4.55pt}{4.82pt}{} & \HoloSegScore{4.244}{(3.220--4.391)}{4.55pt}{4.82pt}{} & \HoloSegScore{3.442}{(2.431--4.941)}{4.55pt}{4.82pt}{} & \HoloSegScore{3.192}{(1.913--5.088)}{4.55pt}{4.82pt}{} \\
\cline{3-11}
 &  &  & \HoloSegMetric{Dice} & \HoloSegScore{0.7764}{(0.7577--0.7937)}{4.55pt}{4.82pt}{} & \HoloSegScore{0.1351}{(0.09130--0.1807)}{4.20pt}{4.48pt}{} & \HoloSegScore{0.8552}{(0.8441--0.8658)}{4.55pt}{4.82pt}{} & \HoloSegScore{0.9343}{(0.9148--0.9515)}{4.55pt}{4.82pt}{} & \HoloSegScore{0.9236}{(0.9195--0.9324)}{4.55pt}{4.82pt}{} & \HoloSegScore{0.8996}{(0.8842--0.9137)}{4.55pt}{4.82pt}{} & \HoloSegScore{0.9328}{(0.9228--0.9422)}{4.55pt}{4.82pt}{} \\*
\softcline{4-11}
 &  & \HoloSegSpan{\makecell[c]{lumbar\\[-0.10ex]vertebrae 4\\[-0.10ex](l4)}}{2.04cm}{0.32cm} & \HoloSegMetric{HD95} & \HoloSegScore{48.94}{(47.00--50.61)}{4.55pt}{4.82pt}{} & \HoloSegScore{41.84}{(38.45--45.26)}{4.55pt}{4.82pt}{} & \HoloSegScore{380.3}{(340.3--414.3)}{4.55pt}{4.82pt}{} & \HoloSegScore{3.815}{(2.051--6.043)}{4.55pt}{4.82pt}{} & \HoloSegScore{4.141}{(3.206--7.114)}{4.55pt}{4.82pt}{} & \HoloSegScore{29.72}{(8.124--59.82)}{4.55pt}{4.82pt}{} & \HoloSegScore{2.585}{(2.044--3.405)}{4.55pt}{4.82pt}{} \\
\cline{3-11}
 &  &  & \HoloSegMetric{Dice} & \HoloSegScore{0.8936}{(0.8458--0.9252)}{4.55pt}{4.82pt}{} & \HoloSegScore{0.01211}{(0.003800--0.02174)}{3.85pt}{4.12pt}{} & \HoloSegScore{0.8119}{(0.7890--0.8299)}{4.55pt}{4.82pt}{} & \HoloSegScore{0.9066}{(0.8702--0.9386)}{4.55pt}{4.82pt}{} & \HoloSegScore{0.8761}{(0.8527--0.8906)}{4.55pt}{4.82pt}{} & \HoloSegScore{0.9097}{(0.8811--0.9309)}{4.55pt}{4.82pt}{} & \HoloSegScore{0.9152}{(0.8900--0.9344)}{4.55pt}{4.82pt}{} \\*
\softcline{4-11}
 &  & \HoloSegSpan{\makecell[c]{lumbar\\[-0.10ex]vertebrae 5\\[-0.10ex](l5)}}{2.04cm}{0.32cm} & \HoloSegMetric{HD95} & \HoloSegScore{4.553}{(2.660--7.054)}{4.55pt}{4.82pt}{} & \HoloSegScore{61.21}{(57.77--64.84)}{4.55pt}{4.82pt}{} & \HoloSegScore{410.6}{(381.5--429.6)}{4.55pt}{4.82pt}{} & \HoloSegScore{5.295}{(2.972--8.298)}{4.55pt}{4.82pt}{} & \HoloSegScore{4.991}{(2.918--5.515)}{4.55pt}{4.82pt}{} & \HoloSegScore{3.901}{(2.546--5.621)}{4.55pt}{4.82pt}{} & \HoloSegScore{2.861}{(2.117--3.973)}{4.55pt}{4.82pt}{} \\
\cline{3-11}
 &  &  & \HoloSegMetric{Dice} & \HoloSegScore{0.0000}{(0.0000--0.0000)}{4.55pt}{4.82pt}{} & \HoloSegScore{0.0000}{(0.0000--0.0000)}{4.55pt}{4.82pt}{} & \HoloSegScore{0.7729}{(0.6902--0.8384)}{4.55pt}{4.82pt}{} & \HoloSegScore{0.0000}{(0.0000--0.0000)}{4.55pt}{4.82pt}{} & \HoloSegScore{0.7162}{(0.7055--0.7314)}{4.55pt}{4.82pt}{} & \HoloSegScore{0.6772}{(0.5914--0.7467)}{4.55pt}{4.82pt}{} & \HoloSegScore{0.8080}{(0.7169--0.8774)}{4.55pt}{4.82pt}{} \\*
\softcline{4-11}
 &  & \HoloSegSpan{\makecell[c]{left rib 1}}{2.04cm}{0.32cm} & \HoloSegMetric{HD95} & \HoloSegScore{293.8}{(281.6--308.4)}{4.55pt}{4.82pt}{} & \HoloSegScore{299.4}{(291.1--308.2)}{4.55pt}{4.82pt}{} & \HoloSegScore{39.71}{(15.24--74.58)}{4.55pt}{4.82pt}{} & \HoloSegScore{294.2}{(286.5--303.1)}{4.55pt}{4.82pt}{} & \HoloSegScore{16.31}{(7.073--26.27)}{4.55pt}{4.82pt}{} & \HoloSegScore{15.64}{(6.509--27.33)}{4.55pt}{4.82pt}{} & \HoloSegScore{17.54}{(8.816--27.97)}{4.55pt}{4.82pt}{} \\
\hline
\pagebreak[4]
