# Supplementary material for: A 3D foundation model unifying CT interpretation and segmentation
Source: arXiv:2611.06471 source file (2026-11-04)
Supplement: Supplementary file 9 [file table1_subtask1_part2.tex]

&  &  & \HoloSegMetric{Dice} & \HoloSegScore{0.0000}{(0.0000--0.0000)}{4.55pt}{4.82pt}{} & \HoloSegScore{0.0000}{(0.0000--0.0000)}{4.55pt}{4.82pt}{} & \HoloSegScore{0.7755}{(0.6977--0.8295)}{4.55pt}{4.82pt}{} & \HoloSegScore{0.0000}{(0.0000--0.0000)}{4.55pt}{4.82pt}{} & \HoloSegScore{0.7675}{(0.7536--0.7806)}{4.55pt}{4.82pt}{} & \HoloSegScore{0.8306}{(0.7547--0.8872)}{4.55pt}{4.82pt}{} & \HoloSegScore{0.8588}{(0.7941--0.9031)}{4.55pt}{4.82pt}{} \\*
\softcline{4-11}
 &  & \HoloSegSpan{\makecell[c]{right rib 1}}{2.04cm}{0.32cm} & \HoloSegMetric{HD95} & \HoloSegScore{287.4}{(275.8--300.3)}{4.55pt}{4.82pt}{} & \HoloSegScore{296.8}{(290.1--303.5)}{4.55pt}{4.82pt}{} & \HoloSegScore{50.91}{(22.26--85.79)}{4.55pt}{4.82pt}{} & \HoloSegScore{293.0}{(285.8--300.4)}{4.55pt}{4.82pt}{} & \HoloSegScore{9.462}{(2.332--17.00)}{4.55pt}{4.82pt}{} & \HoloSegScore{10.10}{(1.929--21.87)}{4.55pt}{4.82pt}{} & \HoloSegScore{7.922}{(1.645--18.58)}{4.55pt}{4.82pt}{} \\
\cline{3-11}
 &  &  & \HoloSegMetric{Dice} & \HoloSegScore{0.0000}{(0.0000--0.0000)}{4.55pt}{4.82pt}{} & \HoloSegScore{0.0000}{(0.0000--0.0000)}{4.55pt}{4.82pt}{} & \HoloSegScore{0.7736}{(0.6890--0.8472)}{4.55pt}{4.82pt}{} & \HoloSegScore{0.0000}{(0.0000--0.0000)}{4.55pt}{4.82pt}{} & \HoloSegScore{0.7522}{(0.7478--0.7524)}{4.55pt}{4.82pt}{} & \HoloSegScore{0.6456}{(0.5473--0.7278)}{4.55pt}{4.82pt}{} & \HoloSegScore{0.8224}{(0.7352--0.8967)}{4.55pt}{4.82pt}{} \\*
\softcline{4-11}
 &  & \HoloSegSpan{\makecell[c]{left rib 2}}{2.04cm}{0.32cm} & \HoloSegMetric{HD95} & \HoloSegScore{265.4}{(253.2--278.8)}{4.55pt}{4.82pt}{} & \HoloSegScore{265.5}{(259.9--271.3)}{4.55pt}{4.82pt}{} & \HoloSegScore{14.36}{(4.206--29.27)}{4.55pt}{4.82pt}{} & \HoloSegScore{--}{(--\,--)}{4.55pt}{4.82pt}{} & \HoloSegScore{8.816}{(3.597--15.62)}{4.55pt}{4.82pt}{} & \HoloSegScore{21.70}{(13.04--31.70)}{4.55pt}{4.82pt}{} & \HoloSegScore{6.982}{(1.399--13.93)}{4.55pt}{4.82pt}{} \\
\cline{3-11}
 &  &  & \HoloSegMetric{Dice} & \HoloSegScore{0.0000}{(0.0000--0.0000)}{4.55pt}{4.82pt}{} & \HoloSegScore{0.0000}{(0.0000--0.0000)}{4.55pt}{4.82pt}{} & \HoloSegScore{0.7712}{(0.6881--0.8461)}{4.55pt}{4.82pt}{} & \HoloSegScore{0.0000}{(0.0000--0.0000)}{4.55pt}{4.82pt}{} & \HoloSegScore{0.7581}{(0.7574--0.7635)}{4.55pt}{4.82pt}{} & \HoloSegScore{0.7247}{(0.6201--0.8117)}{4.55pt}{4.82pt}{} & \HoloSegScore{0.8306}{(0.7435--0.9051)}{4.55pt}{4.82pt}{} \\*
\softcline{4-11}
 &  & \HoloSegSpan{\makecell[c]{right rib 2}}{2.04cm}{0.32cm} & \HoloSegMetric{HD95} & \HoloSegScore{246.8}{(236.2--256.8)}{4.55pt}{4.82pt}{} & \HoloSegScore{268.4}{(261.4--275.9)}{4.55pt}{4.82pt}{} & \HoloSegScore{15.04}{(4.525--29.01)}{4.55pt}{4.82pt}{} & \HoloSegScore{--}{(--\,--)}{4.55pt}{4.82pt}{} & \HoloSegScore{15.07}{(4.737--26.54)}{4.55pt}{4.82pt}{} & \HoloSegScore{18.03}{(7.981--31.17)}{4.55pt}{4.82pt}{} & \HoloSegScore{11.27}{(2.336--23.72)}{4.55pt}{4.82pt}{} \\
\cline{3-11}
 &  &  & \HoloSegMetric{Dice} & \HoloSegScore{0.0000}{(0.0000--0.0000)}{4.55pt}{4.82pt}{} & \HoloSegScore{0.0000}{(0.0000--0.0000)}{4.55pt}{4.82pt}{} & \HoloSegScore{0.8032}{(0.7306--0.8623)}{4.55pt}{4.82pt}{} & \HoloSegScore{0.0000}{(0.0000--0.0000)}{4.55pt}{4.82pt}{} & \HoloSegScore{0.7801}{(0.7613--0.7812)}{4.55pt}{4.82pt}{} & \HoloSegScore{0.7716}{(0.6998--0.8332)}{4.55pt}{4.82pt}{} & \HoloSegScore{0.8746}{(0.8037--0.9214)}{4.55pt}{4.82pt}{} \\*
\softcline{4-11}
 &  & \HoloSegSpan{\makecell[c]{left rib 3}}{2.04cm}{0.32cm} & \HoloSegMetric{HD95} & \HoloSegScore{227.5}{(218.1--237.4)}{4.55pt}{4.82pt}{} & \HoloSegScore{216.6}{(208.5--225.6)}{4.55pt}{4.82pt}{} & \HoloSegScore{11.97}{(3.101--28.67)}{4.55pt}{4.82pt}{} & \HoloSegScore{298.9}{(298.9--298.9)}{4.55pt}{4.82pt}{} & \HoloSegScore{13.60}{(12.53--14.31)}{4.55pt}{4.82pt}{} & \HoloSegScore{34.20}{(24.59--47.82)}{4.55pt}{4.82pt}{} & \HoloSegScore{8.379}{(0.9367--21.99)}{4.55pt}{4.82pt}{} \\
\cline{3-11}
 &  &  & \HoloSegMetric{Dice} & \HoloSegScore{0.0000}{(0.0000--0.0000)}{4.55pt}{4.82pt}{} & \HoloSegScore{0.0000}{(0.0000--0.0000)}{4.55pt}{4.82pt}{} & \HoloSegScore{0.8061}{(0.7329--0.8642)}{4.55pt}{4.82pt}{} & \HoloSegScore{0.0000}{(0.0000--0.0000)}{4.55pt}{4.82pt}{} & \HoloSegScore{0.7979}{(0.7927--0.8071)}{4.55pt}{4.82pt}{} & \HoloSegScore{0.7313}{(0.6718--0.7791)}{4.55pt}{4.82pt}{} & \HoloSegScore{0.8875}{(0.8325--0.9185)}{4.55pt}{4.82pt}{} \\*
\softcline{4-11}
 &  & \HoloSegSpan{\makecell[c]{right rib 3}}{2.04cm}{0.32cm} & \HoloSegMetric{HD95} & \HoloSegScore{213.5}{(208.5--219.0)}{4.55pt}{4.82pt}{} & \HoloSegScore{220.2}{(215.3--225.3)}{4.55pt}{4.82pt}{} & \HoloSegScore{6.308}{(2.856--11.17)}{4.55pt}{4.82pt}{} & \HoloSegScore{279.8}{(254.0--307.7)}{4.55pt}{4.82pt}{} & \HoloSegScore{6.677}{(4.253--12.01)}{4.55pt}{4.82pt}{} & \HoloSegScore{28.36}{(24.42--32.26)}{4.55pt}{4.82pt}{} & \HoloSegScore{3.284}{(1.104--7.394)}{4.55pt}{4.82pt}{} \\
\cline{3-11}
 &  &  & \HoloSegMetric{Dice} & \HoloSegScore{0.0000}{(0.0000--0.0000)}{4.55pt}{4.82pt}{} & \HoloSegScore{0.0000}{(0.0000--0.0000)}{4.55pt}{4.82pt}{} & \HoloSegScore{0.7814}{(0.6971--0.8553)}{4.55pt}{4.82pt}{} & \HoloSegScore{0.0000}{(0.0000--0.0000)}{4.55pt}{4.82pt}{} & \HoloSegScore{0.7715}{(0.7602--0.7726)}{4.55pt}{4.82pt}{} & \HoloSegScore{0.6545}{(0.5981--0.6924)}{4.55pt}{4.82pt}{} & \HoloSegScore{0.8582}{(0.7786--0.9194)}{4.55pt}{4.82pt}{} \\*
\softcline{4-11}
 &  & \HoloSegSpan{\makecell[c]{left rib 4}}{2.04cm}{0.32cm} & \HoloSegMetric{HD95} & \HoloSegScore{159.7}{(154.1--165.0)}{4.55pt}{4.82pt}{} & \HoloSegScore{164.3}{(158.9--169.7)}{4.55pt}{4.82pt}{} & \HoloSegScore{7.470}{(4.416--11.11)}{4.55pt}{4.82pt}{} & \HoloSegScore{189.9}{(179.8--200.3)}{4.55pt}{4.82pt}{} & \HoloSegScore{7.044}{(3.020--11.94)}{4.55pt}{4.82pt}{} & \HoloSegScore{178.8}{(167.9--189.1)}{4.55pt}{4.82pt}{} & \HoloSegScore{4.229}{(1.593--7.544)}{4.55pt}{4.82pt}{} \\
\cline{3-11}
 &  &  & \HoloSegMetric{Dice} & \HoloSegScore{0.0000}{(0.0000--0.0000)}{4.55pt}{4.82pt}{} & \HoloSegScore{0.0000}{(0.0000--0.0000)}{4.55pt}{4.82pt}{} & \HoloSegScore{0.8036}{(0.7327--0.8625)}{4.55pt}{4.82pt}{} & \HoloSegScore{0.0000}{(0.0000--0.0000)}{4.55pt}{4.82pt}{} & \HoloSegScore{0.7809}{(0.7769--0.7813)}{4.55pt}{4.82pt}{} & \HoloSegScore{0.7743}{(0.7175--0.8135)}{4.55pt}{4.82pt}{} & \HoloSegScore{0.9019}{(0.8464--0.9311)}{4.55pt}{4.82pt}{} \\*
\softcline{4-11}
 &  & \HoloSegSpan{\makecell[c]{right rib 4}}{2.04cm}{0.32cm} & \HoloSegMetric{HD95} & \HoloSegScore{160.5}{(156.3--165.0)}{4.55pt}{4.82pt}{} & \HoloSegScore{170.1}{(164.5--176.2)}{4.55pt}{4.82pt}{} & \HoloSegScore{5.985}{(2.412--10.65)}{4.55pt}{4.82pt}{} & \HoloSegScore{211.3}{(198.0--224.5)}{4.55pt}{4.82pt}{} & \HoloSegScore{8.714}{(3.735--13.39)}{4.55pt}{4.82pt}{} & \HoloSegScore{36.68}{(30.74--43.92)}{4.55pt}{4.82pt}{} & \HoloSegScore{3.432}{(0.8995--7.819)}{4.55pt}{4.82pt}{} \\
\cline{3-11}
 &  &  & \HoloSegMetric{Dice} & \HoloSegScore{0.0000}{(0.0000--0.0000)}{4.55pt}{4.82pt}{} & \HoloSegScore{0.0000}{(0.0000--0.0000)}{4.55pt}{4.82pt}{} & \HoloSegScore{0.7616}{(0.6606--0.8390)}{4.55pt}{4.82pt}{} & \HoloSegScore{0.0000}{(0.0000--0.0000)}{4.55pt}{4.82pt}{} & \HoloSegScore{0.7439}{(0.7365--0.7447)}{4.55pt}{4.82pt}{} & \HoloSegScore{0.8175}{(0.7319--0.8862)}{4.55pt}{4.82pt}{} & \HoloSegScore{0.8469}{(0.7685--0.9110)}{4.55pt}{4.82pt}{} \\*
\softcline{4-11}
 &  & \HoloSegSpan{\makecell[c]{left rib 5}}{2.04cm}{0.32cm} & \HoloSegMetric{HD95} & \HoloSegScore{108.5}{(101.8--117.4)}{4.55pt}{4.82pt}{} & \HoloSegScore{115.7}{(107.7--126.2)}{4.55pt}{4.82pt}{} & \HoloSegScore{16.57}{(5.943--33.02)}{4.55pt}{4.82pt}{} & \HoloSegScore{166.8}{(150.5--184.5)}{4.55pt}{4.82pt}{} & \HoloSegScore{20.16}{(12.66--29.90)}{4.55pt}{4.82pt}{} & \HoloSegScore{16.99}{(6.043--32.45)}{4.55pt}{4.82pt}{} & \HoloSegScore{13.15}{(2.246--28.49)}{4.55pt}{4.82pt}{} \\
\cline{3-11}
 &  &  & \HoloSegMetric{Dice} & \HoloSegScore{0.0000}{(0.0000--0.0000)}{4.55pt}{4.82pt}{} & \HoloSegScore{0.0000}{(0.0000--0.0000)}{4.55pt}{4.82pt}{} & \HoloSegScore{0.7945}{(0.7215--0.8514)}{4.55pt}{4.82pt}{} & \HoloSegScore{0.0000}{(0.0000--0.0000)}{4.55pt}{4.82pt}{} & \HoloSegScore{0.7794}{(0.7718--0.7855)}{4.55pt}{4.82pt}{} & \HoloSegScore{0.8766}{(0.8192--0.9099)}{4.55pt}{4.82pt}{} & \HoloSegScore{0.8869}{(0.8311--0.9185)}{4.55pt}{4.82pt}{} \\*
\softcline{4-11}
 &  & \HoloSegSpan{\makecell[c]{right rib 5}}{2.04cm}{0.32cm} & \HoloSegMetric{HD95} & \HoloSegScore{103.7}{(100.1--107.2)}{4.55pt}{4.82pt}{} & \HoloSegScore{116.9}{(112.0--121.6)}{4.55pt}{4.82pt}{} & \HoloSegScore{5.993}{(2.725--10.70)}{4.55pt}{4.82pt}{} & \HoloSegScore{158.7}{(145.3--173.5)}{4.55pt}{4.82pt}{} & \HoloSegScore{9.059}{(6.756--13.63)}{4.55pt}{4.82pt}{} & \HoloSegScore{5.986}{(2.038--10.31)}{4.55pt}{4.82pt}{} & \HoloSegScore{4.832}{(0.9457--9.613)}{4.55pt}{4.82pt}{} \\
\cline{3-11}
 &  &  & \HoloSegMetric{Dice} & \HoloSegScore{0.03498}{(0.006075--0.07448)}{3.85pt}{4.12pt}{} & \HoloSegScore{0.01384}{(0.007653--0.02123)}{3.85pt}{4.12pt}{} & \HoloSegScore{0.8008}{(0.7258--0.8626)}{4.55pt}{4.82pt}{} & \HoloSegScore{0.8408}{(0.7673--0.9056)}{4.55pt}{4.82pt}{} & \HoloSegScore{0.8353}{(0.8168--0.8561)}{4.55pt}{4.82pt}{} & \HoloSegScore{0.6925}{(0.6299--0.7575)}{4.55pt}{4.82pt}{} & \HoloSegScore{0.8828}{(0.8360--0.9195)}{4.55pt}{4.82pt}{} \\*
\softcline{4-11}
\HoloSegSpan{\makecell[c]{\textbf{Internal}}}{1.20cm}{0.32cm} & \HoloSegSpan{\makecell[c]{DAP-Atlas\\[-0.10ex](AutoPETIII)}}{1.86cm}{0.32cm} & \HoloSegSpan{\makecell[c]{left rib 6}}{2.04cm}{0.32cm} & \HoloSegMetric{HD95} & \HoloSegScore{38.75}{(35.25--42.84)}{4.55pt}{4.82pt}{} & \HoloSegScore{61.33}{(56.42--66.46)}{4.55pt}{4.82pt}{} & \HoloSegScore{7.162}{(3.859--11.49)}{4.55pt}{4.82pt}{} & \HoloSegScore{9.775}{(5.861--13.59)}{4.55pt}{4.82pt}{} & \HoloSegScore{7.435}{(3.558--10.66)}{4.55pt}{4.82pt}{} & \HoloSegScore{20.93}{(16.82--24.54)}{4.55pt}{4.82pt}{} & \HoloSegScore{5.378}{(1.913--9.863)}{4.55pt}{4.82pt}{} \\
\cline{3-11}
 &  &  & \HoloSegMetric{Dice} & \HoloSegScore{0.04803}{(0.01547--0.09125)}{4.20pt}{4.48pt}{} & \HoloSegScore{0.008577}{(0.002090--0.01766)}{3.85pt}{4.12pt}{} & \HoloSegScore{0.7928}{(0.7256--0.8428)}{4.55pt}{4.82pt}{} & \HoloSegScore{0.8795}{(0.8132--0.9249)}{4.55pt}{4.82pt}{} & \HoloSegScore{0.8528}{(0.8449--0.8635)}{4.55pt}{4.82pt}{} & \HoloSegScore{0.7825}{(0.7190--0.8305)}{4.55pt}{4.82pt}{} & \HoloSegScore{0.8913}{(0.8332--0.9247)}{4.55pt}{4.82pt}{} \\*
\softcline{4-11}
 &  & \HoloSegSpan{\makecell[c]{right rib 6}}{2.04cm}{0.32cm} & \HoloSegMetric{HD95} & \HoloSegScore{48.16}{(35.06--69.09)}{4.55pt}{4.82pt}{} & \HoloSegScore{94.67}{(77.44--113.3)}{4.55pt}{4.82pt}{} & \HoloSegScore{8.075}{(3.956--13.77)}{4.55pt}{4.82pt}{} & \HoloSegScore{10.31}{(5.466--15.71)}{4.55pt}{4.82pt}{} & \HoloSegScore{7.632}{(3.311--11.70)}{4.55pt}{4.82pt}{} & \HoloSegScore{23.06}{(19.16--26.80)}{4.55pt}{4.82pt}{} & \HoloSegScore{5.215}{(0.9992--11.09)}{4.55pt}{4.82pt}{} \\
\cline{3-11}
 &  &  & \HoloSegMetric{Dice} & \HoloSegScore{0.05600}{(0.006283--0.1203)}{4.20pt}{4.48pt}{} & \HoloSegScore{0.1169}{(0.09759--0.1367)}{4.20pt}{4.48pt}{} & \HoloSegScore{0.7754}{(0.6882--0.8498)}{4.55pt}{4.82pt}{} & \HoloSegScore{0.8414}{(0.7519--0.9124)}{4.55pt}{4.82pt}{} & \HoloSegScore{0.8179}{(0.7930--0.8311)}{4.55pt}{4.82pt}{} & \HoloSegScore{0.6368}{(0.5791--0.6923)}{4.55pt}{4.82pt}{} & \HoloSegScore{0.8661}{(0.8345--0.8923)}{4.55pt}{4.82pt}{} \\*
\softcline{4-11}
 &  & \HoloSegSpan{\makecell[c]{left rib 7}}{2.04cm}{0.32cm} & \HoloSegMetric{HD95} & \HoloSegScore{36.14}{(33.79--38.77)}{4.55pt}{4.82pt}{} & \HoloSegScore{40.27}{(36.22--44.47)}{4.55pt}{4.82pt}{} & \HoloSegScore{7.266}{(3.834--11.57)}{4.55pt}{4.82pt}{} & \HoloSegScore{9.182}{(5.219--12.99)}{4.55pt}{4.82pt}{} & \HoloSegScore{8.917}{(7.668--10.43)}{4.55pt}{4.82pt}{} & \HoloSegScore{24.14}{(22.24--25.92)}{4.55pt}{4.82pt}{} & \HoloSegScore{7.022}{(3.074--12.17)}{4.55pt}{4.82pt}{} \\
\cline{3-11}
 &  &  & \HoloSegMetric{Dice} & \HoloSegScore{0.01763}{(0.001467--0.04477)}{3.85pt}{4.12pt}{} & \HoloSegScore{0.1298}{(0.1072--0.1524)}{4.55pt}{4.82pt}{} & \HoloSegScore{0.7912}{(0.7118--0.8455)}{4.55pt}{4.82pt}{} & \HoloSegScore{0.8693}{(0.7863--0.9288)}{4.55pt}{4.82pt}{} & \HoloSegScore{0.7878}{(0.7589--0.8255)}{4.55pt}{4.82pt}{} & \HoloSegScore{0.6777}{(0.6125--0.7335)}{4.55pt}{4.82pt}{} & \HoloSegScore{0.8814}{(0.8253--0.9138)}{4.55pt}{4.82pt}{} \\*
\softcline{4-11}
 &  & \HoloSegSpan{\makecell[c]{right rib 7}}{2.04cm}{0.32cm} & \HoloSegMetric{HD95} & \HoloSegScore{38.03}{(35.63--40.97)}{4.55pt}{4.82pt}{} & \HoloSegScore{40.43}{(33.90--47.43)}{4.55pt}{4.82pt}{} & \HoloSegScore{6.101}{(3.036--11.17)}{4.55pt}{4.82pt}{} & \HoloSegScore{10.83}{(6.243--16.10)}{4.55pt}{4.82pt}{} & \HoloSegScore{10.10}{(7.682--12.52)}{4.55pt}{4.82pt}{} & \HoloSegScore{24.89}{(22.14--28.34)}{4.55pt}{4.82pt}{} & \HoloSegScore{5.009}{(1.683--10.74)}{4.55pt}{4.82pt}{} \\
\cline{3-11}
 &  &  & \HoloSegMetric{Dice} & \HoloSegScore{0.0000}{(0.0000--0.0000)}{4.55pt}{4.82pt}{} & \HoloSegScore{0.001722}{(0.0000--0.005053)}{4.20pt}{4.48pt}{} & \HoloSegScore{0.7498}{(0.6549--0.8283)}{4.55pt}{4.82pt}{} & \HoloSegScore{0.0000}{(0.0000--0.0000)}{4.55pt}{4.82pt}{} & \HoloSegScore{0.7123}{(0.6958--0.7165)}{4.55pt}{4.82pt}{} & \HoloSegScore{0.3965}{(0.3275--0.4670)}{4.55pt}{4.82pt}{} & \HoloSegScore{0.8754}{(0.8457--0.8988)}{4.55pt}{4.82pt}{} \\*
\softcline{4-11}
 &  & \HoloSegSpan{\makecell[c]{left rib 8}}{2.04cm}{0.32cm} & \HoloSegMetric{HD95} & \HoloSegScore{104.7}{(99.97--109.3)}{4.55pt}{4.82pt}{} & \HoloSegScore{81.06}{(76.53--85.52)}{4.55pt}{4.82pt}{} & \HoloSegScore{9.550}{(4.742--15.71)}{4.55pt}{4.82pt}{} & \HoloSegScore{173.1}{(139.0--205.9)}{4.55pt}{4.82pt}{} & \HoloSegScore{10.43}{(6.927--14.70)}{4.55pt}{4.82pt}{} & \HoloSegScore{21.92}{(19.80--23.93)}{4.55pt}{4.82pt}{} & \HoloSegScore{5.318}{(2.148--9.859)}{4.55pt}{4.82pt}{} \\
\cline{3-11}
 &  &  & \HoloSegMetric{Dice} & \HoloSegScore{0.0004303}{(0.0000--0.001291)}{4.20pt}{4.48pt}{} & \HoloSegScore{0.006221}{(0.00001330--0.01751)}{3.52pt}{3.80pt}{} & \HoloSegScore{0.7834}{(0.7100--0.8365)}{4.55pt}{4.82pt}{} & \HoloSegScore{0.0000}{(0.0000--0.0000)}{4.55pt}{4.82pt}{} & \HoloSegScore{0.7785}{(0.7732--0.7816)}{4.55pt}{4.82pt}{} & \HoloSegScore{0.3387}{(0.2788--0.4004)}{4.55pt}{4.82pt}{} & \HoloSegScore{0.8886}{(0.8334--0.9202)}{4.55pt}{4.82pt}{} \\*
\softcline{4-11}
 &  & \HoloSegSpan{\makecell[c]{right rib 8}}{2.04cm}{0.32cm} & \HoloSegMetric{HD95} & \HoloSegScore{127.6}{(106.8--152.4)}{4.55pt}{4.82pt}{} & \HoloSegScore{76.60}{(71.65--81.08)}{4.55pt}{4.82pt}{} & \HoloSegScore{5.766}{(2.967--9.718)}{4.55pt}{4.82pt}{} & \HoloSegScore{176.9}{(142.0--212.1)}{4.55pt}{4.82pt}{} & \HoloSegScore{6.514}{(3.465--12.39)}{4.55pt}{4.82pt}{} & \HoloSegScore{24.76}{(22.78--27.23)}{4.55pt}{4.82pt}{} & \HoloSegScore{3.792}{(1.543--7.700)}{4.55pt}{4.82pt}{} \\
\cline{3-11}
 &  &  & \HoloSegMetric{Dice} & \HoloSegScore{0.0000}{(0.0000--0.0000)}{4.55pt}{4.82pt}{} & \HoloSegScore{0.0000}{(0.0000--0.0000)}{4.55pt}{4.82pt}{} & \HoloSegScore{0.7535}{(0.6645--0.8213)}{4.55pt}{4.82pt}{} & \HoloSegScore{0.8421}{(0.7421--0.9207)}{4.55pt}{4.82pt}{} & \HoloSegScore{0.8154}{(0.8015--0.8206)}{4.55pt}{4.82pt}{} & \HoloSegScore{0.5507}{(0.4867--0.5983)}{4.55pt}{4.82pt}{} & \HoloSegScore{0.8766}{(0.8408--0.9049)}{4.55pt}{4.82pt}{} \\*
\softcline{4-11}
 &  & \HoloSegSpan{\makecell[c]{left rib 9}}{2.04cm}{0.32cm} & \HoloSegMetric{HD95} & \HoloSegScore{164.6}{(158.9--171.2)}{4.55pt}{4.82pt}{} & \HoloSegScore{135.8}{(129.8--141.7)}{4.55pt}{4.82pt}{} & \HoloSegScore{11.28}{(4.818--21.08)}{4.55pt}{4.82pt}{} & \HoloSegScore{5.300}{(2.402--8.808)}{4.55pt}{4.82pt}{} & \HoloSegScore{8.459}{(4.534--13.17)}{4.55pt}{4.82pt}{} & \HoloSegScore{30.78}{(24.92--39.37)}{4.55pt}{4.82pt}{} & \HoloSegScore{10.94}{(4.196--20.82)}{4.55pt}{4.82pt}{} \\
\cline{3-11}
 &  &  & \HoloSegMetric{Dice} & \HoloSegScore{0.0000}{(0.0000--0.0000)}{4.55pt}{4.82pt}{} & \HoloSegScore{0.0000}{(0.0000--0.0000)}{4.55pt}{4.82pt}{} & \HoloSegScore{0.7678}{(0.6983--0.8197)}{4.55pt}{4.82pt}{} & \HoloSegScore{0.8798}{(0.7975--0.9350)}{4.55pt}{4.82pt}{} & \HoloSegScore{0.7603}{(0.7482--0.7684)}{4.55pt}{4.82pt}{} & \HoloSegScore{0.5612}{(0.5077--0.6102)}{4.55pt}{4.82pt}{} & \HoloSegScore{0.8923}{(0.8374--0.9227)}{4.55pt}{4.82pt}{} \\*
\softcline{4-11}
 &  & \HoloSegSpan{\makecell[c]{right rib 9}}{2.04cm}{0.32cm} & \HoloSegMetric{HD95} & \HoloSegScore{186.8}{(168.8--207.5)}{4.55pt}{4.82pt}{} & \HoloSegScore{132.5}{(125.1--139.2)}{4.55pt}{4.82pt}{} & \HoloSegScore{5.421}{(2.584--9.582)}{4.55pt}{4.82pt}{} & \HoloSegScore{4.869}{(1.460--9.581)}{4.55pt}{4.82pt}{} & \HoloSegScore{6.220}{(4.330--12.33)}{4.55pt}{4.82pt}{} & \HoloSegScore{24.74}{(23.04--26.78)}{4.55pt}{4.82pt}{} & \HoloSegScore{3.293}{(1.006--7.497)}{4.55pt}{4.82pt}{} \\
\cline{3-11}
 &  &  & \HoloSegMetric{Dice} & \HoloSegScore{0.0000}{(0.0000--0.0000)}{4.55pt}{4.82pt}{} & \HoloSegScore{0.0000}{(0.0000--0.0000)}{4.55pt}{4.82pt}{} & \HoloSegScore{0.7451}{(0.6666--0.8074)}{4.55pt}{4.82pt}{} & \HoloSegScore{0.8350}{(0.7417--0.9106)}{4.55pt}{4.82pt}{} & \HoloSegScore{0.7343}{(0.7195--0.7368)}{4.55pt}{4.82pt}{} & \HoloSegScore{0.6687}{(0.6071--0.7237)}{4.55pt}{4.82pt}{} & \HoloSegScore{0.8501}{(0.8024--0.8920)}{4.55pt}{4.82pt}{} \\*
\softcline{4-11}
 &  & \HoloSegSpan{\makecell[c]{left rib 10}}{2.04cm}{0.32cm} & \HoloSegMetric{HD95} & \HoloSegScore{222.7}{(216.8--229.3)}{4.55pt}{4.82pt}{} & \HoloSegScore{189.3}{(183.0--195.5)}{4.55pt}{4.82pt}{} & \HoloSegScore{18.42}{(4.726--37.01)}{4.55pt}{4.82pt}{} & \HoloSegScore{6.436}{(2.736--10.58)}{4.55pt}{4.82pt}{} & \HoloSegScore{7.472}{(2.577--11.44)}{4.55pt}{4.82pt}{} & \HoloSegScore{29.29}{(23.04--39.76)}{4.55pt}{4.82pt}{} & \HoloSegScore{8.170}{(4.556--12.18)}{4.55pt}{4.82pt}{} \\
\cline{3-11}
 &  &  & \HoloSegMetric{Dice} & \HoloSegScore{0.0000}{(0.0000--0.0000)}{4.55pt}{4.82pt}{} & \HoloSegScore{0.0000}{(0.0000--0.0000)}{4.55pt}{4.82pt}{} & \HoloSegScore{0.7573}{(0.7008--0.7970)}{4.55pt}{4.82pt}{} & \HoloSegScore{0.8833}{(0.8136--0.9294)}{4.55pt}{4.82pt}{} & \HoloSegScore{0.8469}{(0.8435--0.8587)}{4.55pt}{4.82pt}{} & \HoloSegScore{0.8015}{(0.7522--0.8394)}{4.55pt}{4.82pt}{} & \HoloSegScore{0.8829}{(0.8486--0.9075)}{4.55pt}{4.82pt}{} \\*
\softcline{4-11}
 &  & \HoloSegSpan{\makecell[c]{right rib 10}}{2.04cm}{0.32cm} & \HoloSegMetric{HD95} & \HoloSegScore{36.42}{(31.15--41.83)}{4.55pt}{4.82pt}{} & \HoloSegScore{186.2}{(178.2--193.0)}{4.55pt}{4.82pt}{} & \HoloSegScore{5.291}{(2.500--8.643)}{4.55pt}{4.82pt}{} & \HoloSegScore{9.410}{(1.007--24.49)}{4.55pt}{4.82pt}{} & \HoloSegScore{6.317}{(5.008--11.28)}{4.55pt}{4.82pt}{} & \HoloSegScore{16.01}{(12.74--19.50)}{4.55pt}{4.82pt}{} & \HoloSegScore{4.370}{(1.947--7.824)}{4.55pt}{4.82pt}{} \\
\hline
\pagebreak[4]
 &  &  & \HoloSegMetric{Dice} & \HoloSegScore{0.0000}{(0.0000--0.0000)}{4.55pt}{4.82pt}{} & \HoloSegScore{0.0000}{(0.0000--0.0000)}{4.55pt}{4.82pt}{} & \HoloSegScore{0.6567}{(0.5751--0.7249)}{4.55pt}{4.82pt}{} & \HoloSegScore{0.8215}{(0.7182--0.9033)}{4.55pt}{4.82pt}{} & \HoloSegScore{0.8162}{(0.8081--0.8215)}{4.55pt}{4.82pt}{} & \HoloSegScore{0.7618}{(0.6705--0.8301)}{4.55pt}{4.82pt}{} & \HoloSegScore{0.8394}{(0.7657--0.8949)}{4.55pt}{4.82pt}{} \\*
\softcline{4-11}
 &  & \HoloSegSpan{\makecell[c]{left rib 11}}{2.04cm}{0.32cm} & \HoloSegMetric{HD95} & \HoloSegScore{275.8}{(270.0--281.6)}{4.55pt}{4.82pt}{} & \HoloSegScore{236.5}{(230.5--242.8)}{4.55pt}{4.82pt}{} & \HoloSegScore{158.7}{(113.9--200.2)}{4.55pt}{4.82pt}{} & \HoloSegScore{5.350}{(1.948--9.408)}{4.55pt}{4.82pt}{} & \HoloSegScore{5.920}{(2.209--10.12)}{4.55pt}{4.82pt}{} & \HoloSegScore{33.87}{(11.98--60.50)}{4.55pt}{4.82pt}{} & \HoloSegScore{7.218}{(3.470--11.64)}{4.55pt}{4.82pt}{} \\
\cline{3-11}
 &  &  & \HoloSegMetric{Dice} & \HoloSegScore{0.0000}{(0.0000--0.0000)}{4.55pt}{4.82pt}{} & \HoloSegScore{0.0000}{(0.0000--0.0000)}{4.55pt}{4.82pt}{} & \HoloSegScore{0.6795}{(0.5988--0.7405)}{4.55pt}{4.82pt}{} & \HoloSegScore{0.8431}{(0.7598--0.9228)}{4.55pt}{4.82pt}{} & \HoloSegScore{0.6684}{(0.6572--0.6761)}{4.55pt}{4.82pt}{} & \HoloSegScore{0.8112}{(0.7345--0.8761)}{4.55pt}{4.82pt}{} & \HoloSegScore{0.8699}{(0.8228--0.9066)}{4.55pt}{4.82pt}{} \\*
\softcline{4-11}
 &  & \HoloSegSpan{\makecell[c]{right rib 11}}{2.04cm}{0.32cm} & \HoloSegMetric{HD95} & \HoloSegScore{269.5}{(264.8--274.0)}{4.55pt}{4.82pt}{} & \HoloSegScore{231.7}{(225.5--238.5)}{4.55pt}{4.82pt}{} & \HoloSegScore{133.5}{(91.90--174.9)}{4.55pt}{4.82pt}{} & \HoloSegScore{3.825}{(1.289--6.959)}{4.55pt}{4.82pt}{} & \HoloSegScore{5.081}{(2.618--8.333)}{4.55pt}{4.82pt}{} & \HoloSegScore{8.034}{(3.905--12.68)}{4.55pt}{4.82pt}{} & \HoloSegScore{4.726}{(2.096--8.500)}{4.55pt}{4.82pt}{} \\
\cline{3-11}
 &  &  & \HoloSegMetric{Dice} & \HoloSegScore{0.0000}{(0.0000--0.0000)}{4.55pt}{4.82pt}{} & \HoloSegScore{0.0000}{(0.0000--0.0000)}{4.55pt}{4.82pt}{} & \HoloSegScore{0.6567}{(0.5732--0.7254)}{4.55pt}{4.82pt}{} & \HoloSegScore{0.8071}{(0.7029--0.8883)}{4.55pt}{4.82pt}{} & \HoloSegScore{0.8000}{(0.7981--0.8044)}{4.55pt}{4.82pt}{} & \HoloSegScore{0.7527}{(0.6694--0.8239)}{4.55pt}{4.82pt}{} & \HoloSegScore{0.8147}{(0.7255--0.8889)}{4.55pt}{4.82pt}{} \\*
\softcline{4-11}
 &  & \HoloSegSpan{\makecell[c]{left rib 12}}{2.04cm}{0.32cm} & \HoloSegMetric{HD95} & \HoloSegScore{293.0}{(285.1--299.5)}{4.55pt}{4.82pt}{} & \HoloSegScore{266.5}{(258.8--276.1)}{4.55pt}{4.82pt}{} & \HoloSegScore{160.2}{(115.6--204.7)}{4.55pt}{4.82pt}{} & \HoloSegScore{10.59}{(2.381--20.61)}{4.55pt}{4.82pt}{} & \HoloSegScore{14.22}{(7.281--21.41)}{4.55pt}{4.82pt}{} & \HoloSegScore{187.5}{(148.8--224.2)}{4.55pt}{4.82pt}{} & \HoloSegScore{10.69}{(2.719--20.55)}{4.55pt}{4.82pt}{} \\
\cline{3-11}
 &  &  & \HoloSegMetric{Dice} & \HoloSegScore{0.0000}{(0.0000--0.0000)}{4.55pt}{4.82pt}{} & \HoloSegScore{0.0000}{(0.0000--0.0000)}{4.55pt}{4.82pt}{} & \HoloSegScore{0.6617}{(0.5933--0.7222)}{4.55pt}{4.82pt}{} & \HoloSegScore{0.8167}{(0.7267--0.8955)}{4.55pt}{4.82pt}{} & \HoloSegScore{0.7891}{(0.7802--0.7979)}{4.55pt}{4.82pt}{} & \HoloSegScore{0.7979}{(0.7378--0.8493)}{4.55pt}{4.82pt}{} & \HoloSegScore{0.8572}{(0.7990--0.8979)}{4.55pt}{4.82pt}{} \\*
\softcline{4-11}
 &  & \HoloSegSpan{\makecell[c]{right rib 12}}{2.04cm}{0.32cm} & \HoloSegMetric{HD95} & \HoloSegScore{290.5}{(284.0--297.7)}{4.55pt}{4.82pt}{} & \HoloSegScore{260.1}{(251.3--269.5)}{4.55pt}{4.82pt}{} & \HoloSegScore{158.6}{(115.6--200.6)}{4.55pt}{4.82pt}{} & \HoloSegScore{9.132}{(3.362--15.68)}{4.55pt}{4.82pt}{} & \HoloSegScore{11.69}{(4.299--16.96)}{4.55pt}{4.82pt}{} & \HoloSegScore{33.50}{(16.34--56.27)}{4.55pt}{4.82pt}{} & \HoloSegScore{7.081}{(2.707--12.59)}{4.55pt}{4.82pt}{} \\
\cline{3-11}
 &  &  & \HoloSegMetric{Dice} & \HoloSegScore{0.7651}{(0.7524--0.7776)}{4.55pt}{4.82pt}{} & \HoloSegScore{0.004292}{(0.001973--0.006857)}{3.85pt}{4.12pt}{} & \HoloSegScore{0.8707}{(0.8614--0.8791)}{4.55pt}{4.82pt}{} & \HoloSegScore{0.8665}{(0.8527--0.8779)}{4.55pt}{4.82pt}{} & \HoloSegScore{0.8487}{(0.8341--0.8704)}{4.55pt}{4.82pt}{} & \HoloSegScore{0.8162}{(0.8026--0.8276)}{4.55pt}{4.82pt}{} & \HoloSegScore{0.8314}{(0.8172--0.8438)}{4.55pt}{4.82pt}{} \\*
\softcline{4-11}
 &  & \HoloSegSpan{\makecell[c]{rib\\[-0.10ex]cartilage}}{2.04cm}{0.32cm} & \HoloSegMetric{HD95} & \HoloSegScore{39.58}{(26.14--54.30)}{4.55pt}{4.82pt}{} & \HoloSegScore{262.7}{(239.3--291.8)}{4.55pt}{4.82pt}{} & \HoloSegScore{4.480}{(2.825--6.827)}{4.55pt}{4.82pt}{} & \HoloSegScore{51.17}{(29.20--77.69)}{4.55pt}{4.82pt}{} & \HoloSegScore{5.076}{(3.219--7.223)}{4.55pt}{4.82pt}{} & \HoloSegScore{60.84}{(38.93--89.34)}{4.55pt}{4.82pt}{} & \HoloSegScore{58.09}{(36.45--86.83)}{4.55pt}{4.82pt}{} \\
\cline{3-11}
 &  &  & \HoloSegMetric{Dice} & \HoloSegScore{0.6086}{(0.5766--0.6299)}{4.55pt}{4.82pt}{} & \HoloSegScore{0.0000}{(0.0000--0.0000)}{4.55pt}{4.82pt}{} & \HoloSegScore{0.8617}{(0.8035--0.8962)}{4.55pt}{4.82pt}{} & \HoloSegScore{0.6398}{(0.5998--0.6640)}{4.55pt}{4.82pt}{} & \HoloSegScore{0.8090}{(0.7799--0.8267)}{4.55pt}{4.82pt}{} & \HoloSegScore{0.8767}{(0.8142--0.9136)}{4.55pt}{4.82pt}{} & \HoloSegScore{0.8783}{(0.8135--0.9151)}{4.55pt}{4.82pt}{} \\*
\softcline{4-11}
 &  & \HoloSegSpan{\makecell[c]{sternum}}{2.04cm}{0.32cm} & \HoloSegMetric{HD95} & \HoloSegScore{83.57}{(59.88--111.4)}{4.55pt}{4.82pt}{} & \HoloSegScore{209.1}{(188.2--233.9)}{4.55pt}{4.82pt}{} & \HoloSegScore{38.07}{(13.26--68.86)}{4.55pt}{4.82pt}{} & \HoloSegScore{87.02}{(60.05--117.0)}{4.55pt}{4.82pt}{} & \HoloSegScore{42.71}{(22.34--67.87)}{4.55pt}{4.82pt}{} & \HoloSegScore{50.43}{(20.30--89.72)}{4.55pt}{4.82pt}{} & \HoloSegScore{49.92}{(19.79--89.78)}{4.55pt}{4.82pt}{} \\
\cline{3-11}
 &  &  & \HoloSegMetric{Dice} & \HoloSegScore{0.9119}{(0.9015--0.9208)}{4.55pt}{4.82pt}{} & \HoloSegScore{0.1040}{(0.07896--0.1290)}{4.20pt}{4.48pt}{} & \HoloSegScore{0.9000}{(0.8934--0.9067)}{4.55pt}{4.82pt}{} & \HoloSegScore{0.9497}{(0.9464--0.9525)}{4.55pt}{4.82pt}{} & \HoloSegScore{0.9430}{(0.9346--0.9472)}{4.55pt}{4.82pt}{} & \HoloSegScore{0.9515}{(0.9440--0.9577)}{4.55pt}{4.82pt}{} & \HoloSegScore{0.9505}{(0.9456--0.9545)}{4.55pt}{4.82pt}{} \\*
\softcline{4-11}
 &  & \HoloSegSpan{\makecell[c]{left\\[-0.10ex]clavicle}}{2.04cm}{0.32cm} & \HoloSegMetric{HD95} & \HoloSegScore{29.38}{(4.073--62.78)}{4.55pt}{4.82pt}{} & \HoloSegScore{66.41}{(52.36--80.13)}{4.55pt}{4.82pt}{} & \HoloSegScore{2.408}{(2.338--2.468)}{4.55pt}{4.82pt}{} & \HoloSegScore{0.9654}{(0.8845--1.077)}{4.55pt}{4.82pt}{} & \HoloSegScore{2.854}{(1.913--3.932)}{4.55pt}{4.82pt}{} & \HoloSegScore{11.02}{(1.064--28.48)}{4.55pt}{4.82pt}{} & \HoloSegScore{1.012}{(0.9015--1.151)}{4.55pt}{4.82pt}{} \\
\cline{3-11}
 &  &  & \HoloSegMetric{Dice} & \HoloSegScore{0.9150}{(0.9101--0.9192)}{4.55pt}{4.82pt}{} & \HoloSegScore{0.1167}{(0.08780--0.1434)}{4.20pt}{4.48pt}{} & \HoloSegScore{0.8997}{(0.8924--0.9067)}{4.55pt}{4.82pt}{} & \HoloSegScore{0.9508}{(0.9484--0.9531)}{4.55pt}{4.82pt}{} & \HoloSegScore{0.9361}{(0.9337--0.9435)}{4.55pt}{4.82pt}{} & \HoloSegScore{0.9536}{(0.9506--0.9570)}{4.55pt}{4.82pt}{} & \HoloSegScore{0.9508}{(0.9475--0.9539)}{4.55pt}{4.82pt}{} \\*
\softcline{4-11}
 &  & \HoloSegSpan{\makecell[c]{right\\[-0.10ex]clavicle}}{2.04cm}{0.32cm} & \HoloSegMetric{HD95} & \HoloSegScore{43.17}{(4.440--97.51)}{4.55pt}{4.82pt}{} & \HoloSegScore{74.00}{(61.34--86.97)}{4.55pt}{4.82pt}{} & \HoloSegScore{48.91}{(2.467--109.7)}{4.55pt}{4.82pt}{} & \HoloSegScore{0.9665}{(0.8961--1.045)}{4.55pt}{4.82pt}{} & \HoloSegScore{4.045}{(3.026--4.748)}{4.55pt}{4.82pt}{} & \HoloSegScore{2.528}{(1.339--4.255)}{4.55pt}{4.82pt}{} & \HoloSegScore{1.101}{(0.9699--1.238)}{4.55pt}{4.82pt}{} \\
\cline{3-11}
 &  &  & \HoloSegMetric{Dice} & \HoloSegScore{0.8681}{(0.8550--0.8797)}{4.55pt}{4.82pt}{} & \HoloSegScore{0.4403}{(0.4199--0.4584)}{4.55pt}{4.82pt}{} & \HoloSegScore{0.9127}{(0.9080--0.9164)}{4.55pt}{4.82pt}{} & \HoloSegScore{0.9290}{(0.9263--0.9311)}{4.55pt}{4.82pt}{} & \HoloSegScore{0.9020}{(0.8858--0.9066)}{4.55pt}{4.82pt}{} & \HoloSegScore{0.9299}{(0.9221--0.9355)}{4.55pt}{4.82pt}{} & \HoloSegScore{0.9362}{(0.9319--0.9393)}{4.55pt}{4.82pt}{} \\*
\softcline{4-11}
 &  & \HoloSegSpan{\makecell[c]{left scapula}}{2.04cm}{0.32cm} & \HoloSegMetric{HD95} & \HoloSegScore{11.21}{(6.958--15.63)}{4.55pt}{4.82pt}{} & \HoloSegScore{25.78}{(19.56--35.64)}{4.55pt}{4.82pt}{} & \HoloSegScore{1.859}{(1.790--1.937)}{4.55pt}{4.82pt}{} & \HoloSegScore{0.9944}{(0.9189--1.100)}{4.55pt}{4.82pt}{} & \HoloSegScore{2.518}{(2.008--4.047)}{4.55pt}{4.82pt}{} & \HoloSegScore{1.858}{(0.9838--3.114)}{4.55pt}{4.82pt}{} & \HoloSegScore{0.9449}{(0.8768--1.035)}{4.55pt}{4.82pt}{} \\
\cline{3-11}
 &  &  & \HoloSegMetric{Dice} & \HoloSegScore{0.8925}{(0.8821--0.9010)}{4.55pt}{4.82pt}{} & \HoloSegScore{0.4064}{(0.3834--0.4258)}{4.55pt}{4.82pt}{} & \HoloSegScore{0.9126}{(0.9049--0.9181)}{4.55pt}{4.82pt}{} & \HoloSegScore{0.9278}{(0.9218--0.9322)}{4.55pt}{4.82pt}{} & \HoloSegScore{0.9032}{(0.8891--0.9069)}{4.55pt}{4.82pt}{} & \HoloSegScore{0.9212}{(0.9154--0.9268)}{4.55pt}{4.82pt}{} & \HoloSegScore{0.9370}{(0.9330--0.9406)}{4.55pt}{4.82pt}{} \\*
\softcline{4-11}
\HoloSegSpan{\makecell[c]{\textbf{Internal}}}{1.20cm}{0.32cm} & \HoloSegSpan{\makecell[c]{DAP-Atlas\\[-0.10ex](AutoPETIII)}}{1.86cm}{0.32cm} & \HoloSegSpan{\makecell[c]{right\\[-0.10ex]scapula}}{2.04cm}{0.32cm} & \HoloSegMetric{HD95} & \HoloSegScore{11.68}{(8.108--15.05)}{4.55pt}{4.82pt}{} & \HoloSegScore{36.79}{(25.11--51.11)}{4.55pt}{4.82pt}{} & \HoloSegScore{2.218}{(1.823--2.919)}{4.55pt}{4.82pt}{} & \HoloSegScore{1.718}{(0.9676--3.054)}{4.55pt}{4.82pt}{} & \HoloSegScore{1.870}{(1.610--3.240)}{4.55pt}{4.82pt}{} & \HoloSegScore{7.234}{(2.445--14.64)}{4.55pt}{4.82pt}{} & \HoloSegScore{1.188}{(0.9483--1.529)}{4.55pt}{4.82pt}{} \\
\cline{3-11}
 &  &  & \HoloSegMetric{Dice} & \HoloSegScore{0.4440}{(0.4258--0.4631)}{4.55pt}{4.82pt}{} & \HoloSegScore{0.3937}{(0.3594--0.4244)}{4.55pt}{4.82pt}{} & \HoloSegScore{0.9260}{(0.9118--0.9373)}{4.55pt}{4.82pt}{} & \HoloSegScore{0.9145}{(0.8986--0.9284)}{4.55pt}{4.82pt}{} & \HoloSegScore{0.9212}{(0.9131--0.9284)}{4.55pt}{4.82pt}{} & \HoloSegScore{0.9318}{(0.9190--0.9424)}{4.55pt}{4.82pt}{} & \HoloSegScore{0.9473}{(0.9383--0.9556)}{4.55pt}{4.82pt}{} \\*
\softcline{4-11}
 &  & \HoloSegSpan{\makecell[c]{left humerus}}{2.04cm}{0.32cm} & \HoloSegMetric{HD95} & \HoloSegScore{71.47}{(69.86--72.97)}{4.55pt}{4.82pt}{} & \HoloSegScore{38.73}{(28.62--51.20)}{4.55pt}{4.82pt}{} & \HoloSegScore{15.29}{(2.654--36.41)}{4.55pt}{4.82pt}{} & \HoloSegScore{27.70}{(10.50--48.53)}{4.55pt}{4.82pt}{} & \HoloSegScore{15.96}{(5.705--29.08)}{4.55pt}{4.82pt}{} & \HoloSegScore{20.51}{(8.737--34.91)}{4.55pt}{4.82pt}{} & \HoloSegScore{5.814}{(2.690--9.590)}{4.55pt}{4.82pt}{} \\
\cline{3-11}
 &  &  & \HoloSegMetric{Dice} & \HoloSegScore{0.6257}{(0.6024--0.6481)}{4.55pt}{4.82pt}{} & \HoloSegScore{0.3731}{(0.3273--0.4182)}{4.55pt}{4.82pt}{} & \HoloSegScore{0.9296}{(0.9182--0.9383)}{4.55pt}{4.82pt}{} & \HoloSegScore{0.9224}{(0.9123--0.9324)}{4.55pt}{4.82pt}{} & \HoloSegScore{0.9190}{(0.8905--0.9285)}{4.55pt}{4.82pt}{} & \HoloSegScore{0.9370}{(0.9267--0.9458)}{4.55pt}{4.82pt}{} & \HoloSegScore{0.9385}{(0.9282--0.9470)}{4.55pt}{4.82pt}{} \\*
\softcline{4-11}
 &  & \HoloSegSpan{\makecell[c]{right\\[-0.10ex]humerus}}{2.04cm}{0.32cm} & \HoloSegMetric{HD95} & \HoloSegScore{66.45}{(64.31--68.27)}{4.55pt}{4.82pt}{} & \HoloSegScore{47.88}{(29.26--79.01)}{4.55pt}{4.82pt}{} & \HoloSegScore{19.24}{(4.726--39.86)}{4.55pt}{4.82pt}{} & \HoloSegScore{19.30}{(7.555--32.98)}{4.55pt}{4.82pt}{} & \HoloSegScore{12.86}{(6.103--23.54)}{4.55pt}{4.82pt}{} & \HoloSegScore{26.81}{(10.41--47.14)}{4.55pt}{4.82pt}{} & \HoloSegScore{11.37}{(5.179--19.08)}{4.55pt}{4.82pt}{} \\
\cline{3-11}
 &  &  & \HoloSegMetric{Dice} & \HoloSegScore{0.7588}{(0.7518--0.7668)}{4.55pt}{4.82pt}{} & \HoloSegScore{0.1191}{(0.09238--0.1434)}{4.20pt}{4.48pt}{} & \HoloSegScore{0.1822}{(0.1355--0.2501)}{4.55pt}{4.82pt}{} & \HoloSegScore{0.8450}{(0.8393--0.8509)}{4.55pt}{4.82pt}{} & \HoloSegScore{0.8154}{(0.8124--0.8346)}{4.55pt}{4.82pt}{} & \HoloSegScore{0.8704}{(0.8648--0.8764)}{4.55pt}{4.82pt}{} & \HoloSegScore{0.8768}{(0.8711--0.8836)}{4.55pt}{4.82pt}{} \\*
\softcline{4-11}
 &  & \HoloSegSpan{\makecell[c]{skull}}{2.04cm}{0.32cm} & \HoloSegMetric{HD95} & \HoloSegScore{34.42}{(18.34--51.90)}{4.55pt}{4.82pt}{} & \HoloSegScore{142.5}{(93.98--200.6)}{4.55pt}{4.82pt}{} & \HoloSegScore{736.1}{(666.7--786.1)}{4.55pt}{4.82pt}{} & \HoloSegScore{5.132}{(3.126--8.688)}{4.55pt}{4.82pt}{} & \HoloSegScore{6.176}{(1.867--9.256)}{4.55pt}{4.82pt}{} & \HoloSegScore{10.92}{(4.050--19.63)}{4.55pt}{4.82pt}{} & \HoloSegScore{60.67}{(7.712--125.7)}{4.55pt}{4.82pt}{} \\
\cline{3-11}
 &  &  & \HoloSegMetric{Dice} & \HoloSegScore{0.9385}{(0.9329--0.9431)}{4.55pt}{4.82pt}{} & \HoloSegScore{0.5903}{(0.5805--0.5999)}{4.55pt}{4.82pt}{} & \HoloSegScore{0.8820}{(0.8732--0.8903)}{4.55pt}{4.82pt}{} & \HoloSegScore{0.9659}{(0.9621--0.9687)}{4.55pt}{4.82pt}{} & \HoloSegScore{0.9583}{(0.9542--0.9596)}{4.55pt}{4.82pt}{} & \HoloSegScore{0.9551}{(0.9494--0.9588)}{4.55pt}{4.82pt}{} & \HoloSegScore{0.9587}{(0.9552--0.9618)}{4.55pt}{4.82pt}{} \\*
\softcline{4-11}
 &  & \HoloSegSpan{\makecell[c]{left hip}}{2.04cm}{0.32cm} & \HoloSegMetric{HD95} & \HoloSegScore{31.81}{(25.12--38.95)}{4.55pt}{4.82pt}{} & \HoloSegScore{21.90}{(19.60--24.73)}{4.55pt}{4.82pt}{} & \HoloSegScore{401.8}{(392.7--410.0)}{4.55pt}{4.82pt}{} & \HoloSegScore{1.363}{(1.023--1.757)}{4.55pt}{4.82pt}{} & \HoloSegScore{3.547}{(3.133--4.707)}{4.55pt}{4.82pt}{} & \HoloSegScore{15.98}{(7.405--27.34)}{4.55pt}{4.82pt}{} & \HoloSegScore{1.692}{(1.346--2.145)}{4.55pt}{4.82pt}{} \\
\cline{3-11}
 &  &  & \HoloSegMetric{Dice} & \HoloSegScore{0.9062}{(0.8974--0.9133)}{4.55pt}{4.82pt}{} & \HoloSegScore{0.5697}{(0.5329--0.5957)}{4.55pt}{4.82pt}{} & \HoloSegScore{0.9242}{(0.9202--0.9281)}{4.55pt}{4.82pt}{} & \HoloSegScore{0.9658}{(0.9613--0.9692)}{4.55pt}{4.82pt}{} & \HoloSegScore{0.9632}{(0.9537--0.9749)}{4.55pt}{4.82pt}{} & \HoloSegScore{0.9576}{(0.9520--0.9614)}{4.55pt}{4.82pt}{} & \HoloSegScore{0.9572}{(0.9540--0.9601)}{4.55pt}{4.82pt}{} \\*
\softcline{4-11}
 &  & \HoloSegSpan{\makecell[c]{right hip}}{2.04cm}{0.32cm} & \HoloSegMetric{HD95} & \HoloSegScore{45.00}{(42.48--47.58)}{4.55pt}{4.82pt}{} & \HoloSegScore{47.64}{(23.40--77.97)}{4.55pt}{4.82pt}{} & \HoloSegScore{363.9}{(318.1--397.9)}{4.55pt}{4.82pt}{} & \HoloSegScore{1.689}{(1.009--2.737)}{4.55pt}{4.82pt}{} & \HoloSegScore{2.386}{(2.113--3.142)}{4.55pt}{4.82pt}{} & \HoloSegScore{1.806}{(1.277--2.468)}{4.55pt}{4.82pt}{} & \HoloSegScore{1.691}{(1.262--2.266)}{4.55pt}{4.82pt}{} \\
\cline{3-11}
 &  &  & \HoloSegMetric{Dice} & \HoloSegScore{0.7911}{(0.7831--0.7992)}{4.55pt}{4.82pt}{} & \HoloSegScore{0.4763}{(0.4492--0.4989)}{4.55pt}{4.82pt}{} & \HoloSegScore{0.8692}{(0.8661--0.8724)}{4.55pt}{4.82pt}{} & \HoloSegScore{0.9402}{(0.9329--0.9474)}{4.55pt}{4.82pt}{} & \HoloSegScore{0.8754}{(0.8640--0.8792)}{4.55pt}{4.82pt}{} & \HoloSegScore{0.9147}{(0.9068--0.9222)}{4.55pt}{4.82pt}{} & \HoloSegScore{0.9284}{(0.9212--0.9348)}{4.55pt}{4.82pt}{} \\*
\softcline{4-11}
 &  & \HoloSegSpan{\makecell[c]{sacrum}}{2.04cm}{0.32cm} & \HoloSegMetric{HD95} & \HoloSegScore{41.46}{(38.39--43.39)}{4.55pt}{4.82pt}{} & \HoloSegScore{21.23}{(16.68--29.87)}{4.55pt}{4.82pt}{} & \HoloSegScore{418.8}{(409.4--427.1)}{4.55pt}{4.82pt}{} & \HoloSegScore{1.956}{(1.592--2.427)}{4.55pt}{4.82pt}{} & \HoloSegScore{3.733}{(2.605--4.513)}{4.55pt}{4.82pt}{} & \HoloSegScore{3.274}{(2.856--3.697)}{4.55pt}{4.82pt}{} & \HoloSegScore{2.674}{(2.267--3.093)}{4.55pt}{4.82pt}{} \\
\cline{3-11}
 &  &  & \HoloSegMetric{Dice} & \HoloSegScore{0.8730}{(0.8624--0.8835)}{4.55pt}{4.82pt}{} & \HoloSegScore{0.6658}{(0.6516--0.6800)}{4.55pt}{4.82pt}{} & \HoloSegScore{0.8119}{(0.7978--0.8255)}{4.55pt}{4.82pt}{} & \HoloSegScore{0.9629}{(0.9595--0.9659)}{4.55pt}{4.82pt}{} & \HoloSegScore{0.9283}{(0.9240--0.9383)}{4.55pt}{4.82pt}{} & \HoloSegScore{0.9717}{(0.9680--0.9743)}{4.55pt}{4.82pt}{} & \HoloSegScore{0.9746}{(0.9719--0.9766)}{4.55pt}{4.82pt}{} \\*
\softcline{4-11}
 &  & \HoloSegSpan{\makecell[c]{left femur}}{2.04cm}{0.32cm} & \HoloSegMetric{HD95} & \HoloSegScore{55.97}{(52.36--59.55)}{4.55pt}{4.82pt}{} & \HoloSegScore{17.25}{(15.93--18.55)}{4.55pt}{4.82pt}{} & \HoloSegScore{606.3}{(589.0--622.5)}{4.55pt}{4.82pt}{} & \HoloSegScore{1.579}{(1.266--1.999)}{4.55pt}{4.82pt}{} & \HoloSegScore{2.888}{(2.195--3.226)}{4.55pt}{4.82pt}{} & \HoloSegScore{1.496}{(1.214--1.858)}{4.55pt}{4.82pt}{} & \HoloSegScore{1.109}{(0.9289--1.319)}{4.55pt}{4.82pt}{} \\
\cline{3-11}
 &  &  & \HoloSegMetric{Dice} & \HoloSegScore{0.8147}{(0.8017--0.8272)}{4.55pt}{4.82pt}{} & \HoloSegScore{0.6831}{(0.6730--0.6930)}{4.55pt}{4.82pt}{} & \HoloSegScore{0.7965}{(0.7796--0.8102)}{4.55pt}{4.82pt}{} & \HoloSegScore{0.9618}{(0.9595--0.9638)}{4.55pt}{4.82pt}{} & \HoloSegScore{0.9349}{(0.9244--0.9530)}{4.55pt}{4.82pt}{} & \HoloSegScore{0.9718}{(0.9655--0.9757)}{4.55pt}{4.82pt}{} & \HoloSegScore{0.9742}{(0.9714--0.9766)}{4.55pt}{4.82pt}{} \\*
\softcline{4-11}
 &  & \HoloSegSpan{\makecell[c]{right femur}}{2.04cm}{0.32cm} & \HoloSegMetric{HD95} & \HoloSegScore{66.08}{(63.69--68.35)}{4.55pt}{4.82pt}{} & \HoloSegScore{19.64}{(14.50--29.31)}{4.55pt}{4.82pt}{} & \HoloSegScore{622.9}{(602.5--647.4)}{4.55pt}{4.82pt}{} & \HoloSegScore{1.554}{(1.381--1.754)}{4.55pt}{4.82pt}{} & \HoloSegScore{2.752}{(2.642--3.579)}{4.55pt}{4.82pt}{} & \HoloSegScore{1.695}{(1.247--2.435)}{4.55pt}{4.82pt}{} & \HoloSegScore{1.171}{(0.9767--1.461)}{4.55pt}{4.82pt}{} \\
\cline{3-11}
 &  &  & \HoloSegMetric{Dice} & \HoloSegScore{0.04151}{(0.03750--0.04599)}{4.20pt}{4.48pt}{} & \HoloSegScore{0.05205}{(0.04385--0.06060)}{4.20pt}{4.48pt}{} & \HoloSegScore{0.8007}{(0.7689--0.8181)}{4.55pt}{4.82pt}{} & \HoloSegScore{0.6634}{(0.6348--0.6894)}{4.55pt}{4.82pt}{} & \HoloSegScore{0.7794}{(0.7784--0.7971)}{4.55pt}{4.82pt}{} & \HoloSegScore{0.7407}{(0.7326--0.7487)}{4.55pt}{4.82pt}{} & \HoloSegScore{0.7233}{(0.7133--0.7319)}{4.55pt}{4.82pt}{} \\*
\softcline{4-11}
 &  & \HoloSegSpan{\makecell[c]{heart}}{2.04cm}{0.32cm} & \HoloSegMetric{HD95} & \HoloSegScore{234.6}{(180.9--284.0)}{4.55pt}{4.82pt}{} & \HoloSegScore{58.91}{(55.79--62.27)}{4.55pt}{4.82pt}{} & \HoloSegScore{2.908}{(2.543--3.604)}{4.55pt}{4.82pt}{} & \HoloSegScore{8.978}{(7.583--10.71)}{4.55pt}{4.82pt}{} & \HoloSegScore{5.532}{(4.187--5.804)}{4.55pt}{4.82pt}{} & \HoloSegScore{8.180}{(7.393--9.052)}{4.55pt}{4.82pt}{} & \HoloSegScore{6.264}{(5.707--6.988)}{4.55pt}{4.82pt}{} \\
\hline
\pagebreak[4]
 &  &  & \HoloSegMetric{Dice} &  & \HoloSegScore{0.4086}{(0.3667--0.4459)}{4.55pt}{4.82pt}{} & \HoloSegScore{0.9000}{(0.8874--0.9120)}{4.55pt}{4.82pt}{} & \HoloSegScore{0.9572}{(0.9541--0.9602)}{4.55pt}{4.82pt}{} & \HoloSegScore{0.9459}{(0.9378--0.9659)}{4.55pt}{4.82pt}{} & \HoloSegScore{0.9143}{(0.9088--0.9196)}{4.55pt}{4.82pt}{} & \HoloSegScore{0.9460}{(0.9420--0.9498)}{4.55pt}{4.82pt}{} \\*
\softcline{4-4}\softcline{6-11}
 &  & \HoloSegSpan{\makecell[c]{left heart\\[-0.10ex]atrium}}{2.04cm}{0.32cm} & \HoloSegMetric{HD95} & \raisebox{0.32cm}[0pt][0pt]{\HoloSegUnsupported} & \HoloSegScore{32.78}{(28.32--38.37)}{4.55pt}{4.82pt}{} & \HoloSegScore{309.3}{(252.8--360.9)}{4.55pt}{4.82pt}{} & \HoloSegScore{1.867}{(1.702--2.034)}{4.55pt}{4.82pt}{} & \HoloSegScore{3.953}{(3.455--6.030)}{4.55pt}{4.82pt}{} & \HoloSegScore{3.973}{(3.676--4.290)}{4.55pt}{4.82pt}{} & \HoloSegScore{8.327}{(3.777--13.28)}{4.55pt}{4.82pt}{} \\
\cline{3-11}
 &  &  & \HoloSegMetric{Dice} &  & \HoloSegScore{0.05063}{(0.03829--0.06230)}{4.20pt}{4.48pt}{} & \HoloSegScore{0.7843}{(0.7603--0.8061)}{4.55pt}{4.82pt}{} & \HoloSegScore{0.7367}{(0.7039--0.7634)}{4.55pt}{4.82pt}{} & \HoloSegScore{0.7710}{(0.7583--0.7923)}{4.55pt}{4.82pt}{} & \HoloSegScore{0.7164}{(0.6850--0.7417)}{4.55pt}{4.82pt}{} & \HoloSegScore{0.7113}{(0.6820--0.7351)}{4.55pt}{4.82pt}{} \\*
\softcline{4-4}\softcline{6-11}
 &  & \HoloSegSpan{\makecell[c]{heart tissue}}{2.04cm}{0.32cm} & \HoloSegMetric{HD95} & \raisebox{0.32cm}[0pt][0pt]{\HoloSegUnsupported} & \HoloSegScore{58.52}{(54.73--62.63)}{4.55pt}{4.82pt}{} & \HoloSegScore{2.599}{(2.472--2.795)}{4.55pt}{4.82pt}{} & \HoloSegScore{6.358}{(5.330--7.444)}{4.55pt}{4.82pt}{} & \HoloSegScore{7.237}{(5.886--8.624)}{4.55pt}{4.82pt}{} & \HoloSegScore{5.995}{(4.292--8.004)}{4.55pt}{4.82pt}{} & \HoloSegScore{8.919}{(7.472--10.61)}{4.55pt}{4.82pt}{} \\
\cline{3-11}
 &  &  & \HoloSegMetric{Dice} &  & \HoloSegScore{0.2813}{(0.2133--0.3488)}{4.55pt}{4.82pt}{} & \HoloSegScore{0.9449}{(0.9378--0.9496)}{4.55pt}{4.82pt}{} & \HoloSegScore{0.9340}{(0.9273--0.9393)}{4.55pt}{4.82pt}{} & \HoloSegScore{0.9216}{(0.9135--0.9329)}{4.55pt}{4.82pt}{} & \HoloSegScore{0.9160}{(0.9081--0.9229)}{4.55pt}{4.82pt}{} & \HoloSegScore{0.9141}{(0.9040--0.9212)}{4.55pt}{4.82pt}{} \\*
\softcline{4-4}\softcline{6-11}
 &  & \HoloSegSpan{\makecell[c]{right heart\\[-0.10ex]atrium}}{2.04cm}{0.32cm} & \HoloSegMetric{HD95} & \raisebox{0.32cm}[0pt][0pt]{\HoloSegUnsupported} & \HoloSegScore{41.05}{(33.88--49.12)}{4.55pt}{4.82pt}{} & \HoloSegScore{2.484}{(2.322--2.702)}{4.55pt}{4.82pt}{} & \HoloSegScore{2.924}{(2.735--3.159)}{4.55pt}{4.82pt}{} & \HoloSegScore{5.011}{(5.002--6.248)}{4.55pt}{4.82pt}{} & \HoloSegScore{5.133}{(3.474--8.087)}{4.55pt}{4.82pt}{} & \HoloSegScore{3.797}{(3.356--4.372)}{4.55pt}{4.82pt}{} \\
\cline{3-11}
 &  &  & \HoloSegMetric{Dice} &  & \HoloSegScore{0.2702}{(0.2313--0.3028)}{4.55pt}{4.82pt}{} & \HoloSegScore{0.9061}{(0.9023--0.9096)}{4.55pt}{4.82pt}{} & \HoloSegScore{0.8890}{(0.8812--0.8957)}{4.55pt}{4.82pt}{} & \HoloSegScore{0.8751}{(0.8388--0.8822)}{4.55pt}{4.82pt}{} & \HoloSegScore{0.7880}{(0.7765--0.7978)}{4.55pt}{4.82pt}{} & \HoloSegScore{0.8903}{(0.8829--0.8971)}{4.55pt}{4.82pt}{} \\*
\softcline{4-4}\softcline{6-11}
 &  & \HoloSegSpan{\makecell[c]{myocardium}}{2.04cm}{0.32cm} & \HoloSegMetric{HD95} & \raisebox{0.32cm}[0pt][0pt]{\HoloSegUnsupported} & \HoloSegScore{38.70}{(28.07--55.32)}{4.55pt}{4.82pt}{} & \HoloSegScore{2.505}{(2.500--2.516)}{4.55pt}{4.82pt}{} & \HoloSegScore{2.757}{(2.602--2.937)}{4.55pt}{4.82pt}{} & \HoloSegScore{3.162}{(2.927--3.990)}{4.55pt}{4.82pt}{} & \HoloSegScore{3.767}{(3.501--4.107)}{4.55pt}{4.82pt}{} & \HoloSegScore{2.492}{(2.402--2.574)}{4.55pt}{4.82pt}{} \\
\cline{3-11}
 &  &  & \HoloSegMetric{Dice} &  & \HoloSegScore{0.3833}{(0.3306--0.4331)}{4.55pt}{4.82pt}{} & \HoloSegScore{0.9479}{(0.9433--0.9515)}{4.55pt}{4.82pt}{} & \HoloSegScore{0.7039}{(0.6985--0.7098)}{4.55pt}{4.82pt}{} & \HoloSegScore{0.9109}{(0.8894--0.9217)}{4.55pt}{4.82pt}{} & \HoloSegScore{0.9053}{(0.8982--0.9114)}{4.55pt}{4.82pt}{} & \HoloSegScore{0.8937}{(0.8860--0.9010)}{4.55pt}{4.82pt}{} \\*
\softcline{4-4}\softcline{6-11}
 &  & \HoloSegSpan{\makecell[c]{left heart\\[-0.10ex]ventricle}}{2.04cm}{0.32cm} & \HoloSegMetric{HD95} & \raisebox{0.32cm}[0pt][0pt]{\HoloSegUnsupported} & \HoloSegScore{34.21}{(28.17--41.15)}{4.55pt}{4.82pt}{} & \HoloSegScore{21.71}{(2.496--51.06)}{4.55pt}{4.82pt}{} & \HoloSegScore{9.343}{(9.060--9.642)}{4.55pt}{4.82pt}{} & \HoloSegScore{4.996}{(4.590--6.756)}{4.55pt}{4.82pt}{} & \HoloSegScore{3.321}{(3.045--3.684)}{4.55pt}{4.82pt}{} & \HoloSegScore{3.773}{(3.504--4.057)}{4.55pt}{4.82pt}{} \\
\cline{3-11}
 &  &  & \HoloSegMetric{Dice} &  & \HoloSegScore{0.4086}{(0.3400--0.4727)}{4.55pt}{4.82pt}{} & \HoloSegScore{0.9515}{(0.9493--0.9536)}{4.55pt}{4.82pt}{} & \HoloSegScore{0.9482}{(0.9444--0.9513)}{4.55pt}{4.82pt}{} & \HoloSegScore{0.9095}{(0.9045--0.9179)}{4.55pt}{4.82pt}{} & \HoloSegScore{0.9291}{(0.9246--0.9333)}{4.55pt}{4.82pt}{} & \HoloSegScore{0.9312}{(0.9277--0.9345)}{4.55pt}{4.82pt}{} \\*
\softcline{4-4}\softcline{6-11}
 &  & \HoloSegSpan{\makecell[c]{right heart\\[-0.10ex]ventricle}}{2.04cm}{0.32cm} & \HoloSegMetric{HD95} & \raisebox{0.32cm}[0pt][0pt]{\HoloSegUnsupported} & \HoloSegScore{32.60}{(25.03--41.70)}{4.55pt}{4.82pt}{} & \HoloSegScore{2.497}{(2.448--2.531)}{4.55pt}{4.82pt}{} & \HoloSegScore{2.630}{(2.477--2.808)}{4.55pt}{4.82pt}{} & \HoloSegScore{3.587}{(3.432--4.547)}{4.55pt}{4.82pt}{} & \HoloSegScore{3.865}{(3.516--4.223)}{4.55pt}{4.82pt}{} & \HoloSegScore{3.230}{(2.997--3.497)}{4.55pt}{4.82pt}{} \\
\cline{3-11}
 &  &  & \HoloSegMetric{Dice} & \HoloSegScore{0.7955}{(0.7760--0.8139)}{4.55pt}{4.82pt}{} & \HoloSegScore{0.1794}{(0.1518--0.2043)}{4.55pt}{4.82pt}{} & \HoloSegScore{0.7190}{(0.6996--0.7388)}{4.55pt}{4.82pt}{} & \HoloSegScore{0.8889}{(0.8732--0.9024)}{4.55pt}{4.82pt}{} & \HoloSegScore{0.8853}{(0.8670--0.8974)}{4.55pt}{4.82pt}{} & \HoloSegScore{0.8490}{(0.8287--0.8670)}{4.55pt}{4.82pt}{} & \HoloSegScore{0.8620}{(0.8500--0.8742)}{4.55pt}{4.82pt}{} \\*
\softcline{4-11}
 &  & \HoloSegSpan{\makecell[c]{left iliac\\[-0.10ex]artery}}{2.04cm}{0.32cm} & \HoloSegMetric{HD95} & \HoloSegScore{34.38}{(30.62--37.63)}{4.55pt}{4.82pt}{} & \HoloSegScore{37.28}{(28.74--48.63)}{4.55pt}{4.82pt}{} & \HoloSegScore{374.1}{(365.5--382.3)}{4.55pt}{4.82pt}{} & \HoloSegScore{12.71}{(4.340--24.04)}{4.55pt}{4.82pt}{} & \HoloSegScore{13.37}{(6.081--21.96)}{4.55pt}{4.82pt}{} & \HoloSegScore{12.68}{(4.496--24.90)}{4.55pt}{4.82pt}{} & \HoloSegScore{13.19}{(5.144--24.80)}{4.55pt}{4.82pt}{} \\
\cline{3-11}
 &  &  & \HoloSegMetric{Dice} & \HoloSegScore{0.6567}{(0.6356--0.6774)}{4.55pt}{4.82pt}{} & \HoloSegScore{0.1349}{(0.1080--0.1621)}{4.55pt}{4.82pt}{} & \HoloSegScore{0.6620}{(0.6387--0.6875)}{4.55pt}{4.82pt}{} & \HoloSegScore{0.8887}{(0.8748--0.9018)}{4.55pt}{4.82pt}{} & \HoloSegScore{0.8695}{(0.8570--0.8824)}{4.55pt}{4.82pt}{} & \HoloSegScore{0.8699}{(0.8523--0.8853)}{4.55pt}{4.82pt}{} & \HoloSegScore{0.8887}{(0.8772--0.8990)}{4.55pt}{4.82pt}{} \\*
\softcline{4-11}
 &  & \HoloSegSpan{\makecell[c]{right iliac\\[-0.10ex]artery}}{2.04cm}{0.32cm} & \HoloSegMetric{HD95} & \HoloSegScore{32.74}{(31.95--33.55)}{4.55pt}{4.82pt}{} & \HoloSegScore{44.59}{(33.94--57.55)}{4.55pt}{4.82pt}{} & \HoloSegScore{369.2}{(358.8--378.5)}{4.55pt}{4.82pt}{} & \HoloSegScore{21.81}{(8.067--37.18)}{4.55pt}{4.82pt}{} & \HoloSegScore{22.30}{(15.86--32.64)}{4.55pt}{4.82pt}{} & \HoloSegScore{33.29}{(11.02--63.89)}{4.55pt}{4.82pt}{} & \HoloSegScore{21.54}{(7.319--38.00)}{4.55pt}{4.82pt}{} \\
\cline{3-11}
 &  &  & \HoloSegMetric{Dice} & \HoloSegScore{0.9444}{(0.9420--0.9468)}{4.55pt}{4.82pt}{} & \HoloSegScore{0.5825}{(0.5550--0.6068)}{4.55pt}{4.82pt}{} & \HoloSegScore{0.9539}{(0.9518--0.9561)}{4.55pt}{4.82pt}{} & \HoloSegScore{0.9467}{(0.9434--0.9494)}{4.55pt}{4.82pt}{} & \HoloSegScore{0.9355}{(0.9228--0.9578)}{4.55pt}{4.82pt}{} & \HoloSegScore{0.9575}{(0.9545--0.9604)}{4.55pt}{4.82pt}{} & \HoloSegScore{0.9546}{(0.9504--0.9582)}{4.55pt}{4.82pt}{} \\*
\softcline{4-11}
 &  & \HoloSegSpan{\makecell[c]{aorta}}{2.04cm}{0.32cm} & \HoloSegMetric{HD95} & \HoloSegScore{2.553}{(2.299--2.930)}{4.55pt}{4.82pt}{} & \HoloSegScore{24.05}{(21.94--26.29)}{4.55pt}{4.82pt}{} & \HoloSegScore{1.974}{(1.877--2.074)}{4.55pt}{4.82pt}{} & \HoloSegScore{1.476}{(1.282--1.716)}{4.55pt}{4.82pt}{} & \HoloSegScore{1.811}{(1.461--1.855)}{4.55pt}{4.82pt}{} & \HoloSegScore{2.158}{(1.506--2.981)}{4.55pt}{4.82pt}{} & \HoloSegScore{1.972}{(1.560--2.577)}{4.55pt}{4.82pt}{} \\
\cline{3-11}
 &  &  & \HoloSegMetric{Dice} & \HoloSegScore{0.8826}{(0.8668--0.8966)}{4.55pt}{4.82pt}{} & \HoloSegScore{0.1877}{(0.1446--0.2320)}{4.55pt}{4.82pt}{} & \HoloSegScore{0.8555}{(0.8428--0.8677)}{4.55pt}{4.82pt}{} & \HoloSegScore{0.9016}{(0.8838--0.9173)}{4.55pt}{4.82pt}{} & \HoloSegScore{0.8702}{(0.8409--0.8871)}{4.55pt}{4.82pt}{} & \HoloSegScore{0.8763}{(0.8602--0.8902)}{4.55pt}{4.82pt}{} & \HoloSegScore{0.8986}{(0.8853--0.9102)}{4.55pt}{4.82pt}{} \\*
\softcline{4-11}
\HoloSegSpan{\makecell[c]{\textbf{Internal}}}{1.20cm}{0.32cm} & \HoloSegSpan{\makecell[c]{DAP-Atlas\\[-0.10ex](AutoPETIII)}}{1.86cm}{0.32cm} & \HoloSegSpan{\makecell[c]{left iliac\\[-0.10ex]vena}}{2.04cm}{0.32cm} & \HoloSegMetric{HD95} & \HoloSegScore{11.12}{(3.599--21.04)}{4.55pt}{4.82pt}{} & \HoloSegScore{58.08}{(38.93--79.16)}{4.55pt}{4.82pt}{} & \HoloSegScore{319.5}{(271.5--360.8)}{4.55pt}{4.82pt}{} & \HoloSegScore{9.915}{(2.566--19.44)}{4.55pt}{4.82pt}{} & \HoloSegScore{10.05}{(3.134--19.23)}{4.55pt}{4.82pt}{} & \HoloSegScore{10.96}{(4.076--20.61)}{4.55pt}{4.82pt}{} & \HoloSegScore{9.247}{(2.298--19.15)}{4.55pt}{4.82pt}{} \\
\cline{3-11}
 &  &  & \HoloSegMetric{Dice} & \HoloSegScore{0.8070}{(0.7831--0.8299)}{4.55pt}{4.82pt}{} & \HoloSegScore{0.2097}{(0.1729--0.2475)}{4.55pt}{4.82pt}{} & \HoloSegScore{0.8318}{(0.8151--0.8475)}{4.55pt}{4.82pt}{} & \HoloSegScore{0.8854}{(0.8615--0.9053)}{4.55pt}{4.82pt}{} & \HoloSegScore{0.8647}{(0.8518--0.8759)}{4.55pt}{4.82pt}{} & \HoloSegScore{0.8635}{(0.8412--0.8843)}{4.55pt}{4.82pt}{} & \HoloSegScore{0.8867}{(0.8683--0.9018)}{4.55pt}{4.82pt}{} \\*
\softcline{4-11}
 &  & \HoloSegSpan{\makecell[c]{right iliac\\[-0.10ex]vena}}{2.04cm}{0.32cm} & \HoloSegMetric{HD95} & \HoloSegScore{30.13}{(28.07--31.69)}{4.55pt}{4.82pt}{} & \HoloSegScore{47.02}{(32.97--62.99)}{4.55pt}{4.82pt}{} & \HoloSegScore{311.1}{(254.6--360.9)}{4.55pt}{4.82pt}{} & \HoloSegScore{15.45}{(5.299--27.17)}{4.55pt}{4.82pt}{} & \HoloSegScore{15.95}{(5.687--26.32)}{4.55pt}{4.82pt}{} & \HoloSegScore{14.89}{(4.671--26.90)}{4.55pt}{4.82pt}{} & \HoloSegScore{17.04}{(5.911--29.27)}{4.55pt}{4.82pt}{} \\
\cline{3-11}
 &  &  & \HoloSegMetric{Dice} & \HoloSegScore{0.9140}{(0.9080--0.9198)}{4.55pt}{4.82pt}{} & \HoloSegScore{0.6443}{(0.6211--0.6660)}{4.55pt}{4.82pt}{} & \HoloSegScore{0.9400}{(0.9363--0.9435)}{4.55pt}{4.82pt}{} & \HoloSegScore{0.9362}{(0.9316--0.9408)}{4.55pt}{4.82pt}{} & \HoloSegScore{0.9010}{(0.8988--0.9079)}{4.55pt}{4.82pt}{} & \HoloSegScore{0.9110}{(0.9028--0.9190)}{4.55pt}{4.82pt}{} & \HoloSegScore{0.9116}{(0.9022--0.9208)}{4.55pt}{4.82pt}{} \\*
\softcline{4-11}
 &  & \HoloSegSpan{\makecell[c]{inferior\\[-0.10ex]vena cava}}{2.04cm}{0.32cm} & \HoloSegMetric{HD95} & \HoloSegScore{4.336}{(3.412--5.380)}{4.55pt}{4.82pt}{} & \HoloSegScore{17.21}{(14.72--20.08)}{4.55pt}{4.82pt}{} & \HoloSegScore{2.134}{(1.963--2.312)}{4.55pt}{4.82pt}{} & \HoloSegScore{2.698}{(2.132--3.622)}{4.55pt}{4.82pt}{} & \HoloSegScore{2.674}{(2.126--3.375)}{4.55pt}{4.82pt}{} & \HoloSegScore{3.747}{(3.252--4.309)}{4.55pt}{4.82pt}{} & \HoloSegScore{3.557}{(2.779--4.754)}{4.55pt}{4.82pt}{} \\
\cline{3-11}
 &  &  & \HoloSegMetric{Dice} & \HoloSegScore{0.8498}{(0.8399--0.8596)}{4.55pt}{4.82pt}{} & \HoloSegScore{0.2180}{(0.1927--0.2445)}{4.55pt}{4.82pt}{} & \HoloSegScore{0.8641}{(0.8592--0.8685)}{4.55pt}{4.82pt}{} & \HoloSegScore{0.9029}{(0.8959--0.9084)}{4.55pt}{4.82pt}{} & \HoloSegScore{0.8818}{(0.8757--0.8840)}{4.55pt}{4.82pt}{} & \HoloSegScore{0.8990}{(0.8930--0.9040)}{4.55pt}{4.82pt}{} & \HoloSegScore{0.9012}{(0.8964--0.9057)}{4.55pt}{4.82pt}{} \\*
\softcline{4-11}
 &  & \HoloSegSpan{\makecell[c]{portal vein\\[-0.10ex]and splenic\\[-0.10ex]vein}}{2.04cm}{0.32cm} & \HoloSegMetric{HD95} & \HoloSegScore{7.703}{(5.828--9.654)}{4.55pt}{4.82pt}{} & \HoloSegScore{54.82}{(47.05--63.06)}{4.55pt}{4.82pt}{} & \HoloSegScore{2.476}{(2.394--2.576)}{4.55pt}{4.82pt}{} & \HoloSegScore{4.566}{(3.290--6.183)}{4.55pt}{4.82pt}{} & \HoloSegScore{4.813}{(4.630--5.936)}{4.55pt}{4.82pt}{} & \HoloSegScore{2.538}{(2.234--2.895)}{4.55pt}{4.82pt}{} & \HoloSegScore{3.283}{(2.827--3.792)}{4.55pt}{4.82pt}{} \\
\cline{3-11}
 &  &  & \HoloSegMetric{Dice} &  & \HoloSegScore{0.001992}{(0.0005469--0.003963)}{3.52pt}{3.80pt}{} & \HoloSegScore{0.7930}{(0.7688--0.8161)}{4.55pt}{4.82pt}{} & \HoloSegScore{0.8351}{(0.8100--0.8590)}{4.55pt}{4.82pt}{} & \HoloSegScore{0.7977}{(0.7864--0.8066)}{4.55pt}{4.82pt}{} & \HoloSegScore{0.8265}{(0.8017--0.8498)}{4.55pt}{4.82pt}{} & \HoloSegScore{0.8565}{(0.8304--0.8771)}{4.55pt}{4.82pt}{} \\*
\softcline{4-4}\softcline{6-11}
 &  & \HoloSegSpan{\makecell[c]{celiac trunk}}{2.04cm}{0.32cm} & \HoloSegMetric{HD95} & \raisebox{0.32cm}[0pt][0pt]{\HoloSegUnsupported} & \HoloSegScore{158.9}{(144.5--173.4)}{4.55pt}{4.82pt}{} & \HoloSegScore{5.895}{(3.326--9.285)}{4.55pt}{4.82pt}{} & \HoloSegScore{5.753}{(3.524--8.671)}{4.55pt}{4.82pt}{} & \HoloSegScore{6.086}{(5.102--9.636)}{4.55pt}{4.82pt}{} & \HoloSegScore{12.34}{(4.206--26.21)}{4.55pt}{4.82pt}{} & \HoloSegScore{3.847}{(2.377--5.845)}{4.55pt}{4.82pt}{} \\
\cline{3-11}
 &  &  & \HoloSegMetric{Dice} & \HoloSegScore{0.9508}{(0.9374--0.9590)}{4.55pt}{4.82pt}{} & \HoloSegScore{0.6236}{(0.5901--0.6596)}{4.55pt}{4.82pt}{} & \HoloSegScore{0.9484}{(0.9395--0.9544)}{4.55pt}{4.82pt}{} & \HoloSegScore{0.9564}{(0.9463--0.9629)}{4.55pt}{4.82pt}{} & \HoloSegScore{0.9360}{(0.9194--0.9517)}{4.55pt}{4.82pt}{} & \HoloSegScore{0.9013}{(0.8857--0.9156)}{4.55pt}{4.82pt}{} & \HoloSegScore{0.9240}{(0.9118--0.9356)}{4.55pt}{4.82pt}{} \\*
\softcline{4-11}
 &  & \HoloSegSpan{\makecell[c]{left lung\\[-0.10ex]lower lobe}}{2.04cm}{0.32cm} & \HoloSegMetric{HD95} & \HoloSegScore{9.940}{(6.569--13.52)}{4.55pt}{4.82pt}{} & \HoloSegScore{38.53}{(31.96--45.58)}{4.55pt}{4.82pt}{} & \HoloSegScore{4.307}{(3.692--4.996)}{4.55pt}{4.82pt}{} & \HoloSegScore{11.21}{(9.895--12.55)}{4.55pt}{4.82pt}{} & \HoloSegScore{11.99}{(10.26--15.00)}{4.55pt}{4.82pt}{} & \HoloSegScore{11.66}{(10.03--13.48)}{4.55pt}{4.82pt}{} & \HoloSegScore{20.26}{(10.32--38.39)}{4.55pt}{4.82pt}{} \\
\cline{3-11}
 &  &  & \HoloSegMetric{Dice} & \HoloSegScore{0.9633}{(0.9525--0.9716)}{4.55pt}{4.82pt}{} & \HoloSegScore{0.6563}{(0.6309--0.6816)}{4.55pt}{4.82pt}{} & \HoloSegScore{0.9566}{(0.9477--0.9628)}{4.55pt}{4.82pt}{} & \HoloSegScore{0.9641}{(0.9516--0.9724)}{4.55pt}{4.82pt}{} & \HoloSegScore{0.9338}{(0.9303--0.9574)}{4.55pt}{4.82pt}{} & \HoloSegScore{0.9335}{(0.9233--0.9424)}{4.55pt}{4.82pt}{} & \HoloSegScore{0.9406}{(0.9297--0.9500)}{4.55pt}{4.82pt}{} \\*
\softcline{4-11}
 &  & \HoloSegSpan{\makecell[c]{left lung\\[-0.10ex]upper lobe}}{2.04cm}{0.32cm} & \HoloSegMetric{HD95} & \HoloSegScore{10.52}{(8.006--13.70)}{4.55pt}{4.82pt}{} & \HoloSegScore{26.88}{(23.30--31.73)}{4.55pt}{4.82pt}{} & \HoloSegScore{3.915}{(3.242--4.827)}{4.55pt}{4.82pt}{} & \HoloSegScore{7.646}{(6.400--9.193)}{4.55pt}{4.82pt}{} & \HoloSegScore{4.211}{(3.496--5.825)}{4.55pt}{4.82pt}{} & \HoloSegScore{11.48}{(10.00--13.09)}{4.55pt}{4.82pt}{} & \HoloSegScore{9.471}{(8.084--10.83)}{4.55pt}{4.82pt}{} \\
\cline{3-11}
 &  &  & \HoloSegMetric{Dice} & \HoloSegScore{0.9490}{(0.9221--0.9635)}{4.55pt}{4.82pt}{} & \HoloSegScore{0.6257}{(0.6050--0.6473)}{4.55pt}{4.82pt}{} & \HoloSegScore{0.9511}{(0.9466--0.9546)}{4.55pt}{4.82pt}{} & \HoloSegScore{0.9564}{(0.9464--0.9634)}{4.55pt}{4.82pt}{} & \HoloSegScore{0.9372}{(0.9224--0.9390)}{4.55pt}{4.82pt}{} & \HoloSegScore{0.9189}{(0.9074--0.9301)}{4.55pt}{4.82pt}{} & \HoloSegScore{0.9318}{(0.9232--0.9400)}{4.55pt}{4.82pt}{} \\*
\softcline{4-11}
 &  & \HoloSegSpan{\makecell[c]{right lung\\[-0.10ex]lower lobe}}{2.04cm}{0.32cm} & \HoloSegMetric{HD95} & \HoloSegScore{13.54}{(12.07--15.45)}{4.55pt}{4.82pt}{} & \HoloSegScore{30.87}{(27.94--34.20)}{4.55pt}{4.82pt}{} & \HoloSegScore{4.041}{(3.563--4.560)}{4.55pt}{4.82pt}{} & \HoloSegScore{11.37}{(10.13--12.58)}{4.55pt}{4.82pt}{} & \HoloSegScore{12.41}{(11.37--14.68)}{4.55pt}{4.82pt}{} & \HoloSegScore{11.75}{(10.44--13.25)}{4.55pt}{4.82pt}{} & \HoloSegScore{12.40}{(10.95--14.09)}{4.55pt}{4.82pt}{} \\
\cline{3-11}
 &  &  & \HoloSegMetric{Dice} & \HoloSegScore{0.9091}{(0.8707--0.9344)}{4.55pt}{4.82pt}{} & \HoloSegScore{0.3246}{(0.2741--0.3787)}{4.55pt}{4.82pt}{} & \HoloSegScore{0.9088}{(0.8883--0.9249)}{4.55pt}{4.82pt}{} & \HoloSegScore{0.9057}{(0.8795--0.9254)}{4.55pt}{4.82pt}{} & \HoloSegScore{0.9011}{(0.8825--0.9282)}{4.55pt}{4.82pt}{} & \HoloSegScore{0.8539}{(0.8257--0.8768)}{4.55pt}{4.82pt}{} & \HoloSegScore{0.8673}{(0.8364--0.8869)}{4.55pt}{4.82pt}{} \\*
\softcline{4-11}
 &  & \HoloSegSpan{\makecell[c]{right lung\\[-0.10ex]middle lobe}}{2.04cm}{0.32cm} & \HoloSegMetric{HD95} & \HoloSegScore{22.06}{(6.496--48.50)}{4.55pt}{4.82pt}{} & \HoloSegScore{41.85}{(35.62--48.42)}{4.55pt}{4.82pt}{} & \HoloSegScore{5.373}{(4.296--6.692)}{4.55pt}{4.82pt}{} & \HoloSegScore{8.951}{(7.637--10.35)}{4.55pt}{4.82pt}{} & \HoloSegScore{9.358}{(9.156--11.30)}{4.55pt}{4.82pt}{} & \HoloSegScore{11.47}{(9.731--13.48)}{4.55pt}{4.82pt}{} & \HoloSegScore{9.371}{(8.233--10.69)}{4.55pt}{4.82pt}{} \\
\cline{3-11}
 &  &  & \HoloSegMetric{Dice} & \HoloSegScore{0.9583}{(0.9544--0.9619)}{4.55pt}{4.82pt}{} & \HoloSegScore{0.6734}{(0.6592--0.6883)}{4.55pt}{4.82pt}{} & \HoloSegScore{0.9470}{(0.9436--0.9503)}{4.55pt}{4.82pt}{} & \HoloSegScore{0.9572}{(0.9520--0.9618)}{4.55pt}{4.82pt}{} & \HoloSegScore{0.9480}{(0.9264--0.9530)}{4.55pt}{4.82pt}{} & \HoloSegScore{0.9271}{(0.9205--0.9329)}{4.55pt}{4.82pt}{} & \HoloSegScore{0.9393}{(0.9325--0.9449)}{4.55pt}{4.82pt}{} \\*
\softcline{4-11}
 &  & \HoloSegSpan{\makecell[c]{right lung\\[-0.10ex]upper lobe}}{2.04cm}{0.32cm} & \HoloSegMetric{HD95} & \HoloSegScore{9.265}{(7.795--11.31)}{4.55pt}{4.82pt}{} & \HoloSegScore{24.05}{(21.59--26.79)}{4.55pt}{4.82pt}{} & \HoloSegScore{5.028}{(4.496--5.597)}{4.55pt}{4.82pt}{} & \HoloSegScore{8.283}{(7.113--9.525)}{4.55pt}{4.82pt}{} & \HoloSegScore{8.711}{(6.287--10.53)}{4.55pt}{4.82pt}{} & \HoloSegScore{10.06}{(8.625--11.63)}{4.55pt}{4.82pt}{} & \HoloSegScore{8.901}{(7.688--10.17)}{4.55pt}{4.82pt}{} \\
\hline
\pagebreak[4]
 &  &  & \HoloSegMetric{Dice} & \HoloSegScore{0.1935}{(0.1825--0.2044)}{4.55pt}{4.82pt}{} & \HoloSegScore{0.001621}{(0.001136--0.002129)}{3.85pt}{4.12pt}{} & \HoloSegScore{0.7220}{(0.7096--0.7339)}{4.55pt}{4.82pt}{} & \HoloSegScore{0.7774}{(0.7628--0.7916)}{4.55pt}{4.82pt}{} & \HoloSegScore{0.7678}{(0.7522--0.7752)}{4.55pt}{4.82pt}{} & \HoloSegScore{0.6934}{(0.6777--0.7091)}{4.55pt}{4.82pt}{} & \HoloSegScore{0.7332}{(0.7193--0.7476)}{4.55pt}{4.82pt}{} \\*
\softcline{4-11}
 &  & \HoloSegSpan{\makecell[c]{bronchie}}{2.04cm}{0.32cm} & \HoloSegMetric{HD95} & \HoloSegScore{124.0}{(107.5--149.6)}{4.55pt}{4.82pt}{} & \HoloSegScore{85.37}{(82.10--88.64)}{4.55pt}{4.82pt}{} & \HoloSegScore{3.114}{(2.815--3.448)}{4.55pt}{4.82pt}{} & \HoloSegScore{16.53}{(14.57--18.60)}{4.55pt}{4.82pt}{} & \HoloSegScore{3.853}{(1.889--4.030)}{4.55pt}{4.82pt}{} & \HoloSegScore{13.07}{(11.48--14.95)}{4.55pt}{4.82pt}{} & \HoloSegScore{19.42}{(17.43--21.23)}{4.55pt}{4.82pt}{} \\
\cline{3-11}
 &  &  & \HoloSegMetric{Dice} & \HoloSegScore{0.8897}{(0.8810--0.8967)}{4.55pt}{4.82pt}{} & \HoloSegScore{0.4201}{(0.3873--0.4509)}{4.55pt}{4.82pt}{} & \HoloSegScore{0.9256}{(0.9201--0.9309)}{4.55pt}{4.82pt}{} & \HoloSegScore{0.9363}{(0.9278--0.9432)}{4.55pt}{4.82pt}{} & \HoloSegScore{0.9306}{(0.9236--0.9393)}{4.55pt}{4.82pt}{} & \HoloSegScore{0.9204}{(0.9140--0.9264)}{4.55pt}{4.82pt}{} & \HoloSegScore{0.9264}{(0.9196--0.9318)}{4.55pt}{4.82pt}{} \\*
\softcline{4-11}
 &  & \HoloSegSpan{\makecell[c]{trachea}}{2.04cm}{0.32cm} & \HoloSegMetric{HD95} & \HoloSegScore{7.150}{(6.071--8.367)}{4.55pt}{4.82pt}{} & \HoloSegScore{29.79}{(26.01--34.29)}{4.55pt}{4.82pt}{} & \HoloSegScore{1.900}{(1.681--2.222)}{4.55pt}{4.82pt}{} & \HoloSegScore{2.537}{(1.774--3.372)}{4.55pt}{4.82pt}{} & \HoloSegScore{2.046}{(1.409--2.090)}{4.55pt}{4.82pt}{} & \HoloSegScore{3.180}{(2.614--3.805)}{4.55pt}{4.82pt}{} & \HoloSegScore{2.513}{(2.072--3.097)}{4.55pt}{4.82pt}{} \\
\cline{3-11}
 &  &  & \HoloSegMetric{Dice} &  & \HoloSegScore{0.2201}{(0.1846--0.2580)}{4.55pt}{4.82pt}{} & \HoloSegScore{0.8639}{(0.8577--0.8698)}{4.55pt}{4.82pt}{} & \HoloSegScore{0.8976}{(0.8911--0.9033)}{4.55pt}{4.82pt}{} & \HoloSegScore{0.8901}{(0.8847--0.9075)}{4.55pt}{4.82pt}{} & \HoloSegScore{0.8419}{(0.8305--0.8524)}{4.55pt}{4.82pt}{} & \HoloSegScore{0.8536}{(0.8414--0.8643)}{4.55pt}{4.82pt}{} \\*
\softcline{4-4}\softcline{6-11}
 &  & \HoloSegSpan{\makecell[c]{pulmonary\\[-0.10ex]artery}}{2.04cm}{0.32cm} & \HoloSegMetric{HD95} & \raisebox{0.32cm}[0pt][0pt]{\HoloSegUnsupported} & \HoloSegScore{69.19}{(63.97--74.71)}{4.55pt}{4.82pt}{} & \HoloSegScore{3.180}{(2.792--3.835)}{4.55pt}{4.82pt}{} & \HoloSegScore{10.87}{(10.23--11.53)}{4.55pt}{4.82pt}{} & \HoloSegScore{3.746}{(3.675--5.235)}{4.55pt}{4.82pt}{} & \HoloSegScore{35.03}{(32.74--37.39)}{4.55pt}{4.82pt}{} & \HoloSegScore{26.28}{(24.63--28.04)}{4.55pt}{4.82pt}{} \\
\cline{3-11}
 &  &  & \HoloSegMetric{Dice} &  & \HoloSegScore{0.0000}{(0.0000--0.0000)}{4.55pt}{4.82pt}{} & \HoloSegScore{0.6021}{(0.5242--0.6763)}{4.55pt}{4.82pt}{} & \HoloSegScore{0.8524}{(0.8215--0.8764)}{4.55pt}{4.82pt}{} & \HoloSegScore{0.7623}{(0.7339--0.8048)}{4.55pt}{4.82pt}{} & \HoloSegScore{0.7582}{(0.7128--0.7959)}{4.55pt}{4.82pt}{} & \HoloSegScore{0.8461}{(0.8073--0.8750)}{4.55pt}{4.82pt}{} \\*
\softcline{4-4}\softcline{6-11}
 &  & \HoloSegSpan{\makecell[c]{left cheek}}{2.04cm}{0.32cm} & \HoloSegMetric{HD95} & \raisebox{0.32cm}[0pt][0pt]{\HoloSegUnsupported} & \HoloSegScore{617.6}{(572.1--651.2)}{4.55pt}{4.82pt}{} & \HoloSegScore{589.8}{(544.1--627.4)}{4.55pt}{4.82pt}{} & \HoloSegScore{2.719}{(2.376--3.079)}{4.55pt}{4.82pt}{} & \HoloSegScore{5.421}{(4.088--7.167)}{4.55pt}{4.82pt}{} & \HoloSegScore{4.765}{(4.167--5.377)}{4.55pt}{4.82pt}{} & \HoloSegScore{5.016}{(2.368--10.03)}{4.55pt}{4.82pt}{} \\
\cline{3-11}
 &  &  & \HoloSegMetric{Dice} &  & \HoloSegScore{0.00004926}{(0.0000--0.0001478)}{3.85pt}{4.12pt}{} & \HoloSegScore{0.6020}{(0.5057--0.7009)}{4.55pt}{4.82pt}{} & \HoloSegScore{0.7784}{(0.6956--0.8442)}{4.55pt}{4.82pt}{} & \HoloSegScore{0.7763}{(0.7716--0.7820)}{4.55pt}{4.82pt}{} & \HoloSegScore{0.7641}{(0.6811--0.8281)}{4.55pt}{4.82pt}{} & \HoloSegScore{0.7839}{(0.6969--0.8455)}{4.55pt}{4.82pt}{} \\*
\softcline{4-4}\softcline{6-11}
 &  & \HoloSegSpan{\makecell[c]{right cheek}}{2.04cm}{0.32cm} & \HoloSegMetric{HD95} & \raisebox{0.32cm}[0pt][0pt]{\HoloSegUnsupported} & \HoloSegScore{210.6}{(159.4--266.9)}{4.55pt}{4.82pt}{} & \HoloSegScore{505.9}{(429.4--566.4)}{4.55pt}{4.82pt}{} & \HoloSegScore{3.300}{(2.710--3.950)}{4.55pt}{4.82pt}{} & \HoloSegScore{5.423}{(3.645--7.751)}{4.55pt}{4.82pt}{} & \HoloSegScore{4.264}{(3.125--5.701)}{4.55pt}{4.82pt}{} & \HoloSegScore{23.46}{(2.557--65.00)}{4.55pt}{4.82pt}{} \\
\cline{3-11}
 &  &  & \HoloSegMetric{Dice} &  & \HoloSegScore{0.0000}{(0.0000--0.0000)}{4.55pt}{4.82pt}{} & \HoloSegScore{0.8342}{(0.8085--0.8557)}{4.55pt}{4.82pt}{} & \HoloSegScore{0.7543}{(0.7138--0.7904)}{4.55pt}{4.82pt}{} & \HoloSegScore{0.8340}{(0.8231--0.8509)}{4.55pt}{4.82pt}{} & \HoloSegScore{0.8617}{(0.8430--0.8787)}{4.55pt}{4.82pt}{} & \HoloSegScore{0.8062}{(0.7699--0.8376)}{4.55pt}{4.82pt}{} \\*
\softcline{4-4}\softcline{6-11}
 &  & \HoloSegSpan{\makecell[c]{left eyeball}}{2.04cm}{0.32cm} & \HoloSegMetric{HD95} & \raisebox{0.32cm}[0pt][0pt]{\HoloSegUnsupported} & \HoloSegScore{631.6}{(596.0--665.5)}{4.55pt}{4.82pt}{} & \HoloSegScore{2.338}{(2.151--2.552)}{4.55pt}{4.82pt}{} & \HoloSegScore{3.411}{(2.933--3.937)}{4.55pt}{4.82pt}{} & \HoloSegScore{3.995}{(3.988--5.619)}{4.55pt}{4.82pt}{} & \HoloSegScore{2.126}{(1.935--2.323)}{4.55pt}{4.82pt}{} & \HoloSegScore{2.396}{(2.124--2.680)}{4.55pt}{4.82pt}{} \\
\cline{3-11}
 &  &  & \HoloSegMetric{Dice} &  & \HoloSegScore{0.0000}{(0.0000--0.0000)}{4.55pt}{4.82pt}{} & \HoloSegScore{0.8133}{(0.7784--0.8390)}{4.55pt}{4.82pt}{} & \HoloSegScore{0.7375}{(0.6815--0.7808)}{4.55pt}{4.82pt}{} & \HoloSegScore{0.7959}{(0.7956--0.8021)}{4.55pt}{4.82pt}{} & \HoloSegScore{0.8080}{(0.7742--0.8344)}{4.55pt}{4.82pt}{} & \HoloSegScore{0.8079}{(0.7531--0.8474)}{4.55pt}{4.82pt}{} \\*
\softcline{4-4}\softcline{6-11}
 &  & \HoloSegSpan{\makecell[c]{right\\[-0.10ex]eyeball}}{2.04cm}{0.32cm} & \HoloSegMetric{HD95} & \raisebox{0.32cm}[0pt][0pt]{\HoloSegUnsupported} & \HoloSegScore{531.9}{(489.4--576.0)}{4.55pt}{4.82pt}{} & \HoloSegScore{2.521}{(2.277--2.872)}{4.55pt}{4.82pt}{} & \HoloSegScore{3.568}{(2.972--4.309)}{4.55pt}{4.82pt}{} & \HoloSegScore{3.020}{(2.825--4.115)}{4.55pt}{4.82pt}{} & \HoloSegScore{2.307}{(2.018--2.688)}{4.55pt}{4.82pt}{} & \HoloSegScore{2.366}{(2.167--2.575)}{4.55pt}{4.82pt}{} \\
\cline{3-11}
 &  &  & \HoloSegMetric{Dice} &  & \HoloSegScore{0.000004220}{(0.0000--0.00001266)}{3.85pt}{4.12pt}{} & \HoloSegScore{0.4648}{(0.4356--0.4934)}{4.55pt}{4.82pt}{} & \HoloSegScore{0.8291}{(0.8180--0.8398)}{4.55pt}{4.82pt}{} & \HoloSegScore{0.8246}{(0.8152--0.8414)}{4.55pt}{4.82pt}{} & \HoloSegScore{0.8135}{(0.8033--0.8229)}{4.55pt}{4.82pt}{} & \HoloSegScore{0.7790}{(0.7673--0.7914)}{4.55pt}{4.82pt}{} \\*
\softcline{4-4}\softcline{6-11}
 &  & \HoloSegSpan{\makecell[c]{nasal cavity}}{2.04cm}{0.32cm} & \HoloSegMetric{HD95} & \raisebox{0.32cm}[0pt][0pt]{\HoloSegUnsupported} & \HoloSegScore{224.5}{(213.8--236.3)}{4.55pt}{4.82pt}{} & \HoloSegScore{603.7}{(580.3--626.9)}{4.55pt}{4.82pt}{} & \HoloSegScore{8.195}{(7.300--9.164)}{4.55pt}{4.82pt}{} & \HoloSegScore{9.806}{(7.515--12.58)}{4.55pt}{4.82pt}{} & \HoloSegScore{8.999}{(6.358--13.41)}{4.55pt}{4.82pt}{} & \HoloSegScore{9.875}{(8.829--11.26)}{4.55pt}{4.82pt}{} \\
\cline{3-11}
 &  &  & \HoloSegMetric{Dice} & \HoloSegScore{0.7044}{(0.6733--0.7359)}{4.55pt}{4.82pt}{} & \HoloSegScore{0.001229}{(0.000007105--0.003369)}{3.52pt}{3.80pt}{} & \HoloSegScore{0.8131}{(0.7902--0.8333)}{4.55pt}{4.82pt}{} & \HoloSegScore{0.8180}{(0.7957--0.8372)}{4.55pt}{4.82pt}{} & \HoloSegScore{0.8075}{(0.8046--0.8113)}{4.55pt}{4.82pt}{} & \HoloSegScore{0.7222}{(0.6977--0.7451)}{4.55pt}{4.82pt}{} & \HoloSegScore{0.8342}{(0.8216--0.8452)}{4.55pt}{4.82pt}{} \\*
\softcline{4-11}
 &  & \HoloSegSpan{\makecell[c]{right common\\[-0.10ex]carotid\\[-0.10ex]artery}}{2.04cm}{0.32cm} & \HoloSegMetric{HD95} & \HoloSegScore{17.20}{(7.349--35.21)}{4.55pt}{4.82pt}{} & \HoloSegScore{262.9}{(217.1--306.9)}{4.55pt}{4.82pt}{} & \HoloSegScore{81.85}{(27.35--137.8)}{4.55pt}{4.82pt}{} & \HoloSegScore{13.30}{(7.653--20.13)}{4.55pt}{4.82pt}{} & \HoloSegScore{7.149}{(4.790--11.66)}{4.55pt}{4.82pt}{} & \HoloSegScore{5.964}{(4.302--7.799)}{4.55pt}{4.82pt}{} & \HoloSegScore{3.790}{(2.327--5.654)}{4.55pt}{4.82pt}{} \\
\cline{3-11}
 &  &  & \HoloSegMetric{Dice} & \HoloSegScore{0.7553}{(0.7315--0.7749)}{4.55pt}{4.82pt}{} & \HoloSegScore{0.004649}{(0.002764--0.007214)}{3.85pt}{4.12pt}{} & \HoloSegScore{0.7765}{(0.7503--0.7997)}{4.55pt}{4.82pt}{} & \HoloSegScore{0.8694}{(0.8574--0.8801)}{4.55pt}{4.82pt}{} & \HoloSegScore{0.7726}{(0.7517--0.7926)}{4.55pt}{4.82pt}{} & \HoloSegScore{0.7841}{(0.7680--0.7995)}{4.55pt}{4.82pt}{} & \HoloSegScore{0.8585}{(0.8469--0.8687)}{4.55pt}{4.82pt}{} \\*
\softcline{4-11}
\HoloSegSpan{\makecell[c]{\textbf{Internal}}}{1.20cm}{0.32cm} & \HoloSegSpan{\makecell[c]{DAP-Atlas\\[-0.10ex](AutoPETIII)}}{1.86cm}{0.32cm} & \HoloSegSpan{\makecell[c]{left common\\[-0.10ex]carotid\\[-0.10ex]artery}}{2.04cm}{0.32cm} & \HoloSegMetric{HD95} & \HoloSegScore{8.814}{(6.060--11.89)}{4.55pt}{4.82pt}{} & \HoloSegScore{297.9}{(275.7--315.6)}{4.55pt}{4.82pt}{} & \HoloSegScore{264.2}{(194.9--329.3)}{4.55pt}{4.82pt}{} & \HoloSegScore{5.067}{(3.351--7.494)}{4.55pt}{4.82pt}{} & \HoloSegScore{6.471}{(4.017--8.771)}{4.55pt}{4.82pt}{} & \HoloSegScore{4.304}{(3.068--5.635)}{4.55pt}{4.82pt}{} & \HoloSegScore{2.077}{(1.619--2.618)}{4.55pt}{4.82pt}{} \\
\cline{3-11}
 &  &  & \HoloSegMetric{Dice} &  & \HoloSegScore{0.0000}{(0.0000--0.0000)}{4.55pt}{4.82pt}{} & \HoloSegScore{0.8706}{(0.8140--0.9006)}{4.55pt}{4.82pt}{} & \HoloSegScore{0.9008}{(0.8438--0.9342)}{4.55pt}{4.82pt}{} & \HoloSegScore{0.8574}{(0.8039--0.8841)}{4.55pt}{4.82pt}{} & \HoloSegScore{0.8864}{(0.8294--0.9202)}{4.55pt}{4.82pt}{} & \HoloSegScore{0.9003}{(0.8434--0.9305)}{4.55pt}{4.82pt}{} \\*
\softcline{4-4}\softcline{6-11}
 &  & \HoloSegSpan{\makecell[c]{manubrium of\\[-0.10ex]sternum}}{2.04cm}{0.32cm} & \HoloSegMetric{HD95} & \raisebox{0.32cm}[0pt][0pt]{\HoloSegUnsupported} & \HoloSegScore{132.2}{(125.7--138.5)}{4.55pt}{4.82pt}{} & \HoloSegScore{36.96}{(4.096--73.63)}{4.55pt}{4.82pt}{} & \HoloSegScore{4.173}{(2.400--7.237)}{4.55pt}{4.82pt}{} & \HoloSegScore{4.296}{(3.655--8.133)}{4.55pt}{4.82pt}{} & \HoloSegScore{5.473}{(3.499--8.517)}{4.55pt}{4.82pt}{} & \HoloSegScore{3.647}{(2.072--6.526)}{4.55pt}{4.82pt}{} \\
\cline{3-11}
 &  &  & \HoloSegMetric{Dice} &  & \HoloSegScore{0.0000}{(0.0000--0.0000)}{4.55pt}{4.82pt}{} & \HoloSegScore{0.7431}{(0.7190--0.7682)}{4.55pt}{4.82pt}{} & \HoloSegScore{0.6977}{(0.6567--0.7328)}{4.55pt}{4.82pt}{} & \HoloSegScore{0.6838}{(0.6551--0.7024)}{4.55pt}{4.82pt}{} & \HoloSegScore{0.5546}{(0.5166--0.5878)}{4.55pt}{4.82pt}{} & \HoloSegScore{0.7460}{(0.7259--0.7651)}{4.55pt}{4.82pt}{} \\*
\softcline{4-4}\softcline{6-11}
 &  & \HoloSegSpan{\makecell[c]{right\\[-0.10ex]internal\\[-0.10ex]carotid\\[-0.10ex]artery}}{2.04cm}{0.32cm} & \HoloSegMetric{HD95} & \raisebox{0.32cm}[0pt][0pt]{\HoloSegUnsupported} & \HoloSegScore{489.4}{(454.5--527.1)}{4.55pt}{4.82pt}{} & \HoloSegScore{3.881}{(2.250--5.760)}{4.55pt}{4.82pt}{} & \HoloSegScore{7.902}{(6.019--10.14)}{4.55pt}{4.82pt}{} & \HoloSegScore{9.794}{(8.409--10.97)}{4.55pt}{4.82pt}{} & \HoloSegScore{8.210}{(6.336--10.61)}{4.55pt}{4.82pt}{} & \HoloSegScore{3.496}{(2.780--4.543)}{4.55pt}{4.82pt}{} \\
\cline{3-11}
 &  &  & \HoloSegMetric{Dice} &  & \HoloSegScore{0.0000}{(0.0000--0.0000)}{4.55pt}{4.82pt}{} & \HoloSegScore{0.7193}{(0.6836--0.7522)}{4.55pt}{4.82pt}{} & \HoloSegScore{0.6930}{(0.6427--0.7351)}{4.55pt}{4.82pt}{} & \HoloSegScore{0.7161}{(0.7097--0.7216)}{4.55pt}{4.82pt}{} & \HoloSegScore{0.5012}{(0.4571--0.5462)}{4.55pt}{4.82pt}{} & \HoloSegScore{0.6857}{(0.6545--0.7116)}{4.55pt}{4.82pt}{} \\*
\softcline{4-4}\softcline{6-11}
 &  & \HoloSegSpan{\makecell[c]{left\\[-0.10ex]internal\\[-0.10ex]carotid\\[-0.10ex]artery}}{2.04cm}{0.32cm} & \HoloSegMetric{HD95} & \raisebox{0.32cm}[0pt][0pt]{\HoloSegUnsupported} & \HoloSegScore{493.7}{(453.6--530.8)}{4.55pt}{4.82pt}{} & \HoloSegScore{4.096}{(2.985--5.364)}{4.55pt}{4.82pt}{} & \HoloSegScore{6.939}{(4.845--9.418)}{4.55pt}{4.82pt}{} & \HoloSegScore{8.430}{(8.410--9.471)}{4.55pt}{4.82pt}{} & \HoloSegScore{11.66}{(8.410--15.79)}{4.55pt}{4.82pt}{} & \HoloSegScore{22.00}{(4.136--57.20)}{4.55pt}{4.82pt}{} \\
\cline{3-11}
 &  &  & \HoloSegMetric{Dice} &  & \HoloSegScore{0.0000}{(0.0000--0.0000)}{4.55pt}{4.82pt}{} & \HoloSegScore{0.8405}{(0.7933--0.8723)}{4.55pt}{4.82pt}{} & \HoloSegScore{0.8869}{(0.8575--0.9125)}{4.55pt}{4.82pt}{} & \HoloSegScore{0.8828}{(0.8801--0.8910)}{4.55pt}{4.82pt}{} & \HoloSegScore{0.7248}{(0.6761--0.7660)}{4.55pt}{4.82pt}{} & \HoloSegScore{0.8436}{(0.8001--0.8785)}{4.55pt}{4.82pt}{} \\*
\softcline{4-4}\softcline{6-11}
 &  & \HoloSegSpan{\makecell[c]{right\\[-0.10ex]internal\\[-0.10ex]jugular vein}}{2.04cm}{0.32cm} & \HoloSegMetric{HD95} & \raisebox{0.32cm}[0pt][0pt]{\HoloSegUnsupported} & \HoloSegScore{349.8}{(329.4--372.3)}{4.55pt}{4.82pt}{} & \HoloSegScore{185.9}{(111.0--261.8)}{4.55pt}{4.82pt}{} & \HoloSegScore{7.732}{(2.358--15.38)}{4.55pt}{4.82pt}{} & \HoloSegScore{8.191}{(6.077--9.213)}{4.55pt}{4.82pt}{} & \HoloSegScore{9.242}{(5.016--16.55)}{4.55pt}{4.82pt}{} & \HoloSegScore{7.338}{(2.438--15.82)}{4.55pt}{4.82pt}{} \\
\cline{3-11}
 &  &  & \HoloSegMetric{Dice} &  & \HoloSegScore{0.0000}{(0.0000--0.0000)}{4.55pt}{4.82pt}{} & \HoloSegScore{0.7837}{(0.7625--0.8034)}{4.55pt}{4.82pt}{} & \HoloSegScore{0.8833}{(0.8665--0.8973)}{4.55pt}{4.82pt}{} & \HoloSegScore{0.8359}{(0.8248--0.8512)}{4.55pt}{4.82pt}{} & \HoloSegScore{0.7659}{(0.7405--0.7902)}{4.55pt}{4.82pt}{} & \HoloSegScore{0.8475}{(0.8316--0.8620)}{4.55pt}{4.82pt}{} \\*
\softcline{4-4}\softcline{6-11}
 &  & \HoloSegSpan{\makecell[c]{left\\[-0.10ex]internal\\[-0.10ex]jugular vein}}{2.04cm}{0.32cm} & \HoloSegMetric{HD95} & \raisebox{0.32cm}[0pt][0pt]{\HoloSegUnsupported} & \HoloSegScore{460.1}{(431.3--488.8)}{4.55pt}{4.82pt}{} & \HoloSegScore{429.2}{(381.9--468.7)}{4.55pt}{4.82pt}{} & \HoloSegScore{3.949}{(2.398--6.378)}{4.55pt}{4.82pt}{} & \HoloSegScore{7.319}{(6.881--10.65)}{4.55pt}{4.82pt}{} & \HoloSegScore{10.56}{(6.761--15.48)}{4.55pt}{4.82pt}{} & \HoloSegScore{9.436}{(6.057--13.91)}{4.55pt}{4.82pt}{} \\
\cline{3-11}
 &  &  & \HoloSegMetric{Dice} & \HoloSegScore{0.7131}{(0.6837--0.7389)}{4.55pt}{4.82pt}{} & \HoloSegScore{0.01764}{(0.01304--0.02257)}{4.20pt}{4.48pt}{} & \HoloSegScore{0.7839}{(0.7574--0.8070)}{4.55pt}{4.82pt}{} & \HoloSegScore{0.8492}{(0.8293--0.8649)}{4.55pt}{4.82pt}{} & \HoloSegScore{0.8279}{(0.8179--0.8340)}{4.55pt}{4.82pt}{} & \HoloSegScore{0.8519}{(0.8364--0.8654)}{4.55pt}{4.82pt}{} & \HoloSegScore{0.8727}{(0.8617--0.8828)}{4.55pt}{4.82pt}{} \\*
\softcline{4-11}
 &  & \HoloSegSpan{\makecell[c]{brachiocephalic\\[-0.10ex]trunk}}{2.04cm}{0.32cm} & \HoloSegMetric{HD95} & \HoloSegScore{31.67}{(24.45--38.38)}{4.55pt}{4.82pt}{} & \HoloSegScore{259.5}{(235.6--278.8)}{4.55pt}{4.82pt}{} & \HoloSegScore{398.6}{(322.2--462.7)}{4.55pt}{4.82pt}{} & \HoloSegScore{5.000}{(4.036--6.013)}{4.55pt}{4.82pt}{} & \HoloSegScore{4.498}{(4.292--5.115)}{4.55pt}{4.82pt}{} & \HoloSegScore{5.242}{(3.861--6.642)}{4.55pt}{4.82pt}{} & \HoloSegScore{2.994}{(2.442--3.763)}{4.55pt}{4.82pt}{} \\
\cline{3-11}
 &  &  & \HoloSegMetric{Dice} & \HoloSegScore{0.5967}{(0.5697--0.6251)}{4.55pt}{4.82pt}{} & \HoloSegScore{0.0000}{(0.0000--0.0000)}{4.55pt}{4.82pt}{} & \HoloSegScore{0.8423}{(0.8200--0.8608)}{4.55pt}{4.82pt}{} & \HoloSegScore{0.8532}{(0.8285--0.8733)}{4.55pt}{4.82pt}{} & \HoloSegScore{0.8531}{(0.8399--0.8551)}{4.55pt}{4.82pt}{} & \HoloSegScore{0.8335}{(0.8155--0.8512)}{4.55pt}{4.82pt}{} & \HoloSegScore{0.8505}{(0.8384--0.8638)}{4.55pt}{4.82pt}{} \\*
\softcline{4-11}
 &  & \HoloSegSpan{\makecell[c]{right\\[-0.10ex]brachiocephalic\\[-0.10ex]vein}}{2.04cm}{0.32cm} & \HoloSegMetric{HD95} & \HoloSegScore{23.48}{(21.11--25.50)}{4.55pt}{4.82pt}{} & \HoloSegScore{361.0}{(334.0--387.3)}{4.55pt}{4.82pt}{} & \HoloSegScore{4.802}{(3.228--7.091)}{4.55pt}{4.82pt}{} & \HoloSegScore{5.831}{(4.203--8.042)}{4.55pt}{4.82pt}{} & \HoloSegScore{5.676}{(3.909--7.417)}{4.55pt}{4.82pt}{} & \HoloSegScore{9.650}{(6.274--14.09)}{4.55pt}{4.82pt}{} & \HoloSegScore{5.927}{(4.254--8.131)}{4.55pt}{4.82pt}{} \\
\cline{3-11}
 &  &  & \HoloSegMetric{Dice} & \HoloSegScore{0.2992}{(0.2731--0.3256)}{4.55pt}{4.82pt}{} & \HoloSegScore{0.0000}{(0.0000--0.0000)}{4.55pt}{4.82pt}{} & \HoloSegScore{0.7839}{(0.7537--0.8095)}{4.55pt}{4.82pt}{} & \HoloSegScore{0.8582}{(0.8366--0.8780)}{4.55pt}{4.82pt}{} & \HoloSegScore{0.8483}{(0.8375--0.8755)}{4.55pt}{4.82pt}{} & \HoloSegScore{0.8408}{(0.8151--0.8631)}{4.55pt}{4.82pt}{} & \HoloSegScore{0.8738}{(0.8624--0.8842)}{4.55pt}{4.82pt}{} \\*
\softcline{4-11}
 &  & \HoloSegSpan{\makecell[c]{left\\[-0.10ex]brachiocephalic\\[-0.10ex]vein}}{2.04cm}{0.32cm} & \HoloSegMetric{HD95} & \HoloSegScore{49.32}{(48.30--50.25)}{4.55pt}{4.82pt}{} & \HoloSegScore{390.4}{(360.0--419.9)}{4.55pt}{4.82pt}{} & \HoloSegScore{173.2}{(104.7--243.6)}{4.55pt}{4.82pt}{} & \HoloSegScore{5.495}{(3.887--7.681)}{4.55pt}{4.82pt}{} & \HoloSegScore{6.837}{(6.031--8.795)}{4.55pt}{4.82pt}{} & \HoloSegScore{16.37}{(9.353--24.34)}{4.55pt}{4.82pt}{} & \HoloSegScore{3.426}{(2.648--4.439)}{4.55pt}{4.82pt}{} \\
\cline{3-11}
 &  &  & \HoloSegMetric{Dice} & \HoloSegScore{0.6952}{(0.6765--0.7120)}{4.55pt}{4.82pt}{} & \HoloSegScore{0.0002523}{(0.0000--0.0007574)}{3.85pt}{4.12pt}{} & \HoloSegScore{0.7656}{(0.7467--0.7828)}{4.55pt}{4.82pt}{} & \HoloSegScore{0.8016}{(0.7854--0.8166)}{4.55pt}{4.82pt}{} & \HoloSegScore{0.7878}{(0.7744--0.7922)}{4.55pt}{4.82pt}{} & \HoloSegScore{0.7804}{(0.7583--0.8012)}{4.55pt}{4.82pt}{} & \HoloSegScore{0.8090}{(0.7945--0.8241)}{4.55pt}{4.82pt}{} \\*
\softcline{4-11}
 &  & \HoloSegSpan{\makecell[c]{right\\[-0.10ex]subclavian\\[-0.10ex]artery}}{2.04cm}{0.32cm} & \HoloSegMetric{HD95} & \HoloSegScore{45.73}{(10.83--84.18)}{4.55pt}{4.82pt}{} & \HoloSegScore{272.3}{(230.3--317.7)}{4.55pt}{4.82pt}{} & \HoloSegScore{30.23}{(4.168--67.93)}{4.55pt}{4.82pt}{} & \HoloSegScore{8.730}{(6.845--10.88)}{4.55pt}{4.82pt}{} & \HoloSegScore{10.96}{(8.097--14.42)}{4.55pt}{4.82pt}{} & \HoloSegScore{7.036}{(5.164--9.132)}{4.55pt}{4.82pt}{} & \HoloSegScore{6.104}{(4.345--8.447)}{4.55pt}{4.82pt}{} \\
\hline
\pagebreak[4]
 &  &  & \HoloSegMetric{Dice} & \HoloSegScore{0.4970}{(0.4317--0.5579)}{4.55pt}{4.82pt}{} & \HoloSegScore{0.0006889}{(0.0000--0.002056)}{4.20pt}{4.48pt}{} & \HoloSegScore{0.7630}{(0.7402--0.7839)}{4.55pt}{4.82pt}{} & \HoloSegScore{0.8524}{(0.8378--0.8658)}{4.55pt}{4.82pt}{} & \HoloSegScore{0.7489}{(0.7314--0.7903)}{4.55pt}{4.82pt}{} & \HoloSegScore{0.8163}{(0.7978--0.8340)}{4.55pt}{4.82pt}{} & \HoloSegScore{0.8282}{(0.8087--0.8451)}{4.55pt}{4.82pt}{} \\*
\softcline{4-11}
 & \HoloSegSpan{\makecell[c]{DAP-Atlas\\[-0.10ex](AutoPETIII)}}{1.86cm}{0.32cm} & \HoloSegSpan{\makecell[c]{left\\[-0.10ex]subclavian\\[-0.10ex]artery}}{2.04cm}{0.32cm} & \HoloSegMetric{HD95} & \HoloSegScore{61.48}{(60.25--62.77)}{4.55pt}{4.82pt}{} & \HoloSegScore{338.6}{(290.2--387.5)}{4.55pt}{4.82pt}{} & \HoloSegScore{245.6}{(173.9--314.6)}{4.55pt}{4.82pt}{} & \HoloSegScore{5.119}{(3.683--6.605)}{4.55pt}{4.82pt}{} & \HoloSegScore{6.036}{(4.774--8.516)}{4.55pt}{4.82pt}{} & \HoloSegScore{7.034}{(3.805--12.04)}{4.55pt}{4.82pt}{} & \HoloSegScore{5.676}{(4.345--7.089)}{4.55pt}{4.82pt}{} \\
\cline{2-11}
 &  &  & \HoloSegMetric{Dice} &  & \HoloSegScore{0.01693}{(0.0005908--0.04238)}{3.85pt}{4.12pt}{} & \HoloSegScore{0.2523}{(0.08824--0.4299)}{4.20pt}{4.48pt}{} & \HoloSegScore{0.6329}{(0.3842--0.7930)}{4.55pt}{4.82pt}{} & \HoloSegScore{0.6576}{(0.6373--0.6712)}{4.55pt}{4.82pt}{} & \HoloSegScore{0.5593}{(0.3316--0.7671)}{4.55pt}{4.82pt}{} & \HoloSegScore{0.6613}{(0.4730--0.8039)}{4.55pt}{4.82pt}{} \\*
\softcline{4-4}\softcline{6-11}
 & \HoloSegSpan{\makecell[c]{FUMPE}}{1.86cm}{0.32cm} & \HoloSegSpan{\makecell[c]{pulmonary\\[-0.10ex]embolism}}{2.04cm}{0.32cm} & \HoloSegMetric{HD95} & \raisebox{0.32cm}[0pt][0pt]{\HoloSegUnsupported} & \HoloSegScore{71.29}{(60.01--83.89)}{4.55pt}{4.82pt}{} & \HoloSegScore{29.91}{(16.67--43.34)}{4.55pt}{4.82pt}{} & \HoloSegScore{29.49}{(7.115--61.80)}{4.55pt}{4.82pt}{} & \HoloSegScore{16.96}{(5.256--29.15)}{4.55pt}{4.82pt}{} & \HoloSegScore{21.02}{(8.213--37.26)}{4.55pt}{4.82pt}{} & \HoloSegScore{18.68}{(9.391--28.36)}{4.55pt}{4.82pt}{} \\
\cline{2-11}
 &  &  & \HoloSegMetric{Dice} & \HoloSegScore{0.07889}{(0.02078--0.1486)}{4.20pt}{4.48pt}{} & \HoloSegScore{0.02781}{(0.000002581--0.06910)}{3.52pt}{3.80pt}{} & \HoloSegScore{0.2075}{(0.1288--0.2919)}{4.55pt}{4.82pt}{} & \HoloSegScore{0.3976}{(0.2999--0.4837)}{4.55pt}{4.82pt}{} & \HoloSegScore{0.4286}{(0.3901--0.4768)}{4.55pt}{4.82pt}{} & \HoloSegScore{0.2866}{(0.2116--0.3738)}{4.55pt}{4.82pt}{} & \HoloSegScore{0.2431}{(0.1748--0.3177)}{4.55pt}{4.82pt}{} \\*
\softcline{4-11}
 & \HoloSegSpan{\makecell[c]{LNDb}}{1.86cm}{0.32cm} & \HoloSegSpan{\makecell[c]{pulmonary\\[-0.10ex]nodule}}{2.04cm}{0.32cm} & \HoloSegMetric{HD95} & \HoloSegScore{143.6}{(120.9--165.6)}{4.55pt}{4.82pt}{} & \HoloSegScore{133.8}{(119.7--148.9)}{4.55pt}{4.82pt}{} & \HoloSegScore{109.4}{(84.78--137.0)}{4.55pt}{4.82pt}{} & \HoloSegScore{111.0}{(87.85--133.4)}{4.55pt}{4.82pt}{} & \HoloSegScore{73.17}{(58.55--89.63)}{4.55pt}{4.82pt}{} & \HoloSegScore{117.6}{(97.83--138.5)}{4.55pt}{4.82pt}{} & \HoloSegScore{101.9}{(80.54--120.9)}{4.55pt}{4.82pt}{} \\
\cline{2-11}
 &  &  & \HoloSegMetric{Dice} &  & \HoloSegScore{0.6081}{(0.5764--0.6324)}{4.55pt}{4.82pt}{} & \HoloSegScore{0.8590}{(0.8444--0.8735)}{4.55pt}{4.82pt}{} & \HoloSegScore{0.5957}{(0.5483--0.6717)}{4.55pt}{4.82pt}{} & \HoloSegScore{0.8313}{(0.7728--0.8543)}{4.55pt}{4.82pt}{} & \HoloSegScore{0.9054}{(0.8950--0.9249)}{4.55pt}{4.82pt}{} & \HoloSegScore{0.9276}{(0.9203--0.9393)}{4.55pt}{4.82pt}{} \\*
\softcline{4-4}\softcline{6-11}
 &  & \HoloSegSpan{\makecell[c]{myocardium}}{2.04cm}{0.32cm} & \HoloSegMetric{HD95} & \raisebox{0.32cm}[0pt][0pt]{\HoloSegUnsupported} & \HoloSegScore{28.93}{(24.38--32.67)}{4.55pt}{4.82pt}{} & \HoloSegScore{3.614}{(3.039--4.306)}{4.55pt}{4.82pt}{} & \HoloSegScore{48.65}{(36.67--59.17)}{4.55pt}{4.82pt}{} & \HoloSegScore{15.38}{(11.66--19.83)}{4.55pt}{4.82pt}{} & \HoloSegScore{2.587}{(2.317--3.006)}{4.55pt}{4.82pt}{} & \HoloSegScore{1.993}{(1.764--2.223)}{4.55pt}{4.82pt}{} \\
\cline{3-11}
 &  &  & \HoloSegMetric{Dice} &  & \HoloSegScore{0.6115}{(0.3514--0.7949)}{4.55pt}{4.82pt}{} & \HoloSegScore{0.9207}{(0.8762--0.9583)}{4.55pt}{4.82pt}{} & \HoloSegScore{0.8315}{(0.8184--0.8446)}{4.55pt}{4.82pt}{} & \HoloSegScore{0.9171}{(0.9085--0.9397)}{4.55pt}{4.82pt}{} & \HoloSegScore{0.9351}{(0.9146--0.9555)}{4.55pt}{4.82pt}{} & \HoloSegScore{0.9602}{(0.9478--0.9726)}{4.55pt}{4.82pt}{} \\*
\softcline{4-4}\softcline{6-11}
 &  & \HoloSegSpan{\makecell[c]{left heart\\[-0.10ex]atrium}}{2.04cm}{0.32cm} & \HoloSegMetric{HD95} & \raisebox{0.32cm}[0pt][0pt]{\HoloSegUnsupported} & \HoloSegScore{27.07}{(12.00--38.92)}{4.55pt}{4.82pt}{} & \HoloSegScore{4.429}{(2.025--6.832)}{4.55pt}{4.82pt}{} & \HoloSegScore{39.38}{(15.60--64.78)}{4.55pt}{4.82pt}{} & \HoloSegScore{5.050}{(2.439--7.131)}{4.55pt}{4.82pt}{} & \HoloSegScore{5.219}{(3.677--8.122)}{4.55pt}{4.82pt}{} & \HoloSegScore{2.027}{(1.550--2.748)}{4.55pt}{4.82pt}{} \\
\cline{3-11}
 &  &  & \HoloSegMetric{Dice} &  & \HoloSegScore{0.6943}{(0.4306--0.8603)}{4.55pt}{4.82pt}{} & \HoloSegScore{0.8864}{(0.8572--0.9157)}{4.55pt}{4.82pt}{} & \HoloSegScore{0.5935}{(0.5135--0.6734)}{4.55pt}{4.82pt}{} & \HoloSegScore{0.8828}{(0.8584--0.8948)}{4.55pt}{4.82pt}{} & \HoloSegScore{0.9441}{(0.9257--0.9626)}{4.55pt}{4.82pt}{} & \HoloSegScore{0.9442}{(0.9253--0.9631)}{4.55pt}{4.82pt}{} \\*
\softcline{4-4}\softcline{6-11}
 &  & \HoloSegSpan{\makecell[c]{left heart\\[-0.10ex]ventricle}}{2.04cm}{0.32cm} & \HoloSegMetric{HD95} & \raisebox{0.32cm}[0pt][0pt]{\HoloSegUnsupported} & \HoloSegScore{19.52}{(7.927--36.93)}{4.55pt}{4.82pt}{} & \HoloSegScore{4.674}{(3.499--5.439)}{4.55pt}{4.82pt}{} & \HoloSegScore{25.21}{(13.34--40.02)}{4.55pt}{4.82pt}{} & \HoloSegScore{6.664}{(6.587--7.614)}{4.55pt}{4.82pt}{} & \HoloSegScore{2.360}{(1.775--3.189)}{4.55pt}{4.82pt}{} & \HoloSegScore{2.265}{(1.820--2.709)}{4.55pt}{4.82pt}{} \\
\cline{3-11}
 &  &  & \HoloSegMetric{Dice} &  & \HoloSegScore{0.2231}{(0.005519--0.4406)}{4.20pt}{4.48pt}{} & \HoloSegScore{0.8987}{(0.8805--0.9169)}{4.55pt}{4.82pt}{} & \HoloSegScore{0.6648}{(0.5830--0.7465)}{4.55pt}{4.82pt}{} & \HoloSegScore{0.8788}{(0.8592--0.9031)}{4.55pt}{4.82pt}{} & \HoloSegScore{0.9248}{(0.9120--0.9323)}{4.55pt}{4.82pt}{} & \HoloSegScore{0.9318}{(0.9231--0.9383)}{4.55pt}{4.82pt}{} \\*
\softcline{4-4}\softcline{6-11}
 & \HoloSegSpan{\makecell[c]{MM-WHS-CT}}{1.86cm}{0.32cm} & \HoloSegSpan{\makecell[c]{right heart\\[-0.10ex]atrium}}{2.04cm}{0.32cm} & \HoloSegMetric{HD95} & \raisebox{0.32cm}[0pt][0pt]{\HoloSegUnsupported} & \HoloSegScore{43.99}{(34.19--54.00)}{4.55pt}{4.82pt}{} & \HoloSegScore{4.969}{(3.809--6.923)}{4.55pt}{4.82pt}{} & \HoloSegScore{57.93}{(47.03--68.45)}{4.55pt}{4.82pt}{} & \HoloSegScore{9.052}{(5.461--10.95)}{4.55pt}{4.82pt}{} & \HoloSegScore{3.451}{(3.159--3.714)}{4.55pt}{4.82pt}{} & \HoloSegScore{2.908}{(2.815--3.029)}{4.55pt}{4.82pt}{} \\
\cline{3-11}
 &  &  & \HoloSegMetric{Dice} &  & \HoloSegScore{0.3194}{(0.09066--0.5370)}{4.20pt}{4.48pt}{} & \HoloSegScore{0.8801}{(0.8400--0.9247)}{4.55pt}{4.82pt}{} & \HoloSegScore{0.7211}{(0.5942--0.8481)}{4.55pt}{4.82pt}{} & \HoloSegScore{0.8574}{(0.8231--0.9139)}{4.55pt}{4.82pt}{} & \HoloSegScore{0.9106}{(0.8794--0.9278)}{4.55pt}{4.82pt}{} & \HoloSegScore{0.9412}{(0.9311--0.9540)}{4.55pt}{4.82pt}{} \\*
\softcline{4-4}\softcline{6-11}
 &  & \HoloSegSpan{\makecell[c]{right heart\\[-0.10ex]ventricle}}{2.04cm}{0.32cm} & \HoloSegMetric{HD95} & \raisebox{0.32cm}[0pt][0pt]{\HoloSegUnsupported} & \HoloSegScore{42.50}{(34.95--51.98)}{4.55pt}{4.82pt}{} & \HoloSegScore{6.131}{(3.849--8.351)}{4.55pt}{4.82pt}{} & \HoloSegScore{18.52}{(9.775--27.26)}{4.55pt}{4.82pt}{} & \HoloSegScore{7.463}{(5.694--8.146)}{4.55pt}{4.82pt}{} & \HoloSegScore{3.989}{(3.255--4.967)}{4.55pt}{4.82pt}{} & \HoloSegScore{2.444}{(2.000--2.750)}{4.55pt}{4.82pt}{} \\
\cline{3-11}
 &  &  & \HoloSegMetric{Dice} &  & \HoloSegScore{0.1904}{(0.0000--0.5455)}{4.55pt}{4.82pt}{} & \HoloSegScore{0.9573}{(0.9509--0.9625)}{4.55pt}{4.82pt}{} & \HoloSegScore{0.9511}{(0.9417--0.9593)}{4.55pt}{4.82pt}{} & \HoloSegScore{0.9397}{(0.9263--0.9497)}{4.55pt}{4.82pt}{} & \HoloSegScore{0.9702}{(0.9600--0.9777)}{4.55pt}{4.82pt}{} & \HoloSegScore{0.9747}{(0.9718--0.9771)}{4.55pt}{4.82pt}{} \\*
\softcline{4-4}\softcline{6-11}
 &  & \HoloSegSpan{\makecell[c]{heart\\[-0.10ex]ascending\\[-0.10ex]aorta}}{2.04cm}{0.32cm} & \HoloSegMetric{HD95} & \raisebox{0.32cm}[0pt][0pt]{\HoloSegUnsupported} & \HoloSegScore{83.21}{(37.65--111.2)}{4.55pt}{4.82pt}{} & \HoloSegScore{1.397}{(1.385--1.414)}{4.55pt}{4.82pt}{} & \HoloSegScore{38.77}{(15.74--61.81)}{4.55pt}{4.82pt}{} & \HoloSegScore{2.480}{(2.303--2.935)}{4.55pt}{4.82pt}{} & \HoloSegScore{1.529}{(0.8414--2.347)}{4.55pt}{4.82pt}{} & \HoloSegScore{0.9220}{(0.7687--1.042)}{4.55pt}{4.82pt}{} \\
\cline{3-11}
 &  &  & \HoloSegMetric{Dice} &  & \HoloSegScore{0.5160}{(0.4455--0.5702)}{4.55pt}{4.82pt}{} & \HoloSegScore{0.8511}{(0.8214--0.8899)}{4.55pt}{4.82pt}{} & \HoloSegScore{0.6634}{(0.5639--0.7630)}{4.55pt}{4.82pt}{} & \HoloSegScore{0.8473}{(0.8358--0.8645)}{4.55pt}{4.82pt}{} & \HoloSegScore{0.9289}{(0.9135--0.9426)}{4.55pt}{4.82pt}{} & \HoloSegScore{0.9409}{(0.9326--0.9498)}{4.55pt}{4.82pt}{} \\*
\softcline{4-4}\softcline{6-11}
\HoloSegSpan{\makecell[c]{\textbf{Internal}}}{1.20cm}{0.32cm} &  & \HoloSegSpan{\makecell[c]{pulmonary\\[-0.10ex]artery}}{2.04cm}{0.32cm} & \HoloSegMetric{HD95} & \raisebox{0.32cm}[0pt][0pt]{\HoloSegUnsupported} & \HoloSegScore{26.11}{(11.01--49.00)}{4.55pt}{4.82pt}{} & \HoloSegScore{12.62}{(5.990--16.83)}{4.55pt}{4.82pt}{} & \HoloSegScore{60.64}{(49.40--78.45)}{4.55pt}{4.82pt}{} & \HoloSegScore{12.46}{(6.757--16.83)}{4.55pt}{4.82pt}{} & \HoloSegScore{6.162}{(2.967--9.357)}{4.55pt}{4.82pt}{} & \HoloSegScore{4.429}{(2.413--6.446)}{4.55pt}{4.82pt}{} \\
\cline{2-11}
 &  &  & \HoloSegMetric{Dice} &  & \HoloSegScore{0.6153}{(0.5603--0.6702)}{4.55pt}{4.82pt}{} & \HoloSegScore{0.8625}{(0.8477--0.8749)}{4.55pt}{4.82pt}{} & \HoloSegScore{0.8420}{(0.8162--0.8658)}{4.55pt}{4.82pt}{} & \HoloSegScore{0.8273}{(0.8071--0.8351)}{4.55pt}{4.82pt}{} & \HoloSegScore{0.8754}{(0.8597--0.8892)}{4.55pt}{4.82pt}{} & \HoloSegScore{0.8819}{(0.8675--0.8937)}{4.55pt}{4.82pt}{} \\*
\softcline{4-4}\softcline{6-11}
 &  & \HoloSegSpan{\makecell[c]{brainstem}}{2.04cm}{0.32cm} & \HoloSegMetric{HD95} & \raisebox{0.32cm}[0pt][0pt]{\HoloSegUnsupported} & \HoloSegScore{9.847}{(7.874--12.45)}{4.55pt}{4.82pt}{} & \HoloSegScore{3.884}{(3.238--4.656)}{4.55pt}{4.82pt}{} & \HoloSegScore{6.226}{(4.205--8.293)}{4.55pt}{4.82pt}{} & \HoloSegScore{5.746}{(4.387--6.782)}{4.55pt}{4.82pt}{} & \HoloSegScore{3.726}{(3.100--4.454)}{4.55pt}{4.82pt}{} & \HoloSegScore{3.211}{(2.724--3.688)}{4.55pt}{4.82pt}{} \\
\cline{3-11}
 &  &  & \HoloSegMetric{Dice} &  & \HoloSegScore{0.0000}{(0.0000--0.0000)}{4.55pt}{4.82pt}{} & \HoloSegScore{0.5630}{(0.4955--0.6301)}{4.55pt}{4.82pt}{} & \HoloSegScore{0.4431}{(0.3986--0.4980)}{4.55pt}{4.82pt}{} & \HoloSegScore{0.4965}{(0.4574--0.5488)}{4.55pt}{4.82pt}{} & \HoloSegScore{0.6481}{(0.6062--0.6896)}{4.55pt}{4.82pt}{} & \HoloSegScore{0.7737}{(0.7439--0.7999)}{4.55pt}{4.82pt}{} \\*
\softcline{4-4}\softcline{6-11}
 &  & \HoloSegSpan{\makecell[c]{optic chiasm}}{2.04cm}{0.32cm} & \HoloSegMetric{HD95} & \raisebox{0.32cm}[0pt][0pt]{\HoloSegUnsupported} & \HoloSegScore{175.9}{(171.7--181.1)}{4.55pt}{4.82pt}{} & \HoloSegScore{3.822}{(3.291--4.444)}{4.55pt}{4.82pt}{} & \HoloSegScore{5.338}{(4.598--6.106)}{4.55pt}{4.82pt}{} & \HoloSegScore{5.315}{(3.458--5.822)}{4.55pt}{4.82pt}{} & \HoloSegScore{3.282}{(2.928--3.815)}{4.55pt}{4.82pt}{} & \HoloSegScore{2.741}{(1.802--3.896)}{4.55pt}{4.82pt}{} \\
\cline{3-11}
 &  &  & \HoloSegMetric{Dice} &  & \HoloSegScore{0.5184}{(0.4733--0.5575)}{4.55pt}{4.82pt}{} & \HoloSegScore{0.8954}{(0.8873--0.9033)}{4.55pt}{4.82pt}{} & \HoloSegScore{0.8949}{(0.8826--0.9076)}{4.55pt}{4.82pt}{} & \HoloSegScore{0.8638}{(0.8474--0.8830)}{4.55pt}{4.82pt}{} & \HoloSegScore{0.8673}{(0.8469--0.8848)}{4.55pt}{4.82pt}{} & \HoloSegScore{0.9125}{(0.9052--0.9193)}{4.55pt}{4.82pt}{} \\*
\softcline{4-4}\softcline{6-11}
 &  & \HoloSegSpan{\makecell[c]{mandible}}{2.04cm}{0.32cm} & \HoloSegMetric{HD95} & \raisebox{0.32cm}[0pt][0pt]{\HoloSegUnsupported} & \HoloSegScore{15.28}{(12.02--18.88)}{4.55pt}{4.82pt}{} & \HoloSegScore{2.492}{(2.183--2.762)}{4.55pt}{4.82pt}{} & \HoloSegScore{2.156}{(1.724--2.576)}{4.55pt}{4.82pt}{} & \HoloSegScore{3.863}{(3.050--3.866)}{4.55pt}{4.82pt}{} & \HoloSegScore{7.679}{(3.631--12.67)}{4.55pt}{4.82pt}{} & \HoloSegScore{1.938}{(1.500--2.398)}{4.55pt}{4.82pt}{} \\
\cline{3-11}
 &  &  & \HoloSegMetric{Dice} &  & \HoloSegScore{0.0000}{(0.0000--0.0000)}{4.55pt}{4.82pt}{} & \HoloSegScore{0.7070}{(0.6452--0.7620)}{4.55pt}{4.82pt}{} & \HoloSegScore{0.6626}{(0.6272--0.6959)}{4.55pt}{4.82pt}{} & \HoloSegScore{0.6577}{(0.6156--0.7051)}{4.55pt}{4.82pt}{} & \HoloSegScore{0.7765}{(0.7505--0.8053)}{4.55pt}{4.82pt}{} & \HoloSegScore{0.8098}{(0.7812--0.8354)}{4.55pt}{4.82pt}{} \\*
\softcline{4-4}\softcline{6-11}
 &  & \HoloSegSpan{\makecell[c]{left optic\\[-0.10ex]nerve}}{2.04cm}{0.32cm} & \HoloSegMetric{HD95} & \raisebox{0.32cm}[0pt][0pt]{\HoloSegUnsupported} & \HoloSegScore{106.5}{(77.89--133.2)}{4.55pt}{4.82pt}{} & \HoloSegScore{2.792}{(1.774--3.960)}{4.55pt}{4.82pt}{} & \HoloSegScore{11.85}{(9.834--13.80)}{4.55pt}{4.82pt}{} & \HoloSegScore{3.332}{(2.372--4.161)}{4.55pt}{4.82pt}{} & \HoloSegScore{10.58}{(2.947--19.88)}{4.55pt}{4.82pt}{} & \HoloSegScore{1.654}{(1.200--2.174)}{4.55pt}{4.82pt}{} \\
\cline{3-11}
 &  &  & \HoloSegMetric{Dice} &  & \HoloSegScore{0.02323}{(0.006107--0.04765)}{3.85pt}{4.12pt}{} & \HoloSegScore{0.6973}{(0.6530--0.7342)}{4.55pt}{4.82pt}{} & \HoloSegScore{0.6758}{(0.6194--0.7272)}{4.55pt}{4.82pt}{} & \HoloSegScore{0.6794}{(0.6733--0.7025)}{4.55pt}{4.82pt}{} & \HoloSegScore{0.7632}{(0.7186--0.8023)}{4.55pt}{4.82pt}{} & \HoloSegScore{0.7601}{(0.7186--0.7974)}{4.55pt}{4.82pt}{} \\*
\softcline{4-4}\softcline{6-11}
 & \HoloSegSpan{\makecell[c]{PDDCA}}{1.86cm}{0.32cm} & \HoloSegSpan{\makecell[c]{right optic\\[-0.10ex]nerve}}{2.04cm}{0.32cm} & \HoloSegMetric{HD95} & \raisebox{0.32cm}[0pt][0pt]{\HoloSegUnsupported} & \HoloSegScore{68.86}{(39.27--103.1)}{4.55pt}{4.82pt}{} & \HoloSegScore{2.606}{(2.055--3.097)}{4.55pt}{4.82pt}{} & \HoloSegScore{8.878}{(7.019--10.64)}{4.55pt}{4.82pt}{} & \HoloSegScore{5.081}{(3.547--8.034)}{4.55pt}{4.82pt}{} & \HoloSegScore{5.623}{(2.312--10.04)}{4.55pt}{4.82pt}{} & \HoloSegScore{1.983}{(1.344--2.747)}{4.55pt}{4.82pt}{} \\
\cline{3-11}
 &  &  & \HoloSegMetric{Dice} &  & \HoloSegScore{0.5095}{(0.3683--0.6314)}{4.55pt}{4.82pt}{} & \HoloSegScore{0.8597}{(0.8442--0.8744)}{4.55pt}{4.82pt}{} & \HoloSegScore{0.8560}{(0.8368--0.8737)}{4.55pt}{4.82pt}{} & \HoloSegScore{0.8591}{(0.8443--0.8683)}{4.55pt}{4.82pt}{} & \HoloSegScore{0.8626}{(0.8442--0.8784)}{4.55pt}{4.82pt}{} & \HoloSegScore{0.8806}{(0.8696--0.8898)}{4.55pt}{4.82pt}{} \\*
\softcline{4-4}\softcline{6-11}
 &  & \HoloSegSpan{\makecell[c]{left parotid\\[-0.10ex]gland}}{2.04cm}{0.32cm} & \HoloSegMetric{HD95} & \raisebox{0.32cm}[0pt][0pt]{\HoloSegUnsupported} & \HoloSegScore{24.98}{(11.64--43.96)}{4.55pt}{4.82pt}{} & \HoloSegScore{4.398}{(3.305--5.606)}{4.55pt}{4.82pt}{} & \HoloSegScore{6.265}{(4.040--9.234)}{4.55pt}{4.82pt}{} & \HoloSegScore{6.543}{(4.460--6.710)}{4.55pt}{4.82pt}{} & \HoloSegScore{3.965}{(3.183--5.232)}{4.55pt}{4.82pt}{} & \HoloSegScore{3.348}{(2.822--4.028)}{4.55pt}{4.82pt}{} \\
\cline{3-11}
 &  &  & \HoloSegMetric{Dice} &  & \HoloSegScore{0.4319}{(0.3026--0.5364)}{4.55pt}{4.82pt}{} & \HoloSegScore{0.8115}{(0.7407--0.8584)}{4.55pt}{4.82pt}{} & \HoloSegScore{0.8049}{(0.7109--0.8639)}{4.55pt}{4.82pt}{} & \HoloSegScore{0.7940}{(0.7560--0.8142)}{4.55pt}{4.82pt}{} & \HoloSegScore{0.8499}{(0.8137--0.8795)}{4.55pt}{4.82pt}{} & \HoloSegScore{0.8803}{(0.8674--0.8915)}{4.55pt}{4.82pt}{} \\*
\softcline{4-4}\softcline{6-11}
 &  & \HoloSegSpan{\makecell[c]{right\\[-0.10ex]parotid\\[-0.10ex]gland}}{2.04cm}{0.32cm} & \HoloSegMetric{HD95} & \raisebox{0.32cm}[0pt][0pt]{\HoloSegUnsupported} & \HoloSegScore{39.31}{(21.77--62.28)}{4.55pt}{4.82pt}{} & \HoloSegScore{5.413}{(3.928--7.804)}{4.55pt}{4.82pt}{} & \HoloSegScore{9.726}{(5.397--13.99)}{4.55pt}{4.82pt}{} & \HoloSegScore{7.985}{(6.031--9.407)}{4.55pt}{4.82pt}{} & \HoloSegScore{5.249}{(3.556--7.514)}{4.55pt}{4.82pt}{} & \HoloSegScore{3.204}{(2.621--4.069)}{4.55pt}{4.82pt}{} \\
\cline{3-11}
 &  &  & \HoloSegMetric{Dice} &  & \HoloSegScore{0.2459}{(0.1449--0.3622)}{4.55pt}{4.82pt}{} & \HoloSegScore{0.7976}{(0.7579--0.8336)}{4.55pt}{4.82pt}{} & \HoloSegScore{0.8127}{(0.7682--0.8477)}{4.55pt}{4.82pt}{} & \HoloSegScore{0.7917}{(0.7705--0.8159)}{4.55pt}{4.82pt}{} & \HoloSegScore{0.8431}{(0.8226--0.8623)}{4.55pt}{4.82pt}{} & \HoloSegScore{0.8555}{(0.8369--0.8771)}{4.55pt}{4.82pt}{} \\*
\softcline{4-4}\softcline{6-11}
 &  & \HoloSegSpan{\makecell[c]{left\\[-0.10ex]submandibular\\[-0.10ex]gland}}{2.04cm}{0.32cm} & \HoloSegMetric{HD95} & \raisebox{0.32cm}[0pt][0pt]{\HoloSegUnsupported} & \HoloSegScore{63.69}{(40.89--84.26)}{4.55pt}{4.82pt}{} & \HoloSegScore{4.417}{(3.253--5.760)}{4.55pt}{4.82pt}{} & \HoloSegScore{4.063}{(3.114--5.333)}{4.55pt}{4.82pt}{} & \HoloSegScore{6.889}{(6.157--8.636)}{4.55pt}{4.82pt}{} & \HoloSegScore{3.208}{(2.399--4.338)}{4.55pt}{4.82pt}{} & \HoloSegScore{2.354}{(1.970--2.694)}{4.55pt}{4.82pt}{} \\
\cline{3-11}
 &  &  & \HoloSegMetric{Dice} &  & \HoloSegScore{0.2038}{(0.1526--0.2576)}{4.55pt}{4.82pt}{} & \HoloSegScore{0.7851}{(0.7607--0.8089)}{4.55pt}{4.82pt}{} & \HoloSegScore{0.7615}{(0.7223--0.7995)}{4.55pt}{4.82pt}{} & \HoloSegScore{0.7455}{(0.7187--0.7795)}{4.55pt}{4.82pt}{} & \HoloSegScore{0.8442}{(0.8220--0.8634)}{4.55pt}{4.82pt}{} & \HoloSegScore{0.8433}{(0.8210--0.8637)}{4.55pt}{4.82pt}{} \\*
\softcline{4-4}\softcline{6-11}
 &  & \HoloSegSpan{\makecell[c]{right\\[-0.10ex]submandibular\\[-0.10ex]gland}}{2.04cm}{0.32cm} & \HoloSegMetric{HD95} & \raisebox{0.32cm}[0pt][0pt]{\HoloSegUnsupported} & \HoloSegScore{42.13}{(24.70--60.87)}{4.55pt}{4.82pt}{} & \HoloSegScore{4.741}{(3.549--6.021)}{4.55pt}{4.82pt}{} & \HoloSegScore{5.828}{(4.385--7.428)}{4.55pt}{4.82pt}{} & \HoloSegScore{5.632}{(3.594--7.057)}{4.55pt}{4.82pt}{} & \HoloSegScore{2.553}{(2.305--2.847)}{4.55pt}{4.82pt}{} & \HoloSegScore{2.601}{(2.379--2.873)}{4.55pt}{4.82pt}{} \\
\hline
\pagebreak[4]
 &  &  & \HoloSegMetric{Dice} &  & \HoloSegScore{0.4241}{(0.4018--0.4473)}{4.55pt}{4.82pt}{} & \HoloSegScore{0.7171}{(0.6921--0.7391)}{4.55pt}{4.82pt}{} & \HoloSegScore{0.7607}{(0.7380--0.7802)}{4.55pt}{4.82pt}{} & \HoloSegScore{0.7608}{(0.7444--0.7797)}{4.55pt}{4.82pt}{} & \HoloSegScore{0.6592}{(0.6368--0.6813)}{4.55pt}{4.82pt}{} & \HoloSegScore{0.6863}{(0.6633--0.7088)}{4.55pt}{4.82pt}{} \\*
\softcline{4-4}\softcline{6-11}
 & \HoloSegSpan{\makecell[c]{Parse2022}}{1.86cm}{0.32cm} & \HoloSegSpan{\makecell[c]{pulmonary\\[-0.10ex]artery}}{2.04cm}{0.32cm} & \HoloSegMetric{HD95} & \raisebox{0.32cm}[0pt][0pt]{\HoloSegUnsupported} & \HoloSegScore{91.97}{(88.05--95.73)}{4.55pt}{4.82pt}{} & \HoloSegScore{12.71}{(9.875--16.87)}{4.55pt}{4.82pt}{} & \HoloSegScore{10.51}{(10.04--10.98)}{4.55pt}{4.82pt}{} & \HoloSegScore{15.15}{(14.31--16.02)}{4.55pt}{4.82pt}{} & \HoloSegScore{37.47}{(35.63--39.20)}{4.55pt}{4.82pt}{} & \HoloSegScore{17.88}{(16.90--19.02)}{4.55pt}{4.82pt}{} \\
\cline{2-11}
 &  &  & \HoloSegMetric{Dice} & \HoloSegScore{0.7740}{(0.6601--0.8384)}{4.55pt}{4.82pt}{} & \HoloSegScore{0.5003}{(0.3442--0.6359)}{4.55pt}{4.82pt}{} & \HoloSegScore{0.8306}{(0.7755--0.8700)}{4.55pt}{4.82pt}{} & \HoloSegScore{0.8418}{(0.8217--0.8637)}{4.55pt}{4.82pt}{} & \HoloSegScore{0.8664}{(0.8567--0.8931)}{4.55pt}{4.82pt}{} & \HoloSegScore{0.8479}{(0.8235--0.8706)}{4.55pt}{4.82pt}{} & \HoloSegScore{0.8711}{(0.8524--0.8904)}{4.55pt}{4.82pt}{} \\*
\softcline{4-11}
 & \HoloSegSpan{\makecell[c]{SEGA}}{1.86cm}{0.32cm} & \HoloSegSpan{\makecell[c]{aorta}}{2.04cm}{0.32cm} & \HoloSegMetric{HD95} & \HoloSegScore{13.70}{(9.765--17.13)}{4.55pt}{4.82pt}{} & \HoloSegScore{109.0}{(77.64--139.2)}{4.55pt}{4.82pt}{} & \HoloSegScore{41.59}{(20.42--66.65)}{4.55pt}{4.82pt}{} & \HoloSegScore{133.3}{(89.68--175.8)}{4.55pt}{4.82pt}{} & \HoloSegScore{16.95}{(10.61--22.16)}{4.55pt}{4.82pt}{} & \HoloSegScore{82.98}{(45.52--126.3)}{4.55pt}{4.82pt}{} & \HoloSegScore{44.09}{(23.92--80.65)}{4.55pt}{4.82pt}{} \\
\cline{2-11}
 &  &  & \HoloSegMetric{Dice} & \HoloSegScore{0.9660}{(0.9634--0.9679)}{4.55pt}{4.82pt}{} & \HoloSegScore{0.1132}{(0.05332--0.1867)}{4.20pt}{4.48pt}{} & \HoloSegScore{0.9655}{(0.9640--0.9669)}{4.55pt}{4.82pt}{} & \HoloSegScore{0.9783}{(0.9775--0.9791)}{4.55pt}{4.82pt}{} & \HoloSegScore{0.9673}{(0.9599--0.9791)}{4.55pt}{4.82pt}{} & \HoloSegScore{0.9692}{(0.9677--0.9706)}{4.55pt}{4.82pt}{} & \HoloSegScore{0.9755}{(0.9747--0.9763)}{4.55pt}{4.82pt}{} \\*
\softcline{4-11}
 &  & \HoloSegSpan{\makecell[c]{brain}}{2.04cm}{0.32cm} & \HoloSegMetric{HD95} & \HoloSegScore{33.44}{(3.443--73.77)}{4.55pt}{4.82pt}{} & \HoloSegScore{78.50}{(70.50--85.79)}{4.55pt}{4.82pt}{} & \HoloSegScore{21.30}{(14.64--27.55)}{4.55pt}{4.82pt}{} & \HoloSegScore{2.783}{(2.657--2.894)}{4.55pt}{4.82pt}{} & \HoloSegScore{5.422}{(4.875--6.679)}{4.55pt}{4.82pt}{} & \HoloSegScore{15.54}{(10.17--21.44)}{4.55pt}{4.82pt}{} & \HoloSegScore{25.93}{(3.705--60.01)}{4.55pt}{4.82pt}{} \\
\cline{3-11}
 &  &  & \HoloSegMetric{Dice} &  & \HoloSegScore{0.4554}{(0.3789--0.5264)}{4.55pt}{4.82pt}{} & \HoloSegScore{0.9065}{(0.8986--0.9140)}{4.55pt}{4.82pt}{} & \HoloSegScore{0.8634}{(0.8476--0.8785)}{4.55pt}{4.82pt}{} & \HoloSegScore{0.8930}{(0.8798--0.8990)}{4.55pt}{4.82pt}{} & \HoloSegScore{0.8884}{(0.8836--0.8940)}{4.55pt}{4.82pt}{} & \HoloSegScore{0.8853}{(0.8777--0.8924)}{4.55pt}{4.82pt}{} \\*
\softcline{4-4}\softcline{6-11}
 &  & \HoloSegSpan{\makecell[c]{brainstem}}{2.04cm}{0.32cm} & \HoloSegMetric{HD95} & \raisebox{0.32cm}[0pt][0pt]{\HoloSegUnsupported} & \HoloSegScore{27.82}{(19.52--37.81)}{4.55pt}{4.82pt}{} & \HoloSegScore{3.224}{(2.956--3.552)}{4.55pt}{4.82pt}{} & \HoloSegScore{4.249}{(3.554--5.067)}{4.55pt}{4.82pt}{} & \HoloSegScore{4.565}{(4.262--5.158)}{4.55pt}{4.82pt}{} & \HoloSegScore{3.266}{(3.052--3.559)}{4.55pt}{4.82pt}{} & \HoloSegScore{3.147}{(2.936--3.413)}{4.55pt}{4.82pt}{} \\
\cline{3-11}
 &  &  & \HoloSegMetric{Dice} &  & \HoloSegScore{0.0000}{(0.0000--0.0000)}{4.55pt}{4.82pt}{} & \HoloSegScore{0.6811}{(0.6291--0.7325)}{4.55pt}{4.82pt}{} & \HoloSegScore{0.5421}{(0.4857--0.5945)}{4.55pt}{4.82pt}{} & \HoloSegScore{0.6743}{(0.6635--0.6854)}{4.55pt}{4.82pt}{} & \HoloSegScore{0.6744}{(0.6394--0.7064)}{4.55pt}{4.82pt}{} & \HoloSegScore{0.7272}{(0.6940--0.7570)}{4.55pt}{4.82pt}{} \\*
\softcline{4-4}\softcline{6-11}
 &  & \HoloSegSpan{\makecell[c]{optic chiasm}}{2.04cm}{0.32cm} & \HoloSegMetric{HD95} & \raisebox{0.32cm}[0pt][0pt]{\HoloSegUnsupported} & \HoloSegScore{144.2}{(126.9--157.2)}{4.55pt}{4.82pt}{} & \HoloSegScore{13.89}{(2.634--36.01)}{4.55pt}{4.82pt}{} & \HoloSegScore{4.145}{(3.810--4.527)}{4.55pt}{4.82pt}{} & \HoloSegScore{5.145}{(4.137--7.064)}{4.55pt}{4.82pt}{} & \HoloSegScore{3.276}{(3.100--3.490)}{4.55pt}{4.82pt}{} & \HoloSegScore{2.714}{(2.430--2.986)}{4.55pt}{4.82pt}{} \\
\cline{3-11}
 &  &  & \HoloSegMetric{Dice} &  & \HoloSegScore{0.0005553}{(0.0000--0.001666)}{4.20pt}{4.48pt}{} & \HoloSegScore{0.9352}{(0.9273--0.9413)}{4.55pt}{4.82pt}{} & \HoloSegScore{0.9117}{(0.9032--0.9193)}{4.55pt}{4.82pt}{} & \HoloSegScore{0.9339}{(0.9300--0.9388)}{4.55pt}{4.82pt}{} & \HoloSegScore{0.8920}{(0.8825--0.8998)}{4.55pt}{4.82pt}{} & \HoloSegScore{0.9183}{(0.9103--0.9248)}{4.55pt}{4.82pt}{} \\*
\softcline{4-4}\softcline{6-11}
 &  & \HoloSegSpan{\makecell[c]{left\\[-0.10ex]temporal\\[-0.10ex]lobe}}{2.04cm}{0.32cm} & \HoloSegMetric{HD95} & \raisebox{0.32cm}[0pt][0pt]{\HoloSegUnsupported} & \HoloSegScore{74.62}{(67.20--86.61)}{4.55pt}{4.82pt}{} & \HoloSegScore{35.01}{(2.894--83.21)}{4.55pt}{4.82pt}{} & \HoloSegScore{4.066}{(3.545--4.633)}{4.55pt}{4.82pt}{} & \HoloSegScore{5.290}{(4.008--5.398)}{4.55pt}{4.82pt}{} & \HoloSegScore{4.539}{(4.079--5.163)}{4.55pt}{4.82pt}{} & \HoloSegScore{17.46}{(3.903--44.21)}{4.55pt}{4.82pt}{} \\
\cline{3-11}
 &  &  & \HoloSegMetric{Dice} &  & \HoloSegScore{0.0000}{(0.0000--0.0000)}{4.55pt}{4.82pt}{} & \HoloSegScore{0.9380}{(0.9335--0.9424)}{4.55pt}{4.82pt}{} & \HoloSegScore{0.9169}{(0.9089--0.9241)}{4.55pt}{4.82pt}{} & \HoloSegScore{0.9239}{(0.9214--0.9298)}{4.55pt}{4.82pt}{} & \HoloSegScore{0.9067}{(0.8996--0.9132)}{4.55pt}{4.82pt}{} & \HoloSegScore{0.8993}{(0.8883--0.9085)}{4.55pt}{4.82pt}{} \\*
\softcline{4-4}\softcline{6-11}
 &  & \HoloSegSpan{\makecell[c]{right\\[-0.10ex]temporal\\[-0.10ex]lobe}}{2.04cm}{0.32cm} & \HoloSegMetric{HD95} & \raisebox{0.32cm}[0pt][0pt]{\HoloSegUnsupported} & \HoloSegScore{75.77}{(72.17--80.32)}{4.55pt}{4.82pt}{} & \HoloSegScore{3.025}{(2.903--3.159)}{4.55pt}{4.82pt}{} & \HoloSegScore{4.164}{(3.634--4.730)}{4.55pt}{4.82pt}{} & \HoloSegScore{3.767}{(2.429--5.315)}{4.55pt}{4.82pt}{} & \HoloSegScore{4.333}{(3.892--4.881)}{4.55pt}{4.82pt}{} & \HoloSegScore{4.173}{(3.787--4.560)}{4.55pt}{4.82pt}{} \\
\cline{3-11}
 &  &  & \HoloSegMetric{Dice} &  & \HoloSegScore{0.0000}{(0.0000--0.0000)}{4.55pt}{4.82pt}{} & \HoloSegScore{0.7873}{(0.7573--0.8163)}{4.55pt}{4.82pt}{} & \HoloSegScore{0.7328}{(0.6903--0.7691)}{4.55pt}{4.82pt}{} & \HoloSegScore{0.7801}{(0.7795--0.7856)}{4.55pt}{4.82pt}{} & \HoloSegScore{0.7372}{(0.7076--0.7640)}{4.55pt}{4.82pt}{} & \HoloSegScore{0.7952}{(0.7728--0.8166)}{4.55pt}{4.82pt}{} \\*
\softcline{4-4}\softcline{6-11}
 &  & \HoloSegSpan{\makecell[c]{left\\[-0.10ex]hippocampus}}{2.04cm}{0.32cm} & \HoloSegMetric{HD95} & \raisebox{0.32cm}[0pt][0pt]{\HoloSegUnsupported} & \HoloSegScore{113.9}{(99.57--132.9)}{4.55pt}{4.82pt}{} & \HoloSegScore{2.803}{(2.541--3.078)}{4.55pt}{4.82pt}{} & \HoloSegScore{18.74}{(3.289--49.20)}{4.55pt}{4.82pt}{} & \HoloSegScore{3.809}{(2.731--4.990)}{4.55pt}{4.82pt}{} & \HoloSegScore{3.821}{(3.393--4.332)}{4.55pt}{4.82pt}{} & \HoloSegScore{2.938}{(2.613--3.380)}{4.55pt}{4.82pt}{} \\
\cline{3-11}
 &  &  & \HoloSegMetric{Dice} &  & \HoloSegScore{0.0000}{(0.0000--0.0000)}{4.55pt}{4.82pt}{} & \HoloSegScore{0.7719}{(0.7319--0.8033)}{4.55pt}{4.82pt}{} & \HoloSegScore{0.7289}{(0.6923--0.7629)}{4.55pt}{4.82pt}{} & \HoloSegScore{0.7565}{(0.7495--0.7736)}{4.55pt}{4.82pt}{} & \HoloSegScore{0.7405}{(0.7113--0.7651)}{4.55pt}{4.82pt}{} & \HoloSegScore{0.7559}{(0.7269--0.7866)}{4.55pt}{4.82pt}{} \\*
\softcline{4-4}\softcline{6-11}
 &  & \HoloSegSpan{\makecell[c]{right\\[-0.10ex]hippocampus}}{2.04cm}{0.32cm} & \HoloSegMetric{HD95} & \raisebox{0.32cm}[0pt][0pt]{\HoloSegUnsupported} & \HoloSegScore{127.3}{(117.7--142.7)}{4.55pt}{4.82pt}{} & \HoloSegScore{2.823}{(2.546--3.165)}{4.55pt}{4.82pt}{} & \HoloSegScore{3.707}{(3.217--4.227)}{4.55pt}{4.82pt}{} & \HoloSegScore{5.969}{(5.365--6.873)}{4.55pt}{4.82pt}{} & \HoloSegScore{9.871}{(5.584--15.69)}{4.55pt}{4.82pt}{} & \HoloSegScore{3.796}{(2.854--5.174)}{4.55pt}{4.82pt}{} \\
\cline{3-11}
 &  &  & \HoloSegMetric{Dice} &  & \HoloSegScore{0.3173}{(0.2483--0.3906)}{4.55pt}{4.82pt}{} & \HoloSegScore{0.9342}{(0.9266--0.9404)}{4.55pt}{4.82pt}{} & \HoloSegScore{0.8972}{(0.8738--0.9129)}{4.55pt}{4.82pt}{} & \HoloSegScore{0.8747}{(0.8502--0.8843)}{4.55pt}{4.82pt}{} & \HoloSegScore{0.9198}{(0.9133--0.9262)}{4.55pt}{4.82pt}{} & \HoloSegScore{0.9368}{(0.9309--0.9428)}{4.55pt}{4.82pt}{} \\*
\softcline{4-4}\softcline{6-11}
\HoloSegSpan{\makecell[c]{\textbf{Internal}}}{1.20cm}{0.32cm} &  & \HoloSegSpan{\makecell[c]{left eyeball}}{2.04cm}{0.32cm} & \HoloSegMetric{HD95} & \raisebox{0.32cm}[0pt][0pt]{\HoloSegUnsupported} & \HoloSegScore{30.06}{(13.69--55.30)}{4.55pt}{4.82pt}{} & \HoloSegScore{1.623}{(1.355--1.932)}{4.55pt}{4.82pt}{} & \HoloSegScore{2.054}{(1.783--2.346)}{4.55pt}{4.82pt}{} & \HoloSegScore{3.295}{(3.281--4.255)}{4.55pt}{4.82pt}{} & \HoloSegScore{2.019}{(1.732--2.271)}{4.55pt}{4.82pt}{} & \HoloSegScore{14.05}{(1.278--39.38)}{4.55pt}{4.82pt}{} \\
\cline{3-11}
 &  &  & \HoloSegMetric{Dice} &  & \HoloSegScore{0.3824}{(0.3106--0.4545)}{4.55pt}{4.82pt}{} & \HoloSegScore{0.9232}{(0.9099--0.9335)}{4.55pt}{4.82pt}{} & \HoloSegScore{0.8977}{(0.8828--0.9107)}{4.55pt}{4.82pt}{} & \HoloSegScore{0.8816}{(0.8675--0.8871)}{4.55pt}{4.82pt}{} & \HoloSegScore{0.9141}{(0.9025--0.9243)}{4.55pt}{4.82pt}{} & \HoloSegScore{0.9287}{(0.9199--0.9365)}{4.55pt}{4.82pt}{} \\*
\softcline{4-4}\softcline{6-11}
 & \HoloSegSpan{\makecell[c]{SegRap2023-\\[-0.10ex]Task1}}{1.86cm}{0.32cm} & \HoloSegSpan{\makecell[c]{right\\[-0.10ex]eyeball}}{2.04cm}{0.32cm} & \HoloSegMetric{HD95} & \raisebox{0.32cm}[0pt][0pt]{\HoloSegUnsupported} & \HoloSegScore{17.24}{(11.09--24.63)}{4.55pt}{4.82pt}{} & \HoloSegScore{1.753}{(1.497--2.038)}{4.55pt}{4.82pt}{} & \HoloSegScore{2.343}{(2.068--2.632)}{4.55pt}{4.82pt}{} & \HoloSegScore{2.920}{(2.178--3.799)}{4.55pt}{4.82pt}{} & \HoloSegScore{4.567}{(1.791--9.789)}{4.55pt}{4.82pt}{} & \HoloSegScore{1.577}{(1.313--1.875)}{4.55pt}{4.82pt}{} \\
\cline{3-11}
 &  &  & \HoloSegMetric{Dice} &  & \HoloSegScore{0.04166}{(0.02331--0.06401)}{4.20pt}{4.48pt}{} & \HoloSegScore{0.7540}{(0.7287--0.7778)}{4.55pt}{4.82pt}{} & \HoloSegScore{0.7133}{(0.6823--0.7454)}{4.55pt}{4.82pt}{} & \HoloSegScore{0.7263}{(0.7120--0.7416)}{4.55pt}{4.82pt}{} & \HoloSegScore{0.7640}{(0.7416--0.7864)}{4.55pt}{4.82pt}{} & \HoloSegScore{0.8307}{(0.8036--0.8555)}{4.55pt}{4.82pt}{} \\*
\softcline{4-4}\softcline{6-11}
 &  & \HoloSegSpan{\makecell[c]{left lens}}{2.04cm}{0.32cm} & \HoloSegMetric{HD95} & \raisebox{0.32cm}[0pt][0pt]{\HoloSegUnsupported} & \HoloSegScore{62.95}{(42.04--85.42)}{4.55pt}{4.82pt}{} & \HoloSegScore{2.128}{(1.757--2.487)}{4.55pt}{4.82pt}{} & \HoloSegScore{2.438}{(2.053--2.757)}{4.55pt}{4.82pt}{} & \HoloSegScore{3.600}{(2.501--3.757)}{4.55pt}{4.82pt}{} & \HoloSegScore{1.821}{(1.519--2.153)}{4.55pt}{4.82pt}{} & \HoloSegScore{1.130}{(0.8656--1.469)}{4.55pt}{4.82pt}{} \\
\cline{3-11}
 &  &  & \HoloSegMetric{Dice} &  & \HoloSegScore{0.03684}{(0.01618--0.06324)}{4.20pt}{4.48pt}{} & \HoloSegScore{0.7605}{(0.7235--0.7948)}{4.55pt}{4.82pt}{} & \HoloSegScore{0.7313}{(0.6976--0.7669)}{4.55pt}{4.82pt}{} & \HoloSegScore{0.7467}{(0.7234--0.7789)}{4.55pt}{4.82pt}{} & \HoloSegScore{0.7547}{(0.7262--0.7824)}{4.55pt}{4.82pt}{} & \HoloSegScore{0.8195}{(0.8018--0.8374)}{4.55pt}{4.82pt}{} \\*
\softcline{4-4}\softcline{6-11}
 &  & \HoloSegSpan{\makecell[c]{right lens}}{2.04cm}{0.32cm} & \HoloSegMetric{HD95} & \raisebox{0.32cm}[0pt][0pt]{\HoloSegUnsupported} & \HoloSegScore{63.51}{(44.47--83.19)}{4.55pt}{4.82pt}{} & \HoloSegScore{1.711}{(1.411--2.037)}{4.55pt}{4.82pt}{} & \HoloSegScore{2.128}{(1.771--2.488)}{4.55pt}{4.82pt}{} & \HoloSegScore{2.483}{(1.624--2.490)}{4.55pt}{4.82pt}{} & \HoloSegScore{2.071}{(1.647--2.476)}{4.55pt}{4.82pt}{} & \HoloSegScore{8.196}{(1.322--15.33)}{4.55pt}{4.82pt}{} \\
\cline{3-11}
 &  &  & \HoloSegMetric{Dice} &  & \HoloSegScore{0.0009220}{(0.0000--0.002766)}{4.20pt}{4.48pt}{} & \HoloSegScore{0.7755}{(0.7482--0.8006)}{4.55pt}{4.82pt}{} & \HoloSegScore{0.7598}{(0.7413--0.7773)}{4.55pt}{4.82pt}{} & \HoloSegScore{0.7495}{(0.7327--0.7567)}{4.55pt}{4.82pt}{} & \HoloSegScore{0.7995}{(0.7769--0.8188)}{4.55pt}{4.82pt}{} & \HoloSegScore{0.8215}{(0.8018--0.8385)}{4.55pt}{4.82pt}{} \\*
\softcline{4-4}\softcline{6-11}
 &  & \HoloSegSpan{\makecell[c]{left optic\\[-0.10ex]nerve}}{2.04cm}{0.32cm} & \HoloSegMetric{HD95} & \raisebox{0.32cm}[0pt][0pt]{\HoloSegUnsupported} & \HoloSegScore{103.7}{(83.60--121.3)}{4.55pt}{4.82pt}{} & \HoloSegScore{2.035}{(1.680--2.424)}{4.55pt}{4.82pt}{} & \HoloSegScore{2.774}{(2.420--3.156)}{4.55pt}{4.82pt}{} & \HoloSegScore{3.546}{(1.610--3.894)}{4.55pt}{4.82pt}{} & \HoloSegScore{22.74}{(14.96--30.25)}{4.55pt}{4.82pt}{} & \HoloSegScore{17.84}{(2.496--47.29)}{4.55pt}{4.82pt}{} \\
\cline{3-11}
 &  &  & \HoloSegMetric{Dice} &  & \HoloSegScore{0.01034}{(0.001394--0.02128)}{3.85pt}{4.12pt}{} & \HoloSegScore{0.8024}{(0.7733--0.8275)}{4.55pt}{4.82pt}{} & \HoloSegScore{0.7717}{(0.7498--0.7938)}{4.55pt}{4.82pt}{} & \HoloSegScore{0.7902}{(0.7797--0.8266)}{4.55pt}{4.82pt}{} & \HoloSegScore{0.8175}{(0.7963--0.8375)}{4.55pt}{4.82pt}{} & \HoloSegScore{0.8423}{(0.8283--0.8563)}{4.55pt}{4.82pt}{} \\*
\softcline{4-4}\softcline{6-11}
 &  & \HoloSegSpan{\makecell[c]{right optic\\[-0.10ex]nerve}}{2.04cm}{0.32cm} & \HoloSegMetric{HD95} & \raisebox{0.32cm}[0pt][0pt]{\HoloSegUnsupported} & \HoloSegScore{83.99}{(62.35--103.5)}{4.55pt}{4.82pt}{} & \HoloSegScore{2.061}{(1.511--2.678)}{4.55pt}{4.82pt}{} & \HoloSegScore{3.075}{(2.714--3.488)}{4.55pt}{4.82pt}{} & \HoloSegScore{3.725}{(3.323--4.670)}{4.55pt}{4.82pt}{} & \HoloSegScore{2.234}{(1.844--2.579)}{4.55pt}{4.82pt}{} & \HoloSegScore{17.63}{(1.674--49.11)}{4.55pt}{4.82pt}{} \\
\cline{3-11}
 &  &  & \HoloSegMetric{Dice} &  & \HoloSegScore{0.0000}{(0.0000--0.0000)}{4.55pt}{4.82pt}{} & \HoloSegScore{0.8427}{(0.7932--0.8794)}{4.55pt}{4.82pt}{} & \HoloSegScore{0.6232}{(0.5797--0.6611)}{4.55pt}{4.82pt}{} & \HoloSegScore{0.8193}{(0.8128--0.8275)}{4.55pt}{4.82pt}{} & \HoloSegScore{0.8025}{(0.7626--0.8323)}{4.55pt}{4.82pt}{} & \HoloSegScore{0.8228}{(0.7924--0.8507)}{4.55pt}{4.82pt}{} \\*
\softcline{4-4}\softcline{6-11}
 &  & \HoloSegSpan{\makecell[c]{left middle\\[-0.10ex]ear}}{2.04cm}{0.32cm} & \HoloSegMetric{HD95} & \raisebox{0.32cm}[0pt][0pt]{\HoloSegUnsupported} & \HoloSegScore{101.4}{(99.47--103.4)}{4.55pt}{4.82pt}{} & \HoloSegScore{1.573}{(1.104--2.223)}{4.55pt}{4.82pt}{} & \HoloSegScore{8.420}{(7.658--9.161)}{4.55pt}{4.82pt}{} & \HoloSegScore{5.287}{(5.028--6.574)}{4.55pt}{4.82pt}{} & \HoloSegScore{4.505}{(2.365--8.399)}{4.55pt}{4.82pt}{} & \HoloSegScore{2.265}{(1.918--2.628)}{4.55pt}{4.82pt}{} \\
\cline{3-11}
 &  &  & \HoloSegMetric{Dice} &  & \HoloSegScore{0.0000}{(0.0000--0.0000)}{4.55pt}{4.82pt}{} & \HoloSegScore{0.8382}{(0.7939--0.8684)}{4.55pt}{4.82pt}{} & \HoloSegScore{0.5335}{(0.4938--0.5701)}{4.55pt}{4.82pt}{} & \HoloSegScore{0.8198}{(0.8179--0.8260)}{4.55pt}{4.82pt}{} & \HoloSegScore{0.7367}{(0.6920--0.7738)}{4.55pt}{4.82pt}{} & \HoloSegScore{0.8236}{(0.7975--0.8486)}{4.55pt}{4.82pt}{} \\*
\softcline{4-4}\softcline{6-11}
 &  & \HoloSegSpan{\makecell[c]{right middle\\[-0.10ex]ear}}{2.04cm}{0.32cm} & \HoloSegMetric{HD95} & \raisebox{0.32cm}[0pt][0pt]{\HoloSegUnsupported} & \HoloSegScore{100.8}{(96.03--104.6)}{4.55pt}{4.82pt}{} & \HoloSegScore{1.765}{(1.343--2.267)}{4.55pt}{4.82pt}{} & \HoloSegScore{10.75}{(10.20--11.29)}{4.55pt}{4.82pt}{} & \HoloSegScore{2.284}{(2.064--5.129)}{4.55pt}{4.82pt}{} & \HoloSegScore{2.827}{(2.534--3.217)}{4.55pt}{4.82pt}{} & \HoloSegScore{2.323}{(1.999--2.658)}{4.55pt}{4.82pt}{} \\
\cline{3-11}
 &  &  & \HoloSegMetric{Dice} &  & \HoloSegScore{0.0000}{(0.0000--0.0000)}{4.55pt}{4.82pt}{} & \HoloSegScore{0.8296}{(0.8025--0.8549)}{4.55pt}{4.82pt}{} & \HoloSegScore{0.7951}{(0.7654--0.8206)}{4.55pt}{4.82pt}{} & \HoloSegScore{0.8013}{(0.7912--0.8242)}{4.55pt}{4.82pt}{} & \HoloSegScore{0.7869}{(0.7336--0.8285)}{4.55pt}{4.82pt}{} & \HoloSegScore{0.8231}{(0.7931--0.8504)}{4.55pt}{4.82pt}{} \\*
\softcline{4-4}\softcline{6-11}
 &  & \HoloSegSpan{\makecell[c]{left\\[-0.10ex]internal\\[-0.10ex]auditory\\[-0.10ex]canal}}{2.04cm}{0.32cm} & \HoloSegMetric{HD95} & \raisebox{0.32cm}[0pt][0pt]{\HoloSegUnsupported} & \HoloSegScore{97.83}{(92.50--102.6)}{4.55pt}{4.82pt}{} & \HoloSegScore{1.024}{(0.7869--1.283)}{4.55pt}{4.82pt}{} & \HoloSegScore{1.396}{(1.084--1.735)}{4.55pt}{4.82pt}{} & \HoloSegScore{3.227}{(1.484--4.340)}{4.55pt}{4.82pt}{} & \HoloSegScore{7.363}{(1.711--14.49)}{4.55pt}{4.82pt}{} & \HoloSegScore{1.286}{(0.9647--1.630)}{4.55pt}{4.82pt}{} \\
\cline{3-11}
 &  &  & \HoloSegMetric{Dice} &  & \HoloSegScore{0.0000}{(0.0000--0.0000)}{4.55pt}{4.82pt}{} & \HoloSegScore{0.8229}{(0.7985--0.8445)}{4.55pt}{4.82pt}{} & \HoloSegScore{0.8197}{(0.7914--0.8453)}{4.55pt}{4.82pt}{} & \HoloSegScore{0.7710}{(0.7673--0.7793)}{4.55pt}{4.82pt}{} & \HoloSegScore{0.8139}{(0.7904--0.8332)}{4.55pt}{4.82pt}{} & \HoloSegScore{0.8406}{(0.8083--0.8680)}{4.55pt}{4.82pt}{} \\*
\softcline{4-4}\softcline{6-11}
 &  & \HoloSegSpan{\makecell[c]{right\\[-0.10ex]internal\\[-0.10ex]auditory\\[-0.10ex]canal}}{2.04cm}{0.32cm} & \HoloSegMetric{HD95} & \raisebox{0.32cm}[0pt][0pt]{\HoloSegUnsupported} & \HoloSegScore{105.9}{(100.4--111.2)}{4.55pt}{4.82pt}{} & \HoloSegScore{1.096}{(0.8031--1.463)}{4.55pt}{4.82pt}{} & \HoloSegScore{1.524}{(1.118--1.918)}{4.55pt}{4.82pt}{} & \HoloSegScore{2.125}{(1.995--3.533)}{4.55pt}{4.82pt}{} & \HoloSegScore{1.281}{(1.021--1.568)}{4.55pt}{4.82pt}{} & \HoloSegScore{1.055}{(0.7603--1.383)}{4.55pt}{4.82pt}{} \\
\hline
\pagebreak[4]
 &  &  & \HoloSegMetric{Dice} &  & \HoloSegScore{0.0000}{(0.0000--0.0000)}{4.55pt}{4.82pt}{} & \HoloSegScore{0.7740}{(0.7468--0.8000)}{4.55pt}{4.82pt}{} & \HoloSegScore{0.7242}{(0.6853--0.7621)}{4.55pt}{4.82pt}{} & \HoloSegScore{0.7736}{(0.7720--0.7801)}{4.55pt}{4.82pt}{} & \HoloSegScore{0.7040}{(0.6653--0.7399)}{4.55pt}{4.82pt}{} & \HoloSegScore{0.7873}{(0.7634--0.8118)}{4.55pt}{4.82pt}{} \\*
\softcline{4-4}\softcline{6-11}
 &  & \HoloSegSpan{\makecell[c]{left\\[-0.10ex]tympanic\\[-0.10ex]cavity}}{2.04cm}{0.32cm} & \HoloSegMetric{HD95} & \raisebox{0.32cm}[0pt][0pt]{\HoloSegUnsupported} & \HoloSegScore{99.75}{(95.55--103.6)}{4.55pt}{4.82pt}{} & \HoloSegScore{2.007}{(1.702--2.327)}{4.55pt}{4.82pt}{} & \HoloSegScore{2.356}{(2.025--2.652)}{4.55pt}{4.82pt}{} & \HoloSegScore{6.398}{(6.051--7.854)}{4.55pt}{4.82pt}{} & \HoloSegScore{3.161}{(2.389--4.442)}{4.55pt}{4.82pt}{} & \HoloSegScore{1.726}{(1.503--2.000)}{4.55pt}{4.82pt}{} \\
\cline{3-11}
 &  &  & \HoloSegMetric{Dice} &  & \HoloSegScore{0.0000}{(0.0000--0.0000)}{4.55pt}{4.82pt}{} & \HoloSegScore{0.7953}{(0.7622--0.8243)}{4.55pt}{4.82pt}{} & \HoloSegScore{0.7564}{(0.7189--0.7892)}{4.55pt}{4.82pt}{} & \HoloSegScore{0.7323}{(0.6928--0.7506)}{4.55pt}{4.82pt}{} & \HoloSegScore{0.7465}{(0.7035--0.7938)}{4.55pt}{4.82pt}{} & \HoloSegScore{0.7339}{(0.6984--0.7718)}{4.55pt}{4.82pt}{} \\*
\softcline{4-4}\softcline{6-11}
 &  & \HoloSegSpan{\makecell[c]{right\\[-0.10ex]tympanic\\[-0.10ex]cavity}}{2.04cm}{0.32cm} & \HoloSegMetric{HD95} & \raisebox{0.32cm}[0pt][0pt]{\HoloSegUnsupported} & \HoloSegScore{98.81}{(93.21--103.7)}{4.55pt}{4.82pt}{} & \HoloSegScore{1.868}{(1.547--2.207)}{4.55pt}{4.82pt}{} & \HoloSegScore{2.309}{(2.003--2.619)}{4.55pt}{4.82pt}{} & \HoloSegScore{3.297}{(2.943--4.379)}{4.55pt}{4.82pt}{} & \HoloSegScore{1.946}{(1.631--2.276)}{4.55pt}{4.82pt}{} & \HoloSegScore{1.866}{(1.600--2.128)}{4.55pt}{4.82pt}{} \\
\cline{3-11}
 &  &  & \HoloSegMetric{Dice} &  & \HoloSegScore{0.0000}{(0.0000--0.0000)}{4.55pt}{4.82pt}{} & \HoloSegScore{0.8257}{(0.8007--0.8481)}{4.55pt}{4.82pt}{} & \HoloSegScore{0.7883}{(0.7602--0.8140)}{4.55pt}{4.82pt}{} & \HoloSegScore{0.8093}{(0.8042--0.8258)}{4.55pt}{4.82pt}{} & \HoloSegScore{0.7808}{(0.7615--0.8007)}{4.55pt}{4.82pt}{} & \HoloSegScore{0.7726}{(0.7391--0.7982)}{4.55pt}{4.82pt}{} \\*
\softcline{4-4}\softcline{6-11}
 &  & \HoloSegSpan{\makecell[c]{left\\[-0.10ex]vestibule\\[-0.10ex]semicircular\\[-0.10ex]canal}}{2.04cm}{0.32cm} & \HoloSegMetric{HD95} & \raisebox{0.32cm}[0pt][0pt]{\HoloSegUnsupported} & \HoloSegScore{90.92}{(87.15--94.57)}{4.55pt}{4.82pt}{} & \HoloSegScore{1.197}{(0.8641--1.579)}{4.55pt}{4.82pt}{} & \HoloSegScore{1.900}{(1.559--2.283)}{4.55pt}{4.82pt}{} & \HoloSegScore{2.205}{(1.846--3.174)}{4.55pt}{4.82pt}{} & \HoloSegScore{16.76}{(5.152--28.92)}{4.55pt}{4.82pt}{} & \HoloSegScore{1.383}{(1.098--1.694)}{4.55pt}{4.82pt}{} \\
\cline{3-11}
 &  &  & \HoloSegMetric{Dice} &  & \HoloSegScore{0.0000}{(0.0000--0.0000)}{4.55pt}{4.82pt}{} & \HoloSegScore{0.8026}{(0.7791--0.8234)}{4.55pt}{4.82pt}{} & \HoloSegScore{0.7946}{(0.7728--0.8157)}{4.55pt}{4.82pt}{} & \HoloSegScore{0.7967}{(0.7597--0.8263)}{4.55pt}{4.82pt}{} & \HoloSegScore{0.7144}{(0.6839--0.7419)}{4.55pt}{4.82pt}{} & \HoloSegScore{0.7915}{(0.7500--0.8258)}{4.55pt}{4.82pt}{} \\*
\softcline{4-4}\softcline{6-11}
 &  & \HoloSegSpan{\makecell[c]{right\\[-0.10ex]vestibule\\[-0.10ex]semicircular\\[-0.10ex]canal}}{2.04cm}{0.32cm} & \HoloSegMetric{HD95} & \raisebox{0.32cm}[0pt][0pt]{\HoloSegUnsupported} & \HoloSegScore{96.76}{(91.51--102.7)}{4.55pt}{4.82pt}{} & \HoloSegScore{1.160}{(0.8867--1.475)}{4.55pt}{4.82pt}{} & \HoloSegScore{1.540}{(1.208--1.941)}{4.55pt}{4.82pt}{} & \HoloSegScore{1.787}{(1.457--2.393)}{4.55pt}{4.82pt}{} & \HoloSegScore{2.581}{(2.272--2.907)}{4.55pt}{4.82pt}{} & \HoloSegScore{1.494}{(1.148--1.856)}{4.55pt}{4.82pt}{} \\
\cline{3-11}
 &  &  & \HoloSegMetric{Dice} &  & \HoloSegScore{0.0000}{(0.0000--0.0000)}{4.55pt}{4.82pt}{} & \HoloSegScore{0.8313}{(0.8083--0.8536)}{4.55pt}{4.82pt}{} & \HoloSegScore{0.8022}{(0.7797--0.8240)}{4.55pt}{4.82pt}{} & \HoloSegScore{0.7953}{(0.7670--0.8135)}{4.55pt}{4.82pt}{} & \HoloSegScore{0.8057}{(0.7686--0.8340)}{4.55pt}{4.82pt}{} & \HoloSegScore{0.8193}{(0.7936--0.8420)}{4.55pt}{4.82pt}{} \\*
\softcline{4-4}\softcline{6-11}
 &  & \HoloSegSpan{\makecell[c]{left cochlea}}{2.04cm}{0.32cm} & \HoloSegMetric{HD95} & \raisebox{0.32cm}[0pt][0pt]{\HoloSegUnsupported} & \HoloSegScore{106.9}{(88.20--135.2)}{4.55pt}{4.82pt}{} & \HoloSegScore{1.064}{(0.7804--1.412)}{4.55pt}{4.82pt}{} & \HoloSegScore{1.402}{(1.063--1.799)}{4.55pt}{4.82pt}{} & \HoloSegScore{1.752}{(1.541--2.636)}{4.55pt}{4.82pt}{} & \HoloSegScore{1.630}{(1.196--2.037)}{4.55pt}{4.82pt}{} & \HoloSegScore{0.9620}{(0.7490--1.236)}{4.55pt}{4.82pt}{} \\
\cline{3-11}
 &  &  & \HoloSegMetric{Dice} &  & \HoloSegScore{0.0000}{(0.0000--0.0000)}{4.55pt}{4.82pt}{} & \HoloSegScore{0.8188}{(0.7821--0.8483)}{4.55pt}{4.82pt}{} & \HoloSegScore{0.8190}{(0.7921--0.8410)}{4.55pt}{4.82pt}{} & \HoloSegScore{0.8051}{(0.8026--0.8075)}{4.55pt}{4.82pt}{} & \HoloSegScore{0.8136}{(0.7916--0.8350)}{4.55pt}{4.82pt}{} & \HoloSegScore{0.8175}{(0.7987--0.8358)}{4.55pt}{4.82pt}{} \\*
\softcline{4-4}\softcline{6-11}
 &  & \HoloSegSpan{\makecell[c]{right\\[-0.10ex]cochlea}}{2.04cm}{0.32cm} & \HoloSegMetric{HD95} & \raisebox{0.32cm}[0pt][0pt]{\HoloSegUnsupported} & \HoloSegScore{101.0}{(87.69--113.1)}{4.55pt}{4.82pt}{} & \HoloSegScore{1.060}{(0.8283--1.359)}{4.55pt}{4.82pt}{} & \HoloSegScore{1.140}{(0.8660--1.471)}{4.55pt}{4.82pt}{} & \HoloSegScore{2.035}{(1.469--3.151)}{4.55pt}{4.82pt}{} & \HoloSegScore{1.758}{(1.316--2.173)}{4.55pt}{4.82pt}{} & \HoloSegScore{1.161}{(0.8825--1.487)}{4.55pt}{4.82pt}{} \\
\cline{3-11}
 &  &  & \HoloSegMetric{Dice} &  & \HoloSegScore{0.0000}{(0.0000--0.0000)}{4.55pt}{4.82pt}{} & \HoloSegScore{0.7966}{(0.7725--0.8175)}{4.55pt}{4.82pt}{} & \HoloSegScore{0.7415}{(0.7181--0.7709)}{4.55pt}{4.82pt}{} & \HoloSegScore{0.7215}{(0.6943--0.7564)}{4.55pt}{4.82pt}{} & \HoloSegScore{0.7354}{(0.7145--0.7575)}{4.55pt}{4.82pt}{} & \HoloSegScore{0.7144}{(0.6772--0.7521)}{4.55pt}{4.82pt}{} \\*
\softcline{4-4}\softcline{6-11}
 &  & \HoloSegSpan{\makecell[c]{left\\[-0.10ex]eustachian\\[-0.10ex]tube bone}}{2.04cm}{0.32cm} & \HoloSegMetric{HD95} & \raisebox{0.32cm}[0pt][0pt]{\HoloSegUnsupported} & \HoloSegScore{78.80}{(77.06--80.60)}{4.55pt}{4.82pt}{} & \HoloSegScore{1.523}{(1.169--1.907)}{4.55pt}{4.82pt}{} & \HoloSegScore{2.024}{(1.673--2.383)}{4.55pt}{4.82pt}{} & \HoloSegScore{2.978}{(2.408--3.375)}{4.55pt}{4.82pt}{} & \HoloSegScore{1.962}{(1.658--2.243)}{4.55pt}{4.82pt}{} & \HoloSegScore{1.778}{(1.515--2.072)}{4.55pt}{4.82pt}{} \\
\cline{3-11}
 &  &  & \HoloSegMetric{Dice} &  & \HoloSegScore{0.0000}{(0.0000--0.0000)}{4.55pt}{4.82pt}{} & \HoloSegScore{0.7901}{(0.7505--0.8217)}{4.55pt}{4.82pt}{} & \HoloSegScore{0.7267}{(0.6954--0.7560)}{4.55pt}{4.82pt}{} & \HoloSegScore{0.7725}{(0.7643--0.7782)}{4.55pt}{4.82pt}{} & \HoloSegScore{0.7646}{(0.7303--0.7954)}{4.55pt}{4.82pt}{} & \HoloSegScore{0.7876}{(0.7619--0.8111)}{4.55pt}{4.82pt}{} \\*
\softcline{4-4}\softcline{6-11}
 &  & \HoloSegSpan{\makecell[c]{right\\[-0.10ex]eustachian\\[-0.10ex]tube bone}}{2.04cm}{0.32cm} & \HoloSegMetric{HD95} & \raisebox{0.32cm}[0pt][0pt]{\HoloSegUnsupported} & \HoloSegScore{80.10}{(76.35--84.03)}{4.55pt}{4.82pt}{} & \HoloSegScore{1.430}{(1.094--1.782)}{4.55pt}{4.82pt}{} & \HoloSegScore{2.147}{(1.850--2.485)}{4.55pt}{4.82pt}{} & \HoloSegScore{2.605}{(2.398--3.855)}{4.55pt}{4.82pt}{} & \HoloSegScore{1.632}{(1.356--1.924)}{4.55pt}{4.82pt}{} & \HoloSegScore{1.653}{(1.322--1.975)}{4.55pt}{4.82pt}{} \\
\cline{3-11}
 &  &  & \HoloSegMetric{Dice} &  & \HoloSegScore{0.0000}{(0.0000--0.0000)}{4.55pt}{4.82pt}{} & \HoloSegScore{0.7516}{(0.7059--0.7943)}{4.55pt}{4.82pt}{} & \HoloSegScore{0.6432}{(0.5977--0.6878)}{4.55pt}{4.82pt}{} & \HoloSegScore{0.6317}{(0.5931--0.6589)}{4.55pt}{4.82pt}{} & \HoloSegScore{0.6987}{(0.6580--0.7374)}{4.55pt}{4.82pt}{} & \HoloSegScore{0.7089}{(0.6176--0.7863)}{4.55pt}{4.82pt}{} \\*
\softcline{4-4}\softcline{6-11}
 &  & \HoloSegSpan{\makecell[c]{pituitary\\[-0.10ex]gland}}{2.04cm}{0.32cm} & \HoloSegMetric{HD95} & \raisebox{0.32cm}[0pt][0pt]{\HoloSegUnsupported} & \HoloSegScore{141.6}{(136.4--147.2)}{4.55pt}{4.82pt}{} & \HoloSegScore{1.840}{(1.403--2.292)}{4.55pt}{4.82pt}{} & \HoloSegScore{2.848}{(2.533--3.192)}{4.55pt}{4.82pt}{} & \HoloSegScore{2.909}{(1.857--3.028)}{4.55pt}{4.82pt}{} & \HoloSegScore{2.621}{(2.317--2.886)}{4.55pt}{4.82pt}{} & \HoloSegScore{2.272}{(1.899--2.643)}{4.55pt}{4.82pt}{} \\
\cline{3-11}
 &  &  & \HoloSegMetric{Dice} &  & \HoloSegScore{0.5814}{(0.5512--0.6106)}{4.55pt}{4.82pt}{} & \HoloSegScore{0.9180}{(0.9076--0.9271)}{4.55pt}{4.82pt}{} & \HoloSegScore{0.8707}{(0.8613--0.8797)}{4.55pt}{4.82pt}{} & \HoloSegScore{0.9082}{(0.9031--0.9202)}{4.55pt}{4.82pt}{} & \HoloSegScore{0.9003}{(0.8910--0.9075)}{4.55pt}{4.82pt}{} & \HoloSegScore{0.9165}{(0.9106--0.9221)}{4.55pt}{4.82pt}{} \\*
\softcline{4-4}\softcline{6-11}
\HoloSegSpan{\makecell[c]{\textbf{Internal}}}{1.20cm}{0.32cm} & \HoloSegSpan{\makecell[c]{SegRap2023-\\[-0.10ex]Task1}}{1.86cm}{0.32cm} & \HoloSegSpan{\makecell[c]{oral cavity}}{2.04cm}{0.32cm} & \HoloSegMetric{HD95} & \raisebox{0.32cm}[0pt][0pt]{\HoloSegUnsupported} & \HoloSegScore{17.08}{(15.36--19.15)}{4.55pt}{4.82pt}{} & \HoloSegScore{3.781}{(3.430--4.247)}{4.55pt}{4.82pt}{} & \HoloSegScore{6.309}{(5.498--7.258)}{4.55pt}{4.82pt}{} & \HoloSegScore{4.176}{(3.530--4.416)}{4.55pt}{4.82pt}{} & \HoloSegScore{14.20}{(3.987--34.50)}{4.55pt}{4.82pt}{} & \HoloSegScore{4.723}{(3.831--5.858)}{4.55pt}{4.82pt}{} \\
\cline{3-11}
 &  &  & \HoloSegMetric{Dice} &  & \HoloSegScore{0.4324}{(0.4092--0.4519)}{4.55pt}{4.82pt}{} & \HoloSegScore{0.9357}{(0.9299--0.9404)}{4.55pt}{4.82pt}{} & \HoloSegScore{0.9187}{(0.9141--0.9228)}{4.55pt}{4.82pt}{} & \HoloSegScore{0.9286}{(0.9260--0.9372)}{4.55pt}{4.82pt}{} & \HoloSegScore{0.9274}{(0.9212--0.9320)}{4.55pt}{4.82pt}{} & \HoloSegScore{0.9258}{(0.9205--0.9304)}{4.55pt}{4.82pt}{} \\*
\softcline{4-4}\softcline{6-11}
 &  & \HoloSegSpan{\makecell[c]{left\\[-0.10ex]mandible}}{2.04cm}{0.32cm} & \HoloSegMetric{HD95} & \raisebox{0.32cm}[0pt][0pt]{\HoloSegUnsupported} & \HoloSegScore{74.77}{(71.26--78.22)}{4.55pt}{4.82pt}{} & \HoloSegScore{1.788}{(1.574--2.032)}{4.55pt}{4.82pt}{} & \HoloSegScore{2.412}{(2.147--2.638)}{4.55pt}{4.82pt}{} & \HoloSegScore{2.663}{(1.826--3.067)}{4.55pt}{4.82pt}{} & \HoloSegScore{7.625}{(1.731--19.24)}{4.55pt}{4.82pt}{} & \HoloSegScore{6.087}{(2.503--12.97)}{4.55pt}{4.82pt}{} \\
\cline{3-11}
 &  &  & \HoloSegMetric{Dice} &  & \HoloSegScore{0.4186}{(0.4033--0.4344)}{4.55pt}{4.82pt}{} & \HoloSegScore{0.9388}{(0.9327--0.9435)}{4.55pt}{4.82pt}{} & \HoloSegScore{0.9198}{(0.9158--0.9240)}{4.55pt}{4.82pt}{} & \HoloSegScore{0.9191}{(0.8919--0.9322)}{4.55pt}{4.82pt}{} & \HoloSegScore{0.9177}{(0.9108--0.9235)}{4.55pt}{4.82pt}{} & \HoloSegScore{0.9352}{(0.9298--0.9396)}{4.55pt}{4.82pt}{} \\*
\softcline{4-4}\softcline{6-11}
 &  & \HoloSegSpan{\makecell[c]{right\\[-0.10ex]mandible}}{2.04cm}{0.32cm} & \HoloSegMetric{HD95} & \raisebox{0.32cm}[0pt][0pt]{\HoloSegUnsupported} & \HoloSegScore{78.61}{(76.11--81.26)}{4.55pt}{4.82pt}{} & \HoloSegScore{1.715}{(1.490--1.952)}{4.55pt}{4.82pt}{} & \HoloSegScore{2.190}{(1.952--2.416)}{4.55pt}{4.82pt}{} & \HoloSegScore{2.079}{(1.732--4.093)}{4.55pt}{4.82pt}{} & \HoloSegScore{21.63}{(2.594--51.25)}{4.55pt}{4.82pt}{} & \HoloSegScore{1.611}{(1.372--1.865)}{4.55pt}{4.82pt}{} \\
\cline{3-11}
 &  &  & \HoloSegMetric{Dice} &  & \HoloSegScore{0.2330}{(0.1479--0.3233)}{4.55pt}{4.82pt}{} & \HoloSegScore{0.8765}{(0.8527--0.8965)}{4.55pt}{4.82pt}{} & \HoloSegScore{0.8372}{(0.8232--0.8495)}{4.55pt}{4.82pt}{} & \HoloSegScore{0.8220}{(0.8161--0.8279)}{4.55pt}{4.82pt}{} & \HoloSegScore{0.8415}{(0.8276--0.8571)}{4.55pt}{4.82pt}{} & \HoloSegScore{0.8844}{(0.8663--0.9000)}{4.55pt}{4.82pt}{} \\*
\softcline{4-4}\softcline{6-11}
 &  & \HoloSegSpan{\makecell[c]{left\\[-0.10ex]submandibular\\[-0.10ex]gland}}{2.04cm}{0.32cm} & \HoloSegMetric{HD95} & \raisebox{0.32cm}[0pt][0pt]{\HoloSegUnsupported} & \HoloSegScore{53.27}{(40.93--65.07)}{4.55pt}{4.82pt}{} & \HoloSegScore{2.481}{(2.063--2.980)}{4.55pt}{4.82pt}{} & \HoloSegScore{2.981}{(2.687--3.286)}{4.55pt}{4.82pt}{} & \HoloSegScore{5.078}{(4.921--5.476)}{4.55pt}{4.82pt}{} & \HoloSegScore{3.088}{(2.811--3.386)}{4.55pt}{4.82pt}{} & \HoloSegScore{2.429}{(1.884--3.248)}{4.55pt}{4.82pt}{} \\
\cline{3-11}
 &  &  & \HoloSegMetric{Dice} &  & \HoloSegScore{0.2871}{(0.2123--0.3590)}{4.55pt}{4.82pt}{} & \HoloSegScore{0.8723}{(0.8514--0.8904)}{4.55pt}{4.82pt}{} & \HoloSegScore{0.8442}{(0.8282--0.8602)}{4.55pt}{4.82pt}{} & \HoloSegScore{0.8638}{(0.8498--0.8840)}{4.55pt}{4.82pt}{} & \HoloSegScore{0.8490}{(0.8302--0.8662)}{4.55pt}{4.82pt}{} & \HoloSegScore{0.8767}{(0.8642--0.8888)}{4.55pt}{4.82pt}{} \\*
\softcline{4-4}\softcline{6-11}
 &  & \HoloSegSpan{\makecell[c]{right\\[-0.10ex]submandibular\\[-0.10ex]gland}}{2.04cm}{0.32cm} & \HoloSegMetric{HD95} & \raisebox{0.32cm}[0pt][0pt]{\HoloSegUnsupported} & \HoloSegScore{45.84}{(34.18--57.92)}{4.55pt}{4.82pt}{} & \HoloSegScore{2.492}{(2.103--2.948)}{4.55pt}{4.82pt}{} & \HoloSegScore{2.793}{(2.545--3.122)}{4.55pt}{4.82pt}{} & \HoloSegScore{3.005}{(1.478--3.328)}{4.55pt}{4.82pt}{} & \HoloSegScore{14.93}{(2.636--39.11)}{4.55pt}{4.82pt}{} & \HoloSegScore{2.266}{(1.964--2.507)}{4.55pt}{4.82pt}{} \\
\cline{3-11}
 &  &  & \HoloSegMetric{Dice} &  & \HoloSegScore{0.4154}{(0.3494--0.4743)}{4.55pt}{4.82pt}{} & \HoloSegScore{0.9170}{(0.9113--0.9228)}{4.55pt}{4.82pt}{} & \HoloSegScore{0.8788}{(0.8675--0.8887)}{4.55pt}{4.82pt}{} & \HoloSegScore{0.8688}{(0.8658--0.8738)}{4.55pt}{4.82pt}{} & \HoloSegScore{0.8954}{(0.8895--0.9007)}{4.55pt}{4.82pt}{} & \HoloSegScore{0.9085}{(0.9022--0.9139)}{4.55pt}{4.82pt}{} \\*
\softcline{4-4}\softcline{6-11}
 &  & \HoloSegSpan{\makecell[c]{left parotid\\[-0.10ex]gland}}{2.04cm}{0.32cm} & \HoloSegMetric{HD95} & \raisebox{0.32cm}[0pt][0pt]{\HoloSegUnsupported} & \HoloSegScore{34.94}{(22.96--47.82)}{4.55pt}{4.82pt}{} & \HoloSegScore{2.396}{(2.153--2.634)}{4.55pt}{4.82pt}{} & \HoloSegScore{3.442}{(3.034--3.997)}{4.55pt}{4.82pt}{} & \HoloSegScore{3.517}{(2.488--3.691)}{4.55pt}{4.82pt}{} & \HoloSegScore{3.325}{(3.057--3.647)}{4.55pt}{4.82pt}{} & \HoloSegScore{2.725}{(2.423--3.059)}{4.55pt}{4.82pt}{} \\
\cline{3-11}
 &  &  & \HoloSegMetric{Dice} &  & \HoloSegScore{0.4737}{(0.3963--0.5456)}{4.55pt}{4.82pt}{} & \HoloSegScore{0.9050}{(0.8918--0.9149)}{4.55pt}{4.82pt}{} & \HoloSegScore{0.8764}{(0.8681--0.8847)}{4.55pt}{4.82pt}{} & \HoloSegScore{0.8998}{(0.8946--0.9068)}{4.55pt}{4.82pt}{} & \HoloSegScore{0.8740}{(0.8636--0.8838)}{4.55pt}{4.82pt}{} & \HoloSegScore{0.8916}{(0.8853--0.8987)}{4.55pt}{4.82pt}{} \\*
\softcline{4-4}\softcline{6-11}
 &  & \HoloSegSpan{\makecell[c]{right\\[-0.10ex]parotid\\[-0.10ex]gland}}{2.04cm}{0.32cm} & \HoloSegMetric{HD95} & \raisebox{0.32cm}[0pt][0pt]{\HoloSegUnsupported} & \HoloSegScore{29.54}{(17.23--42.58)}{4.55pt}{4.82pt}{} & \HoloSegScore{2.881}{(2.608--3.137)}{4.55pt}{4.82pt}{} & \HoloSegScore{4.190}{(3.613--4.811)}{4.55pt}{4.82pt}{} & \HoloSegScore{4.127}{(3.867--5.500)}{4.55pt}{4.82pt}{} & \HoloSegScore{5.468}{(4.635--6.460)}{4.55pt}{4.82pt}{} & \HoloSegScore{4.190}{(3.343--5.439)}{4.55pt}{4.82pt}{} \\
\cline{3-11}
 &  &  & \HoloSegMetric{Dice} &  & \HoloSegScore{0.0000}{(0.0000--0.0000)}{4.55pt}{4.82pt}{} & \HoloSegScore{0.9001}{(0.8912--0.9084)}{4.55pt}{4.82pt}{} & \HoloSegScore{0.8625}{(0.8505--0.8737)}{4.55pt}{4.82pt}{} & \HoloSegScore{0.8583}{(0.8519--0.8801)}{4.55pt}{4.82pt}{} & \HoloSegScore{0.8804}{(0.8674--0.8926)}{4.55pt}{4.82pt}{} & \HoloSegScore{0.8896}{(0.8799--0.8993)}{4.55pt}{4.82pt}{} \\*
\softcline{4-4}\softcline{6-11}
 &  & \HoloSegSpan{\makecell[c]{left mastoid\\[-0.10ex]process}}{2.04cm}{0.32cm} & \HoloSegMetric{HD95} & \raisebox{0.32cm}[0pt][0pt]{\HoloSegUnsupported} & \HoloSegScore{88.12}{(78.53--103.5)}{4.55pt}{4.82pt}{} & \HoloSegScore{2.132}{(1.899--2.388)}{4.55pt}{4.82pt}{} & \HoloSegScore{3.638}{(3.181--4.263)}{4.55pt}{4.82pt}{} & \HoloSegScore{4.105}{(2.892--4.359)}{4.55pt}{4.82pt}{} & \HoloSegScore{4.731}{(2.613--8.690)}{4.55pt}{4.82pt}{} & \HoloSegScore{2.622}{(2.339--2.905)}{4.55pt}{4.82pt}{} \\
\cline{3-11}
 &  &  & \HoloSegMetric{Dice} &  & \HoloSegScore{0.0000}{(0.0000--0.0000)}{4.55pt}{4.82pt}{} & \HoloSegScore{0.9016}{(0.8836--0.9153)}{4.55pt}{4.82pt}{} & \HoloSegScore{0.8576}{(0.8386--0.8731)}{4.55pt}{4.82pt}{} & \HoloSegScore{0.8836}{(0.8820--0.8944)}{4.55pt}{4.82pt}{} & \HoloSegScore{0.8717}{(0.8497--0.8882)}{4.55pt}{4.82pt}{} & \HoloSegScore{0.8858}{(0.8717--0.8970)}{4.55pt}{4.82pt}{} \\*
\softcline{4-4}\softcline{6-11}
 &  & \HoloSegSpan{\makecell[c]{right\\[-0.10ex]mastoid\\[-0.10ex]process}}{2.04cm}{0.32cm} & \HoloSegMetric{HD95} & \raisebox{0.32cm}[0pt][0pt]{\HoloSegUnsupported} & \HoloSegScore{88.99}{(84.59--93.08)}{4.55pt}{4.82pt}{} & \HoloSegScore{2.460}{(1.910--3.495)}{4.55pt}{4.82pt}{} & \HoloSegScore{3.515}{(2.942--4.307)}{4.55pt}{4.82pt}{} & \HoloSegScore{3.660}{(2.745--5.490)}{4.55pt}{4.82pt}{} & \HoloSegScore{2.979}{(2.666--3.341)}{4.55pt}{4.82pt}{} & \HoloSegScore{2.964}{(2.529--3.510)}{4.55pt}{4.82pt}{} \\
\cline{3-11}
 &  &  & \HoloSegMetric{Dice} &  & \HoloSegScore{0.002152}{(0.00004084--0.004916)}{3.52pt}{3.80pt}{} & \HoloSegScore{0.8665}{(0.8439--0.8876)}{4.55pt}{4.82pt}{} & \HoloSegScore{0.8346}{(0.8170--0.8510)}{4.55pt}{4.82pt}{} & \HoloSegScore{0.8516}{(0.8462--0.8533)}{4.55pt}{4.82pt}{} & \HoloSegScore{0.8147}{(0.7916--0.8355)}{4.55pt}{4.82pt}{} & \HoloSegScore{0.8676}{(0.8518--0.8832)}{4.55pt}{4.82pt}{} \\*
\softcline{4-4}\softcline{6-11}
 &  & \HoloSegSpan{\makecell[c]{left\\[-0.10ex]temporomandibular\\[-0.10ex]joint}}{2.04cm}{0.32cm} & \HoloSegMetric{HD95} & \raisebox{0.32cm}[0pt][0pt]{\HoloSegUnsupported} & \HoloSegScore{101.2}{(99.04--103.3)}{4.55pt}{4.82pt}{} & \HoloSegScore{2.156}{(1.802--2.527)}{4.55pt}{4.82pt}{} & \HoloSegScore{2.785}{(2.585--2.939)}{4.55pt}{4.82pt}{} & \HoloSegScore{3.614}{(2.983--3.750)}{4.55pt}{4.82pt}{} & \HoloSegScore{24.30}{(10.24--38.55)}{4.55pt}{4.82pt}{} & \HoloSegScore{2.385}{(2.072--2.670)}{4.55pt}{4.82pt}{} \\
\hline
\pagebreak[4]
 &  &  & \HoloSegMetric{Dice} &  & \HoloSegScore{0.009331}{(0.002716--0.01814)}{3.85pt}{4.12pt}{} & \HoloSegScore{0.8894}{(0.8763--0.9004)}{4.55pt}{4.82pt}{} & \HoloSegScore{0.8466}{(0.8321--0.8601)}{4.55pt}{4.82pt}{} & \HoloSegScore{0.8785}{(0.8555--0.8929)}{4.55pt}{4.82pt}{} & \HoloSegScore{0.7384}{(0.7136--0.7646)}{4.55pt}{4.82pt}{} & \HoloSegScore{0.8687}{(0.8535--0.8824)}{4.55pt}{4.82pt}{} \\*
\softcline{4-4}\softcline{6-11}
 &  & \HoloSegSpan{\makecell[c]{right\\[-0.10ex]temporomandibular\\[-0.10ex]joint}}{2.04cm}{0.32cm} & \HoloSegMetric{HD95} & \raisebox{0.32cm}[0pt][0pt]{\HoloSegUnsupported} & \HoloSegScore{93.57}{(84.93--100.5)}{4.55pt}{4.82pt}{} & \HoloSegScore{2.022}{(1.711--2.372)}{4.55pt}{4.82pt}{} & \HoloSegScore{2.740}{(2.548--2.912)}{4.55pt}{4.82pt}{} & \HoloSegScore{5.153}{(4.454--5.202)}{4.55pt}{4.82pt}{} & \HoloSegScore{19.16}{(3.782--49.41)}{4.55pt}{4.82pt}{} & \HoloSegScore{2.330}{(2.057--2.621)}{4.55pt}{4.82pt}{} \\
\cline{3-11}
 &  &  & \HoloSegMetric{Dice} & \HoloSegScore{0.7975}{(0.7839--0.8107)}{4.55pt}{4.82pt}{} & \HoloSegScore{0.1869}{(0.1496--0.2226)}{4.55pt}{4.82pt}{} & \HoloSegScore{0.8709}{(0.8525--0.8862)}{4.55pt}{4.82pt}{} & \HoloSegScore{0.8239}{(0.7806--0.8604)}{4.55pt}{4.82pt}{} & \HoloSegScore{0.8319}{(0.8033--0.8507)}{4.55pt}{4.82pt}{} & \HoloSegScore{0.8396}{(0.8222--0.8547)}{4.55pt}{4.82pt}{} & \HoloSegScore{0.8623}{(0.8448--0.8775)}{4.55pt}{4.82pt}{} \\*
\softcline{4-11}
 &  & \HoloSegSpan{\makecell[c]{spinal cord}}{2.04cm}{0.32cm} & \HoloSegMetric{HD95} & \HoloSegScore{7.998}{(4.392--12.72)}{4.55pt}{4.82pt}{} & \HoloSegScore{110.4}{(99.98--120.9)}{4.55pt}{4.82pt}{} & \HoloSegScore{5.125}{(2.021--9.731)}{4.55pt}{4.82pt}{} & \HoloSegScore{43.10}{(7.395--82.88)}{4.55pt}{4.82pt}{} & \HoloSegScore{5.727}{(2.054--10.91)}{4.55pt}{4.82pt}{} & \HoloSegScore{7.202}{(3.840--11.83)}{4.55pt}{4.82pt}{} & \HoloSegScore{25.43}{(11.31--41.74)}{4.55pt}{4.82pt}{} \\
\cline{3-11}
 &  &  & \HoloSegMetric{Dice} & \HoloSegScore{0.6289}{(0.6077--0.6512)}{4.55pt}{4.82pt}{} & \HoloSegScore{0.09060}{(0.05086--0.1324)}{4.20pt}{4.48pt}{} & \HoloSegScore{0.7896}{(0.7726--0.8043)}{4.55pt}{4.82pt}{} & \HoloSegScore{0.7504}{(0.7336--0.7663)}{4.55pt}{4.82pt}{} & \HoloSegScore{0.7850}{(0.7714--0.7871)}{4.55pt}{4.82pt}{} & \HoloSegScore{0.8123}{(0.7943--0.8293)}{4.55pt}{4.82pt}{} & \HoloSegScore{0.8198}{(0.8038--0.8360)}{4.55pt}{4.82pt}{} \\*
\softcline{4-11}
 &  & \HoloSegSpan{\makecell[c]{esophagus}}{2.04cm}{0.32cm} & \HoloSegMetric{HD95} & \HoloSegScore{12.22}{(10.78--13.81)}{4.55pt}{4.82pt}{} & \HoloSegScore{96.59}{(80.59--114.1)}{4.55pt}{4.82pt}{} & \HoloSegScore{3.381}{(2.816--4.080)}{4.55pt}{4.82pt}{} & \HoloSegScore{4.376}{(3.837--4.921)}{4.55pt}{4.82pt}{} & \HoloSegScore{4.496}{(3.445--5.751)}{4.55pt}{4.82pt}{} & \HoloSegScore{3.294}{(2.871--3.873)}{4.55pt}{4.82pt}{} & \HoloSegScore{3.510}{(2.976--4.112)}{4.55pt}{4.82pt}{} \\
\cline{3-11}
 &  &  & \HoloSegMetric{Dice} &  & \HoloSegScore{0.02382}{(0.006618--0.05056)}{3.85pt}{4.12pt}{} & \HoloSegScore{0.8597}{(0.8258--0.8803)}{4.55pt}{4.82pt}{} & \HoloSegScore{0.7720}{(0.7524--0.7914)}{4.55pt}{4.82pt}{} & \HoloSegScore{0.8651}{(0.8496--0.8683)}{4.55pt}{4.82pt}{} & \HoloSegScore{0.9003}{(0.8898--0.9087)}{4.55pt}{4.82pt}{} & \HoloSegScore{0.9029}{(0.8955--0.9099)}{4.55pt}{4.82pt}{} \\*
\softcline{4-4}\softcline{6-11}
 &  & \HoloSegSpan{\makecell[c]{larynx}}{2.04cm}{0.32cm} & \HoloSegMetric{HD95} & \raisebox{0.32cm}[0pt][0pt]{\HoloSegUnsupported} & \HoloSegScore{71.01}{(64.22--78.57)}{4.55pt}{4.82pt}{} & \HoloSegScore{30.49}{(8.881--62.24)}{4.55pt}{4.82pt}{} & \HoloSegScore{21.37}{(10.13--42.58)}{4.55pt}{4.82pt}{} & \HoloSegScore{7.188}{(5.649--10.95)}{4.55pt}{4.82pt}{} & \HoloSegScore{24.15}{(4.508--54.72)}{4.55pt}{4.82pt}{} & \HoloSegScore{3.837}{(3.228--4.595)}{4.55pt}{4.82pt}{} \\
\cline{3-11}
 &  &  & \HoloSegMetric{Dice} &  & \HoloSegScore{0.1967}{(0.1373--0.2578)}{4.55pt}{4.82pt}{} & \HoloSegScore{0.7457}{(0.7108--0.7799)}{4.55pt}{4.82pt}{} & \HoloSegScore{0.6913}{(0.6665--0.7126)}{4.55pt}{4.82pt}{} & \HoloSegScore{0.7078}{(0.6653--0.7273)}{4.55pt}{4.82pt}{} & \HoloSegScore{0.7432}{(0.7107--0.7746)}{4.55pt}{4.82pt}{} & \HoloSegScore{0.7731}{(0.7452--0.8003)}{4.55pt}{4.82pt}{} \\*
\softcline{4-4}\softcline{6-11}
 & \HoloSegSpan{\makecell[c]{SegRap2023-\\[-0.10ex]Task1}}{1.86cm}{0.32cm} & \HoloSegSpan{\makecell[c]{larynx\\[-0.10ex]glottis}}{2.04cm}{0.32cm} & \HoloSegMetric{HD95} & \raisebox{0.32cm}[0pt][0pt]{\HoloSegUnsupported} & \HoloSegScore{16.26}{(13.47--19.24)}{4.55pt}{4.82pt}{} & \HoloSegScore{14.75}{(3.112--37.68)}{4.55pt}{4.82pt}{} & \HoloSegScore{3.873}{(3.534--4.288)}{4.55pt}{4.82pt}{} & \HoloSegScore{6.623}{(5.703--7.933)}{4.55pt}{4.82pt}{} & \HoloSegScore{3.567}{(3.289--3.897)}{4.55pt}{4.82pt}{} & \HoloSegScore{2.992}{(2.827--3.179)}{4.55pt}{4.82pt}{} \\
\cline{3-11}
 &  &  & \HoloSegMetric{Dice} &  & \HoloSegScore{0.2230}{(0.1535--0.2908)}{4.55pt}{4.82pt}{} & \HoloSegScore{0.8223}{(0.7946--0.8490)}{4.55pt}{4.82pt}{} & \HoloSegScore{0.7856}{(0.7660--0.8056)}{4.55pt}{4.82pt}{} & \HoloSegScore{0.7797}{(0.7510--0.7838)}{4.55pt}{4.82pt}{} & \HoloSegScore{0.8235}{(0.8035--0.8416)}{4.55pt}{4.82pt}{} & \HoloSegScore{0.8269}{(0.8133--0.8403)}{4.55pt}{4.82pt}{} \\*
\softcline{4-4}\softcline{6-11}
 &  & \HoloSegSpan{\makecell[c]{larynx\\[-0.10ex]supraglottis}}{2.04cm}{0.32cm} & \HoloSegMetric{HD95} & \raisebox{0.32cm}[0pt][0pt]{\HoloSegUnsupported} & \HoloSegScore{44.00}{(33.76--53.85)}{4.55pt}{4.82pt}{} & \HoloSegScore{3.013}{(2.614--3.517)}{4.55pt}{4.82pt}{} & \HoloSegScore{4.192}{(3.678--4.703)}{4.55pt}{4.82pt}{} & \HoloSegScore{3.982}{(3.792--4.973)}{4.55pt}{4.82pt}{} & \HoloSegScore{3.269}{(3.030--3.557)}{4.55pt}{4.82pt}{} & \HoloSegScore{3.135}{(3.005--3.295)}{4.55pt}{4.82pt}{} \\
\cline{3-11}
 &  &  & \HoloSegMetric{Dice} &  & \HoloSegScore{0.03987}{(0.02739--0.05410)}{4.20pt}{4.48pt}{} & \HoloSegScore{0.7754}{(0.7549--0.7938)}{4.55pt}{4.82pt}{} & \HoloSegScore{0.7443}{(0.7206--0.7646)}{4.55pt}{4.82pt}{} & \HoloSegScore{0.7726}{(0.7623--0.7801)}{4.55pt}{4.82pt}{} & \HoloSegScore{0.7229}{(0.7106--0.7369)}{4.55pt}{4.82pt}{} & \HoloSegScore{0.7880}{(0.7767--0.7989)}{4.55pt}{4.82pt}{} \\*
\softcline{4-4}\softcline{6-11}
 &  & \HoloSegSpan{\makecell[c]{pharynx\\[-0.10ex]constrictor\\[-0.10ex]muscle}}{2.04cm}{0.32cm} & \HoloSegMetric{HD95} & \raisebox{0.32cm}[0pt][0pt]{\HoloSegUnsupported} & \HoloSegScore{29.24}{(26.77--32.01)}{4.55pt}{4.82pt}{} & \HoloSegScore{14.99}{(2.933--38.85)}{4.55pt}{4.82pt}{} & \HoloSegScore{3.632}{(3.085--4.306)}{4.55pt}{4.82pt}{} & \HoloSegScore{5.987}{(3.404--6.582)}{4.55pt}{4.82pt}{} & \HoloSegScore{15.16}{(3.236--38.74)}{4.55pt}{4.82pt}{} & \HoloSegScore{2.394}{(2.205--2.624)}{4.55pt}{4.82pt}{} \\
\cline{3-11}
 &  &  & \HoloSegMetric{Dice} & \HoloSegScore{0.7331}{(0.7136--0.7501)}{4.55pt}{4.82pt}{} & \HoloSegScore{0.0000}{(0.0000--0.0000)}{4.55pt}{4.82pt}{} & \HoloSegScore{0.8539}{(0.8384--0.8666)}{4.55pt}{4.82pt}{} & \HoloSegScore{0.8239}{(0.8074--0.8400)}{4.55pt}{4.82pt}{} & \HoloSegScore{0.7876}{(0.7789--0.7981)}{4.55pt}{4.82pt}{} & \HoloSegScore{0.8320}{(0.8192--0.8443)}{4.55pt}{4.82pt}{} & \HoloSegScore{0.8466}{(0.8339--0.8587)}{4.55pt}{4.82pt}{} \\*
\softcline{4-11}
 &  & \HoloSegSpan{\makecell[c]{thyroid}}{2.04cm}{0.32cm} & \HoloSegMetric{HD95} & \HoloSegScore{6.385}{(5.551--7.396)}{4.55pt}{4.82pt}{} & \HoloSegScore{110.8}{(104.9--116.3)}{4.55pt}{4.82pt}{} & \HoloSegScore{3.018}{(2.842--3.226)}{4.55pt}{4.82pt}{} & \HoloSegScore{3.268}{(2.959--3.752)}{4.55pt}{4.82pt}{} & \HoloSegScore{3.315}{(3.009--3.725)}{4.55pt}{4.82pt}{} & \HoloSegScore{2.907}{(2.697--3.091)}{4.55pt}{4.82pt}{} & \HoloSegScore{3.002}{(2.774--3.245)}{4.55pt}{4.82pt}{} \\
\cline{3-11}
 &  &  & \HoloSegMetric{Dice} & \HoloSegScore{0.5316}{(0.5136--0.5516)}{4.55pt}{4.82pt}{} & \HoloSegScore{0.009948}{(0.0000--0.02355)}{4.20pt}{4.48pt}{} & \HoloSegScore{0.8612}{(0.8376--0.8831)}{4.55pt}{4.82pt}{} & \HoloSegScore{0.8221}{(0.7862--0.8502)}{4.55pt}{4.82pt}{} & \HoloSegScore{0.8424}{(0.8394--0.8568)}{4.55pt}{4.82pt}{} & \HoloSegScore{0.8784}{(0.8633--0.8932)}{4.55pt}{4.82pt}{} & \HoloSegScore{0.8993}{(0.8839--0.9139)}{4.55pt}{4.82pt}{} \\*
\softcline{4-11}
 &  & \HoloSegSpan{\makecell[c]{trachea}}{2.04cm}{0.32cm} & \HoloSegMetric{HD95} & \HoloSegScore{36.33}{(31.81--40.35)}{4.55pt}{4.82pt}{} & \HoloSegScore{166.1}{(145.6--184.9)}{4.55pt}{4.82pt}{} & \HoloSegScore{11.87}{(7.287--17.43)}{4.55pt}{4.82pt}{} & \HoloSegScore{10.83}{(7.197--15.84)}{4.55pt}{4.82pt}{} & \HoloSegScore{11.52}{(7.207--15.70)}{4.55pt}{4.82pt}{} & \HoloSegScore{5.006}{(3.575--6.777)}{4.55pt}{4.82pt}{} & \HoloSegScore{5.039}{(3.185--7.666)}{4.55pt}{4.82pt}{} \\
\cline{2-11}
 &  &  & \HoloSegMetric{Dice} &  & \HoloSegScore{0.002187}{(0.0001856--0.005513)}{3.52pt}{3.80pt}{} & \HoloSegScore{0.7788}{(0.7398--0.8097)}{4.55pt}{4.82pt}{} & \HoloSegScore{0.3064}{(0.2417--0.3724)}{4.55pt}{4.82pt}{} & \HoloSegScore{0.8296}{(0.8294--0.8526)}{4.55pt}{4.82pt}{} & \HoloSegScore{0.6328}{(0.5843--0.6755)}{4.55pt}{4.82pt}{} & \HoloSegScore{0.7244}{(0.6923--0.7484)}{4.55pt}{4.82pt}{} \\*
\softcline{4-4}\softcline{6-11}
\HoloSegSpan{\makecell[c]{\textbf{Internal}}}{1.20cm}{0.32cm} &  & \HoloSegSpan{\makecell[c]{nasopharyngeal\\[-0.10ex]tumor}}{2.04cm}{0.32cm} & \HoloSegMetric{HD95} & \raisebox{0.32cm}[0pt][0pt]{\HoloSegUnsupported} & \HoloSegScore{71.72}{(65.00--78.35)}{4.55pt}{4.82pt}{} & \HoloSegScore{19.98}{(7.535--41.61)}{4.55pt}{4.82pt}{} & \HoloSegScore{38.52}{(21.02--64.17)}{4.55pt}{4.82pt}{} & \HoloSegScore{20.53}{(8.774--41.37)}{4.55pt}{4.82pt}{} & \HoloSegScore{14.47}{(11.22--18.62)}{4.55pt}{4.82pt}{} & \HoloSegScore{29.87}{(14.93--56.91)}{4.55pt}{4.82pt}{} \\
\cline{3-11}
 & \HoloSegSpan{\makecell[c]{SegRap2023-\\[-0.10ex]Task2}}{1.86cm}{0.32cm} &  & \HoloSegMetric{Dice} &  & \HoloSegScore{0.001640}{(0.0000--0.004416)}{4.20pt}{4.48pt}{} & \HoloSegScore{0.6381}{(0.5694--0.6997)}{4.55pt}{4.82pt}{} & \HoloSegScore{0.004323}{(0.0000--0.01297)}{4.20pt}{4.48pt}{} & \HoloSegScore{0.7123}{(0.6978--0.7196)}{4.55pt}{4.82pt}{} & \HoloSegScore{0.3367}{(0.2793--0.3920)}{4.55pt}{4.82pt}{} & \HoloSegScore{0.5250}{(0.4580--0.5865)}{4.55pt}{4.82pt}{} \\*
\softcline{4-4}\softcline{6-11}
 &  & \HoloSegSpan{\makecell[c]{nasopharyngeal\\[-0.10ex]lymph node}}{2.04cm}{0.32cm} & \HoloSegMetric{HD95} & \raisebox{0.32cm}[0pt][0pt]{\HoloSegUnsupported} & \HoloSegScore{64.11}{(59.90--67.79)}{4.55pt}{4.82pt}{} & \HoloSegScore{30.79}{(15.00--59.02)}{4.55pt}{4.82pt}{} & \HoloSegScore{108.0}{(84.78--131.3)}{4.55pt}{4.82pt}{} & \HoloSegScore{23.40}{(20.04--27.76)}{4.55pt}{4.82pt}{} & \HoloSegScore{30.33}{(24.93--36.53)}{4.55pt}{4.82pt}{} & \HoloSegScore{33.31}{(24.50--43.14)}{4.55pt}{4.82pt}{} \\
\cline{2-11}
 &  &  & \HoloSegMetric{Dice} & \HoloSegScore{0.7929}{(0.7621--0.8268)}{4.55pt}{4.82pt}{} & \HoloSegScore{0.3342}{(0.2458--0.4129)}{4.55pt}{4.82pt}{} & \HoloSegScore{0.7966}{(0.7598--0.8337)}{4.55pt}{4.82pt}{} & \HoloSegScore{0.8287}{(0.8036--0.8532)}{4.55pt}{4.82pt}{} & \HoloSegScore{0.8099}{(0.8012--0.8177)}{4.55pt}{4.82pt}{} & \HoloSegScore{0.8294}{(0.8077--0.8500)}{4.55pt}{4.82pt}{} & \HoloSegScore{0.8339}{(0.8143--0.8561)}{4.55pt}{4.82pt}{} \\*
\softcline{4-11}
 &  & \HoloSegSpan{\makecell[c]{esophagus}}{2.04cm}{0.32cm} & \HoloSegMetric{HD95} & \HoloSegScore{8.426}{(4.842--12.72)}{4.55pt}{4.82pt}{} & \HoloSegScore{21.88}{(13.53--35.45)}{4.55pt}{4.82pt}{} & \HoloSegScore{6.908}{(4.097--11.00)}{4.55pt}{4.82pt}{} & \HoloSegScore{3.744}{(3.096--4.567)}{4.55pt}{4.82pt}{} & \HoloSegScore{7.661}{(6.495--8.199)}{4.55pt}{4.82pt}{} & \HoloSegScore{3.664}{(3.053--4.280)}{4.55pt}{4.82pt}{} & \HoloSegScore{3.812}{(2.825--4.952)}{4.55pt}{4.82pt}{} \\
\cline{3-11}
 &  &  & \HoloSegMetric{Dice} & \HoloSegScore{0.7648}{(0.7395--0.7896)}{4.55pt}{4.82pt}{} & \HoloSegScore{0.2601}{(0.1695--0.3392)}{4.55pt}{4.82pt}{} & \HoloSegScore{0.9186}{(0.8740--0.9524)}{4.55pt}{4.82pt}{} & \HoloSegScore{0.9120}{(0.8794--0.9349)}{4.55pt}{4.82pt}{} & \HoloSegScore{0.8955}{(0.8808--0.9100)}{4.55pt}{4.82pt}{} & \HoloSegScore{0.9350}{(0.9256--0.9438)}{4.55pt}{4.82pt}{} & \HoloSegScore{0.9305}{(0.9194--0.9409)}{4.55pt}{4.82pt}{} \\*
\softcline{4-11}
 &  & \HoloSegSpan{\makecell[c]{heart}}{2.04cm}{0.32cm} & \HoloSegMetric{HD95} & \HoloSegScore{29.31}{(27.25--31.12)}{4.55pt}{4.82pt}{} & \HoloSegScore{63.70}{(43.22--90.88)}{4.55pt}{4.82pt}{} & \HoloSegScore{8.279}{(5.200--11.80)}{4.55pt}{4.82pt}{} & \HoloSegScore{11.78}{(7.189--16.80)}{4.55pt}{4.82pt}{} & \HoloSegScore{12.81}{(10.46--13.11)}{4.55pt}{4.82pt}{} & \HoloSegScore{47.16}{(20.97--82.00)}{4.55pt}{4.82pt}{} & \HoloSegScore{31.47}{(6.373--79.55)}{4.55pt}{4.82pt}{} \\
\cline{3-11}
 & \HoloSegSpan{\makecell[c]{SegTHOR}}{1.86cm}{0.32cm} &  & \HoloSegMetric{Dice} & \HoloSegScore{0.8959}{(0.8813--0.9106)}{4.55pt}{4.82pt}{} & \HoloSegScore{0.5922}{(0.5182--0.6514)}{4.55pt}{4.82pt}{} & \HoloSegScore{0.8885}{(0.8750--0.9026)}{4.55pt}{4.82pt}{} & \HoloSegScore{0.9172}{(0.9071--0.9281)}{4.55pt}{4.82pt}{} & \HoloSegScore{0.9016}{(0.8936--0.9099)}{4.55pt}{4.82pt}{} & \HoloSegScore{0.8959}{(0.8908--0.9015)}{4.55pt}{4.82pt}{} & \HoloSegScore{0.9003}{(0.8924--0.9077)}{4.55pt}{4.82pt}{} \\*
\softcline{4-11}
 &  & \HoloSegSpan{\makecell[c]{trachea}}{2.04cm}{0.32cm} & \HoloSegMetric{HD95} & \HoloSegScore{4.159}{(2.820--5.655)}{4.55pt}{4.82pt}{} & \HoloSegScore{26.44}{(14.78--40.81)}{4.55pt}{4.82pt}{} & \HoloSegScore{4.447}{(3.442--5.533)}{4.55pt}{4.82pt}{} & \HoloSegScore{5.246}{(2.574--8.599)}{4.55pt}{4.82pt}{} & \HoloSegScore{6.156}{(5.129--7.758)}{4.55pt}{4.82pt}{} & \HoloSegScore{5.775}{(4.437--7.170)}{4.55pt}{4.82pt}{} & \HoloSegScore{4.669}{(3.653--5.682)}{4.55pt}{4.82pt}{} \\
\cline{3-11}
 &  &  & \HoloSegMetric{Dice} & \HoloSegScore{0.7894}{(0.7438--0.8260)}{4.55pt}{4.82pt}{} & \HoloSegScore{0.6177}{(0.5032--0.6998)}{4.55pt}{4.82pt}{} & \HoloSegScore{0.8495}{(0.7910--0.8990)}{4.55pt}{4.82pt}{} & \HoloSegScore{0.8296}{(0.7816--0.8696)}{4.55pt}{4.82pt}{} & \HoloSegScore{0.8257}{(0.7921--0.8571)}{4.55pt}{4.82pt}{} & \HoloSegScore{0.8597}{(0.8252--0.8894)}{4.55pt}{4.82pt}{} & \HoloSegScore{0.8551}{(0.8073--0.8912)}{4.55pt}{4.82pt}{} \\*
\softcline{4-11}
 &  & \HoloSegSpan{\makecell[c]{aorta}}{2.04cm}{0.32cm} & \HoloSegMetric{HD95} & \HoloSegScore{52.74}{(34.71--76.24)}{4.55pt}{4.82pt}{} & \HoloSegScore{40.05}{(23.19--58.40)}{4.55pt}{4.82pt}{} & \HoloSegScore{30.12}{(10.38--54.99)}{4.55pt}{4.82pt}{} & \HoloSegScore{45.19}{(24.96--69.20)}{4.55pt}{4.82pt}{} & \HoloSegScore{41.08}{(21.89--64.22)}{4.55pt}{4.82pt}{} & \HoloSegScore{43.83}{(21.16--73.13)}{4.55pt}{4.82pt}{} & \HoloSegScore{44.52}{(22.48--73.98)}{4.55pt}{4.82pt}{} \\
\cline{2-11}
 &  &  & \HoloSegMetric{Dice} & \HoloSegScore{0.9487}{(0.9454--0.9521)}{4.55pt}{4.82pt}{} & \HoloSegScore{0.1908}{(0.1360--0.2567)}{4.55pt}{4.82pt}{} & \HoloSegScore{0.9492}{(0.9440--0.9542)}{4.55pt}{4.82pt}{} & \HoloSegScore{0.8216}{(0.7494--0.8873)}{4.55pt}{4.82pt}{} & \HoloSegScore{0.9286}{(0.9194--0.9423)}{4.55pt}{4.82pt}{} & \HoloSegScore{0.9686}{(0.9653--0.9716)}{4.55pt}{4.82pt}{} & \HoloSegScore{0.9780}{(0.9761--0.9796)}{4.55pt}{4.82pt}{} \\*
\softcline{4-11}
 &  & \HoloSegSpan{\makecell[c]{brain}}{2.04cm}{0.32cm} & \HoloSegMetric{HD95} & \HoloSegScore{4.111}{(3.708--4.630)}{4.55pt}{4.82pt}{} & \HoloSegScore{26.39}{(23.04--29.58)}{4.55pt}{4.82pt}{} & \HoloSegScore{5.958}{(4.384--8.392)}{4.55pt}{4.82pt}{} & \HoloSegScore{22.43}{(15.53--28.61)}{4.55pt}{4.82pt}{} & \HoloSegScore{3.987}{(2.675--4.132)}{4.55pt}{4.82pt}{} & \HoloSegScore{14.41}{(8.480--20.76)}{4.55pt}{4.82pt}{} & \HoloSegScore{5.168}{(4.422--5.894)}{4.55pt}{4.82pt}{} \\
\cline{3-11}
 & \HoloSegSpan{\makecell[c]{Seg-CQ500}}{1.86cm}{0.32cm} &  & \HoloSegMetric{Dice} &  & \HoloSegScore{0.02812}{(0.002430--0.07246)}{3.85pt}{4.12pt}{} & \HoloSegScore{0.4952}{(0.2779--0.7230)}{4.55pt}{4.82pt}{} & \HoloSegScore{0.1473}{(0.01200--0.2897)}{4.20pt}{4.48pt}{} & \HoloSegScore{0.8216}{(0.7790--0.8381)}{4.55pt}{4.82pt}{} & \HoloSegScore{0.6198}{(0.4365--0.7955)}{4.55pt}{4.82pt}{} & \HoloSegScore{0.5941}{(0.3719--0.8015)}{4.55pt}{4.82pt}{} \\*
\softcline{4-4}\softcline{6-11}
 &  & \HoloSegSpan{\makecell[c]{intracranial\\[-0.10ex]hemorrhage}}{2.04cm}{0.32cm} & \HoloSegMetric{HD95} & \raisebox{0.32cm}[0pt][0pt]{\HoloSegUnsupported} & \HoloSegScore{84.83}{(76.67--94.50)}{4.55pt}{4.82pt}{} & \HoloSegScore{23.52}{(8.838--41.17)}{4.55pt}{4.82pt}{} & \HoloSegScore{76.04}{(57.66--94.57)}{4.55pt}{4.82pt}{} & \HoloSegScore{5.583}{(4.114--11.80)}{4.55pt}{4.82pt}{} & \HoloSegScore{17.52}{(6.278--31.80)}{4.55pt}{4.82pt}{} & \HoloSegScore{35.20}{(11.78--64.26)}{4.55pt}{4.82pt}{} \\
\cline{2-11}
 &  &  & \HoloSegMetric{Dice} & \HoloSegScore{0.7441}{(0.7082--0.7751)}{4.55pt}{4.82pt}{} & \HoloSegScore{0.3488}{(0.2735--0.4136)}{4.55pt}{4.82pt}{} & \HoloSegScore{0.7510}{(0.7183--0.7785)}{4.55pt}{4.82pt}{} & \HoloSegScore{0.7314}{(0.6948--0.7654)}{4.55pt}{4.82pt}{} & \HoloSegScore{0.7287}{(0.7044--0.7469)}{4.55pt}{4.82pt}{} & \HoloSegScore{0.7622}{(0.7383--0.7843)}{4.55pt}{4.82pt}{} & \HoloSegScore{0.7689}{(0.7436--0.7913)}{4.55pt}{4.82pt}{} \\*
\softcline{4-11}
 &  & \HoloSegSpan{\makecell[c]{esophagus}}{2.04cm}{0.32cm} & \HoloSegMetric{HD95} & \HoloSegScore{14.45}{(10.15--19.22)}{4.55pt}{4.82pt}{} & \HoloSegScore{26.51}{(18.60--36.25)}{4.55pt}{4.82pt}{} & \HoloSegScore{10.72}{(7.604--14.35)}{4.55pt}{4.82pt}{} & \HoloSegScore{12.07}{(8.671--16.01)}{4.55pt}{4.82pt}{} & \HoloSegScore{15.39}{(12.46--20.01)}{4.55pt}{4.82pt}{} & \HoloSegScore{11.11}{(7.256--15.19)}{4.55pt}{4.82pt}{} & \HoloSegScore{10.60}{(7.008--14.54)}{4.55pt}{4.82pt}{} \\
\cline{3-11}
 & \HoloSegSpan{\makecell[c]{NSCLC-\\[-0.10ex]Radiomics}}{1.86cm}{0.32cm} &  & \HoloSegMetric{Dice} & \HoloSegScore{0.3292}{(0.1941--0.4679)}{4.55pt}{4.82pt}{} & \HoloSegScore{0.3666}{(0.2287--0.5092)}{4.55pt}{4.82pt}{} & \HoloSegScore{0.3165}{(0.1727--0.4573)}{4.55pt}{4.82pt}{} & \HoloSegScore{0.7002}{(0.5498--0.8220)}{4.55pt}{4.82pt}{} & \HoloSegScore{0.6031}{(0.4662--0.7297)}{4.55pt}{4.82pt}{} & \HoloSegScore{0.5078}{(0.3461--0.6692)}{4.55pt}{4.82pt}{} & \HoloSegScore{0.6038}{(0.4493--0.7512)}{4.55pt}{4.82pt}{} \\*
\softcline{4-11}
 &  & \HoloSegSpan{\makecell[c]{lung tumor}}{2.04cm}{0.32cm} & \HoloSegMetric{HD95} & \HoloSegScore{120.8}{(81.65--171.3)}{4.55pt}{4.82pt}{} & \HoloSegScore{76.72}{(39.93--120.0)}{4.55pt}{4.82pt}{} & \HoloSegScore{69.50}{(42.54--98.61)}{4.55pt}{4.82pt}{} & \HoloSegScore{48.63}{(21.44--80.43)}{4.55pt}{4.82pt}{} & \HoloSegScore{49.43}{(24.79--77.47)}{4.55pt}{4.82pt}{} & \HoloSegScore{66.03}{(39.77--93.92)}{4.55pt}{4.82pt}{} & \HoloSegScore{45.00}{(23.72--72.16)}{4.55pt}{4.82pt}{} \\
\hline
\pagebreak[4]
 &  &  & \HoloSegMetric{Dice} & \HoloSegScore{0.8111}{(0.7760--0.8462)}{4.55pt}{4.82pt}{} & \HoloSegScore{0.2579}{(0.1326--0.3645)}{4.55pt}{4.82pt}{} & \HoloSegScore{0.8787}{(0.8572--0.9042)}{4.55pt}{4.82pt}{} & \HoloSegScore{0.8588}{(0.8325--0.8830)}{4.55pt}{4.82pt}{} & \HoloSegScore{0.8843}{(0.8501--0.8955)}{4.55pt}{4.82pt}{} & \HoloSegScore{0.8946}{(0.8705--0.9224)}{4.55pt}{4.82pt}{} & \HoloSegScore{0.8947}{(0.8757--0.9175)}{4.55pt}{4.82pt}{} \\*
\softcline{4-11}
 &  & \HoloSegSpan{\makecell[c]{heart}}{2.04cm}{0.32cm} & \HoloSegMetric{HD95} & \HoloSegScore{32.06}{(30.08--35.56)}{4.55pt}{4.82pt}{} & \HoloSegScore{56.88}{(37.64--80.16)}{4.55pt}{4.82pt}{} & \HoloSegScore{13.52}{(10.13--16.90)}{4.55pt}{4.82pt}{} & \HoloSegScore{22.37}{(16.20--29.69)}{4.55pt}{4.82pt}{} & \HoloSegScore{15.02}{(14.76--15.79)}{4.55pt}{4.82pt}{} & \HoloSegScore{26.80}{(10.04--52.09)}{4.55pt}{4.82pt}{} & \HoloSegScore{15.33}{(12.09--20.51)}{4.55pt}{4.82pt}{} \\
\cline{3-11}
 &  &  & \HoloSegMetric{Dice} & \HoloSegScore{0.9452}{(0.9157--0.9669)}{4.55pt}{4.82pt}{} & \HoloSegScore{0.8312}{(0.7301--0.8980)}{4.55pt}{4.82pt}{} & \HoloSegScore{0.9415}{(0.9036--0.9650)}{4.55pt}{4.82pt}{} & \HoloSegScore{0.9616}{(0.9458--0.9734)}{4.55pt}{4.82pt}{} & \HoloSegScore{0.9557}{(0.9400--0.9741)}{4.55pt}{4.82pt}{} & \HoloSegScore{0.9711}{(0.9616--0.9773)}{4.55pt}{4.82pt}{} & \HoloSegScore{0.9678}{(0.9591--0.9737)}{4.55pt}{4.82pt}{} \\*
\softcline{4-11}
 &  & \HoloSegSpan{\makecell[c]{left lung}}{2.04cm}{0.32cm} & \HoloSegMetric{HD95} & \HoloSegScore{12.56}{(5.295--22.32)}{4.55pt}{4.82pt}{} & \HoloSegScore{20.99}{(10.55--39.87)}{4.55pt}{4.82pt}{} & \HoloSegScore{6.996}{(4.826--9.815)}{4.55pt}{4.82pt}{} & \HoloSegScore{5.922}{(3.167--9.832)}{4.55pt}{4.82pt}{} & \HoloSegScore{3.761}{(3.369--5.570)}{4.55pt}{4.82pt}{} & \HoloSegScore{2.970}{(2.524--3.424)}{4.55pt}{4.82pt}{} & \HoloSegScore{4.224}{(3.211--5.400)}{4.55pt}{4.82pt}{} \\
\cline{3-11}
 & \HoloSegSpan{\makecell[c]{NSCLC-\\[-0.10ex]Radiomics}}{1.86cm}{0.32cm} &  & \HoloSegMetric{Dice} & \HoloSegScore{0.9527}{(0.9432--0.9619)}{4.55pt}{4.82pt}{} & \HoloSegScore{0.8164}{(0.6881--0.9053)}{4.55pt}{4.82pt}{} & \HoloSegScore{0.9633}{(0.9523--0.9714)}{4.55pt}{4.82pt}{} & \HoloSegScore{0.9652}{(0.9583--0.9713)}{4.55pt}{4.82pt}{} & \HoloSegScore{0.9296}{(0.9213--0.9411)}{4.55pt}{4.82pt}{} & \HoloSegScore{0.9702}{(0.9635--0.9754)}{4.55pt}{4.82pt}{} & \HoloSegScore{0.9721}{(0.9671--0.9757)}{4.55pt}{4.82pt}{} \\*
\softcline{4-11}
 &  & \HoloSegSpan{\makecell[c]{right lung}}{2.04cm}{0.32cm} & \HoloSegMetric{HD95} & \HoloSegScore{15.28}{(12.32--18.42)}{4.55pt}{4.82pt}{} & \HoloSegScore{24.90}{(10.56--50.77)}{4.55pt}{4.82pt}{} & \HoloSegScore{5.912}{(4.355--7.527)}{4.55pt}{4.82pt}{} & \HoloSegScore{6.316}{(3.701--10.59)}{4.55pt}{4.82pt}{} & \HoloSegScore{6.890}{(3.147--9.680)}{4.55pt}{4.82pt}{} & \HoloSegScore{8.072}{(5.297--11.02)}{4.55pt}{4.82pt}{} & \HoloSegScore{5.759}{(3.182--9.861)}{4.55pt}{4.82pt}{} \\
\cline{3-11}
 &  &  & \HoloSegMetric{Dice} & \HoloSegScore{0.7842}{(0.7344--0.8251)}{4.55pt}{4.82pt}{} & \HoloSegScore{0.006259}{(0.0003417--0.01737)}{3.85pt}{4.12pt}{} & \HoloSegScore{0.3921}{(0.3035--0.4863)}{4.55pt}{4.82pt}{} & \HoloSegScore{0.8107}{(0.7638--0.8503)}{4.55pt}{4.82pt}{} & \HoloSegScore{0.7653}{(0.7064--0.8074)}{4.55pt}{4.82pt}{} & \HoloSegScore{0.7847}{(0.7308--0.8309)}{4.55pt}{4.82pt}{} & \HoloSegScore{0.8163}{(0.7625--0.8645)}{4.55pt}{4.82pt}{} \\*
\softcline{4-11}
 &  & \HoloSegSpan{\makecell[c]{spinal cord}}{2.04cm}{0.32cm} & \HoloSegMetric{HD95} & \HoloSegScore{34.38}{(12.20--61.09)}{4.55pt}{4.82pt}{} & \HoloSegScore{249.5}{(217.2--277.6)}{4.55pt}{4.82pt}{} & \HoloSegScore{60.58}{(38.68--83.81)}{4.55pt}{4.82pt}{} & \HoloSegScore{29.46}{(10.71--53.04)}{4.55pt}{4.82pt}{} & \HoloSegScore{32.95}{(13.76--55.11)}{4.55pt}{4.82pt}{} & \HoloSegScore{46.43}{(27.37--73.98)}{4.55pt}{4.82pt}{} & \HoloSegScore{30.19}{(9.560--56.22)}{4.55pt}{4.82pt}{} \\
\cline{2-11}
 &  &  & \HoloSegMetric{Dice} &  & \HoloSegScore{0.04945}{(0.007386--0.1178)}{4.20pt}{4.48pt}{} & \HoloSegScore{0.5973}{(0.5033--0.6830)}{4.55pt}{4.82pt}{} & \HoloSegScore{0.6690}{(0.5858--0.7394)}{4.55pt}{4.82pt}{} & \HoloSegScore{0.5744}{(0.4791--0.6476)}{4.55pt}{4.82pt}{} & \HoloSegScore{0.5300}{(0.4047--0.6480)}{4.55pt}{4.82pt}{} & \HoloSegScore{0.5465}{(0.4292--0.6523)}{4.55pt}{4.82pt}{} \\*
\softcline{4-4}\softcline{6-11}
 &  & \HoloSegSpan{\makecell[c]{lung\\[-0.10ex]effusion}}{2.04cm}{0.32cm} & \HoloSegMetric{HD95} & \raisebox{0.32cm}[0pt][0pt]{\HoloSegUnsupported} & \HoloSegScore{123.9}{(100.5--146.9)}{4.55pt}{4.82pt}{} & \HoloSegScore{41.69}{(26.59--59.37)}{4.55pt}{4.82pt}{} & \HoloSegScore{53.55}{(35.96--73.33)}{4.55pt}{4.82pt}{} & \HoloSegScore{51.98}{(35.84--71.85)}{4.55pt}{4.82pt}{} & \HoloSegScore{65.09}{(38.85--101.3)}{4.55pt}{4.82pt}{} & \HoloSegScore{48.50}{(34.29--64.61)}{4.55pt}{4.82pt}{} \\
\cline{3-11}
 & \HoloSegSpan{\makecell[c]{PleThora\\[-0.10ex](NSCLC-\\[-0.10ex]Radiomics)}}{1.86cm}{0.32cm} &  & \HoloSegMetric{Dice} &  & \HoloSegScore{0.7464}{(0.6227--0.8425)}{4.55pt}{4.82pt}{} & \HoloSegScore{0.9540}{(0.9455--0.9607)}{4.55pt}{4.82pt}{} & \HoloSegScore{0.2585}{(0.1935--0.3326)}{4.55pt}{4.82pt}{} & \HoloSegScore{0.9407}{(0.9200--0.9543)}{4.55pt}{4.82pt}{} & \HoloSegScore{0.9476}{(0.9375--0.9544)}{4.55pt}{4.82pt}{} & \HoloSegScore{0.9468}{(0.9393--0.9524)}{4.55pt}{4.82pt}{} \\*
\softcline{4-4}\softcline{6-11}
 &  & \HoloSegSpan{\makecell[c]{thoracic\\[-0.10ex]cavity}}{2.04cm}{0.32cm} & \HoloSegMetric{HD95} & \raisebox{0.32cm}[0pt][0pt]{\HoloSegUnsupported} & \HoloSegScore{32.50}{(19.49--53.79)}{4.55pt}{4.82pt}{} & \HoloSegScore{5.425}{(3.570--8.044)}{4.55pt}{4.82pt}{} & \HoloSegScore{32.32}{(28.08--37.18)}{4.55pt}{4.82pt}{} & \HoloSegScore{7.518}{(6.408--10.30)}{4.55pt}{4.82pt}{} & \HoloSegScore{7.958}{(5.830--11.17)}{4.55pt}{4.82pt}{} & \HoloSegScore{9.108}{(6.889--11.58)}{4.55pt}{4.82pt}{} \\
\cline{2-11}
 &  &  & \HoloSegMetric{Dice} & \HoloSegScore{0.9561}{(0.9504--0.9614)}{4.55pt}{4.82pt}{} & \HoloSegScore{0.8224}{(0.8126--0.8315)}{4.55pt}{4.82pt}{} & \HoloSegScore{0.9625}{(0.9587--0.9662)}{4.55pt}{4.82pt}{} & \HoloSegScore{0.9627}{(0.9590--0.9661)}{4.55pt}{4.82pt}{} & \HoloSegScore{0.9276}{(0.9261--0.9276)}{4.55pt}{4.82pt}{} & \HoloSegScore{0.9621}{(0.9585--0.9655)}{4.55pt}{4.82pt}{} & \HoloSegScore{0.9627}{(0.9595--0.9660)}{4.55pt}{4.82pt}{} \\*
\softcline{4-11}
 &  & \HoloSegSpan{\makecell[c]{liver}}{2.04cm}{0.32cm} & \HoloSegMetric{HD95} & \HoloSegScore{5.376}{(3.831--8.065)}{4.55pt}{4.82pt}{} & \HoloSegScore{16.24}{(14.54--18.00)}{4.55pt}{4.82pt}{} & \HoloSegScore{3.539}{(3.175--3.974)}{4.55pt}{4.82pt}{} & \HoloSegScore{4.218}{(3.429--5.193)}{4.55pt}{4.82pt}{} & \HoloSegScore{5.881}{(5.434--6.735)}{4.55pt}{4.82pt}{} & \HoloSegScore{4.207}{(3.348--5.537)}{4.55pt}{4.82pt}{} & \HoloSegScore{4.916}{(3.508--7.178)}{4.55pt}{4.82pt}{} \\
\cline{3-11}
 &  &  & \HoloSegMetric{Dice} & \HoloSegScore{0.9437}{(0.9375--0.9490)}{4.55pt}{4.82pt}{} & \HoloSegScore{0.6545}{(0.5700--0.7203)}{4.55pt}{4.82pt}{} & \HoloSegScore{0.9528}{(0.9485--0.9573)}{4.55pt}{4.82pt}{} & \HoloSegScore{0.9560}{(0.9520--0.9600)}{4.55pt}{4.82pt}{} & \HoloSegScore{0.9422}{(0.9379--0.9472)}{4.55pt}{4.82pt}{} & \HoloSegScore{0.9554}{(0.9508--0.9595)}{4.55pt}{4.82pt}{} & \HoloSegScore{0.9519}{(0.9474--0.9565)}{4.55pt}{4.82pt}{} \\*
\softcline{4-11}
 &  & \HoloSegSpan{\makecell[c]{spleen}}{2.04cm}{0.32cm} & \HoloSegMetric{HD95} & \HoloSegScore{2.760}{(2.437--3.189)}{4.55pt}{4.82pt}{} & \HoloSegScore{25.74}{(14.54--41.17)}{4.55pt}{4.82pt}{} & \HoloSegScore{2.331}{(2.174--2.561)}{4.55pt}{4.82pt}{} & \HoloSegScore{2.091}{(1.739--2.608)}{4.55pt}{4.82pt}{} & \HoloSegScore{2.308}{(2.269--2.728)}{4.55pt}{4.82pt}{} & \HoloSegScore{2.038}{(1.839--2.233)}{4.55pt}{4.82pt}{} & \HoloSegScore{2.189}{(1.897--2.556)}{4.55pt}{4.82pt}{} \\
\cline{3-11}
 &  &  & \HoloSegMetric{Dice} & \HoloSegScore{0.9402}{(0.9339--0.9459)}{4.55pt}{4.82pt}{} & \HoloSegScore{0.6298}{(0.5064--0.7208)}{4.55pt}{4.82pt}{} & \HoloSegScore{0.9498}{(0.9439--0.9554)}{4.55pt}{4.82pt}{} & \HoloSegScore{0.9518}{(0.9458--0.9574)}{4.55pt}{4.82pt}{} & \HoloSegScore{0.9374}{(0.9341--0.9379)}{4.55pt}{4.82pt}{} & \HoloSegScore{0.9505}{(0.9460--0.9550)}{4.55pt}{4.82pt}{} & \HoloSegScore{0.9466}{(0.9404--0.9524)}{4.55pt}{4.82pt}{} \\*
\softcline{4-11}
 &  & \HoloSegSpan{\makecell[c]{left kidney}}{2.04cm}{0.32cm} & \HoloSegMetric{HD95} & \HoloSegScore{2.947}{(2.651--3.360)}{4.55pt}{4.82pt}{} & \HoloSegScore{49.39}{(25.18--80.52)}{4.55pt}{4.82pt}{} & \HoloSegScore{2.750}{(2.492--3.036)}{4.55pt}{4.82pt}{} & \HoloSegScore{2.342}{(2.003--2.726)}{4.55pt}{4.82pt}{} & \HoloSegScore{3.689}{(2.955--4.706)}{4.55pt}{4.82pt}{} & \HoloSegScore{2.578}{(2.351--2.806)}{4.55pt}{4.82pt}{} & \HoloSegScore{3.569}{(2.741--4.480)}{4.55pt}{4.82pt}{} \\
\cline{3-11}
 &  &  & \HoloSegMetric{Dice} & \HoloSegScore{0.9425}{(0.9344--0.9490)}{4.55pt}{4.82pt}{} & \HoloSegScore{0.6971}{(0.6089--0.7622)}{4.55pt}{4.82pt}{} & \HoloSegScore{0.9522}{(0.9455--0.9580)}{4.55pt}{4.82pt}{} & \HoloSegScore{0.9529}{(0.9448--0.9591)}{4.55pt}{4.82pt}{} & \HoloSegScore{0.9374}{(0.9367--0.9603)}{4.55pt}{4.82pt}{} & \HoloSegScore{0.9486}{(0.9416--0.9546)}{4.55pt}{4.82pt}{} & \HoloSegScore{0.9504}{(0.9446--0.9556)}{4.55pt}{4.82pt}{} \\*
\softcline{4-11}
\HoloSegSpan{\makecell[c]{\textbf{Internal}}}{1.20cm}{0.32cm} &  & \HoloSegSpan{\makecell[c]{right kidney}}{2.04cm}{0.32cm} & \HoloSegMetric{HD95} & \HoloSegScore{3.003}{(2.686--3.420)}{4.55pt}{4.82pt}{} & \HoloSegScore{29.79}{(12.19--57.95)}{4.55pt}{4.82pt}{} & \HoloSegScore{2.479}{(2.226--2.697)}{4.55pt}{4.82pt}{} & \HoloSegScore{2.161}{(1.863--2.484)}{4.55pt}{4.82pt}{} & \HoloSegScore{2.594}{(1.848--3.269)}{4.55pt}{4.82pt}{} & \HoloSegScore{2.721}{(2.140--3.507)}{4.55pt}{4.82pt}{} & \HoloSegScore{2.570}{(2.163--3.040)}{4.55pt}{4.82pt}{} \\
\cline{3-11}
 &  &  & \HoloSegMetric{Dice} & \HoloSegScore{0.9248}{(0.9162--0.9333)}{4.55pt}{4.82pt}{} & \HoloSegScore{0.6049}{(0.5649--0.6431)}{4.55pt}{4.82pt}{} & \HoloSegScore{0.8931}{(0.8224--0.9344)}{4.55pt}{4.82pt}{} & \HoloSegScore{0.9230}{(0.9073--0.9349)}{4.55pt}{4.82pt}{} & \HoloSegScore{0.9040}{(0.8936--0.9091)}{4.55pt}{4.82pt}{} & \HoloSegScore{0.9306}{(0.9228--0.9384)}{4.55pt}{4.82pt}{} & \HoloSegScore{0.9310}{(0.9222--0.9406)}{4.55pt}{4.82pt}{} \\*
\softcline{4-11}
 &  & \HoloSegSpan{\makecell[c]{stomach}}{2.04cm}{0.32cm} & \HoloSegMetric{HD95} & \HoloSegScore{8.752}{(5.570--12.66)}{4.55pt}{4.82pt}{} & \HoloSegScore{34.81}{(24.50--46.19)}{4.55pt}{4.82pt}{} & \HoloSegScore{44.23}{(4.850--101.9)}{4.55pt}{4.82pt}{} & \HoloSegScore{9.741}{(6.021--14.58)}{4.55pt}{4.82pt}{} & \HoloSegScore{10.55}{(5.212--14.93)}{4.55pt}{4.82pt}{} & \HoloSegScore{7.678}{(4.563--11.80)}{4.55pt}{4.82pt}{} & \HoloSegScore{7.250}{(3.783--11.83)}{4.55pt}{4.82pt}{} \\
\cline{3-11}
 &  &  & \HoloSegMetric{Dice} & \HoloSegScore{0.6820}{(0.5374--0.8048)}{4.55pt}{4.82pt}{} & \HoloSegScore{0.1990}{(0.1243--0.2705)}{4.55pt}{4.82pt}{} & \HoloSegScore{0.7758}{(0.6790--0.8486)}{4.55pt}{4.82pt}{} & \HoloSegScore{0.6624}{(0.5235--0.7896)}{4.55pt}{4.82pt}{} & \HoloSegScore{0.7604}{(0.6827--0.8236)}{4.55pt}{4.82pt}{} & \HoloSegScore{0.7916}{(0.6927--0.8637)}{4.55pt}{4.82pt}{} & \HoloSegScore{0.8013}{(0.7334--0.8602)}{4.55pt}{4.82pt}{} \\*
\softcline{4-11}
 &  & \HoloSegSpan{\makecell[c]{gallbladder}}{2.04cm}{0.32cm} & \HoloSegMetric{HD95} & \HoloSegScore{11.69}{(5.726--18.98)}{4.55pt}{4.82pt}{} & \HoloSegScore{36.07}{(26.23--47.81)}{4.55pt}{4.82pt}{} & \HoloSegScore{5.879}{(3.664--8.850)}{4.55pt}{4.82pt}{} & \HoloSegScore{11.81}{(6.575--18.22)}{4.55pt}{4.82pt}{} & \HoloSegScore{8.354}{(6.296--9.125)}{4.55pt}{4.82pt}{} & \HoloSegScore{6.723}{(4.002--10.28)}{4.55pt}{4.82pt}{} & \HoloSegScore{5.564}{(4.099--7.152)}{4.55pt}{4.82pt}{} \\
\cline{3-11}
 &  &  & \HoloSegMetric{Dice} & \HoloSegScore{0.7668}{(0.7381--0.7922)}{4.55pt}{4.82pt}{} & \HoloSegScore{0.2922}{(0.2220--0.3561)}{4.55pt}{4.82pt}{} & \HoloSegScore{0.7973}{(0.7758--0.8199)}{4.55pt}{4.82pt}{} & \HoloSegScore{0.7887}{(0.7672--0.8076)}{4.55pt}{4.82pt}{} & \HoloSegScore{0.7910}{(0.7595--0.8096)}{4.55pt}{4.82pt}{} & \HoloSegScore{0.7953}{(0.7757--0.8149)}{4.55pt}{4.82pt}{} & \HoloSegScore{0.8077}{(0.7886--0.8267)}{4.55pt}{4.82pt}{} \\*
\softcline{4-11}
 & \HoloSegSpan{\makecell[c]{WORD}}{1.86cm}{0.32cm} & \HoloSegSpan{\makecell[c]{esophagus}}{2.04cm}{0.32cm} & \HoloSegMetric{HD95} & \HoloSegScore{6.856}{(2.874--12.02)}{4.55pt}{4.82pt}{} & \HoloSegScore{18.86}{(15.61--22.73)}{4.55pt}{4.82pt}{} & \HoloSegScore{5.172}{(3.924--6.774)}{4.55pt}{4.82pt}{} & \HoloSegScore{5.484}{(4.476--6.650)}{4.55pt}{4.82pt}{} & \HoloSegScore{6.299}{(5.175--6.738)}{4.55pt}{4.82pt}{} & \HoloSegScore{4.816}{(3.920--5.804)}{4.55pt}{4.82pt}{} & \HoloSegScore{4.419}{(3.588--5.442)}{4.55pt}{4.82pt}{} \\
\cline{3-11}
 &  &  & \HoloSegMetric{Dice} & \HoloSegScore{0.8051}{(0.7719--0.8312)}{4.55pt}{4.82pt}{} & \HoloSegScore{0.3685}{(0.3015--0.4333)}{4.55pt}{4.82pt}{} & \HoloSegScore{0.8349}{(0.8063--0.8593)}{4.55pt}{4.82pt}{} & \HoloSegScore{0.8217}{(0.7879--0.8483)}{4.55pt}{4.82pt}{} & \HoloSegScore{0.8201}{(0.7803--0.8477)}{4.55pt}{4.82pt}{} & \HoloSegScore{0.8415}{(0.8207--0.8583)}{4.55pt}{4.82pt}{} & \HoloSegScore{0.8442}{(0.8192--0.8638)}{4.55pt}{4.82pt}{} \\*
\softcline{4-11}
 &  & \HoloSegSpan{\makecell[c]{pancreas}}{2.04cm}{0.32cm} & \HoloSegMetric{HD95} & \HoloSegScore{21.78}{(5.518--52.62)}{4.55pt}{4.82pt}{} & \HoloSegScore{28.37}{(20.44--37.13)}{4.55pt}{4.82pt}{} & \HoloSegScore{5.426}{(3.865--7.636)}{4.55pt}{4.82pt}{} & \HoloSegScore{7.738}{(5.342--11.00)}{4.55pt}{4.82pt}{} & \HoloSegScore{5.755}{(4.015--8.534)}{4.55pt}{4.82pt}{} & \HoloSegScore{6.037}{(4.696--7.833)}{4.55pt}{4.82pt}{} & \HoloSegScore{5.675}{(4.309--7.397)}{4.55pt}{4.82pt}{} \\
\cline{3-11}
 &  &  & \HoloSegMetric{Dice} & \HoloSegScore{0.6498}{(0.5802--0.7098)}{4.55pt}{4.82pt}{} & \HoloSegScore{0.3182}{(0.2619--0.3680)}{4.55pt}{4.82pt}{} & \HoloSegScore{0.7024}{(0.6356--0.7593)}{4.55pt}{4.82pt}{} & \HoloSegScore{0.6791}{(0.6088--0.7356)}{4.55pt}{4.82pt}{} & \HoloSegScore{0.6900}{(0.6358--0.7355)}{4.55pt}{4.82pt}{} & \HoloSegScore{0.7156}{(0.6618--0.7573)}{4.55pt}{4.82pt}{} & \HoloSegScore{0.7491}{(0.6938--0.7943)}{4.55pt}{4.82pt}{} \\*
\softcline{4-11}
 &  & \HoloSegSpan{\makecell[c]{duodenum}}{2.04cm}{0.32cm} & \HoloSegMetric{HD95} & \HoloSegScore{18.97}{(13.37--25.85)}{4.55pt}{4.82pt}{} & \HoloSegScore{36.53}{(28.25--45.74)}{4.55pt}{4.82pt}{} & \HoloSegScore{15.10}{(9.578--21.58)}{4.55pt}{4.82pt}{} & \HoloSegScore{19.33}{(13.68--25.90)}{4.55pt}{4.82pt}{} & \HoloSegScore{17.69}{(11.89--24.65)}{4.55pt}{4.82pt}{} & \HoloSegScore{18.18}{(13.85--23.63)}{4.55pt}{4.82pt}{} & \HoloSegScore{13.61}{(8.403--19.70)}{4.55pt}{4.82pt}{} \\
\cline{3-11}
 &  &  & \HoloSegMetric{Dice} & \HoloSegScore{0.7646}{(0.7145--0.8037)}{4.55pt}{4.82pt}{} & \HoloSegScore{0.3529}{(0.2545--0.4412)}{4.55pt}{4.82pt}{} & \HoloSegScore{0.8537}{(0.8273--0.8746)}{4.55pt}{4.82pt}{} & \HoloSegScore{0.7982}{(0.7603--0.8291)}{4.55pt}{4.82pt}{} & \HoloSegScore{0.7949}{(0.7523--0.8196)}{4.55pt}{4.82pt}{} & \HoloSegScore{0.8205}{(0.7846--0.8509)}{4.55pt}{4.82pt}{} & \HoloSegScore{0.8439}{(0.8226--0.8636)}{4.55pt}{4.82pt}{} \\*
\softcline{4-11}
 &  & \HoloSegSpan{\makecell[c]{colon}}{2.04cm}{0.32cm} & \HoloSegMetric{HD95} & \HoloSegScore{33.62}{(24.69--44.81)}{4.55pt}{4.82pt}{} & \HoloSegScore{63.04}{(45.15--81.67)}{4.55pt}{4.82pt}{} & \HoloSegScore{13.31}{(6.995--23.67)}{4.55pt}{4.82pt}{} & \HoloSegScore{39.11}{(23.16--56.89)}{4.55pt}{4.82pt}{} & \HoloSegScore{23.60}{(15.07--33.76)}{4.55pt}{4.82pt}{} & \HoloSegScore{17.79}{(10.44--28.35)}{4.55pt}{4.82pt}{} & \HoloSegScore{20.11}{(13.12--29.16)}{4.55pt}{4.82pt}{} \\
\cline{3-11}
 &  &  & \HoloSegMetric{Dice} &  & \HoloSegScore{0.4437}{(0.3432--0.5353)}{4.55pt}{4.82pt}{} & \HoloSegScore{0.8718}{(0.8613--0.8831)}{4.55pt}{4.82pt}{} & \HoloSegScore{0.7057}{(0.6793--0.7331)}{4.55pt}{4.82pt}{} & \HoloSegScore{0.8536}{(0.8445--0.8619)}{4.55pt}{4.82pt}{} & \HoloSegScore{0.8427}{(0.8270--0.8571)}{4.55pt}{4.82pt}{} & \HoloSegScore{0.8516}{(0.8328--0.8672)}{4.55pt}{4.82pt}{} \\*
\softcline{4-4}\softcline{6-11}
 &  & \HoloSegSpan{\makecell[c]{intestine}}{2.04cm}{0.32cm} & \HoloSegMetric{HD95} & \raisebox{0.32cm}[0pt][0pt]{\HoloSegUnsupported} & \HoloSegScore{42.23}{(28.14--59.90)}{4.55pt}{4.82pt}{} & \HoloSegScore{6.439}{(5.231--7.722)}{4.55pt}{4.82pt}{} & \HoloSegScore{40.65}{(35.26--45.63)}{4.55pt}{4.82pt}{} & \HoloSegScore{7.284}{(5.424--8.345)}{4.55pt}{4.82pt}{} & \HoloSegScore{16.31}{(9.763--26.94)}{4.55pt}{4.82pt}{} & \HoloSegScore{9.200}{(6.981--11.50)}{4.55pt}{4.82pt}{} \\
\cline{3-11}
 &  &  & \HoloSegMetric{Dice} & \HoloSegScore{0.6666}{(0.6256--0.7069)}{4.55pt}{4.82pt}{} & \HoloSegScore{0.1799}{(0.1239--0.2339)}{4.55pt}{4.82pt}{} & \HoloSegScore{0.7212}{(0.6967--0.7446)}{4.55pt}{4.82pt}{} & \HoloSegScore{0.7110}{(0.6752--0.7423)}{4.55pt}{4.82pt}{} & \HoloSegScore{0.6981}{(0.6830--0.7173)}{4.55pt}{4.82pt}{} & \HoloSegScore{0.7223}{(0.6895--0.7550)}{4.55pt}{4.82pt}{} & \HoloSegScore{0.7493}{(0.7253--0.7734)}{4.55pt}{4.82pt}{} \\*
\softcline{4-11}
 &  & \HoloSegSpan{\makecell[c]{adrenal\\[-0.10ex]gland}}{2.04cm}{0.32cm} & \HoloSegMetric{HD95} & \HoloSegScore{7.641}{(5.610--10.48)}{4.55pt}{4.82pt}{} & \HoloSegScore{31.66}{(22.67--42.24)}{4.55pt}{4.82pt}{} & \HoloSegScore{5.437}{(4.164--7.441)}{4.55pt}{4.82pt}{} & \HoloSegScore{6.760}{(4.863--9.333)}{4.55pt}{4.82pt}{} & \HoloSegScore{5.890}{(3.245--6.450)}{4.55pt}{4.82pt}{} & \HoloSegScore{7.579}{(5.000--10.79)}{4.55pt}{4.82pt}{} & \HoloSegScore{5.193}{(3.919--6.912)}{4.55pt}{4.82pt}{} \\
\cline{3-11}
 &  &  & \HoloSegMetric{Dice} &  & \HoloSegScore{0.3615}{(0.2513--0.4570)}{4.55pt}{4.82pt}{} & \HoloSegScore{0.8143}{(0.7940--0.8369)}{4.55pt}{4.82pt}{} & \HoloSegScore{0.7670}{(0.7200--0.8008)}{4.55pt}{4.82pt}{} & \HoloSegScore{0.7936}{(0.7813--0.8252)}{4.55pt}{4.82pt}{} & \HoloSegScore{0.7852}{(0.7314--0.8252)}{4.55pt}{4.82pt}{} & \HoloSegScore{0.7967}{(0.7655--0.8247)}{4.55pt}{4.82pt}{} \\*
\softcline{4-4}\softcline{6-11}
 &  & \HoloSegSpan{\makecell[c]{rectum}}{2.04cm}{0.32cm} & \HoloSegMetric{HD95} & \raisebox{0.32cm}[0pt][0pt]{\HoloSegUnsupported} & \HoloSegScore{55.30}{(23.55--95.91)}{4.55pt}{4.82pt}{} & \HoloSegScore{8.083}{(6.297--10.10)}{4.55pt}{4.82pt}{} & \HoloSegScore{13.12}{(10.46--15.77)}{4.55pt}{4.82pt}{} & \HoloSegScore{10.46}{(7.858--12.74)}{4.55pt}{4.82pt}{} & \HoloSegScore{12.41}{(8.604--16.50)}{4.55pt}{4.82pt}{} & \HoloSegScore{11.46}{(8.807--14.43)}{4.55pt}{4.82pt}{} \\
\hline
\pagebreak[4]
 &  &  & \HoloSegMetric{Dice} & \HoloSegScore{0.9302}{(0.9120--0.9462)}{4.55pt}{4.82pt}{} & \HoloSegScore{0.5440}{(0.4430--0.6387)}{4.55pt}{4.82pt}{} & \HoloSegScore{0.9386}{(0.9188--0.9526)}{4.55pt}{4.82pt}{} & \HoloSegScore{0.9392}{(0.9205--0.9538)}{4.55pt}{4.82pt}{} & \HoloSegScore{0.9259}{(0.9196--0.9583)}{4.55pt}{4.82pt}{} & \HoloSegScore{0.9390}{(0.9175--0.9547)}{4.55pt}{4.82pt}{} & \HoloSegScore{0.9387}{(0.9185--0.9542)}{4.55pt}{4.82pt}{} \\*
\softcline{4-11}
 &  & \HoloSegSpan{\makecell[c]{urinary\\[-0.10ex]bladder}}{2.04cm}{0.32cm} & \HoloSegMetric{HD95} & \HoloSegScore{3.797}{(3.219--4.564)}{4.55pt}{4.82pt}{} & \HoloSegScore{37.30}{(20.22--63.40)}{4.55pt}{4.82pt}{} & \HoloSegScore{3.199}{(2.939--3.555)}{4.55pt}{4.82pt}{} & \HoloSegScore{3.194}{(2.831--3.783)}{4.55pt}{4.82pt}{} & \HoloSegScore{6.697}{(5.355--6.890)}{4.55pt}{4.82pt}{} & \HoloSegScore{5.799}{(2.865--11.05)}{4.55pt}{4.82pt}{} & \HoloSegScore{3.649}{(2.875--4.758)}{4.55pt}{4.82pt}{} \\
\cline{3-11}
 &  &  & \HoloSegMetric{Dice} &  & \HoloSegScore{0.6506}{(0.6189--0.6827)}{4.55pt}{4.82pt}{} & \HoloSegScore{0.9211}{(0.9047--0.9350)}{4.55pt}{4.82pt}{} & \HoloSegScore{0.9208}{(0.9039--0.9364)}{4.55pt}{4.82pt}{} & \HoloSegScore{0.9205}{(0.9185--0.9278)}{4.55pt}{4.82pt}{} & \HoloSegScore{0.9140}{(0.9001--0.9263)}{4.55pt}{4.82pt}{} & \HoloSegScore{0.9246}{(0.9113--0.9351)}{4.55pt}{4.82pt}{} \\*
\softcline{4-4}\softcline{6-11}
 & \HoloSegSpan{\makecell[c]{WORD}}{1.86cm}{0.32cm} & \HoloSegSpan{\makecell[c]{head of left\\[-0.10ex]femur}}{2.04cm}{0.32cm} & \HoloSegMetric{HD95} & \raisebox{0.32cm}[0pt][0pt]{\HoloSegUnsupported} & \HoloSegScore{28.61}{(17.34--41.61)}{4.55pt}{4.82pt}{} & \HoloSegScore{91.48}{(23.69--167.1)}{4.55pt}{4.82pt}{} & \HoloSegScore{7.549}{(4.657--11.45)}{4.55pt}{4.82pt}{} & \HoloSegScore{8.945}{(6.646--12.70)}{4.55pt}{4.82pt}{} & \HoloSegScore{10.51}{(5.966--15.77)}{4.55pt}{4.82pt}{} & \HoloSegScore{28.48}{(9.954--51.01)}{4.55pt}{4.82pt}{} \\
\cline{3-11}
 &  &  & \HoloSegMetric{Dice} &  & \HoloSegScore{0.6252}{(0.5480--0.6835)}{4.55pt}{4.82pt}{} & \HoloSegScore{0.9234}{(0.9062--0.9359)}{4.55pt}{4.82pt}{} & \HoloSegScore{0.9203}{(0.9016--0.9358)}{4.55pt}{4.82pt}{} & \HoloSegScore{0.9059}{(0.8786--0.9314)}{4.55pt}{4.82pt}{} & \HoloSegScore{0.9245}{(0.9105--0.9366)}{4.55pt}{4.82pt}{} & \HoloSegScore{0.9263}{(0.9146--0.9361)}{4.55pt}{4.82pt}{} \\*
\softcline{4-4}\softcline{6-11}
 &  & \HoloSegSpan{\makecell[c]{head of\\[-0.10ex]right femur}}{2.04cm}{0.32cm} & \HoloSegMetric{HD95} & \raisebox{0.32cm}[0pt][0pt]{\HoloSegUnsupported} & \HoloSegScore{32.73}{(17.56--55.25)}{4.55pt}{4.82pt}{} & \HoloSegScore{46.12}{(5.689--100.4)}{4.55pt}{4.82pt}{} & \HoloSegScore{7.149}{(4.382--10.57)}{4.55pt}{4.82pt}{} & \HoloSegScore{9.459}{(4.065--12.59)}{4.55pt}{4.82pt}{} & \HoloSegScore{5.970}{(3.900--9.030)}{4.55pt}{4.82pt}{} & \HoloSegScore{4.915}{(3.471--7.136)}{4.55pt}{4.82pt}{} \\
\cline{2-11}
 &  &  & \HoloSegMetric{Dice} & \HoloSegScore{0.9545}{(0.9493--0.9587)}{4.55pt}{4.82pt}{} & \HoloSegScore{0.8250}{(0.8112--0.8370)}{4.55pt}{4.82pt}{} & \HoloSegScore{0.9596}{(0.9562--0.9628)}{4.55pt}{4.82pt}{} & \HoloSegScore{0.9599}{(0.9556--0.9637)}{4.55pt}{4.82pt}{} & \HoloSegScore{0.9524}{(0.9401--0.9584)}{4.55pt}{4.82pt}{} & \HoloSegScore{0.9614}{(0.9592--0.9634)}{4.55pt}{4.82pt}{} & \HoloSegScore{0.9614}{(0.9586--0.9636)}{4.55pt}{4.82pt}{} \\*
\softcline{4-11}
 &  & \HoloSegSpan{\makecell[c]{liver}}{2.04cm}{0.32cm} & \HoloSegMetric{HD95} & \HoloSegScore{4.994}{(4.014--6.185)}{4.55pt}{4.82pt}{} & \HoloSegScore{14.54}{(13.62--15.52)}{4.55pt}{4.82pt}{} & \HoloSegScore{3.597}{(3.274--3.967)}{4.55pt}{4.82pt}{} & \HoloSegScore{4.561}{(3.546--5.934)}{4.55pt}{4.82pt}{} & \HoloSegScore{6.038}{(4.464--6.394)}{4.55pt}{4.82pt}{} & \HoloSegScore{4.126}{(3.525--4.922)}{4.55pt}{4.82pt}{} & \HoloSegScore{4.382}{(3.571--5.383)}{4.55pt}{4.82pt}{} \\
\cline{3-11}
 &  &  & \HoloSegMetric{Dice} & \HoloSegScore{0.9374}{(0.9306--0.9443)}{4.55pt}{4.82pt}{} & \HoloSegScore{0.7319}{(0.7068--0.7536)}{4.55pt}{4.82pt}{} & \HoloSegScore{0.9418}{(0.9362--0.9472)}{4.55pt}{4.82pt}{} & \HoloSegScore{0.9481}{(0.9418--0.9539)}{4.55pt}{4.82pt}{} & \HoloSegScore{0.9362}{(0.9351--0.9368)}{4.55pt}{4.82pt}{} & \HoloSegScore{0.9524}{(0.9490--0.9555)}{4.55pt}{4.82pt}{} & \HoloSegScore{0.9515}{(0.9484--0.9543)}{4.55pt}{4.82pt}{} \\*
\softcline{4-11}
 &  & \HoloSegSpan{\makecell[c]{spleen}}{2.04cm}{0.32cm} & \HoloSegMetric{HD95} & \HoloSegScore{3.617}{(2.749--4.782)}{4.55pt}{4.82pt}{} & \HoloSegScore{13.28}{(11.68--15.27)}{4.55pt}{4.82pt}{} & \HoloSegScore{2.765}{(2.497--3.053)}{4.55pt}{4.82pt}{} & \HoloSegScore{3.931}{(2.181--6.172)}{4.55pt}{4.82pt}{} & \HoloSegScore{5.082}{(4.815--5.305)}{4.55pt}{4.82pt}{} & \HoloSegScore{2.204}{(2.048--2.366)}{4.55pt}{4.82pt}{} & \HoloSegScore{2.238}{(2.081--2.391)}{4.55pt}{4.82pt}{} \\
\cline{3-11}
 &  &  & \HoloSegMetric{Dice} & \HoloSegScore{0.9365}{(0.9320--0.9409)}{4.55pt}{4.82pt}{} & \HoloSegScore{0.7612}{(0.7403--0.7803)}{4.55pt}{4.82pt}{} & \HoloSegScore{0.9317}{(0.9242--0.9383)}{4.55pt}{4.82pt}{} & \HoloSegScore{0.9464}{(0.9411--0.9511)}{4.55pt}{4.82pt}{} & \HoloSegScore{0.9357}{(0.9313--0.9534)}{4.55pt}{4.82pt}{} & \HoloSegScore{0.9454}{(0.9396--0.9494)}{4.55pt}{4.82pt}{} & \HoloSegScore{0.9429}{(0.9378--0.9467)}{4.55pt}{4.82pt}{} \\*
\softcline{4-11}
 &  & \HoloSegSpan{\makecell[c]{left kidney}}{2.04cm}{0.32cm} & \HoloSegMetric{HD95} & \HoloSegScore{3.354}{(2.971--3.880)}{4.55pt}{4.82pt}{} & \HoloSegScore{11.46}{(10.39--12.60)}{4.55pt}{4.82pt}{} & \HoloSegScore{3.449}{(3.014--4.047)}{4.55pt}{4.82pt}{} & \HoloSegScore{2.765}{(2.332--3.223)}{4.55pt}{4.82pt}{} & \HoloSegScore{4.628}{(2.939--5.962)}{4.55pt}{4.82pt}{} & \HoloSegScore{3.480}{(2.912--4.247)}{4.55pt}{4.82pt}{} & \HoloSegScore{4.980}{(3.242--8.035)}{4.55pt}{4.82pt}{} \\
\cline{3-11}
 &  &  & \HoloSegMetric{Dice} & \HoloSegScore{0.9382}{(0.9313--0.9432)}{4.55pt}{4.82pt}{} & \HoloSegScore{0.7887}{(0.7714--0.8026)}{4.55pt}{4.82pt}{} & \HoloSegScore{0.9365}{(0.9304--0.9425)}{4.55pt}{4.82pt}{} & \HoloSegScore{0.9466}{(0.9384--0.9524)}{4.55pt}{4.82pt}{} & \HoloSegScore{0.9218}{(0.9127--0.9369)}{4.55pt}{4.82pt}{} & \HoloSegScore{0.9438}{(0.9393--0.9480)}{4.55pt}{4.82pt}{} & \HoloSegScore{0.9455}{(0.9420--0.9488)}{4.55pt}{4.82pt}{} \\*
\softcline{4-11}
 &  & \HoloSegSpan{\makecell[c]{right kidney}}{2.04cm}{0.32cm} & \HoloSegMetric{HD95} & \HoloSegScore{3.316}{(2.936--3.992)}{4.55pt}{4.82pt}{} & \HoloSegScore{10.79}{(9.995--11.53)}{4.55pt}{4.82pt}{} & \HoloSegScore{3.147}{(2.857--3.554)}{4.55pt}{4.82pt}{} & \HoloSegScore{2.650}{(2.223--3.359)}{4.55pt}{4.82pt}{} & \HoloSegScore{3.450}{(3.359--3.919)}{4.55pt}{4.82pt}{} & \HoloSegScore{3.410}{(2.927--4.003)}{4.55pt}{4.82pt}{} & \HoloSegScore{7.064}{(4.369--10.71)}{4.55pt}{4.82pt}{} \\
\cline{3-11}
 &  &  & \HoloSegMetric{Dice} & \HoloSegScore{0.8676}{(0.8018--0.9095)}{4.55pt}{4.82pt}{} & \HoloSegScore{0.6473}{(0.5819--0.6971)}{4.55pt}{4.82pt}{} & \HoloSegScore{0.8765}{(0.8121--0.9134)}{4.55pt}{4.82pt}{} & \HoloSegScore{0.8746}{(0.8148--0.9134)}{4.55pt}{4.82pt}{} & \HoloSegScore{0.9041}{(0.8781--0.9612)}{4.55pt}{4.82pt}{} & \HoloSegScore{0.9184}{(0.9081--0.9272)}{4.55pt}{4.82pt}{} & \HoloSegScore{0.9217}{(0.9118--0.9306)}{4.55pt}{4.82pt}{} \\*
\softcline{4-11}
 &  & \HoloSegSpan{\makecell[c]{stomach}}{2.04cm}{0.32cm} & \HoloSegMetric{HD95} & \HoloSegScore{14.78}{(10.02--20.06)}{4.55pt}{4.82pt}{} & \HoloSegScore{22.80}{(17.77--29.24)}{4.55pt}{4.82pt}{} & \HoloSegScore{10.36}{(6.315--16.00)}{4.55pt}{4.82pt}{} & \HoloSegScore{16.39}{(11.43--22.44)}{4.55pt}{4.82pt}{} & \HoloSegScore{8.450}{(4.787--14.38)}{4.55pt}{4.82pt}{} & \HoloSegScore{10.16}{(7.629--13.21)}{4.55pt}{4.82pt}{} & \HoloSegScore{9.883}{(7.418--12.80)}{4.55pt}{4.82pt}{} \\
\cline{3-11}
 &  &  & \HoloSegMetric{Dice} & \HoloSegScore{0.7358}{(0.6713--0.7868)}{4.55pt}{4.82pt}{} & \HoloSegScore{0.3236}{(0.2514--0.3946)}{4.55pt}{4.82pt}{} & \HoloSegScore{0.7673}{(0.7296--0.8033)}{4.55pt}{4.82pt}{} & \HoloSegScore{0.7393}{(0.6812--0.7864)}{4.55pt}{4.82pt}{} & \HoloSegScore{0.8033}{(0.7574--0.8409)}{4.55pt}{4.82pt}{} & \HoloSegScore{0.8169}{(0.7926--0.8393)}{4.55pt}{4.82pt}{} & \HoloSegScore{0.8240}{(0.7975--0.8451)}{4.55pt}{4.82pt}{} \\*
\softcline{4-11}
 &  & \HoloSegSpan{\makecell[c]{gallbladder}}{2.04cm}{0.32cm} & \HoloSegMetric{HD95} & \HoloSegScore{10.92}{(7.612--14.62)}{4.55pt}{4.82pt}{} & \HoloSegScore{20.63}{(17.99--23.60)}{4.55pt}{4.82pt}{} & \HoloSegScore{10.25}{(6.568--15.45)}{4.55pt}{4.82pt}{} & \HoloSegScore{11.35}{(7.865--15.29)}{4.55pt}{4.82pt}{} & \HoloSegScore{7.185}{(6.599--9.051)}{4.55pt}{4.82pt}{} & \HoloSegScore{6.754}{(5.153--8.691)}{4.55pt}{4.82pt}{} & \HoloSegScore{5.886}{(4.651--7.428)}{4.55pt}{4.82pt}{} \\
\cline{3-11}
 &  &  & \HoloSegMetric{Dice} & \HoloSegScore{0.7685}{(0.7353--0.7943)}{4.55pt}{4.82pt}{} & \HoloSegScore{0.4198}{(0.3874--0.4515)}{4.55pt}{4.82pt}{} & \HoloSegScore{0.7760}{(0.7424--0.8036)}{4.55pt}{4.82pt}{} & \HoloSegScore{0.7673}{(0.7385--0.7944)}{4.55pt}{4.82pt}{} & \HoloSegScore{0.8336}{(0.7989--0.8482)}{4.55pt}{4.82pt}{} & \HoloSegScore{0.8053}{(0.7914--0.8180)}{4.55pt}{4.82pt}{} & \HoloSegScore{0.8099}{(0.7964--0.8236)}{4.55pt}{4.82pt}{} \\*
\softcline{4-11}
\HoloSegSpan{\makecell[c]{\textbf{Internal}}}{1.20cm}{0.32cm} &  & \HoloSegSpan{\makecell[c]{esophagus}}{2.04cm}{0.32cm} & \HoloSegMetric{HD95} & \HoloSegScore{30.57}{(8.348--59.75)}{4.55pt}{4.82pt}{} & \HoloSegScore{12.02}{(10.51--13.56)}{4.55pt}{4.82pt}{} & \HoloSegScore{5.966}{(4.438--8.250)}{4.55pt}{4.82pt}{} & \HoloSegScore{6.512}{(4.966--8.513)}{4.55pt}{4.82pt}{} & \HoloSegScore{5.853}{(4.826--6.825)}{4.55pt}{4.82pt}{} & \HoloSegScore{4.492}{(4.014--5.007)}{4.55pt}{4.82pt}{} & \HoloSegScore{4.515}{(3.987--5.036)}{4.55pt}{4.82pt}{} \\
\cline{3-11}
 &  &  & \HoloSegMetric{Dice} & \HoloSegScore{0.7892}{(0.7649--0.8094)}{4.55pt}{4.82pt}{} & \HoloSegScore{0.5131}{(0.4806--0.5411)}{4.55pt}{4.82pt}{} & \HoloSegScore{0.8053}{(0.7818--0.8257)}{4.55pt}{4.82pt}{} & \HoloSegScore{0.8016}{(0.7780--0.8242)}{4.55pt}{4.82pt}{} & \HoloSegScore{0.8129}{(0.7849--0.8556)}{4.55pt}{4.82pt}{} & \HoloSegScore{0.8196}{(0.8013--0.8368)}{4.55pt}{4.82pt}{} & \HoloSegScore{0.8241}{(0.8053--0.8410)}{4.55pt}{4.82pt}{} \\*
\softcline{4-11}
 &  & \HoloSegSpan{\makecell[c]{pancreas}}{2.04cm}{0.32cm} & \HoloSegMetric{HD95} & \HoloSegScore{10.32}{(6.822--14.76)}{4.55pt}{4.82pt}{} & \HoloSegScore{15.70}{(13.43--18.54)}{4.55pt}{4.82pt}{} & \HoloSegScore{7.053}{(5.038--9.524)}{4.55pt}{4.82pt}{} & \HoloSegScore{9.073}{(6.444--12.20)}{4.55pt}{4.82pt}{} & \HoloSegScore{10.90}{(8.258--13.88)}{4.55pt}{4.82pt}{} & \HoloSegScore{9.211}{(7.126--11.75)}{4.55pt}{4.82pt}{} & \HoloSegScore{9.012}{(6.840--11.76)}{4.55pt}{4.82pt}{} \\
\cline{3-11}
 & \HoloSegSpan{\makecell[c]{RAOS}}{1.86cm}{0.32cm} &  & \HoloSegMetric{Dice} & \HoloSegScore{0.6143}{(0.5403--0.6784)}{4.55pt}{4.82pt}{} & \HoloSegScore{0.4098}{(0.3613--0.4537)}{4.55pt}{4.82pt}{} & \HoloSegScore{0.6310}{(0.5575--0.7017)}{4.55pt}{4.82pt}{} & \HoloSegScore{0.6450}{(0.5709--0.7078)}{4.55pt}{4.82pt}{} & \HoloSegScore{0.7201}{(0.6682--0.7556)}{4.55pt}{4.82pt}{} & \HoloSegScore{0.7041}{(0.6704--0.7333)}{4.55pt}{4.82pt}{} & \HoloSegScore{0.7288}{(0.6905--0.7636)}{4.55pt}{4.82pt}{} \\*
\softcline{4-11}
 &  & \HoloSegSpan{\makecell[c]{duodenum}}{2.04cm}{0.32cm} & \HoloSegMetric{HD95} & \HoloSegScore{22.14}{(17.21--28.21)}{4.55pt}{4.82pt}{} & \HoloSegScore{25.75}{(21.40--31.05)}{4.55pt}{4.82pt}{} & \HoloSegScore{19.52}{(14.35--25.32)}{4.55pt}{4.82pt}{} & \HoloSegScore{21.12}{(15.94--26.93)}{4.55pt}{4.82pt}{} & \HoloSegScore{18.45}{(16.18--22.84)}{4.55pt}{4.82pt}{} & \HoloSegScore{25.33}{(22.00--28.73)}{4.55pt}{4.82pt}{} & \HoloSegScore{18.34}{(14.96--21.87)}{4.55pt}{4.82pt}{} \\
\cline{3-11}
 &  &  & \HoloSegMetric{Dice} & \HoloSegScore{0.7469}{(0.7073--0.7825)}{4.55pt}{4.82pt}{} & \HoloSegScore{0.3845}{(0.3066--0.4612)}{4.55pt}{4.82pt}{} & \HoloSegScore{0.7715}{(0.7316--0.8062)}{4.55pt}{4.82pt}{} & \HoloSegScore{0.7669}{(0.7236--0.8037)}{4.55pt}{4.82pt}{} & \HoloSegScore{0.8754}{(0.8502--0.8972)}{4.55pt}{4.82pt}{} & \HoloSegScore{0.8163}{(0.7990--0.8317)}{4.55pt}{4.82pt}{} & \HoloSegScore{0.8351}{(0.8176--0.8495)}{4.55pt}{4.82pt}{} \\*
\softcline{4-11}
 &  & \HoloSegSpan{\makecell[c]{colon}}{2.04cm}{0.32cm} & \HoloSegMetric{HD95} & \HoloSegScore{29.23}{(25.11--33.38)}{4.55pt}{4.82pt}{} & \HoloSegScore{43.23}{(34.60--53.47)}{4.55pt}{4.82pt}{} & \HoloSegScore{17.42}{(13.96--21.16)}{4.55pt}{4.82pt}{} & \HoloSegScore{27.79}{(23.78--32.04)}{4.55pt}{4.82pt}{} & \HoloSegScore{14.72}{(10.72--18.49)}{4.55pt}{4.82pt}{} & \HoloSegScore{22.12}{(17.97--27.24)}{4.55pt}{4.82pt}{} & \HoloSegScore{21.77}{(17.44--26.85)}{4.55pt}{4.82pt}{} \\
\cline{3-11}
 &  &  & \HoloSegMetric{Dice} &  & \HoloSegScore{0.3515}{(0.2814--0.4179)}{4.55pt}{4.82pt}{} & \HoloSegScore{0.8458}{(0.8276--0.8625)}{4.55pt}{4.82pt}{} & \HoloSegScore{0.6839}{(0.6589--0.7069)}{4.55pt}{4.82pt}{} & \HoloSegScore{0.8630}{(0.8469--0.8925)}{4.55pt}{4.82pt}{} & \HoloSegScore{0.8388}{(0.8275--0.8503)}{4.55pt}{4.82pt}{} & \HoloSegScore{0.8505}{(0.8383--0.8626)}{4.55pt}{4.82pt}{} \\*
\softcline{4-4}\softcline{6-11}
 &  & \HoloSegSpan{\makecell[c]{intestine}}{2.04cm}{0.32cm} & \HoloSegMetric{HD95} & \raisebox{0.32cm}[0pt][0pt]{\HoloSegUnsupported} & \HoloSegScore{58.43}{(43.30--75.63)}{4.55pt}{4.82pt}{} & \HoloSegScore{9.352}{(7.254--11.87)}{4.55pt}{4.82pt}{} & \HoloSegScore{41.62}{(36.79--47.07)}{4.55pt}{4.82pt}{} & \HoloSegScore{11.09}{(10.32--13.61)}{4.55pt}{4.82pt}{} & \HoloSegScore{11.89}{(9.730--14.54)}{4.55pt}{4.82pt}{} & \HoloSegScore{9.696}{(7.925--12.25)}{4.55pt}{4.82pt}{} \\
\cline{3-11}
 &  &  & \HoloSegMetric{Dice} & \HoloSegScore{0.01525}{(0.0000--0.04466)}{4.20pt}{4.48pt}{} & \HoloSegScore{0.002400}{(0.0000--0.007201)}{4.20pt}{4.48pt}{} & \HoloSegScore{0.01603}{(0.0000--0.04624)}{4.20pt}{4.48pt}{} & \HoloSegScore{0.01824}{(0.0000--0.05232)}{4.20pt}{4.48pt}{} & \HoloSegScore{0.7215}{(0.7087--0.7407)}{4.55pt}{4.82pt}{} & \HoloSegScore{0.6964}{(0.6529--0.7305)}{4.55pt}{4.82pt}{} & \HoloSegScore{0.7053}{(0.6625--0.7392)}{4.55pt}{4.82pt}{} \\*
\softcline{4-11}
 &  & \HoloSegSpan{\makecell[c]{left adrenal\\[-0.10ex]gland}}{2.04cm}{0.32cm} & \HoloSegMetric{HD95} & \HoloSegScore{71.57}{(68.15--74.92)}{4.55pt}{4.82pt}{} & \HoloSegScore{70.72}{(67.71--73.82)}{4.55pt}{4.82pt}{} & \HoloSegScore{70.32}{(66.90--73.90)}{4.55pt}{4.82pt}{} & \HoloSegScore{71.78}{(67.77--75.30)}{4.55pt}{4.82pt}{} & \HoloSegScore{8.610}{(6.440--12.11)}{4.55pt}{4.82pt}{} & \HoloSegScore{8.615}{(6.024--11.74)}{4.55pt}{4.82pt}{} & \HoloSegScore{9.519}{(6.009--13.69)}{4.55pt}{4.82pt}{} \\
\cline{3-11}
 &  &  & \HoloSegMetric{Dice} & \HoloSegScore{0.0000}{(0.0000--0.0000)}{4.55pt}{4.82pt}{} & \HoloSegScore{0.0000}{(0.0000--0.0000)}{4.55pt}{4.82pt}{} & \HoloSegScore{0.0000}{(0.0000--0.0000)}{4.55pt}{4.82pt}{} & \HoloSegScore{0.0000}{(0.0000--0.0000)}{4.55pt}{4.82pt}{} & \HoloSegScore{0.7193}{(0.7187--0.7233)}{4.55pt}{4.82pt}{} & \HoloSegScore{0.7152}{(0.6723--0.7527)}{4.55pt}{4.82pt}{} & \HoloSegScore{0.7072}{(0.6689--0.7409)}{4.55pt}{4.82pt}{} \\*
\softcline{4-11}
 &  & \HoloSegSpan{\makecell[c]{right\\[-0.10ex]adrenal\\[-0.10ex]gland}}{2.04cm}{0.32cm} & \HoloSegMetric{HD95} & \HoloSegScore{70.44}{(66.85--74.02)}{4.55pt}{4.82pt}{} & \HoloSegScore{70.94}{(65.53--78.46)}{4.55pt}{4.82pt}{} & \HoloSegScore{70.01}{(66.82--73.32)}{4.55pt}{4.82pt}{} & \HoloSegScore{70.49}{(66.92--73.99)}{4.55pt}{4.82pt}{} & \HoloSegScore{11.78}{(9.431--14.44)}{4.55pt}{4.82pt}{} & \HoloSegScore{7.578}{(5.391--10.34)}{4.55pt}{4.82pt}{} & \HoloSegScore{42.40}{(35.89--48.67)}{4.55pt}{4.82pt}{} \\
\cline{3-11}
 &  &  & \HoloSegMetric{Dice} &  & \HoloSegScore{0.1497}{(0.08999--0.2126)}{4.20pt}{4.48pt}{} & \HoloSegScore{0.7783}{(0.7403--0.8119)}{4.55pt}{4.82pt}{} & \HoloSegScore{0.7365}{(0.6982--0.7702)}{4.55pt}{4.82pt}{} & \HoloSegScore{0.8329}{(0.7934--0.8718)}{4.55pt}{4.82pt}{} & \HoloSegScore{0.8072}{(0.7896--0.8219)}{4.55pt}{4.82pt}{} & \HoloSegScore{0.8087}{(0.7921--0.8247)}{4.55pt}{4.82pt}{} \\*
\softcline{4-4}\softcline{6-11}
 &  & \HoloSegSpan{\makecell[c]{rectum}}{2.04cm}{0.32cm} & \HoloSegMetric{HD95} & \raisebox{0.32cm}[0pt][0pt]{\HoloSegUnsupported} & \HoloSegScore{55.81}{(37.81--79.58)}{4.55pt}{4.82pt}{} & \HoloSegScore{9.956}{(8.103--12.00)}{4.55pt}{4.82pt}{} & \HoloSegScore{16.37}{(12.93--20.08)}{4.55pt}{4.82pt}{} & \HoloSegScore{10.50}{(8.550--12.87)}{4.55pt}{4.82pt}{} & \HoloSegScore{16.14}{(10.09--26.96)}{4.55pt}{4.82pt}{} & \HoloSegScore{13.09}{(10.72--15.79)}{4.55pt}{4.82pt}{} \\
\cline{3-11}
 &  &  & \HoloSegMetric{Dice} & \HoloSegScore{0.8954}{(0.8245--0.9367)}{4.55pt}{4.82pt}{} & \HoloSegScore{0.5695}{(0.4928--0.6453)}{4.55pt}{4.82pt}{} & \HoloSegScore{0.9042}{(0.8380--0.9451)}{4.55pt}{4.82pt}{} & \HoloSegScore{0.8928}{(0.8215--0.9368)}{4.55pt}{4.82pt}{} & \HoloSegScore{0.9004}{(0.8574--0.9432)}{4.55pt}{4.82pt}{} & \HoloSegScore{0.9356}{(0.9184--0.9484)}{4.55pt}{4.82pt}{} & \HoloSegScore{0.9369}{(0.9186--0.9497)}{4.55pt}{4.82pt}{} \\*
\softcline{4-11}
 &  & \HoloSegSpan{\makecell[c]{urinary\\[-0.10ex]bladder}}{2.04cm}{0.32cm} & \HoloSegMetric{HD95} & \HoloSegScore{5.114}{(3.745--7.050)}{4.55pt}{4.82pt}{} & \HoloSegScore{23.86}{(17.65--32.51)}{4.55pt}{4.82pt}{} & \HoloSegScore{4.041}{(3.185--5.571)}{4.55pt}{4.82pt}{} & \HoloSegScore{5.695}{(3.991--7.951)}{4.55pt}{4.82pt}{} & \HoloSegScore{7.878}{(6.553--11.25)}{4.55pt}{4.82pt}{} & \HoloSegScore{5.819}{(3.046--9.718)}{4.55pt}{4.82pt}{} & \HoloSegScore{3.461}{(2.895--4.411)}{4.55pt}{4.82pt}{} \\
\cline{3-11}
 &  &  & \HoloSegMetric{Dice} &  & \HoloSegScore{0.6079}{(0.5587--0.6512)}{4.55pt}{4.82pt}{} & \HoloSegScore{0.9151}{(0.8953--0.9317)}{4.55pt}{4.82pt}{} & \HoloSegScore{0.9136}{(0.8943--0.9292)}{4.55pt}{4.82pt}{} & \HoloSegScore{0.8304}{(0.8046--0.8421)}{4.55pt}{4.82pt}{} & \HoloSegScore{0.9106}{(0.8969--0.9213)}{4.55pt}{4.82pt}{} & \HoloSegScore{0.9129}{(0.9005--0.9239)}{4.55pt}{4.82pt}{} \\*
\softcline{4-4}\softcline{6-11}
 &  & \HoloSegSpan{\makecell[c]{head of left\\[-0.10ex]femur}}{2.04cm}{0.32cm} & \HoloSegMetric{HD95} & \raisebox{0.32cm}[0pt][0pt]{\HoloSegUnsupported} & \HoloSegScore{62.66}{(46.11--82.92)}{4.55pt}{4.82pt}{} & \HoloSegScore{46.23}{(11.48--85.58)}{4.55pt}{4.82pt}{} & \HoloSegScore{9.496}{(6.699--13.27)}{4.55pt}{4.82pt}{} & \HoloSegScore{13.99}{(12.78--14.97)}{4.55pt}{4.82pt}{} & \HoloSegScore{13.84}{(7.138--25.02)}{4.55pt}{4.82pt}{} & \HoloSegScore{20.75}{(11.86--33.51)}{4.55pt}{4.82pt}{} \\
\hline
\pagebreak[4]
 &  &  & \HoloSegMetric{Dice} &  & \HoloSegScore{0.5986}{(0.5664--0.6284)}{4.55pt}{4.82pt}{} & \HoloSegScore{0.9209}{(0.9040--0.9342)}{4.55pt}{4.82pt}{} & \HoloSegScore{0.9136}{(0.8945--0.9282)}{4.55pt}{4.82pt}{} & \HoloSegScore{0.7018}{(0.6888--0.7365)}{4.55pt}{4.82pt}{} & \HoloSegScore{0.9118}{(0.8998--0.9233)}{4.55pt}{4.82pt}{} & \HoloSegScore{0.9150}{(0.9043--0.9245)}{4.55pt}{4.82pt}{} \\*
\softcline{4-4}\softcline{6-11}
 &  & \HoloSegSpan{\makecell[c]{head of\\[-0.10ex]right femur}}{2.04cm}{0.32cm} & \HoloSegMetric{HD95} & \raisebox{0.32cm}[0pt][0pt]{\HoloSegUnsupported} & \HoloSegScore{74.17}{(61.63--88.30)}{4.55pt}{4.82pt}{} & \HoloSegScore{6.826}{(4.622--9.580)}{4.55pt}{4.82pt}{} & \HoloSegScore{8.983}{(6.080--12.69)}{4.55pt}{4.82pt}{} & \HoloSegScore{17.04}{(15.10--19.35)}{4.55pt}{4.82pt}{} & \HoloSegScore{9.930}{(7.096--13.17)}{4.55pt}{4.82pt}{} & \HoloSegScore{13.10}{(6.734--24.08)}{4.55pt}{4.82pt}{} \\
\cline{3-11}
 &  &  & \HoloSegMetric{Dice} & \HoloSegScore{0.7673}{(0.7177--0.8065)}{4.55pt}{4.82pt}{} & \HoloSegScore{0.2085}{(0.1081--0.3163)}{4.55pt}{4.82pt}{} & \HoloSegScore{0.7353}{(0.6681--0.7862)}{4.55pt}{4.82pt}{} & \HoloSegScore{0.5378}{(0.4298--0.6341)}{4.55pt}{4.82pt}{} & \HoloSegScore{0.9290}{(0.8990--0.9703)}{4.55pt}{4.82pt}{} & \HoloSegScore{0.8348}{(0.8146--0.8524)}{4.55pt}{4.82pt}{} & \HoloSegScore{0.8129}{(0.7770--0.8421)}{4.55pt}{4.82pt}{} \\*
\softcline{4-11}
 & \HoloSegSpan{\makecell[c]{RAOS}}{1.86cm}{0.32cm} & \HoloSegSpan{\makecell[c]{prostate}}{2.04cm}{0.32cm} & \HoloSegMetric{HD95} & \HoloSegScore{7.388}{(2.587--13.25)}{4.55pt}{4.82pt}{} & \HoloSegScore{29.07}{(17.47--41.76)}{4.55pt}{4.82pt}{} & \HoloSegScore{6.835}{(5.780--8.072)}{4.55pt}{4.82pt}{} & \HoloSegScore{11.71}{(9.720--13.83)}{4.55pt}{4.82pt}{} & \HoloSegScore{6.866}{(5.423--8.651)}{4.55pt}{4.82pt}{} & \HoloSegScore{5.673}{(4.951--6.464)}{4.55pt}{4.82pt}{} & \HoloSegScore{34.36}{(18.55--55.45)}{4.55pt}{4.82pt}{} \\
\cline{3-11}
 &  &  & \HoloSegMetric{Dice} &  & \HoloSegScore{0.02716}{(0.002789--0.06138)}{3.85pt}{4.12pt}{} & \HoloSegScore{0.0000}{(0.0000--0.0000)}{4.55pt}{4.82pt}{} & \HoloSegScore{0.0000}{(0.0000--0.0000)}{4.55pt}{4.82pt}{} & \HoloSegScore{0.8400}{(0.8374--0.8475)}{4.55pt}{4.82pt}{} & \HoloSegScore{0.7599}{(0.7392--0.7789)}{4.55pt}{4.82pt}{} & \HoloSegScore{0.7818}{(0.7598--0.8013)}{4.55pt}{4.82pt}{} \\*
\softcline{4-4}\softcline{6-11}
 &  & \HoloSegSpan{\makecell[c]{seminal\\[-0.10ex]vesicles}}{2.04cm}{0.32cm} & \HoloSegMetric{HD95} & \raisebox{0.32cm}[0pt][0pt]{\HoloSegUnsupported} & \HoloSegScore{189.8}{(85.70--296.9)}{4.55pt}{4.82pt}{} & \HoloSegScore{237.8}{(210.1--269.0)}{4.55pt}{4.82pt}{} & \HoloSegScore{--}{(--\,--)}{4.55pt}{4.82pt}{} & \HoloSegScore{5.419}{(4.215--7.770)}{4.55pt}{4.82pt}{} & \HoloSegScore{6.569}{(5.599--7.540)}{4.55pt}{4.82pt}{} & \HoloSegScore{8.075}{(5.282--12.24)}{4.55pt}{4.82pt}{} \\
\cline{2-11}
 &  &  & \HoloSegMetric{Dice} &  & \HoloSegScore{0.0000}{(0.0000--0.0000)}{4.55pt}{4.82pt}{} & \HoloSegScore{0.08367}{(0.0000--0.1979)}{4.55pt}{4.82pt}{} & \HoloSegScore{0.5030}{(0.3032--0.6733)}{4.55pt}{4.82pt}{} & \HoloSegScore{0.8201}{(0.8127--0.8340)}{4.55pt}{4.82pt}{} & \HoloSegScore{0.3163}{(0.1163--0.4908)}{4.55pt}{4.82pt}{} & \HoloSegScore{0.5493}{(0.3747--0.7037)}{4.55pt}{4.82pt}{} \\*
\softcline{4-4}\softcline{6-11}
 & \HoloSegSpan{\makecell[c]{CT-ICH}}{1.86cm}{0.32cm} & \HoloSegSpan{\makecell[c]{intracranial\\[-0.10ex]hemorrhage}}{2.04cm}{0.32cm} & \HoloSegMetric{HD95} & \raisebox{0.32cm}[0pt][0pt]{\HoloSegUnsupported} & \HoloSegScore{122.8}{(100.2--145.4)}{4.55pt}{4.82pt}{} & \HoloSegScore{82.02}{(54.01--106.7)}{4.55pt}{4.82pt}{} & \HoloSegScore{33.98}{(13.57--54.43)}{4.55pt}{4.82pt}{} & \HoloSegScore{3.460}{(2.367--4.882)}{4.55pt}{4.82pt}{} & \HoloSegScore{47.93}{(27.41--69.88)}{4.55pt}{4.82pt}{} & \HoloSegScore{46.60}{(17.99--75.98)}{4.55pt}{4.82pt}{} \\
\cline{2-11}
 &  &  & \HoloSegMetric{Dice} &  & \HoloSegScore{0.01460}{(0.005448--0.02726)}{3.85pt}{4.12pt}{} & \HoloSegScore{0.0000}{(0.0000--0.0000)}{4.55pt}{4.82pt}{} & \HoloSegScore{0.2783}{(0.2171--0.3352)}{4.55pt}{4.82pt}{} & \HoloSegScore{0.7820}{(0.7806--0.7914)}{4.55pt}{4.82pt}{} & \HoloSegScore{0.5012}{(0.4340--0.5682)}{4.55pt}{4.82pt}{} & \HoloSegScore{0.4822}{(0.4106--0.5526)}{4.55pt}{4.82pt}{} \\*
\softcline{4-4}\softcline{6-11}
 & \HoloSegSpan{\makecell[c]{Mediastinal-\\[-0.10ex]Lymph-\\[-0.10ex]Node-SEG}}{1.86cm}{0.32cm} & \HoloSegSpan{\makecell[c]{mediastinal\\[-0.10ex]lymph node}}{2.04cm}{0.32cm} & \HoloSegMetric{HD95} & \raisebox{0.32cm}[0pt][0pt]{\HoloSegUnsupported} & \HoloSegScore{125.9}{(112.0--140.2)}{4.55pt}{4.82pt}{} & \HoloSegScore{158.7}{(157.0--160.3)}{4.55pt}{4.82pt}{} & \HoloSegScore{62.42}{(54.47--70.47)}{4.55pt}{4.82pt}{} & \HoloSegScore{11.67}{(9.630--15.04)}{4.55pt}{4.82pt}{} & \HoloSegScore{48.21}{(40.38--57.15)}{4.55pt}{4.82pt}{} & \HoloSegScore{35.92}{(30.22--41.89)}{4.55pt}{4.82pt}{} \\
\cline{2-11}
 &  &  & \HoloSegMetric{Dice} &  & \HoloSegScore{0.5845}{(0.4665--0.6773)}{4.55pt}{4.82pt}{} & \HoloSegScore{0.0000}{(0.0000--0.0000)}{4.55pt}{4.82pt}{} & \HoloSegScore{0.9024}{(0.8538--0.9378)}{4.55pt}{4.82pt}{} & \HoloSegScore{0.8171}{(0.7605--0.8559)}{4.55pt}{4.82pt}{} & \HoloSegScore{0.8811}{(0.8263--0.9214)}{4.55pt}{4.82pt}{} & \HoloSegScore{0.8795}{(0.8248--0.9217)}{4.55pt}{4.82pt}{} \\*
\softcline{4-4}\softcline{6-11}
 &  & \HoloSegSpan{\makecell[c]{bone}}{2.04cm}{0.32cm} & \HoloSegMetric{HD95} & \raisebox{0.32cm}[0pt][0pt]{\HoloSegUnsupported} & \HoloSegScore{112.8}{(68.89--156.8)}{4.55pt}{4.82pt}{} & \HoloSegScore{132.9}{(120.0--141.3)}{4.55pt}{4.82pt}{} & \HoloSegScore{11.05}{(1.767--22.89)}{4.55pt}{4.82pt}{} & \HoloSegScore{8.409}{(2.383--13.47)}{4.55pt}{4.82pt}{} & \HoloSegScore{8.229}{(2.000--14.52)}{4.55pt}{4.82pt}{} & \HoloSegScore{7.145}{(2.000--12.29)}{4.55pt}{4.82pt}{} \\
\cline{3-11}
 &  &  & \HoloSegMetric{Dice} & \HoloSegScore{0.9678}{(0.9628--0.9727)}{4.55pt}{4.82pt}{} & \HoloSegScore{0.9222}{(0.9191--0.9251)}{4.55pt}{4.82pt}{} & \HoloSegScore{0.9650}{(0.9598--0.9685)}{4.55pt}{4.82pt}{} & \HoloSegScore{0.9721}{(0.9681--0.9756)}{4.55pt}{4.82pt}{} & \HoloSegScore{0.9677}{(0.9569--0.9792)}{4.55pt}{4.82pt}{} & \HoloSegScore{0.9723}{(0.9688--0.9761)}{4.55pt}{4.82pt}{} & \HoloSegScore{0.9719}{(0.9679--0.9761)}{4.55pt}{4.82pt}{} \\*
\softcline{4-11}
 &  & \HoloSegSpan{\makecell[c]{liver}}{2.04cm}{0.32cm} & \HoloSegMetric{HD95} & \HoloSegScore{3.142}{(2.362--3.896)}{4.55pt}{4.82pt}{} & \HoloSegScore{7.052}{(5.940--8.419)}{4.55pt}{4.82pt}{} & \HoloSegScore{3.091}{(2.711--3.498)}{4.55pt}{4.82pt}{} & \HoloSegScore{2.740}{(1.902--3.886)}{4.55pt}{4.82pt}{} & \HoloSegScore{5.842}{(3.723--7.285)}{4.55pt}{4.82pt}{} & \HoloSegScore{2.468}{(1.957--2.978)}{4.55pt}{4.82pt}{} & \HoloSegScore{2.692}{(2.119--3.195)}{4.55pt}{4.82pt}{} \\
\cline{3-11}
 &  &  & \HoloSegMetric{Dice} & \HoloSegScore{0.4911}{(0.4250--0.5473)}{4.55pt}{4.82pt}{} & \HoloSegScore{0.2635}{(0.2221--0.2957)}{4.55pt}{4.82pt}{} & \HoloSegScore{0.4503}{(0.4146--0.4810)}{4.55pt}{4.82pt}{} & \HoloSegScore{0.5759}{(0.5259--0.6252)}{4.55pt}{4.82pt}{} & \HoloSegScore{0.4812}{(0.4343--0.5168)}{4.55pt}{4.82pt}{} & \HoloSegScore{0.5875}{(0.5317--0.6463)}{4.55pt}{4.82pt}{} & \HoloSegScore{0.6472}{(0.6025--0.6919)}{4.55pt}{4.82pt}{} \\*
\softcline{4-11}
 &  & \HoloSegSpan{\makecell[c]{portal vein\\[-0.10ex]and splenic\\[-0.10ex]vein}}{2.04cm}{0.32cm} & \HoloSegMetric{HD95} & \HoloSegScore{51.78}{(49.72--53.91)}{4.55pt}{4.82pt}{} & \HoloSegScore{42.12}{(35.64--48.35)}{4.55pt}{4.82pt}{} & \HoloSegScore{53.32}{(51.96--55.27)}{4.55pt}{4.82pt}{} & \HoloSegScore{43.72}{(37.14--51.50)}{4.55pt}{4.82pt}{} & \HoloSegScore{42.92}{(41.33--47.20)}{4.55pt}{4.82pt}{} & \HoloSegScore{33.90}{(26.05--45.64)}{4.55pt}{4.82pt}{} & \HoloSegScore{23.68}{(18.46--28.89)}{4.55pt}{4.82pt}{} \\
\cline{3-11}
 &  &  & \HoloSegMetric{Dice} & \HoloSegScore{0.7878}{(0.7393--0.8332)}{4.55pt}{4.82pt}{} & \HoloSegScore{0.7307}{(0.6808--0.7732)}{4.55pt}{4.82pt}{} & \HoloSegScore{0.7872}{(0.7315--0.8250)}{4.55pt}{4.82pt}{} & \HoloSegScore{0.7945}{(0.7518--0.8408)}{4.55pt}{4.82pt}{} & \HoloSegScore{0.7863}{(0.7468--0.8170)}{4.55pt}{4.82pt}{} & \HoloSegScore{0.8036}{(0.7584--0.8318)}{4.55pt}{4.82pt}{} & \HoloSegScore{0.8038}{(0.7523--0.8299)}{4.55pt}{4.82pt}{} \\*
\softcline{4-11}
 &  & \HoloSegSpan{\makecell[c]{aorta}}{2.04cm}{0.32cm} & \HoloSegMetric{HD95} & \HoloSegScore{53.17}{(48.02--60.93)}{4.55pt}{4.82pt}{} & \HoloSegScore{46.47}{(42.87--53.08)}{4.55pt}{4.82pt}{} & \HoloSegScore{47.76}{(43.01--56.13)}{4.55pt}{4.82pt}{} & \HoloSegScore{52.60}{(48.06--59.85)}{4.55pt}{4.82pt}{} & \HoloSegScore{47.15}{(44.49--54.07)}{4.55pt}{4.82pt}{} & \HoloSegScore{51.87}{(46.14--59.70)}{4.55pt}{4.82pt}{} & \HoloSegScore{51.79}{(46.03--59.57)}{4.55pt}{4.82pt}{} \\
\cline{3-11}
 &  &  & \HoloSegMetric{Dice} & \HoloSegScore{0.5198}{(0.2507--0.8050)}{4.55pt}{4.82pt}{} & \HoloSegScore{0.07503}{(0.0000--0.2251)}{4.55pt}{4.82pt}{} & \HoloSegScore{0.4454}{(0.02872--0.7456)}{4.20pt}{4.48pt}{} & \HoloSegScore{0.8311}{(0.7883--0.8941)}{4.55pt}{4.82pt}{} & \HoloSegScore{0.6983}{(0.6132--0.8362)}{4.55pt}{4.82pt}{} & \HoloSegScore{0.8194}{(0.7534--0.9027)}{4.55pt}{4.82pt}{} & \HoloSegScore{0.8457}{(0.8176--0.8923)}{4.55pt}{4.82pt}{} \\*
\softcline{4-11}
\HoloSegSpan{\makecell[c]{\textbf{Internal}}}{1.20cm}{0.32cm} &  & \HoloSegSpan{\makecell[c]{liver tumor}}{2.04cm}{0.32cm} & \HoloSegMetric{HD95} & \HoloSegScore{51.34}{(42.91--66.24)}{4.55pt}{4.82pt}{} & \HoloSegScore{97.45}{(66.08--113.3)}{4.55pt}{4.82pt}{} & \HoloSegScore{20.68}{(3.490--40.96)}{4.55pt}{4.82pt}{} & \HoloSegScore{43.37}{(1.600--93.57)}{4.55pt}{4.82pt}{} & \HoloSegScore{8.199}{(2.845--18.58)}{4.55pt}{4.82pt}{} & \HoloSegScore{2.973}{(1.600--4.644)}{4.55pt}{4.82pt}{} & \HoloSegScore{2.584}{(1.600--3.892)}{4.55pt}{4.82pt}{} \\
\cline{3-11}
 &  &  & \HoloSegMetric{Dice} &  & \HoloSegScore{0.5324}{(0.4392--0.5965)}{4.55pt}{4.82pt}{} & \HoloSegScore{0.0000}{(0.0000--0.0000)}{4.55pt}{4.82pt}{} & \HoloSegScore{0.7299}{(0.6719--0.7918)}{4.55pt}{4.82pt}{} & \HoloSegScore{0.7281}{(0.7268--0.7286)}{4.55pt}{4.82pt}{} & \HoloSegScore{0.6620}{(0.6524--0.6717)}{4.55pt}{4.82pt}{} & \HoloSegScore{0.6669}{(0.6051--0.7344)}{4.55pt}{4.82pt}{} \\*
\softcline{4-4}\softcline{6-11}
 &  & \HoloSegSpan{\makecell[c]{veins}}{2.04cm}{0.32cm} & \HoloSegMetric{HD95} & \raisebox{0.32cm}[0pt][0pt]{\HoloSegUnsupported} & \HoloSegScore{72.67}{(70.04--75.74)}{4.55pt}{4.82pt}{} & \HoloSegScore{--}{(--\,--)}{4.55pt}{4.82pt}{} & \HoloSegScore{29.36}{(12.11--57.09)}{4.55pt}{4.82pt}{} & \HoloSegScore{29.77}{(28.59--34.18)}{4.55pt}{4.82pt}{} & \HoloSegScore{49.66}{(26.73--65.78)}{4.55pt}{4.82pt}{} & \HoloSegScore{37.42}{(20.01--59.97)}{4.55pt}{4.82pt}{} \\
\cline{3-11}
 & \HoloSegSpan{\makecell[c]{3D-ircadb-\\[-0.10ex]01}}{1.86cm}{0.32cm} &  & \HoloSegMetric{Dice} & \HoloSegScore{0.5794}{(0.5794--0.5794)}{4.55pt}{4.82pt}{} & \HoloSegScore{0.5353}{(0.5353--0.5353)}{4.55pt}{4.82pt}{} & \HoloSegScore{0.5705}{(0.5705--0.5705)}{4.55pt}{4.82pt}{} & \HoloSegScore{0.6000}{(0.6000--0.6000)}{4.55pt}{4.82pt}{} & \HoloSegScore{0.5644}{(0.5575--0.5684)}{4.55pt}{4.82pt}{} & \HoloSegScore{0.5829}{(0.5829--0.5829)}{4.55pt}{4.82pt}{} & \HoloSegScore{0.5872}{(0.5872--0.5872)}{4.55pt}{4.82pt}{} \\*
\softcline{4-11}
 &  & \HoloSegSpan{\makecell[c]{inferior\\[-0.10ex]vena cava}}{2.04cm}{0.32cm} & \HoloSegMetric{HD95} & \HoloSegScore{76.57}{(76.57--76.57)}{4.55pt}{4.82pt}{} & \HoloSegScore{80.83}{(80.83--80.83)}{4.55pt}{4.82pt}{} & \HoloSegScore{83.67}{(83.67--83.67)}{4.55pt}{4.82pt}{} & \HoloSegScore{83.29}{(83.29--83.29)}{4.55pt}{4.82pt}{} & \HoloSegScore{78.05}{(78.05--78.83)}{4.55pt}{4.82pt}{} & \HoloSegScore{83.34}{(83.34--83.34)}{4.55pt}{4.82pt}{} & \HoloSegScore{84.85}{(84.85--84.85)}{4.55pt}{4.82pt}{} \\
\cline{3-11}
 &  &  & \HoloSegMetric{Dice} & \HoloSegScore{0.8815}{(0.8815--0.8815)}{4.55pt}{4.82pt}{} & \HoloSegScore{0.6900}{(0.6900--0.6900)}{4.55pt}{4.82pt}{} & \HoloSegScore{0.8776}{(0.8776--0.8776)}{4.55pt}{4.82pt}{} & \HoloSegScore{0.8965}{(0.8965--0.8965)}{4.55pt}{4.82pt}{} & \HoloSegScore{0.8789}{(0.8730--0.8968)}{4.55pt}{4.82pt}{} & \HoloSegScore{0.8867}{(0.8867--0.8867)}{4.55pt}{4.82pt}{} & \HoloSegScore{0.8943}{(0.8943--0.8943)}{4.55pt}{4.82pt}{} \\*
\softcline{4-11}
 &  & \HoloSegSpan{\makecell[c]{gallbladder}}{2.04cm}{0.32cm} & \HoloSegMetric{HD95} & \HoloSegScore{19.75}{(19.75--19.75)}{4.55pt}{4.82pt}{} & \HoloSegScore{14.16}{(14.16--14.16)}{4.55pt}{4.82pt}{} & \HoloSegScore{9.857}{(9.857--9.857)}{4.55pt}{4.82pt}{} & \HoloSegScore{24.64}{(24.64--24.64)}{4.55pt}{4.82pt}{} & \HoloSegScore{14.57}{(14.08--15.08)}{4.55pt}{4.82pt}{} & \HoloSegScore{25.25}{(25.25--25.25)}{4.55pt}{4.82pt}{} & \HoloSegScore{25.01}{(25.01--25.01)}{4.55pt}{4.82pt}{} \\
\cline{3-11}
 &  &  & \HoloSegMetric{Dice} & \HoloSegScore{0.9628}{(0.9628--0.9628)}{4.55pt}{4.82pt}{} & \HoloSegScore{0.9042}{(0.9042--0.9042)}{4.55pt}{4.82pt}{} & \HoloSegScore{0.9499}{(0.9499--0.9499)}{4.55pt}{4.82pt}{} & \HoloSegScore{0.9683}{(0.9683--0.9683)}{4.55pt}{4.82pt}{} & \HoloSegScore{0.9502}{(0.9488--0.9511)}{4.55pt}{4.82pt}{} & \HoloSegScore{0.9592}{(0.9592--0.9592)}{4.55pt}{4.82pt}{} & \HoloSegScore{0.9683}{(0.9683--0.9683)}{4.55pt}{4.82pt}{} \\*
\softcline{4-11}
 &  & \HoloSegSpan{\makecell[c]{left kidney}}{2.04cm}{0.32cm} & \HoloSegMetric{HD95} & \HoloSegScore{1.600}{(1.600--1.600)}{4.55pt}{4.82pt}{} & \HoloSegScore{3.927}{(3.927--3.927)}{4.55pt}{4.82pt}{} & \HoloSegScore{1.755}{(1.755--1.755)}{4.55pt}{4.82pt}{} & \HoloSegScore{1.440}{(1.440--1.440)}{4.55pt}{4.82pt}{} & \HoloSegScore{2.050}{(1.601--3.018)}{4.55pt}{4.82pt}{} & \HoloSegScore{1.610}{(1.610--1.610)}{4.55pt}{4.82pt}{} & \HoloSegScore{1.610}{(1.610--1.610)}{4.55pt}{4.82pt}{} \\
\cline{3-11}
 &  &  & \HoloSegMetric{Dice} & \HoloSegScore{0.9601}{(0.9601--0.9601)}{4.55pt}{4.82pt}{} & \HoloSegScore{0.8177}{(0.8177--0.8177)}{4.55pt}{4.82pt}{} & \HoloSegScore{0.9509}{(0.9509--0.9509)}{4.55pt}{4.82pt}{} & \HoloSegScore{0.9705}{(0.9705--0.9705)}{4.55pt}{4.82pt}{} & \HoloSegScore{0.9538}{(0.9385--0.9619)}{4.55pt}{4.82pt}{} & \HoloSegScore{0.9672}{(0.9672--0.9672)}{4.55pt}{4.82pt}{} & \HoloSegScore{0.9674}{(0.9674--0.9674)}{4.55pt}{4.82pt}{} \\*
\softcline{4-11}
 &  & \HoloSegSpan{\makecell[c]{right kidney}}{2.04cm}{0.32cm} & \HoloSegMetric{HD95} & \HoloSegScore{1.610}{(1.610--1.610)}{4.55pt}{4.82pt}{} & \HoloSegScore{117.9}{(117.9--117.9)}{4.55pt}{4.82pt}{} & \HoloSegScore{1.755}{(1.755--1.755)}{4.55pt}{4.82pt}{} & \HoloSegScore{1.600}{(1.600--1.600)}{4.55pt}{4.82pt}{} & \HoloSegScore{2.339}{(1.620--2.775)}{4.55pt}{4.82pt}{} & \HoloSegScore{3.200}{(3.200--3.200)}{4.55pt}{4.82pt}{} & \HoloSegScore{1.897}{(1.897--1.897)}{4.55pt}{4.82pt}{} \\
\cline{3-11}
 &  &  & \HoloSegMetric{Dice} & \HoloSegScore{0.8121}{(0.8121--0.8121)}{4.55pt}{4.82pt}{} & \HoloSegScore{0.5377}{(0.5377--0.5377)}{4.55pt}{4.82pt}{} & \HoloSegScore{0.8138}{(0.8138--0.8138)}{4.55pt}{4.82pt}{} & \HoloSegScore{0.8982}{(0.8982--0.8982)}{4.55pt}{4.82pt}{} & \HoloSegScore{0.7860}{(0.7815--0.7896)}{4.55pt}{4.82pt}{} & \HoloSegScore{0.8941}{(0.8941--0.8941)}{4.55pt}{4.82pt}{} & \HoloSegScore{0.9046}{(0.9046--0.9046)}{4.55pt}{4.82pt}{} \\*
\softcline{4-11}
 &  & \HoloSegSpan{\makecell[c]{left adrenal\\[-0.10ex]gland}}{2.04cm}{0.32cm} & \HoloSegMetric{HD95} & \HoloSegScore{1.755}{(1.755--1.755)}{4.55pt}{4.82pt}{} & \HoloSegScore{11.06}{(11.06--11.06)}{4.55pt}{4.82pt}{} & \HoloSegScore{1.610}{(1.610--1.610)}{4.55pt}{4.82pt}{} & \HoloSegScore{0.7200}{(0.7200--0.7200)}{4.55pt}{4.82pt}{} & \HoloSegScore{3.289}{(3.089--3.314)}{4.55pt}{4.82pt}{} & \HoloSegScore{1.440}{(1.440--1.440)}{4.55pt}{4.82pt}{} & \HoloSegScore{0.7200}{(0.7200--0.7200)}{4.55pt}{4.82pt}{} \\
\cline{3-11}
 &  &  & \HoloSegMetric{Dice} & \HoloSegScore{0.8104}{(0.8104--0.8104)}{4.55pt}{4.82pt}{} & \HoloSegScore{0.4224}{(0.4224--0.4224)}{4.55pt}{4.82pt}{} & \HoloSegScore{0.8088}{(0.8088--0.8088)}{4.55pt}{4.82pt}{} & \HoloSegScore{0.8991}{(0.8991--0.8991)}{4.55pt}{4.82pt}{} & \HoloSegScore{0.8751}{(0.8606--0.8787)}{4.55pt}{4.82pt}{} & \HoloSegScore{0.8440}{(0.8440--0.8440)}{4.55pt}{4.82pt}{} & \HoloSegScore{0.8821}{(0.8821--0.8821)}{4.55pt}{4.82pt}{} \\*
\softcline{4-11}
 &  & \HoloSegSpan{\makecell[c]{right\\[-0.10ex]adrenal\\[-0.10ex]gland}}{2.04cm}{0.32cm} & \HoloSegMetric{HD95} & \HoloSegScore{2.270}{(2.270--2.270)}{4.55pt}{4.82pt}{} & \HoloSegScore{14.57}{(14.57--14.57)}{4.55pt}{4.82pt}{} & \HoloSegScore{1.610}{(1.610--1.610)}{4.55pt}{4.82pt}{} & \HoloSegScore{0.7200}{(0.7200--0.7200)}{4.55pt}{4.82pt}{} & \HoloSegScore{3.140}{(1.665--3.158)}{4.55pt}{4.82pt}{} & \HoloSegScore{2.270}{(2.270--2.270)}{4.55pt}{4.82pt}{} & \HoloSegScore{1.018}{(1.018--1.018)}{4.55pt}{4.82pt}{} \\
\cline{2-11}
 &  &  & \HoloSegMetric{Dice} & \HoloSegScore{0.9472}{(0.9369--0.9566)}{4.55pt}{4.82pt}{} & \HoloSegScore{0.6152}{(0.5479--0.6779)}{4.55pt}{4.82pt}{} & \HoloSegScore{0.9538}{(0.9436--0.9619)}{4.55pt}{4.82pt}{} & \HoloSegScore{0.9546}{(0.9443--0.9643)}{4.55pt}{4.82pt}{} & \HoloSegScore{0.9392}{(0.9296--0.9462)}{4.55pt}{4.82pt}{} & \HoloSegScore{0.9543}{(0.9440--0.9634)}{4.55pt}{4.82pt}{} & \HoloSegScore{0.9556}{(0.9453--0.9647)}{4.55pt}{4.82pt}{} \\*
\softcline{4-11}
 &  & \HoloSegSpan{\makecell[c]{lung}}{2.04cm}{0.32cm} & \HoloSegMetric{HD95} & \HoloSegScore{49.72}{(30.58--71.65)}{4.55pt}{4.82pt}{} & \HoloSegScore{51.88}{(38.96--64.97)}{4.55pt}{4.82pt}{} & \HoloSegScore{5.690}{(3.152--9.277)}{4.55pt}{4.82pt}{} & \HoloSegScore{6.630}{(4.998--8.923)}{4.55pt}{4.82pt}{} & \HoloSegScore{5.714}{(3.814--7.182)}{4.55pt}{4.82pt}{} & \HoloSegScore{5.979}{(3.594--9.650)}{4.55pt}{4.82pt}{} & \HoloSegScore{4.318}{(3.693--4.981)}{4.55pt}{4.82pt}{} \\
\cline{3-11}
 & \HoloSegSpan{\makecell[c]{NSCLC-\\[-0.10ex]Radiogenomics}}{1.86cm}{0.32cm} &  & \HoloSegMetric{Dice} & \HoloSegScore{0.4320}{(0.2977--0.5661)}{4.55pt}{4.82pt}{} & \HoloSegScore{0.02529}{(0.0000--0.07588)}{4.20pt}{4.48pt}{} & \HoloSegScore{0.3483}{(0.2092--0.4943)}{4.55pt}{4.82pt}{} & \HoloSegScore{0.5581}{(0.4313--0.6751)}{4.55pt}{4.82pt}{} & \HoloSegScore{0.6351}{(0.6127--0.6894)}{4.55pt}{4.82pt}{} & \HoloSegScore{0.5554}{(0.4137--0.6900)}{4.55pt}{4.82pt}{} & \HoloSegScore{0.5672}{(0.4249--0.6971)}{4.55pt}{4.82pt}{} \\*
\softcline{4-11}
 &  & \HoloSegSpan{\makecell[c]{pulmonary\\[-0.10ex]nodule}}{2.04cm}{0.32cm} & \HoloSegMetric{HD95} & \HoloSegScore{93.74}{(66.38--121.2)}{4.55pt}{4.82pt}{} & \HoloSegScore{155.6}{(131.4--180.8)}{4.55pt}{4.82pt}{} & \HoloSegScore{99.94}{(62.40--135.3)}{4.55pt}{4.82pt}{} & \HoloSegScore{112.2}{(77.67--147.0)}{4.55pt}{4.82pt}{} & \HoloSegScore{94.37}{(66.66--121.9)}{4.55pt}{4.82pt}{} & \HoloSegScore{105.8}{(74.06--140.6)}{4.55pt}{4.82pt}{} & \HoloSegScore{104.2}{(68.58--139.1)}{4.55pt}{4.82pt}{} \\
\hline
\pagebreak[4]
 &  &  & \HoloSegMetric{Dice} & \HoloSegScore{0.3638}{(0.2777--0.4394)}{4.55pt}{4.82pt}{} & \HoloSegScore{0.02776}{(0.0000--0.07949)}{4.20pt}{4.48pt}{} & \HoloSegScore{0.3917}{(0.2764--0.5044)}{4.55pt}{4.82pt}{} & \HoloSegScore{0.5069}{(0.4106--0.5937)}{4.55pt}{4.82pt}{} & \HoloSegScore{0.6019}{(0.5772--0.6640)}{4.55pt}{4.82pt}{} & \HoloSegScore{0.5040}{(0.3922--0.6015)}{4.55pt}{4.82pt}{} & \HoloSegScore{0.5293}{(0.4267--0.6226)}{4.55pt}{4.82pt}{} \\*
\softcline{4-11}
 & \HoloSegSpan{\makecell[c]{NSCLC-\\[-0.10ex]Radiogenomics}}{1.86cm}{0.32cm} & \HoloSegSpan{\makecell[c]{lung tumor}}{2.04cm}{0.32cm} & \HoloSegMetric{HD95} & \HoloSegScore{34.78}{(31.30--38.29)}{4.55pt}{4.82pt}{} & \HoloSegScore{205.8}{(158.6--256.4)}{4.55pt}{4.82pt}{} & \HoloSegScore{127.2}{(77.62--181.4)}{4.55pt}{4.82pt}{} & \HoloSegScore{92.41}{(58.31--134.8)}{4.55pt}{4.82pt}{} & \HoloSegScore{45.15}{(28.48--64.70)}{4.55pt}{4.82pt}{} & \HoloSegScore{61.82}{(32.35--98.13)}{4.55pt}{4.82pt}{} & \HoloSegScore{48.41}{(27.87--71.93)}{4.55pt}{4.82pt}{} \\
\cline{2-11}
 &  &  & \HoloSegMetric{Dice} & \HoloSegScore{0.4541}{(0.4300--0.4766)}{4.55pt}{4.82pt}{} & \HoloSegScore{0.7624}{(0.7530--0.7707)}{4.55pt}{4.82pt}{} & \HoloSegScore{0.4356}{(0.4122--0.4581)}{4.55pt}{4.82pt}{} & \HoloSegScore{0.6878}{(0.6647--0.7086)}{4.55pt}{4.82pt}{} & \HoloSegScore{0.8252}{(0.8185--0.8280)}{4.55pt}{4.82pt}{} & \HoloSegScore{0.8672}{(0.8607--0.8740)}{4.55pt}{4.82pt}{} & \HoloSegScore{0.8734}{(0.8673--0.8800)}{4.55pt}{4.82pt}{} \\*
\softcline{4-11}
 &  & \HoloSegSpan{\makecell[c]{aorta}}{2.04cm}{0.32cm} & \HoloSegMetric{HD95} & \HoloSegScore{39.06}{(36.21--42.56)}{4.55pt}{4.82pt}{} & \HoloSegScore{11.29}{(10.18--12.39)}{4.55pt}{4.82pt}{} & \HoloSegScore{42.40}{(38.88--46.10)}{4.55pt}{4.82pt}{} & \HoloSegScore{24.16}{(21.97--26.45)}{4.55pt}{4.82pt}{} & \HoloSegScore{10.55}{(9.339--12.25)}{4.55pt}{4.82pt}{} & \HoloSegScore{12.45}{(11.18--13.63)}{4.55pt}{4.82pt}{} & \HoloSegScore{10.92}{(9.794--12.05)}{4.55pt}{4.82pt}{} \\
\cline{3-11}
 &  &  & \HoloSegMetric{Dice} & \HoloSegScore{0.3369}{(0.3133--0.3618)}{4.55pt}{4.82pt}{} & \HoloSegScore{0.7009}{(0.6881--0.7124)}{4.55pt}{4.82pt}{} & \HoloSegScore{0.3534}{(0.3311--0.3762)}{4.55pt}{4.82pt}{} & \HoloSegScore{0.4062}{(0.3802--0.4316)}{4.55pt}{4.82pt}{} & \HoloSegScore{0.7823}{(0.7732--0.7851)}{4.55pt}{4.82pt}{} & \HoloSegScore{0.7711}{(0.7603--0.7809)}{4.55pt}{4.82pt}{} & \HoloSegScore{0.7961}{(0.7867--0.8050)}{4.55pt}{4.82pt}{} \\*
\softcline{4-11}
 &  & \HoloSegSpan{\makecell[c]{inferior\\[-0.10ex]vena cava}}{2.04cm}{0.32cm} & \HoloSegMetric{HD95} & \HoloSegScore{44.18}{(40.76--47.49)}{4.55pt}{4.82pt}{} & \HoloSegScore{15.35}{(13.83--17.09)}{4.55pt}{4.82pt}{} & \HoloSegScore{43.68}{(39.94--47.21)}{4.55pt}{4.82pt}{} & \HoloSegScore{36.38}{(34.11--38.92)}{4.55pt}{4.82pt}{} & \HoloSegScore{15.07}{(14.41--17.10)}{4.55pt}{4.82pt}{} & \HoloSegScore{16.15}{(14.47--17.86)}{4.55pt}{4.82pt}{} & \HoloSegScore{15.16}{(13.53--16.94)}{4.55pt}{4.82pt}{} \\
\cline{3-11}
 &  &  & \HoloSegMetric{Dice} & \HoloSegScore{0.6077}{(0.5863--0.6305)}{4.55pt}{4.82pt}{} & \HoloSegScore{0.8984}{(0.8939--0.9029)}{4.55pt}{4.82pt}{} & \HoloSegScore{0.6115}{(0.5912--0.6320)}{4.55pt}{4.82pt}{} & \HoloSegScore{0.7486}{(0.7267--0.7695)}{4.55pt}{4.82pt}{} & \HoloSegScore{0.9346}{(0.9340--0.9387)}{4.55pt}{4.82pt}{} & \HoloSegScore{0.9487}{(0.9445--0.9527)}{4.55pt}{4.82pt}{} & \HoloSegScore{0.9505}{(0.9469--0.9538)}{4.55pt}{4.82pt}{} \\*
\softcline{4-11}
 &  & \HoloSegSpan{\makecell[c]{liver}}{2.04cm}{0.32cm} & \HoloSegMetric{HD95} & \HoloSegScore{55.10}{(52.10--58.02)}{4.55pt}{4.82pt}{} & \HoloSegScore{4.960}{(4.622--5.374)}{4.55pt}{4.82pt}{} & \HoloSegScore{51.67}{(48.93--54.40)}{4.55pt}{4.82pt}{} & \HoloSegScore{47.70}{(44.42--50.80)}{4.55pt}{4.82pt}{} & \HoloSegScore{6.835}{(6.480--6.978)}{4.55pt}{4.82pt}{} & \HoloSegScore{6.905}{(6.224--7.635)}{4.55pt}{4.82pt}{} & \HoloSegScore{6.792}{(6.112--7.579)}{4.55pt}{4.82pt}{} \\
\cline{3-11}
 &  &  & \HoloSegMetric{Dice} & \HoloSegScore{0.3325}{(0.3088--0.3542)}{4.55pt}{4.82pt}{} & \HoloSegScore{0.7145}{(0.6999--0.7290)}{4.55pt}{4.82pt}{} & \HoloSegScore{0.2082}{(0.1887--0.2285)}{4.55pt}{4.82pt}{} & \HoloSegScore{0.6270}{(0.6031--0.6500)}{4.55pt}{4.82pt}{} & \HoloSegScore{0.8181}{(0.8083--0.8185)}{4.55pt}{4.82pt}{} & \HoloSegScore{0.7996}{(0.7863--0.8115)}{4.55pt}{4.82pt}{} & \HoloSegScore{0.8022}{(0.7907--0.8141)}{4.55pt}{4.82pt}{} \\*
\softcline{4-11}
 &  & \HoloSegSpan{\makecell[c]{stomach}}{2.04cm}{0.32cm} & \HoloSegMetric{HD95} & \HoloSegScore{67.03}{(63.01--71.02)}{4.55pt}{4.82pt}{} & \HoloSegScore{15.68}{(13.78--17.67)}{4.55pt}{4.82pt}{} & \HoloSegScore{95.60}{(91.47--99.96)}{4.55pt}{4.82pt}{} & \HoloSegScore{43.62}{(40.19--47.28)}{4.55pt}{4.82pt}{} & \HoloSegScore{16.83}{(15.88--17.49)}{4.55pt}{4.82pt}{} & \HoloSegScore{15.18}{(13.86--16.64)}{4.55pt}{4.82pt}{} & \HoloSegScore{15.81}{(14.38--17.34)}{4.55pt}{4.82pt}{} \\
\cline{3-11}
 &  &  & \HoloSegMetric{Dice} & \HoloSegScore{0.5691}{(0.5525--0.5863)}{4.55pt}{4.82pt}{} & \HoloSegScore{0.2119}{(0.1953--0.2293)}{4.55pt}{4.82pt}{} & \HoloSegScore{0.4808}{(0.4648--0.4979)}{4.55pt}{4.82pt}{} & \HoloSegScore{0.6438}{(0.6261--0.6615)}{4.55pt}{4.82pt}{} & \HoloSegScore{0.7847}{(0.7743--0.7968)}{4.55pt}{4.82pt}{} & \HoloSegScore{0.7601}{(0.7502--0.7698)}{4.55pt}{4.82pt}{} & \HoloSegScore{0.7866}{(0.7779--0.7952)}{4.55pt}{4.82pt}{} \\*
\softcline{4-11}
 &  & \HoloSegSpan{\makecell[c]{colon}}{2.04cm}{0.32cm} & \HoloSegMetric{HD95} & \HoloSegScore{37.37}{(35.34--39.56)}{4.55pt}{4.82pt}{} & \HoloSegScore{67.36}{(64.38--70.47)}{4.55pt}{4.82pt}{} & \HoloSegScore{36.46}{(34.39--38.51)}{4.55pt}{4.82pt}{} & \HoloSegScore{36.61}{(34.12--39.06)}{4.55pt}{4.82pt}{} & \HoloSegScore{18.36}{(17.68--20.25)}{4.55pt}{4.82pt}{} & \HoloSegScore{18.40}{(16.85--20.04)}{4.55pt}{4.82pt}{} & \HoloSegScore{16.58}{(15.23--18.03)}{4.55pt}{4.82pt}{} \\
\cline{3-11}
 &  &  & \HoloSegMetric{Dice} & \HoloSegScore{0.3535}{(0.3274--0.3793)}{4.55pt}{4.82pt}{} & \HoloSegScore{0.7908}{(0.7746--0.8069)}{4.55pt}{4.82pt}{} & \HoloSegScore{0.3660}{(0.3407--0.3921)}{4.55pt}{4.82pt}{} & \HoloSegScore{0.4576}{(0.4257--0.4888)}{4.55pt}{4.82pt}{} & \HoloSegScore{0.8913}{(0.8658--0.8949)}{4.55pt}{4.82pt}{} & \HoloSegScore{0.9276}{(0.9168--0.9374)}{4.55pt}{4.82pt}{} & \HoloSegScore{0.9306}{(0.9207--0.9398)}{4.55pt}{4.82pt}{} \\*
\softcline{4-11}
 &  & \HoloSegSpan{\makecell[c]{right lung}}{2.04cm}{0.32cm} & \HoloSegMetric{HD95} & \HoloSegScore{71.01}{(66.95--74.93)}{4.55pt}{4.82pt}{} & \HoloSegScore{20.09}{(17.71--22.62)}{4.55pt}{4.82pt}{} & \HoloSegScore{73.88}{(70.05--77.68)}{4.55pt}{4.82pt}{} & \HoloSegScore{70.62}{(65.90--75.58)}{4.55pt}{4.82pt}{} & \HoloSegScore{10.03}{(9.038--11.11)}{4.55pt}{4.82pt}{} & \HoloSegScore{11.60}{(9.775--13.55)}{4.55pt}{4.82pt}{} & \HoloSegScore{10.90}{(9.086--12.76)}{4.55pt}{4.82pt}{} \\
\cline{3-11}
 &  &  & \HoloSegMetric{Dice} & \HoloSegScore{0.3674}{(0.3403--0.3951)}{4.55pt}{4.82pt}{} & \HoloSegScore{0.7780}{(0.7612--0.7935)}{4.55pt}{4.82pt}{} & \HoloSegScore{0.3600}{(0.3352--0.3870)}{4.55pt}{4.82pt}{} & \HoloSegScore{0.4539}{(0.4228--0.4830)}{4.55pt}{4.82pt}{} & \HoloSegScore{0.8742}{(0.8643--0.8856)}{4.55pt}{4.82pt}{} & \HoloSegScore{0.8983}{(0.8862--0.9103)}{4.55pt}{4.82pt}{} & \HoloSegScore{0.8996}{(0.8876--0.9111)}{4.55pt}{4.82pt}{} \\*
\softcline{4-11}
 &  & \HoloSegSpan{\makecell[c]{left lung}}{2.04cm}{0.32cm} & \HoloSegMetric{HD95} & \HoloSegScore{84.98}{(80.72--89.18)}{4.55pt}{4.82pt}{} & \HoloSegScore{23.14}{(20.44--25.63)}{4.55pt}{4.82pt}{} & \HoloSegScore{88.28}{(84.45--92.56)}{4.55pt}{4.82pt}{} & \HoloSegScore{78.85}{(73.80--83.99)}{4.55pt}{4.82pt}{} & \HoloSegScore{15.52}{(14.19--17.68)}{4.55pt}{4.82pt}{} & \HoloSegScore{17.18}{(14.96--19.70)}{4.55pt}{4.82pt}{} & \HoloSegScore{13.45}{(11.06--15.90)}{4.55pt}{4.82pt}{} \\
\cline{3-11}
 &  &  & \HoloSegMetric{Dice} & \HoloSegScore{0.3120}{(0.2916--0.3341)}{4.55pt}{4.82pt}{} & \HoloSegScore{0.6155}{(0.6051--0.6258)}{4.55pt}{4.82pt}{} & \HoloSegScore{0.2678}{(0.2488--0.2873)}{4.55pt}{4.82pt}{} & \HoloSegScore{0.6739}{(0.6565--0.6903)}{4.55pt}{4.82pt}{} & \HoloSegScore{0.7548}{(0.7394--0.7604)}{4.55pt}{4.82pt}{} & \HoloSegScore{0.7709}{(0.7628--0.7802)}{4.55pt}{4.82pt}{} & \HoloSegScore{0.7892}{(0.7814--0.7976)}{4.55pt}{4.82pt}{} \\*
\softcline{4-11}
 &  & \HoloSegSpan{\makecell[c]{pancreas}}{2.04cm}{0.32cm} & \HoloSegMetric{HD95} & \HoloSegScore{50.85}{(47.33--54.15)}{4.55pt}{4.82pt}{} & \HoloSegScore{11.94}{(10.63--13.38)}{4.55pt}{4.82pt}{} & \HoloSegScore{52.76}{(49.66--56.11)}{4.55pt}{4.82pt}{} & \HoloSegScore{18.11}{(16.57--19.72)}{4.55pt}{4.82pt}{} & \HoloSegScore{8.055}{(8.010--8.980)}{4.55pt}{4.82pt}{} & \HoloSegScore{9.050}{(8.101--10.10)}{4.55pt}{4.82pt}{} & \HoloSegScore{8.815}{(7.881--9.832)}{4.55pt}{4.82pt}{} \\
\cline{3-11}
 &  &  & \HoloSegMetric{Dice} &  & \HoloSegScore{0.008733}{(0.006887--0.01088)}{3.85pt}{4.12pt}{} & \HoloSegScore{0.2638}{(0.2334--0.2947)}{4.55pt}{4.82pt}{} & \HoloSegScore{0.3386}{(0.3039--0.3726)}{4.55pt}{4.82pt}{} & \HoloSegScore{0.6376}{(0.6281--0.6465)}{4.55pt}{4.82pt}{} & \HoloSegScore{0.6529}{(0.6425--0.6633)}{4.55pt}{4.82pt}{} & \HoloSegScore{0.6825}{(0.6723--0.6923)}{4.55pt}{4.82pt}{} \\*
\softcline{4-4}\softcline{6-11}
\HoloSegSpan{\makecell[c]{\textbf{Internal}}}{1.20cm}{0.32cm} &  & \HoloSegSpan{\makecell[c]{veins}}{2.04cm}{0.32cm} & \HoloSegMetric{HD95} & \raisebox{0.32cm}[0pt][0pt]{\HoloSegUnsupported} & \HoloSegScore{62.92}{(61.64--64.21)}{4.55pt}{4.82pt}{} & \HoloSegScore{76.27}{(58.92--92.89)}{4.55pt}{4.82pt}{} & \HoloSegScore{54.28}{(52.44--56.14)}{4.55pt}{4.82pt}{} & \HoloSegScore{18.35}{(17.32--19.29)}{4.55pt}{4.82pt}{} & \HoloSegScore{18.26}{(17.21--19.31)}{4.55pt}{4.82pt}{} & \HoloSegScore{15.13}{(14.14--16.10)}{4.55pt}{4.82pt}{} \\
\cline{3-11}
 & \HoloSegSpan{\makecell[c]{PanTS}}{1.86cm}{0.32cm} &  & \HoloSegMetric{Dice} & \HoloSegScore{0.1957}{(0.1782--0.2141)}{4.55pt}{4.82pt}{} & \HoloSegScore{0.3739}{(0.3607--0.3864)}{4.55pt}{4.82pt}{} & \HoloSegScore{0.1447}{(0.1283--0.1617)}{4.55pt}{4.82pt}{} & \HoloSegScore{0.3238}{(0.2989--0.3461)}{4.55pt}{4.82pt}{} & \HoloSegScore{0.5824}{(0.5626--0.5921)}{4.55pt}{4.82pt}{} & \HoloSegScore{0.6659}{(0.6543--0.6768)}{4.55pt}{4.82pt}{} & \HoloSegScore{0.7012}{(0.6920--0.7095)}{4.55pt}{4.82pt}{} \\*
\softcline{4-11}
 &  & \HoloSegSpan{\makecell[c]{right\\[-0.10ex]adrenal\\[-0.10ex]gland}}{2.04cm}{0.32cm} & \HoloSegMetric{HD95} & \HoloSegScore{28.82}{(26.04--31.51)}{4.55pt}{4.82pt}{} & \HoloSegScore{15.39}{(13.83--17.10)}{4.55pt}{4.82pt}{} & \HoloSegScore{30.33}{(26.52--33.99)}{4.55pt}{4.82pt}{} & \HoloSegScore{32.12}{(29.50--34.83)}{4.55pt}{4.82pt}{} & \HoloSegScore{5.974}{(5.225--6.720)}{4.55pt}{4.82pt}{} & \HoloSegScore{10.81}{(9.769--11.98)}{4.55pt}{4.82pt}{} & \HoloSegScore{4.553}{(4.201--4.928)}{4.55pt}{4.82pt}{} \\
\cline{3-11}
 &  &  & \HoloSegMetric{Dice} & \HoloSegScore{0.2378}{(0.2205--0.2551)}{4.55pt}{4.82pt}{} & \HoloSegScore{0.4751}{(0.4628--0.4867)}{4.55pt}{4.82pt}{} & \HoloSegScore{0.1855}{(0.1695--0.2010)}{4.55pt}{4.82pt}{} & \HoloSegScore{0.4623}{(0.4403--0.4820)}{4.55pt}{4.82pt}{} & \HoloSegScore{0.7457}{(0.7449--0.7597)}{4.55pt}{4.82pt}{} & \HoloSegScore{0.6729}{(0.6620--0.6831)}{4.55pt}{4.82pt}{} & \HoloSegScore{0.7310}{(0.7221--0.7398)}{4.55pt}{4.82pt}{} \\*
\softcline{4-11}
 &  & \HoloSegSpan{\makecell[c]{duodenum}}{2.04cm}{0.32cm} & \HoloSegMetric{HD95} & \HoloSegScore{45.45}{(42.49--48.54)}{4.55pt}{4.82pt}{} & \HoloSegScore{18.66}{(17.49--19.84)}{4.55pt}{4.82pt}{} & \HoloSegScore{55.11}{(51.06--58.75)}{4.55pt}{4.82pt}{} & \HoloSegScore{28.09}{(26.25--30.01)}{4.55pt}{4.82pt}{} & \HoloSegScore{10.83}{(9.180--12.07)}{4.55pt}{4.82pt}{} & \HoloSegScore{13.19}{(12.50--14.07)}{4.55pt}{4.82pt}{} & \HoloSegScore{10.50}{(9.851--11.26)}{4.55pt}{4.82pt}{} \\
\cline{3-11}
 &  &  & \HoloSegMetric{Dice} &  & \HoloSegScore{0.3991}{(0.3864--0.4129)}{4.55pt}{4.82pt}{} & \HoloSegScore{0.004113}{(0.002059--0.006583)}{3.85pt}{4.12pt}{} & \HoloSegScore{0.3186}{(0.3054--0.3323)}{4.55pt}{4.82pt}{} & \HoloSegScore{0.7616}{(0.7581--0.7805)}{4.55pt}{4.82pt}{} & \HoloSegScore{0.7294}{(0.7210--0.7382)}{4.55pt}{4.82pt}{} & \HoloSegScore{0.7756}{(0.7673--0.7839)}{4.55pt}{4.82pt}{} \\*
\softcline{4-4}\softcline{6-11}
 &  & \HoloSegSpan{\makecell[c]{head of\\[-0.10ex]pancreas}}{2.04cm}{0.32cm} & \HoloSegMetric{HD95} & \raisebox{0.32cm}[0pt][0pt]{\HoloSegUnsupported} & \HoloSegScore{60.14}{(58.31--61.85)}{4.55pt}{4.82pt}{} & \HoloSegScore{90.92}{(78.69--104.2)}{4.55pt}{4.82pt}{} & \HoloSegScore{58.14}{(56.32--59.85)}{4.55pt}{4.82pt}{} & \HoloSegScore{6.441}{(5.380--9.631)}{4.55pt}{4.82pt}{} & \HoloSegScore{11.00}{(10.37--11.76)}{4.55pt}{4.82pt}{} & \HoloSegScore{7.414}{(6.752--8.345)}{4.55pt}{4.82pt}{} \\
\cline{3-11}
 &  &  & \HoloSegMetric{Dice} & \HoloSegScore{0.3233}{(0.2969--0.3525)}{4.55pt}{4.82pt}{} & \HoloSegScore{0.7752}{(0.7659--0.7835)}{4.55pt}{4.82pt}{} & \HoloSegScore{0.3198}{(0.2917--0.3488)}{4.55pt}{4.82pt}{} & \HoloSegScore{0.4395}{(0.4065--0.4697)}{4.55pt}{4.82pt}{} & \HoloSegScore{0.9013}{(0.9008--0.9089)}{4.55pt}{4.82pt}{} & \HoloSegScore{0.9292}{(0.9236--0.9339)}{4.55pt}{4.82pt}{} & \HoloSegScore{0.9330}{(0.9285--0.9372)}{4.55pt}{4.82pt}{} \\*
\softcline{4-11}
 &  & \HoloSegSpan{\makecell[c]{right kidney}}{2.04cm}{0.32cm} & \HoloSegMetric{HD95} & \HoloSegScore{74.58}{(70.16--78.80)}{4.55pt}{4.82pt}{} & \HoloSegScore{51.16}{(47.35--54.93)}{4.55pt}{4.82pt}{} & \HoloSegScore{69.94}{(65.56--74.55)}{4.55pt}{4.82pt}{} & \HoloSegScore{68.24}{(63.49--72.90)}{4.55pt}{4.82pt}{} & \HoloSegScore{4.831}{(4.690--5.364)}{4.55pt}{4.82pt}{} & \HoloSegScore{5.436}{(4.592--6.389)}{4.55pt}{4.82pt}{} & \HoloSegScore{3.957}{(3.573--4.345)}{4.55pt}{4.82pt}{} \\
\cline{3-11}
 &  &  & \HoloSegMetric{Dice} & \HoloSegScore{0.3821}{(0.3514--0.4126)}{4.55pt}{4.82pt}{} & \HoloSegScore{0.8462}{(0.8390--0.8536)}{4.55pt}{4.82pt}{} & \HoloSegScore{0.3611}{(0.3337--0.3878)}{4.55pt}{4.82pt}{} & \HoloSegScore{0.4702}{(0.4361--0.5024)}{4.55pt}{4.82pt}{} & \HoloSegScore{0.9031}{(0.8931--0.9206)}{4.55pt}{4.82pt}{} & \HoloSegScore{0.9225}{(0.9143--0.9302)}{4.55pt}{4.82pt}{} & \HoloSegScore{0.9275}{(0.9190--0.9349)}{4.55pt}{4.82pt}{} \\*
\softcline{4-11}
 &  & \HoloSegSpan{\makecell[c]{spleen}}{2.04cm}{0.32cm} & \HoloSegMetric{HD95} & \HoloSegScore{96.24}{(90.27--101.9)}{4.55pt}{4.82pt}{} & \HoloSegScore{4.753}{(4.196--5.447)}{4.55pt}{4.82pt}{} & \HoloSegScore{98.91}{(93.31--104.5)}{4.55pt}{4.82pt}{} & \HoloSegScore{93.12}{(87.54--99.38)}{4.55pt}{4.82pt}{} & \HoloSegScore{4.329}{(2.904--5.500)}{4.55pt}{4.82pt}{} & \HoloSegScore{5.706}{(4.860--6.622)}{4.55pt}{4.82pt}{} & \HoloSegScore{4.516}{(3.821--5.276)}{4.55pt}{4.82pt}{} \\
\cline{3-11}
 &  &  & \HoloSegMetric{Dice} &  & \HoloSegScore{0.2426}{(0.2356--0.2498)}{4.55pt}{4.82pt}{} & \HoloSegScore{0.0001518}{(0.0000--0.0004402)}{3.85pt}{4.12pt}{} & \HoloSegScore{0.3031}{(0.2938--0.3126)}{4.55pt}{4.82pt}{} & \HoloSegScore{0.6637}{(0.6489--0.6666)}{4.55pt}{4.82pt}{} & \HoloSegScore{0.6061}{(0.5937--0.6190)}{4.55pt}{4.82pt}{} & \HoloSegScore{0.6361}{(0.6236--0.6478)}{4.55pt}{4.82pt}{} \\*
\softcline{4-4}\softcline{6-11}
 &  & \HoloSegSpan{\makecell[c]{body of\\[-0.10ex]pancreas}}{2.04cm}{0.32cm} & \HoloSegMetric{HD95} & \raisebox{0.32cm}[0pt][0pt]{\HoloSegUnsupported} & \HoloSegScore{47.47}{(46.35--48.66)}{4.55pt}{4.82pt}{} & \HoloSegScore{112.2}{(96.20--128.6)}{4.55pt}{4.82pt}{} & \HoloSegScore{49.27}{(48.05--50.51)}{4.55pt}{4.82pt}{} & \HoloSegScore{10.81}{(9.444--11.64)}{4.55pt}{4.82pt}{} & \HoloSegScore{18.49}{(17.78--19.25)}{4.55pt}{4.82pt}{} & \HoloSegScore{11.95}{(11.36--12.56)}{4.55pt}{4.82pt}{} \\
\cline{3-11}
 &  &  & \HoloSegMetric{Dice} &  & \HoloSegScore{0.001502}{(0.001262--0.001810)}{3.85pt}{4.12pt}{} & \HoloSegScore{0.0000}{(0.0000--0.0000)}{4.55pt}{4.82pt}{} & \HoloSegScore{0.3106}{(0.2928--0.3284)}{4.55pt}{4.82pt}{} & \HoloSegScore{0.5539}{(0.5474--0.5633)}{4.55pt}{4.82pt}{} & \HoloSegScore{0.5634}{(0.5498--0.5783)}{4.55pt}{4.82pt}{} & \HoloSegScore{0.6331}{(0.6204--0.6454)}{4.55pt}{4.82pt}{} \\*
\softcline{4-4}\softcline{6-11}
 &  & \HoloSegSpan{\makecell[c]{superior\\[-0.10ex]mesenteric\\[-0.10ex]artery}}{2.04cm}{0.32cm} & \HoloSegMetric{HD95} & \raisebox{0.32cm}[0pt][0pt]{\HoloSegUnsupported} & \HoloSegScore{73.68}{(71.21--76.31)}{4.55pt}{4.82pt}{} & \HoloSegScore{95.09}{(77.14--115.3)}{4.55pt}{4.82pt}{} & \HoloSegScore{26.68}{(24.40--28.88)}{4.55pt}{4.82pt}{} & \HoloSegScore{11.01}{(10.02--11.95)}{4.55pt}{4.82pt}{} & \HoloSegScore{10.63}{(9.923--11.48)}{4.55pt}{4.82pt}{} & \HoloSegScore{7.956}{(7.392--8.559)}{4.55pt}{4.82pt}{} \\
\cline{3-11}
 &  &  & \HoloSegMetric{Dice} & \HoloSegScore{0.2265}{(0.2043--0.2490)}{4.55pt}{4.82pt}{} & \HoloSegScore{0.3669}{(0.3469--0.3868)}{4.55pt}{4.82pt}{} & \HoloSegScore{0.1866}{(0.1668--0.2063)}{4.55pt}{4.82pt}{} & \HoloSegScore{0.3553}{(0.3249--0.3846)}{4.55pt}{4.82pt}{} & \HoloSegScore{0.6950}{(0.6900--0.7104)}{4.55pt}{4.82pt}{} & \HoloSegScore{0.6831}{(0.6662--0.6996)}{4.55pt}{4.82pt}{} & \HoloSegScore{0.7001}{(0.6833--0.7178)}{4.55pt}{4.82pt}{} \\*
\softcline{4-11}
 &  & \HoloSegSpan{\makecell[c]{gallbladder}}{2.04cm}{0.32cm} & \HoloSegMetric{HD95} & \HoloSegScore{66.96}{(61.75--71.99)}{4.55pt}{4.82pt}{} & \HoloSegScore{42.18}{(38.88--45.51)}{4.55pt}{4.82pt}{} & \HoloSegScore{60.70}{(55.72--65.77)}{4.55pt}{4.82pt}{} & \HoloSegScore{34.26}{(29.12--39.68)}{4.55pt}{4.82pt}{} & \HoloSegScore{11.05}{(9.813--12.97)}{4.55pt}{4.82pt}{} & \HoloSegScore{12.01}{(11.04--13.00)}{4.55pt}{4.82pt}{} & \HoloSegScore{11.65}{(10.45--12.90)}{4.55pt}{4.82pt}{} \\
\cline{3-11}
 &  &  & \HoloSegMetric{Dice} & \HoloSegScore{0.1753}{(0.1560--0.1937)}{4.55pt}{4.82pt}{} & \HoloSegScore{0.3308}{(0.3183--0.3433)}{4.55pt}{4.82pt}{} & \HoloSegScore{0.1263}{(0.1092--0.1437)}{4.55pt}{4.82pt}{} & \HoloSegScore{0.3644}{(0.3404--0.3902)}{4.55pt}{4.82pt}{} & \HoloSegScore{0.6066}{(0.6063--0.6217)}{4.55pt}{4.82pt}{} & \HoloSegScore{0.6579}{(0.6451--0.6703)}{4.55pt}{4.82pt}{} & \HoloSegScore{0.6926}{(0.6819--0.7022)}{4.55pt}{4.82pt}{} \\*
\softcline{4-11}
 &  & \HoloSegSpan{\makecell[c]{left adrenal\\[-0.10ex]gland}}{2.04cm}{0.32cm} & \HoloSegMetric{HD95} & \HoloSegScore{32.11}{(28.30--36.38)}{4.55pt}{4.82pt}{} & \HoloSegScore{17.12}{(15.75--18.82)}{4.55pt}{4.82pt}{} & \HoloSegScore{36.33}{(32.52--40.04)}{4.55pt}{4.82pt}{} & \HoloSegScore{34.44}{(31.72--37.10)}{4.55pt}{4.82pt}{} & \HoloSegScore{5.939}{(4.865--7.699)}{4.55pt}{4.82pt}{} & \HoloSegScore{8.514}{(7.701--9.484)}{4.55pt}{4.82pt}{} & \HoloSegScore{6.871}{(6.287--7.419)}{4.55pt}{4.82pt}{} \\
\hline
\pagebreak[4]
 &  &  & \HoloSegMetric{Dice} &  & \HoloSegScore{0.1961}{(0.1880--0.2048)}{4.55pt}{4.82pt}{} & \HoloSegScore{0.0002480}{(0.0000--0.0007440)}{3.85pt}{4.12pt}{} & \HoloSegScore{0.2034}{(0.1911--0.2166)}{4.55pt}{4.82pt}{} & \HoloSegScore{0.6605}{(0.6466--0.6652)}{4.55pt}{4.82pt}{} & \HoloSegScore{0.6700}{(0.6553--0.6849)}{4.55pt}{4.82pt}{} & \HoloSegScore{0.6791}{(0.6636--0.6935)}{4.55pt}{4.82pt}{} \\*
\softcline{4-4}\softcline{6-11}
 &  & \HoloSegSpan{\makecell[c]{tail of\\[-0.10ex]pancreas}}{2.04cm}{0.32cm} & \HoloSegMetric{HD95} & \raisebox{0.32cm}[0pt][0pt]{\HoloSegUnsupported} & \HoloSegScore{72.24}{(70.34--74.02)}{4.55pt}{4.82pt}{} & \HoloSegScore{109.8}{(98.81--121.0)}{4.55pt}{4.82pt}{} & \HoloSegScore{66.05}{(64.55--67.68)}{4.55pt}{4.82pt}{} & \HoloSegScore{11.21}{(10.87--11.93)}{4.55pt}{4.82pt}{} & \HoloSegScore{11.46}{(10.63--12.32)}{4.55pt}{4.82pt}{} & \HoloSegScore{11.25}{(10.43--12.14)}{4.55pt}{4.82pt}{} \\
\cline{3-11}
 &  &  & \HoloSegMetric{Dice} & \HoloSegScore{0.3374}{(0.3110--0.3632)}{4.55pt}{4.82pt}{} & \HoloSegScore{0.7646}{(0.7530--0.7757)}{4.55pt}{4.82pt}{} & \HoloSegScore{0.3329}{(0.3060--0.3588)}{4.55pt}{4.82pt}{} & \HoloSegScore{0.4582}{(0.4281--0.4891)}{4.55pt}{4.82pt}{} & \HoloSegScore{0.8613}{(0.8424--0.8699)}{4.55pt}{4.82pt}{} & \HoloSegScore{0.9055}{(0.8970--0.9136)}{4.55pt}{4.82pt}{} & \HoloSegScore{0.9140}{(0.9052--0.9220)}{4.55pt}{4.82pt}{} \\*
\softcline{4-11}
 &  & \HoloSegSpan{\makecell[c]{left kidney}}{2.04cm}{0.32cm} & \HoloSegMetric{HD95} & \HoloSegScore{78.55}{(73.63--83.39)}{4.55pt}{4.82pt}{} & \HoloSegScore{44.43}{(40.84--48.05)}{4.55pt}{4.82pt}{} & \HoloSegScore{74.00}{(69.42--78.65)}{4.55pt}{4.82pt}{} & \HoloSegScore{69.12}{(64.32--73.76)}{4.55pt}{4.82pt}{} & \HoloSegScore{5.424}{(3.630--5.886)}{4.55pt}{4.82pt}{} & \HoloSegScore{9.096}{(7.847--10.44)}{4.55pt}{4.82pt}{} & \HoloSegScore{4.878}{(4.277--5.549)}{4.55pt}{4.82pt}{} \\
\cline{3-11}
 &  &  & \HoloSegMetric{Dice} &  & \HoloSegScore{0.007194}{(0.006046--0.008456)}{3.85pt}{4.12pt}{} & \HoloSegScore{0.00002753}{(0.0000--0.0001101)}{3.85pt}{4.12pt}{} & \HoloSegScore{0.07140}{(0.06078--0.08253)}{4.20pt}{4.48pt}{} & \HoloSegScore{0.4212}{(0.4127--0.4320)}{4.55pt}{4.82pt}{} & \HoloSegScore{0.3648}{(0.3511--0.3783)}{4.55pt}{4.82pt}{} & \HoloSegScore{0.4235}{(0.4089--0.4370)}{4.55pt}{4.82pt}{} \\*
\softcline{4-4}\softcline{6-11}
 &  & \HoloSegSpan{\makecell[c]{common bile\\[-0.10ex]duct}}{2.04cm}{0.32cm} & \HoloSegMetric{HD95} & \raisebox{0.32cm}[0pt][0pt]{\HoloSegUnsupported} & \HoloSegScore{61.56}{(59.49--63.54)}{4.55pt}{4.82pt}{} & \HoloSegScore{90.41}{(83.14--98.09)}{4.55pt}{4.82pt}{} & \HoloSegScore{19.47}{(17.40--21.91)}{4.55pt}{4.82pt}{} & \HoloSegScore{8.625}{(7.538--8.836)}{4.55pt}{4.82pt}{} & \HoloSegScore{9.908}{(9.421--10.37)}{4.55pt}{4.82pt}{} & \HoloSegScore{9.677}{(9.090--10.39)}{4.55pt}{4.82pt}{} \\
\cline{3-11}
 &  &  & \HoloSegMetric{Dice} &  & \HoloSegScore{0.02258}{(0.02044--0.02468)}{4.20pt}{4.48pt}{} & \HoloSegScore{0.04085}{(0.03455--0.04803)}{4.20pt}{4.48pt}{} & \HoloSegScore{0.2139}{(0.2022--0.2247)}{4.55pt}{4.82pt}{} & \HoloSegScore{0.3640}{(0.3432--0.3847)}{4.55pt}{4.82pt}{} & \HoloSegScore{0.4466}{(0.4347--0.4587)}{4.55pt}{4.82pt}{} & \HoloSegScore{0.4465}{(0.4340--0.4593)}{4.55pt}{4.82pt}{} \\*
\softcline{4-4}\softcline{6-11}
 &  & \HoloSegSpan{\makecell[c]{celiac\\[-0.10ex]artery}}{2.04cm}{0.32cm} & \HoloSegMetric{HD95} & \raisebox{0.32cm}[0pt][0pt]{\HoloSegUnsupported} & \HoloSegScore{46.82}{(45.10--48.70)}{4.55pt}{4.82pt}{} & \HoloSegScore{64.97}{(59.38--71.26)}{4.55pt}{4.82pt}{} & \HoloSegScore{50.10}{(48.76--51.36)}{4.55pt}{4.82pt}{} & \HoloSegScore{18.57}{(16.65--20.39)}{4.55pt}{4.82pt}{} & \HoloSegScore{18.01}{(17.08--19.08)}{4.55pt}{4.82pt}{} & \HoloSegScore{18.19}{(17.34--19.11)}{4.55pt}{4.82pt}{} \\
\cline{3-11}
 &  &  & \HoloSegMetric{Dice} &  & \HoloSegScore{0.009559}{(0.008147--0.01087)}{3.85pt}{4.12pt}{} & \HoloSegScore{0.0007438}{(0.0004090--0.001198)}{3.52pt}{3.80pt}{} & \HoloSegScore{0.07934}{(0.06683--0.09165)}{4.20pt}{4.48pt}{} & \HoloSegScore{0.08184}{(0.08122--0.1003)}{4.20pt}{4.48pt}{} & \HoloSegScore{0.09234}{(0.08333--0.1016)}{4.20pt}{4.48pt}{} & \HoloSegScore{0.1093}{(0.09973--0.1195)}{4.20pt}{4.48pt}{} \\*
\softcline{4-4}\softcline{6-11}
 &  & \HoloSegSpan{\makecell[c]{pancreatic\\[-0.10ex]duct}}{2.04cm}{0.32cm} & \HoloSegMetric{HD95} & \raisebox{0.32cm}[0pt][0pt]{\HoloSegUnsupported} & \HoloSegScore{67.08}{(64.85--69.52)}{4.55pt}{4.82pt}{} & \HoloSegScore{61.66}{(53.77--70.42)}{4.55pt}{4.82pt}{} & \HoloSegScore{41.54}{(38.83--44.37)}{4.55pt}{4.82pt}{} & \HoloSegScore{32.57}{(32.19--34.00)}{4.55pt}{4.82pt}{} & \HoloSegScore{30.38}{(28.63--32.10)}{4.55pt}{4.82pt}{} & \HoloSegScore{27.79}{(26.30--29.43)}{4.55pt}{4.82pt}{} \\
\cline{3-11}
 & \HoloSegSpan{\makecell[c]{PanTS}}{1.86cm}{0.32cm} &  & \HoloSegMetric{Dice} & \HoloSegScore{0.04774}{(0.03465--0.06204)}{4.20pt}{4.48pt}{} & \HoloSegScore{0.1568}{(0.1348--0.1784)}{4.55pt}{4.82pt}{} & \HoloSegScore{0.02217}{(0.01417--0.03083)}{4.20pt}{4.48pt}{} & \HoloSegScore{0.2718}{(0.2394--0.3025)}{4.55pt}{4.82pt}{} & \HoloSegScore{0.2682}{(0.2617--0.2841)}{4.55pt}{4.82pt}{} & \HoloSegScore{0.2815}{(0.2511--0.3122)}{4.55pt}{4.82pt}{} & \HoloSegScore{0.2795}{(0.2489--0.3096)}{4.55pt}{4.82pt}{} \\*
\softcline{4-11}
 &  & \HoloSegSpan{\makecell[c]{urinary\\[-0.10ex]bladder}}{2.04cm}{0.32cm} & \HoloSegMetric{HD95} & \HoloSegScore{126.1}{(117.2--135.4)}{4.55pt}{4.82pt}{} & \HoloSegScore{98.23}{(89.90--106.3)}{4.55pt}{4.82pt}{} & \HoloSegScore{110.3}{(103.0--118.0)}{4.55pt}{4.82pt}{} & \HoloSegScore{36.91}{(27.96--46.14)}{4.55pt}{4.82pt}{} & \HoloSegScore{73.04}{(64.27--80.63)}{4.55pt}{4.82pt}{} & \HoloSegScore{78.51}{(71.14--86.93)}{4.55pt}{4.82pt}{} & \HoloSegScore{92.78}{(85.73--101.0)}{4.55pt}{4.82pt}{} \\
\cline{3-11}
 &  &  & \HoloSegMetric{Dice} & \HoloSegScore{0.02414}{(0.01472--0.03374)}{4.20pt}{4.48pt}{} & \HoloSegScore{0.1537}{(0.1316--0.1765)}{4.55pt}{4.82pt}{} & \HoloSegScore{0.002018}{(0.00004899--0.005162)}{3.52pt}{3.80pt}{} & \HoloSegScore{0.09034}{(0.06799--0.1115)}{4.20pt}{4.48pt}{} & \HoloSegScore{0.3782}{(0.3703--0.3944)}{4.55pt}{4.82pt}{} & \HoloSegScore{0.3281}{(0.3009--0.3537)}{4.55pt}{4.82pt}{} & \HoloSegScore{0.3260}{(0.3014--0.3497)}{4.55pt}{4.82pt}{} \\*
\softcline{4-11}
 &  & \HoloSegSpan{\makecell[c]{prostate}}{2.04cm}{0.32cm} & \HoloSegMetric{HD95} & \HoloSegScore{114.5}{(108.0--121.4)}{4.55pt}{4.82pt}{} & \HoloSegScore{58.18}{(52.87--63.82)}{4.55pt}{4.82pt}{} & \HoloSegScore{105.0}{(96.28--114.0)}{4.55pt}{4.82pt}{} & \HoloSegScore{25.53}{(20.33--31.36)}{4.55pt}{4.82pt}{} & \HoloSegScore{26.05}{(25.27--28.63)}{4.55pt}{4.82pt}{} & \HoloSegScore{29.71}{(26.60--32.61)}{4.55pt}{4.82pt}{} & \HoloSegScore{42.48}{(39.67--45.65)}{4.55pt}{4.82pt}{} \\
\cline{3-11}
 &  &  & \HoloSegMetric{Dice} & \HoloSegScore{0.09359}{(0.06801--0.1187)}{4.20pt}{4.48pt}{} & \HoloSegScore{0.6168}{(0.5817--0.6522)}{4.55pt}{4.82pt}{} & \HoloSegScore{0.05557}{(0.03669--0.07624)}{4.20pt}{4.48pt}{} & \HoloSegScore{0.3236}{(0.2647--0.3829)}{4.55pt}{4.82pt}{} & \HoloSegScore{0.7649}{(0.7563--0.7783)}{4.55pt}{4.82pt}{} & \HoloSegScore{0.7668}{(0.7303--0.8071)}{4.55pt}{4.82pt}{} & \HoloSegScore{0.7817}{(0.7426--0.8198)}{4.55pt}{4.82pt}{} \\*
\softcline{4-11}
 &  & \HoloSegSpan{\makecell[c]{left femur}}{2.04cm}{0.32cm} & \HoloSegMetric{HD95} & \HoloSegScore{181.0}{(173.2--188.8)}{4.55pt}{4.82pt}{} & \HoloSegScore{23.78}{(17.87--29.95)}{4.55pt}{4.82pt}{} & \HoloSegScore{161.1}{(146.9--173.8)}{4.55pt}{4.82pt}{} & \HoloSegScore{128.7}{(113.0--143.3)}{4.55pt}{4.82pt}{} & \HoloSegScore{26.00}{(18.98--34.56)}{4.55pt}{4.82pt}{} & \HoloSegScore{48.65}{(38.41--60.34)}{4.55pt}{4.82pt}{} & \HoloSegScore{41.71}{(31.96--51.47)}{4.55pt}{4.82pt}{} \\
\cline{3-11}
 &  &  & \HoloSegMetric{Dice} & \HoloSegScore{0.1608}{(0.1331--0.1888)}{4.55pt}{4.82pt}{} & \HoloSegScore{0.6020}{(0.5690--0.6328)}{4.55pt}{4.82pt}{} & \HoloSegScore{0.09125}{(0.06707--0.1178)}{4.20pt}{4.48pt}{} & \HoloSegScore{0.3914}{(0.3389--0.4481)}{4.55pt}{4.82pt}{} & \HoloSegScore{0.7943}{(0.7604--0.8202)}{4.55pt}{4.82pt}{} & \HoloSegScore{0.7919}{(0.7636--0.8211)}{4.55pt}{4.82pt}{} & \HoloSegScore{0.8161}{(0.7892--0.8424)}{4.55pt}{4.82pt}{} \\*
\softcline{4-11}
 &  & \HoloSegSpan{\makecell[c]{right femur}}{2.04cm}{0.32cm} & \HoloSegMetric{HD95} & \HoloSegScore{170.7}{(162.0--180.0)}{4.55pt}{4.82pt}{} & \HoloSegScore{61.41}{(50.63--71.63)}{4.55pt}{4.82pt}{} & \HoloSegScore{150.7}{(139.1--163.0)}{4.55pt}{4.82pt}{} & \HoloSegScore{116.4}{(103.1--130.2)}{4.55pt}{4.82pt}{} & \HoloSegScore{10.74}{(9.998--14.10)}{4.55pt}{4.82pt}{} & \HoloSegScore{16.05}{(12.06--20.58)}{4.55pt}{4.82pt}{} & \HoloSegScore{23.12}{(16.90--29.99)}{4.55pt}{4.82pt}{} \\
\cline{3-11}
 &  &  & \HoloSegMetric{Dice} & \HoloSegScore{0.06855}{(0.04504--0.09540)}{4.20pt}{4.48pt}{} & \HoloSegScore{0.1678}{(0.1399--0.1958)}{4.55pt}{4.82pt}{} & \HoloSegScore{0.005854}{(0.0003434--0.01550)}{3.85pt}{4.12pt}{} & \HoloSegScore{0.3028}{(0.2503--0.3549)}{4.55pt}{4.82pt}{} & \HoloSegScore{0.4828}{(0.4786--0.4957)}{4.55pt}{4.82pt}{} & \HoloSegScore{0.3491}{(0.3049--0.3945)}{4.55pt}{4.82pt}{} & \HoloSegScore{0.3888}{(0.3437--0.4361)}{4.55pt}{4.82pt}{} \\*
\softcline{4-11}
\HoloSegSpan{\makecell[c]{\textbf{Internal}}}{1.20cm}{0.32cm} &  & \HoloSegSpan{\makecell[c]{pancreas\\[-0.10ex]lesion}}{2.04cm}{0.32cm} & \HoloSegMetric{HD95} & \HoloSegScore{62.26}{(50.25--74.92)}{4.55pt}{4.82pt}{} & \HoloSegScore{66.19}{(62.26--70.07)}{4.55pt}{4.82pt}{} & \HoloSegScore{87.82}{(73.00--101.2)}{4.55pt}{4.82pt}{} & \HoloSegScore{37.21}{(29.14--45.85)}{4.55pt}{4.82pt}{} & \HoloSegScore{26.08}{(22.17--29.24)}{4.55pt}{4.82pt}{} & \HoloSegScore{35.63}{(30.88--40.20)}{4.55pt}{4.82pt}{} & \HoloSegScore{32.46}{(27.85--37.71)}{4.55pt}{4.82pt}{} \\
\cline{2-11}
 &  &  & \HoloSegMetric{Dice} & \HoloSegScore{0.4279}{(0.3847--0.4730)}{4.55pt}{4.82pt}{} & \HoloSegScore{0.01395}{(0.009369--0.01918)}{3.85pt}{4.12pt}{} & \HoloSegScore{0.006545}{(0.004327--0.009109)}{3.85pt}{4.12pt}{} & \HoloSegScore{0.5506}{(0.4988--0.5993)}{4.55pt}{4.82pt}{} & \HoloSegScore{0.7934}{(0.7689--0.8216)}{4.55pt}{4.82pt}{} & \HoloSegScore{0.6637}{(0.6261--0.6958)}{4.55pt}{4.82pt}{} & \HoloSegScore{0.7201}{(0.6936--0.7437)}{4.55pt}{4.82pt}{} \\*
\softcline{4-11}
 &  & \HoloSegSpan{\makecell[c]{lung tumor}}{2.04cm}{0.32cm} & \HoloSegMetric{HD95} & \HoloSegScore{101.5}{(83.38--126.0)}{4.55pt}{4.82pt}{} & \HoloSegScore{189.5}{(177.4--201.6)}{4.55pt}{4.82pt}{} & \HoloSegScore{167.1}{(159.0--175.3)}{4.55pt}{4.82pt}{} & \HoloSegScore{96.30}{(76.90--121.4)}{4.55pt}{4.82pt}{} & \HoloSegScore{22.45}{(17.12--29.84)}{4.55pt}{4.82pt}{} & \HoloSegScore{44.44}{(36.29--52.47)}{4.55pt}{4.82pt}{} & \HoloSegScore{37.14}{(29.83--44.56)}{4.55pt}{4.82pt}{} \\
\cline{3-11}
 &  &  & \HoloSegMetric{Dice} & \HoloSegScore{0.4881}{(0.4394--0.5376)}{4.55pt}{4.82pt}{} & \HoloSegScore{0.03574}{(0.02355--0.04969)}{4.20pt}{4.48pt}{} & \HoloSegScore{0.02772}{(0.01968--0.03687)}{4.20pt}{4.48pt}{} & \HoloSegScore{0.5305}{(0.4719--0.5863)}{4.55pt}{4.82pt}{} & \HoloSegScore{0.6957}{(0.6581--0.7368)}{4.55pt}{4.82pt}{} & \HoloSegScore{0.6716}{(0.6364--0.7065)}{4.55pt}{4.82pt}{} & \HoloSegScore{0.6913}{(0.6596--0.7221)}{4.55pt}{4.82pt}{} \\*
\softcline{4-11}
 &  & \HoloSegSpan{\makecell[c]{liver tumor}}{2.04cm}{0.32cm} & \HoloSegMetric{HD95} & \HoloSegScore{39.94}{(33.23--48.10)}{4.55pt}{4.82pt}{} & \HoloSegScore{117.2}{(110.1--124.1)}{4.55pt}{4.82pt}{} & \HoloSegScore{95.29}{(90.06--100.8)}{4.55pt}{4.82pt}{} & \HoloSegScore{37.48}{(29.42--45.84)}{4.55pt}{4.82pt}{} & \HoloSegScore{26.89}{(19.73--36.41)}{4.55pt}{4.82pt}{} & \HoloSegScore{22.73}{(18.93--26.96)}{4.55pt}{4.82pt}{} & \HoloSegScore{26.73}{(20.62--33.56)}{4.55pt}{4.82pt}{} \\
\cline{3-11}
 &  &  & \HoloSegMetric{Dice} &  & \HoloSegScore{0.4430}{(0.3823--0.5005)}{4.55pt}{4.82pt}{} & \HoloSegScore{0.0004982}{(0.0000--0.001441)}{4.20pt}{4.48pt}{} & \HoloSegScore{0.1540}{(0.1148--0.1985)}{4.55pt}{4.82pt}{} & \HoloSegScore{0.8062}{(0.7848--0.8385)}{4.55pt}{4.82pt}{} & \HoloSegScore{0.7456}{(0.7043--0.7881)}{4.55pt}{4.82pt}{} & \HoloSegScore{0.7763}{(0.7367--0.8117)}{4.55pt}{4.82pt}{} \\*
\softcline{4-4}\softcline{6-11}
 &  & \HoloSegSpan{\makecell[c]{gallbladder\\[-0.10ex]cancer}}{2.04cm}{0.32cm} & \HoloSegMetric{HD95} & \raisebox{0.32cm}[0pt][0pt]{\HoloSegUnsupported} & \HoloSegScore{45.06}{(34.06--57.59)}{4.55pt}{4.82pt}{} & \HoloSegScore{131.0}{(102.2--157.0)}{4.55pt}{4.82pt}{} & \HoloSegScore{35.93}{(31.44--41.89)}{4.55pt}{4.82pt}{} & \HoloSegScore{16.27}{(12.44--22.91)}{4.55pt}{4.82pt}{} & \HoloSegScore{7.748}{(5.708--10.40)}{4.55pt}{4.82pt}{} & \HoloSegScore{12.45}{(7.990--17.78)}{4.55pt}{4.82pt}{} \\
\cline{3-11}
 &  &  & \HoloSegMetric{Dice} & \HoloSegScore{0.01734}{(0.002756--0.03950)}{3.85pt}{4.12pt}{} & \HoloSegScore{0.3699}{(0.3314--0.4104)}{4.55pt}{4.82pt}{} & \HoloSegScore{0.003484}{(0.0008306--0.007482)}{3.52pt}{3.80pt}{} & \HoloSegScore{0.01990}{(0.006567--0.03696)}{3.85pt}{4.12pt}{} & \HoloSegScore{0.6022}{(0.5486--0.6739)}{4.55pt}{4.82pt}{} & \HoloSegScore{0.3708}{(0.3132--0.4311)}{4.55pt}{4.82pt}{} & \HoloSegScore{0.3767}{(0.3221--0.4324)}{4.55pt}{4.82pt}{} \\*
\softcline{4-11}
 &  & \HoloSegSpan{\makecell[c]{pancreas\\[-0.10ex]tumor}}{2.04cm}{0.32cm} & \HoloSegMetric{HD95} & \HoloSegScore{146.4}{(121.9--168.9)}{4.55pt}{4.82pt}{} & \HoloSegScore{30.77}{(24.47--37.25)}{4.55pt}{4.82pt}{} & \HoloSegScore{100.1}{(90.48--110.4)}{4.55pt}{4.82pt}{} & \HoloSegScore{74.93}{(60.82--90.05)}{4.55pt}{4.82pt}{} & \HoloSegScore{26.52}{(18.81--38.27)}{4.55pt}{4.82pt}{} & \HoloSegScore{31.13}{(26.32--36.00)}{4.55pt}{4.82pt}{} & \HoloSegScore{28.02}{(22.70--33.80)}{4.55pt}{4.82pt}{} \\
\cline{3-11}
 &  &  & \HoloSegMetric{Dice} &  & \HoloSegScore{0.006366}{(0.0007561--0.01462)}{3.85pt}{4.12pt}{} & \HoloSegScore{0.2960}{(0.2506--0.3421)}{4.55pt}{4.82pt}{} & \HoloSegScore{0.09959}{(0.07436--0.1272)}{4.20pt}{4.48pt}{} & \HoloSegScore{0.8244}{(0.8095--0.8478)}{4.55pt}{4.82pt}{} & \HoloSegScore{0.8083}{(0.7784--0.8332)}{4.55pt}{4.82pt}{} & \HoloSegScore{0.8506}{(0.8377--0.8615)}{4.55pt}{4.82pt}{} \\*
\softcline{4-4}\softcline{6-11}
 & \HoloSegSpan{\makecell[c]{PASTA-Gen-\\[-0.10ex]30K-\\[-0.10ex]Lesions}}{1.86cm}{0.32cm} & \HoloSegSpan{\makecell[c]{esophageal\\[-0.10ex]cancer}}{2.04cm}{0.32cm} & \HoloSegMetric{HD95} & \raisebox{0.32cm}[0pt][0pt]{\HoloSegUnsupported} & \HoloSegScore{150.9}{(141.8--159.8)}{4.55pt}{4.82pt}{} & \HoloSegScore{13.78}{(11.09--17.00)}{4.55pt}{4.82pt}{} & \HoloSegScore{45.59}{(37.20--55.10)}{4.55pt}{4.82pt}{} & \HoloSegScore{17.58}{(13.27--24.66)}{4.55pt}{4.82pt}{} & \HoloSegScore{54.55}{(42.78--67.33)}{4.55pt}{4.82pt}{} & \HoloSegScore{31.27}{(24.93--38.35)}{4.55pt}{4.82pt}{} \\
\cline{3-11}
 &  &  & \HoloSegMetric{Dice} &  & \HoloSegScore{0.2462}{(0.1820--0.3161)}{4.55pt}{4.82pt}{} & \HoloSegScore{0.0000}{(0.0000--0.0000)}{4.55pt}{4.82pt}{} & \HoloSegScore{0.08088}{(0.07075--0.09160)}{4.20pt}{4.48pt}{} & \HoloSegScore{0.6613}{(0.6154--0.7218)}{4.55pt}{4.82pt}{} & \HoloSegScore{0.7031}{(0.6769--0.7264)}{4.55pt}{4.82pt}{} & \HoloSegScore{0.7764}{(0.7565--0.7939)}{4.55pt}{4.82pt}{} \\*
\softcline{4-4}\softcline{6-11}
 &  & \HoloSegSpan{\makecell[c]{gastric\\[-0.10ex]cancer}}{2.04cm}{0.32cm} & \HoloSegMetric{HD95} & \raisebox{0.32cm}[0pt][0pt]{\HoloSegUnsupported} & \HoloSegScore{86.61}{(76.22--98.79)}{4.55pt}{4.82pt}{} & \HoloSegScore{270.3}{(263.2--276.9)}{4.55pt}{4.82pt}{} & \HoloSegScore{86.32}{(80.36--91.68)}{4.55pt}{4.82pt}{} & \HoloSegScore{22.40}{(15.92--31.77)}{4.55pt}{4.82pt}{} & \HoloSegScore{19.13}{(13.11--26.75)}{4.55pt}{4.82pt}{} & \HoloSegScore{53.48}{(47.46--60.57)}{4.55pt}{4.82pt}{} \\
\cline{3-11}
 &  &  & \HoloSegMetric{Dice} & \HoloSegScore{0.1073}{(0.07417--0.1438)}{4.20pt}{4.48pt}{} & \HoloSegScore{0.002069}{(0.0009012--0.003467)}{3.52pt}{3.80pt}{} & \HoloSegScore{0.001519}{(0.0004687--0.002943)}{3.52pt}{3.80pt}{} & \HoloSegScore{0.0001242}{(0.0000--0.0003301)}{3.85pt}{4.12pt}{} & \HoloSegScore{0.6411}{(0.5862--0.7084)}{4.55pt}{4.82pt}{} & \HoloSegScore{0.6195}{(0.5787--0.6594)}{4.55pt}{4.82pt}{} & \HoloSegScore{0.6655}{(0.6316--0.6985)}{4.55pt}{4.82pt}{} \\*
\softcline{4-11}
 &  & \HoloSegSpan{\makecell[c]{colorectal\\[-0.10ex]cancer}}{2.04cm}{0.32cm} & \HoloSegMetric{HD95} & \HoloSegScore{88.28}{(74.84--102.0)}{4.55pt}{4.82pt}{} & \HoloSegScore{143.7}{(135.6--152.3)}{4.55pt}{4.82pt}{} & \HoloSegScore{190.3}{(180.7--200.1)}{4.55pt}{4.82pt}{} & \HoloSegScore{134.1}{(120.4--149.3)}{4.55pt}{4.82pt}{} & \HoloSegScore{37.01}{(26.35--51.92)}{4.55pt}{4.82pt}{} & \HoloSegScore{34.62}{(25.25--44.54)}{4.55pt}{4.82pt}{} & \HoloSegScore{35.49}{(26.28--46.02)}{4.55pt}{4.82pt}{} \\
\cline{3-11}
 &  &  & \HoloSegMetric{Dice} &  & \HoloSegScore{0.3110}{(0.2776--0.3425)}{4.55pt}{4.82pt}{} & \HoloSegScore{0.2623}{(0.2332--0.2889)}{4.55pt}{4.82pt}{} & \HoloSegScore{0.5417}{(0.4866--0.6001)}{4.55pt}{4.82pt}{} & \HoloSegScore{0.7915}{(0.7658--0.8197)}{4.55pt}{4.82pt}{} & \HoloSegScore{0.8265}{(0.7977--0.8499)}{4.55pt}{4.82pt}{} & \HoloSegScore{0.8641}{(0.8349--0.8853)}{4.55pt}{4.82pt}{} \\*
\softcline{4-4}\softcline{6-11}
 &  & \HoloSegSpan{\makecell[c]{kidney tumor}}{2.04cm}{0.32cm} & \HoloSegMetric{HD95} & \raisebox{0.32cm}[0pt][0pt]{\HoloSegUnsupported} & \HoloSegScore{89.77}{(80.50--98.65)}{4.55pt}{4.82pt}{} & \HoloSegScore{67.42}{(60.52--74.62)}{4.55pt}{4.82pt}{} & \HoloSegScore{50.37}{(41.08--59.57)}{4.55pt}{4.82pt}{} & \HoloSegScore{19.60}{(14.21--27.83)}{4.55pt}{4.82pt}{} & \HoloSegScore{14.91}{(10.34--20.13)}{4.55pt}{4.82pt}{} & \HoloSegScore{15.36}{(10.48--21.63)}{4.55pt}{4.82pt}{} \\
\cline{3-11}
 &  &  & \HoloSegMetric{Dice} &  & \HoloSegScore{0.4614}{(0.3896--0.5333)}{4.55pt}{4.82pt}{} & \HoloSegScore{0.00003449}{(0.000004922--0.00007862)}{3.25pt}{3.52pt}{} & \HoloSegScore{0.07388}{(0.06005--0.08933)}{4.20pt}{4.48pt}{} & \HoloSegScore{0.7379}{(0.7015--0.7814)}{4.55pt}{4.82pt}{} & \HoloSegScore{0.7979}{(0.7626--0.8288)}{4.55pt}{4.82pt}{} & \HoloSegScore{0.8236}{(0.7932--0.8480)}{4.55pt}{4.82pt}{} \\*
\softcline{4-4}\softcline{6-11}
 &  & \HoloSegSpan{\makecell[c]{bladder\\[-0.10ex]cancer}}{2.04cm}{0.32cm} & \HoloSegMetric{HD95} & \raisebox{0.32cm}[0pt][0pt]{\HoloSegUnsupported} & \HoloSegScore{68.22}{(55.58--81.90)}{4.55pt}{4.82pt}{} & \HoloSegScore{105.2}{(95.22--115.3)}{4.55pt}{4.82pt}{} & \HoloSegScore{62.66}{(59.45--66.08)}{4.55pt}{4.82pt}{} & \HoloSegScore{14.40}{(10.82--20.47)}{4.55pt}{4.82pt}{} & \HoloSegScore{11.99}{(8.791--15.45)}{4.55pt}{4.82pt}{} & \HoloSegScore{16.04}{(10.12--23.14)}{4.55pt}{4.82pt}{} \\
\hline
\pagebreak[4]
 &  &  & \HoloSegMetric{Dice} & \HoloSegScore{0.01197}{(0.008088--0.01644)}{3.85pt}{4.12pt}{} & \HoloSegScore{0.4279}{(0.3890--0.4665)}{4.55pt}{4.82pt}{} & \HoloSegScore{0.01553}{(0.0000001250--0.03821)}{3.52pt}{3.80pt}{} & \HoloSegScore{0.0000}{(0.0000--0.0000)}{4.55pt}{4.82pt}{} & \HoloSegScore{0.7108}{(0.6684--0.7693)}{4.55pt}{4.82pt}{} & \HoloSegScore{0.2995}{(0.2623--0.3387)}{4.55pt}{4.82pt}{} & \HoloSegScore{0.3649}{(0.3278--0.4015)}{4.55pt}{4.82pt}{} \\*
\softcline{4-11}
 &  & \HoloSegSpan{\makecell[c]{bone\\[-0.10ex]metastasis}}{2.04cm}{0.32cm} & \HoloSegMetric{HD95} & \HoloSegScore{131.9}{(124.1--140.1)}{4.55pt}{4.82pt}{} & \HoloSegScore{103.4}{(92.78--113.9)}{4.55pt}{4.82pt}{} & \HoloSegScore{168.0}{(71.42--262.8)}{4.55pt}{4.82pt}{} & \HoloSegScore{215.0}{(187.1--241.7)}{4.55pt}{4.82pt}{} & \HoloSegScore{34.27}{(24.11--48.62)}{4.55pt}{4.82pt}{} & \HoloSegScore{91.15}{(83.77--98.51)}{4.55pt}{4.82pt}{} & \HoloSegScore{98.35}{(90.91--105.1)}{4.55pt}{4.82pt}{} \\
\cline{3-11}
 &  &  & \HoloSegMetric{Dice} &  & \HoloSegScore{0.006115}{(0.003762--0.009278)}{3.85pt}{4.12pt}{} & \HoloSegScore{0.0003101}{(0.000001329--0.0009211)}{3.25pt}{3.52pt}{} & \HoloSegScore{0.01456}{(0.005277--0.02461)}{3.85pt}{4.12pt}{} & \HoloSegScore{0.6381}{(0.5794--0.7098)}{4.55pt}{4.82pt}{} & \HoloSegScore{0.8138}{(0.7956--0.8307)}{4.55pt}{4.82pt}{} & \HoloSegScore{0.8255}{(0.8101--0.8392)}{4.55pt}{4.82pt}{} \\*
\softcline{4-4}\softcline{6-11}
 &  & \HoloSegSpan{\makecell[c]{liver cyst}}{2.04cm}{0.32cm} & \HoloSegMetric{HD95} & \raisebox{0.32cm}[0pt][0pt]{\HoloSegUnsupported} & \HoloSegScore{120.3}{(113.5--128.4)}{4.55pt}{4.82pt}{} & \HoloSegScore{176.3}{(167.8--184.7)}{4.55pt}{4.82pt}{} & \HoloSegScore{119.5}{(109.7--130.0)}{4.55pt}{4.82pt}{} & \HoloSegScore{25.03}{(17.66--36.84)}{4.55pt}{4.82pt}{} & \HoloSegScore{14.85}{(11.42--18.52)}{4.55pt}{4.82pt}{} & \HoloSegScore{13.27}{(9.722--16.73)}{4.55pt}{4.82pt}{} \\
\cline{3-11}
 &  &  & \HoloSegMetric{Dice} &  & \HoloSegScore{0.4721}{(0.4139--0.5271)}{4.55pt}{4.82pt}{} & \HoloSegScore{0.4089}{(0.3366--0.4879)}{4.55pt}{4.82pt}{} & \HoloSegScore{0.0000}{(0.0000--0.0000)}{4.55pt}{4.82pt}{} & \HoloSegScore{0.6763}{(0.6325--0.7411)}{4.55pt}{4.82pt}{} & \HoloSegScore{0.7688}{(0.7371--0.7984)}{4.55pt}{4.82pt}{} & \HoloSegScore{0.7761}{(0.7336--0.8113)}{4.55pt}{4.82pt}{} \\*
\softcline{4-4}\softcline{6-11}
 &  & \HoloSegSpan{\makecell[c]{gallstone}}{2.04cm}{0.32cm} & \HoloSegMetric{HD95} & \raisebox{0.32cm}[0pt][0pt]{\HoloSegUnsupported} & \HoloSegScore{14.78}{(10.93--20.20)}{4.55pt}{4.82pt}{} & \HoloSegScore{17.94}{(10.05--27.94)}{4.55pt}{4.82pt}{} & \HoloSegScore{30.37}{(24.47--36.59)}{4.55pt}{4.82pt}{} & \HoloSegScore{18.83}{(13.42--27.56)}{4.55pt}{4.82pt}{} & \HoloSegScore{8.742}{(4.750--13.41)}{4.55pt}{4.82pt}{} & \HoloSegScore{4.607}{(2.787--6.945)}{4.55pt}{4.82pt}{} \\
\cline{3-11}
 & \HoloSegSpan{\makecell[c]{PASTA-Gen-\\[-0.10ex]30K-\\[-0.10ex]Lesions}}{1.86cm}{0.32cm} &  & \HoloSegMetric{Dice} &  & \HoloSegScore{0.5222}{(0.4887--0.5526)}{4.55pt}{4.82pt}{} & \HoloSegScore{0.005648}{(0.002598--0.009657)}{3.85pt}{4.12pt}{} & \HoloSegScore{0.2784}{(0.2087--0.3438)}{4.55pt}{4.82pt}{} & \HoloSegScore{0.7108}{(0.6659--0.7724)}{4.55pt}{4.82pt}{} & \HoloSegScore{0.7639}{(0.7166--0.8089)}{4.55pt}{4.82pt}{} & \HoloSegScore{0.8040}{(0.7586--0.8439)}{4.55pt}{4.82pt}{} \\*
\softcline{4-4}\softcline{6-11}
 &  & \HoloSegSpan{\makecell[c]{pancreatic\\[-0.10ex]cyst}}{2.04cm}{0.32cm} & \HoloSegMetric{HD95} & \raisebox{0.32cm}[0pt][0pt]{\HoloSegUnsupported} & \HoloSegScore{16.05}{(13.56--18.98)}{4.55pt}{4.82pt}{} & \HoloSegScore{95.03}{(86.87--103.6)}{4.55pt}{4.82pt}{} & \HoloSegScore{29.16}{(17.67--42.84)}{4.55pt}{4.82pt}{} & \HoloSegScore{18.92}{(13.11--28.73)}{4.55pt}{4.82pt}{} & \HoloSegScore{17.73}{(12.08--23.86)}{4.55pt}{4.82pt}{} & \HoloSegScore{9.400}{(4.893--15.48)}{4.55pt}{4.82pt}{} \\
\cline{3-11}
 &  &  & \HoloSegMetric{Dice} & \HoloSegScore{0.3112}{(0.2537--0.3720)}{4.55pt}{4.82pt}{} & \HoloSegScore{0.05148}{(0.03418--0.07201)}{4.20pt}{4.48pt}{} & \HoloSegScore{0.07921}{(0.06116--0.09887)}{4.20pt}{4.48pt}{} & \HoloSegScore{0.0000}{(0.0000--0.0000)}{4.55pt}{4.82pt}{} & \HoloSegScore{0.7190}{(0.6718--0.7796)}{4.55pt}{4.82pt}{} & \HoloSegScore{0.8236}{(0.7919--0.8527)}{4.55pt}{4.82pt}{} & \HoloSegScore{0.8643}{(0.8420--0.8847)}{4.55pt}{4.82pt}{} \\*
\softcline{4-11}
 &  & \HoloSegSpan{\makecell[c]{kidney cyst}}{2.04cm}{0.32cm} & \HoloSegMetric{HD95} & \HoloSegScore{90.18}{(78.70--102.9)}{4.55pt}{4.82pt}{} & \HoloSegScore{98.92}{(89.19--108.4)}{4.55pt}{4.82pt}{} & \HoloSegScore{73.51}{(67.42--79.96)}{4.55pt}{4.82pt}{} & \HoloSegScore{--}{(--\,--)}{4.55pt}{4.82pt}{} & \HoloSegScore{25.64}{(17.95--37.42)}{4.55pt}{4.82pt}{} & \HoloSegScore{26.68}{(17.73--36.61)}{4.55pt}{4.82pt}{} & \HoloSegScore{20.05}{(13.54--27.38)}{4.55pt}{4.82pt}{} \\
\cline{3-11}
 &  &  & \HoloSegMetric{Dice} &  & \HoloSegScore{0.1707}{(0.1419--0.2009)}{4.55pt}{4.82pt}{} & \HoloSegScore{0.01014}{(0.005443--0.01647)}{3.85pt}{4.12pt}{} & \HoloSegScore{0.0000}{(0.0000--0.0000)}{4.55pt}{4.82pt}{} & \HoloSegScore{0.7153}{(0.6691--0.7818)}{4.55pt}{4.82pt}{} & \HoloSegScore{0.5778}{(0.5225--0.6277)}{4.55pt}{4.82pt}{} & \HoloSegScore{0.5190}{(0.4672--0.5714)}{4.55pt}{4.82pt}{} \\*
\softcline{4-4}\softcline{6-11}
 &  & \HoloSegSpan{\makecell[c]{kidney stone}}{2.04cm}{0.32cm} & \HoloSegMetric{HD95} & \raisebox{0.32cm}[0pt][0pt]{\HoloSegUnsupported} & \HoloSegScore{84.94}{(72.41--97.52)}{4.55pt}{4.82pt}{} & \HoloSegScore{106.4}{(96.56--116.0)}{4.55pt}{4.82pt}{} & \HoloSegScore{--}{(--\,--)}{4.55pt}{4.82pt}{} & \HoloSegScore{28.40}{(19.86--41.57)}{4.55pt}{4.82pt}{} & \HoloSegScore{49.32}{(38.38--60.23)}{4.55pt}{4.82pt}{} & \HoloSegScore{57.87}{(46.78--70.08)}{4.55pt}{4.82pt}{} \\
\cline{2-11}
 &  &  & \HoloSegMetric{Dice} & \HoloSegScore{0.7650}{(0.7571--0.7730)}{4.55pt}{4.82pt}{} & \HoloSegScore{0.2788}{(0.2680--0.2894)}{4.55pt}{4.82pt}{} & \HoloSegScore{0.7483}{(0.7393--0.7555)}{4.55pt}{4.82pt}{} & \HoloSegScore{0.7462}{(0.7368--0.7550)}{4.55pt}{4.82pt}{} & \HoloSegScore{0.7993}{(0.7761--0.8004)}{4.55pt}{4.82pt}{} & \HoloSegScore{0.8295}{(0.8233--0.8349)}{4.55pt}{4.82pt}{} & \HoloSegScore{0.8267}{(0.8212--0.8318)}{4.55pt}{4.82pt}{} \\*
\softcline{4-11}
 &  & \HoloSegSpan{\makecell[c]{left adrenal\\[-0.10ex]gland}}{2.04cm}{0.32cm} & \HoloSegMetric{HD95} & \HoloSegScore{4.087}{(3.670--4.587)}{4.55pt}{4.82pt}{} & \HoloSegScore{21.72}{(20.41--23.06)}{4.55pt}{4.82pt}{} & \HoloSegScore{4.808}{(3.624--6.391)}{4.55pt}{4.82pt}{} & \HoloSegScore{5.076}{(4.558--5.606)}{4.55pt}{4.82pt}{} & \HoloSegScore{6.599}{(6.083--8.839)}{4.55pt}{4.82pt}{} & \HoloSegScore{3.642}{(3.137--4.235)}{4.55pt}{4.82pt}{} & \HoloSegScore{4.604}{(3.963--5.334)}{4.55pt}{4.82pt}{} \\
\cline{3-11}
 &  &  & \HoloSegMetric{Dice} & \HoloSegScore{0.7105}{(0.7035--0.7166)}{4.55pt}{4.82pt}{} & \HoloSegScore{0.3388}{(0.3294--0.3486)}{4.55pt}{4.82pt}{} & \HoloSegScore{0.6825}{(0.6746--0.6907)}{4.55pt}{4.82pt}{} & \HoloSegScore{0.6876}{(0.6782--0.6957)}{4.55pt}{4.82pt}{} & \HoloSegScore{0.7390}{(0.7271--0.7430)}{4.55pt}{4.82pt}{} & \HoloSegScore{0.8195}{(0.8135--0.8254)}{4.55pt}{4.82pt}{} & \HoloSegScore{0.8124}{(0.8069--0.8180)}{4.55pt}{4.82pt}{} \\*
\softcline{4-11}
 &  & \HoloSegSpan{\makecell[c]{right\\[-0.10ex]adrenal\\[-0.10ex]gland}}{2.04cm}{0.32cm} & \HoloSegMetric{HD95} & \HoloSegScore{4.278}{(3.856--4.798)}{4.55pt}{4.82pt}{} & \HoloSegScore{17.89}{(16.54--19.43)}{4.55pt}{4.82pt}{} & \HoloSegScore{3.779}{(3.382--4.210)}{4.55pt}{4.82pt}{} & \HoloSegScore{4.883}{(4.434--5.440)}{4.55pt}{4.82pt}{} & \HoloSegScore{3.219}{(2.501--3.661)}{4.55pt}{4.82pt}{} & \HoloSegScore{4.699}{(3.786--5.929)}{4.55pt}{4.82pt}{} & \HoloSegScore{3.804}{(3.287--4.341)}{4.55pt}{4.82pt}{} \\
\cline{3-11}
 &  &  & \HoloSegMetric{Dice} & \HoloSegScore{0.8651}{(0.8589--0.8713)}{4.55pt}{4.82pt}{} & \HoloSegScore{0.7653}{(0.7587--0.7726)}{4.55pt}{4.82pt}{} & \HoloSegScore{0.8516}{(0.8449--0.8580)}{4.55pt}{4.82pt}{} & \HoloSegScore{0.8823}{(0.8768--0.8876)}{4.55pt}{4.82pt}{} & \HoloSegScore{0.8718}{(0.8620--0.8775)}{4.55pt}{4.82pt}{} & \HoloSegScore{0.9017}{(0.8961--0.9070)}{4.55pt}{4.82pt}{} & \HoloSegScore{0.9015}{(0.8960--0.9067)}{4.55pt}{4.82pt}{} \\*
\softcline{4-11}
 &  & \HoloSegSpan{\makecell[c]{aorta}}{2.04cm}{0.32cm} & \HoloSegMetric{HD95} & \HoloSegScore{29.72}{(27.84--31.94)}{4.55pt}{4.82pt}{} & \HoloSegScore{13.62}{(12.20--15.17)}{4.55pt}{4.82pt}{} & \HoloSegScore{34.58}{(31.94--37.23)}{4.55pt}{4.82pt}{} & \HoloSegScore{24.86}{(22.74--27.03)}{4.55pt}{4.82pt}{} & \HoloSegScore{15.05}{(13.92--16.54)}{4.55pt}{4.82pt}{} & \HoloSegScore{13.19}{(11.60--14.79)}{4.55pt}{4.82pt}{} & \HoloSegScore{13.35}{(11.82--14.96)}{4.55pt}{4.82pt}{} \\
\cline{3-11}
 &  &  & \HoloSegMetric{Dice} & \HoloSegScore{0.7610}{(0.7341--0.7882)}{4.55pt}{4.82pt}{} & \HoloSegScore{0.3943}{(0.3735--0.4181)}{4.55pt}{4.82pt}{} & \HoloSegScore{0.6965}{(0.6685--0.7243)}{4.55pt}{4.82pt}{} & \HoloSegScore{0.6662}{(0.6391--0.6928)}{4.55pt}{4.82pt}{} & \HoloSegScore{0.7558}{(0.7239--0.7862)}{4.55pt}{4.82pt}{} & \HoloSegScore{0.6983}{(0.6707--0.7253)}{4.55pt}{4.82pt}{} & \HoloSegScore{0.7063}{(0.6777--0.7337)}{4.55pt}{4.82pt}{} \\*
\softcline{4-11}
\HoloSegSpan{\makecell[c]{\textbf{Internal}}}{1.20cm}{0.32cm} &  & \HoloSegSpan{\makecell[c]{urinary\\[-0.10ex]bladder}}{2.04cm}{0.32cm} & \HoloSegMetric{HD95} & \HoloSegScore{16.54}{(13.33--20.07)}{4.55pt}{4.82pt}{} & \HoloSegScore{86.65}{(78.95--93.84)}{4.55pt}{4.82pt}{} & \HoloSegScore{14.47}{(10.61--18.84)}{4.55pt}{4.82pt}{} & \HoloSegScore{25.47}{(20.17--31.23)}{4.55pt}{4.82pt}{} & \HoloSegScore{17.17}{(11.41--19.18)}{4.55pt}{4.82pt}{} & \HoloSegScore{37.18}{(30.38--44.05)}{4.55pt}{4.82pt}{} & \HoloSegScore{51.67}{(44.15--60.22)}{4.55pt}{4.82pt}{} \\
\cline{3-11}
 &  &  & \HoloSegMetric{Dice} &  & \HoloSegScore{0.02728}{(0.02520--0.02949)}{4.20pt}{4.48pt}{} & \HoloSegScore{0.2691}{(0.2611--0.2769)}{4.55pt}{4.82pt}{} & \HoloSegScore{0.2524}{(0.2424--0.2619)}{4.55pt}{4.82pt}{} & \HoloSegScore{0.5306}{(0.5146--0.5448)}{4.55pt}{4.82pt}{} & \HoloSegScore{0.5901}{(0.5807--0.5989)}{4.55pt}{4.82pt}{} & \HoloSegScore{0.6144}{(0.6045--0.6234)}{4.55pt}{4.82pt}{} \\*
\softcline{4-4}\softcline{6-11}
 &  & \HoloSegSpan{\makecell[c]{celiac\\[-0.10ex]artery}}{2.04cm}{0.32cm} & \HoloSegMetric{HD95} & \raisebox{0.32cm}[0pt][0pt]{\HoloSegUnsupported} & \HoloSegScore{51.61}{(49.89--53.24)}{4.55pt}{4.82pt}{} & \HoloSegScore{52.48}{(51.06--54.13)}{4.55pt}{4.82pt}{} & \HoloSegScore{52.43}{(51.53--53.43)}{4.55pt}{4.82pt}{} & \HoloSegScore{15.57}{(12.99--15.69)}{4.55pt}{4.82pt}{} & \HoloSegScore{14.50}{(13.30--15.80)}{4.55pt}{4.82pt}{} & \HoloSegScore{12.27}{(11.32--13.28)}{4.55pt}{4.82pt}{} \\
\cline{3-11}
 &  &  & \HoloSegMetric{Dice} &  & \HoloSegScore{0.003588}{(0.002881--0.004415)}{3.85pt}{4.12pt}{} & \HoloSegScore{0.5584}{(0.5413--0.5736)}{4.55pt}{4.82pt}{} & \HoloSegScore{0.5017}{(0.4830--0.5200)}{4.55pt}{4.82pt}{} & \HoloSegScore{0.5682}{(0.5319--0.5734)}{4.55pt}{4.82pt}{} & \HoloSegScore{0.6290}{(0.6119--0.6460)}{4.55pt}{4.82pt}{} & \HoloSegScore{0.6711}{(0.6540--0.6875)}{4.55pt}{4.82pt}{} \\*
\softcline{4-4}\softcline{6-11}
 &  & \HoloSegSpan{\makecell[c]{celiac trunk}}{2.04cm}{0.32cm} & \HoloSegMetric{HD95} & \raisebox{0.32cm}[0pt][0pt]{\HoloSegUnsupported} & \HoloSegScore{77.53}{(74.52--80.92)}{4.55pt}{4.82pt}{} & \HoloSegScore{19.38}{(15.76--23.01)}{4.55pt}{4.82pt}{} & \HoloSegScore{20.76}{(17.92--23.65)}{4.55pt}{4.82pt}{} & \HoloSegScore{12.63}{(10.89--16.54)}{4.55pt}{4.82pt}{} & \HoloSegScore{23.91}{(20.38--27.48)}{4.55pt}{4.82pt}{} & \HoloSegScore{14.30}{(11.55--17.32)}{4.55pt}{4.82pt}{} \\
\cline{3-11}
 &  &  & \HoloSegMetric{Dice} & \HoloSegScore{0.8091}{(0.8013--0.8166)}{4.55pt}{4.82pt}{} & \HoloSegScore{0.2006}{(0.1870--0.2139)}{4.55pt}{4.82pt}{} & \HoloSegScore{0.7939}{(0.7858--0.8014)}{4.55pt}{4.82pt}{} & \HoloSegScore{0.6895}{(0.6765--0.7019)}{4.55pt}{4.82pt}{} & \HoloSegScore{0.8666}{(0.8558--0.8764)}{4.55pt}{4.82pt}{} & \HoloSegScore{0.8660}{(0.8603--0.8716)}{4.55pt}{4.82pt}{} & \HoloSegScore{0.8778}{(0.8721--0.8834)}{4.55pt}{4.82pt}{} \\*
\softcline{4-11}
 & \HoloSegSpan{\makecell[c]{AbdomenAtlas\\[-0.10ex]3.0}}{1.86cm}{0.32cm} & \HoloSegSpan{\makecell[c]{colon}}{2.04cm}{0.32cm} & \HoloSegMetric{HD95} & \HoloSegScore{40.78}{(37.68--44.58)}{4.55pt}{4.82pt}{} & \HoloSegScore{87.81}{(84.22--91.37)}{4.55pt}{4.82pt}{} & \HoloSegScore{26.99}{(25.22--28.74)}{4.55pt}{4.82pt}{} & \HoloSegScore{63.05}{(58.16--68.24)}{4.55pt}{4.82pt}{} & \HoloSegScore{30.13}{(27.88--33.51)}{4.55pt}{4.82pt}{} & \HoloSegScore{18.07}{(16.24--20.34)}{4.55pt}{4.82pt}{} & \HoloSegScore{19.95}{(17.01--23.28)}{4.55pt}{4.82pt}{} \\
\cline{3-11}
 &  &  & \HoloSegMetric{Dice} &  & \HoloSegScore{0.009287}{(0.007782--0.01110)}{3.85pt}{4.12pt}{} & \HoloSegScore{0.0000}{(0.0000--0.0000)}{4.55pt}{4.82pt}{} & \HoloSegScore{0.1886}{(0.1734--0.2035)}{4.55pt}{4.82pt}{} & \HoloSegScore{0.5641}{(0.5492--0.5682)}{4.55pt}{4.82pt}{} & \HoloSegScore{0.5712}{(0.5594--0.5824)}{4.55pt}{4.82pt}{} & \HoloSegScore{0.6131}{(0.6015--0.6246)}{4.55pt}{4.82pt}{} \\*
\softcline{4-4}\softcline{6-11}
 &  & \HoloSegSpan{\makecell[c]{common bile\\[-0.10ex]duct}}{2.04cm}{0.32cm} & \HoloSegMetric{HD95} & \raisebox{0.32cm}[0pt][0pt]{\HoloSegUnsupported} & \HoloSegScore{77.27}{(75.55--79.26)}{4.55pt}{4.82pt}{} & \HoloSegScore{135.2}{(117.3--157.0)}{4.55pt}{4.82pt}{} & \HoloSegScore{19.30}{(18.11--20.76)}{4.55pt}{4.82pt}{} & \HoloSegScore{9.119}{(8.284--9.133)}{4.55pt}{4.82pt}{} & \HoloSegScore{9.101}{(8.674--9.525)}{4.55pt}{4.82pt}{} & \HoloSegScore{8.856}{(7.804--10.09)}{4.55pt}{4.82pt}{} \\
\cline{3-11}
 &  &  & \HoloSegMetric{Dice} & \HoloSegScore{0.7783}{(0.7719--0.7847)}{4.55pt}{4.82pt}{} & \HoloSegScore{0.4695}{(0.4601--0.4785)}{4.55pt}{4.82pt}{} & \HoloSegScore{0.7657}{(0.7576--0.7729)}{4.55pt}{4.82pt}{} & \HoloSegScore{0.7390}{(0.7290--0.7482)}{4.55pt}{4.82pt}{} & \HoloSegScore{0.8393}{(0.8312--0.8533)}{4.55pt}{4.82pt}{} & \HoloSegScore{0.8258}{(0.8192--0.8322)}{4.55pt}{4.82pt}{} & \HoloSegScore{0.8461}{(0.8400--0.8515)}{4.55pt}{4.82pt}{} \\*
\softcline{4-11}
 &  & \HoloSegSpan{\makecell[c]{duodenum}}{2.04cm}{0.32cm} & \HoloSegMetric{HD95} & \HoloSegScore{13.76}{(12.52--15.42)}{4.55pt}{4.82pt}{} & \HoloSegScore{22.02}{(20.89--23.35)}{4.55pt}{4.82pt}{} & \HoloSegScore{10.76}{(9.866--11.74)}{4.55pt}{4.82pt}{} & \HoloSegScore{16.45}{(15.54--17.27)}{4.55pt}{4.82pt}{} & \HoloSegScore{8.450}{(8.357--8.499)}{4.55pt}{4.82pt}{} & \HoloSegScore{10.82}{(9.553--12.30)}{4.55pt}{4.82pt}{} & \HoloSegScore{8.857}{(7.713--10.47)}{4.55pt}{4.82pt}{} \\
\cline{3-11}
 &  &  & \HoloSegMetric{Dice} & \HoloSegScore{0.7541}{(0.7454--0.7624)}{4.55pt}{4.82pt}{} & \HoloSegScore{0.4656}{(0.4535--0.4767)}{4.55pt}{4.82pt}{} & \HoloSegScore{0.7561}{(0.7468--0.7645)}{4.55pt}{4.82pt}{} & \HoloSegScore{0.7425}{(0.7327--0.7515)}{4.55pt}{4.82pt}{} & \HoloSegScore{0.7543}{(0.7499--0.7647)}{4.55pt}{4.82pt}{} & \HoloSegScore{0.8015}{(0.7936--0.8094)}{4.55pt}{4.82pt}{} & \HoloSegScore{0.7946}{(0.7868--0.8026)}{4.55pt}{4.82pt}{} \\*
\softcline{4-11}
 &  & \HoloSegSpan{\makecell[c]{esophagus}}{2.04cm}{0.32cm} & \HoloSegMetric{HD95} & \HoloSegScore{35.49}{(31.49--39.72)}{4.55pt}{4.82pt}{} & \HoloSegScore{20.98}{(19.36--22.74)}{4.55pt}{4.82pt}{} & \HoloSegScore{17.22}{(15.08--19.16)}{4.55pt}{4.82pt}{} & \HoloSegScore{16.31}{(14.68--18.02)}{4.55pt}{4.82pt}{} & \HoloSegScore{15.28}{(12.55--17.77)}{4.55pt}{4.82pt}{} & \HoloSegScore{17.16}{(15.30--19.12)}{4.55pt}{4.82pt}{} & \HoloSegScore{17.19}{(15.31--19.20)}{4.55pt}{4.82pt}{} \\
\cline{3-11}
 &  &  & \HoloSegMetric{Dice} & \HoloSegScore{0.6586}{(0.6237--0.6938)}{4.55pt}{4.82pt}{} & \HoloSegScore{0.4990}{(0.4716--0.5238)}{4.55pt}{4.82pt}{} & \HoloSegScore{0.6362}{(0.6021--0.6696)}{4.55pt}{4.82pt}{} & \HoloSegScore{0.6750}{(0.6425--0.7063)}{4.55pt}{4.82pt}{} & \HoloSegScore{0.8216}{(0.7872--0.8446)}{4.55pt}{4.82pt}{} & \HoloSegScore{0.7515}{(0.7242--0.7750)}{4.55pt}{4.82pt}{} & \HoloSegScore{0.7624}{(0.7383--0.7864)}{4.55pt}{4.82pt}{} \\*
\softcline{4-11}
 &  & \HoloSegSpan{\makecell[c]{left femur}}{2.04cm}{0.32cm} & \HoloSegMetric{HD95} & \HoloSegScore{34.07}{(33.27--34.86)}{4.55pt}{4.82pt}{} & \HoloSegScore{82.03}{(74.45--90.22)}{4.55pt}{4.82pt}{} & \HoloSegScore{154.0}{(138.8--169.4)}{4.55pt}{4.82pt}{} & \HoloSegScore{72.90}{(63.18--81.70)}{4.55pt}{4.82pt}{} & \HoloSegScore{49.50}{(43.22--58.01)}{4.55pt}{4.82pt}{} & \HoloSegScore{117.7}{(107.5--128.6)}{4.55pt}{4.82pt}{} & \HoloSegScore{107.4}{(98.92--115.6)}{4.55pt}{4.82pt}{} \\
\cline{3-11}
 &  &  & \HoloSegMetric{Dice} & \HoloSegScore{0.6249}{(0.5891--0.6603)}{4.55pt}{4.82pt}{} & \HoloSegScore{0.4810}{(0.4567--0.5055)}{4.55pt}{4.82pt}{} & \HoloSegScore{0.6058}{(0.5707--0.6368)}{4.55pt}{4.82pt}{} & \HoloSegScore{0.6638}{(0.6278--0.6966)}{4.55pt}{4.82pt}{} & \HoloSegScore{0.7936}{(0.7850--0.8074)}{4.55pt}{4.82pt}{} & \HoloSegScore{0.7210}{(0.6921--0.7473)}{4.55pt}{4.82pt}{} & \HoloSegScore{0.7384}{(0.7078--0.7665)}{4.55pt}{4.82pt}{} \\*
\softcline{4-11}
 &  & \HoloSegSpan{\makecell[c]{right femur}}{2.04cm}{0.32cm} & \HoloSegMetric{HD95} & \HoloSegScore{229.5}{(211.1--247.8)}{4.55pt}{4.82pt}{} & \HoloSegScore{127.6}{(119.1--135.6)}{4.55pt}{4.82pt}{} & \HoloSegScore{175.7}{(159.1--194.7)}{4.55pt}{4.82pt}{} & \HoloSegScore{62.44}{(53.87--71.29)}{4.55pt}{4.82pt}{} & \HoloSegScore{45.53}{(39.63--52.37)}{4.55pt}{4.82pt}{} & \HoloSegScore{113.0}{(103.1--122.8)}{4.55pt}{4.82pt}{} & \HoloSegScore{85.94}{(77.80--94.24)}{4.55pt}{4.82pt}{} \\
\cline{3-11}
 &  &  & \HoloSegMetric{Dice} & \HoloSegScore{0.7897}{(0.7716--0.8078)}{4.55pt}{4.82pt}{} & \HoloSegScore{0.4004}{(0.3830--0.4195)}{4.55pt}{4.82pt}{} & \HoloSegScore{0.7723}{(0.7546--0.7894)}{4.55pt}{4.82pt}{} & \HoloSegScore{0.7636}{(0.7430--0.7814)}{4.55pt}{4.82pt}{} & \HoloSegScore{0.8220}{(0.8051--0.8239)}{4.55pt}{4.82pt}{} & \HoloSegScore{0.8358}{(0.8212--0.8498)}{4.55pt}{4.82pt}{} & \HoloSegScore{0.8347}{(0.8192--0.8486)}{4.55pt}{4.82pt}{} \\*
\softcline{4-11}
 &  & \HoloSegSpan{\makecell[c]{gallbladder}}{2.04cm}{0.32cm} & \HoloSegMetric{HD95} & \HoloSegScore{10.98}{(9.099--13.27)}{4.55pt}{4.82pt}{} & \HoloSegScore{37.03}{(34.13--40.14)}{4.55pt}{4.82pt}{} & \HoloSegScore{7.786}{(6.727--8.931)}{4.55pt}{4.82pt}{} & \HoloSegScore{11.61}{(10.18--13.20)}{4.55pt}{4.82pt}{} & \HoloSegScore{7.270}{(6.360--7.973)}{4.55pt}{4.82pt}{} & \HoloSegScore{7.792}{(6.896--8.740)}{4.55pt}{4.82pt}{} & \HoloSegScore{9.688}{(7.594--12.14)}{4.55pt}{4.82pt}{} \\
\hline
\pagebreak[4]
 &  &  & \HoloSegMetric{Dice} & \HoloSegScore{0.4706}{(0.4561--0.4864)}{4.55pt}{4.82pt}{} & \HoloSegScore{0.06012}{(0.05445--0.06569)}{4.20pt}{4.48pt}{} & \HoloSegScore{0.4884}{(0.4726--0.5028)}{4.55pt}{4.82pt}{} & \HoloSegScore{0.2513}{(0.2407--0.2617)}{4.55pt}{4.82pt}{} & \HoloSegScore{0.4980}{(0.4807--0.5089)}{4.55pt}{4.82pt}{} & \HoloSegScore{0.5590}{(0.5449--0.5721)}{4.55pt}{4.82pt}{} & \HoloSegScore{0.5906}{(0.5765--0.6037)}{4.55pt}{4.82pt}{} \\*
\softcline{4-11}
 &  & \HoloSegSpan{\makecell[c]{hepatic vein}}{2.04cm}{0.32cm} & \HoloSegMetric{HD95} & \HoloSegScore{30.83}{(29.36--32.34)}{4.55pt}{4.82pt}{} & \HoloSegScore{62.55}{(60.43--64.79)}{4.55pt}{4.82pt}{} & \HoloSegScore{28.35}{(26.35--30.74)}{4.55pt}{4.82pt}{} & \HoloSegScore{55.53}{(54.00--57.09)}{4.55pt}{4.82pt}{} & \HoloSegScore{29.01}{(26.59--32.53)}{4.55pt}{4.82pt}{} & \HoloSegScore{26.03}{(24.53--27.86)}{4.55pt}{4.82pt}{} & \HoloSegScore{22.64}{(21.22--24.23)}{4.55pt}{4.82pt}{} \\
\cline{3-11}
 &  &  & \HoloSegMetric{Dice} &  & \HoloSegScore{0.2127}{(0.1994--0.2272)}{4.55pt}{4.82pt}{} & \HoloSegScore{0.8005}{(0.7935--0.8077)}{4.55pt}{4.82pt}{} & \HoloSegScore{0.6354}{(0.6270--0.6444)}{4.55pt}{4.82pt}{} & \HoloSegScore{0.8575}{(0.8558--0.8868)}{4.55pt}{4.82pt}{} & \HoloSegScore{0.8630}{(0.8573--0.8678)}{4.55pt}{4.82pt}{} & \HoloSegScore{0.8664}{(0.8610--0.8712)}{4.55pt}{4.82pt}{} \\*
\softcline{4-4}\softcline{6-11}
 &  & \HoloSegSpan{\makecell[c]{intestine}}{2.04cm}{0.32cm} & \HoloSegMetric{HD95} & \raisebox{0.32cm}[0pt][0pt]{\HoloSegUnsupported} & \HoloSegScore{81.55}{(78.74--84.60)}{4.55pt}{4.82pt}{} & \HoloSegScore{13.93}{(12.97--15.11)}{4.55pt}{4.82pt}{} & \HoloSegScore{55.41}{(53.01--57.93)}{4.55pt}{4.82pt}{} & \HoloSegScore{13.52}{(11.08--15.26)}{4.55pt}{4.82pt}{} & \HoloSegScore{11.48}{(10.61--12.40)}{4.55pt}{4.82pt}{} & \HoloSegScore{11.35}{(10.46--12.37)}{4.55pt}{4.82pt}{} \\
\cline{3-11}
 &  &  & \HoloSegMetric{Dice} & \HoloSegScore{0.9243}{(0.9173--0.9308)}{4.55pt}{4.82pt}{} & \HoloSegScore{0.7681}{(0.7605--0.7762)}{4.55pt}{4.82pt}{} & \HoloSegScore{0.9164}{(0.9094--0.9231)}{4.55pt}{4.82pt}{} & \HoloSegScore{0.9316}{(0.9253--0.9380)}{4.55pt}{4.82pt}{} & \HoloSegScore{0.9190}{(0.8993--0.9303)}{4.55pt}{4.82pt}{} & \HoloSegScore{0.9446}{(0.9378--0.9507)}{4.55pt}{4.82pt}{} & \HoloSegScore{0.9432}{(0.9358--0.9495)}{4.55pt}{4.82pt}{} \\*
\softcline{4-11}
 &  & \HoloSegSpan{\makecell[c]{left kidney}}{2.04cm}{0.32cm} & \HoloSegMetric{HD95} & \HoloSegScore{6.562}{(5.666--7.738)}{4.55pt}{4.82pt}{} & \HoloSegScore{44.13}{(40.48--47.37)}{4.55pt}{4.82pt}{} & \HoloSegScore{6.370}{(5.282--7.583)}{4.55pt}{4.82pt}{} & \HoloSegScore{5.649}{(4.906--6.495)}{4.55pt}{4.82pt}{} & \HoloSegScore{6.265}{(5.196--7.706)}{4.55pt}{4.82pt}{} & \HoloSegScore{4.750}{(3.807--5.770)}{4.55pt}{4.82pt}{} & \HoloSegScore{4.517}{(3.747--5.320)}{4.55pt}{4.82pt}{} \\
\cline{3-11}
 &  &  & \HoloSegMetric{Dice} &  & \HoloSegScore{0.2352}{(0.1965--0.2734)}{4.55pt}{4.82pt}{} & \HoloSegScore{0.00000001668}{(0.0000--0.00000005005)}{3.52pt}{3.80pt}{} & \HoloSegScore{0.3382}{(0.2926--0.3862)}{4.55pt}{4.82pt}{} & \HoloSegScore{0.6902}{(0.6877--0.6956)}{4.55pt}{4.82pt}{} & \HoloSegScore{0.5990}{(0.5575--0.6357)}{4.55pt}{4.82pt}{} & \HoloSegScore{0.6667}{(0.6323--0.6999)}{4.55pt}{4.82pt}{} \\*
\softcline{4-4}\softcline{6-11}
 &  & \HoloSegSpan{\makecell[c]{kidney\\[-0.10ex]lesion}}{2.04cm}{0.32cm} & \HoloSegMetric{HD95} & \raisebox{0.32cm}[0pt][0pt]{\HoloSegUnsupported} & \HoloSegScore{103.6}{(94.81--112.5)}{4.55pt}{4.82pt}{} & \HoloSegScore{282.4}{(242.9--316.0)}{4.55pt}{4.82pt}{} & \HoloSegScore{100.7}{(86.55--116.1)}{4.55pt}{4.82pt}{} & \HoloSegScore{30.88}{(24.86--41.08)}{4.55pt}{4.82pt}{} & \HoloSegScore{39.23}{(31.93--46.49)}{4.55pt}{4.82pt}{} & \HoloSegScore{39.48}{(33.32--46.10)}{4.55pt}{4.82pt}{} \\
\cline{3-11}
 &  &  & \HoloSegMetric{Dice} & \HoloSegScore{0.9269}{(0.9205--0.9328)}{4.55pt}{4.82pt}{} & \HoloSegScore{0.7719}{(0.7640--0.7794)}{4.55pt}{4.82pt}{} & \HoloSegScore{0.9241}{(0.9169--0.9304)}{4.55pt}{4.82pt}{} & \HoloSegScore{0.9299}{(0.9227--0.9366)}{4.55pt}{4.82pt}{} & \HoloSegScore{0.9158}{(0.9075--0.9211)}{4.55pt}{4.82pt}{} & \HoloSegScore{0.9547}{(0.9501--0.9585)}{4.55pt}{4.82pt}{} & \HoloSegScore{0.9559}{(0.9513--0.9599)}{4.55pt}{4.82pt}{} \\*
\softcline{4-11}
 &  & \HoloSegSpan{\makecell[c]{right kidney}}{2.04cm}{0.32cm} & \HoloSegMetric{HD95} & \HoloSegScore{7.516}{(6.441--8.757)}{4.55pt}{4.82pt}{} & \HoloSegScore{48.09}{(44.58--51.57)}{4.55pt}{4.82pt}{} & \HoloSegScore{5.636}{(4.764--6.727)}{4.55pt}{4.82pt}{} & \HoloSegScore{6.810}{(5.900--7.838)}{4.55pt}{4.82pt}{} & \HoloSegScore{6.163}{(4.900--7.583)}{4.55pt}{4.82pt}{} & \HoloSegScore{4.418}{(3.370--5.707)}{4.55pt}{4.82pt}{} & \HoloSegScore{3.300}{(2.817--3.830)}{4.55pt}{4.82pt}{} \\
\cline{3-11}
 &  &  & \HoloSegMetric{Dice} & \HoloSegScore{0.9699}{(0.9680--0.9718)}{4.55pt}{4.82pt}{} & \HoloSegScore{0.8725}{(0.8689--0.8762)}{4.55pt}{4.82pt}{} & \HoloSegScore{0.9666}{(0.9651--0.9681)}{4.55pt}{4.82pt}{} & \HoloSegScore{0.9691}{(0.9673--0.9707)}{4.55pt}{4.82pt}{} & \HoloSegScore{0.9621}{(0.9609--0.9714)}{4.55pt}{4.82pt}{} & \HoloSegScore{0.9736}{(0.9719--0.9750)}{4.55pt}{4.82pt}{} & \HoloSegScore{0.9724}{(0.9708--0.9738)}{4.55pt}{4.82pt}{} \\*
\softcline{4-11}
 &  & \HoloSegSpan{\makecell[c]{liver}}{2.04cm}{0.32cm} & \HoloSegMetric{HD95} & \HoloSegScore{18.24}{(14.07--22.60)}{4.55pt}{4.82pt}{} & \HoloSegScore{11.79}{(11.34--12.30)}{4.55pt}{4.82pt}{} & \HoloSegScore{3.915}{(3.525--4.366)}{4.55pt}{4.82pt}{} & \HoloSegScore{8.304}{(6.995--9.789)}{4.55pt}{4.82pt}{} & \HoloSegScore{8.300}{(5.619--9.131)}{4.55pt}{4.82pt}{} & \HoloSegScore{4.308}{(3.831--4.797)}{4.55pt}{4.82pt}{} & \HoloSegScore{4.297}{(3.806--4.819)}{4.55pt}{4.82pt}{} \\
\cline{3-11}
 &  &  & \HoloSegMetric{Dice} & \HoloSegScore{0.5379}{(0.4548--0.6162)}{4.55pt}{4.82pt}{} & \HoloSegScore{0.1881}{(0.1427--0.2382)}{4.55pt}{4.82pt}{} & \HoloSegScore{0.3760}{(0.3319--0.4223)}{4.55pt}{4.82pt}{} & \HoloSegScore{0.5086}{(0.4621--0.5528)}{4.55pt}{4.82pt}{} & \HoloSegScore{0.6286}{(0.5803--0.6713)}{4.55pt}{4.82pt}{} & \HoloSegScore{0.6848}{(0.6557--0.7116)}{4.55pt}{4.82pt}{} & \HoloSegScore{0.6800}{(0.6482--0.7099)}{4.55pt}{4.82pt}{} \\*
\softcline{4-11}
 &  & \HoloSegSpan{\makecell[c]{liver lesion}}{2.04cm}{0.32cm} & \HoloSegMetric{HD95} & \HoloSegScore{75.95}{(47.65--109.8)}{4.55pt}{4.82pt}{} & \HoloSegScore{95.82}{(86.04--104.9)}{4.55pt}{4.82pt}{} & \HoloSegScore{52.29}{(39.01--66.55)}{4.55pt}{4.82pt}{} & \HoloSegScore{61.50}{(51.60--72.13)}{4.55pt}{4.82pt}{} & \HoloSegScore{32.20}{(27.03--40.36)}{4.55pt}{4.82pt}{} & \HoloSegScore{26.20}{(21.70--31.36)}{4.55pt}{4.82pt}{} & \HoloSegScore{42.32}{(36.23--48.52)}{4.55pt}{4.82pt}{} \\
\cline{3-11}
 &  &  & \HoloSegMetric{Dice} &  & \HoloSegScore{0.02273}{(0.01939--0.02635)}{4.20pt}{4.48pt}{} & \HoloSegScore{0.6012}{(0.5887--0.6144)}{4.55pt}{4.82pt}{} & \HoloSegScore{0.4472}{(0.4367--0.4578)}{4.55pt}{4.82pt}{} & \HoloSegScore{0.7899}{(0.7881--0.7907)}{4.55pt}{4.82pt}{} & \HoloSegScore{0.8236}{(0.8172--0.8297)}{4.55pt}{4.82pt}{} & \HoloSegScore{0.8207}{(0.8141--0.8273)}{4.55pt}{4.82pt}{} \\*
\softcline{4-4}\softcline{6-11}
 &  & \HoloSegSpan{\makecell[c]{caudate lobe}}{2.04cm}{0.32cm} & \HoloSegMetric{HD95} & \raisebox{0.32cm}[0pt][0pt]{\HoloSegUnsupported} & \HoloSegScore{154.4}{(148.8--159.9)}{4.55pt}{4.82pt}{} & \HoloSegScore{124.9}{(116.1--134.3)}{4.55pt}{4.82pt}{} & \HoloSegScore{27.17}{(26.50--28.00)}{4.55pt}{4.82pt}{} & \HoloSegScore{8.128}{(7.078--8.463)}{4.55pt}{4.82pt}{} & \HoloSegScore{7.140}{(6.782--7.495)}{4.55pt}{4.82pt}{} & \HoloSegScore{6.837}{(6.534--7.155)}{4.55pt}{4.82pt}{} \\
\cline{3-11}
 &  &  & \HoloSegMetric{Dice} &  & \HoloSegScore{0.0000}{(0.0000--0.0000)}{4.55pt}{4.82pt}{} & \HoloSegScore{0.7362}{(0.7241--0.7468)}{4.55pt}{4.82pt}{} & \HoloSegScore{0.7302}{(0.7188--0.7407)}{4.55pt}{4.82pt}{} & \HoloSegScore{0.8985}{(0.8876--0.9059)}{4.55pt}{4.82pt}{} & \HoloSegScore{0.9114}{(0.9062--0.9157)}{4.55pt}{4.82pt}{} & \HoloSegScore{0.9055}{(0.9003--0.9100)}{4.55pt}{4.82pt}{} \\*
\softcline{4-4}\softcline{6-11}
 &  & \HoloSegSpan{\makecell[c]{left lateral\\[-0.10ex]superior\\[-0.10ex]segment of\\[-0.10ex]liver}}{2.04cm}{0.32cm} & \HoloSegMetric{HD95} & \raisebox{0.32cm}[0pt][0pt]{\HoloSegUnsupported} & \HoloSegScore{133.2}{(131.5--135.1)}{4.55pt}{4.82pt}{} & \HoloSegScore{29.90}{(27.37--32.69)}{4.55pt}{4.82pt}{} & \HoloSegScore{19.53}{(18.64--20.59)}{4.55pt}{4.82pt}{} & \HoloSegScore{5.728}{(4.197--7.049)}{4.55pt}{4.82pt}{} & \HoloSegScore{6.452}{(5.981--6.946)}{4.55pt}{4.82pt}{} & \HoloSegScore{5.936}{(5.548--6.424)}{4.55pt}{4.82pt}{} \\
\cline{3-11}
 &  &  & \HoloSegMetric{Dice} &  & \HoloSegScore{0.0000}{(0.0000--0.0000)}{4.55pt}{4.82pt}{} & \HoloSegScore{0.6724}{(0.6583--0.6875)}{4.55pt}{4.82pt}{} & \HoloSegScore{0.6725}{(0.6615--0.6824)}{4.55pt}{4.82pt}{} & \HoloSegScore{0.8418}{(0.8291--0.8463)}{4.55pt}{4.82pt}{} & \HoloSegScore{0.8879}{(0.8810--0.8945)}{4.55pt}{4.82pt}{} & \HoloSegScore{0.8828}{(0.8755--0.8894)}{4.55pt}{4.82pt}{} \\*
\softcline{4-4}\softcline{6-11}
\HoloSegSpan{\makecell[c]{\textbf{Internal}}}{1.20cm}{0.32cm} & \HoloSegSpan{\makecell[c]{AbdomenAtlas\\[-0.10ex]3.0}}{1.86cm}{0.32cm} & \HoloSegSpan{\makecell[c]{left lateral\\[-0.10ex]inferior\\[-0.10ex]segment of\\[-0.10ex]liver}}{2.04cm}{0.32cm} & \HoloSegMetric{HD95} & \raisebox{0.32cm}[0pt][0pt]{\HoloSegUnsupported} & \HoloSegScore{146.2}{(144.1--148.2)}{4.55pt}{4.82pt}{} & \HoloSegScore{20.01}{(17.78--22.68)}{4.55pt}{4.82pt}{} & \HoloSegScore{26.83}{(25.64--28.11)}{4.55pt}{4.82pt}{} & \HoloSegScore{7.668}{(6.665--9.803)}{4.55pt}{4.82pt}{} & \HoloSegScore{6.121}{(5.636--6.742)}{4.55pt}{4.82pt}{} & \HoloSegScore{6.640}{(6.014--7.277)}{4.55pt}{4.82pt}{} \\
\cline{3-11}
 &  &  & \HoloSegMetric{Dice} &  & \HoloSegScore{0.0001119}{(0.0000--0.0003358)}{3.85pt}{4.12pt}{} & \HoloSegScore{0.4737}{(0.4557--0.4914)}{4.55pt}{4.82pt}{} & \HoloSegScore{0.6394}{(0.6259--0.6537)}{4.55pt}{4.82pt}{} & \HoloSegScore{0.8833}{(0.8819--0.8911)}{4.55pt}{4.82pt}{} & \HoloSegScore{0.8733}{(0.8668--0.8795)}{4.55pt}{4.82pt}{} & \HoloSegScore{0.8844}{(0.8777--0.8904)}{4.55pt}{4.82pt}{} \\*
\softcline{4-4}\softcline{6-11}
 &  & \HoloSegSpan{\makecell[c]{left medial\\[-0.10ex]segment of\\[-0.10ex]liver}}{2.04cm}{0.32cm} & \HoloSegMetric{HD95} & \raisebox{0.32cm}[0pt][0pt]{\HoloSegUnsupported} & \HoloSegScore{161.3}{(159.5--163.2)}{4.55pt}{4.82pt}{} & \HoloSegScore{42.59}{(39.92--45.35)}{4.55pt}{4.82pt}{} & \HoloSegScore{31.31}{(30.11--32.55)}{4.55pt}{4.82pt}{} & \HoloSegScore{9.313}{(8.210--10.93)}{4.55pt}{4.82pt}{} & \HoloSegScore{11.70}{(10.72--12.89)}{4.55pt}{4.82pt}{} & \HoloSegScore{7.633}{(6.970--8.428)}{4.55pt}{4.82pt}{} \\
\cline{3-11}
 &  &  & \HoloSegMetric{Dice} &  & \HoloSegScore{0.004746}{(0.003353--0.006413)}{3.85pt}{4.12pt}{} & \HoloSegScore{0.4646}{(0.4470--0.4824)}{4.55pt}{4.82pt}{} & \HoloSegScore{0.6710}{(0.6602--0.6820)}{4.55pt}{4.82pt}{} & \HoloSegScore{0.8840}{(0.8708--0.8921)}{4.55pt}{4.82pt}{} & \HoloSegScore{0.8849}{(0.8775--0.8925)}{4.55pt}{4.82pt}{} & \HoloSegScore{0.8789}{(0.8707--0.8863)}{4.55pt}{4.82pt}{} \\*
\softcline{4-4}\softcline{6-11}
 &  & \HoloSegSpan{\makecell[c]{right\\[-0.10ex]anterior\\[-0.10ex]inferior\\[-0.10ex]segment of\\[-0.10ex]liver}}{2.04cm}{0.32cm} & \HoloSegMetric{HD95} & \raisebox{0.32cm}[0pt][0pt]{\HoloSegUnsupported} & \HoloSegScore{88.80}{(86.67--90.97)}{4.55pt}{4.82pt}{} & \HoloSegScore{37.44}{(34.01--41.35)}{4.55pt}{4.82pt}{} & \HoloSegScore{26.70}{(24.71--28.97)}{4.55pt}{4.82pt}{} & \HoloSegScore{9.850}{(8.409--12.29)}{4.55pt}{4.82pt}{} & \HoloSegScore{10.29}{(8.802--11.96)}{4.55pt}{4.82pt}{} & \HoloSegScore{11.09}{(9.585--12.69)}{4.55pt}{4.82pt}{} \\
\cline{3-11}
 &  &  & \HoloSegMetric{Dice} &  & \HoloSegScore{0.01492}{(0.01234--0.01768)}{4.20pt}{4.48pt}{} & \HoloSegScore{0.4959}{(0.4810--0.5105)}{4.55pt}{4.82pt}{} & \HoloSegScore{0.6315}{(0.6221--0.6413)}{4.55pt}{4.82pt}{} & \HoloSegScore{0.8588}{(0.8374--0.8664)}{4.55pt}{4.82pt}{} & \HoloSegScore{0.8733}{(0.8654--0.8803)}{4.55pt}{4.82pt}{} & \HoloSegScore{0.8780}{(0.8702--0.8849)}{4.55pt}{4.82pt}{} \\*
\softcline{4-4}\softcline{6-11}
 &  & \HoloSegSpan{\makecell[c]{right\\[-0.10ex]posterior\\[-0.10ex]inferior\\[-0.10ex]segment of\\[-0.10ex]liver}}{2.04cm}{0.32cm} & \HoloSegMetric{HD95} & \raisebox{0.32cm}[0pt][0pt]{\HoloSegUnsupported} & \HoloSegScore{78.61}{(75.09--82.56)}{4.55pt}{4.82pt}{} & \HoloSegScore{30.55}{(28.03--33.41)}{4.55pt}{4.82pt}{} & \HoloSegScore{38.66}{(35.24--42.40)}{4.55pt}{4.82pt}{} & \HoloSegScore{20.98}{(16.32--23.63)}{4.55pt}{4.82pt}{} & \HoloSegScore{14.45}{(11.59--17.30)}{4.55pt}{4.82pt}{} & \HoloSegScore{15.29}{(12.40--18.61)}{4.55pt}{4.82pt}{} \\
\cline{3-11}
 &  &  & \HoloSegMetric{Dice} &  & \HoloSegScore{0.006630}{(0.005476--0.008073)}{3.85pt}{4.12pt}{} & \HoloSegScore{0.5426}{(0.5263--0.5577)}{4.55pt}{4.82pt}{} & \HoloSegScore{0.6981}{(0.6883--0.7068)}{4.55pt}{4.82pt}{} & \HoloSegScore{0.8481}{(0.8434--0.8601)}{4.55pt}{4.82pt}{} & \HoloSegScore{0.8980}{(0.8917--0.9037)}{4.55pt}{4.82pt}{} & \HoloSegScore{0.9092}{(0.9032--0.9146)}{4.55pt}{4.82pt}{} \\*
\softcline{4-4}\softcline{6-11}
 &  & \HoloSegSpan{\makecell[c]{right\\[-0.10ex]posterior\\[-0.10ex]superior\\[-0.10ex]segment of\\[-0.10ex]liver}}{2.04cm}{0.32cm} & \HoloSegMetric{HD95} & \raisebox{0.32cm}[0pt][0pt]{\HoloSegUnsupported} & \HoloSegScore{106.3}{(102.0--111.2)}{4.55pt}{4.82pt}{} & \HoloSegScore{48.56}{(45.00--52.39)}{4.55pt}{4.82pt}{} & \HoloSegScore{43.86}{(39.45--48.60)}{4.55pt}{4.82pt}{} & \HoloSegScore{22.79}{(19.18--27.13)}{4.55pt}{4.82pt}{} & \HoloSegScore{14.12}{(11.16--17.79)}{4.55pt}{4.82pt}{} & \HoloSegScore{13.67}{(10.61--17.47)}{4.55pt}{4.82pt}{} \\
\cline{3-11}
 &  &  & \HoloSegMetric{Dice} &  & \HoloSegScore{0.0002546}{(0.00007141--0.0004958)}{3.52pt}{3.80pt}{} & \HoloSegScore{0.3987}{(0.3795--0.4180)}{4.55pt}{4.82pt}{} & \HoloSegScore{0.6655}{(0.6557--0.6751)}{4.55pt}{4.82pt}{} & \HoloSegScore{0.8822}{(0.8736--0.8944)}{4.55pt}{4.82pt}{} & \HoloSegScore{0.8838}{(0.8779--0.8896)}{4.55pt}{4.82pt}{} & \HoloSegScore{0.8957}{(0.8900--0.9012)}{4.55pt}{4.82pt}{} \\*
\softcline{4-4}\softcline{6-11}
 &  & \HoloSegSpan{\makecell[c]{right\\[-0.10ex]anterior\\[-0.10ex]superior\\[-0.10ex]segment of\\[-0.10ex]liver}}{2.04cm}{0.32cm} & \HoloSegMetric{HD95} & \raisebox{0.32cm}[0pt][0pt]{\HoloSegUnsupported} & \HoloSegScore{117.3}{(114.3--120.5)}{4.55pt}{4.82pt}{} & \HoloSegScore{47.12}{(44.97--49.37)}{4.55pt}{4.82pt}{} & \HoloSegScore{40.47}{(37.21--43.93)}{4.55pt}{4.82pt}{} & \HoloSegScore{17.12}{(15.83--20.93)}{4.55pt}{4.82pt}{} & \HoloSegScore{12.25}{(9.878--15.14)}{4.55pt}{4.82pt}{} & \HoloSegScore{11.67}{(9.352--14.37)}{4.55pt}{4.82pt}{} \\
\cline{3-11}
 &  &  & \HoloSegMetric{Dice} & \HoloSegScore{0.9262}{(0.9173--0.9346)}{4.55pt}{4.82pt}{} & \HoloSegScore{0.7406}{(0.7270--0.7536)}{4.55pt}{4.82pt}{} & \HoloSegScore{0.9254}{(0.9175--0.9327)}{4.55pt}{4.82pt}{} & \HoloSegScore{0.9231}{(0.9139--0.9319)}{4.55pt}{4.82pt}{} & \HoloSegScore{0.9367}{(0.9312--0.9540)}{4.55pt}{4.82pt}{} & \HoloSegScore{0.9497}{(0.9427--0.9558)}{4.55pt}{4.82pt}{} & \HoloSegScore{0.9507}{(0.9438--0.9568)}{4.55pt}{4.82pt}{} \\*
\softcline{4-11}
 &  & \HoloSegSpan{\makecell[c]{left lung}}{2.04cm}{0.32cm} & \HoloSegMetric{HD95} & \HoloSegScore{13.33}{(11.55--15.38)}{4.55pt}{4.82pt}{} & \HoloSegScore{30.46}{(27.84--33.43)}{4.55pt}{4.82pt}{} & \HoloSegScore{14.37}{(12.30--16.50)}{4.55pt}{4.82pt}{} & \HoloSegScore{18.41}{(15.81--21.23)}{4.55pt}{4.82pt}{} & \HoloSegScore{14.59}{(12.15--15.47)}{4.55pt}{4.82pt}{} & \HoloSegScore{12.86}{(10.94--14.83)}{4.55pt}{4.82pt}{} & \HoloSegScore{10.49}{(8.562--12.35)}{4.55pt}{4.82pt}{} \\
\cline{3-11}
 &  &  & \HoloSegMetric{Dice} & \HoloSegScore{0.9281}{(0.9195--0.9364)}{4.55pt}{4.82pt}{} & \HoloSegScore{0.7441}{(0.7285--0.7573)}{4.55pt}{4.82pt}{} & \HoloSegScore{0.9151}{(0.9067--0.9221)}{4.55pt}{4.82pt}{} & \HoloSegScore{0.9316}{(0.9217--0.9409)}{4.55pt}{4.82pt}{} & \HoloSegScore{0.9351}{(0.9195--0.9511)}{4.55pt}{4.82pt}{} & \HoloSegScore{0.9568}{(0.9499--0.9632)}{4.55pt}{4.82pt}{} & \HoloSegScore{0.9578}{(0.9514--0.9640)}{4.55pt}{4.82pt}{} \\*
\softcline{4-11}
 &  & \HoloSegSpan{\makecell[c]{right lung}}{2.04cm}{0.32cm} & \HoloSegMetric{HD95} & \HoloSegScore{15.14}{(13.03--17.34)}{4.55pt}{4.82pt}{} & \HoloSegScore{34.13}{(31.64--36.66)}{4.55pt}{4.82pt}{} & \HoloSegScore{18.82}{(16.56--21.21)}{4.55pt}{4.82pt}{} & \HoloSegScore{17.56}{(15.39--20.10)}{4.55pt}{4.82pt}{} & \HoloSegScore{13.98}{(9.792--15.31)}{4.55pt}{4.82pt}{} & \HoloSegScore{10.46}{(8.985--12.01)}{4.55pt}{4.82pt}{} & \HoloSegScore{16.70}{(13.80--19.76)}{4.55pt}{4.82pt}{} \\
\cline{3-11}
 &  &  & \HoloSegMetric{Dice} & \HoloSegScore{0.8632}{(0.8563--0.8700)}{4.55pt}{4.82pt}{} & \HoloSegScore{0.5804}{(0.5705--0.5894)}{4.55pt}{4.82pt}{} & \HoloSegScore{0.8569}{(0.8487--0.8636)}{4.55pt}{4.82pt}{} & \HoloSegScore{0.8382}{(0.8298--0.8460)}{4.55pt}{4.82pt}{} & \HoloSegScore{0.8500}{(0.8498--0.8504)}{4.55pt}{4.82pt}{} & \HoloSegScore{0.8780}{(0.8719--0.8840)}{4.55pt}{4.82pt}{} & \HoloSegScore{0.8804}{(0.8737--0.8865)}{4.55pt}{4.82pt}{} \\*
\softcline{4-11}
 &  & \HoloSegSpan{\makecell[c]{pancreas}}{2.04cm}{0.32cm} & \HoloSegMetric{HD95} & \HoloSegScore{9.028}{(7.748--10.64)}{4.55pt}{4.82pt}{} & \HoloSegScore{15.12}{(14.29--16.09)}{4.55pt}{4.82pt}{} & \HoloSegScore{6.515}{(5.665--7.556)}{4.55pt}{4.82pt}{} & \HoloSegScore{10.19}{(9.023--11.45)}{4.55pt}{4.82pt}{} & \HoloSegScore{9.791}{(8.389--10.31)}{4.55pt}{4.82pt}{} & \HoloSegScore{6.216}{(5.412--7.156)}{4.55pt}{4.82pt}{} & \HoloSegScore{7.195}{(5.962--8.863)}{4.55pt}{4.82pt}{} \\
\cline{3-11}
 &  &  & \HoloSegMetric{Dice} &  & \HoloSegScore{0.2245}{(0.2183--0.2303)}{4.55pt}{4.82pt}{} & \HoloSegScore{0.0000}{(0.0000--0.0000)}{4.55pt}{4.82pt}{} & \HoloSegScore{0.3327}{(0.3267--0.3382)}{4.55pt}{4.82pt}{} & \HoloSegScore{0.7523}{(0.7443--0.7636)}{4.55pt}{4.82pt}{} & \HoloSegScore{0.7367}{(0.7272--0.7461)}{4.55pt}{4.82pt}{} & \HoloSegScore{0.7519}{(0.7418--0.7610)}{4.55pt}{4.82pt}{} \\*
\softcline{4-4}\softcline{6-11}
 &  & \HoloSegSpan{\makecell[c]{body of\\[-0.10ex]pancreas}}{2.04cm}{0.32cm} & \HoloSegMetric{HD95} & \raisebox{0.32cm}[0pt][0pt]{\HoloSegUnsupported} & \HoloSegScore{54.14}{(53.36--54.96)}{4.55pt}{4.82pt}{} & \HoloSegScore{360.5}{(331.2--382.1)}{4.55pt}{4.82pt}{} & \HoloSegScore{59.01}{(58.18--59.85)}{4.55pt}{4.82pt}{} & \HoloSegScore{12.07}{(9.701--13.74)}{4.55pt}{4.82pt}{} & \HoloSegScore{18.02}{(17.16--18.90)}{4.55pt}{4.82pt}{} & \HoloSegScore{12.83}{(12.17--13.56)}{4.55pt}{4.82pt}{} \\
\hline
\pagebreak[4]
 &  &  & \HoloSegMetric{Dice} &  & \HoloSegScore{0.4275}{(0.4175--0.4367)}{4.55pt}{4.82pt}{} & \HoloSegScore{0.0006126}{(0.0001487--0.001251)}{3.52pt}{3.80pt}{} & \HoloSegScore{0.4152}{(0.4052--0.4247)}{4.55pt}{4.82pt}{} & \HoloSegScore{0.8342}{(0.8219--0.8395)}{4.55pt}{4.82pt}{} & \HoloSegScore{0.8053}{(0.7950--0.8138)}{4.55pt}{4.82pt}{} & \HoloSegScore{0.8352}{(0.8247--0.8443)}{4.55pt}{4.82pt}{} \\*
\softcline{4-4}\softcline{6-11}
 &  & \HoloSegSpan{\makecell[c]{head of\\[-0.10ex]pancreas}}{2.04cm}{0.32cm} & \HoloSegMetric{HD95} & \raisebox{0.32cm}[0pt][0pt]{\HoloSegUnsupported} & \HoloSegScore{67.64}{(66.20--69.01)}{4.55pt}{4.82pt}{} & \HoloSegScore{257.2}{(212.3--302.8)}{4.55pt}{4.82pt}{} & \HoloSegScore{77.32}{(76.08--78.61)}{4.55pt}{4.82pt}{} & \HoloSegScore{8.377}{(6.042--11.32)}{4.55pt}{4.82pt}{} & \HoloSegScore{13.99}{(13.03--15.03)}{4.55pt}{4.82pt}{} & \HoloSegScore{10.06}{(8.082--12.23)}{4.55pt}{4.82pt}{} \\
\cline{3-11}
 &  &  & \HoloSegMetric{Dice} &  & \HoloSegScore{0.1686}{(0.1609--0.1765)}{4.55pt}{4.82pt}{} & \HoloSegScore{0.0000}{(0.0000--0.0000)}{4.55pt}{4.82pt}{} & \HoloSegScore{0.3645}{(0.3551--0.3735)}{4.55pt}{4.82pt}{} & \HoloSegScore{0.8170}{(0.8114--0.8202)}{4.55pt}{4.82pt}{} & \HoloSegScore{0.7965}{(0.7857--0.8068)}{4.55pt}{4.82pt}{} & \HoloSegScore{0.8057}{(0.7947--0.8163)}{4.55pt}{4.82pt}{} \\*
\softcline{4-4}\softcline{6-11}
 &  & \HoloSegSpan{\makecell[c]{tail of\\[-0.10ex]pancreas}}{2.04cm}{0.32cm} & \HoloSegMetric{HD95} & \raisebox{0.32cm}[0pt][0pt]{\HoloSegUnsupported} & \HoloSegScore{78.96}{(77.73--80.26)}{4.55pt}{4.82pt}{} & \HoloSegScore{341.9}{(307.8--375.1)}{4.55pt}{4.82pt}{} & \HoloSegScore{72.06}{(71.19--73.02)}{4.55pt}{4.82pt}{} & \HoloSegScore{11.69}{(11.05--12.44)}{4.55pt}{4.82pt}{} & \HoloSegScore{11.35}{(10.35--12.44)}{4.55pt}{4.82pt}{} & \HoloSegScore{9.428}{(8.599--10.44)}{4.55pt}{4.82pt}{} \\
\cline{3-11}
 &  &  & \HoloSegMetric{Dice} & \HoloSegScore{0.1120}{(0.05198--0.1821)}{4.20pt}{4.48pt}{} & \HoloSegScore{0.1324}{(0.1039--0.1610)}{4.55pt}{4.82pt}{} & \HoloSegScore{0.1563}{(0.1094--0.2077)}{4.55pt}{4.82pt}{} & \HoloSegScore{0.3278}{(0.2762--0.3808)}{4.55pt}{4.82pt}{} & \HoloSegScore{0.4751}{(0.4361--0.5097)}{4.55pt}{4.82pt}{} & \HoloSegScore{0.4138}{(0.3700--0.4594)}{4.55pt}{4.82pt}{} & \HoloSegScore{0.4684}{(0.4245--0.5148)}{4.55pt}{4.82pt}{} \\*
\softcline{4-11}
 &  & \HoloSegSpan{\makecell[c]{pancreas\\[-0.10ex]lesion}}{2.04cm}{0.32cm} & \HoloSegMetric{HD95} & \HoloSegScore{147.8}{(110.6--184.3)}{4.55pt}{4.82pt}{} & \HoloSegScore{79.15}{(71.15--89.01)}{4.55pt}{4.82pt}{} & \HoloSegScore{56.93}{(34.52--82.53)}{4.55pt}{4.82pt}{} & \HoloSegScore{46.23}{(35.45--57.72)}{4.55pt}{4.82pt}{} & \HoloSegScore{35.23}{(27.13--43.13)}{4.55pt}{4.82pt}{} & \HoloSegScore{36.19}{(31.16--41.88)}{4.55pt}{4.82pt}{} & \HoloSegScore{34.26}{(29.28--39.53)}{4.55pt}{4.82pt}{} \\
\cline{3-11}
 &  &  & \HoloSegMetric{Dice} & \HoloSegScore{0.5962}{(0.5831--0.6090)}{4.55pt}{4.82pt}{} & \HoloSegScore{0.2105}{(0.2024--0.2189)}{4.55pt}{4.82pt}{} & \HoloSegScore{0.5868}{(0.5738--0.5995)}{4.55pt}{4.82pt}{} & \HoloSegScore{0.5693}{(0.5570--0.5822)}{4.55pt}{4.82pt}{} & \HoloSegScore{0.6163}{(0.5958--0.6431)}{4.55pt}{4.82pt}{} & \HoloSegScore{0.6534}{(0.6413--0.6665)}{4.55pt}{4.82pt}{} & \HoloSegScore{0.6635}{(0.6509--0.6767)}{4.55pt}{4.82pt}{} \\*
\softcline{4-11}
 &  & \HoloSegSpan{\makecell[c]{portal vein\\[-0.10ex]and splenic\\[-0.10ex]vein}}{2.04cm}{0.32cm} & \HoloSegMetric{HD95} & \HoloSegScore{41.44}{(37.95--45.04)}{4.55pt}{4.82pt}{} & \HoloSegScore{51.12}{(48.52--54.03)}{4.55pt}{4.82pt}{} & \HoloSegScore{27.58}{(24.90--30.31)}{4.55pt}{4.82pt}{} & \HoloSegScore{53.61}{(49.93--57.30)}{4.55pt}{4.82pt}{} & \HoloSegScore{29.22}{(26.14--33.21)}{4.55pt}{4.82pt}{} & \HoloSegScore{42.25}{(38.95--45.64)}{4.55pt}{4.82pt}{} & \HoloSegScore{43.56}{(39.97--47.06)}{4.55pt}{4.82pt}{} \\
\cline{3-11}
 &  &  & \HoloSegMetric{Dice} & \HoloSegScore{0.8189}{(0.8091--0.8285)}{4.55pt}{4.82pt}{} & \HoloSegScore{0.6919}{(0.6825--0.7010)}{4.55pt}{4.82pt}{} & \HoloSegScore{0.8221}{(0.8121--0.8316)}{4.55pt}{4.82pt}{} & \HoloSegScore{0.8153}{(0.8059--0.8253)}{4.55pt}{4.82pt}{} & \HoloSegScore{0.8035}{(0.7892--0.8158)}{4.55pt}{4.82pt}{} & \HoloSegScore{0.8345}{(0.8254--0.8429)}{4.55pt}{4.82pt}{} & \HoloSegScore{0.8371}{(0.8285--0.8451)}{4.55pt}{4.82pt}{} \\*
\softcline{4-11}
 &  & \HoloSegSpan{\makecell[c]{inferior\\[-0.10ex]vena cava}}{2.04cm}{0.32cm} & \HoloSegMetric{HD95} & \HoloSegScore{25.72}{(23.41--27.99)}{4.55pt}{4.82pt}{} & \HoloSegScore{23.05}{(21.05--25.14)}{4.55pt}{4.82pt}{} & \HoloSegScore{21.93}{(19.56--24.42)}{4.55pt}{4.82pt}{} & \HoloSegScore{23.56}{(21.17--26.27)}{4.55pt}{4.82pt}{} & \HoloSegScore{22.08}{(19.59--23.71)}{4.55pt}{4.82pt}{} & \HoloSegScore{21.63}{(19.60--23.97)}{4.55pt}{4.82pt}{} & \HoloSegScore{21.17}{(19.20--23.43)}{4.55pt}{4.82pt}{} \\
\cline{3-11}
 &  &  & \HoloSegMetric{Dice} & \HoloSegScore{0.4815}{(0.4529--0.5108)}{4.55pt}{4.82pt}{} & \HoloSegScore{0.2388}{(0.2200--0.2583)}{4.55pt}{4.82pt}{} & \HoloSegScore{0.3241}{(0.2971--0.3530)}{4.55pt}{4.82pt}{} & \HoloSegScore{0.2307}{(0.2082--0.2537)}{4.55pt}{4.82pt}{} & \HoloSegScore{0.6270}{(0.5852--0.6459)}{4.55pt}{4.82pt}{} & \HoloSegScore{0.5800}{(0.5544--0.6069)}{4.55pt}{4.82pt}{} & \HoloSegScore{0.5470}{(0.5244--0.5707)}{4.55pt}{4.82pt}{} \\*
\softcline{4-11}
 &  & \HoloSegSpan{\makecell[c]{prostate}}{2.04cm}{0.32cm} & \HoloSegMetric{HD95} & \HoloSegScore{155.9}{(144.2--167.9)}{4.55pt}{4.82pt}{} & \HoloSegScore{68.28}{(61.72--75.28)}{4.55pt}{4.82pt}{} & \HoloSegScore{34.55}{(31.58--37.62)}{4.55pt}{4.82pt}{} & \HoloSegScore{38.64}{(34.77--43.06)}{4.55pt}{4.82pt}{} & \HoloSegScore{39.24}{(33.81--43.73)}{4.55pt}{4.82pt}{} & \HoloSegScore{37.00}{(31.16--44.16)}{4.55pt}{4.82pt}{} & \HoloSegScore{74.84}{(69.05--80.70)}{4.55pt}{4.82pt}{} \\
\cline{3-11}
 & \HoloSegSpan{\makecell[c]{AbdomenAtlas\\[-0.10ex]3.0}}{1.86cm}{0.32cm} &  & \HoloSegMetric{Dice} &  & \HoloSegScore{0.02811}{(0.02303--0.03378)}{4.20pt}{4.48pt}{} & \HoloSegScore{0.5733}{(0.5495--0.5960)}{4.55pt}{4.82pt}{} & \HoloSegScore{0.5293}{(0.5069--0.5519)}{4.55pt}{4.82pt}{} & \HoloSegScore{0.7238}{(0.7093--0.7362)}{4.55pt}{4.82pt}{} & \HoloSegScore{0.6933}{(0.6740--0.7121)}{4.55pt}{4.82pt}{} & \HoloSegScore{0.7071}{(0.6895--0.7247)}{4.55pt}{4.82pt}{} \\*
\softcline{4-4}\softcline{6-11}
 &  & \HoloSegSpan{\makecell[c]{rectum}}{2.04cm}{0.32cm} & \HoloSegMetric{HD95} & \raisebox{0.32cm}[0pt][0pt]{\HoloSegUnsupported} & \HoloSegScore{75.69}{(70.43--80.91)}{4.55pt}{4.82pt}{} & \HoloSegScore{29.15}{(24.97--35.03)}{4.55pt}{4.82pt}{} & \HoloSegScore{27.81}{(25.72--29.99)}{4.55pt}{4.82pt}{} & \HoloSegScore{13.64}{(12.63--15.31)}{4.55pt}{4.82pt}{} & \HoloSegScore{46.08}{(36.21--57.06)}{4.55pt}{4.82pt}{} & \HoloSegScore{30.73}{(24.22--37.58)}{4.55pt}{4.82pt}{} \\
\cline{3-11}
 &  &  & \HoloSegMetric{Dice} & \HoloSegScore{0.9445}{(0.9374--0.9516)}{4.55pt}{4.82pt}{} & \HoloSegScore{0.7915}{(0.7843--0.7984)}{4.55pt}{4.82pt}{} & \HoloSegScore{0.9425}{(0.9367--0.9479)}{4.55pt}{4.82pt}{} & \HoloSegScore{0.9423}{(0.9353--0.9482)}{4.55pt}{4.82pt}{} & \HoloSegScore{0.9225}{(0.9182--0.9380)}{4.55pt}{4.82pt}{} & \HoloSegScore{0.9563}{(0.9507--0.9609)}{4.55pt}{4.82pt}{} & \HoloSegScore{0.9560}{(0.9506--0.9607)}{4.55pt}{4.82pt}{} \\*
\softcline{4-11}
 &  & \HoloSegSpan{\makecell[c]{spleen}}{2.04cm}{0.32cm} & \HoloSegMetric{HD95} & \HoloSegScore{13.08}{(9.766--16.63)}{4.55pt}{4.82pt}{} & \HoloSegScore{11.25}{(10.49--12.10)}{4.55pt}{4.82pt}{} & \HoloSegScore{10.15}{(7.131--13.69)}{4.55pt}{4.82pt}{} & \HoloSegScore{8.321}{(7.027--9.793)}{4.55pt}{4.82pt}{} & \HoloSegScore{5.294}{(3.950--6.147)}{4.55pt}{4.82pt}{} & \HoloSegScore{2.727}{(2.220--3.352)}{4.55pt}{4.82pt}{} & \HoloSegScore{2.726}{(2.366--3.109)}{4.55pt}{4.82pt}{} \\
\cline{3-11}
 &  &  & \HoloSegMetric{Dice} & \HoloSegScore{0.8853}{(0.8756--0.8954)}{4.55pt}{4.82pt}{} & \HoloSegScore{0.6867}{(0.6758--0.6981)}{4.55pt}{4.82pt}{} & \HoloSegScore{0.7114}{(0.6891--0.7338)}{4.55pt}{4.82pt}{} & \HoloSegScore{0.8495}{(0.8384--0.8604)}{4.55pt}{4.82pt}{} & \HoloSegScore{0.8811}{(0.8744--0.8905)}{4.55pt}{4.82pt}{} & \HoloSegScore{0.9018}{(0.8934--0.9101)}{4.55pt}{4.82pt}{} & \HoloSegScore{0.8980}{(0.8894--0.9062)}{4.55pt}{4.82pt}{} \\*
\softcline{4-11}
 &  & \HoloSegSpan{\makecell[c]{stomach}}{2.04cm}{0.32cm} & \HoloSegMetric{HD95} & \HoloSegScore{15.92}{(14.09--17.80)}{4.55pt}{4.82pt}{} & \HoloSegScore{18.40}{(17.28--19.72)}{4.55pt}{4.82pt}{} & \HoloSegScore{89.39}{(80.73--98.49)}{4.55pt}{4.82pt}{} & \HoloSegScore{21.06}{(19.22--23.08)}{4.55pt}{4.82pt}{} & \HoloSegScore{13.06}{(11.54--15.51)}{4.55pt}{4.82pt}{} & \HoloSegScore{12.16}{(10.80--13.51)}{4.55pt}{4.82pt}{} & \HoloSegScore{13.65}{(12.10--15.37)}{4.55pt}{4.82pt}{} \\
\cline{3-11}
 &  &  & \HoloSegMetric{Dice} &  & \HoloSegScore{0.001816}{(0.001635--0.002024)}{3.85pt}{4.12pt}{} & \HoloSegScore{0.001417}{(0.0004707--0.002726)}{3.52pt}{3.80pt}{} & \HoloSegScore{0.4793}{(0.4660--0.4938)}{4.55pt}{4.82pt}{} & \HoloSegScore{0.7078}{(0.7009--0.7167)}{4.55pt}{4.82pt}{} & \HoloSegScore{0.7758}{(0.7682--0.7829)}{4.55pt}{4.82pt}{} & \HoloSegScore{0.8231}{(0.8185--0.8277)}{4.55pt}{4.82pt}{} \\*
\softcline{4-4}\softcline{6-11}
\HoloSegSpan{\makecell[c]{\textbf{Internal}}}{1.20cm}{0.32cm} &  & \HoloSegSpan{\makecell[c]{superior\\[-0.10ex]mesenteric\\[-0.10ex]artery}}{2.04cm}{0.32cm} & \HoloSegMetric{HD95} & \raisebox{0.32cm}[0pt][0pt]{\HoloSegUnsupported} & \HoloSegScore{121.8}{(118.9--124.9)}{4.55pt}{4.82pt}{} & \HoloSegScore{102.1}{(95.29--109.1)}{4.55pt}{4.82pt}{} & \HoloSegScore{34.19}{(32.06--36.41)}{4.55pt}{4.82pt}{} & \HoloSegScore{9.399}{(8.015--12.35)}{4.55pt}{4.82pt}{} & \HoloSegScore{7.994}{(7.363--8.600)}{4.55pt}{4.82pt}{} & \HoloSegScore{5.130}{(4.742--5.562)}{4.55pt}{4.82pt}{} \\
\cline{3-11}
 &  &  & \HoloSegMetric{Dice} &  & \HoloSegScore{0.004697}{(0.003654--0.005945)}{3.85pt}{4.12pt}{} & \HoloSegScore{0.1213}{(0.1039--0.1426)}{4.55pt}{4.82pt}{} & \HoloSegScore{0.2205}{(0.2075--0.2328)}{4.55pt}{4.82pt}{} & \HoloSegScore{0.7868}{(0.7805--0.7894)}{4.55pt}{4.82pt}{} & \HoloSegScore{0.8061}{(0.7992--0.8128)}{4.55pt}{4.82pt}{} & \HoloSegScore{0.8175}{(0.8109--0.8238)}{4.55pt}{4.82pt}{} \\*
\softcline{4-4}\softcline{6-11}
 &  & \HoloSegSpan{\makecell[c]{veins}}{2.04cm}{0.32cm} & \HoloSegMetric{HD95} & \raisebox{0.32cm}[0pt][0pt]{\HoloSegUnsupported} & \HoloSegScore{78.25}{(77.35--79.14)}{4.55pt}{4.82pt}{} & \HoloSegScore{85.69}{(79.34--93.03)}{4.55pt}{4.82pt}{} & \HoloSegScore{67.01}{(66.06--67.49)}{4.55pt}{4.82pt}{} & \HoloSegScore{12.00}{(8.766--13.33)}{4.55pt}{4.82pt}{} & \HoloSegScore{9.079}{(8.488--9.803)}{4.55pt}{4.82pt}{} & \HoloSegScore{7.477}{(6.890--8.078)}{4.55pt}{4.82pt}{} \\
\cline{3-11}
 &  &  & \HoloSegMetric{Dice} &  & \HoloSegScore{0.03393}{(0.0001163--0.08354)}{3.85pt}{4.12pt}{} & \HoloSegScore{0.0000}{(0.0000--0.0000)}{4.55pt}{4.82pt}{} & \HoloSegScore{0.6030}{(0.4972--0.7061)}{4.55pt}{4.82pt}{} & \HoloSegScore{0.6854}{(0.6839--0.6893)}{4.55pt}{4.82pt}{} & \HoloSegScore{0.6212}{(0.5086--0.7165)}{4.55pt}{4.82pt}{} & \HoloSegScore{0.6518}{(0.5500--0.7353)}{4.55pt}{4.82pt}{} \\*
\softcline{4-4}\softcline{6-11}
 &  & \HoloSegSpan{\makecell[c]{colon lesion}}{2.04cm}{0.32cm} & \HoloSegMetric{HD95} & \raisebox{0.32cm}[0pt][0pt]{\HoloSegUnsupported} & \HoloSegScore{186.9}{(157.3--217.6)}{4.55pt}{4.82pt}{} & \HoloSegScore{--}{(--\,--)}{4.55pt}{4.82pt}{} & \HoloSegScore{70.07}{(39.90--104.8)}{4.55pt}{4.82pt}{} & \HoloSegScore{34.54}{(11.62--66.17)}{4.55pt}{4.82pt}{} & \HoloSegScore{28.56}{(14.76--46.14)}{4.55pt}{4.82pt}{} & \HoloSegScore{41.25}{(17.06--72.64)}{4.55pt}{4.82pt}{} \\
\cline{2-11}
 &  &  & \HoloSegMetric{Dice} & \HoloSegScore{0.8720}{(0.8141--0.9192)}{4.55pt}{4.82pt}{} & \HoloSegScore{0.08766}{(0.002237--0.2003)}{4.20pt}{4.48pt}{} & \HoloSegScore{0.7628}{(0.6613--0.8643)}{4.55pt}{4.82pt}{} & \HoloSegScore{0.6592}{(0.5397--0.7613)}{4.55pt}{4.82pt}{} & \HoloSegScore{0.9381}{(0.9266--0.9466)}{4.55pt}{4.82pt}{} & \HoloSegScore{0.9429}{(0.9254--0.9578)}{4.55pt}{4.82pt}{} & \HoloSegScore{0.9495}{(0.9384--0.9592)}{4.55pt}{4.82pt}{} \\*
\softcline{4-11}
 &  & \HoloSegSpan{\makecell[c]{liver}}{2.04cm}{0.32cm} & \HoloSegMetric{HD95} & \HoloSegScore{13.45}{(9.159--18.01)}{4.55pt}{4.82pt}{} & \HoloSegScore{133.9}{(108.8--157.0)}{4.55pt}{4.82pt}{} & \HoloSegScore{19.03}{(12.44--26.55)}{4.55pt}{4.82pt}{} & \HoloSegScore{102.9}{(69.36--137.4)}{4.55pt}{4.82pt}{} & \HoloSegScore{8.283}{(6.750--11.90)}{4.55pt}{4.82pt}{} & \HoloSegScore{7.824}{(4.504--12.57)}{4.55pt}{4.82pt}{} & \HoloSegScore{6.202}{(4.424--8.453)}{4.55pt}{4.82pt}{} \\
\cline{3-11}
 &  &  & \HoloSegMetric{Dice} &  & \HoloSegScore{0.0000}{(0.0000--0.0000)}{4.55pt}{4.82pt}{} & \HoloSegScore{0.0000}{(0.0000--0.0000)}{4.55pt}{4.82pt}{} & \HoloSegScore{0.0000}{(0.0000--0.0000)}{4.55pt}{4.82pt}{} & \HoloSegScore{0.6831}{(0.6823--0.7010)}{4.55pt}{4.82pt}{} & \HoloSegScore{0.5513}{(0.3939--0.6726)}{4.55pt}{4.82pt}{} & \HoloSegScore{0.5525}{(0.3805--0.6922)}{4.55pt}{4.82pt}{} \\*
\softcline{4-4}\softcline{6-11}
 &  & \HoloSegSpan{\makecell[c]{liver cyst}}{2.04cm}{0.32cm} & \HoloSegMetric{HD95} & \raisebox{0.32cm}[0pt][0pt]{\HoloSegUnsupported} & \HoloSegScore{--}{(--\,--)}{4.55pt}{4.82pt}{} & \HoloSegScore{400.7}{(385.3--416.2)}{4.55pt}{4.82pt}{} & \HoloSegScore{--}{(--\,--)}{4.55pt}{4.82pt}{} & \HoloSegScore{13.29}{(6.723--23.73)}{4.55pt}{4.82pt}{} & \HoloSegScore{26.29}{(6.734--49.53)}{4.55pt}{4.82pt}{} & \HoloSegScore{37.64}{(23.66--53.32)}{4.55pt}{4.82pt}{} \\
\cline{3-11}
 &  &  & \HoloSegMetric{Dice} &  & \HoloSegScore{0.0000}{(0.0000--0.0000)}{4.55pt}{4.82pt}{} & \HoloSegScore{0.3428}{(0.1047--0.5815)}{4.55pt}{4.82pt}{} & \HoloSegScore{0.2417}{(0.0000--0.5089)}{4.55pt}{4.82pt}{} & \HoloSegScore{0.7385}{(0.7292--0.7385)}{4.55pt}{4.82pt}{} & \HoloSegScore{0.7789}{(0.7022--0.8441)}{4.55pt}{4.82pt}{} & \HoloSegScore{0.7105}{(0.5357--0.8288)}{4.55pt}{4.82pt}{} \\*
\softcline{4-4}\softcline{6-11}
 & \HoloSegSpan{\makecell[c]{LiMT}}{1.86cm}{0.32cm} & \HoloSegSpan{\makecell[c]{liver\\[-0.10ex]hemangioma}}{2.04cm}{0.32cm} & \HoloSegMetric{HD95} & \raisebox{0.32cm}[0pt][0pt]{\HoloSegUnsupported} & \HoloSegScore{--}{(--\,--)}{4.55pt}{4.82pt}{} & \HoloSegScore{87.16}{(49.97--125.0)}{4.55pt}{4.82pt}{} & \HoloSegScore{71.59}{(5.750--153.7)}{4.55pt}{4.82pt}{} & \HoloSegScore{38.57}{(14.58--68.21)}{4.55pt}{4.82pt}{} & \HoloSegScore{19.56}{(8.792--31.53)}{4.55pt}{4.82pt}{} & \HoloSegScore{40.47}{(11.82--69.13)}{4.55pt}{4.82pt}{} \\
\cline{3-11}
 &  &  & \HoloSegMetric{Dice} & \HoloSegScore{0.3684}{(0.09556--0.6286)}{4.20pt}{4.48pt}{} & \HoloSegScore{0.0000}{(0.0000--0.0000)}{4.55pt}{4.82pt}{} & \HoloSegScore{0.02375}{(0.0000--0.06959)}{4.20pt}{4.48pt}{} & \HoloSegScore{0.1174}{(0.0000--0.3203)}{4.55pt}{4.82pt}{} & \HoloSegScore{0.4385}{(0.4141--0.4834)}{4.55pt}{4.82pt}{} & \HoloSegScore{0.3798}{(0.1154--0.5868)}{4.55pt}{4.82pt}{} & \HoloSegScore{0.4520}{(0.1643--0.6442)}{4.55pt}{4.82pt}{} \\*
\softcline{4-11}
 &  & \HoloSegSpan{\makecell[c]{metastatic\\[-0.10ex]liver cancer}}{2.04cm}{0.32cm} & \HoloSegMetric{HD95} & \HoloSegScore{50.23}{(26.19--76.95)}{4.55pt}{4.82pt}{} & \HoloSegScore{177.9}{(177.9--177.9)}{4.55pt}{4.82pt}{} & \HoloSegScore{136.7}{(94.46--177.7)}{4.55pt}{4.82pt}{} & \HoloSegScore{83.57}{(46.14--126.0)}{4.55pt}{4.82pt}{} & \HoloSegScore{50.87}{(28.55--75.34)}{4.55pt}{4.82pt}{} & \HoloSegScore{40.42}{(19.15--74.88)}{4.55pt}{4.82pt}{} & \HoloSegScore{40.53}{(18.05--75.66)}{4.55pt}{4.82pt}{} \\
\cline{3-11}
 &  &  & \HoloSegMetric{Dice} & \HoloSegScore{0.4323}{(0.1632--0.6778)}{4.55pt}{4.82pt}{} & \HoloSegScore{0.000001252}{(0.0000--0.000003756)}{3.52pt}{3.80pt}{} & \HoloSegScore{0.3477}{(0.1408--0.5614)}{4.55pt}{4.82pt}{} & \HoloSegScore{0.3747}{(0.1390--0.6476)}{4.55pt}{4.82pt}{} & \HoloSegScore{0.7234}{(0.6444--0.7951)}{4.55pt}{4.82pt}{} & \HoloSegScore{0.7394}{(0.6181--0.8488)}{4.55pt}{4.82pt}{} & \HoloSegScore{0.6927}{(0.4554--0.8568)}{4.55pt}{4.82pt}{} \\*
\softcline{4-11}
 &  & \HoloSegSpan{\makecell[c]{primary\\[-0.10ex]liver cancer}}{2.04cm}{0.32cm} & \HoloSegMetric{HD95} & \HoloSegScore{62.16}{(36.32--87.10)}{4.55pt}{4.82pt}{} & \HoloSegScore{168.5}{(141.0--212.4)}{4.55pt}{4.82pt}{} & \HoloSegScore{46.39}{(25.89--69.49)}{4.55pt}{4.82pt}{} & \HoloSegScore{43.99}{(16.66--79.89)}{4.55pt}{4.82pt}{} & \HoloSegScore{22.60}{(11.26--35.78)}{4.55pt}{4.82pt}{} & \HoloSegScore{40.33}{(11.73--75.55)}{4.55pt}{4.82pt}{} & \HoloSegScore{31.25}{(15.05--54.17)}{4.55pt}{4.82pt}{} \\
\cline{2-11}
 &  &  & \HoloSegMetric{Dice} &  & \HoloSegScore{0.3935}{(0.3192--0.4668)}{4.55pt}{4.82pt}{} & \HoloSegScore{0.0001014}{(0.0000--0.0003043)}{3.85pt}{4.12pt}{} & \HoloSegScore{0.7737}{(0.7098--0.8330)}{4.55pt}{4.82pt}{} & \HoloSegScore{0.7771}{(0.7251--0.7936)}{4.55pt}{4.82pt}{} & \HoloSegScore{0.7338}{(0.6647--0.7955)}{4.55pt}{4.82pt}{} & \HoloSegScore{0.7705}{(0.7142--0.8215)}{4.55pt}{4.82pt}{} \\*
\softcline{4-4}\softcline{6-11}
 & \HoloSegSpan{\makecell[c]{ULS23-\\[-0.10ex]KiTS23}}{1.86cm}{0.32cm} & \HoloSegSpan{\makecell[c]{kidney\\[-0.10ex]lesion}}{2.04cm}{0.32cm} & \HoloSegMetric{HD95} & \raisebox{0.32cm}[0pt][0pt]{\HoloSegUnsupported} & \HoloSegScore{49.15}{(38.58--60.27)}{4.55pt}{4.82pt}{} & \HoloSegScore{111.4}{(97.94--127.8)}{4.55pt}{4.82pt}{} & \HoloSegScore{12.70}{(8.181--17.29)}{4.55pt}{4.82pt}{} & \HoloSegScore{15.65}{(9.966--20.31)}{4.55pt}{4.82pt}{} & \HoloSegScore{21.57}{(13.32--32.14)}{4.55pt}{4.82pt}{} & \HoloSegScore{15.11}{(10.34--20.05)}{4.55pt}{4.82pt}{} \\
\cline{2-11}
 &  &  & \HoloSegMetric{Dice} & \HoloSegScore{0.04586}{(0.01075--0.08097)}{4.20pt}{4.48pt}{} & \HoloSegScore{0.04802}{(0.02934--0.07236)}{4.20pt}{4.48pt}{} & \HoloSegScore{0.1157}{(0.08589--0.1483)}{4.20pt}{4.48pt}{} & \HoloSegScore{0.1277}{(0.09877--0.1616)}{4.20pt}{4.48pt}{} & \HoloSegScore{0.6518}{(0.6444--0.6867)}{4.55pt}{4.82pt}{} & \HoloSegScore{0.3608}{(0.3183--0.4032)}{4.55pt}{4.82pt}{} & \HoloSegScore{0.3647}{(0.3243--0.4019)}{4.55pt}{4.82pt}{} \\*
\softcline{4-11}
 & \HoloSegSpan{\makecell[c]{ULS23-LiTS}}{1.86cm}{0.32cm} & \HoloSegSpan{\makecell[c]{liver tumor}}{2.04cm}{0.32cm} & \HoloSegMetric{HD95} & \HoloSegScore{111.3}{(106.4--116.3)}{4.55pt}{4.82pt}{} & \HoloSegScore{87.46}{(83.62--91.14)}{4.55pt}{4.82pt}{} & \HoloSegScore{70.78}{(66.76--74.79)}{4.55pt}{4.82pt}{} & \HoloSegScore{85.12}{(80.88--89.30)}{4.55pt}{4.82pt}{} & \HoloSegScore{10.10}{(9.703--12.23)}{4.55pt}{4.82pt}{} & \HoloSegScore{34.33}{(30.76--38.01)}{4.55pt}{4.82pt}{} & \HoloSegScore{43.67}{(40.11--47.27)}{4.55pt}{4.82pt}{} \\
\hline
\pagebreak[4]
 &  &  & \HoloSegMetric{Dice} &  & \HoloSegScore{0.02544}{(0.01489--0.03840)}{4.20pt}{4.48pt}{} & \HoloSegScore{0.1377}{(0.1156--0.1602)}{4.55pt}{4.82pt}{} & \HoloSegScore{0.3140}{(0.2770--0.3518)}{4.55pt}{4.82pt}{} & \HoloSegScore{0.6392}{(0.6039--0.6539)}{4.55pt}{4.82pt}{} & \HoloSegScore{0.5756}{(0.5466--0.6013)}{4.55pt}{4.82pt}{} & \HoloSegScore{0.6145}{(0.5862--0.6386)}{4.55pt}{4.82pt}{} \\*
\softcline{4-4}\softcline{6-11}
 & \HoloSegSpan{\makecell[c]{ULS23-\\[-0.10ex]LIDC-IDRI}}{1.86cm}{0.32cm} & \HoloSegSpan{\makecell[c]{pulmonary\\[-0.10ex]nodule}}{2.04cm}{0.32cm} & \HoloSegMetric{HD95} & \raisebox{0.32cm}[0pt][0pt]{\HoloSegUnsupported} & \HoloSegScore{103.3}{(99.73--106.3)}{4.55pt}{4.82pt}{} & \HoloSegScore{64.86}{(60.92--68.74)}{4.55pt}{4.82pt}{} & \HoloSegScore{44.16}{(39.76--48.79)}{4.55pt}{4.82pt}{} & \HoloSegScore{7.559}{(4.777--9.595)}{4.55pt}{4.82pt}{} & \HoloSegScore{11.96}{(9.934--14.08)}{4.55pt}{4.82pt}{} & \HoloSegScore{11.44}{(9.205--13.68)}{4.55pt}{4.82pt}{} \\
\cline{2-11}
 &  &  & \HoloSegMetric{Dice} &  & \HoloSegScore{0.2841}{(0.1097--0.4727)}{4.55pt}{4.82pt}{} & \HoloSegScore{0.5587}{(0.3853--0.7002)}{4.55pt}{4.82pt}{} & \HoloSegScore{0.7853}{(0.6504--0.8695)}{4.55pt}{4.82pt}{} & \HoloSegScore{0.7826}{(0.7051--0.8457)}{4.55pt}{4.82pt}{} & \HoloSegScore{0.7133}{(0.5900--0.8122)}{4.55pt}{4.82pt}{} & \HoloSegScore{0.7365}{(0.6088--0.8291)}{4.55pt}{4.82pt}{} \\*
\softcline{4-4}\softcline{6-11}
 & \HoloSegSpan{\makecell[c]{ULS23-MSD-\\[-0.10ex]lung}}{1.86cm}{0.32cm} & \HoloSegSpan{\makecell[c]{lung tumor}}{2.04cm}{0.32cm} & \HoloSegMetric{HD95} & \raisebox{0.32cm}[0pt][0pt]{\HoloSegUnsupported} & \HoloSegScore{61.46}{(36.31--89.15)}{4.55pt}{4.82pt}{} & \HoloSegScore{20.63}{(6.943--38.43)}{4.55pt}{4.82pt}{} & \HoloSegScore{9.120}{(2.656--20.83)}{4.55pt}{4.82pt}{} & \HoloSegScore{5.581}{(3.685--6.837)}{4.55pt}{4.82pt}{} & \HoloSegScore{19.10}{(3.972--39.28)}{4.55pt}{4.82pt}{} & \HoloSegScore{15.96}{(4.259--36.35)}{4.55pt}{4.82pt}{} \\
\cline{2-11}
 &  &  & \HoloSegMetric{Dice} &  & \HoloSegScore{0.02641}{(0.0003254--0.08548)}{3.85pt}{4.12pt}{} & \HoloSegScore{0.6397}{(0.5143--0.7500)}{4.55pt}{4.82pt}{} & \HoloSegScore{0.7137}{(0.6537--0.7674)}{4.55pt}{4.82pt}{} & \HoloSegScore{0.7484}{(0.7180--0.7704)}{4.55pt}{4.82pt}{} & \HoloSegScore{0.6619}{(0.5737--0.7377)}{4.55pt}{4.82pt}{} & \HoloSegScore{0.6531}{(0.5453--0.7330)}{4.55pt}{4.82pt}{} \\*
\softcline{4-4}\softcline{6-11}
 & \HoloSegSpan{\makecell[c]{ULS23-MSD-\\[-0.10ex]colon}}{1.86cm}{0.32cm} & \HoloSegSpan{\makecell[c]{colon cancer}}{2.04cm}{0.32cm} & \HoloSegMetric{HD95} & \raisebox{0.32cm}[0pt][0pt]{\HoloSegUnsupported} & \HoloSegScore{130.8}{(105.4--156.7)}{4.55pt}{4.82pt}{} & \HoloSegScore{16.26}{(4.970--31.90)}{4.55pt}{4.82pt}{} & \HoloSegScore{11.09}{(7.324--15.67)}{4.55pt}{4.82pt}{} & \HoloSegScore{11.76}{(7.867--15.60)}{4.55pt}{4.82pt}{} & \HoloSegScore{12.15}{(8.331--17.15)}{4.55pt}{4.82pt}{} & \HoloSegScore{20.72}{(10.12--33.79)}{4.55pt}{4.82pt}{} \\
\cline{2-11}
\HoloSegSpan{\makecell[c]{\textbf{Internal}}}{1.20cm}{0.32cm} &  &  & \HoloSegMetric{Dice} &  & \HoloSegScore{0.2248}{(0.1756--0.2756)}{4.55pt}{4.82pt}{} & \HoloSegScore{0.7307}{(0.6583--0.7969)}{4.55pt}{4.82pt}{} & \HoloSegScore{0.6651}{(0.5948--0.7287)}{4.55pt}{4.82pt}{} & \HoloSegScore{0.7768}{(0.7636--0.7950)}{4.55pt}{4.82pt}{} & \HoloSegScore{0.6121}{(0.5635--0.6602)}{4.55pt}{4.82pt}{} & \HoloSegScore{0.6432}{(0.5875--0.6960)}{4.55pt}{4.82pt}{} \\*
\softcline{4-4}\softcline{6-11}
 & \HoloSegSpan{\makecell[c]{ULS23-MSD-\\[-0.10ex]pancreas}}{1.86cm}{0.32cm} & \HoloSegSpan{\makecell[c]{pancreas\\[-0.10ex]tumor}}{2.04cm}{0.32cm} & \HoloSegMetric{HD95} & \raisebox{0.32cm}[0pt][0pt]{\HoloSegUnsupported} & \HoloSegScore{40.33}{(34.17--47.17)}{4.55pt}{4.82pt}{} & \HoloSegScore{4.266}{(3.455--5.159)}{4.55pt}{4.82pt}{} & \HoloSegScore{14.25}{(8.106--21.50)}{4.55pt}{4.82pt}{} & \HoloSegScore{7.176}{(7.052--7.233)}{4.55pt}{4.82pt}{} & \HoloSegScore{16.54}{(11.97--21.90)}{4.55pt}{4.82pt}{} & \HoloSegScore{19.27}{(13.61--25.63)}{4.55pt}{4.82pt}{} \\
\cline{2-11}
 &  &  & \HoloSegMetric{Dice} & \HoloSegScore{0.8720}{(0.8037--0.9206)}{4.55pt}{4.82pt}{} & \HoloSegScore{0.08766}{(0.002036--0.1985)}{4.20pt}{4.48pt}{} & \HoloSegScore{0.7628}{(0.6507--0.8616)}{4.55pt}{4.82pt}{} & \HoloSegScore{0.6592}{(0.5415--0.7704)}{4.55pt}{4.82pt}{} & \HoloSegScore{0.9266}{(0.9169--0.9400)}{4.55pt}{4.82pt}{} & \HoloSegScore{0.9429}{(0.9245--0.9575)}{4.55pt}{4.82pt}{} & \HoloSegScore{0.9495}{(0.9379--0.9596)}{4.55pt}{4.82pt}{} \\*
\softcline{4-11}
 &  & \HoloSegSpan{\makecell[c]{liver}}{2.04cm}{0.32cm} & \HoloSegMetric{HD95} & \HoloSegScore{13.45}{(9.350--17.99)}{4.55pt}{4.82pt}{} & \HoloSegScore{133.9}{(111.2--156.2)}{4.55pt}{4.82pt}{} & \HoloSegScore{19.03}{(12.33--27.20)}{4.55pt}{4.82pt}{} & \HoloSegScore{102.9}{(69.03--139.5)}{4.55pt}{4.82pt}{} & \HoloSegScore{8.071}{(5.867--13.19)}{4.55pt}{4.82pt}{} & \HoloSegScore{7.824}{(4.552--12.56)}{4.55pt}{4.82pt}{} & \HoloSegScore{6.202}{(4.428--8.336)}{4.55pt}{4.82pt}{} \\
\cline{3-11}
 & \HoloSegSpan{\makecell[c]{LiMT-\\[-0.10ex]oneclass}}{1.86cm}{0.32cm} &  & \HoloSegMetric{Dice} & \HoloSegScore{0.07319}{(0.006662--0.1552)}{4.20pt}{4.48pt}{} & \HoloSegScore{0.0000}{(0.0000--0.0000)}{4.55pt}{4.82pt}{} & \HoloSegScore{0.03527}{(0.0000--0.1054)}{4.55pt}{4.82pt}{} & \HoloSegScore{0.04505}{(0.01061--0.09095)}{4.20pt}{4.48pt}{} & \HoloSegScore{0.3532}{(0.3108--0.3904)}{4.55pt}{4.82pt}{} & \HoloSegScore{0.3203}{(0.1757--0.4760)}{4.55pt}{4.82pt}{} & \HoloSegScore{0.2896}{(0.1500--0.4240)}{4.55pt}{4.82pt}{} \\*
\softcline{4-11}
 &  & \HoloSegSpan{\makecell[c]{liver lesion}}{2.04cm}{0.32cm} & \HoloSegMetric{HD95} & \HoloSegScore{94.28}{(58.91--148.4)}{4.55pt}{4.82pt}{} & \HoloSegScore{172.4}{(129.4--210.7)}{4.55pt}{4.82pt}{} & \HoloSegScore{160.6}{(84.52--252.0)}{4.55pt}{4.82pt}{} & \HoloSegScore{117.9}{(94.67--141.2)}{4.55pt}{4.82pt}{} & \HoloSegScore{22.56}{(9.291--38.33)}{4.55pt}{4.82pt}{} & \HoloSegScore{25.61}{(9.964--42.83)}{4.55pt}{4.82pt}{} & \HoloSegScore{41.04}{(24.79--58.20)}{4.55pt}{4.82pt}{} \\
\hline
 &  &  & \HoloSegMetric{Dice} &  & \HoloSegScore{0.02758}{(0.003452--0.05970)}{3.85pt}{4.12pt}{} & \HoloSegScore{0.0000}{(0.0000--0.0000)}{4.55pt}{4.82pt}{} & \HoloSegScore{0.1791}{(0.1326--0.2312)}{4.55pt}{4.82pt}{} & \HoloSegScore{0.05950}{(0.05100--0.06620)}{4.20pt}{4.48pt}{} & \HoloSegScore{0.2901}{(0.2012--0.3765)}{4.55pt}{4.82pt}{} & \HoloSegScore{0.3488}{(0.2669--0.4303)}{4.55pt}{4.82pt}{} \\*
\softcline{4-4}\softcline{6-11}
 & \HoloSegSpan{\makecell[c]{ULS23-NIG-\\[-0.10ex]LN-MED}}{1.86cm}{0.32cm} & \HoloSegSpan{\makecell[c]{mediastinal\\[-0.10ex]lymph node}}{2.04cm}{0.32cm} & \HoloSegMetric{HD95} & \raisebox{0.32cm}[0pt][0pt]{\HoloSegUnsupported} & \HoloSegScore{63.52}{(56.97--70.40)}{4.55pt}{4.82pt}{} & \HoloSegScore{--}{(--\,--)}{4.55pt}{4.82pt}{} & \HoloSegScore{70.65}{(62.13--78.95)}{4.55pt}{4.82pt}{} & \HoloSegScore{79.22}{(65.03--97.30)}{4.55pt}{4.82pt}{} & \HoloSegScore{36.90}{(28.71--46.15)}{4.55pt}{4.82pt}{} & \HoloSegScore{37.37}{(26.98--48.03)}{4.55pt}{4.82pt}{} \\
\cline{2-11}
 &  &  & \HoloSegMetric{Dice} &  & \HoloSegScore{0.1669}{(0.09012--0.2573)}{4.20pt}{4.48pt}{} & \HoloSegScore{0.05259}{(0.0004245--0.1337)}{3.85pt}{4.12pt}{} & \HoloSegScore{0.4539}{(0.2718--0.6191)}{4.55pt}{4.82pt}{} & \HoloSegScore{0.09135}{(0.05473--0.1321)}{4.20pt}{4.48pt}{} & \HoloSegScore{0.5139}{(0.4165--0.5923)}{4.55pt}{4.82pt}{} & \HoloSegScore{0.6181}{(0.5015--0.7177)}{4.55pt}{4.82pt}{} \\*
\softcline{4-4}\softcline{6-11}
 & \HoloSegSpan{\makecell[c]{ULS23-\\[-0.10ex]Radboudumc-\\[-0.10ex]Pancreas}}{1.86cm}{0.32cm} & \HoloSegSpan{\makecell[c]{pancreas\\[-0.10ex]lesion}}{2.04cm}{0.32cm} & \HoloSegMetric{HD95} & \raisebox{0.32cm}[0pt][0pt]{\HoloSegUnsupported} & \HoloSegScore{55.56}{(41.74--67.40)}{4.55pt}{4.82pt}{} & \HoloSegScore{49.52}{(16.31--85.55)}{4.55pt}{4.82pt}{} & \HoloSegScore{17.75}{(9.539--26.41)}{4.55pt}{4.82pt}{} & \HoloSegScore{58.02}{(45.67--83.12)}{4.55pt}{4.82pt}{} & \HoloSegScore{16.92}{(11.31--23.42)}{4.55pt}{4.82pt}{} & \HoloSegScore{24.09}{(14.17--34.74)}{4.55pt}{4.82pt}{} \\
\cline{2-11}
 &  &  & \HoloSegMetric{Dice} &  & \HoloSegScore{0.05771}{(0.01808--0.1121)}{4.20pt}{4.48pt}{} & \HoloSegScore{0.0000}{(0.0000--0.0000)}{4.55pt}{4.82pt}{} & \HoloSegScore{0.1986}{(0.06696--0.3376)}{4.20pt}{4.48pt}{} & \HoloSegScore{0.06686}{(0.05627--0.1174)}{4.20pt}{4.48pt}{} & \HoloSegScore{0.3697}{(0.1488--0.5788)}{4.55pt}{4.82pt}{} & \HoloSegScore{0.3884}{(0.1903--0.5772)}{4.55pt}{4.82pt}{} \\*
\softcline{4-4}\softcline{6-11}
 & \HoloSegSpan{\makecell[c]{CT-Lymph-\\[-0.10ex]Nodes}}{1.86cm}{0.32cm} & \HoloSegSpan{\makecell[c]{mediastinal\\[-0.10ex]lymph node}}{2.04cm}{0.32cm} & \HoloSegMetric{HD95} & \raisebox{0.32cm}[0pt][0pt]{\HoloSegUnsupported} & \HoloSegScore{54.71}{(46.11--64.05)}{4.55pt}{4.82pt}{} & \HoloSegScore{--}{(--\,--)}{4.55pt}{4.82pt}{} & \HoloSegScore{125.6}{(87.19--184.3)}{4.55pt}{4.82pt}{} & \HoloSegScore{55.36}{(30.69--86.93)}{4.55pt}{4.82pt}{} & \HoloSegScore{61.99}{(32.46--95.41)}{4.55pt}{4.82pt}{} & \HoloSegScore{40.74}{(22.61--59.04)}{4.55pt}{4.82pt}{} \\
\cline{2-11}
 &  &  & \HoloSegMetric{Dice} & \HoloSegScore{0.3328}{(0.2779--0.3837)}{4.55pt}{4.82pt}{} & \HoloSegScore{0.1581}{(0.1303--0.1876)}{4.55pt}{4.82pt}{} & \HoloSegScore{0.4150}{(0.3695--0.4605)}{4.55pt}{4.82pt}{} & \HoloSegScore{0.4033}{(0.3490--0.4580)}{4.55pt}{4.82pt}{} & \HoloSegScore{0.1807}{(0.04050--0.3250)}{4.20pt}{4.48pt}{} & \HoloSegScore{0.4617}{(0.4182--0.5073)}{4.55pt}{4.82pt}{} & \HoloSegScore{0.5014}{(0.4577--0.5423)}{4.55pt}{4.82pt}{} \\*
\softcline{4-11}
 &  & \HoloSegSpan{\makecell[c]{left adrenal\\[-0.10ex]gland}}{2.04cm}{0.32cm} & \HoloSegMetric{HD95} & \HoloSegScore{16.67}{(14.52--18.93)}{4.55pt}{4.82pt}{} & \HoloSegScore{20.35}{(18.46--22.45)}{4.55pt}{4.82pt}{} & \HoloSegScore{14.27}{(12.13--16.51)}{4.55pt}{4.82pt}{} & \HoloSegScore{18.96}{(16.24--21.76)}{4.55pt}{4.82pt}{} & \HoloSegScore{37.36}{(23.33--56.47)}{4.55pt}{4.82pt}{} & \HoloSegScore{14.43}{(12.08--17.26)}{4.55pt}{4.82pt}{} & \HoloSegScore{12.42}{(10.44--15.09)}{4.55pt}{4.82pt}{} \\
\cline{3-11}
 &  &  & \HoloSegMetric{Dice} & \HoloSegScore{0.4021}{(0.3543--0.4468)}{4.55pt}{4.82pt}{} & \HoloSegScore{0.1484}{(0.1218--0.1727)}{4.55pt}{4.82pt}{} & \HoloSegScore{0.4416}{(0.3947--0.4879)}{4.55pt}{4.82pt}{} & \HoloSegScore{0.4707}{(0.4147--0.5235)}{4.55pt}{4.82pt}{} & \HoloSegScore{0.1658}{(0.02130--0.3196)}{4.20pt}{4.48pt}{} & \HoloSegScore{0.4782}{(0.4331--0.5189)}{4.55pt}{4.82pt}{} & \HoloSegScore{0.4828}{(0.4391--0.5237)}{4.55pt}{4.82pt}{} \\*
\softcline{4-11}
 &  & \HoloSegSpan{\makecell[c]{right\\[-0.10ex]adrenal\\[-0.10ex]gland}}{2.04cm}{0.32cm} & \HoloSegMetric{HD95} & \HoloSegScore{11.11}{(9.458--13.07)}{4.55pt}{4.82pt}{} & \HoloSegScore{19.89}{(17.32--22.68)}{4.55pt}{4.82pt}{} & \HoloSegScore{8.961}{(7.374--11.13)}{4.55pt}{4.82pt}{} & \HoloSegScore{13.88}{(11.12--16.78)}{4.55pt}{4.82pt}{} & \HoloSegScore{36.48}{(22.42--56.55)}{4.55pt}{4.82pt}{} & \HoloSegScore{8.851}{(7.061--10.96)}{4.55pt}{4.82pt}{} & \HoloSegScore{9.356}{(7.295--11.70)}{4.55pt}{4.82pt}{} \\
\cline{3-11}
 &  &  & \HoloSegMetric{Dice} & \HoloSegScore{0.7850}{(0.7274--0.8385)}{4.55pt}{4.82pt}{} & \HoloSegScore{0.5710}{(0.5129--0.6316)}{4.55pt}{4.82pt}{} & \HoloSegScore{0.7739}{(0.7079--0.8301)}{4.55pt}{4.82pt}{} & \HoloSegScore{0.8063}{(0.7571--0.8493)}{4.55pt}{4.82pt}{} & \HoloSegScore{0.5555}{(0.4462--0.6745)}{4.55pt}{4.82pt}{} & \HoloSegScore{0.8540}{(0.8070--0.8931)}{4.55pt}{4.82pt}{} & \HoloSegScore{0.8585}{(0.8122--0.8968)}{4.55pt}{4.82pt}{} \\*
\softcline{4-11}
 &  & \HoloSegSpan{\makecell[c]{urinary\\[-0.10ex]bladder}}{2.04cm}{0.32cm} & \HoloSegMetric{HD95} & \HoloSegScore{16.89}{(8.583--27.64)}{4.55pt}{4.82pt}{} & \HoloSegScore{24.07}{(17.71--32.67)}{4.55pt}{4.82pt}{} & \HoloSegScore{18.26}{(9.680--29.43)}{4.55pt}{4.82pt}{} & \HoloSegScore{14.15}{(10.15--19.43)}{4.55pt}{4.82pt}{} & \HoloSegScore{28.02}{(17.23--43.70)}{4.55pt}{4.82pt}{} & \HoloSegScore{7.773}{(5.396--10.75)}{4.55pt}{4.82pt}{} & \HoloSegScore{13.09}{(7.888--22.13)}{4.55pt}{4.82pt}{} \\
\cline{3-11}
 &  &  & \HoloSegMetric{Dice} &  & \HoloSegScore{0.5998}{(0.5799--0.6175)}{4.55pt}{4.82pt}{} & \HoloSegScore{0.1139}{(0.05941--0.1722)}{4.20pt}{4.48pt}{} & \HoloSegScore{0.9359}{(0.9306--0.9411)}{4.55pt}{4.82pt}{} & \HoloSegScore{0.6198}{(0.5293--0.7197)}{4.55pt}{4.82pt}{} & \HoloSegScore{0.9031}{(0.8973--0.9089)}{4.55pt}{4.82pt}{} & \HoloSegScore{0.9131}{(0.9083--0.9177)}{4.55pt}{4.82pt}{} \\*
\softcline{4-4}\softcline{6-11}
\HoloSegSpan{\makecell[c]{\textbf{External-}\\[-0.10ex]\textbf{seen}\\[-0.10ex]\textbf{(zero-}\\[-0.10ex]\textbf{shot)}}}{1.20cm}{0.32cm} &  & \HoloSegSpan{\makecell[c]{bone}}{2.04cm}{0.32cm} & \HoloSegMetric{HD95} & \raisebox{0.32cm}[0pt][0pt]{\HoloSegUnsupported} & \HoloSegScore{36.86}{(31.22--42.81)}{4.55pt}{4.82pt}{} & \HoloSegScore{163.7}{(147.7--181.5)}{4.55pt}{4.82pt}{} & \HoloSegScore{4.560}{(2.063--7.881)}{4.55pt}{4.82pt}{} & \HoloSegScore{16.87}{(9.919--26.87)}{4.55pt}{4.82pt}{} & \HoloSegScore{15.49}{(9.998--22.17)}{4.55pt}{4.82pt}{} & \HoloSegScore{18.17}{(11.16--26.16)}{4.55pt}{4.82pt}{} \\
\cline{3-11}
 &  &  & \HoloSegMetric{Dice} &  & \HoloSegScore{0.00008134}{(0.0000--0.0002440)}{3.85pt}{4.12pt}{} & \HoloSegScore{0.3291}{(0.1942--0.4713)}{4.55pt}{4.82pt}{} & \HoloSegScore{0.4196}{(0.3188--0.5381)}{4.55pt}{4.82pt}{} & \HoloSegScore{0.07670}{(0.001400--0.1872)}{4.20pt}{4.48pt}{} & \HoloSegScore{0.3270}{(0.2171--0.4452)}{4.55pt}{4.82pt}{} & \HoloSegScore{0.3445}{(0.2232--0.4686)}{4.55pt}{4.82pt}{} \\*
\softcline{4-4}\softcline{6-11}
 &  & \HoloSegSpan{\makecell[c]{left breast}}{2.04cm}{0.32cm} & \HoloSegMetric{HD95} & \raisebox{0.32cm}[0pt][0pt]{\HoloSegUnsupported} & \HoloSegScore{143.4}{(118.4--174.1)}{4.55pt}{4.82pt}{} & \HoloSegScore{19.92}{(12.37--29.10)}{4.55pt}{4.82pt}{} & \HoloSegScore{83.28}{(49.66--121.3)}{4.55pt}{4.82pt}{} & \HoloSegScore{108.3}{(77.81--149.4)}{4.55pt}{4.82pt}{} & \HoloSegScore{26.16}{(14.11--40.20)}{4.55pt}{4.82pt}{} & \HoloSegScore{61.41}{(23.78--105.6)}{4.55pt}{4.82pt}{} \\
\cline{3-11}
 & \HoloSegSpan{\makecell[c]{Pediatric-\\[-0.10ex]CT-SEG}}{1.86cm}{0.32cm} &  & \HoloSegMetric{Dice} &  & \HoloSegScore{0.0001054}{(0.0000--0.0003140)}{3.85pt}{4.12pt}{} & \HoloSegScore{0.4546}{(0.3291--0.5887)}{4.55pt}{4.82pt}{} & \HoloSegScore{0.3916}{(0.2732--0.5177)}{4.55pt}{4.82pt}{} & \HoloSegScore{0.07520}{(0.004600--0.1924)}{4.20pt}{4.48pt}{} & \HoloSegScore{0.4374}{(0.3272--0.5378)}{4.55pt}{4.82pt}{} & \HoloSegScore{0.4916}{(0.3671--0.5993)}{4.55pt}{4.82pt}{} \\*
\softcline{4-4}\softcline{6-11}
 &  & \HoloSegSpan{\makecell[c]{right breast}}{2.04cm}{0.32cm} & \HoloSegMetric{HD95} & \raisebox{0.32cm}[0pt][0pt]{\HoloSegUnsupported} & \HoloSegScore{131.0}{(119.0--144.6)}{4.55pt}{4.82pt}{} & \HoloSegScore{14.65}{(9.509--20.76)}{4.55pt}{4.82pt}{} & \HoloSegScore{67.96}{(39.73--98.16)}{4.55pt}{4.82pt}{} & \HoloSegScore{132.7}{(92.33--178.9)}{4.55pt}{4.82pt}{} & \HoloSegScore{65.59}{(44.00--94.37)}{4.55pt}{4.82pt}{} & \HoloSegScore{25.16}{(12.23--46.33)}{4.55pt}{4.82pt}{} \\
\cline{3-11}
 &  &  & \HoloSegMetric{Dice} & \HoloSegScore{0.4969}{(0.4485--0.5446)}{4.55pt}{4.82pt}{} & \HoloSegScore{0.3453}{(0.3117--0.3772)}{4.55pt}{4.82pt}{} & \HoloSegScore{0.5253}{(0.4778--0.5714)}{4.55pt}{4.82pt}{} & \HoloSegScore{0.5726}{(0.5348--0.6073)}{4.55pt}{4.82pt}{} & \HoloSegScore{0.2540}{(0.1025--0.3893)}{4.55pt}{4.82pt}{} & \HoloSegScore{0.5661}{(0.5231--0.6074)}{4.55pt}{4.82pt}{} & \HoloSegScore{0.6202}{(0.5858--0.6554)}{4.55pt}{4.82pt}{} \\*
\softcline{4-11}
 &  & \HoloSegSpan{\makecell[c]{duodenum}}{2.04cm}{0.32cm} & \HoloSegMetric{HD95} & \HoloSegScore{16.76}{(14.66--18.83)}{4.55pt}{4.82pt}{} & \HoloSegScore{21.28}{(18.76--24.09)}{4.55pt}{4.82pt}{} & \HoloSegScore{15.47}{(13.13--18.41)}{4.55pt}{4.82pt}{} & \HoloSegScore{20.18}{(16.95--24.18)}{4.55pt}{4.82pt}{} & \HoloSegScore{44.83}{(29.71--63.11)}{4.55pt}{4.82pt}{} & \HoloSegScore{16.15}{(14.21--18.36)}{4.55pt}{4.82pt}{} & \HoloSegScore{12.61}{(11.23--14.33)}{4.55pt}{4.82pt}{} \\
\cline{3-11}
 &  &  & \HoloSegMetric{Dice} & \HoloSegScore{0.6488}{(0.6183--0.6783)}{4.55pt}{4.82pt}{} & \HoloSegScore{0.4391}{(0.4106--0.4666)}{4.55pt}{4.82pt}{} & \HoloSegScore{0.6782}{(0.6439--0.7079)}{4.55pt}{4.82pt}{} & \HoloSegScore{0.6707}{(0.6411--0.6980)}{4.55pt}{4.82pt}{} & \HoloSegScore{0.3341}{(0.2136--0.4616)}{4.55pt}{4.82pt}{} & \HoloSegScore{0.6450}{(0.6118--0.6759)}{4.55pt}{4.82pt}{} & \HoloSegScore{0.6817}{(0.6536--0.7090)}{4.55pt}{4.82pt}{} \\*
\softcline{4-11}
 &  & \HoloSegSpan{\makecell[c]{esophagus}}{2.04cm}{0.32cm} & \HoloSegMetric{HD95} & \HoloSegScore{58.76}{(39.62--79.61)}{4.55pt}{4.82pt}{} & \HoloSegScore{10.71}{(9.638--11.86)}{4.55pt}{4.82pt}{} & \HoloSegScore{6.654}{(5.687--7.805)}{4.55pt}{4.82pt}{} & \HoloSegScore{7.941}{(6.580--9.616)}{4.55pt}{4.82pt}{} & \HoloSegScore{30.92}{(19.80--47.95)}{4.55pt}{4.82pt}{} & \HoloSegScore{10.23}{(7.951--13.00)}{4.55pt}{4.82pt}{} & \HoloSegScore{9.630}{(7.519--12.10)}{4.55pt}{4.82pt}{} \\
\cline{3-11}
 &  &  & \HoloSegMetric{Dice} & \HoloSegScore{0.01970}{(0.006673--0.03838)}{3.85pt}{4.12pt}{} & \HoloSegScore{0.07471}{(0.04781--0.1060)}{4.20pt}{4.48pt}{} & \HoloSegScore{0.003148}{(0.001675--0.005009)}{3.85pt}{4.12pt}{} & \HoloSegScore{0.01868}{(0.01431--0.02310)}{4.20pt}{4.48pt}{} & \HoloSegScore{0.08640}{(0.007300--0.2088)}{4.20pt}{4.48pt}{} & \HoloSegScore{0.4617}{(0.3738--0.5424)}{4.55pt}{4.82pt}{} & \HoloSegScore{0.6304}{(0.5653--0.6907)}{4.55pt}{4.82pt}{} \\*
\softcline{4-11}
 &  & \HoloSegSpan{\makecell[c]{left hip}}{2.04cm}{0.32cm} & \HoloSegMetric{HD95} & \HoloSegScore{82.75}{(77.75--87.59)}{4.55pt}{4.82pt}{} & \HoloSegScore{88.41}{(82.83--94.57)}{4.55pt}{4.82pt}{} & \HoloSegScore{120.6}{(101.3--141.2)}{4.55pt}{4.82pt}{} & \HoloSegScore{87.30}{(78.71--97.08)}{4.55pt}{4.82pt}{} & \HoloSegScore{166.5}{(116.9--215.4)}{4.55pt}{4.82pt}{} & \HoloSegScore{104.1}{(79.58--127.7)}{4.55pt}{4.82pt}{} & \HoloSegScore{246.9}{(206.7--289.4)}{4.55pt}{4.82pt}{} \\
\cline{3-11}
 &  &  & \HoloSegMetric{Dice} & \HoloSegScore{0.01821}{(0.009888--0.02719)}{3.85pt}{4.12pt}{} & \HoloSegScore{0.08068}{(0.06607--0.09556)}{4.20pt}{4.48pt}{} & \HoloSegScore{0.02296}{(0.009777--0.04006)}{3.85pt}{4.12pt}{} & \HoloSegScore{0.01134}{(0.007850--0.01556)}{3.85pt}{4.12pt}{} & \HoloSegScore{0.02440}{(0.007300--0.09330)}{3.85pt}{4.12pt}{} & \HoloSegScore{0.5554}{(0.4570--0.6480)}{4.55pt}{4.82pt}{} & \HoloSegScore{0.5766}{(0.5024--0.6476)}{4.55pt}{4.82pt}{} \\*
\softcline{4-11}
 &  & \HoloSegSpan{\makecell[c]{right hip}}{2.04cm}{0.32cm} & \HoloSegMetric{HD95} & \HoloSegScore{274.0}{(236.5--313.8)}{4.55pt}{4.82pt}{} & \HoloSegScore{148.6}{(131.1--167.5)}{4.55pt}{4.82pt}{} & \HoloSegScore{110.3}{(93.66--130.3)}{4.55pt}{4.82pt}{} & \HoloSegScore{81.66}{(76.29--87.42)}{4.55pt}{4.82pt}{} & \HoloSegScore{152.4}{(106.9--201.8)}{4.55pt}{4.82pt}{} & \HoloSegScore{63.76}{(45.51--85.28)}{4.55pt}{4.82pt}{} & \HoloSegScore{83.77}{(64.61--109.1)}{4.55pt}{4.82pt}{} \\
\hline
\pagebreak[4]
 &  &  & \HoloSegMetric{Dice} & \HoloSegScore{0.8224}{(0.7810--0.8557)}{4.55pt}{4.82pt}{} & \HoloSegScore{0.4515}{(0.3976--0.4994)}{4.55pt}{4.82pt}{} & \HoloSegScore{0.8146}{(0.7670--0.8530)}{4.55pt}{4.82pt}{} & \HoloSegScore{0.8281}{(0.7894--0.8613)}{4.55pt}{4.82pt}{} & \HoloSegScore{0.5037}{(0.3970--0.6212)}{4.55pt}{4.82pt}{} & \HoloSegScore{0.8585}{(0.8331--0.8802)}{4.55pt}{4.82pt}{} & \HoloSegScore{0.8505}{(0.8166--0.8827)}{4.55pt}{4.82pt}{} \\*
\softcline{4-11}
 &  & \HoloSegSpan{\makecell[c]{gallbladder}}{2.04cm}{0.32cm} & \HoloSegMetric{HD95} & \HoloSegScore{7.141}{(4.600--11.12)}{4.55pt}{4.82pt}{} & \HoloSegScore{16.76}{(14.19--19.48)}{4.55pt}{4.82pt}{} & \HoloSegScore{4.967}{(3.629--6.823)}{4.55pt}{4.82pt}{} & \HoloSegScore{6.141}{(4.496--8.171)}{4.55pt}{4.82pt}{} & \HoloSegScore{29.85}{(18.21--43.38)}{4.55pt}{4.82pt}{} & \HoloSegScore{4.343}{(3.349--5.654)}{4.55pt}{4.82pt}{} & \HoloSegScore{5.367}{(3.891--6.904)}{4.55pt}{4.82pt}{} \\
\cline{3-11}
 &  &  & \HoloSegMetric{Dice} &  & \HoloSegScore{0.0002080}{(0.000004660--0.0004483)}{3.25pt}{3.52pt}{} & \HoloSegScore{0.003774}{(0.0000--0.01036)}{4.20pt}{4.48pt}{} & \HoloSegScore{0.00001475}{(0.0000--0.00004425)}{3.85pt}{4.12pt}{} & \HoloSegScore{0.001921}{(0.0006837--0.03588)}{3.85pt}{4.12pt}{} & \HoloSegScore{0.04580}{(0.02509--0.06976)}{4.20pt}{4.48pt}{} & \HoloSegScore{0.04204}{(0.01917--0.07182)}{4.20pt}{4.48pt}{} \\*
\softcline{4-4}\softcline{6-11}
 &  & \HoloSegSpan{\makecell[c]{gonad}}{2.04cm}{0.32cm} & \HoloSegMetric{HD95} & \raisebox{0.32cm}[0pt][0pt]{\HoloSegUnsupported} & \HoloSegScore{148.4}{(132.1--166.0)}{4.55pt}{4.82pt}{} & \HoloSegScore{97.08}{(33.91--215.2)}{4.55pt}{4.82pt}{} & \HoloSegScore{67.28}{(35.99--92.56)}{4.55pt}{4.82pt}{} & \HoloSegScore{115.3}{(79.87--158.7)}{4.55pt}{4.82pt}{} & \HoloSegScore{99.22}{(82.50--119.8)}{4.55pt}{4.82pt}{} & \HoloSegScore{145.5}{(97.65--200.1)}{4.55pt}{4.82pt}{} \\
\cline{3-11}
 &  &  & \HoloSegMetric{Dice} & \HoloSegScore{0.8519}{(0.8417--0.8620)}{4.55pt}{4.82pt}{} & \HoloSegScore{0.2640}{(0.2335--0.2926)}{4.55pt}{4.82pt}{} & \HoloSegScore{0.8782}{(0.8643--0.8889)}{4.55pt}{4.82pt}{} & \HoloSegScore{0.5514}{(0.5044--0.6005)}{4.55pt}{4.82pt}{} & \HoloSegScore{0.5544}{(0.4506--0.6653)}{4.55pt}{4.82pt}{} & \HoloSegScore{0.9110}{(0.9015--0.9197)}{4.55pt}{4.82pt}{} & \HoloSegScore{0.8977}{(0.8880--0.9072)}{4.55pt}{4.82pt}{} \\*
\softcline{4-11}
 &  & \HoloSegSpan{\makecell[c]{heart}}{2.04cm}{0.32cm} & \HoloSegMetric{HD95} & \HoloSegScore{64.07}{(37.07--91.61)}{4.55pt}{4.82pt}{} & \HoloSegScore{34.06}{(31.41--37.30)}{4.55pt}{4.82pt}{} & \HoloSegScore{26.12}{(16.30--38.27)}{4.55pt}{4.82pt}{} & \HoloSegScore{21.66}{(17.31--26.64)}{4.55pt}{4.82pt}{} & \HoloSegScore{49.24}{(32.56--69.05)}{4.55pt}{4.82pt}{} & \HoloSegScore{13.18}{(10.56--16.48)}{4.55pt}{4.82pt}{} & \HoloSegScore{12.92}{(11.18--14.74)}{4.55pt}{4.82pt}{} \\
\cline{3-11}
 &  &  & \HoloSegMetric{Dice} & \HoloSegScore{0.9236}{(0.8841--0.9495)}{4.55pt}{4.82pt}{} & \HoloSegScore{0.7649}{(0.7334--0.7896)}{4.55pt}{4.82pt}{} & \HoloSegScore{0.9318}{(0.8941--0.9565)}{4.55pt}{4.82pt}{} & \HoloSegScore{0.9431}{(0.9168--0.9623)}{4.55pt}{4.82pt}{} & \HoloSegScore{0.6795}{(0.6088--0.7591)}{4.55pt}{4.82pt}{} & \HoloSegScore{0.9573}{(0.9442--0.9666)}{4.55pt}{4.82pt}{} & \HoloSegScore{0.9550}{(0.9402--0.9648)}{4.55pt}{4.82pt}{} \\*
\softcline{4-11}
 &  & \HoloSegSpan{\makecell[c]{left kidney}}{2.04cm}{0.32cm} & \HoloSegMetric{HD95} & \HoloSegScore{4.392}{(3.384--5.890)}{4.55pt}{4.82pt}{} & \HoloSegScore{33.47}{(25.15--41.47)}{4.55pt}{4.82pt}{} & \HoloSegScore{3.944}{(2.382--6.439)}{4.55pt}{4.82pt}{} & \HoloSegScore{5.512}{(3.138--9.007)}{4.55pt}{4.82pt}{} & \HoloSegScore{17.05}{(9.360--26.92)}{4.55pt}{4.82pt}{} & \HoloSegScore{3.527}{(2.273--5.153)}{4.55pt}{4.82pt}{} & \HoloSegScore{4.072}{(3.305--4.959)}{4.55pt}{4.82pt}{} \\
\cline{3-11}
 &  &  & \HoloSegMetric{Dice} & \HoloSegScore{0.9259}{(0.8916--0.9457)}{4.55pt}{4.82pt}{} & \HoloSegScore{0.7739}{(0.7514--0.7946)}{4.55pt}{4.82pt}{} & \HoloSegScore{0.9273}{(0.8890--0.9520)}{4.55pt}{4.82pt}{} & \HoloSegScore{0.9315}{(0.8995--0.9567)}{4.55pt}{4.82pt}{} & \HoloSegScore{0.6911}{(0.6206--0.7853)}{4.55pt}{4.82pt}{} & \HoloSegScore{0.9391}{(0.9087--0.9622)}{4.55pt}{4.82pt}{} & \HoloSegScore{0.9439}{(0.9200--0.9620)}{4.55pt}{4.82pt}{} \\*
\softcline{4-11}
 &  & \HoloSegSpan{\makecell[c]{right kidney}}{2.04cm}{0.32cm} & \HoloSegMetric{HD95} & \HoloSegScore{4.932}{(3.698--6.638)}{4.55pt}{4.82pt}{} & \HoloSegScore{24.81}{(18.19--31.65)}{4.55pt}{4.82pt}{} & \HoloSegScore{4.341}{(2.803--6.436)}{4.55pt}{4.82pt}{} & \HoloSegScore{6.816}{(4.287--10.70)}{4.55pt}{4.82pt}{} & \HoloSegScore{16.13}{(9.237--25.28)}{4.55pt}{4.82pt}{} & \HoloSegScore{4.544}{(2.954--6.534)}{4.55pt}{4.82pt}{} & \HoloSegScore{4.275}{(2.811--6.262)}{4.55pt}{4.82pt}{} \\
\cline{3-11}
 &  &  & \HoloSegMetric{Dice} & \HoloSegScore{0.6503}{(0.6102--0.6834)}{4.55pt}{4.82pt}{} & \HoloSegScore{0.3658}{(0.3231--0.4103)}{4.55pt}{4.82pt}{} & \HoloSegScore{0.6670}{(0.6254--0.7063)}{4.55pt}{4.82pt}{} & \HoloSegScore{0.6280}{(0.5867--0.6666)}{4.55pt}{4.82pt}{} & \HoloSegScore{0.4146}{(0.3097--0.5308)}{4.55pt}{4.82pt}{} & \HoloSegScore{0.6978}{(0.6618--0.7327)}{4.55pt}{4.82pt}{} & \HoloSegScore{0.7040}{(0.6640--0.7417)}{4.55pt}{4.82pt}{} \\*
\softcline{4-11}
 &  & \HoloSegSpan{\makecell[c]{colon}}{2.04cm}{0.32cm} & \HoloSegMetric{HD95} & \HoloSegScore{31.42}{(28.32--34.82)}{4.55pt}{4.82pt}{} & \HoloSegScore{38.11}{(33.84--44.21)}{4.55pt}{4.82pt}{} & \HoloSegScore{25.12}{(21.46--29.73)}{4.55pt}{4.82pt}{} & \HoloSegScore{43.60}{(35.90--52.28)}{4.55pt}{4.82pt}{} & \HoloSegScore{51.61}{(35.68--74.29)}{4.55pt}{4.82pt}{} & \HoloSegScore{36.64}{(28.66--46.83)}{4.55pt}{4.82pt}{} & \HoloSegScore{34.63}{(28.51--40.92)}{4.55pt}{4.82pt}{} \\
\cline{3-11}
 &  &  & \HoloSegMetric{Dice} & \HoloSegScore{0.9533}{(0.9500--0.9564)}{4.55pt}{4.82pt}{} & \HoloSegScore{0.8538}{(0.8464--0.8610)}{4.55pt}{4.82pt}{} & \HoloSegScore{0.9565}{(0.9535--0.9596)}{4.55pt}{4.82pt}{} & \HoloSegScore{0.9582}{(0.9525--0.9624)}{4.55pt}{4.82pt}{} & \HoloSegScore{0.7122}{(0.6480--0.7959)}{4.55pt}{4.82pt}{} & \HoloSegScore{0.9626}{(0.9600--0.9647)}{4.55pt}{4.82pt}{} & \HoloSegScore{0.9642}{(0.9615--0.9665)}{4.55pt}{4.82pt}{} \\*
\softcline{4-11}
 &  & \HoloSegSpan{\makecell[c]{liver}}{2.04cm}{0.32cm} & \HoloSegMetric{HD95} & \HoloSegScore{4.808}{(4.185--5.498)}{4.55pt}{4.82pt}{} & \HoloSegScore{12.65}{(11.41--14.38)}{4.55pt}{4.82pt}{} & \HoloSegScore{3.920}{(3.375--4.598)}{4.55pt}{4.82pt}{} & \HoloSegScore{7.901}{(5.509--10.96)}{4.55pt}{4.82pt}{} & \HoloSegScore{18.71}{(10.62--29.93)}{4.55pt}{4.82pt}{} & \HoloSegScore{4.668}{(3.858--5.729)}{4.55pt}{4.82pt}{} & \HoloSegScore{3.874}{(3.343--4.530)}{4.55pt}{4.82pt}{} \\
\cline{3-11}
 &  &  & \HoloSegMetric{Dice} & \HoloSegScore{0.9170}{(0.8959--0.9339)}{4.55pt}{4.82pt}{} & \HoloSegScore{0.7449}{(0.7066--0.7767)}{4.55pt}{4.82pt}{} & \HoloSegScore{0.9044}{(0.8831--0.9225)}{4.55pt}{4.82pt}{} & \HoloSegScore{0.9268}{(0.9072--0.9438)}{4.55pt}{4.82pt}{} & \HoloSegScore{0.5874}{(0.4965--0.6812)}{4.55pt}{4.82pt}{} & \HoloSegScore{0.9312}{(0.9110--0.9470)}{4.55pt}{4.82pt}{} & \HoloSegScore{0.9343}{(0.9136--0.9512)}{4.55pt}{4.82pt}{} \\*
\softcline{4-11}
 &  & \HoloSegSpan{\makecell[c]{left lung}}{2.04cm}{0.32cm} & \HoloSegMetric{HD95} & \HoloSegScore{14.00}{(11.02--17.43)}{4.55pt}{4.82pt}{} & \HoloSegScore{16.99}{(13.98--20.56)}{4.55pt}{4.82pt}{} & \HoloSegScore{27.10}{(17.90--37.23)}{4.55pt}{4.82pt}{} & \HoloSegScore{15.17}{(11.25--20.38)}{4.55pt}{4.82pt}{} & \HoloSegScore{51.17}{(34.02--73.85)}{4.55pt}{4.82pt}{} & \HoloSegScore{17.20}{(12.39--22.45)}{4.55pt}{4.82pt}{} & \HoloSegScore{9.662}{(6.744--13.16)}{4.55pt}{4.82pt}{} \\
\cline{3-11}
 &  &  & \HoloSegMetric{Dice} & \HoloSegScore{0.9253}{(0.9101--0.9382)}{4.55pt}{4.82pt}{} & \HoloSegScore{0.6514}{(0.5884--0.7069)}{4.55pt}{4.82pt}{} & \HoloSegScore{0.9188}{(0.9005--0.9351)}{4.55pt}{4.82pt}{} & \HoloSegScore{0.9402}{(0.9248--0.9541)}{4.55pt}{4.82pt}{} & \HoloSegScore{0.5866}{(0.5003--0.6913)}{4.55pt}{4.82pt}{} & \HoloSegScore{0.9417}{(0.9289--0.9527)}{4.55pt}{4.82pt}{} & \HoloSegScore{0.9435}{(0.9307--0.9545)}{4.55pt}{4.82pt}{} \\*
\softcline{4-11}
 &  & \HoloSegSpan{\makecell[c]{right lung}}{2.04cm}{0.32cm} & \HoloSegMetric{HD95} & \HoloSegScore{12.81}{(10.28--16.77)}{4.55pt}{4.82pt}{} & \HoloSegScore{27.81}{(22.21--34.07)}{4.55pt}{4.82pt}{} & \HoloSegScore{16.96}{(12.17--22.53)}{4.55pt}{4.82pt}{} & \HoloSegScore{13.59}{(10.04--17.74)}{4.55pt}{4.82pt}{} & \HoloSegScore{46.58}{(30.01--66.73)}{4.55pt}{4.82pt}{} & \HoloSegScore{16.08}{(11.97--20.88)}{4.55pt}{4.82pt}{} & \HoloSegScore{11.46}{(9.065--14.22)}{4.55pt}{4.82pt}{} \\
\cline{3-11}
 &  &  & \HoloSegMetric{Dice} & \HoloSegScore{0.7301}{(0.6896--0.7613)}{4.55pt}{4.82pt}{} & \HoloSegScore{0.4640}{(0.4333--0.4936)}{4.55pt}{4.82pt}{} & \HoloSegScore{0.7338}{(0.6957--0.7650)}{4.55pt}{4.82pt}{} & \HoloSegScore{0.7385}{(0.7051--0.7686)}{4.55pt}{4.82pt}{} & \HoloSegScore{0.5101}{(0.4057--0.6291)}{4.55pt}{4.82pt}{} & \HoloSegScore{0.7732}{(0.7506--0.7948)}{4.55pt}{4.82pt}{} & \HoloSegScore{0.7746}{(0.7483--0.7985)}{4.55pt}{4.82pt}{} \\*
\softcline{4-11}
\HoloSegSpan{\makecell[c]{\textbf{External-}\\[-0.10ex]\textbf{seen}\\[-0.10ex]\textbf{(zero-}\\[-0.10ex]\textbf{shot)}}}{1.20cm}{0.32cm} & \HoloSegSpan{\makecell[c]{Pediatric-\\[-0.10ex]CT-SEG}}{1.86cm}{0.32cm} & \HoloSegSpan{\makecell[c]{pancreas}}{2.04cm}{0.32cm} & \HoloSegMetric{HD95} & \HoloSegScore{9.082}{(7.610--10.75)}{4.55pt}{4.82pt}{} & \HoloSegScore{14.95}{(12.80--17.32)}{4.55pt}{4.82pt}{} & \HoloSegScore{7.807}{(6.306--9.509)}{4.55pt}{4.82pt}{} & \HoloSegScore{13.65}{(10.64--17.31)}{4.55pt}{4.82pt}{} & \HoloSegScore{30.77}{(19.86--47.47)}{4.55pt}{4.82pt}{} & \HoloSegScore{7.570}{(6.497--8.769)}{4.55pt}{4.82pt}{} & \HoloSegScore{8.190}{(6.732--9.881)}{4.55pt}{4.82pt}{} \\
\cline{3-11}
 &  &  & \HoloSegMetric{Dice} & \HoloSegScore{0.1408}{(0.07076--0.2272)}{4.20pt}{4.48pt}{} & \HoloSegScore{0.06738}{(0.02323--0.1193)}{4.20pt}{4.48pt}{} & \HoloSegScore{0.2763}{(0.1836--0.3761)}{4.55pt}{4.82pt}{} & \HoloSegScore{0.1114}{(0.04114--0.1957)}{4.20pt}{4.48pt}{} & \HoloSegScore{0.05250}{(0.002500--0.1658)}{4.20pt}{4.48pt}{} & \HoloSegScore{0.3505}{(0.2618--0.4414)}{4.55pt}{4.82pt}{} & \HoloSegScore{0.2341}{(0.1592--0.3167)}{4.55pt}{4.82pt}{} \\*
\softcline{4-11}
 &  & \HoloSegSpan{\makecell[c]{prostate}}{2.04cm}{0.32cm} & \HoloSegMetric{HD95} & \HoloSegScore{147.8}{(94.27--203.7)}{4.55pt}{4.82pt}{} & \HoloSegScore{50.54}{(38.96--64.15)}{4.55pt}{4.82pt}{} & \HoloSegScore{8.190}{(6.210--10.56)}{4.55pt}{4.82pt}{} & \HoloSegScore{22.06}{(11.18--39.70)}{4.55pt}{4.82pt}{} & \HoloSegScore{32.49}{(19.55--51.89)}{4.55pt}{4.82pt}{} & \HoloSegScore{21.13}{(15.00--28.83)}{4.55pt}{4.82pt}{} & \HoloSegScore{118.9}{(89.17--149.1)}{4.55pt}{4.82pt}{} \\
\cline{3-11}
 &  &  & \HoloSegMetric{Dice} &  & \HoloSegScore{0.08611}{(0.05616--0.1171)}{4.20pt}{4.48pt}{} & \HoloSegScore{0.6553}{(0.6072--0.6984)}{4.55pt}{4.82pt}{} & \HoloSegScore{0.4765}{(0.4177--0.5325)}{4.55pt}{4.82pt}{} & \HoloSegScore{0.007900}{(0.005100--0.09110)}{3.85pt}{4.12pt}{} & \HoloSegScore{0.6589}{(0.6098--0.7050)}{4.55pt}{4.82pt}{} & \HoloSegScore{0.6587}{(0.6087--0.7051)}{4.55pt}{4.82pt}{} \\*
\softcline{4-4}\softcline{6-11}
 &  & \HoloSegSpan{\makecell[c]{rectum}}{2.04cm}{0.32cm} & \HoloSegMetric{HD95} & \raisebox{0.32cm}[0pt][0pt]{\HoloSegUnsupported} & \HoloSegScore{39.90}{(35.84--44.07)}{4.55pt}{4.82pt}{} & \HoloSegScore{29.61}{(18.71--41.90)}{4.55pt}{4.82pt}{} & \HoloSegScore{23.35}{(19.66--27.23)}{4.55pt}{4.82pt}{} & \HoloSegScore{122.2}{(85.49--167.6)}{4.55pt}{4.82pt}{} & \HoloSegScore{59.34}{(33.38--87.80)}{4.55pt}{4.82pt}{} & \HoloSegScore{32.70}{(20.98--48.44)}{4.55pt}{4.82pt}{} \\
\cline{3-11}
 &  &  & \HoloSegMetric{Dice} &  & \HoloSegScore{0.00008226}{(0.00004011--0.0001389)}{3.52pt}{3.80pt}{} & \HoloSegScore{0.6575}{(0.6405--0.6721)}{4.55pt}{4.82pt}{} & \HoloSegScore{0.5786}{(0.5505--0.6057)}{4.55pt}{4.82pt}{} & \HoloSegScore{0.1684}{(0.01960--0.3218)}{4.20pt}{4.48pt}{} & \HoloSegScore{0.6201}{(0.5986--0.6390)}{4.55pt}{4.82pt}{} & \HoloSegScore{0.6621}{(0.6439--0.6789)}{4.55pt}{4.82pt}{} \\*
\softcline{4-4}\softcline{6-11}
 &  & \HoloSegSpan{\makecell[c]{skin}}{2.04cm}{0.32cm} & \HoloSegMetric{HD95} & \raisebox{0.32cm}[0pt][0pt]{\HoloSegUnsupported} & \HoloSegScore{78.94}{(73.08--85.01)}{4.55pt}{4.82pt}{} & \HoloSegScore{11.70}{(9.560--14.04)}{4.55pt}{4.82pt}{} & \HoloSegScore{26.80}{(23.23--30.48)}{4.55pt}{4.82pt}{} & \HoloSegScore{46.66}{(30.59--65.87)}{4.55pt}{4.82pt}{} & \HoloSegScore{15.55}{(12.63--18.96)}{4.55pt}{4.82pt}{} & \HoloSegScore{11.71}{(9.145--14.63)}{4.55pt}{4.82pt}{} \\
\cline{3-11}
 &  &  & \HoloSegMetric{Dice} & \HoloSegScore{0.6352}{(0.5899--0.6782)}{4.55pt}{4.82pt}{} & \HoloSegScore{0.3886}{(0.3400--0.4382)}{4.55pt}{4.82pt}{} & \HoloSegScore{0.6871}{(0.6460--0.7221)}{4.55pt}{4.82pt}{} & \HoloSegScore{0.6624}{(0.6188--0.7013)}{4.55pt}{4.82pt}{} & \HoloSegScore{0.4384}{(0.3298--0.5518)}{4.55pt}{4.82pt}{} & \HoloSegScore{0.7709}{(0.7383--0.7942)}{4.55pt}{4.82pt}{} & \HoloSegScore{0.7641}{(0.7290--0.7914)}{4.55pt}{4.82pt}{} \\*
\softcline{4-11}
 &  & \HoloSegSpan{\makecell[c]{small bowel}}{2.04cm}{0.32cm} & \HoloSegMetric{HD95} & \HoloSegScore{25.98}{(20.84--32.57)}{4.55pt}{4.82pt}{} & \HoloSegScore{39.92}{(32.65--48.25)}{4.55pt}{4.82pt}{} & \HoloSegScore{19.77}{(16.03--26.53)}{4.55pt}{4.82pt}{} & \HoloSegScore{29.32}{(24.19--35.65)}{4.55pt}{4.82pt}{} & \HoloSegScore{48.19}{(30.73--70.83)}{4.55pt}{4.82pt}{} & \HoloSegScore{20.44}{(16.47--26.14)}{4.55pt}{4.82pt}{} & \HoloSegScore{19.18}{(15.49--24.80)}{4.55pt}{4.82pt}{} \\
\cline{3-11}
 &  &  & \HoloSegMetric{Dice} &  & \HoloSegScore{0.002467}{(0.0007330--0.004736)}{3.52pt}{3.80pt}{} & \HoloSegScore{0.7677}{(0.7528--0.7841)}{4.55pt}{4.82pt}{} & \HoloSegScore{0.8668}{(0.8464--0.8816)}{4.55pt}{4.82pt}{} & \HoloSegScore{0.4504}{(0.3487--0.5662)}{4.55pt}{4.82pt}{} & \HoloSegScore{0.7455}{(0.7298--0.7610)}{4.55pt}{4.82pt}{} & \HoloSegScore{0.8563}{(0.8438--0.8671)}{4.55pt}{4.82pt}{} \\*
\softcline{4-4}\softcline{6-11}
 &  & \HoloSegSpan{\makecell[c]{spinal canal}}{2.04cm}{0.32cm} & \HoloSegMetric{HD95} & \raisebox{0.32cm}[0pt][0pt]{\HoloSegUnsupported} & \HoloSegScore{191.9}{(166.0--214.5)}{4.55pt}{4.82pt}{} & \HoloSegScore{54.81}{(51.12--58.85)}{4.55pt}{4.82pt}{} & \HoloSegScore{3.736}{(3.031--4.421)}{4.55pt}{4.82pt}{} & \HoloSegScore{31.64}{(19.39--48.13)}{4.55pt}{4.82pt}{} & \HoloSegScore{77.40}{(72.54--82.94)}{4.55pt}{4.82pt}{} & \HoloSegScore{37.04}{(29.31--44.87)}{4.55pt}{4.82pt}{} \\
\cline{3-11}
 &  &  & \HoloSegMetric{Dice} & \HoloSegScore{0.9306}{(0.9219--0.9389)}{4.55pt}{4.82pt}{} & \HoloSegScore{0.7554}{(0.7367--0.7749)}{4.55pt}{4.82pt}{} & \HoloSegScore{0.9260}{(0.9126--0.9386)}{4.55pt}{4.82pt}{} & \HoloSegScore{0.9239}{(0.9076--0.9374)}{4.55pt}{4.82pt}{} & \HoloSegScore{0.6689}{(0.5956--0.7633)}{4.55pt}{4.82pt}{} & \HoloSegScore{0.9390}{(0.9290--0.9480)}{4.55pt}{4.82pt}{} & \HoloSegScore{0.9453}{(0.9341--0.9534)}{4.55pt}{4.82pt}{} \\*
\softcline{4-11}
 &  & \HoloSegSpan{\makecell[c]{spleen}}{2.04cm}{0.32cm} & \HoloSegMetric{HD95} & \HoloSegScore{4.204}{(3.275--5.541)}{4.55pt}{4.82pt}{} & \HoloSegScore{10.97}{(9.858--12.15)}{4.55pt}{4.82pt}{} & \HoloSegScore{3.972}{(2.858--5.481)}{4.55pt}{4.82pt}{} & \HoloSegScore{11.52}{(8.538--14.69)}{4.55pt}{4.82pt}{} & \HoloSegScore{19.13}{(11.64--30.04)}{4.55pt}{4.82pt}{} & \HoloSegScore{3.791}{(2.803--4.837)}{4.55pt}{4.82pt}{} & \HoloSegScore{3.096}{(2.324--4.184)}{4.55pt}{4.82pt}{} \\
\cline{3-11}
 &  &  & \HoloSegMetric{Dice} & \HoloSegScore{0.8568}{(0.8213--0.8832)}{4.55pt}{4.82pt}{} & \HoloSegScore{0.5876}{(0.5447--0.6264)}{4.55pt}{4.82pt}{} & \HoloSegScore{0.7226}{(0.6561--0.7825)}{4.55pt}{4.82pt}{} & \HoloSegScore{0.7722}{(0.7340--0.8116)}{4.55pt}{4.82pt}{} & \HoloSegScore{0.6390}{(0.5595--0.7466)}{4.55pt}{4.82pt}{} & \HoloSegScore{0.8794}{(0.8513--0.9047)}{4.55pt}{4.82pt}{} & \HoloSegScore{0.8754}{(0.8466--0.9028)}{4.55pt}{4.82pt}{} \\*
\softcline{4-11}
 &  & \HoloSegSpan{\makecell[c]{stomach}}{2.04cm}{0.32cm} & \HoloSegMetric{HD95} & \HoloSegScore{9.943}{(7.632--12.59)}{4.55pt}{4.82pt}{} & \HoloSegScore{19.23}{(16.97--21.48)}{4.55pt}{4.82pt}{} & \HoloSegScore{55.23}{(36.57--75.27)}{4.55pt}{4.82pt}{} & \HoloSegScore{24.25}{(19.66--29.16)}{4.55pt}{4.82pt}{} & \HoloSegScore{26.92}{(16.75--40.13)}{4.55pt}{4.82pt}{} & \HoloSegScore{8.683}{(6.514--11.06)}{4.55pt}{4.82pt}{} & \HoloSegScore{10.62}{(7.803--13.93)}{4.55pt}{4.82pt}{} \\
\cline{3-11}
 &  &  & \HoloSegMetric{Dice} &  & \HoloSegScore{0.007088}{(0.001957--0.01311)}{3.85pt}{4.12pt}{} & \HoloSegScore{0.1952}{(0.1233--0.2787)}{4.55pt}{4.82pt}{} & \HoloSegScore{0.0000}{(0.0000--0.0000)}{4.55pt}{4.82pt}{} & \HoloSegScore{0.1080}{(0.007500--0.2358)}{4.20pt}{4.48pt}{} & \HoloSegScore{0.4862}{(0.4123--0.5558)}{4.55pt}{4.82pt}{} & \HoloSegScore{0.5471}{(0.4676--0.6157)}{4.55pt}{4.82pt}{} \\*
\softcline{4-4}\softcline{6-11}
 &  & \HoloSegSpan{\makecell[c]{thymus}}{2.04cm}{0.32cm} & \HoloSegMetric{HD95} & \raisebox{0.32cm}[0pt][0pt]{\HoloSegUnsupported} & \HoloSegScore{130.4}{(117.1--143.5)}{4.55pt}{4.82pt}{} & \HoloSegScore{22.29}{(17.19--27.32)}{4.55pt}{4.82pt}{} & \HoloSegScore{--}{(--\,--)}{4.55pt}{4.82pt}{} & \HoloSegScore{54.13}{(35.64--79.24)}{4.55pt}{4.82pt}{} & \HoloSegScore{16.80}{(13.37--20.24)}{4.55pt}{4.82pt}{} & \HoloSegScore{22.44}{(12.98--38.40)}{4.55pt}{4.82pt}{} \\
\cline{3-11}
 &  &  & \HoloSegMetric{Dice} &  & \HoloSegScore{0.1226}{(0.07594--0.1710)}{4.20pt}{4.48pt}{} & \HoloSegScore{0.009672}{(0.001133--0.02196)}{3.85pt}{4.12pt}{} & \HoloSegScore{0.1036}{(0.04398--0.1802)}{4.20pt}{4.48pt}{} & \HoloSegScore{0.06510}{(0.002300--0.1836)}{4.20pt}{4.48pt}{} & \HoloSegScore{0.3242}{(0.2396--0.4005)}{4.55pt}{4.82pt}{} & \HoloSegScore{0.3626}{(0.2763--0.4457)}{4.55pt}{4.82pt}{} \\*
\softcline{4-4}\softcline{6-11}
 &  & \HoloSegSpan{\makecell[c]{uterocervix}}{2.04cm}{0.32cm} & \HoloSegMetric{HD95} & \raisebox{0.32cm}[0pt][0pt]{\HoloSegUnsupported} & \HoloSegScore{47.65}{(40.80--54.78)}{4.55pt}{4.82pt}{} & \HoloSegScore{156.6}{(113.9--194.7)}{4.55pt}{4.82pt}{} & \HoloSegScore{42.95}{(31.55--54.10)}{4.55pt}{4.82pt}{} & \HoloSegScore{75.33}{(51.78--107.1)}{4.55pt}{4.82pt}{} & \HoloSegScore{41.42}{(28.67--57.11)}{4.55pt}{4.82pt}{} & \HoloSegScore{34.81}{(24.69--46.68)}{4.55pt}{4.82pt}{} \\
\hline
\pagebreak[4]
 &  &  & \HoloSegMetric{Dice} & \HoloSegScore{0.3136}{(0.2600--0.3601)}{4.55pt}{4.82pt}{} & \HoloSegScore{0.2238}{(0.1629--0.2842)}{4.55pt}{4.82pt}{} & \HoloSegScore{0.1086}{(0.06328--0.1660)}{4.20pt}{4.48pt}{} & \HoloSegScore{0.4117}{(0.3754--0.4468)}{4.55pt}{4.82pt}{} & \HoloSegScore{0.1793}{(0.1651--0.2041)}{4.55pt}{4.82pt}{} & \HoloSegScore{0.3050}{(0.2590--0.3497)}{4.55pt}{4.82pt}{} & \HoloSegScore{0.3460}{(0.3044--0.3822)}{4.55pt}{4.82pt}{} \\*
\softcline{4-11}
 &  & \HoloSegSpan{\makecell[c]{hepatic vein}}{2.04cm}{0.32cm} & \HoloSegMetric{HD95} & \HoloSegScore{27.74}{(25.06--30.48)}{4.55pt}{4.82pt}{} & \HoloSegScore{39.88}{(34.06--47.81)}{4.55pt}{4.82pt}{} & \HoloSegScore{41.34}{(33.04--49.92)}{4.55pt}{4.82pt}{} & \HoloSegScore{21.22}{(18.39--24.76)}{4.55pt}{4.82pt}{} & \HoloSegScore{41.49}{(31.19--45.82)}{4.55pt}{4.82pt}{} & \HoloSegScore{24.66}{(22.24--27.06)}{4.55pt}{4.82pt}{} & \HoloSegScore{26.64}{(24.44--28.67)}{4.55pt}{4.82pt}{} \\
\cline{3-11}
 &  &  & \HoloSegMetric{Dice} &  & \HoloSegScore{0.1366}{(0.08519--0.1931)}{4.20pt}{4.48pt}{} & \HoloSegScore{0.1034}{(0.06409--0.1489)}{4.20pt}{4.48pt}{} & \HoloSegScore{0.4604}{(0.4388--0.4831)}{4.55pt}{4.82pt}{} & \HoloSegScore{0.1030}{(0.06272--0.1246)}{4.20pt}{4.48pt}{} & \HoloSegScore{0.4382}{(0.4020--0.4752)}{4.55pt}{4.82pt}{} & \HoloSegScore{0.4995}{(0.4658--0.5350)}{4.55pt}{4.82pt}{} \\*
\softcline{4-4}\softcline{6-11}
 & \HoloSegSpan{\makecell[c]{VEELA2025}}{1.86cm}{0.32cm} & \HoloSegSpan{\makecell[c]{portal vein}}{2.04cm}{0.32cm} & \HoloSegMetric{HD95} & \raisebox{0.32cm}[0pt][0pt]{\HoloSegUnsupported} & \HoloSegScore{67.87}{(56.94--79.32)}{4.55pt}{4.82pt}{} & \HoloSegScore{69.33}{(57.23--80.76)}{4.55pt}{4.82pt}{} & \HoloSegScore{78.94}{(71.22--87.59)}{4.55pt}{4.82pt}{} & \HoloSegScore{68.92}{(62.11--75.02)}{4.55pt}{4.82pt}{} & \HoloSegScore{32.31}{(30.15--34.55)}{4.55pt}{4.82pt}{} & \HoloSegScore{34.69}{(28.50--42.27)}{4.55pt}{4.82pt}{} \\
\cline{3-11}
 &  &  & \HoloSegMetric{Dice} & \HoloSegScore{0.9693}{(0.9665--0.9720)}{4.55pt}{4.82pt}{} & \HoloSegScore{0.7977}{(0.6556--0.9350)}{4.55pt}{4.82pt}{} & \HoloSegScore{0.9731}{(0.9707--0.9750)}{4.55pt}{4.82pt}{} & \HoloSegScore{0.9717}{(0.9682--0.9748)}{4.55pt}{4.82pt}{} & \HoloSegScore{0.7143}{(0.6828--0.7392)}{4.55pt}{4.82pt}{} & \HoloSegScore{0.9702}{(0.9681--0.9726)}{4.55pt}{4.82pt}{} & \HoloSegScore{0.9728}{(0.9700--0.9757)}{4.55pt}{4.82pt}{} \\*
\softcline{4-11}
 &  & \HoloSegSpan{\makecell[c]{liver}}{2.04cm}{0.32cm} & \HoloSegMetric{HD95} & \HoloSegScore{3.713}{(3.166--4.416)}{4.55pt}{4.82pt}{} & \HoloSegScore{5.482}{(5.057--5.917)}{4.55pt}{4.82pt}{} & \HoloSegScore{2.487}{(2.276--2.702)}{4.55pt}{4.82pt}{} & \HoloSegScore{4.327}{(3.436--5.328)}{4.55pt}{4.82pt}{} & \HoloSegScore{15.87}{(14.64--17.95)}{4.55pt}{4.82pt}{} & \HoloSegScore{4.886}{(4.166--5.696)}{4.55pt}{4.82pt}{} & \HoloSegScore{3.291}{(2.738--3.940)}{4.55pt}{4.82pt}{} \\
\cline{2-11}
 &  &  & \HoloSegMetric{Dice} & \HoloSegScore{0.9347}{(0.9296--0.9393)}{4.55pt}{4.82pt}{} & \HoloSegScore{0.3551}{(0.2878--0.4223)}{4.55pt}{4.82pt}{} & \HoloSegScore{0.9361}{(0.9330--0.9388)}{4.55pt}{4.82pt}{} & \HoloSegScore{0.8502}{(0.7926--0.8976)}{4.55pt}{4.82pt}{} & \HoloSegScore{0.5583}{(0.4634--0.6784)}{4.55pt}{4.82pt}{} & \HoloSegScore{0.8892}{(0.8793--0.8989)}{4.55pt}{4.82pt}{} & \HoloSegScore{0.9284}{(0.9204--0.9353)}{4.55pt}{4.82pt}{} \\*
\softcline{4-11}
 &  & \HoloSegSpan{\makecell[c]{sacrum}}{2.04cm}{0.32cm} & \HoloSegMetric{HD95} & \HoloSegScore{2.290}{(1.712--3.019)}{4.55pt}{4.82pt}{} & \HoloSegScore{52.06}{(38.07--66.36)}{4.55pt}{4.82pt}{} & \HoloSegScore{1.572}{(1.345--1.875)}{4.55pt}{4.82pt}{} & \HoloSegScore{7.080}{(4.229--10.40)}{4.55pt}{4.82pt}{} & \HoloSegScore{16.76}{(9.575--27.19)}{4.55pt}{4.82pt}{} & \HoloSegScore{5.716}{(4.902--6.497)}{4.55pt}{4.82pt}{} & \HoloSegScore{2.844}{(2.285--3.447)}{4.55pt}{4.82pt}{} \\
\cline{3-11}
 &  &  & \HoloSegMetric{Dice} & \HoloSegScore{0.9529}{(0.9515--0.9542)}{4.55pt}{4.82pt}{} & \HoloSegScore{0.3445}{(0.2760--0.4149)}{4.55pt}{4.82pt}{} & \HoloSegScore{0.9570}{(0.9557--0.9582)}{4.55pt}{4.82pt}{} & \HoloSegScore{0.8881}{(0.8350--0.9299)}{4.55pt}{4.82pt}{} & \HoloSegScore{0.5793}{(0.4899--0.6908)}{4.55pt}{4.82pt}{} & \HoloSegScore{0.9562}{(0.9498--0.9607)}{4.55pt}{4.82pt}{} & \HoloSegScore{0.9631}{(0.9545--0.9687)}{4.55pt}{4.82pt}{} \\*
\softcline{4-11}
 & \HoloSegSpan{\makecell[c]{Pengwin}}{1.86cm}{0.32cm} & \HoloSegSpan{\makecell[c]{left hip}}{2.04cm}{0.32cm} & \HoloSegMetric{HD95} & \HoloSegScore{1.215}{(1.175--1.265)}{4.55pt}{4.82pt}{} & \HoloSegScore{76.26}{(61.04--92.17)}{4.55pt}{4.82pt}{} & \HoloSegScore{1.067}{(1.038--1.099)}{4.55pt}{4.82pt}{} & \HoloSegScore{17.68}{(11.13--24.76)}{4.55pt}{4.82pt}{} & \HoloSegScore{18.21}{(9.790--29.56)}{4.55pt}{4.82pt}{} & \HoloSegScore{38.90}{(30.96--47.71)}{4.55pt}{4.82pt}{} & \HoloSegScore{3.594}{(1.534--6.123)}{4.55pt}{4.82pt}{} \\
\cline{3-11}
 &  &  & \HoloSegMetric{Dice} & \HoloSegScore{0.9522}{(0.9505--0.9539)}{4.55pt}{4.82pt}{} & \HoloSegScore{0.3648}{(0.2951--0.4290)}{4.55pt}{4.82pt}{} & \HoloSegScore{0.9559}{(0.9540--0.9575)}{4.55pt}{4.82pt}{} & \HoloSegScore{0.8800}{(0.8322--0.9234)}{4.55pt}{4.82pt}{} & \HoloSegScore{0.5812}{(0.4980--0.6929)}{4.55pt}{4.82pt}{} & \HoloSegScore{0.9628}{(0.9553--0.9677)}{4.55pt}{4.82pt}{} & \HoloSegScore{0.9633}{(0.9575--0.9680)}{4.55pt}{4.82pt}{} \\*
\softcline{4-11}
 &  & \HoloSegSpan{\makecell[c]{right hip}}{2.04cm}{0.32cm} & \HoloSegMetric{HD95} & \HoloSegScore{2.352}{(1.236--4.520)}{4.55pt}{4.82pt}{} & \HoloSegScore{76.50}{(61.79--91.34)}{4.55pt}{4.82pt}{} & \HoloSegScore{1.318}{(1.080--1.773)}{4.55pt}{4.82pt}{} & \HoloSegScore{13.99}{(8.368--20.46)}{4.55pt}{4.82pt}{} & \HoloSegScore{18.10}{(10.47--30.63)}{4.55pt}{4.82pt}{} & \HoloSegScore{5.434}{(1.465--10.81)}{4.55pt}{4.82pt}{} & \HoloSegScore{4.167}{(1.105--8.428)}{4.55pt}{4.82pt}{} \\
\cline{2-11}
\HoloSegSpan{\makecell[c]{\textbf{External-}\\[-0.10ex]\textbf{seen}\\[-0.10ex]\textbf{(zero-}\\[-0.10ex]\textbf{shot)}}}{1.20cm}{0.32cm} &  &  & \HoloSegMetric{Dice} &  & \HoloSegScore{0.0006353}{(0.00002192--0.001675)}{3.52pt}{3.80pt}{} & \HoloSegScore{0.2819}{(0.1972--0.3694)}{4.55pt}{4.82pt}{} & \HoloSegScore{0.2154}{(0.1446--0.2881)}{4.55pt}{4.82pt}{} & \HoloSegScore{0.1873}{(0.09772--0.2877)}{4.20pt}{4.48pt}{} & \HoloSegScore{0.3219}{(0.2393--0.4067)}{4.55pt}{4.82pt}{} & \HoloSegScore{0.4069}{(0.3181--0.4835)}{4.55pt}{4.82pt}{} \\*
\softcline{4-4}\softcline{6-11}
 & \HoloSegSpan{\makecell[c]{MHB-SEG-\\[-0.10ex]oneclass}}{1.86cm}{0.32cm} & \HoloSegSpan{\makecell[c]{intracranial\\[-0.10ex]hemorrhage}}{2.04cm}{0.32cm} & \HoloSegMetric{HD95} & \raisebox{0.32cm}[0pt][0pt]{\HoloSegUnsupported} & \HoloSegScore{87.13}{(80.73--93.08)}{4.55pt}{4.82pt}{} & \HoloSegScore{49.39}{(40.36--58.28)}{4.55pt}{4.82pt}{} & \HoloSegScore{61.83}{(53.43--70.32)}{4.55pt}{4.82pt}{} & \HoloSegScore{79.92}{(70.62--89.30)}{4.55pt}{4.82pt}{} & \HoloSegScore{56.13}{(46.17--65.28)}{4.55pt}{4.82pt}{} & \HoloSegScore{54.52}{(45.81--63.56)}{4.55pt}{4.82pt}{} \\
\cline{2-11}
 &  &  & \HoloSegMetric{Dice} & \HoloSegScore{0.2222}{(0.05556--0.4444)}{4.20pt}{4.48pt}{} & \HoloSegScore{0.05491}{(0.008992--0.1157)}{4.20pt}{4.48pt}{} & \HoloSegScore{0.0001425}{(0.0000--0.0004275)}{3.85pt}{4.12pt}{} & \HoloSegScore{0.04201}{(0.0000--0.1035)}{4.55pt}{4.82pt}{} & \HoloSegScore{0.1389}{(0.1169--0.3456)}{4.55pt}{4.82pt}{} & \HoloSegScore{0.7761}{(0.7302--0.7931)}{4.55pt}{4.82pt}{} & \HoloSegScore{0.7841}{(0.7405--0.8041)}{4.55pt}{4.82pt}{} \\*
\softcline{4-11}
 &  & \HoloSegSpan{\makecell[c]{pancreas}}{2.04cm}{0.32cm} & \HoloSegMetric{HD95} & \HoloSegScore{53.47}{(0.0000--126.3)}{4.55pt}{4.82pt}{} & \HoloSegScore{67.65}{(51.01--83.90)}{4.55pt}{4.82pt}{} & \HoloSegScore{116.3}{(85.79--147.8)}{4.55pt}{4.82pt}{} & \HoloSegScore{78.52}{(44.38--121.6)}{4.55pt}{4.82pt}{} & \HoloSegScore{64.11}{(40.59--100.1)}{4.55pt}{4.82pt}{} & \HoloSegScore{8.600}{(7.439--9.381)}{4.55pt}{4.82pt}{} & \HoloSegScore{7.953}{(6.330--9.587)}{4.55pt}{4.82pt}{} \\
\cline{3-11}
 & \HoloSegSpan{\makecell[c]{QUBIQ2021}}{1.86cm}{0.32cm} &  & \HoloSegMetric{Dice} & \HoloSegScore{0.0000}{(0.0000--0.0000)}{4.55pt}{4.82pt}{} & \HoloSegScore{0.06874}{(0.01625--0.1300)}{4.20pt}{4.48pt}{} & \HoloSegScore{0.0000}{(0.0000--0.0000)}{4.55pt}{4.82pt}{} & \HoloSegScore{0.1035}{(0.02533--0.1865)}{4.20pt}{4.48pt}{} & \HoloSegScore{0.03778}{(0.01692--0.08354)}{4.20pt}{4.48pt}{} & \HoloSegScore{0.2608}{(0.1629--0.3595)}{4.55pt}{4.82pt}{} & \HoloSegScore{0.3342}{(0.2669--0.4065)}{4.55pt}{4.82pt}{} \\*
\softcline{4-11}
 &  & \HoloSegSpan{\makecell[c]{pancreas\\[-0.10ex]lesion}}{2.04cm}{0.32cm} & \HoloSegMetric{HD95} & \HoloSegScore{169.0}{(140.0--199.6)}{4.55pt}{4.82pt}{} & \HoloSegScore{106.0}{(95.29--119.8)}{4.55pt}{4.82pt}{} & \HoloSegScore{67.62}{(46.26--91.31)}{4.55pt}{4.82pt}{} & \HoloSegScore{83.94}{(32.54--140.0)}{4.55pt}{4.82pt}{} & \HoloSegScore{111.3}{(97.42--183.6)}{4.55pt}{4.82pt}{} & \HoloSegScore{39.97}{(32.72--48.42)}{4.55pt}{4.82pt}{} & \HoloSegScore{28.69}{(24.11--33.59)}{4.55pt}{4.82pt}{} \\
\cline{2-11}
 &  &  & \HoloSegMetric{Dice} & \HoloSegScore{0.5862}{(0.5510--0.6225)}{4.55pt}{4.82pt}{} & \HoloSegScore{0.1780}{(0.1482--0.2067)}{4.55pt}{4.82pt}{} & \HoloSegScore{0.2491}{(0.2132--0.2837)}{4.55pt}{4.82pt}{} & \HoloSegScore{0.5485}{(0.5103--0.5844)}{4.55pt}{4.82pt}{} & \HoloSegScore{0.1338}{(0.1127--0.1462)}{4.55pt}{4.82pt}{} & \HoloSegScore{0.6493}{(0.6166--0.6803)}{4.55pt}{4.82pt}{} & \HoloSegScore{0.6936}{(0.6650--0.7204)}{4.55pt}{4.82pt}{} \\*
\softcline{4-11}
 & \HoloSegSpan{\makecell[c]{TotalSeg-\\[-0.10ex]subtask-\\[-0.10ex]liver-\\[-0.10ex]lesion}}{1.86cm}{0.32cm} & \HoloSegSpan{\makecell[c]{liver lesion}}{2.04cm}{0.32cm} & \HoloSegMetric{HD95} & \HoloSegScore{41.44}{(36.53--47.30)}{4.55pt}{4.82pt}{} & \HoloSegScore{83.83}{(78.70--89.34)}{4.55pt}{4.82pt}{} & \HoloSegScore{45.47}{(39.86--51.45)}{4.55pt}{4.82pt}{} & \HoloSegScore{48.04}{(42.68--53.40)}{4.55pt}{4.82pt}{} & \HoloSegScore{84.91}{(81.97--90.66)}{4.55pt}{4.82pt}{} & \HoloSegScore{30.12}{(26.09--34.36)}{4.55pt}{4.82pt}{} & \HoloSegScore{32.69}{(28.54--37.04)}{4.55pt}{4.82pt}{} \\
\cline{2-11}
 &  &  & \HoloSegMetric{Dice} & \HoloSegScore{0.4004}{(0.3189--0.4733)}{4.55pt}{4.82pt}{} & \HoloSegScore{0.7549}{(0.6756--0.8280)}{4.55pt}{4.82pt}{} & \HoloSegScore{0.5683}{(0.5069--0.6276)}{4.55pt}{4.82pt}{} & \HoloSegScore{0.5929}{(0.4990--0.6750)}{4.55pt}{4.82pt}{} & \HoloSegScore{0.3983}{(0.2868--0.4596)}{4.55pt}{4.82pt}{} & \HoloSegScore{0.9241}{(0.9022--0.9420)}{4.55pt}{4.82pt}{} & \HoloSegScore{0.9166}{(0.8905--0.9375)}{4.55pt}{4.82pt}{} \\*
\softcline{4-11}
 & \HoloSegSpan{\makecell[c]{HCC-TACE-\\[-0.10ex]Seg}}{1.86cm}{0.32cm} & \HoloSegSpan{\makecell[c]{liver}}{2.04cm}{0.32cm} & \HoloSegMetric{HD95} & \HoloSegScore{93.19}{(80.65--104.8)}{4.55pt}{4.82pt}{} & \HoloSegScore{25.62}{(16.60--37.10)}{4.55pt}{4.82pt}{} & \HoloSegScore{82.96}{(70.19--95.35)}{4.55pt}{4.82pt}{} & \HoloSegScore{95.30}{(82.89--107.6)}{4.55pt}{4.82pt}{} & \HoloSegScore{87.83}{(84.58--111.0)}{4.55pt}{4.82pt}{} & \HoloSegScore{24.22}{(15.64--33.88)}{4.55pt}{4.82pt}{} & \HoloSegScore{12.84}{(10.20--15.45)}{4.55pt}{4.82pt}{} \\
\cline{2-11}
 &  &  & \HoloSegMetric{Dice} &  & \HoloSegScore{0.01906}{(0.01440--0.02426)}{4.20pt}{4.48pt}{} & \HoloSegScore{0.001345}{(0.0002719--0.003120)}{3.52pt}{3.80pt}{} & \HoloSegScore{0.3549$^{\blacktriangle}$}{(0.3089--0.3980)}{4.55pt}{4.82pt}{} & \HoloSegScore{0.07302}{(0.06472--0.07823)}{4.20pt}{4.48pt}{} & \HoloSegScore{0.1910}{(0.1607--0.2208)}{4.55pt}{4.82pt}{} & \HoloSegScore{0.2647}{(0.2272--0.2997)}{4.55pt}{4.82pt}{} \\*
\softcline{4-4}\softcline{6-11}
 & \HoloSegSpan{\makecell[c]{PANORAMA}}{1.86cm}{0.32cm} & \HoloSegSpan{\makecell[c]{pancreatic\\[-0.10ex]duct}}{2.04cm}{0.32cm} & \HoloSegMetric{HD95} & \raisebox{0.32cm}[0pt][0pt]{\HoloSegUnsupported} & \HoloSegScore{62.18}{(56.79--67.75)}{4.55pt}{4.82pt}{} & \HoloSegScore{70.79}{(50.44--94.79)}{4.55pt}{4.82pt}{} & \HoloSegScore{30.57$^{\blacktriangle}$}{(26.85--34.50)}{4.55pt}{4.82pt}{} & \HoloSegScore{59.85}{(53.11--65.39)}{4.55pt}{4.82pt}{} & \HoloSegScore{43.84}{(40.58--47.13)}{4.55pt}{4.82pt}{} & \HoloSegScore{34.43}{(31.08--38.12)}{4.55pt}{4.82pt}{} \\
\hline
 &  &  & \HoloSegMetric{Dice} &  & \HoloSegScore{0.02013}{(0.006038--0.04199)}{3.85pt}{4.12pt}{} & \HoloSegScore{0.0000}{(0.0000--0.0000)}{4.55pt}{4.82pt}{} & \HoloSegScore{0.1529}{(0.09906--0.2146)}{4.20pt}{4.48pt}{} &  & \HoloSegScore{0.1170}{(0.07211--0.1660)}{4.20pt}{4.48pt}{} & \HoloSegScore{0.2109}{(0.1568--0.2659)}{4.55pt}{4.82pt}{} \\*
\softcline{4-4}\softcline{6-8}\softcline{10-11}
 & \HoloSegSpan{\makecell[c]{ULS23-NIG-\\[-0.10ex]LN-ABD}}{1.86cm}{0.32cm} & \HoloSegSpan{\makecell[c]{abdominal\\[-0.10ex]lymph node}}{2.04cm}{0.32cm} & \HoloSegMetric{HD95} & \raisebox{0.32cm}[0pt][0pt]{\HoloSegUnsupported} & \HoloSegScore{82.61}{(76.86--88.16)}{4.55pt}{4.82pt}{} & \HoloSegScore{38.31}{(38.31--38.31)}{4.55pt}{4.82pt}{} & \HoloSegScore{63.36}{(58.03--68.74)}{4.55pt}{4.82pt}{} & \raisebox{0.32cm}[0pt][0pt]{\HoloSegUnsupported} & \HoloSegScore{43.04}{(36.58--49.25)}{4.55pt}{4.82pt}{} & \HoloSegScore{39.13}{(33.36--45.06)}{4.55pt}{4.82pt}{} \\
\cline{2-11}
 &  &  & \HoloSegMetric{Dice} & \HoloSegScore{0.1648}{(0.0000--0.3696)}{4.55pt}{4.82pt}{} & \HoloSegScore{0.008280}{(0.0003008--0.02242)}{3.85pt}{4.12pt}{} & \HoloSegScore{0.002161}{(0.0001841--0.005225)}{3.52pt}{3.80pt}{} & \HoloSegScore{0.01918}{(0.00008726--0.05219)}{3.52pt}{3.80pt}{} &  & \HoloSegScore{0.08578}{(0.05759--0.1178)}{4.20pt}{4.48pt}{} & \HoloSegScore{0.1538}{(0.1192--0.1906)}{4.55pt}{4.82pt}{} \\*
\softcline{4-8}\softcline{10-11}
 & \HoloSegSpan{\makecell[c]{ULS23-\\[-0.10ex]Radboudumc-\\[-0.10ex]Bone}}{1.86cm}{0.32cm} & \HoloSegSpan{\makecell[c]{bone lesion}}{2.04cm}{0.32cm} & \HoloSegMetric{HD95} & \HoloSegScore{32.85}{(27.73--38.85)}{4.55pt}{4.82pt}{} & \HoloSegScore{89.56}{(81.95--98.03)}{4.55pt}{4.82pt}{} & \HoloSegScore{93.70}{(84.75--102.7)}{4.55pt}{4.82pt}{} & \HoloSegScore{76.63}{(66.01--87.73)}{4.55pt}{4.82pt}{} & \raisebox{0.32cm}[0pt][0pt]{\HoloSegUnsupported} & \HoloSegScore{37.75}{(31.07--46.35)}{4.55pt}{4.82pt}{} & \HoloSegScore{32.35}{(28.07--36.28)}{4.55pt}{4.82pt}{} \\
\cline{2-11}
 &  &  & \HoloSegMetric{Dice} &  & \HoloSegScore{0.004582}{(0.001279--0.009446)}{3.85pt}{4.12pt}{} & \HoloSegScore{0.0004724}{(0.0000--0.001265)}{4.20pt}{4.48pt}{} & \HoloSegScore{0.06145}{(0.02352--0.1064)}{4.20pt}{4.48pt}{} &  & \HoloSegScore{0.1722}{(0.1136--0.2407)}{4.55pt}{4.82pt}{} & \HoloSegScore{0.2102}{(0.1435--0.2798)}{4.55pt}{4.82pt}{} \\*
\softcline{4-4}\softcline{6-8}\softcline{10-11}
 & \HoloSegSpan{\makecell[c]{ULS23-\\[-0.10ex]DeepLesion3D}}{1.86cm}{0.32cm} & \HoloSegSpan{\makecell[c]{lesion}}{2.04cm}{0.32cm} & \HoloSegMetric{HD95} & \raisebox{0.32cm}[0pt][0pt]{\HoloSegUnsupported} & \HoloSegScore{98.13}{(90.15--107.2)}{4.55pt}{4.82pt}{} & \HoloSegScore{94.79}{(87.87--101.8)}{4.55pt}{4.82pt}{} & \HoloSegScore{54.29}{(44.39--64.53)}{4.55pt}{4.82pt}{} & \raisebox{0.32cm}[0pt][0pt]{\HoloSegUnsupported} & \HoloSegScore{40.27}{(31.97--49.39)}{4.55pt}{4.82pt}{} & \HoloSegScore{37.66}{(29.42--46.09)}{4.55pt}{4.82pt}{} \\
\cline{2-11}
 &  &  & \HoloSegMetric{Dice} &  & \HoloSegScore{0.01018}{(0.001135--0.02459)}{3.85pt}{4.12pt}{} & \HoloSegScore{0.0000}{(0.0000--0.0000)}{4.55pt}{4.82pt}{} & \HoloSegScore{0.03879}{(0.01030--0.06972)}{4.20pt}{4.48pt}{} &  & \HoloSegScore{0.1404}{(0.03606--0.2741)}{4.20pt}{4.48pt}{} & \HoloSegScore{0.2723}{(0.08376--0.4746)}{4.20pt}{4.48pt}{} \\*
\softcline{4-4}\softcline{6-8}\softcline{10-11}
\HoloSegSpan{\makecell[c]{\textbf{External-}\\[-0.10ex]\textbf{unseen}\\[-0.10ex]\textbf{(zero-}\\[-0.10ex]\textbf{shot)}}}{1.20cm}{0.32cm} & \HoloSegSpan{\makecell[c]{CT-Lymph-\\[-0.10ex]Nodes}}{1.86cm}{0.32cm} & \HoloSegSpan{\makecell[c]{abdominal\\[-0.10ex]lymph node}}{2.04cm}{0.32cm} & \HoloSegMetric{HD95} & \raisebox{0.32cm}[0pt][0pt]{\HoloSegUnsupported} & \HoloSegScore{164.5}{(104.1--222.7)}{4.55pt}{4.82pt}{} & \HoloSegScore{237.0}{(196.5--280.0)}{4.55pt}{4.82pt}{} & \HoloSegScore{283.3}{(227.3--354.6)}{4.55pt}{4.82pt}{} & \raisebox{0.32cm}[0pt][0pt]{\HoloSegUnsupported} & \HoloSegScore{163.4}{(108.9--210.5)}{4.55pt}{4.82pt}{} & \HoloSegScore{141.8}{(84.89--201.7)}{4.55pt}{4.82pt}{} \\
\cline{2-11}
 &  &  & \HoloSegMetric{Dice} &  & \HoloSegScore{0.0000}{(0.0000--0.0000)}{4.55pt}{4.82pt}{} & \HoloSegScore{0.0000}{(0.0000--0.0000)}{4.55pt}{4.82pt}{} & \HoloSegScore{0.0000}{(0.0000--0.0000)}{4.55pt}{4.82pt}{} &  & \HoloSegScore{0.02401}{(0.0000--0.05538)}{4.20pt}{4.48pt}{} & \HoloSegScore{0.1481}{(0.03280--0.2635)}{4.20pt}{4.48pt}{} \\*
\softcline{4-4}\softcline{6-8}\softcline{10-11}
 &  & \HoloSegSpan{\makecell[c]{epidural\\[-0.10ex]hemorrhage}}{2.04cm}{0.32cm} & \HoloSegMetric{HD95} & \raisebox{0.32cm}[0pt][0pt]{\HoloSegUnsupported} & \HoloSegScore{99.04}{(85.50--112.6)}{4.55pt}{4.82pt}{} & \HoloSegScore{63.25}{(18.36--98.73)}{4.55pt}{4.82pt}{} & \HoloSegScore{100.3}{(100.3--100.3)}{4.55pt}{4.82pt}{} & \raisebox{0.32cm}[0pt][0pt]{\HoloSegUnsupported} & \HoloSegScore{60.53}{(29.79--84.06)}{4.55pt}{4.82pt}{} & \HoloSegScore{65.61}{(43.02--87.97)}{4.55pt}{4.82pt}{} \\
\cline{3-11}
 &  &  & \HoloSegMetric{Dice} &  & \HoloSegScore{0.001488}{(0.0000--0.004252)}{4.20pt}{4.48pt}{} & \HoloSegScore{0.3481}{(0.2215--0.4899)}{4.55pt}{4.82pt}{} & \HoloSegScore{0.2614}{(0.1448--0.3892)}{4.55pt}{4.82pt}{} &  & \HoloSegScore{0.4107}{(0.2589--0.5586)}{4.55pt}{4.82pt}{} & \HoloSegScore{0.4532}{(0.3026--0.6053)}{4.55pt}{4.82pt}{} \\*
\softcline{4-4}\softcline{6-8}\softcline{10-11}
 & \HoloSegSpan{\makecell[c]{MHB-SEG-\\[-0.10ex]multiclass}}{1.86cm}{0.32cm} & \HoloSegSpan{\makecell[c]{subdural\\[-0.10ex]hemorrhage}}{2.04cm}{0.32cm} & \HoloSegMetric{HD95} & \raisebox{0.32cm}[0pt][0pt]{\HoloSegUnsupported} & \HoloSegScore{84.68}{(76.94--93.21)}{4.55pt}{4.82pt}{} & \HoloSegScore{37.66}{(25.78--49.66)}{4.55pt}{4.82pt}{} & \HoloSegScore{69.98}{(57.18--82.05)}{4.55pt}{4.82pt}{} & \raisebox{0.32cm}[0pt][0pt]{\HoloSegUnsupported} & \HoloSegScore{42.69}{(29.71--58.29)}{4.55pt}{4.82pt}{} & \HoloSegScore{46.94}{(31.14--64.33)}{4.55pt}{4.82pt}{} \\
\cline{3-11}
 &  &  & \HoloSegMetric{Dice} &  & \HoloSegScore{0.00005765}{(0.0000--0.0001729)}{3.85pt}{4.12pt}{} & \HoloSegScore{0.2185}{(0.1089--0.3331)}{4.55pt}{4.82pt}{} & \HoloSegScore{0.1549}{(0.05791--0.2796)}{4.20pt}{4.48pt}{} &  & \HoloSegScore{0.1458}{(0.06387--0.2362)}{4.20pt}{4.48pt}{} & \HoloSegScore{0.2698}{(0.1478--0.3947)}{4.55pt}{4.82pt}{} \\*
\softcline{4-4}\softcline{6-8}\softcline{10-11}
 &  & \HoloSegSpan{\makecell[c]{subarachnoid\\[-0.10ex]hemorrhage}}{2.04cm}{0.32cm} & \HoloSegMetric{HD95} & \raisebox{0.32cm}[0pt][0pt]{\HoloSegUnsupported} & \HoloSegScore{81.28}{(73.69--89.61)}{4.55pt}{4.82pt}{} & \HoloSegScore{54.63}{(41.70--67.04)}{4.55pt}{4.82pt}{} & \HoloSegScore{67.43}{(53.18--84.89)}{4.55pt}{4.82pt}{} & \raisebox{0.32cm}[0pt][0pt]{\HoloSegUnsupported} & \HoloSegScore{50.17}{(41.31--60.45)}{4.55pt}{4.82pt}{} & \HoloSegScore{44.32}{(34.48--54.15)}{4.55pt}{4.82pt}{} \\
\hline
\pagebreak[4]
 &  &  & \HoloSegMetric{Dice} &  & \HoloSegScore{0.003667}{(0.0000--0.009758)}{4.20pt}{4.48pt}{} & \HoloSegScore{0.09978}{(0.04260--0.1712)}{4.20pt}{4.48pt}{} & \HoloSegScore{0.07165}{(0.01379--0.1510)}{4.20pt}{4.48pt}{} &  & \HoloSegScore{0.1014}{(0.05298--0.1557)}{4.20pt}{4.48pt}{} & \HoloSegScore{0.1073}{(0.04726--0.1846)}{4.20pt}{4.48pt}{} \\*
\softcline{4-4}\softcline{6-8}\softcline{10-11}
 &  & \HoloSegSpan{\makecell[c]{intraparenchymal\\[-0.10ex]hemorrhage}}{2.04cm}{0.32cm} & \HoloSegMetric{HD95} & \raisebox{0.32cm}[0pt][0pt]{\HoloSegUnsupported} & \HoloSegScore{83.40}{(73.95--92.38)}{4.55pt}{4.82pt}{} & \HoloSegScore{54.88}{(43.18--67.93)}{4.55pt}{4.82pt}{} & \HoloSegScore{78.71}{(63.92--94.72)}{4.55pt}{4.82pt}{} & \raisebox{0.32cm}[0pt][0pt]{\HoloSegUnsupported} & \HoloSegScore{60.88}{(52.72--69.58)}{4.55pt}{4.82pt}{} & \HoloSegScore{62.58}{(51.77--73.73)}{4.55pt}{4.82pt}{} \\
\cline{3-11}
 & \HoloSegSpan{\makecell[c]{MHB-SEG-\\[-0.10ex]multiclass}}{1.86cm}{0.32cm} &  & \HoloSegMetric{Dice} &  & \HoloSegScore{0.001244}{(0.0000--0.003699)}{4.20pt}{4.48pt}{} & \HoloSegScore{0.02984}{(0.01136--0.05626)}{4.20pt}{4.48pt}{} & \HoloSegScore{0.08302}{(0.03221--0.1446)}{4.20pt}{4.48pt}{} &  & \HoloSegScore{0.2030}{(0.1175--0.2972)}{4.55pt}{4.82pt}{} & \HoloSegScore{0.3504}{(0.2483--0.4575)}{4.55pt}{4.82pt}{} \\*
\softcline{4-4}\softcline{6-8}\softcline{10-11}
 &  & \HoloSegSpan{\makecell[c]{intraventricular\\[-0.10ex]hemorrhage}}{2.04cm}{0.32cm} & \HoloSegMetric{HD95} & \raisebox{0.32cm}[0pt][0pt]{\HoloSegUnsupported} & \HoloSegScore{86.53}{(78.41--94.72)}{4.55pt}{4.82pt}{} & \HoloSegScore{75.45}{(66.81--84.17)}{4.55pt}{4.82pt}{} & \HoloSegScore{66.66}{(56.81--77.41)}{4.55pt}{4.82pt}{} & \raisebox{0.32cm}[0pt][0pt]{\HoloSegUnsupported} & \HoloSegScore{64.31}{(52.04--75.83)}{4.55pt}{4.82pt}{} & \HoloSegScore{60.31}{(47.25--73.60)}{4.55pt}{4.82pt}{} \\
\cline{2-11}
 &  &  & \HoloSegMetric{Dice} &  & \HoloSegScore{0.4918}{(0.3794--0.5986)}{4.55pt}{4.82pt}{} & \HoloSegScore{0.4771}{(0.4562--0.4989)}{4.55pt}{4.82pt}{} & \HoloSegScore{0.6579}{(0.5546--0.7651)}{4.55pt}{4.82pt}{} &  & \HoloSegScore{0.8370}{(0.7055--0.9170)}{4.55pt}{4.82pt}{} & \HoloSegScore{0.8923}{(0.8164--0.9342)}{4.55pt}{4.82pt}{} \\*
\softcline{4-4}\softcline{6-8}\softcline{10-11}
 & \HoloSegSpan{\makecell[c]{Adrenal-\\[-0.10ex]ACC-Ki67}}{1.86cm}{0.32cm} & \HoloSegSpan{\makecell[c]{adrenocortical\\[-0.10ex]carcinoma}}{2.04cm}{0.32cm} & \HoloSegMetric{HD95} & \raisebox{0.32cm}[0pt][0pt]{\HoloSegUnsupported} & \HoloSegScore{49.52}{(36.34--63.01)}{4.55pt}{4.82pt}{} & \HoloSegScore{54.61}{(52.81--56.40)}{4.55pt}{4.82pt}{} & \HoloSegScore{23.37}{(14.90--32.49)}{4.55pt}{4.82pt}{} & \raisebox{0.32cm}[0pt][0pt]{\HoloSegUnsupported} & \HoloSegScore{34.18}{(10.40--63.09)}{4.55pt}{4.82pt}{} & \HoloSegScore{18.36}{(4.355--44.44)}{4.55pt}{4.82pt}{} \\
\cline{2-11}
 &  &  & \HoloSegMetric{Dice} &  & \HoloSegScore{0.06358}{(0.03703--0.09149)}{4.20pt}{4.48pt}{} & \HoloSegScore{0.00003823}{(0.0000--0.0001147)}{3.85pt}{4.12pt}{} & \HoloSegScore{0.5403$^{\blacktriangle}$}{(0.4713--0.6060)}{4.55pt}{4.82pt}{} &  & \HoloSegScore{0.4040}{(0.3465--0.4634)}{4.55pt}{4.82pt}{} & \HoloSegScore{0.4382}{(0.3665--0.5032)}{4.55pt}{4.82pt}{} \\*
\softcline{4-4}\softcline{6-8}\softcline{10-11}
 &  & \HoloSegSpan{\makecell[c]{pancreatic\\[-0.10ex]ductal\\[-0.10ex]adenocarcinoma}}{2.04cm}{0.32cm} & \HoloSegMetric{HD95} & \raisebox{0.32cm}[0pt][0pt]{\HoloSegUnsupported} & \HoloSegScore{92.86}{(81.70--104.5)}{4.55pt}{4.82pt}{} & \HoloSegScore{227.4}{(195.0--260.0)}{4.55pt}{4.82pt}{} & \HoloSegScore{21.06$^{\blacktriangle}$}{(14.52--27.61)}{4.55pt}{4.82pt}{} & \raisebox{0.32cm}[0pt][0pt]{\HoloSegUnsupported} & \HoloSegScore{27.52}{(22.95--32.52)}{4.55pt}{4.82pt}{} & \HoloSegScore{28.36}{(22.99--34.05)}{4.55pt}{4.82pt}{} \\
\cline{3-11}
\HoloSegSpan{\makecell[c]{\textbf{External-}\\[-0.10ex]\textbf{unseen}\\[-0.10ex]\textbf{(zero-}\\[-0.10ex]\textbf{shot)}}}{1.20cm}{0.32cm} &  &  & \HoloSegMetric{Dice} &  & \HoloSegScore{0.09721}{(0.08661--0.1081)}{4.20pt}{4.48pt}{} & \HoloSegScore{0.3073}{(0.2752--0.3387)}{4.55pt}{4.82pt}{} & \HoloSegScore{0.8379$^{\blacktriangle}$}{(0.8216--0.8529)}{4.55pt}{4.82pt}{} &  & \HoloSegScore{0.7008}{(0.6835--0.7177)}{4.55pt}{4.82pt}{} & \HoloSegScore{0.7661}{(0.7498--0.7798)}{4.55pt}{4.82pt}{} \\*
\softcline{4-4}\softcline{6-8}\softcline{10-11}
 &  & \HoloSegSpan{\makecell[c]{pancreatic\\[-0.10ex]veins}}{2.04cm}{0.32cm} & \HoloSegMetric{HD95} & \raisebox{0.32cm}[0pt][0pt]{\HoloSegUnsupported} & \HoloSegScore{39.71}{(37.06--43.06)}{4.55pt}{4.82pt}{} & \HoloSegScore{57.15}{(49.05--66.57)}{4.55pt}{4.82pt}{} & \HoloSegScore{15.99$^{\blacktriangle}$}{(13.59--18.85)}{4.55pt}{4.82pt}{} & \raisebox{0.32cm}[0pt][0pt]{\HoloSegUnsupported} & \HoloSegScore{18.00}{(16.31--19.86)}{4.55pt}{4.82pt}{} & \HoloSegScore{25.97}{(24.44--27.81)}{4.55pt}{4.82pt}{} \\
\cline{3-11}
 & \HoloSegSpan{\makecell[c]{PANORAMA}}{1.86cm}{0.32cm} &  & \HoloSegMetric{Dice} &  & \HoloSegScore{0.02302}{(0.02053--0.02560)}{4.20pt}{4.48pt}{} & \HoloSegScore{0.002528}{(0.0000004579--0.007547)}{3.25pt}{3.52pt}{} & \HoloSegScore{0.8251$^{\blacktriangle}$}{(0.8146--0.8356)}{4.55pt}{4.82pt}{} &  & \HoloSegScore{0.4146}{(0.3956--0.4339)}{4.55pt}{4.82pt}{} & \HoloSegScore{0.2630}{(0.2521--0.2734)}{4.55pt}{4.82pt}{} \\*
\softcline{4-4}\softcline{6-8}\softcline{10-11}
 &  & \HoloSegSpan{\makecell[c]{pancreatic\\[-0.10ex]arteries}}{2.04cm}{0.32cm} & \HoloSegMetric{HD95} & \raisebox{0.32cm}[0pt][0pt]{\HoloSegUnsupported} & \HoloSegScore{44.20}{(41.60--47.22)}{4.55pt}{4.82pt}{} & \HoloSegScore{171.9}{(101.8--255.7)}{4.55pt}{4.82pt}{} & \HoloSegScore{15.90$^{\blacktriangle}$}{(14.50--17.34)}{4.55pt}{4.82pt}{} & \raisebox{0.32cm}[0pt][0pt]{\HoloSegUnsupported} & \HoloSegScore{96.76}{(88.29--104.8)}{4.55pt}{4.82pt}{} & \HoloSegScore{86.21}{(73.86--98.08)}{4.55pt}{4.82pt}{} \\
\cline{3-11}
 &  &  & \HoloSegMetric{Dice} &  & \HoloSegScore{0.4686}{(0.4439--0.4942)}{4.55pt}{4.82pt}{} & \HoloSegScore{0.0005745}{(0.00001441--0.001338)}{3.52pt}{3.80pt}{} & \HoloSegScore{0.8422$^{\blacktriangle}$}{(0.8247--0.8587)}{4.55pt}{4.82pt}{} &  & \HoloSegScore{0.8331}{(0.8152--0.8506)}{4.55pt}{4.82pt}{} & \HoloSegScore{0.8521}{(0.8359--0.8686)}{4.55pt}{4.82pt}{} \\*
\softcline{4-4}\softcline{6-8}\softcline{10-11}
 &  & \HoloSegSpan{\makecell[c]{pancreatic\\[-0.10ex]parenchyma}}{2.04cm}{0.32cm} & \HoloSegMetric{HD95} & \raisebox{0.32cm}[0pt][0pt]{\HoloSegUnsupported} & \HoloSegScore{24.27}{(20.89--27.80)}{4.55pt}{4.82pt}{} & \HoloSegScore{223.1}{(187.8--262.0)}{4.55pt}{4.82pt}{} & \HoloSegScore{11.70$^{\blacktriangle}$}{(9.504--14.37)}{4.55pt}{4.82pt}{} & \raisebox{0.32cm}[0pt][0pt]{\HoloSegUnsupported} & \HoloSegScore{6.966}{(5.901--8.070)}{4.55pt}{4.82pt}{} & \HoloSegScore{7.511}{(6.211--8.870)}{4.55pt}{4.82pt}{} \\
\cline{2-11}
 &  &  & \HoloSegMetric{Dice} &  & \HoloSegScore{0.2264}{(0.1120--0.3515)}{4.55pt}{4.82pt}{} & \HoloSegScore{0.2471}{(0.1647--0.3415)}{4.55pt}{4.82pt}{} & \HoloSegScore{0.3140}{(0.2036--0.4299)}{4.55pt}{4.82pt}{} &  & \HoloSegScore{0.5944}{(0.4785--0.7013)}{4.55pt}{4.82pt}{} & \HoloSegScore{0.6428}{(0.5403--0.7401)}{4.55pt}{4.82pt}{} \\*
\softcline{4-4}\softcline{6-8}\softcline{10-11}
 & \HoloSegSpan{\makecell[c]{HCC-TACE-\\[-0.10ex]Seg}}{1.86cm}{0.32cm} & \HoloSegSpan{\makecell[c]{hepatocellular\\[-0.10ex]carcinoma}}{2.04cm}{0.32cm} & \HoloSegMetric{HD95} & \raisebox{0.32cm}[0pt][0pt]{\HoloSegUnsupported} & \HoloSegScore{96.72}{(74.08--119.9)}{4.55pt}{4.82pt}{} & \HoloSegScore{128.8}{(103.2--153.9)}{4.55pt}{4.82pt}{} & \HoloSegScore{133.6}{(109.9--158.4)}{4.55pt}{4.82pt}{} & \raisebox{0.32cm}[0pt][0pt]{\HoloSegUnsupported} & \HoloSegScore{28.84}{(19.96--38.95)}{4.55pt}{4.82pt}{} & \HoloSegScore{21.47}{(15.03--29.33)}{4.55pt}{4.82pt}{} \\
\hline
 &  &  & \HoloSegMetric{Dice} &  & \HoloSegScore{0.009046}{(0.002355--0.01793)}{3.85pt}{4.12pt}{} & \HoloSegScore{0.004320}{(0.0003728--0.01074)}{3.85pt}{4.12pt}{} & \HoloSegScore{0.1070}{(0.06581--0.1499)}{4.20pt}{4.48pt}{} &  & \HoloSegScore{0.3713}{(0.3313--0.4143)}{4.55pt}{4.82pt}{} & \HoloSegScore{0.4880}{(0.4413--0.5308)}{4.55pt}{4.82pt}{} \\*
\softcline{4-4}\softcline{6-8}\softcline{10-11}
 & \HoloSegSpan{\makecell[c]{Private01\\[-0.10ex](laryngeal\\[-0.10ex]cancer)}}{1.86cm}{0.32cm} & \HoloSegSpan{\makecell[c]{laryngeal\\[-0.10ex]cancer}}{2.04cm}{0.32cm} & \HoloSegMetric{HD95} & \raisebox{0.32cm}[0pt][0pt]{\HoloSegUnsupported} & \HoloSegScore{122.0}{(112.4--129.6)}{4.55pt}{4.82pt}{} & \HoloSegScore{44.68}{(28.75--63.27)}{4.55pt}{4.82pt}{} & \HoloSegScore{40.84}{(28.62--54.97)}{4.55pt}{4.82pt}{} & \raisebox{0.32cm}[0pt][0pt]{\HoloSegUnsupported} & \HoloSegScore{16.32}{(12.75--21.19)}{4.55pt}{4.82pt}{} & \HoloSegScore{14.62}{(10.83--20.13)}{4.55pt}{4.82pt}{} \\
\cline{2-11}
 &  &  & \HoloSegMetric{Dice} &  & \HoloSegScore{0.2409}{(0.2038--0.2777)}{4.55pt}{4.82pt}{} & \HoloSegScore{0.4417}{(0.4008--0.4831)}{4.55pt}{4.82pt}{} & \HoloSegScore{0.5428}{(0.5057--0.5794)}{4.55pt}{4.82pt}{} &  & \HoloSegScore{0.6962}{(0.6681--0.7257)}{4.55pt}{4.82pt}{} & \HoloSegScore{0.7152}{(0.6872--0.7412)}{4.55pt}{4.82pt}{} \\*
\softcline{4-4}\softcline{6-8}\softcline{10-11}
 & \HoloSegSpan{\makecell[c]{Private02\\[-0.10ex](lung\\[-0.10ex]cancer)}}{1.86cm}{0.32cm} & \HoloSegSpan{\makecell[c]{lung cancer}}{2.04cm}{0.32cm} & \HoloSegMetric{HD95} & \raisebox{0.32cm}[0pt][0pt]{\HoloSegUnsupported} & \HoloSegScore{112.8}{(101.8--123.5)}{4.55pt}{4.82pt}{} & \HoloSegScore{36.70}{(29.74--44.33)}{4.55pt}{4.82pt}{} & \HoloSegScore{93.66}{(85.68--102.1)}{4.55pt}{4.82pt}{} & \raisebox{0.32cm}[0pt][0pt]{\HoloSegUnsupported} & \HoloSegScore{33.61}{(27.75--40.91)}{4.55pt}{4.82pt}{} & \HoloSegScore{30.01}{(24.21--36.39)}{4.55pt}{4.82pt}{} \\
\cline{2-11}
 &  &  & \HoloSegMetric{Dice} &  & \HoloSegScore{0.0000}{(0.0000--0.0000)}{4.55pt}{4.82pt}{} & \HoloSegScore{0.0000}{(0.0000--0.0000)}{4.55pt}{4.82pt}{} & \HoloSegScore{0.0000}{(0.0000--0.0000)}{4.55pt}{4.82pt}{} &  & \HoloSegScore{0.1116}{(0.04548--0.1923)}{4.20pt}{4.48pt}{} & \HoloSegScore{0.1461}{(0.06687--0.2438)}{4.20pt}{4.48pt}{} \\*
\softcline{4-4}\softcline{6-8}\softcline{10-11}
\HoloSegSpan{\makecell[c]{\textbf{Private}\\[-0.10ex]\textbf{(zero-}\\[-0.10ex]\textbf{shot)}}}{1.20cm}{0.32cm} &  & \HoloSegSpan{\makecell[c]{malignant\\[-0.10ex]thyroid\\[-0.10ex]tumor}}{2.04cm}{0.32cm} & \HoloSegMetric{HD95} & \raisebox{0.32cm}[0pt][0pt]{\HoloSegUnsupported} & \HoloSegScore{143.7}{(122.3--163.2)}{4.55pt}{4.82pt}{} & \HoloSegScore{127.2}{(115.5--138.2)}{4.55pt}{4.82pt}{} & \HoloSegScore{34.60}{(30.97--38.22)}{4.55pt}{4.82pt}{} & \raisebox{0.32cm}[0pt][0pt]{\HoloSegUnsupported} & \HoloSegScore{35.27}{(30.47--40.12)}{4.55pt}{4.82pt}{} & \HoloSegScore{34.83}{(29.40--39.71)}{4.55pt}{4.82pt}{} \\
\cline{3-11}
 & \HoloSegSpan{\makecell[c]{Private03\\[-0.10ex](thyroid\\[-0.10ex]cancer-\\[-0.10ex]multi)}}{1.86cm}{0.32cm} &  & \HoloSegMetric{Dice} &  & \HoloSegScore{0.01230}{(0.0002859--0.02863)}{3.85pt}{4.12pt}{} & \HoloSegScore{0.0003445}{(0.0000--0.001017)}{4.20pt}{4.48pt}{} & \HoloSegScore{0.01297}{(0.001348--0.02792)}{3.85pt}{4.12pt}{} &  & \HoloSegScore{0.5331}{(0.4659--0.5910)}{4.55pt}{4.82pt}{} & \HoloSegScore{0.6232}{(0.5625--0.6787)}{4.55pt}{4.82pt}{} \\*
\softcline{4-4}\softcline{6-8}\softcline{10-11}
 &  & \HoloSegSpan{\makecell[c]{benign\\[-0.10ex]thyroid\\[-0.10ex]tumor}}{2.04cm}{0.32cm} & \HoloSegMetric{HD95} & \raisebox{0.32cm}[0pt][0pt]{\HoloSegUnsupported} & \HoloSegScore{93.72}{(87.13--100.4)}{4.55pt}{4.82pt}{} & \HoloSegScore{127.9}{(123.2--132.7)}{4.55pt}{4.82pt}{} & \HoloSegScore{27.58}{(23.65--31.57)}{4.55pt}{4.82pt}{} & \raisebox{0.32cm}[0pt][0pt]{\HoloSegUnsupported} & \HoloSegScore{24.41}{(21.38--27.49)}{4.55pt}{4.82pt}{} & \HoloSegScore{19.29}{(16.25--22.16)}{4.55pt}{4.82pt}{} \\
\cline{2-11}
 &  &  & \HoloSegMetric{Dice} &  & \HoloSegScore{0.002521}{(0.0006734--0.004839)}{3.52pt}{3.80pt}{} & \HoloSegScore{0.004120}{(0.001315--0.007779)}{3.85pt}{4.12pt}{} & \HoloSegScore{0.1804}{(0.1340--0.2260)}{4.55pt}{4.82pt}{} &  & \HoloSegScore{0.5442}{(0.4878--0.6007)}{4.55pt}{4.82pt}{} & \HoloSegScore{0.6183}{(0.5610--0.6719)}{4.55pt}{4.82pt}{} \\*
\softcline{4-4}\softcline{6-8}\softcline{10-11}
 & \HoloSegSpan{\makecell[c]{Private03\\[-0.10ex](thyroid\\[-0.10ex]cancer-\\[-0.10ex]one)}}{1.86cm}{0.32cm} & \HoloSegSpan{\makecell[c]{thyroid\\[-0.10ex]tumor}}{2.04cm}{0.32cm} & \HoloSegMetric{HD95} & \raisebox{0.32cm}[0pt][0pt]{\HoloSegUnsupported} & \HoloSegScore{103.1}{(94.03--111.9)}{4.55pt}{4.82pt}{} & \HoloSegScore{81.93}{(63.88--103.4)}{4.55pt}{4.82pt}{} & \HoloSegScore{25.88}{(23.33--28.39)}{4.55pt}{4.82pt}{} & \raisebox{0.32cm}[0pt][0pt]{\HoloSegUnsupported} & \HoloSegScore{21.12}{(18.00--24.71)}{4.55pt}{4.82pt}{} & \HoloSegScore{18.74}{(15.26--22.80)}{4.55pt}{4.82pt}{} \\
\hline
 &  &  & \HoloSegMetric{Dice} & \HoloSegScore{0.6157}{(0.5559--0.6720)}{4.55pt}{4.82pt}{} & \HoloSegScore{0.3903}{(0.3372--0.4595)}{4.55pt}{4.82pt}{} & \HoloSegScore{0.4822}{(0.4312--0.5418)}{4.55pt}{4.82pt}{} &  & \HoloSegScore{0.6545}{(0.6017--0.7070)}{4.55pt}{4.82pt}{} & \HoloSegScore{0.6684}{(0.6213--0.7147)}{4.55pt}{4.82pt}{} & \HoloSegScore{0.6839}{(0.6270--0.7202)}{4.55pt}{4.82pt}{} \\*
\softcline{4-7}\softcline{9-11}
 & \HoloSegSpan{\makecell[c]{Private01\\[-0.10ex](laryngeal\\[-0.10ex]cancer)}}{1.86cm}{0.32cm} & \HoloSegSpan{\makecell[c]{laryngeal\\[-0.10ex]cancer}}{2.04cm}{0.32cm} & \HoloSegMetric{HD95} & \HoloSegScore{17.08}{(12.91--23.86)}{4.55pt}{4.82pt}{} & \HoloSegScore{27.04}{(19.56--35.33)}{4.55pt}{4.82pt}{} & \HoloSegScore{19.29}{(13.08--25.48)}{4.55pt}{4.82pt}{} & \raisebox{0.32cm}[0pt][0pt]{\HoloSegUnsupported} & \HoloSegScore{15.34}{(10.69--20.47)}{4.55pt}{4.82pt}{} & \HoloSegScore{13.18}{(9.160--18.31)}{4.55pt}{4.82pt}{} & \HoloSegScore{12.21}{(9.160--18.21)}{4.55pt}{4.82pt}{} \\
\cline{2-11}
 &  &  & \HoloSegMetric{Dice} & \HoloSegScore{0.7440}{(0.7098--0.7685)}{4.55pt}{4.82pt}{} & \HoloSegScore{0.6559}{(0.6163--0.6970)}{4.55pt}{4.82pt}{} & \HoloSegScore{0.7263}{(0.6950--0.7503)}{4.55pt}{4.82pt}{} &  & \HoloSegScore{0.7758}{(0.7415--0.7901)}{4.55pt}{4.82pt}{} & \HoloSegScore{0.7791}{(0.7549--0.8024)}{4.55pt}{4.82pt}{} & \HoloSegScore{0.7859}{(0.7616--0.8090)}{4.55pt}{4.82pt}{} \\*
\softcline{4-7}\softcline{9-11}
 & \HoloSegSpan{\makecell[c]{Private02\\[-0.10ex](lung\\[-0.10ex]cancer)}}{1.86cm}{0.32cm} & \HoloSegSpan{\makecell[c]{lung cancer}}{2.04cm}{0.32cm} & \HoloSegMetric{HD95} & \HoloSegScore{35.99}{(28.97--42.18)}{4.55pt}{4.82pt}{} & \HoloSegScore{46.50}{(37.89--54.87)}{4.55pt}{4.82pt}{} & \HoloSegScore{37.46}{(29.60--43.27)}{4.55pt}{4.82pt}{} & \raisebox{0.32cm}[0pt][0pt]{\HoloSegUnsupported} & \HoloSegScore{31.70}{(25.94--37.91)}{4.55pt}{4.82pt}{} & \HoloSegScore{29.37}{(23.91--35.84)}{4.55pt}{4.82pt}{} & \HoloSegScore{31.94}{(25.44--38.08)}{4.55pt}{4.82pt}{} \\
\cline{2-11}
 &  &  & \HoloSegMetric{Dice} & \HoloSegScore{0.3231}{(0.2288--0.4239)}{4.55pt}{4.82pt}{} & \HoloSegScore{0.2269}{(0.1479--0.3112)}{4.55pt}{4.82pt}{} & \HoloSegScore{0.3020}{(0.2126--0.4095)}{4.55pt}{4.82pt}{} &  & \HoloSegScore{0.3546}{(0.2603--0.4668)}{4.55pt}{4.82pt}{} & \HoloSegScore{0.3746}{(0.2811--0.4902)}{4.55pt}{4.82pt}{} & \HoloSegScore{0.3809}{(0.2874--0.4967)}{4.55pt}{4.82pt}{} \\*
\softcline{4-7}\softcline{9-11}
\HoloSegSpan{\makecell[c]{\textbf{Private}\\[-0.10ex]\textbf{(fine-}\\[-0.10ex]\textbf{tuning)}}}{1.20cm}{0.32cm} &  & \HoloSegSpan{\makecell[c]{malignant\\[-0.10ex]thyroid\\[-0.10ex]tumor}}{2.04cm}{0.32cm} & \HoloSegMetric{HD95} & \HoloSegScore{25.84}{(18.55--32.77)}{4.55pt}{4.82pt}{} & \HoloSegScore{36.32}{(28.19--45.22)}{4.55pt}{4.82pt}{} & \HoloSegScore{28.41}{(20.72--35.03)}{4.55pt}{4.82pt}{} & \raisebox{0.32cm}[0pt][0pt]{\HoloSegUnsupported} & \HoloSegScore{23.26}{(16.42--29.92)}{4.55pt}{4.82pt}{} & \HoloSegScore{21.79}{(15.63--29.31)}{4.55pt}{4.82pt}{} & \HoloSegScore{20.84}{(14.81--27.19)}{4.55pt}{4.82pt}{} \\
\cline{3-11}
 & \HoloSegSpan{\makecell[c]{Private03\\[-0.10ex](thyroid\\[-0.10ex]cancer-\\[-0.10ex]multi)}}{1.86cm}{0.32cm} &  & \HoloSegMetric{Dice} & \HoloSegScore{0.7521}{(0.6819--0.8033)}{4.55pt}{4.82pt}{} & \HoloSegScore{0.6457}{(0.5895--0.7023)}{4.55pt}{4.82pt}{} & \HoloSegScore{0.7339}{(0.6792--0.7943)}{4.55pt}{4.82pt}{} &  & \HoloSegScore{0.7993}{(0.7345--0.8487)}{4.55pt}{4.82pt}{} & \HoloSegScore{0.7941}{(0.7368--0.8472)}{4.55pt}{4.82pt}{} & \HoloSegScore{0.8084}{(0.7512--0.8613)}{4.55pt}{4.82pt}{} \\*
\softcline{4-7}\softcline{9-11}
 &  & \HoloSegSpan{\makecell[c]{benign\\[-0.10ex]thyroid\\[-0.10ex]tumor}}{2.04cm}{0.32cm} & \HoloSegMetric{HD95} & \HoloSegScore{10.44}{(7.080--12.11)}{4.55pt}{4.82pt}{} & \HoloSegScore{16.46}{(12.73--20.72)}{4.55pt}{4.82pt}{} & \HoloSegScore{11.67}{(8.230--14.50)}{4.55pt}{4.82pt}{} & \raisebox{0.32cm}[0pt][0pt]{\HoloSegUnsupported} & \HoloSegScore{8.320}{(6.024--10.54)}{4.55pt}{4.82pt}{} & \HoloSegScore{8.388}{(6.424--9.930)}{4.55pt}{4.82pt}{} & \HoloSegScore{8.126}{(6.453--9.171)}{4.55pt}{4.82pt}{} \\
\cline{2-11}
 &  &  & \HoloSegMetric{Dice} & \HoloSegScore{0.7677}{(0.7141--0.8235)}{4.55pt}{4.82pt}{} & \HoloSegScore{0.6758}{(0.6222--0.7390)}{4.55pt}{4.82pt}{} & \HoloSegScore{0.7577}{(0.7057--0.8077)}{4.55pt}{4.82pt}{} &  & \HoloSegScore{0.8194}{(0.7592--0.8533)}{4.55pt}{4.82pt}{} & \HoloSegScore{0.8049}{(0.7604--0.8501)}{4.55pt}{4.82pt}{} & \HoloSegScore{0.8187}{(0.7742--0.8643)}{4.55pt}{4.82pt}{} \\*
\softcline{4-7}\softcline{9-11}
 & \HoloSegSpan{\makecell[c]{Private03\\[-0.10ex](thyroid\\[-0.10ex]cancer-\\[-0.10ex]one)}}{1.86cm}{0.32cm} & \HoloSegSpan{\makecell[c]{thyroid\\[-0.10ex]tumor}}{2.04cm}{0.32cm} & \HoloSegMetric{HD95} & \HoloSegScore{10.39}{(8.140--12.22)}{4.55pt}{4.82pt}{} & \HoloSegScore{15.46}{(11.14--19.96)}{4.55pt}{4.82pt}{} & \HoloSegScore{11.45}{(8.070--14.25)}{4.55pt}{4.82pt}{} & \raisebox{0.32cm}[0pt][0pt]{\HoloSegUnsupported} & \HoloSegScore{8.528}{(6.322--10.89)}{4.55pt}{4.82pt}{} & \HoloSegScore{8.370}{(6.395--9.747)}{4.55pt}{4.82pt}{} & \HoloSegScore{8.341}{(6.292--9.511)}{4.55pt}{4.82pt}{} \\
\hline
\end{longtable}
\arrayrulecolor{black}
\endgroup
