# Supplementary material for: A 3D foundation model unifying CT interpretation and segmentation
Source: arXiv:2611.06471 source file (2026-11-04)
Supplement: Supplementary file 10 [file table2_subtask2.tex]

\begingroup
\makeatletter
\@ifundefined{color@leftblue}{\definecolor{leftblue}{RGB}{232,242,248}}{}%
\@ifundefined{color@headerblue}{\definecolor{headerblue}{RGB}{218,233,242}}{}%
\makeatother
\setlength{\LTcapwidth}{18.60cm}
\setlength{\LTleft}{\fill}
\setlength{\LTright}{\fill}
\setlength{\LTpre}{0pt}
\setlength{\LTpost}{0pt}
\setlength{\tabcolsep}{0.45pt}
\renewcommand{\arraystretch}{1.00}
\setlength{\extrarowheight}{0pt}
\setlength{\arrayrulewidth}{0.48pt}
\arrayrulecolor{black}
\providecommand{\softcline}[1]{}%
\renewcommand{\softcline}[1]{\arrayrulecolor{black!35}\cline{#1}\arrayrulecolor{black}}
\sloppy
\emergencystretch=2em
\fontsize{5.30pt}{5.90pt}\selectfont
\newcommand{\HoloSegScore}[5]{%
  \parbox[c][0.64cm][c]{1.58cm}{%
    \centering
    {\fontsize{5.30pt}{5.58pt}\selectfont\strut\adjustbox{max width=\linewidth}{#1#5}}\\[-0.38ex]%
    {\fontsize{#3}{#4}\selectfont\strut\adjustbox{max width=\linewidth}{#2}}%
  }%
}%
\newcommand{\HoloSegUnsupported}{%
  \parbox[c][0.64cm][c]{1.58cm}{%
    \centering\fontsize{4.45pt}{4.70pt}\selectfont Not supported%
  }%
}%
\newcommand{\HoloSegMetric}[1]{%
  \parbox[c][0.64cm][c]{1.21cm}{%
    \centering\fontsize{5.45pt}{5.70pt}\selectfont\adjustbox{max width=\linewidth}{\textbf{#1}}%
  }%
}%
\newcommand{\HoloSegSpan}[3]{%
  \raisebox{#3}[0pt][0pt]{%
    \parbox[c]{#2}{\centering\arraybackslash\adjustbox{max width=#2}{#1}}%
  }%
}%
\newcommand{\HoloSegSplitHead}[3]{%
  \parbox[c][0.92cm][c]{#3}{%
    \centering\fontsize{6.20pt}{6.45pt}\selectfont\textbf{#1}\\[-0.52ex]%
    \rule{0pt}{0.58ex}\\[-0.52ex]\textbf{#2}%
  }%
}%
\newcommand{\HoloSegMidHead}[2]{%
  \parbox[c][0.92cm][c]{#2}{%
    \centering\fontsize{5.35pt}{5.65pt}\selectfont\adjustbox{max width=\linewidth}{\textbf{#1}}%
  }%
}%
\begin{longtable}{|>{\columncolor{leftblue}\centering\arraybackslash}m{1.35cm}|>{\columncolor{leftblue}\centering\arraybackslash}m{2.20cm}|>{\columncolor{leftblue}\centering\arraybackslash}m{2.30cm}|>{\columncolor{leftblue}\centering\arraybackslash}m{1.25cm}|>{\centering\arraybackslash}m{1.60cm}|>{\centering\arraybackslash}m{1.60cm}|>{\centering\arraybackslash}m{1.60cm}|>{\centering\arraybackslash}m{1.60cm}|>{\centering\arraybackslash}m{1.60cm}|>{\centering\arraybackslash}m{1.60cm}|>{\centering\arraybackslash}m{1.60cm}|}
\caption[Single-target grounded lesion screening]{\textbf{Detailed sensitivity, specificity, F1, and conditional Dice scores of HoloCT and competing methods on internal, external-seen zero-shot/fine-tuning, external-unseen zero-shot/fine-tuning, and private zero-shot/fine-tuning classification-segmentation benchmarks.}\newline Each score is reported as mean with 95\% confidence interval. Cond. Dice denotes conditional Dice. For the external zero-shot Macro F1 summary in Fig.~3c, unsupported ResNet and nnU-Net targets are scored as zero, so every model is averaged across the same nine targets.}%
\label{tab:classification_segmentation_scores}\\[-0.15ex]
\hline
\rowcolor{headerblue}
\HoloSegSplitHead{Dataset}{Type}{1.35cm} & \HoloSegSplitHead{Dataset}{Name}{2.20cm} & \HoloSegSplitHead{Label}{Name}{2.30cm} & \HoloSegMidHead{Metric}{1.25cm} & \HoloSegMidHead{M3D-Phi3-4B}{1.60cm} & \HoloSegMidHead{nnU-Net}{1.60cm} & \HoloSegMidHead{ResNet}{1.60cm} & \HoloSegMidHead{\makecell[c]{HoloCT-4B\\[-0.18ex]w/o\\[-0.18ex]grounding}}{1.60cm} & \HoloSegMidHead{\makecell[c]{HoloCT-4B\\[-0.18ex]w/\\[-0.18ex]grounding}}{1.60cm} & \HoloSegMidHead{\makecell[c]{HoloCT-8B\\[-0.18ex]w/o\\[-0.18ex]grounding}}{1.60cm} & \HoloSegMidHead{\makecell[c]{HoloCT-8B\\[-0.18ex]w/\\[-0.18ex]grounding}}{1.60cm} \\
\hline
\endfirsthead
\caption*{\textbf{Supplementary Table~\ref{tab:classification_segmentation_scores} (continued)\enspace|\enspace Detailed sensitivity, specificity, F1, and conditional Dice scores of HoloCT and competing methods on internal, external-seen zero-shot/fine-tuning, external-unseen zero-shot/fine-tuning, and private zero-shot/fine-tuning classification-segmentation benchmarks.}\newline Each score is reported as mean with 95\% confidence interval. Cond. Dice denotes conditional Dice. For the external zero-shot Macro F1 summary in Fig.~3c, unsupported ResNet and nnU-Net targets are scored as zero, so every model is averaged across the same nine targets.}\\[-0.15ex]
\hline
\rowcolor{headerblue}
\HoloSegSplitHead{Dataset}{Type}{1.35cm} & \HoloSegSplitHead{Dataset}{Name}{2.20cm} & \HoloSegSplitHead{Label}{Name}{2.30cm} & \HoloSegMidHead{Metric}{1.25cm} & \HoloSegMidHead{M3D-Phi3-4B}{1.60cm} & \HoloSegMidHead{nnU-Net}{1.60cm} & \HoloSegMidHead{ResNet}{1.60cm} & \HoloSegMidHead{\makecell[c]{HoloCT-4B\\[-0.18ex]w/o\\[-0.18ex]grounding}}{1.60cm} & \HoloSegMidHead{\makecell[c]{HoloCT-4B\\[-0.18ex]w/\\[-0.18ex]grounding}}{1.60cm} & \HoloSegMidHead{\makecell[c]{HoloCT-8B\\[-0.18ex]w/o\\[-0.18ex]grounding}}{1.60cm} & \HoloSegMidHead{\makecell[c]{HoloCT-8B\\[-0.18ex]w/\\[-0.18ex]grounding}}{1.60cm} \\
\hline
\endhead
\endfoot
\endlastfoot
 &  &  & \HoloSegMetric{Sens.} & \HoloSegScore{0.5000}{(0.0000--1.000)}{4.55pt}{4.82pt}{} & \HoloSegScore{1.000}{(1.000--1.000)}{4.55pt}{4.82pt}{} & \HoloSegScore{0.8333}{(0.5000--1.000)}{4.55pt}{4.82pt}{} & \HoloSegScore{0.6667}{(0.2500--1.000)}{4.55pt}{4.82pt}{} & \HoloSegScore{0.6667}{(0.2500--1.000)}{4.55pt}{4.82pt}{} & \HoloSegScore{1.000}{(1.000--1.000)}{4.55pt}{4.82pt}{} & \HoloSegScore{0.8333}{(0.4611--1.000)}{4.55pt}{4.82pt}{} \\*
\softcline{4-11}
 &  &  & \HoloSegMetric{Spec.} & \HoloSegScore{0.6529}{(0.5950--0.7137)}{4.55pt}{4.82pt}{} & \HoloSegScore{0.7810}{(0.7265--0.8340)}{4.55pt}{4.82pt}{} & \HoloSegScore{0.7769}{(0.7231--0.8306)}{4.55pt}{4.82pt}{} & \HoloSegScore{0.9752}{(0.9535--0.9918)}{4.55pt}{4.82pt}{} & \HoloSegScore{0.9669}{(0.9419--0.9876)}{4.55pt}{4.82pt}{} & \HoloSegScore{0.9711}{(0.9463--0.9877)}{4.55pt}{4.82pt}{} & \HoloSegScore{0.9752}{(0.9542--0.9918)}{4.55pt}{4.82pt}{} \\*
\softcline{4-11}
 &  & \HoloSegSpan{\makecell[c]{left kidney\\[-0.10ex]cyst}}{2.30cm}{0.32cm} & \HoloSegMetric{F1} & \HoloSegScore{0.06452}{(0.0000--0.1379)}{4.55pt}{4.82pt}{} & \HoloSegScore{0.1846}{(0.06667--0.3158)}{4.20pt}{4.48pt}{} & \HoloSegScore{0.1538}{(0.03704--0.2759)}{4.20pt}{4.48pt}{} & \HoloSegScore{0.5000}{(0.1536--0.7692)}{4.55pt}{4.82pt}{} & \HoloSegScore{0.4444}{(0.1248--0.7059)}{4.55pt}{4.82pt}{} & \HoloSegScore{0.6316}{(0.3071--0.8464)}{4.55pt}{4.82pt}{} & \HoloSegScore{0.5882}{(0.2500--0.8235)}{4.55pt}{4.82pt}{} \\*
\softcline{4-11}
 &  &  & \HoloSegMetric{Cond. Dice} & \HoloSegScore{0.03792}{(0.0000--0.07468)}{4.20pt}{4.48pt}{} & \HoloSegScore{0.7320}{(0.5424--0.8979)}{4.55pt}{4.82pt}{} & \HoloSegUnsupported & \HoloSegUnsupported & \HoloSegScore{0.9016}{(0.8845--0.9240)}{4.55pt}{4.82pt}{} & \HoloSegUnsupported & \HoloSegScore{0.8872}{(0.8380--0.9342)}{4.55pt}{4.82pt}{} \\
\cline{3-11}
 & \HoloSegSpan{\makecell[c]{Total-\\[-0.10ex]SegmentatorV2}}{2.20cm}{0.32cm} &  & \HoloSegMetric{Sens.} & \HoloSegScore{0.5000}{(0.0000--1.000)}{4.55pt}{4.82pt}{} & \HoloSegScore{0.5000}{(0.0000--1.000)}{4.55pt}{4.82pt}{} & \HoloSegScore{0.6667}{(0.2500--1.000)}{4.55pt}{4.82pt}{} & \HoloSegScore{0.5000}{(0.0000--1.000)}{4.55pt}{4.82pt}{} & \HoloSegScore{0.5000}{(0.0000--1.000)}{4.55pt}{4.82pt}{} & \HoloSegScore{0.3333}{(0.0000--0.7537)}{4.55pt}{4.82pt}{} & \HoloSegScore{0.5000}{(0.0000--1.000)}{4.55pt}{4.82pt}{} \\*
\softcline{4-11}
 &  &  & \HoloSegMetric{Spec.} & \HoloSegScore{0.7769}{(0.7231--0.8299)}{4.55pt}{4.82pt}{} & \HoloSegScore{0.8017}{(0.7520--0.8506)}{4.55pt}{4.82pt}{} & \HoloSegScore{0.8347}{(0.7860--0.8776)}{4.55pt}{4.82pt}{} & \HoloSegScore{0.9959}{(0.9874--1.000)}{4.55pt}{4.82pt}{} & \HoloSegScore{0.9917}{(0.9793--1.000)}{4.55pt}{4.82pt}{} & \HoloSegScore{0.9959}{(0.9874--1.000)}{4.55pt}{4.82pt}{} & \HoloSegScore{0.9917}{(0.9793--1.000)}{4.55pt}{4.82pt}{} \\*
\softcline{4-11}
 &  & \HoloSegSpan{\makecell[c]{right kidney\\[-0.10ex]cyst}}{2.30cm}{0.32cm} & \HoloSegMetric{F1} & \HoloSegScore{0.09524}{(0.0000--0.1967)}{4.55pt}{4.82pt}{} & \HoloSegScore{0.1053}{(0.0000--0.2105)}{4.55pt}{4.82pt}{} & \HoloSegScore{0.1600}{(0.03844--0.2963)}{4.20pt}{4.48pt}{} & \HoloSegScore{0.6000}{(0.0000--0.9098)}{4.55pt}{4.82pt}{} & \HoloSegScore{0.5455}{(0.0000--0.8750)}{4.55pt}{4.82pt}{} & \HoloSegScore{0.4444}{(0.0000--0.8240)}{4.55pt}{4.82pt}{} & \HoloSegScore{0.5455}{(0.0000--0.8750)}{4.55pt}{4.82pt}{} \\*
\softcline{4-11}
 &  &  & \HoloSegMetric{Cond. Dice} & \HoloSegScore{0.2163}{(0.0000--0.6490)}{4.55pt}{4.82pt}{} & \HoloSegScore{0.6539}{(0.5931--0.7558)}{4.55pt}{4.82pt}{} & \HoloSegUnsupported & \HoloSegUnsupported & \HoloSegScore{0.8536}{(0.7821--0.9343)}{4.55pt}{4.82pt}{} & \HoloSegUnsupported & \HoloSegScore{0.8563}{(0.7787--0.9328)}{4.55pt}{4.82pt}{} \\
\cline{2-11}
 &  &  & \HoloSegMetric{Sens.} & \HoloSegScore{0.0000}{(0.0000--0.0000)}{4.55pt}{4.82pt}{} & \HoloSegScore{0.8909}{(0.8043--0.9643)}{4.55pt}{4.82pt}{} & \HoloSegScore{0.6727}{(0.5500--0.7917)}{4.55pt}{4.82pt}{} & \HoloSegScore{0.5636}{(0.4259--0.6897)}{4.55pt}{4.82pt}{} & \HoloSegScore{0.6545}{(0.5245--0.7778)}{4.55pt}{4.82pt}{} & \HoloSegScore{0.6909}{(0.5660--0.8085)}{4.55pt}{4.82pt}{} & \HoloSegScore{0.6909}{(0.5671--0.8077)}{4.55pt}{4.82pt}{} \\*
\softcline{4-11}
 &  &  & \HoloSegMetric{Spec.} & \HoloSegScore{1.000}{(1.000--1.000)}{4.55pt}{4.82pt}{} & \HoloSegScore{0.0000}{(0.0000--0.0000)}{4.55pt}{4.82pt}{} & \HoloSegScore{0.4884}{(0.3333--0.6410)}{4.55pt}{4.82pt}{} & \HoloSegScore{0.9535}{(0.8837--1.000)}{4.55pt}{4.82pt}{} & \HoloSegScore{0.9070}{(0.8181--0.9778)}{4.55pt}{4.82pt}{} & \HoloSegScore{0.8372}{(0.7273--0.9459)}{4.55pt}{4.82pt}{} & \HoloSegScore{0.8605}{(0.7561--0.9545)}{4.55pt}{4.82pt}{} \\*
\softcline{4-11}
 & \HoloSegSpan{\makecell[c]{KiTS23}}{2.20cm}{0.32cm} & \HoloSegSpan{\makecell[c]{kidney cyst}}{2.30cm}{0.32cm} & \HoloSegMetric{F1} & \HoloSegScore{0.0000}{(0.0000--0.0000)}{4.55pt}{4.82pt}{} & \HoloSegScore{0.6667}{(0.5693--0.7516)}{4.55pt}{4.82pt}{} & \HoloSegScore{0.6491}{(0.5361--0.7458)}{4.55pt}{4.82pt}{} & \HoloSegScore{0.7045}{(0.5823--0.8036)}{4.55pt}{4.82pt}{} & \HoloSegScore{0.7579}{(0.6506--0.8462)}{4.55pt}{4.82pt}{} & \HoloSegScore{0.7600}{(0.6591--0.8462)}{4.55pt}{4.82pt}{} & \HoloSegScore{0.7677}{(0.6667--0.8519)}{4.55pt}{4.82pt}{} \\*
\softcline{4-11}
 &  &  & \HoloSegMetric{Cond. Dice} & \HoloSegScore{-}{}{4.55pt}{4.82pt}{} & \HoloSegScore{0.2649}{(0.1930--0.3366)}{4.55pt}{4.82pt}{} & \HoloSegUnsupported & \HoloSegUnsupported & \HoloSegScore{0.5781}{(0.4930--0.6636)}{4.55pt}{4.82pt}{} & \HoloSegUnsupported & \HoloSegScore{0.7046}{(0.6268--0.7816)}{4.55pt}{4.82pt}{} \\
\cline{2-11}
 &  &  & \HoloSegMetric{Sens.} & \HoloSegScore{1.000}{(1.000--1.000)}{4.55pt}{4.82pt}{} & \HoloSegScore{1.000}{(1.000--1.000)}{4.55pt}{4.82pt}{} & \HoloSegScore{1.000}{(1.000--1.000)}{4.55pt}{4.82pt}{} & \HoloSegScore{0.2857}{(0.0000--0.6667)}{4.55pt}{4.82pt}{} & \HoloSegScore{0.4286}{(0.0000--0.8333)}{4.55pt}{4.82pt}{} & \HoloSegScore{0.4286}{(0.0000--0.8333)}{4.55pt}{4.82pt}{} & \HoloSegScore{0.4286}{(0.0000--0.8333)}{4.55pt}{4.82pt}{} \\*
\softcline{4-11}
 &  &  & \HoloSegMetric{Spec.} & \HoloSegScore{0.1250}{(0.0000--0.4000)}{4.55pt}{4.82pt}{} & \HoloSegScore{0.8750}{(0.5714--1.000)}{4.55pt}{4.82pt}{} & \HoloSegScore{0.5000}{(0.1424--0.8571)}{4.55pt}{4.82pt}{} & \HoloSegScore{0.7500}{(0.4286--1.000)}{4.55pt}{4.82pt}{} & \HoloSegScore{0.7500}{(0.4000--1.000)}{4.55pt}{4.82pt}{} & \HoloSegScore{0.7500}{(0.4000--1.000)}{4.55pt}{4.82pt}{} & \HoloSegScore{0.7500}{(0.4000--1.000)}{4.55pt}{4.82pt}{} \\*
\softcline{4-11}
 & \HoloSegSpan{\makecell[c]{CT-ICH}}{2.20cm}{0.32cm} & \HoloSegSpan{\makecell[c]{intracranial\\[-0.10ex]hemorrhage}}{2.30cm}{0.32cm} & \HoloSegMetric{F1} & \HoloSegScore{0.6667}{(0.3529--0.8696)}{4.55pt}{4.82pt}{} & \HoloSegScore{0.9333}{(0.7273--1.000)}{4.55pt}{4.82pt}{} & \HoloSegScore{0.7778}{(0.5000--0.9524)}{4.55pt}{4.82pt}{} & \HoloSegScore{0.3636}{(0.0000--0.7143)}{4.55pt}{4.82pt}{} & \HoloSegScore{0.5000}{(0.0000--0.8000)}{4.55pt}{4.82pt}{} & \HoloSegScore{0.5000}{(0.0000--0.8000)}{4.55pt}{4.82pt}{} & \HoloSegScore{0.5000}{(0.0000--0.8000)}{4.55pt}{4.82pt}{} \\*
\softcline{4-11}
 &  &  & \HoloSegMetric{Cond. Dice} & \HoloSegScore{0.0000}{(0.0000--0.0000)}{4.55pt}{4.82pt}{} & \HoloSegScore{0.8793}{(0.7911--0.9419)}{4.55pt}{4.82pt}{} & \HoloSegUnsupported & \HoloSegUnsupported & \HoloSegScore{0.5557}{(0.5180--0.6021)}{4.55pt}{4.82pt}{} & \HoloSegUnsupported & \HoloSegScore{0.6853}{(0.5247--0.8460)}{4.55pt}{4.82pt}{} \\
\cline{2-11}
 &  &  & \HoloSegMetric{Sens.} & \HoloSegScore{0.5894}{(0.5102--0.6690)}{4.55pt}{4.82pt}{} & \HoloSegScore{0.4636}{(0.3831--0.5411)}{4.55pt}{4.82pt}{} & \HoloSegScore{0.5232}{(0.4429--0.6015)}{4.55pt}{4.82pt}{} & \HoloSegScore{0.3046}{(0.2313--0.3784)}{4.55pt}{4.82pt}{} & \HoloSegScore{0.3974}{(0.3200--0.4694)}{4.55pt}{4.82pt}{} & \HoloSegScore{0.4305}{(0.3551--0.5172)}{4.55pt}{4.82pt}{} & \HoloSegScore{0.4834}{(0.4057--0.5690)}{4.55pt}{4.82pt}{} \\*
\softcline{4-11}
 &  &  & \HoloSegMetric{Spec.} & \HoloSegScore{0.3320}{(0.2972--0.3644)}{4.55pt}{4.82pt}{} & \HoloSegScore{0.8867}{(0.8623--0.9073)}{4.55pt}{4.82pt}{} & \HoloSegScore{0.9107}{(0.8899--0.9302)}{4.55pt}{4.82pt}{} & \HoloSegScore{0.9960}{(0.9908--1.000)}{4.55pt}{4.82pt}{} & \HoloSegScore{0.9907}{(0.9827--0.9973)}{4.55pt}{4.82pt}{} & \HoloSegScore{0.9787}{(0.9674--0.9879)}{4.55pt}{4.82pt}{} & \HoloSegScore{0.9760}{(0.9647--0.9863)}{4.55pt}{4.82pt}{} \\*
\softcline{4-11}
\HoloSegSpan{\makecell[c]{\textbf{Internal}}}{1.35cm}{0.32cm} & \HoloSegSpan{\makecell[c]{PanTS}}{2.20cm}{0.32cm} & \HoloSegSpan{\makecell[c]{pancreas\\[-0.10ex]lesion}}{2.30cm}{0.32cm} & \HoloSegMetric{F1} & \HoloSegScore{0.2402}{(0.1983--0.2804)}{4.55pt}{4.82pt}{} & \HoloSegScore{0.4575}{(0.3852--0.5228)}{4.55pt}{4.82pt}{} & \HoloSegScore{0.5320}{(0.4590--0.5970)}{4.55pt}{4.82pt}{} & \HoloSegScore{0.4600}{(0.3696--0.5405)}{4.55pt}{4.82pt}{} & \HoloSegScore{0.5505}{(0.4660--0.6224)}{4.55pt}{4.82pt}{} & \HoloSegScore{0.5603}{(0.4830--0.6360)}{4.55pt}{4.82pt}{} & \HoloSegScore{0.6033}{(0.5315--0.6767)}{4.55pt}{4.82pt}{} \\*
\softcline{4-11}
 &  &  & \HoloSegMetric{Cond. Dice} & \HoloSegScore{0.2034}{(0.1575--0.2502)}{4.55pt}{4.82pt}{} & \HoloSegScore{0.3146}{(0.2930--0.3796)}{4.55pt}{4.82pt}{} & \HoloSegUnsupported & \HoloSegUnsupported & \HoloSegScore{0.4920}{(0.4242--0.5574)}{4.55pt}{4.82pt}{} & \HoloSegUnsupported & \HoloSegScore{0.5412}{(0.4820--0.6016)}{4.55pt}{4.82pt}{} \\
\cline{2-11}
 &  &  & \HoloSegMetric{Sens.} & \HoloSegScore{0.7290}{(0.6779--0.7807)}{4.55pt}{4.82pt}{} & \HoloSegScore{0.7214}{(0.6641--0.7744)}{4.55pt}{4.82pt}{} & \HoloSegScore{0.8588}{(0.8162--0.9011)}{4.55pt}{4.82pt}{} & \HoloSegScore{0.3702}{(0.3113--0.4286)}{4.55pt}{4.82pt}{} & \HoloSegScore{0.5153}{(0.4527--0.5772)}{4.55pt}{4.82pt}{} & \HoloSegScore{0.2939}{(0.2422--0.3494)}{4.55pt}{4.82pt}{} & \HoloSegScore{0.3740}{(0.3162--0.4317)}{4.55pt}{4.82pt}{} \\*
\softcline{4-11}
 &  &  & \HoloSegMetric{Spec.} & \HoloSegScore{0.2319}{(0.1997--0.2633)}{4.55pt}{4.82pt}{} & \HoloSegScore{0.09337}{(0.07217--0.1162)}{4.20pt}{4.48pt}{} & \HoloSegScore{0.6717}{(0.6344--0.7067)}{4.55pt}{4.82pt}{} & \HoloSegScore{0.9714}{(0.9587--0.9826)}{4.55pt}{4.82pt}{} & \HoloSegScore{0.9458}{(0.9286--0.9629)}{4.55pt}{4.82pt}{} & \HoloSegScore{0.9940}{(0.9867--0.9985)}{4.55pt}{4.82pt}{} & \HoloSegScore{0.9804}{(0.9691--0.9898)}{4.55pt}{4.82pt}{} \\*
\softcline{4-11}
 &  & \HoloSegSpan{\makecell[c]{kidney\\[-0.10ex]lesion}}{2.30cm}{0.32cm} & \HoloSegMetric{F1} & \HoloSegScore{0.3967}{(0.3563--0.4353)}{4.55pt}{4.82pt}{} & \HoloSegScore{0.3590}{(0.3224--0.3944)}{4.55pt}{4.82pt}{} & \HoloSegScore{0.6383}{(0.5975--0.6771)}{4.55pt}{4.82pt}{} & \HoloSegScore{0.5132}{(0.4485--0.5714)}{4.55pt}{4.82pt}{} & \HoloSegScore{0.6236}{(0.5670--0.6742)}{4.55pt}{4.82pt}{} & \HoloSegScore{0.4490}{(0.3834--0.5121)}{4.55pt}{4.82pt}{} & \HoloSegScore{0.5255}{(0.4615--0.5829)}{4.55pt}{4.82pt}{} \\*
\softcline{4-11}
 &  &  & \HoloSegMetric{Cond. Dice} & \HoloSegScore{0.2381}{(0.1936--0.2842)}{4.55pt}{4.82pt}{} & \HoloSegScore{0.7081}{(0.6614--0.7303)}{4.55pt}{4.82pt}{} & \HoloSegUnsupported & \HoloSegUnsupported & \HoloSegScore{0.7344}{(0.6924--0.7729)}{4.55pt}{4.82pt}{} & \HoloSegUnsupported & \HoloSegScore{0.8221}{(0.7941--0.8475)}{4.55pt}{4.82pt}{} \\
\cline{3-11}
 &  &  & \HoloSegMetric{Sens.} & \HoloSegScore{0.9776}{(0.9563--0.9954)}{4.55pt}{4.82pt}{} & \HoloSegScore{0.9058}{(0.8643--0.9420)}{4.55pt}{4.82pt}{} & \HoloSegScore{0.4529}{(0.3883--0.5156)}{4.55pt}{4.82pt}{} & \HoloSegScore{0.6502}{(0.5855--0.7129)}{4.55pt}{4.82pt}{} & \HoloSegScore{0.7668}{(0.7110--0.8217)}{4.55pt}{4.82pt}{} & \HoloSegScore{0.8027}{(0.7489--0.8543)}{4.55pt}{4.82pt}{} & \HoloSegScore{0.7130}{(0.6529--0.7718)}{4.55pt}{4.82pt}{} \\*
\softcline{4-11}
 &  &  & \HoloSegMetric{Spec.} & \HoloSegScore{0.03698}{(0.02446--0.05234)}{4.20pt}{4.48pt}{} & \HoloSegScore{0.0000}{(0.0000--0.0000)}{4.55pt}{4.82pt}{} & \HoloSegScore{0.8009}{(0.7717--0.8280)}{4.55pt}{4.82pt}{} & \HoloSegScore{0.9602}{(0.9459--0.9739)}{4.55pt}{4.82pt}{} & \HoloSegScore{0.9388}{(0.9207--0.9558)}{4.55pt}{4.82pt}{} & \HoloSegScore{0.8947}{(0.8712--0.9177)}{4.55pt}{4.82pt}{} & \HoloSegScore{0.9388}{(0.9214--0.9563)}{4.55pt}{4.82pt}{} \\*
\softcline{4-11}
 &  & \HoloSegSpan{\makecell[c]{liver lesion}}{2.30cm}{0.32cm} & \HoloSegMetric{F1} & \HoloSegScore{0.3900}{(0.3539--0.4271)}{4.55pt}{4.82pt}{} & \HoloSegScore{0.3582}{(0.3225--0.3924)}{4.55pt}{4.82pt}{} & \HoloSegScore{0.4353}{(0.3795--0.4907)}{4.55pt}{4.82pt}{} & \HoloSegScore{0.7323}{(0.6808--0.7775)}{4.55pt}{4.82pt}{} & \HoloSegScore{0.7826}{(0.7387--0.8227)}{4.55pt}{4.82pt}{} & \HoloSegScore{0.7521}{(0.7072--0.7936)}{4.55pt}{4.82pt}{} & \HoloSegScore{0.7482}{(0.7005--0.7933)}{4.55pt}{4.82pt}{} \\*
\softcline{4-11}
 &  &  & \HoloSegMetric{Cond. Dice} & \HoloSegScore{0.1827}{(0.1332--0.2372)}{4.55pt}{4.82pt}{} & \HoloSegScore{0.6494}{(0.5935--0.6831)}{4.55pt}{4.82pt}{} & \HoloSegUnsupported & \HoloSegUnsupported & \HoloSegScore{0.7248}{(0.6988--0.7506)}{4.55pt}{4.82pt}{} & \HoloSegUnsupported & \HoloSegScore{0.7102}{(0.6796--0.7402)}{4.55pt}{4.82pt}{} \\
\cline{3-11}
 & \HoloSegSpan{\makecell[c]{AbdomenAtlas\\[-0.10ex]3.0}}{2.20cm}{0.32cm} &  & \HoloSegMetric{Sens.} & \HoloSegScore{0.6277}{(0.5500--0.7045)}{4.55pt}{4.82pt}{} & \HoloSegScore{0.6204}{(0.5378--0.7035)}{4.55pt}{4.82pt}{} & \HoloSegScore{0.4818}{(0.3968--0.5630)}{4.55pt}{4.82pt}{} & \HoloSegScore{0.4745}{(0.3931--0.5573)}{4.55pt}{4.82pt}{} & \HoloSegScore{0.5693}{(0.4857--0.6462)}{4.55pt}{4.82pt}{} & \HoloSegScore{0.6277}{(0.5454--0.7054)}{4.55pt}{4.82pt}{} & \HoloSegScore{0.6131}{(0.5349--0.6957)}{4.55pt}{4.82pt}{} \\*
\softcline{4-11}
 &  &  & \HoloSegMetric{Spec.} & \HoloSegScore{0.4385}{(0.4038--0.4736)}{4.55pt}{4.82pt}{} & \HoloSegScore{0.3118}{(0.2809--0.3442)}{4.55pt}{4.82pt}{} & \HoloSegScore{0.7275}{(0.6975--0.7584)}{4.55pt}{4.82pt}{} & \HoloSegScore{0.9886}{(0.9806--0.9950)}{4.55pt}{4.82pt}{} & \HoloSegScore{0.9797}{(0.9698--0.9887)}{4.55pt}{4.82pt}{} & \HoloSegScore{0.9341}{(0.9160--0.9499)}{4.55pt}{4.82pt}{} & \HoloSegScore{0.9569}{(0.9427--0.9706)}{4.55pt}{4.82pt}{} \\*
\softcline{4-11}
 &  & \HoloSegSpan{\makecell[c]{pancreas\\[-0.10ex]lesion}}{2.30cm}{0.32cm} & \HoloSegMetric{F1} & \HoloSegScore{0.2583}{(0.2140--0.3022)}{4.55pt}{4.82pt}{} & \HoloSegScore{0.2222}{(0.1820--0.2627)}{4.55pt}{4.82pt}{} & \HoloSegScore{0.3158}{(0.2571--0.3723)}{4.55pt}{4.82pt}{} & \HoloSegScore{0.6161}{(0.5384--0.6854)}{4.55pt}{4.82pt}{} & \HoloSegScore{0.6753}{(0.6021--0.7369)}{4.55pt}{4.82pt}{} & \HoloSegScore{0.6255}{(0.5574--0.6869)}{4.55pt}{4.82pt}{} & \HoloSegScore{0.6588}{(0.5892--0.7207)}{4.55pt}{4.82pt}{} \\*
\softcline{4-11}
 &  &  & \HoloSegMetric{Cond. Dice} & \HoloSegScore{0.1387}{(0.09945--0.1816)}{4.20pt}{4.48pt}{} & \HoloSegScore{0.4728}{(0.4217--0.5494)}{4.55pt}{4.82pt}{} & \HoloSegUnsupported & \HoloSegUnsupported & \HoloSegScore{0.5480}{(0.4906--0.6055)}{4.55pt}{4.82pt}{} & \HoloSegUnsupported & \HoloSegScore{0.5712}{(0.5176--0.6266)}{4.55pt}{4.82pt}{} \\
\cline{3-11}
 &  &  & \HoloSegMetric{Sens.} & \HoloSegScore{1.000}{(1.000--1.000)}{4.55pt}{4.82pt}{} & \HoloSegScore{1.000}{(1.000--1.000)}{4.55pt}{4.82pt}{} & \HoloSegScore{0.8000}{(0.6250--0.9545)}{4.55pt}{4.82pt}{} & \HoloSegScore{0.8800}{(0.7391--1.000)}{4.55pt}{4.82pt}{} & \HoloSegScore{0.9200}{(0.7931--1.000)}{4.55pt}{4.82pt}{} & \HoloSegScore{0.5600}{(0.3529--0.7587)}{4.55pt}{4.82pt}{} & \HoloSegScore{0.7200}{(0.5332--0.8889)}{4.55pt}{4.82pt}{} \\*
\softcline{4-11}
 &  &  & \HoloSegMetric{Spec.} & \HoloSegScore{0.05771}{(0.04319--0.07325)}{4.20pt}{4.48pt}{} & \HoloSegScore{0.02775}{(0.01774--0.03859)}{4.20pt}{4.48pt}{} & \HoloSegScore{0.03219}{(0.02111--0.04373)}{4.20pt}{4.48pt}{} & \HoloSegScore{0.9589}{(0.9457--0.9711)}{4.55pt}{4.82pt}{} & \HoloSegScore{0.9345}{(0.9183--0.9501)}{4.55pt}{4.82pt}{} & \HoloSegScore{0.9922}{(0.9865--0.9978)}{4.55pt}{4.82pt}{} & \HoloSegScore{0.9834}{(0.9735--0.9911)}{4.55pt}{4.82pt}{} \\*
\softcline{4-11}
 &  & \HoloSegSpan{\makecell[c]{colon lesion}}{2.30cm}{0.32cm} & \HoloSegMetric{F1} & \HoloSegScore{0.05562}{(0.03778--0.07827)}{4.20pt}{4.48pt}{} & \HoloSegScore{0.05400}{(0.03486--0.07463)}{4.20pt}{4.48pt}{} & \HoloSegScore{0.04362}{(0.02623--0.06243)}{4.20pt}{4.48pt}{} & \HoloSegScore{0.5238}{(0.3846--0.6429)}{4.55pt}{4.82pt}{} & \HoloSegScore{0.4299}{(0.3010--0.5391)}{4.55pt}{4.82pt}{} & \HoloSegScore{0.6087}{(0.4241--0.7619)}{4.55pt}{4.82pt}{} & \HoloSegScore{0.6207}{(0.4641--0.7568)}{4.55pt}{4.82pt}{} \\*
\softcline{4-11}
 &  &  & \HoloSegMetric{Cond. Dice} & \HoloSegScore{0.05536}{(0.001067--0.1158)}{4.20pt}{4.48pt}{} & \HoloSegScore{0.6813}{(0.5886--0.8194)}{4.55pt}{4.82pt}{} & \HoloSegUnsupported & \HoloSegUnsupported & \HoloSegScore{0.6678}{(0.5685--0.7530)}{4.55pt}{4.82pt}{} & \HoloSegUnsupported & \HoloSegScore{0.7231}{(0.6598--0.7816)}{4.55pt}{4.82pt}{} \\
\hline
\pagebreak[4]
 &  &  & \HoloSegMetric{Sens.} & \HoloSegScore{0.0000}{(0.0000--0.0000)}{4.55pt}{4.82pt}{} & \HoloSegScore{0.8000}{(0.5000--1.000)}{4.55pt}{4.82pt}{} & \HoloSegScore{0.0000}{(0.0000--0.0000)}{4.55pt}{4.82pt}{} & \HoloSegScore{0.6000}{(0.2854--0.8892)}{4.55pt}{4.82pt}{} & \HoloSegScore{0.6000}{(0.2857--0.9000)}{4.55pt}{4.82pt}{} & \HoloSegScore{0.7000}{(0.3747--1.000)}{4.55pt}{4.82pt}{} & \HoloSegScore{0.7000}{(0.3747--1.000)}{4.55pt}{4.82pt}{} \\*
\softcline{4-11}
 &  &  & \HoloSegMetric{Spec.} & \HoloSegScore{1.000}{(1.000--1.000)}{4.55pt}{4.82pt}{} & \HoloSegScore{0.7000}{(0.5000--0.9000)}{4.55pt}{4.82pt}{} & \HoloSegScore{0.9500}{(0.8333--1.000)}{4.55pt}{4.82pt}{} & \HoloSegScore{0.9500}{(0.8333--1.000)}{4.55pt}{4.82pt}{} & \HoloSegScore{0.9000}{(0.7500--1.000)}{4.55pt}{4.82pt}{} & \HoloSegScore{0.9000}{(0.7500--1.000)}{4.55pt}{4.82pt}{} & \HoloSegScore{0.9000}{(0.7500--1.000)}{4.55pt}{4.82pt}{} \\*
\softcline{4-11}
 &  & \HoloSegSpan{\makecell[c]{liver cyst}}{2.30cm}{0.32cm} & \HoloSegMetric{F1} & \HoloSegScore{0.0000}{(0.0000--0.0000)}{4.55pt}{4.82pt}{} & \HoloSegScore{0.6667}{(0.4000--0.8667)}{4.55pt}{4.82pt}{} & \HoloSegScore{0.0000}{(0.0000--0.0000)}{4.55pt}{4.82pt}{} & \HoloSegScore{0.7059}{(0.4000--0.9167)}{4.55pt}{4.82pt}{} & \HoloSegScore{0.6667}{(0.3636--0.8750)}{4.55pt}{4.82pt}{} & \HoloSegScore{0.7368}{(0.4444--0.9231)}{4.55pt}{4.82pt}{} & \HoloSegScore{0.7368}{(0.4444--0.9231)}{4.55pt}{4.82pt}{} \\*
\softcline{4-11}
 &  &  & \HoloSegMetric{Cond. Dice} & \HoloSegScore{-}{}{4.55pt}{4.82pt}{} & \HoloSegScore{0.6562}{(0.5824--0.7276)}{4.55pt}{4.82pt}{} & \HoloSegUnsupported & \HoloSegUnsupported & \HoloSegScore{0.6003}{(0.4689--0.7237)}{4.55pt}{4.82pt}{} & \HoloSegUnsupported & \HoloSegScore{0.6448}{(0.5193--0.7476)}{4.55pt}{4.82pt}{} \\
\cline{3-11}
 &  &  & \HoloSegMetric{Sens.} & \HoloSegScore{0.0000}{(0.0000--0.0000)}{4.55pt}{4.82pt}{} & \HoloSegScore{0.8333}{(0.5000--1.000)}{4.55pt}{4.82pt}{} & \HoloSegScore{0.6667}{(0.2000--1.000)}{4.55pt}{4.82pt}{} & \HoloSegScore{0.6667}{(0.2500--1.000)}{4.55pt}{4.82pt}{} & \HoloSegScore{0.6667}{(0.2500--1.000)}{4.55pt}{4.82pt}{} & \HoloSegScore{1.000}{(1.000--1.000)}{4.55pt}{4.82pt}{} & \HoloSegScore{1.000}{(1.000--1.000)}{4.55pt}{4.82pt}{} \\*
\softcline{4-11}
 &  &  & \HoloSegMetric{Spec.} & \HoloSegScore{1.000}{(1.000--1.000)}{4.55pt}{4.82pt}{} & \HoloSegScore{0.7917}{(0.6190--0.9524)}{4.55pt}{4.82pt}{} & \HoloSegScore{0.7500}{(0.5652--0.9200)}{4.55pt}{4.82pt}{} & \HoloSegScore{1.000}{(1.000--1.000)}{4.55pt}{4.82pt}{} & \HoloSegScore{1.000}{(1.000--1.000)}{4.55pt}{4.82pt}{} & \HoloSegScore{0.8750}{(0.7199--1.000)}{4.55pt}{4.82pt}{} & \HoloSegScore{0.8750}{(0.7199--1.000)}{4.55pt}{4.82pt}{} \\*
\softcline{4-11}
 &  & \HoloSegSpan{\makecell[c]{liver\\[-0.10ex]hemangioma}}{2.30cm}{0.32cm} & \HoloSegMetric{F1} & \HoloSegScore{0.0000}{(0.0000--0.0000)}{4.55pt}{4.82pt}{} & \HoloSegScore{0.6250}{(0.2500--0.8462)}{4.55pt}{4.82pt}{} & \HoloSegScore{0.5000}{(0.1429--0.7619)}{4.55pt}{4.82pt}{} & \HoloSegScore{0.8000}{(0.4000--1.000)}{4.55pt}{4.82pt}{} & \HoloSegScore{0.8000}{(0.4000--1.000)}{4.55pt}{4.82pt}{} & \HoloSegScore{0.8000}{(0.5000--1.000)}{4.55pt}{4.82pt}{} & \HoloSegScore{0.8000}{(0.5000--1.000)}{4.55pt}{4.82pt}{} \\*
\softcline{4-11}
 &  &  & \HoloSegMetric{Cond. Dice} & \HoloSegScore{-}{}{4.55pt}{4.82pt}{} & \HoloSegScore{0.6200}{(0.2938--0.8864)}{4.55pt}{4.82pt}{} & \HoloSegUnsupported & \HoloSegUnsupported & \HoloSegScore{0.8313}{(0.7636--0.8765)}{4.55pt}{4.82pt}{} & \HoloSegUnsupported & \HoloSegScore{0.7106}{(0.4914--0.8313)}{4.55pt}{4.82pt}{} \\
\cline{3-11}
 & \HoloSegSpan{\makecell[c]{LiMT}}{2.20cm}{0.32cm} &  & \HoloSegMetric{Sens.} & \HoloSegScore{0.0000}{(0.0000--0.0000)}{4.55pt}{4.82pt}{} & \HoloSegScore{0.7500}{(0.0000--1.000)}{4.55pt}{4.82pt}{} & \HoloSegScore{0.5000}{(0.0000--1.000)}{4.55pt}{4.82pt}{} & \HoloSegScore{0.2500}{(0.0000--0.7625)}{4.55pt}{4.82pt}{} & \HoloSegScore{0.2500}{(0.0000--0.7625)}{4.55pt}{4.82pt}{} & \HoloSegScore{0.2500}{(0.0000--1.000)}{4.55pt}{4.82pt}{} & \HoloSegScore{0.2500}{(0.0000--1.000)}{4.55pt}{4.82pt}{} \\*
\softcline{4-11}
 &  &  & \HoloSegMetric{Spec.} & \HoloSegScore{1.000}{(1.000--1.000)}{4.55pt}{4.82pt}{} & \HoloSegScore{0.7692}{(0.5998--0.9231)}{4.55pt}{4.82pt}{} & \HoloSegScore{0.7308}{(0.5600--0.8846)}{4.55pt}{4.82pt}{} & \HoloSegScore{1.000}{(1.000--1.000)}{4.55pt}{4.82pt}{} & \HoloSegScore{1.000}{(1.000--1.000)}{4.55pt}{4.82pt}{} & \HoloSegScore{0.9615}{(0.8696--1.000)}{4.55pt}{4.82pt}{} & \HoloSegScore{0.9615}{(0.8696--1.000)}{4.55pt}{4.82pt}{} \\*
\softcline{4-11}
\HoloSegSpan{\makecell[c]{\textbf{Internal}}}{1.35cm}{0.32cm} &  & \HoloSegSpan{\makecell[c]{metastatic\\[-0.10ex]liver cancer}}{2.30cm}{0.32cm} & \HoloSegMetric{F1} & \HoloSegScore{0.0000}{(0.0000--0.0000)}{4.55pt}{4.82pt}{} & \HoloSegScore{0.4615}{(0.0000--0.7505)}{4.55pt}{4.82pt}{} & \HoloSegScore{0.3077}{(0.0000--0.6250)}{4.55pt}{4.82pt}{} & \HoloSegScore{0.4000}{(0.0000--0.8651)}{4.55pt}{4.82pt}{} & \HoloSegScore{0.4000}{(0.0000--0.8651)}{4.55pt}{4.82pt}{} & \HoloSegScore{0.3333}{(0.0000--0.8000)}{4.55pt}{4.82pt}{} & \HoloSegScore{0.3333}{(0.0000--0.8000)}{4.55pt}{4.82pt}{} \\*
\softcline{4-11}
 &  &  & \HoloSegMetric{Cond. Dice} & \HoloSegScore{-}{}{4.55pt}{4.82pt}{} & \HoloSegScore{0.4623}{(0.2354--0.6347)}{4.55pt}{4.82pt}{} & \HoloSegUnsupported & \HoloSegUnsupported & \HoloSegScore{0.6313}{(0.6313--0.6313)}{4.55pt}{4.82pt}{} & \HoloSegUnsupported & \HoloSegScore{0.6605}{(0.6605--0.6605)}{4.55pt}{4.82pt}{} \\
\cline{3-11}
 &  &  & \HoloSegMetric{Sens.} & \HoloSegScore{0.0000}{(0.0000--0.0000)}{4.55pt}{4.82pt}{} & \HoloSegScore{0.8571}{(0.5000--1.000)}{4.55pt}{4.82pt}{} & \HoloSegScore{0.8571}{(0.5000--1.000)}{4.55pt}{4.82pt}{} & \HoloSegScore{1.000}{(1.000--1.000)}{4.55pt}{4.82pt}{} & \HoloSegScore{1.000}{(1.000--1.000)}{4.55pt}{4.82pt}{} & \HoloSegScore{1.000}{(1.000--1.000)}{4.55pt}{4.82pt}{} & \HoloSegScore{1.000}{(1.000--1.000)}{4.55pt}{4.82pt}{} \\*
\softcline{4-11}
 &  &  & \HoloSegMetric{Spec.} & \HoloSegScore{1.000}{(1.000--1.000)}{4.55pt}{4.82pt}{} & \HoloSegScore{0.8261}{(0.6538--0.9583)}{4.55pt}{4.82pt}{} & \HoloSegScore{0.7391}{(0.5455--0.9092)}{4.55pt}{4.82pt}{} & \HoloSegScore{1.000}{(1.000--1.000)}{4.55pt}{4.82pt}{} & \HoloSegScore{1.000}{(1.000--1.000)}{4.55pt}{4.82pt}{} & \HoloSegScore{1.000}{(1.000--1.000)}{4.55pt}{4.82pt}{} & \HoloSegScore{1.000}{(1.000--1.000)}{4.55pt}{4.82pt}{} \\*
\softcline{4-11}
 &  & \HoloSegSpan{\makecell[c]{primary\\[-0.10ex]liver cancer}}{2.30cm}{0.32cm} & \HoloSegMetric{F1} & \HoloSegScore{0.0000}{(0.0000--0.0000)}{4.55pt}{4.82pt}{} & \HoloSegScore{0.7059}{(0.4000--0.9091)}{4.55pt}{4.82pt}{} & \HoloSegScore{0.6316}{(0.3077--0.8462)}{4.55pt}{4.82pt}{} & \HoloSegScore{1.000}{(1.000--1.000)}{4.55pt}{4.82pt}{} & \HoloSegScore{1.000}{(1.000--1.000)}{4.55pt}{4.82pt}{} & \HoloSegScore{1.000}{(1.000--1.000)}{4.55pt}{4.82pt}{} & \HoloSegScore{1.000}{(1.000--1.000)}{4.55pt}{4.82pt}{} \\*
\softcline{4-11}
 &  &  & \HoloSegMetric{Cond. Dice} & \HoloSegScore{-}{}{4.55pt}{4.82pt}{} & \HoloSegScore{0.6500}{(0.3433--0.8813)}{4.55pt}{4.82pt}{} & \HoloSegUnsupported & \HoloSegUnsupported & \HoloSegScore{0.7407}{(0.5913--0.8614)}{4.55pt}{4.82pt}{} & \HoloSegUnsupported & \HoloSegScore{0.6904}{(0.4280--0.8608)}{4.55pt}{4.82pt}{} \\
\cline{2-11}
 &  &  & \HoloSegMetric{Sens.} & \HoloSegScore{0.0000}{(0.0000--0.0000)}{4.55pt}{4.82pt}{} & \HoloSegScore{0.4000}{(0.1000--0.7278)}{4.55pt}{4.82pt}{} & \HoloSegScore{0.5000}{(0.1667--0.8333)}{4.55pt}{4.82pt}{} & \HoloSegScore{0.7000}{(0.3750--1.000)}{4.55pt}{4.82pt}{} & \HoloSegScore{0.7000}{(0.3750--1.000)}{4.55pt}{4.82pt}{} & \HoloSegScore{0.9000}{(0.6667--1.000)}{4.55pt}{4.82pt}{} & \HoloSegScore{0.9000}{(0.6667--1.000)}{4.55pt}{4.82pt}{} \\*
\softcline{4-11}
 &  &  & \HoloSegMetric{Spec.} & \HoloSegScore{1.000}{(1.000--1.000)}{4.55pt}{4.82pt}{} & \HoloSegScore{0.7500}{(0.5383--0.9202)}{4.55pt}{4.82pt}{} & \HoloSegScore{0.7500}{(0.5500--0.9375)}{4.55pt}{4.82pt}{} & \HoloSegScore{0.8500}{(0.6667--1.000)}{4.55pt}{4.82pt}{} & \HoloSegScore{0.8500}{(0.6667--1.000)}{4.55pt}{4.82pt}{} & \HoloSegScore{0.8000}{(0.6000--0.9501)}{4.55pt}{4.82pt}{} & \HoloSegScore{0.8000}{(0.6000--0.9501)}{4.55pt}{4.82pt}{} \\*
\softcline{4-11}
 & \HoloSegSpan{\makecell[c]{LiMT-\\[-0.10ex]oneclass}}{2.20cm}{0.32cm} & \HoloSegSpan{\makecell[c]{liver lesion}}{2.30cm}{0.32cm} & \HoloSegMetric{F1} & \HoloSegScore{0.0000}{(0.0000--0.0000)}{4.55pt}{4.82pt}{} & \HoloSegScore{0.4211}{(0.1176--0.6667)}{4.55pt}{4.82pt}{} & \HoloSegScore{0.5000}{(0.1818--0.7410)}{4.55pt}{4.82pt}{} & \HoloSegScore{0.7000}{(0.4211--0.8889)}{4.55pt}{4.82pt}{} & \HoloSegScore{0.7000}{(0.4211--0.8889)}{4.55pt}{4.82pt}{} & \HoloSegScore{0.7826}{(0.5455--0.9375)}{4.55pt}{4.82pt}{} & \HoloSegScore{0.7826}{(0.5455--0.9375)}{4.55pt}{4.82pt}{} \\*
\softcline{4-11}
 &  &  & \HoloSegMetric{Cond. Dice} & \HoloSegScore{-}{}{4.55pt}{4.82pt}{} & \HoloSegScore{0.2835}{(0.2158--0.3212)}{4.55pt}{4.82pt}{} & \HoloSegUnsupported & \HoloSegUnsupported & \HoloSegScore{0.6100}{(0.5105--0.7276)}{4.55pt}{4.82pt}{} & \HoloSegUnsupported & \HoloSegScore{0.5606}{(0.4261--0.6810)}{4.55pt}{4.82pt}{} \\
\hline
 &  &  & \HoloSegMetric{Sens.} & \HoloSegScore{0.0000}{(0.0000--0.0000)}{4.55pt}{4.82pt}{} & \HoloSegScore{0.0000}{(0.0000--0.0000)}{4.55pt}{4.82pt}{} & \HoloSegScore{0.0000}{(0.0000--0.0000)}{4.55pt}{4.82pt}{} & \HoloSegScore{0.1000}{(0.0000--0.3333)}{4.55pt}{4.82pt}{} & \HoloSegScore{0.1000}{(0.0000--0.3333)}{4.55pt}{4.82pt}{} & \HoloSegScore{0.1000}{(0.0000--0.3333)}{4.55pt}{4.82pt}{} & \HoloSegScore{0.2000}{(0.0000--0.5000)}{4.55pt}{4.82pt}{} \\*
\softcline{4-11}
 &  &  & \HoloSegMetric{Spec.} & \HoloSegScore{1.000}{(1.000--1.000)}{4.55pt}{4.82pt}{} & \HoloSegScore{1.000}{(1.000--1.000)}{4.55pt}{4.82pt}{} & \HoloSegScore{0.2500}{(0.0000--0.5714)}{4.55pt}{4.82pt}{} & \HoloSegScore{1.000}{(1.000--1.000)}{4.55pt}{4.82pt}{} & \HoloSegScore{1.000}{(1.000--1.000)}{4.55pt}{4.82pt}{} & \HoloSegScore{1.000}{(1.000--1.000)}{4.55pt}{4.82pt}{} & \HoloSegScore{1.000}{(1.000--1.000)}{4.55pt}{4.82pt}{} \\*
\softcline{4-11}
 & \HoloSegSpan{\makecell[c]{QUBIQ2021}}{2.20cm}{0.32cm} & \HoloSegSpan{\makecell[c]{pancreas\\[-0.10ex]lesion}}{2.30cm}{0.32cm} & \HoloSegMetric{F1} & \HoloSegScore{0.0000}{(0.0000--0.0000)}{4.55pt}{4.82pt}{} & \HoloSegScore{0.0000}{(0.0000--0.0000)}{4.55pt}{4.82pt}{} & \HoloSegScore{0.0000}{(0.0000--0.0000)}{4.55pt}{4.82pt}{} & \HoloSegScore{0.1818}{(0.0000--0.5000)}{4.55pt}{4.82pt}{} & \HoloSegScore{0.1818}{(0.0000--0.5000)}{4.55pt}{4.82pt}{} & \HoloSegScore{0.1818}{(0.0000--0.5000)}{4.55pt}{4.82pt}{} & \HoloSegScore{0.3333}{(0.0000--0.6667)}{4.55pt}{4.82pt}{} \\*
\softcline{4-11}
 &  &  & \HoloSegMetric{Cond. Dice} & \HoloSegScore{-}{}{4.55pt}{4.82pt}{} & \HoloSegScore{-}{}{4.55pt}{4.82pt}{} & \HoloSegUnsupported & \HoloSegUnsupported & \HoloSegScore{0.3361}{(0.3361--0.3361)}{4.55pt}{4.82pt}{} & \HoloSegUnsupported & \HoloSegScore{0.3867}{(0.3384--0.4350)}{4.55pt}{4.82pt}{} \\
\cline{2-11}
 &  &  & \HoloSegMetric{Sens.} & \HoloSegScore{0.0000}{(0.0000--0.0000)}{4.55pt}{4.82pt}{} & \HoloSegScore{0.09191}{(0.05861--0.1301)}{4.20pt}{4.48pt}{} & \HoloSegScore{0.1287}{(0.08855--0.1715)}{4.20pt}{4.48pt}{} & \HoloSegScore{0.8088}{(0.7593--0.8535)}{4.55pt}{4.82pt}{} & \HoloSegScore{0.8676}{(0.8261--0.9074)}{4.55pt}{4.82pt}{} & \HoloSegScore{0.8750}{(0.8327--0.9135)}{4.55pt}{4.82pt}{} & \HoloSegScore{0.7978}{(0.7491--0.8456)}{4.55pt}{4.82pt}{} \\*
\softcline{4-11}
 &  &  & \HoloSegMetric{Spec.} & \HoloSegScore{1.000}{(1.000--1.000)}{4.55pt}{4.82pt}{} & \HoloSegScore{0.1111}{(0.0000--0.3750)}{4.55pt}{4.82pt}{} & \HoloSegScore{0.1111}{(0.0000--0.3750)}{4.55pt}{4.82pt}{} & \HoloSegScore{0.8889}{(0.6248--1.000)}{4.55pt}{4.82pt}{} & \HoloSegScore{0.7778}{(0.4989--1.000)}{4.55pt}{4.82pt}{} & \HoloSegScore{1.000}{(1.000--1.000)}{4.55pt}{4.82pt}{} & \HoloSegScore{1.000}{(1.000--1.000)}{4.55pt}{4.82pt}{} \\*
\softcline{4-11}
\HoloSegSpan{\makecell[c]{\textbf{External-}\\[-0.10ex]\textbf{seen}\\[-0.10ex]\textbf{(zero-}\\[-0.10ex]\textbf{shot)}}}{1.35cm}{0.32cm} & \HoloSegSpan{\makecell[c]{TotalSeg-\\[-0.10ex]subtask-\\[-0.10ex]liver-\\[-0.10ex]lesion}}{2.20cm}{0.32cm} & \HoloSegSpan{\makecell[c]{liver lesion}}{2.30cm}{0.32cm} & \HoloSegMetric{F1} & \HoloSegScore{0.0000}{(0.0000--0.0000)}{4.55pt}{4.82pt}{} & \HoloSegScore{0.1639}{(0.1081--0.2222)}{4.55pt}{4.82pt}{} & \HoloSegScore{0.2222}{(0.1579--0.2866)}{4.55pt}{4.82pt}{} & \HoloSegScore{0.8925}{(0.8613--0.9206)}{4.55pt}{4.82pt}{} & \HoloSegScore{0.9255}{(0.9006--0.9482)}{4.55pt}{4.82pt}{} & \HoloSegScore{0.9333}{(0.9087--0.9548)}{4.55pt}{4.82pt}{} & \HoloSegScore{0.8875}{(0.8565--0.9163)}{4.55pt}{4.82pt}{} \\*
\softcline{4-11}
 &  &  & \HoloSegMetric{Cond. Dice} & \HoloSegScore{-}{}{4.55pt}{4.82pt}{} & \HoloSegScore{0.07529}{(0.03029--0.1113)}{4.20pt}{4.48pt}{} & \HoloSegUnsupported & \HoloSegUnsupported & \HoloSegScore{0.7096}{(0.6827--0.7361)}{4.55pt}{4.82pt}{} & \HoloSegUnsupported & \HoloSegScore{0.7456}{(0.7185--0.7684)}{4.55pt}{4.82pt}{} \\
\cline{2-11}
 &  &  & \HoloSegMetric{Sens.} & \HoloSegScore{0.0000}{(0.0000--0.0000)}{4.55pt}{4.82pt}{} & \HoloSegScore{0.09524}{(0.02273--0.2000)}{4.20pt}{4.48pt}{} & \HoloSegScore{0.1429}{(0.04651--0.2564)}{4.20pt}{4.48pt}{} & \HoloSegScore{0.5714}{(0.4146--0.7251)}{4.55pt}{4.82pt}{} & \HoloSegScore{0.6429}{(0.4878--0.7750)}{4.55pt}{4.82pt}{} & \HoloSegScore{0.5238}{(0.3684--0.6818)}{4.55pt}{4.82pt}{} & \HoloSegScore{0.4762}{(0.3191--0.6364)}{4.55pt}{4.82pt}{} \\*
\softcline{4-11}
 &  &  & \HoloSegMetric{Spec.} & \HoloSegScore{1.000}{(1.000--1.000)}{4.55pt}{4.82pt}{} & \HoloSegScore{0.1667}{(0.0000--0.6000)}{4.55pt}{4.82pt}{} & \HoloSegScore{0.1667}{(0.0000--0.5014)}{4.55pt}{4.82pt}{} & \HoloSegScore{1.000}{(1.000--1.000)}{4.55pt}{4.82pt}{} & \HoloSegScore{1.000}{(1.000--1.000)}{4.55pt}{4.82pt}{} & \HoloSegScore{1.000}{(1.000--1.000)}{4.55pt}{4.82pt}{} & \HoloSegScore{1.000}{(1.000--1.000)}{4.55pt}{4.82pt}{} \\*
\softcline{4-11}
 & \HoloSegSpan{\makecell[c]{MHB-SEG-\\[-0.10ex]oneclass}}{2.20cm}{0.32cm} & \HoloSegSpan{\makecell[c]{intracranial\\[-0.10ex]hemorrhage}}{2.30cm}{0.32cm} & \HoloSegMetric{F1} & \HoloSegScore{0.0000}{(0.0000--0.0000)}{4.55pt}{4.82pt}{} & \HoloSegScore{0.1569}{(0.04082--0.2963)}{4.20pt}{4.48pt}{} & \HoloSegScore{0.2264}{(0.08159--0.3730)}{4.20pt}{4.48pt}{} & \HoloSegScore{0.7273}{(0.5862--0.8406)}{4.55pt}{4.82pt}{} & \HoloSegScore{0.7826}{(0.6557--0.8732)}{4.55pt}{4.82pt}{} & \HoloSegScore{0.6875}{(0.5384--0.8108)}{4.55pt}{4.82pt}{} & \HoloSegScore{0.6452}{(0.4838--0.7778)}{4.55pt}{4.82pt}{} \\*
\softcline{4-11}
 &  &  & \HoloSegMetric{Cond. Dice} & \HoloSegScore{-}{}{4.55pt}{4.82pt}{} & \HoloSegScore{0.1263}{(0.07529--0.1755)}{4.20pt}{4.48pt}{} & \HoloSegUnsupported & \HoloSegUnsupported & \HoloSegScore{0.4056}{(0.2862--0.5260)}{4.55pt}{4.82pt}{} & \HoloSegUnsupported & \HoloSegScore{0.5143}{(0.3883--0.6315)}{4.55pt}{4.82pt}{} \\
\hline
 &  &  & \HoloSegMetric{Sens.} & \HoloSegScore{0.2000}{(0.0000--0.5000)}{4.55pt}{4.82pt}{} & \HoloSegScore{0.9000}{(0.6667--1.000)}{4.55pt}{4.82pt}{} & \HoloSegScore{0.9000}{(0.6667--1.000)}{4.55pt}{4.82pt}{} &  & \HoloSegScore{1.000}{(1.000--1.000)}{4.55pt}{4.82pt}{} &  & \HoloSegScore{0.9000}{(0.7000--1.000)}{4.55pt}{4.82pt}{} \\*
\softcline{4-7}\softcline{9-9}\softcline{11-11}
 &  &  & \HoloSegMetric{Spec.} & \HoloSegScore{0.8750}{(0.6000--1.000)}{4.55pt}{4.82pt}{} & \HoloSegScore{0.7500}{(0.4000--1.000)}{4.55pt}{4.82pt}{} & \HoloSegScore{0.2500}{(0.0000--0.6250)}{4.55pt}{4.82pt}{} &  & \HoloSegScore{0.6250}{(0.2500--1.000)}{4.55pt}{4.82pt}{} &  & \HoloSegScore{1.000}{(1.000--1.000)}{4.55pt}{4.82pt}{} \\*
\softcline{4-7}\softcline{9-9}\softcline{11-11}
\HoloSegSpan{\makecell[c]{\textbf{External-}\\[-0.10ex]\textbf{seen}\\[-0.10ex]\textbf{(fine-}\\[-0.10ex]\textbf{tuning)}}}{1.35cm}{0.32cm} & \HoloSegSpan{\makecell[c]{QUBIQ2021}}{2.20cm}{0.32cm} & \HoloSegSpan{\makecell[c]{pancreas\\[-0.10ex]lesion}}{2.30cm}{0.32cm} & \HoloSegMetric{F1} & \HoloSegScore{0.3077}{(0.0000--0.6154)}{4.55pt}{4.82pt}{} & \HoloSegScore{0.8571}{(0.6250--1.000)}{4.55pt}{4.82pt}{} & \HoloSegScore{0.7200}{(0.4545--0.8966)}{4.55pt}{4.82pt}{} & \raisebox{0.32cm}[0pt][0pt]{\HoloSegUnsupported} & \HoloSegScore{0.8696}{(0.6667--1.000)}{4.55pt}{4.82pt}{} & \raisebox{0.32cm}[0pt][0pt]{\HoloSegUnsupported} & \HoloSegScore{0.9474}{(0.8235--1.000)}{4.55pt}{4.82pt}{} \\*
\softcline{4-7}\softcline{9-9}\softcline{11-11}
 &  &  & \HoloSegMetric{Cond. Dice} & \HoloSegScore{0.1346}{(0.08605--0.1754)}{4.20pt}{4.48pt}{} & \HoloSegScore{0.4318}{(0.2274--0.6469)}{4.55pt}{4.82pt}{} & \HoloSegUnsupported &  & \HoloSegScore{0.7173}{(0.6478--0.7964)}{4.55pt}{4.82pt}{} &  & \HoloSegScore{0.7808}{(0.7108--0.8577)}{4.55pt}{4.82pt}{} \\
\hline
\pagebreak[4]
 &  &  & \HoloSegMetric{Sens.} & \HoloSegScore{0.9265}{(0.8926--0.9554)}{4.55pt}{4.82pt}{} & \HoloSegScore{0.9706}{(0.9485--0.9889)}{4.55pt}{4.82pt}{} & \HoloSegScore{1.000}{(1.000--1.000)}{4.55pt}{4.82pt}{} &  & \HoloSegScore{0.9890}{(0.9743--1.000)}{4.55pt}{4.82pt}{} &  & \HoloSegScore{0.9926}{(0.9814--1.000)}{4.55pt}{4.82pt}{} \\*
\softcline{4-7}\softcline{9-9}\softcline{11-11}
 &  &  & \HoloSegMetric{Spec.} & \HoloSegScore{0.3333}{(0.0000--0.7146)}{4.55pt}{4.82pt}{} & \HoloSegScore{0.2222}{(0.0000--0.5556)}{4.55pt}{4.82pt}{} & \HoloSegScore{0.1111}{(0.0000--0.3750)}{4.55pt}{4.82pt}{} &  & \HoloSegScore{0.7778}{(0.4444--1.000)}{4.55pt}{4.82pt}{} &  & \HoloSegScore{0.8889}{(0.6000--1.000)}{4.55pt}{4.82pt}{} \\*
\softcline{4-7}\softcline{9-9}\softcline{11-11}
 & \HoloSegSpan{\makecell[c]{TotalSeg-\\[-0.10ex]subtask-\\[-0.10ex]liver-\\[-0.10ex]lesion}}{2.20cm}{0.32cm} & \HoloSegSpan{\makecell[c]{liver lesion}}{2.30cm}{0.32cm} & \HoloSegMetric{F1} & \HoloSegScore{0.9509}{(0.9305--0.9669)}{4.55pt}{4.82pt}{} & \HoloSegScore{0.9724}{(0.9568--0.9837)}{4.55pt}{4.82pt}{} & \HoloSegScore{0.9855}{(0.9744--0.9946)}{4.55pt}{4.82pt}{} & \raisebox{0.32cm}[0pt][0pt]{\HoloSegUnsupported} & \HoloSegScore{0.9908}{(0.9814--0.9982)}{4.55pt}{4.82pt}{} & \raisebox{0.32cm}[0pt][0pt]{\HoloSegUnsupported} & \HoloSegScore{0.9945}{(0.9870--1.000)}{4.55pt}{4.82pt}{} \\*
\softcline{4-7}\softcline{9-9}\softcline{11-11}
 &  &  & \HoloSegMetric{Cond. Dice} & \HoloSegScore{0.2444}{(0.2064--0.2807)}{4.55pt}{4.82pt}{} & \HoloSegScore{0.7723}{(0.7427--0.8009)}{4.55pt}{4.82pt}{} & \HoloSegUnsupported &  & \HoloSegScore{0.7171}{(0.6954--0.7444)}{4.55pt}{4.82pt}{} &  & \HoloSegScore{0.7665}{(0.7443--0.7985)}{4.55pt}{4.82pt}{} \\
\cline{2-11}
\HoloSegSpan{\makecell[c]{\textbf{External-}\\[-0.10ex]\textbf{seen}\\[-0.10ex]\textbf{(fine-}\\[-0.10ex]\textbf{tuning)}}}{1.35cm}{0.32cm} &  &  & \HoloSegMetric{Sens.} & \HoloSegScore{0.9286}{(0.8421--1.000)}{4.55pt}{4.82pt}{} & \HoloSegScore{1.000}{(1.000--1.000)}{4.55pt}{4.82pt}{} & \HoloSegScore{0.9762}{(0.9231--1.000)}{4.55pt}{4.82pt}{} &  & \HoloSegScore{1.000}{(1.000--1.000)}{4.55pt}{4.82pt}{} &  & \HoloSegScore{1.000}{(1.000--1.000)}{4.55pt}{4.82pt}{} \\*
\softcline{4-7}\softcline{9-9}\softcline{11-11}
 &  &  & \HoloSegMetric{Spec.} & \HoloSegScore{0.3333}{(0.0000--0.8000)}{4.55pt}{4.82pt}{} & \HoloSegScore{0.3333}{(0.0000--0.7500)}{4.55pt}{4.82pt}{} & \HoloSegScore{0.0000}{(0.0000--0.0000)}{4.55pt}{4.82pt}{} &  & \HoloSegScore{0.6667}{(0.1415--1.000)}{4.55pt}{4.82pt}{} &  & \HoloSegScore{0.8333}{(0.4286--1.000)}{4.55pt}{4.82pt}{} \\*
\softcline{4-7}\softcline{9-9}\softcline{11-11}
 & \HoloSegSpan{\makecell[c]{MHB-SEG-\\[-0.10ex]oneclass}}{2.20cm}{0.32cm} & \HoloSegSpan{\makecell[c]{intracranial\\[-0.10ex]hemorrhage}}{2.30cm}{0.32cm} & \HoloSegMetric{F1} & \HoloSegScore{0.9176}{(0.8500--0.9680)}{4.55pt}{4.82pt}{} & \HoloSegScore{0.9545}{(0.9048--0.9895)}{4.55pt}{4.82pt}{} & \HoloSegScore{0.9213}{(0.8571--0.9787)}{4.55pt}{4.82pt}{} & \raisebox{0.32cm}[0pt][0pt]{\HoloSegUnsupported} & \HoloSegScore{0.9767}{(0.9383--1.000)}{4.55pt}{4.82pt}{} & \raisebox{0.32cm}[0pt][0pt]{\HoloSegUnsupported} & \HoloSegScore{0.9882}{(0.9620--1.000)}{4.55pt}{4.82pt}{} \\*
\softcline{4-7}\softcline{9-9}\softcline{11-11}
 &  &  & \HoloSegMetric{Cond. Dice} & \HoloSegScore{0.1528}{(0.07214--0.1854)}{4.20pt}{4.48pt}{} & \HoloSegScore{0.6995}{(0.6429--0.7484)}{4.55pt}{4.82pt}{} & \HoloSegUnsupported &  & \HoloSegScore{0.5750}{(0.5116--0.6475)}{4.55pt}{4.82pt}{} &  & \HoloSegScore{0.6220}{(0.5651--0.6912)}{4.55pt}{4.82pt}{} \\
\hline
 &  &  & \HoloSegMetric{Sens.} & \HoloSegScore{0.07576}{(0.01639--0.1429)}{4.20pt}{4.48pt}{} &  &  & \HoloSegScore{0.7846}{(0.6849--0.8814)}{4.55pt}{4.82pt}{} & \HoloSegScore{0.8462}{(0.7535--0.9311)}{4.55pt}{4.82pt}{} & \HoloSegScore{0.4923}{(0.3709--0.6112)}{4.55pt}{4.82pt}{} & \HoloSegScore{0.8462}{(0.7581--0.9333)}{4.55pt}{4.82pt}{} \\*
\softcline{4-5}\softcline{8-11}
 &  &  & \HoloSegMetric{Spec.} & \HoloSegScore{0.1234}{(0.07333--0.1768)}{4.20pt}{4.48pt}{} &  &  & \HoloSegScore{0.6883}{(0.6207--0.7639)}{4.55pt}{4.82pt}{} & \HoloSegScore{0.7403}{(0.6730--0.8077)}{4.55pt}{4.82pt}{} & \HoloSegScore{0.9481}{(0.9125--0.9805)}{4.55pt}{4.82pt}{} & \HoloSegScore{0.8442}{(0.7871--0.8976)}{4.55pt}{4.82pt}{} \\*
\softcline{4-5}\softcline{8-11}
 & \HoloSegSpan{\makecell[c]{PANORAMA}}{2.20cm}{0.32cm} & \HoloSegSpan{\makecell[c]{pancreatic\\[-0.10ex]ductal\\[-0.10ex]adenocarcinoma}}{2.30cm}{0.32cm} & \HoloSegMetric{F1} & \HoloSegScore{0.04854}{(0.009950--0.09391)}{3.85pt}{4.12pt}{} & \raisebox{0.32cm}[0pt][0pt]{\HoloSegUnsupported} & \raisebox{0.32cm}[0pt][0pt]{\HoloSegUnsupported} & \HoloSegScore{0.6220}{(0.5393--0.7097)}{4.55pt}{4.82pt}{} & \HoloSegScore{0.6875}{(0.6000--0.7683)}{4.55pt}{4.82pt}{} & \HoloSegScore{0.6095}{(0.4898--0.7091)}{4.55pt}{4.82pt}{} & \HoloSegScore{0.7639}{(0.6880--0.8382)}{4.55pt}{4.82pt}{} \\*
\softcline{4-5}\softcline{8-11}
 &  &  & \HoloSegMetric{Cond. Dice} & \HoloSegScore{0.1064}{(0.07157--0.1459)}{4.20pt}{4.48pt}{} &  &  & \HoloSegUnsupported & \HoloSegScore{0.4112}{(0.3469--0.4737)}{4.55pt}{4.82pt}{} & \HoloSegUnsupported & \HoloSegScore{0.4468}{(0.3702--0.5143)}{4.55pt}{4.82pt}{} \\
\cline{2-11}
 &  &  & \HoloSegMetric{Sens.} & \HoloSegScore{1.000}{(1.000--1.000)}{4.55pt}{4.82pt}{} &  &  & \HoloSegScore{0.0000}{(0.0000--0.0000)}{4.55pt}{4.82pt}{} & \HoloSegScore{0.0000}{(0.0000--0.0000)}{4.55pt}{4.82pt}{} & \HoloSegScore{0.0000}{(0.0000--0.0000)}{4.55pt}{4.82pt}{} & \HoloSegScore{0.0000}{(0.0000--0.0000)}{4.55pt}{4.82pt}{} \\*
\softcline{4-5}\softcline{8-11}
 &  &  & \HoloSegMetric{Spec.} & \HoloSegScore{0.0000}{(0.0000--0.0000)}{4.55pt}{4.82pt}{} &  &  & \HoloSegScore{1.000}{(1.000--1.000)}{4.55pt}{4.82pt}{} & \HoloSegScore{1.000}{(1.000--1.000)}{4.55pt}{4.82pt}{} & \HoloSegScore{1.000}{(1.000--1.000)}{4.55pt}{4.82pt}{} & \HoloSegScore{1.000}{(1.000--1.000)}{4.55pt}{4.82pt}{} \\*
\softcline{4-5}\softcline{8-11}
 &  & \HoloSegSpan{\makecell[c]{epidural\\[-0.10ex]hemorrhage}}{2.30cm}{0.32cm} & \HoloSegMetric{F1} & \HoloSegScore{0.1887}{(0.04082--0.3448)}{4.20pt}{4.48pt}{} & \raisebox{0.32cm}[0pt][0pt]{\HoloSegUnsupported} & \raisebox{0.32cm}[0pt][0pt]{\HoloSegUnsupported} & \HoloSegScore{0.0000}{(0.0000--0.0000)}{4.55pt}{4.82pt}{} & \HoloSegScore{0.0000}{(0.0000--0.0000)}{4.55pt}{4.82pt}{} & \HoloSegScore{0.0000}{(0.0000--0.0000)}{4.55pt}{4.82pt}{} & \HoloSegScore{0.0000}{(0.0000--0.0000)}{4.55pt}{4.82pt}{} \\*
\softcline{4-5}\softcline{8-11}
 &  &  & \HoloSegMetric{Cond. Dice} & \HoloSegScore{0.0000}{(0.0000--0.0000)}{4.55pt}{4.82pt}{} &  &  & \HoloSegUnsupported & \HoloSegScore{-}{}{4.55pt}{4.82pt}{} & \HoloSegUnsupported & \HoloSegScore{-}{}{4.55pt}{4.82pt}{} \\
\cline{3-11}
 &  &  & \HoloSegMetric{Sens.} & \HoloSegScore{0.05000}{(0.0000--0.1667)}{4.55pt}{4.82pt}{} &  &  & \HoloSegScore{0.4000}{(0.1905--0.6190)}{4.55pt}{4.82pt}{} & \HoloSegScore{0.3500}{(0.1429--0.5789)}{4.55pt}{4.82pt}{} & \HoloSegScore{0.3500}{(0.1429--0.5789)}{4.55pt}{4.82pt}{} & \HoloSegScore{0.3500}{(0.1429--0.5789)}{4.55pt}{4.82pt}{} \\*
\softcline{4-5}\softcline{8-11}
 &  &  & \HoloSegMetric{Spec.} & \HoloSegScore{1.000}{(1.000--1.000)}{4.55pt}{4.82pt}{} &  &  & \HoloSegScore{0.9643}{(0.8787--1.000)}{4.55pt}{4.82pt}{} & \HoloSegScore{0.9643}{(0.8787--1.000)}{4.55pt}{4.82pt}{} & \HoloSegScore{0.9643}{(0.8787--1.000)}{4.55pt}{4.82pt}{} & \HoloSegScore{0.9643}{(0.8787--1.000)}{4.55pt}{4.82pt}{} \\*
\softcline{4-5}\softcline{8-11}
 &  & \HoloSegSpan{\makecell[c]{subdural\\[-0.10ex]hemorrhage}}{2.30cm}{0.32cm} & \HoloSegMetric{F1} & \HoloSegScore{0.09524}{(0.0000--0.2857)}{4.55pt}{4.82pt}{} & \raisebox{0.32cm}[0pt][0pt]{\HoloSegUnsupported} & \raisebox{0.32cm}[0pt][0pt]{\HoloSegUnsupported} & \HoloSegScore{0.5517}{(0.2999--0.7500)}{4.55pt}{4.82pt}{} & \HoloSegScore{0.5000}{(0.2353--0.7097)}{4.55pt}{4.82pt}{} & \HoloSegScore{0.5000}{(0.2353--0.7097)}{4.55pt}{4.82pt}{} & \HoloSegScore{0.5000}{(0.2353--0.7097)}{4.55pt}{4.82pt}{} \\*
\softcline{4-5}\softcline{8-11}
 &  &  & \HoloSegMetric{Cond. Dice} & \HoloSegScore{0.002020}{(0.002020--0.002020)}{3.85pt}{4.12pt}{} &  &  & \HoloSegUnsupported & \HoloSegScore{0.6676}{(0.4534--0.8512)}{4.55pt}{4.82pt}{} & \HoloSegUnsupported & \HoloSegScore{0.6724}{(0.4538--0.8441)}{4.55pt}{4.82pt}{} \\
\cline{3-11}
\HoloSegSpan{\makecell[c]{\textbf{External-}\\[-0.10ex]\textbf{unseen}\\[-0.10ex]\textbf{(zero-}\\[-0.10ex]\textbf{shot)}}}{1.35cm}{0.32cm} &  &  & \HoloSegMetric{Sens.} & \HoloSegScore{0.0000}{(0.0000--0.0000)}{4.55pt}{4.82pt}{} &  &  & \HoloSegScore{0.3000}{(0.1153--0.5238)}{4.55pt}{4.82pt}{} & \HoloSegScore{0.2000}{(0.04545--0.4000)}{4.20pt}{4.48pt}{} & \HoloSegScore{0.1000}{(0.0000--0.2500)}{4.55pt}{4.82pt}{} & \HoloSegScore{0.3000}{(0.1111--0.5238)}{4.55pt}{4.82pt}{} \\*
\softcline{4-5}\softcline{8-11}
 &  &  & \HoloSegMetric{Spec.} & \HoloSegScore{1.000}{(1.000--1.000)}{4.55pt}{4.82pt}{} &  &  & \HoloSegScore{0.9286}{(0.8182--1.000)}{4.55pt}{4.82pt}{} & \HoloSegScore{0.9643}{(0.8750--1.000)}{4.55pt}{4.82pt}{} & \HoloSegScore{1.000}{(1.000--1.000)}{4.55pt}{4.82pt}{} & \HoloSegScore{0.9643}{(0.8800--1.000)}{4.55pt}{4.82pt}{} \\*
\softcline{4-5}\softcline{8-11}
 & \HoloSegSpan{\makecell[c]{MHB-SEG-\\[-0.10ex]multiclass}}{2.20cm}{0.32cm} & \HoloSegSpan{\makecell[c]{subarachnoid\\[-0.10ex]hemorrhage}}{2.30cm}{0.32cm} & \HoloSegMetric{F1} & \HoloSegScore{0.0000}{(0.0000--0.0000)}{4.55pt}{4.82pt}{} & \raisebox{0.32cm}[0pt][0pt]{\HoloSegUnsupported} & \raisebox{0.32cm}[0pt][0pt]{\HoloSegUnsupported} & \HoloSegScore{0.4286}{(0.1818--0.6452)}{4.55pt}{4.82pt}{} & \HoloSegScore{0.3200}{(0.08333--0.5386)}{4.20pt}{4.48pt}{} & \HoloSegScore{0.1818}{(0.0000--0.4000)}{4.55pt}{4.82pt}{} & \HoloSegScore{0.4444}{(0.1905--0.6667)}{4.55pt}{4.82pt}{} \\*
\softcline{4-5}\softcline{8-11}
 &  &  & \HoloSegMetric{Cond. Dice} & \HoloSegScore{-}{}{4.55pt}{4.82pt}{} &  &  & \HoloSegUnsupported & \HoloSegScore{0.1777}{(0.0000--0.5956)}{4.55pt}{4.82pt}{} & \HoloSegUnsupported & \HoloSegScore{0.5016}{(0.2761--0.7039)}{4.55pt}{4.82pt}{} \\
\cline{3-11}
 &  &  & \HoloSegMetric{Sens.} & \HoloSegScore{0.0000}{(0.0000--0.0000)}{4.55pt}{4.82pt}{} &  &  & \HoloSegScore{0.0000}{(0.0000--0.0000)}{4.55pt}{4.82pt}{} & \HoloSegScore{0.0000}{(0.0000--0.0000)}{4.55pt}{4.82pt}{} & \HoloSegScore{0.0000}{(0.0000--0.0000)}{4.55pt}{4.82pt}{} & \HoloSegScore{0.0000}{(0.0000--0.0000)}{4.55pt}{4.82pt}{} \\*
\softcline{4-5}\softcline{8-11}
 &  &  & \HoloSegMetric{Spec.} & \HoloSegScore{1.000}{(1.000--1.000)}{4.55pt}{4.82pt}{} &  &  & \HoloSegScore{1.000}{(1.000--1.000)}{4.55pt}{4.82pt}{} & \HoloSegScore{1.000}{(1.000--1.000)}{4.55pt}{4.82pt}{} & \HoloSegScore{1.000}{(1.000--1.000)}{4.55pt}{4.82pt}{} & \HoloSegScore{1.000}{(1.000--1.000)}{4.55pt}{4.82pt}{} \\*
\softcline{4-5}\softcline{8-11}
 &  & \HoloSegSpan{\makecell[c]{intraparenchymal\\[-0.10ex]hemorrhage}}{2.30cm}{0.32cm} & \HoloSegMetric{F1} & \HoloSegScore{0.0000}{(0.0000--0.0000)}{4.55pt}{4.82pt}{} & \raisebox{0.32cm}[0pt][0pt]{\HoloSegUnsupported} & \raisebox{0.32cm}[0pt][0pt]{\HoloSegUnsupported} & \HoloSegScore{0.0000}{(0.0000--0.0000)}{4.55pt}{4.82pt}{} & \HoloSegScore{0.0000}{(0.0000--0.0000)}{4.55pt}{4.82pt}{} & \HoloSegScore{0.0000}{(0.0000--0.0000)}{4.55pt}{4.82pt}{} & \HoloSegScore{0.0000}{(0.0000--0.0000)}{4.55pt}{4.82pt}{} \\*
\softcline{4-5}\softcline{8-11}
 &  &  & \HoloSegMetric{Cond. Dice} & \HoloSegScore{-}{}{4.55pt}{4.82pt}{} &  &  & \HoloSegUnsupported & \HoloSegScore{-}{}{4.55pt}{4.82pt}{} & \HoloSegUnsupported & \HoloSegScore{-}{}{4.55pt}{4.82pt}{} \\
\cline{3-11}
 &  &  & \HoloSegMetric{Sens.} & \HoloSegScore{0.0000}{(0.0000--0.0000)}{4.55pt}{4.82pt}{} &  &  & \HoloSegScore{0.04762}{(0.0000--0.1667)}{4.55pt}{4.82pt}{} & \HoloSegScore{0.04762}{(0.0000--0.1579)}{4.55pt}{4.82pt}{} & \HoloSegScore{0.0000}{(0.0000--0.0000)}{4.55pt}{4.82pt}{} & \HoloSegScore{0.0000}{(0.0000--0.0000)}{4.55pt}{4.82pt}{} \\*
\softcline{4-5}\softcline{8-11}
 &  &  & \HoloSegMetric{Spec.} & \HoloSegScore{1.000}{(1.000--1.000)}{4.55pt}{4.82pt}{} &  &  & \HoloSegScore{1.000}{(1.000--1.000)}{4.55pt}{4.82pt}{} & \HoloSegScore{0.9630}{(0.8749--1.000)}{4.55pt}{4.82pt}{} & \HoloSegScore{0.9630}{(0.8667--1.000)}{4.55pt}{4.82pt}{} & \HoloSegScore{1.000}{(1.000--1.000)}{4.55pt}{4.82pt}{} \\*
\softcline{4-5}\softcline{8-11}
 &  & \HoloSegSpan{\makecell[c]{intraventricular\\[-0.10ex]hemorrhage}}{2.30cm}{0.32cm} & \HoloSegMetric{F1} & \HoloSegScore{0.0000}{(0.0000--0.0000)}{4.55pt}{4.82pt}{} & \raisebox{0.32cm}[0pt][0pt]{\HoloSegUnsupported} & \raisebox{0.32cm}[0pt][0pt]{\HoloSegUnsupported} & \HoloSegScore{0.09091}{(0.0000--0.2857)}{4.55pt}{4.82pt}{} & \HoloSegScore{0.08696}{(0.0000--0.2727)}{4.55pt}{4.82pt}{} & \HoloSegScore{0.0000}{(0.0000--0.0000)}{4.55pt}{4.82pt}{} & \HoloSegScore{0.0000}{(0.0000--0.0000)}{4.55pt}{4.82pt}{} \\*
\softcline{4-5}\softcline{8-11}
 &  &  & \HoloSegMetric{Cond. Dice} & \HoloSegScore{-}{}{4.55pt}{4.82pt}{} &  &  & \HoloSegUnsupported & \HoloSegScore{0.6548}{(0.6548--0.6548)}{4.55pt}{4.82pt}{} & \HoloSegUnsupported & \HoloSegScore{-}{}{4.55pt}{4.82pt}{} \\
\hline
 &  &  & \HoloSegMetric{Sens.} & \HoloSegScore{0.8333}{(0.7376--0.9143)}{4.55pt}{4.82pt}{} & \HoloSegScore{0.6667}{(0.5556--0.7742)}{4.55pt}{4.82pt}{} & \HoloSegScore{0.6970}{(0.5857--0.7937)}{4.55pt}{4.82pt}{} &  & \HoloSegScore{0.8485}{(0.7586--0.9298)}{4.55pt}{4.82pt}{} &  & \HoloSegScore{0.8636}{(0.7750--0.9444)}{4.55pt}{4.82pt}{} \\*
\softcline{4-7}\softcline{9-9}\softcline{11-11}
 &  &  & \HoloSegMetric{Spec.} & \HoloSegScore{0.1883}{(0.1250--0.2483)}{4.55pt}{4.82pt}{} & \HoloSegScore{0.0000}{(0.0000--0.0000)}{4.55pt}{4.82pt}{} & \HoloSegScore{0.2208}{(0.1554--0.2875)}{4.55pt}{4.82pt}{} &  & \HoloSegScore{0.7532}{(0.6818--0.8258)}{4.55pt}{4.82pt}{} &  & \HoloSegScore{0.8442}{(0.7785--0.8968)}{4.55pt}{4.82pt}{} \\*
\softcline{4-7}\softcline{9-9}\softcline{11-11}
\HoloSegSpan{\makecell[c]{\textbf{External-}\\[-0.10ex]\textbf{unseen}\\[-0.10ex]\textbf{(fine-}\\[-0.10ex]\textbf{tuning)}}}{1.35cm}{0.32cm} & \HoloSegSpan{\makecell[c]{PANORAMA}}{2.20cm}{0.32cm} & \HoloSegSpan{\makecell[c]{pancreatic\\[-0.10ex]ductal\\[-0.10ex]adenocarcinoma}}{2.30cm}{0.32cm} & \HoloSegMetric{F1} & \HoloSegScore{0.4472}{(0.3739--0.5152)}{4.55pt}{4.82pt}{} & \HoloSegScore{0.3333}{(0.2609--0.4000)}{4.55pt}{4.82pt}{} & \HoloSegScore{0.3966}{(0.3196--0.4706)}{4.55pt}{4.82pt}{} & \raisebox{0.32cm}[0pt][0pt]{\HoloSegUnsupported} & \HoloSegScore{0.7000}{(0.6182--0.7791)}{4.55pt}{4.82pt}{} & \raisebox{0.32cm}[0pt][0pt]{\HoloSegUnsupported} & \HoloSegScore{0.7755}{(0.6880--0.8400)}{4.55pt}{4.82pt}{} \\*
\softcline{4-7}\softcline{9-9}\softcline{11-11}
 &  &  & \HoloSegMetric{Cond. Dice} & \HoloSegScore{0.2283}{(0.1588--0.3044)}{4.55pt}{4.82pt}{} & \HoloSegScore{0.4000}{(0.3244--0.4844)}{4.55pt}{4.82pt}{} & \HoloSegUnsupported &  & \HoloSegScore{0.5376}{(0.4840--0.6082)}{4.55pt}{4.82pt}{} &  & \HoloSegScore{0.5177}{(0.4665--0.5843)}{4.55pt}{4.82pt}{} \\
\hline
\pagebreak[4]
 &  &  & \HoloSegMetric{Sens.} & \HoloSegScore{0.8000}{(0.3333--1.000)}{4.55pt}{4.82pt}{} & \HoloSegScore{0.8000}{(0.3333--1.000)}{4.55pt}{4.82pt}{} & \HoloSegScore{0.2000}{(0.0000--0.6667)}{4.55pt}{4.82pt}{} &  & \HoloSegScore{0.4000}{(0.0000--0.8857)}{4.55pt}{4.82pt}{} &  & \HoloSegScore{0.6000}{(0.0000--1.000)}{4.55pt}{4.82pt}{} \\*
\softcline{4-7}\softcline{9-9}\softcline{11-11}
 &  &  & \HoloSegMetric{Spec.} & \HoloSegScore{0.5116}{(0.3571--0.6591)}{4.55pt}{4.82pt}{} & \HoloSegScore{0.7442}{(0.6000--0.8667)}{4.55pt}{4.82pt}{} & \HoloSegScore{0.9302}{(0.8409--1.000)}{4.55pt}{4.82pt}{} &  & \HoloSegScore{0.9535}{(0.8810--1.000)}{4.55pt}{4.82pt}{} &  & \HoloSegScore{0.9070}{(0.8140--0.9773)}{4.55pt}{4.82pt}{} \\*
\softcline{4-7}\softcline{9-9}\softcline{11-11}
 &  & \HoloSegSpan{\makecell[c]{epidural\\[-0.10ex]hemorrhage}}{2.30cm}{0.32cm} & \HoloSegMetric{F1} & \HoloSegScore{0.2667}{(0.06897--0.4707)}{4.20pt}{4.48pt}{} & \HoloSegScore{0.4000}{(0.1111--0.6401)}{4.55pt}{4.82pt}{} & \HoloSegScore{0.2222}{(0.0000--0.6000)}{4.55pt}{4.82pt}{} & \raisebox{0.32cm}[0pt][0pt]{\HoloSegUnsupported} & \HoloSegScore{0.4444}{(0.0000--0.8000)}{4.55pt}{4.82pt}{} & \raisebox{0.32cm}[0pt][0pt]{\HoloSegUnsupported} & \HoloSegScore{0.5000}{(0.0000--0.8235)}{4.55pt}{4.82pt}{} \\*
\softcline{4-7}\softcline{9-9}\softcline{11-11}
 &  &  & \HoloSegMetric{Cond. Dice} & \HoloSegScore{0.08540}{(0.02290--0.1635)}{4.20pt}{4.48pt}{} & \HoloSegScore{0.5202}{(0.1516--0.8571)}{4.55pt}{4.82pt}{} & \HoloSegUnsupported &  & \HoloSegScore{0.2678}{(0.1545--0.3922)}{4.55pt}{4.82pt}{} &  & \HoloSegScore{0.3043}{(0.1908--0.4269)}{4.55pt}{4.82pt}{} \\
\cline{3-11}
 &  &  & \HoloSegMetric{Sens.} & \HoloSegScore{0.9000}{(0.7368--1.000)}{4.55pt}{4.82pt}{} & \HoloSegScore{1.000}{(1.000--1.000)}{4.55pt}{4.82pt}{} & \HoloSegScore{0.7500}{(0.5293--0.9412)}{4.55pt}{4.82pt}{} &  & \HoloSegScore{0.9000}{(0.7497--1.000)}{4.55pt}{4.82pt}{} &  & \HoloSegScore{0.9500}{(0.8235--1.000)}{4.55pt}{4.82pt}{} \\*
\softcline{4-7}\softcline{9-9}\softcline{11-11}
 &  &  & \HoloSegMetric{Spec.} & \HoloSegScore{0.1429}{(0.03125--0.2800)}{4.20pt}{4.48pt}{} & \HoloSegScore{0.8214}{(0.6774--0.9600)}{4.55pt}{4.82pt}{} & \HoloSegScore{0.1786}{(0.03996--0.3333)}{4.20pt}{4.48pt}{} &  & \HoloSegScore{0.9286}{(0.8148--1.000)}{4.55pt}{4.82pt}{} &  & \HoloSegScore{0.8929}{(0.7692--1.000)}{4.55pt}{4.82pt}{} \\*
\softcline{4-7}\softcline{9-9}\softcline{11-11}
 &  & \HoloSegSpan{\makecell[c]{subdural\\[-0.10ex]hemorrhage}}{2.30cm}{0.32cm} & \HoloSegMetric{F1} & \HoloSegScore{0.5806}{(0.4209--0.7213)}{4.55pt}{4.82pt}{} & \HoloSegScore{0.8889}{(0.7726--0.9756)}{4.55pt}{4.82pt}{} & \HoloSegScore{0.5172}{(0.3333--0.6667)}{4.55pt}{4.82pt}{} & \raisebox{0.32cm}[0pt][0pt]{\HoloSegUnsupported} & \HoloSegScore{0.9000}{(0.7742--0.9778)}{4.55pt}{4.82pt}{} & \raisebox{0.32cm}[0pt][0pt]{\HoloSegUnsupported} & \HoloSegScore{0.9048}{(0.7878--0.9804)}{4.55pt}{4.82pt}{} \\*
\softcline{4-7}\softcline{9-9}\softcline{11-11}
 &  &  & \HoloSegMetric{Cond. Dice} & \HoloSegScore{0.1231}{(0.06690--0.2047)}{4.20pt}{4.48pt}{} & \HoloSegScore{0.7027}{(0.5860--0.8007)}{4.55pt}{4.82pt}{} & \HoloSegUnsupported &  & \HoloSegScore{0.5851}{(0.4909--0.6855)}{4.55pt}{4.82pt}{} &  & \HoloSegScore{0.6043}{(0.5220--0.6809)}{4.55pt}{4.82pt}{} \\
\cline{3-11}
 &  &  & \HoloSegMetric{Sens.} & \HoloSegScore{0.9000}{(0.7368--1.000)}{4.55pt}{4.82pt}{} & \HoloSegScore{0.9500}{(0.8333--1.000)}{4.55pt}{4.82pt}{} & \HoloSegScore{0.9000}{(0.7368--1.000)}{4.55pt}{4.82pt}{} &  & \HoloSegScore{0.9500}{(0.8400--1.000)}{4.55pt}{4.82pt}{} &  & \HoloSegScore{0.9500}{(0.8421--1.000)}{4.55pt}{4.82pt}{} \\*
\softcline{4-7}\softcline{9-9}\softcline{11-11}
 &  &  & \HoloSegMetric{Spec.} & \HoloSegScore{0.1429}{(0.03125--0.2800)}{4.20pt}{4.48pt}{} & \HoloSegScore{0.8929}{(0.7500--1.000)}{4.55pt}{4.82pt}{} & \HoloSegScore{0.2143}{(0.06897--0.3667)}{4.20pt}{4.48pt}{} &  & \HoloSegScore{0.9286}{(0.8213--1.000)}{4.55pt}{4.82pt}{} &  & \HoloSegScore{0.9643}{(0.8750--1.000)}{4.55pt}{4.82pt}{} \\*
\softcline{4-7}\softcline{9-9}\softcline{11-11}
\HoloSegSpan{\makecell[c]{\textbf{External-}\\[-0.10ex]\textbf{unseen}\\[-0.10ex]\textbf{(fine-}\\[-0.10ex]\textbf{tuning)}}}{1.35cm}{0.32cm} & \HoloSegSpan{\makecell[c]{MHB-SEG-\\[-0.10ex]multiclass}}{2.20cm}{0.32cm} & \HoloSegSpan{\makecell[c]{subarachnoid\\[-0.10ex]hemorrhage}}{2.30cm}{0.32cm} & \HoloSegMetric{F1} & \HoloSegScore{0.5806}{(0.4209--0.7213)}{4.55pt}{4.82pt}{} & \HoloSegScore{0.9048}{(0.7826--0.9804)}{4.55pt}{4.82pt}{} & \HoloSegScore{0.6000}{(0.4313--0.7385)}{4.55pt}{4.82pt}{} & \raisebox{0.32cm}[0pt][0pt]{\HoloSegUnsupported} & \HoloSegScore{0.9268}{(0.8333--1.000)}{4.55pt}{4.82pt}{} & \raisebox{0.32cm}[0pt][0pt]{\HoloSegUnsupported} & \HoloSegScore{0.9500}{(0.8649--1.000)}{4.55pt}{4.82pt}{} \\*
\softcline{4-7}\softcline{9-9}\softcline{11-11}
 &  &  & \HoloSegMetric{Cond. Dice} & \HoloSegScore{0.1073}{(0.05880--0.1898)}{4.20pt}{4.48pt}{} & \HoloSegScore{0.6375}{(0.5301--0.7286)}{4.55pt}{4.82pt}{} & \HoloSegUnsupported &  & \HoloSegScore{0.3712}{(0.2888--0.4706)}{4.55pt}{4.82pt}{} &  & \HoloSegScore{0.4785}{(0.3952--0.5697)}{4.55pt}{4.82pt}{} \\
\cline{3-11}
 &  &  & \HoloSegMetric{Sens.} & \HoloSegScore{0.6500}{(0.4118--0.8637)}{4.55pt}{4.82pt}{} & \HoloSegScore{0.8500}{(0.6814--1.000)}{4.55pt}{4.82pt}{} & \HoloSegScore{0.6500}{(0.4118--0.8637)}{4.55pt}{4.82pt}{} &  & \HoloSegScore{0.8500}{(0.6842--1.000)}{4.55pt}{4.82pt}{} &  & \HoloSegScore{0.9000}{(0.7500--1.000)}{4.55pt}{4.82pt}{} \\*
\softcline{4-7}\softcline{9-9}\softcline{11-11}
 &  &  & \HoloSegMetric{Spec.} & \HoloSegScore{0.3571}{(0.1786--0.5358)}{4.55pt}{4.82pt}{} & \HoloSegScore{0.6786}{(0.5000--0.8463)}{4.55pt}{4.82pt}{} & \HoloSegScore{0.6071}{(0.4074--0.8000)}{4.55pt}{4.82pt}{} &  & \HoloSegScore{0.7500}{(0.5713--0.9000)}{4.55pt}{4.82pt}{} &  & \HoloSegScore{0.7143}{(0.5357--0.8800)}{4.55pt}{4.82pt}{} \\*
\softcline{4-7}\softcline{9-9}\softcline{11-11}
 &  & \HoloSegSpan{\makecell[c]{intraparenchymal\\[-0.10ex]hemorrhage}}{2.30cm}{0.32cm} & \HoloSegMetric{F1} & \HoloSegScore{0.5098}{(0.3254--0.6667)}{4.55pt}{4.82pt}{} & \HoloSegScore{0.7391}{(0.5714--0.8772)}{4.55pt}{4.82pt}{} & \HoloSegScore{0.5909}{(0.4000--0.7500)}{4.55pt}{4.82pt}{} & \raisebox{0.32cm}[0pt][0pt]{\HoloSegUnsupported} & \HoloSegScore{0.7727}{(0.6109--0.9020)}{4.55pt}{4.82pt}{} & \raisebox{0.32cm}[0pt][0pt]{\HoloSegUnsupported} & \HoloSegScore{0.7826}{(0.6285--0.8980)}{4.55pt}{4.82pt}{} \\*
\softcline{4-7}\softcline{9-9}\softcline{11-11}
 &  &  & \HoloSegMetric{Cond. Dice} & \HoloSegScore{0.08500}{(0.03620--0.1527)}{4.20pt}{4.48pt}{} & \HoloSegScore{0.4724}{(0.3697--0.5586)}{4.55pt}{4.82pt}{} & \HoloSegUnsupported &  & \HoloSegScore{0.2283}{(0.1485--0.3382)}{4.55pt}{4.82pt}{} &  & \HoloSegScore{0.2608}{(0.1773--0.3676)}{4.55pt}{4.82pt}{} \\
\cline{3-11}
 &  &  & \HoloSegMetric{Sens.} & \HoloSegScore{0.9048}{(0.7500--1.000)}{4.55pt}{4.82pt}{} & \HoloSegScore{0.9524}{(0.8333--1.000)}{4.55pt}{4.82pt}{} & \HoloSegScore{0.7143}{(0.4814--0.9048)}{4.55pt}{4.82pt}{} &  & \HoloSegScore{0.9048}{(0.7500--1.000)}{4.55pt}{4.82pt}{} &  & \HoloSegScore{0.9524}{(0.8333--1.000)}{4.55pt}{4.82pt}{} \\*
\softcline{4-7}\softcline{9-9}\softcline{11-11}
 &  &  & \HoloSegMetric{Spec.} & \HoloSegScore{0.1481}{(0.03226--0.2917)}{4.20pt}{4.48pt}{} & \HoloSegScore{0.7778}{(0.6154--0.9201)}{4.55pt}{4.82pt}{} & \HoloSegScore{0.2593}{(0.1034--0.4287)}{4.55pt}{4.82pt}{} &  & \HoloSegScore{0.8889}{(0.7500--1.000)}{4.55pt}{4.82pt}{} &  & \HoloSegScore{0.8519}{(0.7083--0.9655)}{4.55pt}{4.82pt}{} \\*
\softcline{4-7}\softcline{9-9}\softcline{11-11}
 &  & \HoloSegSpan{\makecell[c]{intraventricular\\[-0.10ex]hemorrhage}}{2.30cm}{0.32cm} & \HoloSegMetric{F1} & \HoloSegScore{0.6032}{(0.4444--0.7324)}{4.55pt}{4.82pt}{} & \HoloSegScore{0.8511}{(0.7142--0.9434)}{4.55pt}{4.82pt}{} & \HoloSegScore{0.5357}{(0.3555--0.6875)}{4.55pt}{4.82pt}{} & \raisebox{0.32cm}[0pt][0pt]{\HoloSegUnsupported} & \HoloSegScore{0.8837}{(0.7618--0.9730)}{4.55pt}{4.82pt}{} & \raisebox{0.32cm}[0pt][0pt]{\HoloSegUnsupported} & \HoloSegScore{0.8889}{(0.7778--0.9767)}{4.55pt}{4.82pt}{} \\*
\softcline{4-7}\softcline{9-9}\softcline{11-11}
 &  &  & \HoloSegMetric{Cond. Dice} & \HoloSegScore{0.1151}{(0.05780--0.1962)}{4.20pt}{4.48pt}{} & \HoloSegScore{0.4493}{(0.3364--0.5572)}{4.55pt}{4.82pt}{} & \HoloSegUnsupported &  & \HoloSegScore{0.4145}{(0.3327--0.5063)}{4.55pt}{4.82pt}{} &  & \HoloSegScore{0.5169}{(0.4371--0.6078)}{4.55pt}{4.82pt}{} \\
\hline
 &  &  & \HoloSegMetric{Sens.} &  &  &  &  & \HoloSegScore{0.5263}{(0.3823--0.6924)}{4.55pt}{4.82pt}{} &  & \HoloSegScore{0.5526}{(0.4000--0.7106)}{4.55pt}{4.82pt}{} \\*
\softcline{4-4}\softcline{9-9}\softcline{11-11}
 &  &  & \HoloSegMetric{Spec.} &  &  &  &  & \HoloSegScore{0.5922}{(0.4949--0.6789)}{4.55pt}{4.82pt}{} &  & \HoloSegScore{0.6019}{(0.5052--0.6931)}{4.55pt}{4.82pt}{} \\*
\softcline{4-4}\softcline{9-9}\softcline{11-11}
 &  & \HoloSegSpan{\makecell[c]{malignant\\[-0.10ex]thyroid\\[-0.10ex]tumor}}{2.30cm}{0.32cm} & \HoloSegMetric{F1} & \raisebox{0.32cm}[0pt][0pt]{\HoloSegUnsupported} & \raisebox{0.32cm}[0pt][0pt]{\HoloSegUnsupported} & \raisebox{0.32cm}[0pt][0pt]{\HoloSegUnsupported} & \raisebox{0.32cm}[0pt][0pt]{\HoloSegUnsupported} & \HoloSegScore{0.4000}{(0.2782--0.5099)}{4.55pt}{4.82pt}{} & \raisebox{0.32cm}[0pt][0pt]{\HoloSegUnsupported} & \HoloSegScore{0.4200}{(0.2970--0.5358)}{4.55pt}{4.82pt}{} \\*
\softcline{4-4}\softcline{9-9}\softcline{11-11}
 &  &  & \HoloSegMetric{Cond. Dice} &  &  &  &  & \HoloSegScore{0.1403}{(0.05336--0.2679)}{4.20pt}{4.48pt}{} &  & \HoloSegScore{0.1422}{(0.03349--0.2738)}{4.20pt}{4.48pt}{} \\
\cline{3-11}
 & \HoloSegSpan{\makecell[c]{Private03\\[-0.10ex](thyroid\\[-0.10ex]cancer-\\[-0.10ex]multi)}}{2.20cm}{0.32cm} &  & \HoloSegMetric{Sens.} &  &  &  &  & \HoloSegScore{0.3838}{(0.2941--0.4763)}{4.55pt}{4.82pt}{} &  & \HoloSegScore{0.4040}{(0.3157--0.4952)}{4.55pt}{4.82pt}{} \\*
\softcline{4-4}\softcline{9-9}\softcline{11-11}
 &  &  & \HoloSegMetric{Spec.} &  &  &  &  & \HoloSegScore{0.6429}{(0.4998--0.7778)}{4.55pt}{4.82pt}{} &  & \HoloSegScore{0.6429}{(0.5000--0.7839)}{4.55pt}{4.82pt}{} \\*
\softcline{4-4}\softcline{9-9}\softcline{11-11}
 &  & \HoloSegSpan{\makecell[c]{benign\\[-0.10ex]thyroid\\[-0.10ex]tumor}}{2.30cm}{0.32cm} & \HoloSegMetric{F1} & \raisebox{0.32cm}[0pt][0pt]{\HoloSegUnsupported} & \raisebox{0.32cm}[0pt][0pt]{\HoloSegUnsupported} & \raisebox{0.32cm}[0pt][0pt]{\HoloSegUnsupported} & \raisebox{0.32cm}[0pt][0pt]{\HoloSegUnsupported} & \HoloSegScore{0.5000}{(0.4028--0.5898)}{4.55pt}{4.82pt}{} & \raisebox{0.32cm}[0pt][0pt]{\HoloSegUnsupported} & \HoloSegScore{0.5195}{(0.4246--0.6072)}{4.55pt}{4.82pt}{} \\*
\softcline{4-4}\softcline{9-9}\softcline{11-11}
 &  &  & \HoloSegMetric{Cond. Dice} &  &  &  &  & \HoloSegScore{0.6429}{(0.5881--0.6942)}{4.55pt}{4.82pt}{} &  & \HoloSegScore{0.6397}{(0.5802--0.6991)}{4.55pt}{4.82pt}{} \\
\cline{2-11}
\HoloSegSpan{\makecell[c]{\textbf{Private}\\[-0.10ex]\textbf{(zero-}\\[-0.10ex]\textbf{shot)}}}{1.35cm}{0.32cm} &  &  & \HoloSegMetric{Sens.} &  &  &  &  & \HoloSegScore{0.3578}{(0.2752--0.4415)}{4.55pt}{4.82pt}{} &  & \HoloSegScore{0.3761}{(0.2909--0.4602)}{4.55pt}{4.82pt}{} \\*
\softcline{4-4}\softcline{9-9}\softcline{11-11}
 &  &  & \HoloSegMetric{Spec.} &  &  &  &  & \HoloSegScore{0.5938}{(0.4194--0.7667)}{4.55pt}{4.82pt}{} &  & \HoloSegScore{0.5938}{(0.4286--0.7586)}{4.55pt}{4.82pt}{} \\*
\softcline{4-4}\softcline{9-9}\softcline{11-11}
 & \HoloSegSpan{\makecell[c]{Private03\\[-0.10ex](thyroid\\[-0.10ex]cancer-\\[-0.10ex]one)}}{2.20cm}{0.32cm} & \HoloSegSpan{\makecell[c]{thyroid\\[-0.10ex]tumor}}{2.30cm}{0.32cm} & \HoloSegMetric{F1} & \raisebox{0.32cm}[0pt][0pt]{\HoloSegUnsupported} & \raisebox{0.32cm}[0pt][0pt]{\HoloSegUnsupported} & \raisebox{0.32cm}[0pt][0pt]{\HoloSegUnsupported} & \raisebox{0.32cm}[0pt][0pt]{\HoloSegUnsupported} & \HoloSegScore{0.4845}{(0.3875--0.5715)}{4.55pt}{4.82pt}{} & \raisebox{0.32cm}[0pt][0pt]{\HoloSegUnsupported} & \HoloSegScore{0.5031}{(0.4103--0.5883)}{4.55pt}{4.82pt}{} \\*
\softcline{4-4}\softcline{9-9}\softcline{11-11}
 &  &  & \HoloSegMetric{Cond. Dice} &  &  &  &  & \HoloSegScore{0.6475}{(0.5948--0.7016)}{4.55pt}{4.82pt}{} &  & \HoloSegScore{0.6671}{(0.6101--0.7195)}{4.55pt}{4.82pt}{} \\
\cline{2-11}
 &  &  & \HoloSegMetric{Sens.} &  &  &  &  & \HoloSegScore{0.4211}{(0.3182--0.5196)}{4.55pt}{4.82pt}{} &  & \HoloSegScore{0.4421}{(0.3370--0.5422)}{4.55pt}{4.82pt}{} \\*
\softcline{4-4}\softcline{9-9}\softcline{11-11}
 &  &  & \HoloSegMetric{Spec.} &  &  &  &  & \HoloSegScore{0.3803}{(0.2666--0.5000)}{4.55pt}{4.82pt}{} &  & \HoloSegScore{0.3944}{(0.2881--0.5132)}{4.55pt}{4.82pt}{} \\*
\softcline{4-4}\softcline{9-9}\softcline{11-11}
 & \HoloSegSpan{\makecell[c]{Private04(colon\\[-0.10ex]lesion)}}{2.20cm}{0.32cm} & \HoloSegSpan{\makecell[c]{colon lesion}}{2.30cm}{0.32cm} & \HoloSegMetric{F1} & \raisebox{0.32cm}[0pt][0pt]{\HoloSegUnsupported} & \raisebox{0.32cm}[0pt][0pt]{\HoloSegUnsupported} & \raisebox{0.32cm}[0pt][0pt]{\HoloSegUnsupported} & \raisebox{0.32cm}[0pt][0pt]{\HoloSegUnsupported} & \HoloSegScore{0.4469}{(0.3432--0.5326)}{4.55pt}{4.82pt}{} & \raisebox{0.32cm}[0pt][0pt]{\HoloSegUnsupported} & \HoloSegScore{0.4667}{(0.3678--0.5510)}{4.55pt}{4.82pt}{} \\*
\softcline{4-4}\softcline{9-9}\softcline{11-11}
 &  &  & \HoloSegMetric{Cond. Dice} &  &  &  &  & \HoloSegUnsupported &  & \HoloSegUnsupported \\
\hline
\pagebreak[4]
 &  &  & \HoloSegMetric{Sens.} &  & \HoloSegScore{0.5789}{(0.4250--0.7353)}{4.55pt}{4.82pt}{} & \HoloSegScore{0.6316}{(0.4736--0.7813)}{4.55pt}{4.82pt}{} &  & \HoloSegScore{0.6842}{(0.5313--0.8205)}{4.55pt}{4.82pt}{} &  & \HoloSegScore{0.7105}{(0.5581--0.8571)}{4.55pt}{4.82pt}{} \\*
\softcline{4-4}\softcline{6-7}\softcline{9-9}\softcline{11-11}
 &  &  & \HoloSegMetric{Spec.} &  & \HoloSegScore{0.6117}{(0.5200--0.7113)}{4.55pt}{4.82pt}{} & \HoloSegScore{0.6602}{(0.5714--0.7522)}{4.55pt}{4.82pt}{} &  & \HoloSegScore{0.7087}{(0.6176--0.7925)}{4.55pt}{4.82pt}{} &  & \HoloSegScore{0.7184}{(0.6277--0.8036)}{4.55pt}{4.82pt}{} \\*
\softcline{4-4}\softcline{6-7}\softcline{9-9}\softcline{11-11}
 &  & \HoloSegSpan{\makecell[c]{malignant\\[-0.10ex]thyroid\\[-0.10ex]tumor}}{2.30cm}{0.32cm} & \HoloSegMetric{F1} & \raisebox{0.32cm}[0pt][0pt]{\HoloSegUnsupported} & \HoloSegScore{0.4400}{(0.3146--0.5631)}{4.55pt}{4.82pt}{} & \HoloSegScore{0.4948}{(0.3636--0.6111)}{4.55pt}{4.82pt}{} & \raisebox{0.32cm}[0pt][0pt]{\HoloSegUnsupported} & \HoloSegScore{0.5532}{(0.4186--0.6729)}{4.55pt}{4.82pt}{} & \raisebox{0.32cm}[0pt][0pt]{\HoloSegUnsupported} & \HoloSegScore{0.5745}{(0.4565--0.6838)}{4.55pt}{4.82pt}{} \\*
\softcline{4-4}\softcline{6-7}\softcline{9-9}\softcline{11-11}
 &  &  & \HoloSegMetric{Cond. Dice} &  & \HoloSegScore{0.2338}{(0.1930--0.2796)}{4.55pt}{4.82pt}{} & \HoloSegUnsupported &  & \HoloSegScore{0.2137}{(0.1270--0.3335)}{4.55pt}{4.82pt}{} &  & \HoloSegScore{0.2009}{(0.1283--0.3145)}{4.55pt}{4.82pt}{} \\
\cline{3-11}
 & \HoloSegSpan{\makecell[c]{Private03\\[-0.10ex](thyroid\\[-0.10ex]cancer-\\[-0.10ex]multi)}}{2.20cm}{0.32cm} &  & \HoloSegMetric{Sens.} &  & \HoloSegScore{0.4141}{(0.3178--0.5104)}{4.55pt}{4.82pt}{} & \HoloSegScore{0.4545}{(0.3516--0.5521)}{4.55pt}{4.82pt}{} &  & \HoloSegScore{0.5354}{(0.4343--0.6346)}{4.55pt}{4.82pt}{} &  & \HoloSegScore{0.5455}{(0.4454--0.6429)}{4.55pt}{4.82pt}{} \\*
\softcline{4-4}\softcline{6-7}\softcline{9-9}\softcline{11-11}
 &  &  & \HoloSegMetric{Spec.} &  & \HoloSegScore{0.6667}{(0.5143--0.8096)}{4.55pt}{4.82pt}{} & \HoloSegScore{0.7143}{(0.5713--0.8445)}{4.55pt}{4.82pt}{} &  & \HoloSegScore{0.6429}{(0.5000--0.7857)}{4.55pt}{4.82pt}{} &  & \HoloSegScore{0.6667}{(0.5143--0.8095)}{4.55pt}{4.82pt}{} \\*
\softcline{4-4}\softcline{6-7}\softcline{9-9}\softcline{11-11}
 &  & \HoloSegSpan{\makecell[c]{benign\\[-0.10ex]thyroid\\[-0.10ex]tumor}}{2.30cm}{0.32cm} & \HoloSegMetric{F1} & \raisebox{0.32cm}[0pt][0pt]{\HoloSegUnsupported} & \HoloSegScore{0.5325}{(0.4354--0.6216)}{4.55pt}{4.82pt}{} & \HoloSegScore{0.5769}{(0.4755--0.6667)}{4.55pt}{4.82pt}{} & \raisebox{0.32cm}[0pt][0pt]{\HoloSegUnsupported} & \HoloSegScore{0.6347}{(0.5432--0.7135)}{4.55pt}{4.82pt}{} & \raisebox{0.32cm}[0pt][0pt]{\HoloSegUnsupported} & \HoloSegScore{0.6467}{(0.5584--0.7232)}{4.55pt}{4.82pt}{} \\*
\softcline{4-4}\softcline{6-7}\softcline{9-9}\softcline{11-11}
 &  &  & \HoloSegMetric{Cond. Dice} &  & \HoloSegScore{0.6012}{(0.5573--0.6621)}{4.55pt}{4.82pt}{} & \HoloSegUnsupported &  & \HoloSegScore{0.6518}{(0.5906--0.7297)}{4.55pt}{4.82pt}{} &  & \HoloSegScore{0.7152}{(0.6650--0.7737)}{4.55pt}{4.82pt}{} \\
\cline{2-11}
\HoloSegSpan{\makecell[c]{\textbf{Private}\\[-0.10ex]\textbf{(fine-}\\[-0.10ex]\textbf{tuning)}}}{1.35cm}{0.32cm} &  &  & \HoloSegMetric{Sens.} &  & \HoloSegScore{0.3853}{(0.2952--0.4775)}{4.55pt}{4.82pt}{} & \HoloSegScore{0.4220}{(0.3229--0.5176)}{4.55pt}{4.82pt}{} &  & \HoloSegScore{0.8440}{(0.7706--0.9107)}{4.55pt}{4.82pt}{} &  & \HoloSegScore{0.8624}{(0.7909--0.9238)}{4.55pt}{4.82pt}{} \\*
\softcline{4-4}\softcline{6-7}\softcline{9-9}\softcline{11-11}
 &  &  & \HoloSegMetric{Spec.} &  & \HoloSegScore{0.6250}{(0.4500--0.7931)}{4.55pt}{4.82pt}{} & \HoloSegScore{0.6875}{(0.5000--0.8485)}{4.55pt}{4.82pt}{} &  & \HoloSegScore{0.6875}{(0.5294--0.8378)}{4.55pt}{4.82pt}{} &  & \HoloSegScore{0.6563}{(0.5000--0.8236)}{4.55pt}{4.82pt}{} \\*
\softcline{4-4}\softcline{6-7}\softcline{9-9}\softcline{11-11}
 & \HoloSegSpan{\makecell[c]{Private03\\[-0.10ex](thyroid\\[-0.10ex]cancer-\\[-0.10ex]one)}}{2.20cm}{0.32cm} & \HoloSegSpan{\makecell[c]{thyroid\\[-0.10ex]tumor}}{2.30cm}{0.32cm} & \HoloSegMetric{F1} & \raisebox{0.32cm}[0pt][0pt]{\HoloSegUnsupported} & \HoloSegScore{0.5153}{(0.4161--0.6057)}{4.55pt}{4.82pt}{} & \HoloSegScore{0.5576}{(0.4557--0.6437)}{4.55pt}{4.82pt}{} & \raisebox{0.32cm}[0pt][0pt]{\HoloSegUnsupported} & \HoloSegScore{0.8720}{(0.8200--0.9182)}{4.55pt}{4.82pt}{} & \raisebox{0.32cm}[0pt][0pt]{\HoloSegUnsupported} & \HoloSegScore{0.8785}{(0.8293--0.9174)}{4.55pt}{4.82pt}{} \\*
\softcline{4-4}\softcline{6-7}\softcline{9-9}\softcline{11-11}
 &  &  & \HoloSegMetric{Cond. Dice} &  & \HoloSegScore{0.6114}{(0.5725--0.6887)}{4.55pt}{4.82pt}{} & \HoloSegUnsupported &  & \HoloSegScore{0.6592}{(0.6044--0.7289)}{4.55pt}{4.82pt}{} &  & \HoloSegScore{0.7197}{(0.6718--0.7792)}{4.55pt}{4.82pt}{} \\
\cline{2-11}
 &  &  & \HoloSegMetric{Sens.} &  & \HoloSegScore{0.4526}{(0.3535--0.5474)}{4.55pt}{4.82pt}{} & \HoloSegScore{0.5263}{(0.4285--0.6250)}{4.55pt}{4.82pt}{} & \HoloSegScore{0.9053}{(0.8421--0.9588)}{4.55pt}{4.82pt}{} &  & \HoloSegScore{0.9263}{(0.8687--0.9714)}{4.55pt}{4.82pt}{} &  \\*
\softcline{4-4}\softcline{6-7}\softcline{8-8}\softcline{10-10}
 &  &  & \HoloSegMetric{Spec.} &  & \HoloSegScore{0.4085}{(0.2957--0.5352)}{4.55pt}{4.82pt}{} & \HoloSegScore{0.4789}{(0.3662--0.6057)}{4.55pt}{4.82pt}{} & \HoloSegScore{0.8310}{(0.7424--0.9167)}{4.55pt}{4.82pt}{} &  & \HoloSegScore{0.8310}{(0.7368--0.9067)}{4.55pt}{4.82pt}{} &  \\*
\softcline{4-4}\softcline{6-7}\softcline{8-8}\softcline{10-10}
 & \HoloSegSpan{\makecell[c]{Private04(colon\\[-0.10ex]lesion)}}{2.20cm}{0.32cm} & \HoloSegSpan{\makecell[c]{colon lesion}}{2.30cm}{0.32cm} & \HoloSegMetric{F1} & \raisebox{0.32cm}[0pt][0pt]{\HoloSegUnsupported} & \HoloSegScore{0.4778}{(0.3820--0.5672)}{4.55pt}{4.82pt}{} & \HoloSegScore{0.5495}{(0.4578--0.6334)}{4.55pt}{4.82pt}{} & \HoloSegScore{0.8912}{(0.8414--0.9340)}{4.55pt}{4.82pt}{} & \raisebox{0.32cm}[0pt][0pt]{\HoloSegUnsupported} & \HoloSegScore{0.9026}{(0.8528--0.9394)}{4.55pt}{4.82pt}{} & \raisebox{0.32cm}[0pt][0pt]{\HoloSegUnsupported} \\*
\softcline{4-4}\softcline{6-7}\softcline{8-8}\softcline{10-10}
 &  &  & \HoloSegMetric{Cond. Dice} &  & \HoloSegUnsupported & \HoloSegUnsupported & \HoloSegUnsupported &  & \HoloSegUnsupported &  \\
\hline
\end{longtable}
\arrayrulecolor{black}
\endgroup
