# Supplementary material for: A 3D foundation model unifying CT interpretation and segmentation
Source: arXiv:2611.06471 source file (2026-11-04)
Supplement: Supplementary file 11 [file table3_subtask3.tex]

\begingroup
\makeatletter
\@ifundefined{color@leftblue}{\definecolor{leftblue}{RGB}{232,242,248}}{}%
\@ifundefined{color@headerblue}{\definecolor{headerblue}{RGB}{218,233,242}}{}%
\makeatother
\setlength{\LTcapwidth}{18.60cm}
\setlength{\LTleft}{\fill}
\setlength{\LTright}{\fill}
\setlength{\LTpre}{0pt}
\setlength{\LTpost}{0pt}
\setlength{\tabcolsep}{0.45pt}
\renewcommand{\arraystretch}{1.00}
\setlength{\extrarowheight}{0pt}
\setlength{\arrayrulewidth}{0.48pt}
\arrayrulecolor{black}
\providecommand{\softcline}[1]{}%
\renewcommand{\softcline}[1]{\arrayrulecolor{black!35}\cline{#1}\arrayrulecolor{black}}
\sloppy
\emergencystretch=2em
\fontsize{5.30pt}{5.90pt}\selectfont
\newcommand{\HoloSegScore}[5]{%
  \parbox[c][0.64cm][c]{1.83cm}{%
    \centering
    {\fontsize{5.30pt}{5.58pt}\selectfont\strut\mbox{#1#5}}\\[-0.38ex]%
    {\fontsize{#3}{#4}\selectfont\strut\mbox{#2}}%
  }%
}%
\newcommand{\HoloSegUnsupported}{%
  \parbox[c][0.64cm][c]{1.83cm}{%
    \centering\fontsize{4.45pt}{4.70pt}\selectfont Not supported%
  }%
}%
\newcommand{\HoloSegMetric}[1]{%
  \parbox[c][0.64cm][c]{1.21cm}{%
    \centering\fontsize{5.45pt}{5.70pt}\selectfont\textbf{#1}%
  }%
}%
\newcommand{\HoloSegSpan}[3]{%
  \raisebox{#3}[0pt][0pt]{%
    \parbox[c]{#2}{\centering\arraybackslash #1}%
  }%
}%
\newcommand{\HoloSegSplitHead}[3]{%
  \parbox[c][0.92cm][c]{#3}{%
    \centering\fontsize{6.20pt}{6.45pt}\selectfont\textbf{#1}\\[-0.52ex]%
    \rule{0pt}{0.58ex}\\[-0.52ex]\textbf{#2}%
  }%
}%
\newcommand{\HoloSegMidHead}[2]{%
  \parbox[c][0.92cm][c]{#2}{%
    \centering\fontsize{5.25pt}{5.55pt}\selectfont\textbf{#1}%
  }%
}%
\begin{longtable}{|>{\columncolor{leftblue}\centering\arraybackslash}m{1.35cm}|>{\columncolor{leftblue}\centering\arraybackslash}m{2.20cm}|>{\columncolor{leftblue}\centering\arraybackslash}m{2.30cm}|>{\columncolor{leftblue}\centering\arraybackslash}m{1.25cm}|>{\centering\arraybackslash}m{1.85cm}|>{\centering\arraybackslash}m{1.85cm}|>{\centering\arraybackslash}m{1.85cm}|>{\centering\arraybackslash}m{1.85cm}|>{\centering\arraybackslash}m{1.85cm}|>{\centering\arraybackslash}m{1.85cm}|}
\caption[Multiple-target grounded lesion screening]{\textbf{Detailed sensitivity, specificity, F1, and conditional Dice scores of HoloCT and competing methods on internal, external-unseen, and private classification-segmentation benchmarks.}\newline Each score is reported as mean with 95\% confidence interval. Cond. Dice denotes conditional Dice.}%
\label{tab:classification_segmentation_scores}\\[-0.15ex]
\hline
\rowcolor{headerblue}
\HoloSegSplitHead{Dataset}{Type}{1.35cm} & \HoloSegSplitHead{Dataset}{Name}{2.20cm} & \HoloSegSplitHead{Label}{Name}{2.30cm} & \HoloSegMidHead{Metric}{1.25cm} & \HoloSegMidHead{nnU-Net}{1.85cm} & \HoloSegMidHead{ResNet}{1.85cm} & \HoloSegMidHead{\makecell[c]{HoloCT-4B\\[-0.18ex]w/o\\[-0.18ex]grounding}}{1.85cm} & \HoloSegMidHead{\makecell[c]{HoloCT-4B\\[-0.18ex]w/\\[-0.18ex]grounding}}{1.85cm} & \HoloSegMidHead{\makecell[c]{HoloCT-8B\\[-0.18ex]w/o\\[-0.18ex]grounding}}{1.85cm} & \HoloSegMidHead{\makecell[c]{HoloCT-8B\\[-0.18ex]w/\\[-0.18ex]grounding}}{1.85cm} \\
\hline
\endfirsthead
\caption*{\textbf{Supplementary Table~\ref{tab:classification_segmentation_scores} (continued)\enspace|\enspace Detailed sensitivity, specificity, F1, and conditional Dice scores of HoloCT and competing methods on internal, external-unseen, and private classification-segmentation benchmarks.}\newline Each score is reported as mean with 95\% confidence interval. Cond. Dice denotes conditional Dice.}\\[-0.15ex]
\hline
\rowcolor{headerblue}
\HoloSegSplitHead{Dataset}{Type}{1.35cm} & \HoloSegSplitHead{Dataset}{Name}{2.20cm} & \HoloSegSplitHead{Label}{Name}{2.30cm} & \HoloSegMidHead{Metric}{1.25cm} & \HoloSegMidHead{nnU-Net}{1.85cm} & \HoloSegMidHead{ResNet}{1.85cm} & \HoloSegMidHead{\makecell[c]{HoloCT-4B\\[-0.18ex]w/o\\[-0.18ex]grounding}}{1.85cm} & \HoloSegMidHead{\makecell[c]{HoloCT-4B\\[-0.18ex]w/\\[-0.18ex]grounding}}{1.85cm} & \HoloSegMidHead{\makecell[c]{HoloCT-8B\\[-0.18ex]w/o\\[-0.18ex]grounding}}{1.85cm} & \HoloSegMidHead{\makecell[c]{HoloCT-8B\\[-0.18ex]w/\\[-0.18ex]grounding}}{1.85cm} \\
\hline
\endhead
\endfoot
\endlastfoot
 &  &  & \HoloSegMetric{Sens.} & \HoloSegScore{0.6450}{(0.5893--0.7020)}{4.55pt}{4.82pt}{} & \HoloSegScore{0.7786}{(0.7210--0.8296)}{4.55pt}{4.82pt}{} & \HoloSegScore{0.4809}{(0.4196--0.5451)}{4.55pt}{4.82pt}{} & \HoloSegScore{0.6374}{(0.5792--0.6935)}{4.55pt}{4.82pt}{} & \HoloSegScore{0.6489}{(0.5891--0.7043)}{4.55pt}{4.82pt}{} & \HoloSegScore{0.5916}{(0.5323--0.6531)}{4.55pt}{4.82pt}{} \\*
\softcline{4-10}
 &  &  & \HoloSegMetric{Spec.} & \HoloSegScore{0.1792}{(0.1503--0.2073)}{4.55pt}{4.82pt}{} & \HoloSegScore{0.6867}{(0.6514--0.7218)}{4.55pt}{4.82pt}{} & \HoloSegScore{0.9593}{(0.9445--0.9746)}{4.55pt}{4.82pt}{} & \HoloSegScore{0.9051}{(0.8846--0.9259)}{4.55pt}{4.82pt}{} & \HoloSegScore{0.8690}{(0.8422--0.8941)}{4.55pt}{4.82pt}{} & \HoloSegScore{0.9533}{(0.9368--0.9682)}{4.55pt}{4.82pt}{} \\*
\softcline{4-10}
 &  & \HoloSegSpan{\makecell[c]{kidney\\[-0.10ex]lesion}}{2.30cm}{0.32cm} & \HoloSegMetric{F1} & \HoloSegScore{0.3463}{(0.3083--0.3859)}{4.55pt}{4.82pt}{} & \HoloSegScore{0.6053}{(0.5594--0.6455)}{4.55pt}{4.82pt}{} & \HoloSegScore{0.6072}{(0.5436--0.6603)}{4.55pt}{4.82pt}{} & \HoloSegScore{0.6789}{(0.6290--0.7252)}{4.55pt}{4.82pt}{} & \HoloSegScore{0.6551}{(0.6067--0.7002)}{4.55pt}{4.82pt}{} & \HoloSegScore{0.6920}{(0.6380--0.7389)}{4.55pt}{4.82pt}{} \\*
\softcline{4-10}
 &  &  & \HoloSegMetric{Cond. Dice} & \HoloSegScore{0.1775}{(0.09018--0.2727)}{4.20pt}{4.48pt}{} & \HoloSegUnsupported & \HoloSegUnsupported & \HoloSegScore{0.6958}{(0.6515--0.7358)}{4.55pt}{4.82pt}{} & \HoloSegUnsupported & \HoloSegScore{0.7600}{(0.7281--0.7905)}{4.55pt}{4.82pt}{} \\
\cline{3-10}
 &  &  & \HoloSegMetric{Sens.} & \HoloSegScore{0.8565}{(0.8082--0.9032)}{4.55pt}{4.82pt}{} & \HoloSegScore{0.3722}{(0.3100--0.4398)}{4.55pt}{4.82pt}{} & \HoloSegScore{0.6861}{(0.6232--0.7456)}{4.55pt}{4.82pt}{} & \HoloSegScore{0.7668}{(0.7101--0.8211)}{4.55pt}{4.82pt}{} & \HoloSegScore{0.7085}{(0.6403--0.7663)}{4.55pt}{4.82pt}{} & \HoloSegScore{0.7668}{(0.7091--0.8170)}{4.55pt}{4.82pt}{} \\*
\softcline{4-10}
 &  &  & \HoloSegMetric{Spec.} & \HoloSegScore{0.02134}{(0.01131--0.03277)}{4.20pt}{4.48pt}{} & \HoloSegScore{0.8478}{(0.8214--0.8750)}{4.55pt}{4.82pt}{} & \HoloSegScore{0.9516}{(0.9343--0.9653)}{4.55pt}{4.82pt}{} & \HoloSegScore{0.9175}{(0.8950--0.9380)}{4.55pt}{4.82pt}{} & \HoloSegScore{0.9189}{(0.8975--0.9379)}{4.55pt}{4.82pt}{} & \HoloSegScore{0.9161}{(0.8956--0.9365)}{4.55pt}{4.82pt}{} \\*
\softcline{4-10}
 &  & \HoloSegSpan{\makecell[c]{liver lesion}}{2.30cm}{0.32cm} & \HoloSegMetric{F1} & \HoloSegScore{0.3466}{(0.3114--0.3826)}{4.55pt}{4.82pt}{} & \HoloSegScore{0.4019}{(0.3416--0.4628)}{4.55pt}{4.82pt}{} & \HoloSegScore{0.7463}{(0.6966--0.7937)}{4.55pt}{4.82pt}{} & \HoloSegScore{0.7566}{(0.7113--0.7983)}{4.55pt}{4.82pt}{} & \HoloSegScore{0.7215}{(0.6697--0.7664)}{4.55pt}{4.82pt}{} & \HoloSegScore{0.7550}{(0.7107--0.7965)}{4.55pt}{4.82pt}{} \\*
\softcline{4-10}
 &  &  & \HoloSegMetric{Cond. Dice} & \HoloSegScore{0.1392}{(0.03089--0.2260)}{4.20pt}{4.48pt}{} & \HoloSegUnsupported & \HoloSegUnsupported & \HoloSegScore{0.7294}{(0.7031--0.7527)}{4.55pt}{4.82pt}{} & \HoloSegUnsupported & \HoloSegScore{0.6964}{(0.6638--0.7267)}{4.55pt}{4.82pt}{} \\
\cline{3-10}
 & \HoloSegSpan{\makecell[c]{AbdomenAtlas\\[-0.10ex]3.0}}{2.20cm}{0.32cm} &  & \HoloSegMetric{Sens.} & \HoloSegScore{0.4964}{(0.4077--0.5781)}{4.55pt}{4.82pt}{} & \HoloSegScore{0.4088}{(0.3333--0.5000)}{4.55pt}{4.82pt}{} & \HoloSegScore{0.2920}{(0.2170--0.3723)}{4.55pt}{4.82pt}{} & \HoloSegScore{0.4672}{(0.3788--0.5493)}{4.55pt}{4.82pt}{} & \HoloSegScore{0.2263}{(0.1571--0.2986)}{4.55pt}{4.82pt}{} & \HoloSegScore{0.6642}{(0.5789--0.7419)}{4.55pt}{4.82pt}{} \\*
\softcline{4-10}
 &  &  & \HoloSegMetric{Spec.} & \HoloSegScore{0.3992}{(0.3677--0.4320)}{4.55pt}{4.82pt}{} & \HoloSegScore{0.7668}{(0.7396--0.7959)}{4.55pt}{4.82pt}{} & \HoloSegScore{1.000}{(1.000--1.000)}{4.55pt}{4.82pt}{} & \HoloSegScore{0.9861}{(0.9781--0.9934)}{4.55pt}{4.82pt}{} & \HoloSegScore{0.9975}{(0.9936--1.000)}{4.55pt}{4.82pt}{} & \HoloSegScore{0.9341}{(0.9161--0.9506)}{4.55pt}{4.82pt}{} \\*
\softcline{4-10}
 &  & \HoloSegSpan{\makecell[c]{pancreas\\[-0.10ex]lesion}}{2.30cm}{0.32cm} & \HoloSegMetric{F1} & \HoloSegScore{0.2003}{(0.1570--0.2399)}{4.55pt}{4.82pt}{} & \HoloSegScore{0.2971}{(0.2372--0.3609)}{4.55pt}{4.82pt}{} & \HoloSegScore{0.4520}{(0.3567--0.5426)}{4.55pt}{4.82pt}{} & \HoloSegScore{0.6038}{(0.5171--0.6783)}{4.55pt}{4.82pt}{} & \HoloSegScore{0.3647}{(0.2709--0.4531)}{4.55pt}{4.82pt}{} & \HoloSegScore{0.6500}{(0.5789--0.7132)}{4.55pt}{4.82pt}{} \\*
\softcline{4-10}
 &  &  & \HoloSegMetric{Cond. Dice} & \HoloSegScore{0.1421}{(0.01590--0.2152)}{4.20pt}{4.48pt}{} & \HoloSegUnsupported & \HoloSegUnsupported & \HoloSegScore{0.5632}{(0.5086--0.6142)}{4.55pt}{4.82pt}{} & \HoloSegUnsupported & \HoloSegScore{0.5514}{(0.5014--0.5962)}{4.55pt}{4.82pt}{} \\
\cline{3-10}
 &  &  & \HoloSegMetric{Sens.} & \HoloSegScore{0.8000}{(0.6154--0.9524)}{4.55pt}{4.82pt}{} & \HoloSegScore{0.6800}{(0.5000--0.8571)}{4.55pt}{4.82pt}{} & \HoloSegScore{0.4000}{(0.2257--0.5806)}{4.55pt}{4.82pt}{} & \HoloSegScore{0.7200}{(0.5332--0.8929)}{4.55pt}{4.82pt}{} & \HoloSegScore{0.5200}{(0.3181--0.7143)}{4.55pt}{4.82pt}{} & \HoloSegScore{0.6800}{(0.5000--0.8571)}{4.55pt}{4.82pt}{} \\*
\softcline{4-10}
 &  &  & \HoloSegMetric{Spec.} & \HoloSegScore{0.04440}{(0.03182--0.05778)}{4.20pt}{4.48pt}{} & \HoloSegScore{0.03885}{(0.02655--0.05240)}{4.20pt}{4.48pt}{} & \HoloSegScore{0.9933}{(0.9878--0.9978)}{4.55pt}{4.82pt}{} & \HoloSegScore{0.9756}{(0.9653--0.9855)}{4.55pt}{4.82pt}{} & \HoloSegScore{0.9889}{(0.9811--0.9955)}{4.55pt}{4.82pt}{} & \HoloSegScore{0.9778}{(0.9676--0.9867)}{4.55pt}{4.82pt}{} \\*
\softcline{4-10}
 &  & \HoloSegSpan{\makecell[c]{colon lesion}}{2.30cm}{0.32cm} & \HoloSegMetric{F1} & \HoloSegScore{0.04415}{(0.02667--0.06339)}{4.20pt}{4.48pt}{} & \HoloSegScore{0.03744}{(0.02220--0.05507)}{4.20pt}{4.48pt}{} & \HoloSegScore{0.4878}{(0.2939--0.6667)}{4.55pt}{4.82pt}{} & \HoloSegScore{0.5538}{(0.3729--0.6970)}{4.55pt}{4.82pt}{} & \HoloSegScore{0.5417}{(0.3635--0.6977)}{4.55pt}{4.82pt}{} & \HoloSegScore{0.5484}{(0.3793--0.7000)}{4.55pt}{4.82pt}{} \\*
\softcline{4-10}
 &  &  & \HoloSegMetric{Cond. Dice} & \HoloSegScore{0.06071}{(0.009609--0.1507)}{4.20pt}{4.48pt}{} & \HoloSegUnsupported & \HoloSegUnsupported & \HoloSegScore{0.6472}{(0.5216--0.7513)}{4.55pt}{4.82pt}{} & \HoloSegUnsupported & \HoloSegScore{0.7291}{(0.6624--0.7895)}{4.55pt}{4.82pt}{} \\
\cline{2-10}
\HoloSegSpan{\makecell[c]{\textbf{Internal}}}{1.35cm}{0.32cm} &  &  & \HoloSegMetric{Sens.} & \HoloSegScore{0.6000}{(0.2857--0.9000)}{4.55pt}{4.82pt}{} & \HoloSegScore{0.0000}{(0.0000--0.0000)}{4.55pt}{4.82pt}{} & \HoloSegScore{0.7000}{(0.4000--1.000)}{4.55pt}{4.82pt}{} & \HoloSegScore{0.7000}{(0.4000--1.000)}{4.55pt}{4.82pt}{} & \HoloSegScore{0.3000}{(0.0000--0.6000)}{4.55pt}{4.82pt}{} & \HoloSegScore{0.6000}{(0.2857--0.8892)}{4.55pt}{4.82pt}{} \\*
\softcline{4-10}
 &  &  & \HoloSegMetric{Spec.} & \HoloSegScore{0.6000}{(0.3810--0.8125)}{4.55pt}{4.82pt}{} & \HoloSegScore{0.9000}{(0.7647--1.000)}{4.55pt}{4.82pt}{} & \HoloSegScore{0.9000}{(0.7616--1.000)}{4.55pt}{4.82pt}{} & \HoloSegScore{0.8500}{(0.6957--1.000)}{4.55pt}{4.82pt}{} & \HoloSegScore{0.9000}{(0.7500--1.000)}{4.55pt}{4.82pt}{} & \HoloSegScore{0.9000}{(0.7500--1.000)}{4.55pt}{4.82pt}{} \\*
\softcline{4-10}
 &  & \HoloSegSpan{\makecell[c]{liver cyst}}{2.30cm}{0.32cm} & \HoloSegMetric{F1} & \HoloSegScore{0.5000}{(0.2105--0.7200)}{4.55pt}{4.82pt}{} & \HoloSegScore{0.0000}{(0.0000--0.0000)}{4.55pt}{4.82pt}{} & \HoloSegScore{0.7368}{(0.4444--0.9333)}{4.55pt}{4.82pt}{} & \HoloSegScore{0.7000}{(0.4286--0.9000)}{4.55pt}{4.82pt}{} & \HoloSegScore{0.4000}{(0.0000--0.6667)}{4.55pt}{4.82pt}{} & \HoloSegScore{0.6667}{(0.3636--0.8800)}{4.55pt}{4.82pt}{} \\*
\softcline{4-10}
 &  &  & \HoloSegMetric{Cond. Dice} & \HoloSegScore{0.5755}{(0.5165--0.6487)}{4.55pt}{4.82pt}{} & \HoloSegUnsupported & \HoloSegUnsupported & \HoloSegScore{0.5934}{(0.4864--0.6965)}{4.55pt}{4.82pt}{} & \HoloSegUnsupported & \HoloSegScore{0.6870}{(0.5900--0.7691)}{4.55pt}{4.82pt}{} \\
\cline{3-10}
 &  &  & \HoloSegMetric{Sens.} & \HoloSegScore{0.6667}{(0.2000--1.000)}{4.55pt}{4.82pt}{} & \HoloSegScore{0.5000}{(0.0000--1.000)}{4.55pt}{4.82pt}{} & \HoloSegScore{0.6667}{(0.2000--1.000)}{4.55pt}{4.82pt}{} & \HoloSegScore{0.6667}{(0.2500--1.000)}{4.55pt}{4.82pt}{} & \HoloSegScore{1.000}{(1.000--1.000)}{4.55pt}{4.82pt}{} & \HoloSegScore{1.000}{(1.000--1.000)}{4.55pt}{4.82pt}{} \\*
\softcline{4-10}
 &  &  & \HoloSegMetric{Spec.} & \HoloSegScore{0.7083}{(0.5200--0.8750)}{4.55pt}{4.82pt}{} & \HoloSegScore{0.6667}{(0.4783--0.8462)}{4.55pt}{4.82pt}{} & \HoloSegScore{1.000}{(1.000--1.000)}{4.55pt}{4.82pt}{} & \HoloSegScore{1.000}{(1.000--1.000)}{4.55pt}{4.82pt}{} & \HoloSegScore{0.9583}{(0.8636--1.000)}{4.55pt}{4.82pt}{} & \HoloSegScore{0.9583}{(0.8571--1.000)}{4.55pt}{4.82pt}{} \\*
\softcline{4-10}
 &  & \HoloSegSpan{\makecell[c]{liver\\[-0.10ex]hemangioma}}{2.30cm}{0.32cm} & \HoloSegMetric{F1} & \HoloSegScore{0.4706}{(0.1426--0.7202)}{4.55pt}{4.82pt}{} & \HoloSegScore{0.3529}{(0.0000--0.6316)}{4.55pt}{4.82pt}{} & \HoloSegScore{0.8000}{(0.3333--1.000)}{4.55pt}{4.82pt}{} & \HoloSegScore{0.8000}{(0.4000--1.000)}{4.55pt}{4.82pt}{} & \HoloSegScore{0.9231}{(0.6667--1.000)}{4.55pt}{4.82pt}{} & \HoloSegScore{0.9231}{(0.7143--1.000)}{4.55pt}{4.82pt}{} \\*
\softcline{4-10}
 &  &  & \HoloSegMetric{Cond. Dice} & \HoloSegScore{0.5382}{(0.4786--0.6393)}{4.55pt}{4.82pt}{} & \HoloSegUnsupported & \HoloSegUnsupported & \HoloSegScore{0.8327}{(0.7710--0.8788)}{4.55pt}{4.82pt}{} & \HoloSegUnsupported & \HoloSegScore{0.7170}{(0.5129--0.8533)}{4.55pt}{4.82pt}{} \\
\cline{3-10}
 & \HoloSegSpan{\makecell[c]{LiMT}}{2.20cm}{0.32cm} &  & \HoloSegMetric{Sens.} & \HoloSegScore{0.5000}{(0.0000--1.000)}{4.55pt}{4.82pt}{} & \HoloSegScore{0.2500}{(0.0000--1.000)}{4.55pt}{4.82pt}{} & \HoloSegScore{0.5000}{(0.0000--1.000)}{4.55pt}{4.82pt}{} & \HoloSegScore{0.5000}{(0.0000--1.000)}{4.55pt}{4.82pt}{} & \HoloSegScore{0.5000}{(0.0000--1.000)}{4.55pt}{4.82pt}{} & \HoloSegScore{0.5000}{(0.0000--1.000)}{4.55pt}{4.82pt}{} \\*
\softcline{4-10}
 &  &  & \HoloSegMetric{Spec.} & \HoloSegScore{0.6923}{(0.5185--0.8571)}{4.55pt}{4.82pt}{} & \HoloSegScore{0.6923}{(0.5000--0.8750)}{4.55pt}{4.82pt}{} & \HoloSegScore{1.000}{(1.000--1.000)}{4.55pt}{4.82pt}{} & \HoloSegScore{1.000}{(1.000--1.000)}{4.55pt}{4.82pt}{} & \HoloSegScore{0.9615}{(0.8750--1.000)}{4.55pt}{4.82pt}{} & \HoloSegScore{0.9615}{(0.8800--1.000)}{4.55pt}{4.82pt}{} \\*
\softcline{4-10}
 &  & \HoloSegSpan{\makecell[c]{metastatic\\[-0.10ex]liver cancer}}{2.30cm}{0.32cm} & \HoloSegMetric{F1} & \HoloSegScore{0.2857}{(0.0000--0.5885)}{4.55pt}{4.82pt}{} & \HoloSegScore{0.1538}{(0.0000--0.4290)}{4.55pt}{4.82pt}{} & \HoloSegScore{0.6667}{(0.0000--1.000)}{4.55pt}{4.82pt}{} & \HoloSegScore{0.6667}{(0.0000--1.000)}{4.55pt}{4.82pt}{} & \HoloSegScore{0.5714}{(0.0000--1.000)}{4.55pt}{4.82pt}{} & \HoloSegScore{0.5714}{(0.0000--1.000)}{4.55pt}{4.82pt}{} \\*
\softcline{4-10}
 &  &  & \HoloSegMetric{Cond. Dice} & \HoloSegScore{0.3953}{(0.3170--0.4654)}{4.55pt}{4.82pt}{} & \HoloSegUnsupported & \HoloSegUnsupported & \HoloSegScore{0.5243}{(0.4417--0.6070)}{4.55pt}{4.82pt}{} & \HoloSegUnsupported & \HoloSegScore{0.6050}{(0.5343--0.6758)}{4.55pt}{4.82pt}{} \\
\cline{3-10}
 &  &  & \HoloSegMetric{Sens.} & \HoloSegScore{0.8571}{(0.5000--1.000)}{4.55pt}{4.82pt}{} & \HoloSegScore{0.8571}{(0.5000--1.000)}{4.55pt}{4.82pt}{} & \HoloSegScore{0.8571}{(0.5714--1.000)}{4.55pt}{4.82pt}{} & \HoloSegScore{1.000}{(1.000--1.000)}{4.55pt}{4.82pt}{} & \HoloSegScore{1.000}{(1.000--1.000)}{4.55pt}{4.82pt}{} & \HoloSegScore{1.000}{(1.000--1.000)}{4.55pt}{4.82pt}{} \\*
\softcline{4-10}
 &  &  & \HoloSegMetric{Spec.} & \HoloSegScore{0.8696}{(0.7143--1.000)}{4.55pt}{4.82pt}{} & \HoloSegScore{0.7826}{(0.5998--0.9446)}{4.55pt}{4.82pt}{} & \HoloSegScore{1.000}{(1.000--1.000)}{4.55pt}{4.82pt}{} & \HoloSegScore{1.000}{(1.000--1.000)}{4.55pt}{4.82pt}{} & \HoloSegScore{0.9565}{(0.8571--1.000)}{4.55pt}{4.82pt}{} & \HoloSegScore{0.9565}{(0.8571--1.000)}{4.55pt}{4.82pt}{} \\*
\softcline{4-10}
 &  & \HoloSegSpan{\makecell[c]{primary\\[-0.10ex]liver cancer}}{2.30cm}{0.32cm} & \HoloSegMetric{F1} & \HoloSegScore{0.7500}{(0.4000--0.9413)}{4.55pt}{4.82pt}{} & \HoloSegScore{0.6667}{(0.3525--0.8751)}{4.55pt}{4.82pt}{} & \HoloSegScore{0.9231}{(0.7273--1.000)}{4.55pt}{4.82pt}{} & \HoloSegScore{1.000}{(1.000--1.000)}{4.55pt}{4.82pt}{} & \HoloSegScore{0.9333}{(0.7273--1.000)}{4.55pt}{4.82pt}{} & \HoloSegScore{0.9333}{(0.7500--1.000)}{4.55pt}{4.82pt}{} \\*
\softcline{4-10}
 &  &  & \HoloSegMetric{Cond. Dice} & \HoloSegScore{0.6659}{(0.6137--0.7286)}{4.55pt}{4.82pt}{} & \HoloSegUnsupported & \HoloSegUnsupported & \HoloSegScore{0.7219}{(0.5662--0.8506)}{4.55pt}{4.82pt}{} & \HoloSegUnsupported & \HoloSegScore{0.6889}{(0.4131--0.8564)}{4.55pt}{4.82pt}{} \\
\hline
\pagebreak[4]
 &  &  & \HoloSegMetric{Sens.} &  &  & \HoloSegScore{0.0000}{(0.0000--0.0000)}{4.55pt}{4.82pt}{} & \HoloSegScore{0.6000}{(0.0000--1.000)}{4.55pt}{4.82pt}{} & \HoloSegScore{0.0000}{(0.0000--0.0000)}{4.55pt}{4.82pt}{} & \HoloSegScore{0.6000}{(0.0000--1.000)}{4.55pt}{4.82pt}{} \\*
\softcline{4-4}\softcline{7-10}
 &  &  & \HoloSegMetric{Spec.} &  &  & \HoloSegScore{1.000}{(1.000--1.000)}{4.55pt}{4.82pt}{} & \HoloSegScore{0.7674}{(0.6409--0.8838)}{4.55pt}{4.82pt}{} & \HoloSegScore{1.000}{(1.000--1.000)}{4.55pt}{4.82pt}{} & \HoloSegScore{0.8140}{(0.6889--0.9131)}{4.55pt}{4.82pt}{} \\*
\softcline{4-4}\softcline{7-10}
 &  & \HoloSegSpan{\makecell[c]{epidural\\[-0.10ex]hemorrhage}}{2.30cm}{0.32cm} & \HoloSegMetric{F1} & \raisebox{0.32cm}[0pt][0pt]{\HoloSegUnsupported} & \raisebox{0.32cm}[0pt][0pt]{\HoloSegUnsupported} & \HoloSegScore{0.0000}{(0.0000--0.0000)}{4.55pt}{4.82pt}{} & \HoloSegScore{0.3333}{(0.0000--0.6000)}{4.55pt}{4.82pt}{} & \HoloSegScore{0.0000}{(0.0000--0.0000)}{4.55pt}{4.82pt}{} & \HoloSegScore{0.3750}{(0.0000--0.6316)}{4.55pt}{4.82pt}{} \\*
\softcline{4-4}\softcline{7-10}
 &  &  & \HoloSegMetric{Cond. Dice} &  &  & \HoloSegUnsupported & \HoloSegScore{0.07251}{(0.0000--0.1890)}{4.55pt}{4.82pt}{} & \HoloSegUnsupported & \HoloSegScore{0.1517}{(0.0000--0.4220)}{4.55pt}{4.82pt}{} \\
\cline{3-10}
 &  &  & \HoloSegMetric{Sens.} &  &  & \HoloSegScore{0.5000}{(0.2778--0.7200)}{4.55pt}{4.82pt}{} & \HoloSegScore{0.5500}{(0.3182--0.7503)}{4.55pt}{4.82pt}{} & \HoloSegScore{0.6500}{(0.4117--0.8423)}{4.55pt}{4.82pt}{} & \HoloSegScore{0.8000}{(0.6111--0.9545)}{4.55pt}{4.82pt}{} \\*
\softcline{4-4}\softcline{7-10}
 &  &  & \HoloSegMetric{Spec.} &  &  & \HoloSegScore{0.8571}{(0.7308--0.9655)}{4.55pt}{4.82pt}{} & \HoloSegScore{0.6429}{(0.4545--0.8078)}{4.55pt}{4.82pt}{} & \HoloSegScore{0.5714}{(0.3846--0.7576)}{4.55pt}{4.82pt}{} & \HoloSegScore{0.5357}{(0.3448--0.7143)}{4.55pt}{4.82pt}{} \\*
\softcline{4-4}\softcline{7-10}
 &  & \HoloSegSpan{\makecell[c]{subdural\\[-0.10ex]hemorrhage}}{2.30cm}{0.32cm} & \HoloSegMetric{F1} & \raisebox{0.32cm}[0pt][0pt]{\HoloSegUnsupported} & \raisebox{0.32cm}[0pt][0pt]{\HoloSegUnsupported} & \HoloSegScore{0.5882}{(0.3636--0.7692)}{4.55pt}{4.82pt}{} & \HoloSegScore{0.5366}{(0.3333--0.6957)}{4.55pt}{4.82pt}{} & \HoloSegScore{0.5778}{(0.3636--0.7318)}{4.55pt}{4.82pt}{} & \HoloSegScore{0.6531}{(0.4762--0.7931)}{4.55pt}{4.82pt}{} \\*
\softcline{4-4}\softcline{7-10}
 &  &  & \HoloSegMetric{Cond. Dice} &  &  & \HoloSegUnsupported & \HoloSegScore{0.5082}{(0.2943--0.7023)}{4.55pt}{4.82pt}{} & \HoloSegUnsupported & \HoloSegScore{0.4733}{(0.3033--0.6348)}{4.55pt}{4.82pt}{} \\
\cline{3-10}
 &  &  & \HoloSegMetric{Sens.} &  &  & \HoloSegScore{0.0000}{(0.0000--0.0000)}{4.55pt}{4.82pt}{} & \HoloSegScore{0.1000}{(0.0000--0.2384)}{4.55pt}{4.82pt}{} & \HoloSegScore{0.1500}{(0.0000--0.3333)}{4.55pt}{4.82pt}{} & \HoloSegScore{0.3000}{(0.1175--0.5006)}{4.55pt}{4.82pt}{} \\*
\softcline{4-4}\softcline{7-10}
\HoloSegSpan{\makecell[c]{\textbf{External-}\\[-0.10ex]\textbf{unseen}\\[-0.10ex]\textbf{(zero-}\\[-0.10ex]\textbf{shot)}}}{1.35cm}{0pt} & \HoloSegSpan{\makecell[c]{MHB-SEG-\\[-0.10ex]multiclass}}{2.20cm}{0pt} &  & \HoloSegMetric{Spec.} &  &  & \HoloSegScore{0.9643}{(0.8888--1.000)}{4.55pt}{4.82pt}{} & \HoloSegScore{1.000}{(1.000--1.000)}{4.55pt}{4.82pt}{} & \HoloSegScore{1.000}{(1.000--1.000)}{4.55pt}{4.82pt}{} & \HoloSegScore{0.9643}{(0.8889--1.000)}{4.55pt}{4.82pt}{} \\*
\softcline{4-4}\softcline{7-10}
 &  & \HoloSegSpan{\makecell[c]{subarachnoid\\[-0.10ex]hemorrhage}}{2.30cm}{0.32cm} & \HoloSegMetric{F1} & \raisebox{0.32cm}[0pt][0pt]{\HoloSegUnsupported} & \raisebox{0.32cm}[0pt][0pt]{\HoloSegUnsupported} & \HoloSegScore{0.0000}{(0.0000--0.0000)}{4.55pt}{4.82pt}{} & \HoloSegScore{0.1818}{(0.0000--0.3850)}{4.55pt}{4.82pt}{} & \HoloSegScore{0.2609}{(0.0000--0.5000)}{4.55pt}{4.82pt}{} & \HoloSegScore{0.4444}{(0.1998--0.6667)}{4.55pt}{4.82pt}{} \\*
\softcline{4-4}\softcline{7-10}
 &  &  & \HoloSegMetric{Cond. Dice} &  &  & \HoloSegUnsupported & \HoloSegScore{0.0003018}{(0.0000--0.0006036)}{3.85pt}{4.12pt}{} & \HoloSegUnsupported & \HoloSegScore{0.4099}{(0.1943--0.5847)}{4.55pt}{4.82pt}{} \\
\cline{3-10}
 &  &  & \HoloSegMetric{Sens.} &  &  & \HoloSegScore{0.0000}{(0.0000--0.0000)}{4.55pt}{4.82pt}{} & \HoloSegScore{0.05000}{(0.0000--0.1739)}{4.55pt}{4.82pt}{} & \HoloSegScore{0.1000}{(0.0000--0.2500)}{4.55pt}{4.82pt}{} & \HoloSegScore{0.2000}{(0.04343--0.3750)}{4.20pt}{4.48pt}{} \\*
\softcline{4-4}\softcline{7-10}
 &  &  & \HoloSegMetric{Spec.} &  &  & \HoloSegScore{1.000}{(1.000--1.000)}{4.55pt}{4.82pt}{} & \HoloSegScore{0.9643}{(0.8788--1.000)}{4.55pt}{4.82pt}{} & \HoloSegScore{0.9286}{(0.8181--1.000)}{4.55pt}{4.82pt}{} & \HoloSegScore{0.7857}{(0.6154--0.9310)}{4.55pt}{4.82pt}{} \\*
\softcline{4-4}\softcline{7-10}
 &  & \HoloSegSpan{\makecell[c]{intraparenchymal\\[-0.10ex]hemorrhage}}{2.30cm}{0.32cm} & \HoloSegMetric{F1} & \raisebox{0.32cm}[0pt][0pt]{\HoloSegUnsupported} & \raisebox{0.32cm}[0pt][0pt]{\HoloSegUnsupported} & \HoloSegScore{0.0000}{(0.0000--0.0000)}{4.55pt}{4.82pt}{} & \HoloSegScore{0.09091}{(0.0000--0.2857)}{4.55pt}{4.82pt}{} & \HoloSegScore{0.1667}{(0.0000--0.3706)}{4.55pt}{4.82pt}{} & \HoloSegScore{0.2667}{(0.06452--0.4446)}{4.20pt}{4.48pt}{} \\*
\softcline{4-4}\softcline{7-10}
 &  &  & \HoloSegMetric{Cond. Dice} &  &  & \HoloSegUnsupported & \HoloSegScore{0.1675}{(0.1675--0.1675)}{4.55pt}{4.82pt}{} & \HoloSegUnsupported & \HoloSegScore{0.09218}{(0.0000--0.2251)}{4.55pt}{4.82pt}{} \\
\cline{3-10}
 &  &  & \HoloSegMetric{Sens.} &  &  & \HoloSegScore{0.0000}{(0.0000--0.0000)}{4.55pt}{4.82pt}{} & \HoloSegScore{0.0000}{(0.0000--0.0000)}{4.55pt}{4.82pt}{} & \HoloSegScore{0.0000}{(0.0000--0.0000)}{4.55pt}{4.82pt}{} & \HoloSegScore{0.0000}{(0.0000--0.0000)}{4.55pt}{4.82pt}{} \\*
\softcline{4-4}\softcline{7-10}
 &  & \HoloSegSpan{\makecell[c]{intraventricular\\[-0.10ex]hemorrhage}}{2.30cm}{0pt} & \HoloSegMetric{Spec.} & \raisebox{0pt}[0pt][0pt]{\HoloSegUnsupported} & \raisebox{0pt}[0pt][0pt]{\HoloSegUnsupported} & \HoloSegScore{1.000}{(1.000--1.000)}{4.55pt}{4.82pt}{} & \HoloSegScore{1.000}{(1.000--1.000)}{4.55pt}{4.82pt}{} & \HoloSegScore{1.000}{(1.000--1.000)}{4.55pt}{4.82pt}{} & \HoloSegScore{1.000}{(1.000--1.000)}{4.55pt}{4.82pt}{} \\*
\softcline{4-4}\softcline{7-10}
 &  &  & \HoloSegMetric{F1} &  &  & \HoloSegScore{0.0000}{(0.0000--0.0000)}{4.55pt}{4.82pt}{} & \HoloSegScore{0.0000}{(0.0000--0.0000)}{4.55pt}{4.82pt}{} & \HoloSegScore{0.0000}{(0.0000--0.0000)}{4.55pt}{4.82pt}{} & \HoloSegScore{0.0000}{(0.0000--0.0000)}{4.55pt}{4.82pt}{} \\
\hline
 &  &  & \HoloSegMetric{Sens.} & \HoloSegScore{0.6000}{(0.0000--1.000)}{4.55pt}{4.82pt}{} & \HoloSegScore{0.2000}{(0.0000--0.6667)}{4.55pt}{4.82pt}{} &  & \HoloSegScore{0.4000}{(0.0000--1.000)}{4.55pt}{4.82pt}{} &  & \HoloSegScore{0.6000}{(0.0000--1.000)}{4.55pt}{4.82pt}{} \\*
\softcline{4-6}\softcline{8-8}\softcline{10-10}
 &  &  & \HoloSegMetric{Spec.} & \HoloSegScore{0.6744}{(0.5224--0.8050)}{4.55pt}{4.82pt}{} & \HoloSegScore{0.9070}{(0.8049--0.9783)}{4.55pt}{4.82pt}{} &  & \HoloSegScore{0.9302}{(0.8444--1.000)}{4.55pt}{4.82pt}{} &  & \HoloSegScore{0.8837}{(0.7727--0.9744)}{4.55pt}{4.82pt}{} \\*
\softcline{4-6}\softcline{8-8}\softcline{10-10}
 &  & \HoloSegSpan{\makecell[c]{epidural\\[-0.10ex]hemorrhage}}{2.30cm}{0.32cm} & \HoloSegMetric{F1} & \HoloSegScore{0.2727}{(0.0000--0.5217)}{4.55pt}{4.82pt}{} & \HoloSegScore{0.2000}{(0.0000--0.5455)}{4.55pt}{4.82pt}{} & \raisebox{0.32cm}[0pt][0pt]{\HoloSegUnsupported} & \HoloSegScore{0.4000}{(0.0000--0.7500)}{4.55pt}{4.82pt}{} & \raisebox{0.32cm}[0pt][0pt]{\HoloSegUnsupported} & \HoloSegScore{0.4615}{(0.0000--0.7692)}{4.55pt}{4.82pt}{} \\*
\softcline{4-6}\softcline{8-8}\softcline{10-10}
 &  &  & \HoloSegMetric{Cond. Dice} & \HoloSegScore{0.4906}{(0.4688--0.5457)}{4.55pt}{4.82pt}{} & \HoloSegUnsupported &  & \HoloSegScore{0.2990}{(0.1455--0.4622)}{4.55pt}{4.82pt}{} &  & \HoloSegScore{0.3046}{(0.1443--0.4805)}{4.55pt}{4.82pt}{} \\
\cline{3-10}
 &  &  & \HoloSegMetric{Sens.} & \HoloSegScore{0.8000}{(0.6000--0.9524)}{4.55pt}{4.82pt}{} & \HoloSegScore{0.6000}{(0.3683--0.8182)}{4.55pt}{4.82pt}{} &  & \HoloSegScore{0.8500}{(0.6818--1.000)}{4.55pt}{4.82pt}{} &  & \HoloSegScore{0.9000}{(0.7497--1.000)}{4.55pt}{4.82pt}{} \\*
\softcline{4-6}\softcline{8-8}\softcline{10-10}
 &  &  & \HoloSegMetric{Spec.} & \HoloSegScore{0.6786}{(0.5000--0.8485)}{4.55pt}{4.82pt}{} & \HoloSegScore{0.1429}{(0.03226--0.2800)}{4.20pt}{4.48pt}{} &  & \HoloSegScore{0.8929}{(0.7777--1.000)}{4.55pt}{4.82pt}{} &  & \HoloSegScore{0.8571}{(0.7200--0.9667)}{4.55pt}{4.82pt}{} \\*
\softcline{4-6}\softcline{8-8}\softcline{10-10}
\HoloSegSpan{\makecell[c]{\textbf{External-}\\[-0.10ex]\textbf{unseen}\\[-0.10ex]\textbf{(fine-}\\[-0.10ex]\textbf{tuning)}}}{1.35cm}{0.32cm} & \HoloSegSpan{\makecell[c]{MHB-SEG-\\[-0.10ex]multiclass}}{2.20cm}{0.32cm} & \HoloSegSpan{\makecell[c]{subdural\\[-0.10ex]hemorrhage}}{2.30cm}{0.32cm} & \HoloSegMetric{F1} & \HoloSegScore{0.7111}{(0.5263--0.8511)}{4.55pt}{4.82pt}{} & \HoloSegScore{0.4286}{(0.2499--0.5862)}{4.55pt}{4.82pt}{} & \raisebox{0.32cm}[0pt][0pt]{\HoloSegUnsupported} & \HoloSegScore{0.8500}{(0.7179--0.9524)}{4.55pt}{4.82pt}{} & \raisebox{0.32cm}[0pt][0pt]{\HoloSegUnsupported} & \HoloSegScore{0.8571}{(0.7273--0.9545)}{4.55pt}{4.82pt}{} \\*
\softcline{4-6}\softcline{8-8}\softcline{10-10}
 &  &  & \HoloSegMetric{Cond. Dice} & \HoloSegScore{0.6389}{(0.5798--0.6881)}{4.55pt}{4.82pt}{} & \HoloSegUnsupported &  & \HoloSegScore{0.5177}{(0.3939--0.6513)}{4.55pt}{4.82pt}{} &  & \HoloSegScore{0.5340}{(0.4023--0.6668)}{4.55pt}{4.82pt}{} \\
\cline{3-10}
 &  &  & \HoloSegMetric{Sens.} & \HoloSegScore{0.8500}{(0.6814--1.000)}{4.55pt}{4.82pt}{} & \HoloSegScore{0.7500}{(0.5293--0.9412)}{4.55pt}{4.82pt}{} &  & \HoloSegScore{0.9000}{(0.7500--1.000)}{4.55pt}{4.82pt}{} &  & \HoloSegScore{0.9500}{(0.8333--1.000)}{4.55pt}{4.82pt}{} \\*
\softcline{4-6}\softcline{8-8}\softcline{10-10}
 &  &  & \HoloSegMetric{Spec.} & \HoloSegScore{0.7500}{(0.5833--0.9091)}{4.55pt}{4.82pt}{} & \HoloSegScore{0.1429}{(0.03125--0.2857)}{4.20pt}{4.48pt}{} &  & \HoloSegScore{0.8929}{(0.7666--1.000)}{4.55pt}{4.82pt}{} &  & \HoloSegScore{0.9286}{(0.8148--1.000)}{4.55pt}{4.82pt}{} \\*
\softcline{4-6}\softcline{8-8}\softcline{10-10}
 &  & \HoloSegSpan{\makecell[c]{subarachnoid\\[-0.10ex]hemorrhage}}{2.30cm}{0.32cm} & \HoloSegMetric{F1} & \HoloSegScore{0.7727}{(0.6111--0.8980)}{4.55pt}{4.82pt}{} & \HoloSegScore{0.5085}{(0.3273--0.6571)}{4.55pt}{4.82pt}{} & \raisebox{0.32cm}[0pt][0pt]{\HoloSegUnsupported} & \HoloSegScore{0.8780}{(0.7442--0.9730)}{4.55pt}{4.82pt}{} & \raisebox{0.32cm}[0pt][0pt]{\HoloSegUnsupported} & \HoloSegScore{0.9268}{(0.8292--1.000)}{4.55pt}{4.82pt}{} \\*
\softcline{4-6}\softcline{8-8}\softcline{10-10}
 &  &  & \HoloSegMetric{Cond. Dice} & \HoloSegScore{0.5750}{(0.5144--0.6449)}{4.55pt}{4.82pt}{} & \HoloSegUnsupported &  & \HoloSegScore{0.3841}{(0.2803--0.4974)}{4.55pt}{4.82pt}{} &  & \HoloSegScore{0.4089}{(0.3092--0.5146)}{4.55pt}{4.82pt}{} \\
\hline
\pagebreak[4]
 &  &  & \HoloSegMetric{Sens.} & \HoloSegScore{0.7000}{(0.4706--0.9000)}{4.55pt}{4.82pt}{} & \HoloSegScore{0.7000}{(0.4706--0.9000)}{4.55pt}{4.82pt}{} &  & \HoloSegScore{0.8500}{(0.6818--1.000)}{4.55pt}{4.82pt}{} &  & \HoloSegScore{0.9000}{(0.7500--1.000)}{4.55pt}{4.82pt}{} \\*
\softcline{4-6}\softcline{8-8}\softcline{10-10}
 &  &  & \HoloSegMetric{Spec.} & \HoloSegScore{0.5714}{(0.3793--0.7407)}{4.55pt}{4.82pt}{} & \HoloSegScore{0.6429}{(0.4544--0.8182)}{4.55pt}{4.82pt}{} &  & \HoloSegScore{0.7143}{(0.5556--0.8710)}{4.55pt}{4.82pt}{} &  & \HoloSegScore{0.6786}{(0.5000--0.8485)}{4.55pt}{4.82pt}{} \\*
\softcline{4-6}\softcline{8-8}\softcline{10-10}
 &  & \HoloSegSpan{\makecell[c]{intraparenchymal\\[-0.10ex]hemorrhage}}{2.30cm}{0.32cm} & \HoloSegMetric{F1} & \HoloSegScore{0.6087}{(0.4117--0.7600)}{4.55pt}{4.82pt}{} & \HoloSegScore{0.6364}{(0.4499--0.7895)}{4.55pt}{4.82pt}{} & \raisebox{0.32cm}[0pt][0pt]{\HoloSegUnsupported} & \HoloSegScore{0.7556}{(0.5882--0.8780)}{4.55pt}{4.82pt}{} & \raisebox{0.32cm}[0pt][0pt]{\HoloSegUnsupported} & \HoloSegScore{0.7660}{(0.6190--0.8889)}{4.55pt}{4.82pt}{} \\*
\softcline{4-6}\softcline{8-8}\softcline{10-10}
 &  &  & \HoloSegMetric{Cond. Dice} & \HoloSegScore{0.4188}{(0.3323--0.4707)}{4.55pt}{4.82pt}{} & \HoloSegUnsupported &  & \HoloSegScore{0.1604}{(0.09130--0.2585)}{4.20pt}{4.48pt}{} &  & \HoloSegScore{0.1802}{(0.1199--0.2719)}{4.55pt}{4.82pt}{} \\
\cline{3-10}
\HoloSegSpan{\makecell[c]{\textbf{External-}\\[-0.10ex]\textbf{unseen}\\[-0.10ex]\textbf{(fine-}\\[-0.10ex]\textbf{tuning)}}}{1.35cm}{0.32cm} & \HoloSegSpan{\makecell[c]{MHB-SEG-\\[-0.10ex]multiclass}}{2.20cm}{0.32cm} &  & \HoloSegMetric{Sens.} & \HoloSegScore{0.9524}{(0.8333--1.000)}{4.55pt}{4.82pt}{} & \HoloSegScore{0.5714}{(0.3529--0.7895)}{4.55pt}{4.82pt}{} &  & \HoloSegScore{0.8571}{(0.7058--1.000)}{4.55pt}{4.82pt}{} &  & \HoloSegScore{0.9524}{(0.8421--1.000)}{4.55pt}{4.82pt}{} \\*
\softcline{4-6}\softcline{8-8}\softcline{10-10}
 &  &  & \HoloSegMetric{Spec.} & \HoloSegScore{0.8148}{(0.6667--0.9583)}{4.55pt}{4.82pt}{} & \HoloSegScore{0.1852}{(0.04343--0.3478)}{4.20pt}{4.48pt}{} &  & \HoloSegScore{0.8519}{(0.7096--0.9643)}{4.55pt}{4.82pt}{} &  & \HoloSegScore{0.8148}{(0.6667--0.9397)}{4.55pt}{4.82pt}{} \\*
\softcline{4-6}\softcline{8-8}\softcline{10-10}
 &  & \HoloSegSpan{\makecell[c]{intraventricular\\[-0.10ex]hemorrhage}}{2.30cm}{0.32cm} & \HoloSegMetric{F1} & \HoloSegScore{0.8696}{(0.7429--0.9600)}{4.55pt}{4.82pt}{} & \HoloSegScore{0.4364}{(0.2609--0.6000)}{4.55pt}{4.82pt}{} & \raisebox{0.32cm}[0pt][0pt]{\HoloSegUnsupported} & \HoloSegScore{0.8372}{(0.7111--0.9412)}{4.55pt}{4.82pt}{} & \raisebox{0.32cm}[0pt][0pt]{\HoloSegUnsupported} & \HoloSegScore{0.8696}{(0.7500--0.9565)}{4.55pt}{4.82pt}{} \\*
\softcline{4-6}\softcline{8-8}\softcline{10-10}
 &  &  & \HoloSegMetric{Cond. Dice} & \HoloSegScore{0.4707}{(0.4162--0.5493)}{4.55pt}{4.82pt}{} & \HoloSegUnsupported &  & \HoloSegScore{0.3595}{(0.2569--0.4606)}{4.55pt}{4.82pt}{} &  & \HoloSegScore{0.3713}{(0.2787--0.4859)}{4.55pt}{4.82pt}{} \\
\hline
 &  &  & \HoloSegMetric{Sens.} & \HoloSegScore{0.5000}{(0.3448--0.6667)}{4.55pt}{4.82pt}{} & \HoloSegScore{0.5526}{(0.3947--0.7105)}{4.55pt}{4.82pt}{} &  & \HoloSegScore{0.6579}{(0.5143--0.8065)}{4.55pt}{4.82pt}{} &  & \HoloSegScore{0.6842}{(0.5333--0.8333)}{4.55pt}{4.82pt}{} \\*
\softcline{4-6}\softcline{8-8}\softcline{10-10}
 &  &  & \HoloSegMetric{Spec.} & \HoloSegScore{0.5631}{(0.4666--0.6598)}{4.55pt}{4.82pt}{} & \HoloSegScore{0.5922}{(0.4999--0.6882)}{4.55pt}{4.82pt}{} &  & \HoloSegScore{0.6699}{(0.5818--0.7604)}{4.55pt}{4.82pt}{} &  & \HoloSegScore{0.6893}{(0.5943--0.7822)}{4.55pt}{4.82pt}{} \\*
\softcline{4-6}\softcline{8-8}\softcline{10-10}
 &  & \HoloSegSpan{\makecell[c]{malignant\\[-0.10ex]thyroid\\[-0.10ex]tumor}}{2.30cm}{0.32cm} & \HoloSegMetric{F1} & \HoloSegScore{0.3725}{(0.2471--0.4906)}{4.55pt}{4.82pt}{} & \HoloSegScore{0.4158}{(0.2889--0.5377)}{4.55pt}{4.82pt}{} & \raisebox{0.32cm}[0pt][0pt]{\HoloSegUnsupported} & \HoloSegScore{0.5155}{(0.3953--0.6355)}{4.55pt}{4.82pt}{} & \raisebox{0.32cm}[0pt][0pt]{\HoloSegUnsupported} & \HoloSegScore{0.5417}{(0.4054--0.6542)}{4.55pt}{4.82pt}{} \\*
\softcline{4-6}\softcline{8-8}\softcline{10-10}
 &  &  & \HoloSegMetric{Cond. Dice} & \HoloSegScore{0.2906}{(0.1294--0.3550)}{4.55pt}{4.82pt}{} & \HoloSegUnsupported &  & \HoloSegScore{0.2760}{(0.1834--0.3895)}{4.55pt}{4.82pt}{} &  & \HoloSegScore{0.3155}{(0.2262--0.4279)}{4.55pt}{4.82pt}{} \\
\cline{3-10}
\HoloSegSpan{\makecell[c]{\textbf{Private}\\[-0.10ex]\textbf{(fine-}\\[-0.10ex]\textbf{tuning)}}}{1.35cm}{0.32cm} & \HoloSegSpan{\makecell[c]{Private03\\[-0.10ex](thyroid\\[-0.10ex]cancer-\\[-0.10ex]multi)}}{2.20cm}{0.32cm} &  & \HoloSegMetric{Sens.} & \HoloSegScore{0.3636}{(0.2680--0.4600)}{4.55pt}{4.82pt}{} & \HoloSegScore{0.3939}{(0.3000--0.4896)}{4.55pt}{4.82pt}{} &  & \HoloSegScore{0.5859}{(0.4888--0.6863)}{4.55pt}{4.82pt}{} &  & \HoloSegScore{0.6061}{(0.5102--0.7076)}{4.55pt}{4.82pt}{} \\*
\softcline{4-6}\softcline{8-8}\softcline{10-10}
 &  &  & \HoloSegMetric{Spec.} & \HoloSegScore{0.5714}{(0.4146--0.7250)}{4.55pt}{4.82pt}{} & \HoloSegScore{0.6190}{(0.4706--0.7692)}{4.55pt}{4.82pt}{} &  & \HoloSegScore{0.6905}{(0.5435--0.8298)}{4.55pt}{4.82pt}{} &  & \HoloSegScore{0.7381}{(0.5937--0.8684)}{4.55pt}{4.82pt}{} \\*
\softcline{4-6}\softcline{8-8}\softcline{10-10}
 &  & \HoloSegSpan{\makecell[c]{benign\\[-0.10ex]thyroid\\[-0.10ex]tumor}}{2.30cm}{0.32cm} & \HoloSegMetric{F1} & \HoloSegScore{0.4706}{(0.3694--0.5679)}{4.55pt}{4.82pt}{} & \HoloSegScore{0.5065}{(0.4082--0.5987)}{4.55pt}{4.82pt}{} & \raisebox{0.32cm}[0pt][0pt]{\HoloSegUnsupported} & \HoloSegScore{0.6824}{(0.5976--0.7609)}{4.55pt}{4.82pt}{} & \raisebox{0.32cm}[0pt][0pt]{\HoloSegUnsupported} & \HoloSegScore{0.7059}{(0.6173--0.7865)}{4.55pt}{4.82pt}{} \\*
\softcline{4-6}\softcline{8-8}\softcline{10-10}
 &  &  & \HoloSegMetric{Cond. Dice} & \HoloSegScore{0.5451}{(0.4786--0.6173)}{4.55pt}{4.82pt}{} & \HoloSegUnsupported &  & \HoloSegScore{0.6932}{(0.6231--0.7659)}{4.55pt}{4.82pt}{} &  & \HoloSegScore{0.7309}{(0.6735--0.8079)}{4.55pt}{4.82pt}{} \\
\hline
\end{longtable}
\arrayrulecolor{black}
\endgroup
