# Supplementary material for: A 3D foundation model unifying CT interpretation and segmentation
Source: arXiv:2611.06471 source file (2026-11-04)
Supplement: Supplementary file 12 [file table4_close_ended_vqa.tex]

\begingroup
\makeatletter
\@ifundefined{color@leftblue}{\definecolor{leftblue}{RGB}{232,242,248}}{}%
\@ifundefined{color@headerblue}{\definecolor{headerblue}{RGB}{218,233,242}}{}%
\makeatother
\setlength{\LTcapwidth}{18.60cm}
\setlength{\LTleft}{\fill}
\setlength{\LTright}{\fill}
\setlength{\LTpre}{0pt}
\setlength{\LTpost}{0pt}
\setlength{\tabcolsep}{0.45pt}
\renewcommand{\arraystretch}{1.00}
\setlength{\extrarowheight}{0pt}
\setlength{\arrayrulewidth}{0.48pt}
\arrayrulecolor{black}
\providecommand{\softcline}[1]{}%
\renewcommand{\softcline}[1]{\arrayrulecolor{black!35}\cline{#1}\arrayrulecolor{black}}
\sloppy
\emergencystretch=2em
\fontsize{5.15pt}{5.75pt}\selectfont
\newcommand{\HoloTaskScore}[4]{%
  \parbox[c][0.64cm][c]{1.70cm}{%
    \centering
    {\fontsize{5.15pt}{5.43pt}\selectfont\strut\mbox{#1}}\\[-0.38ex]%
    {\fontsize{#3}{#4}\selectfont\strut\mbox{#2}}%
  }%
}%
\newcommand{\HoloTaskMetricGroup}[1]{%
  \parbox[c][0.64cm][c]{1.045cm}{%
    \centering\fontsize{5.20pt}{5.48pt}\selectfont\textbf{#1}%
  }%
}%
\newcommand{\HoloTaskMetric}[1]{%
  \parbox[c][0.64cm][c]{1.045cm}{%
    \centering\fontsize{5.20pt}{5.48pt}\selectfont\textbf{#1}%
  }%
}%
\newcommand{\HoloTaskMergedMetric}[1]{%
  \parbox[c][0.64cm][c]{2.13cm}{%
    \centering\fontsize{5.20pt}{5.48pt}\selectfont\textbf{#1}%
  }%
}%
\newcommand{\HoloTaskRowSpan}[2]{%
  \parbox[c][0.64cm][c]{#2}{%
    \centering\arraybackslash #1%
  }%
}%
\newcommand{\HoloTaskSpan}[3]{%
  \raisebox{\dimexpr#3-0.11cm\relax}[0pt][0pt]{%
    \parbox[c][0.64cm][c]{#2}{%
      \centering\arraybackslash #1%
    }%
  }%
}%
\newcommand{\HoloTaskSplitHead}[3]{%
  \parbox[c][0.92cm][c]{#3}{%
    \centering\fontsize{6.05pt}{6.30pt}\selectfont\textbf{#1}\\[-0.52ex]%
    \rule{0pt}{0.58ex}\\[-0.52ex]\textbf{#2}%
  }%
}%
\newcommand{\HoloTaskMidHead}[2]{%
  \parbox[c][0.92cm][c]{#2}{%
    \centering\fontsize{6.05pt}{6.30pt}\selectfont\textbf{#1}%
  }%
}%
\newcommand{\HoloTaskModelHead}[2]{%
  \parbox[c][0.92cm][c]{#2}{%
    \centering\fontsize{5.50pt}{5.75pt}\selectfont\textbf{#1}%
  }%
}%
\begin{longtable}{|>{\columncolor{leftblue}\centering\arraybackslash}m{1.35cm}|>{\columncolor{leftblue}\centering\arraybackslash}m{2.05cm}|>{\columncolor{leftblue}\centering\arraybackslash}m{1.085cm}|>{\columncolor{leftblue}\centering\arraybackslash}m{1.085cm}|>{\centering\arraybackslash}m{1.72cm}|>{\centering\arraybackslash}m{1.72cm}|>{\centering\arraybackslash}m{1.72cm}|>{\centering\arraybackslash}m{1.72cm}|>{\centering\arraybackslash}m{1.72cm}|>{\centering\arraybackslash}m{1.72cm}|>{\centering\arraybackslash}m{1.72cm}|}
\caption[Detailed closed-ended VQA scores across benchmarks]{\textbf{Detailed closed-ended VQA performance of HoloCT and competing methods across internal benchmarks.}\newline Each score is reported as mean with 95\% confidence interval. Accu. denotes accuracy. For DeepTumorVQA, Recog., Meas., Vis.R., and Med.R. denote recognition, measurement, visual reasoning, and medical reasoning, respectively. For AMOS-MM-VQA, Anat.I., Attr.R., Quant.A., Dis.A., Risk.E., and Ther.S. denote anatomical identification, attribute recognition, quantitative assessment, disease analysis, risk evaluation, and therapeutic suggestion, respectively.}%
\label{tab:close_ended_vqa_scores}\\[-0.15ex]
\hline
\rowcolor{headerblue}
\HoloTaskSplitHead{Dataset}{Type}{1.35cm} & \HoloTaskSplitHead{Dataset}{Name}{2.05cm} & \multicolumn{2}{>{\columncolor{headerblue}\centering\arraybackslash}m{\dimexpr1.085cm+1.085cm+2\tabcolsep+\arrayrulewidth\relax}|}{\HoloTaskMidHead{Metric}{\dimexpr1.085cm+1.085cm+2\tabcolsep+\arrayrulewidth\relax}} & \HoloTaskModelHead{\makecell[c]{Qwen3-VL-\\[-0.18ex]32B}}{1.72cm} & \HoloTaskModelHead{\makecell[c]{MedGemma1.5-\\[-0.18ex]4B}}{1.72cm} & \HoloTaskModelHead{\makecell[c]{M3D-Phi3-\\[-0.18ex]4B}}{1.72cm} & \HoloTaskModelHead{\makecell[c]{RadFM-\\[-0.18ex]14B}}{1.72cm} & \HoloTaskModelHead{\makecell[c]{HuluMed-\\[-0.18ex]32B}}{1.72cm} & \HoloTaskModelHead{\makecell[c]{HoloCT-\\[-0.18ex]4B}}{1.72cm} & \HoloTaskModelHead{\makecell[c]{HoloCT-\\[-0.18ex]8B}}{1.72cm} \\
\hline
\endfirsthead
\caption*{\textbf{Supplementary Table~\ref{tab:close_ended_vqa_scores} (continued)\enspace|\enspace Detailed closed-ended VQA performance of HoloCT and competing methods across internal benchmarks.}\newline Each score is reported as mean with 95\% confidence interval. Accu. denotes accuracy. For DeepTumorVQA, Recog., Meas., Vis.R., and Med.R. denote recognition, measurement, visual reasoning, and medical reasoning, respectively. For AMOS-MM-VQA, Anat.I., Attr.R., Quant.A., Dis.A., Risk.E., and Ther.S. denote anatomical identification, attribute recognition, quantitative assessment, disease analysis, risk evaluation, and therapeutic suggestion, respectively.}\\[-0.15ex]
\hline
\rowcolor{headerblue}
\HoloTaskSplitHead{Dataset}{Type}{1.35cm} & \HoloTaskSplitHead{Dataset}{Name}{2.05cm} & \multicolumn{2}{>{\columncolor{headerblue}\centering\arraybackslash}m{\dimexpr1.085cm+1.085cm+2\tabcolsep+\arrayrulewidth\relax}|}{\HoloTaskMidHead{Metric}{\dimexpr1.085cm+1.085cm+2\tabcolsep+\arrayrulewidth\relax}} & \HoloTaskModelHead{\makecell[c]{Qwen3-VL-\\[-0.18ex]32B}}{1.72cm} & \HoloTaskModelHead{\makecell[c]{MedGemma1.5-\\[-0.18ex]4B}}{1.72cm} & \HoloTaskModelHead{\makecell[c]{M3D-Phi3-\\[-0.18ex]4B}}{1.72cm} & \HoloTaskModelHead{\makecell[c]{RadFM-\\[-0.18ex]14B}}{1.72cm} & \HoloTaskModelHead{\makecell[c]{HuluMed-\\[-0.18ex]32B}}{1.72cm} & \HoloTaskModelHead{\makecell[c]{HoloCT-\\[-0.18ex]4B}}{1.72cm} & \HoloTaskModelHead{\makecell[c]{HoloCT-\\[-0.18ex]8B}}{1.72cm} \\
\hline
\endhead
\endfoot
\endlastfoot
 & \HoloTaskRowSpan{\makecell[c]{CT-RATE-\\[-0.10ex]option}}{2.05cm} & \multicolumn{2}{>{\columncolor{leftblue}\centering\arraybackslash}m{\dimexpr1.085cm+1.085cm+2\tabcolsep+\arrayrulewidth\relax}|}{\HoloTaskMergedMetric{Accuracy}} & \HoloTaskScore{0.6732}{(0.6691--0.6867)}{4.35pt}{4.62pt} & \HoloTaskScore{0.6117}{(0.6029--0.6243)}{4.35pt}{4.62pt} & \HoloTaskScore{0.6892}{(0.6793--0.6988)}{4.35pt}{4.62pt} & \HoloTaskScore{0.3234}{(0.3168--0.3308)}{4.35pt}{4.62pt} & \HoloTaskScore{0.8473}{(0.8393--0.8545)}{4.35pt}{4.62pt} & \HoloTaskScore{0.9264}{(0.9202--0.9317)}{4.35pt}{4.62pt} & \HoloTaskScore{0.9343}{(0.9285--0.9395)}{4.35pt}{4.62pt} \\
\cline{2-11}
 & \HoloTaskRowSpan{\makecell[c]{FLARE-2025}}{2.05cm} & \multicolumn{2}{>{\columncolor{leftblue}\centering\arraybackslash}m{\dimexpr1.085cm+1.085cm+2\tabcolsep+\arrayrulewidth\relax}|}{\HoloTaskMergedMetric{Accuracy}} & \HoloTaskScore{0.5988}{(0.5887--0.6063)}{4.35pt}{4.62pt} & \HoloTaskScore{0.4944}{(0.4812--0.5057)}{4.35pt}{4.62pt} & \HoloTaskScore{0.5473}{(0.5342--0.5592)}{4.35pt}{4.62pt} & \HoloTaskScore{0.2767}{(0.2675--0.2863)}{4.35pt}{4.62pt} & \HoloTaskScore{0.7100}{(0.6990--0.7208)}{4.35pt}{4.62pt} & \HoloTaskScore{0.7630}{(0.7519--0.7725)}{4.35pt}{4.62pt} & \HoloTaskScore{0.7997}{(0.7900--0.8095)}{4.35pt}{4.62pt} \\
\cline{2-11}
 & \HoloTaskRowSpan{\makecell[c]{3D-RAD\\[-0.10ex]Existence}}{2.05cm} & \multicolumn{2}{>{\columncolor{leftblue}\centering\arraybackslash}m{\dimexpr1.085cm+1.085cm+2\tabcolsep+\arrayrulewidth\relax}|}{\HoloTaskMergedMetric{Accuracy}} & \HoloTaskScore{0.6128}{(0.6086--0.6299)}{4.35pt}{4.62pt} & \HoloTaskScore{0.6874}{(0.6781--0.6938)}{4.35pt}{4.62pt} & \HoloTaskScore{0.4086}{(0.3902--0.4269)}{4.35pt}{4.62pt} & \HoloTaskScore{0.3098}{(0.2865--0.3184)}{4.35pt}{4.62pt} & \HoloTaskScore{0.8226}{(0.8117--0.8396)}{4.35pt}{4.62pt} & \HoloTaskScore{0.8662}{(0.8619--0.8705)}{4.35pt}{4.62pt} & \HoloTaskScore{0.8588}{(0.8544--0.8631)}{4.35pt}{4.62pt} \\
\cline{2-11}
 & \HoloTaskRowSpan{\makecell[c]{3D-RAD\\[-0.10ex]Static.}}{2.05cm} & \multicolumn{2}{>{\columncolor{leftblue}\centering\arraybackslash}m{\dimexpr1.085cm+1.085cm+2\tabcolsep+\arrayrulewidth\relax}|}{\HoloTaskMergedMetric{Accuracy}} & \HoloTaskScore{0.2039}{(0.1803--0.2252)}{4.35pt}{4.62pt} & \HoloTaskScore{0.3805}{(0.3651--0.4026)}{4.35pt}{4.62pt} & \HoloTaskScore{0.2551}{(0.2426--0.2620)}{4.35pt}{4.62pt} & \HoloTaskScore{0.4331}{(0.4323--0.4692)}{4.35pt}{4.62pt} & \HoloTaskScore{0.6549}{(0.6354--0.6737)}{4.35pt}{4.62pt} & \HoloTaskScore{0.6947}{(0.6780--0.7111)}{4.35pt}{4.62pt} & \HoloTaskScore{0.6519}{(0.6345--0.6686)}{4.35pt}{4.62pt} \\
\cline{2-11}
 & \HoloTaskRowSpan{\makecell[c]{3D-RAD\\[-0.10ex]Longitudinal.}}{2.05cm} & \multicolumn{2}{>{\columncolor{leftblue}\centering\arraybackslash}m{\dimexpr1.085cm+1.085cm+2\tabcolsep+\arrayrulewidth\relax}|}{\HoloTaskMergedMetric{Accuracy}} & \HoloTaskScore{0.4416}{(0.4293--0.4662)}{4.35pt}{4.62pt} & \HoloTaskScore{0.4287}{(0.4060--0.4616)}{4.35pt}{4.62pt} & \HoloTaskScore{0.2440}{(0.2267--0.2744)}{4.35pt}{4.62pt} & \HoloTaskScore{0.4390}{(0.4014--0.4617)}{4.35pt}{4.62pt} & \HoloTaskScore{0.8193}{(0.7931--0.8304)}{4.35pt}{4.62pt} & \HoloTaskScore{0.8493}{(0.8364--0.8629)}{4.35pt}{4.62pt} & \HoloTaskScore{0.8441}{(0.8312--0.8583)}{4.35pt}{4.62pt} \\
\cline{2-11}
 &  & \HoloTaskRowSpan{\makecell[c]{\textbf{Anat.I.}}}{1.085cm} & \HoloTaskMetric{Accu.} & \HoloTaskScore{0.4348}{(0.3876--0.4740)}{4.35pt}{4.62pt} & \HoloTaskScore{0.3832}{(0.3205--0.4373)}{4.35pt}{4.62pt} & \HoloTaskScore{0.4846}{(0.4415--0.5298)}{4.35pt}{4.62pt} & \HoloTaskScore{0.3478}{(0.3150--0.3786)}{4.35pt}{4.62pt} & \HoloTaskScore{0.7269}{(0.6879--0.7639)}{4.35pt}{4.62pt} & \HoloTaskScore{0.6923}{(0.5577--0.8077)}{4.35pt}{4.62pt} & \HoloTaskScore{0.7692}{(0.6538--0.8846)}{4.35pt}{4.62pt} \\*
\cline{3-11}
 &  & \HoloTaskRowSpan{\makecell[c]{\textbf{Attr.R.}}}{1.085cm} & \HoloTaskMetric{Accu.} & \HoloTaskScore{0.4951}{(0.4546--0.5332)}{4.35pt}{4.62pt} & \HoloTaskScore{0.4458}{(0.3940--0.4804)}{4.35pt}{4.62pt} & \HoloTaskScore{0.5745}{(0.5350--0.6158)}{4.35pt}{4.62pt} & \HoloTaskScore{0.4077}{(0.3808--0.4329)}{4.35pt}{4.62pt} & \HoloTaskScore{0.8600}{(0.8312--0.8887)}{4.35pt}{4.62pt} & \HoloTaskScore{0.9286}{(0.8333--1.000)}{4.35pt}{4.62pt} & \HoloTaskScore{1.000}{(1.000--1.000)}{4.35pt}{4.62pt} \\*
\cline{3-11}
\HoloTaskSpan{\makecell[c]{\textbf{Internal}}}{1.35cm}{0pt} &  & \HoloTaskRowSpan{\makecell[c]{\textbf{Quant.A.}}}{1.085cm} & \HoloTaskMetric{Accu.} & \HoloTaskScore{0.3777}{(0.3189--0.4260)}{4.35pt}{4.62pt} & \HoloTaskScore{0.3231}{(0.2540--0.3830)}{4.35pt}{4.62pt} & \HoloTaskScore{0.4711}{(0.4309--0.5113)}{4.35pt}{4.62pt} & \HoloTaskScore{0.4479}{(0.4206--0.4753)}{4.35pt}{4.62pt} & \HoloTaskScore{0.7492}{(0.7154--0.7830)}{4.35pt}{4.62pt} & \HoloTaskScore{0.7097}{(0.5968--0.8226)}{4.35pt}{4.62pt} & \HoloTaskScore{0.9032}{(0.8226--0.9677)}{4.35pt}{4.62pt} \\*
\cline{3-11}
 & \HoloTaskSpan{\makecell[c]{AMOS-MM-VQA}}{2.05cm}{0.32cm} & \HoloTaskRowSpan{\makecell[c]{\textbf{Dis.A.}}}{1.085cm} & \HoloTaskMetric{Accu.} & \HoloTaskScore{0.4062}{(0.3560--0.4692)}{4.35pt}{4.62pt} & \HoloTaskScore{0.3530}{(0.2905--0.4121)}{4.35pt}{4.62pt} & \HoloTaskScore{0.4920}{(0.4462--0.5424)}{4.35pt}{4.62pt} & \HoloTaskScore{0.4053}{(0.3755--0.4328)}{4.35pt}{4.62pt} & \HoloTaskScore{0.7506}{(0.7071--0.7918)}{4.35pt}{4.62pt} & \HoloTaskScore{0.8056}{(0.6944--0.9167)}{4.35pt}{4.62pt} & \HoloTaskScore{0.9167}{(0.8056--1.000)}{4.35pt}{4.62pt} \\*
\cline{3-11}
 &  & \HoloTaskRowSpan{\makecell[c]{\textbf{Risk.E.}}}{1.085cm} & \HoloTaskMetric{Accu.} & \HoloTaskScore{0.3447}{(0.2828--0.3949)}{4.35pt}{4.62pt} & \HoloTaskScore{0.3957}{(0.3277--0.4542)}{4.35pt}{4.62pt} & \HoloTaskScore{0.4537}{(0.4073--0.5000)}{4.35pt}{4.62pt} & \HoloTaskScore{0.4024}{(0.3707--0.4341)}{4.35pt}{4.62pt} & \HoloTaskScore{0.7195}{(0.6805--0.7610)}{4.35pt}{4.62pt} & \HoloTaskScore{0.7561}{(0.6341--0.8780)}{4.35pt}{4.62pt} & \HoloTaskScore{0.8780}{(0.7561--0.9756)}{4.35pt}{4.62pt} \\*
\cline{3-11}
 &  & \HoloTaskRowSpan{\makecell[c]{\textbf{Ther.S.}}}{1.085cm} & \HoloTaskMetric{Accu.} & \HoloTaskScore{0.3851}{(0.3223--0.4321)}{4.35pt}{4.62pt} & \HoloTaskScore{0.4491}{(0.3786--0.5062)}{4.35pt}{4.62pt} & \HoloTaskScore{0.4124}{(0.3503--0.4708)}{4.35pt}{4.62pt} & \HoloTaskScore{0.3511}{(0.3168--0.3803)}{4.35pt}{4.62pt} & \HoloTaskScore{0.8212}{(0.7737--0.8650)}{4.35pt}{4.62pt} & \HoloTaskScore{0.6333}{(0.4667--0.8000)}{4.35pt}{4.62pt} & \HoloTaskScore{0.7333}{(0.5667--0.8667)}{4.35pt}{4.62pt} \\
\cline{2-11}
 &  & \HoloTaskRowSpan{\makecell[c]{\textbf{Recog.}}}{1.085cm} & \HoloTaskMetric{Accu.} & \HoloTaskScore{0.4557}{(0.4365--0.4785)}{4.35pt}{4.62pt} & \HoloTaskScore{0.4025}{(0.3858--0.4247)}{4.35pt}{4.62pt} & \HoloTaskScore{0.4205}{(0.3996--0.4404)}{4.35pt}{4.62pt} & \HoloTaskScore{0.4309}{(0.4098--0.4541)}{4.35pt}{4.62pt} & \HoloTaskScore{0.5522}{(0.5304--0.5734)}{4.35pt}{4.62pt} & \HoloTaskScore{0.7121}{(0.6800--0.7409)}{4.35pt}{4.62pt} & \HoloTaskScore{0.8128}{(0.7852--0.8394)}{4.35pt}{4.62pt} \\*
\cline{3-11}
 &  & \HoloTaskRowSpan{\makecell[c]{\textbf{Meas.}}}{1.085cm} & \HoloTaskMetric{Accu.} & \HoloTaskScore{0.2041}{(0.1841--0.2280)}{4.35pt}{4.62pt} & \HoloTaskScore{0.1853}{(0.1683--0.2038)}{4.35pt}{4.62pt} & \HoloTaskScore{0.1706}{(0.1547--0.1874)}{4.35pt}{4.62pt} & \HoloTaskScore{0.2148}{(0.1963--0.2344)}{4.35pt}{4.62pt} & \HoloTaskScore{0.2951}{(0.2748--0.3159)}{4.35pt}{4.62pt} & \HoloTaskScore{0.5686}{(0.5421--0.5967)}{4.35pt}{4.62pt} & \HoloTaskScore{0.5934}{(0.5653--0.6215)}{4.35pt}{4.62pt} \\*
\cline{3-11}
 & \HoloTaskSpan{\makecell[c]{DeepTumorVQA}}{2.05cm}{0.32cm} & \HoloTaskRowSpan{\makecell[c]{\textbf{Vis.R.}}}{1.085cm} & \HoloTaskMetric{Accu.} & \HoloTaskScore{0.3191}{(0.2993--0.3211)}{4.35pt}{4.62pt} & \HoloTaskScore{0.2806}{(0.2732--0.3028)}{4.35pt}{4.62pt} & \HoloTaskScore{0.2907}{(0.2768--0.3036)}{4.35pt}{4.62pt} & \HoloTaskScore{0.2621}{(0.2479--0.2768)}{4.35pt}{4.62pt} & \HoloTaskScore{0.4149}{(0.3999--0.4302)}{4.35pt}{4.62pt} & \HoloTaskScore{0.5812}{(0.5610--0.6022)}{4.35pt}{4.62pt} & \HoloTaskScore{0.5944}{(0.5738--0.6155)}{4.35pt}{4.62pt} \\*
\cline{3-11}
 &  & \HoloTaskRowSpan{\makecell[c]{\textbf{Med.R.}}}{1.085cm} & \HoloTaskMetric{Accu.} & \HoloTaskScore{0.2715}{(0.2522--0.2980)}{4.35pt}{4.62pt} & \HoloTaskScore{0.2448}{(0.2266--0.2620)}{4.35pt}{4.62pt} & \HoloTaskScore{0.2583}{(0.2378--0.2772)}{4.35pt}{4.62pt} & \HoloTaskScore{0.2032}{(0.1849--0.2222)}{4.35pt}{4.62pt} & \HoloTaskScore{0.3318}{(0.3108--0.3528)}{4.35pt}{4.62pt} & \HoloTaskScore{0.6168}{(0.5888--0.6431)}{4.35pt}{4.62pt} & \HoloTaskScore{0.6752}{(0.6480--0.7015)}{4.35pt}{4.62pt} \\
\hline
\end{longtable}
\arrayrulecolor{black}
\endgroup
