# Supplementary material for: A 3D foundation model unifying CT interpretation and segmentation
Source: arXiv:2611.06471 source file (2026-11-04)
Supplement: Supplementary file 13 [file table5_open_ended_vqa.tex]

\begingroup
\makeatletter
\@ifundefined{color@leftblue}{\definecolor{leftblue}{RGB}{232,242,248}}{}%
\@ifundefined{color@headerblue}{\definecolor{headerblue}{RGB}{218,233,242}}{}%
\makeatother
\setlength{\LTcapwidth}{18.60cm}
\setlength{\LTleft}{\fill}
\setlength{\LTright}{\fill}
\setlength{\LTpre}{0pt}
\setlength{\LTpost}{0pt}
\setlength{\tabcolsep}{0.45pt}
\renewcommand{\arraystretch}{1.00}
\setlength{\extrarowheight}{0pt}
\setlength{\arrayrulewidth}{0.48pt}
\arrayrulecolor{black}
\providecommand{\softcline}[1]{}%
\renewcommand{\softcline}[1]{\arrayrulecolor{black!35}\cline{#1}\arrayrulecolor{black}}
\sloppy
\emergencystretch=2em
\fontsize{5.15pt}{5.75pt}\selectfont
\newcommand{\HoloTaskScore}[4]{%
  \parbox[c][0.64cm][c]{1.70cm}{%
    \centering
    {\fontsize{5.15pt}{5.43pt}\selectfont\strut\mbox{#1}}\\[-0.38ex]%
    {\fontsize{#3}{#4}\selectfont\strut\mbox{#2}}%
  }%
}%
\newcommand{\HoloTaskMetricGroup}[1]{%
  \parbox[c][0.64cm][c]{1.045cm}{%
    \centering\fontsize{4.35pt}{4.65pt}\selectfont\textbf{\mbox{#1}}%
  }%
}%
\newcommand{\HoloTaskMetric}[1]{%
  \parbox[c][0.64cm][c]{1.045cm}{%
    \centering\fontsize{4.35pt}{4.65pt}\selectfont\textbf{#1}%
  }%
}%
\newcommand{\HoloTaskMergedMetric}[1]{%
  \parbox[c][0.64cm][c]{2.13cm}{%
    \centering\fontsize{4.35pt}{4.65pt}\selectfont\textbf{\mbox{#1}}%
  }%
}%
\newcommand{\HoloTaskRowSpan}[2]{%
  \parbox[c][0.64cm][c]{#2}{%
    \centering\arraybackslash #1%
  }%
}%
\newcommand{\HoloTaskSpan}[3]{%
  \raisebox{\dimexpr#3-0.11cm\relax}[0pt][0pt]{%
    \parbox[c][0.64cm][c]{#2}{%
      \centering\arraybackslash #1%
    }%
  }%
}%
\newcommand{\HoloTaskSplitHead}[3]{%
  \parbox[c][0.92cm][c]{#3}{%
    \centering\fontsize{6.05pt}{6.30pt}\selectfont\textbf{#1}\\[-0.52ex]%
    \rule{0pt}{0.58ex}\\[-0.52ex]\textbf{#2}%
  }%
}%
\newcommand{\HoloTaskMidHead}[2]{%
  \parbox[c][0.92cm][c]{#2}{%
    \centering\fontsize{6.05pt}{6.30pt}\selectfont\textbf{#1}%
  }%
}%
\newcommand{\HoloTaskModelHead}[2]{%
  \parbox[c][0.92cm][c]{#2}{%
    \centering\fontsize{5.50pt}{5.75pt}\selectfont\textbf{#1}%
  }%
}%
\begin{longtable}{|>{\columncolor{leftblue}\centering\arraybackslash}m{1.35cm}|>{\columncolor{leftblue}\centering\arraybackslash}m{2.05cm}|>{\columncolor{leftblue}\centering\arraybackslash}m{1.085cm}|>{\columncolor{leftblue}\centering\arraybackslash}m{1.085cm}|>{\centering\arraybackslash}m{1.72cm}|>{\centering\arraybackslash}m{1.72cm}|>{\centering\arraybackslash}m{1.72cm}|>{\centering\arraybackslash}m{1.72cm}|>{\centering\arraybackslash}m{1.72cm}|>{\centering\arraybackslash}m{1.72cm}|>{\centering\arraybackslash}m{1.72cm}|}
\caption[Detailed open-ended VQA scores across benchmarks]{\textbf{Detailed open-ended VQA performance of HoloCT and competing methods on internal and external benchmarks.}\newline Each score is reported as mean with 95\% confidence interval. NLP metrics include BLEU-4, ROUGE-L, and METEOR; the clinical metric is LlamaScore.}%
\label{tab:open_ended_vqa_scores}\\[-0.15ex]
\hline
\rowcolor{headerblue}
\HoloTaskSplitHead{Dataset}{Type}{1.35cm} & \HoloTaskSplitHead{Dataset}{Name}{2.05cm} & \multicolumn{2}{>{\columncolor{headerblue}\centering\arraybackslash}m{\dimexpr1.085cm+1.085cm+2\tabcolsep+\arrayrulewidth\relax}|}{\HoloTaskMidHead{Metric}{\dimexpr1.085cm+1.085cm+2\tabcolsep+\arrayrulewidth\relax}} & \HoloTaskModelHead{\makecell[c]{Qwen3-VL-\\[-0.18ex]32B}}{1.72cm} & \HoloTaskModelHead{\makecell[c]{MedGemma1.5-\\[-0.18ex]4B}}{1.72cm} & \HoloTaskModelHead{\makecell[c]{M3D-Phi3-\\[-0.18ex]4B}}{1.72cm} & \HoloTaskModelHead{\makecell[c]{RadFM-\\[-0.18ex]14B}}{1.72cm} & \HoloTaskModelHead{\makecell[c]{HuluMed-\\[-0.18ex]32B}}{1.72cm} & \HoloTaskModelHead{\makecell[c]{HoloCT-\\[-0.18ex]4B}}{1.72cm} & \HoloTaskModelHead{\makecell[c]{HoloCT-\\[-0.18ex]8B}}{1.72cm} \\
\hline
\endfirsthead
\caption*{\textbf{Supplementary Table~\ref{tab:open_ended_vqa_scores} (continued)\enspace|\enspace Detailed open-ended VQA performance of HoloCT and competing methods on internal and external benchmarks.}\newline Each score is reported as mean with 95\% confidence interval. NLP metrics include BLEU-4, ROUGE-L, and METEOR; the clinical metric is LlamaScore.}\\[-0.15ex]
\hline
\rowcolor{headerblue}
\HoloTaskSplitHead{Dataset}{Type}{1.35cm} & \HoloTaskSplitHead{Dataset}{Name}{2.05cm} & \multicolumn{2}{>{\columncolor{headerblue}\centering\arraybackslash}m{\dimexpr1.085cm+1.085cm+2\tabcolsep+\arrayrulewidth\relax}|}{\HoloTaskMidHead{Metric}{\dimexpr1.085cm+1.085cm+2\tabcolsep+\arrayrulewidth\relax}} & \HoloTaskModelHead{\makecell[c]{Qwen3-VL-\\[-0.18ex]32B}}{1.72cm} & \HoloTaskModelHead{\makecell[c]{MedGemma1.5-\\[-0.18ex]4B}}{1.72cm} & \HoloTaskModelHead{\makecell[c]{M3D-Phi3-\\[-0.18ex]4B}}{1.72cm} & \HoloTaskModelHead{\makecell[c]{RadFM-\\[-0.18ex]14B}}{1.72cm} & \HoloTaskModelHead{\makecell[c]{HuluMed-\\[-0.18ex]32B}}{1.72cm} & \HoloTaskModelHead{\makecell[c]{HoloCT-\\[-0.18ex]4B}}{1.72cm} & \HoloTaskModelHead{\makecell[c]{HoloCT-\\[-0.18ex]8B}}{1.72cm} \\
\hline
\endhead
\endfoot
\endlastfoot
 &  &  & \HoloTaskMetric{\makecell[c]{\mbox{BLEU-4}}} & \HoloTaskScore{0.3328}{(0.3255--0.3489)}{4.35pt}{4.62pt} & \HoloTaskScore{0.2093}{(0.1945--0.2181)}{4.35pt}{4.62pt} & \HoloTaskScore{0.09760}{(0.09634--0.09893)}{4.02pt}{4.28pt} & \HoloTaskScore{0.2799}{(0.2780--0.2820)}{4.35pt}{4.62pt} & \HoloTaskScore{0.3886}{(0.3863--0.3908)}{4.35pt}{4.62pt} & \HoloTaskScore{0.4928}{(0.4904--0.4953)}{4.35pt}{4.62pt} & \HoloTaskScore{0.4917}{(0.4892--0.4941)}{4.35pt}{4.62pt} \\*
\softcline{4-11}
 &  & \HoloTaskSpan{{\fontsize{4.35pt}{4.65pt}\selectfont \makecell[c]{\textbf{NLP}}}}{1.085cm}{0pt} & \HoloTaskMetric{\makecell[c]{\mbox{ROUGE-L}}} & \HoloTaskScore{0.3534}{(0.3444--0.3692)}{4.35pt}{4.62pt} & \HoloTaskScore{0.2257}{(0.2117--0.2339)}{4.35pt}{4.62pt} & \HoloTaskScore{0.1315}{(0.1303--0.1328)}{4.35pt}{4.62pt} & \HoloTaskScore{0.2742}{(0.2724--0.2761)}{4.35pt}{4.62pt} & \HoloTaskScore{0.4122}{(0.4102--0.4143)}{4.35pt}{4.62pt} & \HoloTaskScore{0.5007}{(0.4982--0.5032)}{4.35pt}{4.62pt} & \HoloTaskScore{0.4952}{(0.4926--0.4978)}{4.35pt}{4.62pt} \\*
\softcline{4-11}
 & \HoloTaskSpan{\makecell[c]{CT-RATE-\\[-0.10ex]long}}{2.05cm}{0.32cm} &  & \HoloTaskMetric{\makecell[c]{\mbox{METEOR}}} & \HoloTaskScore{0.3682}{(0.3566--0.3762)}{4.35pt}{4.62pt} & \HoloTaskScore{0.1927}{(0.1820--0.2881)}{4.35pt}{4.62pt} & \HoloTaskScore{0.08947}{(0.08840--0.09045)}{4.02pt}{4.28pt} & \HoloTaskScore{0.2803}{(0.2782--0.2824)}{4.35pt}{4.62pt} & \HoloTaskScore{0.4293}{(0.4271--0.4316)}{4.35pt}{4.62pt} & \HoloTaskScore{0.5199}{(0.5169--0.5227)}{4.35pt}{4.62pt} & \HoloTaskScore{0.5208}{(0.5181--0.5237)}{4.35pt}{4.62pt} \\*
\cline{3-11}
 &  & \HoloTaskRowSpan{{\fontsize{4.35pt}{4.65pt}\selectfont \makecell[c]{\textbf{Clinical}}}}{1.085cm} & \HoloTaskMetric{\makecell[c]{\mbox{Llama}\\[-0.10ex]\mbox{Score}}} & \HoloTaskScore{6.089}{(6.054--6.116)}{4.35pt}{4.62pt} & \HoloTaskScore{5.127}{(5.095--5.152)}{4.35pt}{4.62pt} & \HoloTaskScore{4.920}{(4.898--4.944)}{4.35pt}{4.62pt} & \HoloTaskScore{5.427}{(5.401--5.452)}{4.35pt}{4.62pt} & \HoloTaskScore{6.873}{(6.852--6.895)}{4.35pt}{4.62pt} & \HoloTaskScore{7.544}{(7.525--7.560)}{4.35pt}{4.62pt} & \HoloTaskScore{7.583}{(7.565--7.601)}{4.35pt}{4.62pt} \\
\cline{2-11}
 &  &  & \HoloTaskMetric{\makecell[c]{\mbox{BLEU-4}}} & \HoloTaskScore{0.1528}{(0.1441--0.1691)}{4.35pt}{4.62pt} & \HoloTaskScore{0.1272}{(0.1121--0.1332)}{4.35pt}{4.62pt} & \HoloTaskScore{0.1637}{(0.1593--0.1677)}{4.35pt}{4.62pt} & \HoloTaskScore{0.09063}{(0.08879--0.09251)}{4.02pt}{4.28pt} & \HoloTaskScore{0.07747}{(0.07611--0.07882)}{4.02pt}{4.28pt} & \HoloTaskScore{0.5991}{(0.5925--0.6055)}{4.35pt}{4.62pt} & \HoloTaskScore{0.5964}{(0.5896--0.6029)}{4.35pt}{4.62pt} \\*
\softcline{4-11}
 &  & \HoloTaskSpan{{\fontsize{4.35pt}{4.65pt}\selectfont \makecell[c]{\textbf{NLP}}}}{1.085cm}{0pt} & \HoloTaskMetric{\makecell[c]{\mbox{ROUGE-L}}} & \HoloTaskScore{0.1949}{(0.1885--0.2358)}{4.35pt}{4.62pt} & \HoloTaskScore{0.1391}{(0.1226--0.1479)}{4.35pt}{4.62pt} & \HoloTaskScore{0.2165}{(0.2064--0.2263)}{4.35pt}{4.62pt} & \HoloTaskScore{0.08163}{(0.07888--0.08467)}{4.02pt}{4.28pt} & \HoloTaskScore{0.1080}{(0.1060--0.1100)}{4.35pt}{4.62pt} & \HoloTaskScore{0.5961}{(0.5893--0.6030)}{4.35pt}{4.62pt} & \HoloTaskScore{0.5940}{(0.5866--0.6012)}{4.35pt}{4.62pt} \\*
\softcline{4-11}
 & \HoloTaskSpan{\makecell[c]{CT-RATE-\\[-0.10ex]short}}{2.05cm}{0.32cm} &  & \HoloTaskMetric{\makecell[c]{\mbox{METEOR}}} & \HoloTaskScore{0.1514}{(0.1462--0.1683)}{4.35pt}{4.62pt} & \HoloTaskScore{0.1252}{(0.1126--0.1375)}{4.35pt}{4.62pt} & \HoloTaskScore{0.09350}{(0.08951--0.09728)}{4.02pt}{4.28pt} & \HoloTaskScore{0.1012}{(0.09870--0.1036)}{4.02pt}{4.28pt} & \HoloTaskScore{0.1667}{(0.1639--0.1698)}{4.35pt}{4.62pt} & \HoloTaskScore{0.5108}{(0.5043--0.5171)}{4.35pt}{4.62pt} & \HoloTaskScore{0.4981}{(0.4916--0.5044)}{4.35pt}{4.62pt} \\*
\cline{3-11}
 &  & \HoloTaskRowSpan{{\fontsize{4.35pt}{4.65pt}\selectfont \makecell[c]{\textbf{Clinical}}}}{1.085cm} & \HoloTaskMetric{\makecell[c]{\mbox{Llama}\\[-0.10ex]\mbox{Score}}} & \HoloTaskScore{5.248}{(5.196--5.339)}{4.35pt}{4.62pt} & \HoloTaskScore{4.686}{(4.625--4.748)}{4.35pt}{4.62pt} & \HoloTaskScore{4.346}{(4.249--4.445)}{4.35pt}{4.62pt} & \HoloTaskScore{4.518}{(4.465--4.570)}{4.35pt}{4.62pt} & \HoloTaskScore{5.919}{(5.864--5.971)}{4.35pt}{4.62pt} & \HoloTaskScore{7.399}{(7.348--7.449)}{4.35pt}{4.62pt} & \HoloTaskScore{7.442}{(7.390--7.492)}{4.35pt}{4.62pt} \\
\cline{2-11}
 &  &  & \HoloTaskMetric{\makecell[c]{\mbox{BLEU-4}}} & \HoloTaskScore{0.08660}{(0.06120--0.1018)}{4.02pt}{4.28pt} & \HoloTaskScore{0.1047}{(0.08640--0.1213)}{4.02pt}{4.28pt} & \HoloTaskScore{0.1672}{(0.1489--0.1717)}{4.35pt}{4.62pt} & \HoloTaskScore{0.1239}{(0.09490--0.1343)}{4.02pt}{4.28pt} & \HoloTaskScore{0.2952}{(0.2646--0.3224)}{4.35pt}{4.62pt} & \HoloTaskScore{0.5280}{(0.5019--0.5549)}{4.35pt}{4.62pt} & \HoloTaskScore{0.4967}{(0.4639--0.5286)}{4.35pt}{4.62pt} \\*
\softcline{4-11}
 &  & \HoloTaskSpan{{\fontsize{4.35pt}{4.65pt}\selectfont \makecell[c]{\textbf{NLP}}}}{1.085cm}{0pt} & \HoloTaskMetric{\makecell[c]{\mbox{ROUGE-L}}} & \HoloTaskScore{0.1411}{(0.1259--0.1626)}{4.35pt}{4.62pt} & \HoloTaskScore{0.1660}{(0.1422--0.1861)}{4.35pt}{4.62pt} & \HoloTaskScore{0.2330}{(0.2109--0.2555)}{4.35pt}{4.62pt} & \HoloTaskScore{0.1859}{(0.1709--0.2056)}{4.35pt}{4.62pt} & \HoloTaskScore{0.4181}{(0.3836--0.4343)}{4.35pt}{4.62pt} & \HoloTaskScore{0.6214}{(0.5977--0.6446)}{4.35pt}{4.62pt} & \HoloTaskScore{0.6206}{(0.5961--0.6445)}{4.35pt}{4.62pt} \\*
\softcline{4-11}
\HoloTaskSpan{\makecell[c]{\textbf{Internal}}}{1.35cm}{0.32cm} & \HoloTaskSpan{\makecell[c]{3D-RAD\\[-0.10ex]Anomaly\\[-0.10ex]Detection}}{2.05cm}{0.32cm} &  & \HoloTaskMetric{\makecell[c]{\mbox{METEOR}}} & \HoloTaskScore{0.1110}{(0.09920--0.1386)}{4.02pt}{4.28pt} & \HoloTaskScore{0.1309}{(0.1170--0.1560)}{4.35pt}{4.62pt} & \HoloTaskScore{0.2033}{(0.1894--0.2213)}{4.35pt}{4.62pt} & \HoloTaskScore{0.1551}{(0.1368--0.1629)}{4.35pt}{4.62pt} & \HoloTaskScore{0.3595}{(0.3285--0.3881)}{4.35pt}{4.62pt} & \HoloTaskScore{0.5879}{(0.5657--0.6080)}{4.35pt}{4.62pt} & \HoloTaskScore{0.5748}{(0.5514--0.5955)}{4.35pt}{4.62pt} \\*
\cline{3-11}
 &  & \HoloTaskRowSpan{{\fontsize{4.35pt}{4.65pt}\selectfont \makecell[c]{\textbf{Clinical}}}}{1.085cm} & \HoloTaskMetric{\makecell[c]{\mbox{Llama}\\[-0.10ex]\mbox{Score}}} & \HoloTaskScore{4.984}{(4.770--5.175)}{4.35pt}{4.62pt} & \HoloTaskScore{5.116}{(4.914--5.320)}{4.35pt}{4.62pt} & \HoloTaskScore{5.513}{(5.336--5.689)}{4.35pt}{4.62pt} & \HoloTaskScore{5.238}{(5.049--5.434)}{4.35pt}{4.62pt} & \HoloTaskScore{6.448}{(6.258--6.641)}{4.35pt}{4.62pt} & \HoloTaskScore{7.746}{(7.570--7.918)}{4.35pt}{4.62pt} & \HoloTaskScore{8.016}{(7.853--8.166)}{4.35pt}{4.62pt} \\
\cline{2-11}
 &  &  & \HoloTaskMetric{\makecell[c]{\mbox{BLEU-4}}} & \HoloTaskScore{0.1069}{(0.08650--0.1239)}{4.02pt}{4.28pt} & \HoloTaskScore{0.1256}{(0.1037--0.1472)}{4.35pt}{4.62pt} & \HoloTaskScore{0.1667}{(0.1493--0.1810)}{4.35pt}{4.62pt} & \HoloTaskScore{0.1391}{(0.1260--0.1539)}{4.35pt}{4.62pt} & \HoloTaskScore{0.2716}{(0.2562--0.3041)}{4.35pt}{4.62pt} & \HoloTaskScore{0.5209}{(0.5011--0.5398)}{4.35pt}{4.62pt} & \HoloTaskScore{0.5159}{(0.4954--0.5360)}{4.35pt}{4.62pt} \\*
\softcline{4-11}
 &  & \HoloTaskSpan{{\fontsize{4.35pt}{4.65pt}\selectfont \makecell[c]{\textbf{NLP}}}}{1.085cm}{0pt} & \HoloTaskMetric{\makecell[c]{\mbox{ROUGE-L}}} & \HoloTaskScore{0.1673}{(0.1451--0.1812)}{4.35pt}{4.62pt} & \HoloTaskScore{0.1859}{(0.1606--0.2025)}{4.35pt}{4.62pt} & \HoloTaskScore{0.2477}{(0.2225--0.2518)}{4.35pt}{4.62pt} & \HoloTaskScore{0.2054}{(0.1839--0.2106)}{4.35pt}{4.62pt} & \HoloTaskScore{0.4026}{(0.3864--0.4251)}{4.35pt}{4.62pt} & \HoloTaskScore{0.6126}{(0.5976--0.6264)}{4.35pt}{4.62pt} & \HoloTaskScore{0.6168}{(0.6020--0.6305)}{4.35pt}{4.62pt} \\*
\softcline{4-11}
 & \HoloTaskSpan{\makecell[c]{3D-RAD\\[-0.10ex]Image\\[-0.10ex]Observation}}{2.05cm}{0.32cm} &  & \HoloTaskMetric{\makecell[c]{\mbox{METEOR}}} & \HoloTaskScore{0.1341}{(0.1140--0.1513)}{4.35pt}{4.62pt} & \HoloTaskScore{0.1546}{(0.1360--0.1760)}{4.35pt}{4.62pt} & \HoloTaskScore{0.2038}{(0.1811--0.2209)}{4.35pt}{4.62pt} & \HoloTaskScore{0.1608}{(0.1415--0.1802)}{4.35pt}{4.62pt} & \HoloTaskScore{0.3439}{(0.3217--0.3672)}{4.35pt}{4.62pt} & \HoloTaskScore{0.5731}{(0.5593--0.5867)}{4.35pt}{4.62pt} & \HoloTaskScore{0.5734}{(0.5589--0.5868)}{4.35pt}{4.62pt} \\*
\cline{3-11}
 &  & \HoloTaskRowSpan{{\fontsize{4.35pt}{4.65pt}\selectfont \makecell[c]{\textbf{Clinical}}}}{1.085cm} & \HoloTaskMetric{\makecell[c]{\mbox{Llama}\\[-0.10ex]\mbox{Score}}} & \HoloTaskScore{4.941}{(4.804--5.077)}{4.35pt}{4.62pt} & \HoloTaskScore{5.064}{(4.936--5.201)}{4.35pt}{4.62pt} & \HoloTaskScore{5.376}{(5.254--5.498)}{4.35pt}{4.62pt} & \HoloTaskScore{5.143}{(5.017--5.266)}{4.35pt}{4.62pt} & \HoloTaskScore{6.200}{(6.069--6.327)}{4.35pt}{4.62pt} & \HoloTaskScore{7.449}{(7.341--7.560)}{4.35pt}{4.62pt} & \HoloTaskScore{7.791}{(7.681--7.887)}{4.35pt}{4.62pt} \\
\cline{2-11}
 &  &  & \HoloTaskMetric{\makecell[c]{\mbox{BLEU-4}}} & \HoloTaskScore{0.07190}{(0.05720--0.09230)}{4.02pt}{4.28pt} & \HoloTaskScore{0.1011}{(0.08330--0.1325)}{4.02pt}{4.28pt} & \HoloTaskScore{0.03370}{(0.01180--0.04810)}{4.02pt}{4.28pt} & \HoloTaskScore{0.04690}{(0.03950--0.05250)}{4.02pt}{4.28pt} & \HoloTaskScore{0.3991}{(0.3551--0.4335)}{4.35pt}{4.62pt} & \HoloTaskScore{0.2171}{(0.1933--0.2411)}{4.35pt}{4.62pt} & \HoloTaskScore{0.1724}{(0.1561--0.1918)}{4.35pt}{4.62pt} \\*
\softcline{4-11}
 &  & \HoloTaskSpan{{\fontsize{4.35pt}{4.65pt}\selectfont \makecell[c]{\textbf{NLP}}}}{1.085cm}{0pt} & \HoloTaskMetric{\makecell[c]{\mbox{ROUGE-L}}} & \HoloTaskScore{0.1050}{(0.08920--0.1346)}{4.02pt}{4.28pt} & \HoloTaskScore{0.1575}{(0.1323--0.1839)}{4.35pt}{4.62pt} & \HoloTaskScore{0.05810}{(0.04280--0.07380)}{4.02pt}{4.28pt} & \HoloTaskScore{0.06930}{(0.06420--0.07460)}{4.02pt}{4.28pt} & \HoloTaskScore{0.4099}{(0.3772--0.4361)}{4.35pt}{4.62pt} & \HoloTaskScore{0.6256}{(0.6033--0.6466)}{4.35pt}{4.62pt} & \HoloTaskScore{0.6414}{(0.6196--0.6643)}{4.35pt}{4.62pt} \\*
\softcline{4-11}
 & \HoloTaskSpan{\makecell[c]{3D-RAD\\[-0.10ex]Medical\\[-0.10ex]Computation}}{2.05cm}{0.32cm} &  & \HoloTaskMetric{\makecell[c]{\mbox{METEOR}}} & \HoloTaskScore{0.09060}{(0.07320--0.1141)}{4.02pt}{4.28pt} & \HoloTaskScore{0.1363}{(0.1188--0.1613)}{4.35pt}{4.62pt} & \HoloTaskScore{0.05560}{(0.04080--0.07190)}{4.02pt}{4.28pt} & \HoloTaskScore{0.05400}{(0.04150--0.07150)}{4.02pt}{4.28pt} & \HoloTaskScore{0.3921}{(0.3654--0.4229)}{4.35pt}{4.62pt} & \HoloTaskScore{0.5122}{(0.4885--0.5341)}{4.35pt}{4.62pt} & \HoloTaskScore{0.5695}{(0.5474--0.5918)}{4.35pt}{4.62pt} \\*
\cline{3-11}
 &  & \HoloTaskRowSpan{{\fontsize{4.35pt}{4.65pt}\selectfont \makecell[c]{\textbf{Clinical}}}}{1.085cm} & \HoloTaskMetric{\makecell[c]{\mbox{Llama}\\[-0.10ex]\mbox{Score}}} & \HoloTaskScore{3.920}{(3.682--4.144)}{4.35pt}{4.62pt} & \HoloTaskScore{4.128}{(3.902--4.332)}{4.35pt}{4.62pt} & \HoloTaskScore{3.731}{(3.473--3.975)}{4.35pt}{4.62pt} & \HoloTaskScore{3.787}{(3.535--4.010)}{4.35pt}{4.62pt} & \HoloTaskScore{5.414}{(5.258--5.576)}{4.35pt}{4.62pt} & \HoloTaskScore{7.688}{(7.518--7.849)}{4.35pt}{4.62pt} & \HoloTaskScore{8.110}{(7.949--8.266)}{4.35pt}{4.62pt} \\
\hline
 &  &  & \HoloTaskMetric{\makecell[c]{\mbox{BLEU-4}}} & \HoloTaskScore{0.1952}{(0.1887--0.2763)}{4.35pt}{4.62pt} & \HoloTaskScore{0.1441}{(0.1397--0.1581)}{4.35pt}{4.62pt} & \HoloTaskScore{0.1227}{(0.1197--0.1259)}{4.35pt}{4.62pt} & \HoloTaskScore{0.2114}{(0.2067--0.2163)}{4.35pt}{4.62pt} & \HoloTaskScore{0.2817}{(0.2763--0.2870)}{4.35pt}{4.62pt} & \HoloTaskScore{0.2817}{(0.2762--0.2874)}{4.35pt}{4.62pt} & \HoloTaskScore{0.2749}{(0.2695--0.2802)}{4.35pt}{4.62pt} \\*
\softcline{4-11}
 &  & \HoloTaskSpan{{\fontsize{4.35pt}{4.65pt}\selectfont \makecell[c]{\textbf{NLP}}}}{1.085cm}{0pt} & \HoloTaskMetric{\makecell[c]{\mbox{ROUGE-L}}} & \HoloTaskScore{0.2198}{(0.2148--0.2259)}{4.35pt}{4.62pt} & \HoloTaskScore{0.1564}{(0.1430--0.1617)}{4.35pt}{4.62pt} & \HoloTaskScore{0.1162}{(0.1131--0.1194)}{4.35pt}{4.62pt} & \HoloTaskScore{0.2332}{(0.2289--0.2375)}{4.35pt}{4.62pt} & \HoloTaskScore{0.2993}{(0.2941--0.3050)}{4.35pt}{4.62pt} & \HoloTaskScore{0.2644}{(0.2592--0.2694)}{4.35pt}{4.62pt} & \HoloTaskScore{0.2628}{(0.2577--0.2678)}{4.35pt}{4.62pt} \\*
\softcline{4-11}
\HoloTaskSpan{\makecell[c]{\textbf{External}\\[-0.10ex]\textbf{(zero-}\\[-0.10ex]\textbf{shot)}}}{1.35cm}{0.32cm} & \HoloTaskSpan{\makecell[c]{BIMCV-VQA}}{2.05cm}{0.32cm} &  & \HoloTaskMetric{\makecell[c]{\mbox{METEOR}}} & \HoloTaskScore{0.1880}{(0.1769--0.1934)}{4.35pt}{4.62pt} & \HoloTaskScore{0.1224}{(0.1194--0.1352)}{4.35pt}{4.62pt} & \HoloTaskScore{0.09925}{(0.09661--0.1019)}{4.02pt}{4.28pt} & \HoloTaskScore{0.2135}{(0.2088--0.2184)}{4.35pt}{4.62pt} & \HoloTaskScore{0.2969}{(0.2919--0.3019)}{4.35pt}{4.62pt} & \HoloTaskScore{0.2639}{(0.2586--0.2694)}{4.35pt}{4.62pt} & \HoloTaskScore{0.2603}{(0.2548--0.2657)}{4.35pt}{4.62pt} \\*
\cline{3-11}
 &  & \HoloTaskRowSpan{{\fontsize{4.35pt}{4.65pt}\selectfont \makecell[c]{\textbf{Clinical}}}}{1.085cm} & \HoloTaskMetric{\makecell[c]{\mbox{Llama}\\[-0.10ex]\mbox{Score}}} & \HoloTaskScore{4.551}{(4.482--4.622)}{4.35pt}{4.62pt} & \HoloTaskScore{4.026}{(3.957--4.096)}{4.35pt}{4.62pt} & \HoloTaskScore{3.496}{(3.429--3.565)}{4.35pt}{4.62pt} & \HoloTaskScore{4.197}{(4.130--4.264)}{4.35pt}{4.62pt} & \HoloTaskScore{4.870}{(4.795--4.940)}{4.35pt}{4.62pt} & \HoloTaskScore{5.238}{(5.163--5.310)}{4.35pt}{4.62pt} & \HoloTaskScore{5.357}{(5.281--5.426)}{4.35pt}{4.62pt} \\
\hline
\end{longtable}
\arrayrulecolor{black}
\endgroup
