# Supplementary material for: A 3D foundation model unifying CT interpretation and segmentation
Source: arXiv:2611.06471 source file (2026-11-04)
Supplement: Supplementary file 14 [file table6_narrative_report_generation.tex]

\begingroup
\makeatletter
\@ifundefined{color@leftblue}{\definecolor{leftblue}{RGB}{232,242,248}}{}%
\@ifundefined{color@headerblue}{\definecolor{headerblue}{RGB}{218,233,242}}{}%
\makeatother
\setlength{\LTcapwidth}{18.60cm}
\setlength{\LTleft}{\fill}
\setlength{\LTright}{\fill}
\setlength{\LTpre}{0pt}
\setlength{\LTpost}{0pt}
\setlength{\tabcolsep}{0.45pt}
\renewcommand{\arraystretch}{1.00}
\setlength{\extrarowheight}{0pt}
\setlength{\arrayrulewidth}{0.48pt}
\arrayrulecolor{black}
\providecommand{\softcline}[1]{}%
\renewcommand{\softcline}[1]{\arrayrulecolor{black!35}\cline{#1}\arrayrulecolor{black}}
\sloppy
\emergencystretch=2em
\fontsize{5.15pt}{5.75pt}\selectfont
\newcommand{\HoloTaskScore}[4]{%
  \parbox[c][0.64cm][c]{1.70cm}{%
    \centering
    {\fontsize{5.15pt}{5.43pt}\selectfont\strut\mbox{#1}}\\[-0.38ex]%
    {\fontsize{#3}{#4}\selectfont\strut\mbox{#2}}%
  }%
}%
\newcommand{\HoloTaskMetricGroup}[1]{%
  \parbox[c][0.64cm][c]{1.045cm}{%
    \centering\fontsize{4.35pt}{4.65pt}\selectfont\textbf{\mbox{#1}}%
  }%
}%
\newcommand{\HoloTaskMetric}[1]{%
  \parbox[c][0.64cm][c]{1.045cm}{%
    \centering\fontsize{4.35pt}{4.65pt}\selectfont\textbf{#1}%
  }%
}%
\newcommand{\HoloTaskMergedMetric}[1]{%
  \parbox[c][0.64cm][c]{2.13cm}{%
    \centering\fontsize{4.35pt}{4.65pt}\selectfont\textbf{\mbox{#1}}%
  }%
}%
\newcommand{\HoloTaskRowSpan}[2]{%
  \parbox[c][0.64cm][c]{#2}{%
    \centering\arraybackslash #1%
  }%
}%
\newcommand{\HoloTaskSpan}[3]{%
  \raisebox{\dimexpr#3-0.11cm\relax}[0pt][0pt]{%
    \parbox[c][0.64cm][c]{#2}{%
      \centering\arraybackslash #1%
    }%
  }%
}%
\newcommand{\HoloTaskSplitHead}[3]{%
  \parbox[c][0.92cm][c]{#3}{%
    \centering\fontsize{6.05pt}{6.30pt}\selectfont\textbf{#1}\\[-0.52ex]%
    \rule{0pt}{0.58ex}\\[-0.52ex]\textbf{#2}%
  }%
}%
\newcommand{\HoloTaskMidHead}[2]{%
  \parbox[c][0.92cm][c]{#2}{%
    \centering\fontsize{6.05pt}{6.30pt}\selectfont\textbf{#1}%
  }%
}%
\newcommand{\HoloTaskModelHead}[2]{%
  \parbox[c][0.92cm][c]{#2}{%
    \centering\fontsize{5.50pt}{5.75pt}\selectfont\textbf{#1}%
  }%
}%
\begin{longtable}{|>{\columncolor{leftblue}\centering\arraybackslash}m{1.35cm}|>{\columncolor{leftblue}\centering\arraybackslash}m{2.05cm}|>{\columncolor{leftblue}\centering\arraybackslash}m{1.085cm}|>{\columncolor{leftblue}\centering\arraybackslash}m{1.085cm}|>{\centering\arraybackslash}m{1.72cm}|>{\centering\arraybackslash}m{1.72cm}|>{\centering\arraybackslash}m{1.72cm}|>{\centering\arraybackslash}m{1.72cm}|>{\centering\arraybackslash}m{1.72cm}|>{\centering\arraybackslash}m{1.72cm}|>{\centering\arraybackslash}m{1.72cm}|}
\caption[Detailed narrative report generation scores across benchmarks]{\textbf{Detailed narrative report generation performance of HoloCT and competing methods on internal and external zero-shot benchmarks.}\newline Each score is reported as mean with 95\% confidence interval. NLP metrics include BLEU-4, ROUGE-L, and METEOR; clinical metrics include RaTEScore, LlamaScore, and GREEN.}%
\label{tab:narrative_report_generation_scores}\\[-0.15ex]
\hline
\rowcolor{headerblue}
\HoloTaskSplitHead{Dataset}{Type}{1.35cm} & \HoloTaskSplitHead{Dataset}{Name}{2.05cm} & \multicolumn{2}{>{\columncolor{headerblue}\centering\arraybackslash}m{\dimexpr1.085cm+1.085cm+2\tabcolsep+\arrayrulewidth\relax}|}{\HoloTaskMidHead{Metric}{\dimexpr1.085cm+1.085cm+2\tabcolsep+\arrayrulewidth\relax}} & \HoloTaskModelHead{\makecell[c]{Qwen3-VL-\\[-0.18ex]32B}}{1.72cm} & \HoloTaskModelHead{\makecell[c]{MedGemma1.5-\\[-0.18ex]4B}}{1.72cm} & \HoloTaskModelHead{\makecell[c]{M3D-Phi3-\\[-0.18ex]4B}}{1.72cm} & \HoloTaskModelHead{\makecell[c]{RadFM-\\[-0.18ex]14B}}{1.72cm} & \HoloTaskModelHead{\makecell[c]{HuluMed-\\[-0.18ex]32B}}{1.72cm} & \HoloTaskModelHead{\makecell[c]{HoloCT-\\[-0.18ex]4B}}{1.72cm} & \HoloTaskModelHead{\makecell[c]{HoloCT-\\[-0.18ex]8B}}{1.72cm} \\
\hline
\endfirsthead
\caption*{\textbf{Supplementary Table~\ref{tab:narrative_report_generation_scores} (continued)\enspace|\enspace Detailed narrative report generation performance of HoloCT and competing methods on internal and external zero-shot benchmarks.}\newline Each score is reported as mean with 95\% confidence interval. NLP metrics include BLEU-4, ROUGE-L, and METEOR; clinical metrics include RaTEScore, LlamaScore, and GREEN.}\\[-0.15ex]
\hline
\rowcolor{headerblue}
\HoloTaskSplitHead{Dataset}{Type}{1.35cm} & \HoloTaskSplitHead{Dataset}{Name}{2.05cm} & \multicolumn{2}{>{\columncolor{headerblue}\centering\arraybackslash}m{\dimexpr1.085cm+1.085cm+2\tabcolsep+\arrayrulewidth\relax}|}{\HoloTaskMidHead{Metric}{\dimexpr1.085cm+1.085cm+2\tabcolsep+\arrayrulewidth\relax}} & \HoloTaskModelHead{\makecell[c]{Qwen3-VL-\\[-0.18ex]32B}}{1.72cm} & \HoloTaskModelHead{\makecell[c]{MedGemma1.5-\\[-0.18ex]4B}}{1.72cm} & \HoloTaskModelHead{\makecell[c]{M3D-Phi3-\\[-0.18ex]4B}}{1.72cm} & \HoloTaskModelHead{\makecell[c]{RadFM-\\[-0.18ex]14B}}{1.72cm} & \HoloTaskModelHead{\makecell[c]{HuluMed-\\[-0.18ex]32B}}{1.72cm} & \HoloTaskModelHead{\makecell[c]{HoloCT-\\[-0.18ex]4B}}{1.72cm} & \HoloTaskModelHead{\makecell[c]{HoloCT-\\[-0.18ex]8B}}{1.72cm} \\
\hline
\endhead
\endfoot
\endlastfoot
 &  &  & \HoloTaskMetric{\makecell[c]{\mbox{BLEU-4}}} & \HoloTaskScore{0.08220}{(0.05110--0.1099)}{4.02pt}{4.28pt} & \HoloTaskScore{0.2319}{(0.2033--0.2562)}{4.35pt}{4.62pt} & \HoloTaskScore{0.02401}{(0.02178--0.02628)}{4.02pt}{4.28pt} & \HoloTaskScore{0.03029}{(0.02762--0.03296)}{4.02pt}{4.28pt} & \HoloTaskScore{0.5086}{(0.5027--0.5140)}{4.35pt}{4.62pt} & \HoloTaskScore{0.5496}{(0.5438--0.5556)}{4.35pt}{4.62pt} & \HoloTaskScore{0.5481}{(0.5424--0.5535)}{4.35pt}{4.62pt} \\*
\softcline{4-11}
 &  & \HoloTaskSpan{{\fontsize{4.35pt}{4.65pt}\selectfont \makecell[c]{\textbf{NLP}}}}{1.085cm}{0pt} & \HoloTaskMetric{\makecell[c]{\mbox{ROUGE-L}}} & \HoloTaskScore{0.1087}{(0.07490--0.1307)}{4.02pt}{4.28pt} & \HoloTaskScore{0.1271}{(0.09500--0.1513)}{4.02pt}{4.28pt} & \HoloTaskScore{0.05858}{(0.05717--0.05994)}{4.02pt}{4.28pt} & \HoloTaskScore{0.06645}{(0.06472--0.06807)}{4.02pt}{4.28pt} & \HoloTaskScore{0.3243}{(0.3195--0.3295)}{4.35pt}{4.62pt} & \HoloTaskScore{0.3848}{(0.3785--0.3913)}{4.35pt}{4.62pt} & \HoloTaskScore{0.3579}{(0.3524--0.3637)}{4.35pt}{4.62pt} \\*
\softcline{4-11}
 &  &  & \HoloTaskMetric{\makecell[c]{\mbox{METEOR}}} & \HoloTaskScore{0.09690}{(0.06840--0.1237)}{4.02pt}{4.28pt} & \HoloTaskScore{0.1207}{(0.09770--0.1456)}{4.02pt}{4.28pt} & \HoloTaskScore{0.03613}{(0.03496--0.03722)}{4.02pt}{4.28pt} & \HoloTaskScore{0.04624}{(0.04467--0.04777)}{4.02pt}{4.28pt} & \HoloTaskScore{0.3731}{(0.3683--0.3785)}{4.35pt}{4.62pt} & \HoloTaskScore{0.4175}{(0.4117--0.4233)}{4.35pt}{4.62pt} & \HoloTaskScore{0.4029}{(0.3978--0.4076)}{4.35pt}{4.62pt} \\*
\cline{3-11}
 & \HoloTaskSpan{\makecell[c]{CT-RATE-RG}}{2.05cm}{0.32cm} &  & \HoloTaskMetric{\makecell[c]{\mbox{RaTE}\\[-0.10ex]\mbox{Score}}} & \HoloTaskScore{0.4285}{(0.4027--0.4442)}{4.35pt}{4.62pt} & \HoloTaskScore{0.4571}{(0.4390--0.4761)}{4.35pt}{4.62pt} & \HoloTaskScore{0.3642}{(0.3611--0.3670)}{4.35pt}{4.62pt} & \HoloTaskScore{0.3905}{(0.3876--0.3935)}{4.35pt}{4.62pt} & \HoloTaskScore{0.6384}{(0.6353--0.6415)}{4.35pt}{4.62pt} & \HoloTaskScore{0.6620}{(0.6581--0.6655)}{4.35pt}{4.62pt} & \HoloTaskScore{0.6496}{(0.6466--0.6527)}{4.35pt}{4.62pt} \\*
\softcline{4-11}
 &  & \HoloTaskSpan{{\fontsize{4.35pt}{4.65pt}\selectfont \makecell[c]{\textbf{Clinical}}}}{1.085cm}{0pt} & \HoloTaskMetric{\makecell[c]{\mbox{Llama}\\[-0.10ex]\mbox{Score}}} & \HoloTaskScore{2.434}{(2.316--2.549)}{4.35pt}{4.62pt} & \HoloTaskScore{4.059}{(3.934--4.160)}{4.35pt}{4.62pt} & \HoloTaskScore{1.067}{(1.025--1.110)}{4.35pt}{4.62pt} & \HoloTaskScore{1.794}{(1.744--1.843)}{4.35pt}{4.62pt} & \HoloTaskScore{6.433}{(6.418--6.523)}{4.35pt}{4.62pt} & \HoloTaskScore{6.571}{(6.506--6.631)}{4.35pt}{4.62pt} & \HoloTaskScore{6.430}{(6.368--6.494)}{4.35pt}{4.62pt} \\*
\softcline{4-11}
 &  &  & \HoloTaskMetric{\makecell[c]{\mbox{GREEN}}} & \HoloTaskScore{0.05540}{(0.03650--0.08190)}{4.02pt}{4.28pt} & \HoloTaskScore{0.2854}{(0.2534--0.3165)}{4.35pt}{4.62pt} & \HoloTaskScore{0.005301}{(0.004383--0.006346)}{3.72pt}{3.98pt} & \HoloTaskScore{0.01819}{(0.01614--0.02020)}{4.02pt}{4.28pt} & \HoloTaskScore{0.4060}{(0.3985--0.4129)}{4.35pt}{4.62pt} & \HoloTaskScore{0.4372}{(0.4283--0.4462)}{4.35pt}{4.62pt} & \HoloTaskScore{0.4197}{(0.4115--0.4274)}{4.35pt}{4.62pt} \\
\cline{2-11}
 &  &  & \HoloTaskMetric{\makecell[c]{\mbox{BLEU-4}}} & \HoloTaskScore{0.1524}{(0.1106--0.1885)}{4.35pt}{4.62pt} & \HoloTaskScore{0.1760}{(0.1450--0.2054)}{4.35pt}{4.62pt} & \HoloTaskScore{0.07939}{(0.07291--0.08591)}{4.02pt}{4.28pt} & \HoloTaskScore{0.1253}{(0.1174--0.1332)}{4.35pt}{4.62pt} & \HoloTaskScore{0.2825}{(0.2768--0.2883)}{4.35pt}{4.62pt} & \HoloTaskScore{0.5051}{(0.4922--0.5185)}{4.35pt}{4.62pt} & \HoloTaskScore{0.5704}{(0.5593--0.5813)}{4.35pt}{4.62pt} \\*
\softcline{4-11}
 &  & \HoloTaskSpan{{\fontsize{4.35pt}{4.65pt}\selectfont \makecell[c]{\textbf{NLP}}}}{1.085cm}{0pt} & \HoloTaskMetric{\makecell[c]{\mbox{ROUGE-L}}} & \HoloTaskScore{0.1266}{(0.09610--0.1548)}{4.02pt}{4.28pt} & \HoloTaskScore{0.1357}{(0.1017--0.1613)}{4.35pt}{4.62pt} & \HoloTaskScore{0.09772}{(0.09481--0.1003)}{4.02pt}{4.28pt} & \HoloTaskScore{0.1142}{(0.1110--0.1174)}{4.35pt}{4.62pt} & \HoloTaskScore{0.1596}{(0.1572--0.1621)}{4.35pt}{4.62pt} & \HoloTaskScore{0.4305}{(0.4219--0.4394)}{4.35pt}{4.62pt} & \HoloTaskScore{0.4580}{(0.4495--0.4664)}{4.35pt}{4.62pt} \\*
\softcline{4-11}
 &  &  & \HoloTaskMetric{\makecell[c]{\mbox{METEOR}}} & \HoloTaskScore{0.1065}{(0.07780--0.1322)}{4.02pt}{4.28pt} & \HoloTaskScore{0.1161}{(0.08480--0.1409)}{4.02pt}{4.28pt} & \HoloTaskScore{0.06093}{(0.05854--0.06363)}{4.02pt}{4.28pt} & \HoloTaskScore{0.08546}{(0.08214--0.08878)}{4.02pt}{4.28pt} & \HoloTaskScore{0.1698}{(0.1661--0.1735)}{4.35pt}{4.62pt} & \HoloTaskScore{0.4011}{(0.3918--0.4106)}{4.35pt}{4.62pt} & \HoloTaskScore{0.4731}{(0.4641--0.4825)}{4.35pt}{4.62pt} \\*
\cline{3-11}
\HoloTaskSpan{\makecell[c]{\textbf{Internal}}}{1.35cm}{0.32cm} & \HoloTaskSpan{\makecell[c]{AbdomenAtlas3.0}}{2.05cm}{0.32cm} &  & \HoloTaskMetric{\makecell[c]{\mbox{RaTE}\\[-0.10ex]\mbox{Score}}} & \HoloTaskScore{0.3929}{(0.3682--0.4242)}{4.35pt}{4.62pt} & \HoloTaskScore{0.4066}{(0.3790--0.4369)}{4.35pt}{4.62pt} & \HoloTaskScore{0.3763}{(0.3710--0.3815)}{4.35pt}{4.62pt} & \HoloTaskScore{0.3533}{(0.3467--0.3600)}{4.35pt}{4.62pt} & \HoloTaskScore{0.4602}{(0.4528--0.4674)}{4.35pt}{4.62pt} & \HoloTaskScore{0.7606}{(0.7540--0.7665)}{4.35pt}{4.62pt} & \HoloTaskScore{0.7670}{(0.7611--0.7729)}{4.35pt}{4.62pt} \\*
\softcline{4-11}
 &  & \HoloTaskSpan{{\fontsize{4.35pt}{4.65pt}\selectfont \makecell[c]{\textbf{Clinical}}}}{1.085cm}{0pt} & \HoloTaskMetric{\makecell[c]{\mbox{Llama}\\[-0.10ex]\mbox{Score}}} & \HoloTaskScore{0.6851}{(0.5222--0.8501)}{4.35pt}{4.62pt} & \HoloTaskScore{0.8290}{(0.6778--0.9971)}{4.35pt}{4.62pt} & \HoloTaskScore{0.4582}{(0.4006--0.5157)}{4.35pt}{4.62pt} & \HoloTaskScore{0.2182}{(0.1801--0.2610)}{4.35pt}{4.62pt} & \HoloTaskScore{1.554}{(1.434--1.678)}{4.35pt}{4.62pt} & \HoloTaskScore{4.808}{(4.711--4.914)}{4.35pt}{4.62pt} & \HoloTaskScore{4.663}{(4.562--4.774)}{4.35pt}{4.62pt} \\*
\softcline{4-11}
 &  &  & \HoloTaskMetric{\makecell[c]{\mbox{GREEN}}} & \HoloTaskScore{0.03510}{(0.01880--0.06010)}{4.02pt}{4.28pt} & \HoloTaskScore{0.04510}{(0.02780--0.07430)}{4.02pt}{4.28pt} & \HoloTaskScore{0.008943}{(0.006399--0.01175)}{3.72pt}{3.98pt} & \HoloTaskScore{0.01228}{(0.008561--0.01621)}{3.72pt}{3.98pt} & \HoloTaskScore{0.1281}{(0.1127--0.1446)}{4.35pt}{4.62pt} & \HoloTaskScore{0.3107}{(0.2945--0.3254)}{4.35pt}{4.62pt} & \HoloTaskScore{0.3087}{(0.2953--0.3216)}{4.35pt}{4.62pt} \\
\cline{2-11}
 &  &  & \HoloTaskMetric{\makecell[c]{\mbox{BLEU-4}}} & \HoloTaskScore{0.1460}{(0.1280--0.1609)}{4.35pt}{4.62pt} & \HoloTaskScore{0.1584}{(0.1365--0.1742)}{4.35pt}{4.62pt} & \HoloTaskScore{0.1126}{(0.1083--0.1172)}{4.35pt}{4.62pt} & \HoloTaskScore{0.1433}{(0.1385--0.1485)}{4.35pt}{4.62pt} & \HoloTaskScore{0.1562}{(0.1516--0.1609)}{4.35pt}{4.62pt} & \HoloTaskScore{0.2609}{(0.2532--0.2693)}{4.35pt}{4.62pt} & \HoloTaskScore{0.2908}{(0.2831--0.2992)}{4.35pt}{4.62pt} \\*
\softcline{4-11}
 &  & \HoloTaskSpan{{\fontsize{4.35pt}{4.65pt}\selectfont \makecell[c]{\textbf{NLP}}}}{1.085cm}{0pt} & \HoloTaskMetric{\makecell[c]{\mbox{ROUGE-L}}} & \HoloTaskScore{0.1045}{(0.08410--0.1252)}{4.02pt}{4.28pt} & \HoloTaskScore{0.1111}{(0.09580--0.1383)}{4.02pt}{4.28pt} & \HoloTaskScore{0.08649}{(0.08468--0.08812)}{4.02pt}{4.28pt} & \HoloTaskScore{0.1029}{(0.1008--0.1047)}{4.35pt}{4.62pt} & \HoloTaskScore{0.09737}{(0.09589--0.09874)}{4.02pt}{4.28pt} & \HoloTaskScore{0.2749}{(0.2688--0.2812)}{4.35pt}{4.62pt} & \HoloTaskScore{0.2789}{(0.2728--0.2857)}{4.35pt}{4.62pt} \\*
\softcline{4-11}
 &  &  & \HoloTaskMetric{\makecell[c]{\mbox{METEOR}}} & \HoloTaskScore{0.1213}{(0.1087--0.1401)}{4.35pt}{4.62pt} & \HoloTaskScore{0.1366}{(0.1148--0.1533)}{4.35pt}{4.62pt} & \HoloTaskScore{0.08907}{(0.08669--0.09144)}{4.02pt}{4.28pt} & \HoloTaskScore{0.1135}{(0.1113--0.1160)}{4.35pt}{4.62pt} & \HoloTaskScore{0.1688}{(0.1671--0.1708)}{4.35pt}{4.62pt} & \HoloTaskScore{0.2931}{(0.2858--0.3000)}{4.35pt}{4.62pt} & \HoloTaskScore{0.3151}{(0.3074--0.3221)}{4.35pt}{4.62pt} \\*
\cline{3-11}
 & \HoloTaskSpan{\makecell[c]{INSPECT}}{2.05cm}{0.32cm} &  & \HoloTaskMetric{\makecell[c]{\mbox{RaTE}\\[-0.10ex]\mbox{Score}}} & \HoloTaskScore{0.3516}{(0.3358--0.3781)}{4.35pt}{4.62pt} & \HoloTaskScore{0.3624}{(0.3454--0.3873)}{4.35pt}{4.62pt} & \HoloTaskScore{0.2967}{(0.2929--0.3007)}{4.35pt}{4.62pt} & \HoloTaskScore{0.3430}{(0.3394--0.3468)}{4.35pt}{4.62pt} & \HoloTaskScore{0.3797}{(0.3763--0.3827)}{4.35pt}{4.62pt} & \HoloTaskScore{0.5062}{(0.4998--0.5126)}{4.35pt}{4.62pt} & \HoloTaskScore{0.4942}{(0.4882--0.5001)}{4.35pt}{4.62pt} \\*
\softcline{4-11}
 &  & \HoloTaskSpan{{\fontsize{4.35pt}{4.65pt}\selectfont \makecell[c]{\textbf{Clinical}}}}{1.085cm}{0pt} & \HoloTaskMetric{\makecell[c]{\mbox{Llama}\\[-0.10ex]\mbox{Score}}} & \HoloTaskScore{2.055}{(1.957--2.167)}{4.35pt}{4.62pt} & \HoloTaskScore{2.402}{(2.290--2.513)}{4.35pt}{4.62pt} & \HoloTaskScore{1.072}{(1.012--1.130)}{4.35pt}{4.62pt} & \HoloTaskScore{1.508}{(1.446--1.569)}{4.35pt}{4.62pt} & \HoloTaskScore{4.551}{(4.473--4.624)}{4.35pt}{4.62pt} & \HoloTaskScore{5.208}{(5.121--5.297)}{4.35pt}{4.62pt} & \HoloTaskScore{5.079}{(4.982--5.172)}{4.35pt}{4.62pt} \\*
\softcline{4-11}
 &  &  & \HoloTaskMetric{\makecell[c]{\mbox{GREEN}}} & \HoloTaskScore{0.02900}{(0.01610--0.04120)}{4.02pt}{4.28pt} & \HoloTaskScore{0.03810}{(0.01850--0.05900)}{4.02pt}{4.28pt} & \HoloTaskScore{0.005848}{(0.004210--0.007808)}{3.72pt}{3.98pt} & \HoloTaskScore{0.007954}{(0.006588--0.009438)}{3.72pt}{3.98pt} & \HoloTaskScore{0.03857}{(0.03382--0.04414)}{4.02pt}{4.28pt} & \HoloTaskScore{0.2247}{(0.2173--0.2326)}{4.35pt}{4.62pt} & \HoloTaskScore{0.2163}{(0.2091--0.2246)}{4.35pt}{4.62pt} \\
\hline
 &  &  & \HoloTaskMetric{\makecell[c]{\mbox{BLEU-4}}} & \HoloTaskScore{0.1560}{(0.1201--0.1842)}{4.35pt}{4.62pt} & \HoloTaskScore{0.1769}{(0.1425--0.2018)}{4.35pt}{4.62pt} & \HoloTaskScore{0.1286}{(0.1218--0.1356)}{4.35pt}{4.62pt} & \HoloTaskScore{0.1348}{(0.1275--0.1423)}{4.35pt}{4.62pt} & \HoloTaskScore{0.2647}{(0.2566--0.2716)}{4.35pt}{4.62pt} & \HoloTaskScore{0.1933}{(0.1839--0.2026)}{4.35pt}{4.62pt} & \HoloTaskScore{0.1982}{(0.1887--0.2072)}{4.35pt}{4.62pt} \\*
\softcline{4-11}
 &  & \HoloTaskSpan{{\fontsize{4.35pt}{4.65pt}\selectfont \makecell[c]{\textbf{NLP}}}}{1.085cm}{0pt} & \HoloTaskMetric{\makecell[c]{\mbox{ROUGE-L}}} & \HoloTaskScore{0.1245}{(0.09170--0.1465)}{4.02pt}{4.28pt} & \HoloTaskScore{0.1352}{(0.1066--0.1577)}{4.35pt}{4.62pt} & \HoloTaskScore{0.1069}{(0.1041--0.1095)}{4.35pt}{4.62pt} & \HoloTaskScore{0.1147}{(0.1110--0.1180)}{4.35pt}{4.62pt} & \HoloTaskScore{0.1314}{(0.1291--0.1337)}{4.35pt}{4.62pt} & \HoloTaskScore{0.1706}{(0.1661--0.1745)}{4.35pt}{4.62pt} & \HoloTaskScore{0.1681}{(0.1642--0.1719)}{4.35pt}{4.62pt} \\*
\softcline{4-11}
 &  &  & \HoloTaskMetric{\makecell[c]{\mbox{METEOR}}} & \HoloTaskScore{0.1241}{(0.09290--0.1563)}{4.02pt}{4.28pt} & \HoloTaskScore{0.1451}{(0.1123--0.1734)}{4.35pt}{4.62pt} & \HoloTaskScore{0.09245}{(0.08954--0.09556)}{4.02pt}{4.28pt} & \HoloTaskScore{0.1098}{(0.1053--0.1144)}{4.35pt}{4.62pt} & \HoloTaskScore{0.2042}{(0.2011--0.2074)}{4.35pt}{4.62pt} & \HoloTaskScore{0.1662}{(0.1606--0.1716)}{4.35pt}{4.62pt} & \HoloTaskScore{0.1707}{(0.1658--0.1753)}{4.35pt}{4.62pt} \\*
\cline{3-11}
\HoloTaskSpan{\makecell[c]{\textbf{External}\\[-0.10ex]\textbf{(zero-}\\[-0.10ex]\textbf{shot)}}}{1.35cm}{0.32cm} & \HoloTaskSpan{\makecell[c]{BIMCV-RG}}{2.05cm}{0.32cm} &  & \HoloTaskMetric{\makecell[c]{\mbox{RaTE}\\[-0.10ex]\mbox{Score}}} & \HoloTaskScore{0.3676}{(0.3461--0.3966)}{4.35pt}{4.62pt} & \HoloTaskScore{0.3877}{(0.3622--0.4166)}{4.35pt}{4.62pt} & \HoloTaskScore{0.3421}{(0.3374--0.3464)}{4.35pt}{4.62pt} & \HoloTaskScore{0.3428}{(0.3374--0.3482)}{4.35pt}{4.62pt} & \HoloTaskScore{0.4454}{(0.4414--0.4495)}{4.35pt}{4.62pt} & \HoloTaskScore{0.4601}{(0.4536--0.4661)}{4.35pt}{4.62pt} & \HoloTaskScore{0.4827}{(0.4763--0.4889)}{4.35pt}{4.62pt} \\*
\softcline{4-11}
 &  & \HoloTaskSpan{{\fontsize{4.35pt}{4.65pt}\selectfont \makecell[c]{\textbf{Clinical}}}}{1.085cm}{0pt} & \HoloTaskMetric{\makecell[c]{\mbox{Llama}\\[-0.10ex]\mbox{Score}}} & \HoloTaskScore{1.853}{(1.726--1.996)}{4.35pt}{4.62pt} & \HoloTaskScore{2.209}{(2.068--2.350)}{4.35pt}{4.62pt} & \HoloTaskScore{1.268}{(1.191--1.349)}{4.35pt}{4.62pt} & \HoloTaskScore{1.189}{(1.125--1.248)}{4.35pt}{4.62pt} & \HoloTaskScore{4.006}{(3.898--4.112)}{4.35pt}{4.62pt} & \HoloTaskScore{4.253}{(4.136--4.369)}{4.35pt}{4.62pt} & \HoloTaskScore{4.069}{(3.945--4.184)}{4.35pt}{4.62pt} \\*
\softcline{4-11}
 &  &  & \HoloTaskMetric{\makecell[c]{\mbox{GREEN}}} & \HoloTaskScore{0.03550}{(0.01450--0.05840)}{4.02pt}{4.28pt} & \HoloTaskScore{0.04150}{(0.02710--0.05920)}{4.02pt}{4.28pt} & \HoloTaskScore{0.01097}{(0.008727--0.01360)}{3.72pt}{3.98pt} & \HoloTaskScore{0.01595}{(0.01312--0.01920)}{4.02pt}{4.28pt} & \HoloTaskScore{0.09048}{(0.08202--0.09869)}{4.02pt}{4.28pt} & \HoloTaskScore{0.1642}{(0.1535--0.1758)}{4.35pt}{4.62pt} & \HoloTaskScore{0.1824}{(0.1705--0.1948)}{4.35pt}{4.62pt} \\
\hline
\end{longtable}
\arrayrulecolor{black}
\endgroup
