# Supplementary material for: A 3D foundation model unifying CT interpretation and segmentation
Source: arXiv:2611.06471 source file (2026-11-04)
Supplement: Supplementary file 15 [file table7_structured_report_generation.tex]

\begingroup
\makeatletter
\@ifundefined{color@leftblue}{\definecolor{leftblue}{RGB}{232,242,248}}{}%
\@ifundefined{color@headerblue}{\definecolor{headerblue}{RGB}{218,233,242}}{}%
\makeatother
\setlength{\LTcapwidth}{18.60cm}
\setlength{\LTleft}{\fill}
\setlength{\LTright}{\fill}
\setlength{\LTpre}{0pt}
\setlength{\LTpost}{0pt}
\setlength{\tabcolsep}{0.45pt}
\renewcommand{\arraystretch}{1.00}
\setlength{\extrarowheight}{0pt}
\setlength{\arrayrulewidth}{0.48pt}
\arrayrulecolor{black}
\providecommand{\softcline}[1]{}%
\renewcommand{\softcline}[1]{\arrayrulecolor{black!35}\cline{#1}\arrayrulecolor{black}}
\sloppy
\emergencystretch=2em
\fontsize{5.15pt}{5.75pt}\selectfont
\newcommand{\HoloTaskScore}[5]{%
  \parbox[c][0.64cm][c]{1.70cm}{%
    \centering
    {\fontsize{5.15pt}{5.43pt}\selectfont\strut\mbox{#1#5}}\\[-0.38ex]%
    {\fontsize{#3}{#4}\selectfont\strut\mbox{#2}}%
  }%
}%
\newcommand{\HoloTaskMetricGroup}[1]{%
  \parbox[c][0.64cm][c]{1.045cm}{%
    \centering\fontsize{4.35pt}{4.65pt}\selectfont\textbf{\mbox{#1}}%
  }%
}%
\newcommand{\HoloTaskMetric}[1]{%
  \parbox[c][0.64cm][c]{1.045cm}{%
    \centering\fontsize{4.35pt}{4.65pt}\selectfont\textbf{#1}%
  }%
}%
\newcommand{\HoloTaskMergedMetric}[1]{%
  \parbox[c][0.64cm][c]{2.13cm}{%
    \centering\fontsize{4.35pt}{4.65pt}\selectfont\textbf{\mbox{#1}}%
  }%
}%
\newcommand{\HoloTaskRowSpan}[2]{%
  \parbox[c][0.64cm][c]{#2}{%
    \centering\arraybackslash #1%
  }%
}%
\newcommand{\HoloTaskSpan}[3]{%
  \raisebox{\dimexpr#3-0.11cm\relax}[0pt][0pt]{%
    \parbox[c][0.64cm][c]{#2}{%
      \centering\arraybackslash #1%
    }%
  }%
}%
\newcommand{\HoloTaskSplitHead}[3]{%
  \parbox[c][0.92cm][c]{#3}{%
    \centering\fontsize{6.05pt}{6.30pt}\selectfont\textbf{#1}\\[-0.52ex]%
    \rule{0pt}{0.58ex}\\[-0.52ex]\textbf{#2}%
  }%
}%
\newcommand{\HoloTaskMidHead}[2]{%
  \parbox[c][0.92cm][c]{#2}{%
    \centering\fontsize{6.05pt}{6.30pt}\selectfont\textbf{#1}%
  }%
}%
\newcommand{\HoloTaskModelHead}[2]{%
  \parbox[c][0.92cm][c]{#2}{%
    \centering\fontsize{5.50pt}{5.75pt}\selectfont\textbf{#1}%
  }%
}%
\begin{longtable}{|>{\columncolor{leftblue}\centering\arraybackslash}m{1.35cm}|>{\columncolor{leftblue}\centering\arraybackslash}m{2.05cm}|>{\columncolor{leftblue}\centering\arraybackslash}m{1.085cm}|>{\columncolor{leftblue}\centering\arraybackslash}m{1.085cm}|>{\centering\arraybackslash}m{1.72cm}|>{\centering\arraybackslash}m{1.72cm}|>{\centering\arraybackslash}m{1.72cm}|>{\centering\arraybackslash}m{1.72cm}|>{\centering\arraybackslash}m{1.72cm}|>{\centering\arraybackslash}m{1.72cm}|>{\centering\arraybackslash}m{1.72cm}|}
\caption[Detailed structured report generation scores across benchmarks]{\textbf{Detailed structured report generation performance of HoloCT and competing methods on internal benchmarks.}\newline Each score is reported as mean with 95\% confidence interval. NLP metrics include BLEU-4, ROUGE-L, and METEOR; clinical metrics include RaTEScore, LlamaScore, and GREEN.}%
\label{tab:structured_report_generation_scores}\\[-0.15ex]
\hline
\rowcolor{headerblue}
\HoloTaskSplitHead{Dataset}{Type}{1.35cm} & \HoloTaskSplitHead{Dataset}{Name}{2.05cm} & \multicolumn{2}{>{\columncolor{headerblue}\centering\arraybackslash}m{\dimexpr1.085cm+1.085cm+2\tabcolsep+\arrayrulewidth\relax}|}{\HoloTaskMidHead{Metric}{\dimexpr1.085cm+1.085cm+2\tabcolsep+\arrayrulewidth\relax}} & \HoloTaskModelHead{\makecell[c]{Qwen3-VL-\\[-0.18ex]32B}}{1.72cm} & \HoloTaskModelHead{\makecell[c]{MedGemma1.5-\\[-0.18ex]4B}}{1.72cm} & \HoloTaskModelHead{\makecell[c]{M3D-Phi3-\\[-0.18ex]4B}}{1.72cm} & \HoloTaskModelHead{\makecell[c]{RadFM-\\[-0.18ex]14B}}{1.72cm} & \HoloTaskModelHead{\makecell[c]{HuluMed-\\[-0.18ex]32B}}{1.72cm} & \HoloTaskModelHead{\makecell[c]{HoloCT-\\[-0.18ex]4B}}{1.72cm} & \HoloTaskModelHead{\makecell[c]{HoloCT-\\[-0.18ex]8B}}{1.72cm} \\
\hline
\endfirsthead
\caption*{\textbf{Supplementary Table~\ref{tab:structured_report_generation_scores} (continued)\enspace|\enspace Detailed structured report generation performance of HoloCT and competing methods on internal benchmarks.}\newline Each score is reported as mean with 95\% confidence interval. NLP metrics include BLEU-4, ROUGE-L, and METEOR; clinical metrics include RaTEScore, LlamaScore, and GREEN.}\\[-0.15ex]
\hline
\rowcolor{headerblue}
\HoloTaskSplitHead{Dataset}{Type}{1.35cm} & \HoloTaskSplitHead{Dataset}{Name}{2.05cm} & \multicolumn{2}{>{\columncolor{headerblue}\centering\arraybackslash}m{\dimexpr1.085cm+1.085cm+2\tabcolsep+\arrayrulewidth\relax}|}{\HoloTaskMidHead{Metric}{\dimexpr1.085cm+1.085cm+2\tabcolsep+\arrayrulewidth\relax}} & \HoloTaskModelHead{\makecell[c]{Qwen3-VL-\\[-0.18ex]32B}}{1.72cm} & \HoloTaskModelHead{\makecell[c]{MedGemma1.5-\\[-0.18ex]4B}}{1.72cm} & \HoloTaskModelHead{\makecell[c]{M3D-Phi3-\\[-0.18ex]4B}}{1.72cm} & \HoloTaskModelHead{\makecell[c]{RadFM-\\[-0.18ex]14B}}{1.72cm} & \HoloTaskModelHead{\makecell[c]{HuluMed-\\[-0.18ex]32B}}{1.72cm} & \HoloTaskModelHead{\makecell[c]{HoloCT-\\[-0.18ex]4B}}{1.72cm} & \HoloTaskModelHead{\makecell[c]{HoloCT-\\[-0.18ex]8B}}{1.72cm} \\
\hline
\endhead
\endfoot
\endlastfoot
 &  &  & \HoloTaskMetric{\makecell[c]{\mbox{BLEU-4}}} & \HoloTaskScore{0.2180}{(0.1696--0.2597)}{4.35pt}{4.62pt}{} & \HoloTaskScore{0.2388}{(0.1851--0.2742)}{4.35pt}{4.62pt}{} & \HoloTaskScore{0.02219}{(0.01664--0.02840)}{4.02pt}{4.28pt}{} & \HoloTaskScore{0.07494}{(0.06268--0.08690)}{4.02pt}{4.28pt}{} & \HoloTaskScore{0.4710}{(0.4541--0.4874)}{4.35pt}{4.62pt}{} & \HoloTaskScore{0.5057}{(0.4894--0.5226)}{4.35pt}{4.62pt}{} & \HoloTaskScore{0.5489}{(0.5319--0.5655)}{4.35pt}{4.62pt}{} \\*
\softcline{4-11}
 &  & \HoloTaskSpan{{\fontsize{4.35pt}{4.65pt}\selectfont \makecell[c]{\textbf{NLP}}}}{1.085cm}{0pt} & \HoloTaskMetric{\makecell[c]{\mbox{ROUGE-L}}} & \HoloTaskScore{0.1662}{(0.1256--0.2038)}{4.35pt}{4.62pt}{} & \HoloTaskScore{0.1519}{(0.1108--0.2006)}{4.35pt}{4.62pt}{} & \HoloTaskScore{0.05091}{(0.04573--0.05618)}{4.02pt}{4.28pt}{} & \HoloTaskScore{0.1028}{(0.09691--0.1092)}{4.02pt}{4.28pt}{} & \HoloTaskScore{0.2833}{(0.2747--0.2912)}{4.35pt}{4.62pt}{} & \HoloTaskScore{0.3323}{(0.3232--0.3429)}{4.35pt}{4.62pt}{} & \HoloTaskScore{0.3526}{(0.3390--0.3677)}{4.35pt}{4.62pt}{} \\*
\softcline{4-11}
 &  &  & \HoloTaskMetric{\makecell[c]{\mbox{METEOR}}} & \HoloTaskScore{0.1881}{(0.1489--0.2211)}{4.35pt}{4.62pt}{} & \HoloTaskScore{0.2006}{(0.1666--0.2327)}{4.35pt}{4.62pt}{} & \HoloTaskScore{0.03049}{(0.02669--0.03400)}{4.02pt}{4.28pt}{} & \HoloTaskScore{0.07119}{(0.06528--0.07731)}{4.02pt}{4.28pt}{} & \HoloTaskScore{0.3162}{(0.3061--0.3264)}{4.35pt}{4.62pt}{} & \HoloTaskScore{0.3676}{(0.3570--0.3787)}{4.35pt}{4.62pt}{} & \HoloTaskScore{0.3984}{(0.3847--0.4117)}{4.35pt}{4.62pt}{} \\*
\cline{3-11}
 & \HoloTaskSpan{\makecell[c]{AMOS-MM-RG}}{2.05cm}{0.32cm} &  & \HoloTaskMetric{\makecell[c]{\mbox{RaTE}\\[-0.10ex]\mbox{Score}}} & \HoloTaskScore{0.4915}{(0.4522--0.5358)}{4.35pt}{4.62pt}{} & \HoloTaskScore{0.4579}{(0.4146--0.5012)}{4.35pt}{4.62pt}{} & \HoloTaskScore{0.2686}{(0.2499--0.2874)}{4.35pt}{4.62pt}{} & \HoloTaskScore{0.3599}{(0.3501--0.3701)}{4.35pt}{4.62pt}{} & \HoloTaskScore{0.6314}{(0.6212--0.6415)}{4.35pt}{4.62pt}{} & \HoloTaskScore{0.6831}{(0.6755--0.6911)}{4.35pt}{4.62pt}{} & \HoloTaskScore{0.6955}{(0.6872--0.7046)}{4.35pt}{4.62pt}{} \\*
\softcline{4-11}
 &  & \HoloTaskSpan{{\fontsize{4.35pt}{4.65pt}\selectfont \makecell[c]{\textbf{Clinical}}}}{1.085cm}{0pt} & \HoloTaskMetric{\makecell[c]{\mbox{Llama}\\[-0.10ex]\mbox{Score}}} & \HoloTaskScore{3.524}{(3.284--3.764)}{4.35pt}{4.62pt}{} & \HoloTaskScore{3.422}{(3.186--3.667)}{4.35pt}{4.62pt}{} & \HoloTaskScore{2.376}{(2.062--2.683)}{4.35pt}{4.62pt}{} & \HoloTaskScore{0.4676}{(0.3784--0.5568)}{4.35pt}{4.62pt}{} & \HoloTaskScore{4.885}{(4.700--5.078)}{4.35pt}{4.62pt}{} & \HoloTaskScore{5.228}{(5.065--5.395)}{4.35pt}{4.62pt}{} & \HoloTaskScore{5.160}{(5.000--5.345)}{4.35pt}{4.62pt}{} \\*
\softcline{4-11}
 &  &  & \HoloTaskMetric{\makecell[c]{\mbox{GREEN}}} & \HoloTaskScore{0.1409}{(0.1081--0.1828)}{4.35pt}{4.62pt}{} & \HoloTaskScore{0.1228}{(0.08770--0.1645)}{4.02pt}{4.28pt}{} & \HoloTaskScore{0.01784}{(0.01205--0.02436)}{4.02pt}{4.28pt}{} & \HoloTaskScore{0.01490}{(0.008691--0.02253)}{3.72pt}{3.98pt}{} & \HoloTaskScore{0.3476}{(0.3230--0.3737)}{4.35pt}{4.62pt}{} & \HoloTaskScore{0.3310}{(0.3110--0.3501)}{4.35pt}{4.62pt}{} & \HoloTaskScore{0.3458}{(0.3237--0.3660)}{4.35pt}{4.62pt}{} \\
\cline{2-11}
 &  &  & \HoloTaskMetric{\makecell[c]{\mbox{BLEU-4}}} & \HoloTaskScore{0.2464}{(0.2143--0.2735)}{4.35pt}{4.62pt}{} & \HoloTaskScore{0.2430}{(0.2175--0.2780)}{4.35pt}{4.62pt}{} & \HoloTaskScore{0.03642}{(0.03192--0.04079)}{4.02pt}{4.28pt}{} & \HoloTaskScore{0.1176}{(0.1109--0.1239)}{4.35pt}{4.62pt}{} & \HoloTaskScore{0.5543}{(0.5482--0.5604)}{4.35pt}{4.62pt}{} & \HoloTaskScore{0.6096}{(0.6017--0.6175)}{4.35pt}{4.62pt}{} & \HoloTaskScore{0.6261}{(0.6184--0.6340)}{4.35pt}{4.62pt}{} \\*
\softcline{4-11}
 &  & \HoloTaskSpan{{\fontsize{4.35pt}{4.65pt}\selectfont \makecell[c]{\textbf{NLP}}}}{1.085cm}{0pt} & \HoloTaskMetric{\makecell[c]{\mbox{ROUGE-L}}} & \HoloTaskScore{0.1777}{(0.1410--0.2019)}{4.35pt}{4.62pt}{} & \HoloTaskScore{0.2092}{(0.1785--0.2360)}{4.35pt}{4.62pt}{} & \HoloTaskScore{0.05478}{(0.05186--0.05791)}{4.02pt}{4.28pt}{} & \HoloTaskScore{0.1220}{(0.1195--0.1242)}{4.35pt}{4.62pt}{} & \HoloTaskScore{0.2832}{(0.2800--0.2867)}{4.35pt}{4.62pt}{} & \HoloTaskScore{0.4885}{(0.4788--0.4973)}{4.35pt}{4.62pt}{} & \HoloTaskScore{0.4830}{(0.4732--0.4918)}{4.35pt}{4.62pt}{} \\*
\softcline{4-11}
 &  &  & \HoloTaskMetric{\makecell[c]{\mbox{METEOR}}} & \HoloTaskScore{0.2077}{(0.1782--0.2385)}{4.35pt}{4.62pt}{} & \HoloTaskScore{0.2239}{(0.1866--0.2478)}{4.35pt}{4.62pt}{} & \HoloTaskScore{0.03806}{(0.03565--0.04061)}{4.02pt}{4.28pt}{} & \HoloTaskScore{0.09699}{(0.09411--0.09974)}{4.02pt}{4.28pt}{} & \HoloTaskScore{0.3766}{(0.3710--0.3828)}{4.35pt}{4.62pt}{} & \HoloTaskScore{0.5249}{(0.5151--0.5340)}{4.35pt}{4.62pt}{} & \HoloTaskScore{0.5440}{(0.5349--0.5534)}{4.35pt}{4.62pt}{} \\*
\cline{3-11}
 & \HoloTaskSpan{\makecell[c]{RadGenome}}{2.05cm}{0.32cm} &  & \HoloTaskMetric{\makecell[c]{\mbox{RaTE}\\[-0.10ex]\mbox{Score}}} & \HoloTaskScore{0.5598}{(0.5325--0.5714)}{4.35pt}{4.62pt}{} & \HoloTaskScore{0.5748}{(0.5571--0.5844)}{4.35pt}{4.62pt}{} & \HoloTaskScore{0.2513}{(0.2397--0.2627)}{4.35pt}{4.62pt}{} & \HoloTaskScore{0.5037}{(0.4990--0.5084)}{4.35pt}{4.62pt}{} & \HoloTaskScore{0.6607}{(0.6573--0.6640)}{4.35pt}{4.62pt}{} & \HoloTaskScore{0.7465}{(0.7412--0.7514)}{4.35pt}{4.62pt}{} & \HoloTaskScore{0.7419}{(0.7370--0.7470)}{4.35pt}{4.62pt}{} \\*
\softcline{4-11}
 &  & \HoloTaskSpan{{\fontsize{4.35pt}{4.65pt}\selectfont \makecell[c]{\textbf{Clinical}}}}{1.085cm}{0pt} & \HoloTaskMetric{\makecell[c]{\mbox{Llama}\\[-0.10ex]\mbox{Score}}} & \HoloTaskScore{4.857}{(4.732--4.971)}{4.35pt}{4.62pt}{} & \HoloTaskScore{4.893}{(4.741--4.980)}{4.35pt}{4.62pt}{} & \HoloTaskScore{3.972}{(3.825--4.137)}{4.35pt}{4.62pt}{} & \HoloTaskScore{2.627}{(2.557--2.695)}{4.35pt}{4.62pt}{} & \HoloTaskScore{6.541}{(6.493--6.586)}{4.35pt}{4.62pt}{} & \HoloTaskScore{6.820}{(6.719--6.911)}{4.35pt}{4.62pt}{} & \HoloTaskScore{7.154}{(7.063--7.240)}{4.35pt}{4.62pt}{} \\*
\softcline{4-11}
 &  &  & \HoloTaskMetric{\makecell[c]{\mbox{GREEN}}} & \HoloTaskScore{0.1681}{(0.1395--0.1900)}{4.35pt}{4.62pt}{} & \HoloTaskScore{0.1880}{(0.1502--0.2050)}{4.35pt}{4.62pt}{} & \HoloTaskScore{0.01946}{(0.01603--0.02307)}{4.02pt}{4.28pt}{} & \HoloTaskScore{0.08462}{(0.07777--0.09153)}{4.02pt}{4.28pt}{} & \HoloTaskScore{0.3919}{(0.3811--0.4028)}{4.35pt}{4.62pt}{} & \HoloTaskScore{0.4716}{(0.4580--0.4853)}{4.35pt}{4.62pt}{} & \HoloTaskScore{0.4624}{(0.4499--0.4772)}{4.35pt}{4.62pt}{} \\
\cline{2-11}
\HoloTaskSpan{\makecell[c]{\textbf{Internal}}}{1.35cm}{0.32cm} &  &  & \HoloTaskMetric{\makecell[c]{\mbox{BLEU-4}}} & \HoloTaskScore{0.03657}{(0.01616--0.05573)}{4.02pt}{4.28pt}{} & \HoloTaskScore{0.03931}{(0.02149--0.05132)}{4.02pt}{4.28pt}{} & \HoloTaskScore{0.02809}{(0.02623--0.03018)}{4.02pt}{4.28pt}{} & \HoloTaskScore{0.02491}{(0.02305--0.02684)}{4.02pt}{4.28pt}{} & \HoloTaskScore{0.07043}{(0.06828--0.07278)}{4.02pt}{4.28pt}{} & \HoloTaskScore{0.3799}{(0.3749--0.3849)}{4.35pt}{4.62pt}{} & \HoloTaskScore{0.4393}{(0.4345--0.4442)}{4.35pt}{4.62pt}{} \\*
\softcline{4-11}
 &  & \HoloTaskSpan{{\fontsize{4.35pt}{4.65pt}\selectfont \makecell[c]{\textbf{NLP}}}}{1.085cm}{0pt} & \HoloTaskMetric{\makecell[c]{\mbox{ROUGE-L}}} & \HoloTaskScore{0.05003}{(0.03526--0.07841)}{4.02pt}{4.28pt}{} & \HoloTaskScore{0.05095}{(0.03061--0.07650)}{4.02pt}{4.28pt}{} & \HoloTaskScore{0.05689}{(0.05557--0.05816)}{4.02pt}{4.28pt}{} & \HoloTaskScore{0.04773}{(0.04609--0.04942)}{4.02pt}{4.28pt}{} & \HoloTaskScore{0.09121}{(0.08991--0.09252)}{4.02pt}{4.28pt}{} & \HoloTaskScore{0.2953}{(0.2924--0.2980)}{4.35pt}{4.62pt}{} & \HoloTaskScore{0.2765}{(0.2739--0.2794)}{4.35pt}{4.62pt}{} \\*
\softcline{4-11}
 &  &  & \HoloTaskMetric{\makecell[c]{\mbox{METEOR}}} & \HoloTaskScore{0.03902}{(0.01630--0.05542)}{4.02pt}{4.28pt}{} & \HoloTaskScore{0.03273}{(0.01305--0.05483)}{4.02pt}{4.28pt}{} & \HoloTaskScore{0.03537}{(0.03433--0.03640)}{4.02pt}{4.28pt}{} & \HoloTaskScore{0.03451}{(0.03332--0.03580)}{4.02pt}{4.28pt}{} & \HoloTaskScore{0.07548}{(0.06420--0.07664)}{4.02pt}{4.28pt}{} & \HoloTaskScore{0.3233}{(0.3195--0.3268)}{4.35pt}{4.62pt}{} & \HoloTaskScore{0.3388}{(0.3352--0.3421)}{4.35pt}{4.62pt}{} \\*
\cline{3-11}
 & \HoloTaskSpan{\makecell[c]{Merlin}}{2.05cm}{0.32cm} &  & \HoloTaskMetric{\makecell[c]{\mbox{RaTE}\\[-0.10ex]\mbox{Score}}} & \HoloTaskScore{0.3164}{(0.2914--0.3478)}{4.35pt}{4.62pt}{} & \HoloTaskScore{0.3108}{(0.2825--0.3434)}{4.35pt}{4.62pt}{} & \HoloTaskScore{0.2991}{(0.2942--0.3037)}{4.35pt}{4.62pt}{} & \HoloTaskScore{0.2865}{(0.2823--0.2906)}{4.35pt}{4.62pt}{} & \HoloTaskScore{0.3257}{(0.3227--0.3286)}{4.35pt}{4.62pt}{} & \HoloTaskScore{0.6766}{(0.6748--0.6784)}{4.35pt}{4.62pt}{} & \HoloTaskScore{0.6589}{(0.6573--0.6606)}{4.35pt}{4.62pt}{} \\*
\softcline{4-11}
 &  & \HoloTaskSpan{{\fontsize{4.35pt}{4.65pt}\selectfont \makecell[c]{\textbf{Clinical}}}}{1.085cm}{0pt} & \HoloTaskMetric{\makecell[c]{\mbox{Llama}\\[-0.10ex]\mbox{Score}}} & \HoloTaskScore{1.627}{(1.497--1.759)}{4.35pt}{4.62pt}{} & \HoloTaskScore{1.529}{(1.392--1.655)}{4.35pt}{4.62pt}{} & \HoloTaskScore{1.866}{(1.814--1.923)}{4.35pt}{4.62pt}{} & \HoloTaskScore{0.8213}{(0.7946--0.8487)}{4.35pt}{4.62pt}{} & \HoloTaskScore{1.904}{(1.873--1.936)}{4.35pt}{4.62pt}{} & \HoloTaskScore{5.518}{(5.475--5.561)}{4.35pt}{4.62pt}{} & \HoloTaskScore{5.114}{(5.073--5.155)}{4.35pt}{4.62pt}{} \\*
\softcline{4-11}
 &  &  & \HoloTaskMetric{\makecell[c]{\mbox{GREEN}}} & \HoloTaskScore{0.01973}{(0.008451--0.03200)}{3.72pt}{3.98pt}{} & \HoloTaskScore{0.01719}{(0.004810--0.03717)}{3.72pt}{3.98pt}{} & \HoloTaskScore{0.01402}{(0.01277--0.01543)}{4.02pt}{4.28pt}{} & \HoloTaskScore{0.02245}{(0.02021--0.02461)}{4.02pt}{4.28pt}{} & \HoloTaskScore{0.02246}{(0.02125--0.02388)}{4.02pt}{4.28pt}{} & \HoloTaskScore{0.3344}{(0.3298--0.3393)}{4.35pt}{4.62pt}{} & \HoloTaskScore{0.3178}{(0.3133--0.3228)}{4.35pt}{4.62pt}{} \\
\cline{2-11}
 &  &  & \HoloTaskMetric{\makecell[c]{\mbox{BLEU-4}}} & \HoloTaskScore{0.2420}{(0.2092--0.2816)}{4.35pt}{4.62pt}{} & \HoloTaskScore{0.2188}{(0.1700--0.2554)}{4.35pt}{4.62pt}{} & \HoloTaskScore{0.08584}{(0.07506--0.09732)}{4.02pt}{4.28pt}{} & \HoloTaskScore{0.1370}{(0.1261--0.1485)}{4.35pt}{4.62pt}{} & \HoloTaskScore{0.4895}{(0.4791--0.4987)}{4.35pt}{4.62pt}{} & \HoloTaskScore{0.6048}{(0.5933--0.6161)}{4.35pt}{4.62pt}{} & \HoloTaskScore{0.6039}{(0.5923--0.6170)}{4.35pt}{4.62pt}{} \\*
\softcline{4-11}
 &  & \HoloTaskSpan{{\fontsize{4.35pt}{4.65pt}\selectfont \makecell[c]{\textbf{NLP}}}}{1.085cm}{0pt} & \HoloTaskMetric{\makecell[c]{\mbox{ROUGE-L}}} & \HoloTaskScore{0.1820}{(0.1419--0.2118)}{4.35pt}{4.62pt}{} & \HoloTaskScore{0.1739}{(0.1373--0.2038)}{4.35pt}{4.62pt}{} & \HoloTaskScore{0.1024}{(0.09696--0.1072)}{4.02pt}{4.28pt}{} & \HoloTaskScore{0.1438}{(0.1381--0.1490)}{4.35pt}{4.62pt}{} & \HoloTaskScore{0.2696}{(0.2647--0.2750)}{4.35pt}{4.62pt}{} & \HoloTaskScore{0.4453}{(0.4336--0.4574)}{4.35pt}{4.62pt}{} & \HoloTaskScore{0.4551}{(0.4430--0.4671)}{4.35pt}{4.62pt}{} \\*
\softcline{4-11}
 &  &  & \HoloTaskMetric{\makecell[c]{\mbox{METEOR}}} & \HoloTaskScore{0.2067}{(0.1634--0.2458)}{4.35pt}{4.62pt}{} & \HoloTaskScore{0.1898}{(0.1444--0.2260)}{4.35pt}{4.62pt}{} & \HoloTaskScore{0.07372}{(0.06861--0.07890)}{4.02pt}{4.28pt}{} & \HoloTaskScore{0.1181}{(0.1122--0.1240)}{4.35pt}{4.62pt}{} & \HoloTaskScore{0.3207}{(0.3150--0.3264)}{4.35pt}{4.62pt}{} & \HoloTaskScore{0.4979}{(0.4868--0.5087)}{4.35pt}{4.62pt}{} & \HoloTaskScore{0.5080}{(0.4957--0.5206)}{4.35pt}{4.62pt}{} \\*
\cline{3-11}
 & \HoloTaskSpan{\makecell[c]{FLARE-2025-\\[-0.10ex]RG}}{2.05cm}{0.32cm} &  & \HoloTaskMetric{\makecell[c]{\mbox{RaTE}\\[-0.10ex]\mbox{Score}}} & \HoloTaskScore{0.5462}{(0.5244--0.5805)}{4.35pt}{4.62pt}{} & \HoloTaskScore{0.5141}{(0.4850--0.5507)}{4.35pt}{4.62pt}{} & \HoloTaskScore{0.4091}{(0.3953--0.4239)}{4.35pt}{4.62pt}{} & \HoloTaskScore{0.5004}{(0.4892--0.5103)}{4.35pt}{4.62pt}{} & \HoloTaskScore{0.6438}{(0.6377--0.6499)}{4.35pt}{4.62pt}{} & \HoloTaskScore{0.7570}{(0.7512--0.7626)}{4.35pt}{4.62pt}{} & \HoloTaskScore{0.7609}{(0.7551--0.7670)}{4.35pt}{4.62pt}{} \\*
\softcline{4-11}
 &  & \HoloTaskSpan{{\fontsize{4.35pt}{4.65pt}\selectfont \makecell[c]{\textbf{Clinical}}}}{1.085cm}{0pt} & \HoloTaskMetric{\makecell[c]{\mbox{Llama}\\[-0.10ex]\mbox{Score}}} & \HoloTaskScore{4.387}{(4.062--4.497)}{4.35pt}{4.62pt}{} & \HoloTaskScore{3.958}{(3.759--4.101)}{4.35pt}{4.62pt}{} & \HoloTaskScore{2.876}{(2.710--3.038)}{4.35pt}{4.62pt}{} & \HoloTaskScore{1.977}{(1.874--2.077)}{4.35pt}{4.62pt}{} & \HoloTaskScore{5.916}{(5.747--6.068)}{4.35pt}{4.62pt}{} & \HoloTaskScore{5.880}{(5.742--6.016)}{4.35pt}{4.62pt}{} & \HoloTaskScore{5.803}{(5.662--5.953)}{4.35pt}{4.62pt}{} \\*
\softcline{4-11}
 &  &  & \HoloTaskMetric{\makecell[c]{\mbox{GREEN}}} & \HoloTaskScore{0.1818}{(0.1360--0.2105)}{4.35pt}{4.62pt}{} & \HoloTaskScore{0.1621}{(0.1284--0.2045)}{4.35pt}{4.62pt}{} & \HoloTaskScore{0.05077}{(0.04280--0.05948)}{4.02pt}{4.28pt}{} & \HoloTaskScore{0.08322}{(0.07352--0.09426)}{4.02pt}{4.28pt}{} & \HoloTaskScore{0.4217}{(0.4028--0.4411)}{4.35pt}{4.62pt}{} & \HoloTaskScore{0.4128}{(0.3962--0.4287)}{4.35pt}{4.62pt}{} & \HoloTaskScore{0.4389}{(0.4218--0.4541)}{4.35pt}{4.62pt}{} \\
\hline
\end{longtable}
\arrayrulecolor{black}
\endgroup
