# Supplementary material for: A 3D foundation model unifying CT interpretation and segmentation
Source: arXiv:2611.06471 source file (2026-11-04)
Supplement: Supplementary file 16 [file table8_grounded_vqa_text_quality.tex]

\begingroup
\makeatletter
\@ifundefined{color@leftblue}{\definecolor{leftblue}{RGB}{232,242,248}}{}%
\@ifundefined{color@headerblue}{\definecolor{headerblue}{RGB}{218,233,242}}{}%
\makeatother
\setlength{\LTcapwidth}{18.60cm}
\setlength{\LTleft}{\fill}
\setlength{\LTright}{\fill}
\setlength{\LTpre}{0pt}
\setlength{\LTpost}{0pt}
\setlength{\tabcolsep}{0.45pt}
\renewcommand{\arraystretch}{1.00}
\setlength{\extrarowheight}{0pt}
\setlength{\arrayrulewidth}{0.48pt}
\arrayrulecolor{black}
\providecommand{\softcline}[1]{}%
\renewcommand{\softcline}[1]{\arrayrulecolor{black!35}\cline{#1}\arrayrulecolor{black}}
\sloppy
\emergencystretch=2em
\fontsize{5.30pt}{5.90pt}\selectfont
\newcommand{\HoloTaskScore}[4]{%
  \parbox[c][0.64cm][c]{2.82cm}{%
    \centering
    {\fontsize{5.30pt}{5.58pt}\selectfont\strut\mbox{#1}}\\[-0.38ex]%
    {\fontsize{#3}{#4}\selectfont\strut\mbox{#2}}%
  }%
}%
\newcommand{\HoloTaskMetricGroup}[1]{%
  \parbox[c][0.64cm][c]{1.31cm}{%
    \centering\fontsize{5.25pt}{5.52pt}\selectfont\textbf{#1}%
  }%
}%
\newcommand{\HoloTaskMetric}[1]{%
  \parbox[c][0.64cm][c]{1.11cm}{%
    \centering\fontsize{5.25pt}{5.52pt}\selectfont\textbf{#1}%
  }%
}%
\newcommand{\HoloTaskRowSpan}[2]{%
  \parbox[c][0.64cm][c]{#2}{%
    \centering\arraybackslash #1%
  }%
}%
\newcommand{\HoloTaskSpan}[3]{%
  \raisebox{\dimexpr#3-0.11cm\relax}[0pt][0pt]{%
    \parbox[c][0.64cm][c]{#2}{%
      \centering\arraybackslash #1%
    }%
  }%
}%
\newcommand{\HoloTaskSplitHead}[3]{%
  \parbox[c][0.92cm][c]{#3}{%
    \centering\fontsize{6.05pt}{6.30pt}\selectfont\textbf{#1}\\[-0.52ex]%
    \rule{0pt}{0.58ex}\\[-0.52ex]\textbf{#2}%
  }%
}%
\newcommand{\HoloTaskMidHead}[2]{%
  \parbox[c][0.92cm][c]{#2}{%
    \centering\fontsize{6.05pt}{6.30pt}\selectfont\textbf{#1}%
  }%
}%
\newcommand{\HoloTaskModelHead}[2]{%
  \parbox[c][0.92cm][c]{#2}{%
    \centering\fontsize{5.45pt}{5.72pt}\selectfont\textbf{#1}%
  }%
}%
\begin{longtable}{|>{\columncolor{leftblue}\centering\arraybackslash}m{1.35cm}|>{\columncolor{leftblue}\centering\arraybackslash}m{2.45cm}|>{\columncolor{leftblue}\centering\arraybackslash}m{1.35cm}|>{\columncolor{leftblue}\centering\arraybackslash}m{1.15cm}|>{\centering\arraybackslash}m{2.85cm}|>{\centering\arraybackslash}m{2.85cm}|>{\centering\arraybackslash}m{2.85cm}|>{\centering\arraybackslash}m{2.85cm}|}
\caption[Effect of grounding on AMOS-MM-VQA and DeepTumorVQA]{\textbf{Close-ended VQA performance of HoloCT with and without grounding on AMOS-MM-VQA and DeepTumorVQA.}\newline Each score is reported as mean with 95\% confidence interval. Accu. denotes accuracy. For AMOS-MM-VQA, Anat.I., Attr.R., Quant.A., Dis.A., Risk.E., and Ther.S. denote anatomical identification, attribute recognition, quantitative assessment, disease analysis, risk evaluation, and therapeutic suggestion, respectively. For DeepTumorVQA, Recog., Meas., Vis.R., and Med.R. denote recognition, measurement, visual reasoning, and medical reasoning, respectively.}%
\label{tab:amos_deeptumor_grounded_comparison}\\[-0.15ex]
\hline
\rowcolor{headerblue}
\HoloTaskSplitHead{Dataset}{Type}{1.35cm} & \HoloTaskSplitHead{Dataset}{Name}{2.45cm} & \HoloTaskMidHead{Category}{1.35cm} & \HoloTaskMidHead{Metric}{1.15cm} & \HoloTaskModelHead{\makecell[c]{HoloCT-4B\\[-0.18ex]w/o grounding}}{2.85cm} & \HoloTaskModelHead{\makecell[c]{HoloCT-4B\\[-0.18ex]w/ grounding}}{2.85cm} & \HoloTaskModelHead{\makecell[c]{HoloCT-8B\\[-0.18ex]w/o grounding}}{2.85cm} & \HoloTaskModelHead{\makecell[c]{HoloCT-8B\\[-0.18ex]w/ grounding}}{2.85cm} \\
\hline
\endfirsthead
\caption*{\textbf{Supplementary Table~\ref{tab:amos_deeptumor_grounded_comparison} (continued)\enspace|\enspace Close-ended VQA performance of HoloCT with and without grounding on AMOS-MM-VQA and DeepTumorVQA.}\newline Each score is reported as mean with 95\% confidence interval. Accu. denotes accuracy. For AMOS-MM-VQA, Anat.I., Attr.R., Quant.A., Dis.A., Risk.E., and Ther.S. denote anatomical identification, attribute recognition, quantitative assessment, disease analysis, risk evaluation, and therapeutic suggestion, respectively. For DeepTumorVQA, Recog., Meas., Vis.R., and Med.R. denote recognition, measurement, visual reasoning, and medical reasoning, respectively.}\\[-0.15ex]
\hline
\rowcolor{headerblue}
\HoloTaskSplitHead{Dataset}{Type}{1.35cm} & \HoloTaskSplitHead{Dataset}{Name}{2.45cm} & \HoloTaskMidHead{Category}{1.35cm} & \HoloTaskMidHead{Metric}{1.15cm} & \HoloTaskModelHead{\makecell[c]{HoloCT-4B\\[-0.18ex]w/o grounding}}{2.85cm} & \HoloTaskModelHead{\makecell[c]{HoloCT-4B\\[-0.18ex]w/ grounding}}{2.85cm} & \HoloTaskModelHead{\makecell[c]{HoloCT-8B\\[-0.18ex]w/o grounding}}{2.85cm} & \HoloTaskModelHead{\makecell[c]{HoloCT-8B\\[-0.18ex]w/ grounding}}{2.85cm} \\
\hline
\endhead
\endfoot
\endlastfoot
 &  & \HoloTaskMetricGroup{Anat.I.} & \HoloTaskMetric{Accu.} & \HoloTaskScore{0.6923}{(0.5577--0.8077)}{4.70pt}{4.98pt} & \HoloTaskScore{0.8269}{(0.7303--0.9231)}{4.70pt}{4.98pt} & \HoloTaskScore{0.7692}{(0.6538--0.8846)}{4.70pt}{4.98pt} & \HoloTaskScore{0.7885}{(0.6731--0.8846)}{4.70pt}{4.98pt} \\*
\cline{3-8}
 &  & \HoloTaskMetricGroup{Attr.R.} & \HoloTaskMetric{Accu.} & \HoloTaskScore{0.9286}{(0.8333--1.000)}{4.70pt}{4.98pt} & \HoloTaskScore{0.9286}{(0.8333--1.000)}{4.70pt}{4.98pt} & \HoloTaskScore{1.000}{(1.000--1.000)}{4.70pt}{4.98pt} & \HoloTaskScore{1.000}{(1.000--1.000)}{4.70pt}{4.98pt} \\*
\cline{3-8}
 &  & \HoloTaskMetricGroup{Quant.A.} & \HoloTaskMetric{Accu.} & \HoloTaskScore{0.7097}{(0.5968--0.8226)}{4.70pt}{4.98pt} & \HoloTaskScore{0.8871}{(0.8065--0.9516)}{4.70pt}{4.98pt} & \HoloTaskScore{0.9032}{(0.8226--0.9677)}{4.70pt}{4.98pt} & \HoloTaskScore{0.8710}{(0.7903--0.9516)}{4.70pt}{4.98pt} \\*
\cline{3-8}
 & \HoloTaskSpan{\makecell[c]{AMOS-MM-VQA}}{2.45cm}{0pt} & \HoloTaskMetricGroup{Dis.A.} & \HoloTaskMetric{Accu.} & \HoloTaskScore{0.8056}{(0.6944--0.9167)}{4.70pt}{4.98pt} & \HoloTaskScore{0.8889}{(0.7778--0.9722)}{4.70pt}{4.98pt} & \HoloTaskScore{0.9167}{(0.8056--1.000)}{4.70pt}{4.98pt} & \HoloTaskScore{0.9444}{(0.8611--1.000)}{4.70pt}{4.98pt} \\*
\cline{3-8}
 &  & \HoloTaskMetricGroup{Risk.E.} & \HoloTaskMetric{Accu.} & \HoloTaskScore{0.7561}{(0.6341--0.8780)}{4.70pt}{4.98pt} & \HoloTaskScore{0.8293}{(0.7073--0.9268)}{4.70pt}{4.98pt} & \HoloTaskScore{0.8780}{(0.7561--0.9756)}{4.70pt}{4.98pt} & \HoloTaskScore{0.9024}{(0.8049--0.9756)}{4.70pt}{4.98pt} \\*
\cline{3-8}
 &  & \HoloTaskMetricGroup{Ther.S.} & \HoloTaskMetric{Accu.} & \HoloTaskScore{0.6333}{(0.4667--0.8000)}{4.70pt}{4.98pt} & \HoloTaskScore{0.8333}{(0.7000--0.9333)}{4.70pt}{4.98pt} & \HoloTaskScore{0.7333}{(0.5667--0.8667)}{4.70pt}{4.98pt} & \HoloTaskScore{0.8667}{(0.7333--0.9667)}{4.70pt}{4.98pt} \\*
\cline{3-8}
\HoloTaskSpan{\makecell[c]{\textbf{Internal}}}{1.35cm}{0.32cm} &  & \HoloTaskMetricGroup{Overall} & \HoloTaskMetric{Accu.} & \HoloTaskScore{0.7529}{(0.6996--0.8024)}{4.70pt}{4.98pt} & \HoloTaskScore{0.8669}{(0.8251--0.9087)}{4.70pt}{4.98pt} & \HoloTaskScore{0.8707}{(0.8289--0.9087)}{4.70pt}{4.98pt} & \HoloTaskScore{0.8897}{(0.8479--0.9278)}{4.70pt}{4.98pt} \\
\cline{2-8}
 &  & \HoloTaskMetricGroup{Recog.} & \HoloTaskMetric{Accu.} & \HoloTaskScore{0.7121}{(0.6800--0.7409)}{4.70pt}{4.98pt} & \HoloTaskScore{0.8627}{(0.8405--0.8848)}{4.70pt}{4.98pt} & \HoloTaskScore{0.8128}{(0.7852--0.8394)}{4.70pt}{4.98pt} & \HoloTaskScore{0.8571}{(0.8339--0.8804)}{4.70pt}{4.98pt} \\*
\cline{3-8}
 &  & \HoloTaskMetricGroup{Meas.} & \HoloTaskMetric{Accu.} & \HoloTaskScore{0.5686}{(0.5421--0.5967)}{4.70pt}{4.98pt} & \HoloTaskScore{0.5818}{(0.5529--0.6083)}{4.70pt}{4.98pt} & \HoloTaskScore{0.5934}{(0.5653--0.6215)}{4.70pt}{4.98pt} & \HoloTaskScore{0.5884}{(0.5595--0.6149)}{4.70pt}{4.98pt} \\*
\cline{3-8}
 & \HoloTaskSpan{\makecell[c]{DeepTumorVQA}}{2.45cm}{0pt} & \HoloTaskMetricGroup{Vis.R.} & \HoloTaskMetric{Accu.} & \HoloTaskScore{0.5812}{(0.5610--0.6022)}{4.70pt}{4.98pt} & \HoloTaskScore{0.5770}{(0.5551--0.5972)}{4.70pt}{4.98pt} & \HoloTaskScore{0.5944}{(0.5738--0.6155)}{4.70pt}{4.98pt} & \HoloTaskScore{0.5780}{(0.5560--0.5981)}{4.70pt}{4.98pt} \\*
\cline{3-8}
 &  & \HoloTaskMetricGroup{Med.R.} & \HoloTaskMetric{Accu.} & \HoloTaskScore{0.6168}{(0.5888--0.6431)}{4.70pt}{4.98pt} & \HoloTaskScore{0.7089}{(0.6826--0.7336)}{4.70pt}{4.98pt} & \HoloTaskScore{0.6752}{(0.6480--0.7015)}{4.70pt}{4.98pt} & \HoloTaskScore{0.6982}{(0.6719--0.7229)}{4.70pt}{4.98pt} \\*
\cline{3-8}
 &  & \HoloTaskMetricGroup{Overall} & \HoloTaskMetric{Accu.} & \HoloTaskScore{0.6077}{(0.5948--0.6206)}{4.70pt}{4.98pt} & \HoloTaskScore{0.6539}{(0.6416--0.6675)}{4.70pt}{4.98pt} & \HoloTaskScore{0.6467}{(0.6340--0.6593)}{4.70pt}{4.98pt} & \HoloTaskScore{0.6525}{(0.6405--0.6657)}{4.70pt}{4.98pt} \\
\hline
\end{longtable}
\arrayrulecolor{black}
\endgroup
