# Supplementary material for: A 3D foundation model unifying CT interpretation and segmentation
Source: arXiv:2611.06471 source file (2026-11-04)
Supplement: Supplementary file 17 [file table9_grounded_vqa_segmentation_quality.tex]

\begingroup
\makeatletter
\@ifundefined{color@leftblue}{\definecolor{leftblue}{RGB}{232,242,248}}{}%
\@ifundefined{color@headerblue}{\definecolor{headerblue}{RGB}{218,233,242}}{}%
\makeatother
\setlength{\LTcapwidth}{18.60cm}
\setlength{\LTleft}{\fill}
\setlength{\LTright}{\fill}
\setlength{\LTpre}{0pt}
\setlength{\LTpost}{0pt}
\setlength{\tabcolsep}{0.45pt}
\renewcommand{\arraystretch}{1.00}
\setlength{\extrarowheight}{0pt}
\setlength{\arrayrulewidth}{0.48pt}
\arrayrulecolor{black}
\providecommand{\softcline}[1]{}%
\renewcommand{\softcline}[1]{\arrayrulecolor{black!35}\cline{#1}\arrayrulecolor{black}}
\sloppy
\emergencystretch=2em
\fontsize{5.30pt}{5.90pt}\selectfont
\newcommand{\HoloSegScore}[4]{%
  \parbox[c][0.64cm][c]{2.07cm}{%
    \centering
    {\fontsize{5.30pt}{5.58pt}\selectfont\strut\mbox{#1}}\\[-0.38ex]%
    {\fontsize{#3}{#4}\selectfont\strut\mbox{#2}}%
  }%
}%
\newcommand{\HoloSegUnsupported}{%
  \parbox[c][0.64cm][c]{2.07cm}{%
    \centering\fontsize{4.45pt}{4.70pt}\selectfont Not supported%
  }%
}%
\newcommand{\HoloSegMetric}[1]{%
  \parbox[c][0.64cm][c]{0.86cm}{%
    \centering\fontsize{5.45pt}{5.70pt}\selectfont\textbf{#1}%
  }%
}%
\newcommand{\HoloSegSpan}[3]{%
  \raisebox{#3}[0pt][0pt]{%
    \parbox[c]{#2}{\centering\arraybackslash #1}%
  }%
}%
\newcommand{\HoloSegSplitHead}[3]{%
  \parbox[c][0.92cm][c]{#3}{%
    \centering\fontsize{6.10pt}{6.35pt}\selectfont\textbf{#1}\\[-0.52ex]%
    \rule{0pt}{0.58ex}\\[-0.52ex]\textbf{#2}%
  }%
}%
\newcommand{\HoloSegMidHead}[2]{%
  \parbox[c][0.92cm][c]{#2}{%
    \centering\fontsize{5.55pt}{5.80pt}\selectfont\textbf{#1}%
  }%
}%
\begin{longtable}{|>{\columncolor{leftblue}\centering\arraybackslash}m{1.20cm}|>{\columncolor{leftblue}\centering\arraybackslash}m{2.10cm}|>{\columncolor{leftblue}\centering\arraybackslash}m{2.90cm}|>{\columncolor{leftblue}\centering\arraybackslash}m{0.90cm}|>{\centering\arraybackslash}m{2.10cm}|>{\centering\arraybackslash}m{1.25cm}|>{\centering\arraybackslash}m{2.10cm}|>{\centering\arraybackslash}m{2.10cm}|>{\centering\arraybackslash}m{1.25cm}|>{\centering\arraybackslash}m{2.10cm}|}
\caption[Segmentation performance on AMOS-MM-VQA and DeepTumorVQA]{\textbf{Segmentation performance of HoloCT segmentation and grounded variants on AMOS-MM-VQA and DeepTumorVQA.}\newline Each score is reported as mean with 95\% confidence interval. Match counts denote matched/reference objects; grounded Dice and HD95 use matched objects. Dice measures volumetric overlap; HD95 denotes the 95th-percentile Hausdorff distance in millimetres.}%
\label{tab:amos_deeptumor_segmentation_comparison}\\[-0.15ex]
\hline
\rowcolor{headerblue}
\HoloSegSplitHead{Dataset}{Type}{1.20cm} & \HoloSegSplitHead{Dataset}{Name}{2.10cm} & \HoloSegSplitHead{Label}{Name}{2.90cm} & \HoloSegMidHead{Metric}{0.90cm} & \HoloSegMidHead{\makecell[c]{HoloCT-4B\\[-0.18ex]Segmentation-\\[-0.18ex]only}}{2.10cm} & \HoloSegMidHead{\makecell[c]{Match\\count-4B}}{1.25cm} & \HoloSegMidHead{\makecell[c]{HoloCT-4B\\[-0.18ex]w/ grounding}}{2.10cm} & \HoloSegMidHead{\makecell[c]{HoloCT-8B\\[-0.18ex]Segmentation-\\[-0.18ex]only}}{2.10cm} & \HoloSegMidHead{\makecell[c]{Match\\count-8B}}{1.25cm} & \HoloSegMidHead{\makecell[c]{HoloCT-8B\\[-0.18ex]w/ grounding}}{2.10cm} \\
\hline
\endfirsthead
\caption*{\textbf{Supplementary Table~\ref{tab:amos_deeptumor_segmentation_comparison} (continued)\enspace|\enspace Segmentation performance of HoloCT segmentation and grounded variants on AMOS-MM-VQA and DeepTumorVQA.}\newline Each score is reported as mean with 95\% confidence interval. Match counts denote matched/reference objects; grounded Dice and HD95 use matched objects. Dice measures volumetric overlap; HD95 denotes the 95th-percentile Hausdorff distance in millimetres.}\\[-0.15ex]
\hline
\rowcolor{headerblue}
\HoloSegSplitHead{Dataset}{Type}{1.20cm} & \HoloSegSplitHead{Dataset}{Name}{2.10cm} & \HoloSegSplitHead{Label}{Name}{2.90cm} & \HoloSegMidHead{Metric}{0.90cm} & \HoloSegMidHead{\makecell[c]{HoloCT-4B\\[-0.18ex]Segmentation-\\[-0.18ex]only}}{2.10cm} & \HoloSegMidHead{\makecell[c]{Match\\count-4B}}{1.25cm} & \HoloSegMidHead{\makecell[c]{HoloCT-4B\\[-0.18ex]w/ grounding}}{2.10cm} & \HoloSegMidHead{\makecell[c]{HoloCT-8B\\[-0.18ex]Segmentation-\\[-0.18ex]only}}{2.10cm} & \HoloSegMidHead{\makecell[c]{Match\\count-8B}}{1.25cm} & \HoloSegMidHead{\makecell[c]{HoloCT-8B\\[-0.18ex]w/ grounding}}{2.10cm} \\
\hline
\endhead
\endfoot
\endlastfoot
 &  &  & \HoloSegMetric{Dice} & \HoloSegScore{0.9598}{(0.9453--0.9733)}{4.55pt}{4.82pt} &  & \HoloSegScore{0.9520}{(0.9248--0.9731)}{4.55pt}{4.82pt} & \HoloSegScore{0.9431}{(0.9196--0.9631)}{4.55pt}{4.82pt} &  & \HoloSegScore{0.9383}{(0.9111--0.9625)}{4.55pt}{4.82pt} \\*
\softcline{4-5}\softcline{7-8}\softcline{10-10}
 &  & \HoloSegSpan{\makecell[c]{spleen}}{2.90cm}{0.32cm} & \HoloSegMetric{HD95} & \HoloSegScore{3.535}{(1.379--7.313)}{4.55pt}{4.82pt} & \HoloSegSpan{9/12}{1.25cm}{0.32cm} & \HoloSegScore{4.394}{(1.325--10.13)}{4.55pt}{4.82pt} & \HoloSegScore{4.877}{(1.898--8.202)}{4.55pt}{4.82pt} & \HoloSegSpan{10/12}{1.25cm}{0.32cm} & \HoloSegScore{5.040}{(1.842--9.093)}{4.55pt}{4.82pt} \\
\cline{3-10}
 &  &  & \HoloSegMetric{Dice} & \HoloSegScore{0.9513}{(0.9366--0.9636)}{4.55pt}{4.82pt} &  & \HoloSegScore{0.9493}{(0.9343--0.9626)}{4.55pt}{4.82pt} & \HoloSegScore{0.9503}{(0.9378--0.9614)}{4.55pt}{4.82pt} &  & \HoloSegScore{0.9462}{(0.9332--0.9582)}{4.55pt}{4.82pt} \\*
\softcline{4-5}\softcline{7-8}\softcline{10-10}
 &  & \HoloSegSpan{\makecell[c]{right kidney}}{2.90cm}{0.32cm} & \HoloSegMetric{HD95} & \HoloSegScore{5.181}{(1.681--10.62)}{4.55pt}{4.82pt} & \HoloSegSpan{45/45}{1.25cm}{0.32cm} & \HoloSegScore{5.410}{(1.747--11.21)}{4.55pt}{4.82pt} & \HoloSegScore{3.361}{(1.758--5.521)}{4.55pt}{4.82pt} & \HoloSegSpan{42/45}{1.25cm}{0.32cm} & \HoloSegScore{5.020}{(2.240--8.785)}{4.55pt}{4.82pt} \\
\cline{3-10}
 &  &  & \HoloSegMetric{Dice} & \HoloSegScore{0.9484}{(0.9291--0.9625)}{4.55pt}{4.82pt} &  & \HoloSegScore{0.9497}{(0.9354--0.9617)}{4.55pt}{4.82pt} & \HoloSegScore{0.9368}{(0.9080--0.9595)}{4.55pt}{4.82pt} &  & \HoloSegScore{0.9358}{(0.9078--0.9580)}{4.55pt}{4.82pt} \\*
\softcline{4-5}\softcline{7-8}\softcline{10-10}
 &  & \HoloSegSpan{\makecell[c]{left kidney}}{2.90cm}{0.32cm} & \HoloSegMetric{HD95} & \HoloSegScore{2.924}{(1.672--4.524)}{4.55pt}{4.82pt} & \HoloSegSpan{43/44}{1.25cm}{0.32cm} & \HoloSegScore{2.930}{(1.668--4.566)}{4.55pt}{4.82pt} & \HoloSegScore{3.886}{(1.653--7.375)}{4.55pt}{4.82pt} & \HoloSegSpan{42/44}{1.25cm}{0.32cm} & \HoloSegScore{7.016}{(1.559--14.20)}{4.55pt}{4.82pt} \\
\cline{3-10}
 &  &  & \HoloSegMetric{Dice} & \HoloSegScore{0.8687}{(0.8289--0.9091)}{4.55pt}{4.82pt} &  & \HoloSegScore{0.8728}{(0.8300--0.9125)}{4.55pt}{4.82pt} & \HoloSegScore{0.8790}{(0.8245--0.9285)}{4.55pt}{4.82pt} &  & \HoloSegScore{0.8790}{(0.8163--0.9280)}{4.55pt}{4.82pt} \\*
\softcline{4-5}\softcline{7-8}\softcline{10-10}
 &  & \HoloSegSpan{\makecell[c]{gallbladder}}{2.90cm}{0.32cm} & \HoloSegMetric{HD95} & \HoloSegScore{7.831}{(4.046--12.19)}{4.55pt}{4.82pt} & \HoloSegSpan{24/26}{1.25cm}{0.32cm} & \HoloSegScore{7.453}{(3.611--12.05)}{4.55pt}{4.82pt} & \HoloSegScore{7.239}{(3.035--13.00)}{4.55pt}{4.82pt} & \HoloSegSpan{25/26}{1.25cm}{0.32cm} & \HoloSegScore{7.488}{(3.085--14.03)}{4.55pt}{4.82pt} \\
\cline{3-10}
 &  &  & \HoloSegMetric{Dice} & \HoloSegScore{0.8823}{(0.8823--0.8823)}{4.55pt}{4.82pt} &  & \HoloSegScore{0.8869}{(0.8869--0.8869)}{4.55pt}{4.82pt} & \HoloSegScore{0.8338}{(0.8338--0.8338)}{4.55pt}{4.82pt} &  & \HoloSegScore{0.8395}{(0.8395--0.8395)}{4.55pt}{4.82pt} \\*
\softcline{4-5}\softcline{7-8}\softcline{10-10}
 &  & \HoloSegSpan{\makecell[c]{esophagus}}{2.90cm}{0.32cm} & \HoloSegMetric{HD95} & \HoloSegScore{2.751}{(2.751--2.751)}{4.55pt}{4.82pt} & \HoloSegSpan{2/3}{1.25cm}{0.32cm} & \HoloSegScore{2.461}{(2.461--2.461)}{4.55pt}{4.82pt} & \HoloSegScore{4.922}{(4.922--4.922)}{4.55pt}{4.82pt} & \HoloSegSpan{2/3}{1.25cm}{0.32cm} & \HoloSegScore{4.685}{(4.685--4.685)}{4.55pt}{4.82pt} \\
\cline{3-10}
 &  &  & \HoloSegMetric{Dice} & \HoloSegScore{0.9672}{(0.9599--0.9725)}{4.55pt}{4.82pt} &  & \HoloSegScore{0.9694}{(0.9642--0.9735)}{4.55pt}{4.82pt} & \HoloSegScore{0.9684}{(0.9651--0.9716)}{4.55pt}{4.82pt} &  & \HoloSegScore{0.9694}{(0.9662--0.9724)}{4.55pt}{4.82pt} \\*
\softcline{4-5}\softcline{7-8}\softcline{10-10}
 &  & \HoloSegSpan{\makecell[c]{liver}}{2.90cm}{0.32cm} & \HoloSegMetric{HD95} & \HoloSegScore{3.555}{(2.463--5.295)}{4.55pt}{4.82pt} & \HoloSegSpan{84/87}{1.25cm}{0.32cm} & \HoloSegScore{3.334}{(2.361--4.813)}{4.55pt}{4.82pt} & \HoloSegScore{3.503}{(2.880--4.269)}{4.55pt}{4.82pt} & \HoloSegSpan{83/87}{1.25cm}{0.32cm} & \HoloSegScore{3.115}{(2.640--3.646)}{4.55pt}{4.82pt} \\
\cline{3-10}
 & \HoloSegSpan{\makecell[c]{AMOS-MM-VQA}}{2.10cm}{0.32cm} &  & \HoloSegMetric{Dice} & \HoloSegScore{0.7155}{(0.3183--0.9334)}{4.55pt}{4.82pt} &  & \HoloSegScore{0.7184}{(0.3191--0.9373)}{4.55pt}{4.82pt} & \HoloSegScore{0.6953}{(0.3133--0.9104)}{4.55pt}{4.82pt} &  & \HoloSegScore{0.6920}{(0.3144--0.9092)}{4.55pt}{4.82pt} \\*
\softcline{4-5}\softcline{7-8}\softcline{10-10}
 &  & \HoloSegSpan{\makecell[c]{stomach}}{2.90cm}{0.32cm} & \HoloSegMetric{HD95} & \HoloSegScore{24.63}{(5.719--59.93)}{4.55pt}{4.82pt} & \HoloSegSpan{6/6}{1.25cm}{0.32cm} & \HoloSegScore{23.59}{(4.641--58.33)}{4.55pt}{4.82pt} & \HoloSegScore{25.91}{(8.651--56.16)}{4.55pt}{4.82pt} & \HoloSegSpan{6/6}{1.25cm}{0.32cm} & \HoloSegScore{26.81}{(10.10--54.41)}{4.55pt}{4.82pt} \\
\cline{3-10}
 &  &  & \HoloSegMetric{Dice} & \HoloSegScore{0.9025}{(0.9012--0.9037)}{4.55pt}{4.82pt} &  & \HoloSegScore{0.9080}{(0.8921--0.9238)}{4.55pt}{4.82pt} & \HoloSegScore{0.9082}{(0.9082--0.9082)}{4.55pt}{4.82pt} &  & \HoloSegScore{0.9075}{(0.9075--0.9075)}{4.55pt}{4.82pt} \\*
\softcline{4-5}\softcline{7-8}\softcline{10-10}
 &  & \HoloSegSpan{\makecell[c]{aorta}}{2.90cm}{0.32cm} & \HoloSegMetric{HD95} & \HoloSegScore{36.01}{(8.463--63.56)}{4.55pt}{4.82pt} & \HoloSegSpan{3/3}{1.25cm}{0.32cm} & \HoloSegScore{41.30}{(19.43--63.17)}{4.55pt}{4.82pt} & \HoloSegScore{2.414}{(2.414--2.414)}{4.55pt}{4.82pt} & \HoloSegSpan{2/3}{1.25cm}{0.32cm} & \HoloSegScore{2.545}{(2.545--2.545)}{4.55pt}{4.82pt} \\
\cline{3-10}
 &  &  & \HoloSegMetric{Dice} & \HoloSegScore{0.6788}{(0.3859--0.8834)}{4.55pt}{4.82pt} &  & \HoloSegScore{0.6811}{(0.3897--0.8808)}{4.55pt}{4.82pt} & \HoloSegScore{0.7034}{(0.4378--0.8558)}{4.55pt}{4.82pt} &  & \HoloSegScore{0.7020}{(0.4390--0.8553)}{4.55pt}{4.82pt} \\*
\softcline{4-5}\softcline{7-8}\softcline{10-10}
 &  & \HoloSegSpan{\makecell[c]{pancreas}}{2.90cm}{0.32cm} & \HoloSegMetric{HD95} & \HoloSegScore{18.20}{(3.661--41.24)}{4.55pt}{4.82pt} & \HoloSegSpan{18/20}{1.25cm}{0.32cm} & \HoloSegScore{18.18}{(3.774--42.11)}{4.55pt}{4.82pt} & \HoloSegScore{15.28}{(4.080--39.62)}{4.55pt}{4.82pt} & \HoloSegSpan{19/20}{1.25cm}{0.32cm} & \HoloSegScore{15.49}{(4.092--39.52)}{4.55pt}{4.82pt} \\
\cline{3-10}
\HoloSegSpan{\makecell[c]{\textbf{Internal}}}{1.20cm}{0.32cm} &  &  & \HoloSegMetric{Dice} & \HoloSegScore{0.6892}{(0.6892--0.6892)}{4.55pt}{4.82pt} &  & \HoloSegScore{0.6687}{(0.6687--0.6687)}{4.55pt}{4.82pt} & \HoloSegScore{0.8427}{(0.8427--0.8427)}{4.55pt}{4.82pt} &  & \HoloSegScore{0.8357}{(0.8357--0.8357)}{4.55pt}{4.82pt} \\*
\softcline{4-5}\softcline{7-8}\softcline{10-10}
 &  & \HoloSegSpan{\makecell[c]{left adrenal gland}}{2.90cm}{0.32cm} & \HoloSegMetric{HD95} & \HoloSegScore{3.910}{(3.910--3.910)}{4.55pt}{4.82pt} & \HoloSegSpan{2/2}{1.25cm}{0.32cm} & \HoloSegScore{3.910}{(3.910--3.910)}{4.55pt}{4.82pt} & \HoloSegScore{1.564}{(1.564--1.564)}{4.55pt}{4.82pt} & \HoloSegSpan{2/2}{1.25cm}{0.32cm} & \HoloSegScore{1.564}{(1.564--1.564)}{4.55pt}{4.82pt} \\
\cline{3-10}
 &  &  & \HoloSegMetric{Dice} & \HoloSegScore{0.8488}{(0.7902--0.9073)}{4.55pt}{4.82pt} &  & \HoloSegScore{0.8499}{(0.8009--0.8989)}{4.55pt}{4.82pt} & \HoloSegScore{0.8435}{(0.8114--0.8757)}{4.55pt}{4.82pt} &  & \HoloSegScore{0.8454}{(0.8299--0.8609)}{4.55pt}{4.82pt} \\*
\softcline{4-5}\softcline{7-8}\softcline{10-10}
 &  & \HoloSegSpan{\makecell[c]{urinary bladder}}{2.90cm}{0.32cm} & \HoloSegMetric{HD95} & \HoloSegScore{6.087}{(4.281--7.894)}{4.55pt}{4.82pt} & \HoloSegSpan{3/4}{1.25cm}{0.32cm} & \HoloSegScore{5.669}{(4.641--6.697)}{4.55pt}{4.82pt} & \HoloSegScore{5.000}{(5.000--5.000)}{4.55pt}{4.82pt} & \HoloSegSpan{2/4}{1.25cm}{0.32cm} & \HoloSegScore{5.000}{(5.000--5.000)}{4.55pt}{4.82pt} \\
\cline{3-10}
 &  &  & \HoloSegMetric{Dice} & \HoloSegScore{0.8864}{(0.8603--0.9101)}{4.55pt}{4.82pt} &  & \HoloSegScore{0.8876}{(0.8621--0.9112)}{4.55pt}{4.82pt} & \HoloSegScore{0.8729}{(0.8453--0.8978)}{4.55pt}{4.82pt} &  & \HoloSegScore{0.8845}{(0.8582--0.9089)}{4.55pt}{4.82pt} \\*
\softcline{4-5}\softcline{7-8}\softcline{10-10}
 &  & \HoloSegSpan{\makecell[c]{prostate or uterus}}{2.90cm}{0.32cm} & \HoloSegMetric{HD95} & \HoloSegScore{6.473}{(4.138--9.533)}{4.55pt}{4.82pt} & \HoloSegSpan{28/30}{1.25cm}{0.32cm} & \HoloSegScore{5.730}{(3.695--8.594)}{4.55pt}{4.82pt} & \HoloSegScore{56.25}{(12.57--107.3)}{4.55pt}{4.82pt} & \HoloSegSpan{29/30}{1.25cm}{0.32cm} & \HoloSegScore{32.63}{(6.226--68.06)}{4.55pt}{4.82pt} \\
\cline{2-10}
 &  &  & \HoloSegMetric{Dice} & \HoloSegScore{0.8973}{(0.8776--0.9157)}{4.55pt}{4.82pt} &  & \HoloSegScore{0.8823}{(0.8589--0.9038)}{4.55pt}{4.82pt} & \HoloSegScore{0.8923}{(0.8690--0.9141)}{4.55pt}{4.82pt} &  & \HoloSegScore{0.8893}{(0.8637--0.9119)}{4.55pt}{4.82pt} \\*
\softcline{4-5}\softcline{7-8}\softcline{10-10}
 &  & \HoloSegSpan{\makecell[c]{colon}}{2.90cm}{0.32cm} & \HoloSegMetric{HD95} & \HoloSegScore{11.82}{(5.794--18.78)}{4.55pt}{4.82pt} & \HoloSegSpan{18/31}{1.25cm}{0.32cm} & \HoloSegScore{13.68}{(7.184--21.02)}{4.55pt}{4.82pt} & \HoloSegScore{13.99}{(7.450--20.91)}{4.55pt}{4.82pt} & \HoloSegSpan{17/31}{1.25cm}{0.32cm} & \HoloSegScore{15.07}{(8.466--22.90)}{4.55pt}{4.82pt} \\
\cline{3-10}
 &  &  & \HoloSegMetric{Dice} & \HoloSegScore{0.8169}{(0.7514--0.8824)}{4.55pt}{4.82pt} &  & \HoloSegScore{0.8158}{(0.7544--0.8772)}{4.55pt}{4.82pt} & \HoloSegScore{0.8500}{(0.7412--0.9044)}{4.55pt}{4.82pt} &  & \HoloSegScore{0.8480}{(0.7429--0.9008)}{4.55pt}{4.82pt} \\*
\softcline{4-5}\softcline{7-8}\softcline{10-10}
 &  & \HoloSegSpan{\makecell[c]{intestine}}{2.90cm}{0.32cm} & \HoloSegMetric{HD95} & \HoloSegScore{14.08}{(5.651--22.51)}{4.55pt}{4.82pt} & \HoloSegSpan{6/10}{1.25cm}{0.32cm} & \HoloSegScore{14.48}{(6.162--22.79)}{4.55pt}{4.82pt} & \HoloSegScore{12.53}{(5.260--23.06)}{4.55pt}{4.82pt} & \HoloSegSpan{4/10}{1.25cm}{0.32cm} & \HoloSegScore{12.82}{(5.000--23.18)}{4.55pt}{4.82pt} \\
\cline{3-10}
 &  &  & \HoloSegMetric{Dice} & \HoloSegScore{0.9490}{(0.9408--0.9564)}{4.55pt}{4.82pt} &  & \HoloSegScore{0.9484}{(0.9400--0.9560)}{4.55pt}{4.82pt} & \HoloSegScore{0.9475}{(0.9396--0.9546)}{4.55pt}{4.82pt} &  & \HoloSegScore{0.9481}{(0.9399--0.9554)}{4.55pt}{4.82pt} \\*
\softcline{4-5}\softcline{7-8}\softcline{10-10}
 &  & \HoloSegSpan{\makecell[c]{left kidney}}{2.90cm}{0.32cm} & \HoloSegMetric{HD95} & \HoloSegScore{4.505}{(3.353--5.719)}{4.55pt}{4.82pt} & \HoloSegSpan{671/749}{1.25cm}{0.32cm} & \HoloSegScore{5.129}{(3.879--6.437)}{4.55pt}{4.82pt} & \HoloSegScore{4.495}{(3.535--5.568)}{4.55pt}{4.82pt} & \HoloSegSpan{710/749}{1.25cm}{0.32cm} & \HoloSegScore{4.302}{(3.299--5.389)}{4.55pt}{4.82pt} \\
\cline{3-10}
 & \HoloSegSpan{\makecell[c]{DeepTumorVQA}}{2.10cm}{0.32cm} &  & \HoloSegMetric{Dice} & \HoloSegScore{0.6474}{(0.6100--0.6865)}{4.55pt}{4.82pt} &  & \HoloSegScore{0.6589}{(0.6222--0.6975)}{4.55pt}{4.82pt} & \HoloSegScore{0.7025}{(0.6706--0.7353)}{4.55pt}{4.82pt} &  & \HoloSegScore{0.7061}{(0.6724--0.7387)}{4.55pt}{4.82pt} \\*
\softcline{4-5}\softcline{7-8}\softcline{10-10}
 &  & \HoloSegSpan{\makecell[c]{kidney lesion}}{2.90cm}{0.32cm} & \HoloSegMetric{HD95} & \HoloSegScore{38.35}{(30.85--45.69)}{4.55pt}{4.82pt} & \HoloSegSpan{620/624}{1.25cm}{0.32cm} & \HoloSegScore{42.66}{(34.73--50.05)}{4.55pt}{4.82pt} & \HoloSegScore{39.48}{(32.20--47.08)}{4.55pt}{4.82pt} & \HoloSegSpan{590/624}{1.25cm}{0.32cm} & \HoloSegScore{37.48}{(31.04--44.71)}{4.55pt}{4.82pt} \\
\cline{3-10}
 &  &  & \HoloSegMetric{Dice} & \HoloSegScore{0.9563}{(0.9503--0.9615)}{4.55pt}{4.82pt} &  & \HoloSegScore{0.9567}{(0.9505--0.9624)}{4.55pt}{4.82pt} & \HoloSegScore{0.9567}{(0.9498--0.9621)}{4.55pt}{4.82pt} &  & \HoloSegScore{0.9562}{(0.9492--0.9621)}{4.55pt}{4.82pt} \\*
\softcline{4-5}\softcline{7-8}\softcline{10-10}
 &  & \HoloSegSpan{\makecell[c]{right kidney}}{2.90cm}{0.32cm} & \HoloSegMetric{HD95} & \HoloSegScore{3.588}{(2.918--4.390)}{4.55pt}{4.82pt} & \HoloSegSpan{660/747}{1.25cm}{0.32cm} & \HoloSegScore{3.892}{(2.962--5.157)}{4.55pt}{4.82pt} & \HoloSegScore{3.461}{(2.742--4.317)}{4.55pt}{4.82pt} & \HoloSegSpan{691/747}{1.25cm}{0.32cm} & \HoloSegScore{3.250}{(2.533--4.085)}{4.55pt}{4.82pt} \\
\cline{3-10}
 &  &  & \HoloSegMetric{Dice} & \HoloSegScore{0.9738}{(0.9710--0.9758)}{4.55pt}{4.82pt} &  & \HoloSegScore{0.9734}{(0.9707--0.9755)}{4.55pt}{4.82pt} & \HoloSegScore{0.9723}{(0.9694--0.9744)}{4.55pt}{4.82pt} &  & \HoloSegScore{0.9726}{(0.9696--0.9748)}{4.55pt}{4.82pt} \\*
\softcline{4-5}\softcline{7-8}\softcline{10-10}
 &  & \HoloSegSpan{\makecell[c]{liver}}{2.90cm}{0.32cm} & \HoloSegMetric{HD95} & \HoloSegScore{4.112}{(3.490--4.797)}{4.55pt}{4.82pt} & \HoloSegSpan{647/721}{1.25cm}{0.32cm} & \HoloSegScore{4.252}{(3.620--4.954)}{4.55pt}{4.82pt} & \HoloSegScore{4.164}{(3.534--4.905)}{4.55pt}{4.82pt} & \HoloSegSpan{645/721}{1.25cm}{0.32cm} & \HoloSegScore{4.139}{(3.492--4.902)}{4.55pt}{4.82pt} \\
\hline
\pagebreak[4]
 &  &  & \HoloSegMetric{Dice} & \HoloSegScore{0.6981}{(0.6684--0.7261)}{4.55pt}{4.82pt} &  & \HoloSegScore{0.7031}{(0.6753--0.7305)}{4.55pt}{4.82pt} & \HoloSegScore{0.6917}{(0.6601--0.7194)}{4.55pt}{4.82pt} &  & \HoloSegScore{0.6873}{(0.6554--0.7152)}{4.55pt}{4.82pt} \\*
\softcline{4-5}\softcline{7-8}\softcline{10-10}
 &  & \HoloSegSpan{\makecell[c]{liver lesion}}{2.90cm}{0.32cm} & \HoloSegMetric{HD95} & \HoloSegScore{24.92}{(20.34--29.58)}{4.55pt}{4.82pt} & \HoloSegSpan{1047/1063}{1.25cm}{0.32cm} & \HoloSegScore{25.15}{(20.63--29.63)}{4.55pt}{4.82pt} & \HoloSegScore{40.18}{(34.29--47.56)}{4.55pt}{4.82pt} & \HoloSegSpan{1034/1063}{1.25cm}{0.32cm} & \HoloSegScore{39.42}{(33.57--46.52)}{4.55pt}{4.82pt} \\
\cline{3-10}
 &  &  & \HoloSegMetric{Dice} & \HoloSegScore{0.8221}{(0.8058--0.8370)}{4.55pt}{4.82pt} &  & \HoloSegScore{0.8153}{(0.7982--0.8310)}{4.55pt}{4.82pt} & \HoloSegScore{0.8243}{(0.8103--0.8384)}{4.55pt}{4.82pt} &  & \HoloSegScore{0.8273}{(0.8118--0.8420)}{4.55pt}{4.82pt} \\*
\softcline{4-5}\softcline{7-8}\softcline{10-10}
 &  & \HoloSegSpan{\makecell[c]{caudate lobe}}{2.90cm}{0.32cm} & \HoloSegMetric{HD95} & \HoloSegScore{6.987}{(6.230--7.800)}{4.55pt}{4.82pt} & \HoloSegSpan{127/131}{1.25cm}{0.32cm} & \HoloSegScore{7.214}{(6.421--8.082)}{4.55pt}{4.82pt} & \HoloSegScore{6.820}{(6.010--7.629)}{4.55pt}{4.82pt} & \HoloSegSpan{125/131}{1.25cm}{0.32cm} & \HoloSegScore{6.803}{(6.001--7.639)}{4.55pt}{4.82pt} \\
\cline{3-10}
 &  &  & \HoloSegMetric{Dice} & \HoloSegScore{0.9064}{(0.8882--0.9210)}{4.55pt}{4.82pt} &  & \HoloSegScore{0.9058}{(0.8889--0.9198)}{4.55pt}{4.82pt} & \HoloSegScore{0.9014}{(0.8798--0.9165)}{4.55pt}{4.82pt} &  & \HoloSegScore{0.8979}{(0.8753--0.9138)}{4.55pt}{4.82pt} \\*
\softcline{4-5}\softcline{7-8}\softcline{10-10}
 &  & \HoloSegSpan{\makecell[c]{left lateral superior\\[-0.10ex]segment of liver}}{2.90cm}{0.32cm} & \HoloSegMetric{HD95} & \HoloSegScore{7.427}{(6.136--8.953)}{4.55pt}{4.82pt} & \HoloSegSpan{111/114}{1.25cm}{0.32cm} & \HoloSegScore{7.746}{(6.497--9.263)}{4.55pt}{4.82pt} & \HoloSegScore{7.077}{(5.739--8.853)}{4.55pt}{4.82pt} & \HoloSegSpan{110/114}{1.25cm}{0.32cm} & \HoloSegScore{7.918}{(6.112--10.15)}{4.55pt}{4.82pt} \\
\cline{3-10}
 &  &  & \HoloSegMetric{Dice} & \HoloSegScore{0.9090}{(0.8976--0.9202)}{4.55pt}{4.82pt} &  & \HoloSegScore{0.9091}{(0.8976--0.9207)}{4.55pt}{4.82pt} & \HoloSegScore{0.9094}{(0.8977--0.9202)}{4.55pt}{4.82pt} &  & \HoloSegScore{0.8969}{(0.8800--0.9113)}{4.55pt}{4.82pt} \\*
\softcline{4-5}\softcline{7-8}\softcline{10-10}
 &  & \HoloSegSpan{\makecell[c]{left lateral inferior\\[-0.10ex]segment of liver}}{2.90cm}{0.32cm} & \HoloSegMetric{HD95} & \HoloSegScore{5.320}{(4.443--6.253)}{4.55pt}{4.82pt} & \HoloSegSpan{101/103}{1.25cm}{0.32cm} & \HoloSegScore{5.310}{(4.423--6.207)}{4.55pt}{4.82pt} & \HoloSegScore{7.250}{(5.226--10.29)}{4.55pt}{4.82pt} & \HoloSegSpan{100/103}{1.25cm}{0.32cm} & \HoloSegScore{10.41}{(7.114--14.48)}{4.55pt}{4.82pt} \\
\cline{3-10}
 &  &  & \HoloSegMetric{Dice} & \HoloSegScore{0.8669}{(0.8452--0.8833)}{4.55pt}{4.82pt} &  & \HoloSegScore{0.8630}{(0.8415--0.8800)}{4.55pt}{4.82pt} & \HoloSegScore{0.8585}{(0.8341--0.8798)}{4.55pt}{4.82pt} &  & \HoloSegScore{0.8648}{(0.8422--0.8834)}{4.55pt}{4.82pt} \\*
\softcline{4-5}\softcline{7-8}\softcline{10-10}
 &  & \HoloSegSpan{\makecell[c]{left medial segment\\[-0.10ex]of liver}}{2.90cm}{0.32cm} & \HoloSegMetric{HD95} & \HoloSegScore{12.01}{(9.492--15.42)}{4.55pt}{4.82pt} & \HoloSegSpan{154/158}{1.25cm}{0.32cm} & \HoloSegScore{14.67}{(11.77--18.43)}{4.55pt}{4.82pt} & \HoloSegScore{10.01}{(8.014--12.52)}{4.55pt}{4.82pt} & \HoloSegSpan{153/158}{1.25cm}{0.32cm} & \HoloSegScore{12.80}{(9.575--16.77)}{4.55pt}{4.82pt} \\
\cline{3-10}
 &  &  & \HoloSegMetric{Dice} & \HoloSegScore{0.8724}{(0.8408--0.8968)}{4.55pt}{4.82pt} &  & \HoloSegScore{0.8754}{(0.8442--0.8989)}{4.55pt}{4.82pt} & \HoloSegScore{0.8735}{(0.8412--0.8974)}{4.55pt}{4.82pt} &  & \HoloSegScore{0.8643}{(0.8332--0.8869)}{4.55pt}{4.82pt} \\*
\softcline{4-5}\softcline{7-8}\softcline{10-10}
 &  & \HoloSegSpan{\makecell[c]{right anterior\\[-0.10ex]inferior segment of\\[-0.10ex]liver}}{2.90cm}{0.32cm} & \HoloSegMetric{HD95} & \HoloSegScore{19.59}{(10.29--33.77)}{4.55pt}{4.82pt} & \HoloSegSpan{114/116}{1.25cm}{0.32cm} & \HoloSegScore{18.52}{(10.27--32.63)}{4.55pt}{4.82pt} & \HoloSegScore{19.17}{(10.61--35.37)}{4.55pt}{4.82pt} & \HoloSegSpan{114/116}{1.25cm}{0.32cm} & \HoloSegScore{22.63}{(13.05--38.77)}{4.55pt}{4.82pt} \\
\cline{3-10}
 &  &  & \HoloSegMetric{Dice} & \HoloSegScore{0.8374}{(0.7761--0.8788)}{4.55pt}{4.82pt} &  & \HoloSegScore{0.8382}{(0.7775--0.8796)}{4.55pt}{4.82pt} & \HoloSegScore{0.8495}{(0.7932--0.8899)}{4.55pt}{4.82pt} &  & \HoloSegScore{0.8424}{(0.7868--0.8829)}{4.55pt}{4.82pt} \\*
\softcline{4-5}\softcline{7-8}\softcline{10-10}
 &  & \HoloSegSpan{\makecell[c]{right posterior\\[-0.10ex]inferior segment of\\[-0.10ex]liver}}{2.90cm}{0.32cm} & \HoloSegMetric{HD95} & \HoloSegScore{20.11}{(10.42--32.99)}{4.55pt}{4.82pt} & \HoloSegSpan{118/119}{1.25cm}{0.32cm} & \HoloSegScore{57.19}{(38.79--76.77)}{4.55pt}{4.82pt} & \HoloSegScore{15.94}{(10.04--22.72)}{4.55pt}{4.82pt} & \HoloSegSpan{118/119}{1.25cm}{0.32cm} & \HoloSegScore{13.59}{(9.850--18.01)}{4.55pt}{4.82pt} \\
\cline{3-10}
\HoloSegSpan{\makecell[c]{\textbf{Internal}}}{1.20cm}{0.32cm} & \HoloSegSpan{\makecell[c]{DeepTumorVQA}}{2.10cm}{0.32cm} &  & \HoloSegMetric{Dice} & \HoloSegScore{0.8789}{(0.8521--0.9003)}{4.55pt}{4.82pt} &  & \HoloSegScore{0.8843}{(0.8603--0.9040)}{4.55pt}{4.82pt} & \HoloSegScore{0.9077}{(0.8894--0.9216)}{4.55pt}{4.82pt} &  & \HoloSegScore{0.9042}{(0.8865--0.9191)}{4.55pt}{4.82pt} \\*
\softcline{4-5}\softcline{7-8}\softcline{10-10}
 &  & \HoloSegSpan{\makecell[c]{right posterior\\[-0.10ex]superior segment of\\[-0.10ex]liver}}{2.90cm}{0.32cm} & \HoloSegMetric{HD95} & \HoloSegScore{17.02}{(8.092--31.46)}{4.55pt}{4.82pt} & \HoloSegSpan{115/117}{1.25cm}{0.32cm} & \HoloSegScore{19.70}{(9.431--35.22)}{4.55pt}{4.82pt} & \HoloSegScore{15.36}{(6.817--29.56)}{4.55pt}{4.82pt} & \HoloSegSpan{115/117}{1.25cm}{0.32cm} & \HoloSegScore{16.09}{(7.353--30.50)}{4.55pt}{4.82pt} \\
\cline{3-10}
 &  &  & \HoloSegMetric{Dice} & \HoloSegScore{0.8833}{(0.8645--0.8967)}{4.55pt}{4.82pt} &  & \HoloSegScore{0.8882}{(0.8732--0.9006)}{4.55pt}{4.82pt} & \HoloSegScore{0.8929}{(0.8801--0.9041)}{4.55pt}{4.82pt} &  & \HoloSegScore{0.8923}{(0.8805--0.9025)}{4.55pt}{4.82pt} \\*
\softcline{4-5}\softcline{7-8}\softcline{10-10}
 &  & \HoloSegSpan{\makecell[c]{right anterior\\[-0.10ex]superior segment of\\[-0.10ex]liver}}{2.90cm}{0.32cm} & \HoloSegMetric{HD95} & \HoloSegScore{15.54}{(8.148--27.19)}{4.55pt}{4.82pt} & \HoloSegSpan{149/154}{1.25cm}{0.32cm} & \HoloSegScore{15.86}{(8.426--27.65)}{4.55pt}{4.82pt} & \HoloSegScore{14.79}{(8.687--25.62)}{4.55pt}{4.82pt} & \HoloSegSpan{149/154}{1.25cm}{0.32cm} & \HoloSegScore{14.93}{(8.791--25.82)}{4.55pt}{4.82pt} \\
\cline{3-10}
 &  &  & \HoloSegMetric{Dice} & \HoloSegScore{0.8785}{(0.8707--0.8854)}{4.55pt}{4.82pt} &  & \HoloSegScore{0.8781}{(0.8703--0.8852)}{4.55pt}{4.82pt} & \HoloSegScore{0.8813}{(0.8734--0.8886)}{4.55pt}{4.82pt} &  & \HoloSegScore{0.8803}{(0.8725--0.8878)}{4.55pt}{4.82pt} \\*
\softcline{4-5}\softcline{7-8}\softcline{10-10}
 &  & \HoloSegSpan{\makecell[c]{pancreas}}{2.90cm}{0.32cm} & \HoloSegMetric{HD95} & \HoloSegScore{6.280}{(5.173--7.680)}{4.55pt}{4.82pt} & \HoloSegSpan{1123/1208}{1.25cm}{0.32cm} & \HoloSegScore{6.217}{(5.118--7.553)}{4.55pt}{4.82pt} & \HoloSegScore{6.827}{(5.451--8.438)}{4.55pt}{4.82pt} & \HoloSegSpan{1074/1208}{1.25cm}{0.32cm} & \HoloSegScore{6.889}{(5.527--8.495)}{4.55pt}{4.82pt} \\
\cline{3-10}
 &  &  & \HoloSegMetric{Dice} & \HoloSegScore{0.5822}{(0.5182--0.6458)}{4.55pt}{4.82pt} &  & \HoloSegScore{0.5681}{(0.5049--0.6307)}{4.55pt}{4.82pt} & \HoloSegScore{0.6018}{(0.5465--0.6523)}{4.55pt}{4.82pt} &  & \HoloSegScore{0.5860}{(0.5325--0.6380)}{4.55pt}{4.82pt} \\*
\softcline{4-5}\softcline{7-8}\softcline{10-10}
 &  & \HoloSegSpan{\makecell[c]{pancreas lesion}}{2.90cm}{0.32cm} & \HoloSegMetric{HD95} & \HoloSegScore{21.78}{(15.80--28.71)}{4.55pt}{4.82pt} & \HoloSegSpan{188/267}{1.25cm}{0.32cm} & \HoloSegScore{22.69}{(16.80--29.70)}{4.55pt}{4.82pt} & \HoloSegScore{27.51}{(20.38--35.33)}{4.55pt}{4.82pt} & \HoloSegSpan{224/267}{1.25cm}{0.32cm} & \HoloSegScore{27.99}{(20.83--35.58)}{4.55pt}{4.82pt} \\
\cline{3-10}
 &  &  & \HoloSegMetric{Dice} & \HoloSegScore{0.9589}{(0.9537--0.9634)}{4.55pt}{4.82pt} &  & \HoloSegScore{0.9583}{(0.9531--0.9628)}{4.55pt}{4.82pt} & \HoloSegScore{0.9584}{(0.9531--0.9630)}{4.55pt}{4.82pt} &  & \HoloSegScore{0.9581}{(0.9528--0.9627)}{4.55pt}{4.82pt} \\*
\softcline{4-5}\softcline{7-8}\softcline{10-10}
 &  & \HoloSegSpan{\makecell[c]{spleen}}{2.90cm}{0.32cm} & \HoloSegMetric{HD95} & \HoloSegScore{2.707}{(2.152--3.475)}{4.55pt}{4.82pt} & \HoloSegSpan{1387/1391}{1.25cm}{0.32cm} & \HoloSegScore{2.733}{(2.187--3.502)}{4.55pt}{4.82pt} & \HoloSegScore{2.665}{(2.284--3.114)}{4.55pt}{4.82pt} & \HoloSegSpan{1387/1391}{1.25cm}{0.32cm} & \HoloSegScore{2.657}{(2.277--3.094)}{4.55pt}{4.82pt} \\
\cline{3-10}
 &  &  & \HoloSegMetric{Dice} & \HoloSegScore{0.9488}{(0.9275--0.9632)}{4.55pt}{4.82pt} &  & \HoloSegScore{0.9479}{(0.9260--0.9631)}{4.55pt}{4.82pt} & \HoloSegScore{0.9560}{(0.9429--0.9673)}{4.55pt}{4.82pt} &  & \HoloSegScore{0.9519}{(0.9389--0.9621)}{4.55pt}{4.82pt} \\*
\softcline{4-5}\softcline{7-8}\softcline{10-10}
 &  & \HoloSegSpan{\makecell[c]{stomach}}{2.90cm}{0.32cm} & \HoloSegMetric{HD95} & \HoloSegScore{3.047}{(2.008--4.208)}{4.55pt}{4.82pt} & \HoloSegSpan{7/12}{1.25cm}{0.32cm} & \HoloSegScore{3.181}{(2.014--4.465)}{4.55pt}{4.82pt} & \HoloSegScore{3.941}{(2.848--5.027)}{4.55pt}{4.82pt} & \HoloSegSpan{11/12}{1.25cm}{0.32cm} & \HoloSegScore{8.419}{(3.309--17.17)}{4.55pt}{4.82pt} \\
\cline{3-10}
 &  &  & \HoloSegMetric{Dice} & \HoloSegScore{0.6523}{(0.5210--0.7504)}{4.55pt}{4.82pt} &  & \HoloSegScore{0.6495}{(0.5185--0.7469)}{4.55pt}{4.82pt} & \HoloSegScore{0.6824}{(0.5687--0.7675)}{4.55pt}{4.82pt} &  & \HoloSegScore{0.6737}{(0.5578--0.7659)}{4.55pt}{4.82pt} \\*
\softcline{4-5}\softcline{7-8}\softcline{10-10}
 &  & \HoloSegSpan{\makecell[c]{colon lesion}}{2.90cm}{0.32cm} & \HoloSegMetric{HD95} & \HoloSegScore{30.13}{(10.46--54.70)}{4.55pt}{4.82pt} & \HoloSegSpan{44/44}{1.25cm}{0.32cm} & \HoloSegScore{30.82}{(10.80--55.84)}{4.55pt}{4.82pt} & \HoloSegScore{28.99}{(8.332--59.80)}{4.55pt}{4.82pt} & \HoloSegSpan{40/44}{1.25cm}{0.32cm} & \HoloSegScore{47.77}{(18.86--82.69)}{4.55pt}{4.82pt} \\
\hline
\end{longtable}
\arrayrulecolor{black}
\endgroup
